# Supplementary material for: Next-to-Leading Order Running in the SMEFT
Source: arXiv:2601.19974 ancillary file (2026-03-18)
Supplement: Supplementary file 1 [file SMEFT_Beta_Functions.pdf]

# Two-loop SMEFT $\beta$ -functions

Lukas Born,<sup>1\*</sup> Javier Fuentes-Martín,<sup>2†</sup>  
and Anders Eller Thomsen<sup>1‡</sup>

<sup>1</sup> Albert Einstein Center for Fundamental Physics, Institute for Theoretical Physics, University of Bern, CH-3012 Bern, Switzerland

<sup>2</sup> Departamento de Física Teórica y del Cosmos, Universidad de Granada,  
Campus de Fuentenueva, E-18071 Granada, Spain

*January 23, 2026*

---

\*lukas.born@unibe.ch

†javier.fuentes@ugr.es

‡anders.thomsen@unibe.ch

|      |                                    |    |
|------|------------------------------------|----|
| 1    | Set up . . . . .                   | 5  |
| 1.1  | Conventions . . . . .              | 5  |
| 1.2  | Abbreviations . . . . .            | 5  |
| 1.3  | Ordering . . . . .                 | 6  |
| 2    | Renormalizable couplings . . . . . | 7  |
| 2.1  | Higgs mass . . . . .               | 7  |
| 2.2  | Higgs quartic coupling . . . . .   | 7  |
| 2.3  | Lepton-Yukawa . . . . .            | 11 |
| 2.4  | Up-quark Yukawa . . . . .          | 13 |
| 2.5  | Down-quark Yukawa . . . . .        | 17 |
| 2.6  | $U(1)_Y$ gauge coupling . . . . .  | 20 |
| 2.7  | $SU(2)_L$ gauge coupling . . . . . | 21 |
| 2.8  | $SU(3)_c$ gauge coupling . . . . . | 21 |
| 2.9  | $\theta_B$ coupling . . . . .      | 21 |
| 2.10 | $\theta_W$ coupling . . . . .      | 21 |
| 2.11 | $\theta_G$ coupling . . . . .      | 22 |
| 3    | Weinberg operator . . . . .        | 22 |
| 4    | $H^6$ and $H^4 D^2$ . . . . .      | 22 |
| 4.1  | $C_H$ . . . . .                    | 22 |
| 4.2  | $C_{HD}^{(ll)}$ . . . . .          | 28 |
| 4.3  | $C_{HD}^{(\times)}$ . . . . .      | 31 |
| 5    | $X^2 H^2$ . . . . .                | 33 |
| 5.1  | $C_{HB}$ . . . . .                 | 33 |
| 5.2  | $C_{H\tilde{B}}$ . . . . .         | 34 |
| 5.3  | $C_{HW}$ . . . . .                 | 35 |
| 5.4  | $C_{H\widetilde{W}}$ . . . . .     | 36 |
| 5.5  | $C_{HG}$ . . . . .                 | 37 |
| 5.6  | $C_{H\tilde{G}}$ . . . . .         | 38 |
| 5.7  | $C_{HWB}$ . . . . .                | 39 |
| 5.8  | $C_{H\widetilde{W}B}$ . . . . .    | 40 |

|      |                           |     |
|------|---------------------------|-----|
| 6    | $X^3$                     | 41  |
| 6.1  | $C_W$                     | 41  |
| 6.2  | $C_{\widetilde{W}}$       | 41  |
| 6.3  | $C_G$                     | 42  |
| 6.4  | $C_{\widetilde{G}}$       | 42  |
| 7    | $\psi^2 H^3$              | 42  |
| 7.1  | $C_{eH}$                  | 42  |
| 7.2  | $C_{uH}$                  | 50  |
| 7.3  | $C_{dH}$                  | 65  |
| 8    | $\psi^2 XH$               | 80  |
| 8.1  | $C_{eB}$                  | 80  |
| 8.2  | $C_{eW}$                  | 82  |
| 8.3  | $C_{uB}$                  | 84  |
| 8.4  | $C_{uW}$                  | 87  |
| 8.5  | $C_{uG}$                  | 91  |
| 8.6  | $C_{dB}$                  | 93  |
| 8.7  | $C_{dW}$                  | 97  |
| 8.8  | $C_{dG}$                  | 100 |
| 9    | $\psi^2 HD$               | 103 |
| 9.1  | $C_{H\ell}^{(\parallel)}$ | 103 |
| 9.2  | $C_{H\ell}^{(\times)}$    | 107 |
| 9.3  | $C_{He}$                  | 111 |
| 9.4  | $C_{Hq}^{(\parallel)}$    | 114 |
| 9.5  | $C_{Hq}^{(\times)}$       | 123 |
| 9.6  | $C_{Hu}$                  | 130 |
| 9.7  | $C_{Hd}$                  | 136 |
| 9.8  | $C_{Hud}$                 | 142 |
| 10   | $(\bar{L}L)(\bar{R}R)$    | 145 |
| 10.1 | $C_{\ell e}$              | 145 |
| 10.2 | $C_{\ell u}$              | 151 |
| 10.3 | $C_{\ell d}$              | 155 |
| 10.4 | $C_{qe}$                  | 159 |
| 10.5 | $C_{qu}^{(\parallel)}$    | 165 |

|    |      |                                                   |     |
|----|------|---------------------------------------------------|-----|
|    | 10.6 | $C_{qu}^{(\times)}$                               | 174 |
|    | 10.7 | $C_{qd}^{(\parallel)}$                            | 182 |
|    | 10.8 | $C_{qd}^{(\times)}$                               | 191 |
| 11 |      | $(\bar{R}R)(\bar{R}R)$                            | 199 |
|    | 11.1 | $C_{ee}$                                          | 199 |
|    | 11.2 | $C_{uu}$                                          | 203 |
|    | 11.3 | $C_{dd}$                                          | 209 |
|    | 11.4 | $C_{eu}$                                          | 215 |
|    | 11.5 | $C_{ed}$                                          | 219 |
|    | 11.6 | $C_{ud}^{(\parallel)}$                            | 223 |
|    | 11.7 | $C_{ud}^{(\times)}$                               | 228 |
| 12 |      | $(\bar{L}R)(\bar{R}L)$ and $(\bar{L}R)(\bar{L}R)$ | 233 |
|    | 12.1 | $C_{ledq}$                                        | 233 |
|    | 12.2 | $C_{quqd}^{(\parallel)}$                          | 238 |
|    | 12.3 | $C_{quqd}^{(\times)}$                             | 246 |
|    | 12.4 | $C_{lequ}$                                        | 251 |
|    | 12.5 | $C_{luqe}$                                        | 256 |
| 13 |      | $(\bar{L}L)(\bar{L}L)$                            | 259 |
|    | 13.1 | $C_{\ell\ell}$                                    | 259 |
|    | 13.2 | $C_{qq}^{(\parallel)}$                            | 264 |
|    | 13.3 | $C_{qq}^{(\times)}$                               | 276 |
|    | 13.4 | $C_{\ell q}^{(\parallel)}$                        | 285 |
|    | 13.5 | $C_{\ell q}^{(\times)}$                           | 292 |

# 1 Set up

In this ancillary file, we present the  $\beta$ -functions of the baryon-number-conserving SMEFT up to two-loop order. For a coupling  $X$ , we parameterize its  $\beta$ -function by

$$\beta_X = \frac{dX}{d \ln \bar{\mu}} = \sum_{\ell=1}^{\infty} \frac{\beta_X^{(\ell)}}{(4\pi)^{2\ell}}, \quad (1.1)$$

where  $\bar{\mu}$  is the  $\overline{\text{MS}}$  renormalization scale.

## 1.1 Conventions

The SM Lagrangian is given by

$$\begin{aligned} \mathcal{L}_{\text{SM}} = & -\frac{1}{4}B^{\mu\nu}B_{\mu\nu} - \frac{1}{4}W^{I\mu\nu}W_{\mu\nu}^I - \frac{1}{4}G^{A\mu\nu}G_{\mu\nu}^A + D_\mu H^\dagger D^\mu H + \mu_H^2 H^\dagger H - \frac{\lambda}{2}(H^\dagger H)^2 \\ & + \sum_{\psi \in \{\ell, e, q, u, d\}} i(\bar{\psi} \gamma_\mu D^\mu \psi) - \left[ Y_e^{pr}(\bar{\ell}^p e^r H) + Y_u^{pr}(\bar{q}^p u^r \tilde{H}) + Y_d^{pr}(\bar{q}^p d^r H) + \text{H.c.} \right], \end{aligned} \quad (1.2)$$

with the covariant derivative

$$D_\mu q^{ai} = \partial_\mu q^{ai} - ig_Y Y B_\mu q^{ai} - ig_L t_{ij}^I W_\mu^I q^{aj} - ig_s T_{ab}^A G_\mu^A q^{bi}. \quad (1.3)$$

Additionally, we define the  $\theta$ -terms as

$$\mathcal{L}_\theta = \frac{\theta_B}{32\pi^2} \tilde{B}_{\mu\nu} B^{\mu\nu} + \frac{\theta_W}{32\pi^2} \tilde{W}_{\mu\nu}^I W^{I\mu\nu} + \frac{\theta_G}{32\pi^2} \tilde{G}_{\mu\nu}^A G^{A\mu\nu}, \quad (1.4)$$

with the dual field-strength tensor  $\tilde{F}^{\mu\nu} = \frac{1}{2}\epsilon^{\mu\nu\rho\sigma}F_{\rho\sigma}$ . Including a factor of  $\frac{1}{16\pi^2}$  in the definition of the  $\theta$ -terms formally lowers the loop-order of their  $\beta$ -functions by one. We therefore write  $\beta_{\theta_i}^{(0)}$  and  $\beta_{\theta_i}^{(1)}$  for the one-loop and two-loop  $\beta$ -function, respectively.

Our choice of dimension-five and dimension-six operators can be found in Table 1 and Table 2 of the main paper.

## 1.2 Abbreviations

To condense our results, we replace common structures with symbols. The following list provides all abbreviations that we use:

$$\text{T}_2 = \text{Tr}[Y_e^\dagger Y_e] + 3 \text{Tr}[Y_u^\dagger Y_u] + 3 \text{Tr}[Y_d^\dagger Y_d] \quad (1.5)$$

$$\text{T}_4 = \text{Tr}[(Y_e^\dagger Y_e)^2] + 3 \text{Tr}[(Y_u^\dagger Y_u)^2] + 3 \text{Tr}[(Y_d^\dagger Y_d)^2] \quad (1.6)$$

$$\text{T}_6 = \text{Tr}[(Y_e^\dagger Y_e)^3] + 3 \text{Tr}[(Y_u^\dagger Y_u)^3] + 3 \text{Tr}[(Y_d^\dagger Y_d)^3] \quad (1.7)$$

$$\text{T}_{\ell H} = \text{Tr}[C_{\ell HH}^\dagger C_{\ell HH}] \quad (1.8)$$

### 1.3 Ordering

In each  $\beta$ -function, we first present the SM contribution and the dimension-five (squared) terms, before turning to the dimension-six couplings with the ordering displayed in Tab. 1.

|    |                        |    |                                   |    |                                     |    |                                                                                 |
|----|------------------------|----|-----------------------------------|----|-------------------------------------|----|---------------------------------------------------------------------------------|
| 1  | $C_H$                  | 16 | $C_{eH}^{ab} \ \& \ C_{eH}^{*ab}$ | 31 | $C_{Hq}^{(\times)ab}$               | 46 | $C_{eu}^{abcd}$                                                                 |
| 2  | $C_{HD}^{(\parallel)}$ | 17 | $C_{uH}^{ab} \ \& \ C_{uH}^{*ab}$ | 32 | $C_{Hu}^{ab}$                       | 47 | $C_{ed}^{abcd}$                                                                 |
| 3  | $C_{HD}^{(\times)}$    | 18 | $C_{dH}^{ab} \ \& \ C_{dH}^{*ab}$ | 33 | $C_{Hd}^{ab}$                       | 48 | $C_{ud}^{(\parallel)abcd}$                                                      |
| 4  | $C_{HB}$               | 19 | $C_{eB}^{ab} \ \& \ C_{eB}^{*ab}$ | 34 | $C_{Hud}^{ab} \ \& \ C_{Hud}^{*ab}$ | 49 | $C_{ud}^{(\times)abcd}$                                                         |
| 5  | $C_{H\tilde{B}}$       | 20 | $C_{eW}^{ab} \ \& \ C_{eW}^{*ab}$ | 35 | $C_{\ell e}^{abcd}$                 | 50 | $C_{\ell eq}^{abcd} \ \& \ C_{\ell eq}^{*abcd}$                                 |
| 6  | $C_{HW}$               | 21 | $C_{uB}^{ab} \ \& \ C_{uB}^{*ab}$ | 36 | $C_{\ell u}^{abcd}$                 | 51 | $C_{quqd}^{(\parallel)abcd} \ \& \ \left(C_{quqd}^{(\parallel)*}\right)^{abcd}$ |
| 7  | $C_{H\tilde{W}}$       | 22 | $C_{uW}^{ab} \ \& \ C_{uW}^{*ab}$ | 37 | $C_{\ell d}^{abcd}$                 | 52 | $C_{quqd}^{(\times)abcd} \ \& \ \left(C_{quqd}^{(\times)*}\right)^{abcd}$       |
| 8  | $C_{HG}$               | 23 | $C_{uG}^{ab} \ \& \ C_{uG}^{*ab}$ | 38 | $C_{qe}^{abcd}$                     | 53 | $C_{\ell equ}^{abcd} \ \& \ C_{\ell equ}^{*abcd}$                               |
| 9  | $C_{H\tilde{G}}$       | 24 | $C_{dB}^{ab} \ \& \ C_{dB}^{*ab}$ | 39 | $C_{qu}^{(\parallel)abcd}$          | 54 | $C_{\ell uqe}^{abcd} \ \& \ C_{\ell uqe}^{*abcd}$                               |
| 10 | $C_{HWB}$              | 25 | $C_{dW}^{ab} \ \& \ C_{dW}^{*ab}$ | 40 | $C_{qu}^{(\times)abcd}$             | 55 | $C_{\ell\ell}^{abcd}$                                                           |
| 11 | $C_{H\tilde{W}B}$      | 26 | $C_{dG}^{ab} \ \& \ C_{dG}^{*ab}$ | 41 | $C_{qd}^{(\parallel)abcd}$          | 56 | $C_{qq}^{(\parallel)abcd}$                                                      |
| 12 | $C_W$                  | 27 | $C_{H\ell}^{(\parallel)ab}$       | 42 | $C_{qd}^{(\times)abcd}$             | 57 | $C_{qq}^{(\times)abcd}$                                                         |
| 13 | $C_{\tilde{W}}$        | 28 | $C_{H\ell}^{(\times)ab}$          | 43 | $C_{ee}^{abcd}$                     | 58 | $C_{\ell q}^{(\parallel)abcd}$                                                  |
| 14 | $C_G$                  | 29 | $C_{He}^{ab}$                     | 44 | $C_{uu}^{abcd}$                     | 59 | $C_{\ell q}^{(\times)abcd}$                                                     |
| 15 | $C_{\tilde{G}}$        | 30 | $C_{Hq}^{(\parallel)ab}$          | 45 | $C_{dd}^{abcd}$                     |    |                                                                                 |

Table 1: Ordering of dimension-six couplings

## 2 Renormalizable couplings

### 2.1 Higgs mass

$$\beta_{\mu_H^2}^{(1)} = \mu_H^2 \left\{ 2T_2 + 6\lambda - \frac{3}{2}g_Y^2 - \frac{9}{2}g_L^2 \right\} + 8\mu_H^4 C_{HD}^{(\parallel)} + 4\mu_H^4 C_{HD}^{(\times)}, \quad (2.1)$$

$$\begin{aligned} \beta_{\mu_H^2}^{(2)} = & \mu_H^2 \left\{ \lambda \left( 12g_Y^2 + 36g_L^2 - 12T_2 \right) + g_Y^2 \left( \frac{25}{12} \text{Tr}[Y_d^\dagger Y_d] + \frac{25}{4} \text{Tr}[Y_e^\dagger Y_e] + \frac{85}{12} \text{Tr}[Y_u^\dagger Y_u] \right) + g_s^2 \left( 40 \text{Tr}[Y_d^\dagger Y_d] + 40 \text{Tr}[Y_u^\dagger Y_u] \right) + \frac{15}{8} g_Y^2 g_L^2 \right. \\ & + \frac{15}{4} T_2 g_L^2 + \frac{557}{48} g_Y^4 - \frac{9}{2} T_4 - \frac{145}{16} g_L^4 - 15\lambda^2 - 21 \text{Tr}[Y_d^\dagger Y_d Y_u^\dagger Y_u] \left. \right\} + 8\mu_H^4 T_{\ell H} + \mu_H^4 \left\{ 15g_Y^2 + 45g_L^2 - 20T_2 \right. \\ & - 20\lambda \left. \right\} C_{HD}^{(\parallel)} + \mu_H^4 \left\{ 6g_Y^2 + 24g_L^2 - 10T_2 - 20\lambda \right\} C_{HD}^{(\times)} - 10\mu_H^4 g_Y^4 C_{HB} - 30\mu_H^4 g_L^4 C_{HW} + 9\mu_H^4 g_Y^2 g_L^2 C_{HWB} \\ & + 15\mu_H^4 g_L^6 C_W - 6\mu_H^4 Y_e^{*ab} C_{eH}^{ab} - 6\mu_H^4 C_{eH}^{*ab} Y_e^{ab} - 18\mu_H^4 Y_u^{*ab} C_{uH}^{ab} - 18\mu_H^4 C_{uH}^{*ab} Y_u^{ab} - 18\mu_H^4 Y_d^{*ab} C_{dH}^{ab} - 18\mu_H^4 C_{dH}^{*ab} Y_d^{ab} \\ & + 3\mu_H^4 g_Y^2 Y_e^{*ab} C_{eB}^{ab} + 3\mu_H^4 g_Y^2 C_{eB}^{*ab} Y_e^{ab} - \frac{3}{2}\mu_H^4 g_L^2 Y_e^{*ab} C_{eW}^{ab} - \frac{3}{2}\mu_H^4 g_L^2 C_{eW}^{*ab} Y_e^{ab} - 5\mu_H^4 g_Y^2 Y_u^{*ab} C_{uB}^{ab} - 5\mu_H^4 g_Y^2 C_{uB}^{*ab} Y_u^{ab} \\ & - \frac{9}{2}\mu_H^4 g_L^2 Y_u^{*ab} C_{uW}^{ab} - \frac{9}{2}\mu_H^4 g_L^2 C_{uW}^{*ab} Y_u^{ab} - 16\mu_H^4 g_s^2 Y_u^{*ab} C_{uG}^{ab} - 16\mu_H^4 g_s^2 C_{uG}^{*ab} Y_u^{ab} + \mu_H^4 g_Y^2 Y_d^{*ab} C_{dB}^{ab} + \mu_H^4 g_Y^2 C_{dB}^{*ab} Y_d^{ab} \\ & - \frac{9}{2}\mu_H^4 g_L^2 Y_d^{*ab} C_{dW}^{ab} - \frac{9}{2}\mu_H^4 g_L^2 C_{dW}^{*ab} Y_d^{ab} - 16\mu_H^4 g_s^2 Y_d^{*ab} C_{dG}^{ab} - 16\mu_H^4 g_s^2 C_{dG}^{*ab} Y_d^{ab} + \mu_H^4 \left\{ \frac{4}{3} \delta^{ab} g_Y^2 - \frac{4}{3} (Y_e Y_e^\dagger)^{ba} \right\} C_{H\ell}^{(\parallel)ab} \\ & + \mu_H^4 \left\{ \frac{2}{3} \delta^{ab} g_Y^2 - 2\delta^{ab} g_L^2 - \frac{8}{3} (Y_e Y_e^\dagger)^{ba} \right\} C_{H\ell}^{(\times)ab} + \mu_H^4 \left\{ \frac{4}{3} \delta^{ab} g_Y^2 + \frac{4}{3} (Y_e^\dagger Y_e)^{ba} \right\} C_{He}^{ab} - \mu_H^4 \left\{ \frac{4}{3} \delta^{ab} g_Y^2 + 4 \left( (Y_d Y_d^\dagger)^{ba} - (Y_u Y_u^\dagger)^{ba} \right) \right\} C_{Hq}^{(\parallel)ab} \\ & - \mu_H^4 \left\{ \frac{2}{3} \delta^{ab} g_Y^2 + 4 \left( (Y_u Y_u^\dagger)^{ba} + 2(Y_d Y_d^\dagger)^{ba} \right) + 6\delta^{ab} g_L^2 \right\} C_{Hq}^{(\times)ab} - \mu_H^4 \left\{ \frac{8}{3} \delta^{ab} g_Y^2 + 4(Y_u^\dagger Y_u)^{ba} \right\} C_{Hu}^{ab} + \mu_H^4 \left\{ \frac{4}{3} \delta^{ab} g_Y^2 + 4(Y_d^\dagger Y_d)^{ba} \right\} C_{Hd}^{ab} \\ & + 4\mu_H^4 C_{Hud}^{ab} (Y_d^\dagger Y_u)^{ba} + 4\mu_H^4 C_{Hud}^{*ab} (Y_u^\dagger Y_d)^{ab} - 4\mu_H^4 Y_e^{*ad} C_{\ell e}^{abcd} Y_e^{bc} - 12\mu_H^4 Y_u^{*ad} C_{qu}^{(\parallel)abcd} Y_u^{bc} - 36\mu_H^4 Y_u^{*ad} C_{qu}^{(\times)abcd} Y_u^{bc} \\ & - 12\mu_H^4 Y_d^{*ad} C_{qd}^{(\parallel)abcd} Y_d^{bc} - 36\mu_H^4 Y_d^{*ad} C_{qd}^{(\times)abcd} Y_d^{bc}, \end{aligned} \quad (2.2)$$

### 2.2 Higgs quartic coupling

$$\beta_\lambda^{(1)} = \left\{ \frac{3}{4} g_Y^4 + \lambda \left( 4T_2 - 3g_Y^2 - 9g_L^2 \right) + \frac{3}{2} g_Y^2 g_L^2 + \frac{9}{4} g_L^4 + 12\lambda^2 - 4T_4 \right\} + 48\mu_H^2 C_H + \mu_H^2 \left\{ \frac{17}{3} g_L^2 + 28\lambda - \frac{1}{3} g_Y^2 \right\} C_{HD}^{(\parallel)}$$

$$\begin{aligned}
& + \mu_H^2 \left\{ 24\lambda - \frac{2}{3}g_Y^2 - 6g_L^2 \right\} C_{HD}^{(\times)} + 12\mu_H^2 g_Y^4 C_{HB} + 36\mu_H^2 g_L^4 C_{HW} + 6\mu_H^2 g_Y^2 g_L^2 C_{HWB} + 4\mu_H^2 Y_e^{*ab} C_{eH}^{ab} + 4\mu_H^2 C_{eH}^{*ab} Y_e^{ab} \\
& + 12\mu_H^2 Y_u^{*ab} C_{uH}^{ab} + 12\mu_H^2 C_{uH}^{*ab} Y_u^{ab} + 12\mu_H^2 Y_d^{*ab} C_{dH}^{ab} + 12\mu_H^2 C_{dH}^{*ab} Y_d^{ab} + \mu_H^2 \left\{ \frac{8}{3}\delta^{ab} g_Y^2 + 8(Y_e Y_e^\dagger)^{ba} \right\} C_{H\ell}^{(\parallel)ab} + \mu_H^2 \left\{ \frac{4}{3}\delta^{ab} g_Y^2 \right. \\
& + 8(Y_e Y_e^\dagger)^{ba} - \frac{4}{3}\delta^{ab} g_L^2 \left. \right\} C_{H\ell}^{(\times)ab} + \mu_H^2 \left\{ \frac{8}{3}\delta^{ab} g_Y^2 - 8(Y_e^\dagger Y_e)^{ba} \right\} C_{He}^{ab} + \mu_H^2 \left\{ 24((Y_d Y_d^\dagger)^{ba} - (Y_u Y_u^\dagger)^{ba}) - \frac{8}{3}\delta^{ab} g_Y^2 \right\} C_{Hq}^{(\parallel)ab} + \mu_H^2 \left\{ 24(Y_d Y_d^\dagger)^{ba} \right. \\
& - \frac{4}{3}\delta^{ab} g_Y^2 - 4\delta^{ab} g_L^2 \left. \right\} C_{Hq}^{(\times)ab} + \mu_H^2 \left\{ 24(Y_u^\dagger Y_u)^{ba} - \frac{16}{3}\delta^{ab} g_Y^2 \right\} C_{Hu}^{ab} + \mu_H^2 \left\{ \frac{8}{3}\delta^{ab} g_Y^2 - 24(Y_d^\dagger Y_d)^{ba} \right\} C_{Hd}^{ab}, \tag{2.3}
\end{aligned}$$

$$\begin{aligned}
\beta_\lambda^{(2)} = & \left\{ \lambda^2 (18g_Y^2 + 54g_L^2 - 24T_2) + g_Y^4 \left( \frac{5}{2} \text{Tr}[Y_d^\dagger Y_d] - \frac{19}{2} \text{Tr}[Y_u^\dagger Y_u] - \frac{25}{2} \text{Tr}[Y_e^\dagger Y_e] \right) + g_Y^2 g_L^2 \left( 9 \text{Tr}[Y_d^\dagger Y_d] + 11 \text{Tr}[Y_e^\dagger Y_e] + 21 \text{Tr}[Y_u^\dagger Y_u] \right) \right. \\
& + \lambda \left( g_Y^2 \left( \frac{25}{6} \text{Tr}[Y_d^\dagger Y_d] + \frac{25}{2} \text{Tr}[Y_e^\dagger Y_e] + \frac{85}{6} \text{Tr}[Y_u^\dagger Y_u] \right) + g_s^2 \left( 80 \text{Tr}[Y_d^\dagger Y_d] + 80 \text{Tr}[Y_u^\dagger Y_u] \right) + \frac{15}{2} T_2 g_L^2 + \frac{39}{4} g_Y^2 g_L^2 + \frac{629}{24} g_Y^4 - T_4 \right. \\
& - \frac{73}{8} g_L^4 - 42 \text{Tr}[Y_d^\dagger Y_d Y_u^\dagger Y_u] \left. \right) + g_Y^2 \left( \frac{8}{3} \text{Tr}[Y_d^\dagger Y_d Y_d^\dagger Y_d] - \frac{16}{3} \text{Tr}[Y_u^\dagger Y_u Y_u^\dagger Y_u] - 8 \text{Tr}[Y_e^\dagger Y_e Y_e^\dagger Y_e] \right) + 20T_6 + \frac{305}{8} g_L^6 \\
& - g_s^2 \left( 64 \text{Tr}[Y_d^\dagger Y_d Y_d^\dagger Y_d] + 64 \text{Tr}[Y_u^\dagger Y_u Y_u^\dagger Y_u] \right) - \frac{3}{2} T_2 g_L^4 - 12 \text{Tr}[Y_d^\dagger Y_d Y_u^\dagger Y_u Y_d^\dagger Y_d] - 12 \text{Tr}[Y_d^\dagger Y_d Y_u^\dagger Y_u Y_u^\dagger Y_u] - \frac{289}{24} g_Y^2 g_L^4 - \frac{379}{24} g_Y^6 \\
& - \frac{559}{24} g_Y^4 g_L^2 - 78\lambda^3 \left. \right\} + \mu_H^2 \left( \frac{22}{3} g_L^2 \mathbf{T}_{\ell H} + \frac{38}{3} g_Y^2 \mathbf{T}_{\ell H} + 40\lambda \mathbf{T}_{\ell H} + 40 \text{Tr}[C_{\ell HH}^\dagger C_{\ell HH} Y_e Y_e^\dagger] \right) + \mu_H^2 \left\{ 96g_Y^2 + 288g_L^2 - 96T_2 \right. \\
& - 480\lambda \left. \right\} C_H + \mu_H^2 \left\{ \frac{1}{3} T_2 g_Y^2 + \lambda \left( 56g_Y^2 + \frac{368}{3} g_L^2 - 68T_2 \right) - \frac{17}{3} T_2 g_L^2 - 6 \text{Tr}[Y_d^\dagger Y_d Y_u^\dagger Y_u] - 13T_4 - \frac{1571}{108} g_Y^4 - \frac{793}{54} g_Y^2 g_L^2 \right. \\
& - \frac{403}{12} g_L^4 - 268\lambda^2 \left. \right\} C_{HD}^{(\parallel)} + \mu_H^2 \left\{ \frac{2}{3} T_2 g_Y^2 + \lambda \left( \frac{107}{3} g_Y^2 + 159g_L^2 - 56T_2 \right) + 6T_2 g_L^2 + \frac{241}{24} g_L^4 - 7T_4 - \frac{3611}{216} g_Y^4 \right. \\
& - \frac{4429}{108} g_Y^2 g_L^2 - 54 \text{Tr}[Y_d^\dagger Y_d Y_u^\dagger Y_u] - 282\lambda^2 \left. \right\} C_{HD}^{(\times)} + \mu_H^2 \left\{ g_Y^4 \left( \frac{106}{3} \text{Tr}[Y_d^\dagger Y_d] - \frac{158}{3} \text{Tr}[Y_u^\dagger Y_u] - 86 \text{Tr}[Y_e^\dagger Y_e] \right) + 60\lambda g_Y^4 \right. \\
& - \frac{391}{3} g_Y^4 g_L^2 - \frac{1279}{3} g_Y^6 \left. \right\} C_{HB} + \mu_H^2 \left\{ 6T_2 g_L^4 + \frac{29}{3} g_L^6 + 84\lambda g_L^4 - 141g_Y^2 g_L^4 \right\} C_{HW} - \mu_H^2 g_s^4 \left\{ 704 \text{Tr}[Y_d^\dagger Y_d] \right. \\
& + 704 \text{Tr}[Y_u^\dagger Y_u] \left. \right\} C_{HG} + \mu_H^2 \left\{ g_Y^2 g_L^2 \left( 23 \text{Tr}[Y_e^\dagger Y_e] + 25 \text{Tr}[Y_d^\dagger Y_d] + 47 \text{Tr}[Y_u^\dagger Y_u] \right) + 70\lambda g_Y^2 g_L^2 - 68g_Y^2 g_L^4 - \frac{461}{3} g_Y^4 g_L^2 \right\} C_{HWB}
\end{aligned}$$



$$\begin{aligned}
& + \mu_H^2 \left\{ 12T_2 g_L^6 + 13g_Y^2 g_L^6 - 36\lambda g_L^6 - \frac{221}{3} g_L^8 \right\} C_W + \mu_H^2 \left\{ \frac{13}{2} g_Y^2 Y_e^{*ab} - \frac{9}{2} g_L^2 Y_e^{*ab} - 28\lambda Y_e^{*ab} - 30(Y_e^\dagger Y_e Y_e^\dagger)^{ab} \right\} C_{eH}^{ab} \\
& + \mu_H^2 C_{eH}^{*ab} \left\{ \frac{13}{2} g_Y^2 Y_e^{ab} - \frac{9}{2} g_L^2 Y_e^{ab} - 28\lambda Y_e^{ab} - 30(Y_e Y_e^\dagger Y_e)^{ab} \right\} + \mu_H^2 \left\{ 80g_s^2 Y_u^{*ab} - \frac{23}{6} g_Y^2 Y_u^{*ab} - 6(4(Y_d^\dagger Y_d Y_u^\dagger)^{ab} + 15(Y_u^\dagger Y_u Y_u^\dagger)^{ab}) \right. \\
& - \frac{27}{2} g_L^2 Y_u^{*ab} - 84\lambda Y_u^{*ab} \left. \right\} C_{uH}^{ab} + \mu_H^2 C_{uH}^{*ab} \left\{ 80g_s^2 Y_u^{ab} - \frac{23}{6} g_Y^2 Y_u^{ab} - 6(4(Y_d Y_d^\dagger Y_u)^{ab} + 15(Y_u Y_u^\dagger Y_u)^{ab}) - \frac{27}{2} g_L^2 Y_u^{ab} - 84\lambda Y_u^{ab} \right\} \\
& + \mu_H^2 \left\{ 80g_s^2 Y_d^{*ab} - 6(4(Y_u^\dagger Y_u Y_d^\dagger)^{ab} + 15(Y_d^\dagger Y_d Y_d^\dagger)^{ab}) - \frac{27}{2} g_L^2 Y_d^{*ab} - \frac{83}{6} g_Y^2 Y_d^{*ab} - 84\lambda Y_d^{*ab} \right\} C_{dH}^{ab} + \mu_H^2 C_{dH}^{*ab} \left\{ 80g_s^2 Y_d^{ab} - 6(4(Y_u Y_u^\dagger Y_d)^{ab} \right. \\
& + 15(Y_d Y_d^\dagger Y_d)^{ab}) - \frac{27}{2} g_L^2 Y_d^{ab} - \frac{83}{6} g_Y^2 Y_d^{ab} - 84\lambda Y_d^{ab} \left. \right\} + \mu_H^2 \left\{ 7g_Y^4 Y_e^{*ab} + 12\lambda g_Y^2 Y_e^{*ab} - 3g_Y^2 g_L^2 Y_e^{*ab} - 8g_Y^2 (Y_e^\dagger Y_e Y_e^\dagger)^{ab} \right\} C_{eB}^{ab} \\
& + \mu_H^2 C_{eB}^{*ab} \left\{ 7g_Y^4 Y_e^{ab} + 12\lambda g_Y^2 Y_e^{ab} - 3g_Y^2 g_L^2 Y_e^{ab} - 8g_Y^2 (Y_e Y_e^\dagger Y_e)^{ab} \right\} + \mu_H^2 \left\{ \frac{7}{2} g_Y^2 g_L^2 Y_e^{*ab} + 13g_L^2 (Y_e^\dagger Y_e Y_e^\dagger)^{ab} - 6\lambda g_L^2 Y_e^{*ab} \right. \\
& - \frac{77}{6} g_L^4 Y_e^{*ab} \left. \right\} C_{eW}^{ab} + \mu_H^2 C_{eW}^{*ab} \left\{ \frac{7}{2} g_Y^2 g_L^2 Y_e^{ab} + 13g_L^2 (Y_e Y_e^\dagger Y_e)^{ab} - 6\lambda g_L^2 Y_e^{ab} - \frac{77}{6} g_L^4 Y_e^{ab} \right\} + \mu_H^2 \left\{ 2g_Y^2 (3(Y_d^\dagger Y_d Y_u^\dagger)^{ab} + 8(Y_u^\dagger Y_u Y_u^\dagger)^{ab}) \right. \\
& + \frac{11}{3} g_Y^2 g_L^2 Y_u^{*ab} - \frac{35}{3} g_Y^4 Y_u^{*ab} - 20\lambda g_Y^2 Y_u^{*ab} \left. \right\} C_{uB}^{ab} + \mu_H^2 C_{uB}^{*ab} \left\{ 2g_Y^2 (3(Y_d Y_d^\dagger Y_u)^{ab} + 8(Y_u Y_u^\dagger Y_u)^{ab}) + \frac{11}{3} g_Y^2 g_L^2 Y_u^{ab} - \frac{35}{3} g_Y^4 Y_u^{ab} \right. \\
& - 20\lambda g_Y^2 Y_u^{ab} \left. \right\} + \mu_H^2 \left\{ 3g_L^2 (13(Y_u^\dagger Y_u Y_u^\dagger)^{ab} + 16(Y_d^\dagger Y_d Y_u^\dagger)^{ab}) + \frac{17}{2} g_Y^2 g_L^2 Y_u^{*ab} - 18\lambda g_L^2 Y_u^{*ab} - \frac{77}{2} g_L^4 Y_u^{*ab} \right\} C_{uW}^{ab} \\
& + \mu_H^2 C_{uW}^{*ab} \left\{ 3g_L^2 (13(Y_u Y_u^\dagger Y_u)^{ab} + 16(Y_d Y_d^\dagger Y_u)^{ab}) + \frac{17}{2} g_Y^2 g_L^2 Y_u^{ab} - 18\lambda g_L^2 Y_u^{ab} - \frac{77}{2} g_L^4 Y_u^{ab} \right\} + \mu_H^2 \left\{ \frac{64}{3} g_s^2 g_L^2 Y_u^{*ab} + \frac{64}{3} g_Y^2 g_s^2 Y_u^{*ab} \right. \\
& + 32g_s^2 (Y_u^\dagger Y_u Y_u^\dagger)^{ab} - 64\lambda g_s^2 Y_u^{*ab} \left. \right\} C_{uG}^{ab} + \mu_H^2 C_{uG}^{*ab} \left\{ \frac{64}{3} g_s^2 g_L^2 Y_u^{ab} + \frac{64}{3} g_Y^2 g_s^2 Y_u^{ab} + 32g_s^2 (Y_u Y_u^\dagger Y_u)^{ab} - 64\lambda g_s^2 Y_u^{ab} \right\} \\
& + \mu_H^2 \left\{ \frac{5}{3} g_Y^2 g_L^2 Y_d^{*ab} + \frac{7}{3} g_Y^4 Y_d^{*ab} + 4\lambda g_Y^2 Y_d^{*ab} - 2g_Y^2 (3(Y_u^\dagger Y_u Y_d^\dagger)^{ab} + 4(Y_d^\dagger Y_d Y_d^\dagger)^{ab}) \right\} C_{dB}^{ab} + \mu_H^2 C_{dB}^{*ab} \left\{ \frac{5}{3} g_Y^2 g_L^2 Y_d^{ab} + \frac{7}{3} g_Y^4 Y_d^{ab} + 4\lambda g_Y^2 Y_d^{ab} \right. \\
& - 2g_Y^2 (3(Y_u Y_u^\dagger Y_d)^{ab} + 4(Y_d Y_d^\dagger Y_d)^{ab}) \left. \right\} + \mu_H^2 \left\{ 3g_L^2 (13(Y_d^\dagger Y_d Y_d^\dagger)^{ab} + 16(Y_u^\dagger Y_u Y_d^\dagger)^{ab}) + \frac{13}{2} g_Y^2 g_L^2 Y_d^{*ab} - 18\lambda g_L^2 Y_d^{*ab} - \frac{77}{2} g_L^4 Y_d^{*ab} \right\} C_{dW}^{ab} \\
& + \mu_H^2 C_{dW}^{*ab} \left\{ 3g_L^2 (13(Y_d Y_d^\dagger Y_d)^{ab} + 16(Y_u Y_u^\dagger Y_d)^{ab}) + \frac{13}{2} g_Y^2 g_L^2 Y_d^{ab} - 18\lambda g_L^2 Y_d^{ab} - \frac{77}{2} g_L^4 Y_d^{ab} \right\} + \mu_H^2 \left\{ \frac{64}{3} g_s^2 g_L^2 Y_d^{*ab} + \frac{64}{3} g_Y^2 g_s^2 Y_d^{*ab} \right.
\end{aligned}$$

$$\begin{aligned}
& + 32g_s^2(Y_d^\dagger Y_d Y_d^\dagger)^{ab} - 64\lambda g_s^2 Y_d^{*ab} \Big\} C_{dG}^{ab} + \mu_H^2 C_{dG}^{*ab} \Big\{ \frac{64}{3}g_s^2 g_L^2 Y_d^{ab} + \frac{64}{3}g_Y^2 g_s^2 Y_d^{ab} + 32g_s^2(Y_d Y_d^\dagger Y_d)^{ab} - 64\lambda g_s^2 Y_d^{ab} \Big\} \\
& + \mu_H^2 \Big\{ \frac{178}{27}\delta^{ab} g_Y^4 + \frac{286}{27}\delta^{ab} g_Y^2 g_L^2 + \frac{311}{9}g_Y^2(Y_e Y_e^\dagger)^{ba} - \frac{7}{9}g_L^2(Y_e Y_e^\dagger)^{ba} - \lambda \Big( 8\delta^{ab} g_Y^2 + \frac{40}{3}(Y_e Y_e^\dagger)^{ba} \Big) - 24(Y_e Y_e^\dagger Y_e Y_e^\dagger)^{ba} \Big\} C_{H\ell}^{(\parallel)ab} \\
& + \mu_H^2 \Big\{ \lambda \Big( \frac{16}{3}\delta^{ab} g_L^2 - 4\delta^{ab} g_Y^2 - \frac{68}{3}(Y_e Y_e^\dagger)^{ba} \Big) + \frac{83}{27}\delta^{ab} g_Y^2 g_L^2 + \frac{89}{27}\delta^{ab} g_Y^4 + \frac{148}{9}g_L^2(Y_e Y_e^\dagger)^{ba} + \frac{334}{9}g_Y^2(Y_e Y_e^\dagger)^{ba} - 16(Y_e Y_e^\dagger Y_e Y_e^\dagger)^{ba} \\
& - 18\delta^{ab} g_L^4 \Big\} C_{H\ell}^{(\times)ab} + \mu_H^2 \Big\{ \lambda \Big( \frac{40}{3}(Y_e^\dagger Y_e)^{ba} - 8\delta^{ab} g_Y^2 \Big) + \frac{124}{27}\delta^{ab} g_Y^2 g_L^2 + \frac{340}{27}\delta^{ab} g_Y^4 + 24(Y_e^\dagger Y_e Y_e^\dagger Y_e)^{ba} - \frac{77}{9}g_L^2(Y_e^\dagger Y_e)^{ba} \\
& - \frac{167}{9}g_Y^2(Y_e^\dagger Y_e)^{ba} \Big\} C_{He}^{ab} + \mu_H^2 \Big\{ \frac{1}{3}g_Y^2 \Big( 47(Y_d Y_d^\dagger)^{ba} - 139(Y_u Y_u^\dagger)^{ba} \Big) + \lambda \Big( 8\delta^{ab} g_Y^2 - 40 \Big( (Y_d Y_d^\dagger)^{ba} - (Y_u Y_u^\dagger)^{ba} \Big) \Big) + 160g_s^2 \Big( (Y_d Y_d^\dagger)^{ba} - (Y_u Y_u^\dagger)^{ba} \Big) \\
& - \frac{7}{3}g_L^2 \Big( (Y_d Y_d^\dagger)^{ba} - (Y_u Y_u^\dagger)^{ba} \Big) - \frac{130}{27}\delta^{ab} g_Y^4 - \frac{286}{27}\delta^{ab} g_Y^2 g_L^2 - \frac{32}{3}\delta^{ab} g_Y^2 g_s^2 - 72 \Big( (Y_d Y_d^\dagger Y_d Y_d^\dagger)^{ba} - (Y_u Y_u^\dagger Y_u Y_u^\dagger)^{ba} \Big) \Big\} C_{Hq}^{(\parallel)ab} \\
& + \mu_H^2 \Big\{ \frac{1}{3}g_L^2 \Big( 148(Y_d Y_d^\dagger)^{ba} + 155(Y_u Y_u^\dagger)^{ba} \Big) + g_Y^2 \Big( 5(Y_u Y_u^\dagger)^{ba} + 18(Y_d Y_d^\dagger)^{ba} \Big) + \lambda \Big( 4\delta^{ab} g_Y^2 + 16\delta^{ab} g_L^2 - 4 \Big( 7(Y_u Y_u^\dagger)^{ba} + 17(Y_d Y_d^\dagger)^{ba} \Big) \Big) \\
& + 160g_s^2(Y_d Y_d^\dagger)^{ba} - \frac{65}{27}\delta^{ab} g_Y^4 - \frac{16}{3}\delta^{ab} g_Y^2 g_s^2 - 6 \Big( 8(Y_d Y_d^\dagger Y_d Y_d^\dagger)^{ba} - 4(Y_u Y_u^\dagger Y_u Y_u^\dagger)^{ba} - 5(Y_d Y_d^\dagger Y_u Y_u^\dagger)^{ba} - 5(Y_u Y_u^\dagger Y_d Y_d^\dagger)^{ba} \Big) - \frac{251}{27}\delta^{ab} g_Y^2 g_L^2 \\
& - 16\delta^{ab} g_s^2 g_L^2 - 54\delta^{ab} g_L^4 \Big\} C_{Hq}^{(\times)ab} + \mu_H^2 \Big\{ \lambda \Big( 16\delta^{ab} g_Y^2 - 40(Y_u^\dagger Y_u)^{ba} \Big) + 12 \Big( (Y_u^\dagger Y_d Y_d^\dagger Y_u)^{ba} - 6(Y_u^\dagger Y_u Y_u^\dagger Y_u)^{ba} \Big) + \frac{59}{3}g_Y^2(Y_u^\dagger Y_u)^{ba} \\
& + \frac{77}{3}g_L^2(Y_u^\dagger Y_u)^{ba} + 160g_s^2(Y_u^\dagger Y_u)^{ba} - \frac{248}{27}\delta^{ab} g_Y^2 g_L^2 - \frac{440}{27}\delta^{ab} g_Y^4 - \frac{64}{3}\delta^{ab} g_Y^2 g_s^2 \Big\} C_{Hu}^{ab} + \mu_H^2 \Big\{ \lambda \Big( 40(Y_d^\dagger Y_d)^{ba} - 8\delta^{ab} g_Y^2 \Big) + \frac{124}{27}\delta^{ab} g_Y^2 g_L^2 \\
& + \frac{148}{27}\delta^{ab} g_Y^4 + \frac{32}{3}\delta^{ab} g_Y^2 g_s^2 + 12 \Big( 6(Y_d^\dagger Y_d Y_d^\dagger Y_d)^{ba} - (Y_d^\dagger Y_u Y_u^\dagger Y_d)^{ba} \Big) - \frac{31}{3}g_Y^2(Y_d^\dagger Y_d)^{ba} - \frac{77}{3}g_L^2(Y_d^\dagger Y_d)^{ba} - 160g_s^2(Y_d^\dagger Y_d)^{ba} \Big\} C_{Hd}^{ab} \\
& + \mu_H^2 \Big\{ 28\lambda(Y_d^\dagger Y_u)^{ba} - \frac{17}{3}g_Y^2(Y_d^\dagger Y_u)^{ba} - 24 \Big( (Y_d^\dagger Y_d Y_d^\dagger Y_u)^{ba} + (Y_d^\dagger Y_u Y_u^\dagger Y_u)^{ba} \Big) - \frac{239}{3}g_L^2(Y_d^\dagger Y_u)^{ba} \Big\} C_{Hud}^{ab} + \mu_H^2 C_{Hud}^{*ab} \Big\{ 28\lambda(Y_u^\dagger Y_d)^{ab} \\
& - \frac{17}{3}g_Y^2(Y_u^\dagger Y_d)^{ab} - 24 \Big( (Y_u^\dagger Y_d Y_d^\dagger Y_d)^{ab} + (Y_u^\dagger Y_u Y_u^\dagger Y_d)^{ab} \Big) - \frac{239}{3}g_L^2(Y_u^\dagger Y_d)^{ab} \Big\} + \mu_H^2 \Big\{ 16 \Big( Y_e^{bc}(Y_e^\dagger Y_e Y_e^\dagger)^{ad} + Y_e^{*ad}(Y_e Y_e^\dagger Y_e)^{bc} \Big) - 16\lambda Y_e^{*ad} Y_e^{bc} \Big\} C_{\ell e}^{abcd} \\
& + \mu_H^2 \Big\{ 48 \Big( Y_u^{bc}(Y_u^\dagger Y_u Y_u^\dagger)^{ad} + Y_u^{*ad}(Y_u Y_u^\dagger Y_u)^{bc} \Big) - 48\lambda Y_u^{*ad} Y_u^{bc} \Big\} C_{qu}^{(\parallel)abcd} + \mu_H^2 \Big\{ 144 \Big( Y_u^{bc}(Y_u^\dagger Y_u Y_u^\dagger)^{ad} + Y_u^{*ad}(Y_u Y_u^\dagger Y_u)^{bc} \Big) - 144\lambda Y_u^{*ad} Y_u^{bc} \Big\} C_{qu}^{(\times)abcd}
\end{aligned}$$

$$\begin{aligned}
& + \mu_H^2 \left\{ 48 \left( Y_d^{bc} (Y_d^\dagger Y_d Y_d^\dagger)^{ad} + Y_d^{*ad} (Y_d Y_d^\dagger Y_d)^{bc} \right) - 48 \lambda Y_d^{*ad} Y_d^{bc} \right\} C_{qd}^{(\parallel)abcd} + \mu_H^2 \left\{ 144 \left( Y_d^{bc} (Y_d^\dagger Y_d Y_d^\dagger)^{ad} + Y_d^{*ad} (Y_d Y_d^\dagger Y_d)^{bc} \right) - 144 \lambda Y_d^{*ad} Y_d^{bc} \right\} C_{qd}^{(\times)abcd} \\
& + \mu_H^2 \left\{ \frac{32}{3} \delta^{ad} g_Y^2 (Y_e^\dagger Y_e)^{bc} - \frac{16}{9} \delta^{ab} \delta^{cd} g_Y^4 - 16 (Y_e^\dagger Y_e)^{ba} (Y_e^\dagger Y_e)^{dc} \right\} C_{ee}^{abcd} + \mu_H^2 \left\{ \frac{64}{3} \delta^{ad} g_Y^2 (Y_u^\dagger Y_u)^{bc} - \frac{64}{27} \delta^{ad} \delta^{bc} g_Y^4 - 48 (Y_u^\dagger Y_u)^{bc} (Y_u^\dagger Y_u)^{da} \right\} C_{uu}^{abcd} \\
& + \mu_H^2 \left\{ \frac{32}{3} \delta^{ad} g_Y^2 (Y_d^\dagger Y_d)^{bc} - \frac{16}{27} \delta^{ad} \delta^{bc} g_Y^4 - 48 (Y_d^\dagger Y_d)^{bc} (Y_d^\dagger Y_d)^{da} \right\} C_{dd}^{abcd} + \mu_H^2 \left\{ \frac{16}{3} \delta^{bc} g_L^2 (Y_e Y_e^\dagger)^{da} - \frac{8}{9} \delta^{ad} \delta^{bc} g_L^4 - \frac{8}{9} \delta^{ad} \delta^{bc} g_Y^4 \right. \\
& - \frac{16}{3} \delta^{bc} g_Y^2 (Y_e Y_e^\dagger)^{da} - 16 (Y_e Y_e^\dagger)^{bc} (Y_e Y_e^\dagger)^{da} \left. \right\} C_{\ell\ell}^{abcd} + \mu_H^2 \left\{ \frac{16}{3} g_Y^2 \left( \delta^{bc} (Y_d Y_d^\dagger)^{da} - \delta^{bc} (Y_u Y_u^\dagger)^{da} \right) + 16 g_L^2 \left( \delta^{bc} (Y_d Y_d^\dagger)^{da} + \delta^{bc} (Y_u Y_u^\dagger)^{da} \right) - \frac{8}{27} \delta^{ad} \delta^{bc} g_Y^4 \right. \\
& - \frac{8}{3} \delta^{ad} \delta^{bc} g_L^4 - 48 \left( (Y_d Y_d^\dagger)^{bc} (Y_d Y_d^\dagger)^{da} + (Y_u Y_u^\dagger)^{bc} (Y_u Y_u^\dagger)^{da} \right) \left. \right\} C_{qq}^{(\parallel)abcd} + \mu_H^2 \left\{ \frac{32}{3} g_Y^2 \left( \delta^{bc} (Y_d Y_d^\dagger)^{da} - \delta^{bc} (Y_u Y_u^\dagger)^{da} \right) - \frac{16}{27} \delta^{ad} \delta^{bc} g_Y^4 - 48 \left( (Y_d Y_d^\dagger)^{bc} (Y_d Y_d^\dagger)^{da} \right. \right. \\
& \left. \left. + (Y_u Y_u^\dagger)^{bc} (Y_u Y_u^\dagger)^{da} - 2 (Y_d Y_d^\dagger)^{da} (Y_u Y_u^\dagger)^{bc} \right) \right\} C_{qq}^{(\times)abcd}, \tag{2.4}
\end{aligned}$$

### 2.3 Lepton-Yukawa

$$\begin{aligned}
\beta_{Y_e^{pr}}^{(1)} & = \left\{ \frac{1}{2} \left( 2T_2 Y_e^{pr} + 3(Y_e Y_e^\dagger Y_e)^{pr} \right) - \frac{9}{4} g_L^2 Y_e^{pr} - \frac{15}{4} g_Y^2 Y_e^{pr} \right\} + 2\mu_H^2 C_{HD}^{(\parallel)} Y_e^{pr} + \mu_H^2 C_{HD}^{(\times)} Y_e^{pr} + 6\delta^{pa} \delta^{rb} \mu_H^2 C_{eH}^{ab} + 2\delta^{pa} \mu_H^2 C_{H\ell}^{(\parallel)ab} Y_e^{br} \\
& + 4\delta^{pa} \mu_H^2 C_{H\ell}^{(\times)ab} Y_e^{br} - 2\delta^{rb} \mu_H^2 C_{He}^{ab} Y_e^{pa} - 4\delta^{pa} \delta^{rd} \mu_H^2 C_{\ell e}^{abcd} Y_e^{bc} + 6\delta^{pa} \delta^{rb} \mu_H^2 C_{ledq}^{abcd} Y_d^{dc} - 6\delta^{pa} \delta^{rb} \mu_H^2 Y_u^{*cd} C_{lequ}^{abcd} + 3\delta^{pa} \delta^{rd} \mu_H^2 Y_u^{*cb} C_{luqe}^{abcd}, \tag{2.5} \\
\beta_{Y_e^{pr}}^{(2)} & = \left\{ \frac{15}{16} g_L^2 \left( 2T_2 Y_e^{pr} + 9(Y_e Y_e^\dagger Y_e)^{pr} \right) + g_Y^2 \left( \frac{25}{24} Y_e^{pr} \text{Tr}[Y_d^\dagger Y_d] + \frac{25}{8} Y_e^{pr} \text{Tr}[Y_e^\dagger Y_e] + \frac{85}{24} Y_e^{pr} \text{Tr}[Y_u^\dagger Y_u] + \frac{129}{16} (Y_e Y_e^\dagger Y_e)^{pr} \right) + g_s^2 \left( 20 Y_e^{pr} \text{Tr}[Y_d^\dagger Y_d] \right. \right. \\
& \left. \left. + 20 Y_e^{pr} \text{Tr}[Y_u^\dagger Y_u] \right) + \frac{3}{2} \lambda^2 Y_e^{pr} + \frac{3}{2} Y_e^{pr} \text{Tr}[Y_d^\dagger Y_d Y_u^\dagger Y_u] + \frac{9}{4} g_Y^2 g_L^2 Y_e^{pr} + \frac{457}{24} g_Y^4 Y_e^{pr} - \frac{3}{4} \left( 3T_4 Y_e^{pr} + 3T_2 (Y_e Y_e^\dagger Y_e)^{pr} - 2(Y_e Y_e^\dagger Y_e Y_e^\dagger Y_e)^{pr} \right) \right. \\
& \left. - \frac{23}{4} g_L^4 Y_e^{pr} - 6\lambda (Y_e Y_e^\dagger Y_e)^{pr} \right\} - 10\mu_H^2 Y_e^{pr} T_{\ell H} + \mu_H^2 \left\{ \frac{1}{2} \left( -8T_2 Y_e^{pr} - 9(Y_e Y_e^\dagger Y_e)^{pr} \right) + \frac{199}{36} g_Y^2 Y_e^{pr} + \frac{199}{12} g_L^2 Y_e^{pr} - \frac{1}{2} \lambda Y_e^{pr} \right\} C_{HD}^{(\parallel)} \\
& + \mu_H^2 \left\{ \frac{1}{2} \left( -4T_2 Y_e^{pr} - 9(Y_e Y_e^\dagger Y_e)^{pr} \right) + \frac{91}{18} g_Y^2 Y_e^{pr} + 6g_L^2 Y_e^{pr} - \frac{1}{2} \lambda Y_e^{pr} \right\} C_{HD}^{(\times)} + \frac{3}{2} \mu_H^2 g_Y^4 C_{HB} Y_e^{pr} + \frac{75i}{4} \mu_H^2 g_Y^4 C_{H\tilde{B}} Y_e^{pr} + \frac{9}{2} \mu_H^2 g_L^4 C_{HW} Y_e^{pr} \\
& + \frac{21i}{4} \mu_H^2 g_L^4 C_{H\tilde{W}} Y_e^{pr} + \frac{9}{4} \mu_H^2 g_Y^2 g_L^2 C_{HWB} Y_e^{pr} - \frac{81i}{8} \mu_H^2 g_Y^2 g_L^2 C_{H\tilde{W}B} Y_e^{pr} + 18\mu_H^2 g_L^6 C_W Y_e^{pr} + \frac{5i}{4} \mu_H^2 g_L^6 C_{\tilde{W}} Y_e^{pr} + \mu_H^2 \left\{ 12\delta^{pa} \delta^{rb} g_Y^2 \right.
\end{aligned}$$

$$\begin{aligned}
& + 36\delta^{pa}\delta^{rb}g_L^2 - 3\left(\delta^{pa}(Y_e^\dagger Y_e)^{br} + \delta^{rb}(Y_e Y_e^\dagger)^{pa} + 4T_2\delta^{pa}\delta^{rb}\right) - 15\delta^{pa}\delta^{rb}\lambda \Big\} C_{eH}^{ab} + \mu_H^2 \Big\{ g_Y^2 \Big( \frac{1}{4} \Big( 12Y_e^{*ab}Y_e^{pr} - 58\delta^{rb}(Y_e Y_e^\dagger)^{pa} \\
& - 163\delta^{pa}(Y_e^\dagger Y_e)^{br} \Big) - 3\delta^{pa}\delta^{rb}\text{Tr}[Y_d^\dagger Y_d] - 9\delta^{pa}\delta^{rb}\text{Tr}[Y_e^\dagger Y_e] \Big) + 12\delta^{pa}\delta^{rb}g_Y^2g_L^2 - 48\delta^{pa}\delta^{rb}g_Y^4 \Big\} C_{eB}^{ab} - \frac{1}{4}\mu_H^2g_Y^2C_{eB}^{*ab} \Big\{ 24Y_e^{pr}Y_e^{ab} \\
& + 31Y_e^{pb}Y_e^{ar} \Big\} + \mu_H^2 \Big\{ g_L^2 \Big( \frac{9}{2}\delta^{pa}\delta^{rb}\text{Tr}[Y_e^\dagger Y_e] + \frac{27}{2}\delta^{pa}\delta^{rb}\text{Tr}[Y_d^\dagger Y_d] - \frac{3}{8} \Big( 4Y_e^{*ab}Y_e^{pr} - 9\delta^{pa}(Y_e^\dagger Y_e)^{br} - 42\delta^{rb}(Y_e Y_e^\dagger)^{pa} \Big) \Big) + \frac{27}{2}\delta^{pa}\delta^{rb}g_L^4 \\
& - 6\delta^{pa}\delta^{rb}g_Y^2g_L^2 \Big\} C_{eW}^{ab} + \frac{3}{8}\mu_H^2g_L^2C_{eW}^{*ab} \Big\{ 5Y_e^{pb}Y_e^{ar} + 8Y_e^{pr}Y_e^{ab} \Big\} - 5\mu_H^2g_Y^2Y_u^{*ab}C_{uB}^{ab}Y_e^{pr} - 5\mu_H^2g_Y^2C_{uB}^{*ab}Y_e^{pr}Y_u^{ab} - \frac{9}{2}\mu_H^2g_L^2Y_u^{*ab}C_{uW}^{ab}Y_e^{pr} \\
& - \frac{9}{2}\mu_H^2g_L^2C_{uW}^{*ab}Y_e^{pr}Y_u^{ab} - 16\mu_H^2g_s^2Y_u^{*ab}C_{uG}^{ab}Y_e^{pr} - 16\mu_H^2g_s^2C_{uG}^{*ab}Y_e^{pr}Y_u^{ab} + \mu_H^2g_Y^2Y_d^{*ab}C_{dB}^{ab}Y_e^{pr} - 26\mu_H^2g_Y^2C_{dB}^{*ab}Y_d^{ab}Y_e^{pr} \\
& - \frac{9}{2}\mu_H^2g_L^2Y_d^{*ab}C_{dW}^{ab}Y_e^{pr} + 9\mu_H^2g_L^2C_{dW}^{*ab}Y_d^{ab}Y_e^{pr} - 16\mu_H^2g_s^2Y_d^{*ab}C_{dG}^{ab}Y_e^{pr} - 16\mu_H^2g_s^2C_{dG}^{*ab}Y_d^{ab}Y_e^{pr} + \mu_H^2 \Big\{ \frac{1}{36}g_Y^2 \Big( 16\delta^{ab}Y_e^{pr} - 859\delta^{pa}Y_e^{br} \Big) \\
& + \frac{1}{6} \Big( 3Y_e^{br}(Y_e Y_e^\dagger)^{pa} - 20Y_e^{pr}(Y_e Y_e^\dagger)^{ba} - 24T_2\delta^{pa}Y_e^{br} - 51\delta^{pa}(Y_e Y_e^\dagger Y_e)^{br} \Big) + \frac{21}{4}\delta^{pa}g_L^2Y_e^{br} \Big\} C_{H\ell}^{(\parallel)ab} + \mu_H^2 \Big\{ \frac{1}{36}g_Y^2 \Big( 8\delta^{ab}Y_e^{pr} - 605\delta^{pa}Y_e^{br} \Big) \\
& + \frac{1}{12}g_L^2 \Big( 221\delta^{pa}Y_e^{br} - 8\delta^{ab}Y_e^{pr} \Big) + \frac{1}{3} \Big( 3Y_e^{br}(Y_e Y_e^\dagger)^{pa} - 15\delta^{pa}(Y_e Y_e^\dagger Y_e)^{br} - 20Y_e^{pr}(Y_e Y_e^\dagger)^{ba} - 24T_2\delta^{pa}Y_e^{br} \Big) \Big\} C_{H\ell}^{(\times)ab} + \mu_H^2 \Big\{ \frac{1}{36}g_Y^2 \Big( 16\delta^{ab}Y_e^{pr} \\
& - 431\delta^{rb}Y_e^{pa} \Big) + \frac{1}{3} \Big( 10Y_e^{pr}(Y_e^\dagger Y_e)^{ba} + 12T_2\delta^{rb}Y_e^{pa} + 15\delta^{rb}(Y_e Y_e^\dagger Y_e)^{pa} - 3Y_e^{pa}(Y_e^\dagger Y_e)^{br} \Big) + \frac{21}{4}\delta^{rb}g_L^2Y_e^{pa} \Big\} C_{He}^{ab} - \mu_H^2 \Big\{ \frac{4}{9}\delta^{ab}g_Y^2Y_e^{pr} \\
& + 10 \Big( Y_e^{pr}(Y_d Y_d^\dagger)^{ba} - Y_e^{pr}(Y_u Y_u^\dagger)^{ba} \Big) \Big\} C_{Hq}^{(\parallel)ab} - \mu_H^2 \Big\{ \frac{2}{9}\delta^{ab}g_Y^2Y_e^{pr} + 2\delta^{ab}g_L^2Y_e^{pr} + 10 \Big( Y_e^{pr}(Y_u Y_u^\dagger)^{ba} + 2Y_e^{pr}(Y_d Y_d^\dagger)^{ba} \Big) \Big\} C_{Hq}^{(\times)ab} - \mu_H^2 \Big\{ \frac{8}{9}\delta^{ab}g_Y^2Y_e^{pr} \\
& + 10Y_e^{pr}(Y_u^\dagger Y_u)^{ba} \Big\} C_{Hu}^{ab} + \mu_H^2 \Big\{ \frac{4}{9}\delta^{ab}g_Y^2Y_e^{pr} + 10Y_e^{pr}(Y_d^\dagger Y_d)^{ba} \Big\} C_{Hd}^{ab} + 10\mu_H^2C_{Hud}^{ab}Y_e^{pr}(Y_d^\dagger Y_u)^{ba} + 10\mu_H^2C_{Hud}^{*ab}Y_e^{pr}(Y_u^\dagger Y_d)^{ab} \\
& + \mu_H^2 \Big\{ \frac{1}{18}g_Y^2 \Big( 14\delta^{rd}\delta^{ab}Y_e^{pc} + 70\delta^{pa}\delta^{cd}Y_e^{br} - 81\delta^{pa}\delta^{rd}Y_e^{bc} \Big) + \delta^{pa}Y_e^{bc}(Y_e^\dagger Y_e)^{dr} + 2\delta^{pa}Y_e^{br}(Y_e^\dagger Y_e)^{dc} + 2\delta^{rd}Y_e^{bc}(Y_e Y_e^\dagger)^{pa} + 2\delta^{rd}Y_e^{pc}(Y_e Y_e^\dagger)^{ba} \\
& + 2\delta^{pa}\delta^{rd}Y_e^{bc}\text{Tr}[Y_e^\dagger Y_e] + 3Y_e^{*ad}Y_e^{pc}Y_e^{br} + 24\delta^{pa}\delta^{rd}(Y_e Y_e^\dagger Y_e)^{bc} - \frac{3}{2}\delta^{pa}\delta^{rd}g_L^2Y_e^{bc} - 2Y_e^{*ad}Y_e^{pr}Y_e^{bc} \Big\} C_{\ell e}^{abcd} + \mu_H^2 \Big\{ 6\delta^{pa}Y_e^{br}(Y_u^\dagger Y_u)^{dc} \\
& - \frac{70}{9}\delta^{pa}\delta^{cd}g_Y^2Y_e^{br} \Big\} C_{\ell u}^{abcd} + \mu_H^2 \Big\{ 3\delta^{pa}Y_e^{br}(Y_d^\dagger Y_d)^{dc} + \frac{35}{9}\delta^{pa}\delta^{cd}g_Y^2Y_e^{br} \Big\} C_{\ell d}^{abcd} + \mu_H^2 \Big\{ 3 \Big( \delta^{rd}Y_e^{pc}(Y_d Y_d^\dagger)^{ba} + 2\delta^{rd}Y_e^{pc}(Y_u Y_u^\dagger)^{ba} \Big)
\end{aligned}$$

$$\begin{aligned}
& -\frac{7}{9}\delta^{rd}\delta^{ab}g_Y^2Y_e^{pc}\left\{C_{qe}^{abcd}-12\mu_H^2Y_u^{*ad}C_{qu}^{(\parallel)abcd}Y_e^{pr}Y_u^{bc}-36\mu_H^2Y_u^{*ad}C_{qu}^{(\times)abcd}Y_e^{pr}Y_u^{bc}-12\mu_H^2Y_d^{*ad}C_{qd}^{(\parallel)abcd}Y_d^{bc}Y_e^{pr}-36\mu_H^2Y_d^{*ad}C_{qd}^{(\times)abcd}Y_d^{bc}Y_e^{pr}\right. \\
& +\mu_H^2\left\{\frac{16}{9}\delta^{rb}\delta^{ad}g_Y^2Y_e^{pc}+8\delta^{rb}Y_e^{pa}(Y_e^\dagger Y_e)^{dc}\right\}C_{ee}^{abcd}-\mu_H^2\left\{\frac{14}{9}\delta^{rb}\delta^{cd}g_Y^2Y_e^{pa}+6\delta^{rb}Y_e^{pa}(Y_u^\dagger Y_u)^{dc}\right\}C_{eu}^{abcd}+\mu_H^2\left\{\frac{7}{9}\delta^{rb}\delta^{cd}g_Y^2Y_e^{pa}\right. \\
& +15\delta^{rb}Y_e^{pa}(Y_d^\dagger Y_d)^{dc}\left\}C_{ed}^{abcd}+\mu_H^2\left\{40\delta^{pa}\delta^{rb}g_s^2Y_d^{dc}-\frac{3}{4}\left(3\delta^{pa}Y_d^{dc}(Y_e^\dagger Y_e)^{br}+6\delta^{rb}Y_d^{dc}(Y_e Y_e^\dagger)^{pa}+14\delta^{pa}\delta^{rb}(Y_u Y_u^\dagger Y_d)^{dc}+18\delta^{pa}\delta^{rb}(Y_d Y_d^\dagger Y_d)^{dc}\right)\right. \\
& -3\delta^{pa}\delta^{rb}Y_d^{dc}\text{Tr}[Y_e^\dagger Y_e]-\frac{19}{6}\delta^{pa}\delta^{rb}g_Y^2Y_d^{dc}-\frac{9}{2}\delta^{pa}\delta^{rb}g_L^2Y_d^{dc}\left\}C_{ledq}^{abcd}-\frac{3}{4}\mu_H^2C_{ledq}^{*abcd}\left\{4Y_d^{*dc}Y_e^{pr}Y_e^{ab}+9Y_d^{*dc}Y_e^{pb}Y_e^{ar}\right\}+\mu_H^2\left\{\frac{3}{4}\left(3\delta^{pa}Y_u^{*cd}(Y_e^\dagger Y_e)^{br}\right.\right. \\
& +6\delta^{rb}Y_u^{*cd}(Y_e Y_e^\dagger)^{pa}+14\delta^{pa}\delta^{rb}(Y_d^\dagger Y_d Y_u^\dagger)^{cd}+18\delta^{pa}\delta^{rb}(Y_u^\dagger Y_u Y_u^\dagger)^{cd}\left.\right\}+3\delta^{pa}\delta^{rb}Y_u^{*cd}\text{Tr}[Y_e^\dagger Y_e]-\frac{9}{4}\delta^{pa}\delta^{rb}g_L^2Y_u^{*cd}-\frac{49}{12}\delta^{pa}\delta^{rb}g_Y^2Y_u^{*cd} \\
& -40\delta^{pa}\delta^{rb}g_s^2Y_u^{*cd}\left\}C_{lequ}^{abcd}+\frac{3}{4}\mu_H^2C_{lequ}^{*abcd}\left\{4Y_e^{pr}Y_e^{ab}Y_u^{cd}+9Y_e^{pb}Y_e^{ar}Y_u^{cd}\right\}+\mu_H^2\left\{\frac{239}{24}\delta^{pa}\delta^{rd}g_Y^2Y_u^{*cb}+34\delta^{pa}\delta^{rd}g_s^2Y_u^{*cb}-\frac{3}{8}\left(3\delta^{pa}Y_u^{*cb}(Y_e^\dagger Y_e)^{dr}\right.\right. \\
& +6\delta^{rd}Y_u^{*cb}(Y_e Y_e^\dagger)^{pa}+10\delta^{pa}\delta^{rd}(Y_d^\dagger Y_d Y_u^\dagger)^{cb}+18\delta^{pa}\delta^{rd}(Y_u^\dagger Y_u Y_u^\dagger)^{cb}\left.\right)-\frac{9}{8}\delta^{pa}\delta^{rd}g_L^2Y_u^{*cb}-\frac{3}{2}\delta^{pa}\delta^{rd}Y_u^{*cb}\text{Tr}[Y_e^\dagger Y_e]\left\}C_{luqe}^{abcd}-\frac{3}{8}\mu_H^2C_{luqe}^{*abcd}\left\{4Y_e^{pr}Y_e^{ad}Y_u^{cb}\right.\right. \\
& +9Y_e^{pd}Y_e^{ar}Y_u^{cb}\left.\right\}+\mu_H^2\left\{\frac{5}{9}g_Y^2\left(\delta^{pa}\delta^{bc}Y_e^{dr}+14\delta^{pa}\delta^{cd}Y_e^{br}\right)+8\delta^{pa}Y_e^{br}(Y_e Y_e^\dagger)^{dc}-\frac{1}{3}\delta^{pa}\delta^{bc}g_L^2Y_e^{dr}\right\}C_{\ell\ell}^{abcd}+\mu_H^2\left\{3\left(5\delta^{pa}Y_e^{br}(Y_d Y_d^\dagger)^{dc}\right.\right. \\
& \left.\left.-2\delta^{pa}Y_e^{br}(Y_u Y_u^\dagger)^{dc}\right)-\frac{35}{9}\delta^{pa}\delta^{cd}g_Y^2Y_e^{br}\right\}C_{\ell q}^{(\parallel)abcd}+\mu_H^2\left\{6\left(\delta^{pa}Y_e^{br}(Y_u Y_u^\dagger)^{dc}+5\delta^{pa}Y_e^{br}(Y_d Y_d^\dagger)^{dc}\right)-\frac{35}{18}\delta^{pa}\delta^{cd}g_Y^2Y_e^{br}-\frac{7}{2}\delta^{pa}\delta^{cd}g_L^2Y_e^{br}\right\}C_{\ell q}^{(\times)abcd}, \quad (2.6)
\end{aligned}$$

## 2.4 Up-quark Yukawa

$$\begin{aligned}
\beta_{Y_u^{pr}}^{(1)} &= \left\{\frac{1}{2}\left(2T_2Y_u^{pr}+3(Y_u Y_u^\dagger Y_u)^{pr}-3(Y_d Y_d^\dagger Y_u)^{pr}\right)-\frac{17}{12}g_Y^2Y_u^{pr}-\frac{9}{4}g_L^2Y_u^{pr}-8g_s^2Y_u^{pr}\right\}+2\mu_H^2C_{HD}^{(\parallel)}Y_u^{pr}+\mu_H^2C_{HD}^{(\times)}Y_u^{pr}+6\delta^{pa}\delta^{rb}\mu_H^2C_{uH}^{ab} \\
& -2\delta^{pa}\mu_H^2C_{Hq}^{(\parallel)ab}Y_u^{br}+2\delta^{pa}\mu_H^2C_{Hq}^{(\times)ab}Y_u^{br}+2\delta^{rb}\mu_H^2C_{Hu}^{ab}Y_u^{pa}-2\delta^{ra}\mu_H^2C_{Hud}^{*ab}Y_d^{pb}-4\delta^{pa}\delta^{rd}\mu_H^2C_{qu}^{(\parallel)abcd}Y_u^{bc}-12\delta^{pa}\delta^{rd}\mu_H^2C_{qu}^{(\times)abcd}Y_u^{bc} \\
& +\mu_H^2\left\{\delta^{pc}\delta^{rb}Y_d^{*ad}+6\delta^{pa}\delta^{rb}Y_d^{*cd}\right\}C_{quqd}^{(\parallel)abcd}+\mu_H^2\left\{2\delta^{pa}\delta^{rb}Y_d^{*cd}+3\delta^{pc}\delta^{rb}Y_d^{*ad}\right\}C_{quqd}^{(\times)abcd}-2\delta^{pc}\delta^{rd}\mu_H^2Y_e^{*ab}C_{lequ}^{abcd}+\delta^{pc}\delta^{rb}\mu_H^2Y_e^{*ad}C_{luqe}^{abcd}, \quad (2.7)
\end{aligned}$$

$$\begin{aligned}
\beta_{Y_u^{pr}}^{(2)} &= \left\{\frac{3}{16}g_L^2\left(3(Y_d Y_d^\dagger Y_u)^{pr}+10T_2Y_u^{pr}+45(Y_u Y_u^\dagger Y_u)^{pr}\right)+\frac{1}{4}\left(5T_2(Y_d Y_d^\dagger Y_u)^{pr}+6(Y_u Y_u^\dagger Y_u Y_u^\dagger Y_u)^{pr}+11(Y_d Y_d^\dagger Y_d Y_d^\dagger Y_u)^{pr}\right.\right. \\
& \left.\left.-(Y_u Y_u^\dagger Y_d Y_d^\dagger Y_u)^{pr}-4(Y_d Y_d^\dagger Y_u Y_u^\dagger Y_u)^{pr}-9T_4Y_u^{pr}-9T_2(Y_u Y_u^\dagger Y_u)^{pr}\right)+g_Y^2\left(\frac{1}{48}\left(223(Y_u Y_u^\dagger Y_u)^{pr}-43(Y_d Y_d^\dagger Y_u)^{pr}\right)+\frac{25}{24}Y_u^{pr}\text{Tr}[Y_d^\dagger Y_d]\right)\right\}
\end{aligned}$$

$$\begin{aligned}
& + \frac{25}{8} Y_u^{pr} \text{Tr}[Y_e^\dagger Y_e] + \frac{85}{24} Y_u^{pr} \text{Tr}[Y_u^\dagger Y_u] \Big) + g_s^2 \Big( 20 Y_u^{pr} \text{Tr}[Y_d^\dagger Y_d] + 20 Y_u^{pr} \text{Tr}[Y_u^\dagger Y_u] - 16 \Big( (Y_d Y_d^\dagger Y_u)^{pr} - (Y_u Y_u^\dagger Y_u)^{pr} \Big) + \frac{3}{2} \lambda^2 Y_u^{pr} \\
& + \frac{3}{2} Y_u^{pr} \text{Tr}[Y_d^\dagger Y_d Y_u^\dagger Y_u] + \frac{19}{9} g_Y^2 g_s^2 Y_u^{pr} + \frac{1187}{216} g_Y^4 Y_u^{pr} + 9 g_s^2 g_L^2 Y_u^{pr} - \frac{3}{4} g_Y^2 g_L^2 Y_u^{pr} - \frac{23}{4} g_L^4 Y_u^{pr} - 6 \lambda (Y_u Y_u^\dagger Y_u)^{pr} - 108 g_s^4 Y_u^{pr} \Big\} \\
& - 10 \mu_H^2 Y_u^{pr} \mathbf{T}_{\ell H} + \mu_H^2 \left\{ \frac{1}{2} \Big( (Y_d Y_d^\dagger Y_u)^{pr} - 8 \text{T}_2 Y_u^{pr} - 9 (Y_u Y_u^\dagger Y_u)^{pr} \Big) + \frac{199}{36} g_Y^2 Y_u^{pr} + \frac{199}{12} g_L^2 Y_u^{pr} - \frac{1}{2} \lambda Y_u^{pr} \right\} C_{HD}^{(\text{II})} + \mu_H^2 \left\{ \frac{1}{2} \Big( - (Y_d Y_d^\dagger Y_u)^{pr} \right. \\
& - 4 \text{T}_2 Y_u^{pr} - 9 (Y_u Y_u^\dagger Y_u)^{pr} \Big) + \frac{91}{18} g_Y^2 Y_u^{pr} + 6 g_L^2 Y_u^{pr} - \frac{1}{2} \lambda Y_u^{pr} \Big\} C_{HD}^{(*)} + \frac{3}{2} \mu_H^2 g_Y^4 C_{HB} Y_u^{pr} + \frac{199i}{36} \mu_H^2 g_Y^4 C_{H\bar{B}} Y_u^{pr} + \frac{9}{2} \mu_H^2 g_L^4 C_{HW} Y_u^{pr} \\
& + \frac{21i}{4} \mu_H^2 g_L^4 C_{H\bar{W}} Y_u^{pr} + \frac{136i}{3} \mu_H^2 g_s^4 C_{H\bar{G}} Y_u^{pr} + \frac{9}{4} \mu_H^2 g_Y^2 g_L^2 C_{HWB} Y_u^{pr} - \frac{47i}{8} \mu_H^2 g_Y^2 g_L^2 C_{H\bar{W}B} Y_u^{pr} + 18 \mu_H^2 g_L^6 C_W Y_u^{pr} + \frac{5i}{4} \mu_H^2 g_L^6 C_{\bar{W}} Y_u^{pr} \\
& - 88 \mu_H^2 g_s^6 C_G Y_u^{pr} - \frac{112i}{3} \mu_H^2 g_s^6 C_{\bar{G}} Y_u^{pr} + \mu_H^2 \left\{ 12 \delta^{pa} \delta^{rb} g_Y^2 + 36 \delta^{pa} \delta^{rb} g_L^2 - 3 \Big( \delta^{pa} (Y_u^\dagger Y_u)^{br} + \delta^{rb} (Y_u Y_u^\dagger)^{pa} + 4 \text{T}_2 \delta^{pa} \delta^{rb} \Big) \right. \\
& \left. - 15 \delta^{pa} \delta^{rb} \lambda \right\} C_{uH}^{ab} + 3 \mu_H^2 g_Y^2 Y_e^{*ab} C_{eB}^{ab} Y_u^{pr} + 3 \mu_H^2 g_Y^2 C_{eB}^{*ab} Y_e^{ab} Y_u^{pr} - \frac{3}{2} \mu_H^2 g_L^2 Y_e^{*ab} C_{eW}^{ab} Y_u^{pr} - \frac{3}{2} \mu_H^2 g_L^2 C_{eW}^{*ab} Y_e^{ab} Y_u^{pr} \\
& + \mu_H^2 \left\{ g_Y^2 \Big( \frac{1}{12} \Big( 38 \delta^{rb} (Y_u Y_u^\dagger)^{pa} + 104 \delta^{rb} (Y_d Y_d^\dagger)^{pa} + 373 \delta^{pa} (Y_u^\dagger Y_u)^{br} - 60 Y_u^{*ab} Y_u^{pr} \Big) + 15 \delta^{pa} \delta^{rb} \text{Tr}[Y_u^\dagger Y_u] \Big) + \frac{160}{9} \delta^{pa} \delta^{rb} g_Y^2 g_s^2 + \frac{580}{27} \delta^{pa} \delta^{rb} g_Y^4 \right. \\
& \left. - 10 \delta^{pa} \delta^{rb} g_Y^2 g_L^2 \right\} C_{uB}^{ab} + \frac{1}{4} \mu_H^2 g_Y^2 C_{uB}^{*ab} \left\{ 19 Y_u^{pb} Y_u^{ar} + 40 Y_u^{pr} Y_u^{ab} \right\} + \mu_H^2 \left\{ g_L^2 \Big( \frac{27}{2} \delta^{pa} \delta^{rb} \text{Tr}[Y_u^\dagger Y_u] - \frac{9}{8} \Big( 4 Y_u^{*ab} Y_u^{pr} - 3 \delta^{pa} (Y_u^\dagger Y_u)^{br} \right. \right. \\
& \left. \left. - 14 \delta^{rb} (Y_u Y_u^\dagger)^{pa} - 16 \delta^{rb} (Y_d Y_d^\dagger)^{pa} \Big) \right) + \frac{27}{2} \delta^{pa} \delta^{rb} g_L^4 + 16 \delta^{pa} \delta^{rb} g_s^2 g_L^2 - \frac{17}{3} \delta^{pa} \delta^{rb} g_Y^2 g_L^2 \right\} C_{uW}^{ab} + \frac{3}{8} \mu_H^2 g_L^2 C_{uW}^{*ab} \left\{ 5 Y_u^{pb} Y_u^{ar} + 24 Y_u^{pr} Y_u^{ab} \right\} \\
& + \mu_H^2 \left\{ \frac{56}{27} \delta^{pa} \delta^{rb} g_Y^2 g_s^2 + \frac{224}{9} \delta^{pa} \delta^{rb} g_s^4 - \frac{4}{3} g_s^2 \Big( 12 Y_u^{*ab} Y_u^{pr} - 4 \delta^{rb} (Y_d Y_d^\dagger)^{pa} - 29 \delta^{pa} (Y_u^\dagger Y_u)^{br} - 34 \delta^{rb} (Y_u Y_u^\dagger)^{pa} \Big) - 8 \delta^{pa} \delta^{rb} g_s^2 g_L^2 \right\} C_{uG}^{ab} \\
& + 4 \mu_H^2 g_s^2 C_{uG}^{*ab} \left\{ 3 Y_u^{pb} Y_u^{ar} - 4 Y_u^{pr} Y_u^{ab} \right\} + \frac{1}{4} \mu_H^2 g_Y^2 \left\{ 4 Y_d^{*ab} Y_u^{pr} + 21 \delta^{pa} (Y_d^\dagger Y_u)^{br} \right\} C_{dB}^{ab} + \frac{1}{12} \mu_H^2 g_Y^2 C_{dB}^{*ab} \left\{ 12 Y_d^{ab} Y_u^{pr} - 115 Y_d^{pb} Y_u^{ar} \right\} \\
& - \frac{3}{8} \mu_H^2 g_L^2 \left\{ 12 Y_d^{*ab} Y_u^{pr} - 13 \delta^{pa} (Y_d^\dagger Y_u)^{br} \right\} C_{dW}^{ab} - \frac{3}{8} \mu_H^2 g_L^2 C_{dW}^{*ab} \left\{ 12 Y_d^{ab} Y_u^{pr} - 35 Y_d^{pb} Y_u^{ar} \right\} - 4 \mu_H^2 g_s^2 \left\{ 4 Y_d^{*ab} Y_u^{pr} - 3 \delta^{pa} (Y_d^\dagger Y_u)^{br} \right\} C_{dG}^{ab} \\
& - \frac{4}{3} \mu_H^2 g_s^2 C_{dG}^{*ab} \left\{ 12 Y_d^{ab} Y_u^{pr} + 17 Y_d^{pb} Y_u^{ar} \right\} + \mu_H^2 \left\{ \frac{4}{9} \delta^{ab} g_Y^2 Y_u^{pr} - \frac{10}{3} Y_u^{pr} (Y_e Y_e^\dagger)^{ba} \right\} C_{H\ell}^{(\text{II})ab} + \mu_H^2 \left\{ \frac{2}{9} \delta^{ab} g_Y^2 Y_u^{pr} - \frac{2}{3} \delta^{ab} g_L^2 Y_u^{pr} \right.
\end{aligned}$$

$$\begin{aligned}
& -\frac{20}{3}Y_u^{pr}(Y_e Y_e^\dagger)^{ba} \left\} C_{He}^{(\times)ab} + \mu_H^2 \left\{ \frac{4}{9}\delta^{ab}g_Y^2 Y_u^{pr} + \frac{10}{3}Y_u^{pr}(Y_e^\dagger Y_e)^{ba} \right\} C_{He}^{ab} + \mu_H^2 \left\{ \frac{1}{108}g_Y^2 (1885\delta^{pa}Y_u^{br} - 48\delta^{ab}Y_u^{pr}) + \frac{1}{2}(Y_u^{br}(Y_d Y_d^\dagger)^{pa} \right. \\
& + 8T_2\delta^{pa}Y_u^{br} + 17\delta^{pa}(Y_u Y_u^\dagger Y_u)^{br} + 20Y_u^{pr}(Y_u Y_u^\dagger)^{ba} - Y_u^{br}(Y_u Y_u^\dagger)^{pa} - \delta^{pa}(Y_d Y_d^\dagger Y_u)^{br} - 20Y_u^{pr}(Y_d Y_d^\dagger)^{ba} \Big) - \frac{21}{4}\delta^{pa}g_L^2 Y_u^{br} - \frac{16}{3}\delta^{pa}g_s^2 Y_u^{br} \Big\} C_{Hq}^{(\parallel)ab} \\
& + \mu_H^2 \left\{ \frac{1}{54}g_Y^2 (271\delta^{pa}Y_u^{br} - 12\delta^{ab}Y_u^{pr}) + \frac{1}{6}g_L^2 (79\delta^{pa}Y_u^{br} - 12\delta^{ab}Y_u^{pr}) + \frac{1}{2}(Y_u^{br}(Y_u Y_u^\dagger)^{pa} + 2Y_u^{br}(Y_d Y_d^\dagger)^{pa} + 7\delta^{pa}(Y_u Y_u^\dagger Y_u)^{br} - 2\delta^{pa}(Y_d Y_d^\dagger Y_u)^{br} \right. \\
& - 8T_2\delta^{pa}Y_u^{br} - 20Y_u^{pr}(Y_u Y_u^\dagger)^{ba} - 40Y_u^{pr}(Y_d Y_d^\dagger)^{ba} \Big) + \frac{16}{3}\delta^{pa}g_s^2 Y_u^{br} \Big\} C_{Hq}^{(\times)ab} + \mu_H^2 \left\{ \frac{1}{108}g_Y^2 (265\delta^{rb}Y_u^{pa} - 96\delta^{ab}Y_u^{pr}) + Y_u^{pa}(Y_u^\dagger Y_u)^{br} \right. \\
& + 4\delta^{rb}(Y_d Y_d^\dagger Y_u)^{pa} + \frac{16}{3}\delta^{rb}g_s^2 Y_u^{pa} - 4T_2\delta^{rb}Y_u^{pa} - 5\delta^{rb}(Y_u Y_u^\dagger Y_u)^{pa} - \frac{21}{4}\delta^{rb}g_L^2 Y_u^{pa} - 10Y_u^{pr}(Y_u^\dagger Y_u)^{ba} \Big\} C_{Hu}^{ab} + \mu_H^2 \left\{ \frac{4}{9}\delta^{ab}g_Y^2 Y_u^{pr} \right. \\
& + 10Y_u^{pr}(Y_d^\dagger Y_d)^{ba} \Big\} C_{Hd}^{ab} + \mu_H^2 \left\{ 10Y_u^{pr}(Y_d^\dagger Y_u)^{ba} - Y_u^{pa}(Y_d^\dagger Y_u)^{br} \right\} C_{Hud}^{ab} + \mu_H^2 C_{Hud}^{*ab} \left\{ 3\delta^{ra}(Y_d Y_d^\dagger Y_d)^{pb} + 4T_2\delta^{ra}Y_d^{pb} + \frac{21}{4}\delta^{ra}g_L^2 Y_d^{pb} \right. \\
& + 10Y_u^{pr}(Y_u^\dagger Y_d)^{ab} - 2\delta^{ra}(Y_u Y_u^\dagger Y_d)^{pb} - \frac{16}{3}\delta^{ra}g_s^2 Y_d^{pb} - \frac{271}{36}\delta^{ra}g_Y^2 Y_d^{pb} \Big\} - 4\mu_H^2 Y_e^{*ad} C_{le}^{abcd} Y_e^{bc} Y_u^{pr} + \mu_H^2 \left\{ \frac{7}{27}\delta^{rd}\delta^{ab}g_Y^2 Y_u^{pc} \right. \\
& + 2\delta^{rd}Y_u^{pc}(Y_e Y_e^\dagger)^{ba} \Big\} C_{lu}^{abcd} + \mu_H^2 \left\{ 2\delta^{pa}Y_u^{br}(Y_e^\dagger Y_e)^{dc} - \frac{77}{27}\delta^{pa}\delta^{cd}g_Y^2 Y_u^{br} \right\} C_{qe}^{abcd} + \mu_H^2 \left\{ \frac{1}{54}g_Y^2 (308\delta^{pa}\delta^{cd}Y_u^{br} - 14\delta^{rd}\delta^{ab}Y_u^{pc} - 75\delta^{pa}\delta^{rd}Y_u^{bc}) \right. \\
& + \frac{1}{2}(2\delta^{pa}Y_u^{bc}(Y_u^\dagger Y_u)^{dr} + 4\delta^{rd}Y_u^{bc}(Y_u Y_u^\dagger)^{pa} + 6Y_u^{*ad}Y_u^{pc}Y_u^{br} + 9\delta^{pa}\delta^{rd}(Y_d Y_d^\dagger Y_u)^{bc} + 12\delta^{pa}Y_u^{br}(Y_u^\dagger Y_u)^{dc} + 12\delta^{rd}Y_u^{pc}(Y_d Y_d^\dagger)^{ba} + 12\delta^{rd}Y_u^{pc}(Y_u Y_u^\dagger)^{ba} \\
& + 48\delta^{pa}\delta^{rd}(Y_u Y_u^\dagger Y_u)^{bc} - 4\delta^{rd}Y_u^{bc}(Y_d Y_d^\dagger)^{pa} - 12Y_u^{*ad}Y_u^{pr}Y_u^{bc} \Big) + 6\delta^{pa}\delta^{rd}Y_u^{bc} \text{Tr}[Y_u^\dagger Y_u] - \frac{3}{2}\delta^{pa}\delta^{rd}g_L^2 Y_u^{bc} - \frac{32}{3}\delta^{pa}\delta^{rd}g_s^2 Y_u^{bc} \Big\} C_{qu}^{(\parallel)abcd} \\
& + \mu_H^2 \left\{ \frac{1}{162}g_Y^2 (308\delta^{pa}\delta^{cd}Y_u^{br} - 14\delta^{rd}\delta^{ab}Y_u^{pc} - 675\delta^{pa}\delta^{rd}Y_u^{bc}) + \frac{1}{2}(4\delta^{pa}Y_u^{br}(Y_u^\dagger Y_u)^{dc} + 4\delta^{rd}Y_u^{pc}(Y_d Y_d^\dagger)^{ba} + 4\delta^{rd}Y_u^{pc}(Y_u Y_u^\dagger)^{ba} + 6\delta^{pa}Y_u^{bc}(Y_u^\dagger Y_u)^{dr} \right. \\
& + 12\delta^{rd}Y_u^{bc}(Y_u Y_u^\dagger)^{pa} + 18Y_u^{*ad}Y_u^{pc}Y_u^{br} + 27\delta^{pa}\delta^{rd}(Y_d Y_d^\dagger Y_u)^{bc} + 144\delta^{pa}\delta^{rd}(Y_u Y_u^\dagger Y_u)^{bc} - 12\delta^{rd}Y_u^{bc}(Y_d Y_d^\dagger)^{pa} - 36Y_u^{*ad}Y_u^{pr}Y_u^{bc} \Big) \\
& + 18\delta^{pa}\delta^{rd}Y_u^{bc} \text{Tr}[Y_u^\dagger Y_u] - \frac{16}{27}g_s^2 (216\delta^{pa}\delta^{rd}Y_u^{bc} - 7\delta^{pa}\delta^{cd}Y_u^{br} - 14\delta^{rd}\delta^{ab}Y_u^{pc}) - \frac{9}{2}\delta^{pa}\delta^{rd}g_L^2 Y_u^{bc} \Big\} C_{qu}^{(\times)abcd} + \mu_H^2 \left\{ \frac{1}{2}(3Y_d^{*ad}Y_d^{pc}Y_u^{br} \right. \\
& + 12\delta^{pa}Y_u^{br}(Y_d^\dagger Y_d)^{dc} - 2\delta^{pa}Y_d^{bc}(Y_d^\dagger Y_u)^{dr} - 24Y_d^{*ad}Y_d^{bc}Y_u^{pr} \Big) - \frac{77}{27}\delta^{pa}\delta^{cd}g_Y^2 Y_u^{br} \Big\} C_{qd}^{(\parallel)abcd} + \mu_H^2 \left\{ \frac{1}{2}(4\delta^{pa}Y_u^{br}(Y_d^\dagger Y_d)^{dc} + 9Y_d^{*ad}Y_d^{pc}Y_u^{br} - 6\delta^{pa}Y_d^{bc}(Y_d^\dagger Y_u)^{dr} \right.
\end{aligned}$$

$$\begin{aligned}
& -72Y_d^{*ad}Y_d^{bc}Y_u^{pr}) + \frac{112}{27}\delta^{pa}\delta^{cd}g_s^2Y_u^{br} - \frac{77}{81}\delta^{pa}\delta^{cd}g_Y^2Y_u^{br} \Big\} C_{qd}^{(\times)abcd} + \mu_H^2 \Big\{ \frac{32}{27}\delta^{rb}\delta^{ad}g_s^2Y_u^{pc} + 24\delta^{rb}Y_u^{pa}(Y_u^\dagger Y_u)^{dc} - \frac{4}{81}g_Y^2(\delta^{rb}\delta^{ad}Y_u^{pc} \\
& + 21\delta^{rb}\delta^{cd}Y_u^{pa}) \Big\} C_{uu}^{abcd} + \mu_H^2 \Big\{ \frac{7}{27}\delta^{rd}\delta^{ab}g_Y^2Y_u^{pc} - 2\delta^{rd}Y_u^{pc}(Y_e^\dagger Y_e)^{ba} \Big\} C_{eu}^{abcd} + \mu_H^2 \Big\{ \frac{7}{27}\delta^{rb}\delta^{cd}g_Y^2Y_u^{pa} - \frac{3}{2}(\delta^{rb}Y_d^{pc}(Y_d^\dagger Y_u)^{da} \\
& + 4\delta^{rb}Y_u^{pa}(Y_d^\dagger Y_d)^{dc}) \Big\} C_{ud}^{(\parallel)abcd} + \mu_H^2 \Big\{ \frac{7}{81}\delta^{rb}\delta^{cd}g_Y^2Y_u^{pa} + \frac{1}{2}(-4\delta^{rb}Y_u^{pa}(Y_d^\dagger Y_d)^{dc} - 9\delta^{rb}Y_d^{pc}(Y_d^\dagger Y_u)^{da}) + \frac{112}{27}\delta^{rb}\delta^{cd}g_s^2Y_u^{pa} \Big\} C_{ud}^{(\times)abcd} \\
& - \frac{3}{4}\mu_H^2Y_e^{*ab}C_{ledq}^{abcd}Y_d^{pc}Y_u^{dr} + \frac{3}{4}\delta^{pd}\mu_H^2C_{ledq}^{*abcd}Y_e^{ab}(Y_d^\dagger Y_u)^{cr} + \mu_H^2 \Big\{ \frac{3}{8}g_L^2(6\delta^{pa}\delta^{rb}Y_d^{*cd} - \delta^{pc}\delta^{rb}Y_d^{*ad}) + \frac{3}{8}(\delta^{pa}Y_u^{*cb}(Y_d^\dagger Y_u)^{dr} + 2\delta^{rb}Y_d^{*ad}(Y_d Y_d^\dagger)^{pc} \\
& + 6\delta^{pc}Y_u^{*ab}(Y_d^\dagger Y_u)^{dr} + 12\delta^{rb}Y_d^{*cd}(Y_d Y_d^\dagger)^{pa} - \delta^{pc}Y_d^{*ad}(Y_u^\dagger Y_u)^{br} - 2\delta^{rb}Y_d^{*ad}(Y_u Y_u^\dagger)^{pc} - 2\delta^{pc}\delta^{rb}(Y_u^\dagger Y_u Y_d^\dagger)^{ad} - 6\delta^{pa}Y_d^{*cd}(Y_u^\dagger Y_u)^{br} - 6\delta^{pc}\delta^{rb}(Y_d^\dagger Y_d Y_d^\dagger)^{ad} \\
& - 12\delta^{rb}Y_d^{*cd}(Y_u Y_u^\dagger)^{pa} - 20\delta^{pa}\delta^{rb}(Y_u^\dagger Y_u Y_d^\dagger)^{cd} - 36\delta^{pa}\delta^{rb}(Y_d^\dagger Y_d Y_d^\dagger)^{cd}) + 4g_s^2(3\delta^{pc}\delta^{rb}Y_d^{*ad} + 10\delta^{pa}\delta^{rb}Y_d^{*cd}) - \frac{1}{24}g_Y^2(7\delta^{pc}\delta^{rb}Y_d^{*ad} + 22\delta^{pa}\delta^{rb}Y_d^{*cd}) \\
& - \frac{3}{2}(\delta^{pc}\delta^{rb}Y_d^{*ad} + 6\delta^{pa}\delta^{rb}Y_d^{*cd}) \text{Tr}[Y_u^\dagger Y_u] \Big\} C_{quqd}^{(\parallel)abcd} + \frac{1}{8}\mu_H^2(C_{quqd}^{(\parallel)*})^{abcd} \Big\{ 5Y_d^{pd}Y_u^{ar}Y_u^{cb} + 6Y_d^{pd}Y_u^{ab}Y_u^{cr} - 9Y_d^{ad}Y_u^{pb}Y_u^{cr} - 12Y_d^{ad}Y_u^{pr}Y_u^{cb} - 54Y_d^{cd}Y_u^{pb}Y_u^{ar} \\
& - 72Y_d^{cd}Y_u^{pr}Y_u^{ab} \Big\} + \mu_H^2 \Big\{ \frac{1}{8}(6\delta^{pc}Y_u^{*ab}(Y_d^\dagger Y_u)^{dr} + 9\delta^{pa}Y_u^{*cb}(Y_d^\dagger Y_u)^{dr} + 12\delta^{rb}Y_d^{*cd}(Y_d Y_d^\dagger)^{pa} + 18\delta^{rb}Y_d^{*ad}(Y_d Y_d^\dagger)^{pc} - 6\delta^{pa}Y_d^{*cd}(Y_u^\dagger Y_u)^{br} - 9\delta^{pc}Y_d^{*ad}(Y_u^\dagger Y_u)^{br} \\
& - 12\delta^{rb}Y_d^{*cd}(Y_u Y_u^\dagger)^{pa} - 18\delta^{rb}Y_d^{*ad}(Y_u Y_u^\dagger)^{pc} - 18\delta^{pc}\delta^{rb}(Y_u^\dagger Y_u Y_d^\dagger)^{ad} - 20\delta^{pa}\delta^{rb}(Y_u^\dagger Y_u Y_d^\dagger)^{cd} - 36\delta^{pa}\delta^{rb}(Y_d^\dagger Y_d Y_d^\dagger)^{cd} - 54\delta^{pc}\delta^{rb}(Y_d^\dagger Y_d Y_d^\dagger)^{ad}) \\
& + \frac{3}{8}g_L^2(2\delta^{pa}\delta^{rb}Y_d^{*cd} - 3\delta^{pc}\delta^{rb}Y_d^{*ad}) + \frac{8}{3}g_s^2(5\delta^{pa}\delta^{rb}Y_d^{*cd} + 18\delta^{pc}\delta^{rb}Y_d^{*ad}) - \frac{1}{72}g_Y^2(22\delta^{pa}\delta^{rb}Y_d^{*cd} + 63\delta^{pc}\delta^{rb}Y_d^{*ad}) - \frac{3}{2}(2\delta^{pa}\delta^{rb}Y_d^{*cd} \\
& + 3\delta^{pc}\delta^{rb}Y_d^{*ad}) \text{Tr}[Y_u^\dagger Y_u] \Big\} C_{quqd}^{(\times)abcd} + \frac{1}{8}\mu_H^2(C_{quqd}^{(\times)*})^{abcd} \Big\{ 2Y_d^{pd}Y_u^{ab}Y_u^{cr} + 15Y_d^{pd}Y_u^{ar}Y_u^{cb} - 18Y_d^{cd}Y_u^{pb}Y_u^{ar} - 24Y_d^{cd}Y_u^{pr}Y_u^{ab} - 27Y_d^{ad}Y_u^{pb}Y_u^{cr} \\
& - 36Y_d^{ad}Y_u^{pr}Y_u^{cb} \Big\} + \mu_H^2 \Big\{ \frac{3}{4}(\delta^{pc}Y_e^{*ab}(Y_u^\dagger Y_u)^{dr} + 2\delta^{rd}Y_e^{*ab}(Y_u Y_u^\dagger)^{pc} + 6\delta^{pc}\delta^{rd}(Y_e^\dagger Y_e Y_e^\dagger)^{ab} - 2\delta^{rd}Y_e^{*ab}(Y_d Y_d^\dagger)^{pc}) + 3\delta^{pc}\delta^{rd}Y_e^{*ab} \text{Tr}[Y_u^\dagger Y_u] \\
& - \frac{3}{4}\delta^{pc}\delta^{rd}g_L^2Y_e^{*ab} - \frac{21}{4}\delta^{pc}\delta^{rd}g_Y^2Y_e^{*ab} \Big\} C_{lequ}^{abcd} + \frac{3}{4}\mu_H^2C_{lequ}^{*abcd} \Big\{ 3Y_e^{ab}Y_u^{pd}Y_u^{cr} + 4Y_e^{ab}Y_u^{pr}Y_u^{cd} \Big\} + \mu_H^2 \Big\{ \frac{14}{3}\delta^{pc}\delta^{rb}g_s^2Y_e^{*ad} + \frac{379}{72}\delta^{pc}\delta^{rb}g_Y^2Y_e^{*ad} \\
& - \frac{3}{8}\delta^{pc}\delta^{rb}g_L^2Y_e^{*ad} - \frac{3}{8}(\delta^{pc}Y_e^{*ad}(Y_u^\dagger Y_u)^{br} + 2\delta^{rb}Y_e^{*ad}(Y_u Y_u^\dagger)^{pc} + 6\delta^{pc}\delta^{rb}(Y_e^\dagger Y_e Y_e^\dagger)^{ad} - 2\delta^{rb}Y_e^{*ad}(Y_d Y_d^\dagger)^{pc}) - \frac{3}{2}\delta^{pc}\delta^{rb}Y_e^{*ad} \text{Tr}[Y_u^\dagger Y_u] \Big\} C_{luqe}^{abcd} \\
& - \frac{3}{8}\mu_H^2C_{luqe}^{*abcd} \Big\{ 3Y_e^{ad}Y_u^{pb}Y_u^{cr} + 4Y_e^{ad}Y_u^{pr}Y_u^{cb} \Big\} + \mu_H^2 \Big\{ \frac{11}{81}g_Y^2(\delta^{pa}\delta^{bc}Y_u^{dr} + 42\delta^{pa}\delta^{cd}Y_u^{br}) + \frac{32}{27}\delta^{pa}\delta^{bc}g_s^2Y_u^{dr} - \frac{1}{3}\delta^{pa}\delta^{bc}g_L^2Y_u^{dr} - 3(\delta^{pa}Y_u^{dr}(Y_d Y_d^\dagger)^{bc}
\end{aligned}$$



$$\begin{aligned}
& + 4\delta^{pa}Y_u^{br}(Y_dY_d^\dagger)^{dc} - 8\delta^{pa}Y_u^{br}(Y_uY_u^\dagger)^{dc} \Big\} C_{qq}^{(\parallel)abcd} + \mu_H^2 \left\{ \frac{11}{81}g_Y^2(2\delta^{pa}\delta^{bc}Y_u^{dr} + 21\delta^{pa}\delta^{cd}Y_u^{br}) + \frac{64}{27}\delta^{pa}\delta^{bc}g_s^2Y_u^{dr} + 3(\delta^{pa}Y_u^{dr}(Y_dY_d^\dagger)^{bc} \right. \\
& + 4\delta^{pa}Y_u^{br}(Y_dY_d^\dagger)^{dc} + 16\delta^{pa}Y_u^{br}(Y_uY_u^\dagger)^{dc}) - 7\delta^{pa}\delta^{cd}g_L^2Y_u^{br} \Big\} C_{qq}^{(\times)abcd} - \mu_H^2 \left\{ 2\delta^{pc}Y_u^{dr}(Y_eY_e^\dagger)^{ba} + \frac{77}{27}\delta^{pc}\delta^{ab}g_Y^2Y_u^{dr} \right\} C_{\ell q}^{(\parallel)abcd} + \mu_H^2 \left\{ 2\delta^{pc}Y_u^{dr}(Y_eY_e^\dagger)^{ba} \right. \\
& \left. - \frac{7}{6}\delta^{pc}\delta^{ab}g_L^2Y_u^{dr} - \frac{77}{54}\delta^{pc}\delta^{ab}g_Y^2Y_u^{dr} \right\} C_{\ell q}^{(\times)abcd}, \tag{2.8}
\end{aligned}$$

## 2.5 Down-quark Yukawa

$$\begin{aligned}
\beta_{Y_d^{pr}}^{(1)} = & \left\{ \frac{1}{2}(2T_2Y_d^{pr} + 3(Y_dY_d^\dagger Y_d)^{pr} - 3(Y_uY_u^\dagger Y_d)^{pr}) - \frac{5}{12}g_Y^2Y_d^{pr} - \frac{9}{4}g_L^2Y_d^{pr} - 8g_s^2Y_d^{pr} \right\} + 2\mu_H^2 C_{HD}^{(\parallel)}Y_d^{pr} + \mu_H^2 C_{HD}^{(\times)}Y_d^{pr} + 6\delta^{pa}\delta^{rb}\mu_H^2 C_{dH}^{ab} \\
& + 2\delta^{pa}\mu_H^2 C_{Hq}^{(\parallel)ab}Y_d^{br} + 4\delta^{pa}\mu_H^2 C_{Hq}^{(\times)ab}Y_d^{br} - 2\delta^{rb}\mu_H^2 C_{Hd}^{ab}Y_d^{pa} - 2\delta^{rb}\mu_H^2 C_{Hud}^{ab}Y_u^{pa} - 4\delta^{pa}\delta^{rd}\mu_H^2 C_{qd}^{(\parallel)abcd}Y_d^{bc} - 12\delta^{pa}\delta^{rd}\mu_H^2 C_{qd}^{(\times)abcd}Y_d^{bc} \\
& + 2\delta^{pd}\delta^{rc}\mu_H^2 C_{ledq}^{*abcd}Y_e^{ab} + \mu_H^2 \left\{ \delta^{pa}\delta^{rd}Y_u^{*cb} + 6\delta^{pc}\delta^{rd}Y_u^{*ab} \right\} C_{quqd}^{(\parallel)abcd} + \mu_H^2 \left\{ 2\delta^{pc}\delta^{rd}Y_u^{*ab} + 3\delta^{pa}\delta^{rd}Y_u^{*cb} \right\} C_{quqd}^{(\times)abcd}, \tag{2.9}
\end{aligned}$$

$$\begin{aligned}
\beta_{Y_d^{pr}}^{(2)} = & \left\{ \frac{3}{16}g_L^2(3(Y_uY_u^\dagger Y_d)^{pr} + 10T_2Y_d^{pr} + 45(Y_dY_d^\dagger Y_d)^{pr}) + \frac{1}{4}(5T_2(Y_uY_u^\dagger Y_d)^{pr} + 6(Y_dY_d^\dagger Y_dY_d^\dagger Y_d)^{pr} + 11(Y_uY_u^\dagger Y_uY_u^\dagger Y_d)^{pr} \right. \\
& - (Y_dY_d^\dagger Y_uY_u^\dagger Y_d)^{pr} - 4(Y_uY_u^\dagger Y_dY_d^\dagger Y_d)^{pr} - 9T_4Y_d^{pr} - 9T_2(Y_dY_d^\dagger Y_d)^{pr}) + g_Y^2 \left( \frac{1}{48}(187(Y_dY_d^\dagger Y_d)^{pr} - 79(Y_uY_u^\dagger Y_d)^{pr}) + \frac{25}{24}Y_d^{pr} \text{Tr}[Y_d^\dagger Y_d] \right. \\
& + \frac{25}{8}Y_d^{pr} \text{Tr}[Y_e^\dagger Y_e] + \frac{85}{24}Y_d^{pr} \text{Tr}[Y_u^\dagger Y_u] \Big) + g_s^2(16((Y_dY_d^\dagger Y_d)^{pr} - (Y_uY_u^\dagger Y_d)^{pr}) + 20Y_d^{pr} \text{Tr}[Y_d^\dagger Y_d] + 20Y_d^{pr} \text{Tr}[Y_u^\dagger Y_u] \Big) + \frac{3}{2}\lambda^2Y_d^{pr} \\
& + \frac{3}{2}Y_d^{pr} \text{Tr}[Y_d^\dagger Y_dY_u^\dagger Y_u] + \frac{31}{9}g_Y^2g_s^2Y_d^{pr} + 9g_s^2g_L^2Y_d^{pr} - \frac{127}{216}g_Y^4Y_d^{pr} - \frac{9}{4}g_Y^2g_L^2Y_d^{pr} - \frac{23}{4}g_L^4Y_d^{pr} - 6\lambda(Y_dY_d^\dagger Y_d)^{pr} - 108g_s^4Y_d^{pr} \Big\} \\
& - 10\mu_H^2Y_d^{pr} \mathbf{T}_{\ell H} + \mu_H^2 \left\{ \frac{1}{2}((Y_uY_u^\dagger Y_d)^{pr} - 8T_2Y_d^{pr} - 9(Y_dY_d^\dagger Y_d)^{pr}) + \frac{199}{36}g_Y^2Y_d^{pr} + \frac{199}{12}g_L^2Y_d^{pr} - \frac{1}{2}\lambda Y_d^{pr} \right\} C_{HD}^{(\parallel)} + \mu_H^2 \left\{ \frac{1}{2}(-(Y_uY_u^\dagger Y_d)^{pr} \right. \\
& - 4T_2Y_d^{pr} - 9(Y_dY_d^\dagger Y_d)^{pr}) + \frac{91}{18}g_Y^2Y_d^{pr} + 6g_L^2Y_d^{pr} - \frac{1}{2}\lambda Y_d^{pr} \Big\} C_{HD}^{(\times)} + \frac{3}{2}\mu_H^2g_Y^4C_{HB}Y_d^{pr} - \frac{5i}{36}\mu_H^2g_Y^4C_{H\bar{B}}Y_d^{pr} + \frac{9}{2}\mu_H^2g_L^4C_{HW}Y_d^{pr} \\
& + \frac{21i}{4}\mu_H^2g_L^4C_{H\widetilde{W}}Y_d^{pr} + \frac{136i}{3}\mu_H^2g_s^4C_{HG}Y_d^{pr} + \frac{9}{4}\mu_H^2g_Y^2g_L^2C_{H\widetilde{W}B}Y_d^{pr} - \frac{13i}{8}\mu_H^2g_Y^2g_L^2C_{H\widetilde{W}B}Y_d^{pr} + 18\mu_H^2g_L^6C_WY_d^{pr} + \frac{5i}{4}\mu_H^2g_L^6C_{\widetilde{W}}Y_d^{pr} \\
& - 88\mu_H^2g_s^6C_GY_d^{pr} - \frac{112i}{3}\mu_H^2g_s^6C_{\widetilde{G}}Y_d^{pr} + \mu_H^2 \left\{ 12\delta^{pa}\delta^{rb}g_Y^2 + 36\delta^{pa}\delta^{rb}g_L^2 - 3(\delta^{pa}(Y_d^\dagger Y_d)^{br} + \delta^{rb}(Y_dY_d^\dagger)^{pa} + 4T_2\delta^{pa}\delta^{rb}) \right\}
\end{aligned}$$

$$\begin{aligned}
& -15\delta^{pa}\delta^{rb}\lambda \left\{ C_{dH}^{ab} + 3\mu_H^2 g_Y^2 Y_e^{*ab} C_{eB}^{ab} Y_d^{pr} + 2\mu_H^2 g_Y^2 C_{eB}^{*ab} Y_d^{pr} Y_e^{ab} - \frac{3}{2}\mu_H^2 g_L^2 Y_e^{*ab} C_{eW}^{ab} Y_d^{pr} + 3\mu_H^2 g_L^2 C_{eW}^{*ab} Y_d^{pr} Y_e^{ab} \right. \\
& - \frac{1}{4}\mu_H^2 g_Y^2 \left\{ 9\delta^{pa}(Y_u^\dagger Y_d)^{br} + 20Y_u^{*ab} Y_d^{pr} \right\} C_{uB}^{ab} + \frac{1}{12}\mu_H^2 g_Y^2 C_{uB}^{*ab} \left\{ 47Y_d^{ar} Y_u^{pb} - 60Y_d^{pr} Y_u^{ab} \right\} - \frac{3}{8}\mu_H^2 g_L^2 \left\{ 12Y_u^{*ab} Y_d^{pr} - 13\delta^{pa}(Y_u^\dagger Y_d)^{br} \right\} C_{uW}^{ab} \\
& + \frac{3}{8}\mu_H^2 g_L^2 C_{uW}^{*ab} \left\{ 35Y_d^{ar} Y_u^{pb} - 12Y_d^{pr} Y_u^{ab} \right\} - 4\mu_H^2 g_s^2 \left\{ 4Y_u^{*ab} Y_d^{pr} - 3\delta^{pa}(Y_u^\dagger Y_d)^{br} \right\} C_{uG}^{ab} - \frac{4}{3}\mu_H^2 g_s^2 C_{uG}^{*ab} \left\{ 12Y_d^{pr} Y_u^{ab} + 17Y_d^{ar} Y_u^{pb} \right\} \\
& + \mu_H^2 \left\{ g_Y^2 \left( \frac{1}{12} (12Y_d^{*ab} Y_d^{pr} + 98\delta^{rb}(Y_d Y_d^\dagger)^{pa} - 88\delta^{rb}(Y_u Y_u^\dagger)^{pa} - 257\delta^{pa}(Y_d^\dagger Y_d)^{br} \right) - 3\delta^{pa}\delta^{rb} \text{Tr}[Y_d^\dagger Y_d] - 9\delta^{pa}\delta^{rb} \text{Tr}[Y_e^\dagger Y_e] \right\} + 8\delta^{pa}\delta^{rb} g_Y^2 g_L^2 \\
& - \frac{32}{9}\delta^{pa}\delta^{rb} g_Y^2 g_s^2 - \frac{104}{27}\delta^{pa}\delta^{rb} g_Y^4 \left\{ C_{dB}^{ab} - \frac{1}{4}\mu_H^2 g_Y^2 C_{dB}^{*ab} \left\{ 7Y_d^{pb} Y_d^{ar} + 8Y_d^{pr} Y_d^{ab} \right\} + \mu_H^2 \left\{ g_L^2 \left( \frac{9}{2}\delta^{pa}\delta^{rb} \text{Tr}[Y_e^\dagger Y_e] + \frac{27}{2}\delta^{pa}\delta^{rb} \text{Tr}[Y_d^\dagger Y_d] \right. \right. \right. \\
& - \frac{9}{8} (4Y_d^{*ab} Y_d^{pr} - 3\delta^{pa}(Y_d^\dagger Y_d)^{br} - 14\delta^{rb}(Y_d Y_d^\dagger)^{pa} - 16\delta^{rb}(Y_u Y_u^\dagger)^{pa} \Big) \Big) + \frac{27}{2}\delta^{pa}\delta^{rb} g_L^4 + 16\delta^{pa}\delta^{rb} g_s^2 g_L^2 - \frac{8}{3}\delta^{pa}\delta^{rb} g_Y^2 g_L^2 \left. \right\} C_{dW}^{ab} \\
& + \frac{3}{8}\mu_H^2 g_L^2 C_{dW}^{*ab} \left\{ 5Y_d^{pb} Y_d^{ar} + 24Y_d^{pr} Y_d^{ab} \right\} + \mu_H^2 \left\{ \frac{224}{9}\delta^{pa}\delta^{rb} g_s^4 - \frac{4}{3}g_s^2 (12Y_d^{*ab} Y_d^{pr} - 4\delta^{rb}(Y_u Y_u^\dagger)^{pa} - 29\delta^{pa}(Y_d^\dagger Y_d)^{br} - 34\delta^{rb}(Y_d Y_d^\dagger)^{pa} \right. \\
& - \frac{136}{27}\delta^{pa}\delta^{rb} g_Y^2 g_s^2 - 8\delta^{pa}\delta^{rb} g_s^2 g_L^2 \left. \right\} C_{dG}^{ab} + 4\mu_H^2 g_s^2 C_{dG}^{*ab} \left\{ 3Y_d^{pb} Y_d^{ar} - 4Y_d^{pr} Y_d^{ab} \right\} + \mu_H^2 \left\{ \frac{4}{9}\delta^{ab} g_Y^2 Y_d^{pr} - \frac{10}{3}Y_d^{pr} (Y_e Y_e^\dagger)^{ba} \right\} C_{H\ell}^{(\parallel)ab} \\
& + \mu_H^2 \left\{ \frac{2}{9}\delta^{ab} g_Y^2 Y_d^{pr} - \frac{2}{3}\delta^{ab} g_L^2 Y_d^{pr} - \frac{20}{3}Y_d^{pr} (Y_e Y_e^\dagger)^{ba} \right\} C_{H\ell}^{(\times)ab} + \mu_H^2 \left\{ \frac{4}{9}\delta^{ab} g_Y^2 Y_d^{pr} + \frac{10}{3}Y_d^{pr} (Y_e^\dagger Y_e)^{ba} \right\} C_{He}^{ab} + \mu_H^2 \left\{ \frac{1}{2}(Y_d^{br} (Y_d Y_d^\dagger)^{pa} \right. \\
& + \delta^{pa}(Y_u Y_u^\dagger Y_d)^{br} + 20Y_d^{pr} (Y_u Y_u^\dagger)^{ba} - Y_d^{br} (Y_u Y_u^\dagger)^{pa} - 8T_2\delta^{pa} Y_d^{br} - 17\delta^{pa}(Y_d Y_d^\dagger Y_d)^{br} - 20Y_d^{pr} (Y_d Y_d^\dagger)^{ba} \Big) + \frac{21}{4}\delta^{pa} g_L^2 Y_d^{br} + \frac{16}{3}\delta^{pa} g_s^2 Y_d^{br} \\
& - \frac{1}{108}g_Y^2 (48\delta^{ab} Y_d^{pr} + 1097\delta^{pa} Y_d^{br}) \left. \right\} C_{Hq}^{(\parallel)ab} + \mu_H^2 \left\{ \frac{1}{12}g_L^2 (221\delta^{pa} Y_d^{br} - 24\delta^{ab} Y_d^{pr}) + \frac{1}{2}(Y_d^{br} (Y_u Y_u^\dagger)^{pa} + 2Y_d^{br} (Y_d Y_d^\dagger)^{pa} - \delta^{pa}(Y_u Y_u^\dagger Y_d)^{br} \right. \\
& - 10\delta^{pa}(Y_d Y_d^\dagger Y_d)^{br} - 16T_2\delta^{pa} Y_d^{br} - 20Y_d^{pr} (Y_u Y_u^\dagger)^{ba} - 40Y_d^{pr} (Y_d Y_d^\dagger)^{ba} \Big) + \frac{32}{3}\delta^{pa} g_s^2 Y_d^{br} - \frac{1}{108}g_Y^2 (24\delta^{ab} Y_d^{pr} + 679\delta^{pa} Y_d^{br}) \left. \right\} C_{Hq}^{(\times)ab} \\
& - \mu_H^2 \left\{ \frac{8}{9}\delta^{ab} g_Y^2 Y_d^{pr} + 10Y_d^{pr} (Y_u^\dagger Y_u)^{ba} \right\} C_{Hu}^{ab} + \mu_H^2 \left\{ \frac{1}{108}g_Y^2 (48\delta^{ab} Y_d^{pr} + 667\delta^{rb} Y_d^{pa}) + 4T_2\delta^{rb} Y_d^{pa} + 5\delta^{rb}(Y_d Y_d^\dagger Y_d)^{pa} + \frac{21}{4}\delta^{rb} g_L^2 Y_d^{pa} \right. \\
& + 10Y_d^{pr} (Y_d^\dagger Y_d)^{ba} - Y_d^{pa} (Y_d^\dagger Y_d)^{br} - 4\delta^{rb}(Y_u Y_u^\dagger Y_d)^{pa} - \frac{16}{3}\delta^{rb} g_s^2 Y_d^{pa} \left. \right\} C_{Hd}^{ab} + \mu_H^2 \left\{ 3\delta^{rb}(Y_u Y_u^\dagger Y_u)^{pa} + 4T_2\delta^{rb} Y_u^{pa} + \frac{21}{4}\delta^{rb} g_L^2 Y_u^{pa} \right.
\end{aligned}$$

$$\begin{aligned}
& + 10Y_d^{pr} (Y_d^\dagger Y_u)^{ba} - 2\delta^{rb} (Y_d Y_d^\dagger Y_u)^{pa} - \frac{187}{36} \delta^{rb} g_Y^2 Y_u^{pa} - \frac{16}{3} \delta^{rb} g_s^2 Y_u^{pa} \Big\} C_{Hud}^{ab} + \mu_H^2 C_{Hud}^{*ab} \Big\{ 10Y_d^{pr} (Y_u^\dagger Y_d)^{ab} - Y_d^{pb} (Y_u^\dagger Y_d)^{ar} \Big\} \\
& - 4\mu_H^2 Y_e^{*ad} C_{\ell e}^{abcd} Y_d^{pr} Y_e^{bc} + \mu_H^2 \Big\{ \delta^{rd} Y_d^{pc} (Y_e Y_e^\dagger)^{ba} - \frac{35}{27} \delta^{rd} \delta^{ab} g_Y^2 Y_d^{pc} \Big\} C_{\ell d}^{abcd} + \mu_H^2 \Big\{ \delta^{pa} Y_d^{br} (Y_e^\dagger Y_e)^{dc} + \frac{49}{27} \delta^{pa} \delta^{cd} g_Y^2 Y_d^{br} \Big\} C_{qe}^{abcd} \\
& + \mu_H^2 \Big\{ \frac{1}{2} \Big( 3Y_u^{*ad} Y_d^{br} Y_u^{pc} + 12\delta^{pa} Y_d^{br} (Y_u^\dagger Y_u)^{dc} - 2\delta^{pa} Y_u^{bc} (Y_u^\dagger Y_d)^{dr} - 24Y_u^{*ad} Y_d^{pr} Y_u^{bc} \Big) - \frac{98}{27} \delta^{pa} \delta^{cd} g_Y^2 Y_d^{br} \Big\} C_{qu}^{(\parallel)abcd} + \mu_H^2 \Big\{ \frac{1}{2} \Big( 4\delta^{pa} Y_d^{br} (Y_u^\dagger Y_u)^{dc} \\
& + 9Y_u^{*ad} Y_d^{br} Y_u^{pc} - 6\delta^{pa} Y_u^{bc} (Y_u^\dagger Y_d)^{dr} - 72Y_u^{*ad} Y_d^{pr} Y_u^{bc} \Big) + \frac{112}{27} \delta^{pa} \delta^{cd} g_s^2 Y_d^{br} - \frac{98}{81} \delta^{pa} \delta^{cd} g_Y^2 Y_d^{br} \Big\} C_{qu}^{(\times)abcd} + \mu_H^2 \Big\{ \frac{1}{54} g_Y^2 \Big( 70\delta^{rd} \delta^{ab} Y_d^{pc} + 98\delta^{pa} \delta^{cd} Y_d^{br} \\
& - 3\delta^{pa} \delta^{rd} Y_d^{bc} \Big) + \frac{1}{2} \Big( 2\delta^{pa} Y_d^{bc} (Y_d^\dagger Y_d)^{dr} + 4\delta^{rd} Y_d^{bc} (Y_d Y_d^\dagger)^{pa} + 6Y_d^{*ad} Y_d^{pc} Y_d^{br} + 9\delta^{pa} \delta^{rd} (Y_u Y_u^\dagger Y_d)^{bc} + 12\delta^{pa} Y_d^{br} (Y_d^\dagger Y_d)^{dc} + 12\delta^{rd} Y_d^{pc} (Y_d Y_d^\dagger)^{ba} \\
& + 12\delta^{rd} Y_d^{pc} (Y_u Y_u^\dagger)^{ba} + 48\delta^{pa} \delta^{rd} (Y_d Y_d^\dagger Y_d)^{bc} - 4\delta^{rd} Y_d^{bc} (Y_u Y_u^\dagger)^{pa} - 12Y_d^{*ad} Y_d^{pr} Y_d^{bc} \Big) + 6\delta^{pa} \delta^{rd} Y_d^{bc} \text{Tr}[Y_d^\dagger Y_d] - \frac{3}{2} \delta^{pa} \delta^{rd} g_L^2 Y_d^{bc} \\
& - \frac{32}{3} \delta^{pa} \delta^{rd} g_s^2 Y_d^{bc} \Big\} C_{qd}^{(\parallel)abcd} + \mu_H^2 \Big\{ \frac{1}{162} g_Y^2 \Big( 70\delta^{rd} \delta^{ab} Y_d^{pc} + 98\delta^{pa} \delta^{cd} Y_d^{br} - 27\delta^{pa} \delta^{rd} Y_d^{bc} \Big) + \frac{1}{2} \Big( 4\delta^{pa} Y_d^{br} (Y_d^\dagger Y_d)^{dc} + 4\delta^{rd} Y_d^{pc} (Y_d Y_d^\dagger)^{ba} \\
& + 4\delta^{rd} Y_d^{pc} (Y_u Y_u^\dagger)^{ba} + 6\delta^{pa} Y_d^{bc} (Y_d^\dagger Y_d)^{dr} + 12\delta^{rd} Y_d^{bc} (Y_d Y_d^\dagger)^{pa} + 18Y_d^{*ad} Y_d^{pc} Y_d^{br} + 27\delta^{pa} \delta^{rd} (Y_u Y_u^\dagger Y_d)^{bc} + 144\delta^{pa} \delta^{rd} (Y_d Y_d^\dagger Y_d)^{bc} \\
& - 12\delta^{rd} Y_d^{bc} (Y_u Y_u^\dagger)^{pa} - 36Y_d^{*ad} Y_d^{pr} Y_d^{bc} \Big) + 18\delta^{pa} \delta^{rd} Y_d^{bc} \text{Tr}[Y_d^\dagger Y_d] - \frac{16}{27} g_s^2 \Big( 216\delta^{pa} \delta^{rd} Y_d^{bc} - 7\delta^{pa} \delta^{cd} Y_d^{br} - 14\delta^{rd} \delta^{ab} Y_d^{pc} \Big) - \frac{9}{2} \delta^{pa} \delta^{rd} g_L^2 Y_d^{bc} \Big\} C_{qd}^{(\times)abcd} \\
& + \mu_H^2 \Big\{ \frac{32}{27} \delta^{rb} \delta^{ad} g_s^2 Y_d^{pc} + 24\delta^{rb} Y_d^{pa} (Y_d^\dagger Y_d)^{dc} - \frac{10}{81} g_Y^2 \Big( \delta^{rb} \delta^{ad} Y_d^{pc} + 21\delta^{rb} \delta^{cd} Y_d^{pa} \Big) \Big\} C_{dd}^{abcd} + \mu_H^2 \Big\{ 5\delta^{rd} Y_d^{pc} (Y_e^\dagger Y_e)^{ba} - \frac{35}{27} \delta^{rd} \delta^{ab} g_Y^2 Y_d^{pc} \Big\} C_{ed}^{abcd} \\
& + \mu_H^2 \Big\{ \frac{70}{27} \delta^{rd} \delta^{ab} g_Y^2 Y_d^{pc} - \frac{3}{2} \Big( \delta^{rd} Y_u^{pa} (Y_u^\dagger Y_d)^{bc} + 4\delta^{rd} Y_d^{pc} (Y_u^\dagger Y_u)^{ba} \Big) \Big\} C_{ud}^{(\parallel)abcd} + \mu_H^2 \Big\{ \frac{1}{2} \Big( -4\delta^{rd} Y_d^{pc} (Y_u^\dagger Y_u)^{ba} - 9\delta^{rd} Y_u^{pa} (Y_u^\dagger Y_d)^{bc} \Big) + \frac{70}{81} \delta^{rd} \delta^{ab} g_Y^2 Y_d^{pc} \\
& + \frac{112}{27} \delta^{rd} \delta^{ab} g_s^2 Y_d^{pc} \Big\} C_{ud}^{(\times)abcd} - \frac{3}{4} \mu_H^2 \Big\{ 3Y_e^{*ab} Y_d^{pc} Y_d^{dr} + 4Y_e^{*ab} Y_d^{pr} Y_d^{dc} \Big\} C_{\ell edq}^{abcd} + \mu_H^2 C_{\ell edq}^{*abcd} \Big\{ \frac{9}{2} \delta^{pd} \delta^{rc} g_Y^2 Y_e^{ab} - \frac{3}{4} \Big( \delta^{pd} Y_e^{ab} (Y_d^\dagger Y_d)^{cr} + 2\delta^{rc} Y_e^{ab} (Y_d Y_d^\dagger)^{pd} \\
& + 6\delta^{pd} \delta^{rc} (Y_e Y_e^\dagger Y_e)^{ab} - 2\delta^{rc} Y_e^{ab} (Y_u Y_u^\dagger)^{pd} \Big) - \frac{3}{2} \delta^{pd} \delta^{rc} g_L^2 Y_e^{ab} - 3\delta^{pd} \delta^{rc} Y_e^{ab} \text{Tr}[Y_d^\dagger Y_d] \Big\} + \mu_H^2 \Big\{ \frac{1}{24} g_Y^2 \Big( 13\delta^{pa} \delta^{rd} Y_u^{*cb} + 98\delta^{pc} \delta^{rd} Y_u^{*ab} \Big) \\
& + 4g_s^2 \Big( 3\delta^{pa} \delta^{rd} Y_u^{*cb} + 10\delta^{pc} \delta^{rd} Y_u^{*ab} \Big) - \frac{3}{8} g_L^2 \Big( \delta^{pa} \delta^{rd} Y_u^{*cb} - 6\delta^{pc} \delta^{rd} Y_u^{*ab} \Big) - \frac{3}{8} \Big( \delta^{pa} Y_u^{*cb} (Y_d^\dagger Y_d)^{dr} + 2\delta^{rd} Y_u^{*cb} (Y_d Y_d^\dagger)^{pa} + 2\delta^{pa} \delta^{rd} (Y_d^\dagger Y_d Y_u^\dagger)^{cb} \\
& + 6\delta^{pc} Y_u^{*ab} (Y_d^\dagger Y_d)^{dr} + 6\delta^{pa} \delta^{rd} (Y_u^\dagger Y_u Y_u^\dagger)^{cb} + 12\delta^{rd} Y_u^{*ab} (Y_d Y_d^\dagger)^{pc} + 20\delta^{pc} \delta^{rd} (Y_d^\dagger Y_d Y_u^\dagger)^{ab} + 36\delta^{pc} \delta^{rd} (Y_u^\dagger Y_u Y_u^\dagger)^{ab} - \delta^{pc} Y_d^{*ad} (Y_u^\dagger Y_d)^{br}
\end{aligned}$$

$$\begin{aligned}
& -2\delta^{rd}Y_u^{*cb}(Y_uY_u^\dagger)^{pa} - 6\delta^{pa}Y_d^{*cd}(Y_u^\dagger Y_d)^{br} - 12\delta^{rd}Y_u^{*ab}(Y_uY_u^\dagger)^{pc} \Big) - \frac{3}{2} \Big( \delta^{pa}\delta^{rd}Y_u^{*cb} + 6\delta^{pc}\delta^{rd}Y_u^{*ab} \Big) \text{Tr}[Y_d^\dagger Y_d] \Big\} C_{quqd}^{(\parallel)abcd} + \frac{1}{8}\mu_H^2 \Big( C_{quqd}^{(\parallel)*} \Big)^{abcd} \Big\{ 5Y_d^{ad}Y_d^{cr}Y_u^{pb} \\
& + 6Y_d^{ar}Y_d^{cd}Y_u^{pb} - 9Y_d^{pd}Y_d^{ar}Y_u^{cb} - 12Y_d^{pr}Y_d^{ad}Y_u^{cb} - 54Y_d^{pd}Y_d^{cr}Y_u^{ab} - 72Y_d^{pr}Y_d^{cd}Y_u^{ab} \Big\} + \mu_H^2 \Big\{ \frac{1}{72}g_Y^2 \Big( 98\delta^{pc}\delta^{rd}Y_u^{*ab} + 117\delta^{pa}\delta^{rd}Y_u^{*cb} \Big) \\
& + \frac{1}{8} \Big( 6\delta^{pa}Y_d^{*cd}(Y_u^\dagger Y_d)^{br} + 9\delta^{pc}Y_d^{*ad}(Y_u^\dagger Y_d)^{br} + 12\delta^{rd}Y_u^{*ab}(Y_uY_u^\dagger)^{pc} + 18\delta^{rd}Y_u^{*cb}(Y_uY_u^\dagger)^{pa} - 6\delta^{pc}Y_u^{*ab}(Y_d^\dagger Y_d)^{dr} - 9\delta^{pa}Y_u^{*cb}(Y_d^\dagger Y_d)^{dr} - 12\delta^{rd}Y_u^{*ab}(Y_dY_d^\dagger)^{pc} \\
& - 18\delta^{rd}Y_u^{*cb}(Y_dY_d^\dagger)^{pa} - 18\delta^{pa}\delta^{rd}(Y_d^\dagger Y_dY_u^\dagger)^{cb} - 20\delta^{pc}\delta^{rd}(Y_d^\dagger Y_dY_u^\dagger)^{ab} - 36\delta^{pc}\delta^{rd}(Y_u^\dagger Y_uY_u^\dagger)^{ab} - 54\delta^{pa}\delta^{rd}(Y_u^\dagger Y_uY_u^\dagger)^{cb} \Big) + \frac{8}{3}g_s^2 \Big( 5\delta^{pc}\delta^{rd}Y_u^{*ab} \\
& + 18\delta^{pa}\delta^{rd}Y_u^{*cb} \Big) - \frac{3}{8}g_L^2 \Big( 3\delta^{pa}\delta^{rd}Y_u^{*cb} - 2\delta^{pc}\delta^{rd}Y_u^{*ab} \Big) - \frac{3}{2} \Big( 2\delta^{pc}\delta^{rd}Y_u^{*ab} + 3\delta^{pa}\delta^{rd}Y_u^{*cb} \Big) \text{Tr}[Y_d^\dagger Y_d] \Big\} C_{quqd}^{(\times)abcd} + \frac{1}{8}\mu_H^2 \Big( C_{quqd}^{(\times)*} \Big)^{abcd} \Big\{ 2Y_d^{ar}Y_d^{cd}Y_u^{pb} \\
& + 15Y_d^{ad}Y_d^{cr}Y_u^{pb} - 18Y_d^{pd}Y_d^{cr}Y_u^{ab} - 24Y_d^{pr}Y_d^{cd}Y_u^{ab} - 27Y_d^{pd}Y_d^{ar}Y_u^{cb} - 36Y_d^{pr}Y_d^{ad}Y_u^{cb} \Big\} - \frac{3}{4}\delta^{pc}\mu_H^2 Y_e^{*ab} C_{lequ}^{abcd} (Y_u^\dagger Y_d)^{dr} + \frac{3}{4}\mu_H^2 C_{lequ}^{*abcd} Y_d^{cr}Y_e^{ab}Y_u^{pd} \\
& + \frac{3}{8}\delta^{pc}\mu_H^2 Y_e^{*ad} C_{luqe}^{abcd} (Y_u^\dagger Y_d)^{br} + \frac{1}{8}\mu_H^2 C_{luqe}^{*abcd} Y_d^{cr}Y_e^{ad}Y_u^{pb} + \mu_H^2 \Big\{ \frac{32}{27}\delta^{pa}\delta^{bc}g_s^2 Y_d^{dr} + 3 \Big( 8\delta^{pa}Y_d^{br}(Y_dY_d^\dagger)^{dc} - \delta^{pa}Y_d^{dr}(Y_uY_u^\dagger)^{bc} - 4\delta^{pa}Y_d^{br}(Y_uY_u^\dagger)^{dc} \Big) \\
& - \frac{7}{81}g_Y^2 \Big( \delta^{pa}\delta^{bc}Y_d^{dr} + 42\delta^{pa}\delta^{cd}Y_d^{br} \Big) - \frac{1}{3}\delta^{pa}\delta^{bc}g_L^2 Y_d^{dr} \Big\} C_{qq}^{(\parallel)abcd} + \mu_H^2 \Big\{ \frac{64}{27}\delta^{pa}\delta^{bc}g_s^2 Y_d^{dr} + 3 \Big( \delta^{pa}Y_d^{dr}(Y_uY_u^\dagger)^{bc} + 4\delta^{pa}Y_d^{br}(Y_uY_u^\dagger)^{dc} \\
& + 16\delta^{pa}Y_d^{br}(Y_dY_d^\dagger)^{dc} \Big) - \frac{7}{81}g_Y^2 \Big( 2\delta^{pa}\delta^{bc}Y_d^{dr} + 21\delta^{pa}\delta^{cd}Y_d^{br} \Big) - 7\delta^{pa}\delta^{cd}g_L^2 Y_d^{br} \Big\} C_{qq}^{(\times)abcd} + \mu_H^2 \Big\{ \frac{49}{27}\delta^{pc}\delta^{ab}g_Y^2 Y_d^{dr} + 5\delta^{pc}Y_d^{dr}(Y_eY_e^\dagger)^{ba} \Big\} C_{lq}^{(\parallel)abcd} \\
& + \mu_H^2 \Big\{ \frac{49}{54}\delta^{pc}\delta^{ab}g_Y^2 Y_d^{dr} + 10\delta^{pc}Y_d^{dr}(Y_eY_e^\dagger)^{ba} - \frac{7}{6}\delta^{pc}\delta^{ab}g_L^2 Y_d^{dr} \Big\} C_{lq}^{(\times)abcd}, \tag{2.10}
\end{aligned}$$

## 2.6 $U(1)_Y$ gauge coupling

$$\beta_{g_Y^2}^{(1)} = \frac{41}{3}g_Y^4 - 16\mu_H^2 g_Y^4 C_{HB}, \tag{2.11}$$

$$\begin{aligned}
\beta_{g_Y^2}^{(2)} = & \Big\{ 9g_Y^4 g_L^2 + \frac{199}{9}g_Y^6 + \frac{88}{3}g_Y^4 g_s^2 - g_Y^4 \Big( \frac{5}{3} \text{Tr}[Y_d^\dagger Y_d] + 5 \text{Tr}[Y_e^\dagger Y_e] + \frac{17}{3} \text{Tr}[Y_u^\dagger Y_u] \Big) \Big\} + \mu_H^2 \Big\{ 32T_2 g_Y^4 - 24g_Y^6 - 96g_Y^4 g_L^2 \Big\} C_{HB} \\
& + 6\mu_H^2 g_Y^4 g_L^2 C_{HWB} + 12\mu_H^2 g_Y^4 Y_e^{*ab} C_{eB}^{ab} + 12\mu_H^2 g_Y^4 C_{eB}^{*ab} Y_e^{ab} - 20\mu_H^2 g_Y^4 Y_u^{*ab} C_{uB}^{ab} - 20\mu_H^2 g_Y^4 C_{uB}^{*ab} Y_u^{ab} + 4\mu_H^2 g_Y^4 Y_d^{*ab} C_{dB}^{ab} \\
& + 4\mu_H^2 g_Y^4 C_{dB}^{*ab} Y_d^{ab}, \tag{2.12}
\end{aligned}$$

## 2.7 $SU(2)_L$ gauge coupling

$$\beta_{g_L^2}^{(1)} = -\frac{19}{3}g_L^4 - 16\mu_H^2 g_L^4 C_{HW}, \quad (2.13)$$

$$\begin{aligned} \beta_{g_L^2}^{(2)} = & \left\{ 3g_Y^2 g_L^4 + \frac{35}{3}g_L^6 + 24g_s^2 g_L^4 - T_2 g_L^4 \right\} + \mu_H^2 \left\{ 32T_2 g_L^4 - 32g_Y^2 g_L^4 - 88g_L^6 \right\} C_{HW} + 2\mu_H^2 g_Y^2 g_L^4 C_{HWB} - 228\mu_H^2 g_L^8 C_W \\ & - 2\mu_H^2 g_L^4 Y_e^{*ab} C_{eW}^{ab} - 2\mu_H^2 g_L^4 C_{eW}^{*ab} Y_e^{ab} - 6\mu_H^2 g_L^4 Y_u^{*ab} C_{uW}^{ab} - 6\mu_H^2 g_L^4 C_{uW}^{*ab} Y_u^{ab} - 6\mu_H^2 g_L^4 Y_d^{*ab} C_{dW}^{ab} - 6\mu_H^2 g_L^4 C_{dW}^{*ab} Y_d^{ab}, \end{aligned} \quad (2.14)$$

## 2.8 $SU(3)_c$ gauge coupling

$$\beta_{g_s^2}^{(1)} = -14g_s^4 - 16\mu_H^2 g_s^4 C_{HG}, \quad (2.15)$$

$$\begin{aligned} \beta_{g_s^2}^{(2)} = & \left\{ \frac{11}{3}g_Y^2 g_s^4 + 9g_s^4 g_L^2 - g_s^4 \left( 4 \text{Tr} [Y_d^\dagger Y_d] + 4 \text{Tr} [Y_u^\dagger Y_u] \right) - 52g_s^6 \right\} + \mu_H^2 \left\{ 32T_2 g_s^4 - 32g_Y^2 g_s^4 - 96g_s^4 g_L^2 \right\} C_{HG} - 8\mu_H^2 g_s^4 Y_u^{*ab} C_{uG}^{ab} \\ & - 8\mu_H^2 g_s^4 C_{uG}^{*ab} Y_u^{ab} - 8\mu_H^2 g_s^4 Y_d^{*ab} C_{dG}^{ab} - 8\mu_H^2 g_s^4 C_{dG}^{*ab} Y_d^{ab}, \end{aligned} \quad (2.16)$$

## 2.9 $\theta_B$ coupling

$$\beta_{\theta_B}^{(1)} = -8\mu_H^2 C_{H\tilde{B}}, \quad (2.17)$$

$$\begin{aligned} \beta_{\theta_B}^{(2)} = & \mu_H^2 \left\{ 16T_2 - 12g_Y^2 - 48g_L^2 \right\} C_{H\tilde{B}} + 3\mu_H^2 g_L^2 C_{H\tilde{W}B} + 6i\mu_H^2 Y_e^{*ab} C_{eB}^{ab} - 6i\mu_H^2 C_{eB}^{*ab} Y_e^{ab} - 10i\mu_H^2 Y_u^{*ab} C_{uB}^{ab} + 10i\mu_H^2 C_{uB}^{*ab} Y_u^{ab} \\ & + 2i\mu_H^2 Y_d^{*ab} C_{dB}^{ab} - 2i\mu_H^2 C_{dB}^{*ab} Y_d^{ab}, \end{aligned} \quad (2.18)$$

## 2.10 $\theta_W$ coupling

$$\beta_{\theta_W}^{(1)} = -8\mu_H^2 C_{H\tilde{W}}, \quad (2.19)$$

$$\begin{aligned} \beta_{\theta_W}^{(2)} = & \mu_H^2 \left\{ 16T_2 - 16g_Y^2 - 44g_L^2 \right\} C_{H\tilde{W}} + \mu_H^2 g_Y^2 C_{H\tilde{W}B} - 74\mu_H^2 g_L^4 C_{\tilde{W}} - i\mu_H^2 Y_e^{*ab} C_{eW}^{ab} + 1i\mu_H^2 C_{eW}^{*ab} Y_e^{ab} - 3i\mu_H^2 Y_u^{*ab} C_{uW}^{ab} \\ & + 3i\mu_H^2 C_{uW}^{*ab} Y_u^{ab} - 3i\mu_H^2 Y_d^{*ab} C_{dW}^{ab} + 3i\mu_H^2 C_{dW}^{*ab} Y_d^{ab}, \end{aligned} \quad (2.20)$$

### 2.11 $\theta_G$ coupling

$$\beta_{\theta_G}^{(1)} = -8\mu_H^2 C_{H\tilde{G}}, \quad (2.21)$$

$$\beta_{\theta_G}^{(2)} = \mu_H^2 \left\{ 16T_2 - 16g_Y^2 - 48g_L^2 \right\} C_{H\tilde{G}} - 4i\mu_H^2 Y_u^{*ab} C_{uG}^{ab} + 4i\mu_H^2 C_{uG}^{*ab} Y_u^{ab} - 4i\mu_H^2 Y_d^{*ab} C_{dG}^{ab} + 4i\mu_H^2 C_{dG}^{*ab} Y_d^{ab}, \quad (2.22)$$

## 3 Weinberg operator

$$\beta_{C_{\ell HH}^{pr}}^{(1)} = \frac{1}{2} \left( 4T_2 C_{\ell HH}^{pr} - 3[C_{\ell HH} Y_e Y_e^\dagger + (C_{\ell HH} Y_e Y_e^\dagger)^\Gamma]^{pr} \right) + 2\lambda C_{\ell HH}^{pr} - 3g_L^2 C_{\ell HH}^{pr}, \quad (3.1)$$

$$\begin{aligned} \beta_{C_{\ell HH}^{pr}}^{(2)} &= \frac{3}{16} g_L^2 \left( 11[C_{\ell HH} Y_e Y_e^\dagger + (C_{\ell HH} Y_e Y_e^\dagger)^\Gamma]^{pr} + 20T_2 C_{\ell HH}^{pr} \right) + \frac{1}{4} \left( 5T_2 [C_{\ell HH} Y_e Y_e^\dagger + (C_{\ell HH} Y_e Y_e^\dagger)^\Gamma]^{pr} + 8(Y_e^\dagger Y_e C_{\ell HH} Y_e Y_e^\dagger)^{pr} \right. \\ &\quad \left. + 19[C_{\ell HH} Y_e Y_e^\dagger Y_e Y_e^\dagger + (C_{\ell HH} Y_e Y_e^\dagger Y_e Y_e^\dagger)^\Gamma]^{pr} - 2T_4 C_{\ell HH}^{pr} \right) + g_s^2 \left( 40C_{\ell HH}^{pr} \text{Tr}[Y_d^\dagger Y_d] + 40C_{\ell HH}^{pr} \text{Tr}[Y_u^\dagger Y_u] \right) \\ &\quad + g_Y^2 \left( \frac{25}{12} C_{\ell HH}^{pr} \text{Tr}[Y_d^\dagger Y_d] + \frac{25}{4} C_{\ell HH}^{pr} \text{Tr}[Y_e^\dagger Y_e] + \frac{85}{12} C_{\ell HH}^{pr} \text{Tr}[Y_u^\dagger Y_u] - \frac{57}{16} [C_{\ell HH} Y_e Y_e^\dagger + (C_{\ell HH} Y_e Y_e^\dagger)^\Gamma]^{pr} \right) + 3C_{\ell HH}^{pr} \text{Tr}[Y_d^\dagger Y_d Y_u^\dagger Y_u] \\ &\quad - \lambda \left( 2g_Y^2 C_{\ell HH}^{pr} + 4T_2 C_{\ell HH}^{pr} \right) - 7\lambda^2 C_{\ell HH}^{pr} - \frac{169}{24} g_L^4 C_{\ell HH}^{pr} - \frac{129}{8} g_Y^4 C_{\ell HH}^{pr} - \frac{83}{4} g_Y^2 g_L^2 C_{\ell HH}^{pr}, \end{aligned} \quad (3.2)$$

## 4 $H^6$ and $H^4 D^2$

### 4.1 $C_H$

$$\begin{aligned} \beta_{C_H}^{(1)} &= \left\{ 6T_2 + 54\lambda - \frac{9}{2}g_Y^2 - \frac{27}{2}g_L^2 \right\} C_H + \left\{ \lambda \left( \frac{17}{6}g_L^2 - \frac{1}{6}g_Y^2 \right) + 10\lambda^2 - \frac{3}{4}g_Y^4 - \frac{3}{2}g_Y^2 g_L^2 - \frac{9}{4}g_L^4 \right\} C_{HD}^{(\parallel)} + \left\{ 12\lambda^2 - \frac{3}{4}g_L^4 - \frac{3}{4}g_Y^4 \right. \\ &\quad \left. - \lambda \left( \frac{1}{3}g_Y^2 + 3g_L^2 \right) - \frac{3}{2}g_Y^2 g_L^2 \right\} C_{HD}^{(\times)} + \left\{ 6\lambda g_Y^4 - 3g_Y^4 g_L^2 - 3g_Y^6 \right\} C_{HB} + \left\{ 18\lambda g_L^4 - 3g_Y^2 g_L^4 - 9g_L^6 \right\} C_{HW} + \left\{ 3\lambda g_Y^2 g_L^2 - \frac{3}{2}g_Y^2 g_L^4 \right. \\ &\quad \left. - \frac{3}{2}g_Y^4 g_L^2 \right\} C_{HWB} + \left\{ 2\lambda Y_e^{*ab} - 4(Y_e^\dagger Y_e Y_e^\dagger)^{ab} \right\} C_{eH}^{ab} + C_{eH}^{*ab} \left\{ 2\lambda Y_e^{ab} - 4(Y_e Y_e^\dagger Y_e)^{ab} \right\} + \left\{ 6\lambda Y_u^{*ab} - 12(Y_u^\dagger Y_u Y_u^\dagger)^{ab} \right\} C_{uH}^{ab} \\ &\quad + C_{uH}^{*ab} \left\{ 6\lambda Y_u^{ab} - 12(Y_u Y_u^\dagger Y_u)^{ab} \right\} + \left\{ 6\lambda Y_d^{*ab} - 12(Y_d^\dagger Y_d Y_d^\dagger)^{ab} \right\} C_{dH}^{ab} + C_{dH}^{*ab} \left\{ 6\lambda Y_d^{ab} - 12(Y_d Y_d^\dagger Y_d)^{ab} \right\} + \lambda \left\{ \frac{4}{3}\delta^{ab} g_Y^2 \right. \end{aligned}$$

$$\begin{aligned}
& + 4(Y_e Y_e^\dagger)^{ba} \Big\} C_{H\ell}^{(\parallel)ab} + \lambda \Big\{ \frac{2}{3} \delta^{ab} g_Y^2 + 4(Y_e Y_e^\dagger)^{ba} - \frac{2}{3} \delta^{ab} g_L^2 \Big\} C_{H\ell}^{(\times)ab} + \lambda \Big\{ \frac{4}{3} \delta^{ab} g_Y^2 - 4(Y_e^\dagger Y_e)^{ba} \Big\} C_{He}^{ab} + \lambda \Big\{ 12((Y_d Y_d^\dagger)^{ba} - (Y_u Y_u^\dagger)^{ba}) \\
& - \frac{4}{3} \delta^{ab} g_Y^2 \Big\} C_{Hq}^{(\parallel)ab} + \lambda \Big\{ 12(Y_d Y_d^\dagger)^{ba} - \frac{2}{3} \delta^{ab} g_Y^2 - 2\delta^{ab} g_L^2 \Big\} C_{Hq}^{(\times)ab} + \lambda \Big\{ 12(Y_u^\dagger Y_u)^{ba} - \frac{8}{3} \delta^{ab} g_Y^2 \Big\} C_{Hu}^{ab} + \lambda \Big\{ \frac{4}{3} \delta^{ab} g_Y^2 - 12(Y_d^\dagger Y_d)^{ba} \Big\} C_{Hd}^{ab}, \tag{4.1}
\end{aligned}$$

$$\begin{aligned}
\beta_{CH}^{(2)} = & \lambda \Big( \frac{11}{3} g_L^2 \mathbf{T}_{\ell H} + \frac{19}{3} g_Y^2 \mathbf{T}_{\ell H} + 20 \text{Tr} \Big[ C_{\ell HH}^\dagger C_{\ell HH} Y_e Y_e^\dagger \Big] \Big) + 8 \text{Tr} \Big[ C_{\ell HH}^\dagger C_{\ell HH} Y_e Y_e^\dagger Y_e Y_e^\dagger \Big] + 44 \lambda^2 \mathbf{T}_{\ell H} - 2g_L^4 \mathbf{T}_{\ell H} - 4g_Y^4 \mathbf{T}_{\ell H} \\
& - 8g_Y^2 g_L^2 \mathbf{T}_{\ell H} + \Big\{ \lambda \Big( 72g_Y^2 + 216g_L^2 - 108\mathbf{T}_2 \Big) + g_Y^2 \Big( \frac{25}{4} \text{Tr} \Big[ Y_d^\dagger Y_d \Big] + \frac{75}{4} \text{Tr} \Big[ Y_e^\dagger Y_e \Big] + \frac{85}{4} \text{Tr} \Big[ Y_u^\dagger Y_u \Big] \Big) + g_s^2 \Big( 120 \text{Tr} \Big[ Y_d^\dagger Y_d \Big] + 120 \text{Tr} \Big[ Y_u^\dagger Y_u \Big] \Big) \\
& + \frac{21}{2} \mathbf{T}_4 + \frac{45}{4} \mathbf{T}_2 g_L^2 + \frac{189}{8} g_Y^2 g_L^2 + \frac{701}{16} g_Y^4 - \frac{3}{16} g_L^4 - 63 \text{Tr} \Big[ Y_d^\dagger Y_d Y_u^\dagger Y_u \Big] - 861 \lambda^2 \Big\} C_H + \Big\{ \frac{3}{4} \mathbf{T}_2 g_L^4 + \lambda^2 \Big( 13g_Y^2 + \frac{49}{3} g_L^2 \\
& - 26\mathbf{T}_2 \Big) + g_Y^4 \Big( \frac{19}{4} \text{Tr} \Big[ Y_u^\dagger Y_u \Big] + \frac{25}{4} \text{Tr} \Big[ Y_e^\dagger Y_e \Big] - \frac{5}{4} \text{Tr} \Big[ Y_d^\dagger Y_d \Big] \Big) + \lambda \Big( \frac{1}{6} \mathbf{T}_2 g_Y^2 + \frac{3}{2} \mathbf{T}_4 - \frac{17}{6} \mathbf{T}_2 g_L^2 - 3 \text{Tr} \Big[ Y_d^\dagger Y_d Y_u^\dagger Y_u \Big] - \frac{2219}{216} g_Y^4 \\
& - \frac{1441}{108} g_Y^2 g_L^2 - \frac{619}{24} g_L^4 \Big) + 10\mathbf{T}_6 + \frac{431}{24} g_Y^6 + \frac{445}{24} g_Y^2 g_L^4 + \frac{715}{24} g_Y^4 g_L^2 - g_Y^2 g_L^2 \Big( \frac{9}{2} \text{Tr} \Big[ Y_d^\dagger Y_d \Big] + \frac{11}{2} \text{Tr} \Big[ Y_e^\dagger Y_e \Big] + \frac{21}{2} \text{Tr} \Big[ Y_u^\dagger Y_u \Big] \Big) \\
& - 6 \text{Tr} \Big[ Y_d^\dagger Y_d Y_u^\dagger Y_u Y_d^\dagger Y_d \Big] - 6 \text{Tr} \Big[ Y_d^\dagger Y_d Y_u^\dagger Y_u Y_u^\dagger Y_u \Big] - \frac{253}{8} g_L^6 - 234 \lambda^3 \Big\} C_{HD}^{(\parallel)} + \Big\{ \frac{1}{4} \mathbf{T}_2 g_L^4 + \lambda^2 \Big( \frac{71}{6} g_Y^2 + \frac{123}{2} g_L^2 - 30\mathbf{T}_2 \Big) \\
& + g_Y^4 \Big( \frac{19}{4} \text{Tr} \Big[ Y_u^\dagger Y_u \Big] + \frac{25}{4} \text{Tr} \Big[ Y_e^\dagger Y_e \Big] - \frac{5}{4} \text{Tr} \Big[ Y_d^\dagger Y_d \Big] \Big) + \lambda \Big( \frac{1}{3} \mathbf{T}_2 g_Y^2 + 3\mathbf{T}_2 g_L^2 + \frac{9}{2} \mathbf{T}_4 + \frac{385}{48} g_L^4 - \frac{4907}{432} g_Y^4 - \frac{5725}{216} g_Y^2 g_L^2 \\
& - 27 \text{Tr} \Big[ Y_d^\dagger Y_d Y_u^\dagger Y_u \Big] \Big) + 8\mathbf{T}_6 + \frac{73}{4} g_Y^6 + 22g_Y^2 g_L^4 + \frac{767}{24} g_Y^4 g_L^2 - g_Y^2 g_L^2 \Big( \frac{9}{2} \text{Tr} \Big[ Y_d^\dagger Y_d \Big] + \frac{11}{2} \text{Tr} \Big[ Y_e^\dagger Y_e \Big] + \frac{21}{2} \text{Tr} \Big[ Y_u^\dagger Y_u \Big] \Big) - \frac{305}{24} g_L^6 \\
& - 249 \lambda^3 \Big\} C_{HD}^{(\times)} + \Big\{ \lambda \Big( g_Y^4 \Big( \frac{53}{3} \text{Tr} \Big[ Y_d^\dagger Y_d \Big] - \frac{79}{3} \text{Tr} \Big[ Y_u^\dagger Y_u \Big] - 43 \text{Tr} \Big[ Y_e^\dagger Y_e \Big] \Big) - \frac{559}{6} g_Y^4 g_L^2 - \frac{1447}{6} g_Y^6 \Big) + g_Y^6 \Big( 38 \text{Tr} \Big[ Y_u^\dagger Y_u \Big] + 50 \text{Tr} \Big[ Y_e^\dagger Y_e \Big] \\
& - 10 \text{Tr} \Big[ Y_d^\dagger Y_d \Big] \Big) + g_Y^4 \Big( \frac{32}{3} \text{Tr} \Big[ Y_u^\dagger Y_u Y_u^\dagger Y_u \Big] + 16 \text{Tr} \Big[ Y_e^\dagger Y_e Y_e^\dagger Y_e \Big] - \frac{16}{3} \text{Tr} \Big[ Y_d^\dagger Y_d Y_d^\dagger Y_d \Big] \Big) + 28 \lambda^2 g_Y^4 + \frac{385}{12} g_Y^4 g_L^4 + \frac{411}{4} g_Y^8 + \frac{655}{6} g_Y^6 g_L^2 \\
& - g_Y^4 g_L^2 \Big( 18 \text{Tr} \Big[ Y_d^\dagger Y_d \Big] + 22 \text{Tr} \Big[ Y_e^\dagger Y_e \Big] + 42 \text{Tr} \Big[ Y_u^\dagger Y_u \Big] \Big) \Big\} C_{HB} + \Big\{ \lambda \Big( 3\mathbf{T}_2 g_L^4 - \frac{475}{6} g_L^6 - \frac{197}{2} g_Y^2 g_L^4 \Big) + 6\mathbf{T}_2 g_L^6 + 36 \lambda^2 g_L^4 \\
& + \frac{655}{12} g_Y^4 g_L^4 + \frac{385}{6} g_Y^2 g_L^6 - g_Y^2 g_L^4 \Big( 18 \text{Tr} \Big[ Y_d^\dagger Y_d \Big] + 22 \text{Tr} \Big[ Y_e^\dagger Y_e \Big] + 42 \text{Tr} \Big[ Y_u^\dagger Y_u \Big] \Big) - \frac{819}{4} g_L^8 \Big\} C_{HW} + \Big\{ g_s^4 \Big( 128 \text{Tr} \Big[ Y_d^\dagger Y_d Y_d^\dagger Y_d \Big] \\
& + 128 \text{Tr} \Big[ Y_u^\dagger Y_u Y_u^\dagger Y_u \Big] \Big) - \lambda g_s^4 \Big( 352 \text{Tr} \Big[ Y_d^\dagger Y_d \Big] + 352 \text{Tr} \Big[ Y_u^\dagger Y_u \Big] \Big) \Big\} C_{HG} + \Big\{ g_Y^4 g_L^2 \Big( 7 \text{Tr} \Big[ Y_e^\dagger Y_e \Big] - \text{Tr} \Big[ Y_u^\dagger Y_u \Big] - 7 \text{Tr} \Big[ Y_d^\dagger Y_d \Big] \Big)
\end{aligned}$$

$$\begin{aligned}
& + \lambda \left( g_Y^2 g_L^2 \left( \frac{23}{2} \text{Tr}[Y_e^\dagger Y_e] + \frac{25}{2} \text{Tr}[Y_d^\dagger Y_d] + \frac{47}{2} \text{Tr}[Y_u^\dagger Y_u] \right) - 48 g_Y^2 g_L^4 - \frac{545}{6} g_Y^4 g_L^2 \right) + 20 \lambda^2 g_Y^2 g_L^2 + \frac{959}{24} g_Y^6 g_L^2 + \frac{589}{12} g_Y^4 g_L^4 \\
& - g_Y^2 g_L^4 \left( 3 \text{Tr}[Y_d^\dagger Y_d] + 5 \text{Tr}[Y_e^\dagger Y_e] + 9 \text{Tr}[Y_u^\dagger Y_u] \right) - g_Y^2 g_L^2 \left( 4 \text{Tr}[Y_d^\dagger Y_d Y_d^\dagger Y_d] + 4 \text{Tr}[Y_e^\dagger Y_e Y_e^\dagger Y_e] + 8 \text{Tr}[Y_u^\dagger Y_u Y_u^\dagger Y_u] \right) - \frac{25}{24} g_Y^2 g_L^6 \Big\} C_{HWB} \\
& + \left\{ \lambda \left( 6 T_2 g_L^6 + \frac{13}{2} g_Y^2 g_L^6 - \frac{221}{6} g_L^8 \right) + 6 g_Y^2 g_L^8 + 63 g_L^{10} - 6 g_Y^4 g_L^6 - 33 \lambda^2 g_L^6 \right\} C_W + \left\{ \lambda \left( (Y_e^\dagger Y_e Y_e^\dagger)^{ab} + \frac{13}{4} g_Y^2 Y_e^{*ab} - \frac{9}{4} g_L^2 Y_e^{*ab} \right) \right. \\
& + \frac{11}{2} g_Y^2 g_L^2 Y_e^{*ab} + 46 (Y_e^\dagger Y_e Y_e^\dagger Y_e Y_e^\dagger)^{ba} - \frac{3}{4} g_L^4 Y_e^{*ab} - \frac{25}{4} g_Y^4 Y_e^{*ab} - 8 g_Y^2 (Y_e^\dagger Y_e Y_e^\dagger)^{ab} - 20 \lambda^2 Y_e^{*ab} \Big\} C_{eH}^{ab} + C_{eH}^{*ab} \left\{ \lambda \left( (Y_e Y_e^\dagger Y_e)^{ab} \right. \right. \\
& + \frac{13}{4} g_Y^2 Y_e^{ab} - \frac{9}{4} g_L^2 Y_e^{ab} \Big) + \frac{11}{2} g_Y^2 g_L^2 Y_e^{ab} + 46 (Y_e Y_e^\dagger Y_e Y_e^\dagger Y_e)^{ab} - \frac{3}{4} g_L^4 Y_e^{ab} - \frac{25}{4} g_Y^4 Y_e^{ab} - 8 g_Y^2 (Y_e Y_e^\dagger Y_e)^{ab} - 20 \lambda^2 Y_e^{ab} \Big\} + \left\{ \lambda \left( 3 (Y_u^\dagger Y_u Y_u^\dagger)^{ab} \right. \right. \\
& + 40 g_s^2 Y_u^{*ab} - \frac{23}{12} g_Y^2 Y_u^{*ab} - \frac{27}{4} g_L^2 Y_u^{*ab} - 12 (Y_d^\dagger Y_d Y_u^\dagger)^{ab} \Big) + \frac{21}{2} g_Y^2 g_L^2 Y_u^{*ab} + 138 (Y_u^\dagger Y_u Y_u^\dagger Y_u Y_u^\dagger)^{ba} - \frac{9}{4} g_L^4 Y_u^{*ab} - \frac{19}{4} g_Y^4 Y_u^{*ab} \\
& - \frac{16}{3} g_Y^2 (Y_u^\dagger Y_u Y_u^\dagger)^{ab} - 6 (Y_u^\dagger Y_d Y_d^\dagger Y_d Y_u^\dagger)^{ba} - 6 (Y_u^\dagger Y_d Y_d^\dagger Y_u Y_u^\dagger)^{ba} - 6 (Y_u^\dagger Y_u Y_u^\dagger Y_d Y_d^\dagger)^{ba} - 60 \lambda^2 Y_u^{*ab} - 64 g_s^2 (Y_u^\dagger Y_u Y_u^\dagger)^{ab} \Big\} C_{uH}^{ab} \\
& + C_{uH}^{*ab} \left\{ \lambda \left( 3 (Y_u Y_u^\dagger Y_u)^{ab} + 40 g_s^2 Y_u^{ab} - \frac{23}{12} g_Y^2 Y_u^{ab} - \frac{27}{4} g_L^2 Y_u^{ab} - 12 (Y_d Y_d^\dagger Y_u)^{ab} \right) + \frac{21}{2} g_Y^2 g_L^2 Y_u^{ab} + 138 (Y_u Y_u^\dagger Y_u Y_u^\dagger Y_u)^{ab} - \frac{9}{4} g_L^4 Y_u^{ab} \right. \\
& - \frac{19}{4} g_Y^4 Y_u^{ab} - \frac{16}{3} g_Y^2 (Y_u Y_u^\dagger Y_u)^{ab} - 6 (Y_d Y_d^\dagger Y_d Y_d^\dagger Y_u)^{ab} - 6 (Y_d Y_d^\dagger Y_u Y_u^\dagger Y_u)^{ab} - 6 (Y_u Y_u^\dagger Y_d Y_d^\dagger Y_u)^{ab} - 60 \lambda^2 Y_u^{ab} - 64 g_s^2 (Y_u Y_u^\dagger Y_u)^{ab} \Big\} \\
& + \left\{ \lambda \left( 3 (Y_d^\dagger Y_d Y_d^\dagger)^{ab} + 40 g_s^2 Y_d^{*ab} - \frac{27}{4} g_L^2 Y_d^{*ab} - \frac{83}{12} g_Y^2 Y_d^{*ab} - 12 (Y_u^\dagger Y_u Y_d^\dagger)^{ab} \right) + \frac{5}{4} g_Y^4 Y_d^{*ab} + \frac{8}{3} g_Y^2 (Y_d^\dagger Y_d Y_d^\dagger)^{ab} + \frac{9}{2} g_Y^2 g_L^2 Y_d^{*ab} \right. \\
& + 138 (Y_d^\dagger Y_d Y_d^\dagger Y_d Y_d^\dagger)^{ba} - \frac{9}{4} g_L^4 Y_d^{*ab} - 6 (Y_d^\dagger Y_d Y_d^\dagger Y_u Y_u^\dagger)^{ba} - 6 (Y_d^\dagger Y_u Y_u^\dagger Y_d Y_d^\dagger)^{ba} - 6 (Y_d^\dagger Y_u Y_u^\dagger Y_u Y_u^\dagger)^{ba} - 60 \lambda^2 Y_d^{*ab} \\
& - 64 g_s^2 (Y_d^\dagger Y_d Y_d^\dagger)^{ab} \Big\} C_{dH}^{ab} + C_{dH}^{*ab} \left\{ \lambda \left( 3 (Y_d Y_d^\dagger Y_d)^{ab} + 40 g_s^2 Y_d^{ab} - \frac{27}{4} g_L^2 Y_d^{ab} - \frac{83}{12} g_Y^2 Y_d^{ab} - 12 (Y_u Y_u^\dagger Y_d)^{ab} \right) + \frac{5}{4} g_Y^4 Y_d^{ab} + \frac{8}{3} g_Y^2 (Y_d Y_d^\dagger Y_d)^{ab} \right. \\
& + \frac{9}{2} g_Y^2 g_L^2 Y_d^{ab} + 138 (Y_d Y_d^\dagger Y_d Y_d^\dagger Y_d)^{ab} - \frac{9}{4} g_L^4 Y_d^{ab} - 6 (Y_d Y_d^\dagger Y_u Y_u^\dagger Y_d)^{ab} - 6 (Y_u Y_u^\dagger Y_d Y_d^\dagger Y_d)^{ab} - 6 (Y_u Y_u^\dagger Y_u Y_u^\dagger Y_d)^{ab} - 60 \lambda^2 Y_d^{ab} \\
& - 64 g_s^2 (Y_d Y_d^\dagger Y_d)^{ab} \Big\} + \left\{ \lambda \left( \frac{7}{2} g_Y^4 Y_e^{*ab} - \frac{3}{2} g_Y^2 g_L^2 Y_e^{*ab} - 4 g_Y^2 (Y_e^\dagger Y_e Y_e^\dagger)^{ab} \right) + 2 g_Y^2 g_L^2 (Y_e^\dagger Y_e Y_e^\dagger)^{ab} + \frac{5}{2} g_Y^2 g_L^4 Y_e^{*ab} + 3 \lambda^2 g_Y^2 Y_e^{*ab} \right. \\
& + 24 g_Y^2 (Y_e^\dagger Y_e Y_e^\dagger Y_e Y_e^\dagger)^{ba} - 5 g_Y^4 g_L^2 Y_e^{*ab} - 6 g_Y^4 (Y_e^\dagger Y_e Y_e^\dagger)^{ab} - \frac{15}{2} g_Y^6 Y_e^{*ab} \Big\} C_{eB}^{ab} + C_{eB}^{*ab} \left\{ \lambda \left( \frac{7}{2} g_Y^4 Y_e^{ab} - \frac{3}{2} g_Y^2 g_L^2 Y_e^{ab} - 4 g_Y^2 (Y_e Y_e^\dagger Y_e)^{ab} \right) \right.
\end{aligned}$$



$$\begin{aligned}
& + 2g_Y^2 g_L^2 (Y_e Y_e^\dagger Y_e)^{ab} + \frac{5}{2} g_Y^2 g_L^4 Y_e^{ab} + 3\lambda^2 g_Y^2 Y_e^{ab} + 24g_Y^2 (Y_e Y_e^\dagger Y_e Y_e^\dagger Y_e)^{ab} - 5g_Y^4 g_L^2 Y_e^{ab} - 6g_Y^4 (Y_e Y_e^\dagger Y_e)^{ab} - \frac{15}{2} g_Y^6 Y_e^{ab} \Big\} \\
& + \left\{ \lambda \left( \frac{7}{4} g_Y^2 g_L^2 Y_e^{*ab} + \frac{13}{2} g_L^2 (Y_e^\dagger Y_e Y_e^\dagger)^{ab} - \frac{77}{12} g_L^4 Y_e^{*ab} \right) + \frac{15}{4} g_L^6 Y_e^{*ab} - \frac{3}{2} \lambda^2 g_L^2 Y_e^{*ab} - \frac{5}{2} g_Y^2 g_L^4 Y_e^{*ab} - 3g_L^4 (Y_e^\dagger Y_e Y_e^\dagger)^{ab} \right. \\
& - 3g_Y^2 g_L^2 (Y_e^\dagger Y_e Y_e^\dagger)^{ab} - \frac{15}{4} g_Y^4 g_L^2 Y_e^{*ab} - 6g_L^2 (Y_e^\dagger Y_e Y_e^\dagger Y_e Y_e^\dagger)^{ba} \Big\} C_{eW}^{ab} + C_{eW}^{*ab} \left\{ \lambda \left( \frac{7}{4} g_Y^2 g_L^2 Y_e^{ab} + \frac{13}{2} g_L^2 (Y_e Y_e^\dagger Y_e)^{ab} - \frac{77}{12} g_L^4 Y_e^{ab} \right) + \frac{15}{4} g_L^6 Y_e^{ab} \right. \\
& - \frac{3}{2} \lambda^2 g_L^2 Y_e^{ab} - \frac{5}{2} g_Y^2 g_L^4 Y_e^{ab} - 3g_L^4 (Y_e Y_e^\dagger Y_e)^{ab} - 3g_Y^2 g_L^2 (Y_e Y_e^\dagger Y_e)^{ab} - \frac{15}{4} g_Y^4 g_L^2 Y_e^{ab} - 6g_L^2 (Y_e Y_e^\dagger Y_e Y_e^\dagger Y_e)^{ab} \Big\} + \left\{ \lambda \left( g_Y^2 \left( 3(Y_d^\dagger Y_d Y_u^\dagger)^{ab} \right. \right. \right. \\
& + 8(Y_u^\dagger Y_u Y_u^\dagger)^{ab} \Big) + \frac{11}{6} g_Y^2 g_L^2 Y_u^{*ab} - \frac{35}{6} g_Y^4 Y_u^{*ab} \Big) + 5g_Y^4 g_L^2 Y_u^{*ab} + 10g_Y^4 (Y_u^\dagger Y_u Y_u^\dagger)^{ab} + \frac{25}{2} g_Y^6 Y_u^{*ab} - 5\lambda^2 g_Y^2 Y_u^{*ab} - 6g_Y^2 g_L^2 (Y_u^\dagger Y_u Y_u^\dagger)^{ab} \\
& - \frac{15}{2} g_Y^2 g_L^4 Y_u^{*ab} - 40g_Y^2 (Y_u^\dagger Y_u Y_u^\dagger Y_u Y_u^\dagger)^{ba} \Big\} C_{uB}^{ab} + C_{uB}^{*ab} \left\{ \lambda \left( g_Y^2 \left( 3(Y_d Y_d^\dagger Y_u)^{ab} + 8(Y_u Y_u^\dagger Y_u)^{ab} \right) + \frac{11}{6} g_Y^2 g_L^2 Y_u^{ab} - \frac{35}{6} g_Y^4 Y_u^{ab} \right) + 5g_Y^4 g_L^2 Y_u^{ab} \right. \\
& + 10g_Y^4 (Y_u Y_u^\dagger Y_u)^{ab} + \frac{25}{2} g_Y^6 Y_u^{ab} - 5\lambda^2 g_Y^2 Y_u^{ab} - 6g_Y^2 g_L^2 (Y_u Y_u^\dagger Y_u)^{ab} - \frac{15}{2} g_Y^2 g_L^4 Y_u^{ab} - 40g_Y^2 (Y_u Y_u^\dagger Y_u Y_u^\dagger Y_u)^{ab} \Big\} + \left\{ g_L^4 \left( 18(Y_d^\dagger Y_d Y_u^\dagger)^{ab} \right. \right. \\
& - 9(Y_u^\dagger Y_u Y_u^\dagger)^{ab} \Big) + \lambda \left( g_L^2 \left( \frac{39}{2} (Y_u^\dagger Y_u Y_u^\dagger)^{ab} + 24(Y_d^\dagger Y_d Y_u^\dagger)^{ab} \right) + \frac{17}{4} g_Y^2 g_L^2 Y_u^{*ab} - \frac{77}{4} g_L^4 Y_u^{*ab} \right) + g_L^2 \left( 6(Y_u^\dagger Y_d Y_d^\dagger Y_d Y_d^\dagger)^{ba} - 18(Y_u^\dagger Y_u Y_u^\dagger Y_u Y_u^\dagger)^{ba} \right. \\
& - 24(Y_u^\dagger Y_u Y_u^\dagger Y_d Y_d^\dagger)^{ba} \Big) + \frac{45}{4} g_L^6 Y_u^{*ab} - \frac{5}{2} g_Y^2 g_L^4 Y_u^{*ab} - \frac{9}{2} \lambda^2 g_L^2 Y_u^{*ab} - 5g_Y^2 g_L^2 (Y_u^\dagger Y_u Y_u^\dagger)^{ab} - \frac{25}{4} g_Y^4 g_L^2 Y_u^{*ab} \Big\} C_{uW}^{ab} \\
& + C_{uW}^{*ab} \left\{ g_L^4 \left( 18(Y_d Y_d^\dagger Y_u)^{ab} - 9(Y_u Y_u^\dagger Y_u)^{ab} \right) + \lambda \left( g_L^2 \left( \frac{39}{2} (Y_u Y_u^\dagger Y_u)^{ab} + 24(Y_d Y_d^\dagger Y_u)^{ab} \right) + \frac{17}{4} g_Y^2 g_L^2 Y_u^{ab} - \frac{77}{4} g_L^4 Y_u^{ab} \right) + g_L^2 \left( 6(Y_d Y_d^\dagger Y_d Y_d^\dagger Y_u)^{ab} \right. \right. \\
& - 18(Y_u Y_u^\dagger Y_u Y_u^\dagger Y_u)^{ab} - 24(Y_d Y_d^\dagger Y_u Y_u^\dagger Y_u)^{ab} \Big) + \frac{45}{4} g_L^6 Y_u^{ab} - \frac{5}{2} g_Y^2 g_L^4 Y_u^{ab} - \frac{9}{2} \lambda^2 g_L^2 Y_u^{ab} - 5g_Y^2 g_L^2 (Y_u Y_u^\dagger Y_u)^{ab} - \frac{25}{4} g_Y^4 g_L^2 Y_u^{ab} \Big\} \\
& + \left\{ \lambda \left( \frac{32}{3} g_s^2 g_L^2 Y_u^{*ab} + \frac{32}{3} g_Y^2 g_s^2 Y_u^{*ab} + 16g_s^2 (Y_u^\dagger Y_u Y_u^\dagger)^{ab} \right) - 16\lambda^2 g_s^2 Y_u^{*ab} - 128g_s^2 (Y_u^\dagger Y_u Y_u^\dagger Y_u Y_u^\dagger)^{ba} \right\} C_{uG}^{ab} + C_{uG}^{*ab} \left\{ \lambda \left( \frac{32}{3} g_s^2 g_L^2 Y_u^{ab} \right. \right. \\
& + \frac{32}{3} g_Y^2 g_s^2 Y_u^{ab} + 16g_s^2 (Y_u Y_u^\dagger Y_u)^{ab} \Big) - 16\lambda^2 g_s^2 Y_u^{ab} - 128g_s^2 (Y_u Y_u^\dagger Y_u Y_u^\dagger Y_u)^{ab} \Big\} + \left\{ \lambda^2 g_Y^2 Y_d^{*ab} + \lambda \left( \frac{5}{6} g_Y^2 g_L^2 Y_d^{*ab} + \frac{7}{6} g_Y^4 Y_d^{*ab} \right. \right. \\
& - g_Y^2 \left( 3(Y_u^\dagger Y_u Y_d^\dagger)^{ab} + 4(Y_d^\dagger Y_d Y_d^\dagger)^{ab} \right) \Big) + 5g_Y^4 g_L^2 Y_d^{*ab} + 6g_Y^2 g_L^2 (Y_d^\dagger Y_d Y_d^\dagger)^{ab} + \frac{15}{2} g_Y^2 g_L^4 Y_d^{*ab} + 8g_Y^2 (Y_d^\dagger Y_d Y_d^\dagger Y_d Y_d^\dagger)^{ba} - 2g_Y^4 (Y_d^\dagger Y_d Y_d^\dagger)^{ab} \\
& - \frac{5}{2} g_Y^6 Y_d^{*ab} \Big\} C_{dB}^{ab} + C_{dB}^{*ab} \left\{ \lambda^2 g_Y^2 Y_d^{ab} + \lambda \left( \frac{5}{6} g_Y^2 g_L^2 Y_d^{ab} + \frac{7}{6} g_Y^4 Y_d^{ab} - g_Y^2 \left( 3(Y_u Y_u^\dagger Y_d)^{ab} + 4(Y_d Y_d^\dagger Y_d)^{ab} \right) \right) + 5g_Y^4 g_L^2 Y_d^{ab} + 6g_Y^2 g_L^2 (Y_d Y_d^\dagger Y_d)^{ab} \right. \\
& \left. \left. \left. \right. \right. \right.
\end{aligned}$$

$$\begin{aligned}
& + \frac{15}{2} g_Y^2 g_L^4 Y_d^{ab} + 8 g_Y^2 (Y_d Y_d^\dagger Y_d Y_d^\dagger Y_d)^{ab} - 2 g_Y^4 (Y_d Y_d^\dagger Y_d)^{ab} - \frac{5}{2} g_Y^6 Y_d^{ab} \Bigg\} + \left\{ g_L^4 \left( 18 (Y_u^\dagger Y_u Y_d^\dagger)^{ab} - 9 (Y_d^\dagger Y_d Y_d^\dagger)^{ab} \right) + \lambda \left( g_L^2 \left( \frac{39}{2} (Y_d^\dagger Y_d Y_d^\dagger)^{ab} \right. \right. \right. \\
& + 24 (Y_u^\dagger Y_u Y_d^\dagger)^{ab} \Big) + \frac{13}{4} g_Y^2 g_L^2 Y_d^{*ab} - \frac{77}{4} g_L^4 Y_d^{*ab} \Big) + g_L^2 \left( 6 (Y_d^\dagger Y_u Y_u^\dagger Y_u Y_u^\dagger)^{ba} - 18 (Y_d^\dagger Y_d Y_d^\dagger Y_d Y_d^\dagger)^{ba} - 24 (Y_d^\dagger Y_d Y_d^\dagger Y_u Y_u^\dagger)^{ba} \right) + \frac{5}{2} g_Y^2 g_L^4 Y_d^{*ab} \\
& + \frac{45}{4} g_L^6 Y_d^{*ab} - g_Y^2 g_L^2 (Y_d^\dagger Y_d Y_d^\dagger)^{ab} - \frac{5}{4} g_Y^4 g_L^2 Y_d^{*ab} - \frac{9}{2} \lambda^2 g_L^2 Y_d^{*ab} \Bigg\} C_{dW}^{ab} + C_{dW}^{*ab} \left\{ g_L^4 \left( 18 (Y_u Y_u^\dagger Y_d)^{ab} - 9 (Y_d Y_d^\dagger Y_d)^{ab} \right) + \lambda \left( g_L^2 \left( \frac{39}{2} (Y_d Y_d^\dagger Y_d)^{ab} \right. \right. \right. \\
& + 24 (Y_u Y_u^\dagger Y_d)^{ab} \Big) + \frac{13}{4} g_Y^2 g_L^2 Y_d^{ab} - \frac{77}{4} g_L^4 Y_d^{ab} \Big) + g_L^2 \left( 6 (Y_u Y_u^\dagger Y_u Y_u^\dagger Y_d)^{ab} - 18 (Y_d Y_d^\dagger Y_d Y_d^\dagger Y_d)^{ab} - 24 (Y_u Y_u^\dagger Y_d Y_d^\dagger Y_d)^{ab} \right) + \frac{5}{2} g_Y^2 g_L^4 Y_d^{ab} \\
& + \frac{45}{4} g_L^6 Y_d^{ab} - g_Y^2 g_L^2 (Y_d Y_d^\dagger Y_d)^{ab} - \frac{5}{4} g_Y^4 g_L^2 Y_d^{ab} - \frac{9}{2} \lambda^2 g_L^2 Y_d^{ab} \Bigg\} + \left\{ \lambda \left( \frac{32}{3} g_s^2 g_L^2 Y_d^{*ab} + \frac{32}{3} g_Y^2 g_s^2 Y_d^{*ab} + 16 g_s^2 (Y_d^\dagger Y_d Y_d^\dagger)^{ab} \right) \right. \\
& - 16 \lambda^2 g_s^2 Y_d^{*ab} - 128 g_s^2 (Y_d^\dagger Y_d Y_d^\dagger Y_d Y_d^\dagger)^{ba} \Bigg\} C_{dG}^{ab} + C_{dG}^{*ab} \left\{ \lambda \left( \frac{32}{3} g_s^2 g_L^2 Y_d^{ab} + \frac{32}{3} g_Y^2 g_s^2 Y_d^{ab} + 16 g_s^2 (Y_d Y_d^\dagger Y_d)^{ab} \right) - 16 \lambda^2 g_s^2 Y_d^{ab} \right. \\
& - 128 g_s^2 (Y_d Y_d^\dagger Y_d Y_d^\dagger Y_d)^{ab} \Bigg\} + \left\{ g_L^4 (Y_e Y_e^\dagger)^{ba} + \lambda \left( \frac{89}{27} \delta^{ab} g_Y^4 + \frac{143}{27} \delta^{ab} g_Y^2 g_L^2 + \frac{311}{18} g_Y^2 (Y_e Y_e^\dagger)^{ba} - \frac{7}{18} g_L^2 (Y_e Y_e^\dagger)^{ba} - 12 (Y_e Y_e^\dagger Y_e Y_e^\dagger)^{ba} \right) \right. \\
& - \lambda^2 \left( \frac{16}{3} \delta^{ab} g_Y^2 + \frac{16}{3} (Y_e Y_e^\dagger)^{ba} \right) - \frac{4}{3} \delta^{ab} g_Y^2 g_L^4 - \frac{4}{3} \delta^{ab} g_Y^6 - \frac{8}{3} \delta^{ab} g_Y^4 g_L^2 - 8 g_Y^2 (Y_e Y_e^\dagger Y_e Y_e^\dagger)^{ba} - 10 g_Y^2 g_L^2 (Y_e Y_e^\dagger)^{ba} - 11 g_Y^4 (Y_e Y_e^\dagger)^{ba} \Bigg\} C_{He}^{(II)ab} \\
& + \left\{ \frac{2}{3} \delta^{ab} g_Y^2 g_L^4 + \lambda^2 \left( \frac{14}{3} \delta^{ab} g_L^2 - \frac{8}{3} \delta^{ab} g_Y^2 - \frac{26}{3} (Y_e Y_e^\dagger)^{ba} \right) + \lambda \left( \frac{83}{54} \delta^{ab} g_Y^2 g_L^2 + \frac{89}{54} \delta^{ab} g_Y^4 + \frac{74}{9} g_L^2 (Y_e Y_e^\dagger)^{ba} + \frac{167}{9} g_Y^2 (Y_e Y_e^\dagger)^{ba} \right. \right. \\
& - 8 (Y_e Y_e^\dagger Y_e Y_e^\dagger)^{ba} - 9 \delta^{ab} g_L^4 \Big) + 2 \delta^{ab} g_L^6 + 2 g_L^4 (Y_e Y_e^\dagger)^{ba} - \frac{2}{3} \delta^{ab} g_Y^4 g_L^2 - \frac{2}{3} \delta^{ab} g_Y^6 - 4 (Y_e Y_e^\dagger Y_e Y_e^\dagger Y_e Y_e^\dagger)^{ab} - 8 g_Y^2 (Y_e Y_e^\dagger Y_e Y_e^\dagger)^{ba} \\
& - 10 g_Y^2 g_L^2 (Y_e Y_e^\dagger)^{ba} - 11 g_Y^4 (Y_e Y_e^\dagger)^{ba} \Bigg\} C_{He}^{(\times)ab} + \left\{ \lambda^2 \left( \frac{16}{3} (Y_e^\dagger Y_e)^{ba} - \frac{16}{3} \delta^{ab} g_Y^2 \right) + \lambda \left( \frac{62}{27} \delta^{ab} g_Y^2 g_L^2 + \frac{170}{27} \delta^{ab} g_Y^4 + 12 (Y_e^\dagger Y_e Y_e^\dagger Y_e)^{ba} \right. \right. \\
& - \frac{77}{18} g_L^2 (Y_e^\dagger Y_e)^{ba} - \frac{167}{18} g_Y^2 (Y_e^\dagger Y_e)^{ba} \Big) + 4 g_L^2 (Y_e^\dagger Y_e Y_e^\dagger Y_e)^{ba} + 5 g_L^4 (Y_e^\dagger Y_e)^{ba} - \frac{4}{3} \delta^{ab} g_Y^2 g_L^4 - \frac{4}{3} \delta^{ab} g_Y^6 - 2 g_Y^2 g_L^2 (Y_e^\dagger Y_e)^{ba} - \frac{8}{3} \delta^{ab} g_Y^4 g_L^2 \\
& - 4 g_Y^2 (Y_e^\dagger Y_e Y_e^\dagger Y_e)^{ba} - 7 g_Y^4 (Y_e^\dagger Y_e)^{ba} \Bigg\} C_{He}^{ab} + \left\{ g_L^4 \left( 3 (Y_d Y_d^\dagger)^{ba} - 3 (Y_u Y_u^\dagger)^{ba} \right) + \lambda^2 \left( \frac{16}{3} \delta^{ab} g_Y^2 + 16 (Y_u Y_u^\dagger)^{ba} - 16 (Y_d Y_d^\dagger)^{ba} \right) + g_Y^2 g_L^2 \left( 18 (Y_u Y_u^\dagger)^{ba} \right. \right. \\
& - 6 (Y_d Y_d^\dagger)^{ba} \Big) + g_Y^4 \left( 21 (Y_u Y_u^\dagger)^{ba} - 9 (Y_d Y_d^\dagger)^{ba} \right) + g_Y^2 \left( 16 (Y_u Y_u^\dagger Y_u Y_u^\dagger)^{ba} - 8 (Y_d Y_d^\dagger Y_d Y_d^\dagger)^{ba} \right) + \lambda \left( g_s^2 \left( 80 (Y_d Y_d^\dagger)^{ba} - 80 (Y_u Y_u^\dagger)^{ba} \right) + g_Y^2 \left( \frac{47}{6} (Y_d Y_d^\dagger)^{ba} \right. \right. \\
& - \frac{139}{6} (Y_u Y_u^\dagger)^{ba} \Big) + g_L^2 \left( \frac{7}{6} (Y_u Y_u^\dagger)^{ba} - \frac{7}{6} (Y_d Y_d^\dagger)^{ba} \right) + 36 (Y_u Y_u^\dagger Y_u Y_u^\dagger)^{ba} - \frac{65}{27} \delta^{ab} g_Y^4 - \frac{143}{27} \delta^{ab} g_Y^2 g_L^2 - \frac{16}{3} \delta^{ab} g_Y^2 g_s^2 - 36 (Y_d Y_d^\dagger Y_d Y_d^\dagger)^{ba} \Bigg\}
\end{aligned}$$

$$\begin{aligned}
& + \frac{4}{3}\delta^{ab}g_Y^2g_L^4 + \frac{4}{3}\delta^{ab}g_Y^6 + \frac{8}{3}\delta^{ab}g_Y^4g_L^2 \Big\} C_{Hq}^{(\parallel)ab} + \left\{ \frac{2}{3}\delta^{ab}g_Y^6 + \lambda^2 \left( \frac{8}{3}\delta^{ab}g_Y^2 + 14\delta^{ab}g_L^2 - 10(Y_uY_u^\dagger)^{ba} - 26(Y_dY_d^\dagger)^{ba} \right) + g_L^4 \left( 3(Y_uY_u^\dagger)^{ba} \right. \right. \\
& + 6(Y_dY_d^\dagger)^{ba} \Big) + \lambda \left( g_Y^2 \left( \frac{5}{2}(Y_uY_u^\dagger)^{ba} + 9(Y_dY_d^\dagger)^{ba} \right) + g_L^2 \left( \frac{74}{3}(Y_dY_d^\dagger)^{ba} + \frac{155}{6}(Y_uY_u^\dagger)^{ba} \right) + 12(Y_uY_u^\dagger Y_uY_u^\dagger)^{ba} + 15(Y_dY_d^\dagger Y_uY_u^\dagger)^{ba} + 15(Y_uY_u^\dagger Y_dY_d^\dagger)^{ba} \right. \\
& + 80g_s^2(Y_dY_d^\dagger)^{ba} - \frac{65}{54}\delta^{ab}g_Y^4 - \frac{8}{3}\delta^{ab}g_Y^2g_s^2 - \frac{251}{54}\delta^{ab}g_Y^2g_L^2 - 8\delta^{ab}g_s^2g_L^2 - 24(Y_dY_d^\dagger Y_dY_d^\dagger)^{ba} - 27\delta^{ab}g_L^4 \Big) + \frac{10}{3}\delta^{ab}g_Y^4g_L^2 + \frac{14}{3}\delta^{ab}g_Y^2g_L^4 \\
& + 6\delta^{ab}g_L^6 + 6(Y_dY_d^\dagger Y_dY_d^\dagger Y_uY_u^\dagger)^{ab} + 6(Y_dY_d^\dagger Y_uY_u^\dagger Y_uY_u^\dagger)^{ab} + 6(Y_uY_u^\dagger Y_dY_d^\dagger Y_dY_d^\dagger)^{ab} + 6(Y_uY_u^\dagger Y_uY_u^\dagger Y_dY_d^\dagger)^{ab} - 6g_Y^2g_L^2(Y_dY_d^\dagger)^{ba} \\
& - 8g_Y^2(Y_dY_d^\dagger Y_dY_d^\dagger)^{ba} - 9g_Y^4(Y_dY_d^\dagger)^{ba} - 12(Y_dY_d^\dagger Y_dY_d^\dagger Y_dY_d^\dagger)^{ab} - 12(Y_uY_u^\dagger Y_uY_u^\dagger Y_uY_u^\dagger)^{ab} \Big\} C_{Hq}^{(\times)ab} + \left\{ \lambda^2 \left( \frac{32}{3}\delta^{ab}g_Y^2 - 16(Y_u^\dagger Y_u)^{ba} \right) \right. \\
& + \lambda \left( 6(Y_u^\dagger Y_dY_d^\dagger Y_u)^{ba} + \frac{59}{6}g_Y^2(Y_u^\dagger Y_u)^{ba} + \frac{77}{6}g_L^2(Y_u^\dagger Y_u)^{ba} + 80g_s^2(Y_u^\dagger Y_u)^{ba} - \frac{124}{27}\delta^{ab}g_Y^2g_L^2 - \frac{220}{27}\delta^{ab}g_Y^4 - \frac{32}{3}\delta^{ab}g_Y^2g_s^2 - 36(Y_u^\dagger Y_u Y_u^\dagger Y_u)^{ba} \right. \\
& + \frac{8}{3}\delta^{ab}g_Y^2g_L^4 + \frac{8}{3}\delta^{ab}g_Y^6 + 4g_Y^2(Y_u^\dagger Y_u Y_u^\dagger Y_u)^{ba} + \frac{16}{3}\delta^{ab}g_Y^4g_L^2 + 9g_Y^4(Y_u^\dagger Y_u)^{ba} - 6g_Y^2g_L^2(Y_u^\dagger Y_u)^{ba} - 12g_L^2(Y_u^\dagger Y_u Y_u^\dagger Y_u)^{ba} \\
& - 15g_L^4(Y_u^\dagger Y_u)^{ba} \Big\} C_{Hu}^{ab} + \left\{ \lambda^2 \left( 16(Y_d^\dagger Y_d)^{ba} - \frac{16}{3}\delta^{ab}g_Y^2 \right) + \lambda \left( \frac{62}{27}\delta^{ab}g_Y^2g_L^2 + \frac{74}{27}\delta^{ab}g_Y^4 + \frac{16}{3}\delta^{ab}g_Y^2g_s^2 + 36(Y_d^\dagger Y_d Y_d^\dagger Y_d)^{ba} - \frac{31}{6}g_Y^2(Y_d^\dagger Y_d)^{ba} \right. \right. \\
& - 6(Y_d^\dagger Y_u Y_u^\dagger Y_d)^{ba} - \frac{77}{6}g_L^2(Y_d^\dagger Y_d)^{ba} - 80g_s^2(Y_d^\dagger Y_d)^{ba} \Big) + 3g_Y^4(Y_d^\dagger Y_d)^{ba} + 4g_Y^2(Y_d^\dagger Y_d Y_d^\dagger Y_d)^{ba} + 12g_L^2(Y_d^\dagger Y_d Y_d^\dagger Y_d)^{ba} + 15g_L^4(Y_d^\dagger Y_d)^{ba} \\
& + 18g_Y^2g_L^2(Y_d^\dagger Y_d)^{ba} - \frac{4}{3}\delta^{ab}g_Y^2g_L^4 - \frac{4}{3}\delta^{ab}g_Y^6 - \frac{8}{3}\delta^{ab}g_Y^4g_L^2 \Big\} C_{Hd}^{ab} + \left\{ g_L^2 \left( 6(Y_d^\dagger Y_d Y_d^\dagger Y_u)^{ba} + 6(Y_d^\dagger Y_u Y_u^\dagger Y_u)^{ba} \right) + 10\lambda^2(Y_d^\dagger Y_u)^{ba} \right. \\
& + 15g_L^4(Y_d^\dagger Y_u)^{ba} - \lambda \left( \frac{17}{6}g_Y^2(Y_d^\dagger Y_u)^{ba} + 12(Y_d^\dagger Y_d Y_d^\dagger Y_u)^{ba} + 12(Y_d^\dagger Y_u Y_u^\dagger Y_u)^{ba} + \frac{239}{6}g_L^2(Y_d^\dagger Y_u)^{ba} \right) \Big\} C_{Hud}^{ab} + C_{Hud}^{*ab} \left\{ g_L^2 \left( 6(Y_u^\dagger Y_d Y_d^\dagger Y_d)^{ab} \right. \right. \\
& + 6(Y_u^\dagger Y_u Y_u^\dagger Y_d)^{ab} \Big) + 10\lambda^2(Y_u^\dagger Y_d)^{ab} + 15g_L^4(Y_u^\dagger Y_d)^{ab} - \lambda \left( \frac{17}{6}g_Y^2(Y_u^\dagger Y_d)^{ab} + 12(Y_u^\dagger Y_d Y_d^\dagger Y_d)^{ab} + 12(Y_u^\dagger Y_u Y_u^\dagger Y_d)^{ab} + \frac{239}{6}g_L^2(Y_u^\dagger Y_d)^{ab} \right) \Big\} \\
& + \left\{ \lambda \left( 8Y_e^{bc}(Y_e^\dagger Y_e Y_e^\dagger)^{ad} + 8Y_e^{*ad}(Y_e Y_e^\dagger Y_e)^{bc} \right) - 4\lambda^2 Y_e^{*ad} Y_e^{bc} - 16(Y_e^\dagger Y_e Y_e^\dagger)^{ad}(Y_e Y_e^\dagger Y_e)^{bc} \right\} C_{\ell e}^{abcd} + \left\{ \lambda \left( 24Y_u^{bc}(Y_u^\dagger Y_u Y_u^\dagger)^{ad} \right. \right. \\
& + 24Y_u^{*ad}(Y_u Y_u^\dagger Y_u)^{bc} \Big) - 12\lambda^2 Y_u^{*ad} Y_u^{bc} - 48(Y_u^\dagger Y_u Y_u^\dagger)^{ad}(Y_u Y_u^\dagger Y_u)^{bc} \Big\} C_{qu}^{(\parallel)abcd} + \left\{ \lambda \left( 72Y_u^{bc}(Y_u^\dagger Y_u Y_u^\dagger)^{ad} + 72Y_u^{*ad}(Y_u Y_u^\dagger Y_u)^{bc} \right) \right. \\
& - 36\lambda^2 Y_u^{*ad} Y_u^{bc} - 144(Y_u^\dagger Y_u Y_u^\dagger)^{ad}(Y_u Y_u^\dagger Y_u)^{bc} \Big\} C_{qu}^{(\times)abcd} + \left\{ \lambda \left( 24Y_d^{bc}(Y_d^\dagger Y_d Y_d^\dagger)^{ad} + 24Y_d^{*ad}(Y_d Y_d^\dagger Y_d)^{bc} \right) - 12\lambda^2 Y_d^{*ad} Y_d^{bc} \right. \\
& - 48(Y_d^\dagger Y_d Y_d^\dagger)^{ad}(Y_d Y_d^\dagger Y_d)^{bc} \Big\} C_{qd}^{(\parallel)abcd} + \left\{ \lambda \left( 72Y_d^{bc}(Y_d^\dagger Y_d Y_d^\dagger)^{ad} + 72Y_d^{*ad}(Y_d Y_d^\dagger Y_d)^{bc} \right) - 36\lambda^2 Y_d^{*ad} Y_d^{bc} - 144(Y_d^\dagger Y_d Y_d^\dagger)^{ad}(Y_d Y_d^\dagger Y_d)^{bc} \right\} C_{qd}^{(\times)abcd}
\end{aligned}$$

$$\begin{aligned}
& + \lambda \left\{ \frac{16}{3} \delta^{ad} g_Y^2 (Y_e^\dagger Y_e)^{bc} - \frac{8}{9} \delta^{ab} \delta^{cd} g_Y^4 - 8 (Y_e^\dagger Y_e)^{ba} (Y_e^\dagger Y_e)^{dc} \right\} C_{ee}^{abcd} + \lambda \left\{ \frac{32}{3} \delta^{ad} g_Y^2 (Y_u^\dagger Y_u)^{bc} - \frac{32}{27} \delta^{ad} \delta^{bc} g_Y^4 - 24 (Y_u^\dagger Y_u)^{bc} (Y_u^\dagger Y_u)^{da} \right\} C_{uu}^{abcd} \\
& + \lambda \left\{ \frac{16}{3} \delta^{ad} g_Y^2 (Y_d^\dagger Y_d)^{bc} - \frac{8}{27} \delta^{ad} \delta^{bc} g_Y^4 - 24 (Y_d^\dagger Y_d)^{bc} (Y_d^\dagger Y_d)^{da} \right\} C_{dd}^{abcd} + \lambda \left\{ \frac{8}{3} \delta^{bc} g_L^2 (Y_e Y_e^\dagger)^{da} - \frac{4}{9} \delta^{ad} \delta^{bc} g_L^4 - \frac{4}{9} \delta^{ad} \delta^{bc} g_Y^4 - \frac{8}{3} \delta^{bc} g_Y^2 (Y_e Y_e^\dagger)^{da} \right. \\
& \left. - 8 (Y_e Y_e^\dagger)^{bc} (Y_e Y_e^\dagger)^{da} \right\} C_{\ell\ell}^{abcd} + \lambda \left\{ g_Y^2 \left( \frac{8}{3} \delta^{bc} (Y_d Y_d^\dagger)^{da} - \frac{8}{3} \delta^{bc} (Y_u Y_u^\dagger)^{da} \right) + g_L^2 \left( 8 \delta^{bc} (Y_d Y_d^\dagger)^{da} + 8 \delta^{bc} (Y_u Y_u^\dagger)^{da} \right) - \frac{4}{27} \delta^{ad} \delta^{bc} g_Y^4 - \frac{4}{3} \delta^{ad} \delta^{bc} g_L^4 \right. \\
& \left. - 24 (Y_d Y_d^\dagger)^{bc} (Y_d Y_d^\dagger)^{da} - 24 (Y_u Y_u^\dagger)^{bc} (Y_u Y_u^\dagger)^{da} \right\} C_{qq}^{(\parallel)abcd} + \lambda \left\{ g_Y^2 \left( \frac{16}{3} \delta^{bc} (Y_d Y_d^\dagger)^{da} - \frac{16}{3} \delta^{bc} (Y_u Y_u^\dagger)^{da} \right) + 48 (Y_d Y_d^\dagger)^{da} (Y_u Y_u^\dagger)^{bc} - \frac{8}{27} \delta^{ad} \delta^{bc} g_Y^4 \right. \\
& \left. - 24 (Y_d Y_d^\dagger)^{bc} (Y_d Y_d^\dagger)^{da} - 24 (Y_u Y_u^\dagger)^{bc} (Y_u Y_u^\dagger)^{da} \right\} C_{qq}^{(\times)abcd}, \tag{4.2}
\end{aligned}$$

## 4.2 $C_{HD}^{(\parallel)}$

$$\begin{aligned}
\beta_{C_{HD}^{(\parallel)}}^{(1)} &= -8 \mathbf{T}_{\ell H} + \left\{ 4 \mathbf{T}_2 + 12 \lambda - \frac{4}{3} g_Y^2 - 4 g_L^2 \right\} C_{HD}^{(\parallel)} + \frac{10}{3} g_Y^2 C_{HD}^{(\times)} - \left\{ \frac{4}{3} \delta^{ab} g_Y^2 + 4 (Y_e Y_e^\dagger)^{ba} \right\} C_{H\ell}^{(\parallel)ab} + \left\{ 2 \delta^{ab} g_L^2 - \frac{2}{3} \delta^{ab} g_Y^2 - 8 (Y_e Y_e^\dagger)^{ba} \right\} C_{H\ell}^{(\times)ab} \\
&+ \left\{ 4 (Y_e^\dagger Y_e)^{ba} - \frac{4}{3} \delta^{ab} g_Y^2 \right\} C_{He}^{ab} + \left\{ \frac{4}{3} \delta^{ab} g_Y^2 - 12 \left( (Y_d Y_d^\dagger)^{ba} - (Y_u Y_u^\dagger)^{ba} \right) \right\} C_{Hq}^{(\parallel)ab} + \left\{ \frac{2}{3} \delta^{ab} g_Y^2 + 6 \delta^{ab} g_L^2 - 12 \left( (Y_u Y_u^\dagger)^{ba} + 2 (Y_d Y_d^\dagger)^{ba} \right) \right\} C_{Hq}^{(\times)ab} \\
&+ \left\{ \frac{8}{3} \delta^{ab} g_Y^2 - 12 (Y_u^\dagger Y_u)^{ba} \right\} C_{Hu}^{ab} + \left\{ 12 (Y_d^\dagger Y_d)^{ba} - \frac{4}{3} \delta^{ab} g_Y^2 \right\} C_{Hd}^{ab} + 12 C_{Hud}^{ab} (Y_d^\dagger Y_u)^{ba} + 12 C_{Hud}^{*ab} (Y_u^\dagger Y_d)^{ab}, \tag{4.3}
\end{aligned}$$

$$\begin{aligned}
\beta_{C_{HD}^{(\parallel)}}^{(2)} &= \frac{2}{3} g_Y^2 \mathbf{T}_{\ell H} + 16 \lambda \mathbf{T}_{\ell H} + 22 \text{Tr} \left[ C_{\ell HH}^\dagger C_{\ell HH} Y_e Y_e^\dagger \right] - 28 g_L^2 \mathbf{T}_{\ell H} + \left\{ \lambda \left( 11 g_Y^2 + 33 g_L^2 - 30 \mathbf{T}_2 \right) + g_Y^2 \left( \frac{11}{3} \text{Tr} \left[ Y_d^\dagger Y_d \right] + \frac{37}{3} \text{Tr} \left[ Y_e^\dagger Y_e \right] \right. \right. \\
&+ \left. \frac{41}{3} \text{Tr} \left[ Y_u^\dagger Y_u \right] \right) + g_s^2 \left( 80 \text{Tr} \left[ Y_d^\dagger Y_d \right] + 80 \text{Tr} \left[ Y_u^\dagger Y_u \right] \right) + 7 \mathbf{T}_2 g_L^2 + \frac{523}{72} g_Y^2 g_L^2 + \frac{5545}{432} g_Y^4 + \frac{339}{16} g_L^4 - \frac{7}{2} \mathbf{T}_4 - 45 \text{Tr} \left[ Y_d^\dagger Y_d Y_u^\dagger Y_u \right] \\
&\left. - 51 \lambda^2 \right\} C_{HD}^{(\parallel)} + \left\{ 3 \mathbf{T}_2 g_L^2 + \frac{7}{2} \mathbf{T}_4 - \lambda \left( 2 \mathbf{T}_2 + \frac{40}{3} g_Y^2 \right) - \frac{10}{3} \mathbf{T}_2 g_Y^2 - \frac{65}{18} g_Y^2 g_L^2 - \frac{496}{27} g_Y^4 - 33 \text{Tr} \left[ Y_d^\dagger Y_d Y_u^\dagger Y_u \right] \right\} C_{HD}^{(\times)} \\
&+ \left\{ g_Y^4 \left( 18 \text{Tr} \left[ Y_e^\dagger Y_e \right] - 2 \text{Tr} \left[ Y_u^\dagger Y_u \right] - 26 \text{Tr} \left[ Y_d^\dagger Y_d \right] \right) + 38 g_Y^4 g_L^2 + \frac{298}{3} g_Y^6 - 72 \lambda g_Y^4 \right\} C_{HB} + \left\{ 38 g_Y^2 g_L^4 + 62 g_L^6 - 18 \mathbf{T}_2 g_L^4 \right. \\
&\left. - 216 \lambda g_L^4 \right\} C_{HW} + g_s^4 \left\{ 192 \text{Tr} \left[ Y_d^\dagger Y_d \right] + 192 \text{Tr} \left[ Y_u^\dagger Y_u \right] \right\} C_{HG} + \left\{ g_Y^2 g_L^2 \left( 9 \text{Tr} \left[ Y_e^\dagger Y_e \right] + 15 \text{Tr} \left[ Y_d^\dagger Y_d \right] + 21 \text{Tr} \left[ Y_u^\dagger Y_u \right] \right) + 4 g_Y^2 g_L^4 \right.
\end{aligned}$$

$$\begin{aligned}
& -12\lambda g_Y^2 g_L^2 - 16g_Y^4 g_L^2 \Big\} C_{H\overline{W}B} + \Big\{ 4g_Y^2 g_L^6 + 16g_L^8 + 72\lambda g_L^6 - 18T_2 g_L^6 \Big\} C_W + \Big\{ 3g_Y^2 Y_e^{*ab} + 9g_L^2 Y_e^{*ab} - 6\lambda Y_e^{*ab} \Big\} C_{eH}^{ab} \\
& + C_{eH}^{*ab} \Big\{ 3g_Y^2 Y_e^{ab} + 9g_L^2 Y_e^{ab} - 6\lambda Y_e^{ab} \Big\} + \Big\{ 9g_Y^2 Y_u^{*ab} + 27g_L^2 Y_u^{*ab} - 18\lambda Y_u^{*ab} - 18(Y_d^\dagger Y_d Y_u^\dagger)^{ab} \Big\} C_{uH}^{ab} + C_{uH}^{*ab} \Big\{ 9g_Y^2 Y_u^{ab} + 27g_L^2 Y_u^{ab} \\
& - 18\lambda Y_u^{ab} - 18(Y_d Y_d^\dagger Y_u)^{ab} \Big\} + \Big\{ 9g_Y^2 Y_d^{*ab} + 27g_L^2 Y_d^{*ab} - 18\lambda Y_d^{*ab} - 18(Y_u^\dagger Y_u Y_d^\dagger)^{ab} \Big\} C_{dH}^{ab} + C_{dH}^{*ab} \Big\{ 9g_Y^2 Y_d^{ab} + 27g_L^2 Y_d^{ab} - 18\lambda Y_d^{ab} \\
& - 18(Y_u Y_u^\dagger Y_d)^{ab} \Big\} + \Big\{ \frac{3}{2}g_Y^2 g_L^2 Y_e^{*ab} + \frac{11}{2}g_Y^4 Y_e^{*ab} - 8g_Y^2 (Y_e^\dagger Y_e Y_e^\dagger)^{ab} \Big\} C_{eB}^{ab} + C_{eB}^{*ab} \Big\{ \frac{3}{2}g_Y^2 g_L^2 Y_e^{ab} + \frac{11}{2}g_Y^4 Y_e^{ab} - 8g_Y^2 (Y_e Y_e^\dagger Y_e)^{ab} \Big\} \\
& + \Big\{ \frac{23}{4}g_L^4 Y_e^{*ab} + \frac{23}{4}g_Y^2 g_L^2 Y_e^{*ab} - 6g_L^2 (Y_e^\dagger Y_e Y_e^\dagger)^{ab} \Big\} C_{eW}^{ab} + C_{eW}^{*ab} \Big\{ \frac{23}{4}g_L^4 Y_e^{ab} + \frac{23}{4}g_Y^2 g_L^2 Y_e^{ab} - 6g_L^2 (Y_e Y_e^\dagger Y_e)^{ab} \Big\} + \Big\{ \frac{7}{2}g_Y^2 g_L^2 Y_u^{*ab} \\
& - \frac{55}{6}g_Y^4 Y_u^{*ab} - 18g_Y^2 (Y_d^\dagger Y_d Y_u^\dagger)^{ab} \Big\} C_{uB}^{ab} + C_{uB}^{*ab} \Big\{ \frac{7}{2}g_Y^2 g_L^2 Y_u^{ab} - \frac{55}{6}g_Y^4 Y_u^{ab} - 18g_Y^2 (Y_d Y_d^\dagger Y_u)^{ab} \Big\} + \Big\{ \frac{33}{4}g_Y^2 g_L^2 Y_u^{*ab} + \frac{69}{4}g_L^4 Y_u^{*ab} \\
& - g_L^2 \big( 18(Y_u^\dagger Y_u Y_u^\dagger)^{ab} + 45(Y_d^\dagger Y_d Y_u^\dagger)^{ab} \big) \Big\} C_{uW}^{ab} + C_{uW}^{*ab} \Big\{ \frac{33}{4}g_Y^2 g_L^2 Y_u^{ab} + \frac{69}{4}g_L^4 Y_u^{ab} - g_L^2 \big( 18(Y_u Y_u^\dagger Y_u)^{ab} + 45(Y_d Y_d^\dagger Y_u)^{ab} \big) \Big\} + \Big\{ g_s^2 \big( 96(Y_d^\dagger Y_d Y_u^\dagger)^{ab} \\
& + 96(Y_u^\dagger Y_u Y_u^\dagger)^{ab} \big) - \frac{32}{3}g_Y^2 g_s^2 Y_u^{*ab} - 32g_s^2 g_L^2 Y_u^{*ab} \Big\} C_{uG}^{ab} + C_{uG}^{*ab} \Big\{ g_s^2 \big( 96(Y_d Y_d^\dagger Y_u)^{ab} + 96(Y_u Y_u^\dagger Y_u)^{ab} \big) - \frac{32}{3}g_Y^2 g_s^2 Y_u^{ab} - 32g_s^2 g_L^2 Y_u^{ab} \Big\} \\
& + \Big\{ g_Y^2 \big( 24(Y_d^\dagger Y_d Y_d^\dagger)^{ab} + 42(Y_u^\dagger Y_u Y_d^\dagger)^{ab} \big) + \frac{11}{6}g_Y^4 Y_d^{*ab} - \frac{23}{2}g_Y^2 g_L^2 Y_d^{*ab} \Big\} C_{dB}^{ab} + C_{dB}^{*ab} \Big\{ g_Y^2 \big( 24(Y_d Y_d^\dagger Y_d)^{ab} + 42(Y_u Y_u^\dagger Y_d)^{ab} \big) + \frac{11}{6}g_Y^4 Y_d^{ab} \\
& - \frac{23}{2}g_Y^2 g_L^2 Y_d^{ab} \Big\} + \Big\{ \frac{69}{4}g_L^4 Y_d^{*ab} - \frac{3}{4}g_Y^2 g_L^2 Y_d^{*ab} - g_L^2 \big( 18(Y_d^\dagger Y_d Y_d^\dagger)^{ab} + 45(Y_u^\dagger Y_u Y_d^\dagger)^{ab} \big) \Big\} C_{dW}^{ab} + C_{dW}^{*ab} \Big\{ \frac{69}{4}g_L^4 Y_d^{ab} - \frac{3}{4}g_Y^2 g_L^2 Y_d^{ab} \\
& - g_L^2 \big( 18(Y_d Y_d^\dagger Y_d)^{ab} + 45(Y_u Y_u^\dagger Y_d)^{ab} \big) \Big\} + \Big\{ g_s^2 \big( 96(Y_d^\dagger Y_d Y_d^\dagger)^{ab} + 96(Y_u^\dagger Y_u Y_d^\dagger)^{ab} \big) - \frac{32}{3}g_Y^2 g_s^2 Y_d^{*ab} - 32g_s^2 g_L^2 Y_d^{*ab} \Big\} C_{dG}^{ab} \\
& + C_{dG}^{*ab} \Big\{ g_s^2 \big( 96(Y_d Y_d^\dagger Y_d)^{ab} + 96(Y_u Y_u^\dagger Y_d)^{ab} \big) - \frac{32}{3}g_Y^2 g_s^2 Y_d^{ab} - 32g_s^2 g_L^2 Y_d^{ab} \Big\} + \Big\{ \frac{1}{27}\delta^{ab} g_Y^4 + \lambda \big( 4(Y_e Y_e^\dagger)^{ba} + \frac{20}{3}\delta^{ab} g_Y^2 \big) + \frac{25}{6}g_L^2 (Y_e Y_e^\dagger)^{ba} \\
& + \frac{229}{18}g_Y^2 (Y_e Y_e^\dagger)^{ba} + 26(Y_e Y_e^\dagger Y_e Y_e^\dagger)^{ba} - \frac{17}{9}\delta^{ab} g_Y^2 g_L^2 \Big\} C_{H\ell}^{(\parallel)ab} + \Big\{ \frac{1}{54}\delta^{ab} g_Y^4 + \lambda \big( \frac{10}{3}\delta^{ab} g_Y^2 + 8(Y_e Y_e^\dagger)^{ba} - 10\delta^{ab} g_L^2 \big) + \frac{27}{2}\delta^{ab} g_L^4 \\
& + 43(Y_e Y_e^\dagger Y_e Y_e^\dagger)^{ba} - \frac{158}{9}g_Y^2 (Y_e Y_e^\dagger)^{ba} - \frac{83}{3}g_L^2 (Y_e Y_e^\dagger)^{ba} \Big\} C_{H\ell}^{(\times)ab} + \Big\{ \lambda \big( \frac{20}{3}\delta^{ab} g_Y^2 - 4(Y_e^\dagger Y_e)^{ba} \big) + \frac{10}{9}\delta^{ab} g_Y^2 g_L^2 + \frac{41}{6}g_L^2 (Y_e^\dagger Y_e)^{ba}
\end{aligned}$$

$$\begin{aligned}
& + \frac{545}{18} g_Y^2 (Y_e^\dagger Y_e)^{ba} - \frac{80}{27} \delta^{ab} g_Y^4 - 28 (Y_e^\dagger Y_e Y_e^\dagger Y_e)^{ba} \Big\} C_{He}^{ab} + \left\{ g_Y^2 \left( \frac{85}{6} (Y_d Y_d^\dagger)^{ba} - \frac{197}{6} (Y_u Y_u^\dagger)^{ba} \right) + g_L^2 \left( \frac{25}{2} (Y_d Y_d^\dagger)^{ba} - \frac{25}{2} (Y_u Y_u^\dagger)^{ba} \right) + \lambda \left( 12 (Y_d Y_d^\dagger)^{ba} \right. \right. \\
& - \frac{20}{3} \delta^{ab} g_Y^2 - 12 (Y_u Y_u^\dagger)^{ba} \Big) + g_s^2 \left( 80 (Y_u Y_u^\dagger)^{ba} - 80 (Y_d Y_d^\dagger)^{ba} \right) + \frac{17}{9} \delta^{ab} g_Y^2 g_L^2 + \frac{16}{3} \delta^{ab} g_Y^2 g_s^2 + 78 (Y_d Y_d^\dagger Y_d Y_d^\dagger)^{ba} - \frac{25}{27} \delta^{ab} g_Y^4 \\
& - 78 (Y_u Y_u^\dagger Y_u Y_u^\dagger)^{ba} \Big\} C_{Hq}^{(\parallel)ab} + \left\{ g_Y^2 \left( \frac{22}{3} (Y_d Y_d^\dagger)^{ba} - \frac{253}{6} (Y_u Y_u^\dagger)^{ba} \right) + \lambda \left( 12 (Y_u Y_u^\dagger)^{ba} + 24 (Y_d Y_d^\dagger)^{ba} - \frac{10}{3} \delta^{ab} g_Y^2 - 30 \delta^{ab} g_L^2 \right) + \frac{8}{3} \delta^{ab} g_Y^2 g_s^2 \right. \\
& + 18 (Y_d Y_d^\dagger Y_u Y_u^\dagger)^{ba} + 18 (Y_u Y_u^\dagger Y_d Y_d^\dagger)^{ba} + 24 \delta^{ab} g_s^2 g_L^2 + \frac{81}{2} \delta^{ab} g_L^4 + 51 (Y_u Y_u^\dagger Y_u Y_u^\dagger)^{ba} + 129 (Y_d Y_d^\dagger Y_d Y_d^\dagger)^{ba} - \frac{2}{9} \delta^{ab} g_Y^2 g_L^2 - \frac{25}{54} \delta^{ab} g_Y^4 \\
& - g_s^2 \left( 80 (Y_u Y_u^\dagger)^{ba} + 160 (Y_d Y_d^\dagger)^{ba} \right) - g_L^2 \left( 83 (Y_d Y_d^\dagger)^{ba} + \frac{191}{2} (Y_u Y_u^\dagger)^{ba} \right) \Big\} C_{Hq}^{(\times)ab} + \left\{ \lambda \left( 12 (Y_u^\dagger Y_u)^{ba} - \frac{40}{3} \delta^{ab} g_Y^2 \right) + \frac{40}{27} \delta^{ab} g_Y^4 + \frac{32}{3} \delta^{ab} g_Y^2 g_s^2 \right. \\
& + 84 (Y_u^\dagger Y_u Y_u^\dagger Y_u)^{ba} - \frac{20}{9} \delta^{ab} g_Y^2 g_L^2 - 12 (Y_u^\dagger Y_d Y_d^\dagger Y_u)^{ba} - \frac{41}{2} g_L^2 (Y_u^\dagger Y_u)^{ba} - \frac{233}{6} g_Y^2 (Y_u^\dagger Y_u)^{ba} - 80 g_s^2 (Y_u^\dagger Y_u)^{ba} \Big\} C_{Hu}^{ab} + \left\{ \frac{1}{6} g_Y^2 (Y_d^\dagger Y_d)^{ba} \right. \\
& + \frac{16}{27} \delta^{ab} g_Y^4 + \lambda \left( \frac{20}{3} \delta^{ab} g_Y^2 - 12 (Y_d^\dagger Y_d)^{ba} \right) + \frac{10}{9} \delta^{ab} g_Y^2 g_L^2 + 12 (Y_d^\dagger Y_u Y_u^\dagger Y_d)^{ba} + \frac{41}{2} g_L^2 (Y_d^\dagger Y_d)^{ba} + 80 g_s^2 (Y_d^\dagger Y_d)^{ba} - \frac{16}{3} \delta^{ab} g_Y^2 g_s^2 \\
& - 84 (Y_d^\dagger Y_d Y_d^\dagger Y_d)^{ba} \Big\} C_{Hd}^{ab} + \left\{ \frac{41}{2} g_L^2 (Y_d^\dagger Y_u)^{ba} + \frac{45}{2} g_Y^2 (Y_d^\dagger Y_u)^{ba} + 80 g_s^2 (Y_d^\dagger Y_u)^{ba} - 12 \lambda (Y_d^\dagger Y_u)^{ba} - 36 (Y_d^\dagger Y_d Y_d^\dagger Y_u)^{ba} \right. \\
& - 36 (Y_d^\dagger Y_u Y_u^\dagger Y_u)^{ba} \Big\} C_{Hud}^{ab} + C_{Hud}^{*ab} \left\{ \frac{41}{2} g_L^2 (Y_u^\dagger Y_d)^{ab} + \frac{45}{2} g_Y^2 (Y_u^\dagger Y_d)^{ab} + 80 g_s^2 (Y_u^\dagger Y_d)^{ab} - 12 \lambda (Y_u^\dagger Y_d)^{ab} - 36 (Y_u^\dagger Y_d Y_d^\dagger Y_d)^{ab} \right. \\
& - 36 (Y_u^\dagger Y_u Y_u^\dagger Y_d)^{ab} \Big\} + \left\{ \frac{8}{9} \delta^{ab} \delta^{cd} g_Y^4 + 8 (Y_e^\dagger Y_e)^{ba} (Y_e^\dagger Y_e)^{dc} - \frac{16}{3} \delta^{ad} g_Y^2 (Y_e^\dagger Y_e)^{bc} \right\} C_{ee}^{abcd} + \left\{ \frac{32}{27} \delta^{ad} \delta^{bc} g_Y^4 + 24 (Y_u^\dagger Y_u)^{bc} (Y_u^\dagger Y_u)^{da} \right. \\
& - \frac{32}{3} \delta^{ad} g_Y^2 (Y_u^\dagger Y_u)^{bc} \Big\} C_{uu}^{abcd} + \left\{ \frac{8}{27} \delta^{ad} \delta^{bc} g_Y^4 + 24 (Y_d^\dagger Y_d)^{bc} (Y_d^\dagger Y_d)^{da} - \frac{16}{3} \delta^{ad} g_Y^2 (Y_d^\dagger Y_d)^{bc} \right\} C_{dd}^{abcd} + 48 C_{ud}^{(\parallel)abcd} (Y_d^\dagger Y_u)^{da} (Y_u^\dagger Y_d)^{bc} \\
& + 144 C_{ud}^{(\times)abcd} (Y_d^\dagger Y_u)^{da} (Y_u^\dagger Y_d)^{bc} + \left\{ \frac{4}{9} \delta^{ad} \delta^{bc} g_Y^4 + \frac{4}{3} \delta^{ad} \delta^{bc} g_L^4 + \frac{8}{3} \delta^{bc} g_Y^2 (Y_e Y_e^\dagger)^{da} + 16 (Y_e Y_e^\dagger)^{bc} (Y_e Y_e^\dagger)^{da} - 8 \delta^{bc} g_L^2 (Y_e Y_e^\dagger)^{da} \right\} C_{\ell\ell}^{abcd} \\
& + \left\{ \frac{4}{27} \delta^{ad} \delta^{bc} g_Y^4 + g_Y^2 \left( \frac{8}{3} \delta^{bc} (Y_u Y_u^\dagger)^{da} - \frac{8}{3} \delta^{bc} (Y_d Y_d^\dagger)^{da} \right) + 4 \delta^{ad} \delta^{bc} g_L^4 + 48 (Y_d Y_d^\dagger)^{bc} (Y_d Y_d^\dagger)^{da} + 48 (Y_d Y_d^\dagger)^{da} (Y_u Y_u^\dagger)^{bc} + 48 (Y_u Y_u^\dagger)^{bc} (Y_u Y_u^\dagger)^{da} \right. \\
& - g_L^2 \left( 24 \delta^{bc} (Y_d Y_d^\dagger)^{da} + 24 \delta^{bc} (Y_u Y_u^\dagger)^{da} \right) \Big\} C_{qq}^{(\parallel)abcd} + \left\{ \frac{8}{27} \delta^{ad} \delta^{bc} g_Y^4 + g_Y^2 \left( \frac{16}{3} \delta^{bc} (Y_u Y_u^\dagger)^{da} - \frac{16}{3} \delta^{bc} (Y_d Y_d^\dagger)^{da} \right) + 24 (Y_d Y_d^\dagger)^{bc} (Y_d Y_d^\dagger)^{da} \right. \\
& + 24 (Y_u Y_u^\dagger)^{bc} (Y_u Y_u^\dagger)^{da} - 48 (Y_d Y_d^\dagger)^{da} (Y_u Y_u^\dagger)^{bc} \Big\} C_{qq}^{(\times)abcd}, \tag{4.4}
\end{aligned}$$

### 4.3 $C_{HD}^{(\times)}$

$$\begin{aligned}
\beta_{C_{HD}^{(\times)}}^{(1)} = & -8\mathbf{T}_{\ell H} + \frac{10}{3}g_Y^2 C_{HD}^{(\parallel)} + \left\{ 4\mathbf{T}_2 + \frac{9}{2}g_L^2 + 6\lambda - \frac{5}{6}g_Y^2 \right\} C_{HD}^{(\times)} - \left\{ \frac{8}{3}\delta^{ab}g_Y^2 + 8(Y_e Y_e^\dagger)^{ba} \right\} C_{H\ell}^{(\parallel)ab} - \left\{ \frac{4}{3}\delta^{ab}g_Y^2 + 4(Y_e Y_e^\dagger)^{ba} \right\} C_{H\ell}^{(\times)ab} \\
& + \left\{ 8(Y_e^\dagger Y_e)^{ba} - \frac{8}{3}\delta^{ab}g_Y^2 \right\} C_{He}^{ab} + \left\{ \frac{8}{3}\delta^{ab}g_Y^2 - 24((Y_d Y_d^\dagger)^{ba} - (Y_u Y_u^\dagger)^{ba}) \right\} C_{Hq}^{(\parallel)ab} + \left\{ \frac{4}{3}\delta^{ab}g_Y^2 - 12((Y_d Y_d^\dagger)^{ba} - (Y_u Y_u^\dagger)^{ba}) \right\} C_{Hq}^{(\times)ab} + \left\{ \frac{16}{3}\delta^{ab}g_Y^2 \right. \\
& \left. - 24(Y_u^\dagger Y_u)^{ba} \right\} C_{Hu}^{ab} + \left\{ 24(Y_d^\dagger Y_d)^{ba} - \frac{8}{3}\delta^{ab}g_Y^2 \right\} C_{Hd}^{ab} - 12C_{Hud}^{ab}(Y_d^\dagger Y_u)^{ba} - 12C_{Hud}^{*ab}(Y_u^\dagger Y_d)^{ab}, \tag{4.5}
\end{aligned}$$

$$\begin{aligned}
\beta_{C_{HD}^{(\times)}}^{(2)} = & 4\lambda\mathbf{T}_{\ell H} + 25g_L^2\mathbf{T}_{\ell H} - \frac{17}{3}g_Y^2\mathbf{T}_{\ell H} - 32\text{Tr}[C_{\ell HH}^\dagger C_{\ell HH} Y_e Y_e^\dagger] + \left\{ \frac{5}{2}\mathbf{T}_4 - \frac{10}{3}\mathbf{T}_2 g_Y^2 - \frac{227}{18}g_Y^2 g_L^2 - 15\text{Tr}[Y_d^\dagger Y_d Y_u^\dagger Y_u] - \frac{415}{27}g_Y^4 \right. \\
& \left. - \frac{68}{3}\lambda g_Y^2 \right\} C_{HD}^{(\parallel)} + \left\{ \lambda \left( \frac{5}{2}g_Y^2 - 14\mathbf{T}_2 - \frac{45}{2}g_L^2 \right) + g_Y^2 \left( \frac{13}{6}\text{Tr}[Y_d^\dagger Y_d] + \frac{71}{6}\text{Tr}[Y_e^\dagger Y_e] + \frac{73}{6}\text{Tr}[Y_u^\dagger Y_u] \right) + g_s^2 \left( 80\text{Tr}[Y_d^\dagger Y_d] + 80\text{Tr}[Y_u^\dagger Y_u] \right) \right. \\
& + \frac{2099}{216}g_Y^4 + \frac{41}{2}g_Y^2 g_L^2 + 72\text{Tr}[Y_d^\dagger Y_d Y_u^\dagger Y_u] - 7\mathbf{T}_4 - \frac{15}{2}\mathbf{T}_2 g_L^2 - \frac{121}{8}g_L^4 - 36\lambda^2 \left. \right\} C_{HD}^{(\times)} + \left\{ \frac{32}{3}g_Y^6 + 12g_Y^4 g_L^2 - 48\lambda g_Y^4 \right\} C_{HB} \\
& + 28g_Y^2 g_L^4 C_{HW} + \left\{ 56g_Y^4 g_L^2 - g_Y^2 g_L^2 \left( 18\text{Tr}[Y_e^\dagger Y_e] + 30\text{Tr}[Y_d^\dagger Y_d] + 42\text{Tr}[Y_u^\dagger Y_u] \right) - 10g_Y^2 g_L^4 - 48\lambda g_Y^2 g_L^2 \right\} C_{HWB} + 26g_Y^2 g_L^6 C_W \\
& + \left\{ 3g_Y^2 Y_e^{*ab} - 3(Y_e^\dagger Y_e Y_e^\dagger)^{ab} \right\} C_{eH}^{ab} + C_{eH}^{*ab} \left\{ 3g_Y^2 Y_e^{ab} - 3(Y_e Y_e^\dagger Y_e)^{ab} \right\} + \left\{ 9g_Y^2 Y_u^{*ab} + 9(Y_d^\dagger Y_d Y_u^\dagger)^{ab} - 9(Y_u^\dagger Y_u Y_u^\dagger)^{ab} \right\} C_{uH}^{ab} \\
& + C_{uH}^{*ab} \left\{ 9g_Y^2 Y_u^{ab} + 9(Y_d Y_d^\dagger Y_u)^{ab} - 9(Y_u Y_u^\dagger Y_u)^{ab} \right\} + \left\{ 9g_Y^2 Y_d^{*ab} + 9(Y_u^\dagger Y_u Y_d^\dagger)^{ab} - 9(Y_d^\dagger Y_d Y_d^\dagger)^{ab} \right\} C_{dH}^{ab} + C_{dH}^{*ab} \left\{ 9g_Y^2 Y_d^{ab} + 9(Y_u Y_u^\dagger Y_d)^{ab} \right. \\
& \left. - 9(Y_d Y_d^\dagger Y_d)^{ab} \right\} + \left\{ 11g_Y^4 Y_e^{*ab} - 6g_Y^2 g_L^2 Y_e^{*ab} - 25g_Y^2 (Y_e^\dagger Y_e Y_e^\dagger)^{ab} \right\} C_{eB}^{ab} + C_{eB}^{*ab} \left\{ 11g_Y^4 Y_e^{ab} - 6g_Y^2 g_L^2 Y_e^{ab} - 25g_Y^2 (Y_e Y_e^\dagger Y_e)^{ab} \right\} \\
& + \left\{ \frac{5}{2}g_Y^2 g_L^2 Y_e^{*ab} + \frac{27}{2}g_L^2 (Y_e^\dagger Y_e Y_e^\dagger)^{ab} \right\} C_{eW}^{ab} + C_{eW}^{*ab} \left\{ \frac{5}{2}g_Y^2 g_L^2 Y_e^{ab} + \frac{27}{2}g_L^2 (Y_e Y_e^\dagger Y_e)^{ab} \right\} + \left\{ g_Y^2 \left( 9(Y_d^\dagger Y_d Y_u^\dagger)^{ab} + 51(Y_u^\dagger Y_u Y_u^\dagger)^{ab} \right) \right. \\
& + 18g_Y^2 g_L^2 Y_u^{*ab} - \frac{55}{3}g_Y^4 Y_u^{*ab} \left. \right\} C_{uB}^{ab} + C_{uB}^{*ab} \left\{ g_Y^2 \left( 9(Y_d Y_d^\dagger Y_u)^{ab} + 51(Y_u Y_u^\dagger Y_u)^{ab} \right) + 18g_Y^2 g_L^2 Y_u^{ab} - \frac{55}{3}g_Y^4 Y_u^{ab} \right\} + \left\{ g_L^2 \left( \frac{81}{2}(Y_u^\dagger Y_u Y_u^\dagger)^{ab} \right. \right. \\
& \left. \left. - \frac{81}{2}(Y_d^\dagger Y_d Y_u^\dagger)^{ab} \right) + \frac{3}{2}g_Y^2 g_L^2 Y_u^{*ab} \right\} C_{uW}^{ab} + C_{uW}^{*ab} \left\{ g_L^2 \left( \frac{81}{2}(Y_u Y_u^\dagger Y_u)^{ab} - \frac{81}{2}(Y_d Y_d^\dagger Y_u)^{ab} \right) + \frac{3}{2}g_Y^2 g_L^2 Y_u^{ab} \right\} + \left\{ g_s^2 \left( 96(Y_u^\dagger Y_u Y_u^\dagger)^{ab} - 96(Y_d^\dagger Y_d Y_u^\dagger)^{ab} \right) \right.
\end{aligned}$$

$$\begin{aligned}
& -\frac{64}{3}g_Y^2g_s^2Y_u^{*ab}\left\{C_{uG}^{ab}+C_{uG}^{*ab}\right\}g_s^2\left(96(Y_uY_u^\dagger Y_u)^{ab}-96(Y_dY_d^\dagger Y_u)^{ab}\right)-\frac{64}{3}g_Y^2g_s^2Y_u^{ab}\left\{+\frac{11}{3}g_Y^4Y_d^{*ab}-g_Y^2\left(27(Y_d^\dagger Y_d Y_d^\dagger)^{ab}+33(Y_u^\dagger Y_u Y_d^\dagger)^{ab}\right)\right. \\
& -18g_Y^2g_L^2Y_d^{*ab}\left\{C_{dB}^{ab}+C_{dB}^{*ab}\right\}\frac{11}{3}g_Y^4Y_d^{ab}-g_Y^2\left(27(Y_dY_d^\dagger Y_d)^{ab}+33(Y_uY_u^\dagger Y_d)^{ab}\right)-18g_Y^2g_L^2Y_d^{ab}\left\{+g_L^2\left(\frac{81}{2}(Y_d^\dagger Y_d Y_d^\dagger)^{ab}-\frac{81}{2}(Y_u^\dagger Y_u Y_d^\dagger)^{ab}\right)\right. \\
& -\frac{9}{2}g_Y^2g_L^2Y_d^{*ab}\left\{C_{dW}^{ab}+C_{dW}^{*ab}\right\}g_L^2\left(\frac{81}{2}(Y_dY_d^\dagger Y_d)^{ab}-\frac{81}{2}(Y_uY_u^\dagger Y_d)^{ab}\right)-\frac{9}{2}g_Y^2g_L^2Y_d^{ab}\left\{+g_s^2\left(96(Y_d^\dagger Y_d Y_d^\dagger)^{ab}-96(Y_u^\dagger Y_u Y_d^\dagger)^{ab}\right)\right. \\
& -\frac{64}{3}g_Y^2g_s^2Y_d^{*ab}\left\{C_{dG}^{ab}+C_{dG}^{*ab}\right\}g_s^2\left(96(Y_dY_d^\dagger Y_d)^{ab}-96(Y_uY_u^\dagger Y_d)^{ab}\right)-\frac{64}{3}g_Y^2g_s^2Y_d^{ab}\left\{+\lambda\left(4(Y_eY_e^\dagger)^{ba}+\frac{20}{3}\delta^{ab}g_Y^2\right)+40(Y_eY_e^\dagger Y_eY_e^\dagger)^{ba}\right. \\
& -\frac{25}{27}\delta^{ab}g_Y^4-5\delta^{ab}g_Y^2g_L^2-6g_L^2(Y_eY_e^\dagger)^{ba}-\frac{122}{9}g_Y^2(Y_eY_e^\dagger)^{ba}\left\}C_{H\ell}^{(\parallel)ab}+\left\{\lambda\left(2(Y_eY_e^\dagger)^{ba}+\frac{10}{3}\delta^{ab}g_Y^2\right)+\frac{116}{9}g_Y^2(Y_eY_e^\dagger)^{ba}+32(Y_eY_e^\dagger Y_eY_e^\dagger)^{ba}\right. \\
& -\frac{25}{54}\delta^{ab}g_Y^4-3g_L^2(Y_eY_e^\dagger)^{ba}-\frac{83}{18}\delta^{ab}g_Y^2g_L^2\left\}C_{H\ell}^{(\times)ab}+\left\{\delta^{ab}g_Y^2g_L^2+\lambda\left(\frac{20}{3}\delta^{ab}g_Y^2-4(Y_e^\dagger Y_e)^{ba}\right)+\frac{248}{9}g_Y^2(Y_e^\dagger Y_e)^{ba}-\frac{187}{27}\delta^{ab}g_Y^4\right. \\
& -18g_L^2(Y_e^\dagger Y_e)^{ba}-38(Y_e^\dagger Y_e Y_e^\dagger Y_e)^{ba}\left\}C_{He}^{ab}+\left\{\lambda\left(12(Y_dY_d^\dagger)^{ba}-\frac{20}{3}\delta^{ab}g_Y^2-12(Y_uY_u^\dagger)^{ba}\right)+g_Y^2\left(\frac{10}{3}(Y_uY_u^\dagger)^{ba}+\frac{22}{3}(Y_dY_d^\dagger)^{ba}\right)+g_L^2\left(18(Y_uY_u^\dagger)^{ba}\right.\right. \\
& -18(Y_dY_d^\dagger)^{ba})+g_s^2\left(160(Y_uY_u^\dagger)^{ba}-160(Y_dY_d^\dagger)^{ba}\right)+5\delta^{ab}g_Y^2g_L^2+\frac{32}{3}\delta^{ab}g_Y^2g_s^2+120(Y_dY_d^\dagger Y_dY_d^\dagger)^{ba}-\frac{23}{27}\delta^{ab}g_Y^4 \\
& -120(Y_uY_u^\dagger Y_uY_u^\dagger)^{ba}\left\}C_{Hq}^{(\parallel)ab}+\left\{\lambda\left(6(Y_dY_d^\dagger)^{ba}-\frac{10}{3}\delta^{ab}g_Y^2-6(Y_uY_u^\dagger)^{ba}\right)+g_L^2\left(9(Y_uY_u^\dagger)^{ba}-9(Y_dY_d^\dagger)^{ba}\right)+g_Y^2\left(\frac{32}{3}(Y_dY_d^\dagger)^{ba}+\frac{104}{3}(Y_uY_u^\dagger)^{ba}\right)\right. \\
& +g_s^2\left(80(Y_uY_u^\dagger)^{ba}-80(Y_dY_d^\dagger)^{ba}\right)+\frac{16}{3}\delta^{ab}g_Y^2g_s^2+96(Y_dY_d^\dagger Y_dY_d^\dagger)^{ba}-\frac{23}{54}\delta^{ab}g_Y^4-\frac{23}{6}\delta^{ab}g_Y^2g_L^2-24(Y_uY_u^\dagger Y_uY_u^\dagger)^{ba}-36(Y_dY_d^\dagger Y_uY_u^\dagger)^{ba} \\
& -36(Y_uY_u^\dagger Y_dY_d^\dagger)^{ba}\left\}C_{Hq}^{(\times)ab}+\left\{\lambda\left(12(Y_u^\dagger Y_u)^{ba}-\frac{40}{3}\delta^{ab}g_Y^2\right)+\frac{134}{27}\delta^{ab}g_Y^4+\frac{64}{3}\delta^{ab}g_Y^2g_s^2+54g_L^2(Y_u^\dagger Y_u)^{ba}+114(Y_u^\dagger Y_u Y_u^\dagger Y_u)^{ba}\right. \\
& -2\delta^{ab}g_Y^2g_L^2-6(Y_u^\dagger Y_d Y_d^\dagger Y_u)^{ba}-\frac{80}{3}g_Y^2(Y_u^\dagger Y_u)^{ba}-160g_s^2(Y_u^\dagger Y_u)^{ba}\left\}C_{Hu}^{ab}+\left\{\frac{5}{27}\delta^{ab}g_Y^4+\delta^{ab}g_Y^2g_L^2+\lambda\left(\frac{20}{3}\delta^{ab}g_Y^2-12(Y_d^\dagger Y_d)^{ba}\right)\right. \\
& +6(Y_d^\dagger Y_u Y_u^\dagger Y_d)^{ba}+160g_s^2(Y_d^\dagger Y_d)^{ba}-\frac{8}{3}g_Y^2(Y_d^\dagger Y_d)^{ba}-\frac{32}{3}\delta^{ab}g_Y^2g_s^2-54g_L^2(Y_d^\dagger Y_d)^{ba}-114(Y_d^\dagger Y_d Y_d^\dagger Y_d)^{ba}\left\}C_{Hd}^{ab}+\left\{6\lambda(Y_d^\dagger Y_u)^{ba}\right. \\
& +27g_L^2(Y_d^\dagger Y_u)^{ba}+27(Y_d^\dagger Y_d Y_d^\dagger Y_u)^{ba}+27(Y_d^\dagger Y_u Y_u^\dagger Y_u)^{ba}-14g_Y^2(Y_d^\dagger Y_u)^{ba}-80g_s^2(Y_d^\dagger Y_u)^{ba}\left\}C_{Hud}^{ab}+C_{Hud}^{*ab}\left\{6\lambda(Y_u^\dagger Y_d)^{ab}\right.
\end{aligned}$$



$$\begin{aligned}
& + 27g_L^2(Y_u^\dagger Y_d)^{ab} + 27(Y_u^\dagger Y_d Y_d^\dagger Y_d)^{ab} + 27(Y_u^\dagger Y_u Y_u^\dagger Y_d)^{ab} - 14g_Y^2(Y_u^\dagger Y_d)^{ab} - 80g_s^2(Y_u^\dagger Y_d)^{ab} \Big\} + \Big\{ \frac{16}{9}\delta^{ab}\delta^{cd}g_Y^4 + 16(Y_e^\dagger Y_e)^{ba}(Y_e^\dagger Y_e)^{dc} \\
& - \frac{32}{3}\delta^{ad}g_Y^2(Y_e^\dagger Y_e)^{bc} \Big\} C_{ee}^{abcd} + \Big\{ \frac{64}{27}\delta^{ad}\delta^{bc}g_Y^4 + 48(Y_u^\dagger Y_u)^{bc}(Y_u^\dagger Y_u)^{da} - \frac{64}{3}\delta^{ad}g_Y^2(Y_u^\dagger Y_u)^{bc} \Big\} C_{uu}^{abcd} + \Big\{ \frac{16}{27}\delta^{ad}\delta^{bc}g_Y^4 + 48(Y_d^\dagger Y_d)^{bc}(Y_d^\dagger Y_d)^{da} \\
& - \frac{32}{3}\delta^{ad}g_Y^2(Y_d^\dagger Y_d)^{bc} \Big\} C_{dd}^{abcd} - 48C_{ud}^{(\parallel)abcd}(Y_d^\dagger Y_u)^{da}(Y_u^\dagger Y_d)^{bc} - 144C_{ud}^{(\times)abcd}(Y_d^\dagger Y_u)^{da}(Y_u^\dagger Y_d)^{bc} + \Big\{ \frac{8}{9}\delta^{ad}\delta^{bc}g_Y^4 + \frac{16}{3}\delta^{bc}g_Y^2(Y_e Y_e^\dagger)^{da} \\
& + 8(Y_e Y_e^\dagger)^{bc}(Y_e Y_e^\dagger)^{da} \Big\} C_{\ell\ell}^{abcd} + \Big\{ \frac{8}{27}\delta^{ad}\delta^{bc}g_Y^4 + g_Y^2\left(\frac{16}{3}\delta^{bc}(Y_u Y_u^\dagger)^{da} - \frac{16}{3}\delta^{bc}(Y_d Y_d^\dagger)^{da}\right) + 24(Y_d Y_d^\dagger)^{bc}(Y_d Y_d^\dagger)^{da} + 24(Y_u Y_u^\dagger)^{bc}(Y_u Y_u^\dagger)^{da} \\
& - 48(Y_d Y_d^\dagger)^{da}(Y_u Y_u^\dagger)^{bc} \Big\} C_{qq}^{(\parallel)abcd} + \Big\{ \frac{16}{27}\delta^{ad}\delta^{bc}g_Y^4 + g_Y^2\left(\frac{32}{3}\delta^{bc}(Y_u Y_u^\dagger)^{da} - \frac{32}{3}\delta^{bc}(Y_d Y_d^\dagger)^{da}\right) + 48(Y_d Y_d^\dagger)^{bc}(Y_d Y_d^\dagger)^{da} + 48(Y_u Y_u^\dagger)^{bc}(Y_u Y_u^\dagger)^{da} \\
& - 96(Y_d Y_d^\dagger)^{da}(Y_u Y_u^\dagger)^{bc} \Big\} C_{qq}^{(\times)abcd}, \tag{4.6}
\end{aligned}$$

## 5 $X^2 H^2$

### 5.1 $C_{HB}$

$$\begin{aligned}
\beta_{CHB}^{(1)} &= \left\{ \frac{1}{2}g_Y^2 + 2T_2 + 6\lambda - \frac{9}{2}g_L^2 \right\} C_{HB} + \frac{3}{2}g_L^2 C_{HWB} - 3Y_e^{*ab} C_{eB}^{ab} - 3C_{eB}^{*ab} Y_e^{ab} + 5Y_u^{*ab} C_{uB}^{ab} + 5C_{uB}^{*ab} Y_u^{ab} - Y_d^{*ab} C_{dB}^{ab} - C_{dB}^{*ab} Y_d^{ab}, \tag{5.1} \\
\beta_{CHB}^{(2)} &= T_{\ell H} + \left\{ \frac{5}{12} \text{Tr}[Y_d^\dagger Y_d] + \frac{5}{4} \text{Tr}[Y_e^\dagger Y_e] + \frac{4}{3}g_L^2 + \frac{17}{12} \text{Tr}[Y_u^\dagger Y_u] - \frac{1}{18}g_Y^2 - \lambda \right\} C_{HD}^{(\parallel)} + \left\{ \frac{5}{24} \text{Tr}[Y_d^\dagger Y_d] + \frac{5}{8} \text{Tr}[Y_e^\dagger Y_e] + \frac{23}{36}g_Y^2 + \frac{17}{24} \text{Tr}[Y_u^\dagger Y_u] \right. \\
& - \left. \frac{3}{4}g_L^2 - \lambda \right\} C_{HD}^{(\times)} + \left\{ \lambda(36g_L^2 - 12T_2) + g_s^2(40 \text{Tr}[Y_d^\dagger Y_d] + 40 \text{Tr}[Y_u^\dagger Y_u]) + \frac{15}{4}T_2g_L^2 + \frac{51}{8}g_Y^2g_L^2 + \frac{1505}{48}g_Y^4 - g_Y^2\left(\frac{5}{4} \text{Tr}[Y_e^\dagger Y_e] \right. \right. \\
& + \left. \left. \frac{73}{12} \text{Tr}[Y_u^\dagger Y_u] + \frac{85}{12} \text{Tr}[Y_d^\dagger Y_d] \right) - \frac{9}{2}T_4 - \frac{145}{16}g_L^4 - 15\lambda^2 - 21 \text{Tr}[Y_d^\dagger Y_d Y_u^\dagger Y_u] \right\} C_{HB} + \frac{33}{4}g_L^4 C_{HW} + \frac{88}{3}g_s^4 C_{HG} + \left\{ \frac{3}{4}g_Y^2g_L^2 \right. \\
& + \left. \frac{113}{12}g_L^4 - g_L^2\left(\frac{9}{8} \text{Tr}[Y_e^\dagger Y_e] + \frac{39}{8} \text{Tr}[Y_u^\dagger Y_u] + \frac{51}{8} \text{Tr}[Y_d^\dagger Y_d] \right) - \frac{9}{2}\lambda g_L^2 \right\} C_{HWB} - \frac{45}{8}g_L^6 C_W + \frac{15}{8}Y_e^{*ab} C_{eH}^{ab} + \frac{15}{8}C_{eH}^{*ab} Y_e^{ab} + \frac{17}{8}Y_u^{*ab} C_{uH}^{ab} \\
& + \frac{17}{8}C_{uH}^{*ab} Y_u^{ab} + \frac{5}{8}Y_d^{*ab} C_{dH}^{ab} + \frac{5}{8}C_{dH}^{*ab} Y_d^{ab} + \left\{ \frac{43}{2}(Y_e^\dagger Y_e Y_e^\dagger)^{ab} - \frac{3}{4}g_L^2 Y_e^{*ab} - \frac{9}{2}\lambda Y_e^{*ab} - 12g_Y^2 Y_e^{*ab} \right\} C_{eB}^{ab} + C_{eB}^{*ab} \left\{ \frac{43}{2}(Y_e Y_e^\dagger Y_e)^{ab} \right.
\end{aligned}$$

$$\begin{aligned}
& -\frac{3}{4}g_L^2 Y_e^{ab} - \frac{9}{2}\lambda Y_e^{ab} - 12g_Y^2 Y_e^{ab} \Big\} - \frac{15}{8}g_L^2 Y_e^{*ab} C_{eW}^{ab} - \frac{15}{8}g_L^2 C_{eW}^{*ab} Y_e^{ab} + \left\{ \frac{15}{2}\lambda Y_u^{*ab} + \frac{25}{3}g_Y^2 Y_u^{*ab} + \frac{25}{2}(Y_d^\dagger Y_d Y_u^\dagger)^{ab} + \frac{140}{3}g_s^2 Y_u^{*ab} \right. \\
& - \frac{3}{4}g_L^2 Y_u^{*ab} - \frac{69}{2}(Y_u^\dagger Y_u Y_u^\dagger)^{ab} \Big\} C_{uB}^{ab} + C_{uB}^{*ab} \left\{ \frac{15}{2}\lambda Y_u^{ab} + \frac{25}{3}g_Y^2 Y_u^{ab} + \frac{25}{2}(Y_d Y_d^\dagger Y_u)^{ab} + \frac{140}{3}g_s^2 Y_u^{ab} - \frac{3}{4}g_L^2 Y_u^{ab} - \frac{69}{2}(Y_u Y_u^\dagger Y_u)^{ab} \right\} \\
& - \frac{19}{8}g_L^2 Y_u^{*ab} C_{uW}^{ab} - \frac{19}{8}g_L^2 C_{uW}^{*ab} Y_u^{ab} - \frac{16}{9}g_s^2 Y_u^{*ab} C_{uG}^{ab} - \frac{16}{9}g_s^2 C_{uG}^{*ab} Y_u^{ab} + \left\{ \frac{15}{4}g_L^2 Y_d^{*ab} + \frac{9}{2}(Y_d^\dagger Y_d Y_d^\dagger)^{ab} - \frac{2}{3}g_Y^2 Y_d^{*ab} - \frac{3}{2}\lambda Y_d^{*ab} \right. \\
& - \frac{17}{2}(Y_u^\dagger Y_u Y_d^\dagger)^{ab} - \frac{28}{3}g_s^2 Y_d^{*ab} \Big\} C_{dB}^{ab} + C_{dB}^{*ab} \left\{ \frac{15}{4}g_L^2 Y_d^{ab} + \frac{9}{2}(Y_d Y_d^\dagger Y_d)^{ab} - \frac{2}{3}g_Y^2 Y_d^{ab} - \frac{3}{2}\lambda Y_d^{ab} - \frac{17}{2}(Y_u Y_u^\dagger Y_d)^{ab} - \frac{28}{3}g_s^2 Y_d^{ab} \right\} \\
& - \frac{1}{8}g_L^2 Y_d^{*ab} C_{dW}^{ab} - \frac{1}{8}g_L^2 C_{dW}^{*ab} Y_d^{ab} + \frac{8}{9}g_s^2 Y_d^{*ab} C_{dG}^{ab} + \frac{8}{9}g_s^2 C_{dG}^{*ab} Y_d^{ab} - \left\{ \frac{5}{12}(Y_e Y_e^\dagger)^{ba} + \frac{19}{18}\delta^{ab}g_Y^2 \right\} C_{H\ell}^{(\parallel)ab} + \left\{ \frac{19}{12}\delta^{ab}g_L^2 - \frac{19}{36}\delta^{ab}g_Y^2 \right. \\
& - \frac{5}{6}(Y_e Y_e^\dagger)^{ba} \Big\} C_{H\ell}^{(\times)ab} + \left\{ \frac{41}{12}(Y_e^\dagger Y_e)^{ba} - \frac{23}{9}\delta^{ab}g_Y^2 \right\} C_{He}^{ab} + \left\{ \frac{11}{18}\delta^{ab}g_Y^2 + \frac{11}{12}(Y_u Y_u^\dagger)^{ba} - \frac{23}{12}(Y_d Y_d^\dagger)^{ba} \right\} C_{Hq}^{(\parallel)ab} + \left\{ \frac{11}{36}\delta^{ab}g_Y^2 + \frac{11}{4}\delta^{ab}g_L^2 \right. \\
& - \frac{11}{12}(Y_u Y_u^\dagger)^{ba} - \frac{23}{6}(Y_d Y_d^\dagger)^{ba} \Big\} C_{Hq}^{(\times)ab} + \left\{ \frac{26}{9}\delta^{ab}g_Y^2 - \frac{71}{12}(Y_u^\dagger Y_u)^{ba} \right\} C_{Hu}^{ab} + \left\{ \frac{35}{12}(Y_d^\dagger Y_d)^{ba} - \frac{7}{9}\delta^{ab}g_Y^2 \right\} C_{Hd}^{ab} - \frac{19}{12}C_{Hud}^{ab}(Y_d^\dagger Y_u)^{ba} \\
& - \frac{19}{12}C_{Hud}^{*ab}(Y_u^\dagger Y_d)^{ab} - \frac{9}{2}Y_e^{*ad}C_{\ell e}^{abcd}Y_e^{bc} - \frac{25}{6}Y_u^{*ad}C_{qu}^{(\parallel)abcd}Y_u^{bc} - \frac{25}{2}Y_u^{*ad}C_{qu}^{(\times)abcd}Y_u^{bc} - \frac{1}{6}Y_d^{*ad}C_{qd}^{(\parallel)abcd}Y_d^{bc} - \frac{1}{2}Y_d^{*ad}C_{qd}^{(\times)abcd}Y_d^{bc}, \tag{5.2}
\end{aligned}$$

## 5.2 $C_{H\tilde{B}}$

$$\beta_{C_{H\tilde{B}}}^{(1)} = \left\{ \frac{1}{2}g_Y^2 + 2T_2 + 6\lambda - \frac{9}{2}g_L^2 \right\} C_{H\tilde{B}} + \frac{3}{2}g_L^2 C_{H\tilde{W}B} - 3iY_e^{*ab}C_{eB}^{ab} + 3iC_{eB}^{*ab}Y_e^{ab} + 5iY_u^{*ab}C_{uB}^{ab} - 5iC_{uB}^{*ab}Y_u^{ab} - iY_d^{*ab}C_{dB}^{ab} + iC_{dB}^{*ab}Y_d^{ab}, \tag{5.3}$$

$$\begin{aligned}
\beta_{C_{H\tilde{B}}}^{(2)} = & \left\{ \lambda(36g_L^2 - 12T_2) + g_s^2(40\text{Tr}[Y_d^\dagger Y_d] + 40\text{Tr}[Y_u^\dagger Y_u]) + \frac{15}{4}T_2g_L^2 + \frac{51}{8}g_Y^2g_L^2 + \frac{5891}{144}g_Y^4 - g_Y^2\left(\frac{5}{4}\text{Tr}[Y_e^\dagger Y_e] + \frac{73}{12}\text{Tr}[Y_u^\dagger Y_u] \right. \right. \\
& + \frac{85}{12}\text{Tr}[Y_d^\dagger Y_d]) - \frac{9}{2}T_4 - \frac{145}{16}g_L^4 - 15\lambda^2 - 21\text{Tr}[Y_d^\dagger Y_d Y_u^\dagger Y_u] \Big\} C_{H\tilde{B}} + \frac{33}{4}g_L^4 C_{H\tilde{W}} + 44g_s^4 C_{HG} + \left\{ \frac{3}{4}g_Y^2g_L^2 + \frac{113}{12}g_L^4 \right. \\
& - g_L^2\left(\frac{9}{8}\text{Tr}[Y_e^\dagger Y_e] + \frac{39}{8}\text{Tr}[Y_u^\dagger Y_u] + \frac{51}{8}\text{Tr}[Y_d^\dagger Y_d]\right) - \frac{9}{2}\lambda g_L^2 \Big\} C_{H\tilde{W}B} - \frac{21}{8}g_L^6 C_{\tilde{W}} - \frac{15i}{16}Y_e^{*ab}C_{eH}^{ab} + \frac{15i}{16}C_{eH}^{*ab}Y_e^{ab} - \frac{17i}{16}Y_u^{*ab}C_{uH}^{ab} \\
& + \frac{17i}{16}C_{uH}^{*ab}Y_u^{ab} - \frac{5i}{16}Y_d^{*ab}C_{dH}^{ab} + \frac{5i}{16}C_{dH}^{*ab}Y_d^{ab} + \left\{ \frac{25i}{2}(Y_e^\dagger Y_e Y_e^\dagger)^{ab} - \frac{i}{4}g_Y^2 Y_e^{*ab} - \frac{3i}{4}g_L^2 Y_e^{*ab} - \frac{9i}{2}\lambda Y_e^{*ab} \right\} C_{eB}^{ab} + C_{eB}^{*ab} \left\{ \frac{i}{4}g_Y^2 Y_e^{ab} \right.
\end{aligned}$$

$$\begin{aligned}
& + \frac{3i}{4}g_L^2 Y_e^{ab} + \frac{9i}{2}\lambda Y_e^{ab} - \frac{25i}{2}(Y_e Y_e^\dagger Y_e)^{ab} \Big\} - \frac{91i}{16}g_L^2 Y_e^{*ab} C_{eW}^{ab} + \frac{91i}{16}g_L^2 C_{eW}^{*ab} Y_e^{ab} + \left\{ \frac{107i}{16}g_Y^2 Y_u^{*ab} + \frac{15i}{2}\lambda Y_u^{*ab} \right. \\
& + \frac{23i}{2}(Y_d^\dagger Y_d Y_u^\dagger)^{ab} + \frac{140i}{3}g_s^2 Y_u^{*ab} - \frac{3i}{4}g_L^2 Y_u^{*ab} - \frac{39i}{2}(Y_u^\dagger Y_u Y_u^\dagger)^{ab} \Big\} C_{uB}^{ab} + C_{uB}^{*ab} \left\{ \frac{3i}{4}g_L^2 Y_u^{ab} + \frac{39i}{2}(Y_u Y_u^\dagger Y_u)^{ab} - \frac{107i}{16}g_Y^2 Y_u^{ab} \right. \\
& - \frac{15i}{2}\lambda Y_u^{ab} - \frac{23i}{2}(Y_d Y_d^\dagger Y_u)^{ab} - \frac{140i}{3}g_s^2 Y_u^{ab} \Big\} - \frac{193i}{32}g_L^2 Y_u^{*ab} C_{uW}^{ab} + \frac{193i}{32}g_L^2 C_{uW}^{*ab} Y_u^{ab} - \frac{179i}{18}g_s^2 Y_u^{*ab} C_{uG}^{ab} \\
& + \frac{179i}{18}g_s^2 C_{uG}^{*ab} Y_u^{ab} + \left\{ \frac{3i}{2}(Y_d^\dagger Y_d Y_d^\dagger)^{ab} + \frac{15i}{4}g_L^2 Y_d^{*ab} - \frac{3i}{2}\lambda Y_d^{*ab} - \frac{7i}{2}(Y_u^\dagger Y_u Y_d^\dagger)^{ab} - \frac{28i}{3}g_s^2 Y_d^{*ab} \right\} C_{dB}^{ab} + C_{dB}^{*ab} \left\{ \frac{3i}{2}\lambda Y_d^{ab} \right. \\
& + \frac{7i}{2}(Y_u Y_u^\dagger Y_d)^{ab} + \frac{28i}{3}g_s^2 Y_d^{ab} - \frac{3i}{2}(Y_d Y_d^\dagger Y_d)^{ab} - \frac{15i}{4}g_L^2 Y_d^{ab} \Big\} - \frac{17i}{16}g_L^2 Y_d^{*ab} C_{dW}^{ab} + \frac{17i}{16}g_L^2 C_{dW}^{*ab} Y_d^{ab} - \frac{77i}{18}g_s^2 Y_d^{*ab} C_{dG}^{ab} \\
& + \frac{77i}{18}g_s^2 C_{dG}^{*ab} Y_d^{ab} + \frac{55i}{48}C_{Hud}^{ab} (Y_d^\dagger Y_u)^{ba} - \frac{55i}{48}C_{Hud}^{*ab} (Y_u^\dagger Y_d)^{ab}, \tag{5.4}
\end{aligned}$$

### 5.3 $C_{HW}$

$$\begin{aligned}
\beta_{C_{HW}}^{(1)} = & \left\{ 2T_2 + 6\lambda - \frac{3}{2}g_Y^2 - \frac{5}{2}g_L^2 \right\} C_{HW} + \frac{1}{2}g_Y^2 C_{HWB} + 15g_L^4 C_W + \frac{1}{2}Y_e^{*ab} C_{eW}^{ab} + \frac{1}{2}C_{eW}^{*ab} Y_e^{ab} + \frac{3}{2}Y_u^{*ab} C_{uW}^{ab} + \frac{3}{2}C_{uW}^{*ab} Y_u^{ab} + \frac{3}{2}Y_d^{*ab} C_{dW}^{ab} \\
& + \frac{3}{2}C_{dW}^{*ab} Y_d^{ab}, \tag{5.5}
\end{aligned}$$

$$\begin{aligned}
\beta_{C_{HW}}^{(2)} = & -T_{\ell H} + \left\{ \frac{1}{4}T_2 + \frac{4}{9}g_Y^2 + \frac{1}{2}g_L^2 - \lambda \right\} C_{HD}^{(\parallel)} + \left\{ \frac{1}{8}T_2 + \frac{7}{18}g_Y^2 \right\} C_{HD}^{(\times)} + \frac{11}{4}g_Y^4 C_{HB} + \left\{ \frac{1}{4}T_2 g_L^2 + \lambda(12g_Y^2 + 24g_L^2 - 12T_2) \right. \\
& + g_Y^2 \left( \frac{25}{12} \text{Tr}[Y_d^\dagger Y_d] + \frac{25}{4} \text{Tr}[Y_e^\dagger Y_e] + \frac{85}{12} \text{Tr}[Y_u^\dagger Y_u] \right) + g_s^2 \left( 40 \text{Tr}[Y_d^\dagger Y_d] + 40 \text{Tr}[Y_u^\dagger Y_u] \right) + \frac{27}{8}g_Y^2 g_L^2 + \frac{557}{48}g_Y^4 + \frac{4811}{144}g_L^4 - \frac{9}{2}T_4 - 15\lambda^2 \\
& \left. - 21 \text{Tr}[Y_d^\dagger Y_d Y_u^\dagger Y_u] \right\} C_{HW} + 24g_s^4 C_{HG} + \left\{ 5g_Y^2 g_L^2 - \frac{19}{36}g_Y^4 - g_Y^2 \left( \frac{3}{8} \text{Tr}[Y_e^\dagger Y_e] + \frac{13}{8} \text{Tr}[Y_u^\dagger Y_u] + \frac{17}{8} \text{Tr}[Y_d^\dagger Y_d] \right) - \frac{3}{2}\lambda g_Y^2 \right\} C_{HWB} \\
& + \left\{ \frac{171}{2}\lambda g_L^4 + \frac{515}{6}g_L^6 - \frac{3}{2}T_2 g_L^4 - \frac{177}{8}g_Y^2 g_L^4 \right\} C_W + \frac{3}{8}Y_e^{*ab} C_{eH}^{ab} + \frac{3}{8}C_{eH}^{*ab} Y_e^{ab} + \frac{9}{8}Y_u^{*ab} C_{uH}^{ab} + \frac{9}{8}C_{uH}^{*ab} Y_u^{ab} + \frac{9}{8}Y_d^{*ab} C_{dH}^{ab} + \frac{9}{8}C_{dH}^{*ab} Y_d^{ab} \\
& + \frac{1}{4}g_Y^2 Y_e^{*ab} C_{eB}^{ab} + \frac{1}{4}g_Y^2 C_{eB}^{*ab} Y_e^{ab} + \left\{ \frac{3}{4}\lambda Y_e^{*ab} + \frac{9}{8}g_Y^2 Y_e^{*ab} + 6g_L^2 Y_e^{*ab} - \frac{5}{2}(Y_e^\dagger Y_e Y_e^\dagger)^{ab} \right\} C_{eW}^{ab} + C_{eW}^{*ab} \left\{ \frac{3}{4}\lambda Y_e^{ab} + \frac{9}{8}g_Y^2 Y_e^{ab} + 6g_L^2 Y_e^{ab} \right.
\end{aligned}$$

$$\begin{aligned}
& -\frac{5}{2}(Y_e Y_e^\dagger Y_e)^{ab} \Bigg\} - \frac{3}{4}g_Y^2 Y_u^{*ab} C_{uB}^{ab} - \frac{3}{4}g_Y^2 C_{uB}^{*ab} Y_u^{ab} + \left\{ \frac{7}{24}g_Y^2 Y_u^{*ab} + \frac{9}{4}\lambda Y_u^{*ab} + 3(Y_d^\dagger Y_d Y_u^\dagger)^{ab} + 14g_s^2 Y_u^{*ab} + 18g_L^2 Y_u^{*ab} \right. \\
& - \frac{15}{2}(Y_u^\dagger Y_u Y_u^\dagger)^{ab} \Bigg\} C_{uW}^{ab} + C_{uW}^{*ab} \left\{ \frac{7}{24}g_Y^2 Y_u^{ab} + \frac{9}{4}\lambda Y_u^{ab} + 3(Y_d Y_d^\dagger Y_u)^{ab} + 14g_s^2 Y_u^{ab} + 18g_L^2 Y_u^{ab} - \frac{15}{2}(Y_u Y_u^\dagger Y_u)^{ab} \right\} + \frac{3}{4}g_Y^2 Y_d^{*ab} C_{dB}^{ab} \\
& + \frac{3}{4}g_Y^2 C_{dB}^{*ab} Y_d^{ab} + \left\{ \frac{9}{4}\lambda Y_d^{*ab} + 3(Y_u^\dagger Y_u Y_d^\dagger)^{ab} + 14g_s^2 Y_d^{*ab} + 18g_L^2 Y_d^{*ab} - \frac{11}{24}g_Y^2 Y_d^{*ab} - \frac{15}{2}(Y_d^\dagger Y_d Y_d^\dagger)^{ab} \right\} C_{dW}^{ab} + C_{dW}^{*ab} \left\{ \frac{9}{4}\lambda Y_d^{ab} \right. \\
& + 3(Y_u Y_u^\dagger Y_d)^{ab} + 14g_s^2 Y_d^{ab} + 18g_L^2 Y_d^{ab} - \frac{11}{24}g_Y^2 Y_d^{ab} - \frac{15}{2}(Y_d Y_d^\dagger Y_d)^{ab} \Bigg\} - \left\{ \frac{19}{18}\delta^{ab}g_Y^2 + \frac{17}{12}(Y_e Y_e^\dagger)^{ba} \right\} C_{H\ell}^{(\parallel)ab} + \left\{ \frac{9}{4}\delta^{ab}g_L^2 - \frac{19}{36}\delta^{ab}g_Y^2 \right. \\
& - \frac{5}{6}(Y_e Y_e^\dagger)^{ba} \Bigg\} C_{H\ell}^{(\times)ab} + \left\{ \frac{5}{12}(Y_e^\dagger Y_e)^{ba} - \frac{5}{9}\delta^{ab}g_Y^2 \right\} C_{He}^{ab} + \left\{ \frac{19}{18}\delta^{ab}g_Y^2 + \frac{17}{4}(Y_u Y_u^\dagger)^{ba} - \frac{17}{4}(Y_d Y_d^\dagger)^{ba} \right\} C_{Hq}^{(\parallel)ab} + \left\{ \frac{19}{36}\delta^{ab}g_Y^2 + \frac{7}{4}(Y_u Y_u^\dagger)^{ba} \right. \\
& + \frac{27}{4}\delta^{ab}g_L^2 - \frac{5}{2}(Y_d Y_d^\dagger)^{ba} \Bigg\} C_{Hq}^{(\times)ab} + \left\{ \frac{10}{9}\delta^{ab}g_Y^2 - \frac{5}{4}(Y_u^\dagger Y_u)^{ba} \right\} C_{Hu}^{ab} + \left\{ \frac{5}{4}(Y_d^\dagger Y_d)^{ba} - \frac{5}{9}\delta^{ab}g_Y^2 \right\} C_{Hd}^{ab} + \frac{5}{4}C_{Hud}^{ab}(Y_d^\dagger Y_u)^{ba} + \frac{5}{4}C_{Hud}^{*ab}(Y_u^\dagger Y_d)^{ab} \\
& - \frac{1}{2}Y_e^{*ad} C_{\ell e}^{abcd} Y_e^{bc} - \frac{3}{2}Y_u^{*ad} C_{qu}^{(\parallel)abcd} Y_u^{bc} - \frac{9}{2}Y_u^{*ad} C_{qu}^{(\times)abcd} Y_u^{bc} - \frac{3}{2}Y_d^{*ad} C_{qd}^{(\parallel)abcd} Y_d^{bc} - \frac{9}{2}Y_d^{*ad} C_{qd}^{(\times)abcd} Y_d^{bc}, \tag{5.6}
\end{aligned}$$

#### 5.4 $C_{H\widetilde{W}}$

$$\begin{aligned}
\beta_{C_{H\widetilde{W}}}^{(1)} &= \left\{ 2T_2 + 6\lambda - \frac{3}{2}g_Y^2 - \frac{5}{2}g_L^2 \right\} C_{H\widetilde{W}} + \frac{1}{2}g_Y^2 C_{H\widetilde{W}B} + 15g_L^4 C_{\widetilde{W}} + \frac{i}{2}Y_e^{*ab} C_{eW}^{ab} - \frac{i}{2}C_{eW}^{*ab} Y_e^{ab} + \frac{3i}{2}Y_u^{*ab} C_{uW}^{ab} - \frac{3i}{2}C_{uW}^{*ab} Y_u^{ab} + \frac{3i}{2}Y_d^{*ab} C_{dW}^{ab} \\
& - \frac{3i}{2}C_{dW}^{*ab} Y_d^{ab}, \tag{5.7}
\end{aligned}$$

$$\begin{aligned}
\beta_{C_{H\widetilde{W}}}^{(2)} &= \frac{11}{4}g_Y^4 C_{HB} + \left\{ \frac{1}{4}T_2 g_L^2 + \lambda(12g_Y^2 + 24g_L^2 - 12T_2) + g_Y^2 \left( \frac{25}{12} \text{Tr}[Y_d^\dagger Y_d] + \frac{25}{4} \text{Tr}[Y_e^\dagger Y_e] + \frac{85}{12} \text{Tr}[Y_u^\dagger Y_u] \right) + g_s^2(40 \text{Tr}[Y_d^\dagger Y_d] \right. \\
& + 40 \text{Tr}[Y_u^\dagger Y_u]) + \frac{27}{8}g_Y^2 g_L^2 + \frac{557}{48}g_Y^4 + \frac{7019}{144}g_L^4 - \frac{9}{2}T_4 - 15\lambda^2 - 21 \text{Tr}[Y_d^\dagger Y_d Y_u^\dagger Y_u] \Bigg\} C_{H\widetilde{W}} + 36g_s^4 C_{H\widetilde{G}} + \left\{ g_Y^2 g_L^2 - \frac{19}{36}g_Y^4 \right. \\
& - g_Y^2 \left( \frac{3}{8} \text{Tr}[Y_e^\dagger Y_e] + \frac{13}{8} \text{Tr}[Y_u^\dagger Y_u] + \frac{17}{8} \text{Tr}[Y_d^\dagger Y_d] \right) - \frac{3}{2}\lambda g_Y^2 \Bigg\} C_{H\widetilde{W}B} + \left\{ 55g_L^6 + \frac{111}{2}\lambda g_L^4 - \frac{65}{6}T_2 g_L^4 - \frac{109}{8}g_Y^2 g_L^4 \right\} C_{\widetilde{W}} - \frac{3i}{16}Y_e^{*ab} C_{eH}^{ab} \\
& + \frac{3i}{16}C_{eH}^{*ab} Y_e^{ab} - \frac{9i}{16}Y_u^{*ab} C_{uH}^{ab} + \frac{9i}{16}C_{uH}^{*ab} Y_u^{ab} - \frac{9i}{16}Y_d^{*ab} C_{dH}^{ab} + \frac{9i}{16}C_{dH}^{*ab} Y_d^{ab} + ig_Y^2 Y_e^{*ab} C_{eB}^{ab} - ig_Y^2 C_{eB}^{*ab} Y_e^{ab} + \left\{ \frac{3i}{4}\lambda Y_e^{*ab} \right.
\end{aligned}$$

$$\begin{aligned}
& + \frac{9i}{8} g_Y^2 Y_e^{*ab} + \frac{47i}{16} g_L^2 Y_e^{*ab} - 2i (Y_e^\dagger Y_e Y_e^\dagger)^{ab} \Big\} C_{eW}^{ab} + C_{eW}^{*ab} \Big\{ 2i (Y_e Y_e^\dagger Y_e)^{ab} - \frac{3i}{4} \lambda Y_e^{ab} - \frac{9i}{8} g_Y^2 Y_e^{ab} - \frac{47i}{16} g_L^2 Y_e^{ab} \Big\} \\
& - \frac{187i}{48} g_Y^2 Y_u^{*ab} C_{uB}^{ab} + \frac{187i}{48} g_Y^2 C_{uB}^{*ab} Y_u^{ab} + \Big\{ \frac{7i}{24} g_Y^2 Y_u^{*ab} + \frac{9i}{4} \lambda Y_u^{*ab} + \frac{9i}{2} (Y_d^\dagger Y_d Y_u^\dagger)^{ab} + \frac{147i}{32} g_L^2 Y_u^{*ab} + 14i g_s^2 Y_u^{*ab} \\
& - 6i (Y_u^\dagger Y_u Y_u^\dagger)^{ab} \Big\} C_{uW}^{ab} + C_{uW}^{*ab} \Big\{ 6i (Y_u Y_u^\dagger Y_u)^{ab} - \frac{7i}{24} g_Y^2 Y_u^{ab} - \frac{9i}{4} \lambda Y_u^{ab} - \frac{9i}{2} (Y_d Y_d^\dagger Y_u)^{ab} - \frac{147i}{32} g_L^2 Y_u^{ab} - 14i g_s^2 Y_u^{ab} \Big\} - \frac{73i}{6} g_s^2 Y_u^{*ab} C_{uG}^{ab} \\
& + \frac{73i}{6} g_s^2 C_{uG}^{*ab} Y_u^{ab} + \frac{17i}{12} g_Y^2 Y_d^{*ab} C_{dB}^{ab} - \frac{17i}{12} g_Y^2 C_{dB}^{*ab} Y_d^{ab} + \Big\{ \frac{9i}{4} \lambda Y_d^{*ab} + \frac{9i}{2} (Y_u^\dagger Y_u Y_d^\dagger)^{ab} + \frac{141i}{16} g_L^2 Y_d^{*ab} + 14i g_s^2 Y_d^{*ab} \\
& - \frac{11i}{24} g_Y^2 Y_d^{*ab} - 6i (Y_d^\dagger Y_d Y_d^\dagger)^{ab} \Big\} C_{dW}^{ab} + C_{dW}^{*ab} \Big\{ \frac{11i}{24} g_Y^2 Y_d^{ab} + 6i (Y_d Y_d^\dagger Y_d)^{ab} - \frac{9i}{4} \lambda Y_d^{ab} - \frac{9i}{2} (Y_u Y_u^\dagger Y_d)^{ab} - \frac{141i}{16} g_L^2 Y_d^{ab} - 14i g_s^2 Y_d^{ab} \Big\} \\
& - \frac{19i}{6} g_s^2 Y_d^{*ab} C_{dG}^{ab} + \frac{19i}{6} g_s^2 C_{dG}^{*ab} Y_d^{ab} - \frac{15i}{16} C_{Hud}^{ab} (Y_d^\dagger Y_u)^{ba} + \frac{15i}{16} C_{Hud}^{*ab} (Y_u^\dagger Y_d)^{ab}, \tag{5.8}
\end{aligned}$$

## 5.5 $C_{HG}$

$$\beta_{C_{HG}}^{(1)} = \left\{ 2T_2 + 6\lambda - \frac{3}{2} g_Y^2 - \frac{9}{2} g_L^2 \right\} C_{HG} + 2Y_u^{*ab} C_{uG}^{ab} + 2C_{uG}^{*ab} Y_u^{ab} + 2Y_d^{*ab} C_{dG}^{ab} + 2C_{dG}^{*ab} Y_d^{ab}, \tag{5.9}$$

$$\begin{aligned}
\beta_{C_{HG}}^{(2)} = & \left\{ \text{Tr}[Y_d^\dagger Y_d] + \text{Tr}[Y_u^\dagger Y_u] \right\} C_{HD}^{(\parallel)} + \left\{ \frac{1}{2} \text{Tr}[Y_d^\dagger Y_d] + \frac{1}{2} \text{Tr}[Y_u^\dagger Y_u] \right\} C_{HD}^{(\times)} + \frac{11}{3} g_Y^4 C_{HB} + 9g_L^4 C_{HW} + \left\{ \lambda (12g_Y^2 + 36g_L^2 - 12T_2) \right. \\
& + g_Y^2 \left( \frac{25}{12} \text{Tr}[Y_d^\dagger Y_d] + \frac{25}{4} \text{Tr}[Y_e^\dagger Y_e] + \frac{85}{12} \text{Tr}[Y_u^\dagger Y_u] \right) + g_s^2 (36 \text{Tr}[Y_d^\dagger Y_d] + 36 \text{Tr}[Y_u^\dagger Y_u]) + \frac{15}{8} g_Y^2 g_L^2 + \frac{15}{4} T_2 g_L^2 + \frac{557}{48} g_Y^4 - \frac{9}{2} T_4 \\
& - \frac{145}{16} g_L^4 - 15\lambda^2 - 21 \text{Tr}[Y_d^\dagger Y_d Y_u^\dagger Y_u] - 52g_s^4 \Big\} C_{HG} - g_s^4 \left\{ 207 \text{Tr}[Y_d^\dagger Y_d] + 207 \text{Tr}[Y_u^\dagger Y_u] \right\} C_G + \frac{3}{2} Y_u^{*ab} C_{uH}^{ab} + \frac{3}{2} C_{uH}^{*ab} Y_u^{ab} \\
& + \frac{3}{2} Y_d^{*ab} C_{dH}^{ab} + \frac{3}{2} C_{dH}^{*ab} Y_d^{ab} - \frac{5}{6} g_Y^2 Y_u^{*ab} C_{uB}^{ab} - \frac{5}{6} g_Y^2 C_{uB}^{*ab} Y_u^{ab} - \frac{3}{4} g_L^2 Y_u^{*ab} C_{uW}^{ab} - \frac{3}{4} g_L^2 C_{uW}^{*ab} Y_u^{ab} + \left\{ \frac{3}{2} g_L^2 Y_u^{*ab} + 2(Y_d^\dagger Y_d Y_u^\dagger)^{ab} + \frac{37}{18} g_Y^2 Y_u^{*ab} \right. \\
& + 3\lambda Y_u^{*ab} + 46g_s^2 Y_u^{*ab} - 15(Y_u^\dagger Y_u Y_u^\dagger)^{ab} \Big\} C_{uG}^{ab} + C_{uG}^{*ab} \left\{ \frac{3}{2} g_L^2 Y_u^{ab} + 2(Y_d Y_d^\dagger Y_u)^{ab} + \frac{37}{18} g_Y^2 Y_u^{ab} + 3\lambda Y_u^{ab} + 46g_s^2 Y_u^{ab} - 15(Y_u Y_u^\dagger Y_u)^{ab} \right\} \\
& + \frac{1}{6} g_Y^2 Y_d^{*ab} C_{dB}^{ab} + \frac{1}{6} g_Y^2 C_{dB}^{*ab} Y_d^{ab} - \frac{3}{4} g_L^2 Y_d^{*ab} C_{dW}^{ab} - \frac{3}{4} g_L^2 C_{dW}^{*ab} Y_d^{ab} + \left\{ \frac{3}{2} g_L^2 Y_d^{*ab} + 2(Y_u^\dagger Y_u Y_d^\dagger)^{ab} + 3\lambda Y_d^{*ab} + 46g_s^2 Y_d^{*ab} - \frac{5}{18} g_Y^2 Y_d^{*ab} \right.
\end{aligned}$$

$$\begin{aligned}
& -15(Y_d^\dagger Y_d Y_d^\dagger)^{ab} \Big\} C_{dG}^{ab} + C_{dG}^{*ab} \Big\{ \frac{3}{2} g_L^2 Y_d^{ab} + 2(Y_u Y_u^\dagger Y_d)^{ab} + 3\lambda Y_d^{ab} + 46g_s^2 Y_d^{ab} - \frac{5}{18} g_Y^2 Y_d^{ab} - 15(Y_d Y_d^\dagger Y_d)^{ab} \Big\} + \Big\{ \frac{1}{3} \delta^{ab} g_Y^2 + (Y_u Y_u^\dagger)^{ba} \\
& - (Y_d Y_d^\dagger)^{ba} \Big\} C_{Hq}^{(\parallel)ab} + \Big\{ \frac{1}{6} \delta^{ab} g_Y^2 + \frac{3}{2} \delta^{ab} g_L^2 - (Y_u Y_u^\dagger)^{ba} - 2(Y_d Y_d^\dagger)^{ba} \Big\} C_{Hq}^{(\times)ab} + \Big\{ \frac{2}{3} \delta^{ab} g_Y^2 - (Y_u^\dagger Y_u)^{ba} \Big\} C_{Hu}^{ab} + \Big\{ (Y_d^\dagger Y_d)^{ba} - \frac{1}{3} \delta^{ab} g_Y^2 \Big\} C_{Hd}^{ab} \\
& + C_{Hud}^{ab} (Y_d^\dagger Y_u)^{ba} + C_{Hud}^{*ab} (Y_u^\dagger Y_d)^{ab} - 4Y_u^{*ad} C_{qu}^{(\parallel)abcd} Y_u^{bc} - 4Y_d^{*ad} C_{qd}^{(\parallel)abcd} Y_d^{bc},
\end{aligned} \tag{5.10}$$

## 5.6 $C_{H\tilde{G}}$

$$\beta_{C_{H\tilde{G}}}^{(1)} = \left\{ 2T_2 + 6\lambda - \frac{3}{2} g_Y^2 - \frac{9}{2} g_L^2 \right\} C_{H\tilde{G}} + 2iY_u^{*ab} C_{uG}^{ab} - 2iC_{uG}^{*ab} Y_u^{ab} + 2iY_d^{*ab} C_{dG}^{ab} - 2iC_{dG}^{*ab} Y_d^{ab}, \tag{5.11}$$

$$\begin{aligned}
\beta_{C_{H\tilde{G}}}^{(2)} = & \frac{11}{2} g_Y^4 C_{H\tilde{B}} + \frac{27}{2} g_L^4 C_{H\tilde{W}} + \left\{ \lambda \left( 12g_Y^2 + 36g_L^2 - 12T_2 \right) + g_Y^2 \left( \frac{25}{12} \text{Tr}[Y_d^\dagger Y_d] + \frac{25}{4} \text{Tr}[Y_e^\dagger Y_e] + \frac{85}{12} \text{Tr}[Y_u^\dagger Y_u] \right) + g_s^2 \left( 36 \text{Tr}[Y_d^\dagger Y_d] \right. \right. \\
& \left. \left. + 36 \text{Tr}[Y_u^\dagger Y_u] \right) + \frac{15}{8} g_Y^2 g_L^2 + \frac{15}{4} T_2 g_L^2 + \frac{557}{48} g_Y^4 + 48g_s^4 - \frac{9}{2} T_4 - \frac{145}{16} g_L^4 - 15\lambda^2 - 21 \text{Tr}[Y_d^\dagger Y_d Y_u^\dagger Y_u] \right\} C_{H\tilde{G}} \\
& - g_s^4 \left\{ 211 \text{Tr}[Y_d^\dagger Y_d] + 211 \text{Tr}[Y_u^\dagger Y_u] \right\} C_{\tilde{G}} - \frac{3i}{4} Y_u^{*ab} C_{uH}^{ab} + \frac{3i}{4} C_{uH}^{*ab} Y_u^{ab} - \frac{3i}{4} Y_d^{*ab} C_{dH}^{ab} + \frac{3i}{4} C_{dH}^{*ab} Y_d^{ab} - \frac{23i}{6} g_Y^2 Y_u^{*ab} C_{uB}^{ab} \\
& + \frac{23i}{6} g_Y^2 C_{uB}^{*ab} Y_u^{ab} - \frac{21i}{4} g_L^2 Y_u^{*ab} C_{uW}^{ab} + \frac{21i}{4} g_L^2 C_{uW}^{*ab} Y_u^{ab} + \left\{ \frac{3i}{2} g_L^2 Y_u^{*ab} + \frac{37i}{18} g_Y^2 Y_u^{*ab} + 3i\lambda Y_u^{*ab} + 4i(Y_d^\dagger Y_d Y_u^\dagger)^{ab} + 22ig_s^2 Y_u^{*ab} \right. \\
& \left. - 9i(Y_u^\dagger Y_u Y_u^\dagger)^{ab} \right\} C_{uG}^{ab} + C_{uG}^{*ab} \left\{ 9i(Y_u Y_u^\dagger Y_u)^{ab} - \frac{3i}{2} g_L^2 Y_u^{ab} - \frac{37i}{18} g_Y^2 Y_u^{ab} - 3i\lambda Y_u^{ab} - 4i(Y_d Y_d^\dagger Y_u)^{ab} - 22ig_s^2 Y_u^{ab} \right\} + \frac{5i}{3} g_Y^2 Y_d^{*ab} C_{dB}^{ab} \\
& - \frac{5i}{3} g_Y^2 C_{dB}^{*ab} Y_d^{ab} - 3ig_L^2 Y_d^{*ab} C_{dW}^{ab} + 3ig_L^2 C_{dW}^{*ab} Y_d^{ab} + \left\{ \frac{3i}{2} g_L^2 Y_d^{*ab} + 3i\lambda Y_d^{*ab} + 4i(Y_u^\dagger Y_u Y_d^\dagger)^{ab} + 22ig_s^2 Y_d^{*ab} - \frac{5i}{18} g_Y^2 Y_d^{*ab} \right. \\
& \left. - 9i(Y_d^\dagger Y_d Y_d^\dagger)^{ab} \right\} C_{dG}^{ab} + C_{dG}^{*ab} \left\{ \frac{5i}{18} g_Y^2 Y_d^{ab} + 9i(Y_d Y_d^\dagger Y_d)^{ab} - \frac{3i}{2} g_L^2 Y_d^{ab} - 3i\lambda Y_d^{ab} - 4i(Y_u Y_u^\dagger Y_d)^{ab} - 22ig_s^2 Y_d^{ab} \right\} + \frac{i}{2} C_{Hud}^{ab} (Y_d^\dagger Y_u)^{ba} \\
& - \frac{i}{2} C_{Hud}^{*ab} (Y_u^\dagger Y_d)^{ab},
\end{aligned} \tag{5.12}$$

## 5.7 $C_{HWB}$

$$\begin{aligned}\beta_{C_{HWB}}^{(1)} = & 4g_Y^2 C_{HB} + 4g_L^2 C_{HW} + \left\{ 2T_2 + 2\lambda + \frac{9}{2}g_L^2 - \frac{1}{2}g_Y^2 \right\} C_{HWB} - 6g_L^4 C_W + 2Y_e^{*ab} C_{eB}^{ab} + 2C_{eB}^{*ab} Y_e^{ab} - 3Y_e^{*ab} C_{eW}^{ab} - 3C_{eW}^{*ab} Y_e^{ab} \\ & - 6Y_u^{*ab} C_{uB}^{ab} - 6C_{uB}^{*ab} Y_u^{ab} - 5Y_u^{*ab} C_{uW}^{ab} - 5C_{uW}^{*ab} Y_u^{ab} + 6Y_d^{*ab} C_{dB}^{ab} + 6C_{dB}^{*ab} Y_d^{ab} - Y_d^{*ab} C_{dW}^{ab} - C_{dW}^{*ab} Y_d^{ab},\end{aligned}\quad (5.13)$$

$$\begin{aligned}\beta_{C_{HWB}}^{(2)} = & 4T_{\ell H} + \left\{ \frac{7}{9}g_Y^2 + g_L^2 - 4\lambda \right\} C_{HD}^{(\parallel)} + \left\{ \frac{1}{18}g_Y^2 + \frac{1}{2}g_L^2 + \frac{1}{2}\text{Tr}[Y_d^\dagger Y_d] - \frac{1}{2}\text{Tr}[Y_e^\dagger Y_e] - \frac{1}{2}\text{Tr}[Y_u^\dagger Y_u] - 2\lambda \right\} C_{HD}^{(\times)} + \left\{ -g_Y^2 \left( 3\text{Tr}[Y_e^\dagger Y_e] \right. \right. \\ & + 13\text{Tr}[Y_u^\dagger Y_u] + 17\text{Tr}[Y_d^\dagger Y_d] \Big) - \frac{29}{9}g_Y^4 - 11g_Y^2 g_L^2 - 12\lambda g_Y^2 \Big\} C_{HB} + \left\{ g_Y^2 g_L^2 - g_L^2 \left( 3\text{Tr}[Y_e^\dagger Y_e] + 13\text{Tr}[Y_u^\dagger Y_u] + 17\text{Tr}[Y_d^\dagger Y_d] \right) - \frac{35}{9}g_L^4 \right. \\ & - 12\lambda g_L^2 \Big\} C_{HW} + \left\{ \frac{1}{2}T_2 g_L^2 + g_Y^2 \left( \frac{1}{2}\text{Tr}[Y_u^\dagger Y_u] + \frac{5}{2}\text{Tr}[Y_e^\dagger Y_e] - \frac{5}{2}\text{Tr}[Y_d^\dagger Y_d] \right) + g_s^2 \left( 40\text{Tr}[Y_d^\dagger Y_d] + 40\text{Tr}[Y_u^\dagger Y_u] \right) + \frac{71}{16}g_L^4 + \frac{1231}{144}g_Y^4 \right. \\ & + \frac{107}{8}g_Y^2 g_L^2 + 27\text{Tr}[Y_d^\dagger Y_d Y_u^\dagger Y_u] - \lambda \left( 2g_L^2 + 4T_2 \right) - \frac{9}{2}T_4 - 7\lambda^2 \Big\} C_{HWB} + \left\{ 3T_2 g_L^4 + \frac{503}{12}g_L^6 - \frac{3}{4}g_Y^2 g_L^4 - 9\lambda g_L^4 \right\} C_W \\ & - \frac{1}{2}Y_e^{*ab} C_{eH}^{ab} - \frac{1}{2}C_{eH}^{*ab} Y_e^{ab} - \frac{1}{2}Y_u^{*ab} C_{uH}^{ab} - \frac{1}{2}C_{uH}^{*ab} Y_u^{ab} + \frac{1}{2}Y_d^{*ab} C_{dH}^{ab} + \frac{1}{2}C_{dH}^{*ab} Y_d^{ab} + \left\{ \frac{1}{2}g_Y^2 Y_e^{*ab} + \lambda Y_e^{*ab} + \frac{7}{2}g_L^2 Y_e^{*ab} \right. \\ & - 9(Y_e^\dagger Y_e Y_e^\dagger)^{ab} \Big\} C_{eB}^{ab} + C_{eB}^{*ab} \left\{ \frac{1}{2}g_Y^2 Y_e^{ab} + \lambda Y_e^{ab} + \frac{7}{2}g_L^2 Y_e^{ab} - 9(Y_e Y_e^\dagger Y_e)^{ab} \right\} + \left\{ \frac{11}{4}g_L^2 Y_e^{*ab} + 15(Y_e^\dagger Y_e Y_e^\dagger)^{ab} - \frac{3}{2}\lambda Y_e^{*ab} \right. \\ & - \frac{51}{4}g_Y^2 Y_e^{*ab} \Big\} C_{eW}^{ab} + C_{eW}^{*ab} \left\{ \frac{11}{4}g_L^2 Y_e^{ab} + 15(Y_e Y_e^\dagger Y_e)^{ab} - \frac{3}{2}\lambda Y_e^{ab} - \frac{51}{4}g_Y^2 Y_e^{ab} \right\} + \left\{ \frac{19}{6}g_Y^2 Y_u^{*ab} + 27(Y_u^\dagger Y_u Y_u^\dagger)^{ab} - 3\lambda Y_u^{*ab} \right. \\ & - 9(Y_d^\dagger Y_d Y_u^\dagger)^{ab} - \frac{21}{2}g_L^2 Y_u^{*ab} - 56g_s^2 Y_u^{*ab} \Big\} C_{uB}^{ab} + C_{uB}^{*ab} \left\{ \frac{19}{6}g_Y^2 Y_u^{ab} + 27(Y_u Y_u^\dagger Y_u)^{ab} - 3\lambda Y_u^{ab} - 9(Y_d Y_d^\dagger Y_u)^{ab} - \frac{21}{2}g_L^2 Y_u^{ab} - 56g_s^2 Y_u^{ab} \right\} \\ & + \left\{ \frac{3}{4}g_L^2 Y_u^{*ab} + 25(Y_u^\dagger Y_u Y_u^\dagger)^{ab} - \frac{5}{2}\lambda Y_u^{*ab} - 5(Y_d^\dagger Y_d Y_u^\dagger)^{ab} - \frac{275}{36}g_Y^2 Y_u^{*ab} - \frac{140}{3}g_s^2 Y_u^{*ab} \right\} C_{uW}^{ab} + C_{uW}^{*ab} \left\{ \frac{3}{4}g_L^2 Y_u^{ab} + 25(Y_u Y_u^\dagger Y_u)^{ab} \right. \\ & - \frac{5}{2}\lambda Y_u^{ab} - 5(Y_d Y_d^\dagger Y_u)^{ab} - \frac{275}{36}g_Y^2 Y_u^{ab} - \frac{140}{3}g_s^2 Y_u^{ab} \Big\} + \frac{32}{3}g_s^2 Y_u^{*ab} C_{uG}^{ab} + \frac{32}{3}g_s^2 C_{uG}^{*ab} Y_u^{ab} + \left\{ 3\lambda Y_d^{*ab} + 9(Y_u^\dagger Y_u Y_d^\dagger)^{ab} + \frac{21}{2}g_L^2 Y_d^{*ab} \right. \\ & + 56g_s^2 Y_d^{*ab} - \frac{7}{6}g_Y^2 Y_d^{*ab} - 27(Y_d^\dagger Y_d Y_d^\dagger)^{ab} \Big\} C_{dB}^{ab} + C_{dB}^{*ab} \left\{ 3\lambda Y_d^{ab} + 9(Y_u Y_u^\dagger Y_d)^{ab} + \frac{21}{2}g_L^2 Y_d^{ab} + 56g_s^2 Y_d^{ab} - \frac{7}{6}g_Y^2 Y_d^{ab} - 27(Y_d Y_d^\dagger Y_d)^{ab} \right\}\end{aligned}$$

$$\begin{aligned}
& + \left\{ 5(Y_d^\dagger Y_d Y_d^\dagger)^{ab} - \frac{13}{36} g_Y^2 Y_d^{*ab} - \frac{1}{2} \lambda Y_d^{*ab} - \frac{27}{4} g_L^2 Y_d^{*ab} - 7(Y_u^\dagger Y_u Y_d^\dagger)^{ab} - \frac{28}{3} g_s^2 Y_d^{*ab} \right\} C_{dW}^{ab} + C_{dW}^{*ab} \left\{ 5(Y_d Y_d^\dagger Y_d)^{ab} - \frac{13}{36} g_Y^2 Y_d^{ab} - \frac{1}{2} \lambda Y_d^{ab} \right. \\
& - \frac{27}{4} g_L^2 Y_d^{ab} - 7(Y_u Y_u^\dagger Y_d)^{ab} - \frac{28}{3} g_s^2 Y_d^{ab} \left. \right\} + \frac{16}{3} g_s^2 Y_d^{*ab} C_{dG}^{ab} + \frac{16}{3} g_s^2 C_{dG}^{*ab} Y_d^{ab} + \left\{ \frac{1}{3} (Y_e Y_e^\dagger)^{ba} - 2\delta^{ab} g_L^2 - \frac{20}{9} \delta^{ab} g_Y^2 \right\} C_{H\ell}^{(\parallel)ab} + \left\{ \frac{8}{3} (Y_e Y_e^\dagger)^{ba} \right. \\
& - \frac{1}{9} \delta^{ab} g_Y^2 - 3\delta^{ab} g_L^2 \left. \right\} C_{H\ell}^{(\times)ab} + \left\{ \frac{11}{3} (Y_e^\dagger Y_e)^{ba} - \frac{20}{9} \delta^{ab} g_Y^2 \right\} C_{He}^{ab} + \left\{ 2\delta^{ab} g_L^2 + \frac{20}{9} \delta^{ab} g_Y^2 + 5(Y_u Y_u^\dagger)^{ba} - 11(Y_d Y_d^\dagger)^{ba} \right\} C_{Hq}^{(\parallel)ab} + \left\{ \frac{13}{9} \delta^{ab} g_Y^2 \right. \\
& + 5(Y_u Y_u^\dagger)^{ba} - 5\delta^{ab} g_L^2 - 8(Y_d Y_d^\dagger)^{ba} \left. \right\} C_{Hq}^{(\times)ab} + \left\{ \frac{40}{9} \delta^{ab} g_Y^2 - 9(Y_u^\dagger Y_u)^{ba} \right\} C_{Hu}^{ab} + \left\{ 7(Y_d^\dagger Y_d)^{ba} - \frac{20}{9} \delta^{ab} g_Y^2 \right\} C_{Hd}^{ab} - 4C_{Hud}^{ab} (Y_d^\dagger Y_u)^{ba} \\
& - 4C_{Hud}^{*ab} (Y_u^\dagger Y_d)^{ab} + 6Y_e^{*ad} C_{\ell e}^{abcd} Y_e^{bc} + 10Y_u^{*ad} C_{qu}^{(\parallel)abcd} Y_u^{bc} + 30Y_u^{*ad} C_{qu}^{(\times)abcd} Y_u^{bc} + 2Y_d^{*ad} C_{qd}^{(\parallel)abcd} Y_d^{bc} + 6Y_d^{*ad} C_{qd}^{(\times)abcd} Y_d^{bc}, \tag{5.14}
\end{aligned}$$

## 5.8 $C_{H\widetilde{W}B}$

$$\begin{aligned}
\beta_{C_{H\widetilde{W}B}}^{(1)} & = 4g_Y^2 C_{H\widetilde{B}} + 4g_L^2 C_{H\widetilde{W}} + \left\{ 2T_2 + 2\lambda + \frac{9}{2} g_L^2 - \frac{1}{2} g_Y^2 \right\} C_{H\widetilde{W}B} - 6g_L^4 C_{\widetilde{W}} + 2iY_e^{*ab} C_{eB}^{ab} - 2iC_{eB}^{*ab} Y_e^{ab} - 3iY_e^{*ab} C_{eW}^{ab} + 3iC_{eW}^{*ab} Y_e^{ab} \\
& - 6iY_u^{*ab} C_{uB}^{ab} + 6iC_{uB}^{*ab} Y_u^{ab} - 5iY_u^{*ab} C_{uW}^{ab} + 5iC_{uW}^{*ab} Y_u^{ab} + 6iY_d^{*ab} C_{dB}^{ab} - 6iC_{dB}^{*ab} Y_d^{ab} - iY_d^{*ab} C_{dW}^{ab} + iC_{dW}^{*ab} Y_d^{ab}, \tag{5.15}
\end{aligned}$$

$$\begin{aligned}
\beta_{C_{H\widetilde{W}B}}^{(2)} & = \left\{ -g_Y^2 \left( 3 \text{Tr}[Y_e^\dagger Y_e] + 13 \text{Tr}[Y_u^\dagger Y_u] + 17 \text{Tr}[Y_d^\dagger Y_d] \right) - \frac{29}{9} g_Y^4 - 11g_Y^2 g_L^2 - 12\lambda g_Y^2 \right\} C_{H\widetilde{B}} + \left\{ g_Y^2 g_L^2 + \frac{253}{9} g_L^4 - g_L^2 \left( 3 \text{Tr}[Y_e^\dagger Y_e] \right. \right. \\
& + 13 \text{Tr}[Y_u^\dagger Y_u] + 17 \text{Tr}[Y_d^\dagger Y_d] \left. \right) - 12\lambda g_L^2 \left. \right\} C_{H\widetilde{W}} + \left\{ \frac{1}{2} T_2 g_L^2 + g_Y^2 \left( \frac{1}{2} \text{Tr}[Y_u^\dagger Y_u] + \frac{5}{2} \text{Tr}[Y_e^\dagger Y_e] - \frac{5}{2} \text{Tr}[Y_d^\dagger Y_d] \right) + g_s^2 \left( 40 \text{Tr}[Y_d^\dagger Y_d] \right. \right. \\
& + 40 \text{Tr}[Y_u^\dagger Y_u] \left. \right) + \frac{71}{16} g_L^4 + \frac{1231}{144} g_Y^4 + \frac{107}{8} g_Y^2 g_L^2 + 27 \text{Tr}[Y_d^\dagger Y_d Y_u^\dagger Y_u] - \lambda \left( 2g_L^2 + 4T_2 \right) - \frac{9}{2} T_4 - 7\lambda^2 \left. \right\} C_{H\widetilde{W}B} + \left\{ \frac{1}{4} g_L^6 \right. \\
& + g_L^4 \left( 3 \text{Tr}[Y_e^\dagger Y_e] + \frac{43}{3} \text{Tr}[Y_u^\dagger Y_u] + \frac{59}{3} \text{Tr}[Y_d^\dagger Y_d] \right) - \frac{7}{4} g_Y^2 g_L^4 - 5\lambda g_L^4 \left. \right\} C_{\widetilde{W}} + \frac{i}{4} Y_e^{*ab} C_{eH}^{ab} - \frac{i}{4} C_{eH}^{*ab} Y_e^{ab} + \frac{i}{4} Y_u^{*ab} C_{uH}^{ab} - \frac{i}{4} C_{uH}^{*ab} Y_u^{ab} \\
& - \frac{i}{4} Y_d^{*ab} C_{dH}^{ab} + \frac{i}{4} C_{dH}^{*ab} Y_d^{ab} + \left\{ i\lambda Y_e^{*ab} + \frac{7i}{2} g_L^2 Y_e^{*ab} - 3i(Y_e^\dagger Y_e Y_e^\dagger)^{ab} - \frac{9i}{2} g_Y^2 Y_e^{*ab} \right\} C_{eB}^{ab} + C_{eB}^{*ab} \left\{ 3i(Y_e Y_e^\dagger Y_e)^{ab} + \frac{9i}{2} g_Y^2 Y_e^{ab} - i\lambda Y_e^{ab} \right. \\
& - \frac{7i}{2} g_L^2 Y_e^{ab} \left. \right\} + \left\{ 12i(Y_e^\dagger Y_e Y_e^\dagger)^{ab} - \frac{3i}{2} \lambda Y_e^{*ab} - \frac{5i}{2} g_L^2 Y_e^{*ab} - \frac{51i}{4} g_Y^2 Y_e^{*ab} \right\} C_{eW}^{ab} + C_{eW}^{*ab} \left\{ \frac{3i}{2} \lambda Y_e^{ab} + \frac{5i}{2} g_L^2 Y_e^{ab} + \frac{51i}{4} g_Y^2 Y_e^{ab} \right.
\end{aligned}$$



$$\begin{aligned}
& -12i(Y_e Y_e^\dagger Y_e)^{ab} \Bigg\} + \left\{ 9i(Y_u^\dagger Y_u Y_u^\dagger)^{ab} + \frac{115i}{12} g_Y^2 Y_u^{*ab} - 3i\lambda Y_u^{*ab} - 3i(Y_d^\dagger Y_d Y_u^\dagger)^{ab} - \frac{21i}{2} g_L^2 Y_u^{*ab} - 56ig_s^2 Y_u^{*ab} \right\} C_{uB}^{ab} + C_{uB}^{*ab} \left\{ 3i\lambda Y_u^{ab} \right. \\
& + 3i(Y_d Y_d^\dagger Y_u)^{ab} + \frac{21i}{2} g_L^2 Y_u^{ab} + 56ig_s^2 Y_u^{ab} - 9i(Y_u Y_u^\dagger Y_u)^{ab} - \frac{115i}{12} g_Y^2 Y_u^{ab} \Bigg\} + \left\{ 20i(Y_u^\dagger Y_u Y_u^\dagger)^{ab} - \frac{5i}{2} \lambda Y_u^{*ab} - 6i(Y_d^\dagger Y_d Y_u^\dagger)^{ab} \right. \\
& - \frac{275i}{36} g_Y^2 Y_u^{*ab} - \frac{63i}{8} g_L^2 Y_u^{*ab} - \frac{140i}{3} g_s^2 Y_u^{*ab} \Bigg\} C_{uW}^{ab} + C_{uW}^{*ab} \left\{ \frac{5i}{2} \lambda Y_u^{ab} + 6i(Y_d Y_d^\dagger Y_u)^{ab} + \frac{275i}{36} g_Y^2 Y_u^{ab} + \frac{63i}{8} g_L^2 Y_u^{ab} + \frac{140i}{3} g_s^2 Y_u^{ab} \right. \\
& - 20i(Y_u Y_u^\dagger Y_u)^{ab} \Bigg\} + 34ig_s^2 Y_u^{*ab} C_{uG}^{ab} - 34ig_s^2 C_{uG}^{*ab} Y_u^{ab} + \left\{ 3i\lambda Y_d^{*ab} + 3i(Y_u^\dagger Y_u Y_d^\dagger)^{ab} + \frac{21i}{2} g_L^2 Y_d^{*ab} + 56ig_s^2 Y_d^{*ab} - \frac{i}{2} g_Y^2 Y_d^{*ab} \right. \\
& - 9i(Y_d^\dagger Y_d Y_d^\dagger)^{ab} \Bigg\} C_{dB}^{ab} + C_{dB}^{*ab} \left\{ \frac{i}{2} g_Y^2 Y_d^{ab} + 9i(Y_d Y_d^\dagger Y_d)^{ab} - 3i\lambda Y_d^{ab} - 3i(Y_u Y_u^\dagger Y_d)^{ab} - \frac{21i}{2} g_L^2 Y_d^{ab} - 56ig_s^2 Y_d^{ab} \right\} + \left\{ 4i(Y_d^\dagger Y_d Y_d^\dagger)^{ab} \right. \\
& - \frac{13i}{36} g_Y^2 Y_d^{*ab} - \frac{i}{2} \lambda Y_d^{*ab} - \frac{15i}{2} g_L^2 Y_d^{*ab} - \frac{28i}{3} g_s^2 Y_d^{*ab} - 12i(Y_u^\dagger Y_u Y_d^\dagger)^{ab} \Bigg\} C_{dW}^{ab} + C_{dW}^{*ab} \left\{ \frac{13i}{36} g_Y^2 Y_d^{ab} + \frac{i}{2} \lambda Y_d^{ab} + \frac{15i}{2} g_L^2 Y_d^{ab} \right. \\
& + \frac{28i}{3} g_s^2 Y_d^{ab} + 12i(Y_u Y_u^\dagger Y_d)^{ab} - 4i(Y_d Y_d^\dagger Y_d)^{ab} \Bigg\} + \frac{14i}{3} g_s^2 Y_d^{*ab} C_{dG}^{ab} - \frac{14i}{3} g_s^2 C_{dG}^{*ab} Y_d^{ab} - \frac{i}{4} C_{Hud}^{ab} (Y_d^\dagger Y_u)^{ba} + \frac{i}{4} C_{Hud}^{*ab} (Y_u^\dagger Y_d)^{ab}, \tag{5.16}
\end{aligned}$$

## 6 $X^3$

### 6.1 $C_W$

$$\beta_{C_W}^{(1)} = 24g_L^2 C_W, \tag{6.1}$$

$$\beta_{C_W}^{(2)} = 5g_L^2 C_{HW} - \frac{1}{4} g_Y^2 C_{HWB} + \frac{71}{3} g_L^4 C_W, \tag{6.2}$$

### 6.2 $C_{\widetilde{W}}$

$$\beta_{C_{\widetilde{W}}}^{(1)} = 24g_L^2 C_{\widetilde{W}}, \tag{6.3}$$

$$\beta_{C_{\widetilde{W}}}^{(2)} = 5g_L^2 C_{H\widetilde{W}} - \frac{1}{4} g_Y^2 C_{H\widetilde{W}B} + \frac{289}{9} g_L^4 C_{\widetilde{W}} - \frac{i}{3} Y_e^{*ab} C_{eW}^{ab} + \frac{i}{3} C_{eW}^{*ab} Y_e^{ab} - iY_u^{*ab} C_{uW}^{ab} + iC_{uW}^{*ab} Y_u^{ab} - iY_d^{*ab} C_{dW}^{ab} + iC_{dW}^{*ab} Y_d^{ab}, \tag{6.4}$$

### 6.3 $C_G$

$$\beta_{C_G}^{(1)} = 36g_s^2 C_G, \quad (6.5)$$

$$\beta_{C_G}^{(2)} = 177g_s^4 C_G + Y_u^{*ab} C_{uG}^{ab} + C_{uG}^{*ab} Y_u^{ab} + Y_d^{*ab} C_{dG}^{ab} + C_{dG}^{*ab} Y_d^{ab}, \quad (6.6)$$

### 6.4 $C_{\tilde{G}}$

$$\beta_{C_{\tilde{G}}}^{(1)} = 36g_s^2 C_{\tilde{G}}, \quad (6.7)$$

$$\beta_{C_{\tilde{G}}}^{(2)} = 205g_s^4 C_{\tilde{G}} - \frac{i}{3} Y_u^{*ab} C_{uG}^{ab} + \frac{i}{3} C_{uG}^{*ab} Y_u^{ab} - \frac{i}{3} Y_d^{*ab} C_{dG}^{ab} + \frac{i}{3} C_{dG}^{*ab} Y_d^{ab}, \quad (6.8)$$

## 7 $\psi^2 H^3$

### 7.1 $C_{eH}$

$$\begin{aligned} \beta_{C_{eH}}^{(1)} = & 6(C_{\ell HH}^\dagger C_{\ell HH} Y_e)^{pr} + \left\{ \frac{17}{12} g_L^2 Y_e^{pr} + \frac{3}{2} (Y_e Y_e^\dagger Y_e)^{pr} - \frac{1}{12} g_Y^2 Y_e^{pr} - \lambda Y_e^{pr} \right\} C_{HD}^{(\parallel)} + \left\{ \lambda Y_e^{pr} + (Y_e Y_e^\dagger Y_e)^{pr} - \frac{1}{6} g_Y^2 Y_e^{pr} - \frac{3}{2} g_L^2 Y_e^{pr} \right\} C_{HD}^{(\times)} \\ & + 15g_Y^4 C_{HB} Y_e^{pr} - 15ig_Y^4 C_{H\tilde{B}} Y_e^{pr} + 9g_L^4 C_{HW} Y_e^{pr} - 9ig_L^4 C_{H\tilde{W}} Y_e^{pr} - \frac{3}{2} g_Y^2 g_L^2 C_{HWB} Y_e^{pr} + \frac{3i}{2} g_Y^2 g_L^2 C_{H\tilde{W}B} Y_e^{pr} + \left\{ \frac{1}{2} (4Y_e^{*ab} Y_e^{pr} + 6T_2 \delta^{pa} \delta^{rb} \right. \\ & + 10\delta^{pa} (Y_e^\dagger Y_e)^{br} + 11\delta^{rb} (Y_e Y_e^\dagger)^{pa}) + 12\delta^{pa} \delta^{rb} \lambda - \frac{21}{4} \delta^{pa} \delta^{rb} g_Y^2 - \frac{27}{4} \delta^{pa} \delta^{rb} g_L^2 \left. \right\} C_{eH}^{ab} + 6C_{uH}^{*ab} Y_e^{pr} Y_u^{ab} + 6Y_d^{*ab} C_{dH}^{ab} Y_e^{pr} + \left\{ 3\delta^{pa} \delta^{rb} g_Y^2 g_L^2 \right. \\ & - 9\delta^{pa} \delta^{rb} g_Y^4 - 9g_Y^2 (\delta^{pa} (Y_e^\dagger Y_e)^{br} + \delta^{rb} (Y_e Y_e^\dagger)^{pa}) \left. \right\} C_{eB}^{ab} + \left\{ \frac{3}{2} g_L^2 (\delta^{pa} (Y_e^\dagger Y_e)^{br} - \delta^{rb} (Y_e Y_e^\dagger)^{pa}) + \frac{9}{2} \delta^{pa} \delta^{rb} g_L^4 - \frac{9}{2} \delta^{pa} \delta^{rb} g_Y^2 g_L^2 \right\} C_{eW}^{ab} + \left\{ 2\delta^{pa} \lambda Y_e^{br} \right. \\ & + 2(Y_e^{pr} (Y_e Y_e^\dagger)^{ba} + \delta^{pa} (Y_e Y_e^\dagger Y_e)^{br}) - \frac{2}{3} g_Y^2 (9\delta^{pa} Y_e^{br} - \delta^{ab} Y_e^{pr}) \left. \right\} C_{H\ell}^{(\parallel)ab} + \left\{ \frac{1}{3} g_Y^2 (\delta^{ab} Y_e^{pr} - 18\delta^{pa} Y_e^{br}) + \delta^{pa} (Y_e Y_e^\dagger Y_e)^{br} + 2Y_e^{pr} (Y_e Y_e^\dagger)^{ba} + 4\delta^{pa} \lambda Y_e^{br} \right. \\ & - \frac{1}{3} \delta^{ab} g_L^2 Y_e^{pr} \left. \right\} C_{H\ell}^{(\times)ab} + \left\{ \frac{1}{3} g_Y^2 (2\delta^{ab} Y_e^{pr} - 9\delta^{rb} Y_e^{pa}) + 3\delta^{rb} g_L^2 Y_e^{pa} - 2\delta^{rb} \lambda Y_e^{pa} - 2(Y_e^{pr} (Y_e^\dagger Y_e)^{ba} + \delta^{rb} (Y_e Y_e^\dagger Y_e)^{pa}) \right\} C_{He}^{ab} + \left\{ 6(Y_e^{pr} (Y_d Y_d^\dagger)^{ba} \right. \\ & - Y_e^{pr} (Y_u Y_u^\dagger)^{ba}) - \frac{2}{3} \delta^{ab} g_Y^2 Y_e^{pr} \left. \right\} C_{Hq}^{(\parallel)ab} + \left\{ 6Y_e^{pr} (Y_d Y_d^\dagger)^{ba} - \frac{1}{3} \delta^{ab} g_Y^2 Y_e^{pr} - \delta^{ab} g_L^2 Y_e^{pr} \right\} C_{Hq}^{(\times)ab} + \left\{ 6Y_e^{pr} (Y_u^\dagger Y_u)^{ba} - \frac{4}{3} \delta^{ab} g_Y^2 Y_e^{pr} \right\} C_{Hu}^{ab} + \left\{ \frac{2}{3} \delta^{ab} g_Y^2 Y_e^{pr} \right. \end{aligned}$$

$$\begin{aligned}
& -6Y_e^{pr}(Y_d^\dagger Y_d)^{ba} \Big\} C_{Hd}^{ab} + \left\{ 8\delta^{pa}\delta^{rd}(Y_e Y_e^\dagger Y_e)^{bc} - 4\delta^{pa}\delta^{rd}\lambda Y_e^{bc} \right\} C_{\ell e}^{abcd} + \left\{ 6\delta^{pa}\delta^{rb}\lambda Y_d^{dc} - 12\delta^{pa}\delta^{rb}(Y_d Y_d^\dagger Y_d)^{dc} \right\} C_{\ell edq}^{abcd} \\
& + \left\{ 12\delta^{pa}\delta^{rb}(Y_u^\dagger Y_u Y_u^\dagger)^{cd} - 6\delta^{pa}\delta^{rb}\lambda Y_u^{*cd} \right\} C_{\ell equ}^{abcd} + \left\{ 3\delta^{pa}\delta^{rd}\lambda Y_u^{*cb} - 6\delta^{pa}\delta^{rd}(Y_u^\dagger Y_u Y_u^\dagger)^{cb} \right\} C_{\ell uqe}^{abcd}, \tag{7.1}
\end{aligned}$$

$$\begin{aligned}
\beta_{C_{eH}^{pr}}^{(2)} = & \frac{1}{12}g_L^2 \left( 22Y_e^{pr} \mathbf{T}_{\ell H} - 243(C_{\ell HH}^\dagger C_{\ell HH} Y_e)^{pr} \right) + \frac{1}{12}g_Y^2 \left( 38Y_e^{pr} \mathbf{T}_{\ell H} + 51(C_{\ell HH}^\dagger C_{\ell HH} Y_e)^{pr} \right) + \frac{1}{2} \left( 7(C_{\ell HH}^\dagger C_{\ell HH} Y_e Y_e^\dagger Y_e)^{pr} \right. \\
& + 7(Y_e Y_e^\dagger C_{\ell HH}^\dagger C_{\ell HH} Y_e)^{pr} + 30(Y_e Y_e^\dagger Y_e)^{pr} \mathbf{T}_{\ell H} - 7(C_{\ell HH}^\dagger Y_e^\dagger Y_e C_{\ell HH} Y_e)^{pr} - 10\mathbf{T}_2(C_{\ell HH}^\dagger C_{\ell HH} Y_e)^{pr} \Big) \\
& - \lambda \left( 5(C_{\ell HH}^\dagger C_{\ell HH} Y_e)^{pr} + 24Y_e^{pr} \mathbf{T}_{\ell H} \right) - 6Y_e^{pr} \text{Tr} \left[ C_{\ell HH}^\dagger C_{\ell HH} Y_e Y_e^\dagger \right] + \left\{ 24\lambda Y_e^{pr} - 48(Y_e Y_e^\dagger Y_e)^{pr} \right\} C_H + \left\{ \frac{1}{2}\lambda^2 Y_e^{pr} + \frac{47}{54}g_Y^2 g_L^2 Y_e^{pr} \right. \\
& + \lambda \left( \frac{9}{4}g_L^2 Y_e^{pr} + \frac{163}{36}g_Y^2 Y_e^{pr} + 5\mathbf{T}_2 Y_e^{pr} - \frac{53}{2}(Y_e Y_e^\dagger Y_e)^{pr} \right) + g_Y^2 \left( \frac{1}{12}\mathbf{T}_2 Y_e^{pr} + \frac{71}{16}(Y_e Y_e^\dagger Y_e)^{pr} \right) + \frac{25}{8}(Y_e Y_e^\dagger Y_e Y_e^\dagger Y_e)^{pr} + \frac{45}{2}Y_e^{pr} \text{Tr} \left[ Y_d^\dagger Y_d Y_u^\dagger Y_u \right] \\
& - g_L^2 \left( \frac{17}{12}\mathbf{T}_2 Y_e^{pr} + \frac{23}{16}(Y_e Y_e^\dagger Y_e)^{pr} \right) - \frac{74}{27}g_Y^4 Y_e^{pr} - \frac{71}{24}g_L^4 Y_e^{pr} - \frac{13}{4}\mathbf{T}_4 Y_e^{pr} - \frac{9}{2}\mathbf{T}_2(Y_e Y_e^\dagger Y_e)^{pr} \Big\} C_{HD}^{(\parallel)} + \left\{ \lambda^2 Y_e^{pr} + \lambda \left( \frac{287}{36}g_Y^2 Y_e^{pr} \right. \right. \\
& + \frac{51}{4}g_L^2 Y_e^{pr} - 31(Y_e Y_e^\dagger Y_e)^{pr} \Big) + g_Y^2 \left( \frac{1}{6}\mathbf{T}_2 Y_e^{pr} + \frac{17}{4}(Y_e Y_e^\dagger Y_e)^{pr} \right) + g_L^2 \left( \frac{3}{2}\mathbf{T}_2 Y_e^{pr} + \frac{43}{8}(Y_e Y_e^\dagger Y_e)^{pr} \right) + \frac{133}{96}g_L^4 Y_e^{pr} + 2(Y_e Y_e^\dagger Y_e Y_e^\dagger Y_e)^{pr} \\
& - \frac{7}{4}\mathbf{T}_4 Y_e^{pr} - \frac{1955}{864}g_Y^4 Y_e^{pr} - 3\mathbf{T}_2(Y_e Y_e^\dagger Y_e)^{pr} - \frac{2143}{432}g_Y^2 g_L^2 Y_e^{pr} - \frac{27}{2}Y_e^{pr} \text{Tr} \left[ Y_d^\dagger Y_d Y_u^\dagger Y_u \right] \Big\} C_{HD}^{(\times)} + \left\{ g_Y^4 \left( \frac{53}{6}Y_e^{pr} \text{Tr} \left[ Y_d^\dagger Y_d \right] - \frac{79}{6}Y_e^{pr} \text{Tr} \left[ Y_u^\dagger Y_u \right] \right. \right. \\
& - \frac{43}{2}Y_e^{pr} \text{Tr} \left[ Y_e^\dagger Y_e \right] - \frac{375}{4}(Y_e Y_e^\dagger Y_e)^{pr} \Big) + \frac{49}{2}\lambda g_Y^4 Y_e^{pr} - \frac{49}{3}g_Y^4 g_L^2 Y_e^{pr} - 242g_Y^6 Y_e^{pr} \Big\} C_{HB} + \left\{ g_Y^4 \left( \frac{39i}{2}Y_e^{pr} \text{Tr} \left[ Y_e^\dagger Y_e \right] + \frac{477i}{4}(Y_e Y_e^\dagger Y_e)^{pr} \right. \right. \\
& - \frac{3i}{2}Y_e^{pr} \text{Tr} \left[ Y_d^\dagger Y_d \right] - \frac{33i}{2}Y_e^{pr} \text{Tr} \left[ Y_u^\dagger Y_u \right] \Big) + \frac{153i}{2}\lambda g_Y^4 Y_e^{pr} + \frac{1469i}{12}g_Y^6 Y_e^{pr} - \frac{21i}{4}g_Y^4 g_L^2 Y_e^{pr} \Big\} C_{H\tilde{B}} + \left\{ g_L^4 \left( \frac{3}{2}\mathbf{T}_2 Y_e^{pr} - \frac{243}{4}(Y_e Y_e^\dagger Y_e)^{pr} \right) \right. \\
& + \frac{77}{3}g_L^6 Y_e^{pr} + \frac{147}{2}\lambda g_L^4 Y_e^{pr} - 19g_Y^2 g_L^4 Y_e^{pr} \Big\} C_{HW} + \left\{ g_L^4 \left( \frac{9i}{2}Y_e^{pr} \text{Tr} \left[ Y_e^\dagger Y_e \right] + \frac{27i}{2}Y_e^{pr} \text{Tr} \left[ Y_d^\dagger Y_d \right] + \frac{213i}{4}(Y_e Y_e^\dagger Y_e)^{pr} - \frac{27i}{2}Y_e^{pr} \text{Tr} \left[ Y_u^\dagger Y_u \right] \right) \right. \\
& + \frac{51i}{2}\lambda g_L^4 Y_e^{pr} - \frac{21i}{4}g_Y^2 g_L^4 Y_e^{pr} - \frac{341i}{4}g_L^6 Y_e^{pr} \Big\} C_{H\tilde{W}} - g_s^4 \left\{ 176Y_e^{pr} \text{Tr} \left[ Y_d^\dagger Y_d \right] + 176Y_e^{pr} \text{Tr} \left[ Y_u^\dagger Y_u \right] \right\} C_{HG} + g_s^4 \left\{ 144iY_e^{pr} \text{Tr} \left[ Y_d^\dagger Y_d \right] \right. \\
& - 144iY_e^{pr} \text{Tr} \left[ Y_u^\dagger Y_u \right] \Big\} C_{H\tilde{G}} + \left\{ g_Y^2 g_L^2 \left( \frac{23}{4}Y_e^{pr} \text{Tr} \left[ Y_e^\dagger Y_e \right] + \frac{25}{4}Y_e^{pr} \text{Tr} \left[ Y_d^\dagger Y_d \right] + \frac{33}{4}(Y_e Y_e^\dagger Y_e)^{pr} + \frac{47}{4}Y_e^{pr} \text{Tr} \left[ Y_u^\dagger Y_u \right] \right) + \frac{23}{6}g_Y^2 g_L^4 Y_e^{pr} \right. \\
& + \frac{63}{4}\lambda g_Y^2 g_L^2 Y_e^{pr} - \frac{181}{12}g_Y^4 g_L^2 Y_e^{pr} \Big\} C_{H\tilde{W}B} + \left\{ g_Y^2 g_L^2 \left( \frac{27i}{4}Y_e^{pr} \text{Tr} \left[ Y_u^\dagger Y_u \right] - \frac{9i}{4}Y_e^{pr} \text{Tr} \left[ Y_d^\dagger Y_d \right] - \frac{15i}{4}Y_e^{pr} \text{Tr} \left[ Y_e^\dagger Y_e \right] - 12i(Y_e Y_e^\dagger Y_e)^{pr} \right) \right.
\end{aligned}$$

$$\begin{aligned}
& + \frac{11i}{3} g_Y^4 g_L^2 Y_e^{pr} - \frac{13i}{12} g_Y^2 g_L^4 Y_e^{pr} - \frac{81i}{4} \lambda g_Y^2 g_L^2 Y_e^{pr} \Big\} C_{H\widetilde{WB}} + \left\{ g_L^6 \left( 3T_2 Y_e^{pr} - \frac{9}{4} (Y_e Y_e^\dagger Y_e)^{pr} \right) + \frac{103}{12} g_L^8 Y_e^{pr} - 6\lambda g_L^6 Y_e^{pr} \right. \\
& - \frac{41}{4} g_Y^2 g_L^6 Y_e^{pr} \Big\} C_W + \left\{ \frac{9i}{4} g_L^6 (Y_e Y_e^\dagger Y_e)^{pr} - \frac{15i}{2} g_Y^2 g_L^6 Y_e^{pr} - 39i g_L^8 Y_e^{pr} \right\} C_{\widetilde{W}} + \left\{ \lambda \left( 5Y_e^{*ab} Y_e^{pr} + 18\delta^{pa} \delta^{rb} g_Y^2 + 54\delta^{pa} \delta^{rb} g_L^2 - 24T_2 \delta^{pa} \delta^{rb} \right. \right. \\
& - 42\delta^{pa} (Y_e^\dagger Y_e)^{br} - 42\delta^{rb} (Y_e Y_e^\dagger)^{pa} \Big) + g_L^2 \left( \frac{45}{8} T_2 \delta^{pa} \delta^{rb} + \frac{171}{8} \delta^{pa} (Y_e^\dagger Y_e)^{br} + \frac{387}{16} \delta^{rb} (Y_e Y_e^\dagger)^{pa} - \frac{9}{4} Y_e^{*ab} Y_e^{pr} \right) + g_Y^2 \left( \frac{25}{8} \delta^{pa} \delta^{rb} \text{Tr}[Y_d^\dagger Y_d] \right. \\
& + \frac{13}{4} Y_e^{*ab} Y_e^{pr} + \frac{75}{8} \delta^{pa} \delta^{rb} \text{Tr}[Y_e^\dagger Y_e] + \frac{85}{8} \delta^{pa} \delta^{rb} \text{Tr}[Y_u^\dagger Y_u] + \frac{167}{8} \delta^{pa} (Y_e^\dagger Y_e)^{br} + \frac{341}{16} \delta^{rb} (Y_e Y_e^\dagger)^{pa} \Big) + g_s^2 \left( 60\delta^{pa} \delta^{rb} \text{Tr}[Y_d^\dagger Y_d] \right. \\
& + 60\delta^{pa} \delta^{rb} \text{Tr}[Y_u^\dagger Y_u] \Big) + \frac{45}{8} \delta^{pa} \delta^{rb} g_Y^2 g_L^2 + \frac{1507}{48} \delta^{pa} \delta^{rb} g_Y^4 - \frac{5}{2} (Y_e^\dagger Y_e)^{br} (Y_e Y_e^\dagger)^{pa} - \frac{11}{4} T_4 \delta^{pa} \delta^{rb} - \frac{13}{2} T_2 \delta^{pa} (Y_e^\dagger Y_e)^{br} - \frac{13}{2} Y_e^{*ab} (Y_e Y_e^\dagger Y_e)^{pr} \\
& - \frac{29}{4} T_2 \delta^{rb} (Y_e Y_e^\dagger)^{pa} - \frac{31}{4} \delta^{rb} (Y_e Y_e^\dagger Y_e Y_e^\dagger)^{pa} - \frac{17}{2} \delta^{pa} (Y_e^\dagger Y_e Y_e^\dagger Y_e)^{br} - \frac{201}{16} \delta^{pa} \delta^{rb} g_L^4 - 14Y_e^{pr} (Y_e^\dagger Y_e Y_e^\dagger)^{ab} - \frac{39}{2} \delta^{pa} \delta^{rb} \text{Tr}[Y_d^\dagger Y_d Y_u^\dagger Y_u] \\
& - \frac{153}{2} \delta^{pa} \delta^{rb} \lambda^2 \Big\} C_{eH}^{ab} + C_{eH}^{*ab} \left\{ \lambda \left( 5Y_e^{pr} Y_e^{ab} - 18Y_e^{pb} Y_e^{ar} \right) + \frac{3}{2} g_L^2 Y_e^{pb} Y_e^{ar} + \frac{11}{2} Y_e^{pb} (Y_e Y_e^\dagger Y_e)^{ar} + \frac{23}{4} Y_e^{ar} (Y_e Y_e^\dagger Y_e)^{pb} + \frac{33}{2} g_Y^2 Y_e^{pb} Y_e^{ar} \right. \\
& - 5Y_e^{ab} (Y_e Y_e^\dagger Y_e)^{pr} - 5Y_e^{pr} (Y_e Y_e^\dagger Y_e)^{ab} \Big\} + \left\{ \frac{9}{2} Y_e^{pr} (Y_d^\dagger Y_d Y_u^\dagger)^{ab} + 15\lambda Y_u^{*ab} Y_e^{pr} - 15Y_e^{pr} (Y_u^\dagger Y_u Y_u^\dagger)^{ab} - 15Y_u^{*ab} (Y_e Y_e^\dagger Y_e)^{pr} \right\} C_{uH}^{ab} \\
& + C_{uH}^{*ab} \left\{ \frac{15}{2} Y_e^{pr} (Y_d Y_d^\dagger Y_u)^{ab} + 15\lambda Y_e^{pr} Y_u^{ab} + 40g_s^2 Y_e^{pr} Y_u^{ab} - \frac{23}{12} g_Y^2 Y_e^{pr} Y_u^{ab} - \frac{27}{4} g_L^2 Y_e^{pr} Y_u^{ab} - \frac{39}{2} Y_u^{ab} (Y_e Y_e^\dagger Y_e)^{pr} - 42Y_e^{pr} (Y_u Y_u^\dagger Y_u)^{ab} \right\} \\
& + \left\{ \frac{15}{2} Y_e^{pr} (Y_u^\dagger Y_u Y_d^\dagger)^{ab} + 15\lambda Y_d^{*ab} Y_e^{pr} + 40g_s^2 Y_d^{*ab} Y_e^{pr} - \frac{27}{4} g_L^2 Y_d^{*ab} Y_e^{pr} - \frac{83}{12} g_Y^2 Y_d^{*ab} Y_e^{pr} - \frac{39}{2} Y_d^{*ab} (Y_e Y_e^\dagger Y_e)^{pr} - 42Y_e^{pr} (Y_d^\dagger Y_d Y_d^\dagger)^{ab} \right\} C_{dH}^{ab} \\
& + C_{dH}^{*ab} \left\{ \frac{9}{2} Y_e^{pr} (Y_u Y_u^\dagger Y_d)^{ab} + 15\lambda Y_d^{ab} Y_e^{pr} - 15Y_e^{pr} (Y_d Y_d^\dagger Y_d)^{ab} - 15Y_d^{ab} (Y_e Y_e^\dagger Y_e)^{pr} \right\} + \left\{ \lambda \left( g_Y^2 \left( 3Y_e^{*ab} Y_e^{pr} - 3\delta^{pa} \delta^{rb} \text{Tr}[Y_d^\dagger Y_d] \right. \right. \right. \\
& - \frac{15}{2} \delta^{rb} (Y_e Y_e^\dagger)^{pa} - 9\delta^{pa} \delta^{rb} \text{Tr}[Y_e^\dagger Y_e] - \frac{117}{2} \delta^{pa} (Y_e^\dagger Y_e)^{br} \Big) + 21\delta^{pa} \delta^{rb} g_Y^2 g_L^2 - 75\delta^{pa} \delta^{rb} g_Y^4 \Big) + g_Y^2 g_L^2 \left( \frac{9}{2} Y_e^{*ab} Y_e^{pr} + 9\delta^{pa} \delta^{rb} \text{Tr}[Y_d^\dagger Y_d] \right. \\
& + 11\delta^{pa} \delta^{rb} \text{Tr}[Y_e^\dagger Y_e] + 14\delta^{pa} (Y_e^\dagger Y_e)^{br} + 21\delta^{pa} \delta^{rb} \text{Tr}[Y_u^\dagger Y_u] - \frac{23}{4} \delta^{rb} (Y_e Y_e^\dagger)^{pa} \Big) + g_Y^4 \left( 4Y_e^{*ab} Y_e^{pr} + 57\delta^{pa} \delta^{rb} \text{Tr}[Y_u^\dagger Y_u] + \frac{263}{4} \delta^{rb} (Y_e Y_e^\dagger)^{pa} \right. \\
& + 75\delta^{pa} \delta^{rb} \text{Tr}[Y_e^\dagger Y_e] + \frac{213}{2} \delta^{pa} (Y_e^\dagger Y_e)^{br} - 15\delta^{pa} \delta^{rb} \text{Tr}[Y_d^\dagger Y_d] \Big) + g_Y^2 \left( \frac{3}{2} T_2 \delta^{rb} (Y_e Y_e^\dagger)^{pa} + 6\delta^{pa} \delta^{rb} \text{Tr}[Y_d^\dagger Y_d Y_d^\dagger Y_d] + 18\delta^{pa} \delta^{rb} \text{Tr}[Y_e^\dagger Y_e Y_e^\dagger Y_e] \right. \\
& + \frac{117}{2} \delta^{rb} (Y_e Y_e^\dagger Y_e Y_e^\dagger)^{pa} + \frac{261}{4} \delta^{pa} (Y_e^\dagger Y_e Y_e^\dagger Y_e)^{br} - \frac{3}{2} T_2 \delta^{pa} (Y_e^\dagger Y_e)^{br} - \frac{7}{2} Y_e^{pr} (Y_e^\dagger Y_e Y_e^\dagger)^{ab} \Big) + \frac{427}{2} \delta^{pa} \delta^{rb} g_Y^6 - \frac{7}{3} \delta^{pa} \delta^{rb} g_Y^2 g_L^4 \\
& - \frac{22}{3} \delta^{pa} \delta^{rb} g_Y^4 g_L^2 \Big\} C_{eB}^{ab} + C_{eB}^{*ab} \left\{ g_Y^2 g_L^2 \left( \frac{5}{2} Y_e^{pr} Y_e^{ab} - \frac{9}{2} Y_e^{pb} Y_e^{ar} \right) + g_Y^4 \left( \frac{27}{2} Y_e^{pb} Y_e^{ar} + 37Y_e^{pr} Y_e^{ab} \right) + g_Y^2 \left( \frac{15}{4} Y_e^{ar} (Y_e Y_e^\dagger Y_e)^{pb} + \frac{21}{2} Y_e^{pb} (Y_e Y_e^\dagger Y_e)^{ar} \right. \right.
\end{aligned}$$

$$\begin{aligned}
& + \frac{35}{2} Y_e^{pr} (Y_e Y_e^\dagger Y_e)^{ab} - \lambda g_Y^2 \left( 6 Y_e^{pr} Y_e^{ab} + 42 Y_e^{pb} Y_e^{ar} \right) \Bigg\} + \left\{ g_L^4 \left( \frac{29}{12} Y_e^{*ab} Y_e^{pr} + \frac{191}{24} \delta^{pa} (Y_e^\dagger Y_e)^{br} - \frac{3}{2} T_2 \delta^{pa} \delta^{rb} - \frac{287}{24} \delta^{rb} (Y_e Y_e^\dagger)^{pa} \right) \right. \\
& + \lambda \left( g_L^2 \left( \frac{9}{2} \delta^{pa} \delta^{rb} \text{Tr} [Y_e^\dagger Y_e] + \frac{27}{2} \delta^{pa} \delta^{rb} \text{Tr} [Y_d^\dagger Y_d] + \frac{93}{4} \delta^{rb} (Y_e Y_e^\dagger)^{pa} - \frac{3}{4} \delta^{pa} (Y_e^\dagger Y_e)^{br} - \frac{3}{2} Y_e^{*ab} Y_e^{pr} \right) + 27 \delta^{pa} \delta^{rb} g_L^4 - \frac{39}{2} \delta^{pa} \delta^{rb} g_Y^2 g_L^2 \right) \\
& + g_Y^2 g_L^2 \left( \frac{1}{8} \delta^{rb} (Y_e Y_e^\dagger)^{pa} - \frac{1}{8} \delta^{pa} (Y_e^\dagger Y_e)^{br} - 7 Y_e^{*ab} Y_e^{pr} - \frac{27}{2} \delta^{pa} \delta^{rb} \text{Tr} [Y_d^\dagger Y_d] - \frac{33}{2} \delta^{pa} \delta^{rb} \text{Tr} [Y_e^\dagger Y_e] - \frac{63}{2} \delta^{pa} \delta^{rb} \text{Tr} [Y_u^\dagger Y_u] \right) + g_L^2 \left( \frac{9}{4} T_2 \delta^{rb} (Y_e Y_e^\dagger)^{pa} \right. \\
& + \frac{13}{4} Y_e^{pr} (Y_e^\dagger Y_e Y_e^\dagger)^{ab} - \frac{3}{4} T_2 \delta^{pa} (Y_e^\dagger Y_e)^{br} - \frac{7}{2} (Y_e^\dagger Y_e)^{br} (Y_e Y_e^\dagger)^{pa} - \frac{63}{8} \delta^{pa} (Y_e^\dagger Y_e Y_e^\dagger Y_e)^{br} - 9 \delta^{pa} \delta^{rb} \text{Tr} [Y_e^\dagger Y_e Y_e^\dagger Y_e] - \frac{23}{2} \delta^{rb} (Y_e Y_e^\dagger Y_e Y_e^\dagger)^{pa} \\
& \left. - 27 \delta^{pa} \delta^{rb} \text{Tr} [Y_d^\dagger Y_d Y_d^\dagger Y_d] \right) + \frac{95}{4} \delta^{pa} \delta^{rb} g_Y^2 g_L^4 + \frac{227}{4} \delta^{pa} \delta^{rb} g_Y^4 g_L^2 + \frac{305}{4} \delta^{pa} \delta^{rb} g_L^6 \Bigg\} C_{eW}^{ab} + C_{eW}^{*ab} \left\{ \lambda g_L^2 \left( 3 Y_e^{pr} Y_e^{ab} + \frac{15}{2} Y_e^{pb} Y_e^{ar} \right) \right. \\
& \left. - g_Y^2 g_L^2 \left( \frac{9}{8} Y_e^{pb} Y_e^{ar} + 4 Y_e^{pr} Y_e^{ab} \right) - g_L^4 \left( \frac{79}{12} Y_e^{pr} Y_e^{ab} + \frac{53}{8} Y_e^{pb} Y_e^{ar} \right) - g_L^2 \left( \frac{3}{2} T_2 Y_e^{pb} Y_e^{ar} + \frac{9}{4} Y_e^{pb} (Y_e Y_e^\dagger Y_e)^{ar} + \frac{21}{8} Y_e^{ar} (Y_e Y_e^\dagger Y_e)^{pb} + \frac{23}{4} Y_e^{pr} (Y_e Y_e^\dagger Y_e)^{ab} \right) \right\} \\
& + \left\{ g_Y^2 \left( \frac{3}{2} Y_e^{pr} (Y_d^\dagger Y_d Y_u^\dagger)^{ab} + \frac{3}{2} Y_e^{pr} (Y_u^\dagger Y_u Y_u^\dagger)^{ab} \right) - \frac{13}{3} g_Y^2 g_L^2 Y_u^{*ab} Y_e^{pr} - 5 \lambda g_Y^2 Y_u^{*ab} Y_e^{pr} - \frac{145}{6} g_Y^4 Y_u^{*ab} Y_e^{pr} \right\} C_{uB}^{ab} + C_{uB}^{*ab} \left\{ g_Y^2 \left( \frac{3}{2} Y_e^{pr} (Y_d Y_d^\dagger Y_u)^{ab} \right. \right. \\
& + \frac{13}{2} Y_e^{pr} (Y_u Y_u^\dagger Y_u)^{ab} \Bigg) - 5 \lambda g_Y^2 Y_e^{pr} Y_u^{ab} - \frac{58}{3} g_Y^2 g_L^2 Y_e^{pr} Y_u^{ab} - \frac{265}{6} g_Y^4 Y_e^{pr} Y_u^{ab} \Bigg\} + \left\{ g_L^2 \left( \frac{39}{4} Y_e^{pr} (Y_u^\dagger Y_u Y_u^\dagger)^{ab} - \frac{27}{4} Y_e^{pr} (Y_d^\dagger Y_d Y_u^\dagger)^{ab} \right) - \frac{9}{4} g_Y^2 g_L^2 Y_u^{*ab} Y_e^{pr} \right. \\
& \left. - \frac{9}{2} \lambda g_L^2 Y_u^{*ab} Y_e^{pr} - 13 g_L^4 Y_u^{*ab} Y_e^{pr} \right\} C_{uW}^{ab} + C_{uW}^{*ab} \left\{ \frac{1}{2} g_L^4 Y_e^{pr} Y_u^{ab} + g_L^2 \left( \frac{39}{4} Y_e^{pr} (Y_u Y_u^\dagger Y_u)^{ab} + \frac{123}{4} Y_e^{pr} (Y_d Y_d^\dagger Y_u)^{ab} \right) - \frac{9}{2} \lambda g_L^2 Y_e^{pr} Y_u^{ab} \right. \\
& \left. - \frac{59}{4} g_Y^2 g_L^2 Y_e^{pr} Y_u^{ab} \right\} + \left\{ \frac{16}{3} g_s^2 g_L^2 Y_u^{*ab} Y_e^{pr} + \frac{16}{3} g_Y^2 g_s^2 Y_u^{*ab} Y_e^{pr} - 16 \lambda g_s^2 Y_u^{*ab} Y_e^{pr} \right\} C_{uG}^{ab} + C_{uG}^{*ab} \left\{ \frac{16}{3} g_s^2 g_L^2 Y_e^{pr} Y_u^{ab} + \frac{16}{3} g_Y^2 g_s^2 Y_e^{pr} Y_u^{ab} \right. \\
& + 16 g_s^2 Y_e^{pr} (Y_u Y_u^\dagger Y_u)^{ab} - 16 \lambda g_s^2 Y_e^{pr} Y_u^{ab} \Bigg\} + \left\{ \lambda g_Y^2 Y_d^{*ab} Y_e^{pr} + \frac{4}{3} g_Y^4 Y_d^{*ab} Y_e^{pr} + \frac{97}{6} g_Y^2 g_L^2 Y_d^{*ab} Y_e^{pr} - g_Y^2 \left( \frac{3}{2} Y_e^{pr} (Y_u^\dagger Y_u Y_d^\dagger)^{ab} \right. \right. \\
& + \frac{5}{2} Y_e^{pr} (Y_d^\dagger Y_d Y_d^\dagger)^{ab} \Bigg) \Bigg\} C_{dB}^{ab} + C_{dB}^{*ab} \left\{ g_Y^2 \left( \frac{105}{2} Y_e^{pr} (Y_d Y_d^\dagger Y_d)^{ab} - \frac{3}{2} Y_e^{pr} (Y_u Y_u^\dagger Y_d)^{ab} \right) + \frac{61}{6} g_Y^2 g_L^2 Y_d^{ab} Y_e^{pr} + \frac{37}{3} g_Y^4 Y_d^{ab} Y_e^{pr} - 26 \lambda g_Y^2 Y_d^{ab} Y_e^{pr} \right\} \\
& + \left\{ g_L^2 \left( \frac{39}{4} Y_e^{pr} (Y_d^\dagger Y_d Y_d^\dagger)^{ab} + \frac{123}{4} Y_e^{pr} (Y_u^\dagger Y_u Y_d^\dagger)^{ab} \right) + \frac{29}{4} g_L^4 Y_d^{*ab} Y_e^{pr} - g_Y^2 g_L^2 Y_d^{*ab} Y_e^{pr} - \frac{9}{2} \lambda g_L^2 Y_d^{*ab} Y_e^{pr} \right\} C_{dW}^{ab} + C_{dW}^{*ab} \left\{ 9 \lambda g_L^2 Y_d^{ab} Y_e^{pr} \right. \\
& \left. - g_L^2 \left( \frac{27}{4} Y_e^{pr} (Y_u Y_u^\dagger Y_d)^{ab} + \frac{69}{4} Y_e^{pr} (Y_d Y_d^\dagger Y_d)^{ab} \right) - \frac{79}{4} g_L^4 Y_d^{ab} Y_e^{pr} \right\} + \left\{ \frac{16}{3} g_s^2 g_L^2 Y_d^{*ab} Y_e^{pr} + \frac{16}{3} g_Y^2 g_s^2 Y_d^{*ab} Y_e^{pr} + 16 g_s^2 Y_e^{pr} (Y_d^\dagger Y_d Y_d^\dagger)^{ab} \right. \\
& \left. - 16 \lambda g_s^2 Y_d^{*ab} Y_e^{pr} \right\} C_{dG}^{ab} + C_{dG}^{*ab} \left\{ \frac{16}{3} g_s^2 g_L^2 Y_d^{ab} Y_e^{pr} + \frac{16}{3} g_Y^2 g_s^2 Y_d^{ab} Y_e^{pr} - 16 \lambda g_s^2 Y_d^{ab} Y_e^{pr} \right\} + \left\{ \frac{1}{8} \delta^{pa} g_L^4 Y_e^{br} + g_Y^2 g_L^2 \left( \frac{13}{27} \delta^{ab} Y_e^{pr} + \frac{61}{2} \delta^{pa} Y_e^{br} \right) \right.
\end{aligned}$$

$$\begin{aligned}
& + g_Y^4 \left( \frac{121}{27} \delta^{ab} Y_e^{pr} + \frac{435}{8} \delta^{pa} Y_e^{br} \right) + \lambda \left( 2 Y_e^{br} (Y_e Y_e^\dagger)^{pa} + \frac{15}{4} \delta^{pa} g_L^2 Y_e^{br} - g_Y^2 \left( \frac{26}{9} \delta^{ab} Y_e^{pr} + \frac{1453}{36} \delta^{pa} Y_e^{br} \right) - 4 T_2 \delta^{pa} Y_e^{br} - \frac{16}{3} Y_e^{pr} (Y_e Y_e^\dagger)^{ba} \right. \\
& - 16 \delta^{pa} (Y_e Y_e^\dagger Y_e)^{br} \left. \right) + g_Y^2 \left( \frac{311}{36} Y_e^{pr} (Y_e Y_e^\dagger)^{ba} + \frac{2695}{72} \delta^{pa} (Y_e Y_e^\dagger Y_e)^{br} - \frac{331}{72} Y_e^{br} (Y_e Y_e^\dagger)^{pa} \right) - (Y_e Y_e^\dagger)^{ba} (Y_e Y_e^\dagger Y_e)^{pr} - T_2 \delta^{pa} (Y_e Y_e^\dagger Y_e)^{br} \\
& - g_L^2 \left( \frac{7}{36} Y_e^{pr} (Y_e Y_e^\dagger)^{ba} + \frac{11}{8} Y_e^{br} (Y_e Y_e^\dagger)^{pa} + \frac{27}{8} \delta^{pa} (Y_e Y_e^\dagger Y_e)^{br} \right) - \frac{25}{12} (Y_e Y_e^\dagger)^{pa} (Y_e Y_e^\dagger Y_e)^{br} - \frac{37}{12} Y_e^{br} (Y_e Y_e^\dagger Y_e Y_e^\dagger)^{pa} - 4 T_4 \delta^{pa} Y_e^{br} \\
& - 10 Y_e^{pr} (Y_e Y_e^\dagger Y_e Y_e^\dagger)^{ba} - 25 \delta^{pa} (Y_e Y_e^\dagger Y_e Y_e^\dagger Y_e)^{br} \left. \right\} C_{H\ell}^{(\parallel)ab} + \left\{ \frac{1}{2} (Y_e Y_e^\dagger)^{ba} (Y_e Y_e^\dagger Y_e)^{pr} + \frac{1}{2} T_2 \delta^{pa} (Y_e Y_e^\dagger Y_e)^{br} + g_L^4 \left( \frac{5}{8} \delta^{pa} Y_e^{br} - \frac{15}{4} \delta^{ab} Y_e^{pr} \right) \right. \\
& + g_Y^2 g_L^2 \left( \frac{83}{108} \delta^{ab} Y_e^{pr} + \frac{283}{24} \delta^{pa} Y_e^{br} \right) + g_Y^4 \left( \frac{121}{54} \delta^{ab} Y_e^{pr} + \frac{673}{12} \delta^{pa} Y_e^{br} \right) + \lambda \left( g_L^2 \left( \frac{8}{3} \delta^{ab} Y_e^{pr} + \frac{185}{12} \delta^{pa} Y_e^{br} \right) + \frac{5}{2} Y_e^{br} (Y_e Y_e^\dagger)^{pa} - g_Y^2 \left( \frac{13}{9} \delta^{ab} Y_e^{pr} \right. \right. \\
& + \frac{1199}{36} \delta^{pa} Y_e^{br} \left. \right) - 8 T_2 \delta^{pa} Y_e^{br} - \frac{29}{3} Y_e^{pr} (Y_e Y_e^\dagger)^{ba} - 11 \delta^{pa} (Y_e Y_e^\dagger Y_e)^{br} \left. \right) + g_L^2 \left( \frac{37}{9} Y_e^{pr} (Y_e Y_e^\dagger)^{ba} - \frac{83}{12} \delta^{pa} (Y_e Y_e^\dagger Y_e)^{br} - \frac{23}{3} Y_e^{br} (Y_e Y_e^\dagger)^{pa} \right) \\
& + g_Y^2 \left( \frac{167}{18} Y_e^{pr} (Y_e Y_e^\dagger)^{ba} + \frac{1441}{36} \delta^{pa} (Y_e Y_e^\dagger Y_e)^{br} - \frac{65}{18} Y_e^{br} (Y_e Y_e^\dagger)^{pa} \right) - \frac{35}{12} (Y_e Y_e^\dagger)^{pa} (Y_e Y_e^\dagger Y_e)^{br} - 4 T_4 \delta^{pa} Y_e^{br} - \frac{53}{12} Y_e^{br} (Y_e Y_e^\dagger Y_e Y_e^\dagger)^{pa} \\
& - 8 Y_e^{pr} (Y_e Y_e^\dagger Y_e Y_e^\dagger)^{ba} - \frac{81}{4} \delta^{pa} (Y_e Y_e^\dagger Y_e Y_e^\dagger Y_e)^{br} - 24 \delta^{pa} Y_e^{br} \text{Tr} \left[ Y_d^\dagger Y_d Y_u^\dagger Y_u \right] \left. \right\} C_{H\ell}^{(\times)ab} + \left\{ g_Y^2 g_L^2 \left( \frac{37}{12} \delta^{rb} Y_e^{pa} - \frac{55}{54} \delta^{ab} Y_e^{pr} \right) + g_Y^4 \left( \frac{323}{54} \delta^{ab} Y_e^{pr} \right. \right. \\
& + \frac{45}{4} \delta^{rb} Y_e^{pa} \left. \right) + (Y_e^\dagger Y_e)^{ba} (Y_e Y_e^\dagger Y_e)^{pr} + T_2 \delta^{rb} (Y_e Y_e^\dagger Y_e)^{pa} + g_L^2 \left( \frac{17}{8} Y_e^{pa} (Y_e^\dagger Y_e)^{br} - \frac{77}{36} Y_e^{pr} (Y_e^\dagger Y_e)^{ba} - \frac{129}{8} \delta^{rb} (Y_e Y_e^\dagger Y_e)^{pa} \right) + \lambda \left( 4 T_2 \delta^{rb} Y_e^{pa} \right. \\
& + \frac{16}{3} Y_e^{pr} (Y_e^\dagger Y_e)^{ba} + \frac{25}{2} \delta^{rb} (Y_e Y_e^\dagger Y_e)^{pa} + \frac{57}{4} \delta^{rb} g_L^2 Y_e^{pa} - g_Y^2 \left( \frac{26}{9} \delta^{ab} Y_e^{pr} + \frac{647}{36} \delta^{rb} Y_e^{pa} \right) - \frac{5}{2} Y_e^{pa} (Y_e^\dagger Y_e)^{br} \left. \right) + g_Y^2 \left( \frac{427}{72} Y_e^{pa} (Y_e^\dagger Y_e)^{br} \right. \\
& + \frac{935}{72} \delta^{rb} (Y_e Y_e^\dagger Y_e)^{pa} - \frac{167}{36} Y_e^{pr} (Y_e^\dagger Y_e)^{ba} \left. \right) + \frac{29}{12} (Y_e^\dagger Y_e)^{br} (Y_e Y_e^\dagger Y_e)^{pa} + 4 T_4 \delta^{rb} Y_e^{pa} + \frac{59}{12} Y_e^{pa} (Y_e^\dagger Y_e Y_e^\dagger Y_e)^{br} + 10 Y_e^{pr} (Y_e^\dagger Y_e Y_e^\dagger Y_e)^{ba} \\
& + \frac{39}{2} \delta^{rb} (Y_e Y_e^\dagger Y_e Y_e^\dagger Y_e)^{pa} - \frac{5}{6} \delta^{rb} g_L^4 Y_e^{pa} \left. \right\} C_{He}^{ab} + \left\{ g_s^2 \left( 40 Y_e^{pr} (Y_d Y_d^\dagger)^{ba} - 40 Y_e^{pr} (Y_u Y_u^\dagger)^{ba} \right) + g_Y^2 \left( \frac{47}{12} Y_e^{pr} (Y_d Y_d^\dagger)^{ba} - \frac{139}{12} Y_e^{pr} (Y_u Y_u^\dagger)^{ba} \right) \right. \\
& + g_L^2 \left( \frac{7}{12} Y_e^{pr} (Y_u Y_u^\dagger)^{ba} - \frac{7}{12} Y_e^{pr} (Y_d Y_d^\dagger)^{ba} \right) + \lambda \left( \frac{26}{9} \delta^{ab} g_Y^2 Y_e^{pr} + 16 Y_e^{pr} (Y_u Y_u^\dagger)^{ba} - 16 Y_e^{pr} (Y_d Y_d^\dagger)^{ba} \right) + 3 (Y_u Y_u^\dagger)^{ba} (Y_e Y_e^\dagger Y_e)^{pr} + 30 Y_e^{pr} (Y_u Y_u^\dagger Y_u Y_u^\dagger)^{ba} \\
& - \frac{13}{27} \delta^{ab} g_Y^2 g_L^2 Y_e^{pr} - \frac{8}{3} \delta^{ab} g_Y^2 g_s^2 Y_e^{pr} - 3 (Y_d Y_d^\dagger)^{ba} (Y_e Y_e^\dagger Y_e)^{pr} - \frac{109}{27} \delta^{ab} g_Y^4 Y_e^{pr} - 30 Y_e^{pr} (Y_d Y_d^\dagger Y_d Y_d^\dagger)^{ba} \left. \right\} C_{Hq}^{(\parallel)ab} + \left\{ \lambda \left( \frac{13}{9} \delta^{ab} g_Y^2 Y_e^{pr} \right. \right. \\
& + 8 \delta^{ab} g_L^2 Y_e^{pr} - 13 Y_e^{pr} (Y_u Y_u^\dagger)^{ba} - 29 Y_e^{pr} (Y_d Y_d^\dagger)^{ba} \left. \right) + g_Y^2 \left( \frac{5}{4} Y_e^{pr} (Y_u Y_u^\dagger)^{ba} + \frac{9}{2} Y_e^{pr} (Y_d Y_d^\dagger)^{ba} \right) + g_L^2 \left( \frac{37}{3} Y_e^{pr} (Y_d Y_d^\dagger)^{ba} + \frac{155}{12} Y_e^{pr} (Y_u Y_u^\dagger)^{ba} \right) \\
& + \frac{3}{2} (Y_d Y_d^\dagger)^{ba} (Y_e Y_e^\dagger Y_e)^{pr} + \frac{217}{108} \delta^{ab} g_Y^2 g_L^2 Y_e^{pr} + \frac{9}{2} (Y_u Y_u^\dagger)^{ba} (Y_e Y_e^\dagger Y_e)^{pr} + 6 Y_e^{pr} (Y_u Y_u^\dagger Y_u Y_u^\dagger)^{ba} + 40 g_s^2 Y_e^{pr} (Y_d Y_d^\dagger)^{ba} - \frac{4}{3} \delta^{ab} g_Y^2 g_s^2 Y_e^{pr} \\
& - \frac{109}{54} \delta^{ab} g_Y^4 Y_e^{pr} - 4 \delta^{ab} g_s^2 g_L^2 Y_e^{pr} - \frac{9}{2} Y_e^{pr} (Y_d Y_d^\dagger Y_u Y_u^\dagger)^{ba} - \frac{9}{2} Y_e^{pr} (Y_u Y_u^\dagger Y_d Y_d^\dagger)^{ba} - \frac{45}{4} \delta^{ab} g_L^4 Y_e^{pr} - 24 Y_e^{pr} (Y_d Y_d^\dagger Y_d Y_d^\dagger)^{ba} \left. \right\} C_{Hq}^{(\times)ab}
\end{aligned}$$

$$\begin{aligned}
& + \left\{ \lambda \left( \frac{52}{9} \delta^{ab} g_Y^2 Y_e^{pr} - 16 Y_e^{pr} (Y_u^\dagger Y_u)^{ba} \right) + \frac{55}{27} \delta^{ab} g_Y^2 g_L^2 Y_e^{pr} + 3 Y_e^{pr} (Y_u^\dagger Y_d Y_d^\dagger Y_u)^{ba} + \frac{59}{12} g_Y^2 Y_e^{pr} (Y_u^\dagger Y_u)^{ba} + \frac{77}{12} g_L^2 Y_e^{pr} (Y_u^\dagger Y_u)^{ba} + 40 g_s^2 Y_e^{pr} (Y_u^\dagger Y_u)^{ba} \right. \\
& - 3 (Y_u^\dagger Y_u)^{ba} (Y_e Y_e^\dagger Y_e)^{pr} - \frac{16}{3} \delta^{ab} g_Y^2 g_s^2 Y_e^{pr} - \frac{263}{27} \delta^{ab} g_Y^4 Y_e^{pr} - 30 Y_e^{pr} (Y_u^\dagger Y_u Y_u^\dagger Y_u)^{ba} \left. \right\} C_{Hu}^{ab} + \left\{ \lambda \left( 16 Y_e^{pr} (Y_d^\dagger Y_d)^{ba} - \frac{26}{9} \delta^{ab} g_Y^2 Y_e^{pr} \right) \right. \\
& + \frac{8}{3} \delta^{ab} g_Y^2 g_s^2 Y_e^{pr} + 3 (Y_d^\dagger Y_d)^{ba} (Y_e Y_e^\dagger Y_e)^{pr} + \frac{227}{54} \delta^{ab} g_Y^4 Y_e^{pr} + 30 Y_e^{pr} (Y_d^\dagger Y_d Y_d^\dagger Y_d)^{ba} - \frac{55}{54} \delta^{ab} g_Y^2 g_L^2 Y_e^{pr} - \frac{31}{12} g_Y^2 Y_e^{pr} (Y_d^\dagger Y_d)^{ba} \\
& - 3 Y_e^{pr} (Y_d^\dagger Y_u Y_u^\dagger Y_d)^{ba} - \frac{77}{12} g_L^2 Y_e^{pr} (Y_d^\dagger Y_d)^{ba} - 40 g_s^2 Y_e^{pr} (Y_d^\dagger Y_d)^{ba} \left. \right\} C_{Hd}^{ab} + \left\{ \frac{3}{2} Y_e^{pr} (Y_d^\dagger Y_d Y_d^\dagger Y_u)^{ba} + \frac{3}{2} Y_e^{pr} (Y_d^\dagger Y_u Y_u^\dagger Y_u)^{ba} + 10 \lambda Y_e^{pr} (Y_d^\dagger Y_u)^{ba} \right. \\
& - \frac{17}{12} g_Y^2 Y_e^{pr} (Y_d^\dagger Y_u)^{ba} - \frac{3}{2} (Y_d^\dagger Y_u)^{ba} (Y_e Y_e^\dagger Y_e)^{pr} - \frac{221}{12} g_L^2 Y_e^{pr} (Y_d^\dagger Y_u)^{ba} \left. \right\} C_{Hud}^{ab} + C_{Hud}^{*ab} \left\{ 16 \lambda Y_e^{pr} (Y_u^\dagger Y_d)^{ab} - \frac{17}{12} g_Y^2 Y_e^{pr} (Y_u^\dagger Y_d)^{ab} \right. \\
& - \frac{3}{2} Y_e^{pr} (Y_u^\dagger Y_d Y_d^\dagger Y_d)^{ab} - \frac{3}{2} Y_e^{pr} (Y_u^\dagger Y_u Y_u^\dagger Y_d)^{ab} - \frac{15}{2} (Y_u^\dagger Y_d)^{ab} (Y_e Y_e^\dagger Y_e)^{pr} - \frac{257}{12} g_L^2 Y_e^{pr} (Y_u^\dagger Y_d)^{ab} \left. \right\} + \left\{ \frac{1}{3} Y_e^{*ad} Y_e^{pc} (Y_e Y_e^\dagger Y_e)^{br} + \frac{2}{3} Y_e^{*ad} Y_e^{br} (Y_e Y_e^\dagger Y_e)^{pc} \right. \\
& + g_Y^4 \left( \frac{13}{2} \delta^{pa} \delta^{rd} Y_e^{bc} - \frac{1}{3} \delta^{rd} \delta^{ab} Y_e^{pc} - \frac{13}{6} \delta^{pa} \delta^{cd} Y_e^{br} \right) + g_Y^2 g_L^2 \left( \frac{4}{3} \delta^{rd} \delta^{ab} Y_e^{pc} - \frac{1}{2} \delta^{pa} \delta^{cd} Y_e^{br} - 5 \delta^{pa} \delta^{rd} Y_e^{bc} \right) + g_L^2 \left( \frac{3}{2} \delta^{pa} Y_e^{bc} (Y_e^\dagger Y_e)^{dr} + \frac{3}{2} \delta^{pa} Y_e^{br} (Y_e^\dagger Y_e)^{dc} \right. \\
& - \delta^{rd} Y_e^{pc} (Y_e Y_e^\dagger)^{ba} - \frac{3}{2} Y_e^{*ad} Y_e^{pc} Y_e^{br} - 9 \delta^{pa} \delta^{rd} (Y_e Y_e^\dagger Y_e)^{bc} \left. \right) + g_Y^2 \left( \frac{25}{18} \delta^{ab} Y_e^{pc} (Y_e^\dagger Y_e)^{dr} + \frac{35}{18} \delta^{cd} Y_e^{br} (Y_e Y_e^\dagger)^{pa} + 13 \delta^{pa} \delta^{rd} (Y_e Y_e^\dagger Y_e)^{bc} - Y_e^{*ad} Y_e^{pc} Y_e^{br} \right. \\
& - \frac{43}{18} \delta^{rd} \delta^{ab} (Y_e Y_e^\dagger Y_e)^{pc} - 4 \delta^{rd} Y_e^{bc} (Y_e Y_e^\dagger)^{pa} - \frac{89}{18} \delta^{pa} \delta^{cd} (Y_e Y_e^\dagger Y_e)^{br} - 8 \delta^{rd} Y_e^{pc} (Y_e Y_e^\dagger)^{ba} - \frac{17}{2} \delta^{pa} Y_e^{bc} (Y_e^\dagger Y_e)^{dr} - \frac{31}{2} \delta^{pa} Y_e^{br} (Y_e^\dagger Y_e)^{dc} \left. \right) \\
& + \delta^{pa} Y_e^{bc} (Y_e^\dagger Y_e Y_e^\dagger Y_e)^{dr} + \delta^{rd} Y_e^{bc} (Y_e Y_e^\dagger Y_e Y_e^\dagger)^{pa} + \lambda \left( g_Y^2 \left( \frac{7}{9} \delta^{rd} \delta^{ab} Y_e^{pc} + \frac{35}{9} \delta^{pa} \delta^{cd} Y_e^{br} - \frac{9}{2} \delta^{pa} \delta^{rd} Y_e^{bc} \right) + 2 \delta^{pa} Y_e^{bc} (Y_e^\dagger Y_e)^{dr} + 2 \delta^{pa} Y_e^{br} (Y_e^\dagger Y_e)^{dc} \right. \\
& + 2 \delta^{rd} Y_e^{bc} (Y_e Y_e^\dagger)^{pa} + 2 \delta^{rd} Y_e^{pc} (Y_e Y_e^\dagger)^{ba} + 2 \delta^{pa} \delta^{rd} Y_e^{bc} \text{Tr} [Y_e^\dagger Y_e] + 10 Y_e^{*ad} Y_e^{pc} Y_e^{br} + 28 \delta^{pa} \delta^{rd} (Y_e Y_e^\dagger Y_e)^{bc} - \frac{3}{2} \delta^{pa} \delta^{rd} g_L^2 Y_e^{bc} - 2 Y_e^{*ad} Y_e^{pr} Y_e^{bc} \left. \right) \\
& + \frac{3}{2} \delta^{pa} \delta^{rd} g_L^4 Y_e^{bc} + 2 \delta^{rd} (Y_e Y_e^\dagger)^{pa} (Y_e Y_e^\dagger Y_e)^{bc} + 4 Y_e^{*ad} Y_e^{pr} (Y_e Y_e^\dagger Y_e)^{bc} - \frac{1}{2} Y_e^{br} (Y_e^\dagger Y_e)^{dc} (Y_e Y_e^\dagger)^{pa} - \frac{1}{2} Y_e^{pc} (Y_e^\dagger Y_e)^{dr} (Y_e Y_e^\dagger)^{ba} - \frac{1}{2} \delta^{rd} (Y_e Y_e^\dagger)^{ba} (Y_e Y_e^\dagger Y_e)^{pc} \\
& - \frac{1}{2} \delta^{pa} (Y_e^\dagger Y_e)^{dc} (Y_e Y_e^\dagger Y_e)^{br} - Y_e^{bc} (Y_e^\dagger Y_e)^{dr} (Y_e Y_e^\dagger)^{pa} - 4 \delta^{pa} \delta^{rd} Y_e^{bc} \text{Tr} [Y_e^\dagger Y_e Y_e^\dagger Y_e] - 10 Y_e^{pc} Y_e^{br} (Y_e^\dagger Y_e Y_e^\dagger)^{ad} - 12 \delta^{pa} Y_e^{br} (Y_e^\dagger Y_e Y_e^\dagger Y_e)^{dc} \\
& - 12 \delta^{rd} Y_e^{pc} (Y_e Y_e^\dagger Y_e Y_e^\dagger)^{ba} - 52 \delta^{pa} \delta^{rd} (Y_e Y_e^\dagger Y_e Y_e^\dagger Y_e)^{bc} \left. \right\} C_{\ell e}^{abcd} + \left\{ \delta^{pa} \delta^{cd} g_Y^2 g_L^2 Y_e^{br} + \lambda \left( 6 \delta^{pa} Y_e^{br} (Y_u^\dagger Y_u)^{dc} - \frac{70}{9} \delta^{pa} \delta^{cd} g_Y^2 Y_e^{br} \right) \right. \\
& + g_Y^2 \left( \frac{89}{9} \delta^{pa} \delta^{cd} (Y_e Y_e^\dagger Y_e)^{br} + \frac{45}{2} \delta^{pa} Y_e^{br} (Y_u^\dagger Y_u)^{dc} - \frac{35}{9} \delta^{cd} Y_e^{br} (Y_e Y_e^\dagger)^{pa} \right) + \frac{3}{2} Y_e^{br} (Y_u^\dagger Y_u)^{dc} (Y_e Y_e^\dagger)^{pa} + \frac{3}{2} \delta^{pa} (Y_u^\dagger Y_u)^{dc} (Y_e Y_e^\dagger Y_e)^{br} + \frac{13}{3} \delta^{pa} \delta^{cd} g_Y^4 Y_e^{br} \\
& + 12 \delta^{pa} Y_e^{br} (Y_u^\dagger Y_u Y_u^\dagger Y_u)^{dc} - \frac{9}{2} \delta^{pa} g_L^2 Y_e^{br} (Y_u^\dagger Y_u)^{dc} \left. \right\} C_{\ell u}^{abcd} + \left\{ \lambda \left( 3 \delta^{pa} Y_e^{br} (Y_d^\dagger Y_d)^{dc} + \frac{35}{9} \delta^{pa} \delta^{cd} g_Y^2 Y_e^{br} \right) + g_Y^2 \left( \frac{3}{2} \delta^{pa} Y_e^{br} (Y_d^\dagger Y_d)^{dc} + \frac{35}{18} \delta^{cd} Y_e^{br} (Y_e Y_e^\dagger)^{pa} \right. \right. \\
& \left. \left. - \frac{89}{18} \delta^{pa} \delta^{cd} (Y_e Y_e^\dagger Y_e)^{br} \right) + \frac{9}{2} \delta^{pa} g_L^2 Y_e^{br} (Y_d^\dagger Y_d)^{dc} - \frac{1}{2} \delta^{pa} \delta^{cd} g_Y^2 g_L^2 Y_e^{br} - \frac{3}{2} Y_e^{br} (Y_d^\dagger Y_d)^{dc} (Y_e Y_e^\dagger)^{pa} - \frac{3}{2} \delta^{pa} (Y_d^\dagger Y_d)^{dc} (Y_e Y_e^\dagger Y_e)^{br} - \frac{13}{6} \delta^{pa} \delta^{cd} g_Y^4 Y_e^{br} \right.
\end{aligned}$$

$$\begin{aligned}
& -30\delta^{pa}Y_e^{br}(Y_d^\dagger Y_d Y_d^\dagger Y_d)^{dc} \Big\} C_{\ell d}^{abcd} + \left\{ \frac{1}{3}\delta^{rd}\delta^{ab}g_Y^4 Y_e^{pc} + g_L^2 \left( 3\delta^{rd}Y_e^{pc}(Y_u Y_u^\dagger)^{ba} - 3\delta^{rd}Y_e^{pc}(Y_d Y_d^\dagger)^{ba} \right) + \lambda \left( 3\delta^{rd}Y_e^{pc}(Y_d Y_d^\dagger)^{ba} + 6\delta^{rd}Y_e^{pc}(Y_u Y_u^\dagger)^{ba} \right. \right. \\
& - \frac{7}{9}\delta^{rd}\delta^{ab}g_Y^2 Y_e^{pc} \Big) + g_Y^2 \left( \frac{43}{18}\delta^{rd}\delta^{ab}(Y_e Y_e^\dagger Y_e)^{pc} + 12\delta^{rd}Y_e^{pc}(Y_u Y_u^\dagger)^{ba} - \frac{25}{18}\delta^{ab}Y_e^{pc}(Y_e^\dagger Y_e)^{dr} \right) + \frac{3}{2}Y_e^{pc}(Y_e^\dagger Y_e)^{dr}(Y_u Y_u^\dagger)^{ba} + \frac{3}{2}\delta^{rd}(Y_u Y_u^\dagger)^{ba}(Y_e Y_e^\dagger Y_e)^{pc} \\
& + 12\delta^{rd}Y_e^{pc}(Y_u Y_u^\dagger Y_u Y_u^\dagger)^{ba} - \frac{4}{3}\delta^{rd}\delta^{ab}g_Y^2 g_L^2 Y_e^{pc} - \frac{3}{2}Y_e^{pc}(Y_e^\dagger Y_e)^{dr}(Y_d Y_d^\dagger)^{ba} - \frac{3}{2}\delta^{rd}(Y_d Y_d^\dagger)^{ba}(Y_e Y_e^\dagger Y_e)^{pc} - 30\delta^{rd}Y_e^{pc}(Y_d Y_d^\dagger Y_d Y_d^\dagger)^{ba} \Big\} C_{qe}^{abcd} \\
& + \left\{ 24Y_e^{pr}Y_u^{bc}(Y_u^\dagger Y_u Y_u^\dagger)^{ad} - 12\lambda Y_u^{*ad}Y_e^{pr}Y_u^{bc} \right\} C_{qu}^{(\parallel)abcd} + \left\{ 72Y_e^{pr}Y_u^{bc}(Y_u^\dagger Y_u Y_u^\dagger)^{ad} - 36\lambda Y_u^{*ad}Y_e^{pr}Y_u^{bc} \right\} C_{qu}^{(\times)abcd} + \left\{ 24Y_d^{*ad}Y_e^{pr}(Y_d Y_d^\dagger Y_d)^{bc} \right. \\
& - 12\lambda Y_d^{*ad}Y_d^{bc}Y_e^{pr} \Big\} C_{qd}^{(\parallel)abcd} + \left\{ 72Y_d^{*ad}Y_e^{pr}(Y_d Y_d^\dagger Y_d)^{bc} - 36\lambda Y_d^{*ad}Y_d^{bc}Y_e^{pr} \right\} C_{qd}^{(\times)abcd} + \left\{ g_Y^4 \left( \frac{2}{3}\delta^{rb}\delta^{ad}Y_e^{pc} - \frac{4}{9}\delta^{ab}\delta^{cd}Y_e^{pr} \right) + \lambda \left( \frac{16}{9}\delta^{rb}\delta^{ad}g_Y^2 Y_e^{pc} \right. \right. \\
& + 8\delta^{rb}Y_e^{pa}(Y_e^\dagger Y_e)^{dc} \Big) + g_Y^2 \left( \frac{8}{3}\delta^{ad}Y_e^{pr}(Y_e^\dagger Y_e)^{bc} + \frac{50}{9}\delta^{ad}Y_e^{pc}(Y_e^\dagger Y_e)^{br} - \frac{26}{9}\delta^{rb}\delta^{ad}(Y_e Y_e^\dagger Y_e)^{pc} - 46\delta^{rb}Y_e^{pa}(Y_e^\dagger Y_e)^{dc} \right) + 2Y_e^{pa}(Y_e^\dagger Y_e)^{br}(Y_e^\dagger Y_e)^{dc} \\
& + \frac{10}{3}\delta^{rb}\delta^{ad}g_Y^2 g_L^2 Y_e^{pc} + 8\delta^{rb}Y_e^{pa}(Y_e^\dagger Y_e Y_e^\dagger Y_e)^{dc} - 2\delta^{rb}(Y_e^\dagger Y_e)^{dc}(Y_e Y_e^\dagger Y_e)^{pa} - 4Y_e^{pr}(Y_e^\dagger Y_e)^{ba}(Y_e^\dagger Y_e)^{dc} - 14\delta^{rb}g_L^2 Y_e^{pa}(Y_e^\dagger Y_e)^{dc} \Big\} C_{ee}^{abcd} \\
& + \left\{ \frac{16}{3}\delta^{ad}g_Y^2 Y_e^{pr}(Y_u^\dagger Y_u)^{bc} - \frac{16}{27}\delta^{ad}\delta^{bc}g_Y^4 Y_e^{pr} - 12Y_e^{pr}(Y_u^\dagger Y_u)^{bc}(Y_u^\dagger Y_u)^{da} \right\} C_{uu}^{abcd} + \left\{ \frac{8}{3}\delta^{ad}g_Y^2 Y_e^{pr}(Y_d^\dagger Y_d)^{bc} - \frac{4}{27}\delta^{ad}\delta^{bc}g_Y^4 Y_e^{pr} \right. \\
& - 12Y_e^{pr}(Y_d^\dagger Y_d)^{bc}(Y_d^\dagger Y_d)^{da} \Big\} C_{dd}^{abcd} + \left\{ \frac{2}{3}\delta^{rb}\delta^{cd}g_Y^4 Y_e^{pa} + g_Y^2 \left( \frac{43}{9}\delta^{rb}\delta^{cd}(Y_e Y_e^\dagger Y_e)^{pa} + 18\delta^{rb}Y_e^{pa}(Y_u^\dagger Y_u)^{dc} - \frac{25}{9}\delta^{cd}Y_e^{pa}(Y_e^\dagger Y_e)^{br} \right) + 15\delta^{rb}g_L^2 Y_e^{pa}(Y_u^\dagger Y_u)^{dc} \right. \\
& - \lambda \left( \frac{14}{9}\delta^{rb}\delta^{cd}g_Y^2 Y_e^{pa} + 6\delta^{rb}Y_e^{pa}(Y_u^\dagger Y_u)^{dc} \right) - \frac{3}{2}Y_e^{pa}(Y_e^\dagger Y_e)^{br}(Y_u^\dagger Y_u)^{dc} - \frac{3}{2}\delta^{rb}(Y_u^\dagger Y_u)^{dc}(Y_e Y_e^\dagger Y_e)^{pa} - \frac{8}{3}\delta^{rb}\delta^{cd}g_Y^2 g_L^2 Y_e^{pa} \\
& - 12\delta^{rb}Y_e^{pa}(Y_u^\dagger Y_u Y_u^\dagger Y_u)^{dc} \Big\} C_{eu}^{abcd} + \left\{ \lambda \left( \frac{7}{9}\delta^{rb}\delta^{cd}g_Y^2 Y_e^{pa} + 15\delta^{rb}Y_e^{pa}(Y_d^\dagger Y_d)^{dc} \right) + g_Y^2 \left( \frac{25}{18}\delta^{cd}Y_e^{pa}(Y_e^\dagger Y_e)^{br} - \frac{43}{18}\delta^{rb}\delta^{cd}(Y_e Y_e^\dagger Y_e)^{pa} - 6\delta^{rb}Y_e^{pa}(Y_d^\dagger Y_d)^{dc} \right) \right. \\
& + \frac{4}{3}\delta^{rb}\delta^{cd}g_Y^2 g_L^2 Y_e^{pa} + \frac{3}{2}Y_e^{pa}(Y_d^\dagger Y_d)^{dc}(Y_e^\dagger Y_e)^{br} + \frac{3}{2}\delta^{rb}(Y_d^\dagger Y_d)^{dc}(Y_e Y_e^\dagger Y_e)^{pa} - \frac{1}{3}\delta^{rb}\delta^{cd}g_Y^4 Y_e^{pa} - 6\delta^{rb}Y_e^{pa}(Y_d^\dagger Y_d Y_d^\dagger Y_d)^{dc} \\
& - 15\delta^{rb}g_L^2 Y_e^{pa}(Y_d^\dagger Y_d)^{dc} \Big\} C_{ed}^{abcd} + \left\{ g_Y^2 \left( \frac{21}{8}\delta^{pa}Y_d^{dc}(Y_e^\dagger Y_e)^{br} + \frac{43}{6}\delta^{pa}\delta^{rb}(Y_d Y_d^\dagger Y_d)^{dc} - \frac{33}{8}\delta^{rb}Y_d^{dc}(Y_e Y_e^\dagger)^{pa} \right) + g_L^2 \left( \frac{9}{8}\delta^{rb}Y_d^{dc}(Y_e Y_e^\dagger)^{pa} \right. \right. \\
& + \frac{27}{2}\delta^{pa}\delta^{rb}(Y_d Y_d^\dagger Y_d)^{dc} - \frac{27}{8}\delta^{pa}Y_d^{dc}(Y_e^\dagger Y_e)^{br} \Big) + \lambda \left( 40\delta^{pa}\delta^{rb}g_s^2 Y_d^{dc} - \frac{3}{2}\delta^{pa}\delta^{rb}(Y_d Y_d^\dagger Y_d)^{dc} - 3\delta^{pa}\delta^{rb}Y_d^{dc}\text{Tr}[Y_e^\dagger Y_e] - \frac{19}{6}\delta^{pa}\delta^{rb}g_Y^2 Y_d^{dc} \right. \\
& - \frac{9}{2}\delta^{pa}\delta^{rb}g_L^2 Y_d^{dc} - 9\delta^{pa}Y_d^{dc}(Y_e^\dagger Y_e)^{br} - \frac{21}{2}\delta^{rb}Y_d^{dc}(Y_e Y_e^\dagger)^{pa} - \frac{21}{2}\delta^{pa}\delta^{rb}(Y_u Y_u^\dagger Y_d)^{dc} \Big) + \frac{5}{4}\delta^{pa}\delta^{rb}g_Y^4 Y_d^{dc} + \frac{3}{2}Y_d^{dc}(Y_e^\dagger Y_e)^{br}(Y_e Y_e^\dagger)^{pa} + \frac{9}{2}\delta^{pa}\delta^{rb}g_Y^2 g_L^2 Y_d^{dc} \\
& + 6\delta^{pa}\delta^{rb}Y_d^{dc}\text{Tr}[Y_e^\dagger Y_e Y_e^\dagger Y_e] + 12\delta^{pa}(Y_e^\dagger Y_e)^{br}(Y_d Y_d^\dagger Y_d)^{dc} + 12\delta^{rb}(Y_e Y_e^\dagger)^{pa}(Y_d Y_d^\dagger Y_d)^{dc} + 60\delta^{pa}\delta^{rb}(Y_d Y_d^\dagger Y_d Y_d^\dagger Y_d)^{dc} - \frac{3}{2}\delta^{pa}Y_d^{dc}(Y_e^\dagger Y_e Y_e^\dagger Y_e)^{br}
\end{aligned}$$



$$\begin{aligned}
& -\frac{3}{2}\delta^{rb}Y_d^{dc}(Y_eY_e^\dagger Y_eY_e^\dagger)^{pa} - \frac{9}{4}\delta^{pa}\delta^{rb}g_L^4Y_d^{dc} - 6\delta^{rb}(Y_eY_e^\dagger)^{pa}(Y_uY_u^\dagger Y_d)^{dc} - 6\delta^{pa}\delta^{rb}(Y_dY_d^\dagger Y_uY_u^\dagger Y_d)^{dc} - 6\delta^{pa}\delta^{rb}(Y_uY_u^\dagger Y_dY_d^\dagger Y_d)^{dc} \\
& - 64\delta^{pa}\delta^{rb}g_s^2(Y_dY_d^\dagger Y_d)^{dc} \left\{ C_{ledq}^{abcd} + C_{ledq}^{*abcd} \left\{ \frac{3}{2}g_Y^2Y_d^{*dc}Y_e^{pb}Y_e^{ar} + \frac{9}{4}g_L^2Y_d^{*dc}Y_e^{pb}Y_e^{ar} + 6Y_d^{*dc}Y_e^{pr}(Y_eY_e^\dagger Y_e)^{ab} + 15Y_e^{pb}Y_e^{ar}(Y_d^\dagger Y_dY_d^\dagger)^{dc} \right. \right. \\
& - \frac{1}{2}Y_d^{*dc}Y_e^{pb}(Y_eY_e^\dagger Y_e)^{ar} - \lambda \left( 3Y_d^{*dc}Y_e^{pr}Y_e^{ab} + 15Y_d^{*dc}Y_e^{pb}Y_e^{ar} \right) - Y_d^{*dc}Y_e^{ar}(Y_eY_e^\dagger Y_e)^{pb} \left. \right\} + \left\{ g_L^2 \left( \frac{27}{8}\delta^{pa}Y_u^{*cd}(Y_e^\dagger Y_e)^{br} - \frac{9}{8}\delta^{rb}Y_u^{*cd}(Y_eY_e^\dagger)^{pa} \right) \right. \\
& + g_Y^2 \left( \frac{33}{8}\delta^{rb}Y_u^{*cd}(Y_eY_e^\dagger)^{pa} + \frac{16}{3}\delta^{pa}\delta^{rb}(Y_u^\dagger Y_uY_u^\dagger)^{cd} - \frac{21}{8}\delta^{pa}Y_u^{*cd}(Y_e^\dagger Y_e)^{br} \right) + \lambda \left( \frac{3}{2}\delta^{pa}\delta^{rb}(Y_u^\dagger Y_uY_u^\dagger)^{cd} + 3\delta^{pa}\delta^{rb}Y_u^{*cd}\text{Tr}[Y_e^\dagger Y_e] + 9\delta^{pa}Y_u^{*cd}(Y_e^\dagger Y_e)^{br} \right. \\
& + \frac{21}{2}\delta^{rb}Y_u^{*cd}(Y_eY_e^\dagger)^{pa} + \frac{21}{2}\delta^{pa}\delta^{rb}(Y_d^\dagger Y_dY_u^\dagger)^{cd} - \frac{9}{4}\delta^{pa}\delta^{rb}g_L^2Y_u^{*cd} - \frac{49}{12}\delta^{pa}\delta^{rb}g_Y^2Y_u^{*cd} - 40\delta^{pa}\delta^{rb}g_s^2Y_u^{*cd} \left. \right) + \frac{3}{2}\delta^{pa}Y_u^{*cd}(Y_e^\dagger Y_eY_e^\dagger Y_e)^{br} \\
& + \frac{3}{2}\delta^{rb}Y_u^{*cd}(Y_eY_e^\dagger Y_eY_e^\dagger)^{pa} + \frac{9}{4}\delta^{pa}\delta^{rb}g_L^4Y_u^{*cd} + \frac{19}{4}\delta^{pa}\delta^{rb}g_Y^4Y_u^{*cd} + 6\delta^{rb}(Y_eY_e^\dagger)^{pa}(Y_d^\dagger Y_dY_u^\dagger)^{cd} + 6\delta^{pa}\delta^{rb}(Y_u^\dagger Y_dY_d^\dagger Y_uY_u^\dagger)^{dc} \\
& + 6\delta^{pa}\delta^{rb}(Y_u^\dagger Y_uY_u^\dagger Y_dY_d^\dagger)^{dc} + 64\delta^{pa}\delta^{rb}g_s^2(Y_u^\dagger Y_uY_u^\dagger)^{cd} - \frac{3}{2}Y_u^{*cd}(Y_e^\dagger Y_e)^{br}(Y_eY_e^\dagger)^{pa} - 6\delta^{pa}\delta^{rb}Y_u^{*cd}\text{Tr}[Y_e^\dagger Y_eY_e^\dagger Y_e] - \frac{21}{2}\delta^{pa}\delta^{rb}g_Y^2g_L^2Y_u^{*cd} \\
& - 12\delta^{pa}(Y_e^\dagger Y_e)^{br}(Y_u^\dagger Y_uY_u^\dagger)^{cd} - 12\delta^{rb}(Y_eY_e^\dagger)^{pa}(Y_u^\dagger Y_uY_u^\dagger)^{cd} - 60\delta^{pa}\delta^{rb}(Y_u^\dagger Y_uY_u^\dagger Y_uY_u^\dagger)^{dc} \left. \right\} C_{lequ}^{abcd} + C_{lequ}^{*abcd} \left\{ \frac{1}{2}Y_e^{pb}Y_u^{cd}(Y_eY_e^\dagger Y_e)^{ar} \right. \\
& + \lambda \left( 3Y_e^{pr}Y_e^{ab}Y_u^{cd} + 15Y_e^{pb}Y_e^{ar}Y_u^{cd} \right) + Y_e^{ar}Y_u^{cd}(Y_eY_e^\dagger Y_e)^{pb} - \frac{3}{2}g_Y^2Y_e^{pb}Y_e^{ar}Y_u^{cd} - \frac{9}{4}g_L^2Y_e^{pb}Y_e^{ar}Y_u^{cd} - 6Y_e^{pr}Y_u^{cd}(Y_eY_e^\dagger Y_e)^{ab} - 15Y_e^{pb}Y_e^{ar}(Y_uY_u^\dagger Y_u)^{cd} \left. \right\} \\
& + \left\{ \frac{3}{4}Y_u^{*cb}(Y_e^\dagger Y_e)^{dr}(Y_eY_e^\dagger)^{pa} + g_Y^2 \left( \frac{111}{16}\delta^{pa}Y_u^{*cb}(Y_e^\dagger Y_e)^{dr} + \frac{31}{4}\delta^{pa}\delta^{rd}(Y_u^\dagger Y_uY_u^\dagger)^{cb} - \frac{33}{16}\delta^{rd}Y_u^{*cb}(Y_eY_e^\dagger)^{pa} \right) + g_L^2 \left( 9\delta^{pa}\delta^{rd}(Y_d^\dagger Y_dY_u^\dagger)^{cb} \right. \right. \\
& + \frac{45}{4}\delta^{pa}\delta^{rd}(Y_u^\dagger Y_uY_u^\dagger)^{cb} - \frac{3}{16}\delta^{rd}Y_u^{*cb}(Y_eY_e^\dagger)^{pa} - \frac{69}{16}\delta^{pa}Y_u^{*cb}(Y_e^\dagger Y_e)^{dr} \left. \right) + \lambda \left( \frac{239}{24}\delta^{pa}\delta^{rd}g_Y^2Y_u^{*cb} + 34\delta^{pa}\delta^{rd}g_s^2Y_u^{*cb} - \frac{3}{4}\delta^{pa}\delta^{rd}(Y_u^\dagger Y_uY_u^\dagger)^{cb} \right. \\
& - \frac{9}{8}\delta^{pa}\delta^{rd}g_L^2Y_u^{*cb} - \frac{3}{2}\delta^{pa}\delta^{rd}Y_u^{*cb}\text{Tr}[Y_e^\dagger Y_e] - \frac{15}{4}\delta^{pa}\delta^{rd}(Y_d^\dagger Y_dY_u^\dagger)^{cb} - \frac{9}{2}\delta^{pa}Y_u^{*cb}(Y_e^\dagger Y_e)^{dr} - \frac{21}{4}\delta^{rd}Y_u^{*cb}(Y_eY_e^\dagger)^{pa} \left. \right) + 3\delta^{pa}\delta^{rd}Y_u^{*cb}\text{Tr}[Y_e^\dagger Y_eY_e^\dagger Y_e] \\
& + \frac{9}{2}\delta^{pa}\delta^{rd}g_L^4Y_u^{*cb} + 6\delta^{pa}(Y_e^\dagger Y_e)^{dr}(Y_u^\dagger Y_uY_u^\dagger)^{cb} + 6\delta^{rd}(Y_eY_e^\dagger)^{pa}(Y_u^\dagger Y_uY_u^\dagger)^{cb} + 7\delta^{pa}\delta^{rd}g_Y^4Y_u^{*cb} + 30\delta^{pa}\delta^{rd}(Y_u^\dagger Y_uY_u^\dagger Y_uY_u^\dagger)^{bc} \\
& - \frac{3}{4}\delta^{pa}Y_u^{*cb}(Y_e^\dagger Y_eY_e^\dagger Y_e)^{dr} - \frac{3}{4}\delta^{rd}Y_u^{*cb}(Y_eY_e^\dagger Y_eY_e^\dagger)^{pa} - 3\delta^{rd}(Y_eY_e^\dagger)^{pa}(Y_d^\dagger Y_dY_u^\dagger)^{cb} - 3\delta^{pa}\delta^{rd}(Y_u^\dagger Y_dY_d^\dagger Y_dY_d^\dagger)^{bc} - 3\delta^{pa}\delta^{rd}(Y_u^\dagger Y_dY_d^\dagger Y_uY_u^\dagger)^{bc} \\
& - 3\delta^{pa}\delta^{rd}(Y_u^\dagger Y_uY_u^\dagger Y_dY_d^\dagger)^{bc} - \frac{7}{2}\delta^{pa}\delta^{rd}g_Y^2g_L^2Y_u^{*cb} - 60\delta^{pa}\delta^{rd}g_s^2(Y_u^\dagger Y_uY_u^\dagger)^{cb} \left. \right\} C_{luqe}^{abcd} + C_{luqe}^{*abcd} \left\{ \frac{9}{4}g_L^2Y_e^{pd}Y_e^{ar}Y_u^{cb} + 3Y_e^{pr}Y_u^{cb}(Y_eY_e^\dagger Y_e)^{ad} \right. \\
& + \frac{15}{2}Y_e^{pd}Y_e^{ar}(Y_uY_u^\dagger Y_u)^{cb} + \frac{33}{4}g_Y^2Y_e^{pd}Y_e^{ar}Y_u^{cb} - \frac{1}{4}Y_e^{pd}Y_u^{cb}(Y_eY_e^\dagger Y_e)^{ar} - \frac{1}{2}Y_e^{ar}Y_u^{cb}(Y_eY_e^\dagger Y_e)^{pd} - \lambda \left( \frac{3}{2}Y_e^{pr}Y_e^{ad}Y_u^{cb} + \frac{15}{2}Y_e^{pd}Y_e^{ar}Y_u^{cb} \right) \left. \right\} + \left\{ g_L^4 \left( \frac{3}{2}\delta^{pa}\delta^{bc}Y_e^{dr} \right. \right. \\
& - \frac{2}{9}\delta^{ad}\delta^{bc}Y_e^{pr} \left. \right) + Y_e^{br}(Y_eY_e^\dagger)^{pa}(Y_eY_e^\dagger)^{dc} + \lambda \left( g_Y^2 \left( \frac{5}{9}\delta^{pa}\delta^{bc}Y_e^{dr} + \frac{70}{9}\delta^{pa}\delta^{cd}Y_e^{br} \right) + 8\delta^{pa}Y_e^{br}(Y_eY_e^\dagger)^{dc} - \frac{1}{3}\delta^{pa}\delta^{bc}g_L^2Y_e^{dr} \right) + \delta^{pa}(Y_eY_e^\dagger)^{dc}(Y_eY_e^\dagger Y_e)^{br}
\end{aligned}$$

$$\begin{aligned}
& + g_Y^2 \left( \frac{35}{18} \delta^{bc} Y_e^{dr} (Y_e Y_e^\dagger)^{pa} + \frac{35}{9} \delta^{cd} Y_e^{br} (Y_e Y_e^\dagger)^{pa} - \frac{5}{18} \delta^{pa} \delta^{bc} (Y_e Y_e^\dagger Y_e)^{dr} - \frac{4}{3} \delta^{bc} Y_e^{pr} (Y_e Y_e^\dagger)^{da} - \frac{89}{9} \delta^{pa} \delta^{cd} (Y_e Y_e^\dagger Y_e)^{br} - 29 \delta^{pa} Y_e^{dr} (Y_e Y_e^\dagger)^{bc} \right. \\
& - 41 \delta^{pa} Y_e^{br} (Y_e Y_e^\dagger)^{dc} \Big) + g_L^2 \left( \frac{5}{6} \delta^{pa} \delta^{bc} (Y_e Y_e^\dagger Y_e)^{dr} + \frac{4}{3} \delta^{bc} Y_e^{pr} (Y_e Y_e^\dagger)^{da} - \frac{1}{6} \delta^{bc} Y_e^{dr} (Y_e Y_e^\dagger)^{pa} - 3 \delta^{pa} Y_e^{br} (Y_e Y_e^\dagger)^{dc} - 6 \delta^{pa} Y_e^{dr} (Y_e Y_e^\dagger)^{bc} \right. \\
& + 8 \delta^{pa} Y_e^{dr} (Y_e Y_e^\dagger Y_e Y_e^\dagger)^{bc} - g_Y^2 g_L^2 \left( \frac{1}{3} \delta^{pa} \delta^{bc} Y_e^{dr} + \delta^{pa} \delta^{cd} Y_e^{br} \right) - g_Y^4 \left( \frac{1}{6} \delta^{pa} \delta^{bc} Y_e^{dr} + \frac{2}{9} \delta^{ad} \delta^{bc} Y_e^{pr} + \frac{13}{3} \delta^{pa} \delta^{cd} Y_e^{br} \right) - Y_e^{dr} (Y_e Y_e^\dagger)^{pa} (Y_e Y_e^\dagger)^{bc} \\
& - 2 \delta^{pa} (Y_e Y_e^\dagger)^{bc} (Y_e Y_e^\dagger Y_e)^{dr} - 4 Y_e^{pr} (Y_e Y_e^\dagger)^{bc} (Y_e Y_e^\dagger)^{da} \Big\} C_{\ell\ell}^{abcd} + \left\{ g_Y^2 \left( \frac{4}{3} \delta^{bc} Y_e^{pr} (Y_d Y_d^\dagger)^{da} - \frac{4}{3} \delta^{bc} Y_e^{pr} (Y_u Y_u^\dagger)^{da} \right) + g_L^2 \left( 4 \delta^{bc} Y_e^{pr} (Y_d Y_d^\dagger)^{da} + 4 \delta^{bc} Y_e^{pr} (Y_u Y_u^\dagger)^{da} \right) \right. \\
& - \frac{2}{27} \delta^{ad} \delta^{bc} g_Y^4 Y_e^{pr} - \frac{2}{3} \delta^{ad} \delta^{bc} g_L^4 Y_e^{pr} - 12 Y_e^{pr} (Y_d Y_d^\dagger)^{bc} (Y_d Y_d^\dagger)^{da} - 12 Y_e^{pr} (Y_u Y_u^\dagger)^{bc} (Y_u Y_u^\dagger)^{da} \Big\} C_{qq}^{(\parallel)abcd} + \left\{ g_Y^2 \left( \frac{8}{3} \delta^{bc} Y_e^{pr} (Y_d Y_d^\dagger)^{da} - \frac{8}{3} \delta^{bc} Y_e^{pr} (Y_u Y_u^\dagger)^{da} \right) \right. \\
& + 24 Y_e^{pr} (Y_d Y_d^\dagger)^{da} (Y_u Y_u^\dagger)^{bc} - \frac{4}{27} \delta^{ad} \delta^{bc} g_Y^4 Y_e^{pr} - 12 Y_e^{pr} (Y_d Y_d^\dagger)^{bc} (Y_d Y_d^\dagger)^{da} - 12 Y_e^{pr} (Y_u Y_u^\dagger)^{bc} (Y_u Y_u^\dagger)^{da} \Big\} C_{qq}^{(\times)abcd} + \left\{ \frac{1}{2} \delta^{pa} \delta^{cd} g_Y^2 g_L^2 Y_e^{br} \right. \\
& + \lambda \left( 15 \delta^{pa} Y_e^{br} (Y_d Y_d^\dagger)^{dc} - \frac{35}{9} \delta^{pa} \delta^{cd} g_Y^2 Y_e^{br} - 6 \delta^{pa} Y_e^{br} (Y_u Y_u^\dagger)^{dc} \right) + g_L^2 \left( \frac{9}{2} \delta^{pa} Y_e^{br} (Y_u Y_u^\dagger)^{dc} - \frac{9}{2} \delta^{pa} Y_e^{br} (Y_d Y_d^\dagger)^{dc} \right) + g_Y^2 \left( \frac{89}{18} \delta^{pa} \delta^{cd} (Y_e Y_e^\dagger Y_e)^{br} \right. \\
& + \frac{75}{2} \delta^{pa} Y_e^{br} (Y_u Y_u^\dagger)^{dc} - \frac{35}{18} \delta^{cd} Y_e^{br} (Y_e Y_e^\dagger)^{pa} - \frac{27}{2} \delta^{pa} Y_e^{br} (Y_d Y_d^\dagger)^{dc} \Big) + \frac{3}{2} Y_e^{br} (Y_d Y_d^\dagger)^{dc} (Y_e Y_e^\dagger)^{pa} + \frac{3}{2} \delta^{pa} (Y_d Y_d^\dagger)^{dc} (Y_e Y_e^\dagger Y_e)^{br} + \frac{13}{6} \delta^{pa} \delta^{cd} g_Y^4 Y_e^{br} \\
& - \frac{3}{2} Y_e^{br} (Y_e Y_e^\dagger)^{pa} (Y_u Y_u^\dagger)^{dc} - \frac{3}{2} \delta^{pa} (Y_u Y_u^\dagger)^{dc} (Y_e Y_e^\dagger Y_e)^{br} - 6 \delta^{pa} Y_e^{br} (Y_d Y_d^\dagger Y_d Y_d^\dagger)^{dc} - 12 \delta^{pa} Y_e^{br} (Y_u Y_u^\dagger Y_u Y_u^\dagger)^{dc} \Big\} C_{\ell q}^{(\parallel)abcd} + \left\{ \lambda \left( 6 \delta^{pa} Y_e^{br} (Y_u Y_u^\dagger)^{dc} \right. \right. \\
& + 30 \delta^{pa} Y_e^{br} (Y_d Y_d^\dagger)^{dc} - \frac{35}{18} \delta^{pa} \delta^{cd} g_Y^2 Y_e^{br} - \frac{7}{2} \delta^{pa} \delta^{cd} g_L^2 Y_e^{br} \Big) + g_L^2 \left( \frac{5}{4} \delta^{pa} \delta^{cd} (Y_e Y_e^\dagger Y_e)^{br} - \frac{1}{4} \delta^{cd} Y_e^{br} (Y_e Y_e^\dagger)^{pa} - \frac{9}{2} \delta^{pa} Y_e^{br} (Y_u Y_u^\dagger)^{dc} - 9 \delta^{pa} Y_e^{br} (Y_d Y_d^\dagger)^{dc} \right) \\
& + g_Y^2 \left( \frac{89}{36} \delta^{pa} \delta^{cd} (Y_e Y_e^\dagger Y_e)^{br} - \frac{35}{36} \delta^{cd} Y_e^{br} (Y_e Y_e^\dagger)^{pa} - \frac{27}{2} \delta^{pa} Y_e^{br} (Y_d Y_d^\dagger)^{dc} \right) + \frac{13}{12} \delta^{pa} \delta^{cd} g_Y^4 Y_e^{br} + \frac{9}{4} \delta^{pa} \delta^{cd} g_L^4 Y_e^{br} + \frac{7}{2} \delta^{pa} \delta^{cd} g_Y^2 g_L^2 Y_e^{br} \\
& + \frac{57}{2} \delta^{pa} Y_e^{br} (Y_d Y_d^\dagger Y_u Y_u^\dagger)^{dc} - \frac{3}{2} Y_e^{br} (Y_d Y_d^\dagger)^{dc} (Y_e Y_e^\dagger)^{pa} - \frac{3}{2} \delta^{pa} (Y_u Y_u^\dagger)^{dc} (Y_e Y_e^\dagger Y_e)^{br} - 3 Y_e^{br} (Y_e Y_e^\dagger)^{pa} (Y_u Y_u^\dagger)^{dc} - \frac{9}{2} \delta^{pa} Y_e^{br} (Y_u Y_u^\dagger Y_d Y_d^\dagger)^{dc} \\
& \left. - 24 \delta^{pa} Y_e^{br} (Y_d Y_d^\dagger Y_d Y_d^\dagger)^{dc} \right\} C_{\ell q}^{(\times)abcd}, \tag{7.2}
\end{aligned}$$

## 7.2 $C_{uH}$

$$\begin{aligned}
\beta_{C_{uH}^{pr}}^{(1)} & = \left\{ \frac{17}{12} g_L^2 Y_u^{pr} - \frac{1}{12} g_Y^2 Y_u^{pr} - \lambda Y_u^{pr} - \frac{3}{2} \left( (Y_d Y_d^\dagger Y_u)^{pr} - (Y_u Y_u^\dagger Y_u)^{pr} \right) \right\} C_{HD}^{(\parallel)} + \left\{ \lambda Y_u^{pr} + (Y_u Y_u^\dagger Y_u)^{pr} - \frac{1}{6} g_Y^2 Y_u^{pr} - \frac{3}{2} g_L^2 Y_u^{pr} \right\} C_{HD}^{(\times)} \\
& + \frac{17}{3} g_Y^4 C_{HB} Y_u^{pr} - \frac{17i}{3} g_Y^4 C_{H\tilde{B}} Y_u^{pr} + 9 g_L^4 C_{HW} Y_u^{pr} - 9i g_L^4 C_{H\tilde{W}} Y_u^{pr} + 32 g_s^4 C_{HG} Y_u^{pr} - 32i g_s^4 C_{H\tilde{G}} Y_u^{pr} - \frac{1}{2} g_Y^2 g_L^2 C_{HWB} Y_u^{pr} \\
& + \frac{i}{2} g_Y^2 g_L^2 C_{H\tilde{W}B} Y_u^{pr} + 2 C_{eH}^{*ab} Y_e^{ab} Y_u^{pr} + \left\{ \frac{1}{2} \left( 6 T_2 \delta^{pa} \delta^{rb} + 10 \delta^{pa} (Y_u^\dagger Y_u)^{br} + 11 \delta^{rb} (Y_u Y_u^\dagger)^{pa} + 12 Y_u^{*ab} Y_u^{pr} - 3 \delta^{rb} (Y_d Y_d^\dagger)^{pa} \right) + 12 \delta^{pa} \delta^{rb} \lambda \right.
\end{aligned}$$

$$\begin{aligned}
& -\frac{35}{12}\delta^{pa}\delta^{rb}g_Y^2 - \frac{27}{4}\delta^{pa}\delta^{rb}g_L^2 - 8\delta^{pa}\delta^{rb}g_s^2 \Big\} C_{uH}^{ab} - \delta^{pa}C_{dH}^{ab}(Y_d^\dagger Y_u)^{br} + 2C_{dH}^{*ab} \Big\{ 3Y_d^{ab}Y_u^{pr} - Y_d^{pb}Y_u^{ar} \Big\} + \Big\{ 5\delta^{pa}\delta^{rb}g_Y^4 + 5g_Y^2 \Big( \delta^{pa}(Y_u^\dagger Y_u)^{br} \\
& + \delta^{rb}(Y_u Y_u^\dagger)^{pa} \Big) - 3\delta^{pa}\delta^{rb}g_Y^2 g_L^2 \Big\} C_{uB}^{ab} + \Big\{ \frac{3}{2}g_L^2 \Big( \delta^{pa}(Y_u^\dagger Y_u)^{br} + 4\delta^{rb}(Y_d Y_d^\dagger)^{pa} - \delta^{rb}(Y_u Y_u^\dagger)^{pa} \Big) + \frac{9}{2}\delta^{pa}\delta^{rb}g_L^4 - \frac{5}{2}\delta^{pa}\delta^{rb}g_Y^2 g_L^2 \Big\} C_{uW}^{ab} \\
& + 16g_s^2 \Big\{ \delta^{pa}(Y_u^\dagger Y_u)^{br} + \delta^{rb}(Y_u Y_u^\dagger)^{pa} \Big\} C_{uG}^{ab} + 3\delta^{pa}g_L^2 C_{dW}^{ab}(Y_d^\dagger Y_u)^{br} + \Big\{ \frac{2}{3}\delta^{ab}g_Y^2 Y_u^{pr} + 2Y_u^{pr}(Y_e Y_e^\dagger)^{ba} \Big\} C_{H\ell}^{(\parallel)ab} + \Big\{ \frac{1}{3}\delta^{ab}g_Y^2 Y_u^{pr} + 2Y_u^{pr}(Y_e Y_e^\dagger)^{ba} \\
& - \frac{1}{3}\delta^{ab}g_L^2 Y_u^{pr} \Big\} C_{H\ell}^{(\times)ab} + \Big\{ \frac{2}{3}\delta^{ab}g_Y^2 Y_u^{pr} - 2Y_u^{pr}(Y_e^\dagger Y_e)^{ba} \Big\} C_{He}^{ab} + \Big\{ \frac{2}{3}g_Y^2 \Big( 6\delta^{pa}Y_u^{br} - \delta^{ab}Y_u^{pr} \Big) + 2 \Big( 3Y_u^{pr}(Y_d Y_d^\dagger)^{ba} - \delta^{pa}(Y_u Y_u^\dagger Y_u)^{br} - 3Y_u^{pr}(Y_u Y_u^\dagger)^{ba} \Big) \\
& - 2\delta^{pa}\lambda Y_u^{br} \Big\} C_{Hq}^{(\parallel)ab} + \Big\{ 2\delta^{pa}\lambda Y_u^{br} + 3\delta^{pa}(Y_d Y_d^\dagger Y_u)^{br} + 6Y_u^{pr}(Y_d Y_d^\dagger)^{ba} - \frac{1}{3}\delta^{ab}g_Y^2 Y_u^{pr} - \delta^{ab}g_L^2 Y_u^{pr} - \delta^{pa}(Y_u Y_u^\dagger Y_u)^{br} \Big\} C_{Hq}^{(\times)ab} + \Big\{ \frac{1}{3}g_Y^2 \Big( 3\delta^{rb}Y_u^{pa} \\
& - 4\delta^{ab}Y_u^{pr} \Big) + 2\delta^{rb}\lambda Y_u^{pa} + 2 \Big( \delta^{rb}(Y_u Y_u^\dagger Y_u)^{pa} + 3Y_u^{pr}(Y_u^\dagger Y_u)^{ba} \Big) - 3\delta^{rb}g_L^2 Y_u^{pa} \Big\} C_{Hu}^{ab} + \Big\{ \frac{2}{3}\delta^{ab}g_Y^2 Y_u^{pr} - 6Y_u^{pr}(Y_d^\dagger Y_d)^{ba} \Big\} C_{Hd}^{ab} + C_{Hud}^{*ab} \Big\{ 3\delta^{ra}g_L^2 Y_d^{pb} \\
& - 2\delta^{ra}\lambda Y_d^{pb} - 2\delta^{ra}(Y_d Y_d^\dagger Y_d)^{pb} \Big\} + \Big\{ 8\delta^{pa}\delta^{rd}(Y_u Y_u^\dagger Y_u)^{bc} - 4\delta^{pa}\delta^{rd}\lambda Y_u^{bc} \Big\} C_{qu}^{(\parallel)abcd} + \Big\{ 24\delta^{pa}\delta^{rd}(Y_u Y_u^\dagger Y_u)^{bc} - 12\delta^{pa}\delta^{rd}\lambda Y_u^{bc} \Big\} C_{qu}^{(\times)abcd} \\
& + \Big\{ \lambda \Big( \delta^{pc}\delta^{rb}Y_d^{*ad} + 6\delta^{pa}\delta^{rb}Y_d^{*cd} \Big) - 2 \Big( \delta^{pc}\delta^{rb}(Y_d^\dagger Y_d Y_d^\dagger)^{ad} + 6\delta^{pa}\delta^{rb}(Y_d^\dagger Y_d Y_d^\dagger)^{cd} \Big) \Big\} C_{quqd}^{(\parallel)abcd} + \Big\{ \lambda \Big( 2\delta^{pa}\delta^{rb}Y_d^{*cd} + 3\delta^{pc}\delta^{rb}Y_d^{*ad} \\
& - 2 \Big( 2\delta^{pa}\delta^{rb}(Y_d^\dagger Y_d Y_d^\dagger)^{cd} + 3\delta^{pc}\delta^{rb}(Y_d^\dagger Y_d Y_d^\dagger)^{ad} \Big) \Big\} C_{quqd}^{(\times)abcd} + \Big\{ 4\delta^{pc}\delta^{rd}(Y_e^\dagger Y_e Y_e^\dagger)^{ab} - 2\delta^{pc}\delta^{rd}\lambda Y_e^{*ab} \Big\} C_{lequ}^{abcd} + \Big\{ \delta^{pc}\delta^{rb}\lambda Y_e^{*ad} \\
& - 2\delta^{pc}\delta^{rb}(Y_e^\dagger Y_e Y_e^\dagger)^{ad} \Big\} C_{luqe}^{abcd}, \tag{7.3}
\end{aligned}$$

$$\begin{aligned}
\beta_{C_{uH}^{pr}}^{(2)} &= \frac{11}{6}g_L^2 Y_u^{pr} \mathbf{T}_{\ell H} + \frac{19}{6}g_Y^2 Y_u^{pr} \mathbf{T}_{\ell H} - 5 \Big( (Y_d Y_d^\dagger Y_u)^{pr} \mathbf{T}_{\ell H} - 3(Y_u Y_u^\dagger Y_u)^{pr} \mathbf{T}_{\ell H} \Big) - 6Y_u^{pr} \text{Tr} \Big[ C_{\ell H H}^\dagger C_{\ell H H} Y_e Y_e^\dagger \Big] - 24\lambda Y_u^{pr} \mathbf{T}_{\ell H} + \Big\{ 24\lambda Y_u^{pr} \\
& - 48(Y_u Y_u^\dagger Y_u)^{pr} \Big\} C_H + \Big\{ \frac{1}{2}\lambda^2 Y_u^{pr} + \frac{61}{108}g_Y^2 g_L^2 Y_u^{pr} + \lambda \Big( 2(Y_d Y_d^\dagger Y_u)^{pr} + \frac{9}{4}g_L^2 Y_u^{pr} + \frac{163}{36}g_Y^2 Y_u^{pr} + 5\mathbf{T}_2 Y_u^{pr} - \frac{53}{2}(Y_u Y_u^\dagger Y_u)^{pr} \Big) \\
& + g_Y^2 \Big( \frac{1}{12}\mathbf{T}_2 Y_u^{pr} + \frac{49}{48}(Y_u Y_u^\dagger Y_u)^{pr} - \frac{43}{48}(Y_d Y_d^\dagger Y_u)^{pr} \Big) + g_s^2 \Big( 16(Y_u Y_u^\dagger Y_u)^{pr} - 16(Y_d Y_d^\dagger Y_u)^{pr} \Big) + \frac{5}{2}\mathbf{T}_2(Y_d Y_d^\dagger Y_u)^{pr} + \frac{25}{8}(Y_u Y_u^\dagger Y_u Y_u^\dagger Y_u)^{pr} \\
& + \frac{77}{8}(Y_d Y_d^\dagger Y_d Y_d^\dagger Y_u)^{pr} + \frac{45}{2}Y_u^{pr} \text{Tr} \Big[ Y_d^\dagger Y_d Y_u^\dagger Y_u \Big] - g_L^2 \Big( \frac{7}{16}(Y_d Y_d^\dagger Y_u)^{pr} + \frac{17}{12}\mathbf{T}_2 Y_u^{pr} + \frac{23}{16}(Y_u Y_u^\dagger Y_u)^{pr} \Big) - (Y_u Y_u^\dagger Y_d Y_d^\dagger Y_u)^{pr}
\end{aligned}$$

$$\begin{aligned}
& -2(Y_d Y_d^\dagger Y_u Y_u^\dagger Y_u)^{pr} - \frac{73}{36} g_Y^4 Y_u^{pr} - \frac{71}{24} g_L^4 Y_u^{pr} - \frac{13}{4} T_4 Y_u^{pr} - \frac{9}{2} T_2 (Y_u Y_u^\dagger Y_u)^{pr} \Big\} C_{HD}^{(II)} + \left\{ \frac{1}{4} (Y_d Y_d^\dagger Y_u Y_u^\dagger Y_u)^{pr} + \frac{1}{2} (Y_d Y_d^\dagger Y_d Y_d^\dagger Y_u)^{pr} \right. \\
& + \lambda^2 Y_u^{pr} + \lambda \left( \frac{287}{36} g_Y^2 Y_u^{pr} + \frac{51}{4} g_L^2 Y_u^{pr} - \frac{1}{2} (Y_d Y_d^\dagger Y_u)^{pr} - 31 (Y_u Y_u^\dagger Y_u)^{pr} \right) + g_Y^2 \left( \frac{1}{18} (Y_u Y_u^\dagger Y_u)^{pr} + \frac{1}{6} T_2 Y_u^{pr} + \frac{23}{12} (Y_d Y_d^\dagger Y_u)^{pr} \right) + g_L^2 \left( \frac{3}{2} T_2 Y_u^{pr} \right. \\
& + \frac{23}{8} (Y_d Y_d^\dagger Y_u)^{pr} + \frac{43}{8} (Y_u Y_u^\dagger Y_u)^{pr} \Big) + (Y_u Y_u^\dagger Y_d Y_d^\dagger Y_u)^{pr} + \frac{133}{96} g_L^4 Y_u^{pr} + 2 (Y_u Y_u^\dagger Y_u Y_u^\dagger Y_u)^{pr} + \frac{32}{3} g_s^2 (Y_u Y_u^\dagger Y_u)^{pr} - \frac{241}{288} g_Y^4 Y_u^{pr} - \frac{7}{4} T_4 Y_u^{pr} \\
& - 3 T_2 (Y_u Y_u^\dagger Y_u)^{pr} - \frac{2275}{432} g_Y^2 g_L^2 Y_u^{pr} - \frac{27}{2} Y_u^{pr} \text{Tr}[Y_d^\dagger Y_d Y_u^\dagger Y_u] \Big\} C_{HD}^{(*)} + \left\{ g_Y^4 \left( \frac{43}{12} (Y_d Y_d^\dagger Y_u)^{pr} + \frac{53}{6} Y_u^{pr} \text{Tr}[Y_d^\dagger Y_d] - \frac{79}{6} Y_u^{pr} \text{Tr}[Y_u^\dagger Y_u] \right. \right. \\
& - \frac{43}{2} Y_u^{pr} \text{Tr}[Y_e^\dagger Y_e] - \frac{1511}{36} (Y_u Y_u^\dagger Y_u)^{pr} \Big) + \frac{553}{18} \lambda g_Y^4 Y_u^{pr} - \frac{76}{9} g_Y^4 g_s^2 Y_u^{pr} - 10 g_Y^4 g_L^2 Y_u^{pr} - \frac{2894}{27} g_Y^6 Y_u^{pr} \Big\} C_{HB} + \left\{ g_Y^4 \left( \frac{11i}{12} (Y_d Y_d^\dagger Y_u)^{pr} \right. \right. \\
& + \frac{3i}{2} Y_u^{pr} \text{Tr}[Y_d^\dagger Y_d] + \frac{33i}{2} Y_u^{pr} \text{Tr}[Y_u^\dagger Y_u] + \frac{487i}{12} (Y_u Y_u^\dagger Y_u)^{pr} - \frac{39i}{2} Y_u^{pr} \text{Tr}[Y_e^\dagger Y_e] \Big) + \frac{68i}{3} g_Y^4 g_s^2 Y_u^{pr} + \frac{425i}{18} \lambda g_Y^4 Y_u^{pr} + \frac{4037i}{108} g_Y^6 Y_u^{pr} \\
& - \frac{59i}{12} g_Y^4 g_L^2 Y_u^{pr} \Big\} C_{H\bar{B}} + \left\{ g_L^4 \left( \frac{3}{2} T_2 Y_u^{pr} - \frac{51}{4} (Y_d Y_d^\dagger Y_u)^{pr} - \frac{243}{4} (Y_u Y_u^\dagger Y_u)^{pr} \right) + \frac{77}{3} g_L^6 Y_u^{pr} + \frac{147}{2} \lambda g_L^4 Y_u^{pr} - \frac{38}{3} g_Y^2 g_L^4 Y_u^{pr} \right. \\
& - 36 g_s^2 g_L^4 Y_u^{pr} \Big\} C_{HW} + \left\{ g_L^4 \left( \frac{27i}{2} Y_u^{pr} \text{Tr}[Y_u^\dagger Y_u] + \frac{57i}{4} (Y_d Y_d^\dagger Y_u)^{pr} + \frac{213i}{4} (Y_u Y_u^\dagger Y_u)^{pr} - \frac{9i}{2} Y_u^{pr} \text{Tr}[Y_e^\dagger Y_e] - \frac{27i}{2} Y_u^{pr} \text{Tr}[Y_d^\dagger Y_d] \right) \right. \\
& + \frac{51i}{2} \lambda g_L^4 Y_u^{pr} + 36i g_s^2 g_L^4 Y_u^{pr} - \frac{59i}{12} g_Y^2 g_L^4 Y_u^{pr} - \frac{341i}{4} g_L^6 Y_u^{pr} \Big\} C_{H\widetilde{W}} + \left\{ g_s^4 \left( 64 (Y_d Y_d^\dagger Y_u)^{pr} - 176 Y_u^{pr} \text{Tr}[Y_d^\dagger Y_d] - 176 Y_u^{pr} \text{Tr}[Y_u^\dagger Y_u] \right. \right. \\
& - \frac{584}{3} (Y_u Y_u^\dagger Y_u)^{pr} \Big) + 864 g_s^6 Y_u^{pr} - \frac{76}{9} g_Y^2 g_s^4 Y_u^{pr} - \frac{64}{3} \lambda g_s^4 Y_u^{pr} - 36 g_s^4 g_L^2 Y_u^{pr} \Big\} C_{HG} + \left\{ g_s^4 \left( 32i (Y_d Y_d^\dagger Y_u)^{pr} + 144i Y_u^{pr} \text{Tr}[Y_u^\dagger Y_u] \right. \right. \\
& + 280i (Y_u Y_u^\dagger Y_u)^{pr} - 144i Y_u^{pr} \text{Tr}[Y_d^\dagger Y_d] \Big) + \frac{68i}{3} g_Y^2 g_s^4 Y_u^{pr} + 36i g_s^4 g_L^2 Y_u^{pr} + \frac{544i}{3} \lambda g_s^4 Y_u^{pr} - \frac{1760i}{3} g_s^6 Y_u^{pr} \Big\} C_{H\widetilde{G}} + \left\{ g_Y^2 g_L^2 \left( \frac{5}{4} (Y_u Y_u^\dagger Y_u)^{pr} \right. \right. \\
& + \frac{23}{4} Y_u^{pr} \text{Tr}[Y_e^\dagger Y_e] + \frac{25}{4} Y_u^{pr} \text{Tr}[Y_d^\dagger Y_d] + \frac{47}{4} Y_u^{pr} \text{Tr}[Y_u^\dagger Y_u] - \frac{5}{12} (Y_d Y_d^\dagger Y_u)^{pr} \Big) + \frac{181}{12} \lambda g_Y^2 g_L^2 Y_u^{pr} - \frac{1}{36} g_Y^2 g_L^4 Y_u^{pr} - \frac{26}{3} g_Y^2 g_s^2 g_L^2 Y_u^{pr} \\
& - \frac{88}{9} g_Y^4 g_L^2 Y_u^{pr} \Big\} C_{HWB} + \left\{ \frac{7i}{12} g_Y^4 g_L^2 Y_u^{pr} + \frac{8i}{9} g_Y^2 g_L^4 Y_u^{pr} + g_Y^2 g_L^2 \left( \frac{9i}{4} Y_u^{pr} \text{Tr}[Y_d^\dagger Y_d] + \frac{15i}{4} Y_u^{pr} \text{Tr}[Y_e^\dagger Y_e] - \frac{5i}{6} (Y_d Y_d^\dagger Y_u)^{pr} - \frac{9i}{2} (Y_u Y_u^\dagger Y_u)^{pr} \right. \right. \\
& - \frac{27i}{4} Y_u^{pr} \text{Tr}[Y_u^\dagger Y_u] \Big) - 2i g_Y^2 g_s^2 g_L^2 Y_u^{pr} - \frac{45i}{4} \lambda g_Y^2 g_L^2 Y_u^{pr} \Big\} C_{H\widetilde{WB}} + \left\{ g_L^6 \left( 3 T_2 Y_u^{pr} - \frac{9}{4} (Y_u Y_u^\dagger Y_u)^{pr} - 3 (Y_d Y_d^\dagger Y_u)^{pr} \right) + \frac{103}{12} g_L^8 Y_u^{pr} \right. \\
& - 6 \lambda g_L^6 Y_u^{pr} - \frac{29}{4} g_Y^2 g_L^6 Y_u^{pr} \Big\} C_W + \left\{ g_L^6 \left( \frac{9i}{4} (Y_u Y_u^\dagger Y_u)^{pr} + 12i (Y_d Y_d^\dagger Y_u)^{pr} \right) - \frac{29i}{6} g_Y^2 g_L^6 Y_u^{pr} - 39i g_L^8 Y_u^{pr} \right\} C_{\widetilde{W}} - \left\{ 28 g_s^6 (Y_u Y_u^\dagger Y_u)^{pr} + 88 \lambda g_s^6 Y_u^{pr} \right\} C_G
\end{aligned}$$

$$\begin{aligned}
& + \left\{ 140ig_s^6(Y_u Y_u^\dagger Y_u)^{pr} - 24i\lambda g_s^6 Y_u^{pr} \right\} C_{\tilde{G}} + \left\{ \frac{3}{2} Y_e^{*ab} (Y_d Y_d^\dagger Y_u)^{pr} + 5\lambda Y_e^{*ab} Y_u^{pr} - 5Y_u^{pr} (Y_e^\dagger Y_e Y_e^\dagger)^{ab} - 5Y_e^{*ab} (Y_u Y_u^\dagger Y_u)^{pr} \right\} C_{eH}^{ab} \\
& + C_{eH}^{*ab} \left\{ Y_e^{ab} (Y_d Y_d^\dagger Y_u)^{pr} + \frac{13}{4} g_Y^2 Y_e^{ab} Y_u^{pr} + 5\lambda Y_e^{ab} Y_u^{pr} - \frac{9}{4} g_L^2 Y_e^{ab} Y_u^{pr} - \frac{13}{2} Y_e^{ab} (Y_u Y_u^\dagger Y_u)^{pr} - 14Y_u^{pr} (Y_e Y_e^\dagger Y_e)^{ab} \right\} + \left\{ \frac{1}{4} \delta^{rb} (Y_u Y_u^\dagger Y_d Y_d^\dagger)^{pa} \right. \\
& + \lambda \left( 15Y_u^{*ab} Y_u^{pr} + 18\delta^{pa} \delta^{rb} g_Y^2 + 54\delta^{pa} \delta^{rb} g_L^2 - 24T_2 \delta^{pa} \delta^{rb} - 42\delta^{pa} (Y_u^\dagger Y_u)^{br} - 42\delta^{rb} (Y_u Y_u^\dagger)^{pa} \right) + g_L^2 \left( \frac{57}{16} \delta^{rb} (Y_d Y_d^\dagger)^{pa} + \frac{45}{8} T_2 \delta^{pa} \delta^{rb} \right. \\
& + \frac{171}{8} \delta^{pa} (Y_u^\dagger Y_u)^{br} + \frac{387}{16} \delta^{rb} (Y_u Y_u^\dagger)^{pa} - \frac{27}{4} Y_u^{*ab} Y_u^{pr} \left. \right) + g_Y^2 \left( \frac{25}{8} \delta^{pa} \delta^{rb} \text{Tr}[Y_d^\dagger Y_d] + \frac{75}{8} \delta^{pa} \delta^{rb} \text{Tr}[Y_e^\dagger Y_e] + \frac{85}{8} \delta^{pa} \delta^{rb} \text{Tr}[Y_u^\dagger Y_u] + \frac{827}{72} \delta^{pa} (Y_u^\dagger Y_u)^{br} \right. \\
& + \frac{1793}{144} \delta^{rb} (Y_u Y_u^\dagger)^{pa} - \frac{43}{48} \delta^{rb} (Y_d Y_d^\dagger)^{pa} - \frac{23}{12} Y_u^{*ab} Y_u^{pr} \left. \right) + g_s^2 \left( \frac{104}{3} \delta^{rb} (Y_u Y_u^\dagger)^{pa} + \frac{112}{3} \delta^{pa} (Y_u^\dagger Y_u)^{br} + 40Y_u^{*ab} Y_u^{pr} + 60\delta^{pa} \delta^{rb} \text{Tr}[Y_d^\dagger Y_d] \right. \\
& + 60\delta^{pa} \delta^{rb} \text{Tr}[Y_u^\dagger Y_u] - 16\delta^{rb} (Y_d Y_d^\dagger)^{pa} \left. \right) + \frac{5}{4} T_2 \delta^{rb} (Y_d Y_d^\dagger)^{pa} + \frac{19}{9} \delta^{pa} \delta^{rb} g_Y^2 g_s^2 + \frac{21}{8} \delta^{pa} \delta^{rb} g_Y^2 g_L^2 + 3Y_u^{*ab} (Y_d Y_d^\dagger Y_u)^{pr} + \frac{17}{4} \delta^{pa} (Y_u^\dagger Y_d Y_d^\dagger Y_u)^{br} \\
& + \frac{15}{2} Y_u^{pr} (Y_d^\dagger Y_d Y_u^\dagger)^{ab} + \frac{35}{4} \delta^{rb} (Y_d Y_d^\dagger Y_d Y_d^\dagger)^{pa} + 9\delta^{pa} \delta^{rb} g_s^2 g_L^2 + \frac{7711}{432} \delta^{pa} \delta^{rb} g_Y^4 - \frac{1}{2} (Y_u^\dagger Y_u)^{br} (Y_d Y_d^\dagger)^{pa} - \delta^{rb} (Y_d Y_d^\dagger Y_u Y_u^\dagger)^{pa} - \frac{5}{2} (Y_u^\dagger Y_u)^{br} (Y_u Y_u^\dagger)^{pa} \\
& - \frac{11}{4} T_4 \delta^{pa} \delta^{rb} - \frac{13}{2} T_2 \delta^{pa} (Y_u^\dagger Y_u)^{br} - \frac{29}{4} T_2 \delta^{rb} (Y_u Y_u^\dagger)^{pa} - \frac{31}{4} \delta^{rb} (Y_u Y_u^\dagger Y_u Y_u^\dagger)^{pa} - \frac{17}{2} \delta^{pa} (Y_u^\dagger Y_u Y_u^\dagger Y_u)^{br} - \frac{201}{16} \delta^{pa} \delta^{rb} g_L^4 \\
& - \frac{39}{2} Y_u^{*ab} (Y_u Y_u^\dagger Y_u)^{pr} - \frac{39}{2} \delta^{pa} \delta^{rb} \text{Tr}[Y_d^\dagger Y_d Y_u^\dagger Y_u] - 42Y_u^{pr} (Y_u^\dagger Y_u Y_u^\dagger)^{ab} - \frac{153}{2} \delta^{pa} \delta^{rb} \lambda^2 - 108\delta^{pa} \delta^{rb} g_s^4 \left. \right\} C_{uH}^{ab} + C_{uH}^{*ab} \left\{ \lambda \left( 15Y_u^{pr} Y_u^{ab} \right. \right. \\
& - 18Y_u^{pb} Y_u^{ar} \left. \right) + \frac{3}{2} g_L^2 Y_u^{pb} Y_u^{ar} + \frac{9}{2} Y_u^{ab} (Y_d Y_d^\dagger Y_u)^{pr} + \frac{9}{2} Y_u^{pr} (Y_d Y_d^\dagger Y_u)^{ab} + \frac{11}{2} Y_u^{pb} (Y_u Y_u^\dagger Y_u)^{ar} + \frac{23}{4} Y_u^{ar} (Y_u Y_u^\dagger Y_u)^{pb} + \frac{35}{6} g_Y^2 Y_u^{pb} Y_u^{ar} + 40g_s^2 Y_u^{pb} Y_u^{ar} \\
& - \frac{1}{2} Y_u^{pb} (Y_d Y_d^\dagger Y_u)^{ar} - \frac{7}{4} Y_u^{ar} (Y_d Y_d^\dagger Y_u)^{pb} - 15Y_u^{ab} (Y_u Y_u^\dagger Y_u)^{pr} - 15Y_u^{pr} (Y_u Y_u^\dagger Y_u)^{ab} \left. \right\} + \left\{ \frac{11}{72} \delta^{pa} g_Y^2 (Y_d^\dagger Y_u)^{br} + \frac{1}{4} (Y_d^\dagger Y_u)^{br} (Y_u Y_u^\dagger)^{pa} \right. \\
& + \frac{1}{2} T_2 \delta^{pa} (Y_d^\dagger Y_u)^{br} + \frac{11}{4} (Y_d^\dagger Y_u)^{br} (Y_d Y_d^\dagger)^{pa} + \frac{9}{2} Y_u^{pr} (Y_u^\dagger Y_u Y_d^\dagger)^{ab} + \frac{9}{2} Y_d^{*ab} (Y_d Y_d^\dagger Y_u)^{pr} + 5\delta^{pa} (Y_d^\dagger Y_d Y_d^\dagger Y_u)^{br} + \frac{51}{8} \delta^{pa} g_L^2 (Y_d^\dagger Y_u)^{br} + 15\lambda Y_d^{*ab} Y_u^{pr} \\
& - \frac{1}{2} \delta^{pa} (Y_d^\dagger Y_u Y_u^\dagger Y_u)^{br} - 15Y_u^{pr} (Y_d^\dagger Y_d Y_d^\dagger)^{ab} - 15Y_d^{*ab} (Y_u Y_u^\dagger Y_u)^{pr} - \frac{56}{3} \delta^{pa} g_s^2 (Y_d^\dagger Y_u)^{br} \left. \right\} C_{dH}^{ab} + C_{dH}^{*ab} \left\{ g_s^2 \left( 40Y_d^{ab} Y_u^{pr} - \frac{40}{3} Y_d^{pb} Y_u^{ar} \right) + g_L^2 \left( \frac{3}{2} Y_d^{pb} Y_u^{ar} \right. \right. \\
& - \frac{27}{4} Y_d^{ab} Y_u^{pr} \left. \right) + \lambda \left( 3Y_d^{pb} Y_u^{ar} + 15Y_d^{ab} Y_u^{pr} \right) + 2T_2 Y_d^{pb} Y_u^{ar} + \frac{11}{4} Y_u^{ar} (Y_u Y_u^\dagger Y_d)^{pb} + 3Y_d^{ab} (Y_d Y_d^\dagger Y_u)^{pr} + \frac{23}{4} Y_u^{ar} (Y_d Y_d^\dagger Y_d)^{pb} + \frac{15}{2} Y_u^{pr} (Y_u Y_u^\dagger Y_d)^{ab} \\
& + \frac{19}{2} Y_d^{pb} (Y_d Y_d^\dagger Y_u)^{ar} - g_Y^2 \left( \frac{35}{18} Y_d^{pb} Y_u^{ar} + \frac{83}{12} Y_d^{ab} Y_u^{pr} \right) - 2Y_d^{pb} (Y_u Y_u^\dagger Y_u)^{ar} - \frac{39}{2} Y_d^{ab} (Y_u Y_u^\dagger Y_u)^{pr} - 42Y_u^{pr} (Y_d Y_d^\dagger Y_d)^{ab} \left. \right\} + \left\{ \frac{1}{3} g_Y^2 g_L^2 Y_e^{*ab} Y_u^{pr} \right. \\
& + 3\lambda g_Y^2 Y_e^{*ab} Y_u^{pr} + \frac{31}{6} g_Y^4 Y_e^{*ab} Y_u^{pr} - \frac{1}{2} g_Y^2 Y_u^{pr} (Y_e^\dagger Y_e Y_e^\dagger)^{ab} \left. \right\} C_{eB}^{ab} + C_{eB}^{*ab} \left\{ 3\lambda g_Y^2 Y_e^{ab} Y_u^{pr} + \frac{19}{6} g_Y^4 Y_e^{ab} Y_u^{pr} + \frac{13}{3} g_Y^2 g_L^2 Y_e^{ab} Y_u^{pr} \right.
\end{aligned}$$

$$\begin{aligned}
& -\frac{7}{2}g_Y^2 Y_u^{pr} (Y_e Y_e^\dagger Y_e)^{ab} \Bigg\} + \left\{ \frac{13}{4}g_L^2 Y_u^{pr} (Y_e^\dagger Y_e Y_e^\dagger)^{ab} - \frac{3}{4}g_Y^2 g_L^2 Y_e^{*ab} Y_u^{pr} - \frac{3}{2}\lambda g_L^2 Y_e^{*ab} Y_u^{pr} - \frac{13}{3}g_L^4 Y_e^{*ab} Y_u^{pr} \right\} C_{eW}^{ab} + C_{eW}^{*ab} \left\{ \frac{1}{6}g_L^4 Y_e^{ab} Y_u^{pr} \right. \\
& + \frac{13}{4}g_L^2 Y_u^{pr} (Y_e Y_e^\dagger Y_e)^{ab} - \frac{3}{2}\lambda g_L^2 Y_e^{ab} Y_u^{pr} - \frac{27}{4}g_Y^2 g_L^2 Y_e^{ab} Y_u^{pr} \Bigg\} + \left\{ g_Y^4 \left( \delta^{rb} (Y_d Y_d^\dagger)^{pa} + \frac{25}{3}\delta^{pa}\delta^{rb} \text{Tr}[Y_d^\dagger Y_d] + \frac{80}{9}Y_u^{*ab} Y_u^{pr} - \frac{2713}{108}\delta^{rb} (Y_u Y_u^\dagger)^{pa} \right. \right. \\
& - \frac{95}{3}\delta^{pa}\delta^{rb} \text{Tr}[Y_u^\dagger Y_u] - \frac{125}{3}\delta^{pa}\delta^{rb} \text{Tr}[Y_e^\dagger Y_e] - \frac{1612}{27}\delta^{pa} (Y_u^\dagger Y_u)^{br} \Bigg) + g_Y^2 g_L^2 \left( \frac{151}{12}\delta^{rb} (Y_u Y_u^\dagger)^{pa} - 9\delta^{pa}\delta^{rb} \text{Tr}[Y_d^\dagger Y_d] - \frac{28}{3}\delta^{rb} (Y_d Y_d^\dagger)^{pa} \right. \\
& - 11\delta^{pa}\delta^{rb} \text{Tr}[Y_e^\dagger Y_e] - \frac{71}{6}\delta^{pa} (Y_u^\dagger Y_u)^{br} - \frac{77}{6}Y_u^{*ab} Y_u^{pr} - 21\delta^{pa}\delta^{rb} \text{Tr}[Y_u^\dagger Y_u] \Bigg) + \lambda \left( g_Y^2 \left( \frac{26}{3}\delta^{rb} (Y_d Y_d^\dagger)^{pa} + 15\delta^{pa}\delta^{rb} \text{Tr}[Y_u^\dagger Y_u] + \frac{275}{6}\delta^{pa} (Y_u^\dagger Y_u)^{br} \right. \right. \\
& - 5Y_u^{*ab} Y_u^{pr} - \frac{35}{6}\delta^{rb} (Y_u Y_u^\dagger)^{pa} \Bigg) + \frac{160}{9}\delta^{pa}\delta^{rb} g_Y^2 g_s^2 + \frac{985}{27}\delta^{pa}\delta^{rb} g_Y^4 - 19\delta^{pa}\delta^{rb} g_Y^2 g_L^2 \Bigg) + g_Y^2 \left( \frac{1}{6}(Y_u^\dagger Y_u)^{br} (Y_d Y_d^\dagger)^{pa} + \frac{3}{2}\text{T}_2\delta^{pa} (Y_u^\dagger Y_u)^{br} \right. \\
& + \frac{3}{2}Y_u^{pr} (Y_d^\dagger Y_d Y_u^\dagger)^{ab} + 2\delta^{rb} (Y_d Y_d^\dagger Y_u Y_u^\dagger)^{pa} + \frac{13}{2}Y_u^{pr} (Y_u^\dagger Y_u Y_u^\dagger)^{ab} + \frac{101}{12}\delta^{rb} (Y_u Y_u^\dagger Y_d Y_d^\dagger)^{pa} + 15\delta^{pa} (Y_u^\dagger Y_d Y_d^\dagger Y_u)^{br} - \frac{3}{2}\text{T}_2\delta^{rb} (Y_u Y_u^\dagger)^{pa} \\
& - 3\delta^{rb} (Y_d Y_d^\dagger Y_d Y_d^\dagger)^{pa} - 30\delta^{pa}\delta^{rb} \text{Tr}[Y_u^\dagger Y_u Y_u^\dagger Y_u] - \frac{185}{6}\delta^{rb} (Y_u Y_u^\dagger Y_u Y_u^\dagger)^{pa} - \frac{443}{12}\delta^{pa} (Y_u^\dagger Y_u Y_u^\dagger Y_u)^{br} \Bigg) + \frac{4}{3}\delta^{pa}\delta^{rb} g_Y^2 g_L^4 + \frac{32}{3}\delta^{pa}\delta^{rb} g_Y^2 g_s^2 g_L^2 \\
& + \frac{55}{3}\delta^{pa}\delta^{rb} g_Y^4 g_L^2 - g_Y^2 g_s^2 \left( \frac{88}{9}\delta^{pa} (Y_u^\dagger Y_u)^{br} + \frac{232}{9}\delta^{rb} (Y_u Y_u^\dagger)^{pa} \right) - \frac{160}{9}\delta^{pa}\delta^{rb} g_Y^4 g_s^2 - \frac{5845}{54}\delta^{pa}\delta^{rb} g_Y^6 \Bigg\} C_{uB}^{ab} + C_{uB}^{*ab} \left\{ g_Y^2 g_L^2 \left( \frac{7}{2}Y_u^{pb} Y_u^{ar} \right. \right. \\
& - \frac{23}{6}Y_u^{pr} Y_u^{ab} \Bigg) + \lambda g_Y^2 \left( 10Y_u^{pr} Y_u^{ab} + 24Y_u^{pb} Y_u^{ar} \right) + g_Y^2 \left( \frac{3}{2}Y_u^{pr} (Y_d Y_d^\dagger Y_u)^{ab} + \frac{9}{4}Y_u^{ar} (Y_d Y_d^\dagger Y_u)^{pb} + \frac{11}{3}Y_u^{pb} (Y_d Y_d^\dagger Y_u)^{ar} - \frac{7}{4}Y_u^{ar} (Y_u Y_u^\dagger Y_u)^{pb} \right. \\
& - \frac{13}{2}Y_u^{pb} (Y_u Y_u^\dagger Y_u)^{ar} - \frac{57}{2}Y_u^{pr} (Y_u Y_u^\dagger Y_u)^{ab} \Bigg) - g_Y^4 \left( \frac{128}{27}Y_u^{pb} Y_u^{ar} + \frac{205}{9}Y_u^{pr} Y_u^{ab} \right) - \frac{80}{9}g_Y^2 g_s^2 Y_u^{pb} Y_u^{ar} \Bigg\} + \left\{ g_s^2 g_L^2 \left( \frac{32}{3}\delta^{rb} (Y_d Y_d^\dagger)^{pa} - \frac{44}{3}\delta^{rb} (Y_u Y_u^\dagger)^{pa} \right. \right. \\
& - \frac{100}{3}\delta^{pa} (Y_u^\dagger Y_u)^{br} \Bigg) + g_L^4 \left( \frac{29}{4}Y_u^{*ab} Y_u^{pr} + \frac{191}{24}\delta^{pa} (Y_u^\dagger Y_u)^{br} - \frac{3}{2}\text{T}_2\delta^{pa}\delta^{rb} - \frac{14}{3}\delta^{rb} (Y_d Y_d^\dagger)^{pa} - \frac{287}{24}\delta^{rb} (Y_u Y_u^\dagger)^{pa} \right) + g_Y^2 g_L^2 \left( \frac{331}{72}\delta^{pa} (Y_u^\dagger Y_u)^{br} \right. \\
& - \frac{109}{72}\delta^{rb} (Y_u Y_u^\dagger)^{pa} - \frac{59}{18}\delta^{rb} (Y_d Y_d^\dagger)^{pa} - \frac{15}{2}\delta^{pa}\delta^{rb} \text{Tr}[Y_d^\dagger Y_d] - \frac{55}{6}\delta^{pa}\delta^{rb} \text{Tr}[Y_e^\dagger Y_e] - \frac{28}{3}Y_u^{*ab} Y_u^{pr} - \frac{35}{2}\delta^{pa}\delta^{rb} \text{Tr}[Y_u^\dagger Y_u] \Bigg) \\
& + \lambda \left( g_L^2 \left( \frac{27}{2}\delta^{pa}\delta^{rb} \text{Tr}[Y_u^\dagger Y_u] + \frac{93}{4}\delta^{rb} (Y_u Y_u^\dagger)^{pa} + 30\delta^{rb} (Y_d Y_d^\dagger)^{pa} - \frac{3}{4}\delta^{pa} (Y_u^\dagger Y_u)^{br} - \frac{9}{2}Y_u^{*ab} Y_u^{pr} \right) + 16\delta^{pa}\delta^{rb} g_s^2 g_L^2 + 27\delta^{pa}\delta^{rb} g_L^4 \right. \\
& - \frac{79}{6}\delta^{pa}\delta^{rb} g_Y^2 g_L^2 \Bigg) + g_L^2 \left( \frac{9}{4}\text{T}_2\delta^{rb} (Y_u Y_u^\dagger)^{pa} + \frac{19}{4}(Y_u^\dagger Y_u)^{br} (Y_d Y_d^\dagger)^{pa} + 8\delta^{rb} (Y_d Y_d^\dagger Y_u Y_u^\dagger)^{pa} + \frac{39}{4}Y_u^{pr} (Y_u^\dagger Y_u Y_u^\dagger)^{ab} + \frac{179}{8}\delta^{rb} (Y_u Y_u^\dagger Y_d Y_d^\dagger)^{pa} \right. \\
& + \frac{123}{4}Y_u^{pr} (Y_d^\dagger Y_d Y_u^\dagger)^{ab} - \frac{3}{4}\text{T}_2\delta^{pa} (Y_u^\dagger Y_u)^{br} - \frac{7}{2}(Y_u^\dagger Y_u)^{br} (Y_u Y_u^\dagger)^{pa} - \frac{63}{8}\delta^{pa} (Y_u^\dagger Y_u Y_u^\dagger Y_u)^{br} - \frac{23}{2}\delta^{rb} (Y_u Y_u^\dagger Y_u Y_u^\dagger)^{pa} - 27\delta^{pa}\delta^{rb} \text{Tr}[Y_u^\dagger Y_u Y_u^\dagger Y_u] \\
& - \frac{97}{2}\delta^{rb} (Y_d Y_d^\dagger Y_d Y_d^\dagger)^{pa} \Bigg) + \frac{80}{9}\delta^{pa}\delta^{rb} g_Y^2 g_s^2 g_L^2 + \frac{373}{36}\delta^{pa}\delta^{rb} g_Y^2 g_L^4 + \frac{3359}{108}\delta^{pa}\delta^{rb} g_Y^4 g_L^2 + \frac{305}{4}\delta^{pa}\delta^{rb} g_L^6 - 16\delta^{pa}\delta^{rb} g_s^2 g_L^4 \Bigg\} C_{uW}^{ab} \\
& + C_{uW}^{*ab} \left\{ g_Y^2 g_L^2 \left( \frac{43}{24}Y_u^{pb} Y_u^{ar} - \frac{11}{6}Y_u^{pr} Y_u^{ab} \right) + \lambda g_L^2 \left( \frac{15}{2}Y_u^{pb} Y_u^{ar} + 9Y_u^{pr} Y_u^{ab} \right) + g_L^2 \left( 3Y_u^{pb} (Y_d Y_d^\dagger Y_u)^{ar} + \frac{47}{8}Y_u^{ar} (Y_d Y_d^\dagger Y_u)^{pb} - \frac{3}{2}\text{T}_2Y_u^{pb} Y_u^{ar} \right. \right.
\end{aligned}$$

$$\begin{aligned}
& -\frac{9}{4}Y_u^{pb}(Y_uY_u^\dagger Y_u)^{ar} - \frac{21}{8}Y_u^{ar}(Y_uY_u^\dagger Y_u)^{pb} - \frac{27}{4}Y_u^{pr}(Y_dY_d^\dagger Y_u)^{ab} - \frac{69}{4}Y_u^{pr}(Y_uY_u^\dagger Y_u)^{ab} - g_L^4\left(\frac{53}{8}Y_u^{pb}Y_u^{ar} + \frac{79}{4}Y_u^{pr}Y_u^{ab}\right) - 16g_s^2g_L^2Y_u^{pb}Y_u^{ar}\Bigg\} \\
& + \left\{g_s^2g_L^2\left(\frac{16}{3}Y_u^{*ab}Y_u^{pr} - \frac{26}{3}\delta^{pa}(Y_u^\dagger Y_u)^{br} - \frac{56}{3}\delta^{rb}(Y_dY_d^\dagger)^{pa} - \frac{82}{3}\delta^{rb}(Y_uY_u^\dagger)^{pa}\right) + g_Y^2g_s^2\left(\frac{16}{3}Y_u^{*ab}Y_u^{pr} - \frac{254}{27}\delta^{rb}(Y_uY_u^\dagger)^{pa} - \frac{614}{27}\delta^{pa}(Y_u^\dagger Y_u)^{br}\right) \right. \\
& + \lambda\left(g_s^2\left(\frac{16}{3}\delta^{rb}(Y_dY_d^\dagger)^{pa} + \frac{152}{3}\delta^{pa}(Y_u^\dagger Y_u)^{br} + \frac{160}{3}\delta^{rb}(Y_uY_u^\dagger)^{pa} - 16Y_u^{*ab}Y_u^{pr}\right) + \frac{56}{27}\delta^{pa}\delta^{rb}g_Y^2g_s^2 + \frac{224}{9}\delta^{pa}\delta^{rb}g_s^4 - 8\delta^{pa}\delta^{rb}g_s^2g_L^2\right) \\
& + g_s^2\left(16Y_u^{pr}(Y_u^\dagger Y_uY_u^\dagger)^{ab} + 16\delta^{rb}(Y_dY_d^\dagger Y_uY_u^\dagger)^{pa} + \frac{152}{9}\delta^{pa}\delta^{rb}g_Y^2g_L^2 + \frac{100}{3}\delta^{rb}(Y_uY_u^\dagger Y_dY_d^\dagger)^{pa} + 36\delta^{pa}(Y_u^\dagger Y_dY_d^\dagger Y_u)^{br} - \frac{8}{3}(Y_u^\dagger Y_u)^{br}(Y_dY_d^\dagger)^{pa} \right. \\
& - \frac{332}{3}\delta^{rb}(Y_uY_u^\dagger Y_uY_u^\dagger)^{pa} - \frac{340}{3}\delta^{pa}(Y_u^\dagger Y_uY_u^\dagger Y_u)^{br}\Bigg) + g_s^4\left(\frac{2488}{9}\delta^{pa}(Y_u^\dagger Y_u)^{br} + \frac{2488}{9}\delta^{rb}(Y_uY_u^\dagger)^{pa} - \frac{64}{3}Y_u^{*ab}Y_u^{pr} - 128\delta^{pa}\delta^{rb}\text{Tr}\left[Y_u^\dagger Y_d\right] \right. \\
& - 128\delta^{pa}\delta^{rb}\text{Tr}\left[Y_u^\dagger Y_u\right]\Bigg) + 4\delta^{pa}\delta^{rb}g_s^2g_L^4 - \frac{92}{27}\delta^{pa}\delta^{rb}g_Y^4g_s^2\Bigg\}C_{uG}^{ab} + C_{uG}^{*ab}\left\{g_s^4\left(\frac{1184}{9}Y_u^{pb}Y_u^{ar} - \frac{160}{3}Y_u^{pr}Y_u^{ab}\right) + g_Y^2g_s^2\left(\frac{16}{3}Y_u^{pr}Y_u^{ab} - \frac{28}{27}Y_u^{pb}Y_u^{ar}\right) \right. \\
& + g_s^2g_L^2\left(4Y_u^{pb}Y_u^{ar} + \frac{16}{3}Y_u^{pr}Y_u^{ab}\right) + \lambda g_s^2\left(72Y_u^{pb}Y_u^{ar} - 16Y_u^{pr}Y_u^{ab}\right) + g_s^2\left(\frac{40}{3}Y_u^{pb}(Y_dY_d^\dagger Y_u)^{ar} - 8Y_u^{ar}(Y_uY_u^\dagger Y_u)^{pb} - 16Y_u^{pb}(Y_uY_u^\dagger Y_u)^{ar}\right)\Bigg\} \\
& + \left\{g_Y^2g_L^2\left(\frac{11}{3}Y_d^{*ab}Y_u^{pr} - \frac{47}{12}\delta^{pa}(Y_d^\dagger Y_u)^{br}\right) + g_Y^4\left(\frac{31}{18}Y_d^{*ab}Y_u^{pr} + \frac{15}{4}\delta^{pa}(Y_d^\dagger Y_u)^{br}\right) + \lambda g_Y^2\left(Y_d^{*ab}Y_u^{pr} + 5\delta^{pa}(Y_d^\dagger Y_u)^{br}\right) + g_Y^2\left(\frac{13}{3}\delta^{pa}(Y_d^\dagger Y_dY_d^\dagger Y_u)^{br} \right. \\
& + \frac{31}{6}\delta^{pa}(Y_d^\dagger Y_uY_u^\dagger Y_u)^{br} + \frac{109}{12}(Y_d^\dagger Y_u)^{br}(Y_dY_d^\dagger)^{pa} - \frac{3}{2}Y_u^{pr}(Y_d^\dagger Y_dY_d^\dagger)^{ab} - \frac{3}{2}Y_u^{pr}(Y_u^\dagger Y_uY_d^\dagger)^{ab} - \frac{25}{4}(Y_d^\dagger Y_u)^{br}(Y_uY_u^\dagger)^{pa}\Bigg)\Bigg\}C_{dB}^{ab} + C_{dB}^{*ab}\left\{g_Y^4\left(\frac{19}{18}Y_d^{ab}Y_u^{pr} \right. \right. \\
& - \frac{11}{6}Y_d^{pb}Y_u^{ar}\Bigg) + g_Y^2g_L^2\left(4Y_d^{pb}Y_u^{ar} + \frac{47}{3}Y_d^{ab}Y_u^{pr}\right) + \lambda g_Y^2\left(Y_d^{ab}Y_u^{pr} - \frac{28}{3}Y_d^{pb}Y_u^{ar}\right) + g_Y^2\left(\frac{2}{3}Y_d^{pb}(Y_uY_u^\dagger Y_u)^{ar} + \frac{13}{12}Y_u^{ar}(Y_uY_u^\dagger Y_d)^{pb} - \frac{13}{12}Y_u^{ar}(Y_dY_d^\dagger Y_d)^{pb} \right. \\
& - \frac{3}{2}Y_u^{pr}(Y_uY_u^\dagger Y_d)^{ab} - \frac{5}{2}Y_u^{pr}(Y_dY_d^\dagger Y_d)^{ab} - \frac{13}{3}Y_d^{pb}(Y_dY_d^\dagger Y_u)^{ar}\Bigg)\Bigg\} + \left\{g_Y^2g_L^2\left(\frac{13}{12}Y_d^{*ab}Y_u^{pr} - \frac{61}{18}\delta^{pa}(Y_d^\dagger Y_u)^{br}\right) + g_L^2\left(\frac{7}{4}\delta^{pa}(Y_d^\dagger Y_uY_u^\dagger Y_u)^{br} \right. \right. \\
& + \frac{39}{4}Y_u^{pr}(Y_d^\dagger Y_dY_d^\dagger)^{ab} - \frac{11}{8}(Y_d^\dagger Y_u)^{br}(Y_dY_d^\dagger)^{pa} - \frac{3}{2}\text{T}_2\delta^{pa}(Y_d^\dagger Y_u)^{br} - \frac{23}{8}(Y_d^\dagger Y_u)^{br}(Y_uY_u^\dagger)^{pa} - \frac{27}{4}Y_u^{pr}(Y_u^\dagger Y_uY_d^\dagger)^{ab} - \frac{35}{2}\delta^{pa}(Y_d^\dagger Y_dY_d^\dagger Y_u)^{br}\Bigg) \\
& + \frac{16}{3}\delta^{pa}g_s^2g_L^2(Y_d^\dagger Y_u)^{br} - g_L^4\left(\frac{13}{3}\delta^{pa}(Y_d^\dagger Y_u)^{br} + 13Y_d^{*ab}Y_u^{pr}\right) - \lambda g_L^2\left(\frac{9}{2}Y_d^{*ab}Y_u^{pr} + 6\delta^{pa}(Y_d^\dagger Y_u)^{br}\right)\Bigg)\Bigg\}C_{dW}^{ab} + C_{dW}^{*ab}\left\{g_L^4\left(\frac{1}{2}Y_d^{ab}Y_u^{pr} - \frac{43}{8}Y_d^{pb}Y_u^{ar}\right) \right. \\
& + \lambda g_L^2\left(\frac{51}{2}Y_d^{pb}Y_u^{ar} - \frac{9}{2}Y_d^{ab}Y_u^{pr}\right) + g_L^2\left(\frac{3}{2}\text{T}_2Y_d^{pb}Y_u^{ar} + 2Y_d^{pb}(Y_uY_u^\dagger Y_u)^{ar} + \frac{39}{4}Y_u^{pr}(Y_dY_d^\dagger Y_d)^{ab} + \frac{111}{8}Y_u^{ar}(Y_uY_u^\dagger Y_d)^{pb} + \frac{123}{4}Y_u^{pr}(Y_uY_u^\dagger Y_d)^{ab} \right. \\
& - 2Y_d^{pb}(Y_dY_d^\dagger Y_u)^{ar} - \frac{143}{8}Y_u^{ar}(Y_dY_d^\dagger Y_d)^{pb}\Bigg) + 8g_s^2g_L^2Y_d^{pb}Y_u^{ar} - g_Y^2g_L^2\left(\frac{11}{12}Y_d^{ab}Y_u^{pr} + \frac{29}{8}Y_d^{pb}Y_u^{ar}\right)\Bigg)\Bigg\} + \left\{g_s^2g_L^2\left(\frac{16}{3}Y_d^{*ab}Y_u^{pr} - \frac{40}{3}\delta^{pa}(Y_d^\dagger Y_u)^{br}\right) \right. \\
& + \lambda g_s^2\left(8\delta^{pa}(Y_d^\dagger Y_u)^{br} - 16Y_d^{*ab}Y_u^{pr}\right) + g_s^2\left(\frac{8}{3}\delta^{pa}(Y_d^\dagger Y_dY_d^\dagger Y_u)^{br} + \frac{32}{3}(Y_d^\dagger Y_u)^{br}(Y_dY_d^\dagger)^{pa} + \frac{40}{3}\delta^{pa}(Y_d^\dagger Y_uY_u^\dagger Y_u)^{br} - 8(Y_d^\dagger Y_u)^{br}(Y_uY_u^\dagger)^{pa}\right)
\end{aligned}$$

$$\begin{aligned}
& + \frac{16}{3} g_Y^2 g_s^2 Y_d^{*ab} Y_u^{pr} - \frac{64}{3} g_s^4 Y_d^{*ab} Y_u^{pr} \left\{ C_{dG}^{ab} + C_{dG}^{*ab} \left\{ g_s^2 \left( \frac{4}{3} Y_d^{pb} (Y_u Y_u^\dagger Y_u)^{ar} + 16 Y_u^{pr} (Y_d Y_d^\dagger Y_d)^{ab} - \frac{4}{3} Y_u^{ar} (Y_u Y_u^\dagger Y_d)^{pb} - \frac{20}{3} Y_u^{ar} (Y_d Y_d^\dagger Y_d)^{pb} \right. \right. \right. \\
& - \frac{44}{3} Y_d^{pb} (Y_d Y_d^\dagger Y_u)^{ar} \left. \left. \left. + \frac{16}{3} g_s^2 g_L^2 Y_d^{ab} Y_u^{pr} + \frac{16}{3} g_Y^2 g_s^2 Y_d^{ab} Y_u^{pr} - \lambda g_s^2 \left( 16 Y_d^{ab} Y_u^{pr} + \frac{56}{3} Y_d^{pb} Y_u^{ar} \right) - \frac{160}{3} g_s^4 Y_d^{ab} Y_u^{pr} \right\} + \left\{ \frac{28}{27} \delta^{ab} g_Y^2 g_L^2 Y_u^{pr} \right. \right. \\
& + \frac{17}{9} \delta^{ab} g_Y^4 Y_u^{pr} + \frac{311}{36} g_Y^2 Y_u^{pr} (Y_e Y_e^\dagger)^{ba} - \frac{7}{36} g_L^2 Y_u^{pr} (Y_e Y_e^\dagger)^{ba} - \lambda \left( \frac{26}{9} \delta^{ab} g_Y^2 Y_u^{pr} + \frac{16}{3} Y_u^{pr} (Y_e Y_e^\dagger)^{ba} \right) - (Y_e Y_e^\dagger)^{ba} (Y_u Y_u^\dagger Y_u)^{pr} \\
& - 10 Y_u^{pr} (Y_e Y_e^\dagger Y_e Y_e^\dagger)^{ba} \left. \left. \right\} C_{H\ell}^{(\parallel)ab} + \left\{ \frac{1}{2} (Y_e Y_e^\dagger)^{ba} (Y_u Y_u^\dagger Y_u)^{pr} + \frac{83}{108} \delta^{ab} g_Y^2 g_L^2 Y_u^{pr} + \frac{17}{18} \delta^{ab} g_Y^4 Y_u^{pr} + \lambda \left( \frac{8}{3} \delta^{ab} g_L^2 Y_u^{pr} - \frac{13}{9} \delta^{ab} g_Y^2 Y_u^{pr} \right. \right. \\
& - \frac{29}{3} Y_u^{pr} (Y_e Y_e^\dagger)^{ba} \left. \left. \left. + \frac{37}{9} g_L^2 Y_u^{pr} (Y_e Y_e^\dagger)^{ba} + \frac{167}{18} g_Y^2 Y_u^{pr} (Y_e Y_e^\dagger)^{ba} - \frac{5}{2} (Y_e Y_e^\dagger)^{ba} (Y_d Y_d^\dagger Y_u)^{pr} - \frac{15}{4} \delta^{ab} g_L^4 Y_u^{pr} - 8 Y_u^{pr} (Y_e Y_e^\dagger Y_e Y_e^\dagger)^{ba} \right\} C_{H\ell}^{(\times)ab} \right. \\
& + \left\{ \lambda \left( \frac{16}{3} Y_u^{pr} (Y_e^\dagger Y_e)^{ba} - \frac{26}{9} \delta^{ab} g_Y^2 Y_u^{pr} \right) + (Y_e^\dagger Y_e)^{ba} (Y_u Y_u^\dagger Y_u)^{pr} + \frac{61}{18} \delta^{ab} g_Y^4 Y_u^{pr} + 10 Y_u^{pr} (Y_e^\dagger Y_e Y_e^\dagger Y_e)^{ba} - \frac{25}{54} \delta^{ab} g_Y^2 g_L^2 Y_u^{pr} - \frac{77}{36} g_L^2 Y_u^{pr} (Y_e^\dagger Y_e)^{ba} \right. \\
& - \frac{167}{36} g_Y^2 Y_u^{pr} (Y_e^\dagger Y_e)^{ba} \left. \left. \right\} C_{He}^{ab} + \left\{ \frac{3}{4} (Y_d Y_d^\dagger)^{pa} (Y_u Y_u^\dagger Y_u)^{br} + g_Y^2 g_s^2 \left( \frac{52}{3} \delta^{pa} Y_u^{br} - \frac{8}{3} \delta^{ab} Y_u^{pr} \right) + T_2 \delta^{pa} (Y_u Y_u^\dagger Y_u)^{br} + g_s^2 \left( \frac{4}{3} Y_u^{br} (Y_u Y_u^\dagger)^{pa} + 40 Y_u^{pr} (Y_d Y_d^\dagger)^{ba} \right. \right. \\
& - \frac{68}{3} \delta^{pa} (Y_u Y_u^\dagger Y_u)^{br} - 40 Y_u^{pr} (Y_u Y_u^\dagger)^{ba} \left. \left. \left. + g_Y^2 \left( \frac{15}{4} \delta^{pa} (Y_d Y_d^\dagger Y_u)^{br} + \frac{47}{12} Y_u^{pr} (Y_d Y_d^\dagger)^{ba} + \frac{1009}{216} Y_u^{br} (Y_u Y_u^\dagger)^{pa} - \frac{29}{6} Y_u^{br} (Y_d Y_d^\dagger)^{pa} - \frac{139}{12} Y_u^{pr} (Y_u Y_u^\dagger)^{ba} \right. \right. \right. \\
& - \frac{4021}{216} \delta^{pa} (Y_u Y_u^\dagger Y_u)^{br} \left. \left. \left. + g_L^2 \left( \frac{7}{12} Y_u^{pr} (Y_u Y_u^\dagger)^{ba} + \frac{11}{8} Y_u^{br} (Y_u Y_u^\dagger)^{pa} + \frac{3}{2} Y_u^{br} (Y_d Y_d^\dagger)^{pa} + \frac{27}{8} \delta^{pa} (Y_u Y_u^\dagger Y_u)^{br} - \frac{7}{12} Y_u^{pr} (Y_d Y_d^\dagger)^{ba} - \frac{3}{2} \delta^{pa} (Y_d Y_d^\dagger Y_u)^{br} \right) \right. \right. \\
& + \lambda \left( \frac{1}{2} Y_u^{br} (Y_d Y_d^\dagger)^{pa} + g_Y^2 \left( \frac{26}{9} \delta^{ab} Y_u^{pr} + \frac{3127}{108} \delta^{pa} Y_u^{br} \right) + 4 T_2 \delta^{pa} Y_u^{br} + 16 Y_u^{pr} (Y_u Y_u^\dagger)^{ba} + 16 \delta^{pa} (Y_u Y_u^\dagger Y_u)^{br} - \frac{1}{2} \delta^{pa} (Y_d Y_d^\dagger Y_u)^{br} - 2 Y_u^{br} (Y_u Y_u^\dagger)^{pa} \right. \\
& - \frac{15}{4} \delta^{pa} g_L^2 Y_u^{br} - \frac{16}{3} \delta^{pa} g_s^2 Y_u^{br} - 16 Y_u^{pr} (Y_d Y_d^\dagger)^{ba} \left. \left. \left. + \frac{5}{4} (Y_d Y_d^\dagger)^{pa} (Y_d Y_d^\dagger Y_u)^{br} + \frac{25}{12} (Y_u Y_u^\dagger)^{pa} (Y_u Y_u^\dagger Y_u)^{br} + \frac{9}{4} Y_u^{br} (Y_d Y_d^\dagger Y_u Y_u^\dagger)^{pa} \right. \right. \\
& + 3 (Y_u Y_u^\dagger)^{ba} (Y_u Y_u^\dagger Y_u)^{pr} + \frac{37}{12} Y_u^{br} (Y_u Y_u^\dagger Y_u Y_u^\dagger)^{pa} + 4 T_4 \delta^{pa} Y_u^{br} + \frac{71}{12} Y_u^{br} (Y_u Y_u^\dagger Y_d Y_d^\dagger)^{pa} + 12 \delta^{pa} g_s^2 g_L^2 Y_u^{br} + 25 \delta^{pa} (Y_u Y_u^\dagger Y_u Y_u^\dagger Y_u)^{br} \\
& + 30 Y_u^{pr} (Y_u Y_u^\dagger Y_u Y_u^\dagger)^{ba} - \frac{1}{8} \delta^{pa} g_L^4 Y_u^{br} - g_Y^2 g_L^2 \left( \frac{28}{27} \delta^{ab} Y_u^{pr} + \frac{107}{4} \delta^{pa} Y_u^{br} \right) - g_Y^4 \left( \frac{13}{9} \delta^{ab} Y_u^{pr} + \frac{3145}{72} \delta^{pa} Y_u^{br} \right) - \frac{7}{4} Y_u^{br} (Y_d Y_d^\dagger Y_d Y_d^\dagger)^{pa} \\
& - 2 \delta^{pa} (Y_d Y_d^\dagger Y_d Y_d^\dagger Y_u)^{br} - \frac{25}{12} (Y_u Y_u^\dagger)^{pa} (Y_d Y_d^\dagger Y_u)^{br} - \frac{5}{2} \delta^{pa} (Y_d Y_d^\dagger Y_u Y_u^\dagger Y_u)^{br} - 3 (Y_d Y_d^\dagger)^{ba} (Y_u Y_u^\dagger Y_u)^{pr} - \frac{7}{2} \delta^{pa} (Y_u Y_u^\dagger Y_d Y_d^\dagger Y_u)^{br} \\
& - 30 Y_u^{pr} (Y_d Y_d^\dagger Y_d Y_d^\dagger)^{ba} \left. \left. \right\} C_{Hq}^{(\parallel)ab} + \left\{ g_L^4 \left( \frac{1}{2} \delta^{pa} Y_u^{br} - \frac{45}{4} \delta^{ab} Y_u^{pr} \right) + g_Y^4 \left( \frac{73}{72} \delta^{pa} Y_u^{br} - \frac{13}{18} \delta^{ab} Y_u^{pr} \right) + g_Y^2 g_L^2 \left( \frac{97}{108} \delta^{ab} Y_u^{pr} - \frac{793}{72} \delta^{pa} Y_u^{br} \right) \right. \\
& + g_L^2 \left( \frac{11}{8} Y_u^{br} (Y_d Y_d^\dagger)^{pa} + \frac{37}{3} Y_u^{pr} (Y_d Y_d^\dagger)^{ba} + \frac{155}{12} Y_u^{pr} (Y_u Y_u^\dagger)^{ba} - \frac{79}{24} \delta^{pa} (Y_d Y_d^\dagger Y_u)^{br} - \frac{85}{24} \delta^{pa} (Y_u Y_u^\dagger Y_u)^{br} - \frac{151}{24} Y_u^{br} (Y_u Y_u^\dagger)^{pa} \right) + g_s^2 \left( 8 Y_u^{br} (Y_d Y_d^\dagger)^{pa} \right. \\
& + 24 \delta^{pa} (Y_d Y_d^\dagger Y_u)^{br} + 40 Y_u^{pr} (Y_d Y_d^\dagger)^{ba} - \frac{4}{3} \delta^{pa} (Y_u Y_u^\dagger Y_u)^{br} - \frac{28}{3} Y_u^{br} (Y_u Y_u^\dagger)^{pa} \left. \left. \right) + g_Y^2 \left( \frac{145}{216} \delta^{pa} (Y_u Y_u^\dagger Y_u)^{br} + \frac{5}{4} Y_u^{pr} (Y_u Y_u^\dagger)^{ba} + \frac{581}{216} Y_u^{br} (Y_u Y_u^\dagger)^{pa} \right. \right.
\end{aligned}$$



$$\begin{aligned}
& + \frac{9}{2} Y_u^{pr} (Y_d Y_d^\dagger)^{ba} - \frac{17}{8} \delta^{pa} (Y_d Y_d^\dagger Y_u)^{br} - \frac{127}{24} Y_u^{br} (Y_d Y_d^\dagger)^{pa} + \lambda \left( \frac{1}{2} Y_u^{br} (Y_u Y_u^\dagger)^{pa} + g_Y^2 \left( \frac{13}{9} \delta^{ab} Y_u^{pr} + \frac{271}{54} \delta^{pa} Y_u^{br} \right) + g_L^2 \left( 8 \delta^{ab} Y_u^{pr} + \frac{35}{3} \delta^{pa} Y_u^{br} \right) \right. \\
& + \frac{5}{2} Y_u^{br} (Y_d Y_d^\dagger)^{pa} + 5 \delta^{pa} (Y_u Y_u^\dagger Y_u)^{br} + \frac{16}{3} \delta^{pa} g_s^2 Y_u^{br} - 4 T_2 \delta^{pa} Y_u^{br} - 10 \delta^{pa} (Y_d Y_d^\dagger Y_u)^{br} - 13 Y_u^{pr} (Y_u Y_u^\dagger)^{ba} - 29 Y_u^{pr} (Y_d Y_d^\dagger)^{ba} \\
& + \frac{3}{2} (Y_d Y_d^\dagger)^{ba} (Y_u Y_u^\dagger Y_u)^{pr} + \frac{3}{2} T_2 \delta^{pa} (Y_u Y_u^\dagger Y_u)^{br} + \frac{3}{2} (Y_d Y_d^\dagger)^{pa} (Y_u Y_u^\dagger Y_u)^{br} + 2 \delta^{pa} (Y_u Y_u^\dagger Y_d Y_d^\dagger Y_u)^{br} + \frac{5}{2} Y_u^{br} (Y_d Y_d^\dagger Y_u Y_u^\dagger)^{pa} + \frac{9}{2} (Y_u Y_u^\dagger)^{ba} (Y_u Y_u^\dagger Y_u)^{pr} \\
& + \frac{19}{4} \delta^{pa} (Y_u Y_u^\dagger Y_u Y_u^\dagger Y_u)^{br} + 6 Y_u^{pr} (Y_u Y_u^\dagger Y_u Y_u^\dagger)^{ba} + \frac{127}{12} Y_u^{br} (Y_u Y_u^\dagger Y_d Y_d^\dagger)^{pa} - \frac{1}{2} (Y_d Y_d^\dagger)^{pa} (Y_d Y_d^\dagger Y_u)^{br} - \frac{3}{4} \delta^{pa} (Y_d Y_d^\dagger Y_u Y_u^\dagger Y_u)^{br} \\
& - \frac{5}{6} (Y_u Y_u^\dagger)^{pa} (Y_u Y_u^\dagger Y_u)^{br} - g_s^2 g_L^2 \left( 4 \delta^{ab} Y_u^{pr} + 12 \delta^{pa} Y_u^{br} \right) - \frac{4}{3} \delta^{ab} g_Y^2 g_s^2 Y_u^{pr} - \frac{4}{3} Y_u^{br} (Y_u Y_u^\dagger Y_u Y_u^\dagger)^{pa} - \frac{5}{2} T_2 \delta^{pa} (Y_d Y_d^\dagger Y_u)^{br} - \frac{19}{6} (Y_u Y_u^\dagger)^{pa} (Y_d Y_d^\dagger Y_u)^{br} \\
& - \frac{9}{2} Y_u^{pr} (Y_d Y_d^\dagger Y_u Y_u^\dagger)^{ba} - \frac{9}{2} Y_u^{pr} (Y_u Y_u^\dagger Y_d Y_d^\dagger)^{ba} - \frac{23}{4} Y_u^{br} (Y_d Y_d^\dagger Y_d Y_d^\dagger)^{pa} - \frac{15}{2} (Y_d Y_d^\dagger)^{ba} (Y_d Y_d^\dagger Y_u)^{pr} - \frac{15}{2} (Y_u Y_u^\dagger)^{ba} (Y_d Y_d^\dagger Y_u)^{pr} \\
& - 11 \delta^{pa} (Y_d Y_d^\dagger Y_d Y_d^\dagger Y_u)^{br} - 24 Y_u^{pr} (Y_d Y_d^\dagger Y_d Y_d^\dagger)^{ba} - 24 \delta^{pa} Y_u^{br} \text{Tr} \left[ Y_d^\dagger Y_d Y_u^\dagger Y_u \right] \left. \right\} C_{Hq}^{(\times)ab} + \left\{ \frac{5}{6} \delta^{rb} g_L^4 Y_u^{pa} + g_Y^4 \left( \frac{95}{18} \delta^{rb} Y_u^{pa} - \frac{41}{9} \delta^{ab} Y_u^{pr} \right) \right. \\
& + g_Y^2 g_L^2 \left( \frac{25}{27} \delta^{ab} Y_u^{pr} + \frac{65}{6} \delta^{rb} Y_u^{pa} \right) + \lambda \left( g_Y^2 \left( \frac{373}{108} \delta^{rb} Y_u^{pa} + \frac{52}{9} \delta^{ab} Y_u^{pr} \right) + \frac{5}{2} Y_u^{pa} (Y_u^\dagger Y_u)^{br} + 4 \delta^{rb} (Y_d Y_d^\dagger Y_u)^{pa} + \frac{16}{3} \delta^{rb} g_s^2 Y_u^{pa} - 4 T_2 \delta^{rb} Y_u^{pa} \right. \\
& - \frac{25}{2} \delta^{rb} (Y_u Y_u^\dagger Y_u)^{pa} - \frac{57}{4} \delta^{rb} g_L^2 Y_u^{pa} - 16 Y_u^{pr} (Y_u^\dagger Y_u)^{ba} \left. \right) + g_Y^2 \left( \delta^{rb} (Y_d Y_d^\dagger Y_u)^{pa} + \frac{59}{12} Y_u^{pr} (Y_u^\dagger Y_u)^{ba} - \frac{917}{216} Y_u^{pa} (Y_u^\dagger Y_u)^{br} - \frac{1921}{216} \delta^{rb} (Y_u Y_u^\dagger Y_u)^{pa} \right) \\
& + g_L^2 \left( \frac{77}{12} Y_u^{pr} (Y_u^\dagger Y_u)^{ba} + \frac{129}{8} \delta^{rb} (Y_u Y_u^\dagger Y_u)^{pa} - \frac{17}{8} Y_u^{pa} (Y_u^\dagger Y_u)^{br} - 11 \delta^{rb} (Y_d Y_d^\dagger Y_u)^{pa} \right) + g_s^2 \left( \frac{68}{3} \delta^{rb} (Y_u Y_u^\dagger Y_u)^{pa} + 40 Y_u^{pr} (Y_u^\dagger Y_u)^{ba} - \frac{4}{3} Y_u^{pa} (Y_u^\dagger Y_u)^{br} \right) \\
& + \frac{5}{4} Y_u^{pa} (Y_u^\dagger Y_d Y_d^\dagger Y_u)^{br} + \frac{5}{2} \delta^{rb} (Y_u Y_u^\dagger Y_d Y_d^\dagger Y_u)^{pa} + 3 Y_u^{pr} (Y_u^\dagger Y_d Y_d^\dagger Y_u)^{ba} + 4 \delta^{rb} (Y_d Y_d^\dagger Y_d Y_d^\dagger Y_u)^{pa} + 4 \delta^{rb} (Y_d Y_d^\dagger Y_u Y_u^\dagger Y_u)^{pa} \\
& - \frac{1}{4} (Y_u^\dagger Y_u)^{br} (Y_d Y_d^\dagger Y_u)^{pa} - g_Y^2 g_s^2 \left( \frac{16}{3} \delta^{ab} Y_u^{pr} + \frac{32}{3} \delta^{rb} Y_u^{pa} \right) - T_2 \delta^{rb} (Y_u Y_u^\dagger Y_u)^{pa} - \frac{29}{12} (Y_u^\dagger Y_u)^{br} (Y_u Y_u^\dagger Y_u)^{pa} - 3 (Y_u^\dagger Y_u)^{ba} (Y_u Y_u^\dagger Y_u)^{pr} - 4 T_4 \delta^{rb} Y_u^{pa} \\
& - \frac{59}{12} Y_u^{pa} (Y_u^\dagger Y_u Y_u^\dagger Y_u)^{br} - 16 \delta^{rb} g_s^2 g_L^2 Y_u^{pa} - \frac{39}{2} \delta^{rb} (Y_u Y_u^\dagger Y_u Y_u^\dagger Y_u)^{pa} - 30 Y_u^{pr} (Y_u^\dagger Y_u Y_u^\dagger Y_u)^{ba} \left. \right\} C_{Hu}^{ab} + \left\{ \frac{1}{4} Y_d^{pa} (Y_d^\dagger Y_u Y_u^\dagger Y_u)^{br} \right. \\
& + \lambda \left( 16 Y_u^{pr} (Y_d^\dagger Y_d)^{ba} - \frac{26}{9} \delta^{ab} g_Y^2 Y_u^{pr} \right) + g_Y^2 \left( \frac{11}{6} Y_d^{pa} (Y_d^\dagger Y_u)^{br} - \frac{31}{12} Y_u^{pr} (Y_d^\dagger Y_d)^{ba} \right) + g_L^2 \left( \frac{17}{4} Y_d^{pa} (Y_d^\dagger Y_u)^{br} - \frac{77}{12} Y_u^{pr} (Y_d^\dagger Y_d)^{ba} \right) + \frac{29}{18} \delta^{ab} g_Y^4 Y_u^{pr} \\
& + \frac{7}{4} (Y_d^\dagger Y_u)^{br} (Y_d Y_d^\dagger Y_d)^{pa} + \frac{8}{3} \delta^{ab} g_Y^2 g_s^2 Y_u^{pr} + 3 (Y_d^\dagger Y_d)^{ba} (Y_u Y_u^\dagger Y_u)^{pr} + 30 Y_u^{pr} (Y_d^\dagger Y_d Y_d^\dagger Y_d)^{ba} - \frac{25}{54} \delta^{ab} g_Y^2 g_L^2 Y_u^{pr} - \frac{7}{4} (Y_d^\dagger Y_u)^{br} (Y_u Y_u^\dagger Y_d)^{pa} \\
& - 3 Y_u^{pr} (Y_d^\dagger Y_u Y_u^\dagger Y_d)^{ba} - \frac{19}{4} Y_d^{pa} (Y_d^\dagger Y_d Y_d^\dagger Y_u)^{br} - 40 g_s^2 Y_u^{pr} (Y_d^\dagger Y_d)^{ba} \left. \right\} C_{Hd}^{ab} + \left\{ \frac{1}{4} (Y_d^\dagger Y_u)^{br} (Y_u Y_u^\dagger Y_u)^{pa} + \frac{3}{4} (Y_d^\dagger Y_u)^{br} (Y_d Y_d^\dagger Y_u)^{pa} + g_Y^2 \left( \frac{2}{9} Y_u^{pa} (Y_d^\dagger Y_u)^{br} \right. \right. \\
& - \frac{17}{12} Y_u^{pr} (Y_d^\dagger Y_u)^{ba} \left. \right) + \lambda \left( 16 Y_u^{pr} (Y_d^\dagger Y_u)^{ba} - 2 Y_u^{pa} (Y_d^\dagger Y_u)^{br} \right) + \frac{7}{4} Y_u^{pa} (Y_d^\dagger Y_d Y_d^\dagger Y_u)^{br} + \frac{21}{2} (Y_d^\dagger Y_u)^{ba} (Y_d Y_d^\dagger Y_u)^{pr} - \frac{3}{2} Y_u^{pr} (Y_d^\dagger Y_d Y_d^\dagger Y_u)^{ba} \\
& - \frac{3}{2} Y_u^{pr} (Y_d^\dagger Y_u Y_u^\dagger Y_u)^{ba} - \frac{19}{12} Y_u^{pa} (Y_d^\dagger Y_u Y_u^\dagger Y_u)^{br} - \frac{15}{2} (Y_d^\dagger Y_u)^{ba} (Y_u Y_u^\dagger Y_u)^{pr} - \frac{28}{3} g_s^2 Y_u^{pa} (Y_d^\dagger Y_u)^{br} - \frac{257}{12} g_L^2 Y_u^{pr} (Y_d^\dagger Y_u)^{ba} \left. \right\} C_{Hud}^{ab}
\end{aligned}$$

$$\begin{aligned}
& + \mathcal{C}_{Hud}^{*ab} \left\{ \lambda \left( 4T_2 \delta^{ra} Y_d^{pb} + 10Y_u^{pr} (Y_u^\dagger Y_d)^{ab} + 11\delta^{ra} (Y_d Y_d^\dagger Y_d)^{pb} + \frac{57}{4} \delta^{ra} g_L^2 Y_d^{pb} - \frac{1}{2} Y_d^{pb} (Y_u^\dagger Y_u)^{ar} - \frac{5}{2} \delta^{ra} (Y_u Y_u^\dagger Y_d)^{pb} - \frac{16}{3} \delta^{ra} g_s^2 Y_d^{pb} \right. \right. \\
& - \frac{271}{36} \delta^{ra} g_Y^2 Y_d^{pb} \left. \right) + g_s^2 \left( \frac{32}{3} Y_d^{pb} (Y_u^\dagger Y_u)^{ar} - \frac{4}{3} \delta^{ra} (Y_u Y_u^\dagger Y_d)^{pb} - \frac{64}{3} \delta^{ra} (Y_d Y_d^\dagger Y_d)^{pb} \right) + g_Y^2 \left( \frac{1}{72} \delta^{ra} (Y_u Y_u^\dagger Y_d)^{pb} + \frac{2}{9} \delta^{ra} (Y_d Y_d^\dagger Y_d)^{pb} - \frac{47}{72} Y_d^{pb} (Y_u^\dagger Y_u)^{ar} \right. \\
& - \frac{17}{12} Y_u^{pr} (Y_u^\dagger Y_d)^{ab} \left. \right) + g_L^2 \left( \frac{51}{8} Y_d^{pb} (Y_u^\dagger Y_u)^{ar} + \frac{103}{8} \delta^{ra} (Y_u Y_u^\dagger Y_d)^{pb} - 18\delta^{ra} (Y_d Y_d^\dagger Y_d)^{pb} - \frac{221}{12} Y_u^{pr} (Y_u^\dagger Y_d)^{ab} \right) + \frac{3}{2} Y_u^{pr} (Y_u^\dagger Y_d Y_d^\dagger Y_d)^{ab} \\
& + \frac{3}{2} Y_u^{pr} (Y_u^\dagger Y_u Y_u^\dagger Y_d)^{ab} + \frac{7}{4} (Y_u^\dagger Y_u)^{ar} (Y_d Y_d^\dagger Y_d)^{pb} + 2T_2 \delta^{ra} (Y_d Y_d^\dagger Y_d)^{pb} + \frac{9}{2} (Y_u^\dagger Y_d)^{ab} (Y_d Y_d^\dagger Y_u)^{pr} + \frac{61}{12} \delta^{ra} g_Y^2 g_L^2 Y_d^{pb} + 11\delta^{ra} (Y_d Y_d^\dagger Y_d Y_d^\dagger Y_d)^{pb} \\
& + 16\delta^{ra} g_s^2 g_L^2 Y_d^{pb} + 24\delta^{ra} Y_d^{pb} \text{Tr} [Y_d^\dagger Y_d Y_u^\dagger Y_u] - \frac{1}{12} (Y_u^\dagger Y_u)^{ar} (Y_u Y_u^\dagger Y_d)^{pb} - \frac{1}{4} Y_d^{pb} (Y_u^\dagger Y_u Y_u^\dagger Y_u)^{ar} - \frac{3}{4} Y_d^{pb} (Y_u^\dagger Y_d Y_d^\dagger Y_u)^{ar} - \frac{5}{6} \delta^{ra} g_L^4 Y_d^{pb} \\
& - T_2 \delta^{ra} (Y_u Y_u^\dagger Y_d)^{pb} - \delta^{ra} (Y_d Y_d^\dagger Y_u Y_u^\dagger Y_d)^{pb} - \delta^{ra} (Y_u Y_u^\dagger Y_u Y_u^\dagger Y_d)^{pb} - \frac{3}{2} (Y_u^\dagger Y_d)^{ab} (Y_u Y_u^\dagger Y_u)^{pr} - \frac{9}{4} \delta^{ra} g_Y^4 Y_d^{pb} \left. \right\} + \left\{ 8Y_e^{bc} Y_u^{pr} (Y_e^\dagger Y_e Y_e^\dagger)^{ad} \right. \\
& - 4\lambda Y_e^{*ad} Y_e^{bc} Y_u^{pr} \left. \right\} \mathcal{C}_{le}^{abcd} + \left\{ \frac{1}{2} Y_u^{pc} (Y_u^\dagger Y_u)^{dr} (Y_e Y_e^\dagger)^{ba} + \frac{1}{2} \delta^{rd} (Y_e Y_e^\dagger)^{ba} (Y_u Y_u^\dagger Y_u)^{pc} + \delta^{rd} g_L^2 Y_u^{pc} (Y_e Y_e^\dagger)^{ba} + \lambda \left( \frac{7}{27} \delta^{rd} \delta^{ab} g_Y^2 Y_u^{pc} + 2\delta^{rd} Y_u^{pc} (Y_e Y_e^\dagger)^{ba} \right) \right. \\
& + g_Y^2 \left( \frac{41}{54} \delta^{rd} \delta^{ab} (Y_u Y_u^\dagger Y_u)^{pc} + \frac{5}{3} \delta^{rd} Y_u^{pc} (Y_e Y_e^\dagger)^{ba} - \frac{35}{54} \delta^{ab} Y_u^{pc} (Y_u^\dagger Y_u)^{dr} \right) + 4\delta^{rd} Y_u^{pc} (Y_e Y_e^\dagger Y_e Y_e^\dagger)^{ba} - \frac{2}{9} \delta^{rd} \delta^{ab} g_Y^4 Y_u^{pc} - \frac{4}{3} \delta^{rd} \delta^{ab} g_Y^2 g_L^2 Y_u^{pc} \left. \right\} \mathcal{C}_{lu}^{abcd} \\
& + \left\{ \frac{1}{2} \delta^{pa} \delta^{cd} g_Y^2 g_L^2 Y_u^{br} + \frac{1}{2} Y_u^{br} (Y_e^\dagger Y_e)^{dc} (Y_u Y_u^\dagger)^{pa} + \frac{1}{2} \delta^{pa} (Y_e^\dagger Y_e)^{dc} (Y_u Y_u^\dagger Y_u)^{br} + \lambda \left( 2\delta^{pa} Y_u^{br} (Y_e^\dagger Y_e)^{dc} - \frac{77}{27} \delta^{pa} \delta^{cd} g_Y^2 Y_u^{br} \right) + g_Y^2 \left( \frac{179}{54} \delta^{pa} \delta^{cd} (Y_u Y_u^\dagger Y_u)^{br} \right. \right. \\
& + \frac{59}{6} \delta^{pa} Y_u^{br} (Y_e^\dagger Y_e)^{dc} - \frac{65}{54} \delta^{cd} Y_u^{br} (Y_u Y_u^\dagger)^{pa} \left. \right) + \frac{29}{18} \delta^{pa} \delta^{cd} g_Y^4 Y_u^{br} + 4\delta^{pa} Y_u^{br} (Y_e^\dagger Y_e Y_e^\dagger Y_e)^{dc} - \frac{3}{2} \delta^{pa} g_L^2 Y_u^{br} (Y_e^\dagger Y_e)^{dc} \left. \right\} \mathcal{C}_{qe}^{abcd} + \left\{ \frac{1}{3} Y_u^{*ad} Y_u^{pc} (Y_u Y_u^\dagger Y_u)^{br} \right. \\
& + \frac{2}{3} Y_u^{*ad} Y_u^{br} (Y_u Y_u^\dagger Y_u)^{pc} + g_Y^4 \left( \frac{2}{9} \delta^{rd} \delta^{ab} Y_u^{pc} + \frac{11}{6} \delta^{pa} \delta^{rd} Y_u^{bc} - \frac{29}{9} \delta^{pa} \delta^{cd} Y_u^{br} \right) + g_Y^2 g_L^2 \left( \frac{4}{3} \delta^{rd} \delta^{ab} Y_u^{pc} - \delta^{pa} \delta^{cd} Y_u^{br} - 3\delta^{pa} \delta^{rd} Y_u^{bc} \right) + Y_u^{bc} (Y_u^\dagger Y_u)^{dr} (Y_d Y_d^\dagger)^{pa} \\
& + Y_u^{*ad} Y_u^{pc} (Y_d Y_d^\dagger Y_u)^{br} + g_L^2 \left( \frac{3}{2} \delta^{pa} Y_u^{bc} (Y_u^\dagger Y_u)^{dr} + 3\delta^{rd} Y_u^{pc} (Y_d Y_d^\dagger)^{ba} + \frac{9}{2} \delta^{pa} Y_u^{br} (Y_u^\dagger Y_u)^{dc} - \frac{3}{2} Y_u^{*ad} Y_u^{pc} Y_u^{br} - 3\delta^{rd} Y_u^{bc} (Y_d Y_d^\dagger)^{pa} - 3\delta^{rd} Y_u^{pc} (Y_u Y_u^\dagger)^{ba} \right. \\
& - 9\delta^{pa} \delta^{rd} (Y_u Y_u^\dagger Y_u)^{bc} \left. \right) + g_Y^2 \left( \frac{5}{9} \delta^{pa} \delta^{rd} (Y_u Y_u^\dagger Y_u)^{bc} + \frac{35}{54} \delta^{ab} Y_u^{pc} (Y_u^\dagger Y_u)^{dr} + \frac{65}{27} \delta^{cd} Y_u^{br} (Y_u Y_u^\dagger)^{pa} - \frac{1}{3} \delta^{rd} Y_u^{bc} (Y_u Y_u^\dagger)^{pa} - \frac{41}{54} \delta^{rd} \delta^{ab} (Y_u Y_u^\dagger Y_u)^{pc} \right. \\
& - Y_u^{*ad} Y_u^{pc} Y_u^{br} - \delta^{rd} Y_u^{pc} (Y_u Y_u^\dagger)^{ba} - \frac{17}{6} \delta^{pa} Y_u^{bc} (Y_u^\dagger Y_u)^{dr} - 3\delta^{rd} Y_u^{pc} (Y_d Y_d^\dagger)^{ba} - \frac{179}{27} \delta^{pa} \delta^{cd} (Y_u Y_u^\dagger Y_u)^{br} - \frac{27}{2} \delta^{pa} Y_u^{br} (Y_u^\dagger Y_u)^{dc} \left. \right) \\
& + g_s^2 \left( \frac{128}{3} \delta^{pa} \delta^{rd} (Y_u Y_u^\dagger Y_u)^{bc} - 16\delta^{pa} Y_u^{bc} (Y_u^\dagger Y_u)^{dr} - 16\delta^{rd} Y_u^{bc} (Y_u Y_u^\dagger)^{pa} \right) + \delta^{pa} Y_u^{bc} (Y_u^\dagger Y_u Y_u^\dagger Y_u)^{dr} + \delta^{rd} Y_u^{bc} (Y_u Y_u^\dagger Y_u Y_u^\dagger)^{pa} + \lambda \left( g_Y^2 \left( \frac{154}{27} \delta^{pa} \delta^{cd} Y_u^{br} \right. \right. \\
& - \frac{7}{27} \delta^{rd} \delta^{ab} Y_u^{pc} - \frac{25}{18} \delta^{pa} \delta^{rd} Y_u^{bc} \left. \right) + 2\delta^{pa} Y_u^{bc} (Y_u^\dagger Y_u)^{dr} + 2\delta^{rd} Y_u^{bc} (Y_u Y_u^\dagger)^{pa} + \frac{9}{2} \delta^{pa} \delta^{rd} (Y_d Y_d^\dagger Y_u)^{bc} + 6\delta^{pa} Y_u^{br} (Y_u^\dagger Y_u)^{dc} + 6\delta^{rd} Y_u^{pc} (Y_d Y_d^\dagger)^{ba} \\
& + 6\delta^{rd} Y_u^{pc} (Y_u Y_u^\dagger)^{ba} + 6\delta^{pa} \delta^{rd} Y_u^{bc} \text{Tr} [Y_u^\dagger Y_u] + 10Y_u^{*ad} Y_u^{pc} Y_u^{br} + 28\delta^{pa} \delta^{rd} (Y_u Y_u^\dagger Y_u)^{bc} - \frac{3}{2} \delta^{pa} \delta^{rd} g_L^2 Y_u^{bc} - 2\delta^{rd} Y_u^{bc} (Y_d Y_d^\dagger)^{pa} - 6Y_u^{*ad} Y_u^{pr} Y_u^{bc}
\end{aligned}$$

$$\begin{aligned}
& -\frac{32}{3}\delta^{pa}\delta^{rd}g_s^2Y_u^{bc}) + \frac{3}{2}\delta^{pa}\delta^{rd}g_L^4Y_u^{bc} + \frac{3}{2}Y_u^{pc}(Y_u^\dagger Y_u)^{dr}(Y_dY_d^\dagger)^{ba} + \frac{3}{2}\delta^{rd}(Y_dY_d^\dagger)^{ba}(Y_uY_u^\dagger Y_u)^{pc} + 2\delta^{rd}(Y_uY_u^\dagger)^{pa}(Y_uY_u^\dagger Y_u)^{bc} + 2\delta^{rd}Y_u^{bc}(Y_uY_u^\dagger Y_dY_d^\dagger)^{pa} \\
& + 3\delta^{pa}\delta^{rd}(Y_dY_d^\dagger Y_dY_d^\dagger Y_u)^{bc} + 4\delta^{rd}(Y_uY_u^\dagger)^{pa}(Y_dY_d^\dagger Y_u)^{bc} + 6\delta^{pa}\delta^{rd}(Y_dY_d^\dagger Y_uY_u^\dagger Y_u)^{bc} + 10\delta^{pa}\delta^{rd}(Y_uY_u^\dagger Y_dY_d^\dagger Y_u)^{bc} + 12Y_u^{*ad}Y_u^{pr}(Y_uY_u^\dagger Y_u)^{bc} \\
& + 12\delta^{rd}Y_u^{pc}(Y_dY_d^\dagger Y_dY_d^\dagger)^{ba} - Y_u^{bc}(Y_u^\dagger Y_u)^{dr}(Y_uY_u^\dagger)^{pa} - \frac{3}{2}Y_u^{br}(Y_u^\dagger Y_u)^{dc}(Y_uY_u^\dagger)^{pa} - \frac{3}{2}Y_u^{pc}(Y_u^\dagger Y_u)^{dr}(Y_uY_u^\dagger)^{ba} - \frac{3}{2}\delta^{rd}(Y_uY_u^\dagger)^{ba}(Y_uY_u^\dagger Y_u)^{pc} \\
& - \frac{3}{2}\delta^{pa}(Y_u^\dagger Y_u)^{dc}(Y_uY_u^\dagger Y_u)^{br} - 2\delta^{rd}Y_u^{bc}(Y_dY_d^\dagger Y_dY_d^\dagger)^{pa} - 4\delta^{rd}(Y_dY_d^\dagger)^{pa}(Y_uY_u^\dagger Y_u)^{bc} - 8\delta^{rd}(Y_dY_d^\dagger)^{pa}(Y_dY_d^\dagger Y_u)^{bc} - 10Y_u^{pc}Y_u^{br}(Y_u^\dagger Y_uY_u^\dagger)^{ad} \\
& - 12\delta^{pa}\delta^{rd}Y_u^{bc}\text{Tr}[Y_u^\dagger Y_uY_u^\dagger Y_u] - 36\delta^{pa}Y_u^{br}(Y_u^\dagger Y_uY_u^\dagger Y_u)^{dc} - 36\delta^{rd}Y_u^{pc}(Y_uY_u^\dagger Y_uY_u^\dagger)^{ba} - 52\delta^{pa}\delta^{rd}(Y_uY_u^\dagger Y_uY_u^\dagger Y_u)^{bc} \Big\} C_{qu}^{(\parallel)abcd} \\
& + \left\{ \frac{1}{2}Y_u^{pc}(Y_u^\dagger Y_u)^{dr}(Y_dY_d^\dagger)^{ba} + \frac{1}{2}\delta^{rd}(Y_dY_d^\dagger)^{ba}(Y_uY_u^\dagger Y_u)^{pc} + g_Y^4\left(\frac{2}{27}\delta^{rd}\delta^{ab}Y_u^{pc} + \frac{11}{2}\delta^{pa}\delta^{rd}Y_u^{bc} - \frac{29}{27}\delta^{pa}\delta^{cd}Y_u^{br}\right) + g_Y^2g_L^2\left(\frac{4}{9}\delta^{rd}\delta^{ab}Y_u^{pc} - \frac{1}{3}\delta^{pa}\delta^{cd}Y_u^{br}\right. \right. \\
& - 9\delta^{pa}\delta^{rd}Y_u^{bc}) + Y_u^{*ad}Y_u^{pc}(Y_uY_u^\dagger Y_u)^{br} + g_L^2\left(\delta^{rd}Y_u^{pc}(Y_dY_d^\dagger)^{ba} + \frac{3}{2}\delta^{pa}Y_u^{br}(Y_u^\dagger Y_u)^{dc} + \frac{9}{2}\delta^{pa}Y_u^{bc}(Y_u^\dagger Y_u)^{dr} - \delta^{rd}Y_u^{pc}(Y_uY_u^\dagger)^{ba} - \frac{9}{2}Y_u^{*ad}Y_u^{pc}Y_u^{br} \right. \\
& - 9\delta^{rd}Y_u^{bc}(Y_dY_d^\dagger)^{pa} - 27\delta^{pa}\delta^{rd}(Y_uY_u^\dagger Y_u)^{bc}) + g_Y^2\left(\frac{35}{162}\delta^{ab}Y_u^{pc}(Y_u^\dagger Y_u)^{dr} + \frac{65}{81}\delta^{cd}Y_u^{br}(Y_uY_u^\dagger)^{pa} + \frac{5}{3}\delta^{pa}\delta^{rd}(Y_uY_u^\dagger Y_u)^{bc} - \frac{41}{162}\delta^{rd}\delta^{ab}(Y_uY_u^\dagger Y_u)^{pc} \right. \\
& - \frac{1}{3}\delta^{rd}Y_u^{pc}(Y_uY_u^\dagger)^{ba} - \delta^{rd}Y_u^{pc}(Y_dY_d^\dagger)^{ba} - \delta^{rd}Y_u^{bc}(Y_uY_u^\dagger)^{pa} - \frac{179}{81}\delta^{pa}\delta^{cd}(Y_uY_u^\dagger Y_u)^{br} - 3Y_u^{*ad}Y_u^{pc}Y_u^{br} - \frac{9}{2}\delta^{pa}Y_u^{br}(Y_u^\dagger Y_u)^{dc} - \frac{17}{2}\delta^{pa}Y_u^{bc}(Y_u^\dagger Y_u)^{dr}) \\
& + g_s^2\left(\frac{80}{27}\delta^{cd}Y_u^{br}(Y_uY_u^\dagger)^{pa} + \frac{160}{27}\delta^{ab}Y_u^{pc}(Y_u^\dagger Y_u)^{dr} + 320\delta^{pa}\delta^{rd}(Y_uY_u^\dagger Y_u)^{bc} - \frac{176}{27}\delta^{pa}\delta^{cd}(Y_uY_u^\dagger Y_u)^{br} - \frac{352}{27}\delta^{rd}\delta^{ab}(Y_uY_u^\dagger Y_u)^{pc} - 32\delta^{pa}Y_u^{br}(Y_u^\dagger Y_u)^{dc} \right. \\
& - 32\delta^{rd}Y_u^{pc}(Y_dY_d^\dagger)^{ba} - 32\delta^{rd}Y_u^{pc}(Y_uY_u^\dagger)^{ba}) + \lambda\left(g_Y^2\left(\frac{154}{81}\delta^{pa}\delta^{cd}Y_u^{br} - \frac{7}{81}\delta^{rd}\delta^{ab}Y_u^{pc} - \frac{25}{6}\delta^{pa}\delta^{rd}Y_u^{bc}\right) + g_s^2\left(\frac{112}{27}\delta^{pa}\delta^{cd}Y_u^{br} + \frac{224}{27}\delta^{rd}\delta^{ab}Y_u^{pc} \right. \right. \\
& - 128\delta^{pa}\delta^{rd}Y_u^{bc}) + 2\delta^{pa}Y_u^{br}(Y_u^\dagger Y_u)^{dc} + 2\delta^{rd}Y_u^{pc}(Y_dY_d^\dagger)^{ba} + 2\delta^{rd}Y_u^{pc}(Y_uY_u^\dagger)^{ba} + 6\delta^{pa}Y_u^{bc}(Y_u^\dagger Y_u)^{dr} + 6\delta^{rd}Y_u^{bc}(Y_uY_u^\dagger)^{pa} + \frac{27}{2}\delta^{pa}\delta^{rd}(Y_dY_d^\dagger Y_u)^{bc} \\
& + 18\delta^{pa}\delta^{rd}Y_u^{bc}\text{Tr}[Y_u^\dagger Y_u] + 30Y_u^{*ad}Y_u^{pc}Y_u^{br} + 84\delta^{pa}\delta^{rd}(Y_uY_u^\dagger Y_u)^{bc} - \frac{9}{2}\delta^{pa}\delta^{rd}g_L^2Y_u^{bc} - 6\delta^{rd}Y_u^{bc}(Y_dY_d^\dagger)^{pa} - 18Y_u^{*ad}Y_u^{pr}Y_u^{bc}) \\
& + 2Y_u^{*ad}Y_u^{br}(Y_uY_u^\dagger Y_u)^{pc} + 3Y_u^{bc}(Y_u^\dagger Y_u)^{dr}(Y_dY_d^\dagger)^{pa} + 3Y_u^{*ad}Y_u^{pc}(Y_dY_d^\dagger Y_u)^{br} + 3\delta^{pa}Y_u^{bc}(Y_u^\dagger Y_uY_u^\dagger Y_u)^{dr} + 3\delta^{rd}Y_u^{bc}(Y_uY_u^\dagger Y_uY_u^\dagger)^{pa} \\
& + 4\delta^{rd}Y_u^{pc}(Y_dY_d^\dagger Y_dY_d^\dagger)^{ba} + \frac{9}{2}\delta^{pa}\delta^{rd}g_L^4Y_u^{bc} + 6\delta^{rd}(Y_uY_u^\dagger)^{pa}(Y_uY_u^\dagger Y_u)^{bc} + 6\delta^{rd}Y_u^{bc}(Y_uY_u^\dagger Y_dY_d^\dagger)^{pa} + 9\delta^{pa}\delta^{rd}(Y_dY_d^\dagger Y_dY_d^\dagger Y_u)^{bc} \\
& + 12\delta^{rd}(Y_uY_u^\dagger)^{pa}(Y_dY_d^\dagger Y_u)^{bc} + 18\delta^{pa}\delta^{rd}(Y_dY_d^\dagger Y_uY_u^\dagger Y_u)^{bc} + 30\delta^{pa}\delta^{rd}(Y_uY_u^\dagger Y_dY_d^\dagger Y_u)^{bc} + 36Y_u^{*ad}Y_u^{pr}(Y_uY_u^\dagger Y_u)^{bc} - \frac{1}{2}Y_u^{br}(Y_u^\dagger Y_u)^{dc}(Y_uY_u^\dagger)^{pa} \\
& - \frac{1}{2}Y_u^{pc}(Y_u^\dagger Y_u)^{dr}(Y_uY_u^\dagger)^{ba} - \frac{1}{2}\delta^{rd}(Y_uY_u^\dagger)^{ba}(Y_uY_u^\dagger Y_u)^{pc} - \frac{1}{2}\delta^{pa}(Y_u^\dagger Y_u)^{dc}(Y_uY_u^\dagger Y_u)^{br} - 3Y_u^{bc}(Y_u^\dagger Y_u)^{dr}(Y_uY_u^\dagger)^{pa} - 6\delta^{rd}Y_u^{bc}(Y_dY_d^\dagger Y_dY_d^\dagger)^{pa} \\
& - 12\delta^{rd}(Y_dY_d^\dagger)^{pa}(Y_uY_u^\dagger Y_u)^{bc} - 12\delta^{pa}Y_u^{br}(Y_u^\dagger Y_uY_u^\dagger Y_u)^{dc} - 12\delta^{rd}Y_u^{pc}(Y_uY_u^\dagger Y_uY_u^\dagger)^{ba} - 24\delta^{rd}(Y_dY_d^\dagger)^{pa}(Y_dY_d^\dagger Y_u)^{bc} - 30Y_u^{pc}Y_u^{br}(Y_u^\dagger Y_uY_u^\dagger)^{ad} \\
& - 36\delta^{pa}\delta^{rd}Y_u^{bc}\text{Tr}[Y_u^\dagger Y_uY_u^\dagger Y_u] - 156\delta^{pa}\delta^{rd}(Y_uY_u^\dagger Y_uY_u^\dagger Y_u)^{bc} \Big\} C_{qu}^{(\times)abcd} + \left\{ \frac{1}{2}\delta^{pa}\delta^{cd}g_Y^2g_L^2Y_u^{br} + \frac{2}{3}Y_d^{bc}(Y_d^\dagger Y_u)^{dr}(Y_uY_u^\dagger)^{pa} + \lambda\left(\frac{5}{2}Y_d^{*ad}Y_d^{pc}Y_u^{br} \right. \right.
\end{aligned}$$

$$\begin{aligned}
& + 6\delta^{pa}Y_u^{br}(Y_d^\dagger Y_d)^{dc} - 2\delta^{pa}Y_d^{bc}(Y_d^\dagger Y_u)^{dr} - \frac{77}{27}\delta^{pa}\delta^{cd}g_Y^2Y_u^{br} - 12Y_d^{*ad}Y_d^{bc}Y_u^{pr} + Y_d^{*ad}Y_u^{br}(Y_dY_d^\dagger Y_d)^{pc} + g_Y^2\left(\frac{179}{54}\delta^{pa}\delta^{cd}(Y_uY_u^\dagger Y_u)^{br}\right. \\
& - \frac{65}{54}\delta^{cd}Y_u^{br}(Y_uY_u^\dagger)^{pa} - \frac{5}{2}\delta^{pa}Y_u^{br}(Y_d^\dagger Y_d)^{dc}\Big) + \delta^{pa}Y_d^{bc}(Y_d^\dagger Y_uY_u^\dagger Y_u)^{dr} + \frac{3}{2}Y_u^{br}(Y_d^\dagger Y_d)^{dc}(Y_uY_u^\dagger)^{pa} + \frac{3}{2}\delta^{pa}(Y_d^\dagger Y_d)^{dc}(Y_uY_u^\dagger Y_u)^{br} + \frac{29}{18}\delta^{pa}\delta^{cd}g_Y^4Y_u^{br} \\
& + 12\delta^{pa}Y_u^{br}(Y_d^\dagger Y_dY_d^\dagger Y_d)^{dc} + 24Y_d^{bc}Y_u^{pr}(Y_d^\dagger Y_dY_d^\dagger)^{ad} - \frac{1}{3}Y_d^{*ad}Y_u^{br}(Y_uY_u^\dagger Y_d)^{pc} - g_L^2\left(\frac{3}{2}Y_d^{*ad}Y_d^{pc}Y_u^{br} + \frac{9}{2}\delta^{pa}Y_u^{br}(Y_d^\dagger Y_d)^{dc}\right) - \delta^{pa}Y_d^{bc}(Y_d^\dagger Y_dY_d^\dagger Y_u)^{dr} \\
& - 2\delta^{pa}(Y_d^\dagger Y_u)^{dr}(Y_dY_d^\dagger Y_d)^{bc} - 3Y_d^{pc}Y_u^{br}(Y_d^\dagger Y_dY_d^\dagger)^{ad} - 4\delta^{pa}(Y_d^\dagger Y_u)^{dr}(Y_uY_u^\dagger Y_d)^{bc}\Big\}C_{qd}^{(\parallel)abcd} + \left\{\frac{1}{6}\delta^{pa}\delta^{cd}g_Y^2g_L^2Y_u^{br} + \frac{1}{2}Y_u^{br}(Y_d^\dagger Y_d)^{dc}(Y_uY_u^\dagger)^{pa}\right. \\
& + \frac{1}{2}\delta^{pa}(Y_d^\dagger Y_d)^{dc}(Y_uY_u^\dagger Y_u)^{br} + \frac{29}{54}\delta^{pa}\delta^{cd}g_Y^4Y_u^{br} + \lambda\left(2\delta^{pa}Y_u^{br}(Y_d^\dagger Y_d)^{dc} + \frac{112}{27}\delta^{pa}\delta^{cd}g_s^2Y_u^{br} + \frac{15}{2}Y_d^{*ad}Y_d^{pc}Y_u^{br} - \frac{77}{81}\delta^{pa}\delta^{cd}g_Y^2Y_u^{br}\right. \\
& - 6\delta^{pa}Y_d^{bc}(Y_d^\dagger Y_u)^{dr} - 36Y_d^{*ad}Y_d^{bc}Y_u^{pr}\Big) + g_s^2\left(\frac{80}{27}\delta^{cd}Y_u^{br}(Y_uY_u^\dagger)^{pa} - \frac{176}{27}\delta^{pa}\delta^{cd}(Y_uY_u^\dagger Y_u)^{br} - 32\delta^{pa}Y_u^{br}(Y_d^\dagger Y_d)^{dc}\right) + g_Y^2\left(\frac{179}{162}\delta^{pa}\delta^{cd}(Y_uY_u^\dagger Y_u)^{br}\right. \\
& - \frac{65}{162}\delta^{cd}Y_u^{br}(Y_uY_u^\dagger)^{pa} - \frac{5}{6}\delta^{pa}Y_u^{br}(Y_d^\dagger Y_d)^{dc}\Big) + 2Y_d^{bc}(Y_d^\dagger Y_u)^{dr}(Y_uY_u^\dagger)^{pa} + 3Y_d^{*ad}Y_u^{br}(Y_dY_d^\dagger Y_d)^{pc} + 3\delta^{pa}Y_d^{bc}(Y_d^\dagger Y_uY_u^\dagger Y_u)^{dr} + 4\delta^{pa}Y_u^{br}(Y_d^\dagger Y_dY_d^\dagger Y_d)^{dc} \\
& + 72Y_d^{bc}Y_u^{pr}(Y_d^\dagger Y_dY_d^\dagger)^{ad} - g_L^2\left(\frac{3}{2}\delta^{pa}Y_u^{br}(Y_d^\dagger Y_d)^{dc} + \frac{9}{2}Y_d^{*ad}Y_d^{pc}Y_u^{br}\right) - Y_d^{*ad}Y_u^{br}(Y_uY_u^\dagger Y_d)^{pc} - 3\delta^{pa}Y_d^{bc}(Y_d^\dagger Y_dY_d^\dagger Y_u)^{dr} - 6\delta^{pa}(Y_d^\dagger Y_u)^{dr}(Y_dY_d^\dagger Y_d)^{bc} \\
& - 9Y_d^{pc}Y_u^{br}(Y_d^\dagger Y_dY_d^\dagger)^{ad} - 12\delta^{pa}(Y_d^\dagger Y_u)^{dr}(Y_uY_u^\dagger Y_d)^{bc}\Big\}C_{qd}^{(\times)abcd} + \left\{\frac{8}{3}\delta^{ad}g_Y^2Y_u^{pr}(Y_e^\dagger Y_e)^{bc} - \frac{4}{9}\delta^{ab}\delta^{cd}g_Y^4Y_u^{pr} - 4Y_u^{pr}(Y_e^\dagger Y_e)^{ba}(Y_e^\dagger Y_e)^{dc}\right\}C_{ee}^{abcd} \\
& + \left\{g_Y^4\left(\frac{20}{27}\delta^{rb}\delta^{ad}Y_u^{pc} + \frac{8}{9}\delta^{rb}\delta^{cd}Y_u^{pa} - \frac{16}{27}\delta^{ad}\delta^{bc}Y_u^{pr}\right) + g_Y^2g_L^2\left(\frac{4}{9}\delta^{rb}\delta^{ad}Y_u^{pc} + \frac{16}{3}\delta^{rb}\delta^{cd}Y_u^{pa}\right) + Y_u^{pc}(Y_u^\dagger Y_u)^{br}(Y_u^\dagger Y_u)^{da} + \lambda\left(\frac{32}{27}\delta^{rb}\delta^{ad}g_s^2Y_u^{pc}\right.\right. \\
& + 24\delta^{rb}Y_u^{pa}(Y_u^\dagger Y_u)^{dc} - g_Y^2\left(\frac{4}{81}\delta^{rb}\delta^{ad}Y_u^{pc} + \frac{28}{27}\delta^{rb}\delta^{cd}Y_u^{pa}\right)\Big) + g_Y^2\left(\frac{70}{81}\delta^{ad}Y_u^{pc}(Y_u^\dagger Y_u)^{br} + \frac{86}{81}\delta^{rb}\delta^{ad}(Y_uY_u^\dagger Y_u)^{pc} + \frac{70}{27}\delta^{cd}Y_u^{pa}(Y_u^\dagger Y_u)^{br}\right. \\
& + \frac{16}{3}\delta^{ad}Y_u^{pr}(Y_u^\dagger Y_u)^{bc} - \frac{82}{27}\delta^{rb}\delta^{cd}(Y_uY_u^\dagger Y_u)^{pa} - 8\delta^{rb}Y_u^{pc}(Y_u^\dagger Y_u)^{da} - 18\delta^{rb}Y_u^{pa}(Y_u^\dagger Y_u)^{dc}\Big) + g_s^2\left(\frac{32}{27}\delta^{rb}\delta^{ad}(Y_uY_u^\dagger Y_u)^{pc} + \frac{160}{27}\delta^{ad}Y_u^{pc}(Y_u^\dagger Y_u)^{br}\right. \\
& - 64\delta^{rb}Y_u^{pc}(Y_u^\dagger Y_u)^{da}\Big) + 3Y_u^{pa}(Y_u^\dagger Y_u)^{br}(Y_u^\dagger Y_u)^{dc} + 3\delta^{rb}(Y_u^\dagger Y_u)^{dc}(Y_uY_u^\dagger Y_u)^{pa} + 8\delta^{rb}Y_u^{pc}(Y_u^\dagger Y_uY_u^\dagger Y_u)^{da} - g_L^2\left(4\delta^{rb}Y_u^{pc}(Y_u^\dagger Y_u)^{da} + 30\delta^{rb}Y_u^{pa}(Y_u^\dagger Y_u)^{dc}\right) \\
& - 3\delta^{rb}(Y_u^\dagger Y_u)^{da}(Y_uY_u^\dagger Y_u)^{pc} - 12Y_u^{pr}(Y_u^\dagger Y_u)^{bc}(Y_u^\dagger Y_u)^{da}\Big\}C_{uu}^{abcd} + \left\{\frac{8}{3}\delta^{ad}g_Y^2Y_u^{pr}(Y_d^\dagger Y_d)^{bc} - \frac{4}{27}\delta^{ad}\delta^{bc}g_Y^4Y_u^{pr} - 12Y_u^{pr}(Y_d^\dagger Y_d)^{bc}(Y_d^\dagger Y_d)^{da}\right\}C_{dd}^{abcd} \\
& + \left\{\lambda\left(\frac{7}{27}\delta^{rd}\delta^{ab}g_Y^2Y_u^{pc} - 2\delta^{rd}Y_u^{pc}(Y_e^\dagger Y_e)^{ba}\right) + g_Y^2\left(\frac{41}{54}\delta^{rd}\delta^{ab}(Y_uY_u^\dagger Y_u)^{pc} + \frac{13}{3}\delta^{rd}Y_u^{pc}(Y_e^\dagger Y_e)^{ba} - \frac{35}{54}\delta^{ab}Y_u^{pc}(Y_u^\dagger Y_u)^{dr}\right) + 5\delta^{rd}g_L^2Y_u^{pc}(Y_e^\dagger Y_e)^{ba}\right. \\
& - \frac{2}{9}\delta^{rd}\delta^{ab}g_Y^4Y_u^{pc} - \frac{1}{2}Y_u^{pc}(Y_e^\dagger Y_e)^{ba}(Y_u^\dagger Y_u)^{dr} - \frac{1}{2}\delta^{rd}(Y_e^\dagger Y_e)^{ba}(Y_uY_u^\dagger Y_u)^{pc} - \frac{4}{3}\delta^{rd}\delta^{ab}g_Y^2g_L^2Y_u^{pc} - 4\delta^{rd}Y_u^{pc}(Y_e^\dagger Y_eY_e^\dagger Y_e)^{ba}\Big\}C_{eu}^{abcd} \\
& + \left\{g_L^2\left(15\delta^{rb}Y_u^{pa}(Y_d^\dagger Y_d)^{dc} - 4\delta^{rb}Y_d^{pc}(Y_d^\dagger Y_u)^{da}\right) + \lambda\left(\frac{7}{27}\delta^{rb}\delta^{cd}g_Y^2Y_u^{pa} - \frac{3}{2}\delta^{rb}Y_d^{pc}(Y_d^\dagger Y_u)^{da} - 6\delta^{rb}Y_u^{pa}(Y_d^\dagger Y_d)^{dc}\right) + g_Y^2\left(\frac{41}{54}\delta^{rb}\delta^{cd}(Y_uY_u^\dagger Y_u)^{pa}\right.\right.
\end{aligned}$$

$$\begin{aligned}
& + 5\delta^{rb}Y_u^{pa}(Y_d^\dagger Y_d)^{dc} - \frac{35}{54}\delta^{cd}Y_u^{pa}(Y_u^\dagger Y_u)^{br}) + 2Y_u^{pa}(Y_d^\dagger Y_u)^{dr}(Y_u^\dagger Y_d)^{bc} + 4\delta^{rb}Y_d^{pc}(Y_d^\dagger Y_u Y_u^\dagger Y_u)^{da} + 7\delta^{rb}Y_d^{pc}(Y_d^\dagger Y_d Y_d^\dagger Y_u)^{da} - \frac{2}{9}\delta^{rb}\delta^{cd}g_Y^4 Y_u^{pa} \\
& - Y_d^{pc}(Y_d^\dagger Y_u)^{da}(Y_u^\dagger Y_u)^{br} - \frac{4}{3}\delta^{rb}\delta^{cd}g_Y^2 g_L^2 Y_u^{pa} - \frac{3}{2}Y_u^{pa}(Y_d^\dagger Y_d)^{dc}(Y_u^\dagger Y_u)^{br} - \frac{3}{2}\delta^{rb}(Y_d^\dagger Y_d)^{dc}(Y_u Y_u^\dagger Y_u)^{pa} - 3\delta^{rb}(Y_d^\dagger Y_u)^{da}(Y_u Y_u^\dagger Y_d)^{pc} \\
& - 12\delta^{rb}Y_u^{pa}(Y_d^\dagger Y_d Y_d^\dagger Y_d)^{dc} \Big\} C_{ud}^{(\parallel)abcd} + \Big\{ g_L^2 \Big( 5\delta^{rb}Y_u^{pa}(Y_d^\dagger Y_d)^{dc} - 12\delta^{rb}Y_d^{pc}(Y_d^\dagger Y_u)^{da} \Big) + \lambda \Big( \frac{7}{81}\delta^{rb}\delta^{cd}g_Y^2 Y_u^{pa} + \frac{112}{27}\delta^{rb}\delta^{cd}g_s^2 Y_u^{pa} - 2\delta^{rb}Y_u^{pa}(Y_d^\dagger Y_d)^{dc} \\
& - \frac{9}{2}\delta^{rb}Y_d^{pc}(Y_d^\dagger Y_u)^{da} \Big) + g_s^2 \Big( \frac{80}{27}\delta^{cd}Y_u^{pa}(Y_u^\dagger Y_u)^{br} - \frac{176}{27}\delta^{rb}\delta^{cd}(Y_u Y_u^\dagger Y_u)^{pa} - 32\delta^{rb}Y_u^{pa}(Y_d^\dagger Y_d)^{dc} \Big) + g_Y^2 \Big( \frac{41}{162}\delta^{rb}\delta^{cd}(Y_u Y_u^\dagger Y_u)^{pa} + \frac{5}{3}\delta^{rb}Y_u^{pa}(Y_d^\dagger Y_d)^{dc} \\
& - \frac{35}{162}\delta^{cd}Y_u^{pa}(Y_u^\dagger Y_u)^{br} \Big) + 6Y_u^{pa}(Y_d^\dagger Y_u)^{dr}(Y_u^\dagger Y_d)^{bc} + 12\delta^{rb}Y_d^{pc}(Y_d^\dagger Y_u Y_u^\dagger Y_u)^{da} + 21\delta^{rb}Y_d^{pc}(Y_d^\dagger Y_d Y_d^\dagger Y_u)^{da} - \frac{2}{27}\delta^{rb}\delta^{cd}g_Y^4 Y_u^{pa} - \frac{4}{9}\delta^{rb}\delta^{cd}g_Y^2 g_L^2 Y_u^{pa} \\
& - \frac{1}{2}Y_u^{pa}(Y_d^\dagger Y_d)^{dc}(Y_u^\dagger Y_u)^{br} - \frac{1}{2}\delta^{rb}(Y_d^\dagger Y_d)^{dc}(Y_u Y_u^\dagger Y_u)^{pa} - 3Y_d^{pc}(Y_d^\dagger Y_u)^{da}(Y_u^\dagger Y_u)^{br} - 4\delta^{rb}Y_u^{pa}(Y_d^\dagger Y_d Y_d^\dagger Y_d)^{dc} - 9\delta^{rb}(Y_d^\dagger Y_u)^{da}(Y_u Y_u^\dagger Y_d)^{pc} \Big\} C_{ud}^{(\times)abcd} \\
& + \Big\{ \frac{1}{6}Y_e^{*ab}Y_u^{dr}(Y_u Y_u^\dagger Y_d)^{pc} + \frac{3}{4}g_L^2 Y_e^{*ab}Y_d^{pc}Y_u^{dr} + Y_d^{pc}Y_u^{dr}(Y_e^\dagger Y_e Y_e^\dagger)^{ab} - \frac{1}{2}Y_e^{*ab}Y_u^{dr}(Y_d Y_d^\dagger Y_d)^{pc} - \lambda Y_e^{*ab}Y_d^{pc}Y_u^{dr} \Big\} C_{ledq}^{abcd} \\
& + C_{ledq}^{*abcd} \Big\{ \delta^{pd}\lambda Y_e^{ab}(Y_d^\dagger Y_u)^{cr} + \frac{3}{2}\delta^{pd}Y_e^{ab}(Y_d^\dagger Y_d Y_d^\dagger Y_u)^{cr} - \frac{1}{3}Y_e^{ab}(Y_d^\dagger Y_u)^{cr}(Y_u Y_u^\dagger)^{pd} - \frac{1}{2}\delta^{pd}Y_e^{ab}(Y_d^\dagger Y_u Y_u^\dagger Y_u)^{cr} - \frac{3}{4}\delta^{pd}g_L^2 Y_e^{ab}(Y_d^\dagger Y_u)^{cr} \Big\} \\
& + \Big\{ \frac{1}{4}Y_d^{*ad}(Y_u^\dagger Y_u)^{br}(Y_u Y_u^\dagger)^{pc} + \frac{3}{4}\delta^{pa}Y_u^{*cb}(Y_d^\dagger Y_d Y_d^\dagger Y_u)^{dr} + g_Y^2 g_L^2 \Big( \frac{9}{2}\delta^{pa}\delta^{rb}Y_d^{*cd} - \frac{1}{2}\delta^{pc}\delta^{rb}Y_d^{*ad} \Big) + g_Y^4 \Big( \frac{5}{9}\delta^{pc}\delta^{rb}Y_d^{*ad} + \frac{5}{4}\delta^{pa}\delta^{rb}Y_d^{*cd} \Big) \\
& + g_L^4 \Big( \frac{3}{2}\delta^{pc}\delta^{rb}Y_d^{*ad} - \frac{9}{4}\delta^{pa}\delta^{rb}Y_d^{*cd} \Big) + g_Y^2 \Big( \frac{23}{48}\delta^{pc}Y_d^{*ad}(Y_u^\dagger Y_u)^{br} + \frac{9}{8}\delta^{pa}Y_d^{*cd}(Y_u^\dagger Y_u)^{br} + \frac{61}{36}\delta^{pc}\delta^{rb}(Y_d^\dagger Y_d Y_d^\dagger)^{ad} + \frac{8}{3}\delta^{pa}\delta^{rb}(Y_d^\dagger Y_d Y_d^\dagger)^{cd} \\
& - \frac{25}{48}\delta^{rb}Y_d^{*ad}(Y_u Y_u^\dagger)^{pc} - \frac{21}{8}\delta^{rb}Y_d^{*cd}(Y_u Y_u^\dagger)^{pa} \Big) + \delta^{pa}(Y_d^\dagger Y_u)^{dr}(Y_d^\dagger Y_d Y_u^\dagger)^{cb} + g_L^2 \Big( \frac{9}{8}\delta^{rb}Y_d^{*cd}(Y_u Y_u^\dagger)^{pa} + \frac{5}{2}\delta^{rb}Y_d^{*ad}(Y_d Y_d^\dagger)^{pc} + 3\delta^{pc}\delta^{rb}(Y_u^\dagger Y_u Y_d^\dagger)^{ad} \\
& + \frac{15}{4}\delta^{pc}\delta^{rb}(Y_d^\dagger Y_d Y_d^\dagger)^{ad} - \frac{1}{16}\delta^{rb}Y_d^{*ad}(Y_u Y_u^\dagger)^{pc} - \frac{5}{8}\delta^{pa}Y_u^{*cb}(Y_d^\dagger Y_u)^{dr} - \frac{23}{16}\delta^{pc}Y_d^{*ad}(Y_u^\dagger Y_u)^{br} - \frac{9}{4}\delta^{pc}Y_u^{*ab}(Y_d^\dagger Y_u)^{dr} - \frac{27}{8}\delta^{pa}Y_d^{*cd}(Y_u^\dagger Y_u)^{br} \Big) \\
& + \delta^{rb}Y_d^{*ad}(Y_d Y_d^\dagger Y_d Y_d^\dagger)^{pc} + \lambda \Big( \frac{1}{2}\delta^{pa}Y_u^{*cb}(Y_d^\dagger Y_u)^{dr} + \frac{3}{4}\delta^{rb}Y_d^{*ad}(Y_d Y_d^\dagger)^{pc} + g_L^2 \Big( \frac{9}{4}\delta^{pa}\delta^{rb}Y_d^{*cd} - \frac{3}{8}\delta^{pc}\delta^{rb}Y_d^{*ad} \Big) + g_s^2 \Big( 12\delta^{pc}\delta^{rb}Y_d^{*ad} + 40\delta^{pa}\delta^{rb}Y_d^{*cd} \Big) \\
& + 3\delta^{pc}Y_u^{*ab}(Y_d^\dagger Y_u)^{dr} + \frac{9}{2}\delta^{rb}Y_d^{*cd}(Y_d Y_d^\dagger)^{pa} - \frac{1}{4}\delta^{pc}\delta^{rb}(Y_d^\dagger Y_d Y_d^\dagger)^{ad} - \frac{3}{4}\delta^{pc}\delta^{rb}(Y_u^\dagger Y_u Y_d^\dagger)^{ad} - g_Y^2 \Big( \frac{7}{24}\delta^{pc}\delta^{rb}Y_d^{*ad} + \frac{11}{12}\delta^{pa}\delta^{rb}Y_d^{*cd} \Big) - \Big( \frac{3}{2}\delta^{pc}\delta^{rb}Y_d^{*ad} \\
& + 9\delta^{pa}\delta^{rb}Y_d^{*cd} \Big) \text{Tr}[Y_u^\dagger Y_u] - \frac{3}{2}\delta^{pc}Y_d^{*ad}(Y_u^\dagger Y_u)^{br} - \frac{3}{2}\delta^{pa}\delta^{rb}(Y_d^\dagger Y_d Y_d^\dagger)^{cd} - \frac{7}{4}\delta^{rb}Y_d^{*ad}(Y_u Y_u^\dagger)^{pc} - \frac{15}{2}\delta^{pa}\delta^{rb}(Y_u^\dagger Y_u Y_d^\dagger)^{cd} - 9\delta^{pa}Y_d^{*cd}(Y_u^\dagger Y_u)^{br} \\
& - \frac{21}{2}\delta^{rb}Y_d^{*cd}(Y_u Y_u^\dagger)^{pa} \Big) + \Big( 3\delta^{pc}\delta^{rb}Y_d^{*ad} + 18\delta^{pa}\delta^{rb}Y_d^{*cd} \Big) \text{Tr}[Y_u^\dagger Y_u Y_u^\dagger Y_u] + \frac{3}{2}Y_d^{*cd}(Y_u^\dagger Y_u)^{br}(Y_u Y_u^\dagger)^{pa} + 2\delta^{pc}(Y_u^\dagger Y_u)^{br}(Y_d^\dagger Y_d Y_d^\dagger)^{ad} \\
& + 2\delta^{rb}(Y_u Y_u^\dagger)^{pc}(Y_d^\dagger Y_d Y_d^\dagger)^{ad} + 2\delta^{rb}(Y_d Y_d^\dagger)^{pc}(Y_u^\dagger Y_u Y_d^\dagger)^{ad} + \frac{9}{2}\delta^{pc}Y_u^{*ab}(Y_d^\dagger Y_d Y_d^\dagger Y_u)^{dr} + 6\delta^{pc}(Y_d^\dagger Y_u)^{dr}(Y_d^\dagger Y_d Y_u^\dagger)^{ab} + 6\delta^{rb}Y_d^{*cd}(Y_d Y_d^\dagger Y_d Y_d^\dagger)^{pa} \\
& + 10\delta^{pc}\delta^{rb}(Y_d^\dagger Y_d Y_d^\dagger Y_d Y_d^\dagger)^{da} + 12\delta^{pa}(Y_u^\dagger Y_u)^{br}(Y_d^\dagger Y_d Y_d^\dagger)^{cd} + 12\delta^{rb}(Y_u Y_u^\dagger)^{pa}(Y_d^\dagger Y_d Y_d^\dagger)^{cd} + 12\delta^{rb}(Y_d Y_d^\dagger)^{pa}(Y_u^\dagger Y_u Y_d^\dagger)^{cd}
\end{aligned}$$

$$\begin{aligned}
& + 60\delta^{pa}\delta^{rb}(Y_d^\dagger Y_d Y_d^\dagger Y_d Y_d^\dagger)^{dc} - \frac{1}{6}Y_u^{*cb}(Y_d^\dagger Y_u)^{dr}(Y_u Y_u^\dagger)^{pa} - \frac{1}{4}Y_d^{*ad}(Y_u^\dagger Y_u)^{br}(Y_d Y_d^\dagger)^{pc} - \frac{1}{4}\delta^{pa}Y_u^{*cb}(Y_d^\dagger Y_u Y_u^\dagger Y_u)^{dr} - \frac{1}{4}\delta^{pc}Y_d^{*ad}(Y_u^\dagger Y_u Y_u^\dagger Y_u)^{br} \\
& - \frac{1}{4}\delta^{rb}Y_d^{*ad}(Y_u Y_u^\dagger Y_u Y_u^\dagger)^{pc} - \frac{1}{2}\delta^{rb}Y_d^{*ad}(Y_u Y_u^\dagger Y_d Y_d^\dagger)^{pc} - Y_u^{*ab}(Y_d^\dagger Y_u)^{dr}(Y_u Y_u^\dagger)^{pc} - g_s^2\left(4\delta^{pc}Y_d^{*ad}(Y_u^\dagger Y_u)^{br} + 4\delta^{rb}Y_d^{*ad}(Y_u Y_u^\dagger)^{pc}\right. \\
& + \frac{176}{3}\delta^{pc}\delta^{rb}(Y_d^\dagger Y_d Y_d^\dagger)^{ad} + 64\delta^{pa}\delta^{rb}(Y_d^\dagger Y_d Y_d^\dagger)^{cd}\Big) - \delta^{rb}(Y_u Y_u^\dagger)^{pc}(Y_u^\dagger Y_u Y_d^\dagger)^{ad} - \delta^{pc}\delta^{rb}(Y_d^\dagger Y_d Y_d^\dagger Y_u Y_u^\dagger)^{da} - \delta^{pc}\delta^{rb}(Y_d^\dagger Y_u Y_u^\dagger Y_d Y_d^\dagger)^{da} \\
& - \frac{3}{2}Y_d^{*cd}(Y_u^\dagger Y_u)^{br}(Y_d Y_d^\dagger)^{pa} - \frac{3}{2}\delta^{pc}Y_u^{*ab}(Y_d^\dagger Y_u Y_u^\dagger Y_u)^{dr} - \frac{3}{2}\delta^{pa}Y_d^{*cd}(Y_u^\dagger Y_u Y_u^\dagger Y_u)^{br} - \frac{3}{2}\delta^{rb}Y_d^{*cd}(Y_u Y_u^\dagger Y_u Y_u^\dagger)^{pa} - 2\delta^{pc}\delta^{rb}(Y_d^\dagger Y_u Y_u^\dagger Y_u Y_u^\dagger)^{da} \\
& - 3\delta^{rb}Y_d^{*cd}(Y_u Y_u^\dagger Y_d Y_d^\dagger)^{pa} - 6\delta^{rb}(Y_u Y_u^\dagger)^{pa}(Y_u^\dagger Y_u Y_d^\dagger)^{cd} - 6\delta^{pa}\delta^{rb}(Y_d^\dagger Y_d Y_d^\dagger Y_u Y_u^\dagger)^{dc} - 6\delta^{pa}\delta^{rb}(Y_d^\dagger Y_u Y_u^\dagger Y_d Y_d^\dagger)^{dc} \\
& - 6\delta^{pa}\delta^{rb}(Y_d^\dagger Y_u Y_u^\dagger Y_u Y_u^\dagger)^{dc}\Big\} C_{quqd}^{(\parallel)abcd} + \left(C_{quqd}^{(\parallel)*}\right)^{abcd}\Big\{ \frac{1}{12}Y_u^{ar}Y_u^{cb}(Y_u Y_u^\dagger Y_d)^{pd} + \frac{1}{2}Y_u^{ab}Y_u^{cr}(Y_u Y_u^\dagger Y_d)^{pd} + g_Y^2\left(\frac{19}{36}Y_d^{ad}Y_u^{pb}Y_u^{cr} + \frac{3}{2}Y_d^{cd}Y_u^{pb}Y_u^{ar}\right) \\
& + g_L^2\left(\frac{3}{4}Y_d^{ad}Y_u^{pb}Y_u^{cr} + \frac{3}{2}Y_d^{pd}Y_u^{ar}Y_u^{cb} + \frac{9}{4}Y_d^{cd}Y_u^{pb}Y_u^{ar} + \frac{9}{4}Y_d^{pd}Y_u^{ab}Y_u^{cr}\right) + \lambda\left(\frac{1}{2}Y_d^{pd}Y_u^{ar}Y_u^{cb} - \frac{3}{2}Y_d^{ad}Y_u^{pr}Y_u^{cb} - \frac{5}{2}Y_d^{ad}Y_u^{pb}Y_u^{cr} - 9Y_d^{cd}Y_u^{pr}Y_u^{ab} - 15Y_d^{cd}Y_u^{pb}Y_u^{ar}\right) \\
& + \frac{5}{2}Y_u^{pb}Y_u^{cr}(Y_d Y_d^\dagger Y_d)^{ad} + 3Y_d^{ad}Y_u^{pr}(Y_u Y_u^\dagger Y_u)^{cb} + 15Y_u^{pb}Y_u^{ar}(Y_d Y_d^\dagger Y_d)^{cd} + 18Y_d^{cd}Y_u^{pr}(Y_u Y_u^\dagger Y_u)^{ab} - \frac{1}{12}Y_d^{ad}Y_u^{pb}(Y_u Y_u^\dagger Y_u)^{cr} - \frac{1}{6}Y_d^{ad}Y_u^{cr}(Y_u Y_u^\dagger Y_u)^{pb} \\
& - \frac{1}{4}Y_u^{ar}Y_u^{cb}(Y_d Y_d^\dagger Y_d)^{pd} - \frac{1}{4}Y_d^{ad}Y_u^{pb}(Y_d Y_d^\dagger Y_u)^{cr} - \frac{1}{2}Y_d^{cd}Y_u^{pb}(Y_u Y_u^\dagger Y_u)^{ar} - Y_d^{cd}Y_u^{ar}(Y_u Y_u^\dagger Y_u)^{pb} - \frac{3}{2}Y_u^{ab}Y_u^{cr}(Y_d Y_d^\dagger Y_d)^{pd} - \frac{3}{2}Y_d^{cd}Y_u^{pb}(Y_d Y_d^\dagger Y_u)^{ar} \\
& - \frac{3}{2}Y_d^{pd}Y_u^{ar}(Y_u Y_u^\dagger Y_u)^{cb} - 3Y_d^{pd}Y_u^{cr}(Y_u Y_u^\dagger Y_u)^{ab} - \frac{32}{3}g_s^2Y_d^{ad}Y_u^{pb}Y_u^{cr}\Big\} + \left\{ \frac{1}{2}Y_d^{*cd}(Y_u^\dagger Y_u)^{br}(Y_u Y_u^\dagger)^{pa} + \frac{3}{4}Y_d^{*ad}(Y_u^\dagger Y_u)^{br}(Y_u Y_u^\dagger)^{pc} + g_Y^2 g_L^2\left(\frac{3}{2}\delta^{pa}\delta^{rb}Y_d^{*cd}\right. \right. \\
& - \frac{3}{2}\delta^{pc}\delta^{rb}Y_d^{*ad}\Big) + g_Y^4\left(\frac{5}{12}\delta^{pa}\delta^{rb}Y_d^{*cd} + \frac{5}{3}\delta^{pc}\delta^{rb}Y_d^{*ad}\right) + g_L^4\left(\frac{9}{2}\delta^{pc}\delta^{rb}Y_d^{*ad} - \frac{3}{4}\delta^{pa}\delta^{rb}Y_d^{*cd}\right) + g_Y^2\left(\frac{3}{8}\delta^{pa}Y_d^{*cd}(Y_u^\dagger Y_u)^{br} + \frac{8}{9}\delta^{pa}\delta^{rb}(Y_d^\dagger Y_d Y_d^\dagger)^{cd}\right. \\
& + \frac{23}{16}\delta^{pc}Y_d^{*ad}(Y_u^\dagger Y_u)^{br} + \frac{61}{12}\delta^{pc}\delta^{rb}(Y_d^\dagger Y_d Y_d^\dagger)^{ad} - \frac{7}{8}\delta^{rb}Y_d^{*cd}(Y_u Y_u^\dagger)^{pa} - \frac{25}{16}\delta^{rb}Y_d^{*ad}(Y_u Y_u^\dagger)^{pc}\Big) + g_L^2\left(\frac{3}{8}\delta^{rb}Y_d^{*cd}(Y_u Y_u^\dagger)^{pa} + \frac{15}{2}\delta^{rb}Y_d^{*ad}(Y_d Y_d^\dagger)^{pc}\right. \\
& + 9\delta^{pc}\delta^{rb}(Y_u^\dagger Y_u Y_d^\dagger)^{ad} + \frac{45}{4}\delta^{pc}\delta^{rb}(Y_d^\dagger Y_d Y_d^\dagger)^{ad} - \frac{3}{16}\delta^{rb}Y_d^{*ad}(Y_u Y_u^\dagger)^{pc} - \frac{3}{4}\delta^{pc}Y_u^{*ab}(Y_d^\dagger Y_u)^{dr} - \frac{9}{8}\delta^{pa}Y_d^{*cd}(Y_u^\dagger Y_u)^{br} - \frac{15}{8}\delta^{pa}Y_u^{*cb}(Y_d^\dagger Y_u)^{dr} \\
& - \frac{69}{16}\delta^{pc}Y_d^{*ad}(Y_u^\dagger Y_u)^{br}\Big) + \lambda\left(g_L^2\left(\frac{3}{4}\delta^{pa}\delta^{rb}Y_d^{*cd} - \frac{9}{8}\delta^{pc}\delta^{rb}Y_d^{*ad}\right) + g_s^2\left(\frac{40}{3}\delta^{pa}\delta^{rb}Y_d^{*cd} + 48\delta^{pc}\delta^{rb}Y_d^{*ad}\right) + \delta^{pc}Y_u^{*ab}(Y_d^\dagger Y_u)^{dr} + \frac{3}{2}\delta^{pa}Y_u^{*cb}(Y_d^\dagger Y_u)^{dr}\right. \\
& + \frac{3}{2}\delta^{rb}Y_d^{*cd}(Y_d Y_d^\dagger)^{pa} + \frac{9}{4}\delta^{rb}Y_d^{*ad}(Y_d Y_d^\dagger)^{pc} - \frac{1}{2}\delta^{pa}\delta^{rb}(Y_d^\dagger Y_d Y_d^\dagger)^{cd} - \frac{3}{4}\delta^{pc}\delta^{rb}(Y_d^\dagger Y_d Y_d^\dagger)^{ad} - g_Y^2\left(\frac{11}{36}\delta^{pa}\delta^{rb}Y_d^{*cd} + \frac{7}{8}\delta^{pc}\delta^{rb}Y_d^{*ad}\right) - \left(3\delta^{pa}\delta^{rb}Y_d^{*cd}\right. \\
& + \frac{9}{2}\delta^{pc}\delta^{rb}Y_d^{*ad}\Big)\text{Tr}\left[Y_u^\dagger Y_u\right] - \frac{9}{4}\delta^{pc}\delta^{rb}(Y_u^\dagger Y_u Y_d^\dagger)^{ad} - \frac{5}{2}\delta^{pa}\delta^{rb}(Y_u^\dagger Y_u Y_d^\dagger)^{cd} - 3\delta^{pa}Y_d^{*cd}(Y_u^\dagger Y_u)^{br} - \frac{7}{2}\delta^{rb}Y_d^{*cd}(Y_u Y_u^\dagger)^{pa} - \frac{9}{2}\delta^{pc}Y_d^{*ad}(Y_u^\dagger Y_u)^{br} \\
& - \frac{21}{4}\delta^{rb}Y_d^{*ad}(Y_u Y_u^\dagger)^{pc}\Big) + \left(6\delta^{pa}\delta^{rb}Y_d^{*cd} + 9\delta^{pc}\delta^{rb}Y_d^{*ad}\right)\text{Tr}\left[Y_u^\dagger Y_u Y_u^\dagger Y_u\right] + \frac{3}{2}\delta^{pc}Y_u^{*ab}(Y_d^\dagger Y_d Y_d^\dagger Y_u)^{dr} + 2\delta^{pc}(Y_d^\dagger Y_u)^{dr}(Y_d^\dagger Y_d Y_u^\dagger)^{ab} \\
& + 2\delta^{rb}Y_d^{*cd}(Y_d Y_d^\dagger Y_d Y_d^\dagger)^{pa} + \frac{9}{4}\delta^{pa}Y_u^{*cb}(Y_d^\dagger Y_d Y_d^\dagger Y_u)^{dr} + 3\delta^{pa}(Y_d^\dagger Y_u)^{dr}(Y_d^\dagger Y_d Y_u^\dagger)^{cb} + 3\delta^{rb}Y_d^{*ad}(Y_d Y_d^\dagger Y_d Y_d^\dagger)^{pc} + 4\delta^{pa}(Y_u^\dagger Y_u)^{br}(Y_d^\dagger Y_d Y_d^\dagger)^{cd} \\
& + 4\delta^{rb}(Y_u Y_u^\dagger)^{pa}(Y_d^\dagger Y_d Y_d^\dagger)^{cd} + 4\delta^{rb}(Y_d Y_d^\dagger)^{pa}(Y_u^\dagger Y_u Y_d^\dagger)^{cd} + 6\delta^{pc}(Y_u^\dagger Y_u)^{br}(Y_d^\dagger Y_d Y_d^\dagger)^{ad} + 6\delta^{rb}(Y_u Y_u^\dagger)^{pc}(Y_d^\dagger Y_d Y_d^\dagger)^{ad} + 6\delta^{rb}(Y_d Y_d^\dagger)^{pc}(Y_u^\dagger Y_u Y_d^\dagger)^{ad}
\end{aligned}$$

$$\begin{aligned}
& + 20\delta^{pa}\delta^{rb}(Y_d^\dagger Y_d Y_d^\dagger Y_d Y_d^\dagger)^{dc} + 30\delta^{pc}\delta^{rb}(Y_d^\dagger Y_d Y_d^\dagger Y_d Y_d^\dagger)^{da} - \frac{1}{3}Y_u^{*ab}(Y_d^\dagger Y_u)^{dr}(Y_u Y_u^\dagger)^{pc} - \frac{1}{2}Y_d^{*cd}(Y_u^\dagger Y_u)^{br}(Y_d Y_d^\dagger)^{pa} - \frac{1}{2}Y_u^{*cb}(Y_d^\dagger Y_u)^{dr}(Y_u Y_u^\dagger)^{pa} \\
& - \frac{1}{2}\delta^{pc}Y_u^{*ab}(Y_d^\dagger Y_u Y_u^\dagger Y_u)^{dr} - \frac{1}{2}\delta^{pa}Y_d^{*cd}(Y_u^\dagger Y_u Y_u^\dagger Y_u)^{br} - \frac{1}{2}\delta^{rb}Y_d^{*cd}(Y_u Y_u^\dagger Y_u Y_u^\dagger)^{pa} - \frac{3}{4}Y_d^{*ad}(Y_u^\dagger Y_u)^{br}(Y_d Y_d^\dagger)^{pc} - \frac{3}{4}\delta^{pa}Y_u^{*cb}(Y_d^\dagger Y_u Y_u^\dagger Y_u)^{dr} \\
& - \frac{3}{4}\delta^{pc}Y_d^{*ad}(Y_u^\dagger Y_u Y_u^\dagger Y_u)^{br} - \frac{3}{4}\delta^{rb}Y_d^{*ad}(Y_u Y_u^\dagger Y_u Y_u^\dagger)^{pc} - g_s^2\left(\frac{64}{3}\delta^{pa}\delta^{rb}(Y_d^\dagger Y_d Y_d^\dagger)^{cd} + 88\delta^{pc}\delta^{rb}(Y_d^\dagger Y_d Y_d^\dagger)^{ad}\right) - \delta^{rb}Y_d^{*cd}(Y_u Y_u^\dagger Y_d Y_d^\dagger)^{pa} \\
& - \frac{3}{2}\delta^{rb}Y_d^{*ad}(Y_u Y_u^\dagger Y_d Y_d^\dagger)^{pc} - 2\delta^{rb}(Y_u Y_u^\dagger)^{pa}(Y_u^\dagger Y_u Y_d^\dagger)^{cd} - 2\delta^{pa}\delta^{rb}(Y_d^\dagger Y_d Y_d^\dagger Y_u Y_u^\dagger)^{dc} - 2\delta^{pa}\delta^{rb}(Y_d^\dagger Y_u Y_u^\dagger Y_d Y_d^\dagger)^{dc} - 2\delta^{pa}\delta^{rb}(Y_d^\dagger Y_u Y_u^\dagger Y_u Y_u^\dagger)^{dc} \\
& - 3\delta^{rb}(Y_u Y_u^\dagger)^{pc}(Y_u^\dagger Y_u Y_d^\dagger)^{ad} - 3\delta^{pc}\delta^{rb}(Y_d^\dagger Y_d Y_d^\dagger Y_u Y_u^\dagger)^{da} - 3\delta^{pc}\delta^{rb}(Y_d^\dagger Y_u Y_u^\dagger Y_d Y_d^\dagger)^{da} - 6\delta^{pc}\delta^{rb}(Y_d^\dagger Y_u Y_u^\dagger Y_u Y_u^\dagger)^{da} \Big\} C_{quqd}^{(\times)abcd} \\
& + \left(C_{quqd}^{(\times)*}\right)^{abcd} \Big\{ \frac{1}{6}Y_u^{ab}Y_u^{cr}(Y_u Y_u^\dagger Y_d)^{pd} + \frac{1}{4}Y_u^{ar}Y_u^{cb}(Y_u Y_u^\dagger Y_d)^{pd} + g_Y^2\left(\frac{1}{2}Y_d^{cd}Y_u^{pb}Y_u^{ar} + \frac{19}{12}Y_d^{ad}Y_u^{pb}Y_u^{cr}\right) + g_L^2\left(\frac{3}{4}Y_d^{cd}Y_u^{pb}Y_u^{ar} + \frac{3}{4}Y_d^{pd}Y_u^{ab}Y_u^{cr} + \frac{9}{4}Y_d^{ad}Y_u^{pb}Y_u^{cr} \right. \\
& + \frac{9}{2}Y_d^{pd}Y_u^{ar}Y_u^{cb}) + \lambda\left(\frac{3}{2}Y_d^{pd}Y_u^{ar}Y_u^{cb} - 3Y_d^{cd}Y_u^{pr}Y_u^{ab} - \frac{9}{2}Y_d^{ad}Y_u^{pr}Y_u^{cb} - 5Y_d^{cd}Y_u^{pb}Y_u^{ar} - \frac{15}{2}Y_d^{ad}Y_u^{pb}Y_u^{cr}\right) + 5Y_u^{pb}Y_u^{ar}(Y_d Y_d^\dagger Y_d)^{cd} + 6Y_d^{cd}Y_u^{pr}(Y_u Y_u^\dagger Y_u)^{ab} \\
& + \frac{15}{2}Y_u^{pb}Y_u^{cr}(Y_d Y_d^\dagger Y_d)^{ad} + 9Y_d^{ad}Y_u^{pr}(Y_u Y_u^\dagger Y_u)^{cb} - \frac{1}{6}Y_d^{cd}Y_u^{pb}(Y_u Y_u^\dagger Y_u)^{ar} - \frac{1}{4}Y_d^{ad}Y_u^{pb}(Y_u Y_u^\dagger Y_u)^{cr} - \frac{1}{3}Y_d^{cd}Y_u^{ar}(Y_u Y_u^\dagger Y_u)^{pb} - \frac{1}{2}Y_u^{ab}Y_u^{cr}(Y_d Y_d^\dagger Y_d)^{pd} \\
& \left. - \frac{1}{2}Y_d^{cd}Y_u^{pb}(Y_d Y_d^\dagger Y_u)^{ar} - \frac{1}{2}Y_d^{ad}Y_u^{cr}(Y_u Y_u^\dagger Y_u)^{pb} - \frac{3}{4}Y_u^{ar}Y_u^{cb}(Y_d Y_d^\dagger Y_d)^{pd} - \frac{3}{4}Y_d^{ad}Y_u^{pb}(Y_d Y_d^\dagger Y_u)^{cr} - Y_d^{pd}Y_u^{cr}(Y_u Y_u^\dagger Y_u)^{ab} - \frac{9}{2}Y_d^{pd}Y_u^{ar}(Y_u Y_u^\dagger Y_u)^{cb} \right\} \\
& + \left\{ \frac{1}{2}Y_e^{*ab}(Y_u^\dagger Y_u)^{dr}(Y_d Y_d^\dagger)^{pc} + \frac{1}{2}\delta^{pc}Y_e^{*ab}(Y_u^\dagger Y_u Y_u^\dagger Y_u)^{dr} + \frac{1}{2}\delta^{rd}Y_e^{*ab}(Y_u Y_u^\dagger Y_u Y_u^\dagger)^{pc} + \frac{3}{4}\delta^{pc}\delta^{rd}g_L^4 Y_e^{*ab} + g_L^2\left(\frac{9}{8}\delta^{pc}Y_e^{*ab}(Y_u^\dagger Y_u)^{dr} \right. \right. \\
& - \frac{3}{8}\delta^{rd}Y_e^{*ab}(Y_u Y_u^\dagger)^{pc}) + g_Y^2\left(\frac{7}{8}\delta^{rd}Y_e^{*ab}(Y_u Y_u^\dagger)^{pc} + 8\delta^{pc}\delta^{rd}(Y_e^\dagger Y_e Y_e^\dagger)^{ab} - \frac{3}{8}\delta^{pc}Y_e^{*ab}(Y_u^\dagger Y_u)^{dr}\right) + \delta^{rd}Y_e^{*ab}(Y_u Y_u^\dagger Y_d Y_d^\dagger)^{pc} + \lambda\left(\frac{1}{2}\delta^{pc}\delta^{rd}(Y_e^\dagger Y_e Y_e^\dagger)^{ab} \right. \\
& + 3\delta^{pc}Y_e^{*ab}(Y_u^\dagger Y_u)^{dr} + 3\delta^{pc}\delta^{rd}Y_e^{*ab}\text{Tr}[Y_u^\dagger Y_u] + \frac{7}{2}\delta^{rd}Y_e^{*ab}(Y_u Y_u^\dagger)^{pc} - \frac{3}{4}\delta^{pc}\delta^{rd}g_L^2 Y_e^{*ab} - \frac{3}{2}\delta^{rd}Y_e^{*ab}(Y_d Y_d^\dagger)^{pc} - \frac{21}{4}\delta^{pc}\delta^{rd}g_Y^2 Y_e^{*ab}) \\
& + \frac{25}{4}\delta^{pc}\delta^{rd}g_Y^4 Y_e^{*ab} - \frac{1}{2}Y_e^{*ab}(Y_u^\dagger Y_u)^{dr}(Y_u Y_u^\dagger)^{pc} - 2\delta^{rd}Y_e^{*ab}(Y_d Y_d^\dagger Y_d Y_d^\dagger)^{pc} - 4\delta^{pc}(Y_u^\dagger Y_u)^{dr}(Y_e^\dagger Y_e Y_e^\dagger)^{ab} - 4\delta^{rd}(Y_u Y_u^\dagger)^{pc}(Y_e^\dagger Y_e Y_e^\dagger)^{ab} \\
& \left. - \frac{11}{2}\delta^{pc}\delta^{rd}g_Y^2 g_L^2 Y_e^{*ab} - 6\delta^{pc}\delta^{rd}Y_e^{*ab}\text{Tr}[Y_u^\dagger Y_u Y_u^\dagger Y_u] - 20\delta^{pc}\delta^{rd}(Y_e^\dagger Y_e Y_e^\dagger Y_e Y_e^\dagger)^{ba} \right\} C_{lequ}^{abcd} + C_{lequ}^{*abcd} \Big\{ \frac{1}{6}Y_e^{ab}Y_u^{pd}(Y_u Y_u^\dagger Y_u)^{cr} \\
& + \frac{1}{3}Y_e^{ab}Y_u^{cr}(Y_u Y_u^\dagger Y_u)^{pd} + \frac{1}{2}Y_e^{ab}Y_u^{pd}(Y_d Y_d^\dagger Y_u)^{cr} + \lambda\left(3Y_e^{ab}Y_u^{pr}Y_u^{cd} + 5Y_e^{ab}Y_u^{pd}Y_u^{cr}\right) - \frac{1}{2}g_Y^2 Y_e^{ab}Y_u^{pd}Y_u^{cr} - \frac{3}{4}g_L^2 Y_e^{ab}Y_u^{pd}Y_u^{cr} - 5Y_u^{pd}Y_u^{cr}(Y_e Y_e^\dagger Y_e)^{ab} \\
& - 6Y_e^{ab}Y_u^{pr}(Y_u Y_u^\dagger Y_u)^{cd} \Big\} + \left\{ \frac{1}{4}Y_e^{*ad}(Y_u^\dagger Y_u)^{br}(Y_u Y_u^\dagger)^{pc} + g_Y^2\left(\frac{45}{16}\delta^{pc}Y_e^{*ad}(Y_u^\dagger Y_u)^{br} - \frac{19}{36}\delta^{pc}\delta^{rb}(Y_e^\dagger Y_e Y_e^\dagger)^{ad} - \frac{19}{16}\delta^{rb}Y_e^{*ad}(Y_u Y_u^\dagger)^{pc} \right) \right. \\
& \left. + g_L^2\left(\frac{5}{2}\delta^{rb}Y_e^{*ad}(Y_d Y_d^\dagger)^{pc} + \frac{15}{4}\delta^{pc}\delta^{rb}(Y_e^\dagger Y_e Y_e^\dagger)^{ad} - \frac{1}{16}\delta^{rb}Y_e^{*ad}(Y_u Y_u^\dagger)^{pc} - \frac{23}{16}\delta^{pc}Y_e^{*ad}(Y_u^\dagger Y_u)^{br}\right) + \delta^{rb}Y_e^{*ad}(Y_d Y_d^\dagger Y_d Y_d^\dagger)^{pc} + \lambda\left(\frac{3}{4}\delta^{rb}Y_e^{*ad}(Y_d Y_d^\dagger)^{pc} \right. \right.
\end{aligned}$$

$$\begin{aligned}
& + \frac{14}{3} \delta^{pc} \delta^{rb} g_s^2 Y_e^{*ad} + \frac{379}{72} \delta^{pc} \delta^{rb} g_Y^2 Y_e^{*ad} - \frac{1}{4} \delta^{pc} \delta^{rb} (Y_e^\dagger Y_e Y_e^\dagger)^{ad} - \frac{3}{8} \delta^{pc} \delta^{rb} g_L^2 Y_e^{*ad} - \frac{3}{2} \delta^{pc} Y_e^{*ad} (Y_u^\dagger Y_u)^{br} - \frac{3}{2} \delta^{pc} \delta^{rb} Y_e^{*ad} \text{Tr}[Y_u^\dagger Y_u] \\
& - \frac{7}{4} \delta^{rb} Y_e^{*ad} (Y_u Y_u^\dagger)^{pc} + \frac{3}{2} \delta^{pc} \delta^{rb} g_L^4 Y_e^{*ad} + 2 \delta^{pc} (Y_u^\dagger Y_u)^{br} (Y_e^\dagger Y_e Y_e^\dagger)^{ad} + 2 \delta^{rb} (Y_u Y_u^\dagger)^{pc} (Y_e^\dagger Y_e Y_e^\dagger)^{ad} + 3 \delta^{pc} \delta^{rb} Y_e^{*ad} \text{Tr}[Y_u^\dagger Y_u Y_u^\dagger Y_u] \\
& + 10 \delta^{pc} \delta^{rb} (Y_e^\dagger Y_e Y_e^\dagger Y_e Y_e^\dagger)^{da} - \frac{1}{6} \delta^{pc} \delta^{rb} g_Y^2 g_L^2 Y_e^{*ad} - \frac{1}{4} Y_e^{*ad} (Y_u^\dagger Y_u)^{br} (Y_d Y_d^\dagger)^{pc} - \frac{1}{4} \delta^{pc} Y_e^{*ad} (Y_u^\dagger Y_u Y_u^\dagger Y_u)^{br} - \frac{1}{4} \delta^{rb} Y_e^{*ad} (Y_u Y_u^\dagger Y_u Y_u^\dagger)^{pc} \\
& - \frac{1}{2} \delta^{rb} Y_e^{*ad} (Y_u Y_u^\dagger Y_d Y_d^\dagger)^{pc} - \frac{28}{3} \delta^{pc} \delta^{rb} g_s^2 (Y_e^\dagger Y_e Y_e^\dagger)^{ad} \Big\} C_{\ell u q e}^{abcd} + C_{\ell u q e}^{*abcd} \Big\{ \frac{3}{4} g_L^2 Y_e^{ad} Y_u^{pb} Y_u^{cr} + \frac{5}{2} Y_u^{pb} Y_u^{cr} (Y_e Y_e^\dagger Y_e)^{ad} + \frac{11}{4} g_Y^2 Y_e^{ad} Y_u^{pb} Y_u^{cr} \\
& + 3 Y_e^{ad} Y_u^{pr} (Y_u Y_u^\dagger Y_u)^{cb} - \frac{1}{12} Y_e^{ad} Y_u^{pb} (Y_u Y_u^\dagger Y_u)^{cr} - \frac{1}{6} Y_e^{ad} Y_u^{cr} (Y_u Y_u^\dagger Y_u)^{pb} - \frac{1}{4} Y_e^{ad} Y_u^{pb} (Y_d Y_d^\dagger Y_u)^{cr} - \lambda \Big( \frac{3}{2} Y_e^{ad} Y_u^{pr} Y_u^{cb} + \frac{5}{2} Y_e^{ad} Y_u^{pb} Y_u^{cr} \Big) \Big\} \\
& + \Big\{ \frac{4}{3} \delta^{bc} g_L^2 Y_u^{pr} (Y_e Y_e^\dagger)^{da} - \frac{2}{9} \delta^{ad} \delta^{bc} g_L^4 Y_u^{pr} - \frac{2}{9} \delta^{ad} \delta^{bc} g_Y^4 Y_u^{pr} - \frac{4}{3} \delta^{bc} g_Y^2 Y_u^{pr} (Y_e Y_e^\dagger)^{da} - 4 Y_u^{pr} (Y_e Y_e^\dagger)^{bc} (Y_e Y_e^\dagger)^{da} \Big\} C_{\ell \ell}^{abcd} + \Big\{ g_L^4 \Big( \frac{3}{2} \delta^{pa} \delta^{bc} Y_u^{dr} \\
& - \frac{2}{3} \delta^{ad} \delta^{bc} Y_u^{pr} \Big) + g_Y^2 g_L^2 \Big( \frac{1}{9} \delta^{pa} \delta^{bc} Y_u^{dr} - \delta^{pa} \delta^{cd} Y_u^{br} \Big) + \lambda \Big( g_Y^2 \Big( \frac{11}{81} \delta^{pa} \delta^{bc} Y_u^{dr} + \frac{154}{27} \delta^{pa} \delta^{cd} Y_u^{br} \Big) + \frac{32}{27} \delta^{pa} \delta^{bc} g_s^2 Y_u^{dr} + 24 \delta^{pa} Y_u^{br} (Y_u Y_u^\dagger)^{dc} \\
& - \frac{1}{3} \delta^{pa} \delta^{bc} g_L^2 Y_u^{dr} - 3 \delta^{pa} Y_u^{dr} (Y_d Y_d^\dagger)^{bc} - 12 \delta^{pa} Y_u^{br} (Y_d Y_d^\dagger)^{dc} \Big) + \delta^{pa} (Y_d Y_d^\dagger)^{bc} (Y_u Y_u^\dagger Y_u)^{dr} + g_Y^2 \Big( \frac{65}{162} \delta^{bc} Y_u^{dr} (Y_u Y_u^\dagger)^{pa} + \frac{4}{3} \delta^{bc} Y_u^{pr} (Y_d Y_d^\dagger)^{da} \\
& + \frac{65}{27} \delta^{cd} Y_u^{br} (Y_u Y_u^\dagger)^{pa} + 21 \delta^{pa} Y_u^{br} (Y_d Y_d^\dagger)^{dc} - \frac{23}{162} \delta^{pa} \delta^{bc} (Y_u Y_u^\dagger Y_u)^{dr} - \frac{4}{3} \delta^{bc} Y_u^{pr} (Y_u Y_u^\dagger)^{da} - \frac{179}{27} \delta^{pa} \delta^{cd} (Y_u Y_u^\dagger Y_u)^{br} - \frac{29}{3} \delta^{pa} Y_u^{dr} (Y_u Y_u^\dagger)^{bc} \\
& - 53 \delta^{pa} Y_u^{br} (Y_u Y_u^\dagger)^{dc} \Big) + g_L^2 \Big( \frac{5}{6} \delta^{pa} \delta^{bc} (Y_u Y_u^\dagger Y_u)^{dr} + \delta^{bc} Y_u^{dr} (Y_d Y_d^\dagger)^{pa} + \frac{4}{3} \delta^{pa} \delta^{bc} (Y_d Y_d^\dagger Y_u)^{dr} + 4 \delta^{bc} Y_u^{pr} (Y_d Y_d^\dagger)^{da} + 4 \delta^{bc} Y_u^{pr} (Y_u Y_u^\dagger)^{da} + 9 \delta^{pa} Y_u^{br} (Y_d Y_d^\dagger)^{dc} \\
& - \frac{1}{6} \delta^{bc} Y_u^{dr} (Y_u Y_u^\dagger)^{pa} - 3 \delta^{pa} Y_u^{dr} (Y_d Y_d^\dagger)^{bc} - 6 \delta^{pa} Y_u^{dr} (Y_u Y_u^\dagger)^{bc} - 9 \delta^{pa} Y_u^{br} (Y_u Y_u^\dagger)^{dc} \Big) + g_s^2 \Big( \frac{32}{27} \delta^{pa} \delta^{bc} (Y_u Y_u^\dagger Y_u)^{dr} + \frac{160}{27} \delta^{bc} Y_u^{dr} (Y_u Y_u^\dagger)^{pa} \\
& - 64 \delta^{pa} Y_u^{dr} (Y_u Y_u^\dagger)^{bc} \Big) + 3 Y_u^{dr} (Y_d Y_d^\dagger)^{pa} (Y_d Y_d^\dagger)^{bc} + 3 Y_u^{dr} (Y_d Y_d^\dagger)^{pa} (Y_u Y_u^\dagger)^{bc} + 3 Y_u^{br} (Y_u Y_u^\dagger)^{pa} (Y_u Y_u^\dagger)^{dc} + 3 \delta^{pa} (Y_u Y_u^\dagger)^{dc} (Y_u Y_u^\dagger Y_u)^{br} \\
& + 6 \delta^{pa} Y_u^{dr} (Y_d Y_d^\dagger Y_d Y_d^\dagger)^{bc} + 8 \delta^{pa} Y_u^{dr} (Y_u Y_u^\dagger Y_u Y_u^\dagger)^{bc} + 19 \delta^{pa} Y_u^{dr} (Y_u Y_u^\dagger Y_d Y_d^\dagger)^{bc} - g_Y^4 \Big( \frac{2}{27} \delta^{ad} \delta^{bc} Y_u^{pr} + \frac{5}{54} \delta^{pa} \delta^{bc} Y_u^{dr} + \frac{29}{9} \delta^{pa} \delta^{cd} Y_u^{br} \Big) \\
& - Y_u^{dr} (Y_u Y_u^\dagger)^{pa} (Y_u Y_u^\dagger)^{bc} - 2 Y_u^{br} (Y_d Y_d^\dagger)^{da} (Y_u Y_u^\dagger)^{pc} - 2 \delta^{pa} (Y_u Y_u^\dagger)^{bc} (Y_u Y_u^\dagger Y_u)^{dr} - 3 Y_u^{dr} (Y_d Y_d^\dagger)^{ba} (Y_u Y_u^\dagger)^{pc} - 3 \delta^{pa} (Y_d Y_d^\dagger)^{dc} (Y_u Y_u^\dagger Y_u)^{br} \\
& - 3 \delta^{pa} Y_u^{dr} (Y_d Y_d^\dagger Y_u Y_u^\dagger)^{bc} - 4 \delta^{pa} (Y_d Y_d^\dagger)^{bc} (Y_d Y_d^\dagger Y_u)^{dr} - 4 \delta^{pa} (Y_u Y_u^\dagger)^{bc} (Y_d Y_d^\dagger Y_u)^{dr} - 12 Y_u^{pr} (Y_d Y_d^\dagger)^{bc} (Y_d Y_d^\dagger)^{da} - 12 Y_u^{pr} (Y_u Y_u^\dagger)^{bc} (Y_u Y_u^\dagger)^{da} \\
& - 24 \delta^{pa} Y_u^{br} (Y_d Y_d^\dagger Y_d Y_d^\dagger)^{dc} \Big\} C_{qq}^{(II)abcd} + \Big\{ g_Y^2 g_L^2 \Big( \frac{13}{3} \delta^{pa} \delta^{cd} Y_u^{br} - \frac{1}{3} \delta^{pa} \delta^{bc} Y_u^{dr} \Big) + Y_u^{dr} (Y_u Y_u^\dagger)^{pa} (Y_u Y_u^\dagger)^{bc} + \lambda \Big( g_Y^2 \Big( \frac{22}{81} \delta^{pa} \delta^{bc} Y_u^{dr} + \frac{77}{27} \delta^{pa} \delta^{cd} Y_u^{br} \Big) \\
& + \frac{64}{27} \delta^{pa} \delta^{bc} g_s^2 Y_u^{dr} + 3 \delta^{pa} Y_u^{dr} (Y_d Y_d^\dagger)^{bc} + 12 \delta^{pa} Y_u^{br} (Y_d Y_d^\dagger)^{dc} + 48 \delta^{pa} Y_u^{br} (Y_u Y_u^\dagger)^{dc} - 7 \delta^{pa} \delta^{cd} g_L^2 Y_u^{br} \Big) + g_L^2 \Big( \frac{5}{2} \delta^{pa} \delta^{cd} (Y_u Y_u^\dagger Y_u)^{br} + 3 \delta^{cd} Y_u^{br} (Y_d Y_d^\dagger)^{pa} \\
& + 3 \delta^{pa} Y_u^{dr} (Y_d Y_d^\dagger)^{bc} - \frac{1}{2} \delta^{cd} Y_u^{br} (Y_u Y_u^\dagger)^{pa} - 2 \delta^{pa} \delta^{cd} (Y_d Y_d^\dagger Y_u)^{br} - 3 \delta^{pa} Y_u^{dr} (Y_u Y_u^\dagger)^{bc} - 9 \delta^{pa} Y_u^{br} (Y_d Y_d^\dagger)^{dc} - 18 \delta^{pa} Y_u^{br} (Y_u Y_u^\dagger)^{dc} \Big) + g_Y^2 \Big( \frac{65}{81} \delta^{bc} Y_u^{dr} (Y_u Y_u^\dagger)^{pa}
\end{aligned}$$



$$\begin{aligned}
& + \frac{65}{54} \delta^{cd} Y_u^{br} (Y_u Y_u^\dagger)^{pa} + \frac{8}{3} \delta^{bc} Y_u^{pr} (Y_d Y_d^\dagger)^{da} - \frac{23}{81} \delta^{pa} \delta^{bc} (Y_u Y_u^\dagger Y_u)^{dr} - \delta^{pa} Y_u^{dr} (Y_d Y_d^\dagger)^{bc} - \frac{8}{3} \delta^{bc} Y_u^{pr} (Y_u Y_u^\dagger)^{da} - \frac{179}{54} \delta^{pa} \delta^{cd} (Y_u Y_u^\dagger Y_u)^{br} \\
& - \frac{29}{3} \delta^{pa} Y_u^{dr} (Y_u Y_u^\dagger)^{bc} - 53 \delta^{pa} Y_u^{br} (Y_u Y_u^\dagger)^{dc} \Big) + g_s^2 \Big( \frac{64}{27} \delta^{pa} \delta^{bc} (Y_u Y_u^\dagger Y_u)^{dr} + \frac{320}{27} \delta^{bc} Y_u^{dr} (Y_u Y_u^\dagger)^{pa} - 64 \delta^{pa} Y_u^{dr} (Y_d Y_d^\dagger)^{bc} - 64 \delta^{pa} Y_u^{dr} (Y_u Y_u^\dagger)^{bc} \Big) \\
& + 3 \delta^{pa} (Y_d Y_d^\dagger)^{bc} (Y_u Y_u^\dagger Y_u)^{dr} + \frac{9}{2} \delta^{pa} \delta^{cd} g_L^4 Y_u^{br} + 6 \delta^{pa} (Y_d Y_d^\dagger)^{dc} (Y_d Y_d^\dagger Y_u)^{br} + 6 \delta^{pa} (Y_u Y_u^\dagger)^{dc} (Y_d Y_d^\dagger Y_u)^{br} + 8 \delta^{pa} Y_u^{dr} (Y_u Y_u^\dagger Y_u Y_u^\dagger)^{bc} \\
& + 9 Y_u^{br} (Y_d Y_d^\dagger)^{pa} (Y_d Y_d^\dagger)^{dc} + 9 Y_u^{br} (Y_d Y_d^\dagger)^{pa} (Y_u Y_u^\dagger)^{dc} + 24 Y_u^{pr} (Y_d Y_d^\dagger)^{da} (Y_u Y_u^\dagger)^{bc} + 57 \delta^{pa} Y_u^{br} (Y_u Y_u^\dagger Y_d Y_d^\dagger)^{dc} - g_Y^4 \Big( \frac{4}{27} \delta^{ad} \delta^{bc} Y_u^{pr} + \frac{5}{27} \delta^{pa} \delta^{bc} Y_u^{dr} \\
& + \frac{29}{18} \delta^{pa} \delta^{cd} Y_u^{br} \Big) - Y_u^{br} (Y_d Y_d^\dagger)^{da} (Y_u Y_u^\dagger)^{pc} - 3 Y_u^{br} (Y_u Y_u^\dagger)^{pa} (Y_u Y_u^\dagger)^{dc} - 3 \delta^{pa} (Y_d Y_d^\dagger)^{dc} (Y_u Y_u^\dagger Y_u)^{br} - 3 \delta^{pa} (Y_u Y_u^\dagger)^{bc} (Y_u Y_u^\dagger Y_u)^{dr} - 6 Y_u^{dr} (Y_d Y_d^\dagger)^{ba} (Y_u Y_u^\dagger)^{pc} \\
& - 9 \delta^{pa} Y_u^{br} (Y_d Y_d^\dagger Y_u Y_u^\dagger)^{dc} - 12 Y_u^{pr} (Y_d Y_d^\dagger)^{bc} (Y_d Y_d^\dagger)^{da} - 12 Y_u^{pr} (Y_u Y_u^\dagger)^{bc} (Y_u Y_u^\dagger)^{da} - 14 \delta^{pa} Y_u^{dr} (Y_d Y_d^\dagger Y_d Y_d^\dagger)^{bc} - 24 \delta^{pa} Y_u^{br} (Y_u Y_u^\dagger Y_u Y_u^\dagger)^{dc} \Big\} C_{qq}^{(\times)abcd} \\
& + \left\{ \frac{1}{2} \delta^{pc} \delta^{ab} g_Y^2 g_L^2 Y_u^{dr} + g_Y^2 \Big( \frac{179}{54} \delta^{pc} \delta^{ab} (Y_u Y_u^\dagger Y_u)^{dr} + \frac{85}{6} \delta^{pc} Y_u^{dr} (Y_e Y_e^\dagger)^{ba} - \frac{65}{54} \delta^{ab} Y_u^{dr} (Y_u Y_u^\dagger)^{pc} \Big) + \frac{3}{2} \delta^{pc} g_L^2 Y_u^{dr} (Y_e Y_e^\dagger)^{ba} + \frac{29}{18} \delta^{pc} \delta^{ab} g_Y^4 Y_u^{dr} \right. \\
& - \frac{1}{2} Y_u^{dr} (Y_e Y_e^\dagger)^{ba} (Y_u Y_u^\dagger)^{pc} - \frac{1}{2} \delta^{pc} (Y_e Y_e^\dagger)^{ba} (Y_u Y_u^\dagger Y_u)^{dr} - \lambda \Big( 2 \delta^{pc} Y_u^{dr} (Y_e Y_e^\dagger)^{ba} + \frac{77}{27} \delta^{pc} \delta^{ab} g_Y^2 Y_u^{dr} \Big) - 4 \delta^{pc} Y_u^{dr} (Y_e Y_e^\dagger Y_e Y_e^\dagger)^{ba} \Big\} C_{\ell q}^{(\parallel)abcd} \\
& + \left\{ \frac{3}{4} \delta^{pc} \delta^{ab} g_L^4 Y_u^{dr} + \frac{29}{36} \delta^{pc} \delta^{ab} g_Y^4 Y_u^{dr} + \lambda \Big( 2 \delta^{pc} Y_u^{dr} (Y_e Y_e^\dagger)^{ba} - \frac{7}{6} \delta^{pc} \delta^{ab} g_L^2 Y_u^{dr} - \frac{77}{54} \delta^{pc} \delta^{ab} g_Y^2 Y_u^{dr} \Big) + \delta^{pc} (Y_e Y_e^\dagger)^{ba} (Y_d Y_d^\dagger Y_u)^{dr} \right. \\
& + g_L^2 \Big( \frac{5}{12} \delta^{pc} \delta^{ab} (Y_u Y_u^\dagger Y_u)^{dr} + \frac{1}{2} \delta^{ab} Y_u^{dr} (Y_d Y_d^\dagger)^{pc} - \frac{1}{12} \delta^{ab} Y_u^{dr} (Y_u Y_u^\dagger)^{pc} - \frac{1}{3} \delta^{pc} \delta^{ab} (Y_d Y_d^\dagger Y_u)^{dr} - \frac{3}{2} \delta^{pc} Y_u^{dr} (Y_e Y_e^\dagger)^{ba} \Big) + g_Y^2 \Big( \frac{179}{108} \delta^{pc} \delta^{ab} (Y_u Y_u^\dagger Y_u)^{dr} \\
& - \frac{65}{108} \delta^{ab} Y_u^{dr} (Y_u Y_u^\dagger)^{pc} \Big) + \frac{19}{18} \delta^{pc} \delta^{ab} g_Y^2 g_L^2 Y_u^{dr} + \frac{3}{2} Y_u^{dr} (Y_d Y_d^\dagger)^{pc} (Y_e Y_e^\dagger)^{ba} - \frac{1}{2} \delta^{pc} (Y_e Y_e^\dagger)^{ba} (Y_u Y_u^\dagger Y_u)^{dr} - Y_u^{dr} (Y_e Y_e^\dagger)^{ba} (Y_u Y_u^\dagger)^{pc} \Big\} C_{\ell q}^{(\times)abcd}, \tag{7.4}
\end{aligned}$$

### 7.3 $C_{dH}$

$$\begin{aligned}
\beta_{C_{dH}^{pr}}^{(1)} &= \left\{ \frac{17}{12} g_L^2 Y_d^{pr} + \frac{3}{2} \Big( (Y_d Y_d^\dagger Y_d)^{pr} - (Y_u Y_u^\dagger Y_d)^{pr} \Big) - \frac{1}{12} g_Y^2 Y_d^{pr} - \lambda Y_d^{pr} \right\} C_{HD}^{(\parallel)} + \left\{ \lambda Y_d^{pr} + (Y_d Y_d^\dagger Y_d)^{pr} - \frac{1}{6} g_Y^2 Y_d^{pr} - \frac{3}{2} g_L^2 Y_d^{pr} \right\} C_{HD}^{(\times)} + \frac{5}{3} g_Y^4 C_{HB} Y_d^{pr} \\
& - \frac{5i}{3} g_Y^4 C_{H\tilde{B}} Y_d^{pr} + 9 g_L^4 C_{HW} Y_d^{pr} - 9i g_L^4 C_{H\tilde{W}} Y_d^{pr} + 32 g_s^4 C_{HG} Y_d^{pr} - 32i g_s^4 C_{H\tilde{G}} Y_d^{pr} + \frac{1}{2} g_Y^2 g_L^2 C_{HWB} Y_d^{pr} - \frac{i}{2} g_Y^2 g_L^2 C_{H\tilde{W}B} Y_d^{pr} + 2 Y_e^{*ab} C_{eH}^{ab} Y_d^{pr} \\
& - \delta^{pa} C_{uH}^{ab} (Y_u^\dagger Y_d)^{br} - 2 C_{uH}^{*ab} \left\{ Y_d^{ar} Y_u^{pb} - 3 Y_d^{pr} Y_u^{ab} \right\} + \left\{ \frac{1}{2} \Big( 6 T_2 \delta^{pa} \delta^{rb} + 10 \delta^{pa} (Y_d^\dagger Y_d)^{br} + 11 \delta^{rb} (Y_d Y_d^\dagger)^{pa} + 12 Y_d^{*ab} Y_d^{pr} - 3 \delta^{rb} (Y_u Y_u^\dagger)^{pa} \Big) \right. \\
& + 12 \delta^{pa} \delta^{rb} \lambda - \frac{23}{12} \delta^{pa} \delta^{rb} g_Y^2 - \frac{27}{4} \delta^{pa} \delta^{rb} g_L^2 - 8 \delta^{pa} \delta^{rb} g_s^2 \Big\} C_{dH}^{ab} + 3 \delta^{pa} g_L^2 C_{uW}^{ab} (Y_u^\dagger Y_d)^{br} + \left\{ 3 \delta^{pa} \delta^{rb} g_Y^2 g_L^2 - \delta^{pa} \delta^{rb} g_Y^4 - g_Y^2 \Big( \delta^{pa} (Y_d^\dagger Y_d)^{br} \right. \right.
\end{aligned}$$

$$\begin{aligned}
& + \delta^{rb} (Y_d Y_d^\dagger)^{pa} \Big\} C_{dB}^{ab} + \left\{ \frac{3}{2} g_L^2 \left( \delta^{pa} (Y_d^\dagger Y_d)^{br} + 4 \delta^{rb} (Y_u Y_u^\dagger)^{pa} - \delta^{rb} (Y_d Y_d^\dagger)^{pa} \right) + \frac{9}{2} \delta^{pa} \delta^{rb} g_L^4 - \frac{1}{2} \delta^{pa} \delta^{rb} g_Y^2 g_L^2 \right\} C_{dW}^{ab} + 16 g_s^2 \left\{ \delta^{pa} (Y_d^\dagger Y_d)^{br} \right. \\
& + \delta^{rb} (Y_d Y_d^\dagger)^{pa} \Big\} C_{dG}^{ab} + \left\{ \frac{2}{3} \delta^{ab} g_Y^2 Y_d^{pr} + 2 Y_d^{pr} (Y_e Y_e^\dagger)^{ba} \right\} C_{H\ell}^{(\parallel)ab} + \left\{ \frac{1}{3} \delta^{ab} g_Y^2 Y_d^{pr} + 2 Y_d^{pr} (Y_e Y_e^\dagger)^{ba} - \frac{1}{3} \delta^{ab} g_L^2 Y_d^{pr} \right\} C_{H\ell}^{(\times)ab} + \left\{ \frac{2}{3} \delta^{ab} g_Y^2 Y_d^{pr} \right. \\
& - 2 Y_d^{pr} (Y_e^\dagger Y_e)^{ba} \Big\} C_{He}^{ab} + \left\{ 2 \delta^{pa} \lambda Y_d^{br} + 2 \left( \delta^{pa} (Y_d Y_d^\dagger Y_d)^{br} + 3 Y_d^{pr} (Y_d Y_d^\dagger)^{ba} - 3 Y_d^{pr} (Y_u Y_u^\dagger)^{ba} \right) - \frac{2}{3} g_Y^2 \left( \delta^{ab} Y_d^{pr} + 3 \delta^{pa} Y_d^{br} \right) \right\} C_{Hq}^{(\parallel)ab} + \left\{ \delta^{pa} (Y_d Y_d^\dagger Y_d)^{br} \right. \\
& + 3 \delta^{pa} (Y_u Y_u^\dagger Y_d)^{br} + 4 \delta^{pa} \lambda Y_d^{br} + 6 Y_d^{pr} (Y_d Y_d^\dagger)^{ba} - \frac{1}{3} g_Y^2 \left( \delta^{ab} Y_d^{pr} + 6 \delta^{pa} Y_d^{br} \right) - \delta^{ab} g_L^2 Y_d^{pr} \Big\} C_{Hq}^{(\times)ab} + \left\{ 6 Y_d^{pr} (Y_u^\dagger Y_u)^{ba} - \frac{4}{3} \delta^{ab} g_Y^2 Y_d^{pr} \right\} C_{Hu}^{ab} \\
& + \left\{ \frac{1}{3} g_Y^2 \left( 2 \delta^{ab} Y_d^{pr} + 3 \delta^{rb} Y_d^{pa} \right) + 3 \delta^{rb} g_L^2 Y_d^{pa} - 2 \delta^{rb} \lambda Y_d^{pa} - 2 \left( \delta^{rb} (Y_d Y_d^\dagger Y_d)^{pa} + 3 Y_d^{pr} (Y_d^\dagger Y_d)^{ba} \right) \right\} C_{Hd}^{ab} + \left\{ 3 \delta^{rb} g_L^2 Y_u^{pa} - 2 \delta^{rb} \lambda Y_u^{pa} \right. \\
& - 2 \delta^{rb} (Y_u Y_u^\dagger Y_u)^{pa} \Big\} C_{Hud}^{ab} + \left\{ 8 \delta^{pa} \delta^{rd} (Y_d Y_d^\dagger Y_d)^{bc} - 4 \delta^{pa} \delta^{rd} \lambda Y_d^{bc} \right\} C_{qd}^{(\parallel)abcd} + \left\{ 24 \delta^{pa} \delta^{rd} (Y_d Y_d^\dagger Y_d)^{bc} - 12 \delta^{pa} \delta^{rd} \lambda Y_d^{bc} \right\} C_{qd}^{(\times)abcd} \\
& + C_{ledq}^{*abcd} \left\{ 2 \delta^{pd} \delta^{rc} \lambda Y_e^{ab} - 4 \delta^{pd} \delta^{rc} (Y_e Y_e^\dagger Y_e)^{ab} \right\} + \left\{ \lambda \left( \delta^{pa} \delta^{rd} Y_u^{*cb} + 6 \delta^{pc} \delta^{rd} Y_u^{*ab} \right) - 2 \left( \delta^{pa} \delta^{rd} (Y_u^\dagger Y_u Y_u^\dagger)^{cb} + 6 \delta^{pc} \delta^{rd} (Y_u^\dagger Y_u Y_u^\dagger)^{ab} \right) \right\} C_{quqd}^{(\parallel)abcd} \\
& + \left\{ \lambda \left( 2 \delta^{pc} \delta^{rd} Y_u^{*ab} + 3 \delta^{pa} \delta^{rd} Y_u^{*cb} \right) - 2 \left( 2 \delta^{pc} \delta^{rd} (Y_u^\dagger Y_u Y_u^\dagger)^{ab} + 3 \delta^{pa} \delta^{rd} (Y_u^\dagger Y_u Y_u^\dagger)^{cb} \right) \right\} C_{quqd}^{(\times)abcd}, \tag{7.5}
\end{aligned}$$

$$\begin{aligned}
\beta_{C_{dH}^{pr}}^{(2)} &= \frac{11}{6} g_L^2 Y_d^{pr} \mathbf{T}_{\ell H} + \frac{19}{6} g_Y^2 Y_d^{pr} \mathbf{T}_{\ell H} + 5 \left( 3 (Y_d Y_d^\dagger Y_d)^{pr} \mathbf{T}_{\ell H} - (Y_u Y_u^\dagger Y_d)^{pr} \mathbf{T}_{\ell H} \right) - 6 Y_d^{pr} \text{Tr} \left[ C_{\ell HH}^\dagger C_{\ell HH} Y_e Y_e^\dagger \right] - 24 \lambda Y_d^{pr} \mathbf{T}_{\ell H} + \left\{ 24 \lambda Y_d^{pr} \right. \\
& - 48 (Y_d Y_d^\dagger Y_d)^{pr} \Big\} C_H + \left\{ \frac{7}{27} g_Y^2 g_L^2 Y_d^{pr} + \frac{1}{2} \lambda^2 Y_d^{pr} + g_s^2 \left( 16 (Y_d Y_d^\dagger Y_d)^{pr} - 16 (Y_u Y_u^\dagger Y_d)^{pr} \right) + g_Y^2 \left( \frac{1}{12} \mathbf{T}_2 Y_d^{pr} + \frac{13}{48} (Y_d Y_d^\dagger Y_d)^{pr} - \frac{79}{48} (Y_u Y_u^\dagger Y_d)^{pr} \right) \right. \\
& + \lambda \left( 2 (Y_u Y_u^\dagger Y_d)^{pr} + \frac{9}{4} g_L^2 Y_d^{pr} + \frac{163}{36} g_Y^2 Y_d^{pr} + 5 \mathbf{T}_2 Y_d^{pr} - \frac{53}{2} (Y_d Y_d^\dagger Y_d)^{pr} \right) + \frac{5}{2} \mathbf{T}_2 (Y_u Y_u^\dagger Y_d)^{pr} + \frac{25}{8} (Y_d Y_d^\dagger Y_d Y_d^\dagger Y_d)^{pr} + \frac{77}{8} (Y_u Y_u^\dagger Y_u Y_u^\dagger Y_d)^{pr} \\
& + \frac{45}{2} Y_d^{pr} \text{Tr} \left[ Y_d^\dagger Y_d Y_u^\dagger Y_u \right] - g_L^2 \left( \frac{7}{16} (Y_u Y_u^\dagger Y_d)^{pr} + \frac{17}{12} \mathbf{T}_2 Y_d^{pr} + \frac{23}{16} (Y_d Y_d^\dagger Y_d)^{pr} \right) - (Y_d Y_d^\dagger Y_u Y_u^\dagger Y_d)^{pr} - \frac{31}{18} g_Y^4 Y_d^{pr} - 2 (Y_u Y_u^\dagger Y_d Y_d^\dagger Y_d)^{pr} \\
& - \frac{71}{24} g_L^4 Y_d^{pr} - \frac{13}{4} \mathbf{T}_4 Y_d^{pr} - \frac{9}{2} \mathbf{T}_2 (Y_d Y_d^\dagger Y_d)^{pr} \Big\} C_{HD}^{(\parallel)} + \left\{ \frac{1}{4} (Y_u Y_u^\dagger Y_d Y_d^\dagger Y_d)^{pr} + \frac{1}{2} (Y_u Y_u^\dagger Y_u Y_u^\dagger Y_d)^{pr} + \lambda^2 Y_d^{pr} + \lambda \left( \frac{287}{36} g_Y^2 Y_d^{pr} + \frac{51}{4} g_L^2 Y_d^{pr} \right) \right. \\
& - \frac{1}{2} (Y_u Y_u^\dagger Y_d)^{pr} - 31 (Y_d Y_d^\dagger Y_d)^{pr} \Big\} + g_Y^2 \left( \frac{1}{6} \mathbf{T}_2 Y_d^{pr} + \frac{17}{6} (Y_u Y_u^\dagger Y_d)^{pr} - \frac{85}{36} (Y_d Y_d^\dagger Y_d)^{pr} \right) + g_L^2 \left( \frac{3}{2} \mathbf{T}_2 Y_d^{pr} + \frac{23}{8} (Y_u Y_u^\dagger Y_d)^{pr} + \frac{43}{8} (Y_d Y_d^\dagger Y_d)^{pr} \right) \\
& + (Y_d Y_d^\dagger Y_u Y_u^\dagger Y_d)^{pr} + \frac{133}{96} g_L^4 Y_d^{pr} + 2 (Y_d Y_d^\dagger Y_d Y_d^\dagger Y_d)^{pr} + \frac{32}{3} g_s^2 (Y_d Y_d^\dagger Y_d)^{pr} - \frac{65}{288} g_Y^4 Y_d^{pr} - \frac{7}{4} \mathbf{T}_4 Y_d^{pr} - 3 \mathbf{T}_2 (Y_d Y_d^\dagger Y_d)^{pr}
\end{aligned}$$

$$\begin{aligned}
& -\frac{2407}{432}g_Y^2g_L^2Y_d^{pr} - \frac{27}{2}Y_d^{pr}\text{Tr}[Y_d^\dagger Y_d Y_u^\dagger Y_u] \Big\} C_{HD}^{(\times)} + \left\{ g_Y^4 \left( \frac{79}{12}(Y_u Y_u^\dagger Y_d)^{pr} + \frac{53}{6}Y_d^{pr}\text{Tr}[Y_d^\dagger Y_d] - \frac{79}{6}Y_d^{pr}\text{Tr}[Y_u^\dagger Y_u] - \frac{43}{2}Y_d^{pr}\text{Tr}[Y_e^\dagger Y_e] \right. \right. \\
& - \frac{815}{36}(Y_d Y_d^\dagger Y_d)^{pr} \Big) + \frac{601}{18}\lambda g_Y^4 Y_d^{pr} - \frac{29}{3}g_Y^4 g_L^2 Y_d^{pr} - \frac{124}{9}g_Y^4 g_s^2 Y_d^{pr} - \frac{1274}{27}g_Y^6 Y_d^{pr} \Big\} C_{HB} + \left\{ \frac{17i}{18}\lambda g_Y^4 Y_d^{pr} + g_Y^4 \left( \frac{95i}{12}(Y_u Y_u^\dagger Y_d)^{pr} \right. \right. \\
& + \frac{103i}{12}(Y_d Y_d^\dagger Y_d)^{pr} + \frac{39i}{2}Y_d^{pr}\text{Tr}[Y_e^\dagger Y_e] - \frac{3i}{2}Y_d^{pr}\text{Tr}[Y_d^\dagger Y_d] - \frac{33i}{2}Y_d^{pr}\text{Tr}[Y_u^\dagger Y_u] \Big) + \frac{17i}{12}g_Y^4 g_L^2 Y_d^{pr} + \frac{20i}{3}g_Y^4 g_s^2 Y_d^{pr} \\
& + \frac{821i}{108}g_Y^6 Y_d^{pr} \Big\} C_{H\tilde{B}} + \left\{ g_L^4 \left( \frac{3}{2}\text{T}_2 Y_d^{pr} - \frac{51}{4}(Y_u Y_u^\dagger Y_d)^{pr} - \frac{243}{4}(Y_d Y_d^\dagger Y_d)^{pr} \right) + \frac{77}{3}g_L^6 Y_d^{pr} + \frac{147}{2}\lambda g_L^4 Y_d^{pr} - \frac{37}{3}g_Y^2 g_L^4 Y_d^{pr} \right. \\
& - 36g_s^2 g_L^4 Y_d^{pr} \Big\} C_{HW} + \left\{ g_L^4 \left( \frac{9i}{2}Y_d^{pr}\text{Tr}[Y_e^\dagger Y_e] + \frac{27i}{2}Y_d^{pr}\text{Tr}[Y_d^\dagger Y_d] + \frac{57i}{4}(Y_u Y_u^\dagger Y_d)^{pr} + \frac{213i}{4}(Y_d Y_d^\dagger Y_d)^{pr} - \frac{27i}{2}Y_d^{pr}\text{Tr}[Y_u^\dagger Y_u] \right) \right. \\
& + \frac{17i}{12}g_Y^2 g_L^4 Y_d^{pr} + \frac{51i}{2}\lambda g_L^4 Y_d^{pr} + 36ig_s^2 g_L^4 Y_d^{pr} - \frac{341i}{4}g_L^6 Y_d^{pr} \Big\} C_{H\tilde{W}} + \left\{ g_s^4 \left( 64(Y_u Y_u^\dagger Y_d)^{pr} - 176Y_d^{pr}\text{Tr}[Y_d^\dagger Y_d] - 176Y_d^{pr}\text{Tr}[Y_u^\dagger Y_u] \right. \right. \\
& - \frac{584}{3}(Y_d Y_d^\dagger Y_d)^{pr} \Big) + 864g_s^6 Y_d^{pr} - \frac{124}{9}g_Y^2 g_s^4 Y_d^{pr} - \frac{64}{3}\lambda g_s^4 Y_d^{pr} - 36g_s^4 g_L^2 Y_d^{pr} \Big\} C_{HG} + \left\{ g_s^4 \left( 32i(Y_u Y_u^\dagger Y_d)^{pr} + 144iY_d^{pr}\text{Tr}[Y_d^\dagger Y_d] \right. \right. \\
& + 280i(Y_d Y_d^\dagger Y_d)^{pr} - 144iY_d^{pr}\text{Tr}[Y_u^\dagger Y_u] \Big) + \frac{20i}{3}g_Y^2 g_s^4 Y_d^{pr} + 36ig_s^4 g_L^2 Y_d^{pr} + \frac{544i}{3}\lambda g_s^4 Y_d^{pr} - \frac{1760i}{3}g_s^6 Y_d^{pr} \Big\} C_{H\tilde{G}} + \left\{ g_Y^2 g_L^2 \left( \frac{23}{4}Y_d^{pr}\text{Tr}[Y_e^\dagger Y_e] \right. \right. \\
& + \frac{25}{4}Y_d^{pr}\text{Tr}[Y_d^\dagger Y_d] + \frac{47}{4}Y_d^{pr}\text{Tr}[Y_u^\dagger Y_u] - \frac{11}{6}(Y_u Y_u^\dagger Y_d)^{pr} - \frac{23}{4}(Y_d Y_d^\dagger Y_d)^{pr} \Big) + \frac{173}{12}\lambda g_Y^2 g_L^2 Y_d^{pr} - \frac{35}{9}g_Y^2 g_L^4 Y_d^{pr} - \frac{22}{3}g_Y^2 g_s^2 g_L^2 Y_d^{pr} \\
& - \frac{469}{36}g_Y^4 g_L^2 Y_d^{pr} \Big\} C_{HWB} + \left\{ g_Y^2 g_L^2 \left( \frac{i}{12}(Y_u Y_u^\dagger Y_d)^{pr} + 3i(Y_d Y_d^\dagger Y_d)^{pr} + \frac{27i}{4}Y_d^{pr}\text{Tr}[Y_u^\dagger Y_u] - \frac{9i}{4}Y_d^{pr}\text{Tr}[Y_d^\dagger Y_d] - \frac{15i}{4}Y_d^{pr}\text{Tr}[Y_e^\dagger Y_e] \right) \right. \\
& + 2ig_Y^2 g_s^2 g_L^2 Y_d^{pr} + \frac{37i}{18}g_Y^4 g_L^2 Y_d^{pr} + \frac{103i}{36}g_Y^2 g_L^4 Y_d^{pr} - \frac{9i}{4}\lambda g_Y^2 g_L^2 Y_d^{pr} \Big\} C_{H\tilde{W}B} + \left\{ g_L^6 \left( 3\text{T}_2 Y_d^{pr} - \frac{9}{4}(Y_d Y_d^\dagger Y_d)^{pr} - 3(Y_u Y_u^\dagger Y_d)^{pr} \right) \right. \\
& + \frac{103}{12}g_L^8 Y_d^{pr} - \frac{17}{4}g_Y^2 g_L^6 Y_d^{pr} - 6\lambda g_L^6 Y_d^{pr} \Big\} C_W + \left\{ g_L^6 \left( \frac{9i}{4}(Y_d Y_d^\dagger Y_d)^{pr} + 12i(Y_u Y_u^\dagger Y_d)^{pr} \right) - \frac{13i}{6}g_Y^2 g_L^6 Y_d^{pr} - 39ig_L^8 Y_d^{pr} \right\} C_{\tilde{W}} - \left\{ 28g_s^6(Y_d Y_d^\dagger Y_d)^{pr} \right. \\
& + 88\lambda g_s^6 Y_d^{pr} \Big\} C_G + \left\{ 140ig_s^6(Y_d Y_d^\dagger Y_d)^{pr} - 24i\lambda g_s^6 Y_d^{pr} \right\} C_{\tilde{G}} + \left\{ Y_e^{*ab}(Y_u Y_u^\dagger Y_d)^{pr} + \frac{13}{4}g_Y^2 Y_e^{*ab} Y_d^{pr} + 5\lambda Y_e^{*ab} Y_d^{pr} - \frac{9}{4}g_L^2 Y_e^{*ab} Y_d^{pr} \right. \\
& - \frac{13}{2}Y_e^{*ab}(Y_d Y_d^\dagger Y_d)^{pr} - 14Y_d^{pr}(Y_e^\dagger Y_e Y_e^\dagger)^{ab} \Big\} C_{eH}^{ab} + C_{eH}^{*ab} \left\{ \frac{3}{2}Y_e^{ab}(Y_u Y_u^\dagger Y_d)^{pr} + 5\lambda Y_d^{pr} Y_e^{ab} - 5Y_e^{ab}(Y_d Y_d^\dagger Y_d)^{pr} - 5Y_d^{pr}(Y_e Y_e^\dagger Y_e)^{ab} \right\}
\end{aligned}$$

$$\begin{aligned}
& + \left\{ \frac{1}{4} (Y_u^\dagger Y_d)^{br} (Y_d Y_d^\dagger)^{pa} + \frac{1}{2} T_2 \delta^{pa} (Y_u^\dagger Y_d)^{br} + \frac{11}{4} (Y_u^\dagger Y_d)^{br} (Y_u Y_u^\dagger)^{pa} + \frac{9}{2} Y_d^{pr} (Y_d^\dagger Y_d Y_u^\dagger)^{ab} + \frac{9}{2} Y_u^{*ab} (Y_u Y_u^\dagger Y_d)^{pr} + 5 \delta^{pa} (Y_u^\dagger Y_u Y_u^\dagger Y_d)^{br} \right. \\
& + \frac{51}{8} \delta^{pa} g_L^2 (Y_u^\dagger Y_d)^{br} + 15 \lambda Y_u^{*ab} Y_d^{pr} - \frac{1}{2} \delta^{pa} (Y_u^\dagger Y_d Y_d^\dagger Y_d)^{br} - \frac{49}{72} \delta^{pa} g_Y^2 (Y_u^\dagger Y_d)^{br} - 15 Y_d^{pr} (Y_u^\dagger Y_u Y_u^\dagger)^{ab} - 15 Y_u^{*ab} (Y_d Y_d^\dagger Y_d)^{pr} \\
& - \frac{56}{3} \delta^{pa} g_s^2 (Y_u^\dagger Y_d)^{br} \left. \right\} C_{uH}^{ab} + C_{uH}^{*ab} \left\{ g_L^2 \left( \frac{3}{2} Y_d^{ar} Y_u^{pb} - \frac{27}{4} Y_d^{pr} Y_u^{ab} \right) + g_s^2 \left( 40 Y_d^{pr} Y_u^{ab} - \frac{40}{3} Y_d^{ar} Y_u^{pb} \right) + \lambda \left( 3 Y_d^{ar} Y_u^{pb} + 15 Y_d^{pr} Y_u^{ab} \right) + 2 T_2 Y_d^{ar} Y_u^{pb} \right. \\
& + \frac{11}{4} Y_d^{ar} (Y_d Y_d^\dagger Y_u)^{pb} + 3 Y_u^{ab} (Y_u Y_u^\dagger Y_d)^{pr} + \frac{23}{4} Y_d^{ar} (Y_u Y_u^\dagger Y_u)^{pb} + \frac{15}{2} Y_d^{pr} (Y_d Y_d^\dagger Y_u)^{ab} + \frac{19}{2} Y_u^{pb} (Y_u Y_u^\dagger Y_d)^{ar} - g_Y^2 \left( \frac{23}{12} Y_d^{pr} Y_u^{ab} + \frac{47}{18} Y_d^{ar} Y_u^{pb} \right) \\
& - 2 Y_u^{pb} (Y_d Y_d^\dagger Y_d)^{ar} - \frac{39}{2} Y_u^{ab} (Y_d Y_d^\dagger Y_d)^{pr} - 42 Y_d^{pr} (Y_u Y_u^\dagger Y_u)^{ab} \left. \right\} + \left\{ \frac{1}{4} \delta^{rb} (Y_d Y_d^\dagger Y_u Y_u^\dagger)^{pa} + \lambda \left( 15 Y_d^{*ab} Y_d^{pr} + 18 \delta^{pa} \delta^{rb} g_Y^2 + 54 \delta^{pa} \delta^{rb} g_L^2 \right. \right. \\
& - 24 T_2 \delta^{pa} \delta^{rb} - 42 \delta^{pa} (Y_d^\dagger Y_d)^{br} - 42 \delta^{rb} (Y_d Y_d^\dagger)^{pa} \left. \right) + g_L^2 \left( \frac{57}{16} \delta^{rb} (Y_u Y_u^\dagger)^{pa} + \frac{45}{8} T_2 \delta^{pa} \delta^{rb} + \frac{171}{8} \delta^{pa} (Y_d^\dagger Y_d)^{br} + \frac{387}{16} \delta^{rb} (Y_d Y_d^\dagger)^{pa} - \frac{27}{4} Y_d^{*ab} Y_d^{pr} \right) \\
& + g_Y^2 \left( \frac{25}{8} \delta^{pa} \delta^{rb} \text{Tr} [Y_d^\dagger Y_d] + \frac{599}{72} \delta^{pa} (Y_d^\dagger Y_d)^{br} + \frac{1349}{144} \delta^{rb} (Y_d Y_d^\dagger)^{pa} + \frac{75}{8} \delta^{pa} \delta^{rb} \text{Tr} [Y_e^\dagger Y_e] + \frac{85}{8} \delta^{pa} \delta^{rb} \text{Tr} [Y_u^\dagger Y_u] - \frac{79}{48} \delta^{rb} (Y_u Y_u^\dagger)^{pa} - \frac{83}{12} Y_d^{*ab} Y_d^{pr} \right) \\
& + g_s^2 \left( \frac{104}{3} \delta^{rb} (Y_d Y_d^\dagger)^{pa} + \frac{112}{3} \delta^{pa} (Y_d^\dagger Y_d)^{br} + 40 Y_d^{*ab} Y_d^{pr} + 60 \delta^{pa} \delta^{rb} \text{Tr} [Y_d^\dagger Y_d] + 60 \delta^{pa} \delta^{rb} \text{Tr} [Y_u^\dagger Y_u] - 16 \delta^{rb} (Y_u Y_u^\dagger)^{pa} \right) + \frac{9}{8} \delta^{pa} \delta^{rb} g_Y^2 g_L^2 \\
& + \frac{5}{4} T_2 \delta^{rb} (Y_u Y_u^\dagger)^{pa} + 3 Y_d^{*ab} (Y_u Y_u^\dagger Y_d)^{pr} + \frac{31}{9} \delta^{pa} \delta^{rb} g_Y^2 g_s^2 + \frac{17}{4} \delta^{pa} (Y_d^\dagger Y_u Y_u^\dagger Y_d)^{br} + \frac{15}{2} Y_d^{pr} (Y_u^\dagger Y_u Y_d^\dagger)^{ab} + \frac{35}{4} \delta^{rb} (Y_u Y_u^\dagger Y_u Y_u^\dagger)^{pa} \\
& + 9 \delta^{pa} \delta^{rb} g_s^2 g_L^2 + \frac{5083}{432} \delta^{pa} \delta^{rb} g_Y^4 - \frac{1}{2} (Y_d^\dagger Y_d)^{br} (Y_u Y_u^\dagger)^{pa} - \delta^{rb} (Y_u Y_u^\dagger Y_d Y_d^\dagger)^{pa} - \frac{5}{2} (Y_d^\dagger Y_d)^{br} (Y_d Y_d^\dagger)^{pa} - \frac{11}{4} T_4 \delta^{pa} \delta^{rb} - \frac{13}{2} T_2 \delta^{pa} (Y_d^\dagger Y_d)^{br} \\
& - \frac{29}{4} T_2 \delta^{rb} (Y_d Y_d^\dagger)^{pa} - \frac{31}{4} \delta^{rb} (Y_d Y_d^\dagger Y_d Y_d^\dagger)^{pa} - \frac{17}{2} \delta^{pa} (Y_d^\dagger Y_d Y_d^\dagger Y_d)^{br} - \frac{201}{16} \delta^{pa} \delta^{rb} g_L^4 - \frac{39}{2} Y_d^{*ab} (Y_d Y_d^\dagger Y_d)^{pr} - \frac{39}{2} \delta^{pa} \delta^{rb} \text{Tr} [Y_d^\dagger Y_d Y_u^\dagger Y_u] \\
& - 42 Y_d^{pr} (Y_d^\dagger Y_d Y_d^\dagger)^{ab} - \frac{153}{2} \delta^{pa} \delta^{rb} \lambda^2 - 108 \delta^{pa} \delta^{rb} g_s^4 \left. \right\} C_{dH}^{ab} + C_{dH}^{*ab} \left\{ \lambda \left( 15 Y_d^{pr} Y_d^{ab} - 18 Y_d^{pb} Y_d^{ar} \right) + \frac{3}{2} g_L^2 Y_d^{pb} Y_d^{ar} + \frac{11}{6} g_Y^2 Y_d^{pb} Y_d^{ar} \right. \\
& + \frac{9}{2} Y_d^{ab} (Y_u Y_u^\dagger Y_d)^{pr} + \frac{9}{2} Y_d^{pr} (Y_u Y_u^\dagger Y_d)^{ab} + \frac{11}{2} Y_d^{pb} (Y_d Y_d^\dagger Y_d)^{ar} + \frac{23}{4} Y_d^{ar} (Y_d Y_d^\dagger Y_d)^{pb} + 40 g_s^2 Y_d^{pb} Y_d^{ar} - \frac{1}{2} Y_d^{pb} (Y_u Y_u^\dagger Y_d)^{ar} - \frac{7}{4} Y_d^{ar} (Y_u Y_u^\dagger Y_d)^{pb} \\
& - 15 Y_d^{ab} (Y_d Y_d^\dagger Y_d)^{pr} - 15 Y_d^{pr} (Y_d Y_d^\dagger Y_d)^{ab} \left. \right\} + \left\{ 3 \lambda g_Y^2 Y_e^{*ab} Y_d^{pr} + \frac{19}{6} g_Y^2 g_L^2 Y_e^{*ab} Y_d^{pr} - \frac{7}{2} g_Y^2 Y_d^{pr} (Y_e^\dagger Y_e Y_e^\dagger)^{ab} - \frac{28}{3} g_Y^4 Y_e^{*ab} Y_d^{pr} \right\} C_{eB}^{ab} \\
& + C_{eB}^{*ab} \left\{ \frac{3}{2} g_Y^2 Y_d^{pr} (Y_e Y_e^\dagger Y_e)^{ab} + 2 \lambda g_Y^2 Y_d^{pr} Y_e^{ab} + \frac{11}{3} g_Y^4 Y_d^{pr} Y_e^{ab} - \frac{5}{6} g_Y^2 g_L^2 Y_d^{pr} Y_e^{ab} \right\} + \left\{ \frac{29}{12} g_L^4 Y_e^{*ab} Y_d^{pr} + \frac{13}{4} g_L^2 Y_d^{pr} (Y_e^\dagger Y_e Y_e^\dagger)^{ab} \right. \\
& - \frac{3}{2} \lambda g_L^2 Y_e^{*ab} Y_d^{pr} - 5 g_Y^2 g_L^2 Y_e^{*ab} Y_d^{pr} \left. \right\} C_{eW}^{ab} + C_{eW}^{*ab} \left\{ g_Y^2 g_L^2 Y_d^{pr} Y_e^{ab} + 3 \lambda g_L^2 Y_d^{pr} Y_e^{ab} - \frac{23}{4} g_L^2 Y_d^{pr} (Y_e Y_e^\dagger Y_e)^{ab} - \frac{79}{12} g_L^4 Y_d^{pr} Y_e^{ab} \right\}
\end{aligned}$$

$$\begin{aligned}
& + \left\{ g_Y^2 g_L^2 \left( \frac{7}{12} \delta^{pa} (Y_u^\dagger Y_d)^{br} - \frac{1}{3} Y_u^{*ab} Y_d^{pr} \right) + g_Y^2 \left( \frac{3}{2} Y_d^{pr} (Y_d^\dagger Y_d Y_u^\dagger)^{ab} + \frac{3}{2} Y_d^{pr} (Y_u^\dagger Y_u Y_u^\dagger)^{ab} + \frac{17}{4} (Y_u^\dagger Y_d)^{br} (Y_d Y_d^\dagger)^{pa} - \frac{11}{6} \delta^{pa} (Y_u^\dagger Y_d Y_d^\dagger Y_d)^{br} \right. \right. \\
& - \frac{11}{3} \delta^{pa} (Y_u^\dagger Y_u Y_u^\dagger Y_d)^{br} - \frac{77}{12} (Y_u^\dagger Y_d)^{br} (Y_u Y_u^\dagger)^{pa} \left. \right) - g_Y^4 \left( \frac{1}{4} \delta^{pa} (Y_u^\dagger Y_d)^{br} + \frac{35}{18} Y_u^{*ab} Y_d^{pr} \right) - \lambda g_Y^2 \left( 3 \delta^{pa} (Y_u^\dagger Y_d)^{br} + 5 Y_u^{*ab} Y_d^{pr} \right) \Big\} C_{uB}^{ab} \\
& + C_{uB}^{*ab} \left\{ g_Y^4 \left( \frac{205}{18} Y_d^{pr} Y_u^{ab} - \frac{4}{3} Y_d^{ar} Y_u^{pb} \right) + \lambda g_Y^2 \left( \frac{14}{3} Y_d^{ar} Y_u^{pb} - 5 Y_d^{pr} Y_u^{ab} \right) + g_Y^2 \left( \frac{2}{3} Y_u^{pb} (Y_u Y_u^\dagger Y_d)^{ar} + \frac{3}{2} Y_d^{pr} (Y_d Y_d^\dagger Y_u)^{ab} + \frac{13}{2} Y_d^{pr} (Y_u Y_u^\dagger Y_u)^{ab} \right. \right. \\
& - \frac{1}{3} Y_u^{pb} (Y_d Y_d^\dagger Y_d)^{ar} - \frac{7}{12} Y_d^{ar} (Y_u Y_u^\dagger Y_u)^{pb} - \frac{17}{12} Y_d^{ar} (Y_d Y_d^\dagger Y_u)^{pb} \left. \right) - g_Y^2 g_L^2 \left( 4 Y_d^{ar} Y_u^{pb} + \frac{28}{3} Y_d^{pr} Y_u^{ab} \right) \Big\} + \left\{ g_Y^2 g_L^2 \left( \frac{13}{12} Y_u^{*ab} Y_d^{pr} + \frac{103}{36} \delta^{pa} (Y_u^\dagger Y_d)^{br} \right) \right. \\
& + g_L^2 \left( \frac{7}{4} \delta^{pa} (Y_u^\dagger Y_d Y_d^\dagger Y_d)^{br} + \frac{39}{4} Y_d^{pr} (Y_u^\dagger Y_u Y_u^\dagger)^{ab} - \frac{11}{8} (Y_u^\dagger Y_d)^{br} (Y_u Y_u^\dagger)^{pa} - \frac{3}{2} T_2 \delta^{pa} (Y_u^\dagger Y_d)^{br} - \frac{23}{8} (Y_u^\dagger Y_d)^{br} (Y_d Y_d^\dagger)^{pa} - \frac{27}{4} Y_d^{pr} (Y_d^\dagger Y_d Y_u^\dagger)^{ab} \right. \\
& - \frac{35}{2} \delta^{pa} (Y_u^\dagger Y_u Y_u^\dagger Y_d)^{br} \left. \right) + \frac{16}{3} \delta^{pa} g_s^2 g_L^2 (Y_u^\dagger Y_d)^{br} - g_L^4 \left( \frac{13}{3} \delta^{pa} (Y_u^\dagger Y_d)^{br} + 13 Y_u^{*ab} Y_d^{pr} \right) - \lambda g_L^2 \left( \frac{9}{2} Y_u^{*ab} Y_d^{pr} + 6 \delta^{pa} (Y_u^\dagger Y_d)^{br} \right) \Big\} C_{uW}^{ab} \\
& + C_{uW}^{*ab} \left\{ g_L^4 \left( \frac{1}{2} Y_d^{pr} Y_u^{ab} - \frac{43}{8} Y_d^{ar} Y_u^{pb} \right) + \lambda g_L^2 \left( \frac{51}{2} Y_d^{ar} Y_u^{pb} - \frac{9}{2} Y_d^{pr} Y_u^{ab} \right) + g_L^2 \left( \frac{3}{2} T_2 Y_d^{ar} Y_u^{pb} + 2 Y_u^{pb} (Y_d Y_d^\dagger Y_d)^{ar} + \frac{39}{4} Y_d^{pr} (Y_u Y_u^\dagger Y_u)^{ab} \right. \right. \\
& + \frac{111}{8} Y_d^{ar} (Y_d Y_d^\dagger Y_u)^{pb} + \frac{123}{4} Y_d^{pr} (Y_d Y_d^\dagger Y_u)^{ab} - 2 Y_u^{pb} (Y_u Y_u^\dagger Y_d)^{ar} - \frac{143}{8} Y_d^{ar} (Y_u Y_u^\dagger Y_u)^{pb} \left. \right) + 8 g_s^2 g_L^2 Y_d^{ar} Y_u^{pb} - g_Y^2 g_L^2 \left( \frac{37}{24} Y_d^{ar} Y_u^{pb} + \frac{77}{12} Y_d^{pr} Y_u^{ab} \right) \Big\} \\
& + \left\{ g_s^2 g_L^2 \left( \frac{16}{3} Y_u^{*ab} Y_d^{pr} - \frac{40}{3} \delta^{pa} (Y_u^\dagger Y_d)^{br} \right) + \lambda g_s^2 \left( 8 \delta^{pa} (Y_u^\dagger Y_d)^{br} - 16 Y_u^{*ab} Y_d^{pr} \right) + g_s^2 \left( \frac{8}{3} \delta^{pa} (Y_u^\dagger Y_u Y_u^\dagger Y_d)^{br} + \frac{32}{3} (Y_u^\dagger Y_d)^{br} (Y_u Y_u^\dagger)^{pa} \right. \right. \\
& + \frac{40}{3} \delta^{pa} (Y_u^\dagger Y_d Y_d^\dagger Y_d)^{br} - 8 (Y_u^\dagger Y_d)^{br} (Y_d Y_d^\dagger)^{pa} \left. \right) + \frac{16}{3} g_Y^2 g_s^2 Y_u^{*ab} Y_d^{pr} - \frac{64}{3} g_s^4 Y_u^{*ab} Y_d^{pr} \Big\} C_{uG}^{ab} + C_{uG}^{*ab} \left\{ g_s^2 \left( \frac{4}{3} Y_u^{pb} (Y_d Y_d^\dagger Y_d)^{ar} + 16 Y_d^{pr} (Y_u Y_u^\dagger Y_u)^{ab} \right. \right. \\
& - \frac{4}{3} Y_d^{ar} (Y_d Y_d^\dagger Y_u)^{pb} - \frac{20}{3} Y_d^{ar} (Y_u Y_u^\dagger Y_u)^{pb} - \frac{44}{3} Y_u^{pb} (Y_u Y_u^\dagger Y_d)^{ar} \left. \right) + \frac{16}{3} g_s^2 g_L^2 Y_d^{pr} Y_u^{ab} + \frac{16}{3} g_Y^2 g_s^2 Y_d^{pr} Y_u^{ab} - \lambda g_s^2 \left( 16 Y_d^{pr} Y_u^{ab} + \frac{56}{3} Y_d^{ar} Y_u^{pb} \right) \\
& - \frac{160}{3} g_s^4 Y_d^{pr} Y_u^{ab} \Big\} + \left\{ g_Y^2 g_s^2 \left( \frac{104}{9} \delta^{rb} (Y_d Y_d^\dagger)^{pa} - \frac{40}{9} \delta^{pa} (Y_d^\dagger Y_d)^{br} \right) + \lambda \left( g_Y^2 \left( Y_d^{*ab} Y_d^{pr} + \frac{115}{6} \delta^{rb} (Y_d Y_d^\dagger)^{pa} - 3 \delta^{pa} \delta^{rb} \text{Tr} [Y_d^\dagger Y_d] - \frac{22}{3} \delta^{rb} (Y_u Y_u^\dagger)^{pa} \right. \right. \right. \\
& - 9 \delta^{pa} \delta^{rb} \text{Tr} [Y_e^\dagger Y_e] - \frac{199}{6} \delta^{pa} (Y_d^\dagger Y_d)^{br} \left. \right) + 17 \delta^{pa} \delta^{rb} g_Y^2 g_L^2 - \frac{32}{9} \delta^{pa} \delta^{rb} g_Y^2 g_s^2 - \frac{185}{27} \delta^{pa} \delta^{rb} g_Y^4 \left. \right) + g_Y^4 \left( \delta^{rb} (Y_u Y_u^\dagger)^{pa} + \frac{19}{3} \delta^{pa} \delta^{rb} \text{Tr} [Y_u^\dagger Y_u] \right. \\
& + \frac{25}{3} \delta^{pa} \delta^{rb} \text{Tr} [Y_e^\dagger Y_e] + \frac{1249}{54} \delta^{pa} (Y_d^\dagger Y_d)^{br} - \frac{5}{3} \delta^{pa} \delta^{rb} \text{Tr} [Y_d^\dagger Y_d] - \frac{28}{9} Y_d^{*ab} Y_d^{pr} - \frac{859}{108} \delta^{rb} (Y_d Y_d^\dagger)^{pa} \left. \right) + g_Y^2 g_L^2 \left( \frac{14}{3} \delta^{rb} (Y_u Y_u^\dagger)^{pa} + 9 \delta^{pa} \delta^{rb} \text{Tr} [Y_d^\dagger Y_d] \right. \\
& + \frac{29}{3} \delta^{pa} (Y_d^\dagger Y_d)^{br} + 11 \delta^{pa} \delta^{rb} \text{Tr} [Y_e^\dagger Y_e] + \frac{73}{6} Y_d^{*ab} Y_d^{pr} + 21 \delta^{pa} \delta^{rb} \text{Tr} [Y_u^\dagger Y_u] - \frac{233}{12} \delta^{rb} (Y_d Y_d^\dagger)^{pa} \left. \right) + g_Y^2 \left( \frac{3}{2} T_2 \delta^{rb} (Y_d Y_d^\dagger)^{pa} + 2 \delta^{rb} (Y_u Y_u^\dagger Y_d Y_d^\dagger)^{pa} \right)
\end{aligned}$$

$$\begin{aligned}
& + 3\delta^{rb}(Y_u Y_u^\dagger Y_u Y_u^\dagger)^{pa} + \frac{19}{6}\delta^{rb}(Y_d Y_d^\dagger Y_d Y_d^\dagger)^{pa} + 6\delta^{pa}\delta^{rb}\text{Tr}[Y_d^\dagger Y_d Y_d^\dagger Y_d] + \frac{103}{12}\delta^{pa}(Y_d^\dagger Y_d Y_d^\dagger Y_d)^{br} + 18\delta^{pa}\delta^{rb}\text{Tr}[Y_e^\dagger Y_e Y_e^\dagger Y_e] \\
& - \frac{1}{12}\delta^{rb}(Y_d Y_d^\dagger Y_u Y_u^\dagger)^{pa} - \frac{5}{6}(Y_d^\dagger Y_d)^{br}(Y_u Y_u^\dagger)^{pa} - \frac{3}{2}\text{T}_2\delta^{pa}(Y_d^\dagger Y_d)^{br} - \frac{3}{2}Y_d^{pr}(Y_u^\dagger Y_u Y_d^\dagger)^{ab} - \frac{5}{2}Y_d^{pr}(Y_d^\dagger Y_d Y_d^\dagger)^{ab} - 6\delta^{pa}(Y_d^\dagger Y_u Y_u^\dagger Y_d)^{br} \\
& + \frac{32}{9}\delta^{pa}\delta^{rb}g_Y^4 g_s^2 + \frac{1121}{54}\delta^{pa}\delta^{rb}g_Y^6 - \frac{1}{3}\delta^{pa}\delta^{rb}g_Y^2 g_L^4 - \frac{32}{3}\delta^{pa}\delta^{rb}g_Y^2 g_s^2 g_L^2 - \frac{104}{3}\delta^{pa}\delta^{rb}g_Y^4 g_L^2 \Big\} C_{dB}^{ab} + C_{dB}^{*ab} \Big\{ g_Y^2 g_L^2 \Big( \frac{1}{6}Y_d^{pr}Y_d^{ab} - \frac{5}{2}Y_d^{pb}Y_d^{ar} \Big) \\
& + g_Y^4 \Big( \frac{23}{54}Y_d^{pb}Y_d^{ar} + \frac{11}{9}Y_d^{pr}Y_d^{ab} \Big) + g_Y^2 \Big( \frac{5}{2}Y_d^{pb}(Y_d Y_d^\dagger Y_d)^{ar} + \frac{9}{2}Y_d^{pr}(Y_d Y_d^\dagger Y_d)^{ab} - \frac{1}{4}Y_d^{ar}(Y_d Y_d^\dagger Y_d)^{pb} - \frac{1}{3}Y_d^{pb}(Y_u Y_u^\dagger Y_d)^{ar} - \frac{3}{2}Y_d^{pr}(Y_u Y_u^\dagger Y_d)^{ab} \\
& - \frac{9}{4}Y_d^{ar}(Y_u Y_u^\dagger Y_d)^{pb} \Big) + \frac{16}{9}g_Y^2 g_s^2 Y_d^{pb}Y_d^{ar} - \lambda g_Y^2 \Big( 2Y_d^{pr}Y_d^{ab} + 6Y_d^{pb}Y_d^{ar} \Big) \Big\} + \Big\{ g_L^4 \Big( \frac{29}{4}Y_d^{*ab}Y_d^{pr} + \frac{191}{24}\delta^{pa}(Y_d^\dagger Y_d)^{br} - \frac{3}{2}\text{T}_2\delta^{pa}\delta^{rb} - \frac{14}{3}\delta^{rb}(Y_u Y_u^\dagger)^{pa} \\
& - \frac{287}{24}\delta^{rb}(Y_d Y_d^\dagger)^{pa} \Big) + g_s^2 g_L^2 \Big( \frac{32}{3}\delta^{rb}(Y_u Y_u^\dagger)^{pa} - \frac{44}{3}\delta^{rb}(Y_d Y_d^\dagger)^{pa} - \frac{100}{3}\delta^{pa}(Y_d^\dagger Y_d)^{br} \Big) + \lambda \Big( g_L^2 \Big( \frac{9}{2}\delta^{pa}\delta^{rb}\text{Tr}[Y_e^\dagger Y_e] + \frac{27}{2}\delta^{pa}\delta^{rb}\text{Tr}[Y_d^\dagger Y_d] \\
& + \frac{93}{4}\delta^{rb}(Y_d Y_d^\dagger)^{pa} + 30\delta^{rb}(Y_u Y_u^\dagger)^{pa} - \frac{3}{4}\delta^{pa}(Y_d^\dagger Y_d)^{br} - \frac{9}{2}Y_d^{*ab}Y_d^{pr} \Big) + 16\delta^{pa}\delta^{rb}g_s^2 g_L^2 + 27\delta^{pa}\delta^{rb}g_L^4 - \frac{25}{6}\delta^{pa}\delta^{rb}g_Y^2 g_L^2 \Big) + g_Y^2 g_L^2 \Big( \frac{31}{18}\delta^{rb}(Y_u Y_u^\dagger)^{pa} \\
& + \frac{271}{72}\delta^{pa}(Y_d^\dagger Y_d)^{br} - \frac{1}{3}Y_d^{*ab}Y_d^{pr} - \frac{3}{2}\delta^{pa}\delta^{rb}\text{Tr}[Y_d^\dagger Y_d] - \frac{11}{6}\delta^{pa}\delta^{rb}\text{Tr}[Y_e^\dagger Y_e] - \frac{7}{2}\delta^{pa}\delta^{rb}\text{Tr}[Y_u^\dagger Y_u] - \frac{403}{72}\delta^{rb}(Y_d Y_d^\dagger)^{pa} \Big) + g_L^2 \Big( \frac{9}{4}\text{T}_2\delta^{rb}(Y_d Y_d^\dagger)^{pa} \\
& + \frac{19}{4}(Y_d^\dagger Y_d)^{br}(Y_u Y_u^\dagger)^{pa} + 8\delta^{rb}(Y_u Y_u^\dagger Y_d Y_d^\dagger)^{pa} + \frac{39}{4}Y_d^{pr}(Y_d^\dagger Y_d Y_d^\dagger)^{ab} + \frac{179}{8}\delta^{rb}(Y_d Y_d^\dagger Y_u Y_u^\dagger)^{pa} + \frac{123}{4}Y_d^{pr}(Y_u^\dagger Y_u Y_d^\dagger)^{ab} - \frac{3}{4}\text{T}_2\delta^{pa}(Y_d^\dagger Y_d)^{br} \\
& - \frac{7}{2}(Y_d^\dagger Y_d)^{br}(Y_d Y_d^\dagger)^{pa} - \frac{63}{8}\delta^{pa}(Y_d^\dagger Y_d Y_d^\dagger Y_d)^{br} - 9\delta^{pa}\delta^{rb}\text{Tr}[Y_e^\dagger Y_e Y_e^\dagger Y_e] - \frac{23}{2}\delta^{rb}(Y_d Y_d^\dagger Y_d Y_d^\dagger)^{pa} - 27\delta^{pa}\delta^{rb}\text{Tr}[Y_d^\dagger Y_d Y_d^\dagger Y_d] \\
& - \frac{97}{2}\delta^{rb}(Y_u Y_u^\dagger Y_u Y_u^\dagger)^{pa} \Big) + \frac{16}{9}\delta^{pa}\delta^{rb}g_Y^2 g_s^2 g_L^2 + \frac{781}{108}\delta^{pa}\delta^{rb}g_Y^4 g_L^2 + \frac{305}{4}\delta^{pa}\delta^{rb}g_L^6 - \frac{205}{36}\delta^{pa}\delta^{rb}g_Y^2 g_L^4 - 16\delta^{pa}\delta^{rb}g_s^2 g_L^4 \Big\} C_{dW}^{ab} \\
& + C_{dW}^{*ab} \Big\{ g_Y^2 g_L^2 \Big( \frac{5}{3}Y_d^{pr}Y_d^{ab} + \frac{49}{24}Y_d^{pb}Y_d^{ar} \Big) + \lambda g_L^2 \Big( \frac{15}{2}Y_d^{pb}Y_d^{ar} + 9Y_d^{pr}Y_d^{ab} \Big) + g_L^2 \Big( 3Y_d^{pb}(Y_u Y_u^\dagger Y_d)^{ar} + \frac{47}{8}Y_d^{ar}(Y_u Y_u^\dagger Y_d)^{pb} - \frac{3}{2}\text{T}_2Y_d^{pb}Y_d^{ar} \\
& - \frac{9}{4}Y_d^{pb}(Y_d Y_d^\dagger Y_d)^{ar} - \frac{21}{8}Y_d^{ar}(Y_d Y_d^\dagger Y_d)^{pb} - \frac{27}{4}Y_d^{pr}(Y_u Y_u^\dagger Y_d)^{ab} - \frac{69}{4}Y_d^{pr}(Y_d Y_d^\dagger Y_d)^{ab} \Big) - g_L^4 \Big( \frac{53}{8}Y_d^{pb}Y_d^{ar} + \frac{79}{4}Y_d^{pr}Y_d^{ab} \Big) - 16g_s^2 g_L^2 Y_d^{pb}Y_d^{ar} \Big\} \\
& + \Big\{ g_Y^2 g_s^2 \Big( \frac{16}{3}Y_d^{*ab}Y_d^{pr} - \frac{206}{27}\delta^{rb}(Y_d Y_d^\dagger)^{pa} - \frac{278}{27}\delta^{pa}(Y_d^\dagger Y_d)^{br} \Big) + g_s^2 g_L^2 \Big( \frac{16}{3}Y_d^{*ab}Y_d^{pr} - \frac{26}{3}\delta^{pa}(Y_d^\dagger Y_d)^{br} - \frac{56}{3}\delta^{rb}(Y_u Y_u^\dagger)^{pa} - \frac{82}{3}\delta^{rb}(Y_d Y_d^\dagger)^{pa} \Big) \\
& + \lambda \Big( g_s^2 \Big( \frac{16}{3}\delta^{rb}(Y_u Y_u^\dagger)^{pa} + \frac{152}{3}\delta^{pa}(Y_d^\dagger Y_d)^{br} + \frac{160}{3}\delta^{rb}(Y_d Y_d^\dagger)^{pa} - 16Y_d^{*ab}Y_d^{pr} \Big) + \frac{224}{9}\delta^{pa}\delta^{rb}g_s^4 - \frac{136}{27}\delta^{pa}\delta^{rb}g_Y^2 g_s^2 - 8\delta^{pa}\delta^{rb}g_s^2 g_L^2 \Big) \\
& + g_s^2 \Big( \frac{88}{9}\delta^{pa}\delta^{rb}g_Y^2 g_L^2 + 16Y_d^{pr}(Y_d^\dagger Y_d Y_d^\dagger)^{ab} + 16\delta^{rb}(Y_u Y_u^\dagger Y_d Y_d^\dagger)^{pa} + \frac{100}{3}\delta^{rb}(Y_d Y_d^\dagger Y_u Y_u^\dagger)^{pa} + 36\delta^{pa}(Y_d^\dagger Y_u Y_u^\dagger Y_d)^{br} - \frac{8}{3}(Y_d^\dagger Y_d)^{br}(Y_u Y_u^\dagger)^{pa} \\
& - \frac{332}{3}\delta^{rb}(Y_d Y_d^\dagger Y_d Y_d^\dagger)^{pa} - \frac{340}{3}\delta^{pa}(Y_d^\dagger Y_d Y_d^\dagger Y_d)^{br} \Big) + g_s^4 \Big( \frac{2488}{9}\delta^{pa}(Y_d^\dagger Y_d)^{br} + \frac{2488}{9}\delta^{rb}(Y_d Y_d^\dagger)^{pa} - \frac{64}{3}Y_d^{*ab}Y_d^{pr} - 128\delta^{pa}\delta^{rb}\text{Tr}[Y_d^\dagger Y_d] \Big)
\end{aligned}$$

$$\begin{aligned}
& -128\delta^{pa}\delta^{rb}\text{Tr}\left[Y_u^\dagger Y_u\right] + \frac{100}{27}\delta^{pa}\delta^{rb}g_Y^4g_s^2 + 4\delta^{pa}\delta^{rb}g_s^2g_L^4\left\}C_{dG}^{ab} + C_{dG}^{*ab}\left\{g_s^4\left(\frac{1184}{9}Y_d^{pb}Y_d^{ar} - \frac{160}{3}Y_d^{pr}Y_d^{ab}\right) + g_Y^2g_s^2\left(\frac{68}{27}Y_d^{pb}Y_d^{ar} + \frac{16}{3}Y_d^{pr}Y_d^{ab}\right)\right. \right. \\
& + g_s^2g_L^2\left(4Y_d^{pb}Y_d^{ar} + \frac{16}{3}Y_d^{pr}Y_d^{ab}\right) + \lambda g_s^2\left(72Y_d^{pb}Y_d^{ar} - 16Y_d^{pr}Y_d^{ab}\right) + g_s^2\left(\frac{40}{3}Y_d^{pb}(Y_uY_u^\dagger Y_d)^{ar} - 8Y_d^{ar}(Y_dY_d^\dagger Y_d)^{pb} - 16Y_d^{pb}(Y_dY_d^\dagger Y_d)^{ar}\right)\left. \right\} + \left\{\frac{7}{9}\delta^{ab}g_Y^4Y_d^{pr} \right. \\
& + \frac{43}{27}\delta^{ab}g_Y^2g_L^2Y_d^{pr} + \frac{311}{36}g_Y^2Y_d^{pr}(Y_eY_e^\dagger)^{ba} - \frac{7}{36}g_L^2Y_d^{pr}(Y_eY_e^\dagger)^{ba} - \lambda\left(\frac{26}{9}\delta^{ab}g_Y^2Y_d^{pr} + \frac{16}{3}Y_d^{pr}(Y_eY_e^\dagger)^{ba}\right) - (Y_eY_e^\dagger)^{ba}(Y_dY_d^\dagger Y_d)^{pr} \\
& - 10Y_d^{pr}(Y_eY_e^\dagger Y_eY_e^\dagger)^{ba}\left. \right\}C_{H\ell}^{(\parallel)ab} + \left\{\frac{7}{18}\delta^{ab}g_Y^4Y_d^{pr} + \frac{1}{2}(Y_eY_e^\dagger)^{ba}(Y_dY_d^\dagger Y_d)^{pr} + \frac{83}{108}\delta^{ab}g_Y^2g_L^2Y_d^{pr} + \lambda\left(\frac{8}{3}\delta^{ab}g_L^2Y_d^{pr} - \frac{13}{9}\delta^{ab}g_Y^2Y_d^{pr} \right. \right. \\
& - \frac{29}{3}Y_d^{pr}(Y_eY_e^\dagger)^{ba}) + \frac{37}{9}g_L^2Y_d^{pr}(Y_eY_e^\dagger)^{ba} + \frac{167}{18}g_Y^2Y_d^{pr}(Y_eY_e^\dagger)^{ba} - \frac{5}{2}(Y_eY_e^\dagger)^{ba}(Y_uY_u^\dagger Y_d)^{pr} - \frac{15}{4}\delta^{ab}g_L^4Y_d^{pr} - 8Y_d^{pr}(Y_eY_e^\dagger Y_eY_e^\dagger)^{ba}\left. \right\}C_{H\ell}^{(\times)ab} \\
& + \left\{\frac{5}{54}\delta^{ab}g_Y^2g_L^2Y_d^{pr} + \lambda\left(\frac{16}{3}Y_d^{pr}(Y_e^\dagger Y_e)^{ba} - \frac{26}{9}\delta^{ab}g_Y^2Y_d^{pr}\right) + (Y_e^\dagger Y_e)^{ba}(Y_dY_d^\dagger Y_d)^{pr} + \frac{41}{18}\delta^{ab}g_Y^4Y_d^{pr} + 10Y_d^{pr}(Y_e^\dagger Y_eY_e^\dagger Y_e)^{ba} - \frac{77}{36}g_L^2Y_d^{pr}(Y_e^\dagger Y_e)^{ba} \right. \\
& - \frac{167}{36}g_Y^2Y_d^{pr}(Y_e^\dagger Y_e)^{ba}\left. \right\}C_{He}^{ab} + \left\{\frac{1}{8}\delta^{pa}g_L^4Y_d^{br} + g_Y^2g_L^2\left(21\delta^{pa}Y_d^{br} - \frac{43}{27}\delta^{ab}Y_d^{pr}\right) + g_Y^4\left(\frac{2135}{72}\delta^{pa}Y_d^{br} - \frac{1}{3}\delta^{ab}Y_d^{pr}\right) + g_s^2\left(\frac{68}{3}\delta^{pa}(Y_dY_d^\dagger Y_d)^{br} \right. \right. \\
& + 40Y_d^{pr}(Y_dY_d^\dagger)^{ba} - \frac{4}{3}Y_d^{br}(Y_dY_d^\dagger)^{pa} - 40Y_d^{pr}(Y_uY_u^\dagger)^{ba}) + g_Y^2\left(\frac{773}{216}\delta^{pa}(Y_dY_d^\dagger Y_d)^{br} + \frac{47}{12}Y_d^{pr}(Y_dY_d^\dagger)^{ba} + \frac{17}{3}Y_d^{br}(Y_uY_u^\dagger)^{pa} - \frac{1}{4}\delta^{pa}(Y_uY_u^\dagger Y_d)^{br} \right. \\
& - \frac{1073}{216}Y_d^{br}(Y_dY_d^\dagger)^{pa} - \frac{139}{12}Y_d^{pr}(Y_uY_u^\dagger)^{ba}) + \lambda\left(\frac{1}{2}\delta^{pa}(Y_uY_u^\dagger Y_d)^{br} + g_Y^2\left(\frac{26}{9}\delta^{ab}Y_d^{pr} - \frac{1799}{108}\delta^{pa}Y_d^{br}\right) + 2Y_d^{br}(Y_dY_d^\dagger)^{pa} + \frac{15}{4}\delta^{pa}g_L^2Y_d^{br} + \frac{16}{3}\delta^{pa}g_s^2Y_d^{br} \right. \\
& + 16Y_d^{pr}(Y_uY_u^\dagger)^{ba} - \frac{1}{2}Y_d^{br}(Y_uY_u^\dagger)^{pa} - 4T_2\delta^{pa}Y_d^{br} - 16Y_d^{pr}(Y_dY_d^\dagger)^{ba} - 16\delta^{pa}(Y_dY_d^\dagger Y_d)^{br}) + g_L^2\left(\frac{7}{12}Y_d^{pr}(Y_uY_u^\dagger)^{ba} + \frac{3}{2}\delta^{pa}(Y_uY_u^\dagger Y_d)^{br} \right. \\
& - \frac{7}{12}Y_d^{pr}(Y_dY_d^\dagger)^{ba} - \frac{11}{8}Y_d^{br}(Y_dY_d^\dagger)^{pa} - \frac{3}{2}Y_d^{br}(Y_uY_u^\dagger)^{pa} - \frac{27}{8}\delta^{pa}(Y_dY_d^\dagger Y_d)^{br}) + \frac{7}{4}Y_d^{br}(Y_uY_u^\dagger Y_uY_u^\dagger)^{pa} + 2\delta^{pa}(Y_uY_u^\dagger Y_uY_u^\dagger Y_d)^{br} \\
& + \frac{25}{12}(Y_dY_d^\dagger)^{pa}(Y_uY_u^\dagger Y_d)^{br} + \frac{5}{2}\delta^{pa}(Y_uY_u^\dagger Y_dY_d^\dagger Y_d)^{br} + 3(Y_uY_u^\dagger)^{ba}(Y_dY_d^\dagger Y_d)^{pr} + \frac{7}{2}\delta^{pa}(Y_dY_d^\dagger Y_uY_u^\dagger Y_d)^{br} + 30Y_d^{pr}(Y_uY_u^\dagger Y_uY_u^\dagger)^{ba} \\
& - \frac{3}{4}(Y_uY_u^\dagger)^{pa}(Y_dY_d^\dagger Y_d)^{br} - g_Y^2g_s^2\left(\frac{8}{3}\delta^{ab}Y_d^{pr} + \frac{44}{3}\delta^{pa}Y_d^{br}\right) - T_2\delta^{pa}(Y_dY_d^\dagger Y_d)^{br} - \frac{5}{4}(Y_uY_u^\dagger)^{pa}(Y_uY_u^\dagger Y_d)^{br} - \frac{25}{12}(Y_dY_d^\dagger)^{pa}(Y_dY_d^\dagger Y_d)^{br} \\
& - \frac{9}{4}Y_d^{br}(Y_uY_u^\dagger Y_dY_d^\dagger)^{pa} - 3(Y_dY_d^\dagger)^{ba}(Y_dY_d^\dagger Y_d)^{pr} - \frac{37}{12}Y_d^{br}(Y_dY_d^\dagger Y_dY_d^\dagger)^{pa} - 4T_4\delta^{pa}Y_d^{br} - \frac{71}{12}Y_d^{br}(Y_dY_d^\dagger Y_uY_u^\dagger)^{pa} - 12\delta^{pa}g_s^2g_L^2Y_d^{br} \\
& - 25\delta^{pa}(Y_dY_d^\dagger Y_dY_d^\dagger Y_d)^{br} - 30Y_d^{pr}(Y_dY_d^\dagger Y_dY_d^\dagger)^{ba}\left. \right\}C_{Hq}^{(\parallel)ab} + \left\{\frac{1}{4}Y_d^{br}(Y_uY_u^\dagger Y_dY_d^\dagger)^{pa} + \frac{1}{2}T_2\delta^{pa}(Y_dY_d^\dagger Y_d)^{br} + \frac{3}{4}(Y_uY_u^\dagger)^{pa}(Y_dY_d^\dagger Y_d)^{br} \right. \\
& + g_L^4\left(\frac{5}{8}\delta^{pa}Y_d^{br} - \frac{45}{4}\delta^{ab}Y_d^{pr}\right) + g_Y^2g_L^2\left(\frac{1129}{72}\delta^{pa}Y_d^{br} - \frac{23}{108}\delta^{ab}Y_d^{pr}\right) + g_Y^4\left(\frac{1079}{36}\delta^{pa}Y_d^{br} - \frac{1}{6}\delta^{ab}Y_d^{pr}\right) + \lambda\left(g_Y^2\left(\frac{13}{9}\delta^{ab}Y_d^{pr} - \frac{1381}{108}\delta^{pa}Y_d^{br}\right) + g_L^2\left(8\delta^{ab}Y_d^{pr} \right. \right. \\
& + \frac{185}{12}\delta^{pa}Y_d^{br}) + 2Y_d^{br}(Y_uY_u^\dagger)^{pa} + \frac{5}{2}Y_d^{br}(Y_dY_d^\dagger)^{pa} + \frac{32}{3}\delta^{pa}g_s^2Y_d^{br} - 8T_2\delta^{pa}Y_d^{br} - \frac{19}{2}\delta^{pa}(Y_uY_u^\dagger Y_d)^{br} - 11\delta^{pa}(Y_dY_d^\dagger Y_d)^{br} - 13Y_d^{pr}(Y_uY_u^\dagger)^{ba}
\end{aligned}$$

$$\begin{aligned}
& -29Y_d^{pr}(Y_dY_d^\dagger)^{ba}) + g_L^2 \left( \frac{37}{3}Y_d^{pr}(Y_dY_d^\dagger)^{ba} + \frac{155}{12}Y_d^{pr}(Y_uY_u^\dagger)^{ba} - \frac{1}{8}Y_d^{br}(Y_uY_u^\dagger)^{pa} - \frac{43}{24}\delta^{pa}(Y_uY_u^\dagger Y_d)^{br} - \frac{83}{12}\delta^{pa}(Y_dY_d^\dagger Y_d)^{br} - \frac{23}{3}Y_d^{br}(Y_dY_d^\dagger)^{pa} \right) \\
& + g_Y^2 \left( \frac{1}{8}\delta^{pa}(Y_uY_u^\dagger Y_d)^{br} + \frac{5}{4}Y_d^{pr}(Y_uY_u^\dagger)^{ba} + \frac{227}{108}\delta^{pa}(Y_dY_d^\dagger Y_d)^{br} + \frac{9}{2}Y_d^{pr}(Y_dY_d^\dagger)^{ba} - \frac{35}{24}Y_d^{br}(Y_uY_u^\dagger)^{pa} - \frac{115}{54}Y_d^{br}(Y_dY_d^\dagger)^{pa} \right) + g_s^2 \left( 8Y_d^{br}(Y_uY_u^\dagger)^{pa} \right. \\
& + \frac{64}{3}\delta^{pa}(Y_dY_d^\dagger Y_d)^{br} + 24\delta^{pa}(Y_uY_u^\dagger Y_d)^{br} + 40Y_d^{pr}(Y_dY_d^\dagger)^{ba} - \frac{32}{3}Y_d^{br}(Y_dY_d^\dagger)^{pa} \left. \right) + \frac{3}{2}(Y_dY_d^\dagger)^{ba}(Y_dY_d^\dagger Y_d)^{pr} + \frac{7}{4}\delta^{pa}(Y_uY_u^\dagger Y_dY_d^\dagger Y_d)^{br} \\
& + \frac{9}{2}(Y_uY_u^\dagger)^{ba}(Y_dY_d^\dagger Y_d)^{pr} + \frac{14}{3}Y_d^{br}(Y_dY_d^\dagger Y_uY_u^\dagger)^{pa} + \frac{11}{2}\delta^{pa}(Y_dY_d^\dagger Y_uY_u^\dagger Y_d)^{br} + 6Y_d^{pr}(Y_uY_u^\dagger Y_uY_u^\dagger)^{ba} - g_Y^2 g_s^2 \left( \frac{4}{3}\delta^{ab}Y_d^{pr} + \frac{44}{3}\delta^{pa}Y_d^{br} \right) \\
& - g_s^2 g_L^2 \left( 4\delta^{ab}Y_d^{pr} + 24\delta^{pa}Y_d^{br} \right) - \frac{13}{12}(Y_dY_d^\dagger)^{pa}(Y_uY_u^\dagger Y_d)^{br} - \frac{7}{4}(Y_uY_u^\dagger)^{pa}(Y_uY_u^\dagger Y_d)^{br} - \frac{5}{2}T_2\delta^{pa}(Y_uY_u^\dagger Y_d)^{br} - \frac{35}{12}(Y_dY_d^\dagger)^{pa}(Y_dY_d^\dagger Y_d)^{br} \\
& - 4T_4\delta^{pa}Y_d^{br} - 4Y_d^{br}(Y_uY_u^\dagger Y_uY_u^\dagger)^{pa} - \frac{53}{12}Y_d^{br}(Y_dY_d^\dagger Y_dY_d^\dagger)^{pa} - \frac{9}{2}Y_d^{pr}(Y_dY_d^\dagger Y_uY_u^\dagger)^{ba} - \frac{9}{2}Y_d^{pr}(Y_uY_u^\dagger Y_dY_d^\dagger)^{ba} - \frac{15}{2}(Y_dY_d^\dagger)^{ba}(Y_uY_u^\dagger Y_d)^{pr} \\
& - \frac{15}{2}(Y_uY_u^\dagger)^{ba}(Y_uY_u^\dagger Y_d)^{pr} - 9\delta^{pa}(Y_uY_u^\dagger Y_uY_u^\dagger Y_d)^{br} - \frac{81}{4}\delta^{pa}(Y_dY_d^\dagger Y_dY_d^\dagger Y_d)^{br} - 24Y_d^{pr}(Y_dY_d^\dagger Y_dY_d^\dagger)^{ba} - 24\delta^{pa}Y_d^{br} \text{Tr}[Y_d^\dagger Y_d Y_u^\dagger Y_u] \left. \right\} C_{Hq}^{(\times)ab} \\
& + \left\{ \lambda \left( \frac{52}{9}\delta^{ab}g_Y^2 Y_d^{pr} - 16Y_d^{pr}(Y_u^\dagger Y_u)^{ba} \right) + g_Y^2 \left( \frac{59}{12}Y_d^{pr}(Y_u^\dagger Y_u)^{ba} - \frac{1}{6}Y_u^{pa}(Y_u^\dagger Y_d)^{br} \right) + g_L^2 \left( \frac{77}{12}Y_d^{pr}(Y_u^\dagger Y_u)^{ba} - \frac{17}{4}Y_u^{pa}(Y_u^\dagger Y_d)^{br} \right) + \frac{7}{4}(Y_u^\dagger Y_d)^{br}(Y_dY_d^\dagger Y_u)^{pa} \right. \\
& + 3Y_d^{pr}(Y_u^\dagger Y_dY_d^\dagger Y_u)^{ba} + \frac{19}{4}Y_u^{pa}(Y_u^\dagger Y_uY_u^\dagger Y_d)^{br} + 40g_s^2 Y_d^{pr}(Y_u^\dagger Y_u)^{ba} - \frac{5}{27}\delta^{ab}g_Y^2 g_L^2 Y_d^{pr} - \frac{1}{4}Y_u^{pa}(Y_u^\dagger Y_dY_d^\dagger Y_d)^{br} - \frac{7}{4}(Y_u^\dagger Y_d)^{br}(Y_uY_u^\dagger Y_u)^{pa} \\
& - \frac{7}{3}\delta^{ab}g_Y^4 Y_d^{pr} - 3(Y_u^\dagger Y_u)^{ba}(Y_dY_d^\dagger Y_d)^{pr} - \frac{16}{3}\delta^{ab}g_Y^2 g_s^2 Y_d^{pr} - 30Y_d^{pr}(Y_u^\dagger Y_uY_u^\dagger Y_u)^{ba} \left. \right\} C_{Hu}^{ab} + \left\{ \frac{1}{4}(Y_d^\dagger Y_d)^{br}(Y_uY_u^\dagger Y_d)^{pa} + g_Y^2 g_L^2 \left( \frac{5}{54}\delta^{ab}Y_d^{pr} \right. \right. \\
& - \frac{265}{12}\delta^{rb}Y_d^{pa} \left. \right) + g_Y^4 \left( \frac{1}{2}\delta^{ab}Y_d^{pr} - \frac{785}{36}\delta^{rb}Y_d^{pa} \right) + g_Y^2 g_s^2 \left( \frac{8}{3}\delta^{ab}Y_d^{pr} + \frac{40}{3}\delta^{rb}Y_d^{pa} \right) + T_2\delta^{rb}(Y_dY_d^\dagger Y_d)^{pa} + g_s^2 \left( \frac{4}{3}Y_d^{pa}(Y_d^\dagger Y_d)^{br} - \frac{68}{3}\delta^{rb}(Y_dY_d^\dagger Y_d)^{pa} \right. \\
& - 40Y_d^{pr}(Y_d^\dagger Y_d)^{ba} \left. \right) + \lambda \left( g_Y^2 \left( \frac{1099}{108}\delta^{rb}Y_d^{pa} - \frac{26}{9}\delta^{ab}Y_d^{pr} \right) + 4T_2\delta^{rb}Y_d^{pa} + \frac{25}{2}\delta^{rb}(Y_dY_d^\dagger Y_d)^{pa} + \frac{57}{4}\delta^{rb}g_L^2 Y_d^{pa} + 16Y_d^{pr}(Y_d^\dagger Y_d)^{ba} - \frac{5}{2}Y_d^{pa}(Y_d^\dagger Y_d)^{br} \right. \\
& - 4\delta^{rb}(Y_uY_u^\dagger Y_d)^{pa} - \frac{16}{3}\delta^{rb}g_s^2 Y_d^{pa} \left. \right) + g_Y^2 \left( \delta^{rb}(Y_uY_u^\dagger Y_d)^{pa} + \frac{221}{216}\delta^{rb}(Y_dY_d^\dagger Y_d)^{pa} + \frac{601}{216}Y_d^{pa}(Y_d^\dagger Y_d)^{br} - \frac{31}{12}Y_d^{pr}(Y_d^\dagger Y_d)^{ba} \right) + g_L^2 \left( \frac{17}{8}Y_d^{pa}(Y_d^\dagger Y_d)^{br} \right. \\
& + 11\delta^{rb}(Y_uY_u^\dagger Y_d)^{pa} - \frac{77}{12}Y_d^{pr}(Y_d^\dagger Y_d)^{ba} - \frac{129}{8}\delta^{rb}(Y_dY_d^\dagger Y_d)^{pa} \left. \right) + \frac{29}{12}(Y_d^\dagger Y_d)^{br}(Y_dY_d^\dagger Y_d)^{pa} + 3(Y_d^\dagger Y_d)^{ba}(Y_dY_d^\dagger Y_d)^{pr} + 4T_4\delta^{rb}Y_d^{pa} \\
& + \frac{59}{12}Y_d^{pa}(Y_d^\dagger Y_dY_d^\dagger Y_d)^{br} + 16\delta^{rb}g_s^2 g_L^2 Y_d^{pa} + \frac{39}{2}\delta^{rb}(Y_dY_d^\dagger Y_dY_d^\dagger Y_d)^{pa} + 30Y_d^{pr}(Y_d^\dagger Y_dY_d^\dagger Y_d)^{ba} - \frac{5}{6}\delta^{rb}g_L^4 Y_d^{pa} - \frac{5}{4}Y_d^{pa}(Y_d^\dagger Y_uY_u^\dagger Y_d)^{br} \\
& - \frac{5}{2}\delta^{rb}(Y_dY_d^\dagger Y_uY_u^\dagger Y_d)^{pa} - 3Y_d^{pr}(Y_d^\dagger Y_uY_u^\dagger Y_d)^{ba} - 4\delta^{rb}(Y_uY_u^\dagger Y_dY_d^\dagger Y_d)^{pa} - 4\delta^{rb}(Y_uY_u^\dagger Y_uY_u^\dagger Y_d)^{pa} \left. \right\} C_{Hd}^{ab} + \left\{ g_s^2 \left( \frac{32}{3}Y_u^{pa}(Y_d^\dagger Y_d)^{br} \right. \right. \\
& - \frac{4}{3}\delta^{rb}(Y_dY_d^\dagger Y_u)^{pa} - \frac{64}{3}\delta^{rb}(Y_uY_u^\dagger Y_u)^{pa} \left. \right) + g_L^2 \left( \frac{51}{8}Y_u^{pa}(Y_d^\dagger Y_d)^{br} + \frac{103}{8}\delta^{rb}(Y_dY_d^\dagger Y_u)^{pa} - 18\delta^{rb}(Y_uY_u^\dagger Y_u)^{pa} - \frac{221}{12}Y_d^{pr}(Y_d^\dagger Y_u)^{ba} \right) \\
& + g_Y^2 \left( \frac{121}{72}\delta^{rb}(Y_dY_d^\dagger Y_u)^{pa} - \frac{11}{72}Y_u^{pa}(Y_d^\dagger Y_d)^{br} - \frac{17}{12}Y_d^{pr}(Y_d^\dagger Y_u)^{ba} - \frac{28}{9}\delta^{rb}(Y_uY_u^\dagger Y_u)^{pa} \right) + \lambda \left( 4T_2\delta^{rb}Y_u^{pa} + 10Y_d^{pr}(Y_d^\dagger Y_u)^{ba} + 11\delta^{rb}(Y_uY_u^\dagger Y_u)^{pa} \right.
\end{aligned}$$



$$\begin{aligned}
& + \frac{57}{4} \delta^{rb} g_L^2 Y_u^{pa} - \frac{1}{2} Y_u^{pa} (Y_d^\dagger Y_d)^{br} - \frac{5}{2} \delta^{rb} (Y_d Y_d^\dagger Y_u)^{pa} - \frac{187}{36} \delta^{rb} g_Y^2 Y_u^{pa} - \frac{16}{3} \delta^{rb} g_s^2 Y_u^{pa} + \frac{3}{2} Y_d^{pr} (Y_d^\dagger Y_d Y_d^\dagger Y_u)^{ba} + \frac{3}{2} Y_d^{pr} (Y_d^\dagger Y_u Y_u^\dagger Y_u)^{ba} \\
& + \frac{7}{4} (Y_d^\dagger Y_d)^{br} (Y_u Y_u^\dagger Y_u)^{pa} + 2 T_2 \delta^{rb} (Y_u Y_u^\dagger Y_u)^{pa} + \frac{49}{12} \delta^{rb} g_Y^2 g_L^2 Y_u^{pa} + \frac{9}{2} (Y_d^\dagger Y_u)^{ba} (Y_u Y_u^\dagger Y_d)^{pr} + 11 \delta^{rb} (Y_u Y_u^\dagger Y_u Y_u^\dagger Y_u)^{pa} + 16 \delta^{rb} g_s^2 g_L^2 Y_u^{pa} \\
& + 24 \delta^{rb} Y_u^{pa} \text{Tr} [Y_d^\dagger Y_d Y_u^\dagger Y_u] - \frac{1}{12} (Y_d^\dagger Y_d)^{br} (Y_d Y_d^\dagger Y_u)^{pa} - \frac{1}{4} Y_u^{pa} (Y_d^\dagger Y_d Y_d^\dagger Y_d)^{br} - \frac{3}{4} Y_u^{pa} (Y_d^\dagger Y_u Y_u^\dagger Y_d)^{br} - \frac{5}{6} \delta^{rb} g_L^4 Y_u^{pa} - T_2 \delta^{rb} (Y_d Y_d^\dagger Y_u)^{pa} \\
& - \delta^{rb} (Y_d Y_d^\dagger Y_d Y_d^\dagger Y_u)^{pa} - \delta^{rb} (Y_u Y_u^\dagger Y_d Y_d^\dagger Y_u)^{pa} - \frac{3}{2} (Y_d^\dagger Y_u)^{ba} (Y_d Y_d^\dagger Y_d)^{pr} - \frac{13}{4} \delta^{rb} g_Y^4 Y_u^{pa} \Big\} C_{Hud}^{ab} + C_{Hud}^{*ab} \Big\{ \frac{1}{4} (Y_u^\dagger Y_d)^{ar} (Y_d Y_d^\dagger Y_d)^{pb} \\
& + \frac{3}{4} (Y_u^\dagger Y_d)^{ar} (Y_u Y_u^\dagger Y_d)^{pb} + g_Y^2 \left( \frac{7}{18} Y_d^{pb} (Y_u^\dagger Y_d)^{ar} - \frac{17}{12} Y_d^{pr} (Y_u^\dagger Y_d)^{ab} \right) + \lambda \left( 16 Y_d^{pr} (Y_u^\dagger Y_d)^{ab} - 2 Y_d^{pb} (Y_u^\dagger Y_d)^{ar} \right) + \frac{7}{4} Y_d^{pb} (Y_u^\dagger Y_u Y_u^\dagger Y_d)^{ar} \\
& + \frac{21}{2} (Y_u^\dagger Y_d)^{ab} (Y_u Y_u^\dagger Y_d)^{pr} - \frac{3}{2} Y_d^{pr} (Y_u^\dagger Y_d Y_d^\dagger Y_d)^{ab} - \frac{3}{2} Y_d^{pr} (Y_u^\dagger Y_u Y_u^\dagger Y_d)^{ab} - \frac{19}{12} Y_d^{pb} (Y_u^\dagger Y_d Y_d^\dagger Y_d)^{ar} - \frac{15}{2} (Y_u^\dagger Y_d)^{ab} (Y_d Y_d^\dagger Y_d)^{pr} - \frac{28}{3} g_s^2 Y_d^{pb} (Y_u^\dagger Y_d)^{ar} \\
& - \frac{257}{12} g_L^2 Y_d^{pr} (Y_u^\dagger Y_d)^{ab} \Big\} + \Big\{ 8 Y_e^{*ad} Y_d^{pr} (Y_e Y_e^\dagger Y_e)^{bc} - 4 \lambda Y_e^{*ad} Y_d^{pr} Y_e^{bc} \Big\} C_{\ell e}^{abcd} + \Big\{ \frac{7}{9} \delta^{rd} \delta^{ab} g_Y^4 Y_d^{pc} + \lambda \left( \delta^{rd} Y_d^{pc} (Y_e Y_e^\dagger)^{ba} - \frac{35}{27} \delta^{rd} \delta^{ab} g_Y^2 Y_d^{pc} \right) \\
& + g_Y^2 \left( \frac{47}{54} \delta^{rd} \delta^{ab} (Y_d Y_d^\dagger Y_d)^{pc} + \frac{14}{3} \delta^{rd} Y_d^{pc} (Y_e Y_e^\dagger)^{ba} - \frac{5}{54} \delta^{ab} Y_d^{pc} (Y_d^\dagger Y_d)^{dr} \right) + \frac{4}{3} \delta^{rd} \delta^{ab} g_Y^2 g_L^2 Y_d^{pc} - \frac{1}{2} Y_d^{pc} (Y_d^\dagger Y_d)^{dr} (Y_e Y_e^\dagger)^{ba} - \frac{1}{2} \delta^{rd} (Y_e Y_e^\dagger)^{ba} (Y_d Y_d^\dagger Y_d)^{pc} \\
& - \delta^{rd} g_L^2 Y_d^{pc} (Y_e Y_e^\dagger)^{ba} - 10 \delta^{rd} Y_d^{pc} (Y_e Y_e^\dagger Y_e Y_e^\dagger)^{ba} \Big\} C_{\ell d}^{abcd} + \Big\{ \lambda \left( \delta^{pa} Y_d^{br} (Y_e^\dagger Y_e)^{dc} + \frac{49}{27} \delta^{pa} \delta^{cd} g_Y^2 Y_d^{br} \right) + g_Y^2 \left( \frac{25}{54} \delta^{cd} Y_d^{br} (Y_d Y_d^\dagger)^{pa} - \frac{91}{54} \delta^{pa} \delta^{cd} (Y_d Y_d^\dagger Y_d)^{br} \right. \\
& - \frac{25}{6} \delta^{pa} Y_d^{br} (Y_e^\dagger Y_e)^{dc} \Big) + \frac{3}{2} \delta^{pa} g_L^2 Y_d^{br} (Y_e^\dagger Y_e)^{dc} - \frac{1}{2} \delta^{pa} \delta^{cd} g_Y^2 g_L^2 Y_d^{br} - \frac{1}{2} Y_d^{br} (Y_e^\dagger Y_e)^{dc} (Y_d Y_d^\dagger)^{pa} - \frac{1}{2} \delta^{pa} (Y_e^\dagger Y_e)^{dc} (Y_d Y_d^\dagger Y_d)^{br} - \frac{19}{18} \delta^{pa} \delta^{cd} g_Y^4 Y_d^{br} \\
& - 10 \delta^{pa} Y_d^{br} (Y_e^\dagger Y_e Y_e^\dagger Y_e)^{dc} \Big\} C_{qe}^{abcd} + \Big\{ \frac{2}{3} Y_u^{bc} (Y_u^\dagger Y_d)^{dr} (Y_d Y_d^\dagger)^{pa} + \delta^{pa} \delta^{cd} g_Y^2 g_L^2 Y_d^{br} + \lambda \left( \frac{5}{2} Y_u^{*ad} Y_d^{br} Y_u^{pc} + 6 \delta^{pa} Y_d^{br} (Y_u^\dagger Y_u)^{dc} - 2 \delta^{pa} Y_u^{bc} (Y_u^\dagger Y_d)^{dr} \right. \\
& - \frac{98}{27} \delta^{pa} \delta^{cd} g_Y^2 Y_d^{br} - 12 Y_u^{*ad} Y_d^{pr} Y_u^{bc} \Big) + g_Y^2 \left( \frac{91}{27} \delta^{pa} \delta^{cd} (Y_d Y_d^\dagger Y_d)^{br} + \frac{9}{2} \delta^{pa} Y_d^{br} (Y_u^\dagger Y_u)^{dc} - \frac{25}{27} \delta^{cd} Y_d^{br} (Y_d Y_d^\dagger)^{pa} \right) + Y_u^{*ad} Y_d^{br} (Y_u Y_u^\dagger Y_u)^{pc} \\
& + \delta^{pa} Y_u^{bc} (Y_u^\dagger Y_d Y_d^\dagger Y_d)^{dr} + \frac{3}{2} Y_d^{br} (Y_u^\dagger Y_u)^{dc} (Y_d Y_d^\dagger)^{pa} + \frac{3}{2} \delta^{pa} (Y_u^\dagger Y_u)^{dc} (Y_d Y_d^\dagger Y_d)^{br} + \frac{19}{9} \delta^{pa} \delta^{cd} g_Y^4 Y_d^{br} + 12 \delta^{pa} Y_d^{br} (Y_u^\dagger Y_u Y_u^\dagger Y_u)^{dc} \\
& + 24 Y_d^{pr} Y_u^{bc} (Y_u^\dagger Y_u Y_u^\dagger)^{ad} - \frac{1}{3} Y_u^{*ad} Y_d^{br} (Y_d Y_d^\dagger Y_u)^{pc} - g_L^2 \left( \frac{3}{2} Y_u^{*ad} Y_d^{br} Y_u^{pc} + \frac{9}{2} \delta^{pa} Y_d^{br} (Y_u^\dagger Y_u)^{dc} \right) - \delta^{pa} Y_u^{bc} (Y_u^\dagger Y_u Y_u^\dagger Y_d)^{dr} - 2 \delta^{pa} (Y_u^\dagger Y_d)^{dr} (Y_u Y_u^\dagger Y_u)^{bc} \\
& - 3 Y_d^{br} Y_u^{pc} (Y_u^\dagger Y_u Y_u^\dagger)^{ad} - 4 \delta^{pa} (Y_u^\dagger Y_d)^{dr} (Y_d Y_d^\dagger Y_u)^{bc} \Big\} C_{qu}^{(III)abcd} + \Big\{ \frac{1}{3} \delta^{pa} \delta^{cd} g_Y^2 g_L^2 Y_d^{br} + \frac{1}{2} Y_d^{br} (Y_u^\dagger Y_u)^{dc} (Y_d Y_d^\dagger)^{pa} + \frac{1}{2} \delta^{pa} (Y_u^\dagger Y_u)^{dc} (Y_d Y_d^\dagger Y_d)^{br} \\
& + \frac{19}{27} \delta^{pa} \delta^{cd} g_Y^4 Y_d^{br} + \lambda \left( 2 \delta^{pa} Y_d^{br} (Y_u^\dagger Y_u)^{dc} + \frac{112}{27} \delta^{pa} \delta^{cd} g_s^2 Y_d^{br} + \frac{15}{2} Y_u^{*ad} Y_d^{br} Y_u^{pc} - \frac{98}{81} \delta^{pa} \delta^{cd} g_Y^2 Y_d^{br} - 6 \delta^{pa} Y_u^{bc} (Y_u^\dagger Y_d)^{dr} - 36 Y_u^{*ad} Y_d^{pr} Y_u^{bc} \right) \\
& + g_s^2 \left( \frac{80}{27} \delta^{cd} Y_d^{br} (Y_d Y_d^\dagger)^{pa} - \frac{176}{27} \delta^{pa} \delta^{cd} (Y_d Y_d^\dagger Y_d)^{br} - 32 \delta^{pa} Y_d^{br} (Y_u^\dagger Y_u)^{dc} \right) + g_Y^2 \left( \frac{91}{81} \delta^{pa} \delta^{cd} (Y_d Y_d^\dagger Y_d)^{br} + \frac{3}{2} \delta^{pa} Y_d^{br} (Y_u^\dagger Y_u)^{dc} - \frac{25}{81} \delta^{cd} Y_d^{br} (Y_d Y_d^\dagger)^{pa} \right) \\
& + 2 Y_u^{bc} (Y_u^\dagger Y_d)^{dr} (Y_d Y_d^\dagger)^{pa} + 3 Y_u^{*ad} Y_d^{br} (Y_u Y_u^\dagger Y_u)^{pc} + 3 \delta^{pa} Y_u^{bc} (Y_u^\dagger Y_d Y_d^\dagger Y_d)^{dr} + 4 \delta^{pa} Y_d^{br} (Y_u^\dagger Y_u Y_u^\dagger Y_u)^{dc} + 72 Y_d^{pr} Y_u^{bc} (Y_u^\dagger Y_u Y_u^\dagger)^{ad}
\end{aligned}$$

$$\begin{aligned}
& -g_L^2 \left( \frac{3}{2} \delta^{pa} Y_d^{br} (Y_u^\dagger Y_u)^{dc} + \frac{9}{2} Y_u^{*ad} Y_d^{br} Y_u^{pc} \right) - Y_u^{*ad} Y_d^{br} (Y_d Y_d^\dagger Y_u)^{pc} - 3\delta^{pa} Y_u^{bc} (Y_u^\dagger Y_u Y_u^\dagger Y_d)^{dr} - 6\delta^{pa} (Y_u^\dagger Y_d)^{dr} (Y_u Y_u^\dagger Y_u)^{bc} - 9Y_d^{br} Y_u^{pc} (Y_u^\dagger Y_u Y_u^\dagger)^{ad} \\
& - 12\delta^{pa} (Y_u^\dagger Y_d)^{dr} (Y_d Y_d^\dagger Y_u)^{bc} \Big\} C_{qu}^{(\times)abcd} + \left\{ \frac{1}{3} Y_d^{*ad} Y_d^{pc} (Y_d Y_d^\dagger Y_d)^{br} + \frac{2}{3} Y_d^{*ad} Y_d^{br} (Y_d Y_d^\dagger Y_d)^{pc} + Y_d^{bc} (Y_d^\dagger Y_d)^{dr} (Y_u Y_u^\dagger)^{pa} + g_L^2 \left( \frac{3}{2} \delta^{pa} Y_d^{bc} (Y_d^\dagger Y_d)^{dr} \right. \right. \\
& + 3\delta^{rd} Y_d^{pc} (Y_u Y_u^\dagger)^{ba} + \frac{9}{2} \delta^{pa} Y_d^{br} (Y_d^\dagger Y_d)^{dc} - \frac{3}{2} Y_d^{*ad} Y_d^{pc} Y_d^{br} - 3\delta^{rd} Y_d^{pc} (Y_d Y_d^\dagger)^{ba} - 3\delta^{rd} Y_d^{bc} (Y_u Y_u^\dagger)^{pa} - 9\delta^{pa} \delta^{rd} (Y_d Y_d^\dagger Y_d)^{bc} \Big) + g_Y^2 \left( \frac{5}{54} \delta^{ab} Y_d^{pc} (Y_d^\dagger Y_d)^{dr} \right. \\
& + \frac{1}{6} \delta^{pa} Y_d^{bc} (Y_d^\dagger Y_d)^{dr} + \frac{25}{54} \delta^{cd} Y_d^{br} (Y_d Y_d^\dagger)^{pa} + \frac{2}{3} \delta^{rd} Y_d^{bc} (Y_d Y_d^\dagger)^{pa} + \frac{7}{2} \delta^{pa} Y_d^{br} (Y_d^\dagger Y_d)^{dc} + 6\delta^{rd} Y_d^{pc} (Y_d Y_d^\dagger)^{ba} - \frac{47}{54} \delta^{rd} \delta^{ab} (Y_d Y_d^\dagger Y_d)^{pc} - Y_d^{*ad} Y_d^{pc} Y_d^{br} \\
& - \frac{91}{54} \delta^{pa} \delta^{cd} (Y_d Y_d^\dagger Y_d)^{br} - \frac{43}{9} \delta^{pa} \delta^{rd} (Y_d Y_d^\dagger Y_d)^{bc} - 10\delta^{rd} Y_d^{pc} (Y_u Y_u^\dagger)^{ba} \Big) + g_s^2 \left( \frac{128}{3} \delta^{pa} \delta^{rd} (Y_d Y_d^\dagger Y_d)^{bc} - 16\delta^{pa} Y_d^{bc} (Y_d^\dagger Y_d)^{dr} - 16\delta^{rd} Y_d^{bc} (Y_d Y_d^\dagger)^{pa} \right) \\
& + Y_d^{*ad} Y_d^{pc} (Y_u Y_u^\dagger Y_d)^{br} + \delta^{pa} Y_d^{bc} (Y_d^\dagger Y_d Y_d^\dagger Y_d)^{dr} + \delta^{rd} Y_d^{bc} (Y_d Y_d^\dagger Y_d Y_d^\dagger)^{pa} + \lambda \left( g_Y^2 \left( \frac{35}{27} \delta^{rd} \delta^{ab} Y_d^{pc} + \frac{49}{27} \delta^{pa} \delta^{cd} Y_d^{br} - \frac{1}{18} \delta^{pa} \delta^{rd} Y_d^{bc} \right) + 2\delta^{pa} Y_d^{bc} (Y_d^\dagger Y_d)^{dr} \right. \\
& + 2\delta^{rd} Y_d^{bc} (Y_d Y_d^\dagger)^{pa} + \frac{9}{2} \delta^{pa} \delta^{rd} (Y_u Y_u^\dagger Y_d)^{bc} + 6\delta^{pa} Y_d^{br} (Y_d^\dagger Y_d)^{dc} + 6\delta^{rd} Y_d^{pc} (Y_d Y_d^\dagger)^{ba} + 6\delta^{rd} Y_d^{pc} (Y_u Y_u^\dagger)^{ba} + 6\delta^{pa} \delta^{rd} Y_d^{bc} \text{Tr} \left[ Y_d^\dagger Y_d \right] + 10Y_d^{*ad} Y_d^{pc} Y_d^{br} \\
& + 28\delta^{pa} \delta^{rd} (Y_d Y_d^\dagger Y_d)^{bc} - \frac{3}{2} \delta^{pa} \delta^{rd} g_L^2 Y_d^{bc} - 2\delta^{rd} Y_d^{bc} (Y_u Y_u^\dagger)^{pa} - 6Y_d^{*ad} Y_d^{pr} Y_d^{bc} - \frac{32}{3} \delta^{pa} \delta^{rd} g_s^2 Y_d^{bc} \Big) + \frac{3}{2} \delta^{pa} \delta^{rd} g_L^4 Y_d^{bc} + \frac{3}{2} Y_d^{pc} (Y_d^\dagger Y_d)^{dr} (Y_u Y_u^\dagger)^{ba} \\
& + \frac{3}{2} \delta^{rd} (Y_u Y_u^\dagger)^{ba} (Y_d Y_d^\dagger Y_d)^{pc} + 2\delta^{rd} (Y_d Y_d^\dagger)^{pa} (Y_d Y_d^\dagger Y_d)^{bc} + 2\delta^{rd} Y_d^{bc} (Y_d Y_d^\dagger Y_u Y_u^\dagger)^{pa} + 3\delta^{pa} \delta^{rd} (Y_u Y_u^\dagger Y_u Y_u^\dagger Y_d)^{bc} + 4\delta^{rd} (Y_d Y_d^\dagger)^{pa} (Y_u Y_u^\dagger Y_d)^{bc} \\
& + 6\delta^{pa} \delta^{rd} (Y_u Y_u^\dagger Y_d Y_d^\dagger Y_d)^{bc} + 10\delta^{pa} \delta^{rd} (Y_d Y_d^\dagger Y_u Y_u^\dagger Y_d)^{bc} + 12Y_d^{*ad} Y_d^{pr} (Y_d Y_d^\dagger Y_d)^{bc} + 12\delta^{rd} Y_d^{pc} (Y_u Y_u^\dagger Y_u Y_u^\dagger)^{ba} - g_Y^2 g_L^2 \left( \frac{1}{2} \delta^{pa} \delta^{cd} Y_d^{br} \right. \\
& + \delta^{pa} \delta^{rd} Y_d^{bc} + \frac{4}{3} \delta^{rd} \delta^{ab} Y_d^{pc} \Big) - g_Y^4 \left( \frac{1}{6} \delta^{pa} \delta^{rd} Y_d^{bc} + \frac{7}{9} \delta^{rd} \delta^{ab} Y_d^{pc} + \frac{19}{18} \delta^{pa} \delta^{cd} Y_d^{br} \right) - Y_d^{bc} (Y_d^\dagger Y_d)^{dr} (Y_d Y_d^\dagger)^{pa} - \frac{3}{2} Y_d^{br} (Y_d^\dagger Y_d)^{dc} (Y_d Y_d^\dagger)^{pa} \\
& - \frac{3}{2} Y_d^{pc} (Y_d^\dagger Y_d)^{dr} (Y_d Y_d^\dagger)^{ba} - \frac{3}{2} \delta^{rd} (Y_d Y_d^\dagger)^{ba} (Y_d Y_d^\dagger Y_d)^{pc} - \frac{3}{2} \delta^{pa} (Y_d^\dagger Y_d)^{dc} (Y_d Y_d^\dagger Y_d)^{br} - 2\delta^{rd} Y_d^{bc} (Y_u Y_u^\dagger Y_u Y_u^\dagger)^{pa} - 4\delta^{rd} (Y_u Y_u^\dagger)^{pa} (Y_d Y_d^\dagger Y_d)^{bc} \\
& - 8\delta^{rd} (Y_u Y_u^\dagger)^{pa} (Y_u Y_u^\dagger Y_d)^{bc} - 10Y_d^{pc} Y_d^{br} (Y_d^\dagger Y_d Y_d^\dagger)^{ad} - 12\delta^{pa} \delta^{rd} Y_d^{bc} \text{Tr} \left[ Y_d^\dagger Y_d Y_d^\dagger Y_d \right] - 36\delta^{pa} Y_d^{br} (Y_d^\dagger Y_d Y_d^\dagger Y_d)^{dc} - 36\delta^{rd} Y_d^{pc} (Y_d Y_d^\dagger Y_d Y_d^\dagger)^{ba} \\
& - 52\delta^{pa} \delta^{rd} (Y_d Y_d^\dagger Y_d Y_d^\dagger Y_d)^{bc} \Big\} C_{qd}^{(\parallel)abcd} + \left\{ \frac{1}{2} Y_d^{pc} (Y_d^\dagger Y_d)^{dr} (Y_u Y_u^\dagger)^{ba} + \frac{1}{2} \delta^{rd} (Y_u Y_u^\dagger)^{ba} (Y_d Y_d^\dagger Y_d)^{pc} + Y_d^{*ad} Y_d^{pc} (Y_d Y_d^\dagger Y_d)^{br} + g_L^2 \left( \delta^{rd} Y_d^{pc} (Y_u Y_u^\dagger)^{ba} \right. \right. \\
& + \frac{3}{2} \delta^{pa} Y_d^{br} (Y_d^\dagger Y_d)^{dc} + \frac{9}{2} \delta^{pa} Y_d^{bc} (Y_d^\dagger Y_d)^{dr} - \delta^{rd} Y_d^{pc} (Y_d Y_d^\dagger)^{ba} - \frac{9}{2} Y_d^{*ad} Y_d^{pc} Y_d^{br} - 9\delta^{rd} Y_d^{bc} (Y_u Y_u^\dagger)^{pa} - 27\delta^{pa} \delta^{rd} (Y_d Y_d^\dagger Y_d)^{bc} \Big) + g_Y^2 \left( \frac{5}{162} \delta^{ab} Y_d^{pc} (Y_d^\dagger Y_d)^{dr} \right. \\
& + \frac{25}{162} \delta^{cd} Y_d^{br} (Y_d Y_d^\dagger)^{pa} + \frac{1}{2} \delta^{pa} Y_d^{bc} (Y_d^\dagger Y_d)^{dr} + \frac{7}{6} \delta^{pa} Y_d^{br} (Y_d^\dagger Y_d)^{dc} + 2\delta^{rd} Y_d^{bc} (Y_d Y_d^\dagger)^{pa} + 2\delta^{rd} Y_d^{pc} (Y_d Y_d^\dagger)^{ba} - \frac{47}{162} \delta^{rd} \delta^{ab} (Y_d Y_d^\dagger Y_d)^{pc} \\
& - \frac{91}{162} \delta^{pa} \delta^{cd} (Y_d Y_d^\dagger Y_d)^{br} - 3Y_d^{*ad} Y_d^{pc} Y_d^{br} - \frac{10}{3} \delta^{rd} Y_d^{pc} (Y_u Y_u^\dagger)^{ba} - \frac{43}{3} \delta^{pa} \delta^{rd} (Y_d Y_d^\dagger Y_d)^{bc} \Big) + g_s^2 \left( \frac{80}{27} \delta^{cd} Y_d^{br} (Y_d Y_d^\dagger)^{pa} + \frac{160}{27} \delta^{ab} Y_d^{pc} (Y_d^\dagger Y_d)^{dr} \right. \\
& + 320\delta^{pa} \delta^{rd} (Y_d Y_d^\dagger Y_d)^{bc} - \frac{176}{27} \delta^{pa} \delta^{cd} (Y_d Y_d^\dagger Y_d)^{br} - \frac{352}{27} \delta^{rd} \delta^{ab} (Y_d Y_d^\dagger Y_d)^{pc} - 32\delta^{pa} Y_d^{br} (Y_d^\dagger Y_d)^{dc} - 32\delta^{rd} Y_d^{pc} (Y_d Y_d^\dagger)^{ba} - 32\delta^{rd} Y_d^{pc} (Y_u Y_u^\dagger)^{ba} \Big) \\
& + \lambda \left( g_Y^2 \left( \frac{35}{81} \delta^{rd} \delta^{ab} Y_d^{pc} + \frac{49}{81} \delta^{pa} \delta^{cd} Y_d^{br} - \frac{1}{6} \delta^{pa} \delta^{rd} Y_d^{bc} \right) + g_s^2 \left( \frac{112}{27} \delta^{pa} \delta^{cd} Y_d^{br} + \frac{224}{27} \delta^{rd} \delta^{ab} Y_d^{pc} - 128\delta^{pa} \delta^{rd} Y_d^{bc} \right) + 2\delta^{pa} Y_d^{br} (Y_d^\dagger Y_d)^{dc} \right.
\end{aligned}$$

$$\begin{aligned}
& + 2\delta^{rd}Y_d^{pc}(Y_dY_d^\dagger)^{ba} + 2\delta^{rd}Y_d^{pc}(Y_uY_u^\dagger)^{ba} + 6\delta^{pa}Y_d^{bc}(Y_d^\dagger Y_d)^{dr} + 6\delta^{rd}Y_d^{bc}(Y_dY_d^\dagger)^{pa} + \frac{27}{2}\delta^{pa}\delta^{rd}(Y_uY_u^\dagger Y_d)^{bc} + 18\delta^{pa}\delta^{rd}Y_d^{bc}\text{Tr}[Y_d^\dagger Y_d] + 30Y_d^{*ad}Y_d^{pc}Y_d^{br} \\
& + 84\delta^{pa}\delta^{rd}(Y_dY_d^\dagger Y_d)^{bc} - \frac{9}{2}\delta^{pa}\delta^{rd}g_L^2Y_d^{bc} - 6\delta^{rd}Y_d^{bc}(Y_uY_u^\dagger)^{pa} - 18Y_d^{*ad}Y_d^{pr}Y_d^{bc} + 2Y_d^{*ad}Y_d^{br}(Y_dY_d^\dagger Y_d)^{pc} + 3Y_d^{bc}(Y_d^\dagger Y_d)^{dr}(Y_uY_u^\dagger)^{pa} \\
& + 3Y_d^{*ad}Y_d^{pc}(Y_uY_u^\dagger Y_d)^{br} + 3\delta^{pa}Y_d^{bc}(Y_d^\dagger Y_dY_d^\dagger Y_d)^{dr} + 3\delta^{rd}Y_d^{bc}(Y_dY_d^\dagger Y_dY_d^\dagger)^{pa} + 4\delta^{rd}Y_d^{pc}(Y_uY_u^\dagger Y_uY_u^\dagger)^{ba} + \frac{9}{2}\delta^{pa}\delta^{rd}g_L^4Y_d^{bc} \\
& + 6\delta^{rd}(Y_dY_d^\dagger)^{pa}(Y_dY_d^\dagger Y_d)^{bc} + 6\delta^{rd}Y_d^{bc}(Y_dY_d^\dagger Y_uY_u^\dagger)^{pa} + 9\delta^{pa}\delta^{rd}(Y_uY_u^\dagger Y_uY_u^\dagger Y_d)^{bc} + 12\delta^{rd}(Y_dY_d^\dagger)^{pa}(Y_uY_u^\dagger Y_d)^{bc} + 18\delta^{pa}\delta^{rd}(Y_uY_u^\dagger Y_dY_d^\dagger Y_d)^{bc} \\
& + 30\delta^{pa}\delta^{rd}(Y_dY_d^\dagger Y_uY_u^\dagger Y_d)^{bc} + 36Y_d^{*ad}Y_d^{pr}(Y_dY_d^\dagger Y_d)^{bc} - \frac{1}{2}Y_d^{br}(Y_d^\dagger Y_d)^{dc}(Y_dY_d^\dagger)^{pa} - \frac{1}{2}Y_d^{pc}(Y_d^\dagger Y_d)^{dr}(Y_dY_d^\dagger)^{ba} - \frac{1}{2}\delta^{rd}(Y_dY_d^\dagger)^{ba}(Y_dY_d^\dagger Y_d)^{pc} \\
& - \frac{1}{2}\delta^{pa}(Y_d^\dagger Y_d)^{dc}(Y_dY_d^\dagger Y_d)^{br} - g_Y^2g_L^2\left(\frac{1}{6}\delta^{pa}\delta^{cd}Y_d^{br} + \frac{4}{9}\delta^{rd}\delta^{ab}Y_d^{pc} + 3\delta^{pa}\delta^{rd}Y_d^{bc}\right) - g_Y^4\left(\frac{7}{27}\delta^{rd}\delta^{ab}Y_d^{pc} + \frac{19}{54}\delta^{pa}\delta^{cd}Y_d^{br} + \frac{1}{2}\delta^{pa}\delta^{rd}Y_d^{bc}\right) \\
& - 3Y_d^{bc}(Y_d^\dagger Y_d)^{dr}(Y_dY_d^\dagger)^{pa} - 6\delta^{rd}Y_d^{bc}(Y_uY_u^\dagger Y_uY_u^\dagger)^{pa} - 12\delta^{rd}(Y_uY_u^\dagger)^{pa}(Y_dY_d^\dagger Y_d)^{bc} - 12\delta^{pa}Y_d^{br}(Y_d^\dagger Y_dY_d^\dagger Y_d)^{dc} - 12\delta^{rd}Y_d^{pc}(Y_dY_d^\dagger Y_dY_d^\dagger)^{ba} \\
& - 24\delta^{rd}(Y_uY_u^\dagger)^{pa}(Y_uY_u^\dagger Y_d)^{bc} - 30Y_d^{pc}Y_d^{br}(Y_d^\dagger Y_dY_d^\dagger)^{ad} - 36\delta^{pa}\delta^{rd}Y_d^{bc}\text{Tr}[Y_d^\dagger Y_dY_d^\dagger Y_d] - 156\delta^{pa}\delta^{rd}(Y_dY_d^\dagger Y_dY_d^\dagger Y_d)^{bc} \Big\} C_{qd}^{(\times)abcd} \\
& + \left\{ \frac{8}{3}\delta^{ad}g_Y^2Y_d^{pr}(Y_e^\dagger Y_e)^{bc} - \frac{4}{9}\delta^{ab}\delta^{cd}g_Y^4Y_d^{pr} - 4Y_d^{pr}(Y_e^\dagger Y_e)^{ba}(Y_e^\dagger Y_e)^{dc} \right\} C_{ee}^{abcd} + \left\{ \frac{16}{3}\delta^{ad}g_Y^2Y_d^{pr}(Y_u^\dagger Y_u)^{bc} - \frac{16}{27}\delta^{ad}\delta^{bc}g_Y^4Y_d^{pr} \right. \\
& \left. - 12Y_d^{pr}(Y_u^\dagger Y_u)^{bc}(Y_u^\dagger Y_u)^{da} \right\} C_{uu}^{abcd} + \left\{ g_Y^4\left(\frac{8}{27}\delta^{rb}\delta^{ad}Y_d^{pc} + \frac{14}{9}\delta^{rb}\delta^{cd}Y_d^{pa} - \frac{4}{27}\delta^{ad}\delta^{bc}Y_d^{pr}\right) + g_Y^2g_L^2\left(\frac{2}{9}\delta^{rb}\delta^{ad}Y_d^{pc} + \frac{8}{3}\delta^{rb}\delta^{cd}Y_d^{pa}\right) + Y_d^{pc}(Y_d^\dagger Y_d)^{br}(Y_d^\dagger Y_d)^{da} \right. \\
& + \lambda\left(\frac{32}{27}\delta^{rb}\delta^{ad}g_s^2Y_d^{pc} + 24\delta^{rb}Y_d^{pa}(Y_d^\dagger Y_d)^{dc} - g_Y^2\left(\frac{10}{81}\delta^{rb}\delta^{ad}Y_d^{pc} + \frac{70}{27}\delta^{rb}\delta^{cd}Y_d^{pa}\right)\right) + g_Y^2\left(\frac{35}{81}\delta^{rb}\delta^{ad}(Y_dY_d^\dagger Y_d)^{pc} + \frac{47}{27}\delta^{rb}\delta^{cd}(Y_dY_d^\dagger Y_d)^{pa} \right. \\
& + \frac{8}{3}\delta^{ad}Y_d^{pr}(Y_d^\dagger Y_d)^{bc} - \frac{5}{81}\delta^{ad}Y_d^{pc}(Y_d^\dagger Y_d)^{br} - \frac{5}{27}\delta^{cd}Y_d^{pa}(Y_d^\dagger Y_d)^{br} - \frac{2}{3}\delta^{rb}Y_d^{pc}(Y_d^\dagger Y_d)^{da} - 8\delta^{rb}Y_d^{pa}(Y_d^\dagger Y_d)^{dc} \Big\} + g_s^2\left(\frac{32}{27}\delta^{rb}\delta^{ad}(Y_dY_d^\dagger Y_d)^{pc} \right. \\
& + \frac{160}{27}\delta^{ad}Y_d^{pc}(Y_d^\dagger Y_d)^{br} - 64\delta^{rb}Y_d^{pc}(Y_d^\dagger Y_d)^{da} \Big) + 3Y_d^{pa}(Y_d^\dagger Y_d)^{br}(Y_d^\dagger Y_d)^{dc} + 3\delta^{rb}(Y_d^\dagger Y_d)^{dc}(Y_dY_d^\dagger Y_d)^{pa} + 8\delta^{rb}Y_d^{pc}(Y_d^\dagger Y_dY_d^\dagger Y_d)^{da} - g_L^2\left(4\delta^{rb}Y_d^{pc}(Y_d^\dagger Y_d)^{da} \right. \\
& + 30\delta^{rb}Y_d^{pa}(Y_d^\dagger Y_d)^{dc} \Big) - 3\delta^{rb}(Y_d^\dagger Y_d)^{da}(Y_dY_d^\dagger Y_d)^{pc} - 12Y_d^{pr}(Y_d^\dagger Y_d)^{bc}(Y_d^\dagger Y_d)^{da} \Big\} C_{dd}^{abcd} + \left\{ \frac{1}{2}Y_d^{pc}(Y_d^\dagger Y_d)^{dr}(Y_e^\dagger Y_e)^{ba} + \frac{1}{2}\delta^{rd}(Y_e^\dagger Y_e)^{ba}(Y_dY_d^\dagger Y_d)^{pc} \right. \\
& + \frac{7}{9}\delta^{rd}\delta^{ab}g_Y^4Y_d^{pc} + \lambda\left(5\delta^{rd}Y_d^{pc}(Y_e^\dagger Y_e)^{ba} - \frac{35}{27}\delta^{rd}\delta^{ab}g_Y^2Y_d^{pc}\right) + g_Y^2\left(\frac{47}{54}\delta^{rd}\delta^{ab}(Y_dY_d^\dagger Y_d)^{pc} + \frac{4}{3}\delta^{rd}Y_d^{pc}(Y_e^\dagger Y_e)^{ba} - \frac{5}{54}\delta^{ab}Y_d^{pc}(Y_d^\dagger Y_d)^{dr}\right) \\
& + \frac{4}{3}\delta^{rd}\delta^{ab}g_Y^2g_L^2Y_d^{pc} - 2\delta^{rd}Y_d^{pc}(Y_e^\dagger Y_eY_e^\dagger Y_e)^{ba} - 5\delta^{rd}g_L^2Y_d^{pc}(Y_e^\dagger Y_e)^{ba} \Big\} C_{ed}^{abcd} + \left\{ \lambda\left(\frac{70}{27}\delta^{rd}\delta^{ab}g_Y^2Y_d^{pc} - \frac{3}{2}\delta^{rd}Y_u^{pa}(Y_u^\dagger Y_d)^{bc} - 6\delta^{rd}Y_d^{pc}(Y_u^\dagger Y_u)^{ba}\right) \right. \\
& + g_L^2\left(15\delta^{rd}Y_d^{pc}(Y_u^\dagger Y_u)^{ba} - 4\delta^{rd}Y_u^{pa}(Y_u^\dagger Y_d)^{bc}\right) + g_Y^2\left(\frac{5}{27}\delta^{ab}Y_d^{pc}(Y_d^\dagger Y_d)^{dr} - \frac{47}{27}\delta^{rd}\delta^{ab}(Y_dY_d^\dagger Y_d)^{pc}\right) + 2Y_d^{pc}(Y_d^\dagger Y_u)^{da}(Y_u^\dagger Y_d)^{br} + 4\delta^{rd}Y_u^{pa}(Y_u^\dagger Y_dY_d^\dagger Y_d)^{bc} \\
& + 7\delta^{rd}Y_u^{pa}(Y_u^\dagger Y_uY_u^\dagger Y_d)^{bc} - Y_u^{pa}(Y_d^\dagger Y_d)^{dr}(Y_u^\dagger Y_d)^{bc} - \frac{3}{2}Y_d^{pc}(Y_d^\dagger Y_d)^{dr}(Y_u^\dagger Y_u)^{ba} - \frac{3}{2}\delta^{rd}(Y_u^\dagger Y_u)^{ba}(Y_dY_d^\dagger Y_d)^{pc} - \frac{14}{9}\delta^{rd}\delta^{ab}g_Y^4Y_d^{pc} - \frac{8}{3}\delta^{rd}\delta^{ab}g_Y^2g_L^2Y_d^{pc}
\end{aligned}$$

$$\begin{aligned}
& -3\delta^{rd}(Y_u^\dagger Y_d)^{bc}(Y_d Y_d^\dagger Y_u)^{pa} - 12\delta^{rd}Y_d^{pc}(Y_u^\dagger Y_u Y_u^\dagger Y_u)^{ba} \Big\} C_{ud}^{(\parallel)abcd} + \left\{ \lambda \left( \frac{70}{81}\delta^{rd}\delta^{ab}g_Y^2 Y_d^{pc} + \frac{112}{27}\delta^{rd}\delta^{ab}g_s^2 Y_d^{pc} - 2\delta^{rd}Y_d^{pc}(Y_u^\dagger Y_u)^{ba} \right. \right. \\
& - \frac{9}{2}\delta^{rd}Y_u^{pa}(Y_u^\dagger Y_d)^{bc} \Big) + g_L^2 \left( 5\delta^{rd}Y_d^{pc}(Y_u^\dagger Y_u)^{ba} - 12\delta^{rd}Y_u^{pa}(Y_u^\dagger Y_d)^{bc} \right) + g_s^2 \left( \frac{80}{27}\delta^{ab}Y_d^{pc}(Y_d^\dagger Y_d)^{dr} - \frac{176}{27}\delta^{rd}\delta^{ab}(Y_d Y_d^\dagger Y_d)^{pc} - 32\delta^{rd}Y_d^{pc}(Y_u^\dagger Y_u)^{ba} \right) \\
& + g_Y^2 \left( \frac{5}{81}\delta^{ab}Y_d^{pc}(Y_d^\dagger Y_d)^{dr} - \frac{47}{81}\delta^{rd}\delta^{ab}(Y_d Y_d^\dagger Y_d)^{pc} \right) + 6Y_d^{pc}(Y_d^\dagger Y_u)^{da}(Y_u^\dagger Y_d)^{br} + 12\delta^{rd}Y_u^{pa}(Y_u^\dagger Y_d Y_d^\dagger Y_d)^{bc} + 21\delta^{rd}Y_u^{pa}(Y_u^\dagger Y_u Y_u^\dagger Y_d)^{bc} \\
& - \frac{1}{2}Y_d^{pc}(Y_d^\dagger Y_d)^{dr}(Y_u^\dagger Y_u)^{ba} - \frac{1}{2}\delta^{rd}(Y_u^\dagger Y_u)^{ba}(Y_d Y_d^\dagger Y_d)^{pc} - \frac{14}{27}\delta^{rd}\delta^{ab}g_Y^4 Y_d^{pc} - \frac{8}{9}\delta^{rd}\delta^{ab}g_Y^2 g_L^2 Y_d^{pc} - 3Y_u^{pa}(Y_d^\dagger Y_d)^{dr}(Y_u^\dagger Y_d)^{bc} - 4\delta^{rd}Y_d^{pc}(Y_u^\dagger Y_u Y_u^\dagger Y_u)^{ba} \\
& - 9\delta^{rd}(Y_u^\dagger Y_d)^{bc}(Y_d Y_d^\dagger Y_u)^{pa} \Big\} C_{ud}^{(\times)abcd} + \left\{ \frac{1}{2}g_Y^2 Y_e^{*ab}Y_d^{pc}Y_d^{dr} + \frac{3}{4}g_L^2 Y_e^{*ab}Y_d^{pc}Y_d^{dr} + 5Y_d^{pc}Y_d^{dr}(Y_e^\dagger Y_e Y_e^\dagger)^{ab} + 6Y_e^{*ab}Y_d^{pr}(Y_d Y_d^\dagger Y_d)^{dc} \right. \\
& - \frac{1}{6}Y_e^{*ab}Y_d^{pc}(Y_d Y_d^\dagger Y_d)^{dr} - \frac{1}{3}Y_e^{*ab}Y_d^{dr}(Y_d Y_d^\dagger Y_d)^{pc} - \frac{1}{2}Y_e^{*ab}Y_d^{pc}(Y_u Y_u^\dagger Y_d)^{dr} - \lambda \left( 3Y_e^{*ab}Y_d^{pr}Y_d^{dc} + 5Y_e^{*ab}Y_d^{pc}Y_d^{dr} \right) \Big\} C_{ledq}^{abcd} \\
& + C_{ledq}^{*abcd} \left\{ \frac{1}{2}Y_e^{ab}(Y_d^\dagger Y_d)^{cr}(Y_d Y_d^\dagger)^{pd} + g_L^2 \left( \frac{3}{8}\delta^{rc}Y_e^{ab}(Y_d Y_d^\dagger)^{pd} + \frac{9}{2}\delta^{pd}\delta^{rc}(Y_e Y_e^\dagger Y_e)^{ab} - \frac{9}{8}\delta^{pd}Y_e^{ab}(Y_d^\dagger Y_d)^{cr} \right) + \lambda \left( \frac{3}{2}\delta^{rc}Y_e^{ab}(Y_u Y_u^\dagger)^{pd} + \frac{9}{2}\delta^{pd}\delta^{rc}g_Y^2 Y_e^{ab} \right. \right. \\
& - \frac{1}{2}\delta^{pd}\delta^{rc}(Y_e Y_e^\dagger Y_e)^{ab} - \frac{3}{2}\delta^{pd}\delta^{rc}g_L^2 Y_e^{ab} - 3\delta^{pd}Y_e^{ab}(Y_d^\dagger Y_d)^{cr} - 3\delta^{pd}\delta^{rc}Y_e^{ab}\text{Tr}[Y_d^\dagger Y_d] - \frac{7}{2}\delta^{rc}Y_e^{ab}(Y_d Y_d^\dagger)^{pd} \Big) + 2\delta^{rc}Y_e^{ab}(Y_u Y_u^\dagger Y_u Y_u^\dagger)^{pd} \\
& + 4\delta^{pd}(Y_d^\dagger Y_d)^{cr}(Y_e Y_e^\dagger Y_e)^{ab} + 4\delta^{rc}(Y_d Y_d^\dagger)^{pd}(Y_e Y_e^\dagger Y_e)^{ab} + \frac{11}{2}\delta^{pd}\delta^{rc}g_Y^2 g_L^2 Y_e^{ab} + 6\delta^{pd}\delta^{rc}Y_e^{ab}\text{Tr}[Y_d^\dagger Y_d Y_d^\dagger Y_d] + 20\delta^{pd}\delta^{rc}(Y_e Y_e^\dagger Y_e Y_e^\dagger Y_e)^{ab} \\
& - \frac{1}{2}Y_e^{ab}(Y_d^\dagger Y_d)^{cr}(Y_u Y_u^\dagger)^{pd} - \frac{1}{2}\delta^{pd}Y_e^{ab}(Y_d^\dagger Y_d Y_d^\dagger Y_d)^{cr} - \frac{1}{2}\delta^{rc}Y_e^{ab}(Y_d Y_d^\dagger Y_d Y_d^\dagger)^{pd} - \frac{3}{4}\delta^{pd}\delta^{rc}g_L^4 Y_e^{ab} - g_Y^2 \left( \frac{1}{8}\delta^{pd}Y_e^{ab}(Y_d^\dagger Y_d)^{cr} + \frac{3}{8}\delta^{rc}Y_e^{ab}(Y_d Y_d^\dagger)^{pd} \right. \\
& + \frac{13}{2}\delta^{pd}\delta^{rc}(Y_e Y_e^\dagger Y_e)^{ab} \Big) - \delta^{rc}Y_e^{ab}(Y_d Y_d^\dagger Y_u Y_u^\dagger)^{pd} - \frac{25}{4}\delta^{pd}\delta^{rc}g_Y^4 Y_e^{ab} \Big\} + \left\{ \frac{1}{4}Y_u^{*cb}(Y_d^\dagger Y_d)^{dr}(Y_d Y_d^\dagger)^{pa} + \frac{3}{4}\delta^{pc}Y_d^{*ad}(Y_u^\dagger Y_u Y_u^\dagger Y_d)^{br} + g_L^2 \left( \frac{3}{2}\delta^{pa}\delta^{rd}Y_u^{*cb} \right. \right. \\
& - \frac{9}{4}\delta^{pc}\delta^{rd}Y_u^{*ab} \Big) + g_Y^2 g_L^2 \left( \frac{1}{2}\delta^{pa}\delta^{rd}Y_u^{*cb} + \frac{21}{2}\delta^{pc}\delta^{rd}Y_u^{*ab} \right) + \delta^{pc}(Y_u^\dagger Y_d)^{br}(Y_u^\dagger Y_u Y_d^\dagger)^{ad} + g_Y^2 \left( \frac{13}{36}\delta^{pa}\delta^{rd}(Y_u^\dagger Y_u Y_u^\dagger)^{cb} + \frac{47}{48}\delta^{pa}Y_u^{*cb}(Y_d^\dagger Y_d)^{dr} \right. \\
& - \frac{3}{8}\delta^{pc}Y_u^{*ab}(Y_d^\dagger Y_d)^{dr} - \frac{49}{48}\delta^{rd}Y_u^{*cb}(Y_d Y_d^\dagger)^{pa} - \frac{9}{8}\delta^{rd}Y_u^{*ab}(Y_d Y_d^\dagger)^{pc} - \frac{16}{3}\delta^{pc}\delta^{rd}(Y_u^\dagger Y_u Y_u^\dagger)^{ab} \Big) + g_L^2 \left( \frac{9}{8}\delta^{rd}Y_u^{*ab}(Y_d Y_d^\dagger)^{pc} + \frac{5}{2}\delta^{rd}Y_u^{*cb}(Y_u Y_u^\dagger)^{pa} \right. \\
& + 3\delta^{pa}\delta^{rd}(Y_d^\dagger Y_d Y_u^\dagger)^{cb} + \frac{15}{4}\delta^{pa}\delta^{rd}(Y_u^\dagger Y_u Y_u^\dagger)^{cb} - \frac{1}{16}\delta^{rd}Y_u^{*cb}(Y_d Y_d^\dagger)^{pa} - \frac{5}{8}\delta^{pc}Y_d^{*ad}(Y_u^\dagger Y_d)^{br} - \frac{23}{16}\delta^{pa}Y_u^{*cb}(Y_d^\dagger Y_d)^{dr} - \frac{9}{4}\delta^{pa}Y_d^{*cd}(Y_u^\dagger Y_d)^{br} \\
& - \frac{27}{8}\delta^{pc}Y_u^{*ab}(Y_d^\dagger Y_d)^{dr} \Big) + \delta^{rd}Y_u^{*cb}(Y_u Y_u^\dagger Y_u Y_u^\dagger)^{pa} + \lambda \left( \frac{1}{2}\delta^{pc}Y_d^{*ad}(Y_u^\dagger Y_d)^{br} + \frac{3}{4}\delta^{rd}Y_u^{*cb}(Y_u Y_u^\dagger)^{pa} + g_L^2 \left( \frac{9}{4}\delta^{pc}\delta^{rd}Y_u^{*ab} - \frac{3}{8}\delta^{pa}\delta^{rd}Y_u^{*cb} \right) \right. \\
& + g_Y^2 \left( \frac{13}{24}\delta^{pa}\delta^{rd}Y_u^{*cb} + \frac{49}{12}\delta^{pc}\delta^{rd}Y_u^{*ab} \right) + g_s^2 \left( 12\delta^{pa}\delta^{rd}Y_u^{*cb} + 40\delta^{pc}\delta^{rd}Y_u^{*ab} \right) + 3\delta^{pa}Y_d^{*cd}(Y_u^\dagger Y_d)^{br} + \frac{9}{2}\delta^{rd}Y_u^{*ab}(Y_u Y_u^\dagger)^{pc} - \frac{1}{4}\delta^{pa}\delta^{rd}(Y_u^\dagger Y_u Y_u^\dagger)^{cb} \\
& - \frac{3}{4}\delta^{pa}\delta^{rd}(Y_d^\dagger Y_d Y_u^\dagger)^{cb} - \left( \frac{3}{2}\delta^{pa}\delta^{rd}Y_u^{*cb} + 9\delta^{pc}\delta^{rd}Y_u^{*ab} \right) \text{Tr}[Y_d^\dagger Y_d] - \frac{3}{2}\delta^{pa}Y_u^{*cb}(Y_d^\dagger Y_d)^{dr} - \frac{3}{2}\delta^{pc}\delta^{rd}(Y_u^\dagger Y_u Y_u^\dagger)^{ab} - \frac{7}{4}\delta^{rd}Y_u^{*cb}(Y_d Y_d^\dagger)^{pa}
\end{aligned}$$

$$\begin{aligned}
& -\frac{15}{2}\delta^{pc}\delta^{rd}(Y_d^\dagger Y_d Y_u^\dagger)^{ab} - 9\delta^{pc}Y_u^{*ab}(Y_d^\dagger Y_d)^{dr} - \frac{21}{2}\delta^{rd}Y_u^{*ab}(Y_d Y_d^\dagger)^{pc} + \left(3\delta^{pa}\delta^{rd}Y_u^{*cb} + 18\delta^{pc}\delta^{rd}Y_u^{*ab}\right)\text{Tr}\left[Y_d^\dagger Y_d Y_d^\dagger Y_d\right] + \frac{3}{2}Y_u^{*ab}(Y_d^\dagger Y_d)^{dr}(Y_d Y_d^\dagger)^{pc} \\
& + 2\delta^{rd}(Y_u Y_u^\dagger)^{pa}(Y_d^\dagger Y_d Y_u^\dagger)^{cb} + 2\delta^{pa}(Y_d^\dagger Y_d)^{dr}(Y_u^\dagger Y_u Y_u^\dagger)^{cb} + 2\delta^{rd}(Y_d Y_d^\dagger)^{pa}(Y_u^\dagger Y_u Y_u^\dagger)^{cb} + \frac{9}{2}\delta^{pa}Y_d^{*cd}(Y_u^\dagger Y_u Y_u^\dagger Y_d)^{br} + 6\delta^{pa}(Y_u^\dagger Y_d)^{br}(Y_u^\dagger Y_u Y_d^\dagger)^{cd} \\
& + 6\delta^{rd}Y_u^{*ab}(Y_u Y_u^\dagger Y_u Y_u^\dagger)^{pc} + 10\delta^{pa}\delta^{rd}(Y_u^\dagger Y_u Y_u^\dagger Y_u Y_u^\dagger)^{bc} + 12\delta^{rd}(Y_u Y_u^\dagger)^{pc}(Y_d^\dagger Y_d Y_u^\dagger)^{ab} + 12\delta^{pc}(Y_d^\dagger Y_d)^{dr}(Y_u^\dagger Y_u Y_u^\dagger)^{ab} + 12\delta^{rd}(Y_d Y_d^\dagger)^{pc}(Y_u^\dagger Y_u Y_u^\dagger)^{ab} \\
& + 60\delta^{pc}\delta^{rd}(Y_u^\dagger Y_u Y_u^\dagger Y_u Y_u^\dagger)^{ba} - \frac{1}{6}Y_d^{*ad}(Y_u^\dagger Y_d)^{br}(Y_d Y_d^\dagger)^{pc} - \frac{1}{4}Y_u^{*cb}(Y_d^\dagger Y_d)^{dr}(Y_u Y_u^\dagger)^{pa} - \frac{1}{4}\delta^{pa}Y_u^{*cb}(Y_d^\dagger Y_d Y_d^\dagger Y_d)^{dr} - \frac{1}{4}\delta^{pc}Y_d^{*ad}(Y_u^\dagger Y_d Y_d^\dagger Y_d)^{br} \\
& - \frac{1}{4}\delta^{rd}Y_u^{*cb}(Y_d Y_d^\dagger Y_d Y_d^\dagger)^{pa} - \frac{1}{2}\delta^{rd}Y_u^{*cb}(Y_d Y_d^\dagger Y_u Y_u^\dagger)^{pa} - g_Y^4\left(\frac{4}{9}\delta^{pa}\delta^{rd}Y_u^{*cb} + \frac{19}{4}\delta^{pc}\delta^{rd}Y_u^{*ab}\right) - Y_d^{*cd}(Y_u^\dagger Y_d)^{br}(Y_d Y_d^\dagger)^{pa} - \delta^{rd}(Y_d Y_d^\dagger)^{pa}(Y_d^\dagger Y_d Y_u^\dagger)^{cb} \\
& - g_s^2\left(4\delta^{pa}Y_u^{*cb}(Y_d^\dagger Y_d)^{dr} + 4\delta^{rd}Y_u^{*cb}(Y_d Y_d^\dagger)^{pa} + \frac{176}{3}\delta^{pa}\delta^{rd}(Y_u^\dagger Y_u Y_u^\dagger)^{cb} + 64\delta^{pc}\delta^{rd}(Y_u^\dagger Y_u Y_u^\dagger)^{ab}\right) - \delta^{pa}\delta^{rd}(Y_u^\dagger Y_d Y_d^\dagger Y_u Y_u^\dagger)^{bc} \\
& - \delta^{pa}\delta^{rd}(Y_u^\dagger Y_u Y_u^\dagger Y_d Y_d^\dagger)^{bc} - \frac{3}{2}Y_u^{*ab}(Y_d^\dagger Y_d)^{dr}(Y_u Y_u^\dagger)^{pc} - \frac{3}{2}\delta^{pc}Y_u^{*ab}(Y_d^\dagger Y_d Y_d^\dagger Y_d)^{dr} - \frac{3}{2}\delta^{pa}Y_d^{*cd}(Y_u^\dagger Y_d Y_d^\dagger Y_d)^{br} - \frac{3}{2}\delta^{rd}Y_u^{*ab}(Y_d Y_d^\dagger Y_d Y_d^\dagger)^{pc} \\
& - 2\delta^{pa}\delta^{rd}(Y_u^\dagger Y_d Y_d^\dagger Y_d Y_d^\dagger)^{bc} - 3\delta^{rd}Y_u^{*ab}(Y_d Y_d^\dagger Y_u Y_u^\dagger)^{pc} - 6\delta^{rd}(Y_d Y_d^\dagger)^{pc}(Y_d^\dagger Y_d Y_u^\dagger)^{ab} - 6\delta^{pc}\delta^{rd}(Y_u^\dagger Y_d Y_d^\dagger Y_d Y_d^\dagger)^{ba} - 6\delta^{pc}\delta^{rd}(Y_u^\dagger Y_d Y_d^\dagger Y_u Y_u^\dagger)^{ba} \\
& - 6\delta^{pc}\delta^{rd}(Y_u^\dagger Y_u Y_u^\dagger Y_d Y_d^\dagger)^{ba} \Big\} C_{quqd}^{(\parallel)abcd} + \left(C_{quqd}^{(\parallel)*}\right)^{abcd} \Big\{ \frac{1}{12}Y_d^{ad}Y_d^{cr}(Y_d Y_d^\dagger Y_u)^{pb} + \frac{1}{2}Y_d^{ar}Y_d^{cd}(Y_d Y_d^\dagger Y_u)^{pb} + g_Y^2\left(\frac{19}{36}Y_d^{pd}Y_d^{ar}Y_u^{cb} + \frac{3}{2}Y_d^{pd}Y_d^{cr}Y_u^{ab}\right) \\
& + g_L^2\left(\frac{3}{4}Y_d^{pd}Y_d^{ar}Y_u^{cb} + \frac{3}{2}Y_d^{ad}Y_d^{cr}Y_u^{pb} + \frac{9}{4}Y_d^{ar}Y_d^{cd}Y_u^{pb} + \frac{9}{4}Y_d^{pd}Y_d^{cr}Y_u^{ab}\right) + \lambda\left(\frac{1}{2}Y_d^{ad}Y_d^{cr}Y_u^{pb} - \frac{3}{2}Y_d^{pr}Y_d^{ad}Y_u^{cb} - \frac{5}{2}Y_d^{pd}Y_d^{ar}Y_u^{cb} - 9Y_d^{pr}Y_d^{cd}Y_u^{ab} - 15Y_d^{pd}Y_d^{cr}Y_u^{ab}\right) \\
& + \frac{5}{2}Y_d^{pd}Y_d^{ar}(Y_u Y_u^\dagger Y_u)^{cb} + 3Y_d^{pr}Y_u^{cb}(Y_d Y_d^\dagger Y_d)^{ad} + 15Y_d^{pd}Y_d^{cr}(Y_u Y_u^\dagger Y_u)^{ab} + 18Y_d^{pr}Y_u^{ab}(Y_d Y_d^\dagger Y_d)^{cd} - \frac{1}{12}Y_d^{pd}Y_u^{cb}(Y_d Y_d^\dagger Y_d)^{ar} - \frac{1}{6}Y_d^{ar}Y_u^{cb}(Y_d Y_d^\dagger Y_d)^{pd} \\
& - \frac{1}{4}Y_d^{pd}Y_u^{cb}(Y_u Y_u^\dagger Y_d)^{ar} - \frac{1}{4}Y_d^{ad}Y_d^{cr}(Y_u Y_u^\dagger Y_u)^{pb} - \frac{1}{2}Y_d^{pd}Y_u^{ab}(Y_d Y_d^\dagger Y_d)^{cr} - Y_d^{cr}Y_u^{ab}(Y_d Y_d^\dagger Y_d)^{pd} - \frac{3}{2}Y_d^{cr}Y_u^{pb}(Y_d Y_d^\dagger Y_d)^{ad} - \frac{3}{2}Y_d^{pd}Y_u^{ab}(Y_u Y_u^\dagger Y_d)^{cr} \\
& - \frac{3}{2}Y_d^{ar}Y_d^{cd}(Y_u Y_u^\dagger Y_u)^{pb} - 3Y_d^{ar}Y_u^{pb}(Y_d Y_d^\dagger Y_d)^{cd} - \frac{32}{3}g_s^2Y_d^{pd}Y_d^{ar}Y_u^{cb} \Big\} + \left\{ \frac{1}{2}Y_u^{*ab}(Y_d^\dagger Y_d)^{dr}(Y_d Y_d^\dagger)^{pc} + \frac{3}{4}Y_u^{*cb}(Y_d^\dagger Y_d)^{dr}(Y_d Y_d^\dagger)^{pa} + g_L^4\left(\frac{9}{2}\delta^{pa}\delta^{rd}Y_u^{*cb} \right. \right. \\
& - \frac{3}{4}\delta^{pc}\delta^{rd}Y_u^{*ab}) + g_Y^2g_L^2\left(\frac{3}{2}\delta^{pa}\delta^{rd}Y_u^{*cb} + \frac{7}{2}\delta^{pc}\delta^{rd}Y_u^{*ab}\right) + g_Y^2\left(\frac{13}{12}\delta^{pa}\delta^{rd}(Y_u^\dagger Y_u Y_u^\dagger)^{cb} + \frac{47}{16}\delta^{pa}Y_u^{*cb}(Y_d^\dagger Y_d)^{dr} - \frac{1}{8}\delta^{pc}Y_u^{*ab}(Y_d^\dagger Y_d)^{dr} \right. \\
& - \frac{3}{8}\delta^{rd}Y_u^{*ab}(Y_d Y_d^\dagger)^{pc} - \frac{16}{9}\delta^{pc}\delta^{rd}(Y_u^\dagger Y_u Y_u^\dagger)^{ab} - \frac{49}{16}\delta^{rd}Y_u^{*cb}(Y_d Y_d^\dagger)^{pa} \Big) + g_L^2\left(\frac{3}{8}\delta^{rd}Y_u^{*ab}(Y_d Y_d^\dagger)^{pc} + \frac{15}{2}\delta^{rd}Y_u^{*cb}(Y_u Y_u^\dagger)^{pa} + 9\delta^{pa}\delta^{rd}(Y_d^\dagger Y_d Y_u^\dagger)^{cb} \right. \\
& + \frac{45}{4}\delta^{pa}\delta^{rd}(Y_u^\dagger Y_u Y_u^\dagger)^{cb} - \frac{3}{16}\delta^{rd}Y_u^{*cb}(Y_d Y_d^\dagger)^{pa} - \frac{3}{4}\delta^{pa}Y_d^{*cd}(Y_u^\dagger Y_d)^{br} - \frac{9}{8}\delta^{pc}Y_u^{*ab}(Y_d^\dagger Y_d)^{dr} - \frac{15}{8}\delta^{pc}Y_d^{*ad}(Y_u^\dagger Y_d)^{br} - \frac{69}{16}\delta^{pa}Y_u^{*cb}(Y_d^\dagger Y_d)^{dr} \Big) \\
& + \lambda\left(g_L^2\left(\frac{3}{4}\delta^{pc}\delta^{rd}Y_u^{*ab} - \frac{9}{8}\delta^{pa}\delta^{rd}Y_u^{*cb}\right) + g_Y^2\left(\frac{49}{36}\delta^{pc}\delta^{rd}Y_u^{*ab} + \frac{13}{8}\delta^{pa}\delta^{rd}Y_u^{*cb}\right) + g_s^2\left(\frac{40}{3}\delta^{pc}\delta^{rd}Y_u^{*ab} + 48\delta^{pa}\delta^{rd}Y_u^{*cb}\right) + \delta^{pa}Y_d^{*cd}(Y_u^\dagger Y_d)^{br} \right. \\
& + \frac{3}{2}\delta^{pc}Y_d^{*ad}(Y_u^\dagger Y_d)^{br} + \frac{3}{2}\delta^{rd}Y_u^{*ab}(Y_u Y_u^\dagger)^{pc} + \frac{9}{4}\delta^{rd}Y_u^{*cb}(Y_u Y_u^\dagger)^{pa} - \frac{1}{2}\delta^{pc}\delta^{rd}(Y_u^\dagger Y_u Y_u^\dagger)^{ab} - \frac{3}{4}\delta^{pa}\delta^{rd}(Y_u^\dagger Y_u Y_u^\dagger)^{cb} - \left(3\delta^{pc}\delta^{rd}Y_u^{*ab} \right. \\
& + \frac{9}{2}\delta^{pa}\delta^{rd}Y_u^{*cb})\text{Tr}\left[Y_d^\dagger Y_d\right] - \frac{9}{4}\delta^{pa}\delta^{rd}(Y_d^\dagger Y_d Y_u^\dagger)^{cb} - \frac{5}{2}\delta^{pc}\delta^{rd}(Y_d^\dagger Y_d Y_u^\dagger)^{ab} - 3\delta^{pc}Y_u^{*ab}(Y_d^\dagger Y_d)^{dr} - \frac{7}{2}\delta^{rd}Y_u^{*ab}(Y_d Y_d^\dagger)^{pc} - \frac{9}{2}\delta^{pa}Y_u^{*cb}(Y_d^\dagger Y_d)^{dr}
\end{aligned}$$

$$\begin{aligned}
& -\frac{21}{4}\delta^{rd}Y_u^{*cb}(Y_dY_d^\dagger)^{pa}) + (6\delta^{pc}\delta^{rd}Y_u^{*ab} + 9\delta^{pa}\delta^{rd}Y_u^{*cb})\text{Tr}[Y_d^\dagger Y_d Y_d^\dagger Y_d] + \frac{3}{2}\delta^{pa}Y_d^{*cd}(Y_u^\dagger Y_u Y_u^\dagger Y_d)^{br} + 2\delta^{pa}(Y_u^\dagger Y_d)^{br}(Y_u^\dagger Y_u Y_d^\dagger)^{cd} \\
& + 2\delta^{rd}Y_u^{*ab}(Y_u Y_u^\dagger Y_u Y_u^\dagger)^{pc} + \frac{9}{4}\delta^{pc}Y_d^{*ad}(Y_u^\dagger Y_u Y_u^\dagger Y_d)^{br} + 3\delta^{pc}(Y_u^\dagger Y_d)^{br}(Y_u^\dagger Y_u Y_d^\dagger)^{ad} + 3\delta^{rd}Y_u^{*cb}(Y_u Y_u^\dagger Y_u Y_u^\dagger)^{pa} + 4\delta^{rd}(Y_u Y_u^\dagger)^{pc}(Y_d^\dagger Y_d Y_u^\dagger)^{ab} \\
& + 4\delta^{pc}(Y_d^\dagger Y_d)^{dr}(Y_u^\dagger Y_u Y_u^\dagger)^{ab} + 4\delta^{rd}(Y_d Y_d^\dagger)^{pc}(Y_u^\dagger Y_u Y_u^\dagger)^{ab} + 6\delta^{rd}(Y_u Y_u^\dagger)^{pa}(Y_d^\dagger Y_d Y_u^\dagger)^{cb} + 6\delta^{pa}(Y_d^\dagger Y_d)^{dr}(Y_u^\dagger Y_u Y_u^\dagger)^{cb} + 6\delta^{rd}(Y_d Y_d^\dagger)^{pa}(Y_u^\dagger Y_u Y_u^\dagger)^{cb} \\
& + 20\delta^{pc}\delta^{rd}(Y_u^\dagger Y_u Y_u^\dagger Y_u Y_u^\dagger)^{ba} + 30\delta^{pa}\delta^{rd}(Y_u^\dagger Y_u Y_u^\dagger Y_u Y_u^\dagger)^{bc} - \frac{1}{3}Y_d^{*cd}(Y_u^\dagger Y_d)^{br}(Y_d Y_d^\dagger)^{pa} - \frac{1}{2}Y_d^{*ad}(Y_u^\dagger Y_d)^{br}(Y_d Y_d^\dagger)^{pc} - \frac{1}{2}Y_u^{*ab}(Y_d^\dagger Y_d)^{dr}(Y_u Y_u^\dagger)^{pc} \\
& - \frac{1}{2}\delta^{pc}Y_u^{*ab}(Y_d^\dagger Y_d Y_d^\dagger Y_d)^{dr} - \frac{1}{2}\delta^{pa}Y_d^{*cd}(Y_u^\dagger Y_d Y_d^\dagger Y_d)^{br} - \frac{1}{2}\delta^{rd}Y_u^{*ab}(Y_d Y_d^\dagger Y_d Y_d^\dagger)^{pc} - \frac{3}{4}Y_u^{*cb}(Y_d^\dagger Y_d)^{dr}(Y_u Y_u^\dagger)^{pa} - \frac{3}{4}\delta^{pa}Y_u^{*cb}(Y_d^\dagger Y_d Y_d^\dagger Y_d)^{dr} \\
& - \frac{3}{4}\delta^{pc}Y_d^{*ad}(Y_u^\dagger Y_d Y_d^\dagger Y_d)^{br} - \frac{3}{4}\delta^{rd}Y_u^{*cb}(Y_d Y_d^\dagger Y_d Y_d^\dagger)^{pa} - g_Y^4\left(\frac{4}{3}\delta^{pa}\delta^{rd}Y_u^{*cb} + \frac{19}{12}\delta^{pc}\delta^{rd}Y_u^{*ab}\right) - g_s^2\left(\frac{64}{3}\delta^{pc}\delta^{rd}(Y_u^\dagger Y_u Y_u^\dagger)^{ab} + 88\delta^{pa}\delta^{rd}(Y_u^\dagger Y_u Y_u^\dagger)^{cb}\right) \\
& - \delta^{rd}Y_u^{*ab}(Y_d Y_d^\dagger Y_u Y_u^\dagger)^{pc} - \frac{3}{2}\delta^{rd}Y_u^{*cb}(Y_d Y_d^\dagger Y_u Y_u^\dagger)^{pa} - 2\delta^{rd}(Y_d Y_d^\dagger)^{pc}(Y_d^\dagger Y_d Y_u^\dagger)^{ab} - 2\delta^{pc}\delta^{rd}(Y_u^\dagger Y_d Y_d^\dagger Y_d Y_d^\dagger)^{ba} - 2\delta^{pc}\delta^{rd}(Y_u^\dagger Y_d Y_d^\dagger Y_u Y_u^\dagger)^{ba} \\
& - 2\delta^{pc}\delta^{rd}(Y_u^\dagger Y_u Y_u^\dagger Y_d Y_d^\dagger)^{ba} - 3\delta^{rd}(Y_d Y_d^\dagger)^{pa}(Y_d^\dagger Y_d Y_u^\dagger)^{cb} - 3\delta^{pa}\delta^{rd}(Y_u^\dagger Y_d Y_d^\dagger Y_u Y_u^\dagger)^{bc} - 3\delta^{pa}\delta^{rd}(Y_u^\dagger Y_u Y_u^\dagger Y_d Y_d^\dagger)^{bc} \\
& - 6\delta^{pa}\delta^{rd}(Y_u^\dagger Y_d Y_d^\dagger Y_d Y_d^\dagger)^{bc}\left\{C_{quqd}^{(\times)abcd} + \left(C_{quqd}^{(\times)*}\right)^{abcd}\left\{\frac{1}{6}Y_d^{ar}Y_d^{cd}(Y_d Y_d^\dagger Y_u)^{pb} + \frac{1}{4}Y_d^{ad}Y_d^{cr}(Y_d Y_d^\dagger Y_u)^{pb} + g_Y^2\left(\frac{1}{2}Y_d^{pd}Y_d^{cr}Y_u^{ab} + \frac{19}{12}Y_d^{pd}Y_d^{ar}Y_u^{cb}\right) + g_L^2\left(\frac{3}{4}Y_d^{ar}Y_d^{cd}Y_u^{pb}\right.\right.\right. \\
& + \frac{3}{4}Y_d^{pd}Y_d^{cr}Y_u^{ab} + \frac{9}{4}Y_d^{pd}Y_d^{ar}Y_u^{cb} + \frac{9}{2}Y_d^{ad}Y_d^{cr}Y_u^{pb}) + \lambda\left(\frac{3}{2}Y_d^{ad}Y_d^{cr}Y_u^{pb} - 3Y_d^{pr}Y_d^{cd}Y_u^{ab} - \frac{9}{2}Y_d^{pr}Y_d^{ad}Y_u^{cb} - 5Y_d^{pd}Y_d^{cr}Y_u^{ab} - \frac{15}{2}Y_d^{pd}Y_d^{ar}Y_u^{cb}\right) + 5Y_d^{pd}Y_d^{cr}(Y_u Y_u^\dagger Y_u)^{ab} \\
& + 6Y_d^{pr}Y_u^{ab}(Y_d Y_d^\dagger Y_d)^{cd} + \frac{15}{2}Y_d^{pd}Y_d^{ar}(Y_u Y_u^\dagger Y_u)^{cb} + 9Y_d^{pr}Y_u^{cb}(Y_d Y_d^\dagger Y_d)^{ad} - \frac{1}{6}Y_d^{pd}Y_u^{ab}(Y_d Y_d^\dagger Y_d)^{cr} - \frac{1}{4}Y_d^{pd}Y_u^{cb}(Y_d Y_d^\dagger Y_d)^{ar} - \frac{1}{3}Y_d^{cr}Y_u^{ab}(Y_d Y_d^\dagger Y_d)^{pd} \\
& - \frac{1}{2}Y_d^{ar}Y_u^{cb}(Y_d Y_d^\dagger Y_d)^{pd} - \frac{1}{2}Y_d^{pd}Y_u^{ab}(Y_u Y_u^\dagger Y_d)^{cr} - \frac{1}{2}Y_d^{ar}Y_d^{cd}(Y_u Y_u^\dagger Y_u)^{pb} - \frac{3}{4}Y_d^{pd}Y_u^{cb}(Y_u Y_u^\dagger Y_d)^{ar} - \frac{3}{4}Y_d^{ad}Y_d^{cr}(Y_u Y_u^\dagger Y_u)^{pb} - Y_d^{ar}Y_u^{pb}(Y_d Y_d^\dagger Y_d)^{cd} \\
& - \frac{9}{2}Y_d^{cr}Y_u^{pb}(Y_d Y_d^\dagger Y_d)^{ad}\left.\right\} + \left\{\frac{1}{3}Y_e^{*ab}(Y_u^\dagger Y_d)^{dr}(Y_d Y_d^\dagger)^{pc} + \frac{1}{2}\delta^{pc}Y_e^{*ab}(Y_u^\dagger Y_d Y_d^\dagger Y_d)^{dr} + \frac{3}{4}\delta^{pc}g_L^2Y_e^{*ab}(Y_u^\dagger Y_d)^{dr} - \delta^{pc}\lambda Y_e^{*ab}(Y_u^\dagger Y_d)^{dr}\right. \\
& - \frac{3}{2}\delta^{pc}Y_e^{*ab}(Y_u^\dagger Y_u Y_u^\dagger Y_d)^{dr}\left.\right\}C_{lequ}^{abcd} + C_{lequ}^{*abcd}\left\{\frac{1}{2}Y_d^{cr}Y_e^{ab}(Y_u Y_u^\dagger Y_u)^{pd} + \lambda Y_d^{cr}Y_e^{ab}Y_u^{pd} - \frac{1}{6}Y_d^{cr}Y_e^{ab}(Y_d Y_d^\dagger Y_u)^{pd} - \frac{3}{4}g_L^2Y_d^{cr}Y_e^{ab}Y_u^{pd}\right. \\
& - Y_d^{cr}Y_u^{pd}(Y_e Y_e^\dagger Y_e)^{ab}\left.\right\} + \left\{\frac{1}{2}\delta^{pc}\lambda Y_e^{*ad}(Y_u^\dagger Y_d)^{br} + \frac{3}{4}\delta^{pc}Y_e^{*ad}(Y_u^\dagger Y_u Y_u^\dagger Y_d)^{br} - \frac{1}{6}Y_e^{*ad}(Y_u^\dagger Y_d)^{br}(Y_d Y_d^\dagger)^{pc} - \frac{1}{4}\delta^{pc}Y_e^{*ad}(Y_u^\dagger Y_d Y_d^\dagger Y_d)^{br}\right. \\
& - \frac{5}{8}\delta^{pc}g_L^2Y_e^{*ad}(Y_u^\dagger Y_d)^{br}\left.\right\}C_{luqe}^{abcd} + C_{luqe}^{*abcd}\left\{\frac{1}{12}Y_d^{cr}Y_e^{ad}(Y_d Y_d^\dagger Y_u)^{pb} + \frac{3}{2}g_L^2Y_d^{cr}Y_e^{ad}Y_u^{pb} - \frac{1}{4}Y_d^{cr}Y_e^{ad}(Y_u Y_u^\dagger Y_u)^{pb} - \frac{1}{2}Y_d^{cr}Y_u^{pb}(Y_e Y_e^\dagger Y_e)^{ad}\right\} \\
& + \left\{\frac{4}{3}\delta^{bc}g_L^2Y_d^{pr}(Y_e Y_e^\dagger)^{da} - \frac{2}{9}\delta^{ad}\delta^{bc}g_L^4Y_d^{pr} - \frac{2}{9}\delta^{ad}\delta^{bc}g_Y^4Y_d^{pr} - \frac{4}{3}\delta^{bc}g_Y^2Y_d^{pr}(Y_e Y_e^\dagger)^{da} - 4Y_d^{pr}(Y_e Y_e^\dagger)^{bc}(Y_e Y_e^\dagger)^{da}\right\}C_{\ell\ell}^{abcd} + \left\{g_L^4\left(\frac{3}{2}\delta^{pa}\delta^{bc}Y_d^{dr}\right.\right. \\
& - \frac{2}{3}\delta^{ad}\delta^{bc}Y_d^{pr}) + g_Y^2g_L^2\left(\frac{5}{9}\delta^{pa}\delta^{bc}Y_d^{dr} + \delta^{pa}\delta^{cd}Y_d^{br}\right) + g_Y^4\left(\frac{7}{54}\delta^{pa}\delta^{bc}Y_d^{dr} + \frac{19}{9}\delta^{pa}\delta^{cd}Y_d^{br} - \frac{2}{27}\delta^{ad}\delta^{bc}Y_d^{pr}\right) + \lambda\left(\frac{32}{27}\delta^{pa}\delta^{bc}g_s^2Y_d^{dr} + 24\delta^{pa}Y_d^{br}(Y_d Y_d^\dagger)^{dc}\right.
\end{aligned}$$

$$\begin{aligned}
& -\frac{1}{3}\delta^{pa}\delta^{bc}g_L^2Y_d^{dr}-g_Y^2\left(\frac{7}{81}\delta^{pa}\delta^{bc}Y_d^{dr}+\frac{98}{27}\delta^{pa}\delta^{cd}Y_d^{br}\right)-3\delta^{pa}Y_d^{dr}(Y_uY_u^\dagger)^{bc}-12\delta^{pa}Y_d^{br}(Y_uY_u^\dagger)^{dc}+\delta^{pa}(Y_uY_u^\dagger)^{bc}(Y_dY_d^\dagger Y_d)^{dr} \\
& +g_Y^2\left(\frac{31}{162}\delta^{pa}\delta^{bc}(Y_dY_d^\dagger Y_d)^{dr}+\frac{4}{3}\delta^{bc}Y_d^{pr}(Y_dY_d^\dagger)^{da}+\frac{91}{27}\delta^{pa}\delta^{cd}(Y_dY_d^\dagger Y_d)^{br}+31\delta^{pa}Y_d^{br}(Y_uY_u^\dagger)^{dc}-\frac{25}{162}\delta^{bc}Y_d^{dr}(Y_dY_d^\dagger)^{pa}-\frac{25}{27}\delta^{cd}Y_d^{br}(Y_dY_d^\dagger)^{pa}\right. \\
& -\delta^{pa}Y_d^{dr}(Y_dY_d^\dagger)^{bc}-\frac{4}{3}\delta^{bc}Y_d^{pr}(Y_uY_u^\dagger)^{da}-15\delta^{pa}Y_d^{br}(Y_dY_d^\dagger)^{dc}\Big)+g_s^2\left(\frac{32}{27}\delta^{pa}\delta^{bc}(Y_dY_d^\dagger Y_d)^{dr}+\frac{160}{27}\delta^{bc}Y_d^{dr}(Y_dY_d^\dagger)^{pa}-64\delta^{pa}Y_d^{dr}(Y_dY_d^\dagger)^{bc}\right) \\
& +g_L^2\left(\frac{5}{6}\delta^{pa}\delta^{bc}(Y_dY_d^\dagger Y_d)^{dr}+\delta^{bc}Y_d^{dr}(Y_uY_u^\dagger)^{pa}+\frac{4}{3}\delta^{pa}\delta^{bc}(Y_uY_u^\dagger Y_d)^{dr}+4\delta^{bc}Y_d^{pr}(Y_dY_d^\dagger)^{da}+4\delta^{bc}Y_d^{pr}(Y_uY_u^\dagger)^{da}+9\delta^{pa}Y_d^{br}(Y_uY_u^\dagger)^{dc}-\frac{1}{6}\delta^{bc}Y_d^{dr}(Y_dY_d^\dagger)^{pa}\right. \\
& -3\delta^{pa}Y_d^{dr}(Y_uY_u^\dagger)^{bc}-6\delta^{pa}Y_d^{dr}(Y_dY_d^\dagger)^{bc}-9\delta^{pa}Y_d^{br}(Y_dY_d^\dagger)^{dc}\Big)+3Y_d^{br}(Y_dY_d^\dagger)^{pa}(Y_dY_d^\dagger)^{dc}+3Y_d^{br}(Y_dY_d^\dagger)^{da}(Y_uY_u^\dagger)^{pc}+3Y_d^{dr}(Y_uY_u^\dagger)^{pa}(Y_uY_u^\dagger)^{bc} \\
& +3\delta^{pa}(Y_dY_d^\dagger)^{dc}(Y_dY_d^\dagger Y_d)^{br}+6\delta^{pa}Y_d^{dr}(Y_uY_u^\dagger Y_uY_u^\dagger)^{bc}+8\delta^{pa}Y_d^{dr}(Y_dY_d^\dagger Y_dY_d^\dagger)^{bc}+19\delta^{pa}Y_d^{dr}(Y_dY_d^\dagger Y_uY_u^\dagger)^{bc}-Y_d^{dr}(Y_dY_d^\dagger)^{pa}(Y_dY_d^\dagger)^{bc} \\
& -2Y_d^{dr}(Y_dY_d^\dagger)^{pa}(Y_uY_u^\dagger)^{bc}-2\delta^{pa}(Y_dY_d^\dagger)^{bc}(Y_dY_d^\dagger Y_d)^{dr}-3Y_d^{br}(Y_dY_d^\dagger)^{pa}(Y_uY_u^\dagger)^{dc}-3\delta^{pa}(Y_uY_u^\dagger)^{dc}(Y_dY_d^\dagger Y_d)^{br}-3\delta^{pa}Y_d^{dr}(Y_uY_u^\dagger Y_dY_d^\dagger)^{bc} \\
& -4\delta^{pa}(Y_dY_d^\dagger)^{bc}(Y_uY_u^\dagger Y_d)^{dr}-4\delta^{pa}(Y_uY_u^\dagger)^{bc}(Y_uY_u^\dagger Y_d)^{dr}-12Y_d^{pr}(Y_dY_d^\dagger)^{bc}(Y_dY_d^\dagger)^{da}-12Y_d^{pr}(Y_uY_u^\dagger)^{bc}(Y_uY_u^\dagger)^{da}-24\delta^{pa}Y_d^{br}(Y_uY_u^\dagger Y_uY_u^\dagger)^{dc}\Big\}C_{qq}^{(\parallel)abcd} \\
& +\left\{g_Y^4\left(\frac{7}{27}\delta^{pa}\delta^{bc}Y_d^{dr}+\frac{19}{18}\delta^{pa}\delta^{cd}Y_d^{br}-\frac{4}{27}\delta^{ad}\delta^{bc}Y_d^{pr}\right)+g_Y^2g_L^2\left(\frac{1}{3}\delta^{pa}\delta^{bc}Y_d^{dr}+\frac{11}{3}\delta^{pa}\delta^{cd}Y_d^{br}\right)+Y_d^{dr}(Y_dY_d^\dagger)^{pa}(Y_dY_d^\dagger)^{bc}+\lambda\left(\frac{64}{27}\delta^{pa}\delta^{bc}g_s^2Y_d^{dr}\right.\right. \\
& +3\delta^{pa}Y_d^{dr}(Y_uY_u^\dagger)^{bc}+12\delta^{pa}Y_d^{br}(Y_uY_u^\dagger)^{dc}+48\delta^{pa}Y_d^{br}(Y_dY_d^\dagger)^{dc}-g_Y^2\left(\frac{14}{81}\delta^{pa}\delta^{bc}Y_d^{dr}+\frac{49}{27}\delta^{pa}\delta^{cd}Y_d^{br}\right)-7\delta^{pa}\delta^{cd}g_L^2Y_d^{br}\Big)+g_Y^2\left(\frac{31}{81}\delta^{pa}\delta^{bc}(Y_dY_d^\dagger Y_d)^{dr}\right. \\
& +\frac{91}{54}\delta^{pa}\delta^{cd}(Y_dY_d^\dagger Y_d)^{br}+\frac{8}{3}\delta^{bc}Y_d^{pr}(Y_dY_d^\dagger)^{da}+\frac{19}{3}\delta^{pa}Y_d^{dr}(Y_uY_u^\dagger)^{bc}-\frac{25}{81}\delta^{bc}Y_d^{dr}(Y_dY_d^\dagger)^{pa}-\frac{25}{54}\delta^{cd}Y_d^{br}(Y_dY_d^\dagger)^{pa}-\delta^{pa}Y_d^{dr}(Y_dY_d^\dagger)^{bc}-\frac{8}{3}\delta^{bc}Y_d^{pr}(Y_uY_u^\dagger)^{da} \\
& -15\delta^{pa}Y_d^{br}(Y_dY_d^\dagger)^{dc}\Big)+g_s^2\left(\frac{64}{27}\delta^{pa}\delta^{bc}(Y_dY_d^\dagger Y_d)^{dr}+\frac{320}{27}\delta^{bc}Y_d^{dr}(Y_dY_d^\dagger)^{pa}-64\delta^{pa}Y_d^{dr}(Y_dY_d^\dagger)^{bc}-64\delta^{pa}Y_d^{dr}(Y_uY_u^\dagger)^{bc}\right)+g_L^2\left(\frac{5}{2}\delta^{pa}\delta^{cd}(Y_dY_d^\dagger Y_d)^{br}\right. \\
& +3\delta^{cd}Y_d^{br}(Y_uY_u^\dagger)^{pa}+3\delta^{pa}Y_d^{dr}(Y_uY_u^\dagger)^{bc}-\frac{1}{2}\delta^{cd}Y_d^{br}(Y_dY_d^\dagger)^{pa}-2\delta^{pa}\delta^{cd}(Y_uY_u^\dagger Y_d)^{br}-3\delta^{pa}Y_d^{dr}(Y_dY_d^\dagger)^{bc}-9\delta^{pa}Y_d^{br}(Y_uY_u^\dagger)^{dc}-18\delta^{pa}Y_d^{br}(Y_dY_d^\dagger)^{dc}\Big) \\
& +3\delta^{pa}(Y_uY_u^\dagger)^{bc}(Y_dY_d^\dagger Y_d)^{dr}+\frac{9}{2}\delta^{pa}\delta^{cd}g_L^4Y_d^{br}+6\delta^{pa}(Y_dY_d^\dagger)^{dc}(Y_uY_u^\dagger Y_d)^{br}+6\delta^{pa}(Y_uY_u^\dagger)^{dc}(Y_uY_u^\dagger Y_d)^{br}+8\delta^{pa}Y_d^{dr}(Y_dY_d^\dagger Y_dY_d^\dagger)^{bc} \\
& +9Y_d^{dr}(Y_dY_d^\dagger)^{ba}(Y_uY_u^\dagger)^{pc}+9Y_d^{br}(Y_uY_u^\dagger)^{pa}(Y_uY_u^\dagger)^{dc}+24Y_d^{pr}(Y_dY_d^\dagger)^{da}(Y_uY_u^\dagger)^{bc}+57\delta^{pa}Y_d^{br}(Y_dY_d^\dagger Y_uY_u^\dagger)^{dc}-Y_d^{dr}(Y_dY_d^\dagger)^{pa}(Y_uY_u^\dagger)^{bc} \\
& -3Y_d^{br}(Y_dY_d^\dagger)^{pa}(Y_dY_d^\dagger)^{dc}-3\delta^{pa}(Y_uY_u^\dagger)^{dc}(Y_dY_d^\dagger Y_d)^{br}-3\delta^{pa}(Y_dY_d^\dagger)^{bc}(Y_dY_d^\dagger Y_d)^{dr}-6Y_d^{br}(Y_dY_d^\dagger)^{pa}(Y_uY_u^\dagger)^{dc}-9\delta^{pa}Y_d^{br}(Y_uY_u^\dagger Y_dY_d^\dagger)^{dc} \\
& -12Y_d^{pr}(Y_dY_d^\dagger)^{bc}(Y_dY_d^\dagger)^{da}-12Y_d^{pr}(Y_uY_u^\dagger)^{bc}(Y_uY_u^\dagger)^{da}-14\delta^{pa}Y_d^{dr}(Y_uY_u^\dagger Y_uY_u^\dagger)^{bc}-24\delta^{pa}Y_d^{br}(Y_dY_d^\dagger Y_dY_d^\dagger)^{dc}\Big\}C_{qq}^{(\times)abcd}+\left\{\frac{1}{2}Y_d^{dr}(Y_dY_d^\dagger)^{pc}(Y_eY_e^\dagger)^{ba}\right. \\
& +\frac{1}{2}\delta^{pc}(Y_eY_e^\dagger)^{ba}(Y_dY_d^\dagger Y_d)^{dr}+\lambda\left(\frac{49}{27}\delta^{pc}\delta^{ab}g_Y^2Y_d^{dr}+5\delta^{pc}Y_d^{dr}(Y_eY_e^\dagger)^{ba}\right)+g_Y^2\left(\frac{25}{54}\delta^{ab}Y_d^{dr}(Y_dY_d^\dagger)^{pc}-\frac{91}{54}\delta^{pc}\delta^{ab}(Y_dY_d^\dagger Y_d)^{dr}-\frac{47}{6}\delta^{pc}Y_d^{dr}(Y_eY_e^\dagger)^{ba}\right) \\
& \left.-\frac{1}{2}\delta^{pc}\delta^{ab}g_Y^2g_L^2Y_d^{dr}-\frac{19}{18}\delta^{pc}\delta^{ab}g_Y^4Y_d^{dr}-\frac{3}{2}\delta^{pc}g_L^2Y_d^{dr}(Y_eY_e^\dagger)^{ba}-2\delta^{pc}Y_d^{dr}(Y_eY_e^\dagger Y_eY_e^\dagger)^{ba}\right\}C_{\ell q}^{(\parallel)abcd}+\left\{\frac{5}{18}\delta^{pc}\delta^{ab}g_Y^2g_L^2Y_d^{dr}+\frac{3}{4}\delta^{pc}\delta^{ab}g_L^4Y_d^{dr}\right.
\end{aligned}$$

$$\begin{aligned}
& + \lambda \left( \frac{49}{54} \delta^{pc} \delta^{ab} g_Y^2 Y_d^{dr} + 10 \delta^{pc} Y_d^{dr} (Y_e Y_e^\dagger)^{ba} - \frac{7}{6} \delta^{pc} \delta^{ab} g_L^2 Y_d^{dr} \right) + g_Y^2 \left( \frac{25}{108} \delta^{ab} Y_d^{dr} (Y_d Y_d^\dagger)^{pc} - \frac{91}{108} \delta^{pc} \delta^{ab} (Y_d Y_d^\dagger Y_d)^{dr} - \frac{47}{6} \delta^{pc} Y_d^{dr} (Y_e Y_e^\dagger)^{ba} \right) \\
& + \delta^{pc} (Y_e Y_e^\dagger)^{ba} (Y_u Y_u^\dagger Y_d)^{dr} + g_L^2 \left( \frac{5}{12} \delta^{pc} \delta^{ab} (Y_d Y_d^\dagger Y_d)^{dr} + \frac{1}{2} \delta^{ab} Y_d^{dr} (Y_u Y_u^\dagger)^{pc} - \frac{1}{12} \delta^{ab} Y_d^{dr} (Y_d Y_d^\dagger)^{pc} - \frac{1}{3} \delta^{pc} \delta^{ab} (Y_u Y_u^\dagger Y_d)^{dr} - 3 \delta^{pc} Y_d^{dr} (Y_e Y_e^\dagger)^{ba} \right) \\
& + \frac{3}{2} Y_d^{dr} (Y_e Y_e^\dagger)^{ba} (Y_u Y_u^\dagger)^{pc} - \frac{1}{2} Y_d^{dr} (Y_d Y_d^\dagger)^{pc} (Y_e Y_e^\dagger)^{ba} - \frac{19}{36} \delta^{pc} \delta^{ab} g_Y^4 Y_d^{dr} - 8 \delta^{pc} Y_d^{dr} (Y_e Y_e^\dagger Y_e Y_e^\dagger)^{ba} \Big\} C_{\ell q}^{(\times)abcd}, \tag{7.6}
\end{aligned}$$

## 8 $\psi^2 XH$

### 8.1 $C_{eB}$

$$\begin{aligned}
\beta_{C_{eB}^{pr}}^{(1)} & = -3g_Y^2 C_{HB} Y_e^{pr} + 3ig_Y^2 C_{H\tilde{B}} Y_e^{pr} + \frac{3}{4} g_L^2 C_{HWB} Y_e^{pr} - \frac{3i}{4} g_L^2 C_{H\tilde{W}B} Y_e^{pr} + \left\{ \frac{1}{2} \left( 2T_2 \delta^{pa} \delta^{rb} + 4\delta^{pa} (Y_e^\dagger Y_e)^{br} + 5\delta^{rb} (Y_e Y_e^\dagger)^{pa} \right) + \frac{23}{4} \delta^{pa} \delta^{rb} g_Y^2 \right. \\
& \quad \left. - \frac{9}{4} \delta^{pa} \delta^{rb} g_L^2 \right\} C_{eB}^{ab} - \frac{3}{4} \delta^{pa} \delta^{rb} g_L^2 C_{eW}^{ab} + \frac{5}{4} \delta^{pa} \delta^{rd} Y_u^{*cb} C_{\ell uqe}^{abcd}, \tag{8.1}
\end{aligned}$$

$$\begin{aligned}
\beta_{C_{eB}^{pr}}^{(2)} & = (C_{\ell HH}^\dagger C_{\ell HH} Y_e)^{pr} + \left\{ \frac{1}{8} g_Y^2 Y_e^{pr} + \frac{1}{8} (Y_e Y_e^\dagger Y_e)^{pr} + \frac{1}{4} g_L^2 Y_e^{pr} \right\} C_{HD}^{(II)} - \left\{ \frac{1}{8} (Y_e Y_e^\dagger Y_e)^{pr} + \frac{3}{16} g_L^2 Y_e^{pr} + \frac{5}{16} g_Y^2 Y_e^{pr} \right\} C_{HD}^{(\times)} + \left\{ g_Y^2 \left( \frac{3}{2} T_2 Y_e^{pr} \right. \right. \\
& \quad \left. \left. + \frac{41}{4} (Y_e Y_e^\dagger Y_e)^{pr} \right) + \frac{9}{2} \lambda g_Y^2 Y_e^{pr} + \frac{209}{12} g_Y^4 Y_e^{pr} - \frac{9}{8} g_Y^2 g_L^2 Y_e^{pr} \right\} C_{HB} + \left\{ g_Y^2 \left( -\frac{3i}{2} T_2 Y_e^{pr} - \frac{41i}{4} (Y_e Y_e^\dagger Y_e)^{pr} \right) + \frac{9i}{8} g_Y^2 g_L^2 Y_e^{pr} - \frac{9i}{2} \lambda g_Y^2 Y_e^{pr} \right. \\
& \quad \left. - \frac{209i}{12} g_Y^4 Y_e^{pr} \right\} C_{H\tilde{B}} + \frac{9}{8} g_L^4 C_{HW} Y_e^{pr} - \frac{9i}{8} g_L^4 C_{H\tilde{W}} Y_e^{pr} + \left\{ \frac{425}{96} g_L^4 Y_e^{pr} - \frac{3}{8} \lambda g_L^2 Y_e^{pr} - g_L^2 \left( \frac{3}{8} T_2 Y_e^{pr} + \frac{9}{16} (Y_e Y_e^\dagger Y_e)^{pr} \right) \right. \\
& \quad \left. - \frac{159}{32} g_Y^2 g_L^2 Y_e^{pr} \right\} C_{HWB} + \left\{ \frac{3i}{8} \lambda g_L^2 Y_e^{pr} + g_L^2 \left( \frac{3i}{8} T_2 Y_e^{pr} + \frac{9i}{16} (Y_e Y_e^\dagger Y_e)^{pr} \right) + \frac{159i}{32} g_Y^2 g_L^2 Y_e^{pr} - \frac{425i}{96} g_L^4 Y_e^{pr} \right\} C_{H\tilde{W}B} - \frac{9}{4} g_L^6 C_W Y_e^{pr} \\
& \quad + \frac{5i}{4} g_L^6 C_{\tilde{W}} Y_e^{pr} + \left\{ \frac{3}{8} \delta^{pa} \delta^{rb} g_L^2 - \frac{9}{8} \delta^{pa} \delta^{rb} g_Y^2 - \frac{9}{8} \delta^{pa} (Y_e^\dagger Y_e)^{br} - \frac{9}{8} \delta^{rb} (Y_e Y_e^\dagger)^{pa} \right\} C_{eH}^{ab} + \left\{ g_L^2 \left( \frac{15}{8} T_2 \delta^{pa} \delta^{rb} + \frac{9}{4} Y_e^{*ab} Y_e^{pr} + 9\delta^{pa} (Y_e^\dagger Y_e)^{br} \right. \right. \\
& \quad \left. \left. + \frac{237}{16} \delta^{rb} (Y_e Y_e^\dagger)^{pa} \right) + g_Y^2 \left( \frac{39}{8} \delta^{pa} \delta^{rb} \text{Tr}[Y_e^\dagger Y_e] + \frac{45}{4} Y_e^{*ab} Y_e^{pr} - \frac{3}{8} \delta^{pa} \delta^{rb} \text{Tr}[Y_d^\dagger Y_d] - \frac{27}{8} \delta^{pa} (Y_e^\dagger Y_e)^{br} - \frac{29}{8} \delta^{pa} \delta^{rb} \text{Tr}[Y_u^\dagger Y_u] - \frac{135}{16} \delta^{rb} (Y_e Y_e^\dagger)^{pa} \right) \right. \\
& \quad \left. + g_s^2 \left( 20\delta^{pa} \delta^{rb} \text{Tr}[Y_d^\dagger Y_d] + 20\delta^{pa} \delta^{rb} \text{Tr}[Y_u^\dagger Y_u] \right) + \frac{5}{4} \delta^{pa} (Y_e^\dagger Y_e Y_e^\dagger Y_e)^{br} + \frac{5}{4} \delta^{rb} (Y_e Y_e^\dagger Y_e Y_e^\dagger)^{pa} + \frac{3}{2} \delta^{pa} \delta^{rb} \lambda^2 + \frac{3}{2} \delta^{pa} \delta^{rb} \text{Tr}[Y_d^\dagger Y_d Y_u^\dagger Y_u] \right. \\
& \quad \left. + \frac{69}{16} \delta^{pa} \delta^{rb} g_Y^2 g_L^2 - \lambda \left( \frac{3}{2} \delta^{pa} \delta^{rb} g_Y^2 + 6\delta^{pa} (Y_e^\dagger Y_e)^{br} + 6\delta^{rb} (Y_e Y_e^\dagger)^{pa} \right) - \frac{9}{4} T_4 \delta^{pa} \delta^{rb} - 3T_2 \delta^{pa} (Y_e^\dagger Y_e)^{br} - 3(Y_e^\dagger Y_e)^{br} (Y_e Y_e^\dagger)^{pa} \right\}
\end{aligned}$$



$$\begin{aligned}
& -\frac{15}{4}\text{Tr}_2\delta^{rb}(Y_e Y_e^\dagger)^{pa} - \frac{23}{4}\delta^{pa}\delta^{rb}g_L^4 - \frac{10753}{144}\delta^{pa}\delta^{rb}g_Y^4 \Big\} C_{eB}^{ab} + \left\{ \frac{91}{96}\delta^{pa}\delta^{rb}g_L^4 + g_L^2 \left( \frac{9}{16}\delta^{rb}(Y_e Y_e^\dagger)^{pa} - \frac{3}{16}\delta^{pa}(Y_e^\dagger Y_e)^{br} - \frac{3}{4}\delta^{pa}\delta^{rb}\text{Tr}[Y_u^\dagger Y_u] \right. \right. \\
& - \frac{15}{8}\delta^{pa}\delta^{rb}\text{Tr}[Y_e^\dagger Y_e] - \frac{9}{4}Y_e^{*ab}Y_e^{pr} - \frac{21}{8}\delta^{pa}\delta^{rb}\text{Tr}[Y_d^\dagger Y_d] \Big) + \frac{45}{32}\delta^{pa}\delta^{rb}g_Y^2g_L^2 - \frac{3}{4}\delta^{pa}\delta^{rb}\lambda g_L^2 \Big\} C_{eW}^{ab} + \left\{ \frac{9}{4}g_L^2Y_u^{*ab}Y_e^{pr} + \frac{15}{4}g_Y^2Y_u^{*ab}Y_e^{pr} \right\} C_{uB}^{ab} \\
& + \frac{15}{4}g_Y^2C_{uB}^{*ab}Y_e^{pr}Y_u^{ab} + \frac{15}{8}g_L^2C_{uW}^{*ab}Y_e^{pr}Y_u^{ab} + \left\{ \frac{15}{4}g_Y^2Y_d^{*ab}Y_e^{pr} + \frac{27}{4}g_L^2Y_d^{*ab}Y_e^{pr} \right\} C_{dB}^{ab} - \frac{3}{4}g_L^2Y_d^{*ab}C_{dW}^{ab}Y_e^{pr} + \left\{ -\frac{3}{4}\delta^{pa}g_L^2Y_e^{br} - g_Y^2 \left( \frac{5}{9}\delta^{pa}Y_e^{br} \right. \right. \\
& + \delta^{ab}Y_e^{pr} \Big) - \frac{35}{24}Y_e^{br}(Y_e Y_e^\dagger)^{pa} - \frac{35}{24}\delta^{pa}(Y_e Y_e^\dagger Y_e)^{br} - \frac{3}{2}\delta^{pa}\lambda Y_e^{br} \Big\} C_{H\ell}^{(\parallel)ab} + \left\{ -g_L^2 \left( \frac{1}{24}\delta^{pa}Y_e^{br} + \frac{1}{2}\delta^{ab}Y_e^{pr} \right) - g_Y^2 \left( \frac{1}{2}\delta^{ab}Y_e^{pr} + \frac{101}{72}\delta^{pa}Y_e^{br} \right) \right. \\
& - \frac{25}{24}Y_e^{br}(Y_e Y_e^\dagger)^{pa} - \frac{25}{24}\delta^{pa}(Y_e Y_e^\dagger Y_e)^{br} - \frac{3}{2}\delta^{pa}\lambda Y_e^{br} \Big\} C_{H\ell}^{(\times)ab} + \left\{ \frac{5}{24}Y_e^{pa}(Y_e^\dagger Y_e)^{br} + g_Y^2 \left( \frac{19}{36}\delta^{rb}Y_e^{pa} + \frac{7}{2}\delta^{ab}Y_e^{pr} \right) + \frac{3}{2}\delta^{rb}g_L^2Y_e^{pa} + \frac{41}{24}\delta^{rb}(Y_e Y_e^\dagger Y_e)^{pa} \right. \\
& - \frac{3}{2}\delta^{rb}\lambda Y_e^{pa} \Big\} C_{He}^{ab} - \delta^{ab}g_Y^2C_{Hq}^{(\parallel)ab}Y_e^{pr} + \left\{ \frac{3}{2}\delta^{ab}g_L^2Y_e^{pr} - \frac{1}{2}\delta^{ab}g_Y^2Y_e^{pr} \right\} C_{Hq}^{(\times)ab} + 3\delta^{ab}g_Y^2C_{Hu}^{ab}Y_e^{pr} + \frac{3}{2}\delta^{ab}g_Y^2C_{Hd}^{ab}Y_e^{pr} + \left\{ \frac{7}{12}Y_e^{*ad}Y_e^{pc}Y_e^{br} \right. \\
& + g_Y^2 \left( \frac{15}{2}\delta^{pa}\delta^{rd}Y_e^{bc} - \frac{55}{18}\delta^{rd}\delta^{ab}Y_e^{pc} - \frac{97}{18}\delta^{pa}\delta^{cd}Y_e^{br} \right) + \frac{7}{6}\delta^{pa}Y_e^{bc}(Y_e^\dagger Y_e)^{dr} + \frac{5}{3}\delta^{rd}Y_e^{bc}(Y_e Y_e^\dagger)^{pa} - \frac{3}{2}Y_e^{*ad}Y_e^{pr}Y_e^{bc} - \frac{3}{2}\delta^{pa}Y_e^{br}(Y_e^\dagger Y_e)^{dc} - \frac{3}{2}\delta^{rd}Y_e^{pc}(Y_e Y_e^\dagger)^{ba} \\
& - \frac{3}{2}\delta^{pa}\delta^{rd}Y_e^{bc}\text{Tr}[Y_e^\dagger Y_e] - \frac{9}{4}\delta^{pa}\delta^{rd}(Y_e Y_e^\dagger Y_e)^{bc} \Big\} C_{\ell e}^{abcd} - \left\{ 4\delta^{pa}Y_e^{br}(Y_u^\dagger Y_u)^{dc} + \frac{53}{9}\delta^{pa}\delta^{cd}g_Y^2Y_e^{br} \right\} C_{\ell u}^{abcd} - \left\{ \frac{1}{4}\delta^{pa}Y_e^{br}(Y_d^\dagger Y_d)^{dc} \right. \\
& + \frac{37}{18}\delta^{pa}\delta^{cd}g_Y^2Y_e^{br} \Big\} C_{\ell d}^{abcd} + \left\{ \frac{7}{18}\delta^{rd}\delta^{ab}g_Y^2Y_e^{pc} - \frac{1}{4}\delta^{rd}Y_e^{pc}(Y_d Y_d^\dagger)^{ba} - \delta^{rd}Y_e^{pc}(Y_u Y_u^\dagger)^{ba} \right\} C_{qe}^{abcd} + \frac{106}{9}\delta^{rb}\delta^{ad}g_Y^2C_{ee}^{abcd}Y_e^{pc} + \left\{ \frac{67}{9}\delta^{rb}\delta^{cd}g_Y^2Y_e^{pa} \right. \\
& - 4\delta^{rb}Y_e^{pa}(Y_u^\dagger Y_u)^{dc} \Big\} C_{eu}^{abcd} + \left\{ \frac{5}{18}\delta^{rb}\delta^{cd}g_Y^2Y_e^{pa} - \frac{1}{4}\delta^{rb}Y_e^{pa}(Y_d^\dagger Y_d)^{dc} \right\} C_{ed}^{abcd} + \left\{ \frac{19}{16}\delta^{pa}\delta^{rb}g_Y^2Y_d^{dc} + \frac{9}{4}\delta^{pa}\delta^{rb}Y_d^{dc}\text{Tr}[Y_e^\dagger Y_e] - \frac{1}{4}\delta^{rb}Y_d^{dc}(Y_e Y_e^\dagger)^{pa} \right. \\
& - \frac{5}{8}\delta^{pa}Y_d^{dc}(Y_e^\dagger Y_e)^{br} - \frac{15}{16}\delta^{pa}\delta^{rb}g_L^2Y_d^{dc} \Big\} C_{\ell edq}^{abcd} + C_{\ell edq}^{*abcd} \left\{ \frac{9}{4}Y_d^{*dc}Y_e^{pr}Y_e^{ab} - \frac{7}{8}Y_d^{*dc}Y_e^{pb}Y_e^{ar} \right\} + \left\{ \frac{1}{4}\delta^{rb}Y_u^{*cd}(Y_e Y_e^\dagger)^{pa} + \frac{5}{8}\delta^{pa}Y_u^{*cd}(Y_e^\dagger Y_e)^{br} \right. \\
& + \frac{15}{8}\delta^{pa}\delta^{rb}g_L^2Y_u^{*cd} + \frac{25}{8}\delta^{pa}\delta^{rb}g_Y^2Y_u^{*cd} - \frac{9}{4}\delta^{pa}\delta^{rb}Y_u^{*cd}\text{Tr}[Y_e^\dagger Y_e] \Big\} C_{\ell equ}^{abcd} + C_{\ell equ}^{*abcd} \left\{ \frac{7}{8}Y_e^{pb}Y_e^{ar}Y_u^{cd} - \frac{9}{4}Y_e^{pr}Y_e^{ab}Y_u^{cd} \right\} + \left\{ \frac{9}{8}\delta^{pa}\delta^{rd}Y_u^{*cb}\text{Tr}[Y_e^\dagger Y_e] \right. \\
& + \frac{33}{16}\delta^{pa}\delta^{rd}(Y_d^\dagger Y_d Y_u^\dagger)^{cb} + \frac{65}{6}\delta^{pa}\delta^{rd}g_s^2Y_u^{*cb} - \frac{1}{8}\delta^{rd}Y_u^{*cb}(Y_e Y_e^\dagger)^{pa} - \frac{5}{16}\delta^{pa}Y_u^{*cb}(Y_e^\dagger Y_e)^{dr} - \frac{63}{32}\delta^{pa}\delta^{rd}g_L^2Y_u^{*cb} - \frac{865}{288}\delta^{pa}\delta^{rd}g_Y^2Y_u^{*cb} \\
& - \frac{69}{16}\delta^{pa}\delta^{rd}(Y_u^\dagger Y_u Y_u^\dagger)^{cb} \Big\} C_{\ell uqe}^{abcd} + C_{\ell uqe}^{*abcd} \left\{ \frac{9}{8}Y_e^{pr}Y_e^{ad}Y_u^{cb} - \frac{11}{8}Y_e^{pd}Y_e^{ar}Y_u^{cb} \right\} + \left\{ g_Y^2 \left( \frac{19}{9}\delta^{pa}\delta^{bc}Y_e^{dr} + \frac{38}{9}\delta^{pa}\delta^{cd}Y_e^{br} \right) + \frac{4}{3}\delta^{pa}\delta^{bc}g_L^2Y_e^{dr} \right\} C_{\ell\ell}^{abcd}
\end{aligned}$$

$$\begin{aligned}
& + \left\{ \frac{11}{9} \delta^{pa} \delta^{cd} g_Y^2 Y_e^{br} - \frac{1}{4} \delta^{pa} Y_e^{br} (Y_d Y_d^\dagger)^{dc} - \delta^{pa} Y_e^{br} (Y_u Y_u^\dagger)^{dc} \right\} C_{\ell q}^{(\parallel)abcd} + \left\{ \frac{11}{18} \delta^{pa} \delta^{cd} g_Y^2 Y_e^{br} + \delta^{pa} Y_e^{br} (Y_u Y_u^\dagger)^{dc} - \frac{1}{2} \delta^{pa} Y_e^{br} (Y_d Y_d^\dagger)^{dc} \right. \\
& \left. - \delta^{pa} \delta^{cd} g_L^2 Y_e^{br} \right\} C_{\ell q}^{(\times)abcd},
\end{aligned} \tag{8.2}$$

## 8.2 $C_{eW}$

$$\begin{aligned}
\beta_{C_{eW}^{pr}}^{(1)} &= 2g_L^2 C_{HW} Y_e^{pr} - 2ig_L^2 C_{H\widetilde{W}} Y_e^{pr} - \frac{3}{2} g_Y^2 C_{HWB} Y_e^{pr} + \frac{3i}{2} g_Y^2 C_{H\widetilde{W}B} Y_e^{pr} - \delta^{pa} \delta^{rb} g_Y^2 C_{eB}^{ab} + \left\{ \frac{1}{4} \delta^{pa} \delta^{rb} g_Y^2 + \frac{1}{2} \left( \delta^{rb} (Y_e Y_e^\dagger)^{pa} + 2T_2 \delta^{pa} \delta^{rb} \right. \right. \\
& \left. \left. + 4\delta^{pa} (Y_e^\dagger Y_e)^{br} \right) + \frac{9}{4} \delta^{pa} \delta^{rb} g_L^2 \right\} C_{eW}^{ab} - \frac{3}{2} \delta^{pa} \delta^{rd} Y_u^{*cb} C_{\ell uqe}^{abcd},
\end{aligned} \tag{8.3}$$

$$\begin{aligned}
\beta_{C_{eW}^{pr}}^{(2)} &= -8(C_{\ell LHH}^\dagger C_{\ell LHH} Y_e)^{pr} - \frac{1}{2} g_Y^2 C_{HD}^{(\parallel)} Y_e^{pr} + \left\{ \frac{1}{8} g_L^2 Y_e^{pr} + \frac{1}{8} g_Y^2 Y_e^{pr} \right\} C_{HD}^{(\times)} - \frac{13}{4} g_Y^4 C_{HB} Y_e^{pr} + \frac{13i}{4} g_Y^4 C_{H\widetilde{B}} Y_e^{pr} + \left\{ \frac{271}{18} g_L^4 Y_e^{pr} - g_L^2 (T_2 Y_e^{pr} \right. \\
& \left. + \frac{9}{2} (Y_e Y_e^\dagger Y_e)^{pr}) - 3\lambda g_L^2 Y_e^{pr} - \frac{23}{4} g_Y^2 g_L^2 Y_e^{pr} \right\} C_{HW} + \left\{ g_L^2 (iT_2 Y_e^{pr} + \frac{9i}{2} (Y_e Y_e^\dagger Y_e)^{pr}) + 3i\lambda g_L^2 Y_e^{pr} + \frac{23i}{4} g_Y^2 g_L^2 Y_e^{pr} - \frac{559i}{18} g_L^4 Y_e^{pr} \right\} C_{H\widetilde{W}} \\
& + \left\{ \frac{3}{4} \lambda g_Y^2 Y_e^{pr} + g_Y^2 \left( \frac{3}{4} T_2 Y_e^{pr} + \frac{27}{8} (Y_e Y_e^\dagger Y_e)^{pr} \right) + \frac{301}{48} g_Y^4 Y_e^{pr} - \frac{43}{16} g_Y^2 g_L^2 Y_e^{pr} \right\} C_{HWB} + \left\{ g_Y^2 \left( -\frac{3i}{4} T_2 Y_e^{pr} - \frac{27i}{8} (Y_e Y_e^\dagger Y_e)^{pr} \right) \right. \\
& \left. + \frac{43i}{16} g_Y^2 g_L^2 Y_e^{pr} - \frac{3i}{4} \lambda g_Y^2 Y_e^{pr} - \frac{301i}{48} g_Y^4 Y_e^{pr} \right\} C_{H\widetilde{W}B} + \left\{ 35g_L^6 Y_e^{pr} - \frac{3}{2} g_Y^2 g_L^4 Y_e^{pr} - \frac{3}{2} g_L^4 (Y_e Y_e^\dagger Y_e)^{pr} \right\} C_W + \left\{ \frac{5i}{6} g_L^4 (Y_e Y_e^\dagger Y_e)^{pr} \right. \\
& \left. + \frac{11i}{6} g_Y^2 g_L^4 Y_e^{pr} - \frac{184i}{9} g_L^6 Y_e^{pr} \right\} C_{\widetilde{W}} + \left\{ \frac{1}{4} \delta^{pa} (Y_e^\dagger Y_e)^{br} + \frac{3}{4} \delta^{pa} \delta^{rb} g_L^2 - \frac{1}{4} \delta^{rb} (Y_e Y_e^\dagger)^{pa} - \frac{3}{4} \delta^{pa} \delta^{rb} g_Y^2 \right\} C_{eH}^{ab} + \left\{ g_Y^2 \left( \frac{17}{4} \delta^{rb} (Y_e Y_e^\dagger)^{pa} - \frac{1}{4} \delta^{pa} (Y_e^\dagger Y_e)^{br} \right. \right. \\
& \left. \left. - \delta^{pa} \delta^{rb} \text{Tr}[Y_u^\dagger Y_u] - \frac{5}{2} \delta^{pa} \delta^{rb} \text{Tr}[Y_e^\dagger Y_e] - 3Y_e^{*ab} Y_e^{pr} - \frac{7}{2} \delta^{pa} \delta^{rb} \text{Tr}[Y_d^\dagger Y_d] \right) + \frac{25}{8} \delta^{pa} \delta^{rb} g_Y^2 g_L^2 + \frac{1645}{72} \delta^{pa} \delta^{rb} g_Y^4 - \delta^{pa} \delta^{rb} \lambda g_Y^2 \right\} C_{eB}^{ab} \\
& + \left\{ g_L^2 \left( \frac{1}{8} \delta^{pa} \delta^{rb} \text{Tr}[Y_e^\dagger Y_e] + \frac{3}{8} \delta^{pa} \delta^{rb} \text{Tr}[Y_d^\dagger Y_d] + \frac{9}{8} \delta^{pa} \delta^{rb} \text{Tr}[Y_u^\dagger Y_u] + \frac{7}{4} Y_e^{*ab} Y_e^{pr} + \frac{63}{16} \delta^{rb} (Y_e Y_e^\dagger)^{pa} + \frac{103}{8} \delta^{pa} (Y_e^\dagger Y_e)^{br} \right) + g_Y^2 \left( \frac{25}{24} \delta^{pa} \delta^{rb} \text{Tr}[Y_d^\dagger Y_d] \right. \right. \\
& \left. \left. + \frac{25}{8} \delta^{pa} \delta^{rb} \text{Tr}[Y_e^\dagger Y_e] + \frac{85}{24} \delta^{pa} \delta^{rb} \text{Tr}[Y_u^\dagger Y_u] + 4\delta^{pa} (Y_e^\dagger Y_e)^{br} + \frac{27}{4} Y_e^{*ab} Y_e^{pr} - \frac{25}{16} \delta^{rb} (Y_e Y_e^\dagger)^{pa} \right) + g_s^2 \left( 20\delta^{pa} \delta^{rb} \text{Tr}[Y_d^\dagger Y_d] + 20\delta^{pa} \delta^{rb} \text{Tr}[Y_u^\dagger Y_u] \right) \\
& \left. + \frac{5}{4} \delta^{pa} (Y_e^\dagger Y_e Y_e^\dagger Y_e)^{br} + \frac{3}{2} \delta^{pa} \delta^{rb} \lambda^2 + \frac{3}{2} \delta^{pa} \delta^{rb} \text{Tr}[Y_d^\dagger Y_d Y_u^\dagger Y_u] + \frac{7}{4} \delta^{rb} (Y_e Y_e^\dagger Y_e Y_e^\dagger)^{pa} + \frac{161}{16} \delta^{pa} \delta^{rb} g_L^4 - \frac{3}{4} T_2 \delta^{rb} (Y_e Y_e^\dagger)^{pa} - \lambda \left( \frac{3}{2} \delta^{pa} \delta^{rb} g_L^2 \right. \right.
\end{aligned}$$

$$\begin{aligned}
& + 2\delta^{rb}(Y_e Y_e^\dagger)^{pa} + 6\delta^{pa}(Y_e^\dagger Y_e)^{br} - 2(Y_e^\dagger Y_e)^{br}(Y_e Y_e^\dagger)^{pa} - \frac{9}{4}T_4\delta^{pa}\delta^{rb} - 3T_2\delta^{pa}(Y_e^\dagger Y_e)^{br} - \frac{63}{16}\delta^{pa}\delta^{rb}g_Y^2g_L^2 - \frac{1549}{72}\delta^{pa}\delta^{rb}g_Y^4 \Big\} C_{eW}^{ab} \\
& - \frac{9}{2}g_Y^2 C_{uB}^{*ab} Y_e^{pr} Y_u^{ab} + \left\{ \frac{3}{4}g_L^2 Y_u^{*ab} Y_e^{pr} - \frac{15}{4}g_Y^2 Y_u^{*ab} Y_e^{pr} \right\} C_{uW}^{ab} + \frac{3}{4}g_L^2 C_{uW}^{*ab} Y_e^{pr} Y_u^{ab} - 9g_Y^2 Y_d^{*ab} C_{dB}^{ab} Y_e^{pr} + \left\{ \frac{9}{4}g_Y^2 Y_d^{*ab} Y_e^{pr} \right. \\
& + \left. \frac{21}{4}g_L^2 Y_d^{*ab} Y_e^{pr} \right\} C_{dW}^{ab} + \left\{ g_L^2(\delta^{ab}Y_e^{pr} - 5\delta^{pa}Y_e^{br}) + g_Y^2(\delta^{ab}Y_e^{pr} - \frac{5}{9}\delta^{pa}Y_e^{br}) - \frac{1}{12}\delta^{pa}(Y_e Y_e^\dagger Y_e)^{br} - \delta^{pa}\lambda Y_e^{br} - \frac{19}{12}Y_e^{br}(Y_e Y_e^\dagger)^{pa} \right\} C_{H\ell}^{(\parallel)ab} \\
& + \left\{ g_L^2(\delta^{ab}Y_e^{pr} + \frac{7}{3}\delta^{pa}Y_e^{br}) + g_Y^2(2\delta^{ab}Y_e^{pr} - \frac{7}{9}\delta^{pa}Y_e^{br}) + \frac{25}{12}\delta^{pa}(Y_e Y_e^\dagger Y_e)^{br} - \frac{5}{12}Y_e^{br}(Y_e Y_e^\dagger)^{pa} - 2\delta^{pa}\lambda Y_e^{br} \right\} C_{H\ell}^{(\times)ab} + \left\{ \frac{3}{4}\delta^{rb}(Y_e Y_e^\dagger Y_e)^{pa} \right. \\
& + g_Y^2(\delta^{ab}Y_e^{pr} - \frac{5}{6}\delta^{rb}Y_e^{pa}) - \frac{1}{2}\delta^{rb}g_L^2 Y_e^{pa} - \frac{3}{4}Y_e^{pa}(Y_e^\dagger Y_e)^{br} - \delta^{rb}\lambda Y_e^{pa} \Big\} C_{He}^{ab} + \left\{ 3\delta^{ab}g_L^2 Y_e^{pr} - \delta^{ab}g_Y^2 Y_e^{pr} \right\} C_{Hq}^{(\parallel)ab} + \left\{ 3\delta^{ab}g_L^2 Y_e^{pr} \right. \\
& - 2\delta^{ab}g_Y^2 Y_e^{pr} \Big\} C_{Hq}^{(\times)ab} - 2\delta^{ab}g_Y^2 C_{Hu}^{ab} Y_e^{pr} + \delta^{ab}g_Y^2 C_{Hd}^{ab} Y_e^{pr} + \left\{ \frac{1}{6}Y_e^{*ad}Y_e^{pc}Y_e^{br} + Y_e^{*ad}Y_e^{pr}Y_e^{bc} + g_L^2(2\delta^{rd}\delta^{ab}Y_e^{pc} - \delta^{pa}\delta^{rd}Y_e^{bc}) + g_Y^2(\frac{1}{9}\delta^{pa}\delta^{cd}Y_e^{br} \right. \\
& - \left. \frac{1}{3}\delta^{rd}\delta^{ab}Y_e^{pc} - 5\delta^{pa}\delta^{rd}Y_e^{bc}) + \delta^{pa}Y_e^{br}(Y_e^\dagger Y_e)^{dc} + \delta^{rd}Y_e^{pc}(Y_e Y_e^\dagger)^{ba} + \delta^{pa}\delta^{rd}Y_e^{bc}\text{Tr}[Y_e^\dagger Y_e] + \frac{3}{2}\delta^{pa}\delta^{rd}(Y_e Y_e^\dagger Y_e)^{bc} - \frac{1}{3}\delta^{pa}Y_e^{bc}(Y_e^\dagger Y_e)^{dr} \right\} C_{\ell e}^{abcd} \\
& - \frac{2}{9}\delta^{pa}\delta^{cd}g_Y^2 C_{\ell u}^{abcd} Y_e^{br} + \left\{ \frac{1}{9}\delta^{pa}\delta^{cd}g_Y^2 Y_e^{br} + \frac{3}{2}\delta^{pa}Y_e^{br}(Y_d^\dagger Y_d)^{dc} \right\} C_{\ell d}^{abcd} + \left\{ \frac{1}{3}\delta^{rd}\delta^{ab}g_Y^2 Y_e^{pc} + \frac{3}{2}\delta^{rd}Y_e^{pc}(Y_d Y_d^\dagger)^{ba} + 6\delta^{rd}\delta^{ab}g_L^2 Y_e^{pc} \right. \\
& + \left. 6\delta^{rd}Y_e^{pc}(Y_u Y_u^\dagger)^{ba} \right\} C_{qe}^{abcd} - \frac{4}{3}\delta^{rb}\delta^{ad}g_Y^2 C_{ee}^{abcd} Y_e^{pc} + \frac{2}{3}\delta^{rb}\delta^{cd}g_Y^2 C_{eu}^{abcd} Y_e^{pa} + \left\{ \frac{3}{2}\delta^{rb}Y_e^{pa}(Y_d^\dagger Y_d)^{dc} - \frac{1}{3}\delta^{rb}\delta^{cd}g_Y^2 Y_e^{pa} \right\} C_{ed}^{abcd} + \left\{ \frac{15}{8}\delta^{pa}\delta^{rb}g_Y^2 Y_d^{dc} \right. \\
& - \left. \frac{1}{4}\delta^{pa}Y_d^{dc}(Y_e^\dagger Y_e)^{br} - \frac{3}{2}\delta^{pa}\delta^{rb}Y_d^{dc}\text{Tr}[Y_e^\dagger Y_e] - \frac{15}{8}\delta^{pa}\delta^{rb}g_L^2 Y_d^{dc} \right\} C_{ledq}^{abcd} - C_{ledq}^{*abcd} \left\{ \frac{1}{4}Y_d^{*dc}Y_e^{pb}Y_e^{ar} + \frac{3}{2}Y_d^{*dc}Y_e^{pr}Y_e^{ab} \right\} + \left\{ \frac{1}{4}\delta^{pa}Y_u^{*cd}(Y_e^\dagger Y_e)^{br} \right. \\
& + \left. \frac{3}{2}\delta^{pa}\delta^{rb}Y_u^{*cd}\text{Tr}[Y_e^\dagger Y_e] + \frac{9}{4}\delta^{pa}\delta^{rb}g_L^2 Y_u^{*cd} - \frac{15}{4}\delta^{pa}\delta^{rb}g_Y^2 Y_u^{*cd} \right\} C_{lequ}^{abcd} + C_{lequ}^{*abcd} \left\{ \frac{1}{4}Y_e^{pb}Y_e^{ar}Y_u^{cd} + \frac{3}{2}Y_e^{pr}Y_e^{ab}Y_u^{cd} \right\} + \left\{ \frac{17}{48}\delta^{pa}\delta^{rd}g_Y^2 Y_u^{*cb} \right. \\
& + \left. \frac{27}{8}\delta^{pa}\delta^{rd}(Y_u^\dagger Y_u Y_u^\dagger)^{cb} - \frac{1}{8}\delta^{pa}Y_u^{*cb}(Y_e^\dagger Y_e)^{dr} - \frac{3}{4}\delta^{pa}\delta^{rd}Y_u^{*cb}\text{Tr}[Y_e^\dagger Y_e] - \frac{15}{8}\delta^{pa}\delta^{rd}(Y_d^\dagger Y_d Y_u^\dagger)^{cb} - \frac{123}{16}\delta^{pa}\delta^{rd}g_L^2 Y_u^{*cb} \right. \\
& - \left. 13\delta^{pa}\delta^{rd}g_s^2 Y_u^{*cb} \right\} C_{luqe}^{abcd} + C_{luqe}^{*abcd} \left\{ \frac{1}{4}Y_e^{pd}Y_e^{ar}Y_u^{cb} - \frac{3}{4}Y_e^{pr}Y_e^{ad}Y_u^{cb} \right\} + \left\{ g_Y^2\left(\frac{2}{9}\delta^{pa}\delta^{cd}Y_e^{br} - \frac{44}{9}\delta^{pa}\delta^{bc}Y_e^{dr}\right) - g_L^2\left(2\delta^{pa}\delta^{cd}Y_e^{br} + \frac{8}{3}\delta^{pa}\delta^{bc}Y_e^{dr}\right) \right. \\
& - \left. 2\delta^{pa}Y_e^{dr}(Y_e Y_e^\dagger)^{bc} \right\} C_{\ell\ell}^{abcd} + \left\{ \frac{3}{2}\delta^{pa}Y_e^{br}(Y_d Y_d^\dagger)^{dc} + 6\delta^{pa}Y_e^{br}(Y_u Y_u^\dagger)^{dc} - \frac{1}{9}\delta^{pa}\delta^{cd}g_Y^2 Y_e^{br} - 3\delta^{pa}\delta^{cd}g_L^2 Y_e^{br} \right\} C_{\ell q}^{(\parallel)abcd} + \left\{ \frac{22}{9}\delta^{pa}\delta^{cd}g_Y^2 Y_e^{br} \right.
\end{aligned}$$

$$+ 3\delta^{pa}Y_e^{br}(Y_uY_u^\dagger)^{dc} - 4\delta^{pa}\delta^{cd}g_L^2Y_e^{br}\Big\}C_{\ell q}^{(\times)abcd}, \quad (8.4)$$

### 8.3 $C_{uB}$

$$\begin{aligned} \beta_{C_{uB}^{pr}}^{(1)} = & \frac{5}{3}g_Y^2C_{HB}Y_u^{pr} - \frac{5i}{3}g_Y^2C_{H\tilde{B}}Y_u^{pr} - \frac{3}{4}g_L^2C_{HWB}Y_u^{pr} + \frac{3i}{4}g_L^2C_{H\tilde{W}B}Y_u^{pr} + \left\{\frac{1}{2}\left(2T_2\delta^{pa}\delta^{rb} + 4\delta^{pa}(Y_u^\dagger Y_u)^{br} + 5\delta^{rb}(Y_uY_u^\dagger)^{pa} - 3\delta^{rb}(Y_dY_d^\dagger)^{pa}\right)\right. \\ & + \frac{67}{36}\delta^{pa}\delta^{rb}g_Y^2 + \frac{8}{3}\delta^{pa}\delta^{rb}g_s^2 - \frac{9}{4}\delta^{pa}\delta^{rb}g_L^2\Big\}C_{uB}^{ab} - \frac{1}{4}\delta^{pa}\delta^{rb}g_L^2C_{uW}^{ab} + \frac{40}{9}\delta^{pa}\delta^{rb}g_s^2C_{uG}^{ab} - \delta^{pa}C_{dB}^{ab}(Y_d^\dagger Y_u)^{br} - \frac{1}{12}\delta^{pc}\delta^{rb}Y_d^{*ad}C_{quqd}^{(\parallel)abcd} \\ & - \frac{1}{4}\delta^{pc}\delta^{rb}Y_d^{*ad}C_{quqd}^{(\times)abcd} - \frac{3}{4}\delta^{pc}\delta^{rb}Y_e^{*ad}C_{\ell uqe}^{abcd}, \end{aligned} \quad (8.5)$$

$$\begin{aligned} \beta_{C_{uB}^{pr}}^{(2)} = & \left\{\frac{1}{6}(Y_dY_d^\dagger Y_u)^{pr} - \frac{5}{72}g_Y^2Y_u^{pr} - \frac{1}{8}(Y_uY_u^\dagger Y_u)^{pr} - \frac{1}{4}g_L^2Y_u^{pr}\right\}C_{HD}^{(\parallel)} + \left\{\frac{1}{8}(Y_uY_u^\dagger Y_u)^{pr} + \frac{25}{144}g_Y^2Y_u^{pr} + \frac{3}{16}g_L^2Y_u^{pr} - \frac{1}{6}(Y_dY_d^\dagger Y_u)^{pr}\right\}C_{HD}^{(\times)} \\ & + \left\{\frac{5}{8}g_Y^2g_L^2Y_u^{pr} + g_Y^2\left(\frac{19}{12}(Y_dY_d^\dagger Y_u)^{pr} - \frac{5}{6}T_2Y_u^{pr} - \frac{21}{4}(Y_uY_u^\dagger Y_u)^{pr}\right) - \frac{5}{2}\lambda g_Y^2Y_u^{pr} - \frac{415}{108}g_Y^4Y_u^{pr} - \frac{40}{3}g_Y^2g_s^2Y_u^{pr}\right\}C_{HB} + \left\{g_Y^2\left(\frac{5i}{6}T_2Y_u^{pr}\right.\right. \\ & + \frac{21i}{4}(Y_uY_u^\dagger Y_u)^{pr} - \frac{23i}{12}(Y_dY_d^\dagger Y_u)^{pr}\Big) + \frac{5i}{2}\lambda g_Y^2Y_u^{pr} + \frac{415i}{108}g_Y^4Y_u^{pr} + \frac{40i}{3}g_Y^2g_s^2Y_u^{pr} - \frac{5i}{8}g_Y^2g_L^2Y_u^{pr}\Big\}C_{H\tilde{B}} - \frac{5}{8}g_L^4C_{HW}Y_u^{pr} \\ & + \frac{5i}{8}g_L^4C_{H\tilde{W}}Y_u^{pr} - \frac{20}{3}g_s^4C_{HG}Y_u^{pr} + \frac{20i}{3}g_s^4C_{H\tilde{G}}Y_u^{pr} + \left\{\frac{3}{8}\lambda g_L^2Y_u^{pr} + g_L^2\left(\frac{3}{8}T_2Y_u^{pr} + \frac{9}{16}(Y_uY_u^\dagger Y_u)^{pr} + \frac{15}{16}(Y_dY_d^\dagger Y_u)^{pr}\right) + \frac{43}{32}g_Y^2g_L^2Y_u^{pr}\right. \\ & + 6g_s^2g_L^2Y_u^{pr} - \frac{425}{96}g_L^4Y_u^{pr}\Big\}C_{HWB} + \left\{g_L^2\left(-\frac{3i}{16}(Y_dY_d^\dagger Y_u)^{pr} - \frac{3i}{8}T_2Y_u^{pr} - \frac{9i}{16}(Y_uY_u^\dagger Y_u)^{pr}\right) + \frac{425i}{96}g_L^4Y_u^{pr} - \frac{3i}{8}\lambda g_L^2Y_u^{pr}\right. \\ & - \frac{43i}{32}g_Y^2g_L^2Y_u^{pr} - 6ig_s^2g_L^2Y_u^{pr}\Big\}C_{H\tilde{W}B} + \frac{15}{4}g_L^6C_WY_u^{pr} - \frac{25i}{12}g_L^6C_{\tilde{W}}Y_u^{pr} - 10g_s^6C_GY_u^{pr} + \frac{130i}{9}g_s^6C_{\tilde{G}}Y_u^{pr} + \left\{\frac{5}{8}\delta^{pa}\delta^{rb}g_Y^2 + \frac{5}{8}\delta^{pa}(Y_u^\dagger Y_u)^{br}\right. \\ & + \frac{5}{8}\delta^{rb}(Y_uY_u^\dagger)^{pa} - \frac{3}{8}\delta^{pa}\delta^{rb}g_L^2\Big\}C_{uH}^{ab} + \left\{\frac{3}{4}g_L^2Y_e^{*ab}Y_u^{pr} + \frac{5}{4}g_Y^2Y_e^{*ab}Y_u^{pr}\right\}C_{eB}^{ab} + \frac{5}{4}g_Y^2C_{eB}^{*ab}Y_e^{ab}Y_u^{pr} - \frac{9}{8}g_L^2C_{eW}^{*ab}Y_e^{ab}Y_u^{pr} + \left\{g_L^2\left(\frac{9}{16}\delta^{rb}(Y_dY_d^\dagger)^{pa}\right.\right. \\ & + \frac{15}{8}T_2\delta^{pa}\delta^{rb} + \frac{27}{4}Y_u^{*ab}Y_u^{pr} + 9\delta^{pa}(Y_u^\dagger Y_u)^{br} + \frac{237}{16}\delta^{rb}(Y_uY_u^\dagger)^{pa}\Big) + g_Y^2\left(\frac{151}{144}\delta^{rb}(Y_dY_d^\dagger)^{pa} + \frac{181}{72}\delta^{pa}(Y_u^\dagger Y_u)^{br} + \frac{33}{8}\delta^{pa}\delta^{rb}\text{Tr}[Y_u^\dagger Y_u]\right. \\ & + \frac{125}{12}Y_u^{*ab}Y_u^{pr} - \frac{83}{144}\delta^{rb}(Y_uY_u^\dagger)^{pa} - \frac{17}{8}\delta^{pa}\delta^{rb}\text{Tr}[Y_d^\dagger Y_d] - \frac{19}{8}\delta^{pa}\delta^{rb}\text{Tr}[Y_e^\dagger Y_e]\Big) + g_s^2\left(20\delta^{pa}\delta^{rb}\text{Tr}[Y_d^\dagger Y_d] + 20\delta^{pa}\delta^{rb}\text{Tr}[Y_u^\dagger Y_u]\right. \\ & - \frac{16}{3}\delta^{rb}(Y_dY_d^\dagger)^{pa} - \frac{16}{3}\delta^{rb}(Y_uY_u^\dagger)^{pa} - \frac{32}{3}\delta^{pa}(Y_u^\dagger Y_u)^{br}\Big) + \frac{5}{4}T_2\delta^{rb}(Y_dY_d^\dagger)^{pa} + \frac{5}{4}\delta^{pa}(Y_u^\dagger Y_uY_u^\dagger Y_u)^{br} + \frac{5}{4}\delta^{rb}(Y_uY_u^\dagger Y_uY_u^\dagger)^{pa} + \frac{3}{2}\delta^{pa}\delta^{rb}\lambda^2 \end{aligned}$$

$$\begin{aligned}
& + \frac{3}{2} \delta^{pa} \delta^{rb} \text{Tr} [Y_d^\dagger Y_d Y_u^\dagger Y_u] + \frac{11}{4} \delta^{rb} (Y_d Y_d^\dagger Y_d Y_d^\dagger)^{pa} + \frac{199}{48} \delta^{pa} \delta^{rb} g_Y^2 g_L^2 + \frac{172}{3} \delta^{pa} \delta^{rb} g_s^4 - \frac{1}{4} \delta^{pa} (Y_u^\dagger Y_d Y_d^\dagger Y_u)^{br} - \frac{1}{2} \delta^{rb} (Y_u Y_u^\dagger Y_d Y_d^\dagger)^{pa} \\
& - \lambda \left( \frac{3}{2} \delta^{pa} \delta^{rb} g_Y^2 + 6 \delta^{pa} (Y_u^\dagger Y_u)^{br} + 6 \delta^{rb} (Y_u Y_u^\dagger)^{pa} \right) - \delta^{rb} (Y_d Y_d^\dagger Y_u Y_u^\dagger)^{pa} - \frac{9}{4} \text{T}_4 \delta^{pa} \delta^{rb} - 3 \text{T}_2 \delta^{pa} (Y_u^\dagger Y_u)^{br} - 3 (Y_u^\dagger Y_u)^{br} (Y_u Y_u^\dagger)^{pa} \\
& - \frac{15}{4} \text{T}_2 \delta^{rb} (Y_u Y_u^\dagger)^{pa} - \frac{23}{4} \delta^{pa} \delta^{rb} g_L^4 - 7 \delta^{pa} \delta^{rb} g_s^2 g_L^2 - \frac{451}{27} \delta^{pa} \delta^{rb} g_Y^2 g_s^2 - \frac{25853}{1296} \delta^{pa} \delta^{rb} g_Y^4 \Big\} C_{uB}^{ab} + C_{uB}^{*ab} \Big\{ \frac{1}{2} Y_u^{pb} (Y_d Y_d^\dagger Y_u)^{ar} \\
& - \frac{1}{2} Y_u^{ar} (Y_d Y_d^\dagger Y_u)^{pb} \Big\} + \Big\{ \frac{3}{4} \delta^{pa} \delta^{rb} \lambda g_L^2 + g_L^2 \left( \frac{7}{16} \delta^{pa} (Y_u^\dagger Y_u)^{br} + \frac{15}{4} Y_u^{*ab} Y_u^{pr} + \frac{15}{4} \delta^{pa} \delta^{rb} \text{Tr} [Y_d^\dagger Y_d] + \frac{33}{8} \delta^{pa} \delta^{rb} \text{Tr} [Y_u^\dagger Y_u] - \frac{5}{16} \delta^{rb} (Y_u Y_u^\dagger)^{pa} \right. \\
& - \frac{3}{4} \delta^{pa} \delta^{rb} \text{Tr} [Y_e^\dagger Y_e] - 2 \delta^{rb} (Y_d Y_d^\dagger)^{pa} \Big) - \frac{73}{288} \delta^{pa} \delta^{rb} g_Y^2 g_L^2 - \frac{941}{288} \delta^{pa} \delta^{rb} g_L^4 - \frac{14}{3} \delta^{pa} \delta^{rb} g_s^2 g_L^2 \Big\} C_{uW}^{ab} + \Big\{ g_s^2 \left( \frac{16}{9} \delta^{rb} (Y_d Y_d^\dagger)^{pa} - \frac{26}{9} \delta^{rb} (Y_u Y_u^\dagger)^{pa} \right. \\
& - \frac{70}{9} \delta^{pa} (Y_u^\dagger Y_u)^{br} \Big) + \frac{820}{27} \delta^{pa} \delta^{rb} g_s^4 - \frac{5}{3} \delta^{pa} \delta^{rb} g_s^2 g_L^2 - \frac{205}{81} \delta^{pa} \delta^{rb} g_Y^2 g_s^2 \Big\} C_{uG}^{ab} + \Big\{ \frac{1}{2} \text{T}_2 \delta^{pa} (Y_d^\dagger Y_u)^{br} + g_L^2 \left( \frac{9}{4} Y_d^{*ab} Y_u^{pr} - \frac{39}{8} \delta^{pa} (Y_d^\dagger Y_u)^{br} \right) \\
& + g_Y^2 \left( \frac{5}{12} Y_d^{*ab} Y_u^{pr} + \frac{25}{24} \delta^{pa} (Y_d^\dagger Y_u)^{br} \right) + \frac{5}{2} (Y_d^\dagger Y_u)^{br} (Y_d Y_d^\dagger)^{pa} + \frac{5}{2} \delta^{pa} (Y_d^\dagger Y_d Y_d^\dagger Y_u)^{br} - \frac{1}{2} (Y_d^\dagger Y_u)^{br} (Y_u Y_u^\dagger)^{pa} - \delta^{pa} (Y_d^\dagger Y_u Y_u^\dagger Y_u)^{br} \Big\} C_{dB}^{ab} \\
& + C_{dB}^{*ab} \Big\{ \frac{1}{2} Y_d^{pb} (Y_d Y_d^\dagger Y_u)^{ar} + \text{T}_2 Y_d^{pb} Y_u^{ar} + g_Y^2 \left( \frac{5}{12} Y_d^{ab} Y_u^{pr} - \frac{17}{9} Y_d^{pb} Y_u^{ar} \right) + \frac{5}{2} Y_u^{ar} (Y_d Y_d^\dagger Y_d)^{pb} - Y_d^{pb} (Y_u Y_u^\dagger Y_u)^{ar} - 2 Y_u^{ar} (Y_u Y_u^\dagger Y_d)^{pb} - \frac{9}{4} g_L^2 Y_d^{pb} Y_u^{ar} \\
& - 8 g_s^2 Y_d^{pb} Y_u^{ar} \Big\} + \frac{1}{8} \delta^{pa} g_L^2 C_{dW}^{ab} (Y_d^\dagger Y_u)^{br} + g_L^2 C_{dW}^{*ab} \Big\{ \frac{5}{8} Y_d^{pb} Y_u^{ar} - \frac{3}{8} Y_d^{ab} Y_u^{pr} \Big\} - \frac{28}{9} g_s^2 C_{dG}^{*ab} Y_d^{pb} Y_u^{ar} - \frac{10}{9} \delta^{ab} g_Y^2 C_{H\ell}^{(\parallel)ab} Y_u^{pr} - \Big\{ \frac{5}{9} \delta^{ab} g_Y^2 Y_u^{pr} \\
& + \delta^{ab} g_L^2 Y_u^{pr} \Big\} C_{H\ell}^{(\times)ab} + \frac{25}{18} \delta^{ab} g_Y^2 C_{He}^{ab} Y_u^{pr} + \Big\{ \frac{1}{9} Y_u^{br} (Y_d Y_d^\dagger)^{pa} + \frac{1}{9} \delta^{pa} (Y_d Y_d^\dagger Y_u)^{br} - \frac{8}{81} \delta^{pa} g_Y^2 Y_u^{br} - \frac{1}{4} \delta^{pa} g_L^2 Y_u^{br} - \frac{29}{72} \delta^{pa} (Y_u Y_u^\dagger Y_u)^{br} \\
& - \frac{77}{72} Y_u^{br} (Y_u Y_u^\dagger)^{pa} - \frac{4}{3} \delta^{pa} g_s^2 Y_u^{br} - \frac{3}{2} \delta^{pa} \lambda Y_u^{br} \Big\} C_{Hq}^{(\parallel)ab} + \Big\{ \frac{1}{36} \delta^{pa} (Y_u Y_u^\dagger Y_u)^{br} + \frac{2}{9} Y_u^{br} (Y_d Y_d^\dagger)^{pa} + \frac{2}{9} \delta^{pa} (Y_d Y_d^\dagger Y_u)^{br} + \frac{157}{648} \delta^{pa} g_Y^2 Y_u^{br} + \frac{4}{3} \delta^{pa} g_s^2 Y_u^{br} \\
& - \frac{11}{36} Y_u^{br} (Y_u Y_u^\dagger)^{pa} - \frac{23}{72} \delta^{pa} g_L^2 Y_u^{br} \Big\} C_{Hq}^{(\times)ab} + \Big\{ \frac{5}{6} \delta^{rb} (Y_d Y_d^\dagger Y_u)^{pa} + \delta^{rb} g_L^2 Y_u^{pa} + g_Y^2 \left( \frac{163}{324} \delta^{rb} Y_u^{pa} + \frac{25}{9} \delta^{ab} Y_u^{pr} \right) + \frac{79}{72} \delta^{rb} (Y_u Y_u^\dagger Y_u)^{pa} - \frac{5}{72} Y_u^{pa} (Y_u^\dagger Y_u)^{br} \\
& - \frac{4}{3} \delta^{rb} g_s^2 Y_u^{pa} - \frac{3}{2} \delta^{rb} \lambda Y_u^{pa} \Big\} C_{Hu}^{ab} + \frac{5}{18} \delta^{ab} g_Y^2 C_{Hd}^{ab} Y_u^{pr} + \frac{1}{36} C_{Hud}^{ab} Y_u^{pa} (Y_d^\dagger Y_u)^{br} + C_{Hud}^{*ab} \Big\{ \frac{1}{24} Y_d^{pb} (Y_u^\dagger Y_u)^{ar} + \frac{7}{8} \delta^{ra} g_L^2 Y_d^{pb} + \frac{11}{12} \delta^{ra} (Y_d Y_d^\dagger Y_d)^{pb} \\
& + \frac{4}{3} \delta^{ra} g_s^2 Y_d^{pb} - \frac{25}{72} \delta^{ra} (Y_u Y_u^\dagger Y_d)^{pb} - \frac{79}{72} \delta^{ra} g_Y^2 Y_d^{pb} \Big\} + \Big\{ \frac{71}{162} \delta^{rd} \delta^{ab} g_Y^2 Y_u^{pc} + \delta^{rd} Y_u^{pc} (Y_e Y_e^\dagger)^{ba} \Big\} C_{\ell u}^{abcd} + \Big\{ 2 \delta^{pa} Y_u^{br} (Y_e^\dagger Y_e)^{dc}
\end{aligned}$$

$$\begin{aligned}
& + \frac{455}{162} \delta^{pa} \delta^{cd} g_Y^2 Y_u^{br} \left\{ C_{qe}^{abcd} + \left\{ \frac{1}{3} \delta^{rd} Y_u^{bc} (Y_d Y_d^\dagger)^{pa} + g_Y^2 \left( \frac{145}{162} \delta^{rd} \delta^{ab} Y_u^{pc} + \frac{355}{81} \delta^{pa} \delta^{cd} Y_u^{br} - \frac{25}{27} \delta^{pa} \delta^{rd} Y_u^{bc} \right) + \frac{5}{4} \delta^{pa} \delta^{rd} (Y_u Y_u^\dagger Y_u)^{bc} + \frac{5}{2} Y_u^{*ad} Y_u^{pr} Y_u^{bc} \right. \right. \\
& + \frac{5}{2} \delta^{pa} Y_u^{br} (Y_u^\dagger Y_u)^{dc} + \frac{5}{2} \delta^{rd} Y_u^{pc} (Y_u Y_u^\dagger)^{ba} + \frac{5}{2} \delta^{pa} \delta^{rd} Y_u^{bc} \text{Tr} [Y_u^\dagger Y_u] - \frac{1}{4} Y_u^{*ad} Y_u^{pc} Y_u^{br} - \frac{11}{24} \delta^{pa} \delta^{rd} (Y_d Y_d^\dagger Y_u)^{bc} - \frac{13}{18} \delta^{pa} Y_u^{bc} (Y_u^\dagger Y_u)^{dr} - \frac{7}{9} \delta^{rd} Y_u^{bc} (Y_u Y_u^\dagger)^{pa} \\
& - \delta^{rd} Y_u^{pc} (Y_d Y_d^\dagger)^{ba} - \frac{100}{9} \delta^{pa} \delta^{rd} g_s^2 Y_u^{bc} \left\{ C_{qu}^{(\parallel)abcd} + \left\{ \frac{5}{6} \delta^{pa} Y_u^{br} (Y_u^\dagger Y_u)^{dc} + \frac{5}{6} \delta^{rd} Y_u^{pc} (Y_u Y_u^\dagger)^{ba} + g_Y^2 \left( \frac{145}{486} \delta^{rd} \delta^{ab} Y_u^{pc} + \frac{355}{243} \delta^{pa} \delta^{cd} Y_u^{br} - \frac{25}{9} \delta^{pa} \delta^{rd} Y_u^{bc} \right) \right. \right. \\
& + g_s^2 \left( \frac{344}{81} \delta^{rd} \delta^{ab} Y_u^{pc} + \frac{448}{81} \delta^{pa} \delta^{cd} Y_u^{br} - \frac{100}{3} \delta^{pa} \delta^{rd} Y_u^{bc} \right) + \delta^{rd} Y_u^{bc} (Y_d Y_d^\dagger)^{pa} + \frac{15}{4} \delta^{pa} \delta^{rd} (Y_u Y_u^\dagger Y_u)^{bc} + \frac{15}{2} Y_u^{*ad} Y_u^{pr} Y_u^{bc} + \frac{15}{2} \delta^{pa} \delta^{rd} Y_u^{bc} \text{Tr} [Y_u^\dagger Y_u] \\
& - \frac{1}{3} \delta^{rd} Y_u^{pc} (Y_d Y_d^\dagger)^{ba} - \frac{3}{4} Y_u^{*ad} Y_u^{pc} Y_u^{br} - \frac{11}{8} \delta^{pa} \delta^{rd} (Y_d Y_d^\dagger Y_u)^{bc} - \frac{13}{6} \delta^{pa} Y_u^{bc} (Y_u^\dagger Y_u)^{dr} - \frac{7}{3} \delta^{rd} Y_u^{bc} (Y_u Y_u^\dagger)^{pa} \left\{ C_{qu}^{(\times)abcd} + \left\{ \frac{11}{72} Y_d^{*ad} Y_d^{pc} Y_u^{br} \right. \right. \\
& + \frac{131}{162} \delta^{pa} \delta^{cd} g_Y^2 Y_u^{br} + 2 \delta^{pa} Y_u^{br} (Y_d^\dagger Y_d)^{dc} - \frac{7}{18} \delta^{pa} Y_d^{bc} (Y_d^\dagger Y_u)^{dr} \left\{ C_{qd}^{(\parallel)abcd} + \left\{ \frac{131}{486} \delta^{pa} \delta^{cd} g_Y^2 Y_u^{br} + \frac{11}{24} Y_d^{*ad} Y_d^{pc} Y_u^{br} + \frac{2}{3} \delta^{pa} Y_u^{br} (Y_d^\dagger Y_d)^{dc} \right. \right. \\
& - \frac{7}{6} \delta^{pa} Y_d^{bc} (Y_d^\dagger Y_u)^{dr} - \frac{200}{81} \delta^{pa} \delta^{cd} g_s^2 Y_u^{br} \left\{ C_{qd}^{(\times)abcd} + \left\{ -g_Y^2 \left( \frac{250}{243} \delta^{rb} \delta^{ad} Y_u^{pc} + \frac{250}{81} \delta^{rb} \delta^{cd} Y_u^{pa} \right) - \frac{736}{81} \delta^{rb} \delta^{ad} g_s^2 Y_u^{pc} \right\} C_{uu}^{abcd} + \left\{ 2 \delta^{rd} Y_u^{pc} (Y_e^\dagger Y_e)^{ba} \right. \right. \\
& - \frac{415}{162} \delta^{rd} \delta^{ab} g_Y^2 Y_u^{pc} \left\{ C_{eu}^{abcd} + \left\{ \frac{3}{8} \delta^{rb} Y_d^{pc} (Y_d^\dagger Y_u)^{da} + 2 \delta^{rb} Y_u^{pa} (Y_d^\dagger Y_d)^{dc} - \frac{199}{162} \delta^{rb} \delta^{cd} g_Y^2 Y_u^{pa} \right\} C_{ud}^{(\parallel)abcd} + \left\{ \frac{2}{3} \delta^{rb} Y_u^{pa} (Y_d^\dagger Y_d)^{dc} + \frac{9}{8} \delta^{rb} Y_d^{pc} (Y_d^\dagger Y_u)^{da} \right. \right. \\
& + \frac{280}{81} \delta^{rb} \delta^{cd} g_s^2 Y_u^{pa} - \frac{199}{486} \delta^{rb} \delta^{cd} g_Y^2 Y_u^{pa} \left\{ C_{ud}^{(\times)abcd} - \frac{7}{72} Y_e^{*ab} C_{\ell edq}^{abcd} Y_d^{pc} Y_u^{dr} + \frac{7}{36} \delta^{pd} C_{\ell edq}^{*abcd} Y_e^{ab} (Y_d^\dagger Y_u)^{cr} + \left\{ \frac{11}{144} \delta^{pc} Y_d^{*ad} (Y_u^\dagger Y_u)^{br} \right. \right. \\
& + \frac{3}{16} \delta^{rb} Y_d^{*ad} (Y_d Y_d^\dagger)^{pc} + \frac{3}{16} \delta^{pc} \delta^{rb} (Y_d^\dagger Y_d Y_d^\dagger)^{ad} + \frac{11}{24} \delta^{pa} Y_d^{*cd} (Y_u^\dagger Y_u)^{br} + \frac{7}{12} \delta^{pc} Y_u^{*ab} (Y_d^\dagger Y_u)^{dr} + \frac{7}{8} \delta^{rb} Y_d^{*cd} (Y_d Y_d^\dagger)^{pa} + g_Y^2 \left( \frac{5}{72} \delta^{pa} \delta^{rb} Y_d^{*cd} \right. \\
& + \frac{43}{288} \delta^{pc} \delta^{rb} Y_d^{*ad} \left. \right) + g_L^2 \left( \frac{9}{32} \delta^{pc} \delta^{rb} Y_d^{*ad} + \frac{3}{8} \delta^{pa} \delta^{rb} Y_d^{*cd} \right) + \frac{5}{4} \delta^{pa} \delta^{rb} (Y_u^\dagger Y_u Y_d^\dagger)^{cd} - \frac{1}{72} \delta^{rb} Y_d^{*ad} (Y_u Y_u^\dagger)^{pc} - \frac{1}{12} \delta^{rb} Y_d^{*cd} (Y_u Y_u^\dagger)^{pa} - \frac{1}{9} \delta^{pa} Y_u^{*cb} (Y_d^\dagger Y_u)^{dr} \\
& - \frac{11}{48} \delta^{pc} \delta^{rb} (Y_u^\dagger Y_u Y_d^\dagger)^{ad} - \left( \frac{5}{8} \delta^{pc} \delta^{rb} Y_d^{*ad} + \frac{15}{4} \delta^{pa} \delta^{rb} Y_d^{*cd} \right) \text{Tr} [Y_u^\dagger Y_u] - \frac{11}{3} \delta^{pc} \delta^{rb} g_s^2 Y_d^{*ad} \left\{ C_{quqd}^{(\parallel)abcd} + \left( C_{quqd}^{(\parallel)*} \right)^{abcd} \left\{ \frac{1}{8} Y_d^{ad} Y_u^{pb} Y_u^{cr} + \frac{19}{72} Y_d^{pd} Y_u^{ar} Y_u^{cb} \right. \right. \\
& + \frac{3}{8} Y_d^{cd} Y_u^{pb} Y_u^{ar} + \frac{23}{24} Y_d^{pd} Y_u^{ab} Y_u^{cr} - \frac{5}{8} Y_d^{ad} Y_u^{pr} Y_u^{cb} - \frac{15}{4} Y_d^{cd} Y_u^{pr} Y_u^{ab} \left\} + \left\{ \frac{11}{72} \delta^{pa} Y_d^{*cd} (Y_u^\dagger Y_u)^{br} + \frac{7}{36} \delta^{pc} Y_u^{*ab} (Y_d^\dagger Y_u)^{dr} + \frac{11}{48} \delta^{pc} Y_d^{*ad} (Y_u^\dagger Y_u)^{br} \right. \right. \\
& + \frac{7}{24} \delta^{rb} Y_d^{*cd} (Y_d Y_d^\dagger)^{pa} + \frac{5}{12} \delta^{pa} \delta^{rb} (Y_u^\dagger Y_u Y_d^\dagger)^{cd} + \frac{9}{16} \delta^{rb} Y_d^{*ad} (Y_d Y_d^\dagger)^{pc} + \frac{9}{16} \delta^{pc} \delta^{rb} (Y_d^\dagger Y_d Y_d^\dagger)^{ad} + g_Y^2 \left( \frac{5}{216} \delta^{pa} \delta^{rb} Y_d^{*cd} + \frac{43}{96} \delta^{pc} \delta^{rb} Y_d^{*ad} \right) \\
& + g_L^2 \left( \frac{1}{8} \delta^{pa} \delta^{rb} Y_d^{*cd} + \frac{27}{32} \delta^{pc} \delta^{rb} Y_d^{*ad} \right) - \frac{1}{36} \delta^{rb} Y_d^{*cd} (Y_u Y_u^\dagger)^{pa} - \frac{1}{24} \delta^{rb} Y_d^{*ad} (Y_u Y_u^\dagger)^{pc} - \frac{1}{3} \delta^{pa} Y_u^{*cb} (Y_d^\dagger Y_u)^{dr} - \frac{11}{16} \delta^{pc} \delta^{rb} (Y_u^\dagger Y_u Y_d^\dagger)^{ad}
\end{aligned}$$

$$\begin{aligned}
& -g_s^2 \left( \frac{8}{9} \delta^{pa} \delta^{rb} Y_d^{*cd} + 2 \delta^{pc} \delta^{rb} Y_d^{*ad} \right) - \left( \frac{5}{4} \delta^{pa} \delta^{rb} Y_d^{*cd} + \frac{15}{8} \delta^{pc} \delta^{rb} Y_d^{*ad} \right) \text{Tr} \left[ Y_u^\dagger Y_u \right] \left\{ C_{quqd}^{(\times)abcd} + \left( C_{quqd}^{(\times)*} \right)^{abcd} \left\{ \frac{1}{8} Y_d^{cd} Y_u^{pb} Y_u^{ar} + \frac{23}{72} Y_d^{pd} Y_u^{ab} Y_u^{cr} + \frac{3}{8} Y_d^{ad} Y_u^{pb} Y_u^{cr} \right. \right. \\
& + \frac{19}{24} Y_d^{pd} Y_u^{ar} Y_u^{cb} - \frac{5}{4} Y_d^{cd} Y_u^{pr} Y_u^{ab} - \frac{15}{8} Y_d^{ad} Y_u^{pr} Y_u^{cb} \left. \right\} + \left\{ \frac{1}{36} \delta^{rd} Y_e^{*ab} (Y_u Y_u^\dagger)^{pc} + \frac{5}{4} \delta^{pc} \delta^{rd} Y_e^{*ab} \text{Tr} \left[ Y_u^\dagger Y_u \right] - \frac{11}{72} \delta^{pc} Y_e^{*ab} (Y_u^\dagger Y_u)^{dr} - \frac{7}{24} \delta^{rd} Y_e^{*ab} (Y_d Y_d^\dagger)^{pc} \right. \\
& - \frac{9}{8} \delta^{pc} \delta^{rd} g_L^2 Y_e^{*ab} - \frac{15}{8} \delta^{pc} \delta^{rd} g_Y^2 Y_e^{*ab} \left. \right\} C_{lequ}^{abcd} + C_{lequ}^{*abcd} \left\{ \frac{5}{4} Y_e^{ab} Y_u^{pr} Y_u^{cd} - \frac{1}{8} Y_e^{ab} Y_u^{pd} Y_u^{cr} \right\} + \left\{ \frac{11}{144} \delta^{pc} Y_e^{*ad} (Y_u^\dagger Y_u)^{br} + \frac{9}{32} \delta^{pc} \delta^{rb} g_L^2 Y_e^{*ad} \right. \\
& + \frac{1}{2} \delta^{pc} \delta^{rb} g_s^2 Y_e^{*ad} + \frac{25}{48} \delta^{rb} Y_e^{*ad} (Y_d Y_d^\dagger)^{pc} + \frac{43}{16} \delta^{pc} \delta^{rb} (Y_e^\dagger Y_e Y_e^\dagger)^{ad} - \frac{1}{72} \delta^{rb} Y_e^{*ad} (Y_u Y_u^\dagger)^{pc} - \frac{5}{8} \delta^{pc} \delta^{rb} Y_e^{*ad} \text{Tr} \left[ Y_u^\dagger Y_u \right] - \frac{191}{96} \delta^{pc} \delta^{rb} g_Y^2 Y_e^{*ad} \left. \right\} C_{luqe}^{abcd} \\
& + C_{luqe}^{*abcd} \left\{ \frac{5}{8} Y_e^{ad} Y_u^{pb} Y_u^{cr} - \frac{5}{8} Y_e^{ad} Y_u^{pr} Y_u^{cb} \right\} + \left\{ \frac{3}{4} \delta^{pa} Y_u^{dr} (Y_d Y_d^\dagger)^{bc} - \frac{7}{9} \delta^{pa} \delta^{bc} g_L^2 Y_u^{dr} - g_Y^2 \left( \frac{25}{243} \delta^{pa} \delta^{bc} Y_u^{dr} + \frac{50}{81} \delta^{pa} \delta^{cd} Y_u^{br} \right) - 2 \delta^{pa} Y_u^{br} (Y_d Y_d^\dagger)^{dc} \right. \\
& - \frac{184}{81} \delta^{pa} \delta^{bc} g_s^2 Y_u^{dr} \left. \right\} C_{qq}^{(\parallel)abcd} + \left\{ 2 \delta^{pa} Y_u^{br} (Y_d Y_d^\dagger)^{dc} - \frac{3}{4} \delta^{pa} Y_u^{dr} (Y_d Y_d^\dagger)^{bc} - g_Y^2 \left( \frac{50}{243} \delta^{pa} \delta^{bc} Y_u^{dr} + \frac{25}{81} \delta^{pa} \delta^{cd} Y_u^{br} \right) - \frac{7}{3} \delta^{pa} \delta^{cd} g_L^2 Y_u^{br} \right. \\
& - \frac{368}{81} \delta^{pa} \delta^{bc} g_s^2 Y_u^{dr} \left. \right\} C_{qq}^{(\times)abcd} + \left\{ \delta^{pc} Y_u^{dr} (Y_e Y_e^\dagger)^{ba} - \frac{137}{81} \delta^{pc} \delta^{ab} g_Y^2 Y_u^{dr} \right\} C_{\ell q}^{(\parallel)abcd} + \left\{ \frac{11}{18} \delta^{pc} \delta^{ab} g_L^2 Y_u^{dr} - \frac{137}{162} \delta^{pc} \delta^{ab} g_Y^2 Y_u^{dr} - \delta^{pc} Y_u^{dr} (Y_e Y_e^\dagger)^{ba} \right\} C_{\ell q}^{(\times)abcd}, \quad (8.6)
\end{aligned}$$

#### 8.4 $C_{uW}$

$$\begin{aligned}
\beta_{C_{uW}^{pr}}^{(1)} &= 2g_L^2 C_{HW} Y_u^{pr} - 2ig_L^2 C_{H\widetilde{W}} Y_u^{pr} - \frac{5}{6} g_Y^2 C_{HWB} Y_u^{pr} + \frac{5i}{6} g_Y^2 C_{H\widetilde{W}B} Y_u^{pr} - \frac{1}{3} \delta^{pa} \delta^{rb} g_Y^2 C_{uB}^{ab} + \left\{ \frac{1}{2} \left( \delta^{rb} (Y_u Y_u^\dagger)^{pa} + 2T_2 \delta^{pa} \delta^{rb} + 4\delta^{pa} (Y_u^\dagger Y_u)^{br} \right. \right. \\
& + 5\delta^{rb} (Y_d Y_d^\dagger)^{pa} \left. \right) + \frac{9}{4} \delta^{pa} \delta^{rb} g_L^2 + \frac{8}{3} \delta^{pa} \delta^{rb} g_s^2 - \frac{19}{36} \delta^{pa} \delta^{rb} g_Y^2 \left. \right\} C_{uW}^{ab} + \frac{16}{3} \delta^{pa} \delta^{rb} g_s^2 C_{uG}^{ab} - \delta^{pa} C_{dW}^{ab} (Y_d^\dagger Y_u)^{br} - \frac{1}{2} \delta^{pc} \delta^{rb} Y_d^{*ad} C_{quqd}^{(\parallel)abcd} \\
& - \frac{3}{2} \delta^{pc} \delta^{rb} Y_d^{*ad} C_{quqd}^{(\times)abcd} - \frac{1}{2} \delta^{pc} \delta^{rb} Y_e^{*ad} C_{luqe}^{abcd}, \quad (8.7)
\end{aligned}$$

$$\begin{aligned}
\beta_{C_{uW}^{pr}}^{(2)} &= \left\{ \frac{1}{4} (Y_d Y_d^\dagger Y_u)^{pr} - \frac{5}{18} g_Y^2 Y_u^{pr} \right\} C_{HD}^{(\parallel)} + \left\{ \frac{5}{72} g_Y^2 Y_u^{pr} + \frac{1}{8} g_L^2 Y_u^{pr} + \frac{1}{4} (Y_d Y_d^\dagger Y_u)^{pr} \right\} C_{HD}^{(\times)} - \frac{11}{12} g_Y^4 C_{HB} Y_u^{pr} + \frac{11i}{12} g_Y^4 C_{H\widetilde{B}} Y_u^{pr} + \left\{ g_L^2 \left( \frac{1}{2} (Y_d Y_d^\dagger Y_u)^{pr} \right. \right. \\
& - T_2 Y_u^{pr} - \frac{9}{2} (Y_u Y_u^\dagger Y_u)^{pr} \left. \right) + \frac{271}{18} g_L^4 Y_u^{pr} - \frac{13}{12} g_Y^2 g_L^2 Y_u^{pr} - 3\lambda g_L^2 Y_u^{pr} - 16g_s^2 g_L^2 Y_u^{pr} \left. \right\} C_{HW} + \left\{ g_L^2 \left( iT_2 Y_u^{pr} + \frac{9i}{2} (Y_u Y_u^\dagger Y_u)^{pr} \right. \right. \\
& - \frac{5i}{2} (Y_d Y_d^\dagger Y_u)^{pr} \left. \right) + \frac{13i}{12} g_Y^2 g_L^2 Y_u^{pr} + 3i\lambda g_L^2 Y_u^{pr} + 16ig_s^2 g_L^2 Y_u^{pr} - \frac{559i}{18} g_L^4 Y_u^{pr} \left. \right\} C_{H\widetilde{W}} - 8g_s^4 C_{HG} Y_u^{pr} + 8ig_s^4 C_{H\widetilde{G}} Y_u^{pr} + \left\{ \frac{5}{12} \lambda g_Y^2 Y_u^{pr} \right.
\end{aligned}$$

$$\begin{aligned}
& + g_Y^2 \left( \frac{7}{24} (Y_d Y_d^\dagger Y_u)^{pr} + \frac{5}{12} T_2 Y_u^{pr} + \frac{15}{8} (Y_u Y_u^\dagger Y_u)^{pr} \right) + \frac{665}{432} g_Y^4 Y_u^{pr} + \frac{20}{3} g_Y^2 g_s^2 Y_u^{pr} - \frac{35}{16} g_Y^2 g_L^2 Y_u^{pr} \Big\} C_{HWB} + \left\{ g_Y^2 \left( -\frac{i}{8} (Y_d Y_d^\dagger Y_u)^{pr} - \frac{5i}{12} T_2 Y_u^{pr} \right. \right. \\
& - \frac{15i}{8} (Y_u Y_u^\dagger Y_u)^{pr} \Big) + \frac{35i}{16} g_Y^2 g_L^2 Y_u^{pr} - \frac{5i}{12} \lambda g_Y^2 Y_u^{pr} - \frac{665i}{432} g_Y^4 Y_u^{pr} - \frac{20i}{3} g_Y^2 g_s^2 Y_u^{pr} \Big\} C_{H\widetilde{W}B} + \left\{ \frac{17}{6} g_Y^2 g_L^4 Y_u^{pr} + 35 g_L^6 Y_u^{pr} \right. \\
& - g_L^4 \left( \frac{3}{2} (Y_u Y_u^\dagger Y_u)^{pr} + \frac{27}{2} (Y_d Y_d^\dagger Y_u)^{pr} \right) - 20 g_s^2 g_L^4 Y_u^{pr} \Big\} C_W + \left\{ g_L^4 \left( \frac{5i}{6} (Y_u Y_u^\dagger Y_u)^{pr} + \frac{23i}{2} (Y_d Y_d^\dagger Y_u)^{pr} \right) + \frac{116i}{9} g_s^2 g_L^4 Y_u^{pr} - \frac{95i}{54} g_Y^2 g_L^4 Y_u^{pr} \right. \\
& - \frac{184i}{9} g_L^6 Y_u^{pr} \Big\} C_{\widetilde{W}} - 12 g_s^6 C_G Y_u^{pr} + \frac{52i}{3} g_s^6 C_{\widetilde{G}} Y_u^{pr} + \left\{ \frac{1}{4} \delta^{pa} (Y_u^\dagger Y_u)^{br} + \frac{3}{4} \delta^{pa} \delta^{rb} g_L^2 + \delta^{rb} (Y_d Y_d^\dagger)^{pa} - \frac{1}{4} \delta^{rb} (Y_u Y_u^\dagger)^{pa} - \frac{5}{12} \delta^{pa} \delta^{rb} g_Y^2 \right\} C_{uH}^{ab} \\
& + \frac{1}{2} \delta^{pa} C_{dH}^{ab} (Y_d^\dagger Y_u)^{br} + \frac{5}{6} g_Y^2 C_{eB}^{*ab} Y_e^{ab} Y_u^{pr} + \left\{ \frac{1}{4} g_L^2 Y_e^{*ab} Y_u^{pr} - \frac{5}{4} g_Y^2 Y_e^{*ab} Y_u^{pr} \right\} C_{eW}^{ab} + \frac{1}{4} g_L^2 C_{eW}^{*ab} Y_e^{ab} Y_u^{pr} + \left\{ \delta^{pa} \delta^{rb} \lambda g_Y^2 + g_Y^2 \left( \frac{7}{12} \delta^{pa} (Y_u^\dagger Y_u)^{br} \right. \right. \\
& + \frac{4}{3} \delta^{rb} (Y_d Y_d^\dagger)^{pa} + 5 Y_u^{*ab} Y_u^{pr} + 5 \delta^{pa} \delta^{rb} \text{Tr} [Y_d^\dagger Y_d] + \frac{11}{2} \delta^{pa} \delta^{rb} \text{Tr} [Y_u^\dagger Y_u] - \delta^{pa} \delta^{rb} \text{Tr} [Y_e^\dagger Y_e] - \frac{23}{12} \delta^{rb} (Y_u Y_u^\dagger)^{pa} \Big) - \frac{47}{24} \delta^{pa} \delta^{rb} g_Y^2 g_L^2 \\
& - \frac{56}{9} \delta^{pa} \delta^{rb} g_Y^2 g_s^2 - \frac{481}{72} \delta^{pa} \delta^{rb} g_Y^4 \Big\} C_{uB}^{ab} + \left\{ \delta^{rb} (Y_d Y_d^\dagger Y_u Y_u^\dagger)^{pa} + g_L^2 \left( \frac{3}{8} \delta^{pa} \delta^{rb} \text{Tr} [Y_e^\dagger Y_e] + \frac{3}{8} \delta^{pa} \delta^{rb} \text{Tr} [Y_u^\dagger Y_u] + \frac{9}{8} \delta^{pa} \delta^{rb} \text{Tr} [Y_d^\dagger Y_d] \right. \right. \\
& + \frac{63}{16} \delta^{rb} (Y_u Y_u^\dagger)^{pa} + \frac{21}{4} Y_u^{*ab} Y_u^{pr} + \frac{129}{16} \delta^{rb} (Y_d Y_d^\dagger)^{pa} + \frac{103}{8} \delta^{pa} (Y_u^\dagger Y_u)^{br} \Big) + g_Y^2 \left( \frac{11}{144} \delta^{rb} (Y_u Y_u^\dagger)^{pa} + \frac{25}{24} \delta^{pa} \delta^{rb} \text{Tr} [Y_d^\dagger Y_d] + \frac{431}{144} \delta^{rb} (Y_d Y_d^\dagger)^{pa} \right. \\
& + \frac{25}{8} \delta^{pa} \delta^{rb} \text{Tr} [Y_e^\dagger Y_e] + \frac{85}{24} \delta^{pa} \delta^{rb} \text{Tr} [Y_u^\dagger Y_u] + \frac{46}{9} \delta^{pa} (Y_u^\dagger Y_u)^{br} + \frac{25}{4} Y_u^{*ab} Y_u^{pr} \Big) + g_s^2 \left( 20 \delta^{pa} \delta^{rb} \text{Tr} [Y_d^\dagger Y_d] + 20 \delta^{pa} \delta^{rb} \text{Tr} [Y_u^\dagger Y_u] - \frac{16}{3} \delta^{rb} (Y_d Y_d^\dagger)^{pa} \right. \\
& - \frac{16}{3} \delta^{rb} (Y_u Y_u^\dagger)^{pa} - \frac{32}{3} \delta^{pa} (Y_u^\dagger Y_u)^{br} \Big) + \frac{5}{4} \delta^{pa} (Y_u^\dagger Y_u Y_u^\dagger Y_u)^{br} + \frac{3}{2} \delta^{pa} \delta^{rb} \lambda^2 + \frac{3}{2} \delta^{pa} \delta^{rb} \text{Tr} [Y_d^\dagger Y_d Y_u^\dagger Y_u] + \frac{7}{4} \delta^{rb} (Y_u Y_u^\dagger Y_u Y_u^\dagger)^{pa} + \frac{161}{16} \delta^{pa} \delta^{rb} g_L^4 \\
& + \frac{172}{3} \delta^{pa} \delta^{rb} g_s^4 - \frac{1}{4} \delta^{pa} (Y_u^\dagger Y_d Y_d^\dagger Y_u)^{br} - \frac{3}{4} T_2 \delta^{rb} (Y_u Y_u^\dagger)^{pa} - \lambda \left( \frac{3}{2} \delta^{pa} \delta^{rb} g_L^2 + 2 \delta^{rb} (Y_u Y_u^\dagger)^{pa} + 4 \delta^{rb} (Y_d Y_d^\dagger)^{pa} + 6 \delta^{pa} (Y_u^\dagger Y_u)^{br} \right) \\
& - 2 (Y_u^\dagger Y_u)^{br} (Y_d Y_d^\dagger)^{pa} - 2 (Y_u^\dagger Y_u)^{br} (Y_u Y_u^\dagger)^{pa} - \frac{9}{4} T_4 \delta^{pa} \delta^{rb} - \frac{39}{16} \delta^{pa} \delta^{rb} g_Y^2 g_L^2 - \frac{11}{4} T_2 \delta^{rb} (Y_d Y_d^\dagger)^{pa} - \frac{1831}{648} \delta^{pa} \delta^{rb} g_Y^4 - 3 \delta^{pa} \delta^{rb} g_s^2 g_L^2 \\
& - 3 T_2 \delta^{pa} (Y_u^\dagger Y_u)^{br} - \frac{13}{4} \delta^{rb} (Y_d Y_d^\dagger Y_d Y_d^\dagger)^{pa} - \frac{215}{27} \delta^{pa} \delta^{rb} g_Y^2 g_s^2 \Big\} C_{uW}^{ab} + C_{uW}^{*ab} \left\{ \frac{1}{2} Y_u^{ar} (Y_d Y_d^\dagger Y_u)^{pb} - \frac{1}{2} Y_u^{pb} (Y_d Y_d^\dagger Y_u)^{ar} \right\} + \left\{ \frac{328}{9} \delta^{pa} \delta^{rb} g_s^4 \right. \\
& - g_s^2 \left( \frac{4}{3} \delta^{pa} (Y_u^\dagger Y_u)^{br} + \frac{16}{3} \delta^{rb} (Y_d Y_d^\dagger)^{pa} + \frac{28}{3} \delta^{rb} (Y_u Y_u^\dagger)^{pa} \right) - \frac{82}{27} \delta^{pa} \delta^{rb} g_Y^2 g_s^2 - \frac{14}{3} \delta^{pa} \delta^{rb} g_s^2 g_L^2 \Big\} C_{uG}^{ab} + 2 \delta^{pa} g_Y^2 C_{dB}^{ab} (Y_d^\dagger Y_u)^{br} \\
& + g_Y^2 C_{dB}^{*ab} \left\{ \frac{5}{2} Y_d^{ab} Y_u^{pr} - \frac{3}{2} Y_d^{pb} Y_u^{ar} \right\} + \left\{ \frac{1}{2} T_2 \delta^{pa} (Y_d^\dagger Y_u)^{br} + g_Y^2 \left( \frac{7}{8} \delta^{pa} (Y_d^\dagger Y_u)^{br} - \frac{5}{12} Y_d^{*ab} Y_u^{pr} \right) + g_L^2 \left( \frac{3}{4} Y_d^{*ab} Y_u^{pr} + \frac{39}{8} \delta^{pa} (Y_d^\dagger Y_u)^{br} \right) \right.
\end{aligned}$$



$$\begin{aligned}
& + \frac{5}{2} \delta^{pa} (Y_d^\dagger Y_d Y_d^\dagger Y_u)^{br} - (Y_d^\dagger Y_u)^{br} (Y_d Y_d^\dagger)^{pa} - \delta^{pa} (Y_d^\dagger Y_u Y_u^\dagger Y_u)^{br} \Big\} C_{dW}^{ab} + C_{dW}^{*ab} \Big\{ \frac{1}{2} Y_d^{pb} (Y_d Y_d^\dagger Y_u)^{ar} + g_L^2 \left( \frac{3}{4} Y_d^{ab} Y_u^{pr} + 2 Y_d^{pb} Y_u^{ar} \right) + Y_u^{ar} (Y_u Y_u^\dagger Y_d)^{pb} \\
& + \frac{13}{12} g_Y^2 Y_d^{pb} Y_u^{ar} + 8 g_s^2 Y_d^{pb} Y_u^{ar} - \frac{1}{2} Y_u^{ar} (Y_d Y_d^\dagger Y_d)^{pb} - T_2 Y_d^{pb} Y_u^{ar} - Y_d^{pb} (Y_u Y_u^\dagger Y_u)^{ar} \Big\} - 8 g_s^2 C_{dG}^{*ab} Y_d^{pb} Y_u^{ar} + \Big\{ \frac{5}{9} \delta^{ab} g_Y^2 Y_u^{pr} - \delta^{ab} g_L^2 Y_u^{pr} \Big\} C_{H\ell}^{(\parallel)ab} \\
& - \frac{5}{9} \delta^{ab} g_Y^2 C_{H\ell}^{(\times)ab} Y_u^{pr} + \frac{5}{9} \delta^{ab} g_Y^2 C_{He}^{ab} Y_u^{pr} + \Big\{ \frac{1}{12} \delta^{pa} (Y_u Y_u^\dagger Y_u)^{br} + \delta^{pa} \lambda Y_u^{br} + g_L^2 (5 \delta^{pa} Y_u^{br} - 3 \delta^{ab} Y_u^{pr}) + \frac{19}{12} Y_u^{br} (Y_u Y_u^\dagger)^{pa} + \frac{8}{3} \delta^{pa} g_s^2 Y_u^{br} \\
& - \frac{5}{6} \delta^{pa} (Y_d Y_d^\dagger Y_u)^{br} - g_Y^2 \left( \frac{10}{27} \delta^{pa} Y_u^{br} + \frac{5}{9} \delta^{ab} Y_u^{pr} \right) - \frac{4}{3} Y_u^{br} (Y_d Y_d^\dagger)^{pa} \Big\} C_{Hq}^{(\parallel)ab} + \Big\{ g_Y^2 \left( \frac{5}{9} \delta^{ab} Y_u^{pr} - \frac{14}{27} \delta^{pa} Y_u^{br} \right) + \frac{7}{6} Y_u^{br} (Y_u Y_u^\dagger)^{pa} + \frac{13}{6} \delta^{pa} (Y_u Y_u^\dagger Y_u)^{br} \\
& + \frac{22}{3} \delta^{pa} g_L^2 Y_u^{br} - \delta^{pa} \lambda Y_u^{br} - \frac{5}{3} Y_u^{br} (Y_d Y_d^\dagger)^{pa} - \frac{13}{6} \delta^{pa} (Y_d Y_d^\dagger Y_u)^{br} - \frac{8}{3} \delta^{pa} g_s^2 Y_u^{br} \Big\} C_{Hq}^{(\times)ab} + \Big\{ \frac{1}{2} \delta^{rb} g_L^2 Y_u^{pa} + \frac{3}{4} Y_u^{pa} (Y_u^\dagger Y_u)^{br} + \delta^{rb} \lambda Y_u^{pa} \\
& + g_Y^2 \left( \frac{1}{18} \delta^{rb} Y_u^{pa} - \frac{10}{9} \delta^{ab} Y_u^{pr} \right) + \delta^{rb} (Y_d Y_d^\dagger Y_u)^{pa} + \frac{8}{3} \delta^{rb} g_s^2 Y_u^{pa} - \frac{3}{4} \delta^{rb} (Y_u Y_u^\dagger Y_u)^{pa} \Big\} C_{Hu}^{ab} + \Big\{ \frac{1}{2} Y_d^{pa} (Y_d^\dagger Y_u)^{br} + \frac{5}{9} \delta^{ab} g_Y^2 Y_u^{pr} \Big\} C_{Hd}^{ab} \\
& + C_{Hud}^{*ab} \Big\{ \frac{1}{2} \delta^{ra} (Y_d Y_d^\dagger Y_d)^{pb} - \frac{1}{18} \delta^{ra} g_Y^2 Y_d^{pb} - \frac{1}{4} Y_d^{pb} (Y_u^\dagger Y_u)^{ar} - \frac{1}{2} \delta^{ra} g_L^2 Y_d^{pb} - \frac{3}{4} \delta^{ra} (Y_u Y_u^\dagger Y_d)^{pb} - \delta^{ra} \lambda Y_d^{pb} - \frac{8}{3} \delta^{ra} g_s^2 Y_d^{pb} \Big\} + \Big\{ \frac{1}{3} \delta^{rd} \delta^{ab} g_Y^2 Y_u^{pc} \\
& + 2 \delta^{rd} \delta^{ab} g_L^2 Y_u^{pc} + 2 \delta^{rd} Y_u^{pc} (Y_e Y_e^\dagger)^{ba} \Big\} C_{\ell u}^{abcd} + \frac{5}{27} \delta^{pa} \delta^{cd} g_Y^2 C_{qe}^{abcd} Y_u^{br} + \Big\{ \frac{1}{6} Y_u^{*ad} Y_u^{pc} Y_u^{br} + g_L^2 (6 \delta^{rd} \delta^{ab} Y_u^{pc} - \delta^{pa} \delta^{rd} Y_u^{bc}) + \frac{3}{2} \delta^{pa} \delta^{rd} (Y_u Y_u^\dagger Y_u)^{bc} \\
& + 3 Y_u^{*ad} Y_u^{pr} Y_u^{bc} + 3 \delta^{pa} Y_u^{br} (Y_u^\dagger Y_u)^{dc} + 3 \delta^{rd} Y_u^{pc} (Y_u Y_u^\dagger)^{ba} + 3 \delta^{pa} \delta^{rd} Y_u^{bc} \text{Tr} [Y_u^\dagger Y_u] + 6 \delta^{rd} Y_u^{pc} (Y_d Y_d^\dagger)^{ba} - \frac{1}{3} \delta^{pa} Y_u^{bc} (Y_u^\dagger Y_u)^{dr} - \frac{3}{4} \delta^{pa} \delta^{rd} (Y_d Y_d^\dagger Y_u)^{bc} \\
& - g_Y^2 \left( \frac{1}{3} \delta^{rd} \delta^{ab} Y_u^{pc} + \frac{10}{27} \delta^{pa} \delta^{cd} Y_u^{br} + \frac{10}{9} \delta^{pa} \delta^{rd} Y_u^{bc} \right) - 2 \delta^{rd} Y_u^{bc} (Y_d Y_d^\dagger)^{pa} - \frac{40}{3} \delta^{pa} \delta^{rd} g_s^2 Y_u^{bc} \Big\} C_{qu}^{(\parallel)abcd} + \Big\{ \frac{1}{2} Y_u^{*ad} Y_u^{pc} Y_u^{br} + g_L^2 (2 \delta^{rd} \delta^{ab} Y_u^{pc} \\
& - 3 \delta^{pa} \delta^{rd} Y_u^{bc}) + g_s^2 \left( \frac{32}{27} \delta^{pa} \delta^{cd} Y_u^{br} - 40 \delta^{pa} \delta^{rd} Y_u^{bc} \right) + \delta^{pa} Y_u^{br} (Y_u^\dagger Y_u)^{dc} + \delta^{rd} Y_u^{pc} (Y_u Y_u^\dagger)^{ba} + 2 \delta^{rd} Y_u^{pc} (Y_d Y_d^\dagger)^{ba} + \frac{9}{2} \delta^{pa} \delta^{rd} (Y_u Y_u^\dagger Y_u)^{bc} + 9 Y_u^{*ad} Y_u^{pr} Y_u^{bc} \\
& + 9 \delta^{pa} \delta^{rd} Y_u^{bc} \text{Tr} [Y_u^\dagger Y_u] - g_Y^2 \left( \frac{1}{9} \delta^{rd} \delta^{ab} Y_u^{pc} + \frac{10}{81} \delta^{pa} \delta^{cd} Y_u^{br} + \frac{10}{3} \delta^{pa} \delta^{rd} Y_u^{bc} \right) - \delta^{pa} Y_u^{bc} (Y_u^\dagger Y_u)^{dr} - \frac{9}{4} \delta^{pa} \delta^{rd} (Y_d Y_d^\dagger Y_u)^{bc} - 6 \delta^{rd} Y_u^{bc} (Y_d Y_d^\dagger)^{pa} \Big\} C_{qu}^{(\times)abcd} \\
& + \Big\{ \frac{5}{27} \delta^{pa} \delta^{cd} g_Y^2 Y_u^{br} - \frac{1}{12} Y_d^{*ad} Y_d^{pc} Y_u^{br} - \frac{1}{3} \delta^{pa} Y_d^{bc} (Y_d^\dagger Y_u)^{dr} \Big\} C_{qd}^{(\parallel)abcd} + \Big\{ \frac{5}{81} \delta^{pa} \delta^{cd} g_Y^2 Y_u^{br} + \frac{32}{27} \delta^{pa} \delta^{cd} g_s^2 Y_u^{br} - \frac{1}{4} Y_d^{*ad} Y_d^{pc} Y_u^{br} \\
& - \delta^{pa} Y_d^{bc} (Y_d^\dagger Y_u)^{dr} \Big\} C_{qd}^{(\times)abcd} - g_Y^2 \Big\{ \frac{4}{9} \delta^{rb} \delta^{ad} Y_u^{pc} + \frac{4}{3} \delta^{rb} \delta^{cd} Y_u^{pa} \Big\} C_{uu}^{abcd} + \frac{1}{3} \delta^{rd} \delta^{ab} g_Y^2 C_{eu}^{abcd} Y_u^{pc} + \Big\{ \frac{1}{4} \delta^{rb} Y_d^{pc} (Y_d^\dagger Y_u)^{da} + \frac{1}{3} \delta^{rb} \delta^{cd} g_Y^2 Y_u^{pa} \Big\} C_{ud}^{(\parallel)abcd}
\end{aligned}$$

$$\begin{aligned}
& + \left\{ \frac{1}{9} \delta^{rb} \delta^{cd} g_Y^2 Y_u^{pa} + \frac{3}{4} \delta^{rb} Y_d^{pc} (Y_d^\dagger Y_u)^{da} \right\} C_{ud}^{(\times)abcd} - \frac{1}{12} Y_e^{*ab} C_{ledq}^{abcd} Y_d^{pc} Y_u^{dr} + \frac{2}{3} \delta^{pd} C_{ledq}^{*abcd} Y_e^{ab} (Y_d^\dagger Y_u)^{cr} + \left\{ \frac{1}{8} \delta^{rb} Y_d^{*ad} (Y_d Y_d^\dagger)^{pc} + \frac{7}{12} \delta^{pa} Y_u^{*cb} (Y_d^\dagger Y_u)^{dr} \right. \\
& + g_Y^2 \left( \frac{5}{16} \delta^{pc} \delta^{rb} Y_d^{*ad} + \frac{5}{12} \delta^{pa} \delta^{rb} Y_d^{*cd} \right) + \frac{9}{8} \delta^{pc} \delta^{rb} (Y_d^\dagger Y_d Y_d^\dagger)^{ad} + \frac{3}{2} \delta^{pa} \delta^{rb} (Y_u^\dagger Y_u Y_d^\dagger)^{cd} + 2 \delta^{pc} Y_u^{*ab} (Y_d^\dagger Y_u)^{dr} + \frac{9}{4} \delta^{rb} Y_d^{*cd} (Y_d Y_d^\dagger)^{pa} \\
& - \frac{1}{24} \delta^{pc} Y_d^{*ad} (Y_u^\dagger Y_u)^{br} - \frac{1}{4} \delta^{pa} Y_d^{*cd} (Y_u^\dagger Y_u)^{br} - \frac{3}{8} \delta^{pc} \delta^{rb} (Y_u^\dagger Y_u Y_d^\dagger)^{ad} - g_L^2 \left( \frac{9}{4} \delta^{pa} \delta^{rb} Y_d^{*cd} + \frac{41}{16} \delta^{pc} \delta^{rb} Y_d^{*ad} \right) - \left( \frac{3}{4} \delta^{pc} \delta^{rb} Y_d^{*ad} + \frac{9}{2} \delta^{pa} \delta^{rb} Y_d^{*cd} \right) \text{Tr} [Y_u^\dagger Y_u] \\
& - 6 \delta^{pc} \delta^{rb} g_s^2 Y_d^{*ad} \left\{ C_{quqd}^{(\parallel)abcd} + \left( C_{quqd}^{(\parallel)*} \right)^{abcd} \left\{ \frac{1}{12} Y_d^{ad} Y_u^{pb} Y_u^{cr} + \frac{7}{12} Y_d^{pd} Y_u^{ar} Y_u^{cb} + \frac{5}{4} Y_d^{pd} Y_u^{ab} Y_u^{cr} - \frac{1}{4} Y_d^{cd} Y_u^{pb} Y_u^{ar} - \frac{3}{4} Y_d^{ad} Y_u^{pr} Y_u^{cb} - \frac{9}{2} Y_d^{cd} Y_u^{pr} Y_u^{ab} \right\} \right. \\
& + \left\{ \frac{3}{8} \delta^{rb} Y_d^{*ad} (Y_d Y_d^\dagger)^{pc} + \frac{1}{2} \delta^{pa} \delta^{rb} (Y_u^\dagger Y_u Y_d^\dagger)^{cd} + \frac{2}{3} \delta^{pc} Y_u^{*ab} (Y_d^\dagger Y_u)^{dr} + \frac{3}{4} \delta^{rb} Y_d^{*cd} (Y_d Y_d^\dagger)^{pa} + g_Y^2 \left( \frac{5}{36} \delta^{pa} \delta^{rb} Y_d^{*cd} + \frac{15}{16} \delta^{pc} \delta^{rb} Y_d^{*ad} \right) \right. \\
& + \frac{7}{4} \delta^{pa} Y_u^{*cb} (Y_d^\dagger Y_u)^{dr} + \frac{27}{8} \delta^{pc} \delta^{rb} (Y_d^\dagger Y_d Y_d^\dagger)^{ad} - \frac{1}{12} \delta^{pa} Y_d^{*cd} (Y_u^\dagger Y_u)^{br} - \frac{1}{8} \delta^{pc} Y_d^{*ad} (Y_u^\dagger Y_u)^{br} - g_L^2 \left( \frac{3}{4} \delta^{pa} \delta^{rb} Y_d^{*cd} + \frac{123}{16} \delta^{pc} \delta^{rb} Y_d^{*ad} \right) \\
& - g_s^2 \left( \frac{16}{3} \delta^{pa} \delta^{rb} Y_d^{*cd} + 12 \delta^{pc} \delta^{rb} Y_d^{*ad} \right) - \left( \frac{3}{2} \delta^{pa} \delta^{rb} Y_d^{*cd} + \frac{9}{4} \delta^{pc} \delta^{rb} Y_d^{*ad} \right) \text{Tr} [Y_u^\dagger Y_u] - \frac{9}{8} \delta^{pc} \delta^{rb} (Y_u^\dagger Y_u Y_d^\dagger)^{ad} \left\{ C_{quqd}^{(\times)abcd} + \left( C_{quqd}^{(\times)*} \right)^{abcd} \left\{ \frac{1}{4} Y_d^{ad} Y_u^{pb} Y_u^{cr} \right. \right. \\
& + \frac{5}{12} Y_d^{pd} Y_u^{ab} Y_u^{cr} + \frac{7}{4} Y_d^{pd} Y_u^{ar} Y_u^{cb} - \frac{1}{12} Y_d^{cd} Y_u^{pb} Y_u^{ar} - \frac{3}{2} Y_d^{cd} Y_u^{pr} Y_u^{ab} - \frac{9}{4} Y_d^{ad} Y_u^{pr} Y_u^{cb} \left. \right\} + \left\{ \frac{1}{12} \delta^{pc} Y_e^{*ab} (Y_u^\dagger Y_u)^{dr} + \frac{3}{4} \delta^{pc} \delta^{rd} g_L^2 Y_e^{*ab} \right. \\
& + \frac{3}{2} \delta^{pc} \delta^{rd} Y_e^{*ab} \text{Tr} [Y_u^\dagger Y_u] - \frac{3}{4} \delta^{rd} Y_e^{*ab} (Y_d Y_d^\dagger)^{pc} - \frac{5}{4} \delta^{pc} \delta^{rd} g_Y^2 Y_e^{*ab} \left. \right\} C_{lequ}^{abcd} + C_{lequ}^{*abcd} \left\{ \frac{1}{12} Y_e^{ab} Y_u^{pd} Y_u^{cr} + \frac{3}{2} Y_e^{ab} Y_u^{pr} Y_u^{cd} \right\} + \left\{ \frac{1}{8} \delta^{rb} Y_e^{*ad} (Y_d Y_d^\dagger)^{pc} \right. \\
& + \frac{1}{3} \delta^{pc} \delta^{rb} g_s^2 Y_e^{*ad} + \frac{9}{8} \delta^{pc} \delta^{rb} (Y_e^\dagger Y_e Y_e^\dagger)^{ad} - \frac{1}{24} \delta^{pc} Y_e^{*ad} (Y_u^\dagger Y_u)^{br} - \frac{3}{4} \delta^{pc} \delta^{rb} Y_e^{*ad} \text{Tr} [Y_u^\dagger Y_u] - \frac{203}{144} \delta^{pc} \delta^{rb} g_Y^2 Y_e^{*ad} - \frac{41}{16} \delta^{pc} \delta^{rb} g_L^2 Y_e^{*ad} \left. \right\} C_{luqe}^{abcd} \\
& + C_{luqe}^{*abcd} \left\{ \frac{1}{12} Y_e^{ad} Y_u^{pb} Y_u^{cr} - \frac{3}{4} Y_e^{ad} Y_u^{pr} Y_u^{cb} \right\} + \left\{ \frac{5}{2} \delta^{pa} Y_u^{dr} (Y_d Y_d^\dagger)^{bc} + 12 \delta^{pa} Y_u^{br} (Y_d Y_d^\dagger)^{dc} - g_Y^2 \left( \frac{10}{27} \delta^{pa} \delta^{cd} Y_u^{br} + \frac{86}{81} \delta^{pa} \delta^{bc} Y_u^{dr} \right) - g_L^2 \left( \frac{8}{3} \delta^{pa} \delta^{bc} Y_u^{dr} \right. \right. \\
& + 6 \delta^{pa} \delta^{cd} Y_u^{br} \left. \right) - 2 \delta^{pa} Y_u^{dr} (Y_u Y_u^\dagger)^{bc} - \frac{368}{27} \delta^{pa} \delta^{bc} g_s^2 Y_u^{dr} \left. \right\} C_{qq}^{(\parallel)abcd} + \left\{ \frac{7}{2} \delta^{pa} Y_u^{dr} (Y_d Y_d^\dagger)^{bc} + \frac{128}{27} \delta^{pa} \delta^{bc} g_s^2 Y_u^{dr} + 6 \delta^{pa} Y_u^{br} (Y_d Y_d^\dagger)^{dc} - g_Y^2 \left( \frac{10}{81} \delta^{pa} \delta^{bc} Y_u^{dr} \right. \right. \\
& + \frac{86}{27} \delta^{pa} \delta^{cd} Y_u^{br} \left. \right) - g_L^2 \left( 2 \delta^{pa} \delta^{bc} Y_u^{dr} + 8 \delta^{pa} \delta^{cd} Y_u^{br} \right) - 6 \delta^{pa} Y_u^{br} (Y_u Y_u^\dagger)^{dc} \left. \right\} C_{qq}^{(\times)abcd} + \left\{ \frac{5}{27} \delta^{pc} \delta^{ab} g_Y^2 Y_u^{dr} + 2 \delta^{pc} Y_u^{dr} (Y_e Y_e^\dagger)^{ba} - \delta^{pc} \delta^{ab} g_L^2 Y_u^{dr} \right\} C_{lq}^{(\parallel)abcd} \\
& + \left\{ \delta^{pc} Y_u^{dr} (Y_e Y_e^\dagger)^{ba} + \frac{43}{27} \delta^{pc} \delta^{ab} g_Y^2 Y_u^{dr} - \frac{4}{3} \delta^{pc} \delta^{ab} g_L^2 Y_u^{dr} \right\} C_{lq}^{(\times)abcd}, \tag{8.8}
\end{aligned}$$

## 8.5 $C_{uG}$

$$\begin{aligned} \beta_{C_{uG}^{pr}}^{(1)} = & 4g_s^2 C_{HG} Y_u^{pr} - 4ig_s^2 C_{H\tilde{G}} Y_u^{pr} + 9g_s^4 C_G Y_u^{pr} - 9ig_s^4 C_{\tilde{G}} Y_u^{pr} + \frac{10}{3} \delta^{pa} \delta^{rb} g_Y^2 C_{uB}^{ab} + 3\delta^{pa} \delta^{rb} g_L^2 C_{uW}^{ab} + \left\{ \frac{1}{2} \left( 2T_2 \delta^{pa} \delta^{rb} + 4\delta^{pa} (Y_u^\dagger Y_u)^{br} \right. \right. \\ & \left. \left. + 5\delta^{rb} (Y_u Y_u^\dagger)^{pa} - 3\delta^{rb} (Y_d Y_d^\dagger)^{pa} \right) + \frac{4}{3} \delta^{pa} \delta^{rb} g_s^2 - \frac{19}{36} \delta^{pa} \delta^{rb} g_Y^2 - \frac{9}{4} \delta^{pa} \delta^{rb} g_L^2 \right\} C_{uG}^{ab} - \delta^{pa} C_{dG}^{ab} (Y_d^\dagger Y_u)^{br} + \delta^{pc} \delta^{rb} Y_d^{*ad} C_{quqd}^{(II)abcd}, \end{aligned} \quad (8.9)$$

$$\begin{aligned} \beta_{C_{uG}^{pr}}^{(2)} = & -\frac{1}{2} C_{HD}^{(II)} (Y_d Y_d^\dagger Y_u)^{pr} + \frac{1}{2} C_{HD}^{(\times)} (Y_d Y_d^\dagger Y_u)^{pr} - \frac{11}{6} g_Y^4 C_{HB} Y_u^{pr} + \frac{11i}{6} g_Y^4 C_{H\tilde{B}} Y_u^{pr} - \frac{3}{2} g_L^4 C_{HW} Y_u^{pr} + \frac{3i}{2} g_L^4 C_{H\tilde{W}} Y_u^{pr} + \left\{ g_s^2 \left( 5(Y_d Y_d^\dagger Y_u)^{pr} \right. \right. \\ & \left. \left. - 2T_2 Y_u^{pr} - 15(Y_u Y_u^\dagger Y_u)^{pr} \right) + \frac{3}{2} g_s^2 g_L^2 Y_u^{pr} + \frac{80}{3} g_s^4 Y_u^{pr} - \frac{13}{6} g_Y^2 g_s^2 Y_u^{pr} - 6\lambda g_s^2 Y_u^{pr} \right\} C_{HG} + \left\{ g_s^2 \left( 2iT_2 Y_u^{pr} + 15i(Y_u Y_u^\dagger Y_u)^{pr} - i(Y_d Y_d^\dagger Y_u)^{pr} \right) \right. \\ & \left. + \frac{13i}{6} g_Y^2 g_s^2 Y_u^{pr} + 6i\lambda g_s^2 Y_u^{pr} - \frac{3i}{2} g_s^2 g_L^2 Y_u^{pr} - \frac{224i}{3} g_s^4 Y_u^{pr} \right\} C_{H\tilde{G}} + \frac{9}{4} g_Y^2 g_L^2 C_{H\tilde{W}B} Y_u^{pr} - \frac{9i}{4} g_Y^2 g_L^2 C_{H\tilde{W}\tilde{B}} Y_u^{pr} - \frac{9}{2} g_L^6 C_W Y_u^{pr} + \frac{5i}{2} g_L^6 C_{\tilde{W}} Y_u^{pr} \\ & + \left\{ g_s^4 \left( \frac{45}{2} (Y_d Y_d^\dagger Y_u)^{pr} - 27(Y_u Y_u^\dagger Y_u)^{pr} \right) + 144g_s^6 Y_u^{pr} - \frac{85}{8} g_Y^2 g_s^4 Y_u^{pr} - \frac{135}{8} g_s^4 g_L^2 Y_u^{pr} \right\} C_G + \left\{ g_s^4 \left( 30i(Y_u Y_u^\dagger Y_u)^{pr} - \frac{29i}{2} (Y_d Y_d^\dagger Y_u)^{pr} \right) \right. \\ & \left. + \frac{829i}{72} g_Y^2 g_s^4 Y_u^{pr} + \frac{135i}{8} g_s^4 g_L^2 Y_u^{pr} - \frac{482i}{3} g_s^6 Y_u^{pr} \right\} C_{\tilde{G}} + \left\{ \frac{3}{2} \delta^{pa} (Y_u^\dagger Y_u)^{br} + \frac{3}{2} \delta^{rb} (Y_u Y_u^\dagger)^{pa} \right\} C_{uH}^{ab} + \left\{ g_Y^2 \left( \frac{1}{3} \delta^{rb} (Y_d Y_d^\dagger)^{pa} - \frac{13}{6} \delta^{rb} (Y_u Y_u^\dagger)^{pa} \right. \right. \\ & \left. \left. - \frac{35}{6} \delta^{pa} (Y_u^\dagger Y_u)^{br} \right) + \frac{7}{4} \delta^{pa} \delta^{rb} g_Y^2 g_L^2 + \frac{65}{9} \delta^{pa} \delta^{rb} g_Y^2 g_s^2 - \frac{1105}{36} \delta^{pa} \delta^{rb} g_Y^4 \right\} C_{uB}^{ab} + \left\{ \frac{19}{24} \delta^{pa} \delta^{rb} g_Y^2 g_L^2 + \frac{13}{2} \delta^{pa} \delta^{rb} g_s^2 g_L^2 + \frac{167}{24} \delta^{pa} \delta^{rb} g_L^4 \right. \\ & \left. - g_L^2 \left( \frac{3}{4} \delta^{pa} (Y_u^\dagger Y_u)^{br} + \frac{3}{4} \delta^{rb} (Y_u Y_u^\dagger)^{pa} + \frac{15}{2} \delta^{rb} (Y_d Y_d^\dagger)^{pa} \right) \right\} C_{uW}^{ab} + \left\{ g_L^2 \left( \frac{9}{16} \delta^{rb} (Y_d Y_d^\dagger)^{pa} + \frac{15}{8} T_2 \delta^{pa} \delta^{rb} + 9\delta^{pa} (Y_u^\dagger Y_u)^{br} + \frac{237}{16} \delta^{rb} (Y_u Y_u^\dagger)^{pa} \right) \right. \\ & \left. + g_Y^2 \left( \frac{25}{24} \delta^{pa} \delta^{rb} \text{Tr}[Y_d^\dagger Y_d] + \frac{25}{8} \delta^{pa} \delta^{rb} \text{Tr}[Y_e^\dagger Y_e] + \frac{85}{24} \delta^{pa} \delta^{rb} \text{Tr}[Y_u^\dagger Y_u] + \frac{46}{9} \delta^{pa} (Y_u^\dagger Y_u)^{br} - \frac{1}{144} \delta^{rb} (Y_d Y_d^\dagger)^{pa} - \frac{1}{144} \delta^{rb} (Y_u Y_u^\dagger)^{pa} \right) \right. \\ & \left. + g_s^2 \left( \frac{7}{3} \delta^{rb} (Y_u Y_u^\dagger)^{pa} + \frac{8}{3} \delta^{pa} (Y_u^\dagger Y_u)^{br} + 10Y_u^{*ab} Y_u^{pr} + 16\delta^{pa} \delta^{rb} \text{Tr}[Y_d^\dagger Y_d] + 22\delta^{pa} \delta^{rb} \text{Tr}[Y_u^\dagger Y_u] - \frac{47}{3} \delta^{rb} (Y_d Y_d^\dagger)^{pa} \right) + \frac{5}{4} T_2 \delta^{rb} (Y_d Y_d^\dagger)^{pa} \right. \\ & \left. + \frac{5}{4} \delta^{pa} (Y_u^\dagger Y_u Y_u^\dagger Y_u)^{br} + \frac{5}{4} \delta^{rb} (Y_u Y_u^\dagger Y_u Y_u^\dagger)^{pa} + \frac{3}{2} \delta^{pa} \delta^{rb} \lambda^2 + \frac{3}{2} \delta^{pa} \delta^{rb} \text{Tr}[Y_d^\dagger Y_d Y_u^\dagger Y_u] + \frac{23}{12} \delta^{pa} \delta^{rb} g_Y^2 g_L^2 + \frac{5}{2} \delta^{pa} \delta^{rb} g_s^2 g_L^2 \right. \\ & \left. + \frac{11}{4} \delta^{rb} (Y_d Y_d^\dagger Y_d Y_d^\dagger)^{pa} + \frac{362}{9} \delta^{pa} \delta^{rb} g_s^4 - \frac{1}{4} \delta^{pa} (Y_u^\dagger Y_d Y_d^\dagger Y_u)^{br} - \frac{1}{2} \delta^{rb} (Y_u Y_u^\dagger Y_d Y_d^\dagger)^{pa} - \lambda \left( 6\delta^{pa} (Y_u^\dagger Y_u)^{br} + 6\delta^{rb} (Y_u Y_u^\dagger)^{pa} \right) - \delta^{rb} (Y_d Y_d^\dagger Y_u Y_u^\dagger)^{pa} \right. \\ & \left. - \frac{83}{54} \delta^{pa} \delta^{rb} g_Y^2 g_s^2 - \frac{9}{4} T_4 \delta^{pa} \delta^{rb} - \frac{1831}{648} \delta^{pa} \delta^{rb} g_Y^4 - 3T_2 \delta^{pa} (Y_u^\dagger Y_u)^{br} - 3(Y_u^\dagger Y_u)^{br} (Y_u Y_u^\dagger)^{pa} - \frac{15}{4} T_2 \delta^{rb} (Y_u Y_u^\dagger)^{pa} - \frac{23}{4} \delta^{pa} \delta^{rb} g_L^4 \right\} C_{uG}^{ab} \end{aligned}$$

$$\begin{aligned}
& + C_{uG}^{*ab} \left\{ \frac{1}{2} Y_u^{pb} (Y_d Y_d^\dagger Y_u)^{ar} - \frac{1}{2} Y_u^{ar} (Y_d Y_d^\dagger Y_u)^{pb} \right\} + 2\delta^{pa} g_Y^2 C_{dB}^{ab} (Y_d^\dagger Y_u)^{br} - \frac{1}{3} g_Y^2 C_{dB}^{*ab} Y_d^{pb} Y_u^{ar} - \frac{3}{2} \delta^{pa} g_L^2 C_{dW}^{ab} (Y_d^\dagger Y_u)^{br} + \frac{3}{2} g_L^2 C_{dW}^{*ab} Y_d^{pb} Y_u^{ar} \\
& + \left\{ \frac{1}{2} T_2 \delta^{pa} (Y_d^\dagger Y_u)^{br} + \frac{7}{8} \delta^{pa} g_Y^2 (Y_d^\dagger Y_u)^{br} + \frac{5}{2} (Y_d^\dagger Y_u)^{br} (Y_d Y_d^\dagger)^{pa} + \frac{5}{2} \delta^{pa} (Y_d^\dagger Y_d Y_d^\dagger Y_u)^{br} - \frac{1}{2} (Y_d^\dagger Y_u)^{br} (Y_u Y_u^\dagger)^{pa} - g_s^2 (2Y_d^{*ab} Y_u^{pr} + 16\delta^{pa} (Y_d^\dagger Y_u)^{br}) \right. \\
& - \delta^{pa} (Y_d^\dagger Y_u Y_u^\dagger Y_u)^{br} - \frac{39}{8} \delta^{pa} g_L^2 (Y_d^\dagger Y_u)^{br} \left. \right\} C_{dG}^{ab} + C_{dG}^{*ab} \left\{ \frac{1}{2} Y_d^{pb} (Y_d Y_d^\dagger Y_u)^{ar} + T_2 Y_d^{pb} Y_u^{ar} + \frac{5}{2} Y_u^{ar} (Y_d Y_d^\dagger Y_d)^{pb} - g_s^2 (2Y_d^{ab} Y_u^{pr} + \frac{17}{3} Y_d^{pb} Y_u^{ar}) \right. \\
& - Y_d^{pb} (Y_u Y_u^\dagger Y_u)^{ar} - \frac{13}{12} g_Y^2 Y_d^{pb} Y_u^{ar} - 2Y_u^{ar} (Y_u Y_u^\dagger Y_d)^{pb} - \frac{9}{4} g_L^2 Y_d^{pb} Y_u^{ar} \left. \right\} + \left\{ \frac{2}{3} Y_u^{br} (Y_d Y_d^\dagger)^{pa} + \frac{2}{3} \delta^{pa} (Y_d Y_d^\dagger Y_u)^{br} - \frac{23}{54} \delta^{pa} g_Y^2 Y_u^{br} - \frac{7}{6} Y_u^{br} (Y_u Y_u^\dagger)^{pa} \right. \\
& - \frac{3}{2} \delta^{pa} g_L^2 Y_u^{br} - \frac{19}{6} \delta^{pa} (Y_u Y_u^\dagger Y_u)^{br} - 4\delta^{ab} g_s^2 Y_u^{pr} \left. \right\} C_{Hq}^{(\parallel)ab} + \left\{ \frac{29}{54} \delta^{pa} g_Y^2 Y_u^{br} + \frac{4}{3} Y_u^{br} (Y_d Y_d^\dagger)^{pa} + \frac{4}{3} \delta^{pa} (Y_d Y_d^\dagger Y_u)^{br} - \frac{1}{3} Y_u^{br} (Y_u Y_u^\dagger)^{pa} - \frac{7}{6} \delta^{pa} g_L^2 Y_u^{br} \right. \\
& - \frac{4}{3} \delta^{pa} (Y_u Y_u^\dagger Y_u)^{br} - 2\delta^{ab} g_s^2 Y_u^{pr} \left. \right\} C_{Hq}^{(\times)ab} + \left\{ \frac{43}{54} \delta^{rb} g_Y^2 Y_u^{pa} + \frac{5}{6} Y_u^{pa} (Y_u^\dagger Y_u)^{br} + \frac{3}{2} \delta^{rb} g_L^2 Y_u^{pa} + \frac{11}{6} \delta^{rb} (Y_u Y_u^\dagger Y_u)^{pa} + 2\delta^{ab} g_s^2 Y_u^{pr} \right. \\
& - \delta^{rb} (Y_d Y_d^\dagger Y_u)^{pa} \left. \right\} C_{Hu}^{ab} + 2\delta^{ab} g_s^2 C_{Hd}^{ab} Y_u^{pr} - \frac{1}{3} C_{Hud}^{ab} Y_u^{pa} (Y_d^\dagger Y_u)^{br} + C_{Hud}^{*ab} \left\{ \frac{1}{2} \delta^{ra} g_Y^2 Y_d^{pb} + \frac{7}{6} \delta^{ra} (Y_u Y_u^\dagger Y_d)^{pb} - \frac{1}{2} Y_d^{pb} (Y_u^\dagger Y_u)^{ar} - \frac{3}{2} \delta^{ra} g_L^2 Y_d^{pb} \right. \\
& - 2\delta^{ra} (Y_d Y_d^\dagger Y_d)^{pb} \left. \right\} - \frac{16}{27} \delta^{rd} \delta^{ab} g_Y^2 C_{\ell u}^{abcd} Y_u^{pc} - \frac{4}{27} \delta^{pa} \delta^{cd} g_Y^2 C_{qe}^{abcd} Y_u^{br} + \left\{ g_Y^2 \left( \frac{8}{27} \delta^{pa} \delta^{cd} Y_u^{br} + \frac{16}{27} \delta^{rd} \delta^{ab} Y_u^{pc} - \frac{20}{9} \delta^{pa} \delta^{rd} Y_u^{bc} \right) + g_s^2 \left( 3\delta^{pa} \delta^{cd} Y_u^{br} \right. \right. \\
& + 6\delta^{rd} \delta^{ab} Y_u^{pc} - \frac{8}{3} \delta^{pa} \delta^{rd} Y_u^{bc} \left. \right) + 2\delta^{rd} Y_u^{bc} (Y_d Y_d^\dagger)^{pa} + 3\delta^{pa} \delta^{rd} (Y_u Y_u^\dagger Y_u)^{bc} - \frac{1}{2} \delta^{pa} \delta^{rd} (Y_d Y_d^\dagger Y_u)^{bc} - Y_u^{*ad} Y_u^{pc} Y_u^{br} - \frac{4}{3} \delta^{pa} Y_u^{bc} (Y_u^\dagger Y_u)^{dr} \\
& - \frac{8}{3} \delta^{rd} Y_u^{bc} (Y_u Y_u^\dagger)^{pa} \left. \right\} C_{qu}^{(\parallel)abcd} + \left\{ g_Y^2 \left( \frac{70}{81} \delta^{rd} \delta^{ab} Y_u^{pc} + \frac{170}{81} \delta^{pa} \delta^{cd} Y_u^{br} - \frac{25}{6} \delta^{pa} \delta^{rd} Y_u^{bc} \right) + g_s^2 \left( 4\delta^{pa} \delta^{rd} Y_u^{bc} + \frac{113}{27} \delta^{pa} \delta^{cd} Y_u^{br} + \frac{226}{27} \delta^{rd} \delta^{ab} Y_u^{pc} \right) \right. \\
& + 2\delta^{pa} Y_u^{br} (Y_u^\dagger Y_u)^{dc} + 2\delta^{rd} Y_u^{pc} (Y_u Y_u^\dagger)^{ba} - \delta^{pa} Y_u^{bc} (Y_u^\dagger Y_u)^{dr} - 2\delta^{rd} Y_u^{pc} (Y_d Y_d^\dagger)^{ba} - 2\delta^{rd} Y_u^{bc} (Y_u Y_u^\dagger)^{pa} - 3Y_u^{*ad} Y_u^{pc} Y_u^{br} - \frac{9}{2} \delta^{pa} \delta^{rd} g_L^2 Y_u^{bc} \left. \right\} C_{qu}^{(\times)abcd} \\
& + \left\{ \frac{1}{6} Y_d^{*ad} Y_d^{pc} Y_u^{br} + \frac{2}{3} \delta^{pa} Y_d^{bc} (Y_d^\dagger Y_u)^{dr} + 3\delta^{pa} \delta^{cd} g_s^2 Y_u^{br} - \frac{4}{27} \delta^{pa} \delta^{cd} g_Y^2 Y_u^{br} \right\} C_{qd}^{(\parallel)abcd} + \left\{ \frac{113}{27} \delta^{pa} \delta^{cd} g_s^2 Y_u^{br} - Y_d^{*ad} Y_d^{pc} Y_u^{br} - \delta^{pa} Y_d^{bc} (Y_d^\dagger Y_u)^{dr} \right. \\
& - \frac{85}{81} \delta^{pa} \delta^{cd} g_Y^2 Y_u^{br} - 2\delta^{pa} Y_u^{br} (Y_d^\dagger Y_d)^{dc} \left. \right\} C_{qd}^{(\times)abcd} + \left\{ g_Y^2 \left( \frac{64}{27} \delta^{rb} \delta^{cd} Y_u^{pa} - \frac{152}{81} \delta^{rb} \delta^{ad} Y_u^{pc} \right) - g_s^2 \left( \frac{152}{27} \delta^{rb} \delta^{ad} Y_u^{pc} + 6\delta^{rb} \delta^{cd} Y_u^{pa} \right) \right\} C_{uu}^{abcd} \\
& - \frac{16}{27} \delta^{rd} \delta^{ab} g_Y^2 C_{eu}^{abcd} Y_u^{pc} + \left\{ \frac{3}{2} \delta^{rb} Y_d^{pc} (Y_d^\dagger Y_u)^{da} - \frac{16}{27} \delta^{rb} \delta^{cd} g_Y^2 Y_u^{pa} - 3\delta^{rb} \delta^{cd} g_s^2 Y_u^{pa} \right\} C_{ud}^{(\parallel)abcd} + \left\{ \frac{38}{81} \delta^{rb} \delta^{cd} g_Y^2 Y_u^{pa} - 2\delta^{rb} Y_u^{pa} (Y_d^\dagger Y_d)^{dc} \right.
\end{aligned}$$

$$\begin{aligned}
& -\frac{76}{27}\delta^{rb}\delta^{cd}g_s^2Y_u^{pa}\left\{C_{ud}^{(\times)abcd}+\frac{1}{6}Y_e^{*ab}C_{ledq}^{abcd}Y_d^{pc}Y_u^{dr}-\frac{1}{3}\delta^{pd}C_{ledq}^{*abcd}Y_e^{ab}(Y_d^\dagger Y_u)^{cr}+\left\{\frac{1}{12}\delta^{pc}Y_d^{*ad}(Y_u^\dagger Y_u)^{br}+\frac{1}{6}\delta^{rb}Y_d^{*ad}(Y_u Y_u^\dagger)^{pc}+\frac{1}{2}\delta^{pa}Y_d^{*cd}(Y_u^\dagger Y_u)^{br}\right.\right. \\
& +g_s^2\left(4\delta^{pa}\delta^{rb}Y_d^{*cd}+\frac{19}{2}\delta^{pc}\delta^{rb}Y_d^{*ad}\right)+\delta^{rb}Y_d^{*cd}(Y_u Y_u^\dagger)^{pa}+\frac{9}{8}\delta^{pc}\delta^{rb}g_L^2Y_d^{*ad}+\frac{5}{4}\delta^{pc}\delta^{rb}(Y_u^\dagger Y_u Y_d^\dagger)^{ad}-\frac{7}{24}\delta^{pc}\delta^{rb}g_Y^2Y_d^{*ad}-\frac{2}{3}\delta^{pa}Y_u^{*cb}(Y_d^\dagger Y_u)^{dr} \\
& -\frac{3}{4}\delta^{rb}Y_d^{*ad}(Y_d Y_d^\dagger)^{pc}-\delta^{pc}Y_u^{*ab}(Y_d^\dagger Y_u)^{dr}-\frac{3}{2}\delta^{rb}Y_d^{*cd}(Y_d Y_d^\dagger)^{pa}-\frac{15}{4}\delta^{pc}\delta^{rb}(Y_d^\dagger Y_d Y_d^\dagger)^{ad}\left\}C_{quqd}^{(\parallel)abcd}+\left(C_{quqd}^{(\parallel)*}\right)^{abcd}\left\{\frac{1}{2}Y_d^{pd}Y_u^{ab}Y_u^{cr}+\frac{5}{6}Y_d^{pd}Y_u^{ar}Y_u^{cb}\right. \\
& +\frac{3}{2}Y_d^{cd}Y_u^{pb}Y_u^{ar}-\frac{1}{2}Y_d^{ad}Y_u^{pb}Y_u^{cr}\left\}+\left\{\frac{1}{6}\delta^{pa}Y_d^{*cd}(Y_u^\dagger Y_u)^{br}+\frac{1}{4}\delta^{pc}Y_d^{*ad}(Y_u^\dagger Y_u)^{br}+\frac{1}{3}\delta^{rb}Y_d^{*cd}(Y_u Y_u^\dagger)^{pa}+\frac{1}{2}\delta^{rb}Y_d^{*ad}(Y_u Y_u^\dagger)^{pc}+g_s^2\left(\frac{14}{3}\delta^{pa}\delta^{rb}Y_d^{*cd}\right.\right. \\
& -\frac{3}{2}\delta^{pc}\delta^{rb}Y_d^{*ad}\left)+g_Y^2\left(\frac{5}{8}\delta^{pc}\delta^{rb}Y_d^{*ad}-\frac{5}{18}\delta^{pa}\delta^{rb}Y_d^{*cd}\right)+g_L^2\left(\frac{27}{8}\delta^{pc}\delta^{rb}Y_d^{*ad}-\frac{3}{2}\delta^{pa}\delta^{rb}Y_d^{*cd}\right)+\delta^{pa}\delta^{rb}(Y_u^\dagger Y_u Y_d^\dagger)^{cd}-\frac{1}{3}\delta^{pc}Y_u^{*ab}(Y_d^\dagger Y_u)^{dr} \\
& -\frac{1}{2}\delta^{pa}Y_u^{*cb}(Y_d^\dagger Y_u)^{dr}-\frac{1}{2}\delta^{rb}Y_d^{*cd}(Y_d Y_d^\dagger)^{pa}-\frac{3}{4}\delta^{rb}Y_d^{*ad}(Y_d Y_d^\dagger)^{pc}\left\}C_{quqd}^{(\times)abcd}+\left(C_{quqd}^{(\times)*}\right)^{abcd}\left\{\frac{1}{4}Y_d^{pd}Y_u^{ar}Y_u^{cb}+\frac{1}{2}Y_d^{cd}Y_u^{pb}Y_u^{ar}+\frac{3}{4}Y_d^{ad}Y_u^{pb}Y_u^{cr}+\frac{7}{6}Y_d^{pd}Y_u^{ab}Y_u^{cr}\right\} \\
& +\left\{\frac{1}{2}\delta^{rd}Y_e^{*ab}(Y_d Y_d^\dagger)^{pc}-\frac{1}{6}\delta^{pc}Y_e^{*ab}(Y_u^\dagger Y_u)^{dr}-\frac{1}{3}\delta^{rd}Y_e^{*ab}(Y_u Y_u^\dagger)^{pc}\right\}C_{lequ}^{abcd}-\frac{1}{2}C_{lequ}^{*abcd}Y_e^{ab}Y_u^{pd}Y_u^{cr}+\left\{\frac{1}{12}\delta^{pc}Y_e^{*ad}(Y_u^\dagger Y_u)^{br}+\frac{1}{6}\delta^{rb}Y_e^{*ad}(Y_u Y_u^\dagger)^{pc}\right. \\
& +\frac{9}{8}\delta^{pc}\delta^{rb}g_L^2Y_e^{*ad}+\frac{15}{8}\delta^{pc}\delta^{rb}g_Y^2Y_e^{*ad}-\frac{1}{4}\delta^{rb}Y_e^{*ad}(Y_d Y_d^\dagger)^{pc}\left\}C_{luqe}^{abcd}+\frac{1}{4}C_{luqe}^{*abcd}Y_e^{ad}Y_u^{pb}Y_u^{cr}+\left\{g_Y^2\left(\frac{8}{27}\delta^{pa}\delta^{cd}Y_u^{br}-\frac{77}{81}\delta^{pa}\delta^{bc}Y_u^{dr}\right)\right. \\
& +3\delta^{pa}Y_u^{dr}(Y_d Y_d^\dagger)^{bc}-g_s^2\left(\frac{152}{27}\delta^{pa}\delta^{bc}Y_u^{dr}+12\delta^{pa}\delta^{cd}Y_u^{br}\right)-\frac{5}{3}\delta^{pa}\delta^{bc}g_L^2Y_u^{dr}\left\}C_{qq}^{(\parallel)abcd}+\left\{g_Y^2\left(\frac{4}{27}\delta^{pa}\delta^{cd}Y_u^{br}-\frac{154}{81}\delta^{pa}\delta^{bc}Y_u^{dr}\right)+4\delta^{pa}\delta^{cd}g_L^2Y_u^{br}\right. \\
& \left.-g_s^2\left(6\delta^{pa}\delta^{cd}Y_u^{br}+\frac{304}{27}\delta^{pa}\delta^{bc}Y_u^{dr}\right)-3\delta^{pa}Y_u^{dr}(Y_d Y_d^\dagger)^{bc}\right\}C_{qq}^{(\times)abcd}-\frac{4}{27}\delta^{pc}\delta^{ab}g_Y^2C_{lq}^{(\parallel)abcd}Y_u^{dr}+\left\{\frac{2}{3}\delta^{pc}\delta^{ab}g_L^2Y_u^{dr}-\frac{2}{27}\delta^{pc}\delta^{ab}g_Y^2Y_u^{dr}\right\}C_{lq}^{(\times)abcd}, \tag{8.10}
\end{aligned}$$

## 8.6 $C_{dB}$

$$\begin{aligned}
\beta_{C_{dB}^{pr}}^{(1)} & = -\frac{1}{3}g_Y^2C_{HB}Y_d^{pr}+\frac{i}{3}g_Y^2C_{H\tilde{B}}Y_d^{pr}+\frac{3}{4}g_L^2C_{HWB}Y_d^{pr}-\frac{3i}{4}g_L^2C_{H\widetilde{W}B}Y_d^{pr}-\delta^{pa}C_{uB}^{ab}(Y_u^\dagger Y_d)^{br}+\left\{\frac{7}{36}\delta^{pa}\delta^{rb}g_Y^2+\frac{1}{2}\left(2T_2\delta^{pa}\delta^{rb}+4\delta^{pa}(Y_d^\dagger Y_d)^{br}\right.\right. \\
& +5\delta^{rb}(Y_d Y_d^\dagger)^{pa}-3\delta^{rb}(Y_u Y_u^\dagger)^{pa}\left)+\frac{8}{3}\delta^{pa}\delta^{rb}g_s^2-\frac{9}{4}\delta^{pa}\delta^{rb}g_L^2\right\}C_{dB}^{ab}+\frac{5}{4}\delta^{pa}\delta^{rb}g_L^2C_{dW}^{ab}-\frac{8}{9}\delta^{pa}\delta^{rb}g_s^2C_{dG}^{ab}+\frac{5}{12}\delta^{pa}\delta^{rd}Y_u^{*cb}C_{quqd}^{(\parallel)abcd} \\
& +\frac{5}{4}\delta^{pa}\delta^{rd}Y_u^{*cb}C_{quqd}^{(\times)abcd}, \tag{8.11}
\end{aligned}$$

$$\begin{aligned}
\beta_{\mathbf{C}_{dB}^{pr}}^{(2)} = & \left\{ \frac{1}{72} g_Y^2 Y_d^{pr} + \frac{1}{8} (Y_d Y_d^\dagger Y_d)^{pr} + \frac{1}{4} g_L^2 Y_d^{pr} - \frac{1}{3} (Y_u Y_u^\dagger Y_d)^{pr} \right\} \mathbf{C}_{HD}^{(\parallel)} + \left\{ \frac{1}{3} (Y_u Y_u^\dagger Y_d)^{pr} - \frac{5}{144} g_Y^2 Y_d^{pr} - \frac{1}{8} (Y_d Y_d^\dagger Y_d)^{pr} - \frac{3}{16} g_L^2 Y_d^{pr} \right\} \mathbf{C}_{HD}^{(\times)} \\
& + \left\{ \frac{29}{108} g_Y^4 Y_d^{pr} + \frac{1}{2} \lambda g_Y^2 Y_d^{pr} + g_Y^2 \left( \frac{1}{12} (Y_u Y_u^\dagger Y_d)^{pr} + \frac{1}{6} \text{T}_2 Y_d^{pr} + \frac{1}{4} (Y_d Y_d^\dagger Y_d)^{pr} \right) + \frac{8}{3} g_Y^2 g_s^2 Y_d^{pr} - \frac{1}{8} g_Y^2 g_L^2 Y_d^{pr} \right\} \mathbf{C}_{HB} + \left\{ \frac{i}{8} g_Y^2 g_L^2 Y_d^{pr} \right. \\
& + g_Y^2 \left( \frac{19i}{12} (Y_u Y_u^\dagger Y_d)^{pr} - \frac{i}{6} \text{T}_2 Y_d^{pr} - \frac{i}{4} (Y_d Y_d^\dagger Y_d)^{pr} \right) - \frac{29i}{108} g_Y^4 Y_d^{pr} - \frac{i}{2} \lambda g_Y^2 Y_d^{pr} - \frac{8i}{3} g_Y^2 g_s^2 Y_d^{pr} \left. \right\} \mathbf{C}_{H\tilde{B}} + \frac{1}{8} g_L^4 \mathbf{C}_{HW} Y_d^{pr} - \frac{i}{8} g_L^4 \mathbf{C}_{H\tilde{W}} Y_d^{pr} \\
& + \frac{4}{3} g_s^4 \mathbf{C}_{HG} Y_d^{pr} - \frac{4i}{3} g_s^4 \mathbf{C}_{H\tilde{G}} Y_d^{pr} + \left\{ \frac{9}{32} g_Y^2 g_L^2 Y_d^{pr} + \frac{425}{96} g_L^4 Y_d^{pr} - \frac{3}{8} \lambda g_L^2 Y_d^{pr} - g_L^2 \left( \frac{3}{8} \text{T}_2 Y_d^{pr} + \frac{9}{16} (Y_d Y_d^\dagger Y_d)^{pr} + \frac{15}{16} (Y_u Y_u^\dagger Y_d)^{pr} \right) \right. \\
& - 6 g_s^2 g_L^2 Y_d^{pr} \left. \right\} \mathbf{C}_{HWB} + \left\{ \frac{3i}{8} \lambda g_L^2 Y_d^{pr} + g_L^2 \left( \frac{3i}{16} (Y_u Y_u^\dagger Y_d)^{pr} + \frac{3i}{8} \text{T}_2 Y_d^{pr} + \frac{9i}{16} (Y_d Y_d^\dagger Y_d)^{pr} \right) + 6i g_s^2 g_L^2 Y_d^{pr} - \frac{9i}{32} g_Y^2 g_L^2 Y_d^{pr} \right. \\
& - \frac{425i}{96} g_L^4 Y_d^{pr} \left. \right\} \mathbf{C}_{H\tilde{W}B} - \frac{21}{4} g_L^6 \mathbf{C}_W Y_d^{pr} + \frac{35i}{12} g_L^6 \mathbf{C}_{\tilde{W}} Y_d^{pr} + 2 g_s^6 \mathbf{C}_G Y_d^{pr} - \frac{26i}{9} g_s^6 \mathbf{C}_{\tilde{G}} Y_d^{pr} + \left\{ \frac{3}{8} \delta^{pa} \delta^{rb} g_L^2 - \frac{1}{8} \delta^{pa} \delta^{rb} g_Y^2 - \frac{1}{8} \delta^{pa} (Y_d^\dagger Y_d)^{br} \right. \\
& - \frac{1}{8} \delta^{rb} (Y_d Y_d^\dagger)^{pa} \left. \right\} \mathbf{C}_{dH}^{ab} + \left\{ \frac{5}{4} g_Y^2 Y_e^{*ab} Y_d^{pr} + \frac{9}{4} g_L^2 Y_e^{*ab} Y_d^{pr} \right\} \mathbf{C}_{eB}^{ab} - \frac{9}{4} g_L^2 Y_e^{*ab} \mathbf{C}_{eW}^{ab} Y_d^{pr} + \left\{ \frac{1}{2} \text{T}_2 \delta^{pa} (Y_u^\dagger Y_d)^{br} + g_L^2 \left( \frac{9}{4} Y_u^{*ab} Y_d^{pr} - \frac{39}{8} \delta^{pa} (Y_u^\dagger Y_d)^{br} \right) \right. \\
& + g_Y^2 \left( \frac{5}{12} Y_u^{*ab} Y_d^{pr} - \frac{11}{24} \delta^{pa} (Y_u^\dagger Y_d)^{br} \right) + \frac{5}{2} (Y_u^\dagger Y_d)^{br} (Y_u Y_u^\dagger)^{pa} + \frac{5}{2} \delta^{pa} (Y_u^\dagger Y_u Y_u^\dagger Y_d)^{br} - \frac{1}{2} (Y_u^\dagger Y_d)^{br} (Y_d Y_d^\dagger)^{pa} - \delta^{pa} (Y_u^\dagger Y_d Y_d^\dagger Y_d)^{br} \left. \right\} \mathbf{C}_{uB}^{ab} \\
& + \mathbf{C}_{uB}^{*ab} \left\{ \frac{1}{2} Y_u^{pb} (Y_u Y_u^\dagger Y_d)^{ar} + \text{T}_2 Y_d^{ar} Y_u^{pb} + g_Y^2 \left( \frac{5}{12} Y_d^{pr} Y_u^{ab} - \frac{2}{9} Y_d^{ar} Y_u^{pb} \right) + \frac{5}{2} Y_d^{ar} (Y_u Y_u^\dagger Y_u)^{pb} - Y_u^{pb} (Y_d Y_d^\dagger Y_d)^{ar} - 2 Y_d^{ar} (Y_d Y_d^\dagger Y_u)^{pb} - \frac{9}{4} g_L^2 Y_d^{ar} Y_u^{pb} \right. \\
& - 8 g_s^2 Y_d^{ar} Y_u^{pb} \left. \right\} - \frac{5}{8} \delta^{pa} g_L^2 \mathbf{C}_{uW}^{ab} (Y_u^\dagger Y_d)^{br} + g_L^2 \mathbf{C}_{uW}^{*ab} \left\{ \frac{15}{8} Y_d^{pr} Y_u^{ab} - \frac{1}{8} Y_d^{ar} Y_u^{pb} \right\} + \frac{8}{3} \delta^{pa} g_s^2 \mathbf{C}_{uG}^{ab} (Y_u^\dagger Y_d)^{br} + \frac{44}{9} g_s^2 \mathbf{C}_{uG}^{*ab} Y_d^{ar} Y_u^{pb} \\
& + \left\{ g_L^2 \left( \frac{9}{16} \delta^{rb} (Y_u Y_u^\dagger)^{pa} + \frac{15}{8} \text{T}_2 \delta^{pa} \delta^{rb} + \frac{27}{4} Y_d^{*ab} Y_d^{pr} + 9 \delta^{pa} (Y_d^\dagger Y_d)^{br} + \frac{237}{16} \delta^{rb} (Y_d Y_d^\dagger)^{pa} \right) + g_Y^2 \left( \frac{5}{12} Y_d^{*ab} Y_d^{pr} + \frac{601}{144} \delta^{rb} (Y_d Y_d^\dagger)^{pa} \right. \right. \\
& + \frac{349}{72} \delta^{pa} (Y_d^\dagger Y_d)^{br} + \frac{39}{8} \delta^{pa} \delta^{rb} \text{Tr} [Y_e^\dagger Y_e] - \frac{3}{8} \delta^{pa} \delta^{rb} \text{Tr} [Y_d^\dagger Y_d] - \frac{101}{144} \delta^{rb} (Y_u Y_u^\dagger)^{pa} - \frac{29}{8} \delta^{pa} \delta^{rb} \text{Tr} [Y_u^\dagger Y_u] \left. \right) + g_s^2 \left( 20 \delta^{pa} \delta^{rb} \text{Tr} [Y_d^\dagger Y_d] \right. \\
& + 20 \delta^{pa} \delta^{rb} \text{Tr} [Y_u^\dagger Y_u] - \frac{16}{3} \delta^{rb} (Y_d Y_d^\dagger)^{pa} - \frac{16}{3} \delta^{rb} (Y_u Y_u^\dagger)^{pa} - \frac{32}{3} \delta^{pa} (Y_d^\dagger Y_d)^{br} + \frac{5}{4} \text{T}_2 \delta^{rb} (Y_u Y_u^\dagger)^{pa} + \frac{5}{4} \delta^{pa} (Y_d^\dagger Y_d Y_d^\dagger Y_d)^{br} + \frac{5}{4} \delta^{rb} (Y_d Y_d^\dagger Y_d Y_d^\dagger)^{pa} \\
& + \frac{3}{2} \delta^{pa} \delta^{rb} \lambda^2 + \frac{3}{2} \delta^{pa} \delta^{rb} \text{Tr} [Y_d^\dagger Y_d Y_u^\dagger Y_u] + \frac{103}{48} \delta^{pa} \delta^{rb} g_Y^2 g_L^2 + \frac{11}{4} \delta^{rb} (Y_u Y_u^\dagger Y_u Y_u^\dagger)^{pa} + \frac{172}{3} \delta^{pa} \delta^{rb} g_s^4 - \frac{1}{4} \delta^{pa} (Y_d^\dagger Y_u Y_u^\dagger Y_d)^{br} \\
& - \frac{1}{2} \delta^{rb} (Y_d Y_d^\dagger Y_u Y_u^\dagger)^{pa} - \lambda \left( \frac{3}{2} \delta^{pa} \delta^{rb} g_Y^2 + 6 \delta^{pa} (Y_d^\dagger Y_d)^{br} + 6 \delta^{rb} (Y_d Y_d^\dagger)^{pa} \right) - \delta^{rb} (Y_u Y_u^\dagger Y_d Y_d^\dagger)^{pa} - \frac{31}{27} \delta^{pa} \delta^{rb} g_Y^2 g_s^2 - \frac{1577}{1296} \delta^{pa} \delta^{rb} g_Y^4
\end{aligned}$$

$$\begin{aligned}
& -\frac{9}{4}\text{T}_4\delta^{pa}\delta^{rb} - 3\text{T}_2\delta^{pa}(Y_d^\dagger Y_d)^{br} - 3(Y_d^\dagger Y_d)^{br}(Y_d Y_d^\dagger)^{pa} - \frac{15}{4}\text{T}_2\delta^{rb}(Y_d Y_d^\dagger)^{pa} - \frac{23}{4}\delta^{pa}\delta^{rb}g_L^4 - 7\delta^{pa}\delta^{rb}g_s^2g_L^2 \Big\} C_{dB}^{ab} \\
& + C_{dB}^{*ab} \Big\{ \frac{1}{2}Y_d^{pb}(Y_u Y_u^\dagger Y_d)^{ar} - \frac{1}{2}Y_d^{ar}(Y_u Y_u^\dagger Y_d)^{pb} \Big\} + \Big\{ \frac{221}{288}\delta^{pa}\delta^{rb}g_Y^2g_L^2 + g_L^2\Big(\frac{1}{16}\delta^{rb}(Y_d Y_d^\dagger)^{pa} - \frac{1}{2}\delta^{rb}(Y_u Y_u^\dagger)^{pa} - \frac{11}{16}\delta^{pa}(Y_d^\dagger Y_d)^{br} - \frac{3}{4}Y_d^{*ab}Y_d^{pr} \\
& - \frac{3}{4}\delta^{pa}\delta^{rb}\text{Tr}[Y_u^\dagger Y_u] - \frac{15}{8}\delta^{pa}\delta^{rb}\text{Tr}[Y_e^\dagger Y_e] - \frac{21}{8}\delta^{pa}\delta^{rb}\text{Tr}[Y_d^\dagger Y_d] \Big) + \frac{1609}{288}\delta^{pa}\delta^{rb}g_L^4 - \frac{2}{3}\delta^{pa}\delta^{rb}g_s^2g_L^2 - \frac{3}{4}\delta^{pa}\delta^{rb}\lambda g_L^2 \Big\} C_{dW}^{ab} \\
& + \Big\{ \frac{1}{3}\delta^{pa}\delta^{rb}g_s^2g_L^2 + g_s^2\Big(\frac{16}{9}\delta^{rb}(Y_u Y_u^\dagger)^{pa} + \frac{38}{9}\delta^{pa}(Y_d^\dagger Y_d)^{br} - \frac{14}{9}\delta^{rb}(Y_d Y_d^\dagger)^{pa} \Big) - \frac{7}{81}\delta^{pa}\delta^{rb}g_Y^2g_s^2 - \frac{164}{27}\delta^{pa}\delta^{rb}g_s^4 \Big\} C_{dG}^{ab} - \frac{1}{9}\delta^{ab}g_Y^2C_{H\ell}^{(\parallel)ab}Y_d^{pr} \\
& - \Big\{ \frac{1}{18}\delta^{ab}g_Y^2Y_d^{pr} + \frac{1}{2}\delta^{ab}g_L^2Y_d^{pr} \Big\} C_{H\ell}^{(\times)ab} + \frac{7}{18}\delta^{ab}g_Y^2C_{He}^{ab}Y_d^{pr} + \Big\{ \frac{1}{4}\delta^{pa}g_L^2Y_d^{br} + \frac{47}{72}\delta^{pa}(Y_d Y_d^\dagger Y_d)^{br} + g_Y^2\Big(\frac{19}{81}\delta^{pa}Y_d^{br} - \frac{1}{9}\delta^{ab}Y_d^{pr} \Big) - \frac{1}{9}Y_d^{br}(Y_u Y_u^\dagger)^{pa} \\
& - \frac{1}{9}\delta^{pa}(Y_u Y_u^\dagger Y_d)^{br} - \frac{49}{72}Y_d^{br}(Y_d Y_d^\dagger)^{pa} - \frac{4}{3}\delta^{pa}g_s^2Y_d^{br} - \frac{3}{2}\delta^{pa}\lambda Y_d^{br} \Big\} C_{Hq}^{(\parallel)ab} + \Big\{ \frac{1}{9}Y_d^{br}(Y_u Y_u^\dagger)^{pa} + \frac{1}{9}\delta^{pa}(Y_u Y_u^\dagger Y_d)^{br} + \frac{13}{72}\delta^{pa}(Y_d Y_d^\dagger Y_d)^{br} \\
& + g_Y^2\Big(\frac{211}{648}\delta^{pa}Y_d^{br} - \frac{1}{18}\delta^{ab}Y_d^{pr} \Big) + g_L^2\Big(\frac{13}{72}\delta^{pa}Y_d^{br} + \frac{3}{2}\delta^{ab}Y_d^{pr} \Big) - \frac{35}{72}Y_d^{br}(Y_d Y_d^\dagger)^{pa} - \frac{3}{2}\delta^{pa}\lambda Y_d^{br} - \frac{8}{3}\delta^{pa}g_s^2Y_d^{br} \Big\} C_{Hq}^{(\times)ab} + \frac{1}{3}\delta^{ab}g_Y^2C_{Hu}^{ab}Y_d^{pr} \\
& + \Big\{ \frac{35}{72}\delta^{rb}(Y_d Y_d^\dagger Y_d)^{pa} + \frac{1}{2}\delta^{rb}g_L^2Y_d^{pa} + g_Y^2\Big(\frac{1}{6}\delta^{ab}Y_d^{pr} + \frac{115}{324}\delta^{rb}Y_d^{pa} \Big) + \frac{7}{6}\delta^{rb}(Y_u Y_u^\dagger Y_d)^{pa} - \frac{25}{72}Y_d^{pa}(Y_d^\dagger Y_d)^{br} - \frac{4}{3}\delta^{rb}g_s^2Y_d^{pa} - \frac{3}{2}\delta^{rb}\lambda Y_d^{pa} \Big\} C_{Hd}^{ab} \\
& + \Big\{ \frac{53}{72}\delta^{rb}(Y_d Y_d^\dagger Y_u)^{pa} + \frac{79}{72}\delta^{rb}g_Y^2Y_u^{pa} - \frac{5}{24}Y_u^{pa}(Y_d^\dagger Y_d)^{br} - \frac{4}{3}\delta^{rb}g_s^2Y_u^{pa} - \frac{11}{8}\delta^{rb}g_L^2Y_u^{pa} - \frac{19}{12}\delta^{rb}(Y_u Y_u^\dagger Y_u)^{pa} \Big\} C_{Hud}^{ab} - \frac{5}{36}C_{Hud}^{*ab}Y_d^{pb}(Y_u^\dagger Y_d)^{ar} \\
& - \Big\{ \frac{43}{162}\delta^{rd}\delta^{ab}g_Y^2Y_d^{pc} + \frac{3}{4}\delta^{rd}Y_d^{pc}(Y_e Y_e^\dagger)^{ba} \Big\} C_{\ell d}^{abcd} - \Big\{ \frac{3}{4}\delta^{pa}Y_d^{br}(Y_e^\dagger Y_e)^{dc} + \frac{193}{162}\delta^{pa}\delta^{cd}g_Y^2Y_d^{br} \Big\} C_{qe}^{abcd} + \Big\{ \frac{11}{18}\delta^{pa}Y_u^{bc}(Y_u^\dagger Y_d)^{dr} - \frac{7}{72}Y_u^{*ad}Y_d^{br}Y_u^{pc} \\
& - \frac{77}{81}\delta^{pa}\delta^{cd}g_Y^2Y_d^{br} - 4\delta^{pa}Y_d^{br}(Y_u^\dagger Y_u)^{dc} \Big\} C_{qu}^{(\parallel)abcd} + \Big\{ \frac{11}{6}\delta^{pa}Y_u^{bc}(Y_u^\dagger Y_d)^{dr} + \frac{448}{81}\delta^{pa}\delta^{cd}g_s^2Y_d^{br} - \frac{7}{24}Y_u^{*ad}Y_d^{br}Y_u^{pc} - \frac{77}{243}\delta^{pa}\delta^{cd}g_Y^2Y_d^{br} \\
& - \frac{4}{3}\delta^{pa}Y_d^{br}(Y_u^\dagger Y_u)^{dc} \Big\} C_{qu}^{(\times)abcd} + \Big\{ \frac{5}{18}\delta^{pa}Y_d^{bc}(Y_d^\dagger Y_d)^{dr} + \frac{7}{24}\delta^{pa}\delta^{rd}(Y_u Y_u^\dagger Y_d)^{bc} + \frac{1}{3}\delta^{rd}Y_d^{bc}(Y_u Y_u^\dagger)^{pa} + g_Y^2\Big(\frac{43}{162}\delta^{rd}\delta^{ab}Y_d^{pc} - \frac{5}{54}\delta^{pa}\delta^{rd}Y_d^{bc} \\
& - \frac{85}{162}\delta^{pa}\delta^{cd}Y_d^{br} \Big) + \frac{20}{9}\delta^{pa}\delta^{rd}g_s^2Y_d^{bc} - \frac{1}{12}Y_d^{*ad}Y_d^{pc}Y_d^{br} - \frac{1}{9}\delta^{rd}Y_d^{bc}(Y_d Y_d^\dagger)^{pa} - \frac{1}{4}\delta^{pa}\delta^{rd}(Y_d Y_d^\dagger Y_d)^{bc} - \frac{1}{2}Y_d^{*ad}Y_d^{pr}Y_d^{bc} - \frac{1}{2}\delta^{pa}Y_d^{br}(Y_d^\dagger Y_d)^{dc} \\
& - \frac{1}{2}\delta^{rd}Y_d^{pc}(Y_d Y_d^\dagger)^{ba} - \frac{1}{2}\delta^{pa}\delta^{rd}Y_d^{bc}\text{Tr}[Y_d^\dagger Y_d] - \delta^{rd}Y_d^{pc}(Y_u Y_u^\dagger)^{ba} \Big\} C_{qd}^{(\parallel)abcd} + \Big\{ \frac{5}{6}\delta^{pa}Y_d^{bc}(Y_d^\dagger Y_d)^{dr} + \frac{7}{8}\delta^{pa}\delta^{rd}(Y_u Y_u^\dagger Y_d)^{bc} + g_s^2\Big(\frac{152}{81}\delta^{rd}\delta^{ab}Y_d^{pc}
\end{aligned}$$

$$\begin{aligned}
& + \frac{20}{3} \delta^{pa} \delta^{rd} Y_d^{bc} - \frac{200}{81} \delta^{pa} \delta^{cd} Y_d^{br} \Big) + g_Y^2 \Big( \frac{43}{486} \delta^{rd} \delta^{ab} Y_d^{pc} - \frac{85}{486} \delta^{pa} \delta^{cd} Y_d^{br} - \frac{5}{18} \delta^{pa} \delta^{rd} Y_d^{bc} \Big) + \delta^{rd} Y_d^{bc} (Y_u Y_u^\dagger)^{pa} - \frac{1}{6} \delta^{pa} Y_d^{br} (Y_d^\dagger Y_d)^{dc} - \frac{1}{6} \delta^{rd} Y_d^{pc} (Y_d Y_d^\dagger)^{ba} \\
& - \frac{1}{4} Y_d^{*ad} Y_d^{pc} Y_d^{br} - \frac{1}{3} \delta^{rd} Y_d^{bc} (Y_d Y_d^\dagger)^{pa} - \frac{1}{3} \delta^{rd} Y_d^{pc} (Y_u Y_u^\dagger)^{ba} - \frac{3}{4} \delta^{pa} \delta^{rd} (Y_d Y_d^\dagger Y_d)^{bc} - \frac{3}{2} Y_d^{*ad} Y_d^{pr} Y_d^{bc} - \frac{3}{2} \delta^{pa} \delta^{rd} Y_d^{bc} \text{Tr}[Y_d^\dagger Y_d] \Big\} C_{qd}^{(\times)abcd} \\
& + \left\{ \frac{368}{81} \delta^{rb} \delta^{ad} g_s^2 Y_d^{pc} - g_Y^2 \left( \frac{43}{243} \delta^{rb} \delta^{ad} Y_d^{pc} + \frac{43}{81} \delta^{rb} \delta^{cd} Y_d^{pa} \right) \right\} C_{dd}^{abcd} - \left\{ \frac{43}{162} \delta^{rd} \delta^{ab} g_Y^2 Y_d^{pc} + \frac{3}{4} \delta^{rd} Y_d^{pc} (Y_e^\dagger Y_e)^{ba} \right\} C_{ed}^{abcd} + \left\{ \frac{1}{8} \delta^{rd} Y_u^{pa} (Y_u^\dagger Y_d)^{bc} \right. \\
& + \left. \frac{43}{81} \delta^{rd} \delta^{ab} g_Y^2 Y_d^{pc} - 4 \delta^{rd} Y_d^{pc} (Y_u^\dagger Y_u)^{ba} \right\} C_{ud}^{(\parallel)abcd} + \left\{ \frac{43}{243} \delta^{rd} \delta^{ab} g_Y^2 Y_d^{pc} + \frac{3}{8} \delta^{rd} Y_u^{pa} (Y_u^\dagger Y_d)^{bc} - \frac{4}{3} \delta^{rd} Y_d^{pc} (Y_u^\dagger Y_u)^{ba} - \frac{464}{81} \delta^{rd} \delta^{ab} g_s^2 Y_d^{pc} \right\} C_{ud}^{(\times)abcd} \\
& + \left\{ \frac{1}{24} Y_e^{*ab} Y_d^{pc} Y_d^{dr} + \frac{1}{4} Y_e^{*ab} Y_d^{pr} Y_d^{dc} \right\} C_{ledq}^{abcd} + C_{ledq}^{*abcd} \left\{ \frac{5}{36} \delta^{rc} Y_e^{ab} (Y_d Y_d^\dagger)^{pd} + \frac{3}{16} \delta^{pd} \delta^{rc} g_L^2 Y_e^{ab} + \frac{11}{48} \delta^{pd} \delta^{rc} g_Y^2 Y_e^{ab} + \frac{1}{4} \delta^{pd} \delta^{rc} Y_e^{ab} \text{Tr}[Y_d^\dagger Y_d] \right. \\
& - \left. \frac{7}{72} \delta^{pd} Y_e^{ab} (Y_d^\dagger Y_d)^{cr} - \frac{11}{24} \delta^{rc} Y_e^{ab} (Y_u Y_u^\dagger)^{pd} \right\} + \left\{ \frac{5}{72} \delta^{rd} Y_u^{*cb} (Y_d Y_d^\dagger)^{pa} + \frac{5}{12} \delta^{rd} Y_u^{*ab} (Y_d Y_d^\dagger)^{pc} + \frac{31}{48} \delta^{pa} \delta^{rd} (Y_d^\dagger Y_d Y_u^\dagger)^{cb} + g_L^2 \left( \frac{3}{32} \delta^{pa} \delta^{rd} Y_u^{*cb} \right. \right. \\
& - \left. \frac{15}{8} \delta^{pc} \delta^{rd} Y_u^{*ab} \right) + g_Y^2 \left( \frac{5}{32} \delta^{pa} \delta^{rd} Y_u^{*cb} - \frac{25}{72} \delta^{pc} \delta^{rd} Y_u^{*ab} \right) + \left( \frac{1}{8} \delta^{pa} \delta^{rd} Y_u^{*cb} + \frac{3}{4} \delta^{pc} \delta^{rd} Y_u^{*ab} \right) \text{Tr}[Y_d^\dagger Y_d] + \frac{7}{3} \delta^{pa} \delta^{rd} g_s^2 Y_u^{*cb} - \frac{7}{144} \delta^{pa} Y_u^{*cb} (Y_d^\dagger Y_d)^{dr} \\
& - \frac{1}{9} \delta^{pc} Y_d^{*ad} (Y_u^\dagger Y_d)^{br} - \frac{1}{4} \delta^{pc} \delta^{rd} (Y_d^\dagger Y_d Y_u^\dagger)^{ab} - \frac{7}{24} \delta^{pc} Y_u^{*ab} (Y_d^\dagger Y_d)^{dr} - \frac{7}{16} \delta^{rd} Y_u^{*cb} (Y_u Y_u^\dagger)^{pa} - \frac{11}{12} \delta^{pa} Y_d^{*cd} (Y_u^\dagger Y_d)^{br} - \frac{11}{8} \delta^{rd} Y_u^{*ab} (Y_u Y_u^\dagger)^{pc} \\
& - \left. \frac{23}{16} \delta^{pa} \delta^{rd} (Y_u^\dagger Y_u Y_u^\dagger)^{cb} \right\} C_{quqd}^{(\parallel)abcd} + \left( C_{quqd}^{(\parallel)*} \right)^{abcd} \left\{ \frac{1}{72} Y_d^{ad} Y_d^{cr} Y_u^{pb} + \frac{1}{8} Y_d^{pd} Y_d^{cr} Y_u^{ab} + \frac{1}{8} Y_d^{pr} Y_d^{ad} Y_u^{cb} + \frac{5}{24} Y_d^{ar} Y_d^{cd} Y_u^{pb} + \frac{3}{4} Y_d^{pr} Y_d^{cd} Y_u^{ab} - \frac{7}{24} Y_d^{pd} Y_d^{ar} Y_u^{cb} \right\} \\
& + \left\{ \frac{5}{36} \delta^{rd} Y_u^{*ab} (Y_d Y_d^\dagger)^{pc} + \frac{5}{24} \delta^{rd} Y_u^{*cb} (Y_d Y_d^\dagger)^{pa} + g_L^2 \left( \frac{9}{32} \delta^{pa} \delta^{rd} Y_u^{*cb} - \frac{5}{8} \delta^{pc} \delta^{rd} Y_u^{*ab} \right) + g_Y^2 \left( \frac{15}{32} \delta^{pa} \delta^{rd} Y_u^{*cb} - \frac{25}{216} \delta^{pc} \delta^{rd} Y_u^{*ab} \right) + g_s^2 \left( \frac{40}{9} \delta^{pc} \delta^{rd} Y_u^{*ab} \right. \right. \\
& + \left. 10 \delta^{pa} \delta^{rd} Y_u^{*cb} \right) + \left( \frac{1}{4} \delta^{pc} \delta^{rd} Y_u^{*ab} + \frac{3}{8} \delta^{pa} \delta^{rd} Y_u^{*cb} \right) \text{Tr}[Y_d^\dagger Y_d] + \frac{31}{16} \delta^{pa} \delta^{rd} (Y_d^\dagger Y_d Y_u^\dagger)^{cb} - \frac{1}{12} \delta^{pc} \delta^{rd} (Y_d^\dagger Y_d Y_u^\dagger)^{ab} - \frac{7}{72} \delta^{pc} Y_u^{*ab} (Y_d^\dagger Y_d)^{dr} \\
& - \frac{7}{48} \delta^{pa} Y_u^{*cb} (Y_d^\dagger Y_d)^{dr} - \frac{11}{36} \delta^{pa} Y_d^{*cd} (Y_u^\dagger Y_d)^{br} - \frac{1}{3} \delta^{pc} Y_d^{*ad} (Y_u^\dagger Y_d)^{br} - \frac{11}{24} \delta^{rd} Y_u^{*ab} (Y_u Y_u^\dagger)^{pc} - \frac{21}{16} \delta^{rd} Y_u^{*cb} (Y_u Y_u^\dagger)^{pa} - \frac{69}{16} \delta^{pa} \delta^{rd} (Y_u^\dagger Y_u Y_u^\dagger)^{cb} \Big\} C_{quqd}^{(\times)abcd} \\
& + \left( C_{quqd}^{(\times)*} \right)^{abcd} \left\{ \frac{1}{24} Y_d^{ad} Y_d^{cr} Y_u^{pb} + \frac{1}{24} Y_d^{pd} Y_d^{cr} Y_u^{ab} + \frac{5}{72} Y_d^{ar} Y_d^{cd} Y_u^{pb} + \frac{1}{4} Y_d^{pr} Y_d^{cd} Y_u^{ab} + \frac{3}{8} Y_d^{pr} Y_d^{ad} Y_u^{cb} - \frac{7}{8} Y_d^{pd} Y_d^{ar} Y_u^{cb} \right\} + \frac{11}{36} \delta^{pc} Y_e^{*ab} C_{lequ}^{abcd} (Y_u^\dagger Y_d)^{dr} \\
& - \frac{11}{72} C_{lequ}^{*abcd} Y_d^{cr} Y_e^{ab} Y_u^{pd} + \frac{2}{9} \delta^{pc} Y_e^{*ad} C_{luqe}^{abcd} (Y_u^\dagger Y_d)^{br} - \frac{1}{9} C_{luqe}^{*abcd} Y_d^{cr} Y_e^{ad} Y_u^{pb} + \left\{ \frac{2}{9} \delta^{pa} \delta^{bc} g_L^2 Y_d^{dr} + \frac{1}{4} \delta^{pa} Y_d^{dr} (Y_u Y_u^\dagger)^{bc} + g_Y^2 \left( \frac{29}{243} \delta^{pa} \delta^{bc} Y_d^{dr} \right. \right. \\
& + \left. \frac{58}{81} \delta^{pa} \delta^{cd} Y_d^{br} \right) - 2 \delta^{pa} Y_d^{br} (Y_u Y_u^\dagger)^{dc} - \frac{184}{81} \delta^{pa} \delta^{bc} g_s^2 Y_d^{dr} \Big\} C_{qq}^{(\parallel)abcd} + \left\{ \frac{2}{3} \delta^{pa} \delta^{cd} g_L^2 Y_d^{br} + g_Y^2 \left( \frac{58}{243} \delta^{pa} \delta^{bc} Y_d^{dr} + \frac{29}{81} \delta^{pa} \delta^{cd} Y_d^{br} \right) + 2 \delta^{pa} Y_d^{br} (Y_u Y_u^\dagger)^{dc} \right.
\end{aligned}$$



$$\begin{aligned}
& -\frac{1}{4}\delta^{pa}Y_d^{dr}(Y_uY_u^\dagger)^{bc}-\frac{368}{81}\delta^{pa}\delta^{bc}g_s^2Y_d^{dr}\Bigg\}C_{qq}^{(\times)abcd}+\Bigg\{\frac{25}{81}\delta^{pc}\delta^{ab}g_Y^2Y_d^{dr}-\frac{3}{4}\delta^{pc}Y_d^{dr}(Y_eY_e^\dagger)^{ba}\Bigg\}C_{\ell q}^{(\parallel)abcd}+\Bigg\{\frac{25}{162}\delta^{pc}\delta^{ab}g_Y^2Y_d^{dr}+\frac{10}{9}\delta^{pc}\delta^{ab}g_L^2Y_d^{dr} \\
& -\frac{3}{2}\delta^{pc}Y_d^{dr}(Y_eY_e^\dagger)^{ba}\Bigg\}C_{\ell q}^{(\times)abcd},
\end{aligned} \tag{8.12}$$

## 8.7 $C_{dW}$

$$\begin{aligned}
\beta_{C_{dW}^{pr}}^{(1)} &= 2g_L^2C_{HW}Y_d^{pr}-2ig_L^2C_{H\widetilde{W}}Y_d^{pr}-\frac{1}{6}g_Y^2C_{HWB}Y_d^{pr}+\frac{i}{6}g_Y^2C_{H\widetilde{W}B}Y_d^{pr}-\delta^{pa}C_{uW}^{ab}(Y_u^\dagger Y_d)^{br}+\frac{5}{3}\delta^{pa}\delta^{rb}g_Y^2C_{dB}^{ab}+\Bigg\{\frac{1}{2}\Big(\delta^{rb}(Y_dY_d^\dagger)^{pa}+2T_2\delta^{pa}\delta^{rb} \\
& +4\delta^{pa}(Y_d^\dagger Y_d)^{br}+5\delta^{rb}(Y_uY_u^\dagger)^{pa}\Big)+\frac{9}{4}\delta^{pa}\delta^{rb}g_L^2+\frac{8}{3}\delta^{pa}\delta^{rb}g_s^2-\frac{31}{36}\delta^{pa}\delta^{rb}g_Y^2\Bigg\}C_{dW}^{ab}+\frac{16}{3}\delta^{pa}\delta^{rb}g_s^2C_{dG}^{ab}-\frac{1}{2}\delta^{pa}\delta^{rd}Y_u^{*cb}C_{quqd}^{(\parallel)abcd} \\
& -\frac{3}{2}\delta^{pa}\delta^{rd}Y_u^{*cb}C_{quqd}^{(\times)abcd},
\end{aligned} \tag{8.13}$$

$$\begin{aligned}
\beta_{C_{dW}^{pr}}^{(2)} &= \Bigg\{\frac{1}{4}(Y_uY_u^\dagger Y_d)^{pr}-\frac{1}{18}g_Y^2Y_d^{pr}\Bigg\}C_{HD}^{(\parallel)}+\Bigg\{\frac{1}{72}g_Y^2Y_d^{pr}+\frac{1}{8}g_L^2Y_d^{pr}+\frac{1}{4}(Y_uY_u^\dagger Y_d)^{pr}\Bigg\}C_{HD}^{(\times)}+\frac{1}{12}g_Y^4C_{HB}Y_d^{pr}-\frac{i}{12}g_Y^4C_{H\widetilde{B}}Y_d^{pr}+\Bigg\{\frac{11}{12}g_Y^2g_L^2Y_d^{pr} \\
& +g_L^2\Big(\frac{1}{2}(Y_uY_u^\dagger Y_d)^{pr}-T_2Y_d^{pr}-\frac{9}{2}(Y_dY_d^\dagger Y_d)^{pr}\Big)+\frac{271}{18}g_L^4Y_d^{pr}-3\lambda g_L^2Y_d^{pr}-16g_s^2g_L^2Y_d^{pr}\Bigg\}C_{HW}+\Bigg\{g_L^2\Big(iT_2Y_d^{pr}+\frac{9i}{2}(Y_dY_d^\dagger Y_d)^{pr} \\
& -\frac{5i}{2}(Y_uY_u^\dagger Y_d)^{pr}\Big)+3i\lambda g_L^2Y_d^{pr}+16ig_s^2g_L^2Y_d^{pr}-\frac{11i}{12}g_Y^2g_L^2Y_d^{pr}-\frac{559i}{18}g_L^4Y_d^{pr}\Bigg\}C_{H\widetilde{W}}-8g_s^4C_{HG}Y_d^{pr}+8ig_s^4C_{H\widetilde{G}}Y_d^{pr}+\Bigg\{\frac{1}{12}\lambda g_Y^2Y_d^{pr} \\
& +\frac{61}{432}g_Y^4Y_d^{pr}+g_Y^2\Big(\frac{1}{12}T_2Y_d^{pr}+\frac{3}{8}(Y_dY_d^\dagger Y_d)^{pr}-\frac{13}{24}(Y_uY_u^\dagger Y_d)^{pr}\Big)+\frac{4}{3}g_Y^2g_s^2Y_d^{pr}-\frac{27}{16}g_Y^2g_L^2Y_d^{pr}\Bigg\}C_{HWB}+\Bigg\{g_Y^2\Big(\frac{11i}{8}(Y_uY_u^\dagger Y_d)^{pr}-\frac{i}{12}T_2Y_d^{pr} \\
& -\frac{3i}{8}(Y_dY_d^\dagger Y_d)^{pr}\Big)+\frac{27i}{16}g_Y^2g_L^2Y_d^{pr}-\frac{i}{12}\lambda g_Y^2Y_d^{pr}-\frac{61i}{432}g_Y^4Y_d^{pr}-\frac{4i}{3}g_Y^2g_s^2Y_d^{pr}\Bigg\}C_{H\widetilde{W}B}+\Bigg\{\frac{23}{6}g_Y^2g_L^4Y_d^{pr}+35g_L^6Y_d^{pr}-g_L^4\Big(\frac{3}{2}(Y_dY_d^\dagger Y_d)^{pr} \\
& +\frac{27}{2}(Y_uY_u^\dagger Y_d)^{pr}\Big)-20g_s^2g_L^4Y_d^{pr}\Bigg\}C_W+\Bigg\{g_L^4\Big(\frac{5i}{6}(Y_dY_d^\dagger Y_d)^{pr}+\frac{23i}{2}(Y_uY_u^\dagger Y_d)^{pr}\Big)+\frac{116i}{9}g_s^2g_L^4Y_d^{pr}-\frac{173i}{54}g_Y^2g_L^4Y_d^{pr}-\frac{184i}{9}g_L^6Y_d^{pr}\Bigg\}C_{\widetilde{W}} \\
& -12g_s^6C_GY_d^{pr}+\frac{52i}{3}g_s^6C_{\widetilde{G}}Y_d^{pr}+\frac{1}{2}\delta^{pa}C_{uH}^{ab}(Y_u^\dagger Y_d)^{br}+\Bigg\{\frac{1}{4}\delta^{pa}(Y_d^\dagger Y_d)^{br}+\frac{3}{4}\delta^{pa}\delta^{rb}g_L^2+\delta^{rb}(Y_uY_u^\dagger)^{pa}-\frac{1}{12}\delta^{pa}\delta^{rb}g_Y^2-\frac{1}{4}\delta^{rb}(Y_dY_d^\dagger)^{pa}\Bigg\}C_{dH}^{ab} \\
& -\frac{1}{3}g_Y^2Y_e^{*ab}C_{eB}^{ab}Y_d^{pr}+\Bigg\{\frac{3}{4}g_Y^2Y_e^{*ab}Y_d^{pr}+\frac{7}{4}g_L^2Y_e^{*ab}Y_d^{pr}\Bigg\}C_{eW}^{ab}-2\delta^{pa}g_Y^2C_{uB}^{ab}(Y_u^\dagger Y_d)^{br}-g_Y^2C_{uB}^{*ab}\Bigg\{\frac{1}{2}Y_d^{ar}Y_u^{pb}+\frac{1}{2}Y_d^{pr}Y_u^{ab}\Bigg\}+\Bigg\{\frac{1}{2}T_2\delta^{pa}(Y_u^\dagger Y_d)^{br}
\end{aligned}$$

$$\begin{aligned}
& + g_L^2 \left( \frac{3}{4} Y_u^{*ab} Y_d^{pr} + \frac{39}{8} \delta^{pa} (Y_u^\dagger Y_d)^{br} \right) + \frac{5}{2} \delta^{pa} (Y_u^\dagger Y_u Y_u^\dagger Y_d)^{br} - g_Y^2 \left( \frac{5}{12} Y_u^{*ab} Y_d^{pr} + \frac{5}{8} \delta^{pa} (Y_u^\dagger Y_d)^{br} \right) - (Y_u^\dagger Y_d)^{br} (Y_u Y_u^\dagger)^{pa} - \delta^{pa} (Y_u^\dagger Y_d Y_d^\dagger Y_d)^{br} \Big\} C_{uW}^{ab} \\
& + C_{uW}^{*ab} \left\{ \frac{1}{2} Y_u^{pb} (Y_u Y_u^\dagger Y_d)^{ar} + \frac{3}{4} g_Y^2 Y_d^{ar} Y_u^{pb} + g_L^2 \left( \frac{3}{4} Y_d^{pr} Y_u^{ab} + 2 Y_d^{ar} Y_u^{pb} \right) + Y_d^{ar} (Y_d Y_d^\dagger Y_u)^{pb} + 8 g_s^2 Y_d^{ar} Y_u^{pb} - \frac{1}{2} Y_d^{ar} (Y_u Y_u^\dagger Y_u)^{pb} - \text{T}_2 Y_d^{ar} Y_u^{pb} \right. \\
& \left. - Y_u^{pb} (Y_d Y_d^\dagger Y_d)^{ar} \right\} - 8 g_s^2 C_{uG}^{*ab} Y_d^{ar} Y_u^{pb} + \left\{ \frac{19}{24} \delta^{pa} \delta^{rb} g_Y^2 g_L^2 - \frac{8}{9} \delta^{pa} \delta^{rb} g_Y^2 g_s^2 - \delta^{pa} \delta^{rb} \lambda g_Y^2 - g_Y^2 \left( \frac{5}{12} \delta^{rb} (Y_d Y_d^\dagger)^{pa} + \frac{11}{12} \delta^{pa} (Y_d^\dagger Y_d)^{br} + Y_d^{*ab} Y_d^{pr} \right. \right. \\
& \left. \left. + \delta^{pa} \delta^{rb} \text{Tr} [Y_u^\dagger Y_u] + \frac{5}{2} \delta^{pa} \delta^{rb} \text{Tr} [Y_e^\dagger Y_e] + \frac{8}{3} \delta^{rb} (Y_u Y_u^\dagger)^{pa} + \frac{7}{2} \delta^{pa} \delta^{rb} \text{Tr} [Y_d^\dagger Y_d] \right) - \frac{395}{72} \delta^{pa} \delta^{rb} g_Y^4 \right\} C_{dB}^{ab} + \left\{ \frac{13}{27} \delta^{pa} \delta^{rb} g_Y^2 g_s^2 + \delta^{rb} (Y_u Y_u^\dagger Y_d Y_d^\dagger)^{pa} \right. \\
& \left. + g_L^2 \left( \frac{1}{8} \delta^{pa} \delta^{rb} \text{Tr} [Y_e^\dagger Y_e] + \frac{3}{8} \delta^{pa} \delta^{rb} \text{Tr} [Y_d^\dagger Y_d] + \frac{9}{8} \delta^{pa} \delta^{rb} \text{Tr} [Y_u^\dagger Y_u] + \frac{63}{16} \delta^{rb} (Y_d Y_d^\dagger)^{pa} + \frac{21}{4} Y_d^{*ab} Y_d^{pr} + \frac{129}{16} \delta^{rb} (Y_u Y_u^\dagger)^{pa} + \frac{103}{8} \delta^{pa} (Y_d^\dagger Y_d)^{br} \right) \right. \\
& \left. + g_Y^2 \left( \frac{1}{4} Y_d^{*ab} Y_d^{pr} + \frac{119}{144} \delta^{rb} (Y_d Y_d^\dagger)^{pa} + \frac{25}{24} \delta^{pa} \delta^{rb} \text{Tr} [Y_d^\dagger Y_d] + \frac{25}{8} \delta^{pa} \delta^{rb} \text{Tr} [Y_e^\dagger Y_e] + \frac{85}{24} \delta^{pa} \delta^{rb} \text{Tr} [Y_u^\dagger Y_u] + \frac{40}{9} \delta^{pa} (Y_d^\dagger Y_d)^{br} + \frac{707}{144} \delta^{rb} (Y_u Y_u^\dagger)^{pa} \right) \right. \\
& \left. + g_s^2 \left( 20 \delta^{pa} \delta^{rb} \text{Tr} [Y_d^\dagger Y_d] + 20 \delta^{pa} \delta^{rb} \text{Tr} [Y_u^\dagger Y_u] - \frac{16}{3} \delta^{rb} (Y_d Y_d^\dagger)^{pa} - \frac{16}{3} \delta^{rb} (Y_u Y_u^\dagger)^{pa} - \frac{32}{3} \delta^{pa} (Y_d^\dagger Y_d)^{br} \right) + \frac{5}{4} \delta^{pa} (Y_d^\dagger Y_d Y_d^\dagger Y_d)^{br} + \frac{3}{2} \delta^{pa} \delta^{rb} \lambda^2 \right. \\
& \left. + \frac{3}{2} \delta^{pa} \delta^{rb} \text{Tr} [Y_d^\dagger Y_d Y_u^\dagger Y_u] + \frac{7}{4} \delta^{rb} (Y_d Y_d^\dagger Y_d Y_d^\dagger)^{pa} + \frac{2219}{648} \delta^{pa} \delta^{rb} g_Y^4 + \frac{161}{16} \delta^{pa} \delta^{rb} g_L^4 + \frac{172}{3} \delta^{pa} \delta^{rb} g_s^4 - \frac{1}{4} \delta^{pa} (Y_d^\dagger Y_u Y_u^\dagger Y_d)^{br} \right. \\
& \left. - \frac{3}{4} \text{T}_2 \delta^{rb} (Y_d Y_d^\dagger)^{pa} - \lambda \left( \frac{3}{2} \delta^{pa} \delta^{rb} g_L^2 + 2 \delta^{rb} (Y_d Y_d^\dagger)^{pa} + 4 \delta^{rb} (Y_u Y_u^\dagger)^{pa} + 6 \delta^{pa} (Y_d^\dagger Y_d)^{br} \right) - \frac{23}{16} \delta^{pa} \delta^{rb} g_Y^2 g_L^2 - 2 (Y_d^\dagger Y_d)^{br} (Y_d Y_d^\dagger)^{pa} \right. \\
& \left. - 2 (Y_d^\dagger Y_d)^{br} (Y_u Y_u^\dagger)^{pa} - \frac{9}{4} \text{T}_4 \delta^{pa} \delta^{rb} - \frac{11}{4} \text{T}_2 \delta^{rb} (Y_u Y_u^\dagger)^{pa} - 3 \delta^{pa} \delta^{rb} g_s^2 g_L^2 - 3 \text{T}_2 \delta^{pa} (Y_d^\dagger Y_d)^{br} - \frac{13}{4} \delta^{rb} (Y_u Y_u^\dagger Y_u Y_u^\dagger)^{pa} \right\} C_{dW}^{ab} \\
& + C_{dW}^{*ab} \left\{ \frac{1}{2} Y_d^{ar} (Y_u Y_u^\dagger Y_d)^{pb} - \frac{1}{2} Y_d^{pb} (Y_u Y_u^\dagger Y_d)^{ar} \right\} + \left\{ \frac{14}{27} \delta^{pa} \delta^{rb} g_Y^2 g_s^2 + \frac{328}{9} \delta^{pa} \delta^{rb} g_s^4 - g_s^2 \left( \frac{4}{3} \delta^{pa} (Y_d^\dagger Y_d)^{br} + \frac{16}{3} \delta^{rb} (Y_u Y_u^\dagger)^{pa} + \frac{28}{3} \delta^{rb} (Y_d Y_d^\dagger)^{pa} \right) \right. \\
& \left. - \frac{14}{3} \delta^{pa} \delta^{rb} g_s^2 g_L^2 \right\} C_{dG}^{ab} + \left\{ \frac{1}{9} \delta^{ab} g_Y^2 Y_d^{pr} + \delta^{ab} g_L^2 Y_d^{pr} \right\} C_{H\ell}^{(\parallel)ab} + \left\{ \frac{2}{9} \delta^{ab} g_Y^2 Y_d^{pr} + \delta^{ab} g_L^2 Y_d^{pr} \right\} C_{H\ell}^{(\times)ab} + \frac{1}{9} \delta^{ab} g_Y^2 C_{He}^{ab} Y_d^{pr} + \left\{ \frac{5}{6} \delta^{pa} (Y_u Y_u^\dagger Y_d)^{br} \right. \\
& \left. + g_Y^2 \left( \frac{23}{27} \delta^{pa} Y_d^{br} - \frac{1}{9} \delta^{ab} Y_d^{pr} \right) + g_L^2 \left( 3 \delta^{ab} Y_d^{pr} - 5 \delta^{pa} Y_d^{br} \right) + \frac{4}{3} Y_d^{br} (Y_u Y_u^\dagger)^{pa} - \frac{1}{12} \delta^{pa} (Y_d Y_d^\dagger Y_d)^{br} - \delta^{pa} \lambda Y_d^{br} - \frac{19}{12} Y_d^{br} (Y_d Y_d^\dagger)^{pa} - \frac{8}{3} \delta^{pa} g_s^2 Y_d^{br} \right\} C_{Hq}^{(\parallel)ab} \\
& + \left\{ g_L^2 \left( \frac{7}{3} \delta^{pa} Y_d^{br} + 3 \delta^{ab} Y_d^{pr} \right) + \frac{25}{12} \delta^{pa} (Y_d Y_d^\dagger Y_d)^{br} - \frac{1}{3} Y_d^{br} (Y_u Y_u^\dagger)^{pa} - \frac{5}{12} Y_d^{br} (Y_d Y_d^\dagger)^{pa} - g_Y^2 \left( \frac{2}{9} \delta^{ab} Y_d^{pr} + \frac{11}{27} \delta^{pa} Y_d^{br} \right) - \frac{4}{3} \delta^{pa} (Y_u Y_u^\dagger Y_d)^{br} - 2 \delta^{pa} \lambda Y_d^{br} \right. \\
& \left. - \frac{16}{3} \delta^{pa} g_s^2 Y_d^{br} \right\} C_{Hq}^{(\times)ab} - \left\{ \frac{2}{9} \delta^{ab} g_Y^2 Y_d^{pr} + \frac{1}{2} Y_u^{pa} (Y_u^\dagger Y_d)^{br} \right\} C_{Hu}^{ab} + \left\{ \frac{3}{4} \delta^{rb} (Y_d Y_d^\dagger Y_d)^{pa} + g_Y^2 \left( \frac{1}{9} \delta^{ab} Y_d^{pr} + \frac{5}{18} \delta^{rb} Y_d^{pa} \right) - \frac{1}{2} \delta^{rb} g_L^2 Y_d^{pa} - \frac{3}{4} Y_d^{pa} (Y_d^\dagger Y_d)^{br} \right.
\end{aligned}$$

$$\begin{aligned}
& -\delta^{rb}\lambda Y_d^{pa} - \delta^{rb}(Y_u Y_u^\dagger Y_d)^{pa} - \frac{8}{3}\delta^{rb}g_s^2 Y_d^{pa} \Big\} C_{Hd}^{ab} + \left\{ \frac{1}{2}\delta^{rb}(Y_u Y_u^\dagger Y_u)^{pa} - \frac{1}{18}\delta^{rb}g_Y^2 Y_u^{pa} - \frac{1}{4}Y_u^{pa}(Y_d^\dagger Y_d)^{br} - \frac{1}{2}\delta^{rb}g_L^2 Y_u^{pa} - \frac{3}{4}\delta^{rb}(Y_d Y_d^\dagger Y_u)^{pa} \right. \\
& - \delta^{rb}\lambda Y_u^{pa} - \frac{8}{3}\delta^{rb}g_s^2 Y_u^{pa} \Big\} C_{Hud}^{ab} + \left\{ \frac{1}{2}\delta^{rd}Y_d^{pc}(Y_e Y_e^\dagger)^{ba} + 2\delta^{rd}\delta^{ab}g_L^2 Y_d^{pc} - \frac{1}{3}\delta^{rd}\delta^{ab}g_Y^2 Y_d^{pc} \right\} C_{\ell d}^{abcd} + \left\{ \frac{1}{2}\delta^{pa}Y_d^{br}(Y_e^\dagger Y_e)^{dc} - \frac{13}{27}\delta^{pa}\delta^{cd}g_Y^2 Y_d^{br} \right\} C_{qe}^{abcd} \\
& + \left\{ \frac{26}{27}\delta^{pa}\delta^{cd}g_Y^2 Y_d^{br} - \frac{1}{12}Y_u^{*ad}Y_d^{br}Y_u^{pc} - \frac{1}{3}\delta^{pa}Y_u^{bc}(Y_u^\dagger Y_d)^{dr} \right\} C_{qu}^{(\parallel)abcd} + \left\{ \frac{26}{81}\delta^{pa}\delta^{cd}g_Y^2 Y_d^{br} + \frac{32}{27}\delta^{pa}\delta^{cd}g_s^2 Y_d^{br} - \frac{1}{4}Y_u^{*ad}Y_d^{br}Y_u^{pc} \right. \\
& - \delta^{pa}Y_u^{bc}(Y_u^\dagger Y_d)^{dr} \Big\} C_{qu}^{(\times)abcd} + \left\{ \frac{1}{6}Y_d^{*ad}Y_d^{pc}Y_d^{br} + g_L^2(6\delta^{rd}\delta^{ab}Y_d^{pc} - \delta^{pa}\delta^{rd}Y_d^{bc}) + g_Y^2\left(\frac{1}{3}\delta^{rd}\delta^{ab}Y_d^{pc} + \frac{5}{9}\delta^{pa}\delta^{rd}Y_d^{bc} - \frac{13}{27}\delta^{pa}\delta^{cd}Y_d^{br}\right) + \frac{3}{2}\delta^{pa}\delta^{rd}(Y_d Y_d^\dagger Y_d)^{bc} \right. \\
& + 3Y_d^{*ad}Y_d^{pr}Y_d^{bc} + 3\delta^{pa}Y_d^{br}(Y_d^\dagger Y_d)^{dc} + 3\delta^{rd}Y_d^{pc}(Y_d Y_d^\dagger)^{ba} + 3\delta^{pa}\delta^{rd}Y_d^{bc}\text{Tr}[Y_d^\dagger Y_d] + 6\delta^{rd}Y_d^{pc}(Y_u Y_u^\dagger)^{ba} - \frac{1}{3}\delta^{pa}Y_d^{bc}(Y_d^\dagger Y_d)^{dr} - \frac{3}{4}\delta^{pa}\delta^{rd}(Y_u Y_u^\dagger Y_d)^{bc} \\
& - 2\delta^{rd}Y_d^{bc}(Y_u Y_u^\dagger)^{pa} - \frac{40}{3}\delta^{pa}\delta^{rd}g_s^2 Y_d^{bc} \Big\} C_{qd}^{(\parallel)abcd} + \left\{ \frac{1}{2}Y_d^{*ad}Y_d^{pc}Y_d^{br} + g_L^2(2\delta^{rd}\delta^{ab}Y_d^{pc} - 3\delta^{pa}\delta^{rd}Y_d^{bc}) + g_Y^2\left(\frac{1}{9}\delta^{rd}\delta^{ab}Y_d^{pc} + \frac{5}{3}\delta^{pa}\delta^{rd}Y_d^{bc} - \frac{13}{81}\delta^{pa}\delta^{cd}Y_d^{br}\right) \right. \\
& + g_s^2\left(\frac{32}{27}\delta^{pa}\delta^{cd}Y_d^{br} - 40\delta^{pa}\delta^{rd}Y_d^{bc}\right) + \delta^{pa}Y_d^{br}(Y_d^\dagger Y_d)^{dc} + \delta^{rd}Y_d^{pc}(Y_d Y_d^\dagger)^{ba} + 2\delta^{rd}Y_d^{pc}(Y_u Y_u^\dagger)^{ba} + \frac{9}{2}\delta^{pa}\delta^{rd}(Y_d Y_d^\dagger Y_d)^{bc} + 9Y_d^{*ad}Y_d^{pr}Y_d^{bc} \\
& + 9\delta^{pa}\delta^{rd}Y_d^{bc}\text{Tr}[Y_d^\dagger Y_d] - \delta^{pa}Y_d^{bc}(Y_d^\dagger Y_d)^{dr} - \frac{9}{4}\delta^{pa}\delta^{rd}(Y_u Y_u^\dagger Y_d)^{bc} - 6\delta^{rd}Y_d^{bc}(Y_u Y_u^\dagger)^{pa} \Big\} C_{qd}^{(\times)abcd} - g_Y^2 \left\{ \frac{2}{9}\delta^{rb}\delta^{ad}Y_d^{pc} + \frac{2}{3}\delta^{rb}\delta^{cd}Y_d^{pa} \right\} C_{dd}^{abcd} \\
& + \left\{ \frac{1}{2}\delta^{rd}Y_d^{pc}(Y_e^\dagger Y_e)^{ba} - \frac{1}{3}\delta^{rd}\delta^{ab}g_Y^2 Y_d^{pc} \right\} C_{ed}^{abcd} + \left\{ \frac{1}{4}\delta^{rd}Y_u^{pa}(Y_u^\dagger Y_d)^{bc} + \frac{2}{3}\delta^{rd}\delta^{ab}g_Y^2 Y_d^{pc} \right\} C_{ud}^{(\parallel)abcd} + \left\{ \frac{2}{9}\delta^{rd}\delta^{ab}g_Y^2 Y_d^{pc} + \frac{3}{4}\delta^{rd}Y_u^{pa}(Y_u^\dagger Y_d)^{bc} \right\} C_{ud}^{(\times)abcd} \\
& - \left\{ \frac{1}{12}Y_e^{*ab}Y_d^{pc}Y_d^{dr} + \frac{3}{2}Y_e^{*ab}Y_d^{pr}Y_d^{dc} \right\} C_{\ell edq}^{abcd} + C_{\ell edq}^{*abcd} \left\{ \frac{3}{4}\delta^{rc}Y_e^{ab}(Y_u Y_u^\dagger)^{pd} - \frac{1}{24}\delta^{pd}\delta^{rc}g_Y^2 Y_e^{ab} - \frac{1}{12}\delta^{pd}Y_e^{ab}(Y_d^\dagger Y_d)^{cr} - \frac{5}{8}\delta^{pd}\delta^{rc}g_L^2 Y_e^{ab} \right. \\
& - \frac{3}{2}\delta^{pd}\delta^{rc}Y_e^{ab}\text{Tr}[Y_d^\dagger Y_d] \Big\} + \left\{ \frac{1}{8}\delta^{rd}Y_u^{*cb}(Y_u Y_u^\dagger)^{pa} + \frac{7}{12}\delta^{pc}Y_d^{*ad}(Y_u^\dagger Y_d)^{br} + g_Y^2\left(\frac{5}{12}\delta^{pc}\delta^{rd}Y_u^{*ab} - \frac{7}{16}\delta^{pa}\delta^{rd}Y_u^{*cb}\right) + \frac{9}{8}\delta^{pa}\delta^{rd}(Y_u^\dagger Y_u Y_u^\dagger)^{cb} \right. \\
& + \frac{3}{2}\delta^{pc}\delta^{rd}(Y_d^\dagger Y_d Y_u^\dagger)^{ab} + 2\delta^{pa}Y_d^{*cd}(Y_u^\dagger Y_d)^{br} + \frac{9}{4}\delta^{rd}Y_u^{*ab}(Y_u Y_u^\dagger)^{pc} - \frac{1}{24}\delta^{pa}Y_u^{*cb}(Y_d^\dagger Y_d)^{dr} - \frac{1}{4}\delta^{pc}Y_u^{*ab}(Y_d^\dagger Y_d)^{dr} - \frac{3}{8}\delta^{pa}\delta^{rd}(Y_d^\dagger Y_d Y_u^\dagger)^{cb} \\
& - g_L^2\left(\frac{9}{4}\delta^{pc}\delta^{rd}Y_u^{*ab} + \frac{41}{16}\delta^{pa}\delta^{rd}Y_u^{*cb}\right) - \left(\frac{3}{4}\delta^{pa}\delta^{rd}Y_u^{*cb} + \frac{9}{2}\delta^{pc}\delta^{rd}Y_u^{*ab}\right)\text{Tr}[Y_d^\dagger Y_d] - 6\delta^{pa}\delta^{rd}g_s^2 Y_u^{*cb} \Big\} C_{quqd}^{(\parallel)abcd} + \left(C_{quqd}^{(\parallel)*}\right)^{abcd} \left\{ \frac{1}{12}Y_d^{pd}Y_d^{ar}Y_u^{cb} \right. \\
& + \frac{7}{12}Y_d^{ad}Y_d^{cr}Y_u^{pb} + \frac{5}{4}Y_d^{ar}Y_d^{cd}Y_u^{pb} - \frac{1}{4}Y_d^{pd}Y_d^{cr}Y_u^{ab} - \frac{3}{4}Y_d^{pr}Y_d^{ad}Y_u^{cb} - \frac{9}{2}Y_d^{pr}Y_d^{cd}Y_u^{ab} \Big\} + \left\{ \frac{3}{8}\delta^{rd}Y_u^{*cb}(Y_u Y_u^\dagger)^{pa} + \frac{1}{2}\delta^{pc}\delta^{rd}(Y_d^\dagger Y_d Y_u^\dagger)^{ab} + \frac{2}{3}\delta^{pa}Y_d^{*cd}(Y_u^\dagger Y_d)^{br} \right. \\
& + \frac{3}{4}\delta^{rd}Y_u^{*ab}(Y_u Y_u^\dagger)^{pc} + g_Y^2\left(\frac{5}{36}\delta^{pc}\delta^{rd}Y_u^{*ab} - \frac{21}{16}\delta^{pa}\delta^{rd}Y_u^{*cb}\right) + \frac{7}{4}\delta^{pc}Y_d^{*ad}(Y_u^\dagger Y_d)^{br} + \frac{27}{8}\delta^{pa}\delta^{rd}(Y_u^\dagger Y_u Y_u^\dagger)^{cb} - \frac{1}{12}\delta^{pc}Y_u^{*ab}(Y_d^\dagger Y_d)^{dr}
\end{aligned}$$

$$\begin{aligned}
& -\frac{1}{8}\delta^{pa}Y_u^{*cb}(Y_d^\dagger Y_d)^{dr} - g_L^2\left(\frac{3}{4}\delta^{pc}\delta^{rd}Y_u^{*ab} + \frac{123}{16}\delta^{pa}\delta^{rd}Y_u^{*cb}\right) - g_s^2\left(\frac{16}{3}\delta^{pc}\delta^{rd}Y_u^{*ab} + 12\delta^{pa}\delta^{rd}Y_u^{*cb}\right) - \left(\frac{3}{2}\delta^{pc}\delta^{rd}Y_u^{*ab} + \frac{9}{4}\delta^{pa}\delta^{rd}Y_u^{*cb}\right)\text{Tr}[Y_d^\dagger Y_d] \\
& -\frac{9}{8}\delta^{pa}\delta^{rd}(Y_d^\dagger Y_d Y_u^\dagger)^{cb}\left\{C_{quqd}^{(\times)abcd} + \left(C_{quqd}^{(\times)*}\right)^{abcd}\left\{\frac{1}{4}Y_d^{pd}Y_d^{ar}Y_u^{cb} + \frac{5}{12}Y_d^{ar}Y_d^{cd}Y_u^{pb} + \frac{7}{4}Y_d^{ad}Y_d^{cr}Y_u^{pb} - \frac{1}{12}Y_d^{pd}Y_d^{cr}Y_u^{ab} - \frac{3}{2}Y_d^{pr}Y_d^{cd}Y_u^{ab} - \frac{9}{4}Y_d^{pr}Y_d^{ad}Y_u^{cb}\right\}\right. \\
& -\frac{2}{3}\delta^{pc}Y_e^{*ab}C_{\ell equ}^{abcd}(Y_u^\dagger Y_d)^{dr} + \frac{1}{12}C_{\ell equ}^{*abcd}Y_d^{cr}Y_e^{ab}Y_u^{pd} + \frac{7}{12}\delta^{pc}Y_e^{*ad}C_{\ell uqe}^{abcd}(Y_u^\dagger Y_d)^{br} + \frac{1}{3}C_{\ell uqe}^{*abcd}Y_d^{cr}Y_e^{ad}Y_u^{pb} + \left\{g_Y^2\left(\frac{40}{81}\delta^{pa}\delta^{bc}Y_d^{dr} + \frac{26}{27}\delta^{pa}\delta^{cd}Y_d^{br}\right)\right. \\
& +\frac{5}{2}\delta^{pa}Y_d^{dr}(Y_u Y_u^\dagger)^{bc} + 12\delta^{pa}Y_d^{br}(Y_u Y_u^\dagger)^{dc} - g_L^2\left(\frac{8}{3}\delta^{pa}\delta^{bc}Y_d^{dr} + 6\delta^{pa}\delta^{cd}Y_d^{br}\right) - 2\delta^{pa}Y_d^{dr}(Y_d Y_d^\dagger)^{bc} - \frac{368}{27}\delta^{pa}\delta^{bc}g_s^2Y_d^{dr}\left\{C_{qq}^{(\parallel)abcd} + \left\{g_Y^2\left(\frac{26}{81}\delta^{pa}\delta^{bc}Y_d^{dr}\right.\right.\right. \\
& +\frac{40}{27}\delta^{pa}\delta^{cd}Y_d^{br}\left.\left.\left.\right\} + \frac{7}{2}\delta^{pa}Y_d^{dr}(Y_u Y_u^\dagger)^{bc} + \frac{128}{27}\delta^{pa}\delta^{bc}g_s^2Y_d^{dr} + 6\delta^{pa}Y_d^{br}(Y_u Y_u^\dagger)^{dc} - g_L^2\left(2\delta^{pa}\delta^{bc}Y_d^{dr} + 8\delta^{pa}\delta^{cd}Y_d^{br}\right) - 6\delta^{pa}Y_d^{br}(Y_d Y_d^\dagger)^{dc}\right\}C_{qq}^{(\times)abcd} \\
& +\left\{\frac{1}{2}\delta^{pc}Y_d^{dr}(Y_e Y_e^\dagger)^{ba} - \frac{13}{27}\delta^{pc}\delta^{ab}g_Y^2Y_d^{dr} - \delta^{pc}\delta^{ab}g_L^2Y_d^{dr}\right\}C_{\ell q}^{(\parallel)abcd} - \left\{\frac{20}{27}\delta^{pc}\delta^{ab}g_Y^2Y_d^{dr} + \frac{4}{3}\delta^{pc}\delta^{ab}g_L^2Y_d^{dr}\right\}C_{\ell q}^{(\times)abcd}, \tag{8.14}
\end{aligned}$$

## 8.8 $C_{dG}$

$$\begin{aligned}
\beta_{C_{dG}^{pr}}^{(1)} &= 4g_s^2 C_{HG} Y_d^{pr} - 4ig_s^2 C_{H\tilde{G}} Y_d^{pr} + 9g_s^4 C_G Y_d^{pr} - 9ig_s^4 C_{\tilde{G}} Y_d^{pr} - \delta^{pa} C_{uG}^{ab} (Y_u^\dagger Y_d)^{br} - \frac{2}{3}\delta^{pa}\delta^{rb}g_Y^2 C_{dB}^{ab} + 3\delta^{pa}\delta^{rb}g_L^2 C_{dW}^{ab} + \left\{\frac{1}{2}\left(2T_2\delta^{pa}\delta^{rb}\right.\right. \\
& +4\delta^{pa}(Y_d^\dagger Y_d)^{br} + 5\delta^{rb}(Y_d Y_d^\dagger)^{pa} - 3\delta^{rb}(Y_u Y_u^\dagger)^{pa}\left.\left.\right\} + \frac{4}{3}\delta^{pa}\delta^{rb}g_s^2 - \frac{31}{36}\delta^{pa}\delta^{rb}g_Y^2 - \frac{9}{4}\delta^{pa}\delta^{rb}g_L^2\left\}C_{dG}^{ab} + \delta^{pa}\delta^{rd}Y_u^{*cb}C_{quqd}^{(\parallel)abcd}, \tag{8.15}
\end{aligned}$$

$$\begin{aligned}
\beta_{C_{dG}^{pr}}^{(2)} &= -\frac{1}{2}C_{HD}^{(\parallel)}(Y_u Y_u^\dagger Y_d)^{pr} + \frac{1}{2}C_{HD}^{(\times)}(Y_u Y_u^\dagger Y_d)^{pr} + \frac{1}{6}g_Y^4 C_{HB} Y_d^{pr} - \frac{i}{6}g_Y^4 C_{H\tilde{B}} Y_d^{pr} - \frac{3}{2}g_L^4 C_{HW} Y_d^{pr} + \frac{3i}{2}g_L^4 C_{H\tilde{W}} Y_d^{pr} + \left\{g_s^2\left(5(Y_u Y_u^\dagger Y_d)^{pr} - 2T_2 Y_d^{pr}\right.\right. \\
& -15(Y_d Y_d^\dagger Y_d)^{pr}\left.\left.\right\} + \frac{3}{2}g_s^2 g_L^2 Y_d^{pr} + \frac{11}{6}g_Y^2 g_s^2 Y_d^{pr} + \frac{80}{3}g_s^4 Y_d^{pr} - 6\lambda g_s^2 Y_d^{pr}\left\}C_{HG} + \left\{g_s^2\left(2iT_2 Y_d^{pr} + 15i(Y_d Y_d^\dagger Y_d)^{pr} - i(Y_u Y_u^\dagger Y_d)^{pr}\right)\right.\right. \\
& +6i\lambda g_s^2 Y_d^{pr} - \frac{3i}{2}g_s^2 g_L^2 Y_d^{pr} - \frac{11i}{6}g_Y^2 g_s^2 Y_d^{pr} - \frac{224i}{3}g_s^4 Y_d^{pr}\left\}C_{H\tilde{G}} + \frac{3}{4}g_Y^2 g_L^2 C_{HWB} Y_d^{pr} - \frac{3i}{4}g_Y^2 g_L^2 C_{H\tilde{W}B} Y_d^{pr} - \frac{9}{2}g_L^6 C_W Y_d^{pr} + \frac{5i}{2}g_L^6 C_{\tilde{W}} Y_d^{pr} \\
& +\left\{g_s^4\left(\frac{45}{2}(Y_u Y_u^\dagger Y_d)^{pr} - 27(Y_d Y_d^\dagger Y_d)^{pr}\right) + 144g_s^6 Y_d^{pr} - \frac{25}{8}g_Y^2 g_s^4 Y_d^{pr} - \frac{135}{8}g_s^4 g_L^2 Y_d^{pr}\right\}C_G + \left\{g_s^4\left(30i(Y_d Y_d^\dagger Y_d)^{pr} - \frac{29i}{2}(Y_u Y_u^\dagger Y_d)^{pr}\right)\right. \\
& +\frac{193i}{72}g_Y^2 g_s^4 Y_d^{pr} + \frac{135i}{8}g_s^4 g_L^2 Y_d^{pr} - \frac{482i}{3}g_s^6 Y_d^{pr}\left\}C_{\tilde{G}} + \left\{\frac{3}{2}\delta^{pa}(Y_d^\dagger Y_d)^{br} + \frac{3}{2}\delta^{rb}(Y_d Y_d^\dagger)^{pa}\right\}C_{dH}^{ab} + \frac{5}{3}g_Y^2 C_{uB}^{*ab} Y_d^{ar} Y_u^{pb} - \frac{3}{2}\delta^{pa}g_L^2 C_{uW}^{ab} (Y_u^\dagger Y_d)^{br}
\end{aligned}$$

$$\begin{aligned}
& + \frac{3}{2} g_L^2 \mathbf{C}_{uW}^{*ab} Y_d^{ar} Y_u^{pb} + \left\{ \frac{1}{2} T_2 \delta^{pa} (Y_u^\dagger Y_d)^{br} + \frac{5}{2} (Y_u^\dagger Y_d)^{br} (Y_u Y_u^\dagger)^{pa} + \frac{5}{2} \delta^{pa} (Y_u^\dagger Y_u Y_u^\dagger Y_d)^{br} - \frac{1}{2} (Y_u^\dagger Y_d)^{br} (Y_d Y_d^\dagger)^{pa} - \frac{5}{8} \delta^{pa} g_Y^2 (Y_u^\dagger Y_d)^{br} - g_s^2 \left( 2 Y_u^{*ab} Y_d^{pr} \right. \right. \\
& + 16 \delta^{pa} (Y_u^\dagger Y_d)^{br} \left. \right) - \delta^{pa} (Y_u^\dagger Y_d Y_d^\dagger Y_d)^{br} - \frac{39}{8} \delta^{pa} g_L^2 (Y_u^\dagger Y_d)^{br} \left. \right\} \mathbf{C}_{uG}^{ab} + \mathbf{C}_{uG}^{*ab} \left\{ \frac{1}{2} Y_u^{pb} (Y_u Y_u^\dagger Y_d)^{ar} + T_2 Y_d^{ar} Y_u^{pb} + \frac{5}{2} Y_d^{ar} (Y_u Y_u^\dagger Y_u)^{pb} - \frac{3}{4} g_Y^2 Y_d^{ar} Y_u^{pb} \right. \\
& - g_s^2 \left( 2 Y_d^{pr} Y_u^{ab} + \frac{17}{3} Y_d^{ar} Y_u^{pb} \right) - Y_u^{pb} (Y_d Y_d^\dagger Y_d)^{ar} - 2 Y_d^{ar} (Y_d Y_d^\dagger Y_u)^{pb} - \frac{9}{4} g_L^2 Y_d^{ar} Y_u^{pb} \left. \right\} + \left\{ g_Y^2 \left( \frac{7}{3} \delta^{rb} (Y_u Y_u^\dagger)^{pa} + \frac{19}{6} \delta^{pa} (Y_d^\dagger Y_d)^{br} - \frac{7}{6} \delta^{rb} (Y_d Y_d^\dagger)^{pa} \right) \right. \\
& + \frac{205}{36} \delta^{pa} \delta^{rb} g_Y^4 - \frac{13}{9} \delta^{pa} \delta^{rb} g_Y^2 g_s^2 - \frac{11}{4} \delta^{pa} \delta^{rb} g_Y^2 g_L^2 \left. \right\} \mathbf{C}_{dB}^{ab} + \left\{ \frac{19}{24} \delta^{pa} \delta^{rb} g_Y^2 g_L^2 + \frac{13}{2} \delta^{pa} \delta^{rb} g_s^2 g_L^2 + \frac{167}{24} \delta^{pa} \delta^{rb} g_L^4 - g_L^2 \left( \frac{3}{4} \delta^{pa} (Y_d^\dagger Y_d)^{br} \right. \right. \\
& + \frac{3}{4} \delta^{rb} (Y_d Y_d^\dagger)^{pa} + \frac{15}{2} \delta^{rb} (Y_u Y_u^\dagger)^{pa} \left. \right) \left. \right\} \mathbf{C}_{dW}^{ab} + \left\{ \frac{5}{12} \delta^{pa} \delta^{rb} g_Y^2 g_L^2 + g_L^2 \left( \frac{9}{16} \delta^{rb} (Y_u Y_u^\dagger)^{pa} + \frac{15}{8} T_2 \delta^{pa} \delta^{rb} + 9 \delta^{pa} (Y_d^\dagger Y_d)^{br} + \frac{237}{16} \delta^{rb} (Y_d Y_d^\dagger)^{pa} \right) \right. \\
& + g_Y^2 \left( \frac{25}{24} \delta^{pa} \delta^{rb} \text{Tr} [Y_d^\dagger Y_d] + \frac{25}{8} \delta^{pa} \delta^{rb} \text{Tr} [Y_e^\dagger Y_e] + \frac{85}{24} \delta^{pa} \delta^{rb} \text{Tr} [Y_u^\dagger Y_u] + \frac{635}{144} \delta^{rb} (Y_d Y_d^\dagger)^{pa} + \frac{40}{9} \delta^{pa} (Y_d^\dagger Y_d)^{br} - \frac{301}{144} \delta^{rb} (Y_u Y_u^\dagger)^{pa} \right) \\
& + g_s^2 \left( \frac{7}{3} \delta^{rb} (Y_d Y_d^\dagger)^{pa} + \frac{8}{3} \delta^{pa} (Y_d^\dagger Y_d)^{br} + 10 Y_d^{*ab} Y_d^{pr} + 16 \delta^{pa} \delta^{rb} \text{Tr} [Y_u^\dagger Y_u] + 22 \delta^{pa} \delta^{rb} \text{Tr} [Y_d^\dagger Y_d] - \frac{47}{3} \delta^{rb} (Y_u Y_u^\dagger)^{pa} \right) + \frac{5}{4} T_2 \delta^{rb} (Y_u Y_u^\dagger)^{pa} \\
& + \frac{5}{4} \delta^{pa} (Y_d^\dagger Y_d Y_d^\dagger Y_d)^{br} + \frac{5}{4} \delta^{rb} (Y_d Y_d^\dagger Y_d Y_d^\dagger)^{pa} + \frac{3}{2} \delta^{pa} \delta^{rb} \lambda^2 + \frac{3}{2} \delta^{pa} \delta^{rb} \text{Tr} [Y_d^\dagger Y_d Y_u^\dagger Y_u] + \frac{109}{54} \delta^{pa} \delta^{rb} g_Y^2 g_s^2 + \frac{5}{2} \delta^{pa} \delta^{rb} g_s^2 g_L^2 \\
& + \frac{11}{4} \delta^{rb} (Y_u Y_u^\dagger Y_u Y_u^\dagger)^{pa} + \frac{2219}{648} \delta^{pa} \delta^{rb} g_Y^4 + \frac{362}{9} \delta^{pa} \delta^{rb} g_s^4 - \frac{1}{4} \delta^{pa} (Y_d^\dagger Y_u Y_u^\dagger Y_d)^{br} - \frac{1}{2} \delta^{rb} (Y_d Y_d^\dagger Y_u Y_u^\dagger)^{pa} - \lambda \left( 6 \delta^{pa} (Y_d^\dagger Y_d)^{br} + 6 \delta^{rb} (Y_d Y_d^\dagger)^{pa} \right) \\
& - \delta^{rb} (Y_u Y_u^\dagger Y_d Y_d^\dagger)^{pa} - \frac{9}{4} T_4 \delta^{pa} \delta^{rb} - 3 T_2 \delta^{pa} (Y_d^\dagger Y_d)^{br} - 3 (Y_d^\dagger Y_d)^{br} (Y_d Y_d^\dagger)^{pa} - \frac{15}{4} T_2 \delta^{rb} (Y_d Y_d^\dagger)^{pa} - \frac{23}{4} \delta^{pa} \delta^{rb} g_L^4 \left. \right\} \mathbf{C}_{dG}^{ab} \\
& + \mathbf{C}_{dG}^{*ab} \left\{ \frac{1}{2} Y_d^{pb} (Y_u Y_u^\dagger Y_d)^{ar} - \frac{1}{2} Y_d^{ar} (Y_u Y_u^\dagger Y_d)^{pb} \right\} + \left\{ \frac{31}{54} \delta^{pa} g_Y^2 Y_d^{br} + \frac{7}{6} Y_d^{br} (Y_d Y_d^\dagger)^{pa} + \frac{3}{2} \delta^{pa} g_L^2 Y_d^{br} + \frac{19}{6} \delta^{pa} (Y_d Y_d^\dagger Y_d)^{br} + 4 \delta^{ab} g_s^2 Y_d^{pr} \right. \\
& - \frac{2}{3} Y_d^{br} (Y_u Y_u^\dagger)^{pa} - \frac{2}{3} \delta^{pa} (Y_u Y_u^\dagger Y_d)^{br} \left. \right\} \mathbf{C}_{Hq}^{(ll)ab} + \left\{ \frac{1}{3} \delta^{pa} g_L^2 Y_d^{br} + \frac{2}{3} Y_d^{br} (Y_u Y_u^\dagger)^{pa} + \frac{2}{3} \delta^{pa} (Y_u Y_u^\dagger Y_d)^{br} + \frac{5}{6} Y_d^{br} (Y_d Y_d^\dagger)^{pa} + \frac{28}{27} \delta^{pa} g_Y^2 Y_d^{br} \right. \\
& + \frac{11}{6} \delta^{pa} (Y_d Y_d^\dagger Y_d)^{br} + 2 \delta^{ab} g_s^2 Y_d^{pr} \left. \right\} \mathbf{C}_{Hq}^{(\times)ab} - 2 \delta^{ab} g_s^2 \mathbf{C}_{Hu}^{ab} Y_d^{pr} + \left\{ \delta^{rb} (Y_u Y_u^\dagger Y_d)^{pa} - \frac{35}{54} \delta^{rb} g_Y^2 Y_d^{pa} - \frac{5}{6} Y_d^{pa} (Y_d^\dagger Y_d)^{br} - \frac{3}{2} \delta^{rb} g_L^2 Y_d^{pa} \right. \\
& - \frac{11}{6} \delta^{rb} (Y_d Y_d^\dagger Y_d)^{pa} - 2 \delta^{ab} g_s^2 Y_d^{pr} \left. \right\} \mathbf{C}_{Hd}^{ab} + \left\{ \frac{1}{2} \delta^{rb} g_Y^2 Y_u^{pa} + \frac{7}{6} \delta^{rb} (Y_d Y_d^\dagger Y_u)^{pa} - \frac{1}{2} Y_u^{pa} (Y_d^\dagger Y_d)^{br} - \frac{3}{2} \delta^{rb} g_L^2 Y_u^{pa} - 2 \delta^{rb} (Y_u Y_u^\dagger Y_u)^{pa} \right\} \mathbf{C}_{Hud}^{ab} \\
& - \frac{1}{3} \mathbf{C}_{Hud}^{*ab} Y_d^{pb} (Y_u^\dagger Y_d)^{ar} + \frac{8}{27} \delta^{rd} \delta^{ab} g_Y^2 \mathbf{C}_{\ell d}^{abcd} Y_d^{pc} - \frac{4}{27} \delta^{pa} \delta^{cd} g_Y^2 \mathbf{C}_{qe}^{abcd} Y_d^{br} + \left\{ \frac{1}{6} Y_u^{*ad} Y_d^{br} Y_u^{pc} + \frac{8}{27} \delta^{pa} \delta^{cd} g_Y^2 Y_d^{br} + \frac{2}{3} \delta^{pa} Y_u^{bc} (Y_u^\dagger Y_d)^{dr} \right.
\end{aligned}$$

$$\begin{aligned}
& + 3\delta^{pa}\delta^{cd}g_s^2Y_d^{br}\left\{C_{qu}^{(\parallel)abcd} + \left\{\frac{113}{27}\delta^{pa}\delta^{cd}g_s^2Y_d^{br} - \frac{46}{81}\delta^{pa}\delta^{cd}g_Y^2Y_d^{br} - Y_u^{*ad}Y_d^{br}Y_u^{pc} - \delta^{pa}Y_u^{bc}(Y_u^\dagger Y_d)^{dr} - 2\delta^{pa}Y_d^{br}(Y_u^\dagger Y_u)^{dc}\right\}C_{qu}^{(\times)abcd}\right. \\
& + \left\{g_Y^2\left(\frac{10}{9}\delta^{pa}\delta^{rd}Y_d^{bc} - \frac{4}{27}\delta^{pa}\delta^{cd}Y_d^{br} - \frac{8}{27}\delta^{rd}\delta^{ab}Y_d^{pc}\right) + g_s^2\left(3\delta^{pa}\delta^{cd}Y_d^{br} + 6\delta^{rd}\delta^{ab}Y_d^{pc} - \frac{8}{3}\delta^{pa}\delta^{rd}Y_d^{bc}\right) + 2\delta^{rd}Y_d^{bc}(Y_uY_u^\dagger)^{pa} + 3\delta^{pa}\delta^{rd}(Y_dY_d^\dagger Y_d)^{bc}\right. \\
& - \frac{1}{2}\delta^{pa}\delta^{rd}(Y_uY_u^\dagger Y_d)^{bc} - Y_d^{*ad}Y_d^{pc}Y_d^{br} - \frac{4}{3}\delta^{pa}Y_d^{bc}(Y_d^\dagger Y_d)^{dr} - \frac{8}{3}\delta^{rd}Y_d^{bc}(Y_dY_d^\dagger)^{pa}\left\}C_{qd}^{(\parallel)abcd} + \left\{g_Y^2\left(\frac{23}{81}\delta^{pa}\delta^{cd}Y_d^{br} - \frac{8}{81}\delta^{rd}\delta^{ab}Y_d^{pc} - \frac{1}{6}\delta^{pa}\delta^{rd}Y_d^{bc}\right)\right. \\
& + g_s^2\left(4\delta^{pa}\delta^{rd}Y_d^{bc} + \frac{113}{27}\delta^{pa}\delta^{cd}Y_d^{br} + \frac{226}{27}\delta^{rd}\delta^{ab}Y_d^{pc}\right) + 2\delta^{pa}Y_d^{br}(Y_d^\dagger Y_d)^{dc} + 2\delta^{rd}Y_d^{pc}(Y_dY_d^\dagger)^{ba} - \delta^{pa}Y_d^{bc}(Y_d^\dagger Y_d)^{dr} - 2\delta^{rd}Y_d^{bc}(Y_dY_d^\dagger)^{pa} \\
& - 2\delta^{rd}Y_d^{pc}(Y_uY_u^\dagger)^{ba} - 3Y_d^{*ad}Y_d^{pc}Y_d^{br} - \frac{9}{2}\delta^{pa}\delta^{rd}g_L^2Y_d^{bc}\left\}C_{qd}^{(\times)abcd} + \left\{g_Y^2\left(\frac{16}{81}\delta^{rb}\delta^{ad}Y_d^{pc} + \frac{16}{27}\delta^{rb}\delta^{cd}Y_d^{pa}\right) - g_s^2\left(\frac{152}{27}\delta^{rb}\delta^{ad}Y_d^{pc} + 6\delta^{rb}\delta^{cd}Y_d^{pa}\right)\right\}C_{dd}^{abcd} \\
& + \frac{8}{27}\delta^{rd}\delta^{ab}g_Y^2C_{ed}^{abcd}Y_d^{pc} + \left\{\frac{3}{2}\delta^{rd}Y_u^{pa}(Y_u^\dagger Y_d)^{bc} - \frac{16}{27}\delta^{rd}\delta^{ab}g_Y^2Y_d^{pc} - 3\delta^{rd}\delta^{ab}g_s^2Y_d^{pc}\right\}C_{ud}^{(\parallel)abcd} - \left\{\frac{16}{81}\delta^{rd}\delta^{ab}g_Y^2Y_d^{pc} + 2\delta^{rd}Y_d^{pc}(Y_u^\dagger Y_u)^{ba}\right. \\
& + \frac{76}{27}\delta^{rd}\delta^{ab}g_s^2Y_d^{pc}\left\}C_{ud}^{(\times)abcd} + \frac{1}{2}Y_e^{*ab}C_{ledq}^{abcd}Y_d^{pc}Y_d^{dr} + C_{ledq}^{*abcd}\left\{\frac{1}{6}\delta^{pd}Y_e^{ab}(Y_d^\dagger Y_d)^{cr} + \frac{1}{3}\delta^{rc}Y_e^{ab}(Y_dY_d^\dagger)^{pd} - \frac{1}{2}\delta^{rc}Y_e^{ab}(Y_uY_u^\dagger)^{pd}\right\} + \left\{\frac{1}{12}\delta^{pa}Y_u^{*cb}(Y_d^\dagger Y_d)^{dr}\right. \\
& + \frac{1}{6}\delta^{rd}Y_u^{*cb}(Y_dY_d^\dagger)^{pa} + \frac{1}{2}\delta^{pc}Y_u^{*ab}(Y_d^\dagger Y_d)^{dr} + \frac{7}{8}\delta^{pa}\delta^{rd}g_Y^2Y_u^{*cb} + g_s^2\left(4\delta^{pc}\delta^{rd}Y_u^{*ab} + \frac{19}{2}\delta^{pa}\delta^{rd}Y_u^{*cb}\right) + \delta^{rd}Y_u^{*ab}(Y_dY_d^\dagger)^{pc} + \frac{9}{8}\delta^{pa}\delta^{rd}g_L^2Y_u^{*cb} \\
& + \frac{5}{4}\delta^{pa}\delta^{rd}(Y_d^\dagger Y_dY_u^\dagger)^{cb} - \frac{2}{3}\delta^{pc}Y_d^{*ad}(Y_u^\dagger Y_d)^{br} - \frac{3}{4}\delta^{rd}Y_u^{*cb}(Y_uY_u^\dagger)^{pa} - \delta^{pa}Y_d^{*cd}(Y_u^\dagger Y_d)^{br} - \frac{3}{2}\delta^{rd}Y_u^{*ab}(Y_uY_u^\dagger)^{pc} - \frac{15}{4}\delta^{pa}\delta^{rd}(Y_u^\dagger Y_uY_u^\dagger)^{cb}\left\}C_{quqd}^{(\parallel)abcd} \\
& + \left(C_{quqd}^{(\parallel)*}\right)^{abcd}\left\{\frac{1}{2}Y_d^{ar}Y_d^{cd}Y_u^{pb} + \frac{5}{6}Y_d^{ad}Y_d^{cr}Y_u^{pb} + \frac{3}{2}Y_d^{pd}Y_d^{cr}Y_u^{ab} - \frac{1}{2}Y_d^{pd}Y_d^{ar}Y_u^{cb}\right\} + \left\{\frac{1}{6}\delta^{pc}Y_u^{*ab}(Y_d^\dagger Y_d)^{dr} + \frac{1}{4}\delta^{pa}Y_u^{*cb}(Y_d^\dagger Y_d)^{dr} + \frac{1}{3}\delta^{rd}Y_u^{*ab}(Y_dY_d^\dagger)^{pc}\right. \\
& + \frac{1}{2}\delta^{rd}Y_u^{*cb}(Y_dY_d^\dagger)^{pa} + g_L^2\left(\frac{27}{8}\delta^{pa}\delta^{rd}Y_u^{*cb} - \frac{3}{2}\delta^{pc}\delta^{rd}Y_u^{*ab}\right) + g_Y^2\left(\frac{5}{8}\delta^{pa}\delta^{rd}Y_u^{*cb} - \frac{5}{18}\delta^{pc}\delta^{rd}Y_u^{*ab}\right) + g_s^2\left(\frac{14}{3}\delta^{pc}\delta^{rd}Y_u^{*ab} - \frac{3}{2}\delta^{pa}\delta^{rd}Y_u^{*cb}\right) \\
& + \delta^{pc}\delta^{rd}(Y_d^\dagger Y_dY_u^\dagger)^{ab} - \frac{1}{3}\delta^{pa}Y_d^{*cd}(Y_u^\dagger Y_d)^{br} - \frac{1}{2}\delta^{pc}Y_d^{*ad}(Y_u^\dagger Y_d)^{br} - \frac{1}{2}\delta^{rd}Y_u^{*ab}(Y_uY_u^\dagger)^{pc} - \frac{3}{4}\delta^{rd}Y_u^{*cb}(Y_uY_u^\dagger)^{pa}\left\}C_{quqd}^{(\times)abcd} + \left(C_{quqd}^{(\times)*}\right)^{abcd}\left\{\frac{1}{4}Y_d^{ad}Y_d^{cr}Y_u^{pb}\right. \\
& + \frac{1}{2}Y_d^{pd}Y_d^{cr}Y_u^{ab} + \frac{3}{4}Y_d^{pd}Y_d^{ar}Y_u^{cb} + \frac{7}{6}Y_d^{ar}Y_d^{cd}Y_u^{pb}\left\} + \frac{1}{3}\delta^{pc}Y_e^{*ab}C_{lequ}^{abcd}(Y_u^\dagger Y_d)^{dr} - \frac{1}{6}C_{lequ}^{*abcd}Y_d^{cr}Y_e^{ab}Y_u^{pd} - \frac{1}{6}\delta^{pc}Y_e^{*ad}C_{luqe}^{abcd}(Y_u^\dagger Y_d)^{br} \\
& + \frac{1}{12}C_{luqe}^{*abcd}Y_d^{cr}Y_e^{ad}Y_u^{pb} + \left\{g_Y^2\left(\frac{8}{27}\delta^{pa}\delta^{cd}Y_d^{br} + \frac{31}{81}\delta^{pa}\delta^{bc}Y_d^{dr}\right) + 3\delta^{pa}Y_d^{dr}(Y_uY_u^\dagger)^{bc} - g_s^2\left(\frac{152}{27}\delta^{pa}\delta^{bc}Y_d^{dr} + 12\delta^{pa}\delta^{cd}Y_d^{br}\right) - \frac{5}{3}\delta^{pa}\delta^{bc}g_L^2Y_d^{dr}\right\}C_{qq}^{(\parallel)abcd} \\
& + \left\{g_Y^2\left(\frac{4}{27}\delta^{pa}\delta^{cd}Y_d^{br} + \frac{62}{81}\delta^{pa}\delta^{bc}Y_d^{dr}\right) + 4\delta^{pa}\delta^{cd}g_L^2Y_d^{br} - g_s^2\left(6\delta^{pa}\delta^{cd}Y_d^{br} + \frac{304}{27}\delta^{pa}\delta^{bc}Y_d^{dr}\right) - 3\delta^{pa}Y_d^{dr}(Y_uY_u^\dagger)^{bc}\right\}C_{qq}^{(\times)abcd} - \frac{4}{27}\delta^{pc}\delta^{ab}g_Y^2C_{\ell q}^{(\parallel)abcd}Y_d^{dr}
\end{aligned}$$

$$+ \left\{ \frac{2}{3} \delta^{pc} \delta^{ab} g_L^2 Y_d^{dr} - \frac{2}{27} \delta^{pc} \delta^{ab} g_Y^2 Y_d^{dr} \right\} C_{\ell q}^{(\times) abcd}, \quad (8.16)$$

## 9 $\psi^2 HD$

### 9.1 $C_{H\ell}^{(\parallel)}$

$$\begin{aligned} \beta_{C_{H\ell}^{(\parallel) pr}}^{(1)} = & -10(C_{\ell HH} C_{\ell HH}^\dagger)^{rp} - \left\{ \frac{1}{12} \delta^{pr} g_L^2 + \frac{1}{12} \delta^{pr} g_Y^2 \right\} C_{HD}^{(\parallel)} - \left\{ \frac{1}{6} \delta^{pr} g_Y^2 + \frac{1}{2} (Y_e Y_e^\dagger)^{pr} \right\} C_{HD}^{(\times)} + \left\{ \frac{1}{3} g_Y^2 (\delta^{pa} \delta^{rb} + 2\delta^{pr} \delta^{ab}) + \frac{1}{2} (\delta^{rb} (Y_e Y_e^\dagger)^{pa} \right. \\ & + \delta^{pa} (Y_e Y_e^\dagger)^{br} + 4T_2 \delta^{pa} \delta^{rb}) \left. \right\} C_{H\ell}^{(\parallel) ab} + \left\{ \frac{1}{6} g_L^2 (17\delta^{pa} \delta^{rb} - 2\delta^{pr} \delta^{ab}) + \frac{1}{6} g_Y^2 (\delta^{pa} \delta^{rb} + 2\delta^{pr} \delta^{ab}) + 2(\delta^{rb} (Y_e Y_e^\dagger)^{pa} + \delta^{pa} (Y_e Y_e^\dagger)^{br}) \right\} C_{H\ell}^{(\times) ab} \\ & + \left\{ \frac{2}{3} \delta^{pr} \delta^{ab} g_Y^2 - Y_e^{*rb} Y_e^{pa} \right\} C_{He}^{ab} - \frac{2}{3} \delta^{pr} \delta^{ab} g_Y^2 C_{Hq}^{(\parallel) ab} - \left\{ \frac{1}{3} \delta^{pr} \delta^{ab} g_Y^2 + \delta^{pr} \delta^{ab} g_L^2 \right\} C_{Hq}^{(\times) ab} - \frac{4}{3} \delta^{pr} \delta^{ab} g_Y^2 C_{Hu}^{ab} + \frac{2}{3} \delta^{pr} \delta^{ab} g_Y^2 C_{Hd}^{ab} \\ & + \left\{ 2\delta^{pa} \delta^{rb} (Y_e^\dagger Y_e)^{dc} - \frac{2}{3} \delta^{pa} \delta^{rb} \delta^{cd} g_Y^2 \right\} C_{\ell e}^{abcd} + \left\{ \frac{4}{3} \delta^{pa} \delta^{rb} \delta^{cd} g_Y^2 - 6\delta^{pa} \delta^{rb} (Y_u^\dagger Y_u)^{dc} \right\} C_{\ell u}^{abcd} + \left\{ 6\delta^{pa} \delta^{rb} (Y_d^\dagger Y_d)^{dc} - \frac{2}{3} \delta^{pa} \delta^{rb} \delta^{cd} g_Y^2 \right\} C_{\ell d}^{abcd} \\ & - \left\{ \frac{2}{3} \delta^{pa} \delta^{rd} \delta^{bc} g_L^2 + \frac{2}{3} g_Y^2 (\delta^{pa} \delta^{rd} \delta^{bc} + 2\delta^{pa} \delta^{rb} \delta^{cd}) + 4\delta^{pa} \delta^{rb} (Y_e Y_e^\dagger)^{dc} \right\} C_{\ell \ell}^{abcd} + \left\{ \frac{2}{3} \delta^{pa} \delta^{rb} \delta^{cd} g_Y^2 - 6(\delta^{pa} \delta^{rb} (Y_d Y_d^\dagger)^{dc} - \delta^{pa} \delta^{rb} (Y_u Y_u^\dagger)^{dc}) \right\} C_{\ell q}^{(\parallel) abcd} \\ & + \left\{ \frac{1}{3} \delta^{pa} \delta^{rb} \delta^{cd} g_Y^2 + 6\delta^{pa} \delta^{rb} (Y_u Y_u^\dagger)^{dc} - \delta^{pa} \delta^{rb} \delta^{cd} g_L^2 \right\} C_{\ell q}^{(\times) abcd}, \end{aligned} \quad (9.1)$$

$$\begin{aligned} \beta_{C_{H\ell}^{(\parallel) pr}}^{(2)} = & \frac{1}{6} g_L^2 (11\delta^{pr} T_{\ell H} - 573(C_{\ell HH} C_{\ell HH}^\dagger)^{rp}) + \frac{1}{6} g_Y^2 (19\delta^{pr} T_{\ell H} - 326(C_{\ell HH} C_{\ell HH}^\dagger)^{rp}) + \frac{1}{2} ((C_{\ell HH} Y_e Y_e^\dagger C_{\ell HH}^\dagger)^{rp} + 2(Y_e Y_e^\dagger)^{pr} T_{\ell H} \\ & + 30T_2(C_{\ell HH} C_{\ell HH}^\dagger)^{rp} - 2(Y_e^\dagger Y_e C_{\ell HH} C_{\ell HH}^\dagger)^{rp} - 2(Y_e Y_e^\dagger C_{\ell HH}^\dagger C_{\ell HH})^{pr}) + 10\lambda(C_{\ell HH} C_{\ell HH}^\dagger)^{rp} + \left\{ g_Y^2 \left( \frac{1}{12} T_2 \delta^{pr} \right. \right. \\ & - \frac{1}{8} (Y_e Y_e^\dagger)^{pr} \left. \right) + g_L^2 \left( \frac{1}{12} T_2 \delta^{pr} + \frac{7}{6} (Y_e Y_e^\dagger)^{pr} \right) + \frac{15}{8} (Y_e Y_e^\dagger Y_e Y_e^\dagger)^{pr} - \frac{7}{54} \delta^{pr} g_Y^2 g_L^2 - \frac{3}{8} \delta^{pr} g_L^4 - \frac{20}{27} \delta^{pr} g_Y^4 - \lambda \left( \frac{5}{12} \delta^{pr} g_L^2 + \frac{5}{12} \delta^{pr} g_Y^2 \right) \left. \right\} C_{HD}^{(\parallel)} \\ & + \left\{ \frac{1}{2} T_2 (Y_e Y_e^\dagger)^{pr} + g_Y^2 \left( \frac{1}{6} T_2 \delta^{pr} - \frac{9}{8} (Y_e Y_e^\dagger)^{pr} \right) + \frac{9}{4} (Y_e Y_e^\dagger Y_e Y_e^\dagger)^{pr} - \frac{181}{432} \delta^{pr} g_Y^4 - \lambda \left( \frac{1}{4} (Y_e Y_e^\dagger)^{pr} + \frac{5}{12} \delta^{pr} g_Y^2 \right) - \frac{1225}{432} \delta^{pr} g_Y^2 g_L^2 \right. \\ & \left. - \frac{9}{2} g_L^2 (Y_e Y_e^\dagger)^{pr} \right\} C_{HD}^{(\times)} + \left\{ \frac{1}{2} g_Y^4 (Y_e Y_e^\dagger)^{pr} + 6\delta^{pr} \lambda g_Y^4 - 3\delta^{pr} g_Y^6 - \frac{10}{3} \delta^{pr} g_Y^4 g_L^2 \right\} C_{HB} + \left\{ \frac{9}{2} g_L^4 (Y_e Y_e^\dagger)^{pr} + 6\delta^{pr} \lambda g_L^4 - 6\delta^{pr} g_Y^2 g_L^4 \right. \end{aligned}$$

$$\begin{aligned}
& -\frac{71}{3}\delta^{pr}g_L^6\Big\}C_{HW}+\Big\{\frac{19}{12}\delta^{pr}g_Y^2g_L^4+2\delta^{pr}\lambda g_Y^2g_L^2-\frac{9}{4}\delta^{pr}g_Y^4g_L^2-5g_Y^2g_L^2(Y_eY_e^\dagger)^{pr}\Big\}C_{HWB}+\Big\{g_L^6\Big(3T_2\delta^{pr}+\frac{45}{2}(Y_eY_e^\dagger)^{pr}\Big)+\frac{20}{3}\delta^{pr}g_L^8 \\
& -\frac{17}{2}\delta^{pr}g_Y^2g_L^6\Big\}C_W+\Big\{\frac{3}{4}\delta^{pa}(Y_e^\dagger Y_e Y_e^\dagger)^{rb}-\frac{3}{2}\delta^{pa}g_Y^2Y_e^{*rb}\Big\}C_{eH}^{\textcolor{red}{ab}}+\textcolor{red}{C}_{eH}^{*ab}\Big\{\frac{3}{4}\delta^{ra}(Y_eY_e^\dagger Y_e)^{pb}-\frac{3}{2}\delta^{ra}g_Y^2Y_e^{pb}\Big\}+\Big\{g_Y^2g_L^2\Big(\frac{5}{4}\delta^{pa}Y_e^{*rb}+\frac{9}{4}\delta^{pr}Y_e^{*ab}\Big) \\
& +g_Y^2\Big(\frac{7}{2}Y_e^{*rb}(Y_eY_e^\dagger)^{pa}+\frac{33}{4}\delta^{pa}(Y_e^\dagger Y_e Y_e^\dagger)^{rb}-\frac{1}{2}\delta^{pr}(Y_e^\dagger Y_e Y_e^\dagger)^{ab}\Big)-g_Y^4\Big(\frac{15}{4}\delta^{pa}Y_e^{*rb}+\frac{27}{4}\delta^{pr}Y_e^{*ab}\Big)-3\delta^{pa}\lambda g_Y^2Y_e^{*rb}\Big\}C_{eB}^{\textcolor{red}{ab}}+\textcolor{red}{C}_{eB}^{*ab}\Big\{g_Y^2g_L^2\Big(\frac{5}{4}\delta^{ra}Y_e^{pb} \\
& +\frac{9}{4}\delta^{pr}Y_e^{ab}\Big)+g_Y^2\Big(\frac{7}{2}Y_e^{pb}(Y_eY_e^\dagger)^{ar}+\frac{33}{4}\delta^{ra}(Y_eY_e^\dagger Y_e)^{pb}-\frac{1}{2}\delta^{pr}(Y_eY_e^\dagger Y_e)^{ab}\Big)-g_Y^4\Big(\frac{15}{4}\delta^{ra}Y_e^{pb}+\frac{27}{4}\delta^{pr}Y_e^{ab}\Big)-3\delta^{ra}\lambda g_Y^2Y_e^{pb}\Big\}+\Big\{g_L^4\Big(\frac{29}{24}\delta^{pr}Y_e^{*ab} \\
& -15\delta^{pa}Y_e^{*rb}\Big)+g_L^2\Big(\frac{1}{4}\delta^{pr}(Y_e^\dagger Y_e Y_e^\dagger)^{ab}+\frac{9}{8}\delta^{pa}(Y_e^\dagger Y_e Y_e^\dagger)^{rb}-\frac{3}{4}Y_e^{*rb}(Y_eY_e^\dagger)^{pa}-\frac{3}{2}T_2\delta^{pa}Y_e^{*rb}\Big)-g_Y^2g_L^2\Big(\frac{3}{2}\delta^{pa}Y_e^{*rb}+\frac{29}{8}\delta^{pr}Y_e^{*ab}\Big)\Big\}C_{eW}^{\textcolor{red}{ab}} \\
& +\textcolor{red}{C}_{eW}^{*ab}\Big\{g_L^4\Big(\frac{29}{24}\delta^{pr}Y_e^{ab}-15\delta^{ra}Y_e^{pb}\Big)+g_L^2\Big(\frac{1}{4}\delta^{pr}(Y_eY_e^\dagger Y_e)^{ab}+\frac{9}{8}\delta^{ra}(Y_eY_e^\dagger Y_e)^{pb}-\frac{3}{4}Y_e^{pb}(Y_eY_e^\dagger)^{ar}-\frac{3}{2}T_2\delta^{ra}Y_e^{pb}\Big)-g_Y^2g_L^2\Big(\frac{3}{2}\delta^{ra}Y_e^{pb}+\frac{29}{8}\delta^{pr}Y_e^{ab}\Big)\Big\} \\
& +\Big\{\frac{11}{12}\delta^{pr}g_Y^2g_L^2Y_u^{*ab}+g_Y^2\Big(\frac{3}{2}\delta^{pr}(Y_d^\dagger Y_d Y_u^\dagger)^{ab}+\frac{3}{2}\delta^{pr}(Y_u^\dagger Y_u Y_u^\dagger)^{ab}\Big)-\frac{15}{4}\delta^{pr}g_Y^4Y_u^{*ab}\Big\}C_{uB}^{\textcolor{red}{ab}}+\textcolor{red}{C}_{uB}^{*ab}\Big\{\frac{11}{12}\delta^{pr}g_Y^2g_L^2Y_u^{ab}+g_Y^2\Big(\frac{3}{2}\delta^{pr}(Y_dY_d^\dagger Y_u)^{ab} \\
& +\frac{3}{2}\delta^{pr}(Y_uY_u^\dagger Y_u)^{ab}\Big)-\frac{15}{4}\delta^{pr}g_Y^4Y_u^{ab}\Big\}+\Big\{g_L^2\Big(\frac{3}{4}\delta^{pr}(Y_d^\dagger Y_d Y_u^\dagger)^{ab}+\frac{3}{4}\delta^{pr}(Y_u^\dagger Y_u Y_u^\dagger)^{ab}\Big)+\frac{17}{8}\delta^{pr}g_Y^2g_L^2Y_u^{*ab}-\frac{79}{8}\delta^{pr}g_Y^4Y_u^{*ab}\Big\}C_{uW}^{\textcolor{red}{ab}} \\
& +\textcolor{red}{C}_{uW}^{*ab}\Big\{g_L^2\Big(\frac{3}{4}\delta^{pr}(Y_dY_d^\dagger Y_u)^{ab}+\frac{3}{4}\delta^{pr}(Y_uY_u^\dagger Y_u)^{ab}\Big)+\frac{17}{8}\delta^{pr}g_Y^2g_L^2Y_u^{ab}-\frac{79}{8}\delta^{pr}g_Y^4Y_u^{ab}\Big\}+\Big\{\frac{16}{3}\delta^{pr}g_s^2g_L^2Y_u^{*ab}+\frac{16}{3}\delta^{pr}g_Y^2g_s^2Y_u^{*ab}\Big\}C_{uG}^{\textcolor{red}{ab}} \\
& +\textcolor{red}{C}_{uG}^{*ab}\Big\{\frac{16}{3}\delta^{pr}g_s^2g_L^2Y_u^{ab}+\frac{16}{3}\delta^{pr}g_Y^2g_s^2Y_u^{ab}\Big\}+\Big\{\frac{113}{12}\delta^{pr}g_Y^2g_L^2Y_d^{*ab}-g_Y^2\Big(\frac{3}{2}\delta^{pr}(Y_d^\dagger Y_d Y_d^\dagger)^{ab}+\frac{3}{2}\delta^{pr}(Y_u^\dagger Y_u Y_d^\dagger)^{ab}\Big)-\frac{9}{4}\delta^{pr}g_Y^4Y_d^{*ab}\Big\}C_{dB}^{\textcolor{red}{ab}} \\
& +\textcolor{red}{C}_{dB}^{*ab}\Big\{\frac{113}{12}\delta^{pr}g_Y^2g_L^2Y_d^{ab}-g_Y^2\Big(\frac{3}{2}\delta^{pr}(Y_dY_d^\dagger Y_d)^{ab}+\frac{3}{2}\delta^{pr}(Y_uY_u^\dagger Y_d)^{ab}\Big)-\frac{9}{4}\delta^{pr}g_Y^4Y_d^{ab}\Big\}+\Big\{\frac{1}{8}\delta^{pr}g_Y^2g_L^2Y_d^{*ab}+g_L^2\Big(\frac{3}{4}\delta^{pr}(Y_d^\dagger Y_d Y_d^\dagger)^{ab} \\
& +\frac{3}{4}\delta^{pr}(Y_u^\dagger Y_u Y_d^\dagger)^{ab}\Big)+\frac{29}{8}\delta^{pr}g_L^4Y_d^{*ab}\Big\}C_{dW}^{\textcolor{red}{ab}}+\textcolor{red}{C}_{dW}^{*ab}\Big\{\frac{1}{8}\delta^{pr}g_Y^2g_L^2Y_d^{ab}+g_L^2\Big(\frac{3}{4}\delta^{pr}(Y_dY_d^\dagger Y_d)^{ab}+\frac{3}{4}\delta^{pr}(Y_uY_u^\dagger Y_d)^{ab}\Big)+\frac{29}{8}\delta^{pr}g_L^4Y_d^{ab}\Big\} \\
& +\Big\{\frac{16}{3}\delta^{pr}g_s^2g_L^2Y_d^{*ab}+\frac{16}{3}\delta^{pr}g_Y^2g_s^2Y_d^{*ab}\Big\}C_{dG}^{\textcolor{red}{ab}}+\textcolor{red}{C}_{dG}^{*ab}\Big\{\frac{16}{3}\delta^{pr}g_s^2g_L^2Y_d^{ab}+\frac{16}{3}\delta^{pr}g_Y^2g_s^2Y_d^{ab}\Big\}+\Big\{\frac{1}{2}(Y_eY_e^\dagger)^{pr}(Y_eY_e^\dagger)^{ba}+g_Y^2g_L^2\Big(\frac{133}{108}\delta^{pr}\delta^{ab} \\
& -\frac{185}{54}\delta^{pa}\delta^{rb}\Big)+g_Y^4\Big(\frac{187}{108}\delta^{pr}\delta^{ab}-\frac{131}{54}\delta^{pa}\delta^{rb}\Big)+g_L^4\Big(\frac{9}{2}\delta^{pr}\delta^{ab}-9\delta^{pa}\delta^{rb}\Big)+g_L^2\Big(\frac{11}{36}\delta^{pr}(Y_eY_e^\dagger)^{ba}+\frac{779}{144}\delta^{rb}(Y_eY_e^\dagger)^{pa}+\frac{779}{144}\delta^{pa}(Y_eY_e^\dagger)^{br} \\
\end{aligned}$$



$$\begin{aligned}
& -\frac{3}{4}\text{T}_2\delta^{pa}\delta^{rb}) + \delta^{rb}(Y_e Y_e^\dagger Y_e Y_e^\dagger)^{pa} + \delta^{pa}(Y_e Y_e^\dagger Y_e Y_e^\dagger)^{br} + g_Y^2 \left( \frac{65}{144}\delta^{rb}(Y_e Y_e^\dagger)^{pa} + \frac{65}{144}\delta^{pa}(Y_e Y_e^\dagger)^{br} + \frac{19}{12}\delta^{pa}\delta^{rb}\text{Tr}[Y_u^\dagger Y_u] + \frac{53}{12}\delta^{pa}\delta^{rb}\text{Tr}[Y_e^\dagger Y_e] \right. \\
& - \frac{49}{36}\delta^{pr}(Y_e Y_e^\dagger)^{ba} - \frac{41}{12}\delta^{pa}\delta^{rb}\text{Tr}[Y_d^\dagger Y_d] \left. \right) + g_s^2 \left( 40\delta^{pa}\delta^{rb}\text{Tr}[Y_d^\dagger Y_d] + 40\delta^{pa}\delta^{rb}\text{Tr}[Y_u^\dagger Y_u] \right) + 6\delta^{pa}\delta^{rb}\text{Tr}[Y_d^\dagger Y_d Y_u^\dagger Y_u] - \frac{3}{4}\text{T}_2\delta^{rb}(Y_e Y_e^\dagger)^{pa} \\
& - \frac{3}{4}\text{T}_2\delta^{pa}(Y_e Y_e^\dagger)^{br} - \lambda \left( 3\delta^{rb}(Y_e Y_e^\dagger)^{pa} + 3\delta^{pa}(Y_e Y_e^\dagger)^{br} \right) - \frac{9}{2}(Y_e Y_e^\dagger)^{pa}(Y_e Y_e^\dagger)^{br} - 6\text{T}_4\delta^{pa}\delta^{rb} \left. \right\} C_{H\ell}^{(\parallel)ab} + \left\{ g_Y^2 g_L^2 \left( \frac{877}{108}\delta^{pa}\delta^{rb} - \frac{73}{108}\delta^{pr}\delta^{ab} \right) \right. \\
& + g_L^4 \left( \frac{83}{36}\delta^{pa}\delta^{rb} - \frac{11}{72}\delta^{pr}\delta^{ab} \right) + g_Y^4 \left( \frac{31}{108}\delta^{pa}\delta^{rb} + \frac{187}{216}\delta^{pr}\delta^{ab} \right) + g_L^2 \left( \frac{10}{9}\delta^{pr}(Y_e Y_e^\dagger)^{ba} + \frac{185}{72}\delta^{rb}(Y_e Y_e^\dagger)^{pa} + \frac{185}{72}\delta^{pa}(Y_e Y_e^\dagger)^{br} - \delta^{ab}(Y_e Y_e^\dagger)^{pr} \right. \\
& - 3\delta^{pa}\delta^{rb}\text{Tr}[Y_e^\dagger Y_e] - \frac{17}{2}\delta^{pa}\delta^{rb}\text{Tr}[Y_d^\dagger Y_d] - \frac{17}{2}\delta^{pa}\delta^{rb}\text{Tr}[Y_u^\dagger Y_u] \left. \right) + g_Y^2 \left( \frac{233}{72}\delta^{rb}(Y_e Y_e^\dagger)^{pa} + \frac{233}{72}\delta^{pa}(Y_e Y_e^\dagger)^{br} - \frac{1}{6}\delta^{ab}(Y_e Y_e^\dagger)^{pr} - \frac{1}{3}\delta^{pa}\delta^{rb}\text{Tr}[Y_e^\dagger Y_e] \right. \\
& - \frac{1}{2}\delta^{pa}\delta^{rb}\text{Tr}[Y_d^\dagger Y_d] - \frac{1}{2}\delta^{pa}\delta^{rb}\text{Tr}[Y_u^\dagger Y_u] - \frac{13}{18}\delta^{pr}(Y_e Y_e^\dagger)^{ba} \left. \right) + 3\delta^{pa}\delta^{rb}\text{Tr}[Y_d^\dagger Y_d Y_u^\dagger Y_u] - \frac{1}{2}\text{T}_4\delta^{pa}\delta^{rb} - \frac{1}{2}(Y_e Y_e^\dagger)^{pr}(Y_e Y_e^\dagger)^{ba} - \lambda \left( \frac{3}{2}\delta^{rb}(Y_e Y_e^\dagger)^{pa} \right. \\
& + \frac{3}{2}\delta^{pa}(Y_e Y_e^\dagger)^{br} \left. \right) - 2\text{T}_2\delta^{rb}(Y_e Y_e^\dagger)^{pa} - 2\text{T}_2\delta^{pa}(Y_e Y_e^\dagger)^{br} - \frac{21}{4}(Y_e Y_e^\dagger)^{pa}(Y_e Y_e^\dagger)^{br} - \frac{25}{4}\delta^{rb}(Y_e Y_e^\dagger Y_e Y_e^\dagger)^{pa} - \frac{25}{4}\delta^{pa}(Y_e Y_e^\dagger Y_e Y_e^\dagger)^{br} \left. \right\} C_{H\ell}^{(\times)ab} \\
& + \left\{ \frac{3}{2}\text{T}_2 Y_e^{*rb} Y_e^{pa} + \frac{7}{2} Y_e^{pa} (Y_e^\dagger Y_e Y_e^\dagger)^{rb} + \frac{7}{2} Y_e^{*rb} (Y_e Y_e^\dagger Y_e)^{pa} - \frac{29}{108}\delta^{pr}\delta^{ab} g_Y^2 g_L^2 - \frac{1}{2}(Y_e^\dagger Y_e)^{ba} (Y_e Y_e^\dagger)^{pr} - g_L^2 \left( \frac{5}{36}\delta^{pr}(Y_e^\dagger Y_e)^{ba} + \frac{33}{8} Y_e^{*rb} Y_e^{pa} \right) \right. \\
& - g_Y^2 \left( \frac{7}{8} Y_e^{*rb} Y_e^{pa} + \frac{77}{36}\delta^{pr}(Y_e^\dagger Y_e)^{ba} \right) - \frac{137}{108}\delta^{pr}\delta^{ab} g_Y^4 \left. \right\} C_{He}^{ab} + \left\{ \frac{77}{108}\delta^{pr}\delta^{ab} g_Y^4 + g_L^2 \left( \frac{11}{12}\delta^{pr}(Y_d Y_d^\dagger)^{ba} - \frac{11}{12}\delta^{pr}(Y_u Y_u^\dagger)^{ba} \right) + g_Y^2 \left( \frac{7}{12}\delta^{pr}(Y_d Y_d^\dagger)^{ba} \right. \right. \\
& + \frac{7}{4}\delta^{pr}(Y_u Y_u^\dagger)^{ba} \left. \right) + \frac{3}{2}(Y_d Y_d^\dagger)^{ba} (Y_e Y_e^\dagger)^{pr} + \frac{27}{2}\delta^{pr}\delta^{ab} g_L^4 - \frac{133}{108}\delta^{pr}\delta^{ab} g_Y^2 g_L^2 - \frac{3}{2}(Y_e Y_e^\dagger)^{pr} (Y_u Y_u^\dagger)^{ba} - \frac{8}{3}\delta^{pr}\delta^{ab} g_Y^2 g_s^2 \left. \right\} C_{Hq}^{(\parallel)ab} + \left\{ \frac{77}{216}\delta^{pr}\delta^{ab} g_Y^4 \right. \\
& + g_Y^2 \left( \frac{7}{6}\delta^{pr}(Y_d Y_d^\dagger)^{ba} + \frac{5}{4}\delta^{pr}(Y_u Y_u^\dagger)^{ba} \right) + g_L^2 \left( \frac{29}{12}\delta^{pr}(Y_u Y_u^\dagger)^{ba} + \frac{10}{3}\delta^{pr}(Y_d Y_d^\dagger)^{ba} - \frac{5}{2}\delta^{ab}(Y_e Y_e^\dagger)^{pr} \right) + \frac{217}{108}\delta^{pr}\delta^{ab} g_Y^2 g_L^2 - \frac{5}{8}\delta^{pr}\delta^{ab} g_L^4 - \frac{4}{3}\delta^{pr}\delta^{ab} g_Y^2 g_s^2 \\
& - \frac{3}{2}(Y_d Y_d^\dagger)^{ba} (Y_e Y_e^\dagger)^{pr} - 3(Y_e Y_e^\dagger)^{pr} (Y_u Y_u^\dagger)^{ba} - 4\delta^{pr}\delta^{ab} g_s^2 g_L^2 \left. \right\} C_{Hq}^{(\times)ab} + \left\{ \frac{5}{12}\delta^{pr} g_L^2 (Y_u^\dagger Y_u)^{ba} + \frac{29}{54}\delta^{pr}\delta^{ab} g_Y^2 g_L^2 + \frac{3}{2}(Y_u^\dagger Y_u)^{ba} (Y_e Y_e^\dagger)^{pr} \right. \\
& + \frac{49}{12}\delta^{pr} g_Y^2 (Y_u^\dagger Y_u)^{ba} - \frac{283}{54}\delta^{pr}\delta^{ab} g_Y^4 - \frac{16}{3}\delta^{pr}\delta^{ab} g_Y^2 g_s^2 \left. \right\} C_{Hu}^{ab} + \left\{ \frac{8}{3}\delta^{pr}\delta^{ab} g_Y^2 g_s^2 - \frac{29}{108}\delta^{pr}\delta^{ab} g_Y^2 g_L^2 - \frac{5}{12}\delta^{pr} g_L^2 (Y_d^\dagger Y_d)^{ba} - \frac{113}{108}\delta^{pr}\delta^{ab} g_Y^4 \right. \\
& - \frac{3}{2}(Y_d^\dagger Y_d)^{ba} (Y_e Y_e^\dagger)^{pr} - \frac{7}{4}\delta^{pr} g_Y^2 (Y_d^\dagger Y_d)^{ba} \left. \right\} C_{Hd}^{ab} - \left\{ \frac{5}{12}\delta^{pr} g_L^2 (Y_d^\dagger Y_u)^{ba} + \frac{17}{12}\delta^{pr} g_Y^2 (Y_d^\dagger Y_u)^{ba} + \frac{3}{2}(Y_d^\dagger Y_u)^{ba} (Y_e Y_e^\dagger)^{pr} \right\} C_{Hud}^{ab} \\
& - C_{Hud}^{*ab} \left\{ \frac{5}{12}\delta^{pr} g_L^2 (Y_u^\dagger Y_d)^{ab} + \frac{17}{12}\delta^{pr} g_Y^2 (Y_u^\dagger Y_d)^{ab} + \frac{3}{2}(Y_u^\dagger Y_d)^{ab} (Y_e Y_e^\dagger)^{pr} \right\} + \left\{ \frac{17}{27}\delta^{pa}\delta^{rb}\delta^{cd} g_Y^2 g_L^2 + g_Y^2 \left( \frac{5}{9}\delta^{pa} Y_e^{*rd} Y_e^{bc} + \frac{5}{9}\delta^{rb} Y_e^{*ad} Y_e^{pc} \right. \right. \\
& + \frac{29}{12}\delta^{pa}\delta^{rb} (Y_e^\dagger Y_e)^{dc} \left. \right) + \frac{62}{27}\delta^{pa}\delta^{rb}\delta^{cd} g_Y^4 - g_L^2 \left( \frac{29}{18}\delta^{pa} Y_e^{*rd} Y_e^{bc} + \frac{29}{18}\delta^{rb} Y_e^{*ad} Y_e^{pc} + \frac{15}{4}\delta^{pa}\delta^{rb} (Y_e^\dagger Y_e)^{dc} \right) - \delta^{pa} Y_e^{bc} (Y_e^\dagger Y_e Y_e^\dagger)^{rd} - \delta^{rb} Y_e^{*ad} (Y_e Y_e^\dagger Y_e)^{pc}
\end{aligned}$$

$$\begin{aligned}
& -\frac{3}{2}\delta^{rb}Y_e^{pc}(Y_e^\dagger Y_e Y_e^\dagger)^{ad} - \frac{3}{2}\delta^{pa}Y_e^{*rd}(Y_e Y_e^\dagger Y_e)^{bc} - 6\delta^{pa}\delta^{rb}(Y_e^\dagger Y_e Y_e^\dagger Y_e)^{dc} \Big\} C_{\ell e}^{abcd} + \left\{ \frac{16}{3}\delta^{pa}\delta^{rb}\delta^{cd}g_Y^2g_s^2 + \frac{146}{27}\delta^{pa}\delta^{rb}\delta^{cd}g_Y^4 \right. \\
& + 18\delta^{pa}\delta^{rb}(Y_u^\dagger Y_u Y_u^\dagger Y_u)^{dc} - \frac{34}{27}\delta^{pa}\delta^{rb}\delta^{cd}g_Y^2g_L^2 - 3\delta^{pa}\delta^{rb}(Y_u^\dagger Y_d Y_d^\dagger Y_u)^{dc} - \frac{27}{4}\delta^{pa}\delta^{rb}g_L^2(Y_u^\dagger Y_u)^{dc} - \frac{199}{12}\delta^{pa}\delta^{rb}g_Y^2(Y_u^\dagger Y_u)^{dc} \\
& \left. - 40\delta^{pa}\delta^{rb}g_s^2(Y_u^\dagger Y_u)^{dc} \right\} C_{\ell u}^{abcd} + \left\{ \frac{17}{27}\delta^{pa}\delta^{rb}\delta^{cd}g_Y^2g_L^2 + \frac{44}{27}\delta^{pa}\delta^{rb}\delta^{cd}g_Y^4 + 3\delta^{pa}\delta^{rb}(Y_d^\dagger Y_u Y_u^\dagger Y_d)^{dc} + 40\delta^{pa}\delta^{rb}g_s^2(Y_d^\dagger Y_d)^{dc} - \frac{8}{3}\delta^{pa}\delta^{rb}\delta^{cd}g_Y^2g_s^2 \right. \\
& - \frac{45}{4}\delta^{pa}\delta^{rb}g_L^2(Y_d^\dagger Y_d)^{dc} - \frac{137}{12}\delta^{pa}\delta^{rb}g_Y^2(Y_d^\dagger Y_d)^{dc} - 18\delta^{pa}\delta^{rb}(Y_d^\dagger Y_d Y_d^\dagger Y_d)^{dc} \Big\} C_{\ell d}^{abcd} + \left\{ g_Y^2\left(\frac{4}{3}\delta^{ad}Y_e^{*rb}Y_e^{pc} + \frac{8}{3}\delta^{pr}\delta^{ad}(Y_e^\dagger Y_e)^{bc}\right) - \frac{8}{9}\delta^{pr}\delta^{ab}\delta^{cd}g_Y^4 \right. \\
& \left. - 4Y_e^{*rb}Y_e^{pa}(Y_e^\dagger Y_e)^{dc} \right\} C_{ee}^{abcd} + \left\{ \frac{16}{3}\delta^{pr}\delta^{ad}g_Y^2(Y_u^\dagger Y_u)^{bc} - \frac{32}{27}\delta^{pr}\delta^{ad}\delta^{bc}g_Y^4 \right\} C_{uu}^{abcd} + \left\{ \frac{8}{3}\delta^{pr}\delta^{ad}g_Y^2(Y_d^\dagger Y_d)^{bc} - \frac{8}{27}\delta^{pr}\delta^{ad}\delta^{bc}g_Y^4 \right\} C_{dd}^{abcd} \\
& + \left\{ \frac{3}{4}\delta^{pa}Y_e^{*rb}(Y_d Y_d^\dagger Y_d)^{dc} + \frac{29}{12}\delta^{pa}g_L^2Y_e^{*rb}Y_d^{dc} + 3\delta^{pa}Y_d^{dc}(Y_e^\dagger Y_e Y_e^\dagger)^{rb} - \frac{3}{4}\delta^{pa}Y_e^{*rb}(Y_u Y_u^\dagger Y_d)^{dc} - \frac{5}{6}\delta^{pa}g_Y^2Y_e^{*rb}Y_d^{dc} \right\} C_{\ell edq}^{abcd} \\
& + C_{\ell edq}^{*abcd} \left\{ \frac{3}{4}\delta^{ra}Y_e^{pb}(Y_d^\dagger Y_d Y_d^\dagger)^{dc} + \frac{29}{12}\delta^{ra}g_L^2Y_d^{*dc}Y_e^{pb} + 3\delta^{ra}Y_d^{*dc}(Y_e Y_e^\dagger Y_e)^{pb} - \frac{3}{4}\delta^{ra}Y_e^{pb}(Y_u^\dagger Y_u Y_d^\dagger)^{dc} - \frac{5}{6}\delta^{ra}g_Y^2Y_d^{*dc}Y_e^{pb} \right\} \\
& + \left\{ \frac{3}{4}\delta^{pa}Y_e^{*rb}(Y_d^\dagger Y_d Y_u^\dagger)^{cd} + \frac{5}{6}\delta^{pa}g_Y^2Y_e^{*rb}Y_u^{cd} - \frac{3}{4}\delta^{pa}Y_e^{*rb}(Y_u^\dagger Y_u Y_u^\dagger)^{cd} - \frac{29}{12}\delta^{pa}g_L^2Y_e^{*rb}Y_u^{cd} - 3\delta^{pa}Y_u^{cd}(Y_e^\dagger Y_e Y_e^\dagger)^{rb} \right\} C_{\ell equ}^{abcd} \\
& + C_{\ell equ}^{*abcd} \left\{ \frac{3}{4}\delta^{ra}Y_e^{pb}(Y_d Y_d^\dagger Y_u)^{cd} + \frac{5}{6}\delta^{ra}g_Y^2Y_e^{pb}Y_u^{cd} - \frac{3}{4}\delta^{ra}Y_e^{pb}(Y_u Y_u^\dagger Y_u)^{cd} - \frac{29}{12}\delta^{ra}g_L^2Y_e^{pb}Y_u^{cd} - 3\delta^{ra}Y_u^{cd}(Y_e Y_e^\dagger Y_e)^{pb} \right\} + \left\{ \frac{3}{2}\delta^{pa}Y_u^{*cb}(Y_e^\dagger Y_e Y_e^\dagger)^{rd} \right. \\
& + \frac{53}{24}\delta^{pa}g_L^2Y_e^{*rd}Y_u^{*cb} + \frac{21}{4}\delta^{pa}Y_e^{*rd}(Y_d^\dagger Y_d Y_u^\dagger)^{cb} - \frac{7}{24}\delta^{pa}g_Y^2Y_e^{*rd}Y_u^{*cb} \Big\} C_{\ell uqe}^{abcd} + C_{\ell uqe}^{*abcd} \left\{ \frac{3}{2}\delta^{ra}Y_u^{cb}(Y_e Y_e^\dagger Y_e)^{pd} + \frac{53}{24}\delta^{ra}g_L^2Y_e^{pd}Y_u^{cb} \right. \\
& + \frac{21}{4}\delta^{ra}Y_e^{pd}(Y_d Y_d^\dagger Y_u)^{cb} - \frac{7}{24}\delta^{ra}g_Y^2Y_e^{pd}Y_u^{cb} \Big\} + \left\{ g_Y^2g_L^2\left(\frac{2}{27}\delta^{pa}\delta^{rd}\delta^{bc} + \frac{2}{9}\delta^{pr}\delta^{ad}\delta^{bc} + \frac{7}{27}\delta^{pa}\delta^{rb}\delta^{cd}\right) + g_Y^4\left(\frac{16}{27}\delta^{pa}\delta^{rb}\delta^{cd} + \frac{29}{27}\delta^{pa}\delta^{rd}\delta^{bc} \right. \right. \\
& - \frac{4}{9}\delta^{pr}\delta^{ad}\delta^{bc} \Big) + g_L^4\left(\frac{7}{3}\delta^{pa}\delta^{rb}\delta^{cd} - \frac{2}{9}\delta^{pr}\delta^{ad}\delta^{bc} - \frac{64}{9}\delta^{pa}\delta^{rd}\delta^{bc}\right) + g_L^2\left(\frac{4}{3}\delta^{pr}\delta^{bc}(Y_e Y_e^\dagger)^{da} + \frac{19}{3}\delta^{pa}\delta^{rd}(Y_e Y_e^\dagger)^{bc} - \frac{1}{3}\delta^{rd}\delta^{bc}(Y_e Y_e^\dagger)^{pa} - \frac{1}{3}\delta^{pa}\delta^{bc}(Y_e Y_e^\dagger)^{dr} \right. \\
& - \frac{7}{2}\delta^{pa}\delta^{rb}(Y_e Y_e^\dagger)^{dc} \Big) + g_Y^2\left(2\delta^{pa}\delta^{rd}(Y_e Y_e^\dagger)^{bc} + \frac{61}{6}\delta^{pa}\delta^{rb}(Y_e Y_e^\dagger)^{dc} - \frac{4}{3}\delta^{pr}\delta^{bc}(Y_e Y_e^\dagger)^{da} \right) + 12\delta^{pa}\delta^{rb}(Y_e Y_e^\dagger Y_e Y_e^\dagger)^{dc} - \delta^{pa}\delta^{rd}(Y_e Y_e^\dagger Y_e Y_e^\dagger)^{bc} \\
& - 3\delta^{rd}(Y_e Y_e^\dagger)^{pa}(Y_e Y_e^\dagger)^{bc} - 3\delta^{pa}(Y_e Y_e^\dagger)^{bc}(Y_e Y_e^\dagger)^{dr} \Big\} C_{\ell \ell}^{abcd} + \left\{ g_Y^2\left(\frac{4}{3}\delta^{pr}\delta^{bc}(Y_d Y_d^\dagger)^{da} - \frac{4}{3}\delta^{pr}\delta^{bc}(Y_u Y_u^\dagger)^{da}\right) + g_L^2\left(4\delta^{pr}\delta^{bc}(Y_d Y_d^\dagger)^{da} + 4\delta^{pr}\delta^{bc}(Y_u Y_u^\dagger)^{da}\right) \right. \\
& \left. - \frac{4}{27}\delta^{pr}\delta^{ad}\delta^{bc}g_Y^4 - \frac{4}{3}\delta^{pr}\delta^{ad}\delta^{bc}g_L^4 \right\} C_{qq}^{(\parallel)abcd} + \left\{ g_Y^2\left(\frac{8}{3}\delta^{pr}\delta^{bc}(Y_d Y_d^\dagger)^{da} - \frac{8}{3}\delta^{pr}\delta^{bc}(Y_u Y_u^\dagger)^{da}\right) - \frac{8}{27}\delta^{pr}\delta^{ad}\delta^{bc}g_Y^4 \right\} C_{qq}^{(\times)abcd} + \left\{ \frac{1}{2}\delta^{pa}\delta^{rb}\delta^{cd}g_L^4 \right.
\end{aligned}$$

$$\begin{aligned}
& + \frac{47}{54} \delta^{pa} \delta^{rb} \delta^{cd} g_Y^2 g_L^2 + g_Y^2 \left( \frac{71}{12} \delta^{pa} \delta^{rb} (Y_d Y_d^\dagger)^{dc} + \frac{181}{12} \delta^{pa} \delta^{rb} (Y_u Y_u^\dagger)^{dc} \right) + g_s^2 \left( 40 \delta^{pa} \delta^{rb} (Y_u Y_u^\dagger)^{dc} - 40 \delta^{pa} \delta^{rb} (Y_d Y_d^\dagger)^{dc} \right) + \frac{8}{3} \delta^{pa} \delta^{rb} \delta^{cd} g_Y^2 g_s^2 \\
& + 18 \delta^{pa} \delta^{rb} (Y_d Y_d^\dagger Y_d Y_d^\dagger)^{dc} - \frac{14}{27} \delta^{pa} \delta^{rb} \delta^{cd} g_Y^4 - g_L^2 \left( \frac{21}{4} \delta^{pa} \delta^{rb} (Y_d Y_d^\dagger)^{dc} + \frac{39}{4} \delta^{pa} \delta^{rb} (Y_u Y_u^\dagger)^{dc} \right) - 18 \delta^{pa} \delta^{rb} (Y_u Y_u^\dagger Y_u Y_u^\dagger)^{dc} \Big\} C_{\ell q}^{(\parallel) abcd} \\
& + \left\{ g_L^4 \left( \frac{1}{3} \delta^{pr} \delta^{ab} \delta^{cd} - \frac{31}{6} \delta^{pa} \delta^{rb} \delta^{cd} \right) + g_Y^2 g_L^2 \left( \frac{1}{3} \delta^{pr} \delta^{ab} \delta^{cd} + \frac{68}{27} \delta^{pa} \delta^{rb} \delta^{cd} \right) + g_L^2 \left( \frac{35}{2} \delta^{pa} \delta^{rb} (Y_d Y_d^\dagger)^{dc} - \frac{1}{2} \delta^{rb} \delta^{cd} (Y_e Y_e^\dagger)^{pa} - \frac{1}{2} \delta^{pa} \delta^{cd} (Y_e Y_e^\dagger)^{br} \right. \right. \\
& - \frac{29}{4} \delta^{pa} \delta^{rb} (Y_u Y_u^\dagger)^{dc} \Big) + \frac{4}{3} \delta^{pa} \delta^{rb} \delta^{cd} g_Y^2 g_s^2 + \frac{3}{2} \delta^{rb} (Y_d Y_d^\dagger)^{dc} (Y_e Y_e^\dagger)^{pa} + \frac{3}{2} \delta^{pa} (Y_d Y_d^\dagger)^{dc} (Y_e Y_e^\dagger)^{br} + \frac{3}{2} \delta^{rb} (Y_e Y_e^\dagger)^{pa} (Y_u Y_u^\dagger)^{dc} + \frac{3}{2} \delta^{pa} (Y_e Y_e^\dagger)^{br} (Y_u Y_u^\dagger)^{dc} \\
& + \frac{3}{2} \delta^{pa} \delta^{rb} (Y_d Y_d^\dagger Y_d Y_d^\dagger)^{dc} + \frac{193}{12} \delta^{pa} \delta^{rb} g_Y^2 (Y_u Y_u^\dagger)^{dc} + 40 \delta^{pa} \delta^{rb} g_s^2 (Y_u Y_u^\dagger)^{dc} - \frac{7}{27} \delta^{pa} \delta^{rb} \delta^{cd} g_Y^4 - 4 \delta^{pa} \delta^{rb} \delta^{cd} g_s^2 g_L^2 \\
& \left. - \frac{33}{2} \delta^{pa} \delta^{rb} (Y_u Y_u^\dagger Y_u Y_u^\dagger)^{dc} \right\} C_{\ell q}^{(\times) abcd}, \tag{9.2}
\end{aligned}$$

## 9.2 $C_{H\ell}^{(\times)}$

$$\begin{aligned}
\beta_{C_{H\ell}^{(\times) pr}}^{(1)} &= 8(C_{\ell H H} C_{\ell H H}^\dagger)^{rp} + \left\{ \frac{1}{6} \delta^{pr} g_L^2 - \frac{1}{2} (Y_e Y_e^\dagger)^{pr} \right\} C_{HD}^{(\parallel)} + 3 \left\{ \delta^{rb} (Y_e Y_e^\dagger)^{pa} + \delta^{pa} (Y_e Y_e^\dagger)^{br} \right\} C_{H\ell}^{(\parallel) ab} + \left\{ \frac{1}{3} g_L^2 (2 \delta^{pr} \delta^{ab} - 17 \delta^{pa} \delta^{rb}) + \frac{1}{2} (4 T_2 \delta^{pa} \delta^{rb} \right. \\
& + 5 \delta^{rb} (Y_e Y_e^\dagger)^{pa} + 5 \delta^{pa} (Y_e Y_e^\dagger)^{br}) \Big\} C_{H\ell}^{(\times) ab} + 2 \delta^{pr} \delta^{ab} g_L^2 C_{Hq}^{(\times) ab} + \left\{ \frac{4}{3} \delta^{pa} \delta^{rd} \delta^{bc} g_L^2 - 4 \delta^{pa} \delta^{rd} (Y_e Y_e^\dagger)^{bc} \right\} C_{\ell\ell}^{abcd} + \left\{ 2 \delta^{pa} \delta^{rb} \delta^{cd} g_L^2 - 6 (\delta^{pa} \delta^{rb} (Y_d Y_d^\dagger)^{dc} \right. \\
& \left. + \delta^{pa} \delta^{rb} (Y_u Y_u^\dagger)^{dc}) \right\} C_{\ell q}^{(\times) abcd}, \tag{9.3}
\end{aligned}$$

$$\begin{aligned}
\beta_{C_{H\ell}^{(\times) pr}}^{(2)} &= \frac{1}{3} g_L^2 (240 (C_{\ell H H} C_{\ell H H}^\dagger)^{rp} - 11 \delta^{pr} T_{\ell H}) + \frac{1}{2} (2 (Y_e Y_e^\dagger)^{pr} T_{\ell H} - 5 (Y_e^\dagger Y_e C_{\ell H H} C_{\ell H H}^\dagger)^{rp} - 5 (Y_e Y_e^\dagger C_{\ell H H}^\dagger C_{\ell H H})^{pr} \\
& - 16 (C_{\ell H H} Y_e Y_e^\dagger C_{\ell H H}^\dagger)^{rp} - 24 T_2 (C_{\ell H H} C_{\ell H H}^\dagger)^{rp}) + 42 g_Y^2 (C_{\ell H H} C_{\ell H H}^\dagger)^{rp} - 8 \lambda (C_{\ell H H} C_{\ell H H}^\dagger)^{rp} + \left\{ \frac{7}{108} \delta^{pr} g_Y^2 g_L^2 \right. \\
& + \frac{1}{2} T_2 (Y_e Y_e^\dagger)^{pr} + \frac{3}{4} \delta^{pr} g_L^4 + \frac{5}{6} \delta^{pr} \lambda g_L^2 + \frac{5}{4} (Y_e Y_e^\dagger Y_e Y_e^\dagger)^{pr} - \frac{89}{144} g_Y^2 (Y_e Y_e^\dagger)^{pr} - g_L^2 \left( \frac{1}{6} T_2 \delta^{pr} + \frac{51}{16} (Y_e Y_e^\dagger)^{pr} \right) \Big\} C_{HD}^{(\parallel)} + \left\{ \frac{1}{2} \lambda (Y_e Y_e^\dagger)^{pr} \right. \\
& + \frac{59}{108} \delta^{pr} g_Y^2 g_L^2 + \frac{8}{9} g_Y^2 (Y_e Y_e^\dagger)^{pr} + \frac{7}{4} (Y_e Y_e^\dagger Y_e Y_e^\dagger)^{pr} \Big\} C_{HD}^{(\times)} + \left\{ \frac{11}{3} \delta^{pr} g_Y^4 g_L^2 + 7 g_Y^4 (Y_e Y_e^\dagger)^{pr} \right\} C_{HB} + \left\{ \delta^{pr} g_Y^2 g_L^4 + \frac{142}{3} \delta^{pr} g_L^6 \right. \\
& \left. - 12 \delta^{pr} \lambda g_L^4 \right\} C_{HW} + \left\{ \frac{1}{4} g_Y^2 g_L^2 (Y_e Y_e^\dagger)^{pr} + \frac{7}{4} \delta^{pr} g_Y^4 g_L^2 - \frac{11}{12} \delta^{pr} g_Y^2 g_L^4 - \delta^{pr} \lambda g_Y^2 g_L^2 \right\} C_{HWB} + \left\{ g_L^6 (12 (Y_e Y_e^\dagger)^{pr} - 6 T_2 \delta^{pr}) + 3 \delta^{pr} g_Y^2 g_L^6 \right.
\end{aligned}$$

$$\begin{aligned}
& -\frac{40}{3}\delta^{pr}g_L^8\Big\}C_W + \Big\{\frac{3}{2}\delta^{pa}\lambda Y_e^{*rb} - \frac{3}{2}\delta^{pa}g_Y^2Y_e^{*rb}\Big\}C_{eH}^{ab} + C_{eH}^{*ab}\Big\{\frac{3}{2}\delta^{ra}\lambda Y_e^{pb} - \frac{3}{2}\delta^{ra}g_Y^2Y_e^{pb}\Big\} + \Big\{g_Y^2g_L^2\Big(\frac{31}{8}\delta^{pa}Y_e^{*rb} - \frac{3}{2}\delta^{pr}Y_e^{*ab}\Big) \\
& + \frac{55}{8}\delta^{pa}g_Y^4Y_e^{*rb} - g_Y^2\Big(\frac{3}{2}T_2\delta^{pa}Y_e^{*rb} + \frac{9}{2}\delta^{pa}(Y_e^\dagger Y_e Y_e^\dagger)^{rb}\Big) - 3\delta^{pa}\lambda g_Y^2Y_e^{*rb}\Big\}C_{eB}^{ab} + C_{eB}^{*ab}\Big\{g_Y^2g_L^2\Big(\frac{31}{8}\delta^{ra}Y_e^{pb} - \frac{3}{2}\delta^{pr}Y_e^{ab}\Big) + \frac{55}{8}\delta^{ra}g_Y^4Y_e^{pb} \\
& - g_Y^2\Big(\frac{3}{2}T_2\delta^{ra}Y_e^{pb} + \frac{9}{2}\delta^{ra}(Y_e Y_e^\dagger Y_e)^{pb}\Big) - 3\delta^{ra}\lambda g_Y^2Y_e^{pb}\Big\} + \Big\{g_Y^2g_L^2\Big(\frac{47}{16}\delta^{pa}Y_e^{*rb} + 6\delta^{pr}Y_e^{*ab}\Big) + g_L^4\Big(\frac{25}{12}\delta^{pr}Y_e^{*ab} + \frac{87}{16}\delta^{pa}Y_e^{*rb}\Big) \\
& + g_L^2\Big(\frac{3}{4}T_2\delta^{pa}Y_e^{*rb} - \frac{1}{2}\delta^{pr}(Y_e^\dagger Y_e Y_e^\dagger)^{ab} - \frac{3}{4}\delta^{pa}(Y_e^\dagger Y_e Y_e^\dagger)^{rb} - \frac{3}{2}Y_e^{*rb}(Y_e Y_e^\dagger)^{pa}\Big) - \frac{9}{2}\delta^{pa}\lambda g_L^2Y_e^{*rb}\Big\}C_{eW}^{ab} + C_{eW}^{*ab}\Big\{g_Y^2g_L^2\Big(\frac{47}{16}\delta^{ra}Y_e^{pb} + 6\delta^{pr}Y_e^{ab}\Big) \\
& + g_L^4\Big(\frac{25}{12}\delta^{pr}Y_e^{ab} + \frac{87}{16}\delta^{ra}Y_e^{pb}\Big) + g_L^2\Big(\frac{3}{4}T_2\delta^{ra}Y_e^{pb} - \frac{1}{2}\delta^{pr}(Y_e Y_e^\dagger Y_e)^{ab} - \frac{3}{4}\delta^{ra}(Y_e Y_e^\dagger Y_e)^{pb} - \frac{3}{2}Y_e^{pb}(Y_e Y_e^\dagger)^{ar}\Big) - \frac{9}{2}\delta^{ra}\lambda g_L^2Y_e^{pb}\Big\} \\
& - \frac{65}{6}\delta^{pr}g_Y^2g_L^2Y_u^{*ab}C_{uB}^{ab} - \frac{65}{6}\delta^{pr}g_Y^2g_L^2C_{uB}^{*ab}Y_u^{ab} + \Big\{\frac{25}{4}\delta^{pr}g_L^4Y_u^{*ab} - g_L^2\Big(\frac{3}{2}\delta^{pr}(Y_d^\dagger Y_d Y_u^\dagger)^{ab} + \frac{3}{2}\delta^{pr}(Y_u^\dagger Y_u Y_u^\dagger)^{ab}\Big) - 5\delta^{pr}g_Y^2g_L^2Y_u^{*ab}\Big\}C_{uW}^{ab} \\
& + C_{uW}^{*ab}\Big\{\frac{25}{4}\delta^{pr}g_L^4Y_u^{ab} - g_L^2\Big(\frac{3}{2}\delta^{pr}(Y_d Y_d^\dagger Y_u)^{ab} + \frac{3}{2}\delta^{pr}(Y_u Y_u^\dagger Y_u)^{ab}\Big) - 5\delta^{pr}g_Y^2g_L^2Y_u^{ab}\Big\} - \frac{32}{3}\delta^{pr}g_s^2g_L^2Y_u^{*ab}C_{uG}^{ab} - \frac{32}{3}\delta^{pr}g_s^2g_L^2C_{uG}^{*ab}Y_u^{ab} \\
& - \frac{59}{6}\delta^{pr}g_Y^2g_L^2Y_d^{*ab}C_{dB}^{ab} - \frac{59}{6}\delta^{pr}g_Y^2g_L^2C_{dB}^{*ab}Y_d^{ab} + \Big\{2\delta^{pr}g_Y^2g_L^2Y_d^{*ab} + \frac{25}{4}\delta^{pr}g_L^4Y_d^{*ab} - g_L^2\Big(\frac{3}{2}\delta^{pr}(Y_d^\dagger Y_d Y_d^\dagger)^{ab} + \frac{3}{2}\delta^{pr}(Y_u^\dagger Y_u Y_d^\dagger)^{ab}\Big)\Big\}C_{dW}^{ab} \\
& + C_{dW}^{*ab}\Big\{2\delta^{pr}g_Y^2g_L^2Y_d^{ab} + \frac{25}{4}\delta^{pr}g_L^4Y_d^{ab} - g_L^2\Big(\frac{3}{2}\delta^{pr}(Y_d Y_d^\dagger Y_d)^{ab} + \frac{3}{2}\delta^{pr}(Y_u Y_u^\dagger Y_d)^{ab}\Big)\Big\} - \frac{32}{3}\delta^{pr}g_s^2g_L^2Y_d^{*ab}C_{dG}^{ab} - \frac{32}{3}\delta^{pr}g_s^2g_L^2C_{dG}^{*ab}Y_d^{ab} \\
& + \Big\{g_Y^2g_L^2\Big(\frac{29}{54}\delta^{pr}\delta^{ab} + \frac{347}{27}\delta^{pa}\delta^{rb}\Big) + g_L^2\Big(\frac{68}{9}\delta^{rb}(Y_e Y_e^\dagger)^{pa} + \frac{68}{9}\delta^{pa}(Y_e Y_e^\dagger)^{br} - \frac{11}{18}\delta^{pr}(Y_e Y_e^\dagger)^{ba}\Big) - \frac{1}{2}(Y_e Y_e^\dagger)^{pr}(Y_e Y_e^\dagger)^{ba} - g_Y^2\Big(\frac{11}{36}\delta^{rb}(Y_e Y_e^\dagger)^{pa} \\
& + \frac{11}{36}\delta^{pa}(Y_e Y_e^\dagger)^{br} + \frac{31}{18}\delta^{ab}(Y_e Y_e^\dagger)^{pr}\Big) - \lambda\Big(3\delta^{rb}(Y_e Y_e^\dagger)^{pa} + 3\delta^{pa}(Y_e Y_e^\dagger)^{br}\Big) - \frac{7}{2}T_2\delta^{rb}(Y_e Y_e^\dagger)^{pa} - \frac{7}{2}T_2\delta^{pa}(Y_e Y_e^\dagger)^{br} - \frac{25}{4}\delta^{rb}(Y_e Y_e^\dagger Y_e Y_e^\dagger)^{pa} \\
& - \frac{25}{4}\delta^{pa}(Y_e Y_e^\dagger Y_e Y_e^\dagger)^{br}\Big\}C_{H\ell}^{(||)ab} + \Big\{\frac{3}{4}\delta^{rb}(Y_e Y_e^\dagger Y_e Y_e^\dagger)^{pa} + \frac{3}{4}\delta^{pa}(Y_e Y_e^\dagger Y_e Y_e^\dagger)^{br} + g_Y^2g_L^2\Big(\frac{407}{108}\delta^{pr}\delta^{ab} + \frac{160}{27}\delta^{pa}\delta^{rb}\Big) + g_L^4\Big(\frac{173}{36}\delta^{pr}\delta^{ab} \\
& - \frac{245}{18}\delta^{pa}\delta^{rb}\Big) + g_Y^2\Big(\frac{31}{12}\delta^{pa}\delta^{rb}\text{Tr}[Y_u^\dagger Y_u] + \frac{19}{4}\delta^{pa}\delta^{rb}\text{Tr}[Y_e^\dagger Y_e] - \frac{31}{36}\delta^{ab}(Y_e Y_e^\dagger)^{pr} - \frac{29}{12}\delta^{pa}\delta^{rb}\text{Tr}[Y_d^\dagger Y_d] - \frac{517}{144}\delta^{rb}(Y_e Y_e^\dagger)^{pa} - \frac{517}{144}\delta^{pa}(Y_e Y_e^\dagger)^{br} \\
& + g_L^2\Big(\frac{67}{12}\delta^{pa}\delta^{rb}\text{Tr}[Y_e^\dagger Y_e] + \frac{2029}{144}\delta^{rb}(Y_e Y_e^\dagger)^{pa} + \frac{2029}{144}\delta^{pa}(Y_e Y_e^\dagger)^{br} + \frac{59}{4}\delta^{pa}\delta^{rb}\text{Tr}[Y_d^\dagger Y_d] + \frac{59}{4}\delta^{pa}\delta^{rb}\text{Tr}[Y_u^\dagger Y_u] - \frac{5}{12}\delta^{ab}(Y_e Y_e^\dagger)^{pr} \\
& - \frac{17}{9}\delta^{pr}(Y_e Y_e^\dagger)^{ba}\Big) + g_s^2\Big(40\delta^{pa}\delta^{rb}\text{Tr}[Y_d^\dagger Y_d] + 40\delta^{pa}\delta^{rb}\text{Tr}[Y_u^\dagger Y_u]\Big) - \frac{1}{2}(Y_e Y_e^\dagger)^{pr}(Y_e Y_e^\dagger)^{ba} - \lambda\Big(6\delta^{rb}(Y_e Y_e^\dagger)^{pa} + 6\delta^{pa}(Y_e Y_e^\dagger)^{br}\Big) - 3\delta^{pa}\delta^{rb}g_Y^4
\end{aligned}$$

$$\begin{aligned}
& -\frac{15}{4}\text{Tr}_2\delta^{rb}(Y_e Y_e^\dagger)^{pa} - \frac{15}{4}\text{Tr}_2\delta^{pa}(Y_e Y_e^\dagger)^{br} - 6\delta^{pa}\delta^{rb}\text{Tr}[Y_e^\dagger Y_e Y_e^\dagger Y_e] - 15\delta^{pa}\delta^{rb}\text{Tr}[Y_d^\dagger Y_d Y_d^\dagger Y_d] - 15\delta^{pa}\delta^{rb}\text{Tr}[Y_u^\dagger Y_u Y_u^\dagger Y_u] \Big\} C_{Hl}^{(\times)ab} \\
& + \left\{ \frac{1}{12}Y_e^{pa}(Y_e^\dagger Y_e Y_e^\dagger)^{rb} + \frac{1}{12}Y_e^{*rb}(Y_e Y_e^\dagger Y_e)^{pa} + \frac{1}{2}(Y_e^\dagger Y_e)^{ba}(Y_e Y_e^\dagger)^{pr} + \frac{29}{54}\delta^{pr}\delta^{ab}g_Y^2g_L^2 + g_L^2\left(\frac{5}{18}\delta^{pr}(Y_e^\dagger Y_e)^{ba} + \frac{3}{4}Y_e^{*rb}Y_e^{pa}\right) - g_Y^2\left(\frac{53}{36}Y_e^{*rb}Y_e^{pa} \right. \right. \\
& + \left. \frac{31}{18}\delta^{ab}(Y_e Y_e^\dagger)^{pr}\right) \Big\} C_{He}^{ab} + \left\{ g_L^2\left(\frac{11}{6}\delta^{pr}(Y_u Y_u^\dagger)^{ba} - \frac{11}{6}\delta^{pr}(Y_d Y_d^\dagger)^{ba}\right) + \frac{3}{2}(Y_e Y_e^\dagger)^{pr}(Y_u Y_u^\dagger)^{ba} + \frac{31}{18}\delta^{ab}g_Y^2(Y_e Y_e^\dagger)^{pr} - \frac{29}{54}\delta^{pr}\delta^{ab}g_Y^2g_L^2 \right. \\
& - \left. \frac{3}{2}(Y_d Y_d^\dagger)^{ba}(Y_e Y_e^\dagger)^{pr}\right) \Big\} C_{Hq}^{(\parallel)ab} + \left\{ \frac{31}{36}\delta^{ab}g_Y^2(Y_e Y_e^\dagger)^{pr} + \frac{3}{2}(Y_d Y_d^\dagger)^{ba}(Y_e Y_e^\dagger)^{pr} + 3(Y_e Y_e^\dagger)^{pr}(Y_u Y_u^\dagger)^{ba} + 8\delta^{pr}\delta^{ab}g_s^2g_L^2 + \frac{59}{4}\delta^{pr}\delta^{ab}g_L^4 \right. \\
& - \left. g_L^2\left(\frac{9}{4}\delta^{ab}(Y_e Y_e^\dagger)^{pr} + \frac{29}{6}\delta^{pr}(Y_u Y_u^\dagger)^{ba} + \frac{20}{3}\delta^{pr}(Y_d Y_d^\dagger)^{ba}\right) - \frac{335}{108}\delta^{pr}\delta^{ab}g_Y^2g_L^2 \right\} C_{Hq}^{(\times)ab} + \left\{ \frac{31}{9}\delta^{ab}g_Y^2(Y_e Y_e^\dagger)^{pr} - \frac{5}{6}\delta^{pr}g_L^2(Y_u^\dagger Y_u)^{ba} - \frac{29}{27}\delta^{pr}\delta^{ab}g_Y^2g_L^2 \right. \\
& - \left. \frac{3}{2}(Y_u^\dagger Y_u)^{ba}(Y_e Y_e^\dagger)^{pr}\right) \Big\} C_{Hu}^{ab} + \left\{ \frac{29}{54}\delta^{pr}\delta^{ab}g_Y^2g_L^2 + \frac{5}{6}\delta^{pr}g_L^2(Y_d^\dagger Y_d)^{ba} + \frac{3}{2}(Y_d^\dagger Y_d)^{ba}(Y_e Y_e^\dagger)^{pr} - \frac{31}{18}\delta^{ab}g_Y^2(Y_e Y_e^\dagger)^{pr} \right\} C_{Hd}^{ab} + \left\{ \frac{5}{6}\delta^{pr}g_L^2(Y_d^\dagger Y_u)^{ba} \right. \\
& + \left. \frac{3}{2}(Y_d^\dagger Y_u)^{ba}(Y_e Y_e^\dagger)^{pr}\right) \Big\} C_{Hud}^{ab} + C_{Hud}^{*ab} \left\{ \frac{5}{6}\delta^{pr}g_L^2(Y_u^\dagger Y_d)^{ab} + \frac{3}{2}(Y_u^\dagger Y_d)^{ab}(Y_e Y_e^\dagger)^{pr} \right\} + \left\{ \frac{2}{3}Y_e^{*rd}Y_e^{bc}(Y_e Y_e^\dagger)^{pa} + \frac{2}{3}Y_e^{*ad}Y_e^{pc}(Y_e Y_e^\dagger)^{br} \right. \\
& + g_L^2\left(6\delta^{pa}\delta^{rb}(Y_e^\dagger Y_e)^{dc} - \frac{19}{36}\delta^{pa}Y_e^{*rd}Y_e^{bc} - \frac{19}{36}\delta^{rb}Y_e^{*ad}Y_e^{pc}\right) + g_Y^2\left(\frac{13}{9}\delta^{rb}\delta^{cd}(Y_e Y_e^\dagger)^{pa} + \frac{13}{9}\delta^{pa}\delta^{cd}(Y_e Y_e^\dagger)^{br} + \frac{7}{4}\delta^{pa}Y_e^{*rd}Y_e^{bc} + \frac{7}{4}\delta^{rb}Y_e^{*ad}Y_e^{pc} \right. \\
& - \left. \frac{5}{9}\delta^{ab}Y_e^{*rd}Y_e^{pc}\right) - \frac{1}{2}\delta^{rb}Y_e^{pc}(Y_e^\dagger Y_e Y_e^\dagger)^{ad} - \frac{1}{2}\delta^{pa}Y_e^{*rd}(Y_e Y_e^\dagger Y_e)^{bc} - \delta^{rb}(Y_e^\dagger Y_e)^{dc}(Y_e Y_e^\dagger)^{pa} - \delta^{pa}(Y_e^\dagger Y_e)^{dc}(Y_e Y_e^\dagger)^{br} - Y_e^{*rd}Y_e^{pc}(Y_e Y_e^\dagger)^{ba} \\
& - \left. \frac{34}{27}\delta^{pa}\delta^{rb}\delta^{cd}g_Y^2g_L^2 \right\} C_{le}^{abcd} + \left\{ \frac{68}{27}\delta^{pa}\delta^{rb}\delta^{cd}g_Y^2g_L^2 + 3\delta^{rb}(Y_u^\dagger Y_u)^{dc}(Y_e Y_e^\dagger)^{pa} + 3\delta^{pa}(Y_u^\dagger Y_u)^{dc}(Y_e Y_e^\dagger)^{br} + 18\delta^{pa}\delta^{rb}g_L^2(Y_u^\dagger Y_u)^{dc} \right. \\
& - \left. g_Y^2\left(\frac{26}{9}\delta^{rb}\delta^{cd}(Y_e Y_e^\dagger)^{pa} + \frac{26}{9}\delta^{pa}\delta^{cd}(Y_e Y_e^\dagger)^{br}\right) \right\} C_{lu}^{abcd} + \left\{ g_Y^2\left(\frac{13}{9}\delta^{rb}\delta^{cd}(Y_e Y_e^\dagger)^{pa} + \frac{13}{9}\delta^{pa}\delta^{cd}(Y_e Y_e^\dagger)^{br}\right) + 18\delta^{pa}\delta^{rb}g_L^2(Y_d^\dagger Y_d)^{dc} - \frac{34}{27}\delta^{pa}\delta^{rb}\delta^{cd}g_Y^2g_L^2 \right. \\
& - \left. 3\delta^{rb}(Y_d^\dagger Y_d)^{dc}(Y_e Y_e^\dagger)^{pa} - 3\delta^{pa}(Y_d^\dagger Y_d)^{dc}(Y_e Y_e^\dagger)^{br}\right) \Big\} C_{ld}^{abcd} + \left\{ \frac{5}{9}\delta^{ab}g_Y^2Y_e^{*rd}Y_e^{pc} + 3Y_e^{*rd}Y_e^{pc}(Y_u Y_u^\dagger)^{ba} - 3Y_e^{*rd}Y_e^{pc}(Y_d Y_d^\dagger)^{ba} \right\} C_{qe}^{abcd} \\
& + \left\{ 4Y_e^{*rb}Y_e^{pa}(Y_e^\dagger Y_e)^{dc} - \frac{20}{9}\delta^{ad}g_Y^2Y_e^{*rb}Y_e^{pc} \right\} C_{ee}^{abcd} + \left\{ \frac{10}{9}\delta^{cd}g_Y^2Y_e^{*rb}Y_e^{pa} - 3Y_e^{*rb}Y_e^{pa}(Y_u^\dagger Y_u)^{dc} \right\} C_{eu}^{abcd} + \left\{ 3Y_e^{*rb}Y_e^{pa}(Y_d^\dagger Y_d)^{dc} \right. \\
& - \left. \frac{5}{9}\delta^{cd}g_Y^2Y_e^{*rb}Y_e^{pa} \right\} C_{ed}^{abcd} + \left\{ \frac{3}{4}\delta^{pa}Y_e^{*rb}(Y_d Y_d^\dagger Y_d)^{dc} + \frac{3}{4}\delta^{pa}Y_e^{*rb}(Y_u Y_u^\dagger Y_d)^{dc} + \frac{19}{24}\delta^{pa}g_L^2Y_e^{*rb}Y_d^{dc} - Y_e^{*rb}Y_d^{dc}(Y_e Y_e^\dagger)^{pa} - \frac{21}{8}\delta^{pa}g_Y^2Y_e^{*rb}Y_d^{dc} \right\} C_{ledq}^{abcd}
\end{aligned}$$

$$\begin{aligned}
& + C_{\ell edq}^{*abcd} \left\{ \frac{3}{4} \delta^{ra} Y_e^{pb} (Y_d^\dagger Y_d Y_d^\dagger)^{dc} + \frac{3}{4} \delta^{ra} Y_e^{pb} (Y_u^\dagger Y_u Y_d^\dagger)^{dc} + \frac{19}{24} \delta^{ra} g_L^2 Y_d^{*dc} Y_e^{pb} - Y_d^{*dc} Y_e^{pb} (Y_e Y_e^\dagger)^{ar} - \frac{21}{8} \delta^{ra} g_Y^2 Y_d^{*dc} Y_e^{pb} \right\} + \left\{ Y_e^{*rb} Y_u^{*cd} (Y_e Y_e^\dagger)^{pa} \right. \\
& + \frac{21}{8} \delta^{pa} g_Y^2 Y_e^{*rb} Y_u^{*cd} - \frac{3}{4} \delta^{pa} Y_e^{*rb} (Y_d^\dagger Y_d Y_u^\dagger)^{cd} - \frac{3}{4} \delta^{pa} Y_e^{*rb} (Y_u^\dagger Y_u Y_u^\dagger)^{cd} - \frac{19}{24} \delta^{pa} g_L^2 Y_e^{*rb} Y_u^{*cd} \left. \right\} C_{\ell equ}^{abcd} + C_{\ell equ}^{*abcd} \left\{ Y_e^{pb} Y_u^{cd} (Y_e Y_e^\dagger)^{ar} \right. \\
& + \frac{21}{8} \delta^{ra} g_Y^2 Y_e^{pb} Y_u^{cd} - \frac{3}{4} \delta^{ra} Y_e^{pb} (Y_d Y_d^\dagger Y_u)^{cd} - \frac{3}{4} \delta^{ra} Y_e^{pb} (Y_u Y_u^\dagger Y_u)^{cd} - \frac{19}{24} \delta^{ra} g_L^2 Y_e^{pb} Y_u^{cd} \left. \right\} + \left\{ \frac{3}{2} \delta^{pa} g_Y^2 Y_e^{*rd} Y_u^{*cb} + \frac{7}{3} \delta^{pa} g_L^2 Y_e^{*rd} Y_u^{*cb} \right. \\
& - \frac{1}{2} Y_e^{*rd} Y_u^{*cb} (Y_e Y_e^\dagger)^{pa} - \frac{3}{4} \delta^{pa} Y_e^{*rd} (Y_u^\dagger Y_u Y_u^\dagger)^{cb} - \frac{21}{4} \delta^{pa} Y_e^{*rd} (Y_d^\dagger Y_d Y_u^\dagger)^{cb} \left. \right\} C_{\ell uqe}^{abcd} + C_{\ell uqe}^{*abcd} \left\{ \frac{3}{2} \delta^{ra} g_Y^2 Y_e^{pd} Y_u^{cb} + \frac{7}{3} \delta^{ra} g_L^2 Y_e^{pd} Y_u^{cb} - \frac{1}{2} Y_e^{pd} Y_u^{cb} (Y_e Y_e^\dagger)^{ar} \right. \\
& - \frac{3}{4} \delta^{ra} Y_e^{pd} (Y_u Y_u^\dagger Y_u)^{cb} - \frac{21}{4} \delta^{ra} Y_e^{pd} (Y_d Y_d^\dagger Y_u)^{cb} \left. \right\} + \left\{ g_L^4 \left( \frac{4}{9} \delta^{pr} \delta^{ad} \delta^{bc} + \frac{128}{9} \delta^{pa} \delta^{rd} \delta^{bc} - \frac{14}{3} \delta^{pa} \delta^{rb} \delta^{cd} \right) + g_Y^2 \left( \frac{26}{9} \delta^{rb} \delta^{cd} (Y_e Y_e^\dagger)^{pa} \right. \right. \\
& + \frac{26}{9} \delta^{pa} \delta^{cd} (Y_e Y_e^\dagger)^{br} - \frac{2}{9} \delta^{rd} \delta^{bc} (Y_e Y_e^\dagger)^{pa} - \frac{2}{9} \delta^{pa} \delta^{bc} (Y_e Y_e^\dagger)^{dr} - \frac{3}{2} \delta^{pa} \delta^{rd} (Y_e Y_e^\dagger)^{bc} \left. \right) + g_L^2 \left( \frac{4}{3} \delta^{pa} \delta^{rd} \delta^{bc} \text{Tr} [Y_e^\dagger Y_e] + 22 \delta^{pa} \delta^{rb} (Y_e Y_e^\dagger)^{dc} \right. \\
& - \frac{2}{3} \delta^{rd} \delta^{bc} (Y_e Y_e^\dagger)^{pa} - \frac{2}{3} \delta^{pa} \delta^{bc} (Y_e Y_e^\dagger)^{dr} - \frac{4}{3} \delta^{pr} \delta^{bc} (Y_e Y_e^\dagger)^{da} - \frac{67}{6} \delta^{pa} \delta^{rd} (Y_e Y_e^\dagger)^{bc} \left. \right) + 2 \delta^{rb} (Y_e Y_e^\dagger)^{pa} (Y_e Y_e^\dagger)^{dc} + 2 \delta^{pa} (Y_e Y_e^\dagger)^{br} (Y_e Y_e^\dagger)^{dc} \\
& + 18 \delta^{pa} \delta^{rd} (Y_e Y_e^\dagger Y_e Y_e^\dagger)^{bc} - g_Y^2 g_L^2 \left( \frac{58}{27} \delta^{pa} \delta^{rd} \delta^{bc} + \frac{68}{27} \delta^{pa} \delta^{rb} \delta^{cd} \right) - 2 \delta^{rd} (Y_e Y_e^\dagger)^{pa} (Y_e Y_e^\dagger)^{bc} - 2 \delta^{pa} (Y_e Y_e^\dagger)^{bc} (Y_e Y_e^\dagger)^{dr} \left. \right\} C_{\ell \ell}^{abcd} + \left\{ \frac{8}{3} \delta^{pr} \delta^{ad} \delta^{bc} g_L^4 \right. \\
& - g_L^2 \left( 8 \delta^{pr} \delta^{bc} (Y_d Y_d^\dagger)^{da} + 8 \delta^{pr} \delta^{bc} (Y_u Y_u^\dagger)^{da} \right) \left. \right\} C_{qq}^{(\parallel)abcd} + \left\{ g_L^2 \left( 15 \delta^{pa} \delta^{rb} (Y_d Y_d^\dagger)^{dc} + 15 \delta^{pa} \delta^{rb} (Y_u Y_u^\dagger)^{dc} \right) + \frac{34}{27} \delta^{pa} \delta^{rb} \delta^{cd} g_Y^2 g_L^2 + 3 \delta^{rb} (Y_d Y_d^\dagger)^{dc} (Y_e Y_e^\dagger)^{pa} \right. \\
& + 3 \delta^{pa} (Y_d Y_d^\dagger)^{dc} (Y_e Y_e^\dagger)^{br} - \delta^{pa} \delta^{rb} \delta^{cd} g_L^4 - g_Y^2 \left( \frac{13}{9} \delta^{rb} \delta^{cd} (Y_e Y_e^\dagger)^{pa} + \frac{13}{9} \delta^{pa} \delta^{cd} (Y_e Y_e^\dagger)^{br} \right) - 3 \delta^{rb} (Y_e Y_e^\dagger)^{pa} (Y_u Y_u^\dagger)^{dc} - 3 \delta^{pa} (Y_e Y_e^\dagger)^{br} (Y_u Y_u^\dagger)^{dc} \left. \right\} C_{\ell q}^{(\parallel)abcd} \\
& + \left\{ \frac{26}{27} \delta^{pa} \delta^{rb} \delta^{cd} g_Y^2 g_L^2 + g_L^4 \left( \frac{31}{3} \delta^{pa} \delta^{rb} \delta^{cd} - \frac{2}{3} \delta^{pr} \delta^{ab} \delta^{cd} \right) + g_Y^2 \left( \frac{71}{12} \delta^{pa} \delta^{rb} (Y_d Y_d^\dagger)^{dc} - \frac{13}{18} \delta^{rb} \delta^{cd} (Y_e Y_e^\dagger)^{pa} - \frac{13}{18} \delta^{pa} \delta^{cd} (Y_e Y_e^\dagger)^{br} \right. \right. \\
& - \frac{205}{12} \delta^{pa} \delta^{rb} (Y_u Y_u^\dagger)^{dc} \left. \right) + g_L^2 \left( 2 \delta^{pr} \delta^{cd} (Y_e Y_e^\dagger)^{ba} + 2 \delta^{pa} \delta^{rb} \delta^{cd} \text{Tr} [Y_e^\dagger Y_e] - \frac{5}{2} \delta^{rb} \delta^{cd} (Y_e Y_e^\dagger)^{pa} - \frac{5}{2} \delta^{pa} \delta^{cd} (Y_e Y_e^\dagger)^{br} - \frac{41}{4} \delta^{pa} \delta^{rb} (Y_d Y_d^\dagger)^{dc} \right. \\
& - \frac{41}{4} \delta^{pa} \delta^{rb} (Y_u Y_u^\dagger)^{dc} \left. \right) + 3 \delta^{rb} (Y_d Y_d^\dagger)^{dc} (Y_e Y_e^\dagger)^{pa} + 3 \delta^{pa} (Y_d Y_d^\dagger)^{dc} (Y_e Y_e^\dagger)^{br} + 8 \delta^{pa} \delta^{rb} \delta^{cd} g_s^2 g_L^2 + 15 \delta^{pa} \delta^{rb} (Y_d Y_d^\dagger Y_d Y_d^\dagger)^{dc} + 15 \delta^{pa} \delta^{rb} (Y_u Y_u^\dagger Y_u Y_u^\dagger)^{dc} \\
& \left. - g_s^2 \left( 40 \delta^{pa} \delta^{rb} (Y_d Y_d^\dagger)^{dc} + 40 \delta^{pa} \delta^{rb} (Y_u Y_u^\dagger)^{dc} \right) \right\} C_{\ell q}^{(\times)abcd}, \tag{9.4}
\end{aligned}$$

### 9.3 $C_{He}$

$$\begin{aligned}
\beta_{C_{He}^{pr}}^{(1)} = & \left\{ \frac{1}{2} (Y_e^\dagger Y_e)^{pr} - \frac{1}{6} \delta^{pr} g_Y^2 \right\} C_{HD}^{(\parallel)} + \left\{ (Y_e^\dagger Y_e)^{pr} - \frac{1}{3} \delta^{pr} g_Y^2 \right\} C_{HD}^{(\times)} + \left\{ \frac{4}{3} \delta^{pr} \delta^{ab} g_Y^2 - 2 Y_e^{*ap} Y_e^{br} \right\} C_{H\ell}^{(\parallel)ab} + \left\{ \frac{2}{3} \delta^{pr} \delta^{ab} g_Y^2 - Y_e^{*ap} Y_e^{br} \right\} C_{H\ell}^{(\times)ab} \\
& + \left\{ \frac{1}{3} g_Y^2 (\delta^{pa} \delta^{rb} + 4 \delta^{pr} \delta^{ab}) + 2 (T_2 \delta^{pa} \delta^{rb} + 2 \delta^{rb} (Y_e^\dagger Y_e)^{pa} + 2 \delta^{pa} (Y_e^\dagger Y_e)^{br}) \right\} C_{He}^{ab} - \frac{4}{3} \delta^{pr} \delta^{ab} g_Y^2 C_{Hq}^{(\parallel)ab} - \frac{2}{3} \delta^{pr} \delta^{ab} g_Y^2 C_{Hq}^{(\times)ab} - \frac{8}{3} \delta^{pr} \delta^{ab} g_Y^2 C_{Hu}^{ab} \\
& + \frac{4}{3} \delta^{pr} \delta^{ab} g_Y^2 C_{Hd}^{ab} - \left\{ \frac{2}{3} \delta^{pc} \delta^{rd} \delta^{ab} g_Y^2 + 2 \delta^{pc} \delta^{rd} (Y_e Y_e^\dagger)^{ba} \right\} C_{\ell e}^{abcd} + \left\{ \frac{2}{3} \delta^{pc} \delta^{rd} \delta^{ab} g_Y^2 - 6 (\delta^{pc} \delta^{rd} (Y_d Y_d^\dagger)^{ba} - \delta^{pc} \delta^{rd} (Y_u Y_u^\dagger)^{ba}) \right\} C_{qe}^{abcd} \\
& + \left\{ 8 \delta^{pa} \delta^{rb} (Y_e^\dagger Y_e)^{dc} - \frac{8}{3} \delta^{pa} \delta^{rb} \delta^{cd} g_Y^2 \right\} C_{ee}^{abcd} + \left\{ \frac{4}{3} \delta^{pa} \delta^{rb} \delta^{cd} g_Y^2 - 6 \delta^{pa} \delta^{rb} (Y_u^\dagger Y_u)^{dc} \right\} C_{eu}^{abcd} + \left\{ 6 \delta^{pa} \delta^{rb} (Y_d^\dagger Y_d)^{dc} - \frac{2}{3} \delta^{pa} \delta^{rb} \delta^{cd} g_Y^2 \right\} C_{ed}^{abcd}, \tag{9.5}
\end{aligned}$$

$$\begin{aligned}
\beta_{C_{He}^{pr}}^{(2)} = & \frac{19}{3} \delta^{pr} g_Y^2 T_{\ell H} - 3 (Y_e^\dagger Y_e)^{pr} T_{\ell H} - 5 (Y_e^\dagger C_{\ell HH}^\dagger C_{\ell HH} Y_e)^{pr} + \left\{ g_Y^2 \left( \frac{1}{6} T_2 \delta^{pr} + \frac{485}{144} (Y_e^\dagger Y_e)^{pr} \right) + \frac{137}{48} g_L^2 (Y_e^\dagger Y_e)^{pr} - \frac{7}{36} \delta^{pr} g_Y^2 g_L^2 \right. \\
& - \frac{1}{2} T_2 (Y_e^\dagger Y_e)^{pr} - \frac{5}{6} \delta^{pr} \lambda g_Y^2 - \frac{40}{27} \delta^{pr} g_Y^4 - 4 (Y_e^\dagger Y_e Y_e^\dagger Y_e)^{pr} \left. \right\} C_{HD}^{(\parallel)} + \left\{ g_Y^2 \left( \frac{1}{3} T_2 \delta^{pr} - \frac{7}{18} (Y_e^\dagger Y_e)^{pr} \right) + 9 g_L^2 (Y_e^\dagger Y_e)^{pr} - \frac{5}{6} \delta^{pr} \lambda g_Y^2 \right. \\
& - \frac{181}{216} \delta^{pr} g_Y^4 - T_2 (Y_e^\dagger Y_e)^{pr} - 5 (Y_e^\dagger Y_e Y_e^\dagger Y_e)^{pr} - \frac{41}{8} \delta^{pr} g_Y^2 g_L^2 \left. \right\} C_{HD}^{(\times)} + \left\{ 12 \delta^{pr} \lambda g_Y^4 - 3 \delta^{pr} g_Y^4 g_L^2 - 11 g_Y^4 (Y_e^\dagger Y_e)^{pr} - 15 \delta^{pr} g_Y^6 \right\} C_{HB} \\
& - 2 \delta^{pr} g_Y^2 g_L^4 C_{HW} + \left\{ 3 \delta^{pr} \lambda g_Y^2 g_L^2 + \frac{15}{4} g_Y^2 g_L^2 (Y_e^\dagger Y_e)^{pr} + \frac{27}{4} \delta^{pr} g_Y^2 g_L^4 - \frac{11}{4} \delta^{pr} g_Y^4 g_L^2 \right\} C_{HWB} + \left\{ 3 g_L^6 (Y_e^\dagger Y_e)^{pr} - 4 \delta^{pr} g_Y^2 g_L^6 \right\} C_W \\
& + \left\{ \frac{9}{4} \delta^{rb} g_L^2 Y_e^{*ap} - \frac{3}{2} \delta^{rb} \lambda Y_e^{*ap} - \frac{3}{2} \delta^{rb} (Y_e^\dagger Y_e Y_e^\dagger)^{ap} - \frac{9}{4} \delta^{rb} g_Y^2 Y_e^{*ap} \right\} C_{eH}^{ab} + C_{eH}^{*ab} \left\{ \frac{9}{4} \delta^{pb} g_L^2 Y_e^{ar} - \frac{3}{2} \delta^{pb} \lambda Y_e^{ar} - \frac{3}{2} \delta^{pb} (Y_e Y_e^\dagger Y_e)^{ar} \right. \\
& - \frac{9}{4} \delta^{pb} g_Y^2 Y_e^{ar} \left. \right\} + \left\{ g_Y^2 g_L^2 \left( 3 \delta^{pr} Y_e^{*ab} - \frac{33}{8} \delta^{rb} Y_e^{*ap} \right) + g_Y^4 \left( \frac{27}{2} \delta^{pr} Y_e^{*ab} + \frac{155}{8} \delta^{rb} Y_e^{*ap} \right) - g_Y^2 \left( \delta^{pr} (Y_e^\dagger Y_e Y_e^\dagger)^{ab} + \frac{3}{2} T_2 \delta^{rb} Y_e^{*ap} + 10 Y_e^{*ap} (Y_e^\dagger Y_e)^{br} \right) \right. \\
& - 9 \delta^{rb} \lambda g_Y^2 Y_e^{*ap} \left. \right\} C_{eB}^{ab} + C_{eB}^{*ab} \left\{ g_Y^2 g_L^2 \left( 3 \delta^{pr} Y_e^{ab} - \frac{33}{8} \delta^{pb} Y_e^{ar} \right) + g_Y^4 \left( \frac{27}{2} \delta^{pr} Y_e^{ab} + \frac{155}{8} \delta^{pb} Y_e^{ar} \right) - g_Y^2 \left( \delta^{pr} (Y_e Y_e^\dagger Y_e)^{ab} + \frac{3}{2} T_2 \delta^{pb} Y_e^{ar} \right. \right. \\
& + 10 Y_e^{ar} (Y_e^\dagger Y_e)^{pb} \left. \right) - 9 \delta^{pb} \lambda g_Y^2 Y_e^{ar} \left. \right\} + \left\{ g_Y^2 g_L^2 \left( \frac{79}{16} \delta^{rb} Y_e^{*ap} - \frac{5}{4} \delta^{pr} Y_e^{*ab} \right) + g_L^2 \left( \frac{9}{2} \delta^{rb} (Y_e^\dagger Y_e Y_e^\dagger)^{ap} - \frac{9}{4} T_2 \delta^{rb} Y_e^{*ap} \right) - \frac{69}{16} \delta^{rb} g_L^4 Y_e^{*ap} \right. \\
& - \frac{9}{2} \delta^{rb} \lambda g_L^2 Y_e^{*ap} \left. \right\} C_{eW}^{ab} + C_{eW}^{*ab} \left\{ g_Y^2 g_L^2 \left( \frac{79}{16} \delta^{pb} Y_e^{ar} - \frac{5}{4} \delta^{pr} Y_e^{ab} \right) + g_L^2 \left( \frac{9}{2} \delta^{pb} (Y_e Y_e^\dagger Y_e)^{ar} - \frac{9}{4} T_2 \delta^{pb} Y_e^{ar} \right) - \frac{69}{16} \delta^{pb} g_L^4 Y_e^{ar} - \frac{9}{2} \delta^{pb} \lambda g_L^2 Y_e^{ar} \right\}
\end{aligned}$$

$$\begin{aligned}
& + \left\{ g_Y^2 \left( 3\delta^{pr} (Y_d^\dagger Y_d Y_u^\dagger)^{ab} + 3\delta^{pr} (Y_u^\dagger Y_u Y_u^\dagger)^{ab} \right) + \frac{75}{2} \delta^{pr} g_Y^4 Y_u^{*ab} - 9\delta^{pr} g_Y^2 g_L^2 Y_u^{*ab} \right\} C_{uB}^{ab} + C_{uB}^{*ab} \left\{ g_Y^2 \left( 3\delta^{pr} (Y_d Y_d^\dagger Y_u)^{ab} + 3\delta^{pr} (Y_u Y_u^\dagger Y_u)^{ab} \right) \right. \\
& + \frac{75}{2} \delta^{pr} g_Y^4 Y_u^{ab} - 9\delta^{pr} g_Y^2 g_L^2 Y_u^{ab} \left. \right\} - \frac{3}{4} \delta^{pr} g_Y^2 g_L^2 Y_u^{*ab} C_{uW}^{ab} - \frac{3}{4} \delta^{pr} g_Y^2 g_L^2 C_{uW}^{*ab} Y_u^{ab} + \frac{32}{3} \delta^{pr} g_Y^2 g_s^2 Y_u^{*ab} C_{uG}^{ab} + \frac{32}{3} \delta^{pr} g_Y^2 g_s^2 C_{uG}^{*ab} Y_u^{ab} \\
& + \left\{ \frac{9}{2} \delta^{pr} g_Y^4 Y_d^{*ab} + 9\delta^{pr} g_Y^2 g_L^2 Y_d^{*ab} - g_Y^2 \left( 3\delta^{pr} (Y_d^\dagger Y_d Y_d^\dagger)^{ab} + 3\delta^{pr} (Y_u^\dagger Y_u Y_d^\dagger)^{ab} \right) \right\} C_{dB}^{ab} + C_{dB}^{*ab} \left\{ \frac{9}{2} \delta^{pr} g_Y^4 Y_d^{ab} + 9\delta^{pr} g_Y^2 g_L^2 Y_d^{ab} \right. \\
& - g_Y^2 \left( 3\delta^{pr} (Y_d Y_d^\dagger Y_d)^{ab} + 3\delta^{pr} (Y_u Y_u^\dagger Y_d)^{ab} \right) \left. \right\} + \frac{9}{4} \delta^{pr} g_Y^2 g_L^2 Y_d^{*ab} C_{dW}^{ab} + \frac{9}{4} \delta^{pr} g_Y^2 g_L^2 C_{dW}^{*ab} Y_d^{ab} + \frac{32}{3} \delta^{pr} g_Y^2 g_s^2 Y_d^{*ab} C_{dG}^{ab} + \frac{32}{3} \delta^{pr} g_Y^2 g_s^2 C_{dG}^{*ab} Y_d^{ab} \\
& + \left\{ g_Y^2 \left( \frac{11}{18} Y_e^{*ap} Y_e^{br} - \frac{49}{18} \delta^{pr} (Y_e Y_e^\dagger)^{ba} - \frac{59}{18} \delta^{ab} (Y_e^\dagger Y_e)^{pr} \right) + 3T_2 Y_e^{*ap} Y_e^{br} + 3\delta^{pr} \delta^{ab} g_Y^2 g_L^2 + \frac{47}{12} Y_e^{br} (Y_e^\dagger Y_e Y_e^\dagger)^{ap} + \frac{47}{12} Y_e^{*ap} (Y_e Y_e^\dagger Y_e)^{br} \right. \\
& - \frac{1}{2} (Y_e^\dagger Y_e)^{pr} (Y_e Y_e^\dagger)^{ba} - \frac{299}{54} \delta^{pr} \delta^{ab} g_Y^4 - 12g_L^2 Y_e^{*ap} Y_e^{br} \left. \right\} C_{H\ell}^{(\parallel)ab} + \left\{ \frac{1}{2} (Y_e^\dagger Y_e)^{pr} (Y_e Y_e^\dagger)^{ba} + \frac{3}{2} T_2 Y_e^{*ap} Y_e^{br} + \frac{83}{36} \delta^{pr} \delta^{ab} g_Y^2 g_L^2 + \frac{29}{6} Y_e^{br} (Y_e^\dagger Y_e Y_e^\dagger)^{ap} \right. \\
& + \frac{29}{6} Y_e^{*ap} (Y_e Y_e^\dagger Y_e)^{br} - g_L^2 \left( \frac{1}{12} \delta^{ab} (Y_e^\dagger Y_e)^{pr} + \frac{151}{24} Y_e^{*ap} Y_e^{br} \right) - g_Y^2 \left( \frac{13}{9} \delta^{pr} (Y_e Y_e^\dagger)^{ba} + \frac{59}{36} \delta^{ab} (Y_e^\dagger Y_e)^{pr} + \frac{167}{72} Y_e^{*ap} Y_e^{br} \right) - \frac{299}{108} \delta^{pr} \delta^{ab} g_Y^4 \left. \right\} C_{H\ell}^{(\times)ab} \\
& + \left\{ g_Y^4 \left( \frac{829}{54} \delta^{pr} \delta^{ab} - \frac{346}{27} \delta^{pa} \delta^{rb} \right) + g_L^2 \left( \frac{93}{8} \delta^{rb} (Y_e^\dagger Y_e)^{pa} + \frac{93}{8} \delta^{pa} (Y_e^\dagger Y_e)^{br} - \frac{3}{4} T_2 \delta^{pa} \delta^{rb} \right) + g_Y^2 \left( \frac{19}{12} \delta^{pa} \delta^{rb} \text{Tr}[Y_u^\dagger Y_u] + \frac{61}{12} \delta^{pa} \delta^{rb} \text{Tr}[Y_e^\dagger Y_e] \right. \right. \\
& + \frac{721}{72} \delta^{rb} (Y_e^\dagger Y_e)^{pa} + \frac{721}{72} \delta^{pa} (Y_e^\dagger Y_e)^{br} - \frac{53}{18} \delta^{ab} (Y_e^\dagger Y_e)^{pr} - \frac{41}{12} \delta^{pa} \delta^{rb} \text{Tr}[Y_d^\dagger Y_d] - \frac{71}{18} \delta^{pr} (Y_e^\dagger Y_e)^{ba} \left. \right) + g_s^2 \left( 40\delta^{pa} \delta^{rb} \text{Tr}[Y_d^\dagger Y_d] + 40\delta^{pa} \delta^{rb} \text{Tr}[Y_u^\dagger Y_u] \right) \\
& + 3\delta^{pa} \delta^{rb} g_Y^2 g_L^2 + 6\delta^{pa} \delta^{rb} \text{Tr}[Y_d^\dagger Y_d Y_u^\dagger Y_u] - \frac{1}{2} (Y_e^\dagger Y_e)^{pr} (Y_e^\dagger Y_e)^{ba} - \lambda \left( 9\delta^{rb} (Y_e^\dagger Y_e)^{pa} + 9\delta^{pa} (Y_e^\dagger Y_e)^{br} \right) - \frac{9}{2} (Y_e^\dagger Y_e)^{pa} (Y_e^\dagger Y_e)^{br} - 5T_2 \delta^{rb} (Y_e^\dagger Y_e)^{pa} \\
& - 5T_2 \delta^{pa} (Y_e^\dagger Y_e)^{br} - \frac{27}{4} \delta^{rb} (Y_e^\dagger Y_e Y_e^\dagger Y_e)^{pa} - \frac{27}{4} \delta^{pa} (Y_e^\dagger Y_e Y_e^\dagger Y_e)^{br} - 7\delta^{pa} \delta^{rb} \text{Tr}[Y_e^\dagger Y_e Y_e^\dagger Y_e] - 18\delta^{pa} \delta^{rb} \text{Tr}[Y_d^\dagger Y_d Y_d^\dagger Y_d] \\
& - 18\delta^{pa} \delta^{rb} \text{Tr}[Y_u^\dagger Y_u Y_u^\dagger Y_u] \left. \right\} C_{He}^{ab} + \left\{ g_Y^2 \left( \frac{7}{6} \delta^{pr} (Y_d Y_d^\dagger)^{ba} + \frac{59}{18} \delta^{ab} (Y_e^\dagger Y_e)^{pr} + \frac{7}{2} \delta^{pr} (Y_u Y_u^\dagger)^{ba} \right) + \frac{3}{2} (Y_e^\dagger Y_e)^{pr} (Y_u Y_u^\dagger)^{ba} - \frac{3}{2} (Y_e^\dagger Y_e)^{pr} (Y_d Y_d^\dagger)^{ba} \right. \\
& - \frac{85}{54} \delta^{pr} \delta^{ab} g_Y^4 - 3\delta^{pr} \delta^{ab} g_Y^2 g_L^2 - \frac{16}{3} \delta^{pr} \delta^{ab} g_Y^2 g_s^2 \left. \right\} C_{Hq}^{(\parallel)ab} + \left\{ \frac{11}{12} \delta^{pr} \delta^{ab} g_Y^2 g_L^2 + g_Y^2 \left( \frac{59}{36} \delta^{ab} (Y_e^\dagger Y_e)^{pr} + \frac{7}{3} \delta^{pr} (Y_d Y_d^\dagger)^{ba} + \frac{5}{2} \delta^{pr} (Y_u Y_u^\dagger)^{ba} \right) \right. \\
& + \frac{3}{2} (Y_e^\dagger Y_e)^{pr} (Y_d Y_d^\dagger)^{ba} + 3(Y_e^\dagger Y_e)^{pr} (Y_u Y_u^\dagger)^{ba} - \frac{1}{4} \delta^{ab} g_L^2 (Y_e^\dagger Y_e)^{pr} - \frac{85}{108} \delta^{pr} \delta^{ab} g_Y^4 - \frac{8}{3} \delta^{pr} \delta^{ab} g_Y^2 g_s^2 \left. \right\} C_{Hq}^{(\times)ab} + \left\{ g_Y^2 \left( \frac{59}{9} \delta^{ab} (Y_e^\dagger Y_e)^{pr} + \frac{49}{6} \delta^{pr} (Y_u^\dagger Y_u)^{ba} \right) \right. \\
& + \frac{365}{27} \delta^{pr} \delta^{ab} g_Y^4 - \frac{3}{2} (Y_e^\dagger Y_e)^{pr} (Y_u^\dagger Y_u)^{ba} - \frac{32}{3} \delta^{pr} \delta^{ab} g_Y^2 g_s^2 \left. \right\} C_{Hu}^{ab} + \left\{ \frac{3}{2} (Y_d^\dagger Y_d)^{ba} (Y_e^\dagger Y_e)^{pr} + \frac{211}{54} \delta^{pr} \delta^{ab} g_Y^4 + \frac{16}{3} \delta^{pr} \delta^{ab} g_Y^2 g_s^2 - g_Y^2 \left( \frac{59}{18} \delta^{ab} (Y_e^\dagger Y_e)^{pr} \right. \right.
\end{aligned}$$



$$\begin{aligned}
& + \frac{7}{2} \delta^{pr} (Y_d^\dagger Y_d)^{ba} \Big) \Big\} C_{Hd}^{ab} + \left\{ \frac{3}{2} (Y_d^\dagger Y_u)^{ba} (Y_e^\dagger Y_e)^{pr} - \frac{17}{6} \delta^{pr} g_Y^2 (Y_d^\dagger Y_u)^{ba} \right\} C_{Hud}^{ab} + C_{Hud}^{*ab} \left\{ \frac{3}{2} (Y_e^\dagger Y_e)^{pr} (Y_u^\dagger Y_d)^{ab} - \frac{17}{6} \delta^{pr} g_Y^2 (Y_u^\dagger Y_d)^{ab} \right\} \\
& + \left\{ g_Y^4 \left( \frac{2}{9} \delta^{pr} \delta^{ab} \delta^{cd} + \frac{319}{54} \delta^{pc} \delta^{rd} \delta^{ab} \right) + \delta^{rd} (Y_e^\dagger Y_e)^{pc} (Y_e Y_e^\dagger)^{ba} + \delta^{pc} (Y_e^\dagger Y_e)^{dr} (Y_e Y_e^\dagger)^{ba} + g_L^2 \left( \frac{3}{4} \delta^{pc} \delta^{rd} (Y_e Y_e^\dagger)^{ba} - \frac{3}{4} \delta^{pc} Y_e^{*ad} Y_e^{br} - \frac{3}{4} \delta^{rd} Y_e^{*ap} Y_e^{bc} \right) \right. \\
& + \delta^{rd} Y_e^{bc} (Y_e^\dagger Y_e Y_e^\dagger)^{ap} + \delta^{pc} Y_e^{*ad} (Y_e Y_e^\dagger Y_e)^{br} + g_Y^2 \left( \frac{4}{9} \delta^{cd} Y_e^{*ap} Y_e^{br} + \frac{119}{36} \delta^{pc} Y_e^{*ad} Y_e^{br} + \frac{119}{36} \delta^{rd} Y_e^{*ap} Y_e^{bc} - \frac{2}{9} \delta^{rd} \delta^{ab} (Y_e^\dagger Y_e)^{pc} - \frac{2}{9} \delta^{pc} \delta^{ab} (Y_e^\dagger Y_e)^{dr} \right. \\
& - \frac{2}{3} \delta^{pr} \delta^{ab} (Y_e^\dagger Y_e)^{dc} - \frac{2}{3} \delta^{pc} \delta^{rd} \delta^{ab} \text{Tr}[Y_e^\dagger Y_e] - \frac{35}{4} \delta^{pc} \delta^{rd} (Y_e Y_e^\dagger)^{ba} \Big) + \frac{3}{2} \delta^{pc} Y_e^{br} (Y_e^\dagger Y_e Y_e^\dagger)^{ad} + \frac{3}{2} \delta^{rd} Y_e^{*ap} (Y_e Y_e^\dagger Y_e)^{bc} + 2 Y_e^{*ap} Y_e^{br} (Y_e^\dagger Y_e)^{dc} \\
& + 7 \delta^{pc} \delta^{rd} (Y_e Y_e^\dagger Y_e Y_e^\dagger)^{ba} - \frac{1}{3} Y_e^{*ad} Y_e^{br} (Y_e^\dagger Y_e)^{pc} - \frac{1}{3} Y_e^{*ap} Y_e^{bc} (Y_e^\dagger Y_e)^{dr} - \frac{3}{2} \delta^{pc} \delta^{rd} \delta^{ab} g_Y^2 g_L^2 \Big\} C_{\ell e}^{abcd} - \left\{ \frac{14}{9} \delta^{cd} g_Y^2 Y_e^{*ap} Y_e^{br} + 3 Y_e^{*ap} Y_e^{br} (Y_u^\dagger Y_u)^{dc} \right\} C_{\ell u}^{abcd} \\
& + \left\{ \frac{7}{9} \delta^{cd} g_Y^2 Y_e^{*ap} Y_e^{br} + 3 Y_e^{*ap} Y_e^{br} (Y_d^\dagger Y_d)^{dc} \right\} C_{\ell d}^{abcd} + \left\{ g_L^2 \left( \frac{9}{4} \delta^{pc} \delta^{rd} (Y_d Y_d^\dagger)^{ba} - \frac{9}{4} \delta^{pc} \delta^{rd} (Y_u Y_u^\dagger)^{ba} \right) + g_s^2 \left( 40 \delta^{pc} \delta^{rd} (Y_u Y_u^\dagger)^{ba} - 40 \delta^{pc} \delta^{rd} (Y_d Y_d^\dagger)^{ba} \right) \right. \\
& + g_Y^2 \left( \frac{2}{9} \delta^{rd} \delta^{ab} (Y_e^\dagger Y_e)^{pc} + \frac{2}{9} \delta^{pc} \delta^{ab} (Y_e^\dagger Y_e)^{dr} + \frac{2}{3} \delta^{pr} \delta^{ab} (Y_e^\dagger Y_e)^{dc} + \frac{2}{3} \delta^{pc} \delta^{rd} \delta^{ab} \text{Tr}[Y_e^\dagger Y_e] - \frac{197}{12} \delta^{pc} \delta^{rd} (Y_u Y_u^\dagger)^{ba} - \frac{199}{12} \delta^{pc} \delta^{rd} (Y_d Y_d^\dagger)^{ba} \right) \\
& + \frac{3}{2} \delta^{pc} \delta^{rd} \delta^{ab} g_Y^2 g_L^2 + \frac{8}{3} \delta^{pc} \delta^{rd} \delta^{ab} g_Y^2 g_s^2 + 3 \delta^{rd} (Y_e^\dagger Y_e)^{pc} (Y_d Y_d^\dagger)^{ba} + 3 \delta^{pc} (Y_e^\dagger Y_e)^{dr} (Y_d Y_d^\dagger)^{ba} + 18 \delta^{pc} \delta^{rd} (Y_d Y_d^\dagger Y_d Y_d^\dagger)^{ba} - g_Y^4 \left( \frac{2}{9} \delta^{pr} \delta^{ab} \delta^{cd} \right. \\
& + \frac{79}{54} \delta^{pc} \delta^{rd} \delta^{ab} \Big) - 3 \delta^{rd} (Y_e^\dagger Y_e)^{pc} (Y_u Y_u^\dagger)^{ba} - 3 \delta^{pc} (Y_e^\dagger Y_e)^{dr} (Y_u Y_u^\dagger)^{ba} - 18 \delta^{pc} \delta^{rd} (Y_u Y_u^\dagger Y_u Y_u^\dagger)^{ba} \Big\} C_{qe}^{abcd} + \left\{ g_Y^4 \left( \frac{320}{27} \delta^{pa} \delta^{rb} \delta^{cd} - \frac{8}{9} \delta^{pr} \delta^{ab} \delta^{cd} \right) \right. \\
& + g_Y^2 \left( \frac{8}{3} \delta^{pr} \delta^{ad} (Y_e^\dagger Y_e)^{bc} - \frac{2}{9} \delta^{rb} \delta^{ad} (Y_e^\dagger Y_e)^{pc} - \frac{2}{9} \delta^{pa} \delta^{cd} (Y_e^\dagger Y_e)^{br} - \frac{8}{3} \delta^{pa} \delta^{rb} \delta^{cd} \text{Tr}[Y_e^\dagger Y_e] - \frac{134}{3} \delta^{pa} \delta^{rb} (Y_e^\dagger Y_e)^{dc} \right) + 2 \delta^{rb} (Y_e^\dagger Y_e)^{pa} (Y_e^\dagger Y_e)^{dc} \\
& + 2 \delta^{pa} (Y_e^\dagger Y_e)^{br} (Y_e^\dagger Y_e)^{dc} + 6 \delta^{pa} \delta^{rb} g_L^2 (Y_e^\dagger Y_e)^{dc} - 32 \delta^{pa} \delta^{rb} (Y_e^\dagger Y_e Y_e^\dagger Y_e)^{dc} \Big\} C_{ee}^{abcd} + \left\{ \frac{32}{3} \delta^{pr} \delta^{ad} g_Y^2 (Y_u^\dagger Y_u)^{bc} - \frac{64}{27} \delta^{pr} \delta^{ad} \delta^{bc} g_Y^4 \right\} C_{uu}^{abcd} \\
& + \left\{ \frac{16}{3} \delta^{pr} \delta^{ad} g_Y^2 (Y_d^\dagger Y_d)^{bc} - \frac{16}{27} \delta^{pr} \delta^{ad} \delta^{bc} g_Y^4 \right\} C_{dd}^{abcd} + \left\{ g_Y^2 \left( \frac{4}{9} \delta^{rb} \delta^{cd} (Y_e^\dagger Y_e)^{pa} + \frac{4}{9} \delta^{pa} \delta^{cd} (Y_e^\dagger Y_e)^{br} + \frac{4}{3} \delta^{pr} \delta^{cd} (Y_e^\dagger Y_e)^{ba} + \frac{4}{3} \delta^{pa} \delta^{rb} \delta^{cd} \text{Tr}[Y_e^\dagger Y_e] \right. \right. \\
& - \frac{379}{12} \delta^{pa} \delta^{rb} (Y_u^\dagger Y_u)^{dc} \Big) + \frac{9}{4} \delta^{pa} \delta^{rb} g_L^2 (Y_u^\dagger Y_u)^{dc} + 3 \delta^{rb} (Y_e^\dagger Y_e)^{pa} (Y_u^\dagger Y_u)^{dc} + 3 \delta^{pa} (Y_e^\dagger Y_e)^{br} (Y_u^\dagger Y_u)^{dc} + \frac{16}{3} \delta^{pa} \delta^{rb} \delta^{cd} g_Y^2 g_s^2 + 18 \delta^{pa} \delta^{rb} (Y_u^\dagger Y_u Y_u^\dagger Y_u)^{dc} \\
& - g_Y^4 \left( \frac{4}{9} \delta^{pr} \delta^{ab} \delta^{cd} + \frac{76}{27} \delta^{pa} \delta^{rb} \delta^{cd} \right) - 3 \delta^{pa} \delta^{rb} (Y_u^\dagger Y_d Y_d^\dagger Y_u)^{dc} - 40 \delta^{pa} \delta^{rb} g_s^2 (Y_u^\dagger Y_u)^{dc} \Big\} C_{eu}^{abcd} + \left\{ g_Y^4 \left( \frac{2}{9} \delta^{pr} \delta^{ab} \delta^{cd} + \frac{74}{27} \delta^{pa} \delta^{rb} \delta^{cd} \right) \right. \\
& + 3 \delta^{pa} \delta^{rb} (Y_d^\dagger Y_u Y_u^\dagger Y_d)^{dc} + 40 \delta^{pa} \delta^{rb} g_s^2 (Y_d^\dagger Y_d)^{dc} - g_Y^2 \left( \frac{2}{9} \delta^{rb} \delta^{cd} (Y_e^\dagger Y_e)^{pa} + \frac{2}{9} \delta^{pa} \delta^{cd} (Y_e^\dagger Y_e)^{br} + \frac{2}{3} \delta^{pr} \delta^{cd} (Y_e^\dagger Y_e)^{ba} + \frac{2}{3} \delta^{pa} \delta^{rb} \delta^{cd} \text{Tr}[Y_e^\dagger Y_e] \right. \\
& + \frac{65}{12} \delta^{pa} \delta^{rb} (Y_d^\dagger Y_d)^{dc} \Big) - \frac{9}{4} \delta^{pa} \delta^{rb} g_L^2 (Y_d^\dagger Y_d)^{dc} - \frac{8}{3} \delta^{pa} \delta^{rb} \delta^{cd} g_Y^2 g_s^2 - 3 \delta^{rb} (Y_d^\dagger Y_d)^{dc} (Y_e^\dagger Y_e)^{pa} - 3 \delta^{pa} (Y_d^\dagger Y_d)^{dc} (Y_e^\dagger Y_e)^{br}
\end{aligned}$$

$$\begin{aligned}
& -18\delta^{pa}\delta^{rb}(Y_d^\dagger Y_d Y_d^\dagger Y_d)^{dc} \Big\} C_{ed}^{abcd} + \left\{ \frac{1}{2} Y_e^{*ap} Y_d^{dc} (Y_e^\dagger Y_e)^{br} + \frac{3}{4} \delta^{rb} Y_e^{*ap} (Y_u Y_u^\dagger Y_d)^{dc} + \frac{9}{8} \delta^{rb} g_L^2 Y_e^{*ap} Y_d^{dc} - \frac{9}{4} \delta^{rb} Y_e^{*ap} (Y_d Y_d^\dagger Y_d)^{dc} \right. \\
& - 3\delta^{rb} Y_d^{dc} (Y_e^\dagger Y_e Y_e^\dagger)^{ap} - \frac{107}{24} \delta^{rb} g_Y^2 Y_e^{*ap} Y_d^{dc} \Big\} C_{ledq}^{abcd} + C_{ledq}^{*abcd} \left\{ \frac{1}{2} Y_d^{*dc} Y_e^{ar} (Y_e^\dagger Y_e)^{pb} + \frac{3}{4} \delta^{pb} Y_e^{ar} (Y_u^\dagger Y_u Y_d^\dagger)^{dc} + \frac{9}{8} \delta^{pb} g_L^2 Y_d^{*dc} Y_e^{ar} \right. \\
& - \frac{9}{4} \delta^{pb} Y_e^{ar} (Y_d^\dagger Y_d Y_d^\dagger)^{dc} - 3\delta^{pb} Y_d^{*dc} (Y_e Y_e^\dagger Y_e)^{ar} - \frac{107}{24} \delta^{pb} g_Y^2 Y_d^{*dc} Y_e^{ar} \Big\} + \left\{ \frac{9}{4} \delta^{rb} Y_e^{*ap} (Y_u^\dagger Y_u Y_u^\dagger)^{cd} + 3\delta^{rb} Y_u^{*cd} (Y_e^\dagger Y_e Y_e^\dagger)^{ap} + \frac{107}{24} \delta^{rb} g_Y^2 Y_e^{*ap} Y_u^{*cd} \right. \\
& - \frac{1}{2} Y_e^{*ap} Y_u^{*cd} (Y_e^\dagger Y_e)^{br} - \frac{3}{4} \delta^{rb} Y_e^{*ap} (Y_d^\dagger Y_d Y_u^\dagger)^{cd} - \frac{9}{8} \delta^{rb} g_L^2 Y_e^{*ap} Y_u^{*cd} \Big\} C_{lequ}^{abcd} + C_{lequ}^{*abcd} \left\{ \frac{9}{4} \delta^{pb} Y_e^{ar} (Y_u Y_u^\dagger Y_u)^{cd} + 3\delta^{pb} Y_u^{cd} (Y_e Y_e^\dagger Y_e)^{ar} \right. \\
& + \frac{107}{24} \delta^{pb} g_Y^2 Y_e^{ar} Y_u^{cd} - \frac{1}{2} Y_e^{ar} Y_u^{cd} (Y_e^\dagger Y_e)^{pb} - \frac{3}{4} \delta^{pb} Y_e^{ar} (Y_d Y_d^\dagger Y_u)^{cd} - \frac{9}{8} \delta^{pb} g_L^2 Y_e^{ar} Y_u^{cd} \Big\} + \left\{ \frac{1}{4} Y_e^{*ap} Y_u^{*cb} (Y_e^\dagger Y_e)^{dr} + \frac{3}{2} \delta^{rd} Y_e^{*ap} (Y_u^\dagger Y_u Y_u^\dagger)^{cb} \right. \\
& + \frac{9}{2} \delta^{rd} Y_e^{*ap} (Y_d^\dagger Y_d Y_u^\dagger)^{cb} - \frac{3}{2} \delta^{rd} Y_u^{*cb} (Y_e^\dagger Y_e Y_e^\dagger)^{ap} - \frac{43}{6} \delta^{rd} g_Y^2 Y_e^{*ap} Y_u^{*cb} \Big\} C_{luqe}^{abcd} + C_{luqe}^{*abcd} \left\{ \frac{1}{4} Y_e^{ar} Y_u^{cb} (Y_e^\dagger Y_e)^{pd} + \frac{3}{2} \delta^{pd} Y_e^{ar} (Y_u Y_u^\dagger Y_u)^{cb} \right. \\
& + \frac{9}{2} \delta^{pd} Y_e^{ar} (Y_d Y_d^\dagger Y_u)^{cb} - \frac{3}{2} \delta^{pd} Y_u^{cb} (Y_e Y_e^\dagger Y_e)^{ar} - \frac{43}{6} \delta^{pd} g_Y^2 Y_e^{ar} Y_u^{cb} \Big\} + \left\{ \frac{1}{3} \delta^{bc} g_L^2 Y_e^{*ap} Y_e^{dr} + g_Y^2 \left( \frac{14}{9} \delta^{cd} Y_e^{*ap} Y_e^{br} + \frac{19}{9} \delta^{bc} Y_e^{*ap} Y_e^{dr} - \frac{8}{3} \delta^{pr} \delta^{bc} (Y_e Y_e^\dagger)^{da} \right) \right. \\
& - \frac{8}{9} \delta^{pr} \delta^{ad} \delta^{bc} g_Y^4 - 2Y_e^{*ap} Y_e^{br} (Y_e Y_e^\dagger)^{dc} \Big\} C_{\ell\ell}^{abcd} + \left\{ g_Y^2 \left( \frac{8}{3} \delta^{pr} \delta^{bc} (Y_d Y_d^\dagger)^{da} - \frac{8}{3} \delta^{pr} \delta^{bc} (Y_u Y_u^\dagger)^{da} \right) - \frac{8}{27} \delta^{pr} \delta^{ad} \delta^{bc} g_Y^4 \right\} C_{qq}^{(\parallel)abcd} + \left\{ g_Y^2 \left( \frac{16}{3} \delta^{pr} \delta^{bc} (Y_d Y_d^\dagger)^{da} \right. \right. \\
& - \frac{16}{3} \delta^{pr} \delta^{bc} (Y_u Y_u^\dagger)^{da} \Big) - \frac{16}{27} \delta^{pr} \delta^{ad} \delta^{bc} g_Y^4 \Big\} C_{qq}^{(\times)abcd} + \left\{ 3Y_e^{*ap} Y_e^{br} (Y_u Y_u^\dagger)^{dc} - \frac{7}{9} \delta^{cd} g_Y^2 Y_e^{*ap} Y_e^{br} - 3Y_e^{*ap} Y_e^{br} (Y_d Y_d^\dagger)^{dc} \right\} C_{\ell q}^{(\parallel)abcd} + \left\{ \frac{1}{2} \delta^{cd} g_L^2 Y_e^{*ap} Y_e^{br} \right. \\
& - \frac{7}{18} \delta^{cd} g_Y^2 Y_e^{*ap} Y_e^{br} - 3Y_e^{*ap} Y_e^{br} (Y_u Y_u^\dagger)^{dc} - 6Y_e^{*ap} Y_e^{br} (Y_d Y_d^\dagger)^{dc} \Big\} C_{\ell q}^{(\times)abcd}, \tag{9.6}
\end{aligned}$$

#### 9.4 $C_{Hq}^{(\parallel)}$

$$\begin{aligned}
\beta_{C_{Hq}^{(\parallel)pr}}^{(1)} &= \left\{ \frac{1}{36} \delta^{pr} g_Y^2 + \frac{1}{2} (Y_u Y_u^\dagger)^{pr} - \frac{1}{12} \delta^{pr} g_L^2 \right\} C_{HD}^{(\parallel)} + \left\{ \frac{1}{18} \delta^{pr} g_Y^2 + \frac{1}{2} ((Y_u Y_u^\dagger)^{pr} - (Y_d Y_d^\dagger)^{pr}) \right\} C_{HD}^{(\times)} - \frac{2}{9} \delta^{pr} \delta^{ab} g_Y^2 C_{H\ell}^{(\parallel)ab} - \left\{ \frac{1}{9} \delta^{pr} \delta^{ab} g_Y^2 \right. \\
& + \frac{1}{3} \delta^{pr} \delta^{ab} g_L^2 \Big\} C_{H\ell}^{(\times)ab} - \frac{2}{9} \delta^{pr} \delta^{ab} g_Y^2 C_{He}^{ab} + \left\{ \frac{1}{9} g_Y^2 (2\delta^{pr} \delta^{ab} + 3\delta^{pa} \delta^{rb}) + \frac{1}{2} (\delta^{rb} (Y_d Y_d^\dagger)^{pa} + \delta^{pa} (Y_d Y_d^\dagger)^{br} + 4T_2 \delta^{pa} \delta^{rb} + 7\delta^{rb} (Y_u Y_u^\dagger)^{pa} \right. \\
& + 7\delta^{pa} (Y_u Y_u^\dagger)^{br}) \Big\} C_{Hq}^{(\parallel)ab} + \left\{ \frac{1}{18} g_Y^2 (2\delta^{pr} \delta^{ab} + 3\delta^{pa} \delta^{rb}) + \frac{1}{6} g_L^2 (17\delta^{pa} \delta^{rb} - 6\delta^{pr} \delta^{ab}) + 2\delta^{rb} (Y_d Y_d^\dagger)^{pa} + 2\delta^{pa} (Y_d Y_d^\dagger)^{br} - \delta^{rb} (Y_u Y_u^\dagger)^{pa} \right.
\end{aligned}$$

$$\begin{aligned}
& -\delta^{pa}(Y_u Y_u^\dagger)^{br} \left\{ C_{Hq}^{(\times)ab} + \left\{ \frac{4}{9} \delta^{pr} \delta^{ab} g_Y^2 - Y_u^{*rb} Y_u^{pa} \right\} C_{Hu}^{ab} - \left\{ \frac{2}{9} \delta^{pr} \delta^{ab} g_Y^2 + Y_d^{*rb} Y_d^{pa} \right\} C_{Hd}^{ab} + \left\{ 2\delta^{pa} \delta^{rb} (Y_e^\dagger Y_e)^{dc} - \frac{2}{3} \delta^{pa} \delta^{rb} \delta^{cd} g_Y^2 \right\} C_{qe}^{abcd} \right. \\
& + \left\{ \frac{4}{3} \delta^{pa} \delta^{rb} \delta^{cd} g_Y^2 - 6\delta^{pa} \delta^{rb} (Y_u^\dagger Y_u)^{dc} \right\} C_{qu}^{(\parallel)abcd} + \left\{ \frac{4}{9} \delta^{pa} \delta^{rb} \delta^{cd} g_Y^2 - 2\delta^{pa} \delta^{rb} (Y_u^\dagger Y_u)^{dc} \right\} C_{qu}^{(\times)abcd} + \left\{ 6\delta^{pa} \delta^{rb} (Y_d^\dagger Y_d)^{dc} - \frac{2}{3} \delta^{pa} \delta^{rb} \delta^{cd} g_Y^2 \right\} C_{qd}^{(\parallel)abcd} \\
& + \left\{ 2\delta^{pa} \delta^{rb} (Y_d^\dagger Y_d)^{dc} - \frac{2}{9} \delta^{pa} \delta^{rb} \delta^{cd} g_Y^2 \right\} C_{qd}^{(\times)abcd} + \left\{ \frac{2}{9} g_Y^2 (\delta^{pa} \delta^{rd} \delta^{bc} + 6\delta^{pa} \delta^{rb} \delta^{cd}) - \frac{2}{3} \delta^{pa} \delta^{rd} \delta^{bc} g_L^2 - 4(3\delta^{pa} \delta^{rb} (Y_d Y_d^\dagger)^{dc} - \delta^{pa} \delta^{rd} (Y_u Y_u^\dagger)^{bc} \right. \\
& \left. - 3\delta^{pa} \delta^{rb} (Y_u Y_u^\dagger)^{dc}) \right\} C_{qq}^{(\parallel)abcd} + \left\{ \frac{2}{9} g_Y^2 (2\delta^{pa} \delta^{rd} \delta^{bc} + 3\delta^{pa} \delta^{rb} \delta^{cd}) - 2\delta^{pa} \delta^{rb} \delta^{cd} g_L^2 - 4(\delta^{pa} \delta^{rd} (Y_d Y_d^\dagger)^{bc} - \delta^{pa} \delta^{rd} (Y_u Y_u^\dagger)^{bc} - 3\delta^{pa} \delta^{rb} (Y_u Y_u^\dagger)^{dc}) \right\} C_{qq}^{(\times)abcd} \\
& \left. - \left\{ \frac{2}{3} \delta^{pc} \delta^{rd} \delta^{ab} g_Y^2 + 2\delta^{pc} \delta^{rd} (Y_e Y_e^\dagger)^{ba} \right\} C_{\ell q}^{(\parallel)abcd} - \left\{ \frac{1}{3} \delta^{pc} \delta^{rd} \delta^{ab} g_L^2 + \frac{1}{3} \delta^{pc} \delta^{rd} \delta^{ab} g_Y^2 \right\} C_{\ell q}^{(\times)abcd} \right\}, \tag{9.7}
\end{aligned}$$

$$\begin{aligned}
\beta_{C_{Hq}^{(\parallel)pr}}^{(2)} &= (Y_d Y_d^\dagger)^{pr} \mathbf{T}_{\ell H} + \frac{11}{6} \delta^{pr} g_L^2 \mathbf{T}_{\ell H} - \frac{19}{18} \delta^{pr} g_Y^2 \mathbf{T}_{\ell H} - 2(Y_u Y_u^\dagger)^{pr} \mathbf{T}_{\ell H} + \left\{ \frac{20}{81} \delta^{pr} g_Y^4 + \lambda \left( \frac{5}{36} \delta^{pr} g_Y^2 - \frac{5}{12} \delta^{pr} g_L^2 \right) + g_Y^2 \left( \frac{227}{144} (Y_u Y_u^\dagger)^{pr} - \frac{1}{36} \mathbf{T}_2 \delta^{pr} \right. \right. \\
& - \frac{9}{8} (Y_d Y_d^\dagger)^{pr} \left. \right) + g_L^2 \left( \frac{1}{12} \mathbf{T}_2 \delta^{pr} + \frac{7}{6} (Y_d Y_d^\dagger)^{pr} + \frac{97}{48} (Y_u Y_u^\dagger)^{pr} \right) + \frac{15}{8} (Y_d Y_d^\dagger Y_d Y_d^\dagger)^{pr} - \frac{3}{8} \delta^{pr} g_L^4 - \frac{3}{8} (Y_d Y_d^\dagger Y_u Y_u^\dagger)^{pr} - \frac{3}{8} (Y_u Y_u^\dagger Y_d Y_d^\dagger)^{pr} \\
& - \frac{1}{2} \mathbf{T}_2 (Y_u Y_u^\dagger)^{pr} - \frac{8}{3} g_s^2 (Y_u Y_u^\dagger)^{pr} - \frac{25}{8} (Y_u Y_u^\dagger Y_u Y_u^\dagger)^{pr} \left\} C_{HD}^{(\parallel)} + \left\{ \frac{181}{1296} \delta^{pr} g_Y^4 + \frac{1}{2} \mathbf{T}_2 (Y_d Y_d^\dagger)^{pr} + \frac{251}{432} \delta^{pr} g_Y^2 g_L^2 + \frac{5}{8} (Y_d Y_d^\dagger Y_u Y_u^\dagger)^{pr} \right. \\
& + \frac{5}{8} (Y_u Y_u^\dagger Y_d Y_d^\dagger)^{pr} + g_s^2 \left( \frac{8}{3} (Y_d Y_d^\dagger)^{pr} - \frac{8}{3} (Y_u Y_u^\dagger)^{pr} \right) + \lambda \left( \frac{5}{36} \delta^{pr} g_Y^2 - \frac{1}{4} (Y_d Y_d^\dagger)^{pr} - \frac{1}{4} (Y_u Y_u^\dagger)^{pr} \right) + g_Y^2 \left( \frac{11}{8} (Y_u Y_u^\dagger)^{pr} - \frac{1}{18} \mathbf{T}_2 \delta^{pr} - \frac{53}{72} (Y_d Y_d^\dagger)^{pr} \right) \\
& + g_L^2 \left( \frac{9}{2} (Y_u Y_u^\dagger)^{pr} - \frac{9}{2} (Y_d Y_d^\dagger)^{pr} \right) + \frac{9}{4} (Y_d Y_d^\dagger Y_d Y_d^\dagger)^{pr} - \frac{1}{2} \mathbf{T}_2 (Y_u Y_u^\dagger)^{pr} - 4(Y_u Y_u^\dagger Y_u Y_u^\dagger)^{pr} \left\} C_{HD}^{(\times)} + \left\{ \frac{5}{9} \delta^{pr} g_Y^6 - g_Y^4 \left( \frac{5}{6} (Y_d Y_d^\dagger)^{pr} + \frac{19}{18} (Y_u Y_u^\dagger)^{pr} \right) \right. \\
& - 2\delta^{pr} \lambda g_Y^4 \left\} C_{HB} + \left\{ g_L^4 \left( \frac{9}{2} (Y_d Y_d^\dagger)^{pr} - \frac{9}{2} (Y_u Y_u^\dagger)^{pr} \right) + \frac{4}{3} \delta^{pr} g_Y^2 g_L^4 + 6\delta^{pr} \lambda g_L^4 - \frac{71}{3} \delta^{pr} g_L^6 \right\} C_{HW} + \left\{ \frac{8}{3} \delta^{pr} g_Y^2 g_s^4 - 8\delta^{pr} g_s^4 g_L^2 \right. \\
& - \frac{80}{3} g_s^4 (Y_u Y_u^\dagger)^{pr} \left\} C_{HG} + \left\{ \frac{1}{12} \delta^{pr} g_Y^2 g_L^4 + \frac{1}{4} \delta^{pr} g_Y^4 g_L^2 + g_Y^2 g_L^2 \left( \frac{35}{12} (Y_u Y_u^\dagger)^{pr} - \frac{2}{3} (Y_d Y_d^\dagger)^{pr} \right) \right\} C_{HWB} + \left\{ \frac{5}{6} \delta^{pr} g_Y^2 g_L^6 + g_L^6 \left( 3\mathbf{T}_2 \delta^{pr} + \frac{45}{2} (Y_d Y_d^\dagger)^{pr} \right. \right. \\
& - \frac{69}{2} (Y_u Y_u^\dagger)^{pr} \left. \right) + \frac{20}{3} \delta^{pr} g_L^8 \left\} C_W + \left\{ \frac{40}{9} \delta^{pr} g_Y^2 g_s^6 + 8g_s^6 (Y_u Y_u^\dagger)^{pr} - \frac{40}{3} \delta^{pr} g_s^6 g_L^2 \right\} C_G + \left\{ 2\delta^{pa} g_Y^2 Y_u^{*rb} - \frac{3}{4} \delta^{pa} (Y_d^\dagger Y_d Y_u^\dagger)^{rb} - \frac{3}{4} \delta^{pa} (Y_u^\dagger Y_u Y_u^\dagger)^{rb} \right. \\
& \left. - \frac{3}{2} \delta^{pa} \lambda Y_u^{*rb} \right\} C_{uH}^{ab} + C_{uH}^{*ab} \left\{ 2\delta^{ra} g_Y^2 Y_u^{pb} - \frac{3}{4} \delta^{ra} (Y_d Y_d^\dagger Y_u)^{pb} - \frac{3}{4} \delta^{ra} (Y_u Y_u^\dagger Y_u)^{pb} - \frac{3}{2} \delta^{ra} \lambda Y_u^{pb} \right\} + \left\{ \frac{3}{4} \delta^{pa} (Y_d^\dagger Y_d Y_d^\dagger)^{rb} - \frac{1}{2} \delta^{pa} g_Y^2 Y_d^{*rb} \right.
\end{aligned}$$

$$\begin{aligned}
& -\frac{3}{4}\delta^{pa}(Y_u^\dagger Y_u Y_d^\dagger)^{rb} \Big\} C_{dH}^{ab} + C_{dH}^{*ab} \Big\{ \frac{3}{4}\delta^{ra}(Y_d Y_d^\dagger Y_d)^{pb} - \frac{1}{2}\delta^{ra}g_Y^2 Y_d^{pb} - \frac{3}{4}\delta^{ra}(Y_u Y_u^\dagger Y_d)^{pb} \Big\} + \Big\{ \frac{1}{6}\delta^{pr}g_Y^2(Y_e^\dagger Y_e Y_e^\dagger)^{ab} + \frac{1}{4}\delta^{pr}g_Y^4 Y_e^{*ab} \\
& -\frac{7}{4}\delta^{pr}g_Y^2 g_L^2 Y_e^{*ab} \Big\} C_{eB}^{ab} + C_{eB}^{*ab} \Big\{ \frac{1}{6}\delta^{pr}g_Y^2(Y_e Y_e^\dagger Y_e)^{ab} + \frac{1}{4}\delta^{pr}g_Y^4 Y_e^{ab} - \frac{7}{4}\delta^{pr}g_Y^2 g_L^2 Y_e^{ab} \Big\} + \Big\{ \frac{5}{24}\delta^{pr}g_Y^2 g_L^2 Y_e^{*ab} + \frac{1}{4}\delta^{pr}g_L^2(Y_e^\dagger Y_e Y_e^\dagger)^{ab} \\
& +\frac{29}{24}\delta^{pr}g_L^4 Y_e^{*ab} \Big\} C_{eW}^{ab} + C_{eW}^{*ab} \Big\{ \frac{5}{24}\delta^{pr}g_Y^2 g_L^2 Y_e^{ab} + \frac{1}{4}\delta^{pr}g_L^2(Y_e Y_e^\dagger Y_e)^{ab} + \frac{29}{24}\delta^{pr}g_L^4 Y_e^{ab} \Big\} + \Big\{ g_Y^2 g_L^2 \Big( \frac{11}{12}\delta^{pr}Y_u^{*ab} + \frac{329}{72}\delta^{pa}Y_u^{*rb} \Big) \\
& +g_Y^4 \Big( \frac{685}{72}\delta^{pa}Y_u^{*rb} - \frac{25}{12}\delta^{pr}Y_u^{*ab} \Big) + g_Y^2 \Big( \frac{1}{2}Y_u^{*rb}(Y_u Y_u^\dagger)^{pa} + \frac{2}{3}Y_u^{*rb}(Y_d Y_d^\dagger)^{pa} + \frac{25}{12}\delta^{pa}(Y_u^\dagger Y_u Y_u^\dagger)^{rb} + \frac{9}{4}\delta^{pa}(Y_d^\dagger Y_d Y_u^\dagger)^{rb} - \frac{1}{2}\delta^{pr}(Y_d^\dagger Y_d Y_u^\dagger)^{ab} \\
& -\frac{1}{2}\delta^{pr}(Y_u^\dagger Y_u Y_u^\dagger)^{ab} - \frac{3}{2}T_2\delta^{pa}Y_u^{*rb} \Big) - 6\delta^{pa}\lambda g_Y^2 Y_u^{*rb} - \frac{104}{9}\delta^{pa}g_Y^2 g_s^2 Y_u^{*rb} \Big\} C_{uB}^{ab} + C_{uB}^{*ab} \Big\{ g_Y^2 g_L^2 \Big( \frac{11}{12}\delta^{pr}Y_u^{ab} + \frac{329}{72}\delta^{ra}Y_u^{pb} \Big) + g_Y^4 \Big( \frac{685}{72}\delta^{ra}Y_u^{pb} \\
& -\frac{25}{12}\delta^{pr}Y_u^{ab} \Big) + g_Y^2 \Big( \frac{1}{2}Y_u^{pb}(Y_u Y_u^\dagger)^{ar} + \frac{2}{3}Y_u^{pb}(Y_d Y_d^\dagger)^{ar} + \frac{25}{12}\delta^{ra}(Y_u Y_u^\dagger Y_u)^{pb} + \frac{9}{4}\delta^{ra}(Y_d Y_d^\dagger Y_u)^{pb} - \frac{1}{2}\delta^{pr}(Y_d Y_d^\dagger Y_u)^{ab} - \frac{1}{2}\delta^{pr}(Y_u Y_u^\dagger Y_u)^{ab} - \frac{3}{2}T_2\delta^{ra}Y_u^{pb} \Big) \\
& -6\delta^{ra}\lambda g_Y^2 Y_u^{pb} - \frac{104}{9}\delta^{ra}g_Y^2 g_s^2 Y_u^{pb} \Big\} + \Big\{ g_L^4 \Big( \frac{153}{16}\delta^{pa}Y_u^{*rb} - \frac{79}{8}\delta^{pr}Y_u^{*ab} \Big) + g_L^2 \Big( \frac{3}{4}T_2\delta^{pa}Y_u^{*rb} + \frac{3}{4}\delta^{pr}(Y_d^\dagger Y_d Y_u^\dagger)^{ab} + \frac{3}{4}\delta^{pr}(Y_u^\dagger Y_u Y_u^\dagger)^{ab} \\
& +\frac{15}{8}\delta^{pa}(Y_d^\dagger Y_d Y_u^\dagger)^{rb} + \frac{9}{4}Y_u^{*rb}(Y_u Y_u^\dagger)^{pa} + \frac{5}{2}Y_u^{*rb}(Y_d Y_d^\dagger)^{pa} - \frac{3}{8}\delta^{pa}(Y_u^\dagger Y_u Y_u^\dagger)^{rb} \Big) + \frac{9}{2}\delta^{pa}\lambda g_L^2 Y_u^{*rb} - g_Y^2 g_L^2 \Big( \frac{83}{144}\delta^{pa}Y_u^{*rb} + \frac{19}{8}\delta^{pr}Y_u^{*ab} \Big) \\
& -\frac{20}{3}\delta^{pa}g_s^2 g_L^2 Y_u^{*rb} \Big\} C_{uW}^{ab} + C_{uW}^{*ab} \Big\{ g_L^4 \Big( \frac{153}{16}\delta^{ra}Y_u^{pb} - \frac{79}{8}\delta^{pr}Y_u^{ab} \Big) + g_L^2 \Big( \frac{3}{4}T_2\delta^{ra}Y_u^{pb} + \frac{3}{4}\delta^{pr}(Y_d Y_d^\dagger Y_u)^{ab} + \frac{3}{4}\delta^{pr}(Y_u Y_u^\dagger Y_u)^{ab} + \frac{15}{8}\delta^{ra}(Y_d Y_d^\dagger Y_u)^{pb} \\
& +\frac{9}{4}Y_u^{pb}(Y_u Y_u^\dagger)^{ar} + \frac{5}{2}Y_u^{pb}(Y_d Y_d^\dagger)^{ar} - \frac{3}{8}\delta^{ra}(Y_u Y_u^\dagger Y_u)^{pb} \Big) + \frac{9}{2}\delta^{ra}\lambda g_L^2 Y_u^{pb} - g_Y^2 g_L^2 \Big( \frac{83}{144}\delta^{ra}Y_u^{pb} + \frac{19}{8}\delta^{pr}Y_u^{ab} \Big) - \frac{20}{3}\delta^{ra}g_s^2 g_L^2 Y_u^{pb} \Big\} \\
& + \Big\{ g_s^2 g_L^2 \Big( \frac{20}{9}\delta^{pa}Y_u^{*rb} + \frac{16}{3}\delta^{pr}Y_u^{*ab} \Big) + g_s^4 \Big( \frac{320}{9}\delta^{pa}Y_u^{*rb} - 16\delta^{pr}Y_u^{*ab} \Big) + g_s^2 \Big( \frac{20}{3}\delta^{pa}(Y_u^\dagger Y_u Y_u^\dagger)^{rb} + 12Y_u^{*rb}(Y_u Y_u^\dagger)^{pa} - \frac{8}{3}Y_u^{*rb}(Y_d Y_d^\dagger)^{pa} \\
& -g_Y^2 g_s^2 \Big( \frac{4}{9}\delta^{pa}Y_u^{*rb} + \frac{16}{9}\delta^{pr}Y_u^{*ab} \Big) \Big\} C_{uG}^{ab} + C_{uG}^{*ab} \Big\{ g_s^2 g_L^2 \Big( \frac{20}{9}\delta^{ra}Y_u^{pb} + \frac{16}{3}\delta^{pr}Y_u^{ab} \Big) + g_s^4 \Big( \frac{320}{9}\delta^{ra}Y_u^{pb} - 16\delta^{pr}Y_u^{ab} \Big) + g_s^2 \Big( \frac{20}{3}\delta^{ra}(Y_u Y_u^\dagger Y_u)^{pb} \\
& +12Y_u^{pb}(Y_u Y_u^\dagger)^{ar} - \frac{8}{3}Y_u^{pb}(Y_d Y_d^\dagger)^{ar} \Big) - g_Y^2 g_s^2 \Big( \frac{4}{9}\delta^{ra}Y_u^{pb} + \frac{16}{9}\delta^{pr}Y_u^{ab} \Big) \Big\} + \Big\{ g_Y^4 \Big( \frac{1}{12}\delta^{pr}Y_d^{*ab} - \frac{1}{108}\delta^{pa}Y_d^{*rb} \Big) + g_Y^2 g_L^2 \Big( \frac{121}{36}\delta^{pa}Y_d^{*rb} - \frac{31}{12}\delta^{pr}Y_d^{*ab} \Big) \\
& +g_Y^2 \Big( \frac{1}{2}\delta^{pr}(Y_d^\dagger Y_d Y_d^\dagger)^{ab} + \frac{1}{2}\delta^{pr}(Y_u^\dagger Y_u Y_d^\dagger)^{ab} + \frac{3}{4}\delta^{pa}(Y_u^\dagger Y_u Y_d^\dagger)^{rb} + \frac{7}{6}Y_d^{*rb}(Y_u Y_u^\dagger)^{pa} + \frac{9}{4}\delta^{pa}(Y_d^\dagger Y_d Y_d^\dagger)^{rb} - \frac{5}{2}Y_d^{*rb}(Y_d Y_d^\dagger)^{pa} \Big) - \frac{8}{3}\delta^{pa}g_Y^2 g_s^2 Y_d^{*rb} \\
& -3\delta^{pa}\lambda g_Y^2 Y_d^{*rb} \Big\} C_{dB}^{ab} + C_{dB}^{*ab} \Big\{ g_Y^4 \Big( \frac{1}{12}\delta^{pr}Y_d^{ab} - \frac{1}{108}\delta^{ra}Y_d^{pb} \Big) + g_Y^2 g_L^2 \Big( \frac{121}{36}\delta^{ra}Y_d^{pb} - \frac{31}{12}\delta^{pr}Y_d^{ab} \Big) + g_Y^2 \Big( \frac{1}{2}\delta^{pr}(Y_d Y_d^\dagger Y_d)^{ab} + \frac{1}{2}\delta^{pr}(Y_u Y_u^\dagger Y_d)^{ab}
\end{aligned}$$

$$\begin{aligned}
& + \frac{3}{4} \delta^{ra} (Y_u Y_u^\dagger Y_d)^{pb} + \frac{7}{6} Y_d^{pb} (Y_u Y_u^\dagger)^{ar} + \frac{9}{4} \delta^{ra} (Y_d Y_d^\dagger Y_d)^{pb} - \frac{5}{2} Y_d^{pb} (Y_d Y_d^\dagger)^{ar} - \frac{8}{3} \delta^{ra} g_Y^2 g_s^2 Y_d^{pb} - 3 \delta^{ra} \lambda g_Y^2 Y_d^{pb} \Bigg\} + \left\{ g_L^4 \left( \frac{29}{8} \delta^{pr} Y_d^{*ab} - 15 \delta^{pa} Y_d^{*rb} \right) \right. \\
& + g_Y^2 g_L^2 \left( \frac{11}{18} \delta^{pa} Y_d^{*rb} - \frac{3}{8} \delta^{pr} Y_d^{*ab} \right) + g_L^2 \left( \frac{1}{4} Y_d^{*rb} (Y_u Y_u^\dagger)^{pa} + \frac{3}{4} \delta^{pr} (Y_d^\dagger Y_d Y_d^\dagger)^{ab} + \frac{3}{4} \delta^{pr} (Y_u^\dagger Y_u Y_d^\dagger)^{ab} + \frac{9}{8} \delta^{pa} (Y_d^\dagger Y_d Y_d^\dagger)^{rb} - \frac{3}{4} Y_d^{*rb} (Y_d Y_d^\dagger)^{pa} \right. \\
& - \frac{3}{2} T_2 \delta^{pa} Y_d^{*rb} - \frac{45}{8} \delta^{pa} (Y_u^\dagger Y_u Y_d^\dagger)^{rb} \Bigg) + \frac{4}{3} \delta^{pa} g_s^2 g_L^2 Y_d^{*rb} \Bigg\} C_{dW}^{ab} + C_{dW}^{*ab} \left\{ g_L^4 \left( \frac{29}{8} \delta^{pr} Y_d^{ab} - 15 \delta^{ra} Y_d^{pb} \right) + g_Y^2 g_L^2 \left( \frac{11}{18} \delta^{ra} Y_d^{pb} - \frac{3}{8} \delta^{pr} Y_d^{ab} \right) \right. \\
& + g_L^2 \left( \frac{1}{4} Y_d^{pb} (Y_u Y_u^\dagger)^{ar} + \frac{3}{4} \delta^{pr} (Y_d Y_d^\dagger Y_d)^{ab} + \frac{3}{4} \delta^{pr} (Y_u Y_u^\dagger Y_d)^{ab} + \frac{9}{8} \delta^{ra} (Y_d Y_d^\dagger Y_d)^{pb} - \frac{3}{4} Y_d^{pb} (Y_d Y_d^\dagger)^{ar} - \frac{3}{2} T_2 \delta^{ra} Y_d^{pb} - \frac{45}{8} \delta^{ra} (Y_u Y_u^\dagger Y_d)^{pb} \right. \\
& + \frac{4}{3} \delta^{ra} g_s^2 g_L^2 Y_d^{pb} \Bigg\} + \left\{ g_Y^2 g_s^2 \left( \frac{34}{27} \delta^{pa} Y_d^{*rb} - \frac{16}{9} \delta^{pr} Y_d^{*ab} \right) + g_s^2 g_L^2 \left( \frac{38}{9} \delta^{pa} Y_d^{*rb} + \frac{16}{3} \delta^{pr} Y_d^{*ab} \right) + g_s^2 \left( \frac{4}{3} Y_d^{*rb} (Y_u Y_u^\dagger)^{pa} + 4 \delta^{pa} (Y_u^\dagger Y_u Y_d^\dagger)^{rb} \right. \right. \\
& - 12 Y_d^{*rb} (Y_d Y_d^\dagger)^{pa} - 12 \delta^{pa} (Y_d^\dagger Y_d Y_d^\dagger)^{rb} \Bigg) + 16 \delta^{pr} g_s^4 Y_d^{*ab} \Bigg\} C_{dG}^{ab} + C_{dG}^{*ab} \left\{ g_Y^2 g_s^2 \left( \frac{34}{27} \delta^{ra} Y_d^{pb} - \frac{16}{9} \delta^{pr} Y_d^{ab} \right) + g_s^2 g_L^2 \left( \frac{38}{9} \delta^{ra} Y_d^{pb} + \frac{16}{3} \delta^{pr} Y_d^{ab} \right) \right. \\
& + g_s^2 \left( \frac{4}{3} Y_d^{pb} (Y_u Y_u^\dagger)^{ar} + 4 \delta^{ra} (Y_u Y_u^\dagger Y_d)^{pb} - 12 Y_d^{pb} (Y_d Y_d^\dagger)^{ar} - 12 \delta^{ra} (Y_d Y_d^\dagger Y_d)^{pb} \right) + 16 \delta^{pr} g_s^4 Y_d^{ab} \Bigg\} + \left\{ \frac{29}{324} \delta^{pr} \delta^{ab} g_Y^4 + \frac{11}{36} \delta^{pr} g_L^2 (Y_e Y_e^\dagger)^{ba} \right. \\
& + \frac{1}{2} (Y_d Y_d^\dagger)^{pr} (Y_e Y_e^\dagger)^{ba} + g_Y^2 \left( \frac{49}{108} \delta^{pr} (Y_e Y_e^\dagger)^{ba} + \frac{11}{18} \delta^{ab} (Y_u Y_u^\dagger)^{pr} \right) + \frac{9}{2} \delta^{pr} \delta^{ab} g_L^4 - \frac{83}{108} \delta^{pr} \delta^{ab} g_Y^2 g_L^2 \Bigg\} C_{He}^{(ll)ab} + \left\{ \frac{29}{648} \delta^{pr} \delta^{ab} g_Y^4 + g_Y^2 \left( \frac{13}{54} \delta^{pr} (Y_e Y_e^\dagger)^{ba} \right. \right. \\
& + \frac{11}{36} \delta^{ab} (Y_u Y_u^\dagger)^{pr} \Bigg) + g_L^2 \left( \frac{10}{9} \delta^{pr} (Y_e Y_e^\dagger)^{ba} + \frac{19}{12} \delta^{ab} (Y_u Y_u^\dagger)^{pr} - \frac{5}{6} \delta^{ab} (Y_d Y_d^\dagger)^{pr} \right) - \frac{5}{24} \delta^{pr} \delta^{ab} g_L^4 - \frac{29}{108} \delta^{pr} \delta^{ab} g_Y^2 g_L^2 - \frac{1}{2} (Y_d Y_d^\dagger)^{pr} (Y_e Y_e^\dagger)^{ba} \Bigg\} C_{He}^{(\times)ab} \\
& + \left\{ g_Y^2 \left( \frac{11}{18} \delta^{ab} (Y_u Y_u^\dagger)^{pr} + \frac{77}{108} \delta^{pr} (Y_e^\dagger Y_e)^{ba} \right) - \frac{5}{36} \delta^{pr} g_L^2 (Y_e^\dagger Y_e)^{ba} - \frac{29}{108} \delta^{pr} \delta^{ab} g_Y^2 g_L^2 - \frac{1}{2} (Y_e^\dagger Y_e)^{ba} (Y_d Y_d^\dagger)^{pr} - \frac{295}{324} \delta^{pr} \delta^{ab} g_Y^4 \right\} C_{He}^{ab} \\
& + \left\{ \frac{1}{4} \delta^{pa} (Y_d Y_d^\dagger Y_u Y_u^\dagger)^{br} + \frac{1}{4} \delta^{rb} (Y_u Y_u^\dagger Y_d Y_d^\dagger)^{pa} + \frac{8}{9} \delta^{pr} \delta^{ab} g_Y^2 g_s^2 + g_Y^4 \left( \frac{301}{486} \delta^{pa} \delta^{rb} - \frac{5}{324} \delta^{pr} \delta^{ab} \right) + g_Y^2 g_L^2 \left( \frac{83}{108} \delta^{pr} \delta^{ab} + \frac{833}{162} \delta^{pa} \delta^{rb} \right) \right. \\
& + g_L^4 \left( \frac{27}{2} \delta^{pr} \delta^{ab} - 9 \delta^{pa} \delta^{rb} \right) + g_L^2 \left( \frac{11}{12} \delta^{pr} (Y_d Y_d^\dagger)^{ba} + \frac{779}{144} \delta^{rb} (Y_d Y_d^\dagger)^{pa} + \frac{779}{144} \delta^{pa} (Y_d Y_d^\dagger)^{br} + \frac{1867}{144} \delta^{rb} (Y_u Y_u^\dagger)^{pa} + \frac{1867}{144} \delta^{pa} (Y_u Y_u^\dagger)^{br} - \frac{3}{4} T_2 \delta^{pa} \delta^{rb} \right. \\
& - \frac{11}{12} \delta^{pr} (Y_u Y_u^\dagger)^{ba} \Bigg) + \delta^{rb} (Y_d Y_d^\dagger Y_d Y_d^\dagger)^{pa} + \delta^{pa} (Y_d Y_d^\dagger Y_d Y_d^\dagger)^{br} + g_Y^2 \left( \frac{571}{432} \delta^{rb} (Y_d Y_d^\dagger)^{pa} + \frac{571}{432} \delta^{pa} (Y_d Y_d^\dagger)^{br} + \frac{193}{144} \delta^{rb} (Y_u Y_u^\dagger)^{pa} + \frac{193}{144} \delta^{pa} (Y_u Y_u^\dagger)^{br} \right. \\
& + \frac{19}{12} \delta^{pa} \delta^{rb} \text{Tr} [Y_u^\dagger Y_u] + \frac{53}{12} \delta^{pa} \delta^{rb} \text{Tr} [Y_e^\dagger Y_e] - \frac{7}{36} \delta^{pr} (Y_d Y_d^\dagger)^{ba} - \frac{7}{12} \delta^{pr} (Y_u Y_u^\dagger)^{ba} - \frac{11}{18} \delta^{ab} (Y_u Y_u^\dagger)^{pr} - \frac{41}{12} \delta^{pa} \delta^{rb} \text{Tr} [Y_d^\dagger Y_d] \Bigg) + g_s^2 \left( 4 \delta^{rb} (Y_u Y_u^\dagger)^{pa} \right. \\
& + 4 \delta^{pa} (Y_u Y_u^\dagger)^{br} + 40 \delta^{pa} \delta^{rb} \text{Tr} [Y_d^\dagger Y_d] + 40 \delta^{pa} \delta^{rb} \text{Tr} [Y_u^\dagger Y_u] - \frac{8}{3} \delta^{rb} (Y_d Y_d^\dagger)^{pa} - \frac{8}{3} \delta^{pa} (Y_d Y_d^\dagger)^{br} \Bigg) + \frac{5}{4} (Y_d Y_d^\dagger)^{br} (Y_u Y_u^\dagger)^{pa} + \frac{5}{4} (Y_d Y_d^\dagger)^{pa} (Y_u Y_u^\dagger)^{br} \\
& + \frac{3}{2} (Y_d Y_d^\dagger)^{pr} (Y_d Y_d^\dagger)^{ba} + \frac{11}{4} \delta^{rb} (Y_d Y_d^\dagger Y_u Y_u^\dagger)^{pa} + \frac{11}{4} \delta^{pa} (Y_u Y_u^\dagger Y_d Y_d^\dagger)^{br} + 6 \delta^{pa} \delta^{rb} \text{Tr} [Y_d^\dagger Y_d Y_u^\dagger Y_u] + 16 \delta^{pr} \delta^{ab} g_s^4 - \frac{3}{4} T_2 \delta^{rb} (Y_d Y_d^\dagger)^{pa}
\end{aligned}$$

$$\begin{aligned}
& -\frac{3}{4}\text{T}_2\delta^{pa}(Y_dY_d^\dagger)^{br} - \lambda\left(3\delta^{rb}(Y_dY_d^\dagger)^{pa} + 3\delta^{pa}(Y_dY_d^\dagger)^{br} + 6\delta^{rb}(Y_uY_u^\dagger)^{pa} + 6\delta^{pa}(Y_uY_u^\dagger)^{br}\right) - \frac{3}{2}(Y_dY_d^\dagger)^{pr}(Y_uY_u^\dagger)^{ba} - \frac{17}{4}\text{T}_2\delta^{rb}(Y_uY_u^\dagger)^{pa} \\
& - \frac{17}{4}\text{T}_2\delta^{pa}(Y_uY_u^\dagger)^{br} - \frac{9}{2}(Y_dY_d^\dagger)^{pa}(Y_dY_d^\dagger)^{br} - \frac{9}{2}(Y_uY_u^\dagger)^{pa}(Y_uY_u^\dagger)^{br} - \frac{21}{4}\delta^{rb}(Y_uY_u^\dagger Y_uY_u^\dagger)^{pa} - \frac{21}{4}\delta^{pa}(Y_uY_u^\dagger Y_uY_u^\dagger)^{br} - 6\text{T}_4\delta^{pa}\delta^{rb} \Big\} C_{Hq}^{(\parallel)ab} \\
& + \left\{ \frac{4}{9}\delta^{pr}\delta^{ab}g_Y^2g_s^2 + \frac{3}{4}(Y_uY_u^\dagger)^{pa}(Y_uY_u^\dagger)^{br} + g_s^2g_L^2(4\delta^{pa}\delta^{rb} - 4\delta^{pr}\delta^{ab}) + g_L^4\left(\frac{77}{36}\delta^{pa}\delta^{rb} - \frac{5}{8}\delta^{pr}\delta^{ab}\right) + g_Y^4\left(\frac{463}{972}\delta^{pa}\delta^{rb} - \frac{5}{648}\delta^{pr}\delta^{ab}\right) \right. \\
& + g_s^2\left(\frac{16}{3}\delta^{rb}(Y_dY_d^\dagger)^{pa} + \frac{16}{3}\delta^{pa}(Y_dY_d^\dagger)^{br} - \frac{4}{3}\delta^{rb}(Y_uY_u^\dagger)^{pa} - \frac{4}{3}\delta^{pa}(Y_uY_u^\dagger)^{br}\right) + \lambda\left(\frac{3}{2}\delta^{rb}(Y_uY_u^\dagger)^{pa} + \frac{3}{2}\delta^{pa}(Y_uY_u^\dagger)^{br} - \frac{3}{2}\delta^{rb}(Y_dY_d^\dagger)^{pa} - \frac{3}{2}\delta^{pa}(Y_dY_d^\dagger)^{br}\right) \\
& + g_Y^2\left(\frac{259}{216}\delta^{rb}(Y_dY_d^\dagger)^{pa} + \frac{259}{216}\delta^{pa}(Y_dY_d^\dagger)^{br} - \frac{1}{6}\text{T}_2\delta^{pa}\delta^{rb} - \frac{11}{36}\delta^{ab}(Y_uY_u^\dagger)^{pr} - \frac{7}{18}\delta^{pr}(Y_dY_d^\dagger)^{ba} - \frac{5}{12}\delta^{pr}(Y_uY_u^\dagger)^{ba} - \frac{2}{3}\delta^{rb}(Y_uY_u^\dagger)^{pa} - \frac{2}{3}\delta^{pa}(Y_uY_u^\dagger)^{br}\right) \\
& + g_L^2\left(\frac{29}{12}\delta^{pr}(Y_uY_u^\dagger)^{ba} + \frac{209}{72}\delta^{rb}(Y_dY_d^\dagger)^{pa} + \frac{209}{72}\delta^{pa}(Y_dY_d^\dagger)^{br} + \frac{10}{3}\delta^{pr}(Y_dY_d^\dagger)^{ba} + \frac{19}{4}\delta^{ab}(Y_uY_u^\dagger)^{pr} - \frac{5}{2}\delta^{ab}(Y_dY_d^\dagger)^{pr} - \frac{17}{6}\text{T}_2\delta^{pa}\delta^{rb} \right. \\
& - \frac{145}{36}\delta^{rb}(Y_uY_u^\dagger)^{pa} - \frac{145}{36}\delta^{pa}(Y_uY_u^\dagger)^{br} \Big) + \frac{5}{4}\delta^{rb}(Y_uY_u^\dagger Y_uY_u^\dagger)^{pa} + \frac{5}{4}\delta^{pa}(Y_uY_u^\dagger Y_uY_u^\dagger)^{br} + \frac{3}{2}\text{T}_2\delta^{rb}(Y_uY_u^\dagger)^{pa} + \frac{3}{2}(Y_dY_d^\dagger)^{br}(Y_uY_u^\dagger)^{pa} \\
& + \frac{3}{2}\text{T}_2\delta^{pa}(Y_uY_u^\dagger)^{br} + \frac{3}{2}(Y_dY_d^\dagger)^{pa}(Y_uY_u^\dagger)^{br} + 3\delta^{rb}(Y_dY_d^\dagger Y_uY_u^\dagger)^{pa} + 3\delta^{pa}(Y_uY_u^\dagger Y_dY_d^\dagger)^{br} + 3\delta^{pa}\delta^{rb}\text{Tr}[Y_d^\dagger Y_d Y_u^\dagger Y_u] + 8\delta^{pr}\delta^{ab}g_s^4 - \frac{1}{2}\text{T}_4\delta^{pa}\delta^{rb} \\
& - g_Y^2g_L^2\left(\frac{65}{108}\delta^{pr}\delta^{ab} + \frac{343}{324}\delta^{pa}\delta^{rb}\right) - \frac{3}{2}(Y_dY_d^\dagger)^{pr}(Y_dY_d^\dagger)^{ba} - 2\text{T}_2\delta^{rb}(Y_dY_d^\dagger)^{pa} - 2\text{T}_2\delta^{pa}(Y_dY_d^\dagger)^{br} - 2\delta^{pa}(Y_dY_d^\dagger Y_uY_u^\dagger)^{br} - 2\delta^{rb}(Y_uY_u^\dagger Y_dY_d^\dagger)^{pa} \\
& - 3(Y_dY_d^\dagger)^{pr}(Y_uY_u^\dagger)^{ba} - \frac{21}{4}(Y_dY_d^\dagger)^{pa}(Y_dY_d^\dagger)^{br} - \frac{29}{4}\delta^{rb}(Y_dY_d^\dagger Y_dY_d^\dagger)^{pa} - \frac{29}{4}\delta^{pa}(Y_dY_d^\dagger Y_dY_d^\dagger)^{br} \Big\} C_{Hq}^{(\times)ab} + \left\{ \frac{29}{54}\delta^{pr}\delta^{ab}g_Y^2g_L^2 + g_L^2\left(\frac{5}{12}\delta^{pr}(Y_u^\dagger Y_u)^{ba} \right. \right. \\
& - \frac{27}{8}Y_u^{*rb}Y_u^{pa} \Big) + \frac{3}{2}\text{T}_2Y_u^{*rb}Y_u^{pa} + \frac{3}{2}(Y_u^\dagger Y_u)^{ba}(Y_dY_d^\dagger)^{pr} + \frac{16}{9}\delta^{pr}\delta^{ab}g_Y^2g_s^2 + \frac{43}{12}Y_u^{pa}(Y_u^\dagger Y_uY_u^\dagger)^{rb} + \frac{43}{12}Y_u^{*rb}(Y_uY_u^\dagger Y_u)^{pa} - \frac{5}{162}\delta^{pr}\delta^{ab}g_Y^4 \\
& - \frac{3}{4}Y_u^{pa}(Y_d^\dagger Y_d Y_u^\dagger)^{rb} - \frac{3}{4}Y_u^{*rb}(Y_dY_d^\dagger Y_u)^{pa} - g_Y^2\left(\frac{11}{9}\delta^{ab}(Y_uY_u^\dagger)^{pr} + \frac{49}{36}\delta^{pr}(Y_u^\dagger Y_u)^{ba} + \frac{431}{216}Y_u^{*rb}Y_u^{pa}\right) - 8\delta^{pr}\delta^{ab}g_s^4 \Big\} C_{Hu}^{ab} + \left\{ \frac{1}{2}Y_d^{pa}(Y_u^\dagger Y_uY_d^\dagger)^{rb} \right. \\
& + \frac{1}{2}Y_d^{*rb}(Y_uY_u^\dagger Y_d)^{pa} + g_Y^2\left(\frac{7}{12}\delta^{pr}(Y_d^\dagger Y_d)^{ba} + \frac{11}{18}\delta^{ab}(Y_uY_u^\dagger)^{pr} - \frac{151}{72}Y_d^{*rb}Y_d^{pa}\right) + \frac{3}{2}\text{T}_2Y_d^{*rb}Y_d^{pa} + \frac{7}{2}Y_d^{pa}(Y_d^\dagger Y_d Y_d^\dagger)^{rb} + \frac{7}{2}Y_d^{*rb}(Y_dY_d^\dagger Y_d)^{pa} \\
& + \frac{16}{3}g_s^2Y_d^{*rb}Y_d^{pa} - \frac{31}{324}\delta^{pr}\delta^{ab}g_Y^4 - \frac{29}{108}\delta^{pr}\delta^{ab}g_Y^2g_L^2 - \frac{8}{9}\delta^{pr}\delta^{ab}g_Y^2g_s^2 - g_L^2\left(\frac{5}{12}\delta^{pr}(Y_d^\dagger Y_d)^{ba} + \frac{33}{8}Y_d^{*rb}Y_d^{pa}\right) - \frac{3}{2}(Y_d^\dagger Y_d)^{ba}(Y_dY_d^\dagger)^{pr} \\
& - 8\delta^{pr}\delta^{ab}g_s^4 \Big\} C_{Hd}^{ab} + \left\{ \frac{1}{6}Y_u^{pa}(Y_u^\dagger Y_uY_d^\dagger)^{rb} + g_Y^2\left(\frac{13}{72}Y_d^{*rb}Y_u^{pa} + \frac{17}{36}\delta^{pr}(Y_d^\dagger Y_u)^{ba}\right) + \frac{5}{4}Y_u^{pa}(Y_d^\dagger Y_d Y_d^\dagger)^{rb} + \frac{8}{3}g_s^2Y_d^{*rb}Y_u^{pa} - \frac{1}{4}Y_d^{*rb}(Y_uY_u^\dagger Y_u)^{pa} \right. \\
& - g_L^2\left(\frac{3}{8}Y_d^{*rb}Y_u^{pa} + \frac{5}{12}\delta^{pr}(Y_d^\dagger Y_u)^{ba}\right) - \frac{3}{2}(Y_d^\dagger Y_u)^{ba}(Y_dY_d^\dagger)^{pr} \Big\} C_{Hud}^{ab} + C_{Hud}^{*ab} \left\{ \frac{1}{6}Y_u^{*ra}(Y_uY_u^\dagger Y_d)^{pb} + g_Y^2\left(\frac{13}{72}Y_u^{*ra}Y_d^{pb} + \frac{17}{36}\delta^{pr}(Y_u^\dagger Y_d)^{ab}\right) \right. \\
& + \frac{5}{4}Y_u^{*ra}(Y_dY_d^\dagger Y_d)^{pb} + \frac{8}{3}g_s^2Y_u^{*ra}Y_d^{pb} - \frac{1}{4}Y_d^{pb}(Y_u^\dagger Y_uY_u^\dagger)^{ra} - g_L^2\left(\frac{3}{8}Y_u^{*ra}Y_d^{pb} + \frac{5}{12}\delta^{pr}(Y_u^\dagger Y_d)^{ab}\right) - \frac{3}{2}(Y_u^\dagger Y_d)^{ab}(Y_dY_d^\dagger)^{pr} \Big\} - \left\{ \frac{7}{27}\delta^{ab}g_Y^2Y_u^{*rd}Y_u^{pc} \right.
\end{aligned}$$

$$\begin{aligned}
& + Y_u^{*rd} Y_u^{pc} (Y_e Y_e^\dagger)^{ba} \Big\} C_{\ell u}^{abcd} + \left\{ g_Y^2 \left( \frac{25}{27} \delta^{rb} \delta^{cd} (Y_u Y_u^\dagger)^{pa} + \frac{25}{27} \delta^{pa} \delta^{cd} (Y_u Y_u^\dagger)^{br} + \frac{31}{4} \delta^{pa} \delta^{rb} (Y_e^\dagger Y_e)^{dc} \right) - \frac{17}{81} \delta^{pa} \delta^{rb} \delta^{cd} g_Y^2 g_L^2 - \delta^{rb} (Y_e^\dagger Y_e)^{dc} (Y_u Y_u^\dagger)^{pa} \right. \\
& - \delta^{pa} (Y_e^\dagger Y_e)^{dc} (Y_u Y_u^\dagger)^{br} - \frac{766}{243} \delta^{pa} \delta^{rb} \delta^{cd} g_Y^4 - \frac{15}{4} \delta^{pa} \delta^{rb} g_L^2 (Y_e^\dagger Y_e)^{dc} - 6 \delta^{pa} \delta^{rb} (Y_e^\dagger Y_e Y_e^\dagger Y_e)^{dc} \Big\} C_{qe}^{abcd} + \left\{ \frac{2}{243} \delta^{pa} \delta^{rb} \delta^{cd} g_Y^4 + \frac{34}{81} \delta^{pa} \delta^{rb} \delta^{cd} g_Y^2 g_L^2 \right. \\
& + g_L^2 \left( \frac{77}{36} \delta^{pa} Y_u^{*rd} Y_u^{bc} + \frac{77}{36} \delta^{rb} Y_u^{*ad} Y_u^{pc} - \frac{27}{4} \delta^{pa} \delta^{rb} (Y_u^\dagger Y_u)^{dc} \right) + Y_u^{*rd} Y_u^{bc} (Y_d Y_d^\dagger)^{pa} + Y_u^{*ad} Y_u^{pc} (Y_d Y_d^\dagger)^{br} + g_Y^2 \left( \frac{7}{27} \delta^{ab} Y_u^{*rd} Y_u^{pc} - \frac{125}{108} \delta^{pa} Y_u^{*rd} Y_u^{bc} \right. \\
& - \frac{125}{108} \delta^{rb} Y_u^{*ad} Y_u^{pc} - \frac{50}{27} \delta^{rb} \delta^{cd} (Y_u Y_u^\dagger)^{pa} - \frac{50}{27} \delta^{pa} \delta^{cd} (Y_u Y_u^\dagger)^{br} - \frac{23}{12} \delta^{pa} \delta^{rb} (Y_u^\dagger Y_u)^{dc} \Big) + \delta^{pa} Y_u^{bc} (Y_u^\dagger Y_u Y_u^\dagger)^{rd} + \delta^{rb} Y_u^{*ad} (Y_u Y_u^\dagger Y_u)^{pc} \\
& + 2 \delta^{rb} Y_u^{pc} (Y_u^\dagger Y_u Y_u^\dagger)^{ad} + 2 \delta^{pa} Y_u^{*rd} (Y_u Y_u^\dagger Y_u)^{bc} + 3 \delta^{rb} (Y_u^\dagger Y_u)^{dc} (Y_u Y_u^\dagger)^{pa} + 3 \delta^{pa} (Y_u^\dagger Y_u)^{dc} (Y_u Y_u^\dagger)^{br} + 3 Y_u^{*rd} Y_u^{pc} (Y_u Y_u^\dagger)^{ba} + \frac{16}{3} \delta^{pa} \delta^{rb} \delta^{cd} g_Y^2 g_s^2 \\
& + 18 \delta^{pa} \delta^{rb} (Y_u^\dagger Y_u Y_u^\dagger Y_u)^{dc} - \frac{2}{3} Y_u^{*rd} Y_u^{bc} (Y_u Y_u^\dagger)^{pa} - \frac{2}{3} Y_u^{*ad} Y_u^{pc} (Y_u Y_u^\dagger)^{br} - 3 Y_u^{*rd} Y_u^{pc} (Y_d Y_d^\dagger)^{ba} - 3 \delta^{pa} \delta^{rb} (Y_u^\dagger Y_d Y_d^\dagger Y_u)^{dc} \\
& - 40 \delta^{pa} \delta^{rb} g_s^2 (Y_u^\dagger Y_u)^{dc} \Big\} C_{qu}^{(\parallel)abcd} + \left\{ \frac{2}{729} \delta^{pa} \delta^{rb} \delta^{cd} g_Y^4 + \frac{34}{243} \delta^{pa} \delta^{rb} \delta^{cd} g_Y^2 g_L^2 + g_L^2 \left( \frac{83}{12} \delta^{pa} Y_u^{*rd} Y_u^{bc} + \frac{83}{12} \delta^{rb} Y_u^{*ad} Y_u^{pc} - \frac{9}{4} \delta^{pa} \delta^{rb} (Y_u^\dagger Y_u)^{dc} \right) \right. \\
& + \delta^{rb} (Y_u^\dagger Y_u)^{dc} (Y_u Y_u^\dagger)^{pa} + \delta^{pa} (Y_u^\dagger Y_u)^{dc} (Y_u Y_u^\dagger)^{br} + g_Y^2 \left( \frac{16}{81} \delta^{ab} Y_u^{*rd} Y_u^{pc} - \frac{19}{36} \delta^{pa} \delta^{rb} (Y_u^\dagger Y_u)^{dc} - \frac{50}{81} \delta^{rb} \delta^{cd} (Y_u Y_u^\dagger)^{pa} - \frac{50}{81} \delta^{pa} \delta^{cd} (Y_u Y_u^\dagger)^{br} \right. \\
& - \frac{131}{36} \delta^{pa} Y_u^{*rd} Y_u^{bc} - \frac{131}{36} \delta^{rb} Y_u^{*ad} Y_u^{pc} \Big) + g_s^2 \left( \frac{2}{3} \delta^{pr} \delta^{cd} (Y_d Y_d^\dagger)^{ba} + \frac{2}{3} \delta^{pa} \delta^{rb} \delta^{cd} \text{Tr} [Y_d^\dagger Y_d] + \frac{64}{27} \delta^{ab} Y_u^{*rd} Y_u^{pc} - \frac{2}{27} \delta^{rb} \delta^{cd} (Y_u Y_u^\dagger)^{pa} - \frac{2}{27} \delta^{pa} \delta^{cd} (Y_u Y_u^\dagger)^{br} \right. \\
& - \frac{2}{3} \delta^{pr} \delta^{cd} (Y_u Y_u^\dagger)^{ba} - \frac{2}{3} \delta^{pa} \delta^{rb} \delta^{cd} \text{Tr} [Y_u^\dagger Y_u] - \frac{32}{3} \delta^{pa} \delta^{rb} (Y_u^\dagger Y_u)^{dc} \Big) + \frac{82}{81} \delta^{pa} \delta^{rb} \delta^{cd} g_s^2 g_L^2 + 2 Y_u^{*rd} Y_u^{pc} (Y_u Y_u^\dagger)^{ba} + 3 Y_u^{*rd} Y_u^{bc} (Y_d Y_d^\dagger)^{pa} \\
& + 3 Y_u^{*ad} Y_u^{pc} (Y_d Y_d^\dagger)^{br} + 3 \delta^{pa} Y_u^{bc} (Y_u^\dagger Y_u Y_u^\dagger)^{rd} + 3 \delta^{rb} Y_u^{pc} (Y_u^\dagger Y_u Y_u^\dagger)^{ad} + 3 \delta^{rb} Y_u^{*ad} (Y_u Y_u^\dagger Y_u)^{pc} + 3 \delta^{pa} Y_u^{*rd} (Y_u Y_u^\dagger Y_u)^{bc} + 7 \delta^{pa} \delta^{rb} (Y_u^\dagger Y_u Y_u^\dagger Y_u)^{dc} \\
& - g_Y^2 g_s^2 \left( \frac{2}{27} \delta^{pr} \delta^{ab} \delta^{cd} + \frac{1288}{243} \delta^{pa} \delta^{rb} \delta^{cd} \right) - 2 Y_u^{*rd} Y_u^{pc} (Y_d Y_d^\dagger)^{ba} - 2 Y_u^{*rd} Y_u^{bc} (Y_u Y_u^\dagger)^{pa} - 2 Y_u^{*ad} Y_u^{pc} (Y_u Y_u^\dagger)^{br} - 2 \delta^{pa} \delta^{rb} (Y_u^\dagger Y_d Y_d^\dagger Y_u)^{dc} \Big\} C_{qu}^{(\times)abcd} \\
& + \left\{ \frac{1}{2} \delta^{rb} Y_d^{pc} (Y_u^\dagger Y_u Y_d^\dagger)^{ad} + \frac{1}{2} \delta^{pa} Y_d^{*rd} (Y_u Y_u^\dagger Y_d)^{bc} + g_Y^2 \left( \frac{7}{27} \delta^{pa} Y_d^{*rd} Y_d^{bc} + \frac{7}{27} \delta^{rb} Y_d^{*ad} Y_d^{pc} + \frac{25}{27} \delta^{rb} \delta^{cd} (Y_u Y_u^\dagger)^{pa} + \frac{25}{27} \delta^{pa} \delta^{cd} (Y_u Y_u^\dagger)^{br} \right. \right. \\
& + \frac{23}{12} \delta^{pa} \delta^{rb} (Y_d^\dagger Y_d)^{dc} \Big) + \delta^{pa} Y_d^{bc} (Y_u^\dagger Y_u Y_d^\dagger)^{rd} + \delta^{rb} Y_d^{*ad} (Y_u Y_u^\dagger Y_d)^{pc} + 3 \delta^{pa} \delta^{rb} (Y_d^\dagger Y_u Y_u^\dagger Y_d)^{dc} + 40 \delta^{pa} \delta^{rb} g_s^2 (Y_d^\dagger Y_d)^{dc} - \frac{17}{81} \delta^{pa} \delta^{rb} \delta^{cd} g_Y^2 g_L^2 \\
& - \frac{136}{243} \delta^{pa} \delta^{rb} \delta^{cd} g_Y^4 - g_L^2 \left( \frac{29}{18} \delta^{pa} Y_d^{*rd} Y_d^{bc} + \frac{29}{18} \delta^{rb} Y_d^{*ad} Y_d^{pc} + \frac{45}{4} \delta^{pa} \delta^{rb} (Y_d^\dagger Y_d)^{dc} \right) - \delta^{pa} Y_d^{bc} (Y_d^\dagger Y_d Y_d^\dagger)^{rd} - \delta^{rb} Y_d^{*ad} (Y_d Y_d^\dagger Y_d)^{pc} \\
& - \frac{3}{2} \delta^{rb} Y_d^{pc} (Y_d^\dagger Y_d Y_d^\dagger)^{ad} - \frac{3}{2} \delta^{pa} Y_d^{*rd} (Y_d Y_d^\dagger Y_d)^{bc} - \frac{8}{3} \delta^{pa} \delta^{rb} \delta^{cd} g_Y^2 g_s^2 - 3 \delta^{rb} (Y_d^\dagger Y_d)^{dc} (Y_u Y_u^\dagger)^{pa} - 3 \delta^{pa} (Y_d^\dagger Y_d)^{dc} (Y_u Y_u^\dagger)^{br} \\
& - 18 \delta^{pa} \delta^{rb} (Y_d^\dagger Y_d Y_d^\dagger Y_d)^{dc} \Big\} C_{qd}^{(\parallel)abcd} + \left\{ g_Y^2 g_s^2 \left( \frac{440}{243} \delta^{pa} \delta^{rb} \delta^{cd} - \frac{2}{27} \delta^{pr} \delta^{ab} \delta^{cd} \right) + g_Y^2 \left( \frac{1}{9} \delta^{ab} Y_d^{*rd} Y_d^{pc} + \frac{25}{81} \delta^{rb} \delta^{cd} (Y_u Y_u^\dagger)^{pa} + \frac{25}{81} \delta^{pa} \delta^{cd} (Y_u Y_u^\dagger)^{br} \right. \right.
\end{aligned}$$

$$\begin{aligned}
& + \frac{11}{18} \delta^{pa} Y_d^{*rd} Y_d^{bc} + \frac{11}{18} \delta^{rb} Y_d^{*ad} Y_d^{pc} + \frac{3}{4} \delta^{pa} \delta^{rb} (Y_d^\dagger Y_d)^{dc} + Y_d^{*rd} Y_d^{pc} (Y_u Y_u^\dagger)^{ba} + g_s^2 \left( \frac{2}{3} \delta^{pr} \delta^{cd} (Y_d^\dagger Y_d^\dagger)^{ba} + \frac{2}{3} \delta^{pa} \delta^{rb} \delta^{cd} \text{Tr} [Y_d^\dagger Y_d] + \frac{32}{3} \delta^{pa} \delta^{rb} (Y_d^\dagger Y_d)^{dc} \right. \\
& - \frac{2}{27} \delta^{rb} \delta^{cd} (Y_u Y_u^\dagger)^{pa} - \frac{2}{27} \delta^{pa} \delta^{cd} (Y_u Y_u^\dagger)^{br} - \frac{2}{3} \delta^{pr} \delta^{cd} (Y_u Y_u^\dagger)^{ba} - \frac{2}{3} \delta^{pa} \delta^{rb} \delta^{cd} \text{Tr} [Y_u^\dagger Y_u] \left. \right) + \frac{82}{81} \delta^{pa} \delta^{rb} \delta^{cd} g_s^2 g_L^2 + 2 \delta^{pa} \delta^{rb} (Y_d^\dagger Y_u Y_u^\dagger Y_d)^{dc} \\
& + 3 \delta^{pa} Y_d^{bc} (Y_u^\dagger Y_u Y_d^\dagger)^{rd} + 3 \delta^{rb} Y_d^{*ad} (Y_u Y_u^\dagger Y_d)^{pc} - \frac{17}{243} \delta^{pa} \delta^{rb} \delta^{cd} g_Y^2 g_L^2 - \frac{136}{729} \delta^{pa} \delta^{rb} \delta^{cd} g_Y^4 - g_L^2 \left( \frac{15}{4} \delta^{pa} \delta^{rb} (Y_d^\dagger Y_d)^{dc} + \frac{13}{3} \delta^{pa} Y_d^{*rd} Y_d^{bc} \right. \\
& + \frac{13}{3} \delta^{rb} Y_d^{*ad} Y_d^{pc} \left. \right) - Y_d^{*rd} Y_d^{pc} (Y_d Y_d^\dagger)^{ba} - \delta^{rb} (Y_d^\dagger Y_d)^{dc} (Y_u Y_u^\dagger)^{pa} - \delta^{pa} (Y_d^\dagger Y_d)^{dc} (Y_u Y_u^\dagger)^{br} - \frac{3}{2} \delta^{rb} Y_d^{pc} (Y_u^\dagger Y_u Y_d^\dagger)^{ad} - \frac{3}{2} \delta^{pa} Y_d^{*rd} (Y_u Y_u^\dagger Y_d)^{bc} \\
& - 3 \delta^{pa} Y_d^{bc} (Y_d^\dagger Y_d Y_d^\dagger)^{rd} - 3 \delta^{rb} Y_d^{*ad} (Y_d Y_d^\dagger Y_d)^{pc} - \frac{9}{2} \delta^{rb} Y_d^{pc} (Y_d^\dagger Y_d Y_d^\dagger)^{ad} - \frac{9}{2} \delta^{pa} Y_d^{*rd} (Y_d Y_d^\dagger Y_d)^{bc} - 7 \delta^{pa} \delta^{rb} (Y_d^\dagger Y_d Y_d^\dagger Y_d)^{dc} \left. \right\} C_{qd}^{(\times)abcd} \\
& + \left\{ \frac{8}{27} \delta^{pr} \delta^{ab} \delta^{cd} g_Y^4 - \frac{8}{9} \delta^{pr} \delta^{ad} g_Y^2 (Y_e^\dagger Y_e)^{bc} \right\} C_{ee}^{abcd} + \left\{ \frac{32}{81} \delta^{pr} \delta^{ad} \delta^{bc} g_Y^4 + g_Y^2 \left( \frac{28}{27} \delta^{cd} Y_u^{*rb} Y_u^{pa} - \frac{44}{81} \delta^{ad} Y_u^{*rb} Y_u^{pc} - \frac{16}{9} \delta^{pr} \delta^{ad} (Y_u^\dagger Y_u)^{bc} \right) \right. \\
& + 2 Y_u^{*rb} Y_u^{pc} (Y_u^\dagger Y_u)^{da} + \frac{64}{27} \delta^{ad} g_s^2 Y_u^{*rb} Y_u^{pc} - 6 Y_u^{*rb} Y_u^{pa} (Y_u^\dagger Y_u)^{dc} \left. \right\} C_{uu}^{abcd} + \left\{ \frac{8}{81} \delta^{pr} \delta^{ad} \delta^{bc} g_Y^4 + g_Y^2 \left( \frac{4}{9} \delta^{ad} Y_d^{*rb} Y_d^{pc} - \frac{8}{9} \delta^{pr} \delta^{ad} (Y_d^\dagger Y_d)^{bc} \right) \right. \\
& - 4 Y_d^{*rb} Y_d^{pc} (Y_d^\dagger Y_d)^{da} \left. \right\} C_{dd}^{abcd} + \left\{ Y_u^{*rd} Y_u^{pc} (Y_e^\dagger Y_e)^{ba} - \frac{7}{27} \delta^{ab} g_Y^2 Y_u^{*rd} Y_u^{pc} \right\} C_{eu}^{abcd} + \left\{ 3 Y_u^{*rb} Y_u^{pa} (Y_d^\dagger Y_d)^{dc} - \frac{7}{27} \delta^{cd} g_Y^2 Y_u^{*rb} Y_u^{pa} - Y_u^{*rb} Y_d^{pc} (Y_d^\dagger Y_u)^{da} \right. \\
& - Y_d^{*rd} Y_u^{pa} (Y_u^\dagger Y_d)^{bc} \left. \right\} C_{ud}^{(\parallel)abcd} + \left\{ Y_u^{*rb} Y_u^{pa} (Y_d^\dagger Y_d)^{dc} + \frac{32}{27} \delta^{cd} g_s^2 Y_u^{*rb} Y_u^{pa} - \frac{7}{81} \delta^{cd} g_Y^2 Y_u^{*rb} Y_u^{pa} - 3 Y_u^{*rb} Y_d^{pc} (Y_d^\dagger Y_u)^{da} - 3 Y_d^{*rd} Y_u^{pa} (Y_u^\dagger Y_d)^{bc} \right\} C_{ud}^{(\times)abcd} \\
& + \left\{ \frac{1}{4} \delta^{rd} Y_d^{pc} (Y_e^\dagger Y_e Y_e^\dagger)^{ab} + \frac{29}{36} \delta^{rd} g_L^2 Y_e^{*ab} Y_d^{pc} + \delta^{rd} Y_e^{*ab} (Y_d Y_d^\dagger Y_d)^{pc} - \frac{7}{54} \delta^{rd} g_Y^2 Y_e^{*ab} Y_d^{pc} - \frac{1}{2} \delta^{rd} Y_e^{*ab} (Y_u Y_u^\dagger Y_d)^{pc} \right\} C_{ledq}^{abcd} \\
& + C_{ledq}^{*abcd} \left\{ \frac{1}{4} \delta^{pd} Y_d^{*rc} (Y_e Y_e^\dagger Y_e)^{ab} + \frac{29}{36} \delta^{pd} g_L^2 Y_d^{*rc} Y_e^{ab} + \delta^{pd} Y_e^{ab} (Y_d^\dagger Y_d Y_d^\dagger)^{rc} - \frac{7}{54} \delta^{pd} g_Y^2 Y_d^{*rc} Y_e^{ab} - \frac{1}{2} \delta^{pd} Y_e^{ab} (Y_u^\dagger Y_u Y_d^\dagger)^{rc} \right\} + \left\{ \frac{1}{6} Y_d^{*ad} Y_u^{*rb} (Y_u Y_u^\dagger)^{pc} \right. \\
& + \frac{1}{2} \delta^{pa} Y_u^{*cb} (Y_d^\dagger Y_d Y_d^\dagger)^{rd} + \frac{3}{4} \delta^{pc} Y_u^{*rb} (Y_d^\dagger Y_d Y_d^\dagger)^{ad} + \frac{3}{4} \delta^{pc} Y_d^{*rd} (Y_u^\dagger Y_u Y_u^\dagger)^{ab} + g_Y^2 \left( \frac{31}{216} \delta^{pc} Y_d^{*ad} Y_u^{*rb} + \frac{125}{72} \delta^{pa} Y_d^{*cd} Y_u^{*rb} - \frac{11}{216} \delta^{pa} Y_d^{*rd} Y_u^{*cb} \right. \\
& - \frac{7}{18} \delta^{pc} Y_d^{*rd} Y_u^{*ab} \left. \right) + g_L^2 \left( \frac{47}{72} \delta^{pa} Y_d^{*rd} Y_u^{*cb} + \frac{29}{12} \delta^{pc} Y_d^{*rd} Y_u^{*ab} - \frac{115}{72} \delta^{pc} Y_d^{*ad} Y_u^{*rb} - \frac{77}{24} \delta^{pa} Y_d^{*cd} Y_u^{*rb} \right) + Y_d^{*cd} Y_u^{*rb} (Y_u Y_u^\dagger)^{pa} \\
& + \frac{9}{4} \delta^{pa} Y_d^{*rd} (Y_d^\dagger Y_d Y_u^\dagger)^{cb} + 3 \delta^{pc} Y_u^{*ab} (Y_d^\dagger Y_d Y_d^\dagger)^{rd} + \frac{16}{3} \delta^{pc} g_s^2 Y_d^{*ad} Y_u^{*rb} - \frac{1}{4} Y_d^{*ad} Y_u^{*rb} (Y_d Y_d^\dagger)^{pc} - \frac{1}{4} \delta^{pa} Y_u^{*cb} (Y_u^\dagger Y_u Y_d^\dagger)^{rd} - \frac{1}{2} \delta^{pc} Y_d^{*ad} (Y_u^\dagger Y_u Y_u^\dagger)^{rb} \\
& - \frac{3}{4} \delta^{pc} Y_d^{*rd} (Y_d^\dagger Y_d Y_u^\dagger)^{ab} - \frac{3}{2} Y_d^{*cd} Y_u^{*rb} (Y_d Y_d^\dagger)^{pa} - \frac{3}{2} \delta^{pa} Y_u^{*rb} (Y_d^\dagger Y_d Y_d^\dagger)^{cd} - \frac{3}{2} \delta^{pc} Y_u^{*ab} (Y_u^\dagger Y_u Y_d^\dagger)^{rd} - 3 \delta^{pa} Y_d^{*cd} (Y_u^\dagger Y_u Y_u^\dagger)^{rb} \left. \right\} C_{quqd}^{(\parallel)abcd} \\
& + \left( C_{quqd}^{(\parallel)*} \right)^{abcd} \left\{ \frac{1}{6} Y_d^{ad} Y_u^{pb} (Y_u Y_u^\dagger)^{cr} + \frac{1}{2} \delta^{ra} Y_u^{cb} (Y_d Y_d^\dagger Y_d)^{pd} + \frac{3}{4} \delta^{rc} Y_u^{pb} (Y_d Y_d^\dagger Y_d)^{ad} + \frac{3}{4} \delta^{rc} Y_d^{pd} (Y_u Y_u^\dagger Y_u)^{ab} + g_Y^2 \left( \frac{31}{216} \delta^{rc} Y_d^{ad} Y_u^{pb} + \frac{125}{72} \delta^{ra} Y_d^{cd} Y_u^{pb} \right. \right.
\end{aligned}$$



$$\begin{aligned}
& -\frac{11}{216}\delta^{ra}Y_d^{pd}Y_u^{cb}-\frac{7}{18}\delta^{rc}Y_d^{pd}Y_u^{ab})+g_L^2\left(\frac{47}{72}\delta^{ra}Y_d^{pd}Y_u^{cb}+\frac{29}{12}\delta^{rc}Y_d^{pd}Y_u^{ab}-\frac{115}{72}\delta^{rc}Y_d^{ad}Y_u^{pb}-\frac{77}{24}\delta^{ra}Y_d^{cd}Y_u^{pb}\right)+Y_d^{cd}Y_u^{pb}(Y_uY_u^\dagger)^{ar}+\frac{9}{4}\delta^{ra}Y_d^{pd}(Y_dY_d^\dagger Y_u)^{cb}\\
& +3\delta^{rc}Y_u^{ab}(Y_dY_d^\dagger Y_d)^{pd}+\frac{16}{3}\delta^{rc}g_s^2Y_d^{ad}Y_u^{pb}-\frac{1}{4}Y_d^{ad}Y_u^{pb}(Y_dY_d^\dagger)^{cr}-\frac{1}{4}\delta^{ra}Y_u^{cb}(Y_uY_u^\dagger Y_d)^{pd}-\frac{1}{2}\delta^{rc}Y_d^{ad}(Y_uY_u^\dagger Y_u)^{pb}-\frac{3}{4}\delta^{rc}Y_d^{pd}(Y_dY_d^\dagger Y_u)^{ab}\\
& -\frac{3}{2}Y_d^{cd}Y_u^{pb}(Y_dY_d^\dagger)^{ar}-\frac{3}{2}\delta^{ra}Y_u^{pb}(Y_dY_d^\dagger Y_d)^{cd}-\frac{3}{2}\delta^{rc}Y_u^{ab}(Y_uY_u^\dagger Y_d)^{pd}-3\delta^{ra}Y_d^{cd}(Y_uY_u^\dagger Y_u)^{pb}\Bigg\}+\left\{\frac{1}{4}\delta^{pc}Y_d^{*rd}(Y_u^\dagger Y_u Y_u^\dagger)^{ab}+\frac{1}{3}Y_d^{*cd}Y_u^{*rb}(Y_uY_u^\dagger)^{pa}\right.\\
& +\frac{1}{2}Y_d^{*ad}Y_u^{*rb}(Y_uY_u^\dagger)^{pc}+\frac{3}{4}\delta^{pc}Y_u^{*rb}(Y_d^\dagger Y_d Y_d^\dagger)^{ad}+g_Y^2\left(\frac{37}{72}\delta^{pc}Y_d^{*ad}Y_u^{*rb}+\frac{131}{216}\delta^{pa}Y_d^{*cd}Y_u^{*rb}-\frac{5}{72}\delta^{pa}Y_d^{*rd}Y_u^{*cb}-\frac{11}{108}\delta^{pc}Y_d^{*rd}Y_u^{*ab}\right)\\
& +g_L^2\left(\frac{8}{9}\delta^{pc}Y_d^{*rd}Y_u^{*ab}+\frac{53}{24}\delta^{pa}Y_d^{*rd}Y_u^{*cb}-\frac{71}{72}\delta^{pa}Y_d^{*cd}Y_u^{*rb}-\frac{109}{24}\delta^{pc}Y_d^{*ad}Y_u^{*rb}\right)+\delta^{pc}Y_u^{*ab}(Y_d^\dagger Y_d Y_d^\dagger)^{rd}+\frac{3}{2}\delta^{pa}Y_u^{*cb}(Y_d^\dagger Y_d Y_d^\dagger)^{rd}\\
& +\frac{21}{4}\delta^{pa}Y_d^{*rd}(Y_d^\dagger Y_d Y_u^\dagger)^{cb}-\frac{1}{2}Y_d^{*cd}Y_u^{*rb}(Y_dY_d^\dagger)^{pa}-\frac{1}{2}\delta^{pc}Y_u^{*ab}(Y_u^\dagger Y_u Y_d^\dagger)^{rd}-\frac{3}{4}Y_d^{*ad}Y_u^{*rb}(Y_dY_d^\dagger)^{pc}-\frac{3}{4}\delta^{pc}Y_d^{*rd}(Y_d^\dagger Y_d Y_u^\dagger)^{ab}-\frac{3}{4}\delta^{pa}Y_u^{*cb}(Y_u^\dagger Y_u Y_d^\dagger)^{rd}\\
& -\delta^{pa}Y_u^{*rb}(Y_d^\dagger Y_d Y_d^\dagger)^{cd}-\delta^{pa}Y_d^{*cd}(Y_u^\dagger Y_u Y_u^\dagger)^{rb}-\frac{3}{2}\delta^{pc}Y_d^{*ad}(Y_u^\dagger Y_u Y_u^\dagger)^{rb}\Bigg\}C_{quqd}^{(\times)abcd}+\left(C_{quqd}^{(\times)*}\right)^{abcd}\left\{\frac{1}{4}\delta^{rc}Y_d^{pd}(Y_uY_u^\dagger Y_u)^{ab}+\frac{1}{3}Y_d^{cd}Y_u^{pb}(Y_uY_u^\dagger)^{ar}\right.\\
& +\frac{1}{2}Y_d^{ad}Y_u^{pb}(Y_uY_u^\dagger)^{cr}+\frac{3}{4}\delta^{rc}Y_u^{pb}(Y_dY_d^\dagger Y_d)^{ad}+g_Y^2\left(\frac{37}{72}\delta^{rc}Y_d^{ad}Y_u^{pb}+\frac{131}{216}\delta^{ra}Y_d^{cd}Y_u^{pb}-\frac{5}{72}\delta^{ra}Y_d^{pd}Y_u^{cb}-\frac{11}{108}\delta^{rc}Y_d^{pd}Y_u^{ab}\right)+g_L^2\left(\frac{8}{9}\delta^{rc}Y_d^{pd}Y_u^{ab}\right.\\
& +\frac{53}{24}\delta^{ra}Y_d^{pd}Y_u^{cb}-\frac{71}{72}\delta^{ra}Y_d^{cd}Y_u^{pb}-\frac{109}{24}\delta^{rc}Y_d^{ad}Y_u^{pb})+\delta^{rc}Y_u^{ab}(Y_dY_d^\dagger Y_d)^{pd}+\frac{3}{2}\delta^{ra}Y_u^{cb}(Y_dY_d^\dagger Y_d)^{pd}+\frac{21}{4}\delta^{ra}Y_d^{pd}(Y_dY_d^\dagger Y_u)^{cb}-\frac{1}{2}Y_d^{cd}Y_u^{pb}(Y_dY_d^\dagger)^{ar}\\
& -\frac{1}{2}\delta^{rc}Y_u^{ab}(Y_uY_u^\dagger Y_d)^{pd}-\frac{3}{4}Y_d^{ad}Y_u^{pb}(Y_dY_d^\dagger)^{cr}-\frac{3}{4}\delta^{rc}Y_d^{pd}(Y_dY_d^\dagger Y_u)^{ab}-\frac{3}{4}\delta^{ra}Y_u^{cb}(Y_uY_u^\dagger Y_d)^{pd}-\delta^{ra}Y_u^{pb}(Y_dY_d^\dagger Y_d)^{cd}-\delta^{ra}Y_d^{cd}(Y_uY_u^\dagger Y_u)^{pb}\\
& -\frac{3}{2}\delta^{rc}Y_d^{ad}(Y_uY_u^\dagger Y_u)^{pb}\Bigg\}+\left\{\frac{1}{2}Y_e^{*ab}Y_u^{*rd}(Y_dY_d^\dagger)^{pc}+\frac{1}{2}\delta^{pc}Y_u^{*rd}(Y_e^\dagger Y_e Y_e^\dagger)^{ab}+\delta^{pc}Y_e^{*ab}(Y_u^\dagger Y_u Y_u^\dagger)^{rd}+\frac{77}{72}\delta^{pc}g_L^2Y_e^{*ab}Y_u^{*rd}-\frac{1}{3}Y_e^{*ab}Y_u^{*rd}(Y_uY_u^\dagger)^{pc}\right.\\
& -\frac{125}{216}\delta^{pc}g_Y^2Y_e^{*ab}Y_u^{*rd}\Bigg\}C_{lequ}^{abcd}+C_{lequ}^{*abcd}\left\{\frac{1}{2}Y_e^{ab}Y_u^{pd}(Y_dY_d^\dagger)^{cr}+\frac{1}{2}\delta^{rc}Y_u^{pd}(Y_eY_e^\dagger Y_e)^{ab}+\delta^{rc}Y_e^{ab}(Y_uY_u^\dagger Y_u)^{pd}+\frac{77}{72}\delta^{rc}g_L^2Y_e^{ab}Y_u^{pd}-\frac{1}{3}Y_e^{ab}Y_u^{pd}(Y_uY_u^\dagger)^{cr}\right.\\
& -\frac{125}{216}\delta^{rc}g_Y^2Y_e^{ab}Y_u^{pd}\Bigg\}+\left\{\frac{1}{6}Y_e^{*ad}Y_u^{*rb}(Y_uY_u^\dagger)^{pc}+\frac{1}{4}\delta^{pc}Y_u^{*rb}(Y_e^\dagger Y_e Y_e^\dagger)^{ad}-\frac{1}{4}Y_e^{*ad}Y_u^{*rb}(Y_dY_d^\dagger)^{pc}-\frac{95}{216}\delta^{pc}g_Y^2Y_e^{*ad}Y_u^{*rb}-\frac{1}{2}\delta^{pc}Y_e^{*ad}(Y_u^\dagger Y_u Y_u^\dagger)^{rb}\right.\\
& -\frac{109}{72}\delta^{pc}g_L^2Y_e^{*ad}Y_u^{*rb}\Bigg\}C_{luqe}^{abcd}+C_{luqe}^{*abcd}\left\{\frac{1}{6}Y_e^{ad}Y_u^{pb}(Y_uY_u^\dagger)^{cr}+\frac{1}{4}\delta^{rc}Y_u^{pb}(Y_eY_e^\dagger Y_e)^{ad}-\frac{1}{4}Y_e^{ad}Y_u^{pb}(Y_dY_d^\dagger)^{cr}-\frac{95}{216}\delta^{rc}g_Y^2Y_e^{ad}Y_u^{pb}\right.\\
& -\frac{1}{2}\delta^{rc}Y_e^{ad}(Y_uY_u^\dagger Y_u)^{pb}-\frac{109}{72}\delta^{rc}g_L^2Y_e^{ad}Y_u^{pb}\Bigg\}+\left\{\frac{4}{27}\delta^{pr}\delta^{ad}\delta^{bc}g_Y^4+\frac{4}{9}\delta^{pr}\delta^{bc}g_Y^2(Y_eY_e^\dagger)^{da}+\frac{4}{3}\delta^{pr}\delta^{bc}g_L^2(Y_eY_e^\dagger)^{da}-\frac{4}{9}\delta^{pr}\delta^{ad}\delta^{bc}g_L^4\right\}C_{\ell\ell}^{abcd}\\
& +\left\{g_Y^4\left(\frac{4}{81}\delta^{pr}\delta^{ad}\delta^{bc}-\frac{29}{729}\delta^{pa}\delta^{rd}\delta^{bc}-\frac{16}{243}\delta^{pa}\delta^{rb}\delta^{cd}\right)+g_L^4\left(\delta^{pa}\delta^{rb}\delta^{cd}-\frac{4}{3}\delta^{pr}\delta^{ad}\delta^{bc}-\frac{70}{9}\delta^{pa}\delta^{rd}\delta^{bc}\right)+g_Y^2g_L^2\left(\frac{277}{81}\delta^{pa}\delta^{rb}\delta^{cd}-\frac{232}{243}\delta^{pa}\delta^{rd}\delta^{bc}\right)\right\}
\end{aligned}$$

$$\begin{aligned}
& + g_Y^2 g_s^2 \left( \frac{22}{243} \delta^{pa} \delta^{rd} \delta^{bc} + 4 \delta^{pa} \delta^{rb} \delta^{cd} - \frac{4}{27} \delta^{pr} \delta^{ad} \delta^{bc} \right) + \delta^{rb} (Y_d Y_d^\dagger)^{da} (Y_u Y_u^\dagger)^{pc} + \delta^{pa} (Y_d Y_d^\dagger)^{bc} (Y_u Y_u^\dagger)^{dr} + g_L^2 \left( \delta^{rd} \delta^{bc} (Y_d Y_d^\dagger)^{pa} + \delta^{pa} \delta^{bc} (Y_d Y_d^\dagger)^{dr} \right. \\
& + 4 \delta^{pr} \delta^{bc} (Y_d Y_d^\dagger)^{da} + 4 \delta^{pr} \delta^{bc} (Y_u Y_u^\dagger)^{da} + \frac{55}{3} \delta^{pa} \delta^{rd} (Y_d Y_d^\dagger)^{bc} - \frac{1}{3} \delta^{rd} \delta^{bc} (Y_u Y_u^\dagger)^{pa} - \frac{1}{3} \delta^{pa} \delta^{bc} (Y_u Y_u^\dagger)^{dr} - \frac{43}{6} \delta^{pa} \delta^{rd} (Y_u Y_u^\dagger)^{bc} - \frac{21}{2} \delta^{pa} \delta^{rb} (Y_d Y_d^\dagger)^{dc} \\
& - \frac{39}{2} \delta^{pa} \delta^{rb} (Y_u Y_u^\dagger)^{dc} \left. \right) + g_Y^2 \left( \frac{8}{81} \delta^{rd} \delta^{bc} (Y_u Y_u^\dagger)^{pa} + \frac{8}{81} \delta^{pa} \delta^{bc} (Y_u Y_u^\dagger)^{dr} + \frac{4}{9} \delta^{pr} \delta^{bc} (Y_u Y_u^\dagger)^{da} + \frac{5}{2} \delta^{pa} \delta^{rb} (Y_d Y_d^\dagger)^{dc} + \frac{47}{18} \delta^{pa} \delta^{rd} (Y_u Y_u^\dagger)^{bc} - \frac{2}{9} \delta^{pa} \delta^{rd} (Y_d Y_d^\dagger)^{bc} \right. \\
& - \frac{4}{9} \delta^{pr} \delta^{bc} (Y_d Y_d^\dagger)^{da} - \frac{50}{27} \delta^{rb} \delta^{cd} (Y_u Y_u^\dagger)^{pa} - \frac{50}{27} \delta^{pa} \delta^{cd} (Y_u Y_u^\dagger)^{br} - \frac{17}{2} \delta^{pa} \delta^{rb} (Y_u Y_u^\dagger)^{dc} \left. \right) + g_s^2 \left( \frac{4}{3} \delta^{pr} \delta^{bc} (Y_d Y_d^\dagger)^{da} + \frac{4}{3} \delta^{pa} \delta^{rd} \delta^{bc} \text{Tr} [Y_d^\dagger Y_d] \right. \\
& + \frac{92}{27} \delta^{rd} \delta^{bc} (Y_u Y_u^\dagger)^{pa} + \frac{92}{27} \delta^{pa} \delta^{bc} (Y_u Y_u^\dagger)^{dr} + 4 \delta^{pa} \delta^{rd} (Y_u Y_u^\dagger)^{bc} + 68 \delta^{pa} \delta^{rb} (Y_u Y_u^\dagger)^{dc} - \frac{4}{3} \delta^{pr} \delta^{bc} (Y_u Y_u^\dagger)^{da} - \frac{4}{3} \delta^{pa} \delta^{rd} \delta^{bc} \text{Tr} [Y_u^\dagger Y_u] \\
& - 68 \delta^{pa} \delta^{rb} (Y_d Y_d^\dagger)^{dc} \left. \right) + 2 \delta^{pa} \delta^{rd} (Y_d Y_d^\dagger Y_u Y_u^\dagger)^{bc} + 2 \delta^{pa} \delta^{rd} (Y_u Y_u^\dagger Y_d Y_d^\dagger)^{bc} + 5 \delta^{rd} (Y_u Y_u^\dagger)^{pa} (Y_u Y_u^\dagger)^{bc} + 5 \delta^{pa} (Y_u Y_u^\dagger)^{bc} (Y_u Y_u^\dagger)^{dr} + 6 \delta^{rd} (Y_d Y_d^\dagger)^{ba} (Y_u Y_u^\dagger)^{pc} \\
& + 6 \delta^{pa} (Y_d Y_d^\dagger)^{dc} (Y_u Y_u^\dagger)^{br} + 36 \delta^{pa} \delta^{rb} (Y_d Y_d^\dagger Y_d Y_d^\dagger)^{dc} - \delta^{pa} \delta^{rd} (Y_d Y_d^\dagger Y_d Y_d^\dagger)^{bc} - \frac{130}{81} \delta^{pa} \delta^{rd} \delta^{bc} g_s^2 g_L^2 - 3 \delta^{rd} (Y_d Y_d^\dagger)^{pa} (Y_d Y_d^\dagger)^{bc} \\
& - 3 \delta^{pa} (Y_d Y_d^\dagger)^{bc} (Y_d Y_d^\dagger)^{dr} - 3 \delta^{rd} (Y_d Y_d^\dagger)^{pa} (Y_u Y_u^\dagger)^{bc} - 3 \delta^{pa} (Y_d Y_d^\dagger)^{dr} (Y_u Y_u^\dagger)^{bc} - 6 \delta^{rb} (Y_u Y_u^\dagger)^{pa} (Y_u Y_u^\dagger)^{dc} - 6 \delta^{pa} (Y_u Y_u^\dagger)^{br} (Y_u Y_u^\dagger)^{dc} \\
& - 17 \delta^{pa} \delta^{rd} (Y_u Y_u^\dagger Y_u Y_u^\dagger)^{bc} - 36 \delta^{pa} \delta^{rb} (Y_u Y_u^\dagger Y_u Y_u^\dagger)^{dc} \left. \right\} C_{qq}^{(\parallel)abcd} + \left\{ g_L^4 \left( \frac{7}{3} \delta^{pa} \delta^{rd} \delta^{bc} - \frac{37}{3} \delta^{pa} \delta^{rb} \delta^{cd} \right) + g_s^2 g_L^2 \left( \frac{136}{81} \delta^{pa} \delta^{rd} \delta^{bc} - 6 \delta^{pa} \delta^{rb} \delta^{cd} \right) \right. \\
& + g_Y^2 g_L^2 \left( \frac{265}{243} \delta^{pa} \delta^{rd} \delta^{bc} - \frac{64}{81} \delta^{pa} \delta^{rb} \delta^{cd} \right) + g_Y^4 \left( \frac{8}{81} \delta^{pr} \delta^{ad} \delta^{bc} - \frac{8}{243} \delta^{pa} \delta^{rb} \delta^{cd} - \frac{58}{729} \delta^{pa} \delta^{rd} \delta^{bc} \right) + g_Y^2 g_s^2 \left( \frac{44}{243} \delta^{pa} \delta^{rd} \delta^{bc} + 2 \delta^{pa} \delta^{rb} \delta^{cd} \right. \\
& - \frac{8}{27} \delta^{pr} \delta^{ad} \delta^{bc} \left. \right) + g_L^2 \left( 2 \delta^{rb} \delta^{cd} (Y_u Y_u^\dagger)^{pa} + 2 \delta^{pa} \delta^{cd} (Y_u Y_u^\dagger)^{br} + 3 \delta^{rb} \delta^{cd} (Y_d Y_d^\dagger)^{pa} + 3 \delta^{pa} \delta^{cd} (Y_d Y_d^\dagger)^{br} + 35 \delta^{pa} \delta^{rb} (Y_d Y_d^\dagger)^{dc} - \frac{7}{2} \delta^{pa} \delta^{rd} (Y_u Y_u^\dagger)^{bc} \right. \\
& - \frac{29}{2} \delta^{pa} \delta^{rb} (Y_u Y_u^\dagger)^{dc} - \frac{37}{2} \delta^{pa} \delta^{rd} (Y_d Y_d^\dagger)^{bc} \left. \right) + g_Y^2 \left( \frac{16}{81} \delta^{rd} \delta^{bc} (Y_u Y_u^\dagger)^{pa} + \frac{16}{81} \delta^{pa} \delta^{bc} (Y_u Y_u^\dagger)^{dr} + \frac{8}{9} \delta^{pr} \delta^{bc} (Y_u Y_u^\dagger)^{da} + \frac{31}{18} \delta^{pa} \delta^{rd} (Y_u Y_u^\dagger)^{bc} \right. \\
& - \frac{11}{18} \delta^{pa} \delta^{rd} (Y_d Y_d^\dagger)^{bc} - \frac{8}{9} \delta^{pr} \delta^{bc} (Y_d Y_d^\dagger)^{da} - \frac{25}{27} \delta^{rb} \delta^{cd} (Y_u Y_u^\dagger)^{pa} - \frac{25}{27} \delta^{pa} \delta^{cd} (Y_u Y_u^\dagger)^{br} - \frac{13}{2} \delta^{pa} \delta^{rb} (Y_u Y_u^\dagger)^{dc} \left. \right) + g_s^2 \left( \frac{8}{3} \delta^{pr} \delta^{bc} (Y_d Y_d^\dagger)^{da} \right. \\
& + \frac{8}{3} \delta^{pa} \delta^{rd} \delta^{bc} \text{Tr} [Y_d^\dagger Y_d] + 4 \delta^{pa} \delta^{rd} (Y_u Y_u^\dagger)^{bc} + \frac{184}{27} \delta^{rd} \delta^{bc} (Y_u Y_u^\dagger)^{pa} + \frac{184}{27} \delta^{pa} \delta^{bc} (Y_u Y_u^\dagger)^{dr} + 68 \delta^{pa} \delta^{rb} (Y_u Y_u^\dagger)^{dc} - \frac{8}{3} \delta^{pr} \delta^{bc} (Y_u Y_u^\dagger)^{da} \\
& - \frac{8}{3} \delta^{pa} \delta^{rd} \delta^{bc} \text{Tr} [Y_u^\dagger Y_u] - 4 \delta^{pa} \delta^{rd} (Y_d Y_d^\dagger)^{bc} \left. \right) + 3 \delta^{rb} (Y_d Y_d^\dagger)^{pa} (Y_d Y_d^\dagger)^{dc} + 3 \delta^{pa} (Y_d Y_d^\dagger)^{br} (Y_d Y_d^\dagger)^{dc} + 3 \delta^{rb} (Y_d Y_d^\dagger)^{pa} (Y_u Y_u^\dagger)^{dc} + 3 \delta^{pa} (Y_d Y_d^\dagger)^{br} (Y_u Y_u^\dagger)^{dc} \\
& + 3 \delta^{pa} \delta^{rb} (Y_d Y_d^\dagger Y_d Y_d^\dagger)^{dc} + 4 \delta^{rd} (Y_u Y_u^\dagger)^{pa} (Y_u Y_u^\dagger)^{bc} + 4 \delta^{pa} (Y_u Y_u^\dagger)^{bc} (Y_u Y_u^\dagger)^{dr} + 16 \delta^{pa} \delta^{rd} (Y_d Y_d^\dagger Y_d Y_d^\dagger)^{bc} - 3 \delta^{rd} (Y_d Y_d^\dagger)^{ba} (Y_u Y_u^\dagger)^{pc} \\
& - 3 \delta^{pa} (Y_d Y_d^\dagger)^{dc} (Y_u Y_u^\dagger)^{br} - 4 \delta^{rb} (Y_d Y_d^\dagger)^{da} (Y_u Y_u^\dagger)^{pc} - 4 \delta^{pa} (Y_d Y_d^\dagger)^{bc} (Y_u Y_u^\dagger)^{dr} - 9 \delta^{rb} (Y_u Y_u^\dagger)^{pa} (Y_u Y_u^\dagger)^{dc} - 9 \delta^{pa} (Y_u Y_u^\dagger)^{br} (Y_u Y_u^\dagger)^{dc} \\
& - 16 \delta^{pa} \delta^{rd} (Y_u Y_u^\dagger Y_u Y_u^\dagger)^{bc} - 33 \delta^{pa} \delta^{rb} (Y_u Y_u^\dagger Y_u Y_u^\dagger)^{dc} \left. \right\} C_{qq}^{(\times)abcd} + \left\{ \frac{1}{6} \delta^{pc} \delta^{rd} \delta^{ab} g_L^4 + \delta^{rd} (Y_e Y_e^\dagger)^{ba} (Y_u Y_u^\dagger)^{pc} + \delta^{pc} (Y_e Y_e^\dagger)^{ba} (Y_u Y_u^\dagger)^{dr} \right. \\
& + g_Y^2 \left( \frac{25}{27} \delta^{rd} \delta^{ab} (Y_u Y_u^\dagger)^{pc} + \frac{25}{27} \delta^{pc} \delta^{ab} (Y_u Y_u^\dagger)^{dr} - \frac{25}{4} \delta^{pc} \delta^{rd} (Y_e Y_e^\dagger)^{ba} \right) + 6 \delta^{pc} \delta^{rd} (Y_e Y_e^\dagger Y_e Y_e^\dagger)^{ba} - \frac{118}{243} \delta^{pc} \delta^{rd} \delta^{ab} g_Y^4 - \frac{277}{162} \delta^{pc} \delta^{rd} \delta^{ab} g_Y^2 g_L^2
\end{aligned}$$

$$\begin{aligned}
& -\frac{7}{4}\delta^{pc}\delta^{rd}g_L^2(Y_eY_e^\dagger)^{ba}\left\{C_{\ell q}^{(\parallel)abcd}\right\} + \left\{\frac{1}{2}\delta^{rd}(Y_dY_d^\dagger)^{pc}(Y_eY_e^\dagger)^{ba} + \frac{1}{2}\delta^{pc}(Y_dY_d^\dagger)^{dr}(Y_eY_e^\dagger)^{ba} + \frac{1}{2}\delta^{pc}\delta^{rd}(Y_eY_e^\dagger Y_eY_e^\dagger)^{ba} + g_L^2\left(\frac{1}{3}\delta^{rd}\delta^{ab}(Y_uY_u^\dagger)^{pc}\right.\right. \\
& + \frac{1}{3}\delta^{pc}\delta^{ab}(Y_uY_u^\dagger)^{dr} + \frac{1}{2}\delta^{rd}\delta^{ab}(Y_dY_d^\dagger)^{pc} + \frac{1}{2}\delta^{pc}\delta^{ab}(Y_dY_d^\dagger)^{dr} + \frac{35}{6}\delta^{pc}\delta^{rd}(Y_eY_e^\dagger)^{ba}) + g_Y^2\left(\frac{25}{54}\delta^{rd}\delta^{ab}(Y_uY_u^\dagger)^{pc} + \frac{25}{54}\delta^{pc}\delta^{ab}(Y_uY_u^\dagger)^{dr} + \frac{2}{3}\delta^{pc}\delta^{rd}(Y_eY_e^\dagger)^{ba}\right) \\
& \left.\left.-\frac{59}{243}\delta^{pc}\delta^{rd}\delta^{ab}g_Y^4 - \frac{1}{2}\delta^{rd}(Y_eY_e^\dagger)^{ba}(Y_uY_u^\dagger)^{pc} - \frac{1}{2}\delta^{pc}(Y_eY_e^\dagger)^{ba}(Y_uY_u^\dagger)^{dr} - \frac{97}{81}\delta^{pc}\delta^{rd}\delta^{ab}g_Y^2g_L^2 - \frac{37}{18}\delta^{pc}\delta^{rd}\delta^{ab}g_L^4\right\}C_{\ell q}^{(\times)abcd}, \tag{9.8}
\end{aligned}$$

## 9.5 $C_{Hq}^{(\times)}$

$$\begin{aligned}
\beta_{C_{Hq}^{(\times)pr}}^{(1)} &= \left\{\frac{1}{6}\delta^{pr}g_L^2 + \frac{1}{2}\left(-(Y_dY_d^\dagger)^{pr} - (Y_uY_u^\dagger)^{pr}\right)\right\}C_{HD}^{(\parallel)} + \frac{2}{3}\delta^{pr}\delta^{ab}g_L^2C_{H\ell}^{(\times)ab} + 3\left\{\delta^{rb}(Y_dY_d^\dagger)^{pa} + \delta^{pa}(Y_dY_d^\dagger)^{br} - \delta^{rb}(Y_uY_u^\dagger)^{pa} - \delta^{pa}(Y_uY_u^\dagger)^{br}\right\}C_{Hq}^{(\parallel)ab} \\
&+ \left\{\frac{1}{3}g_L^2(6\delta^{pr}\delta^{ab} - 17\delta^{pa}\delta^{rb}) + \frac{1}{2}\left(4T_2\delta^{pa}\delta^{rb} + 5\delta^{rb}(Y_dY_d^\dagger)^{pa} + 5\delta^{pa}(Y_dY_d^\dagger)^{br} - \delta^{rb}(Y_uY_u^\dagger)^{pa} - \delta^{pa}(Y_uY_u^\dagger)^{br}\right)\right\}C_{Hq}^{(\times)ab} + \left\{\frac{4}{3}\delta^{pa}\delta^{rd}\delta^{bc}g_L^2\right. \\
&- 4\left(\delta^{pa}\delta^{rd}(Y_dY_d^\dagger)^{bc} + \delta^{pa}\delta^{rd}(Y_uY_u^\dagger)^{bc}\right)\left\}C_{qq}^{(\parallel)abcd} + \left\{4\delta^{pa}\delta^{rb}\delta^{cd}g_L^2 - 12\left(\delta^{pa}\delta^{rb}(Y_dY_d^\dagger)^{dc} + \delta^{pa}\delta^{rb}(Y_uY_u^\dagger)^{dc}\right)\right\}C_{qq}^{(\times)abcd} + \left\{\frac{2}{3}\delta^{pc}\delta^{rd}\delta^{ab}g_L^2\right. \\
&\left.- 2\delta^{pc}\delta^{rd}(Y_eY_e^\dagger)^{ba}\right\}C_{\ell q}^{(\times)abcd}, \tag{9.9}
\end{aligned}$$

$$\begin{aligned}
\beta_{C_{Hq}^{(\times)pr}}^{(2)} &= (Y_dY_d^\dagger)^{pr}T_{\ell H} + (Y_uY_u^\dagger)^{pr}T_{\ell H} - \frac{11}{3}\delta^{pr}g_L^2T_{\ell H} + \left\{\frac{7}{108}\delta^{pr}g_Y^2g_L^2 + \frac{1}{2}T_2(Y_dY_d^\dagger)^{pr} + \frac{1}{2}T_2(Y_uY_u^\dagger)^{pr} + \frac{3}{4}\delta^{pr}g_L^4 + \frac{3}{4}(Y_dY_d^\dagger Y_uY_u^\dagger)^{pr}\right. \\
&+ \frac{3}{4}(Y_uY_u^\dagger Y_dY_d^\dagger)^{pr} + \frac{5}{6}\delta^{pr}\lambda g_L^2 + g_s^2\left(\frac{8}{3}(Y_dY_d^\dagger)^{pr} + \frac{8}{3}(Y_uY_u^\dagger)^{pr}\right) + \frac{5}{4}(Y_dY_d^\dagger Y_dY_d^\dagger)^{pr} + \frac{5}{4}(Y_uY_u^\dagger Y_uY_u^\dagger)^{pr} - g_Y^2\left(\frac{121}{144}(Y_dY_d^\dagger)^{pr} + \frac{137}{144}(Y_uY_u^\dagger)^{pr}\right) \\
&- g_L^2\left(\frac{1}{6}T_2\delta^{pr} + \frac{51}{16}(Y_dY_d^\dagger)^{pr} + \frac{51}{16}(Y_uY_u^\dagger)^{pr}\right)\left\}C_{HD}^{(\parallel)} + \left\{\frac{59}{108}\delta^{pr}g_Y^2g_L^2 + \lambda\left(\frac{1}{2}(Y_dY_d^\dagger)^{pr} + \frac{1}{2}(Y_uY_u^\dagger)^{pr}\right) + \frac{7}{4}(Y_dY_d^\dagger Y_dY_d^\dagger)^{pr} + \frac{7}{4}(Y_uY_u^\dagger Y_uY_u^\dagger)^{pr}\right. \\
&- g_Y^2\left(\frac{2}{9}(Y_uY_u^\dagger)^{pr} + \frac{4}{3}(Y_dY_d^\dagger)^{pr}\right) - \frac{5}{4}(Y_dY_d^\dagger Y_uY_u^\dagger)^{pr} - \frac{5}{4}(Y_uY_u^\dagger Y_dY_d^\dagger)^{pr}\left\}C_{HD}^{(\times)} + \left\{\delta^{pr}g_Y^4g_L^2 + g_Y^4\left(\frac{11}{9}(Y_uY_u^\dagger)^{pr} - \frac{1}{9}(Y_dY_d^\dagger)^{pr}\right)\right\}C_{HB} + \left\{\delta^{pr}g_Y^2g_L^4\right. \\
&+ \frac{142}{3}\delta^{pr}g_L^6 - 12\delta^{pr}\lambda g_L^4\left\}C_{HW} + \left\{g_s^4\left(\frac{80}{3}(Y_dY_d^\dagger)^{pr} + \frac{80}{3}(Y_uY_u^\dagger)^{pr}\right) + 16\delta^{pr}g_s^4g_L^2\right\}C_{HG} + \left\{\frac{5}{12}\delta^{pr}g_Y^4g_L^2 - \frac{11}{12}\delta^{pr}g_Y^2g_L^4 - \delta^{pr}\lambda g_Y^2g_L^2\right. \\
&- g_Y^2g_L^2\left(\frac{1}{12}(Y_uY_u^\dagger)^{pr} + \frac{5}{12}(Y_dY_d^\dagger)^{pr}\right)\left\}C_{HWB} + \left\{g_L^6\left(12(Y_dY_d^\dagger)^{pr} + 12(Y_uY_u^\dagger)^{pr} - 6T_2\delta^{pr}\right) + 3\delta^{pr}g_Y^2g_L^6 - \frac{40}{3}\delta^{pr}g_L^8\right\}C_W + \left\{\frac{80}{3}\delta^{pr}g_s^6g_L^2\right.
\end{aligned}$$

$$\begin{aligned}
& -g_s^6 \left( 8(Y_d Y_d^\dagger)^{pr} + 8(Y_u Y_u^\dagger)^{pr} \right) \Big\} C_G + \left\{ \frac{3}{2} \delta^{pa} \lambda Y_u^{*rb} + \frac{3}{2} \delta^{pa} (Y_d^\dagger Y_d Y_u^\dagger)^{rb} - \delta^{pa} g_Y^2 Y_u^{*rb} \right\} C_{uH}^{ab} + C_{uH}^{*ab} \left\{ \frac{3}{2} \delta^{ra} \lambda Y_u^{pb} + \frac{3}{2} \delta^{ra} (Y_d Y_d^\dagger Y_u)^{pb} - \delta^{ra} g_Y^2 Y_u^{pb} \right\} \\
& + \left\{ \frac{3}{2} \delta^{pa} \lambda Y_d^{*rb} + \frac{3}{2} \delta^{pa} (Y_u^\dagger Y_u Y_d^\dagger)^{rb} - \frac{1}{2} \delta^{pa} g_Y^2 Y_d^{*rb} \right\} C_{dH}^{ab} + C_{dH}^{*ab} \left\{ \frac{3}{2} \delta^{ra} \lambda Y_d^{pb} + \frac{3}{2} \delta^{ra} (Y_u Y_u^\dagger Y_d)^{pb} - \frac{1}{2} \delta^{ra} g_Y^2 Y_d^{pb} \right\} + \frac{5}{2} \delta^{pr} g_Y^2 g_L^2 Y_e^{*ab} C_{eB}^{ab} \\
& + \frac{5}{2} \delta^{pr} g_Y^2 g_L^2 C_{eB}^{*ab} Y_e^{ab} + \left\{ \frac{25}{12} \delta^{pr} g_L^4 Y_e^{*ab} - \frac{1}{2} \delta^{pr} g_L^2 (Y_e^\dagger Y_e Y_e^\dagger)^{ab} \right\} C_{eW}^{ab} + C_{eW}^{*ab} \left\{ \frac{25}{12} \delta^{pr} g_L^4 Y_e^{ab} - \frac{1}{2} \delta^{pr} g_L^2 (Y_e Y_e^\dagger Y_e)^{ab} \right\} + \left\{ g_Y^2 g_L^2 \left( \frac{7}{6} \delta^{pr} Y_u^{*ab} \right. \right. \\
& - \frac{163}{72} \delta^{pa} Y_u^{*rb} \Big) + g_Y^2 \left( \frac{1}{6} Y_u^{*rb} (Y_d Y_d^\dagger)^{pa} + \frac{3}{2} T_2 \delta^{pa} Y_u^{*rb} + \frac{19}{6} \delta^{pa} (Y_u^\dagger Y_u Y_u^\dagger)^{rb} - \frac{5}{2} \delta^{pa} (Y_d^\dagger Y_d Y_u^\dagger)^{rb} \right) + 3 \delta^{pa} \lambda g_Y^2 Y_u^{*rb} + \frac{80}{9} \delta^{pa} g_Y^2 g_s^2 Y_u^{*rb} \\
& - \frac{2333}{216} \delta^{pa} g_Y^4 Y_u^{*rb} \Big\} C_{uB}^{ab} + C_{uB}^{*ab} \left\{ g_Y^2 g_L^2 \left( \frac{7}{6} \delta^{pr} Y_u^{ab} - \frac{163}{72} \delta^{ra} Y_u^{pb} \right) + g_Y^2 \left( \frac{1}{6} Y_u^{pb} (Y_d Y_d^\dagger)^{ar} + \frac{3}{2} T_2 \delta^{ra} Y_u^{pb} + \frac{19}{6} \delta^{ra} (Y_u Y_u^\dagger Y_u)^{pb} - \frac{5}{2} \delta^{ra} (Y_d Y_d^\dagger Y_u)^{pb} \right) \right. \\
& + 3 \delta^{ra} \lambda g_Y^2 Y_u^{pb} + \frac{80}{9} \delta^{ra} g_Y^2 g_s^2 Y_u^{pb} - \frac{2333}{216} \delta^{ra} g_Y^4 Y_u^{pb} \Big\} + \left\{ g_Y^2 g_L^2 \left( \frac{163}{144} \delta^{pa} Y_u^{*rb} + 5 \delta^{pr} Y_u^{*ab} \right) + g_L^4 \left( \frac{87}{16} \delta^{pa} Y_u^{*rb} + \frac{25}{4} \delta^{pr} Y_u^{*ab} \right) \right. \\
& + g_L^2 \left( \frac{3}{4} T_2 \delta^{pa} Y_u^{*rb} + \frac{15}{4} \delta^{pa} (Y_d^\dagger Y_d Y_u^\dagger)^{rb} - \frac{3}{4} \delta^{pa} (Y_u^\dagger Y_u Y_u^\dagger)^{rb} - \frac{3}{2} Y_u^{*rb} (Y_u Y_u^\dagger)^{pa} - \frac{3}{2} \delta^{pr} (Y_d^\dagger Y_d Y_u^\dagger)^{ab} - \frac{3}{2} \delta^{pr} (Y_u^\dagger Y_u Y_u^\dagger)^{ab} - \frac{11}{4} Y_u^{*rb} (Y_d Y_d^\dagger)^{pa} \right) \\
& + \frac{16}{3} \delta^{pa} g_s^2 g_L^2 Y_u^{*rb} - \frac{9}{2} \delta^{pa} \lambda g_L^2 Y_u^{*rb} \Big\} C_{uW}^{ab} + C_{uW}^{*ab} \left\{ g_Y^2 g_L^2 \left( \frac{163}{144} \delta^{ra} Y_u^{pb} + 5 \delta^{pr} Y_u^{ab} \right) + g_L^4 \left( \frac{87}{16} \delta^{ra} Y_u^{pb} + \frac{25}{4} \delta^{pr} Y_u^{ab} \right) + g_L^2 \left( \frac{3}{4} T_2 \delta^{ra} Y_u^{pb} \right. \right. \\
& + \frac{15}{4} \delta^{ra} (Y_d Y_d^\dagger Y_u)^{pb} - \frac{3}{4} \delta^{ra} (Y_u Y_u^\dagger Y_u)^{pb} - \frac{3}{2} Y_u^{pb} (Y_u Y_u^\dagger)^{ar} - \frac{3}{2} \delta^{pr} (Y_d Y_d^\dagger Y_u)^{ab} - \frac{3}{2} \delta^{pr} (Y_u Y_u^\dagger Y_u)^{ab} - \frac{11}{4} Y_u^{pb} (Y_d Y_d^\dagger)^{ar} \Big) + \frac{16}{3} \delta^{ra} g_s^2 g_L^2 Y_u^{pb} \\
& - \frac{9}{2} \delta^{ra} \lambda g_L^2 Y_u^{pb} \Big\} + \left\{ g_s^2 \left( \frac{4}{3} Y_u^{*rb} (Y_d Y_d^\dagger)^{pa} + \frac{16}{3} \delta^{pa} (Y_u^\dagger Y_u Y_u^\dagger)^{rb} - 4 \delta^{pa} (Y_d^\dagger Y_d Y_u^\dagger)^{rb} \right) - g_s^2 g_L^2 \left( \frac{58}{9} \delta^{pa} Y_u^{*rb} + \frac{32}{3} \delta^{pr} Y_u^{*ab} \right) - \frac{62}{27} \delta^{pa} g_Y^2 g_s^2 Y_u^{*rb} \right. \\
& - \frac{320}{9} \delta^{pa} g_s^4 Y_u^{*rb} \Big\} C_{uG}^{ab} + C_{uG}^{*ab} \left\{ g_s^2 \left( \frac{4}{3} Y_u^{pb} (Y_d Y_d^\dagger)^{ar} + \frac{16}{3} \delta^{ra} (Y_u Y_u^\dagger Y_u)^{pb} - 4 \delta^{ra} (Y_d Y_d^\dagger Y_u)^{pb} \right) - g_s^2 g_L^2 \left( \frac{58}{9} \delta^{ra} Y_u^{pb} + \frac{32}{3} \delta^{pr} Y_u^{ab} \right) - \frac{62}{27} \delta^{ra} g_Y^2 g_s^2 Y_u^{pb} \right. \\
& - \frac{320}{9} \delta^{ra} g_s^4 Y_u^{pb} \Big\} + \left\{ g_Y^2 g_L^2 \left( \frac{47}{72} \delta^{pa} Y_d^{*rb} + \frac{13}{6} \delta^{pr} Y_d^{*ab} \right) + g_Y^2 \left( \frac{1}{6} Y_d^{*rb} (Y_u Y_u^\dagger)^{pa} + \frac{3}{2} \delta^{pa} (Y_u^\dagger Y_u Y_d^\dagger)^{rb} - \frac{3}{2} T_2 \delta^{pa} Y_d^{*rb} - \frac{11}{6} \delta^{pa} (Y_d^\dagger Y_d Y_d^\dagger)^{rb} \right) \right. \\
& + \frac{2509}{216} \delta^{pa} g_Y^4 Y_d^{*rb} - \frac{16}{9} \delta^{pa} g_Y^2 g_s^2 Y_d^{*rb} - 3 \delta^{pa} \lambda g_Y^2 Y_d^{*rb} \Big\} C_{dB}^{ab} + C_{dB}^{*ab} \left\{ g_Y^2 g_L^2 \left( \frac{47}{72} \delta^{ra} Y_d^{pb} + \frac{13}{6} \delta^{pr} Y_d^{ab} \right) + g_Y^2 \left( \frac{1}{6} Y_d^{pb} (Y_u Y_u^\dagger)^{ar} \right. \right. \\
& + \frac{3}{2} \delta^{ra} (Y_u Y_u^\dagger Y_d)^{pb} - \frac{3}{2} T_2 \delta^{ra} Y_d^{pb} - \frac{11}{6} \delta^{ra} (Y_d Y_d^\dagger Y_d)^{pb} \Big) + \frac{2509}{216} \delta^{ra} g_Y^4 Y_d^{pb} - \frac{16}{9} \delta^{ra} g_Y^2 g_s^2 Y_d^{pb} - 3 \delta^{ra} \lambda g_Y^2 Y_d^{pb} \Big\} + \left\{ \frac{31}{144} \delta^{pa} g_Y^2 g_L^2 Y_d^{*rb} \right. \\
& + g_L^4 \left( \frac{87}{16} \delta^{pa} Y_d^{*rb} + \frac{25}{4} \delta^{pr} Y_d^{*ab} \right) + g_L^2 \left( \frac{3}{4} T_2 \delta^{pa} Y_d^{*rb} + \frac{15}{4} \delta^{pa} (Y_u^\dagger Y_u Y_d^\dagger)^{rb} - \frac{3}{4} \delta^{pa} (Y_d^\dagger Y_d Y_d^\dagger)^{rb} - \frac{3}{2} Y_d^{*rb} (Y_d Y_d^\dagger)^{pa} - \frac{3}{2} \delta^{pr} (Y_d^\dagger Y_d Y_d^\dagger)^{ab} \right.
\end{aligned}$$

$$\begin{aligned}
& -\frac{3}{2}\delta^{pr}(Y_u^\dagger Y_u Y_d^\dagger)^{ab} - \frac{11}{4}Y_d^{*rb}(Y_u Y_u^\dagger)^{pa}) + \frac{16}{3}\delta^{pa}g_s^2g_L^2Y_d^{*rb} - \frac{9}{2}\delta^{pa}\lambda g_L^2Y_d^{*rb} \Big\} C_{dW}^{ab} + C_{dW}^{*ab} \Big\{ \frac{31}{144}\delta^{ra}g_Y^2g_L^2Y_d^{pb} + g_L^4\Big(\frac{87}{16}\delta^{ra}Y_d^{pb} + \frac{25}{4}\delta^{pr}Y_d^{ab}\Big) \\
& + g_L^2\Big(\frac{3}{4}T_2\delta^{ra}Y_d^{pb} + \frac{15}{4}\delta^{ra}(Y_u Y_u^\dagger Y_d)^{pb} - \frac{3}{4}\delta^{ra}(Y_d Y_d^\dagger Y_d)^{pb} - \frac{3}{2}Y_d^{pb}(Y_d Y_d^\dagger)^{ar} - \frac{3}{2}\delta^{pr}(Y_d Y_d^\dagger Y_d)^{ab} - \frac{3}{2}\delta^{pr}(Y_u Y_u^\dagger Y_d)^{ab} - \frac{11}{4}Y_d^{pb}(Y_u Y_u^\dagger)^{ar}\Big) \\
& + \frac{16}{3}\delta^{ra}g_s^2g_L^2Y_d^{pb} - \frac{9}{2}\delta^{ra}\lambda g_L^2Y_d^{pb} \Big\} + \Big\{ g_s^2\Big(\frac{4}{3}Y_d^{*rb}(Y_u Y_u^\dagger)^{pa} + \frac{16}{3}\delta^{pa}(Y_d^\dagger Y_d Y_d^\dagger)^{rb} - 4\delta^{pa}(Y_u^\dagger Y_u Y_d^\dagger)^{rb}\Big) - g_s^2g_L^2\Big(\frac{58}{9}\delta^{pa}Y_d^{*rb} + \frac{32}{3}\delta^{pr}Y_d^{*ab}\Big) \\
& - \frac{86}{27}\delta^{pa}g_Y^2g_s^2Y_d^{*rb} - \frac{320}{9}\delta^{pa}g_s^4Y_d^{*rb} \Big\} C_{dG}^{ab} + C_{dG}^{*ab} \Big\{ g_s^2\Big(\frac{4}{3}Y_d^{pb}(Y_u Y_u^\dagger)^{ar} + \frac{16}{3}\delta^{ra}(Y_d Y_d^\dagger Y_d)^{pb} - 4\delta^{ra}(Y_u Y_u^\dagger Y_d)^{pb}\Big) - g_s^2g_L^2\Big(\frac{58}{9}\delta^{ra}Y_d^{pb} \\
& + \frac{32}{3}\delta^{pr}Y_d^{ab}\Big) - \frac{86}{27}\delta^{ra}g_Y^2g_s^2Y_d^{pb} - \frac{320}{9}\delta^{ra}g_s^4Y_d^{pb} \Big\} + \Big\{ \frac{29}{54}\delta^{pr}\delta^{ab}g_Y^2g_L^2 + g_Y^2\Big(\frac{1}{2}\delta^{ab}(Y_d Y_d^\dagger)^{pr} - \frac{11}{18}\delta^{ab}(Y_u Y_u^\dagger)^{pr}\Big) - \frac{1}{2}(Y_d Y_d^\dagger)^{pr}(Y_e Y_e^\dagger)^{ba} \\
& - \frac{1}{2}(Y_e Y_e^\dagger)^{ba}(Y_u Y_u^\dagger)^{pr} - \frac{11}{18}\delta^{pr}g_L^2(Y_e Y_e^\dagger)^{ba} \Big\} C_{H\ell}^{(\parallel)ab} + \Big\{ \frac{1}{2}(Y_d Y_d^\dagger)^{pr}(Y_e Y_e^\dagger)^{ba} + \frac{1}{2}(Y_e Y_e^\dagger)^{ba}(Y_u Y_u^\dagger)^{pr} + g_Y^2\Big(\frac{1}{4}\delta^{ab}(Y_d Y_d^\dagger)^{pr} - \frac{11}{36}\delta^{ab}(Y_u Y_u^\dagger)^{pr}\Big) \\
& + \frac{59}{12}\delta^{pr}\delta^{ab}g_L^4 - \frac{25}{108}\delta^{pr}\delta^{ab}g_Y^2g_L^2 - g_L^2\Big(\frac{3}{4}\delta^{ab}(Y_d Y_d^\dagger)^{pr} + \frac{3}{4}\delta^{ab}(Y_u Y_u^\dagger)^{pr} + \frac{20}{9}\delta^{pr}(Y_e Y_e^\dagger)^{ba}\Big) \Big\} C_{H\ell}^{(\times)ab} + \Big\{ \frac{5}{18}\delta^{pr}g_L^2(Y_e^\dagger Y_e)^{ba} + \frac{1}{2}(Y_e^\dagger Y_e)^{ba}(Y_d Y_d^\dagger)^{pr} \\
& + \frac{1}{2}(Y_e^\dagger Y_e)^{ba}(Y_u Y_u^\dagger)^{pr} + \frac{29}{54}\delta^{pr}\delta^{ab}g_Y^2g_L^2 + g_Y^2\Big(\frac{1}{2}\delta^{ab}(Y_d Y_d^\dagger)^{pr} - \frac{11}{18}\delta^{ab}(Y_u Y_u^\dagger)^{pr}\Big) \Big\} C_{He}^{ab} + \Big\{ g_s^2\Big(\frac{20}{3}\delta^{rb}(Y_d Y_d^\dagger)^{pa} + \frac{20}{3}\delta^{pa}(Y_d Y_d^\dagger)^{br} - \frac{20}{3}\delta^{rb}(Y_u Y_u^\dagger)^{pa} \\
& - \frac{20}{3}\delta^{pa}(Y_u Y_u^\dagger)^{br}\Big) + g_Y^2\Big(\frac{11}{18}\delta^{ab}(Y_u Y_u^\dagger)^{pr} + \frac{203}{108}\delta^{rb}(Y_d Y_d^\dagger)^{pa} + \frac{203}{108}\delta^{pa}(Y_d Y_d^\dagger)^{br} - \frac{25}{108}\delta^{rb}(Y_u Y_u^\dagger)^{pa} - \frac{25}{108}\delta^{pa}(Y_u Y_u^\dagger)^{br} - \frac{1}{2}\delta^{ab}(Y_d Y_d^\dagger)^{pr}\Big) \\
& + \lambda\Big(3\delta^{rb}(Y_u Y_u^\dagger)^{pa} + 3\delta^{pa}(Y_u Y_u^\dagger)^{br} - 3\delta^{rb}(Y_d Y_d^\dagger)^{pa} - 3\delta^{pa}(Y_d Y_d^\dagger)^{br}\Big) + g_L^2\Big(\frac{11}{6}\delta^{pr}(Y_u Y_u^\dagger)^{ba} + \frac{68}{9}\delta^{rb}(Y_d Y_d^\dagger)^{pa} + \frac{68}{9}\delta^{pa}(Y_d Y_d^\dagger)^{br} - \frac{11}{6}\delta^{pr}(Y_d Y_d^\dagger)^{ba} \\
& - \frac{68}{9}\delta^{rb}(Y_u Y_u^\dagger)^{pa} - \frac{68}{9}\delta^{pa}(Y_u Y_u^\dagger)^{br}\Big) + \frac{3}{2}(Y_d Y_d^\dagger)^{pr}(Y_u Y_u^\dagger)^{ba} + \frac{3}{2}(Y_u Y_u^\dagger)^{pr}(Y_u Y_u^\dagger)^{ba} + \frac{5}{2}\delta^{pa}(Y_d Y_d^\dagger Y_u Y_u^\dagger)^{br} + \frac{5}{2}\delta^{rb}(Y_u Y_u^\dagger Y_d Y_d^\dagger)^{pa} + \frac{7}{2}T_2\delta^{rb}(Y_u Y_u^\dagger)^{pa} \\
& + \frac{7}{2}T_2\delta^{pa}(Y_u Y_u^\dagger)^{br} + \frac{25}{4}\delta^{rb}(Y_u Y_u^\dagger Y_u Y_u^\dagger)^{pa} + \frac{25}{4}\delta^{pa}(Y_u Y_u^\dagger Y_u Y_u^\dagger)^{br} - g_Y^2g_L^2\Big(\frac{29}{54}\delta^{pr}\delta^{ab} + \frac{347}{81}\delta^{pa}\delta^{rb}\Big) - \frac{3}{2}(Y_d Y_d^\dagger)^{pr}(Y_d Y_d^\dagger)^{ba} - \frac{3}{2}(Y_d Y_d^\dagger)^{ba}(Y_u Y_u^\dagger)^{pr} \\
& - \frac{5}{2}\delta^{rb}(Y_d Y_d^\dagger Y_u Y_u^\dagger)^{pa} - \frac{5}{2}\delta^{pa}(Y_u Y_u^\dagger Y_d Y_d^\dagger)^{br} - \frac{7}{2}T_2\delta^{rb}(Y_d Y_d^\dagger)^{pa} - \frac{7}{2}T_2\delta^{pa}(Y_d Y_d^\dagger)^{br} - \frac{25}{4}\delta^{rb}(Y_d Y_d^\dagger Y_d Y_d^\dagger)^{pa} - \frac{25}{4}\delta^{pa}(Y_d Y_d^\dagger Y_d Y_d^\dagger)^{br} \Big\} C_{Hq}^{(\parallel)ab} \\
& + \Big\{ \frac{3}{4}\delta^{rb}(Y_d Y_d^\dagger Y_d Y_d^\dagger)^{pa} + \frac{3}{4}\delta^{pa}(Y_d Y_d^\dagger Y_d Y_d^\dagger)^{br} + g_Y^2g_L^2\Big(\frac{97}{108}\delta^{pr}\delta^{ab} - \frac{106}{81}\delta^{pa}\delta^{rb}\Big) + g_s^2g_L^2\Big(8\delta^{pr}\delta^{ab} - 8\delta^{pa}\delta^{rb}\Big) + g_L^4\Big(\frac{59}{4}\delta^{pr}\delta^{ab} - \frac{239}{18}\delta^{pa}\delta^{rb}\Big) \\
& + g_L^2\Big(\frac{59}{12}T_2\delta^{pa}\delta^{rb} + \frac{941}{144}\delta^{rb}(Y_u Y_u^\dagger)^{pa} + \frac{941}{144}\delta^{pa}(Y_u Y_u^\dagger)^{br} + \frac{2029}{144}\delta^{rb}(Y_d Y_d^\dagger)^{pa} + \frac{2029}{144}\delta^{pa}(Y_d Y_d^\dagger)^{br} - \frac{9}{4}\delta^{ab}(Y_d Y_d^\dagger)^{pr} - \frac{9}{4}\delta^{ab}(Y_u Y_u^\dagger)^{pr} \\
& - \frac{29}{6}\delta^{pr}(Y_u Y_u^\dagger)^{ba} - \frac{20}{3}\delta^{pr}(Y_d Y_d^\dagger)^{ba}\Big) + g_Y^2\Big(\frac{73}{432}\delta^{rb}(Y_u Y_u^\dagger)^{pa} + \frac{73}{432}\delta^{pa}(Y_u Y_u^\dagger)^{br} + \frac{11}{36}\delta^{ab}(Y_u Y_u^\dagger)^{pr} + \frac{31}{12}\delta^{pa}\delta^{rb}\text{Tr}[Y_u^\dagger Y_u] + \frac{1897}{432}\delta^{rb}(Y_d Y_d^\dagger)^{pa}
\end{aligned}$$

$$\begin{aligned}
& + \frac{1897}{432} \delta^{pa} (Y_d Y_d^\dagger)^{br} + \frac{19}{4} \delta^{pa} \delta^{rb} \text{Tr} [Y_e^\dagger Y_e] - \frac{1}{4} \delta^{ab} (Y_d Y_d^\dagger)^{pr} - \frac{29}{12} \delta^{pa} \delta^{rb} \text{Tr} [Y_d^\dagger Y_d] \Big) + g_s^2 \Big( 40 \delta^{pa} \delta^{rb} \text{Tr} [Y_d^\dagger Y_d] + 40 \delta^{pa} \delta^{rb} \text{Tr} [Y_u^\dagger Y_u] \\
& - \frac{20}{3} \delta^{rb} (Y_u Y_u^\dagger)^{pa} - \frac{20}{3} \delta^{pa} (Y_u Y_u^\dagger)^{br} \Big) + \frac{3}{2} (Y_d Y_d^\dagger)^{pr} (Y_d Y_d^\dagger)^{ba} + \frac{3}{2} (Y_d Y_d^\dagger)^{ba} (Y_u Y_u^\dagger)^{pr} + \frac{7}{4} \delta^{pa} (Y_d Y_d^\dagger Y_u Y_u^\dagger)^{br} + \frac{7}{4} \delta^{rb} (Y_u Y_u^\dagger Y_d Y_d^\dagger)^{pa} + 3 (Y_d Y_d^\dagger)^{pr} (Y_u Y_u^\dagger)^{ba} \\
& + 3 (Y_u Y_u^\dagger)^{pr} (Y_u Y_u^\dagger)^{ba} + 7 \delta^{rb} (Y_u Y_u^\dagger Y_u Y_u^\dagger)^{pa} + 7 \delta^{pa} (Y_u Y_u^\dagger Y_u Y_u^\dagger)^{br} - \frac{1}{4} \text{T}_2 \delta^{rb} (Y_u Y_u^\dagger)^{pa} - \frac{1}{4} \text{T}_2 \delta^{pa} (Y_u Y_u^\dagger)^{br} - \frac{1}{3} \delta^{pa} \delta^{rb} g_Y^4 - \frac{3}{4} \delta^{rb} (Y_d Y_d^\dagger Y_u Y_u^\dagger)^{pa} \\
& - \frac{3}{4} \delta^{pa} (Y_u Y_u^\dagger Y_d Y_d^\dagger)^{br} - \lambda \Big( 3 \delta^{rb} (Y_u Y_u^\dagger)^{pa} + 3 \delta^{pa} (Y_u Y_u^\dagger)^{br} + 6 \delta^{rb} (Y_d Y_d^\dagger)^{pa} + 6 \delta^{pa} (Y_d Y_d^\dagger)^{br} \Big) - \frac{7}{4} (Y_d Y_d^\dagger)^{br} (Y_u Y_u^\dagger)^{pa} - \frac{7}{4} (Y_d Y_d^\dagger)^{pa} (Y_u Y_u^\dagger)^{br} \\
& - \frac{15}{4} \text{T}_2 \delta^{rb} (Y_d Y_d^\dagger)^{pa} - \frac{15}{4} \text{T}_2 \delta^{pa} (Y_d Y_d^\dagger)^{br} - 5 \text{T}_4 \delta^{pa} \delta^{rb} \Big\} \mathcal{C}_{Hq}^{(\times)ab} + \Big\{ g_Y^2 \Big( \frac{7}{108} Y_u^{*rb} Y_u^{pa} + \frac{11}{9} \delta^{ab} (Y_u Y_u^\dagger)^{pr} - \delta^{ab} (Y_d Y_d^\dagger)^{pr} \Big) + \frac{5}{4} Y_u^{pa} (Y_d^\dagger Y_d Y_u^\dagger)^{rb} \\
& + \frac{5}{4} Y_u^{*rb} (Y_d Y_d^\dagger Y_u)^{pa} + \frac{16}{3} g_s^2 Y_u^{*rb} Y_u^{pa} - \frac{1}{12} Y_u^{pa} (Y_u^\dagger Y_u Y_u^\dagger)^{rb} - \frac{1}{12} Y_u^{*rb} (Y_u Y_u^\dagger Y_u)^{pa} - g_L^2 \Big( \frac{3}{4} Y_u^{*rb} Y_u^{pa} + \frac{5}{6} \delta^{pr} (Y_u^\dagger Y_u)^{ba} \Big) - \frac{29}{27} \delta^{pr} \delta^{ab} g_Y^2 g_L^2 \\
& - \frac{3}{2} (Y_u^\dagger Y_u)^{ba} (Y_d Y_d^\dagger)^{pr} - \frac{3}{2} (Y_u^\dagger Y_u)^{ba} (Y_u Y_u^\dagger)^{pr} \Big\} \mathcal{C}_{Hu}^{ab} + \Big\{ \frac{1}{12} Y_d^{pa} (Y_d^\dagger Y_d Y_d^\dagger)^{rb} + \frac{1}{12} Y_d^{*rb} (Y_d Y_d^\dagger Y_d)^{pa} + \frac{29}{54} \delta^{pr} \delta^{ab} g_Y^2 g_L^2 + g_L^2 \Big( \frac{3}{4} Y_d^{*rb} Y_d^{pa} + \frac{5}{6} \delta^{pr} (Y_d^\dagger Y_d)^{ba} \Big) \\
& + g_Y^2 \Big( \frac{49}{108} Y_d^{*rb} Y_d^{pa} + \frac{1}{2} \delta^{ab} (Y_d Y_d^\dagger)^{pr} - \frac{11}{18} \delta^{ab} (Y_u Y_u^\dagger)^{pr} \Big) + \frac{3}{2} (Y_d^\dagger Y_d)^{ba} (Y_d Y_d^\dagger)^{pr} + \frac{3}{2} (Y_d^\dagger Y_d)^{ba} (Y_u Y_u^\dagger)^{pr} - \frac{5}{4} Y_d^{pa} (Y_u^\dagger Y_u Y_d^\dagger)^{rb} - \frac{5}{4} Y_d^{*rb} (Y_u Y_u^\dagger Y_d)^{pa} \\
& - \frac{16}{3} g_s^2 Y_d^{*rb} Y_d^{pa} \Big\} \mathcal{C}_{Hd}^{ab} + \Big\{ g_L^2 \Big( \frac{3}{4} Y_d^{*rb} Y_u^{pa} + \frac{5}{6} \delta^{pr} (Y_d^\dagger Y_u)^{ba} \Big) + \frac{3}{2} (Y_d^\dagger Y_u)^{ba} (Y_d Y_d^\dagger)^{pr} + \frac{3}{2} (Y_d^\dagger Y_u)^{ba} (Y_u Y_u^\dagger)^{pr} - \frac{1}{6} Y_u^{pa} (Y_u^\dagger Y_u Y_d^\dagger)^{rb} - \frac{1}{6} Y_d^{*rb} (Y_d Y_d^\dagger Y_u)^{pa} \\
& - \frac{13}{36} g_Y^2 Y_d^{*rb} Y_u^{pa} - Y_u^{pa} (Y_d^\dagger Y_d Y_d^\dagger)^{rb} - Y_d^{*rb} (Y_u Y_u^\dagger Y_u)^{pa} - \frac{16}{3} g_s^2 Y_d^{*rb} Y_u^{pa} \Big\} \mathcal{C}_{Hud}^{ab} + \mathcal{C}_{Hud}^{*ab} \Big\{ g_L^2 \Big( \frac{3}{4} Y_u^{*ra} Y_d^{pb} + \frac{5}{6} \delta^{pr} (Y_u^\dagger Y_d)^{ab} \Big) + \frac{3}{2} (Y_u^\dagger Y_d)^{ab} (Y_d Y_d^\dagger)^{pr} \\
& + \frac{3}{2} (Y_u^\dagger Y_d)^{ab} (Y_u Y_u^\dagger)^{pr} - \frac{1}{6} Y_d^{pb} (Y_d^\dagger Y_d Y_u^\dagger)^{ra} - \frac{1}{6} Y_u^{*ra} (Y_u Y_u^\dagger Y_d)^{pb} - \frac{13}{36} g_Y^2 Y_u^{*ra} Y_d^{pb} - Y_d^{pb} (Y_u^\dagger Y_u Y_u^\dagger)^{ra} - Y_u^{*ra} (Y_d Y_d^\dagger Y_d)^{pb} - \frac{16}{3} g_s^2 Y_u^{*ra} Y_d^{pb} \Big\} \\
& + \Big\{ \frac{7}{27} \delta^{ab} g_Y^2 Y_u^{*rd} Y_u^{pc} + Y_u^{*rd} Y_u^{pc} (Y_e Y_e^\dagger)^{ba} \Big\} \mathcal{C}_{lu}^{abcd} + \Big\{ \frac{1}{27} \delta^{ab} g_Y^2 Y_d^{*rd} Y_d^{pc} - Y_d^{*rd} Y_d^{pc} (Y_e Y_e^\dagger)^{ba} \Big\} \mathcal{C}_{ld}^{abcd} + \Big\{ \frac{34}{81} \delta^{pa} \delta^{rb} \delta^{cd} g_Y^2 g_L^2 + \delta^{rb} (Y_e^\dagger Y_e)^{dc} (Y_u Y_u^\dagger)^{pa} \\
& + \delta^{pa} (Y_e^\dagger Y_e)^{dc} (Y_u Y_u^\dagger)^{br} + g_Y^2 \Big( \frac{11}{27} \delta^{rb} \delta^{cd} (Y_d Y_d^\dagger)^{pa} + \frac{11}{27} \delta^{pa} \delta^{cd} (Y_d Y_d^\dagger)^{br} - \frac{25}{27} \delta^{rb} \delta^{cd} (Y_u Y_u^\dagger)^{pa} - \frac{25}{27} \delta^{pa} \delta^{cd} (Y_u Y_u^\dagger)^{br} \Big) + 6 \delta^{pa} \delta^{rb} g_L^2 (Y_e^\dagger Y_e)^{dc} \\
& - \delta^{rb} (Y_e^\dagger Y_e)^{dc} (Y_d Y_d^\dagger)^{pa} - \delta^{pa} (Y_e^\dagger Y_e)^{dc} (Y_d Y_d^\dagger)^{br} \Big\} \mathcal{C}_{qe}^{abcd} + \Big\{ \frac{2}{3} Y_u^{*rd} Y_u^{bc} (Y_u Y_u^\dagger)^{pa} + \frac{2}{3} Y_u^{*ad} Y_u^{pc} (Y_u Y_u^\dagger)^{br} + g_L^2 \Big( 18 \delta^{pa} \delta^{rb} (Y_u^\dagger Y_u)^{dc} - \frac{19}{36} \delta^{pa} Y_u^{*rd} Y_u^{bc} \\
& - \frac{19}{36} \delta^{rb} Y_u^{*ad} Y_u^{pc} \Big) + g_Y^2 \Big( \frac{3}{4} \delta^{pa} Y_u^{*rd} Y_u^{bc} + \frac{3}{4} \delta^{rb} Y_u^{*ad} Y_u^{pc} + \frac{50}{27} \delta^{rb} \delta^{cd} (Y_u Y_u^\dagger)^{pa} + \frac{50}{27} \delta^{pa} \delta^{cd} (Y_u Y_u^\dagger)^{br} - \frac{7}{27} \delta^{ab} Y_u^{*rd} Y_u^{pc} - \frac{22}{27} \delta^{rb} \delta^{cd} (Y_d Y_d^\dagger)^{pa} \\
& - \frac{22}{27} \delta^{pa} \delta^{cd} (Y_d Y_d^\dagger)^{br} \Big) + 3 \delta^{rb} (Y_u^\dagger Y_u)^{dc} (Y_d Y_d^\dagger)^{pa} + 3 \delta^{pa} (Y_u^\dagger Y_u)^{dc} (Y_d Y_d^\dagger)^{br} + 3 Y_u^{*rd} Y_u^{pc} (Y_d Y_d^\dagger)^{ba} - \frac{1}{2} \delta^{rb} Y_u^{pc} (Y_d^\dagger Y_d Y_u^\dagger)^{ad} - \frac{1}{2} \delta^{rb} Y_u^{pc} (Y_u^\dagger Y_u Y_u^\dagger)^{ad} \\
& - \frac{1}{2} \delta^{pa} Y_u^{*rd} (Y_d Y_d^\dagger Y_u)^{bc} - \frac{1}{2} \delta^{pa} Y_u^{*rd} (Y_u Y_u^\dagger Y_u)^{bc} - \frac{68}{81} \delta^{pa} \delta^{rb} \delta^{cd} g_Y^2 g_L^2 - Y_u^{*rd} Y_u^{bc} (Y_d Y_d^\dagger)^{pa} - Y_u^{*ad} Y_u^{pc} (Y_d Y_d^\dagger)^{br} - \delta^{pa} Y_u^{bc} (Y_d^\dagger Y_d Y_u^\dagger)^{rd}
\end{aligned}$$

$$\begin{aligned}
& -\delta^{rb}Y_u^{*ad}(Y_dY_d^\dagger Y_u)^{pc} - 3\delta^{rb}(Y_u^\dagger Y_u)^{dc}(Y_uY_u^\dagger)^{pa} - 3\delta^{pa}(Y_u^\dagger Y_u)^{dc}(Y_uY_u^\dagger)^{br} - 3Y_u^{*rd}Y_u^{pc}(Y_uY_u^\dagger)^{ba} \Big\} C_{qu}^{(\parallel)abcd} + \left\{ g_L^2 \left( 6\delta^{pa}\delta^{rb}(Y_u^\dagger Y_u)^{dc} - \frac{31}{12}\delta^{pa}Y_u^{*rd}Y_u^{bc} \right. \right. \\
& - \frac{31}{12}\delta^{rb}Y_u^{*ad}Y_u^{pc} \Big) + \delta^{rb}(Y_u^\dagger Y_u)^{dc}(Y_dY_d^\dagger)^{pa} + \delta^{pa}(Y_u^\dagger Y_u)^{dc}(Y_dY_d^\dagger)^{br} + Y_u^{*rd}Y_u^{pc}(Y_dY_d^\dagger)^{ba} + g_s^2 \left( \frac{2}{27}\delta^{rb}\delta^{cd}(Y_dY_d^\dagger)^{pa} + \frac{2}{27}\delta^{pa}\delta^{cd}(Y_dY_d^\dagger)^{br} \right. \\
& + \frac{2}{27}\delta^{rb}\delta^{cd}(Y_uY_u^\dagger)^{pa} + \frac{2}{27}\delta^{pa}\delta^{cd}(Y_uY_u^\dagger)^{br} - \frac{64}{27}\delta^{ab}Y_u^{*rd}Y_u^{pc} \Big) + g_Y^2 \left( \frac{50}{81}\delta^{rb}\delta^{cd}(Y_uY_u^\dagger)^{pa} + \frac{50}{81}\delta^{pa}\delta^{cd}(Y_uY_u^\dagger)^{br} + \frac{9}{4}\delta^{pa}Y_u^{*rd}Y_u^{bc} + \frac{9}{4}\delta^{rb}Y_u^{*ad}Y_u^{pc} \right. \\
& - \frac{7}{81}\delta^{ab}Y_u^{*rd}Y_u^{pc} - \frac{22}{81}\delta^{rb}\delta^{cd}(Y_dY_d^\dagger)^{pa} - \frac{22}{81}\delta^{pa}\delta^{cd}(Y_dY_d^\dagger)^{br} \Big) + \frac{3}{2}\delta^{rb}Y_u^{pc}(Y_d^\dagger Y_d Y_u^\dagger)^{ad} + \frac{3}{2}\delta^{rb}Y_u^{pc}(Y_u^\dagger Y_u Y_u^\dagger)^{ad} + \frac{3}{2}\delta^{pa}Y_u^{*rd}(Y_dY_d^\dagger Y_u)^{bc} \\
& + \frac{3}{2}\delta^{pa}Y_u^{*rd}(Y_uY_u^\dagger Y_u)^{bc} + 2Y_u^{*rd}Y_u^{bc}(Y_uY_u^\dagger)^{pa} + 2Y_u^{*ad}Y_u^{pc}(Y_uY_u^\dagger)^{br} - \frac{68}{243}\delta^{pa}\delta^{rb}\delta^{cd}g_Y^2g_L^2 - \delta^{rb}(Y_u^\dagger Y_u)^{dc}(Y_uY_u^\dagger)^{pa} - \delta^{pa}(Y_u^\dagger Y_u)^{dc}(Y_uY_u^\dagger)^{br} \\
& - Y_u^{*rd}Y_u^{pc}(Y_uY_u^\dagger)^{ba} - \frac{164}{81}\delta^{pa}\delta^{rb}\delta^{cd}g_s^2g_L^2 - 3Y_u^{*rd}Y_u^{bc}(Y_dY_d^\dagger)^{pa} - 3Y_u^{*ad}Y_u^{pc}(Y_dY_d^\dagger)^{br} - 3\delta^{pa}Y_u^{bc}(Y_d^\dagger Y_d Y_u^\dagger)^{rd} - 3\delta^{rb}Y_u^{*ad}(Y_dY_d^\dagger Y_u)^{pc} \Big\} C_{qu}^{(\times)abcd} \\
& + \left\{ \frac{34}{81}\delta^{pa}\delta^{rb}\delta^{cd}g_Y^2g_L^2 + \frac{2}{3}Y_d^{*rd}Y_d^{bc}(Y_dY_d^\dagger)^{pa} + \frac{2}{3}Y_d^{*ad}Y_d^{pc}(Y_dY_d^\dagger)^{br} + g_L^2 \left( 18\delta^{pa}\delta^{rb}(Y_d^\dagger Y_d)^{dc} - \frac{19}{36}\delta^{pa}Y_d^{*rd}Y_d^{bc} - \frac{19}{36}\delta^{rb}Y_d^{*ad}Y_d^{pc} \right) \right. \\
& + g_Y^2 \left( \frac{11}{27}\delta^{rb}\delta^{cd}(Y_dY_d^\dagger)^{pa} + \frac{11}{27}\delta^{pa}\delta^{cd}(Y_dY_d^\dagger)^{br} - \frac{1}{27}\delta^{ab}Y_d^{*rd}Y_d^{pc} - \frac{1}{4}\delta^{pa}Y_d^{*rd}Y_d^{bc} - \frac{1}{4}\delta^{rb}Y_d^{*ad}Y_d^{pc} - \frac{25}{27}\delta^{rb}\delta^{cd}(Y_uY_u^\dagger)^{pa} - \frac{25}{27}\delta^{pa}\delta^{cd}(Y_uY_u^\dagger)^{br} \right) \\
& + 3\delta^{rb}(Y_d^\dagger Y_d)^{dc}(Y_uY_u^\dagger)^{pa} + 3\delta^{pa}(Y_d^\dagger Y_d)^{dc}(Y_uY_u^\dagger)^{br} + 3Y_d^{*rd}Y_d^{pc}(Y_uY_u^\dagger)^{ba} - \frac{1}{2}\delta^{rb}Y_d^{pc}(Y_d^\dagger Y_d Y_d^\dagger)^{ad} - \frac{1}{2}\delta^{rb}Y_d^{pc}(Y_u^\dagger Y_u Y_d^\dagger)^{ad} - \frac{1}{2}\delta^{pa}Y_d^{*rd}(Y_dY_d^\dagger Y_d)^{bc} \\
& - \frac{1}{2}\delta^{pa}Y_d^{*rd}(Y_uY_u^\dagger Y_d)^{bc} - Y_d^{*rd}Y_d^{bc}(Y_uY_u^\dagger)^{pa} - Y_d^{*ad}Y_d^{pc}(Y_uY_u^\dagger)^{br} - \delta^{pa}Y_d^{bc}(Y_u^\dagger Y_u Y_d^\dagger)^{rd} - \delta^{rb}Y_d^{*ad}(Y_uY_u^\dagger Y_d)^{pc} - 3\delta^{rb}(Y_d^\dagger Y_d)^{dc}(Y_dY_d^\dagger)^{pa} \\
& - 3\delta^{pa}(Y_d^\dagger Y_d)^{dc}(Y_dY_d^\dagger)^{br} - 3Y_d^{*rd}Y_d^{pc}(Y_dY_d^\dagger)^{ba} \Big\} C_{qd}^{(\parallel)abcd} + \left\{ \frac{34}{243}\delta^{pa}\delta^{rb}\delta^{cd}g_Y^2g_L^2 + g_L^2 \left( 6\delta^{pa}\delta^{rb}(Y_d^\dagger Y_d)^{dc} - \frac{31}{12}\delta^{pa}Y_d^{*rd}Y_d^{bc} - \frac{31}{12}\delta^{rb}Y_d^{*ad}Y_d^{pc} \right) \right. \\
& + \delta^{rb}(Y_d^\dagger Y_d)^{dc}(Y_uY_u^\dagger)^{pa} + \delta^{pa}(Y_d^\dagger Y_d)^{dc}(Y_uY_u^\dagger)^{br} + g_Y^2 \left( \frac{11}{81}\delta^{rb}\delta^{cd}(Y_dY_d^\dagger)^{pa} + \frac{11}{81}\delta^{pa}\delta^{cd}(Y_dY_d^\dagger)^{br} - \frac{1}{81}\delta^{ab}Y_d^{*rd}Y_d^{pc} - \frac{25}{81}\delta^{rb}\delta^{cd}(Y_uY_u^\dagger)^{pa} \right. \\
& - \frac{25}{81}\delta^{pa}\delta^{cd}(Y_uY_u^\dagger)^{br} - \frac{3}{4}\delta^{pa}Y_d^{*rd}Y_d^{bc} - \frac{3}{4}\delta^{rb}Y_d^{*ad}Y_d^{pc} \Big) + g_s^2 \left( \frac{2}{27}\delta^{rb}\delta^{cd}(Y_dY_d^\dagger)^{pa} + \frac{2}{27}\delta^{pa}\delta^{cd}(Y_dY_d^\dagger)^{br} + \frac{2}{27}\delta^{rb}\delta^{cd}(Y_uY_u^\dagger)^{pa} + \frac{2}{27}\delta^{pa}\delta^{cd}(Y_uY_u^\dagger)^{br} \right. \\
& - \frac{64}{27}\delta^{ab}Y_d^{*rd}Y_d^{pc} \Big) + Y_d^{*rd}Y_d^{pc}(Y_uY_u^\dagger)^{ba} + \frac{3}{2}\delta^{rb}Y_d^{pc}(Y_d^\dagger Y_d Y_d^\dagger)^{ad} + \frac{3}{2}\delta^{rb}Y_d^{pc}(Y_u^\dagger Y_u Y_d^\dagger)^{ad} + \frac{3}{2}\delta^{pa}Y_d^{*rd}(Y_dY_d^\dagger Y_d)^{bc} + \frac{3}{2}\delta^{pa}Y_d^{*rd}(Y_uY_u^\dagger Y_d)^{bc} \\
& + 2Y_d^{*rd}Y_d^{bc}(Y_dY_d^\dagger)^{pa} + 2Y_d^{*ad}Y_d^{pc}(Y_dY_d^\dagger)^{br} - \delta^{rb}(Y_d^\dagger Y_d)^{dc}(Y_dY_d^\dagger)^{pa} - \delta^{pa}(Y_d^\dagger Y_d)^{dc}(Y_dY_d^\dagger)^{br} - Y_d^{*rd}Y_d^{pc}(Y_dY_d^\dagger)^{ba} - \frac{164}{81}\delta^{pa}\delta^{rb}\delta^{cd}g_s^2g_L^2 \\
& - 3Y_d^{*rd}Y_d^{bc}(Y_uY_u^\dagger)^{pa} - 3Y_d^{*ad}Y_d^{pc}(Y_uY_u^\dagger)^{br} - 3\delta^{pa}Y_d^{bc}(Y_u^\dagger Y_u Y_d^\dagger)^{rd} - 3\delta^{rb}Y_d^{*ad}(Y_uY_u^\dagger Y_d)^{pc} \Big\} C_{qd}^{(\times)abcd} + \left\{ 2Y_u^{*rb}Y_u^{pc}(Y_u^\dagger Y_u)^{da} + 6Y_u^{*rb}Y_u^{pa}(Y_u^\dagger Y_u)^{dc} \right. \\
& - g_Y^2 \left( \frac{28}{81}\delta^{ad}Y_u^{*rb}Y_u^{pc} + \frac{28}{27}\delta^{cd}Y_u^{*rb}Y_u^{pa} \right) - \frac{64}{27}\delta^{ad}g_s^2Y_u^{*rb}Y_u^{pc} \Big\} C_{uu}^{abcd} + \left\{ g_Y^2 \left( \frac{2}{81}\delta^{ad}Y_d^{*rb}Y_d^{pc} + \frac{2}{27}\delta^{cd}Y_d^{*rb}Y_d^{pa} \right) + 2Y_d^{*rb}Y_d^{pc}(Y_d^\dagger Y_d)^{da} \right.
\end{aligned}$$

$$\begin{aligned}
& + 6Y_d^{*rb}Y_d^{pa}(Y_d^\dagger Y_d)^{dc} - \frac{64}{27}\delta^{ad}g_s^2Y_d^{*rb}Y_d^{pc} \Big\} C_{dd}^{abcd} + \left\{ \frac{7}{27}\delta^{ab}g_Y^2Y_u^{*rd}Y_u^{pc} - Y_u^{*rd}Y_u^{pc}(Y_e^\dagger Y_e)^{ba} \right\} C_{eu}^{abcd} + \left\{ \frac{1}{27}\delta^{ab}g_Y^2Y_d^{*rd}Y_d^{pc} + Y_d^{*rd}Y_d^{pc}(Y_e^\dagger Y_e)^{ba} \right\} C_{ed}^{abcd} \\
& + \left\{ g_Y^2 \left( \frac{7}{27}\delta^{cd}Y_u^{*rb}Y_u^{pa} - \frac{2}{27}\delta^{ab}Y_d^{*rd}Y_d^{pc} \right) + 2Y_u^{*rb}Y_d^{pc}(Y_d^\dagger Y_u)^{da} + 2Y_d^{*rd}Y_u^{pa}(Y_u^\dagger Y_d)^{bc} - 3Y_u^{*rb}Y_u^{pa}(Y_d^\dagger Y_d)^{dc} - 3Y_d^{*rd}Y_d^{pc}(Y_u^\dagger Y_u)^{ba} \right\} C_{ud}^{(||)abcd} \\
& + \left\{ g_Y^2 \left( \frac{7}{81}\delta^{cd}Y_u^{*rb}Y_u^{pa} - \frac{2}{81}\delta^{ab}Y_d^{*rd}Y_d^{pc} \right) + 6Y_u^{*rb}Y_d^{pc}(Y_d^\dagger Y_u)^{da} + 6Y_d^{*rd}Y_u^{pa}(Y_u^\dagger Y_d)^{bc} - g_s^2 \left( \frac{32}{27}\delta^{ab}Y_d^{*rd}Y_d^{pc} + \frac{32}{27}\delta^{cd}Y_u^{*rb}Y_u^{pa} \right) - Y_u^{*rb}Y_u^{pa}(Y_d^\dagger Y_d)^{dc} \right. \\
& - Y_d^{*rd}Y_d^{pc}(Y_u^\dagger Y_u)^{ba} \Big\} C_{ud}^{(\times)abcd} + \left\{ \frac{1}{8}\delta^{rd}g_Y^2Y_e^{*ab}Y_d^{pc} + \frac{1}{4}\delta^{rd}Y_d^{pc}(Y_e^\dagger Y_e Y_e^\dagger)^{ab} + \frac{19}{72}\delta^{rd}g_L^2Y_e^{*ab}Y_d^{pc} + \frac{1}{2}Y_e^{*ab}Y_d^{pc}(Y_u Y_u^\dagger)^{dr} + \frac{1}{2}\delta^{rd}Y_e^{*ab}(Y_u Y_u^\dagger Y_d)^{pc} \right. \\
& - \frac{1}{3}Y_e^{*ab}Y_d^{pc}(Y_d Y_d^\dagger)^{dr} \Big\} C_{ledq}^{abcd} + C_{ledq}^{*abcd} \left\{ \frac{1}{8}\delta^{pd}g_Y^2Y_d^{*rc}Y_e^{ab} + \frac{1}{4}\delta^{pd}Y_d^{*rc}(Y_e Y_e^\dagger Y_e)^{ab} + \frac{19}{72}\delta^{pd}g_L^2Y_d^{*rc}Y_e^{ab} + \frac{1}{2}Y_d^{*rc}Y_e^{ab}(Y_u Y_u^\dagger)^{pd} \right. \\
& + \frac{1}{2}\delta^{pd}Y_e^{ab}(Y_u^\dagger Y_u Y_d^\dagger)^{rc} - \frac{1}{3}Y_d^{*rc}Y_e^{ab}(Y_d Y_d^\dagger)^{pd} \Big\} + \left\{ \frac{1}{4}Y_d^{*ad}Y_u^{*rb}(Y_d Y_d^\dagger)^{pc} + \frac{1}{4}Y_d^{*rd}Y_u^{*cb}(Y_u Y_u^\dagger)^{pa} + \frac{1}{4}\delta^{pc}Y_d^{*ad}(Y_d^\dagger Y_d Y_u^\dagger)^{rb} + \frac{1}{4}\delta^{pa}Y_u^{*cb}(Y_u^\dagger Y_u Y_d^\dagger)^{rd} \right. \\
& + \frac{3}{4}\delta^{pa}Y_u^{*rb}(Y_d^\dagger Y_d Y_d^\dagger)^{cd} + \frac{3}{4}\delta^{pc}Y_d^{*rd}(Y_d^\dagger Y_d Y_u^\dagger)^{ab} + \frac{3}{4}\delta^{pa}Y_u^{*rb}(Y_u^\dagger Y_u Y_d^\dagger)^{cd} + \frac{3}{4}\delta^{pc}Y_d^{*rd}(Y_u^\dagger Y_u Y_u^\dagger)^{ab} + g_Y^2 \left( \frac{3}{8}\delta^{pc}Y_d^{*rd}Y_u^{*ab} - \frac{1}{9}\delta^{pa}Y_d^{*rd}Y_u^{*cb} \right. \\
& - \frac{1}{9}\delta^{pc}Y_d^{*ad}Y_u^{*rb} - \frac{9}{8}\delta^{pa}Y_d^{*cd}Y_u^{*rb} \Big) + g_L^2 \left( \frac{19}{24}\delta^{pa}Y_d^{*cd}Y_u^{*rb} + \frac{19}{24}\delta^{pc}Y_d^{*rd}Y_u^{*ab} + \frac{17}{18}\delta^{pa}Y_d^{*rd}Y_u^{*cb} + \frac{17}{18}\delta^{pc}Y_d^{*ad}Y_u^{*rb} \right) + \frac{3}{2}Y_d^{*cd}Y_u^{*rb}(Y_d Y_d^\dagger)^{pa} \\
& + \frac{3}{2}Y_d^{*rd}Y_u^{*ab}(Y_u Y_u^\dagger)^{pc} + \frac{3}{2}\delta^{pa}Y_d^{*cd}(Y_d^\dagger Y_d Y_u^\dagger)^{rb} + \frac{3}{2}\delta^{pc}Y_u^{*ab}(Y_u^\dagger Y_u Y_d^\dagger)^{rd} - \frac{1}{6}Y_d^{*rd}Y_u^{*cb}(Y_d Y_d^\dagger)^{pa} - \frac{1}{6}Y_d^{*ad}Y_u^{*rb}(Y_u Y_u^\dagger)^{pc} - \frac{3}{4}\delta^{pc}Y_u^{*rb}(Y_d^\dagger Y_d Y_d^\dagger)^{ad} \\
& - \frac{3}{4}\delta^{pa}Y_d^{*rd}(Y_u^\dagger Y_u Y_u^\dagger)^{cb} - g_s^2 \left( \frac{16}{3}\delta^{pa}Y_d^{*rd}Y_u^{*cb} + \frac{16}{3}\delta^{pc}Y_d^{*ad}Y_u^{*rb} \right) - Y_d^{*rd}Y_u^{*ab}(Y_d Y_d^\dagger)^{pc} - Y_d^{*cd}Y_u^{*rb}(Y_u Y_u^\dagger)^{pa} - \frac{9}{4}\delta^{pa}Y_d^{*rd}(Y_d^\dagger Y_d Y_u^\dagger)^{cb} \\
& - \frac{9}{4}\delta^{pc}Y_u^{*rb}(Y_u^\dagger Y_u Y_d^\dagger)^{ad} \Big\} C_{quqd}^{(||)abcd} + \left( C_{quqd}^{(||)*} \right)^{abcd} \left\{ \frac{1}{4}Y_d^{*ad}Y_u^{*pb}(Y_d Y_d^\dagger)^{cr} + \frac{1}{4}Y_d^{*pd}Y_u^{*cb}(Y_u Y_u^\dagger)^{ar} + \frac{1}{4}\delta^{rc}Y_d^{*ad}(Y_d Y_d^\dagger Y_u)^{pb} + \frac{1}{4}\delta^{ra}Y_u^{*cb}(Y_u Y_u^\dagger Y_d)^{pd} \right. \\
& + \frac{3}{4}\delta^{ra}Y_u^{*pb}(Y_d Y_d^\dagger Y_d)^{cd} + \frac{3}{4}\delta^{rc}Y_d^{*pd}(Y_d Y_d^\dagger Y_u)^{ab} + \frac{3}{4}\delta^{ra}Y_u^{*pb}(Y_u Y_u^\dagger Y_d)^{cd} + \frac{3}{4}\delta^{rc}Y_d^{*pd}(Y_u Y_u^\dagger Y_u)^{ab} + g_Y^2 \left( \frac{3}{8}\delta^{rc}Y_d^{*pd}Y_u^{*ab} - \frac{1}{9}\delta^{ra}Y_d^{*pd}Y_u^{*cb} - \frac{1}{9}\delta^{rc}Y_d^{*ad}Y_u^{*pb} \right. \\
& - \frac{9}{8}\delta^{ra}Y_d^{*cd}Y_u^{*pb} \Big) + g_L^2 \left( \frac{19}{24}\delta^{ra}Y_d^{*cd}Y_u^{*pb} + \frac{19}{24}\delta^{rc}Y_d^{*pd}Y_u^{*ab} + \frac{17}{18}\delta^{ra}Y_d^{*pd}Y_u^{*cb} + \frac{17}{18}\delta^{rc}Y_d^{*ad}Y_u^{*pb} \right) + \frac{3}{2}Y_d^{*cd}Y_u^{*pb}(Y_d Y_d^\dagger)^{ar} + \frac{3}{2}Y_d^{*pd}Y_u^{*ab}(Y_u Y_u^\dagger)^{cr} + \frac{3}{2}\delta^{ra}Y_d^{*cd}(Y_d Y_d^\dagger Y_u)^{pb} \\
& + \frac{3}{2}\delta^{rc}Y_u^{*ab}(Y_u Y_u^\dagger Y_d)^{pd} - \frac{1}{6}Y_d^{*pd}Y_u^{*cb}(Y_d Y_d^\dagger)^{ar} - \frac{1}{6}Y_d^{*ad}Y_u^{*pb}(Y_u Y_u^\dagger)^{cr} - \frac{3}{4}\delta^{rc}Y_u^{*pb}(Y_d Y_d^\dagger Y_d)^{ad} - \frac{3}{4}\delta^{ra}Y_d^{*pd}(Y_u Y_u^\dagger Y_u)^{cb} - g_s^2 \left( \frac{16}{3}\delta^{ra}Y_d^{*pd}Y_u^{*cb} + \frac{16}{3}\delta^{rc}Y_d^{*ad}Y_u^{*pb} \right) \\
& - Y_d^{*pd}Y_u^{*ab}(Y_d Y_d^\dagger)^{cr} - Y_d^{*cd}Y_u^{*pb}(Y_u Y_u^\dagger)^{ar} - \frac{9}{4}\delta^{ra}Y_d^{*pd}(Y_d Y_d^\dagger Y_u)^{cb} - \frac{9}{4}\delta^{rc}Y_u^{*pb}(Y_u Y_u^\dagger Y_d)^{ad} \Big\} + \left\{ \frac{1}{2}Y_d^{*cd}Y_u^{*rb}(Y_d Y_d^\dagger)^{pa} + \frac{1}{2}Y_d^{*rd}Y_u^{*ab}(Y_u Y_u^\dagger)^{pc} \right. \\
& + \frac{1}{2}\delta^{pa}Y_d^{*cd}(Y_d^\dagger Y_d Y_u^\dagger)^{rb} + \frac{1}{2}\delta^{pc}Y_u^{*ab}(Y_u^\dagger Y_u Y_d^\dagger)^{rd} + \frac{3}{4}Y_d^{*ad}Y_u^{*rb}(Y_d Y_d^\dagger)^{pc} + \frac{3}{4}Y_d^{*rd}Y_u^{*cb}(Y_u Y_u^\dagger)^{pa} + \frac{3}{4}\delta^{pa}Y_u^{*rb}(Y_d^\dagger Y_d Y_d^\dagger)^{cd} + \frac{3}{4}\delta^{pc}Y_d^{*ad}(Y_d^\dagger Y_d Y_u^\dagger)^{rb}
\end{aligned}$$



$$\begin{aligned}
& + \frac{3}{4} \delta^{pc} Y_d^{*rd} (Y_d^\dagger Y_d Y_u^\dagger)^{ab} + \frac{3}{4} \delta^{pa} Y_u^{*cb} (Y_u^\dagger Y_u Y_d^\dagger)^{rd} + \frac{3}{4} \delta^{pa} Y_u^{*rb} (Y_u^\dagger Y_u Y_d^\dagger)^{cd} + \frac{3}{4} \delta^{pc} Y_d^{*rd} (Y_u^\dagger Y_u Y_u^\dagger)^{ab} + g_L^2 \left( \frac{7}{72} \delta^{pa} Y_d^{*cd} Y_u^{*rb} + \frac{7}{72} \delta^{pc} Y_d^{*rd} Y_u^{*ab} \right. \\
& + \frac{7}{3} \delta^{pa} Y_d^{*rd} Y_u^{*cb} + \frac{7}{3} \delta^{pc} Y_d^{*ad} Y_u^{*rb} \Big) + g_Y^2 \left( \frac{1}{8} \delta^{pc} Y_d^{*rd} Y_u^{*ab} - \frac{1}{3} \delta^{pa} Y_d^{*rd} Y_u^{*cb} - \frac{1}{3} \delta^{pc} Y_d^{*ad} Y_u^{*rb} - \frac{3}{8} \delta^{pa} Y_d^{*cd} Y_u^{*rb} \right) - \frac{1}{3} Y_d^{*rd} Y_u^{*ab} (Y_d Y_d^\dagger)^{pc} \\
& - \frac{1}{3} Y_d^{*cd} Y_u^{*rb} (Y_u Y_u^\dagger)^{pa} - \frac{1}{2} Y_d^{*rd} Y_u^{*cb} (Y_d Y_d^\dagger)^{pa} - \frac{1}{2} Y_d^{*ad} Y_u^{*rb} (Y_u Y_u^\dagger)^{pc} - \frac{3}{4} \delta^{pc} Y_u^{*rb} (Y_d^\dagger Y_d Y_d^\dagger)^{ad} - \frac{3}{4} \delta^{pa} Y_d^{*rd} (Y_u^\dagger Y_u Y_u^\dagger)^{cb} - \frac{21}{4} \delta^{pa} Y_d^{*rd} (Y_d^\dagger Y_d Y_u^\dagger)^{cb} \\
& - \frac{21}{4} \delta^{pc} Y_u^{*rb} (Y_u^\dagger Y_u Y_d^\dagger)^{ad} \Big\} C_{quqd}^{(\times)abcd} + \left( C_{quqd}^{(\times)*} \right)^{abcd} \left\{ \frac{1}{2} Y_d^{cd} Y_u^{pb} (Y_d Y_d^\dagger)^{ar} + \frac{1}{2} Y_d^{pd} Y_u^{ab} (Y_u Y_u^\dagger)^{cr} + \frac{1}{2} \delta^{ra} Y_d^{cd} (Y_d Y_d^\dagger Y_u)^{pb} + \frac{1}{2} \delta^{rc} Y_u^{ab} (Y_u Y_u^\dagger Y_d)^{pd} \right. \\
& + \frac{3}{4} Y_d^{ad} Y_u^{pb} (Y_d Y_d^\dagger)^{cr} + \frac{3}{4} Y_d^{pd} Y_u^{cb} (Y_u Y_u^\dagger)^{ar} + \frac{3}{4} \delta^{ra} Y_u^{pb} (Y_d Y_d^\dagger Y_d)^{cd} + \frac{3}{4} \delta^{rc} Y_d^{ad} (Y_d Y_d^\dagger Y_u)^{pb} + \frac{3}{4} \delta^{rc} Y_d^{pd} (Y_d Y_d^\dagger Y_u)^{ab} + \frac{3}{4} \delta^{ra} Y_u^{cb} (Y_u Y_u^\dagger Y_d)^{pd} \\
& + \frac{3}{4} \delta^{ra} Y_u^{pb} (Y_u Y_u^\dagger Y_d)^{cd} + \frac{3}{4} \delta^{rc} Y_d^{pd} (Y_u Y_u^\dagger Y_u)^{ab} + g_L^2 \left( \frac{7}{72} \delta^{ra} Y_d^{cd} Y_u^{pb} + \frac{7}{72} \delta^{rc} Y_d^{pd} Y_u^{ab} + \frac{7}{3} \delta^{ra} Y_d^{pd} Y_u^{cb} + \frac{7}{3} \delta^{rc} Y_d^{ad} Y_u^{pb} \right) + g_Y^2 \left( \frac{1}{8} \delta^{rc} Y_d^{pd} Y_u^{ab} - \frac{1}{3} \delta^{ra} Y_d^{pd} Y_u^{cb} \right. \\
& - \frac{1}{3} \delta^{rc} Y_d^{ad} Y_u^{pb} - \frac{3}{8} \delta^{ra} Y_d^{cd} Y_u^{pb} \Big) - \frac{1}{3} Y_d^{pd} Y_u^{ab} (Y_d Y_d^\dagger)^{cr} - \frac{1}{3} Y_d^{cd} Y_u^{pb} (Y_u Y_u^\dagger)^{ar} - \frac{1}{2} Y_d^{pd} Y_u^{cb} (Y_d Y_d^\dagger)^{ar} - \frac{1}{2} Y_d^{ad} Y_u^{pb} (Y_u Y_u^\dagger)^{cr} - \frac{3}{4} \delta^{rc} Y_u^{pb} (Y_d Y_d^\dagger Y_d)^{ad} \\
& - \frac{3}{4} \delta^{ra} Y_d^{pd} (Y_u Y_u^\dagger Y_u)^{cb} - \frac{21}{4} \delta^{ra} Y_d^{pd} (Y_d Y_d^\dagger Y_u)^{cb} - \frac{21}{4} \delta^{rc} Y_u^{pb} (Y_u Y_u^\dagger Y_d)^{ad} \Big\} + \left\{ \frac{1}{3} Y_e^{*ab} Y_u^{*rd} (Y_u Y_u^\dagger)^{pc} + \frac{3}{8} \delta^{pc} g_Y^2 Y_e^{*ab} Y_u^{*rd} - \frac{1}{4} \delta^{pc} Y_u^{*rd} (Y_e^\dagger Y_e Y_e^\dagger)^{ab} \right. \\
& - \frac{19}{72} \delta^{pc} g_L^2 Y_e^{*ab} Y_u^{*rd} - \frac{1}{2} Y_e^{*ab} Y_u^{*rd} (Y_d Y_d^\dagger)^{pc} - \frac{1}{2} \delta^{pc} Y_e^{*ab} (Y_d^\dagger Y_d Y_u^\dagger)^{rd} \Big\} C_{lequ}^{abcd} + C_{lequ}^{*abcd} \left\{ \frac{1}{3} Y_e^{ab} Y_u^{pd} (Y_u Y_u^\dagger)^{cr} + \frac{3}{8} \delta^{rc} g_Y^2 Y_e^{ab} Y_u^{pd} \right. \\
& - \frac{1}{4} \delta^{rc} Y_u^{pd} (Y_e Y_e^\dagger Y_e)^{ab} - \frac{19}{72} \delta^{rc} g_L^2 Y_e^{ab} Y_u^{pd} - \frac{1}{2} Y_e^{ab} Y_u^{pd} (Y_d Y_d^\dagger)^{cr} - \frac{1}{2} \delta^{rc} Y_e^{ab} (Y_d Y_d^\dagger Y_u)^{pd} \Big\} + \left\{ \frac{1}{4} Y_e^{*ad} Y_u^{*rb} (Y_d Y_d^\dagger)^{pc} + \frac{1}{4} \delta^{pc} Y_e^{*ad} (Y_d^\dagger Y_d Y_u^\dagger)^{rb} \right. \\
& + \frac{1}{2} \delta^{pc} g_Y^2 Y_e^{*ad} Y_u^{*rb} + \frac{7}{9} \delta^{pc} g_L^2 Y_e^{*ad} Y_u^{*rb} - \frac{1}{6} Y_e^{*ad} Y_u^{*rb} (Y_u Y_u^\dagger)^{pc} - \frac{1}{4} \delta^{pc} Y_u^{*rb} (Y_e^\dagger Y_e Y_e^\dagger)^{ad} \Big\} C_{luqe}^{abcd} + C_{luqe}^{*abcd} \left\{ \frac{1}{4} Y_e^{ad} Y_u^{pb} (Y_d Y_d^\dagger)^{cr} \right. \\
& + \frac{1}{4} \delta^{rc} Y_e^{ad} (Y_d Y_d^\dagger Y_u)^{pb} + \frac{1}{2} \delta^{rc} g_Y^2 Y_e^{ad} Y_u^{pb} + \frac{7}{9} \delta^{rc} g_L^2 Y_e^{ad} Y_u^{pb} - \frac{1}{6} Y_e^{ad} Y_u^{pb} (Y_u Y_u^\dagger)^{cr} - \frac{1}{4} \delta^{rc} Y_u^{pb} (Y_e Y_e^\dagger Y_e)^{ad} \Big\} + \left\{ \frac{8}{9} \delta^{pr} \delta^{ad} \delta^{bc} g_L^4 \right. \\
& - \frac{8}{3} \delta^{pr} \delta^{bc} g_L^2 (Y_e Y_e^\dagger)^{da} \Big\} C_{\ell\ell}^{abcd} + \left\{ g_L^4 \left( \frac{8}{3} \delta^{pr} \delta^{ad} \delta^{bc} + \frac{140}{9} \delta^{pa} \delta^{rd} \delta^{bc} - 2 \delta^{pa} \delta^{rb} \delta^{cd} \right) + g_Y^2 \left( \frac{10}{81} \delta^{rd} \delta^{bc} (Y_d Y_d^\dagger)^{pa} + \frac{10}{81} \delta^{pa} \delta^{bc} (Y_d Y_d^\dagger)^{dr} \right. \right. \\
& + \frac{50}{27} \delta^{rb} \delta^{cd} (Y_u Y_u^\dagger)^{pa} + \frac{50}{27} \delta^{pa} \delta^{cd} (Y_u Y_u^\dagger)^{br} - \frac{8}{81} \delta^{rd} \delta^{bc} (Y_u Y_u^\dagger)^{pa} - \frac{8}{81} \delta^{pa} \delta^{bc} (Y_u Y_u^\dagger)^{dr} - \frac{1}{6} \delta^{pa} \delta^{rd} (Y_d Y_d^\dagger)^{bc} - \frac{22}{27} \delta^{rb} \delta^{cd} (Y_d Y_d^\dagger)^{pa} - \frac{22}{27} \delta^{pa} \delta^{cd} (Y_d Y_d^\dagger)^{br} \\
& - \frac{7}{2} \delta^{pa} \delta^{rd} (Y_u Y_u^\dagger)^{bc} \Big) + g_L^2 \left( 30 \delta^{pa} \delta^{rb} (Y_d Y_d^\dagger)^{dc} + 30 \delta^{pa} \delta^{rb} (Y_u Y_u^\dagger)^{dc} - \frac{2}{3} \delta^{rd} \delta^{bc} (Y_d Y_d^\dagger)^{pa} - \frac{2}{3} \delta^{pa} \delta^{bc} (Y_d Y_d^\dagger)^{dr} - \frac{2}{3} \delta^{rd} \delta^{bc} (Y_u Y_u^\dagger)^{pa} - \frac{2}{3} \delta^{pa} \delta^{bc} (Y_u Y_u^\dagger)^{dr} \right. \\
& - 8 \delta^{pr} \delta^{bc} (Y_d Y_d^\dagger)^{da} - 8 \delta^{pr} \delta^{bc} (Y_u Y_u^\dagger)^{da} - \frac{67}{6} \delta^{pa} \delta^{rd} (Y_d Y_d^\dagger)^{bc} - \frac{67}{6} \delta^{pa} \delta^{rd} (Y_u Y_u^\dagger)^{bc} \Big) + 2 \delta^{rb} (Y_d Y_d^\dagger)^{da} (Y_u Y_u^\dagger)^{pc} + 2 \delta^{rd} (Y_d Y_d^\dagger)^{pa} (Y_u Y_u^\dagger)^{bc} \\
& + 2 \delta^{pa} (Y_d Y_d^\dagger)^{dr} (Y_u Y_u^\dagger)^{bc} + 2 \delta^{pa} (Y_d Y_d^\dagger)^{bc} (Y_u Y_u^\dagger)^{dr} + \frac{260}{81} \delta^{pa} \delta^{rd} \delta^{bc} g_s^2 g_L^2 + 6 \delta^{rb} (Y_d Y_d^\dagger)^{pa} (Y_d Y_d^\dagger)^{dc} + 6 \delta^{pa} (Y_d Y_d^\dagger)^{br} (Y_d Y_d^\dagger)^{dc} + 6 \delta^{rb} (Y_u Y_u^\dagger)^{pa} (Y_u Y_u^\dagger)^{dc}
\end{aligned}$$

$$\begin{aligned}
& + 6\delta^{pa}(Y_u Y_u^\dagger)^{br}(Y_u Y_u^\dagger)^{dc} + 18\delta^{pa}\delta^{rd}(Y_d Y_d^\dagger Y_d Y_d^\dagger)^{bc} + 18\delta^{pa}\delta^{rd}(Y_u Y_u^\dagger Y_u Y_u^\dagger)^{bc} - g_Y^2 g_L^2 \left( \frac{58}{243} \delta^{pa} \delta^{rd} \delta^{bc} + \frac{68}{81} \delta^{pa} \delta^{rb} \delta^{cd} \right) - g_s^2 \left( \frac{92}{27} \delta^{rd} \delta^{bc} (Y_d Y_d^\dagger)^{pa} \right. \\
& + \frac{92}{27} \delta^{pa} \delta^{bc} (Y_d Y_d^\dagger)^{dr} + \frac{92}{27} \delta^{rd} \delta^{bc} (Y_u Y_u^\dagger)^{pa} + \frac{92}{27} \delta^{pa} \delta^{bc} (Y_u Y_u^\dagger)^{dr} + 4\delta^{pa} \delta^{rd} (Y_d Y_d^\dagger)^{bc} + 4\delta^{pa} \delta^{rd} (Y_u Y_u^\dagger)^{bc} \Big) - 2\delta^{rd} (Y_d Y_d^\dagger)^{pa} (Y_d Y_d^\dagger)^{bc} \\
& - 2\delta^{pa} (Y_d Y_d^\dagger)^{bc} (Y_d Y_d^\dagger)^{dr} - 2\delta^{rd} (Y_u Y_u^\dagger)^{pa} (Y_u Y_u^\dagger)^{bc} - 2\delta^{pa} (Y_u Y_u^\dagger)^{bc} (Y_u Y_u^\dagger)^{dr} - 4\delta^{pa} \delta^{rd} (Y_d Y_d^\dagger Y_u Y_u^\dagger)^{bc} - 4\delta^{pa} \delta^{rd} (Y_u Y_u^\dagger Y_d Y_d^\dagger)^{bc} \\
& - 6\delta^{rd} (Y_d Y_d^\dagger)^{ba} (Y_u Y_u^\dagger)^{pc} - 6\delta^{pa} (Y_d Y_d^\dagger)^{dc} (Y_u Y_u^\dagger)^{br} - 6\delta^{rb} (Y_d Y_d^\dagger)^{pa} (Y_u Y_u^\dagger)^{dc} - 6\delta^{pa} (Y_d Y_d^\dagger)^{br} (Y_u Y_u^\dagger)^{dc} \Big\} C_{qq}^{(\parallel)abcd} + \left\{ g_s^2 g_L^2 \left( 12\delta^{pa} \delta^{rb} \delta^{cd} \right. \right. \\
& - \frac{272}{81} \delta^{pa} \delta^{rd} \delta^{bc} \Big) + g_L^4 \left( \frac{74}{3} \delta^{pa} \delta^{rb} \delta^{cd} - \frac{14}{3} \delta^{pa} \delta^{rd} \delta^{bc} \right) + g_L^2 \left( 22\delta^{pa} \delta^{rd} (Y_d Y_d^\dagger)^{bc} + 22\delta^{pa} \delta^{rd} (Y_u Y_u^\dagger)^{bc} - 5\delta^{rb} \delta^{cd} (Y_d Y_d^\dagger)^{pa} - 5\delta^{pa} \delta^{cd} (Y_d Y_d^\dagger)^{br} \right. \\
& - 5\delta^{rb} \delta^{cd} (Y_u Y_u^\dagger)^{pa} - 5\delta^{pa} \delta^{cd} (Y_u Y_u^\dagger)^{br} - \frac{41}{2} \delta^{pa} \delta^{rb} (Y_d Y_d^\dagger)^{dc} - \frac{41}{2} \delta^{pa} \delta^{rb} (Y_u Y_u^\dagger)^{dc} \Big) + g_Y^2 \left( \frac{20}{81} \delta^{rd} \delta^{bc} (Y_d Y_d^\dagger)^{pa} + \frac{20}{81} \delta^{pa} \delta^{bc} (Y_d Y_d^\dagger)^{dr} \right. \\
& + \frac{25}{27} \delta^{rb} \delta^{cd} (Y_u Y_u^\dagger)^{pa} + \frac{25}{27} \delta^{pa} \delta^{cd} (Y_u Y_u^\dagger)^{br} + \frac{5}{2} \delta^{pa} \delta^{rb} (Y_d Y_d^\dagger)^{dc} + \frac{9}{2} \delta^{pa} \delta^{rb} (Y_u Y_u^\dagger)^{dc} - \frac{16}{81} \delta^{rd} \delta^{bc} (Y_u Y_u^\dagger)^{pa} - \frac{16}{81} \delta^{pa} \delta^{bc} (Y_u Y_u^\dagger)^{dr} - \frac{11}{27} \delta^{rb} \delta^{cd} (Y_d Y_d^\dagger)^{pa} \\
& - \frac{11}{27} \delta^{pa} \delta^{cd} (Y_d Y_d^\dagger)^{br} \Big) + 4\delta^{rb} (Y_d Y_d^\dagger)^{da} (Y_u Y_u^\dagger)^{pc} + 4\delta^{rd} (Y_d Y_d^\dagger)^{pa} (Y_u Y_u^\dagger)^{bc} + 4\delta^{pa} (Y_d Y_d^\dagger)^{dr} (Y_u Y_u^\dagger)^{bc} + 4\delta^{pa} (Y_d Y_d^\dagger)^{bc} (Y_u Y_u^\dagger)^{dr} + 6\delta^{rb} (Y_d Y_d^\dagger)^{pa} (Y_d Y_d^\dagger)^{dc} \\
& + 6\delta^{pa} (Y_d Y_d^\dagger)^{br} (Y_d Y_d^\dagger)^{dc} + 6\delta^{rb} (Y_u Y_u^\dagger)^{pa} (Y_u Y_u^\dagger)^{dc} + 6\delta^{pa} (Y_u Y_u^\dagger)^{br} (Y_u Y_u^\dagger)^{dc} + 30\delta^{pa} \delta^{rb} (Y_d Y_d^\dagger Y_d Y_d^\dagger)^{dc} + 30\delta^{pa} \delta^{rb} (Y_u Y_u^\dagger Y_u Y_u^\dagger)^{dc} \\
& - g_Y^2 g_L^2 \left( \frac{44}{243} \delta^{pa} \delta^{rd} \delta^{bc} + \frac{16}{81} \delta^{pa} \delta^{rb} \delta^{cd} \right) - g_s^2 \left( \frac{184}{27} \delta^{rd} \delta^{bc} (Y_d Y_d^\dagger)^{pa} + \frac{184}{27} \delta^{pa} \delta^{bc} (Y_d Y_d^\dagger)^{dr} + \frac{184}{27} \delta^{rd} \delta^{bc} (Y_u Y_u^\dagger)^{pa} + \frac{184}{27} \delta^{pa} \delta^{bc} (Y_u Y_u^\dagger)^{dr} \right. \\
& + 68\delta^{pa} \delta^{rb} (Y_d Y_d^\dagger)^{dc} + 68\delta^{pa} \delta^{rb} (Y_u Y_u^\dagger)^{dc} \Big) - 4\delta^{rd} (Y_d Y_d^\dagger)^{pa} (Y_d Y_d^\dagger)^{bc} - 4\delta^{pa} (Y_d Y_d^\dagger)^{bc} (Y_d Y_d^\dagger)^{dr} - 4\delta^{rd} (Y_u Y_u^\dagger)^{pa} (Y_u Y_u^\dagger)^{bc} \\
& - 4\delta^{pa} (Y_u Y_u^\dagger)^{bc} (Y_u Y_u^\dagger)^{dr} \Big\} C_{qq}^{(\times)abcd} + \left\{ \frac{34}{81} \delta^{pc} \delta^{rd} \delta^{ab} g_Y^2 g_L^2 + \delta^{rd} (Y_d Y_d^\dagger)^{pc} (Y_e Y_e^\dagger)^{ba} + \delta^{pc} (Y_d Y_d^\dagger)^{dr} (Y_e Y_e^\dagger)^{ba} + g_Y^2 \left( \frac{11}{27} \delta^{rd} \delta^{ab} (Y_d Y_d^\dagger)^{pc} \right. \right. \\
& + \frac{11}{27} \delta^{pc} \delta^{ab} (Y_d Y_d^\dagger)^{dr} - \frac{25}{27} \delta^{rd} \delta^{ab} (Y_u Y_u^\dagger)^{pc} - \frac{25}{27} \delta^{pc} \delta^{ab} (Y_u Y_u^\dagger)^{dr} \Big) + 5\delta^{pc} \delta^{rd} g_L^2 (Y_e Y_e^\dagger)^{ba} - \frac{1}{3} \delta^{pc} \delta^{rd} \delta^{ab} g_L^4 - \delta^{rd} (Y_e Y_e^\dagger)^{ba} (Y_u Y_u^\dagger)^{pc} \\
& - \delta^{pc} (Y_e Y_e^\dagger)^{ba} (Y_u Y_u^\dagger)^{dr} \Big\} C_{\ell q}^{(\parallel)abcd} + \left\{ \frac{62}{81} \delta^{pc} \delta^{rd} \delta^{ab} g_Y^2 g_L^2 + \delta^{rd} (Y_d Y_d^\dagger)^{pc} (Y_e Y_e^\dagger)^{ba} + \delta^{pc} (Y_d Y_d^\dagger)^{dr} (Y_e Y_e^\dagger)^{ba} + g_Y^2 \left( \frac{11}{54} \delta^{rd} \delta^{ab} (Y_d Y_d^\dagger)^{pc} + \frac{11}{54} \delta^{pc} \delta^{ab} (Y_d Y_d^\dagger)^{dr} \right. \right. \\
& - \frac{25}{54} \delta^{rd} \delta^{ab} (Y_u Y_u^\dagger)^{pc} - \frac{25}{54} \delta^{pc} \delta^{ab} (Y_u Y_u^\dagger)^{dr} - \frac{91}{12} \delta^{pc} \delta^{rd} (Y_e Y_e^\dagger)^{ba} \Big) + \frac{37}{9} \delta^{pc} \delta^{rd} \delta^{ab} g_L^4 + 5\delta^{pc} \delta^{rd} (Y_e Y_e^\dagger Y_e Y_e^\dagger)^{ba} - g_L^2 \left( \frac{5}{6} \delta^{rd} \delta^{ab} (Y_d Y_d^\dagger)^{pc} \right. \\
& + \frac{5}{6} \delta^{pc} \delta^{ab} (Y_d Y_d^\dagger)^{dr} + \frac{5}{6} \delta^{rd} \delta^{ab} (Y_u Y_u^\dagger)^{pc} + \frac{5}{6} \delta^{pc} \delta^{ab} (Y_u Y_u^\dagger)^{dr} + \frac{41}{12} \delta^{pc} \delta^{rd} (Y_e Y_e^\dagger)^{ba} \Big) \Big\} C_{\ell q}^{(\times)abcd}, \tag{9.10}
\end{aligned}$$

## 9.6 $C_{Hu}$

$$\beta_{C_{Hu}^{pr}}^{(1)} = \left\{ \frac{1}{9} \delta^{pr} g_Y^2 - \frac{1}{2} (Y_u^\dagger Y_u)^{pr} \right\} C_{HD}^{(\parallel)} + \left\{ \frac{2}{9} \delta^{pr} g_Y^2 - (Y_u^\dagger Y_u)^{pr} \right\} C_{HD}^{(\times)} - \frac{8}{9} \delta^{pr} \delta^{ab} g_Y^2 C_{He}^{(\parallel)ab} - \frac{4}{9} \delta^{pr} \delta^{ab} g_Y^2 C_{He}^{(\times)ab} - \frac{8}{9} \delta^{pr} \delta^{ab} g_Y^2 C_{He}^{ab} + \left\{ \frac{8}{9} \delta^{pr} \delta^{ab} g_Y^2 \right.$$

$$\begin{aligned}
& -2Y_u^{*ap}Y_u^{br}\Big\}C_{Hq}^{(\parallel)ab} + \Big\{\frac{4}{9}\delta^{pr}\delta^{ab}g_Y^2 - Y_u^{*ap}Y_u^{br}\Big\}C_{Hq}^{(\times)ab} + \Big\{\frac{1}{9}g_Y^2\big(3\delta^{pa}\delta^{rb} + 16\delta^{pr}\delta^{ab}\big) + 2\big(\text{T}_2\delta^{pa}\delta^{rb} + 2\delta^{rb}(Y_u^\dagger Y_u)^{pa} + 2\delta^{pa}(Y_u^\dagger Y_u)^{br}\big)\Big\}C_{Hu}^{ab} \\
& -\frac{8}{9}\delta^{pr}\delta^{ab}g_Y^2C_{Hd}^{ab} + \delta^{pa}C_{Hud}^{ab}(Y_d^\dagger Y_u)^{br} + \delta^{ra}C_{Hud}^{*ab}(Y_u^\dagger Y_d)^{pb} - \Big\{\frac{2}{3}\delta^{pc}\delta^{rd}\delta^{ab}g_Y^2 + 2\delta^{pc}\delta^{rd}(Y_e Y_e^\dagger)^{ba}\Big\}C_{\ell u}^{abcd} + \Big\{\frac{2}{3}\delta^{pc}\delta^{rd}\delta^{ab}g_Y^2 \\
& -6\big(\delta^{pc}\delta^{rd}(Y_d Y_d^\dagger)^{ba} - \delta^{pc}\delta^{rd}(Y_u Y_u^\dagger)^{ba}\big)\Big\}C_{qu}^{(\parallel)abcd} + \Big\{\frac{2}{9}\delta^{pc}\delta^{rd}\delta^{ab}g_Y^2 - 2\big(\delta^{pc}\delta^{rd}(Y_d Y_d^\dagger)^{ba} - \delta^{pc}\delta^{rd}(Y_u Y_u^\dagger)^{ba}\big)\Big\}C_{qu}^{(\times)abcd} + \Big\{\frac{8}{9}g_Y^2\big(\delta^{pa}\delta^{rd}\delta^{bc} + 3\delta^{pa}\delta^{rb}\delta^{cd}\big) \\
& -4\big(\delta^{pa}\delta^{rd}(Y_u^\dagger Y_u)^{bc} + 3\delta^{pa}\delta^{rb}(Y_u^\dagger Y_u)^{dc}\big)\Big\}C_{uu}^{abcd} + \Big\{2\delta^{pc}\delta^{rd}(Y_e^\dagger Y_e)^{ba} - \frac{2}{3}\delta^{pc}\delta^{rd}\delta^{ab}g_Y^2\Big\}C_{eu}^{abcd} + \Big\{6\delta^{pa}\delta^{rb}(Y_d^\dagger Y_d)^{dc} - \frac{2}{3}\delta^{pa}\delta^{rb}\delta^{cd}g_Y^2\Big\}C_{ud}^{(\parallel)abcd} \\
& + \Big\{2\delta^{pa}\delta^{rb}(Y_d^\dagger Y_d)^{dc} - \frac{2}{9}\delta^{pa}\delta^{rb}\delta^{cd}g_Y^2\Big\}C_{ud}^{(\times)abcd}, \tag{9.11}
\end{aligned}$$

$$\begin{aligned}
\beta_{C_{Hu}^{pr}}^{(2)} &= 3(Y_u^\dagger Y_u)^{pr}\mathbf{T}_{\ell H} - \frac{38}{9}\delta^{pr}g_Y^2\mathbf{T}_{\ell H} + \Big\{\frac{7}{54}\delta^{pr}g_Y^2g_L^2 + \frac{1}{2}\text{T}_2(Y_u^\dagger Y_u)^{pr} + \frac{5}{9}\delta^{pr}\lambda g_Y^2 + \frac{80}{81}\delta^{pr}g_Y^4 + \frac{8}{3}g_s^2(Y_u^\dagger Y_u)^{pr} + 4(Y_u^\dagger Y_u Y_u^\dagger Y_u)^{pr} \\
& -g_Y^2\Big(\frac{1}{9}\text{T}_2\delta^{pr} + \frac{517}{144}(Y_u^\dagger Y_u)^{pr}\Big) - 2(Y_u^\dagger Y_d Y_d^\dagger Y_u)^{pr} - \frac{137}{48}g_L^2(Y_u^\dagger Y_u)^{pr}\Big\}C_{HD}^{(\parallel)} + \Big\{\frac{5}{9}\delta^{pr}\lambda g_Y^2 + \frac{181}{324}\delta^{pr}g_Y^4 + \text{T}_2(Y_u^\dagger Y_u)^{pr} + 2(Y_u^\dagger Y_d Y_d^\dagger Y_u)^{pr} \\
& + \frac{41}{12}\delta^{pr}g_Y^2g_L^2 + 5(Y_u^\dagger Y_u Y_u^\dagger Y_u)^{pr} + \frac{16}{3}g_s^2(Y_u^\dagger Y_u)^{pr} - g_Y^2\Big(\frac{2}{9}\text{T}_2\delta^{pr} + \frac{14}{9}(Y_u^\dagger Y_u)^{pr}\Big) - 9g_L^2(Y_u^\dagger Y_u)^{pr}\Big\}C_{HD}^{(\times)} + \Big\{2\delta^{pr}g_Y^4g_L^2 + \frac{23}{9}g_Y^4(Y_u^\dagger Y_u)^{pr} \\
& + \frac{50}{9}\delta^{pr}g_Y^6 - 8\delta^{pr}\lambda g_Y^4\Big\}C_{HB} + \frac{4}{3}\delta^{pr}g_Y^2g_L^4C_{HW} + \Big\{\frac{32}{3}\delta^{pr}g_Y^2g_s^4 + \frac{80}{3}g_s^4(Y_u^\dagger Y_u)^{pr}\Big\}C_{HG} + \Big\{\frac{11}{6}\delta^{pr}g_Y^4g_L^2 - 2\delta^{pr}\lambda g_Y^2g_L^2 \\
& - \frac{11}{4}g_Y^2g_L^2(Y_u^\dagger Y_u)^{pr} - \frac{9}{2}\delta^{pr}g_Y^2g_L^4\Big\}C_{HWB} + \Big\{\frac{8}{3}\delta^{pr}g_Y^2g_L^6 - 3g_L^6(Y_u^\dagger Y_u)^{pr}\Big\}C_W + \Big\{\frac{160}{9}\delta^{pr}g_Y^2g_s^6 - 8g_s^6(Y_u^\dagger Y_u)^{pr}\Big\}C_G + \Big\{\frac{3}{4}\delta^{rb}g_Y^2Y_u^{*ap} \\
& + \frac{3}{2}\delta^{rb}\lambda Y_u^{*ap} + \frac{3}{2}\delta^{rb}(Y_u^\dagger Y_u Y_u^\dagger)^{ap} - \frac{9}{4}\delta^{rb}g_L^2Y_u^{*ap}\Big\}C_{uH}^{ab} + C_{uH}^{*ab}\Big\{\frac{3}{4}\delta^{pb}g_Y^2Y_u^{ar} + \frac{3}{2}\delta^{pb}\lambda Y_u^{ar} + \frac{3}{2}\delta^{pb}(Y_u Y_u^\dagger Y_u)^{ar} - \frac{9}{4}\delta^{pb}g_L^2Y_u^{ar}\Big\} \\
& + \Big\{\frac{2}{3}\delta^{pr}g_Y^2(Y_e^\dagger Y_e Y_e^\dagger)^{ab} + 11\delta^{pr}g_Y^4Y_e^{*ab} - 2\delta^{pr}g_Y^2g_L^2Y_e^{*ab}\Big\}C_{eB}^{ab} + C_{eB}^{*ab}\Big\{\frac{2}{3}\delta^{pr}g_Y^2(Y_e Y_e^\dagger Y_e)^{ab} + 11\delta^{pr}g_Y^4Y_e^{ab} - 2\delta^{pr}g_Y^2g_L^2Y_e^{ab}\Big\} \\
& + \frac{5}{6}\delta^{pr}g_Y^2g_L^2Y_e^{*ab}C_{eW}^{ab} + \frac{5}{6}\delta^{pr}g_Y^2g_L^2C_{eW}^{*ab}Y_e^{ab} + \Big\{g_Y^2g_L^2\big(6\delta^{pr}Y_u^{*ab} - \frac{13}{8}\delta^{rb}Y_u^{*ap}\big) + g_Y^4\big(\frac{25}{3}\delta^{pr}Y_u^{*ab} + \frac{1019}{72}\delta^{rb}Y_u^{*ap}\big) + g_Y^2\big(\frac{1}{3}\delta^{rb}(Y_u^\dagger Y_u Y_u^\dagger)^{ap}
\end{aligned}$$

$$\begin{aligned}
& -\frac{1}{6}\delta^{rb}(Y_d^\dagger Y_d Y_u^\dagger)^{ap} - \frac{3}{2}T_2\delta^{rb}Y_u^{*ap} - 2\delta^{pr}(Y_d^\dagger Y_d Y_u^\dagger)^{ab} - 2\delta^{pr}(Y_u^\dagger Y_u Y_u^\dagger)^{ab} - 7Y_u^{*ap}(Y_u^\dagger Y_u)^{br}) + \frac{32}{9}\delta^{rb}g_Y^2g_s^2Y_u^{*ap} - 9\delta^{rb}\lambda g_Y^2Y_u^{*ap}\Big\}C_{uB}^{ab} \\
& + C_{uB}^{*ab}\Big\{g_Y^2g_L^2\Big(6\delta^{pr}Y_u^{ab} - \frac{13}{8}\delta^{pb}Y_u^{ar}\Big) + g_Y^4\Big(\frac{25}{3}\delta^{pr}Y_u^{ab} + \frac{1019}{72}\delta^{pb}Y_u^{ar}\Big) + g_Y^2\Big(\frac{1}{3}\delta^{pb}(Y_u Y_u^\dagger Y_u)^{ar} - \frac{1}{6}\delta^{pb}(Y_d Y_d^\dagger Y_u)^{ar} - \frac{3}{2}T_2\delta^{pb}Y_u^{ar} \\
& - 2\delta^{pr}(Y_d Y_d^\dagger Y_u)^{ab} - 2\delta^{pr}(Y_u Y_u^\dagger Y_u)^{ab} - 7Y_u^{ar}(Y_u^\dagger Y_u)^{pb}\Big) + \frac{32}{9}\delta^{pb}g_Y^2g_s^2Y_u^{ar} - 9\delta^{pb}\lambda g_Y^2Y_u^{ar}\Big\} + \Big\{g_Y^2g_L^2\Big(\frac{1}{2}\delta^{pr}Y_u^{*ab} - \frac{75}{16}\delta^{rb}Y_u^{*ap}\Big) \\
& + g_L^2\Big(\frac{9}{4}T_2\delta^{rb}Y_u^{*ap} + \frac{21}{4}\delta^{rb}(Y_d^\dagger Y_d Y_u^\dagger)^{ap} - \frac{9}{2}\delta^{rb}(Y_u^\dagger Y_u Y_u^\dagger)^{ap}\Big) + \frac{69}{16}\delta^{rb}g_L^4Y_u^{*ap} + \frac{9}{2}\delta^{rb}\lambda g_L^2Y_u^{*ap} + 8\delta^{rb}g_s^2g_L^2Y_u^{*ap}\Big\}C_{uW}^{ab} \\
& + C_{uW}^{*ab}\Big\{g_Y^2g_L^2\Big(\frac{1}{2}\delta^{pr}Y_u^{ab} - \frac{75}{16}\delta^{pb}Y_u^{ar}\Big) + g_L^2\Big(\frac{9}{4}T_2\delta^{pb}Y_u^{ar} + \frac{21}{4}\delta^{pb}(Y_d Y_d^\dagger Y_u)^{ar} - \frac{9}{2}\delta^{pb}(Y_u Y_u^\dagger Y_u)^{ar}\Big) + \frac{69}{16}\delta^{pb}g_L^4Y_u^{ar} + \frac{9}{2}\delta^{pb}\lambda g_L^2Y_u^{ar} \\
& + 8\delta^{pb}g_s^2g_L^2Y_u^{ar}\Big\} + \Big\{g_s^4\Big(16\delta^{pr}Y_u^{*ab} - \frac{320}{9}\delta^{rb}Y_u^{*ap}\Big) + g_Y^2g_s^2\Big(\frac{22}{9}\delta^{rb}Y_u^{*ap} - \frac{64}{9}\delta^{pr}Y_u^{*ab}\Big) + g_s^2\Big(\frac{8}{3}\delta^{rb}(Y_d^\dagger Y_d Y_u^\dagger)^{ap} - \frac{4}{3}\delta^{rb}(Y_u^\dagger Y_u Y_u^\dagger)^{ap} \\
& - 12Y_u^{*ap}(Y_u^\dagger Y_u)^{br}\Big) - 10\delta^{rb}g_s^2g_L^2Y_u^{*ap}\Big\}C_{uG}^{ab} + C_{uG}^{*ab}\Big\{g_s^4\Big(16\delta^{pr}Y_u^{ab} - \frac{320}{9}\delta^{pb}Y_u^{ar}\Big) + g_Y^2g_s^2\Big(\frac{22}{9}\delta^{pb}Y_u^{ar} - \frac{64}{9}\delta^{pr}Y_u^{ab}\Big) + g_s^2\Big(\frac{8}{3}\delta^{pb}(Y_d Y_d^\dagger Y_u)^{ar} \\
& - \frac{4}{3}\delta^{pb}(Y_u Y_u^\dagger Y_u)^{ar} - 12Y_u^{ar}(Y_u^\dagger Y_u)^{pb}\Big) - 10\delta^{pb}g_s^2g_L^2Y_u^{ar}\Big\} + \Big\{g_Y^2\Big(2\delta^{pr}(Y_d^\dagger Y_d Y_d^\dagger)^{ab} + 2\delta^{pr}(Y_u^\dagger Y_u Y_d^\dagger)^{ab} + \frac{17}{3}Y_u^{*ap}(Y_d^\dagger Y_u)^{br}\Big) + \frac{11}{3}\delta^{pr}g_Y^4Y_d^{*ab} \\
& - 6\delta^{pr}g_Y^2g_L^2Y_d^{*ab}\Big\}C_{dB}^{ab} + C_{dB}^{*ab}\Big\{g_Y^2\Big(2\delta^{pr}(Y_d Y_d^\dagger Y_d)^{ab} + 2\delta^{pr}(Y_u Y_u^\dagger Y_d)^{ab} + \frac{17}{3}Y_u^{ar}(Y_u^\dagger Y_d)^{pb}\Big) + \frac{11}{3}\delta^{pr}g_Y^4Y_d^{ab} - 6\delta^{pr}g_Y^2g_L^2Y_d^{ab}\Big\} \\
& - \frac{3}{2}\delta^{pr}g_Y^2g_L^2Y_d^{*ab}C_{dW}^{ab} - \frac{3}{2}\delta^{pr}g_Y^2g_L^2C_{dW}^{*ab}Y_d^{ab} + \Big\{\frac{40}{3}g_s^2Y_u^{*ap}(Y_d^\dagger Y_u)^{br} - \frac{64}{9}\delta^{pr}g_Y^2g_s^2Y_d^{*ab} - 16\delta^{pr}g_s^4Y_d^{*ab}\Big\}C_{dG}^{ab} \\
& + C_{dG}^{*ab}\Big\{\frac{40}{3}g_s^2Y_u^{ar}(Y_u^\dagger Y_d)^{pb} - \frac{64}{9}\delta^{pr}g_Y^2g_s^2Y_d^{ab} - 16\delta^{pr}g_s^4Y_d^{ab}\Big\} + \Big\{\frac{1}{2}(Y_u^\dagger Y_u)^{pr}(Y_e Y_e^\dagger)^{ba} + g_Y^2\Big(\frac{49}{27}\delta^{pr}(Y_e Y_e^\dagger)^{ba} + \frac{13}{6}\delta^{ab}(Y_u^\dagger Y_u)^{pr}\Big) - 2\delta^{pr}\delta^{ab}g_Y^2g_L^2 \\
& - \frac{241}{81}\delta^{pr}\delta^{ab}g_Y^4\Big\}C_{H\ell}^{(\parallel)ab} + \Big\{\frac{1}{12}\delta^{ab}g_L^2(Y_u^\dagger Y_u)^{pr} + g_Y^2\Big(\frac{26}{27}\delta^{pr}(Y_e Y_e^\dagger)^{ba} + \frac{13}{12}\delta^{ab}(Y_u^\dagger Y_u)^{pr}\Big) - \frac{1}{2}(Y_u^\dagger Y_u)^{pr}(Y_e Y_e^\dagger)^{ba} - \frac{241}{162}\delta^{pr}\delta^{ab}g_Y^4 \\
& - \frac{83}{54}\delta^{pr}\delta^{ab}g_Y^2g_L^2\Big\}C_{H\ell}^{(\times)ab} + \Big\{g_Y^2\Big(\frac{13}{6}\delta^{ab}(Y_u^\dagger Y_u)^{pr} + \frac{77}{27}\delta^{pr}(Y_e^\dagger Y_e)^{ba}\Big) + \frac{245}{81}\delta^{pr}\delta^{ab}g_Y^4 - \frac{1}{2}(Y_e^\dagger Y_e)^{ba}(Y_u^\dagger Y_u)^{pr}\Big\}C_{He}^{ab} + \Big\{\frac{3}{2}(Y_u^\dagger Y_u)^{pr}(Y_d Y_d^\dagger)^{ba} \\
& + 2\delta^{pr}\delta^{ab}g_Y^2g_L^2 + 3T_2Y_u^{*ap}Y_u^{br} + \frac{32}{9}\delta^{pr}\delta^{ab}g_Y^2g_s^2 + \frac{43}{12}Y_u^{br}(Y_d^\dagger Y_d Y_u^\dagger)^{ap} + \frac{43}{12}Y_u^{*ap}(Y_d Y_d^\dagger Y_u)^{br} + \frac{47}{12}Y_u^{br}(Y_u^\dagger Y_u Y_u^\dagger)^{ap} + \frac{47}{12}Y_u^{*ap}(Y_u Y_u^\dagger Y_u)^{br}
\end{aligned}$$

$$\begin{aligned}
& + \frac{16}{3} g_s^2 Y_u^{*ap} Y_u^{br} - g_Y^2 \left( \frac{7}{9} \delta^{pr} (Y_d Y_d^\dagger)^{ba} + \frac{97}{54} Y_u^{*ap} Y_u^{br} + \frac{13}{6} \delta^{ab} (Y_u^\dagger Y_u)^{pr} + \frac{7}{3} \delta^{pr} (Y_u Y_u^\dagger)^{ba} \right) - \frac{95}{81} \delta^{pr} \delta^{ab} g_Y^4 - \frac{3}{2} (Y_u^\dagger Y_u)^{pr} (Y_u Y_u^\dagger)^{ba} - 12 g_L^2 Y_u^{*ap} Y_u^{br} \\
& - 16 \delta^{pr} \delta^{ab} g_s^4 \left\{ C_{Hq}^{(\parallel)ab} + \left\{ g_L^2 \left( \frac{1}{4} \delta^{ab} (Y_u^\dagger Y_u)^{pr} - \frac{137}{24} Y_u^{*ap} Y_u^{br} \right) + \frac{3}{2} T_2 Y_u^{*ap} Y_u^{br} + \frac{16}{9} \delta^{pr} \delta^{ab} g_Y^2 g_s^2 + \frac{77}{12} Y_u^{br} (Y_d^\dagger Y_d Y_u^\dagger)^{ap} + \frac{77}{12} Y_u^{*ap} (Y_d Y_d^\dagger Y_u)^{br} \right. \right. \\
& + \frac{32}{3} g_s^2 Y_u^{*ap} Y_u^{br} - \frac{95}{162} \delta^{pr} \delta^{ab} g_Y^4 - \frac{11}{18} \delta^{pr} \delta^{ab} g_Y^2 g_L^2 - \frac{11}{12} Y_u^{br} (Y_u^\dagger Y_u Y_u^\dagger)^{ap} - \frac{11}{12} Y_u^{*ap} (Y_u Y_u^\dagger Y_u)^{br} - g_Y^2 \left( \frac{131}{216} Y_u^{*ap} Y_u^{br} + \frac{13}{12} \delta^{ab} (Y_u^\dagger Y_u)^{pr} \right. \\
& + \frac{14}{9} \delta^{pr} (Y_d Y_d^\dagger)^{ba} + \frac{5}{3} \delta^{pr} (Y_u Y_u^\dagger)^{ba} \left. \left. - \frac{3}{2} (Y_u^\dagger Y_u)^{pr} (Y_d Y_d^\dagger)^{ba} - 3 (Y_u^\dagger Y_u)^{pr} (Y_u Y_u^\dagger)^{ba} - 8 \delta^{pr} \delta^{ab} g_s^4 \right\} C_{Hq}^{(\times)ab} + \left\{ g_Y^4 \left( \frac{710}{81} \delta^{pr} \delta^{ab} - \frac{1237}{243} \delta^{pa} \delta^{rb} \right) \right. \right. \\
& + g_L^2 \left( \frac{93}{8} \delta^{rb} (Y_u^\dagger Y_u)^{pa} + \frac{93}{8} \delta^{pa} (Y_u^\dagger Y_u)^{br} - \frac{3}{4} T_2 \delta^{pa} \delta^{rb} \right) + g_Y^2 \left( \frac{19}{12} \delta^{pa} \delta^{rb} \text{Tr}[Y_u^\dagger Y_u] + \frac{53}{12} \delta^{pa} \delta^{rb} \text{Tr}[Y_e^\dagger Y_e] + \frac{1739}{216} \delta^{rb} (Y_u^\dagger Y_u)^{pa} + \frac{1739}{216} \delta^{pa} (Y_u^\dagger Y_u)^{br} \right. \\
& - \frac{41}{12} \delta^{pa} \delta^{rb} \text{Tr}[Y_d^\dagger Y_d] - \frac{13}{3} \delta^{ab} (Y_u^\dagger Y_u)^{pr} - \frac{49}{9} \delta^{pr} (Y_u^\dagger Y_u)^{ba} \left. \left. + g_s^2 \left( \frac{4}{3} \delta^{rb} (Y_u^\dagger Y_u)^{pa} + \frac{4}{3} \delta^{pa} (Y_u^\dagger Y_u)^{br} + 40 \delta^{pa} \delta^{rb} \text{Tr}[Y_d^\dagger Y_d] + 40 \delta^{pa} \delta^{rb} \text{Tr}[Y_u^\dagger Y_u] \right) \right. \right. \\
& + \frac{3}{2} (Y_u^\dagger Y_u)^{pr} (Y_u^\dagger Y_u)^{ba} + 3 \delta^{pa} \delta^{rb} g_Y^2 g_L^2 + 3 \delta^{rb} (Y_u^\dagger Y_d Y_d^\dagger Y_u)^{pa} + 3 \delta^{pa} (Y_u^\dagger Y_d Y_d^\dagger Y_u)^{br} + 6 \delta^{pa} \delta^{rb} \text{Tr}[Y_d^\dagger Y_d Y_u^\dagger Y_u] + \frac{64}{9} \delta^{pr} \delta^{ab} g_Y^2 g_s^2 + 8 \delta^{pr} \delta^{ab} g_s^4 \\
& - \lambda \left( 9 \delta^{rb} (Y_u^\dagger Y_u)^{pa} + 9 \delta^{pa} (Y_u^\dagger Y_u)^{br} \right) - \frac{9}{2} (Y_u^\dagger Y_u)^{pa} (Y_u^\dagger Y_u)^{br} - 5 T_2 \delta^{rb} (Y_u^\dagger Y_u)^{pa} - 5 T_2 \delta^{pa} (Y_u^\dagger Y_u)^{br} - 6 T_4 \delta^{pa} \delta^{rb} - \frac{31}{4} \delta^{rb} (Y_u^\dagger Y_u Y_u^\dagger Y_u)^{pa} \\
& - \frac{31}{4} \delta^{pa} (Y_u^\dagger Y_u Y_u^\dagger Y_u)^{br} \left\{ C_{Hu}^{ab} + \left\{ g_Y^2 \left( \frac{13}{6} \delta^{ab} (Y_u^\dagger Y_u)^{pr} + \frac{7}{3} \delta^{pr} (Y_d^\dagger Y_d)^{ba} \right) + \frac{149}{81} \delta^{pr} \delta^{ab} g_Y^4 + 8 \delta^{pr} \delta^{ab} g_s^4 - \frac{3}{2} (Y_d^\dagger Y_d)^{ba} (Y_u^\dagger Y_u)^{pr} - 2 (Y_d^\dagger Y_u)^{br} (Y_u^\dagger Y_d)^{pa} \right. \right. \\
& - \frac{32}{9} \delta^{pr} \delta^{ab} g_Y^2 g_s^2 \left. \left. \right\} C_{Hd}^{ab} + \left\{ \frac{1}{4} (Y_d^\dagger Y_u)^{br} (Y_u^\dagger Y_u)^{pa} + \frac{1}{2} \delta^{pa} (Y_d^\dagger Y_u Y_u^\dagger Y_u)^{br} + g_Y^2 \left( \frac{16}{27} \delta^{pa} (Y_d^\dagger Y_u)^{br} + \frac{17}{9} \delta^{pr} (Y_d^\dagger Y_u)^{ba} \right) + 4 \delta^{pa} g_s^2 (Y_d^\dagger Y_u)^{br} \right. \right. \\
& - \frac{1}{2} T_2 \delta^{pa} (Y_d^\dagger Y_u)^{br} - \frac{3}{2} (Y_d^\dagger Y_u)^{ba} (Y_u^\dagger Y_u)^{pr} - \frac{21}{4} \delta^{pa} (Y_d^\dagger Y_d Y_d^\dagger Y_u)^{br} \left. \left. \right\} C_{Hud}^{ab} + C_{Hud}^{*ab} \left\{ \frac{1}{4} (Y_u^\dagger Y_d)^{pb} (Y_u^\dagger Y_u)^{ar} + \frac{1}{2} \delta^{ra} (Y_u^\dagger Y_u Y_u^\dagger Y_d)^{pb} \right. \right. \\
& + g_Y^2 \left( \frac{16}{27} \delta^{ra} (Y_u^\dagger Y_d)^{pb} + \frac{17}{9} \delta^{pr} (Y_u^\dagger Y_d)^{ab} \right) + 4 \delta^{ra} g_s^2 (Y_u^\dagger Y_d)^{pb} - \frac{1}{2} T_2 \delta^{ra} (Y_u^\dagger Y_d)^{pb} - \frac{3}{2} (Y_u^\dagger Y_d)^{ab} (Y_u^\dagger Y_u)^{pr} - \frac{21}{4} \delta^{ra} (Y_u^\dagger Y_d Y_d^\dagger Y_d)^{pb} \left. \left. \right\} \right. \\
& + \left\{ \frac{3}{4} \delta^{pc} \delta^{rd} g_L^2 (Y_e Y_e^\dagger)^{ba} + \delta^{rd} (Y_u^\dagger Y_u)^{pc} (Y_e Y_e^\dagger)^{ba} + \delta^{pc} (Y_u^\dagger Y_u)^{dr} (Y_e Y_e^\dagger)^{ba} + 6 \delta^{pc} \delta^{rd} (Y_e Y_e^\dagger Y_e Y_e^\dagger)^{ba} - g_Y^2 \left( \frac{1}{12} \delta^{pc} \delta^{rd} (Y_e Y_e^\dagger)^{ba} + \frac{10}{27} \delta^{rd} \delta^{ab} (Y_u^\dagger Y_u)^{pc} \right. \right. \\
& + \frac{10}{27} \delta^{pc} \delta^{ab} (Y_u^\dagger Y_u)^{dr} \left. \left. \right) - \frac{3}{2} \delta^{pc} \delta^{rd} \delta^{ab} g_Y^2 g_L^2 - \frac{887}{486} \delta^{pc} \delta^{rd} \delta^{ab} g_Y^4 \right\} C_{lu}^{abcd} + \left\{ \frac{13}{27} \delta^{cd} g_Y^2 Y_u^{*ap} Y_u^{br} + Y_u^{*ap} Y_u^{br} (Y_e^\dagger Y_e)^{dc} \right\} C_{qe}^{abcd} + \left\{ \frac{1}{3} Y_u^{*ad} Y_u^{br} (Y_u^\dagger Y_u)^{pc} \right. \\
& + \frac{1}{3} Y_u^{*ap} Y_u^{bc} (Y_u^\dagger Y_u)^{dr} + g_L^2 \left( \frac{3}{4} \delta^{pc} Y_u^{*ad} Y_u^{br} + \frac{3}{4} \delta^{rd} Y_u^{*ap} Y_u^{bc} + \frac{9}{4} \delta^{pc} \delta^{rd} (Y_d Y_d^\dagger)^{ba} - \frac{9}{4} \delta^{pc} \delta^{rd} (Y_u Y_u^\dagger)^{ba} \right) + g_Y^2 \left( \frac{10}{27} \delta^{rd} \delta^{ab} (Y_u^\dagger Y_u)^{pc} + \frac{10}{27} \delta^{pc} \delta^{ab} (Y_u^\dagger Y_u)^{dr} \right. \\
& + \frac{143}{12} \delta^{pc} \delta^{rd} (Y_u Y_u^\dagger)^{ba} + \frac{181}{12} \delta^{pc} \delta^{rd} (Y_d Y_d^\dagger)^{ba} - \frac{26}{27} \delta^{cd} Y_u^{*ap} Y_u^{br} - \frac{181}{108} \delta^{pc} Y_u^{*ad} Y_u^{br} - \frac{181}{108} \delta^{rd} Y_u^{*ap} Y_u^{bc} \left. \left. \right) + g_s^2 \left( 40 \delta^{pc} \delta^{rd} (Y_u Y_u^\dagger)^{ba} \right. \right.
\end{aligned}$$

$$\begin{aligned}
& -40\delta^{pc}\delta^{rd}(Y_d Y_d^\dagger)^{ba}) + \frac{3}{2}\delta^{pc}\delta^{rd}\delta^{ab}g_Y^2g_L^2 + \frac{3}{2}\delta^{pc}Y_u^{br}(Y_d^\dagger Y_d Y_u^\dagger)^{ad} + \frac{3}{2}\delta^{rd}Y_u^{*ap}(Y_d Y_d^\dagger Y_u)^{bc} + \frac{8}{3}\delta^{pc}\delta^{rd}\delta^{ab}g_Y^2g_s^2 + 3\delta^{rd}(Y_u^\dagger Y_u)^{pc}(Y_d Y_d^\dagger)^{ba} \\
& + 3\delta^{pc}(Y_u^\dagger Y_u)^{dr}(Y_d Y_d^\dagger)^{ba} + 18\delta^{pc}\delta^{rd}(Y_d Y_d^\dagger Y_d Y_d^\dagger)^{ba} - \delta^{rd}Y_u^{bc}(Y_u^\dagger Y_u Y_u^\dagger)^{ap} - \delta^{pc}Y_u^{*ad}(Y_u Y_u^\dagger Y_u)^{br} - \frac{913}{486}\delta^{pc}\delta^{rd}\delta^{ab}g_Y^4 - \frac{5}{2}\delta^{pc}Y_u^{br}(Y_u^\dagger Y_u Y_u^\dagger)^{ad} \\
& - \frac{5}{2}\delta^{rd}Y_u^{*ap}(Y_u Y_u^\dagger Y_u)^{bc} - 3Y_u^{*ap}Y_u^{br}(Y_u^\dagger Y_u)^{dc} - 3\delta^{rd}(Y_u^\dagger Y_u)^{pc}(Y_u Y_u^\dagger)^{ba} - 3\delta^{pc}(Y_u^\dagger Y_u)^{dr}(Y_u Y_u^\dagger)^{ba} - 18\delta^{pc}\delta^{rd}(Y_u Y_u^\dagger Y_u Y_u^\dagger)^{ba} \Big\} C_{qu}^{(\parallel)abcd} \\
& + \left\{ \frac{1}{2}\delta^{pc}\delta^{rd}\delta^{ab}g_Y^2g_L^2 + Y_u^{*ad}Y_u^{br}(Y_u^\dagger Y_u)^{pc} + Y_u^{*ap}Y_u^{bc}(Y_u^\dagger Y_u)^{dr} + \delta^{rd}(Y_u^\dagger Y_u)^{pc}(Y_d Y_d^\dagger)^{ba} + \delta^{pc}(Y_u^\dagger Y_u)^{dr}(Y_d Y_d^\dagger)^{ba} + g_L^2\left(\frac{3}{4}\delta^{pc}\delta^{rd}(Y_d Y_d^\dagger)^{ba} + \frac{9}{4}\delta^{pc}Y_u^{*ad}Y_u^{br} \right. \right. \\
& + \frac{9}{4}\delta^{rd}Y_u^{*ap}Y_u^{bc} - \frac{3}{4}\delta^{pc}\delta^{rd}(Y_u Y_u^\dagger)^{ba}) + g_Y^2\left(\frac{10}{81}\delta^{cd}Y_u^{*ap}Y_u^{br} + \frac{10}{81}\delta^{rd}\delta^{ab}(Y_u^\dagger Y_u)^{pc} + \frac{10}{81}\delta^{pc}\delta^{ab}(Y_u^\dagger Y_u)^{dr} + \frac{53}{12}\delta^{pc}\delta^{rd}(Y_u Y_u^\dagger)^{ba} + \frac{181}{36}\delta^{pc}\delta^{rd}(Y_d Y_d^\dagger)^{ba} \right. \\
& - \frac{229}{36}\delta^{pc}Y_u^{*ad}Y_u^{br} - \frac{229}{36}\delta^{rd}Y_u^{*ap}Y_u^{bc}) + g_s^2\left(\frac{4}{27}\delta^{rd}\delta^{ab}(Y_u^\dagger Y_u)^{pc} + \frac{4}{27}\delta^{pc}\delta^{ab}(Y_u^\dagger Y_u)^{dr} + \frac{4}{3}\delta^{pr}\delta^{ab}(Y_u^\dagger Y_u)^{dc} + \frac{4}{3}\delta^{pc}\delta^{rd}\delta^{ab}\text{Tr}[Y_u^\dagger Y_u] \right. \\
& + \frac{32}{3}\delta^{pc}\delta^{rd}(Y_u Y_u^\dagger)^{ba} - \frac{32}{27}\delta^{cd}Y_u^{*ap}Y_u^{br} - \frac{32}{3}\delta^{pc}\delta^{rd}(Y_d Y_d^\dagger)^{ba}) + \frac{9}{2}\delta^{pc}Y_u^{br}(Y_d^\dagger Y_d Y_u^\dagger)^{ad} + \frac{9}{2}\delta^{rd}Y_u^{*ap}(Y_d Y_d^\dagger Y_u)^{bc} + 6\delta^{pc}\delta^{rd}(Y_d Y_d^\dagger Y_d Y_d^\dagger)^{ba} \\
& - \frac{913}{1458}\delta^{pc}\delta^{rd}\delta^{ab}g_Y^4 - g_Y^2g_s^2\left(\frac{8}{27}\delta^{pr}\delta^{ab}\delta^{cd} + \frac{1448}{243}\delta^{pc}\delta^{rd}\delta^{ab}\right) - \delta^{rd}(Y_u^\dagger Y_u)^{pc}(Y_u Y_u^\dagger)^{ba} - \delta^{pc}(Y_u^\dagger Y_u)^{dr}(Y_u Y_u^\dagger)^{ba} - \frac{3}{2}\delta^{pc}Y_u^{br}(Y_u^\dagger Y_u Y_u^\dagger)^{ad} \\
& - \frac{3}{2}\delta^{rd}Y_u^{*ap}(Y_u Y_u^\dagger Y_u)^{bc} - 3Y_u^{*ap}Y_u^{br}(Y_u^\dagger Y_u)^{dc} - 3\delta^{rd}Y_u^{bc}(Y_u^\dagger Y_u Y_u^\dagger)^{ap} - 3\delta^{pc}Y_u^{*ad}(Y_u Y_u^\dagger Y_u)^{br} - 8\delta^{pc}\delta^{rd}(Y_u Y_u^\dagger Y_u Y_u^\dagger)^{ba} \Big\} C_{qu}^{(\times)abcd} \\
& + \left\{ \frac{13}{27}\delta^{cd}g_Y^2Y_u^{*ap}Y_u^{br} + 3Y_u^{*ap}Y_u^{br}(Y_d^\dagger Y_d)^{dc} - \frac{2}{3}Y_u^{*ap}Y_d^{bc}(Y_d^\dagger Y_u)^{dr} - \frac{2}{3}Y_d^{*ad}Y_u^{br}(Y_u^\dagger Y_d)^{pc} \right\} C_{qd}^{(\parallel)abcd} + \left\{ \frac{13}{81}\delta^{cd}g_Y^2Y_u^{*ap}Y_u^{br} + Y_u^{*ap}Y_u^{br}(Y_d^\dagger Y_d)^{dc} \right. \\
& - \frac{32}{27}\delta^{cd}g_s^2Y_u^{*ap}Y_u^{br} - 2Y_u^{*ap}Y_d^{bc}(Y_d^\dagger Y_u)^{dr} - 2Y_d^{*ad}Y_u^{br}(Y_u^\dagger Y_d)^{pc} \Big\} C_{qd}^{(\times)abcd} + \left\{ \frac{32}{27}\delta^{pr}\delta^{ab}\delta^{cd}g_Y^4 - \frac{32}{9}\delta^{pr}\delta^{ad}g_Y^2(Y_e^\dagger Y_e)^{bc} \right\} C_{ee}^{abcd} + \left\{ g_Y^4\left(\frac{128}{81}\delta^{pr}\delta^{ad}\delta^{bc} \right. \right. \\
& - \frac{512}{243}\delta^{pa}\delta^{rb}\delta^{cd} - \frac{1856}{729}\delta^{pa}\delta^{rd}\delta^{bc}) + g_Y^2g_s^2\left(\frac{304}{243}\delta^{pa}\delta^{rd}\delta^{bc} + 8\delta^{pa}\delta^{rb}\delta^{cd} - \frac{8}{27}\delta^{pr}\delta^{ad}\delta^{bc}\right) + g_L^2\left(\frac{9}{2}\delta^{pa}\delta^{rb}(Y_u^\dagger Y_u)^{dc} - \frac{15}{2}\delta^{pa}\delta^{rd}(Y_u^\dagger Y_u)^{bc} \right. \\
& + g_Y^2\left(\frac{52}{81}\delta^{rb}\delta^{ad}(Y_u^\dagger Y_u)^{pc} + \frac{52}{81}\delta^{pa}\delta^{bc}(Y_u^\dagger Y_u)^{dr} + \frac{40}{27}\delta^{rb}\delta^{cd}(Y_u^\dagger Y_u)^{pa} + \frac{40}{27}\delta^{pa}\delta^{cd}(Y_u^\dagger Y_u)^{br} + \frac{199}{18}\delta^{pa}\delta^{rd}(Y_u^\dagger Y_u)^{bc} + \frac{47}{2}\delta^{pa}\delta^{rb}(Y_u^\dagger Y_u)^{dc} \right. \\
& - \frac{64}{9}\delta^{pr}\delta^{ad}(Y_u^\dagger Y_u)^{bc}) + g_s^2\left(\frac{4}{3}\delta^{pr}\delta^{ad}(Y_u^\dagger Y_u)^{bc} + \frac{4}{3}\delta^{pa}\delta^{rd}\delta^{bc}\text{Tr}[Y_u^\dagger Y_u] - \frac{92}{27}\delta^{rb}\delta^{ad}(Y_u^\dagger Y_u)^{pc} - \frac{92}{27}\delta^{pa}\delta^{bc}(Y_u^\dagger Y_u)^{dr} - 4\delta^{pa}\delta^{rd}(Y_u^\dagger Y_u)^{bc} \right. \\
& - 68\delta^{pa}\delta^{rb}(Y_u^\dagger Y_u)^{dc}) + 6\delta^{rb}(Y_u^\dagger Y_u)^{pa}(Y_u^\dagger Y_u)^{dc} + 6\delta^{pa}(Y_u^\dagger Y_u)^{br}(Y_u^\dagger Y_u)^{dc} + 20\delta^{pa}\delta^{rd}(Y_u^\dagger Y_u Y_u^\dagger Y_u)^{bc} + 36\delta^{pa}\delta^{rb}(Y_u^\dagger Y_u Y_u^\dagger Y_u)^{dc} \\
& - 4\delta^{pa}(Y_u^\dagger Y_u)^{bc}(Y_u^\dagger Y_u)^{dr} - 4\delta^{rb}(Y_u^\dagger Y_u)^{pc}(Y_u^\dagger Y_u)^{da} - 6\delta^{pa}\delta^{rd}(Y_u^\dagger Y_d Y_d^\dagger Y_u)^{bc} - 6\delta^{pa}\delta^{rb}(Y_u^\dagger Y_d Y_d^\dagger Y_u)^{dc} \Big\} C_{uu}^{abcd} + \left\{ \frac{32}{81}\delta^{pr}\delta^{ad}\delta^{bc}g_Y^4 \right. \\
& - \frac{32}{9}\delta^{pr}\delta^{ad}g_Y^2(Y_d^\dagger Y_d)^{bc} \Big\} C_{dd}^{abcd} + \left\{ g_Y^2\left(\frac{205}{12}\delta^{pc}\delta^{rd}(Y_e^\dagger Y_e)^{ba} - \frac{10}{27}\delta^{rd}\delta^{ab}(Y_u^\dagger Y_u)^{pc} - \frac{10}{27}\delta^{pc}\delta^{ab}(Y_u^\dagger Y_u)^{dr}\right) - \frac{3}{4}\delta^{pc}\delta^{rd}g_L^2(Y_e^\dagger Y_e)^{ba} - \delta^{rd}(Y_e^\dagger Y_e)^{ba}(Y_u^\dagger Y_u)^{pc} \right.
\end{aligned}$$

$$\begin{aligned}
& -\delta^{pc}(Y_e^\dagger Y_e)^{ba}(Y_u^\dagger Y_u)^{dr} - \frac{322}{243}\delta^{pc}\delta^{rd}\delta^{ab}g_Y^4 - 6\delta^{pc}\delta^{rd}(Y_e^\dagger Y_e Y_e^\dagger Y_e)^{ba} \Big\} C_{eu}^{abcd} + \left\{ \frac{182}{243}\delta^{pa}\delta^{rb}\delta^{cd}g_Y^4 + g_Y^2 \left( \frac{5}{4}\delta^{pa}\delta^{rb}(Y_d^\dagger Y_d)^{dc} - \frac{10}{27}\delta^{rb}\delta^{cd}(Y_u^\dagger Y_u)^{pa} \right. \right. \\
& - \frac{10}{27}\delta^{pa}\delta^{cd}(Y_u^\dagger Y_u)^{br} \Big) + 2\delta^{rb}(Y_d^\dagger Y_u)^{da}(Y_u^\dagger Y_d)^{pc} + 2\delta^{pa}(Y_d^\dagger Y_u)^{dr}(Y_u^\dagger Y_d)^{bc} + 3\delta^{pa}\delta^{rb}(Y_d^\dagger Y_u Y_u^\dagger Y_d)^{dc} + 40\delta^{pa}\delta^{rb}g_s^2(Y_d^\dagger Y_d)^{dc} - \frac{9}{4}\delta^{pa}\delta^{rb}g_L^2(Y_d^\dagger Y_d)^{dc} \\
& - \frac{8}{3}\delta^{pa}\delta^{rb}\delta^{cd}g_Y^2g_s^2 - 3\delta^{rb}(Y_d^\dagger Y_d)^{dc}(Y_u^\dagger Y_u)^{pa} - 3\delta^{pa}(Y_d^\dagger Y_d)^{dc}(Y_u^\dagger Y_u)^{br} - 18\delta^{pa}\delta^{rb}(Y_d^\dagger Y_d Y_d^\dagger Y_d)^{dc} \Big\} C_{ud}^{(\parallel)abcd} + \left\{ \frac{182}{729}\delta^{pa}\delta^{rb}\delta^{cd}g_Y^4 \right. \\
& + g_Y^2 \left( \frac{5}{12}\delta^{pa}\delta^{rb}(Y_d^\dagger Y_d)^{dc} - \frac{10}{81}\delta^{rb}\delta^{cd}(Y_u^\dagger Y_u)^{pa} - \frac{10}{81}\delta^{pa}\delta^{cd}(Y_u^\dagger Y_u)^{br} \right) + \delta^{pa}\delta^{rb}(Y_d^\dagger Y_u Y_u^\dagger Y_d)^{dc} + g_s^2 \left( \frac{2}{27}\delta^{rb}\delta^{cd}(Y_u^\dagger Y_u)^{pa} + \frac{2}{27}\delta^{pa}\delta^{cd}(Y_u^\dagger Y_u)^{br} \right. \\
& + \frac{2}{3}\delta^{pr}\delta^{cd}(Y_u^\dagger Y_u)^{ba} + \frac{2}{3}\delta^{pa}\delta^{rb}\delta^{cd}\text{Tr}[Y_u^\dagger Y_u] - 16\delta^{pa}\delta^{rb}(Y_d^\dagger Y_d)^{dc} \Big) + 6\delta^{rb}(Y_d^\dagger Y_u)^{da}(Y_u^\dagger Y_d)^{pc} + 6\delta^{pa}(Y_d^\dagger Y_u)^{dr}(Y_u^\dagger Y_d)^{bc} - \frac{3}{4}\delta^{pa}\delta^{rb}g_L^2(Y_d^\dagger Y_d)^{dc} \\
& - g_Y^2g_s^2 \left( \frac{4}{27}\delta^{pr}\delta^{ab}\delta^{cd} + \frac{580}{243}\delta^{pa}\delta^{rb}\delta^{cd} \right) - \delta^{rb}(Y_d^\dagger Y_d)^{dc}(Y_u^\dagger Y_u)^{pa} - \delta^{pa}(Y_d^\dagger Y_d)^{dc}(Y_u^\dagger Y_u)^{br} - 6\delta^{pa}\delta^{rb}(Y_d^\dagger Y_d Y_d^\dagger Y_d)^{dc} \Big\} C_{ud}^{(\times)abcd} \\
& + \frac{1}{3}Y_e^{*ab}C_{ledq}^{abcd}Y_u^{dr}(Y_u^\dagger Y_d)^{pc} + \frac{1}{3}C_{ledq}^{*abcd}Y_u^{dp}Y_e^{ab}(Y_d^\dagger Y_u)^{cr} + \left\{ \frac{1}{6}Y_u^{*ap}Y_u^{*cb}(Y_d^\dagger Y_u)^{dr} + \frac{1}{2}\delta^{rb}Y_d^{*ad}(Y_u^\dagger Y_u Y_u^\dagger)^{cp} + g_Y^2 \left( \frac{19}{27}\delta^{rb}Y_d^{*ad}Y_u^{*cp} \right. \right. \\
& + \frac{181}{72}\delta^{rb}Y_d^{*cd}Y_u^{*ap} \Big) + Y_u^{*ab}Y_u^{*cp}(Y_d^\dagger Y_u)^{dr} + \frac{9}{4}\delta^{rb}Y_u^{*ap}(Y_d^\dagger Y_d Y_d^\dagger)^{cd} + 3\delta^{rb}Y_d^{*cd}(Y_u^\dagger Y_u Y_u^\dagger)^{ap} - \frac{1}{12}Y_d^{*ad}Y_u^{*cp}(Y_u^\dagger Y_u)^{br} - \frac{1}{4}\delta^{rb}Y_d^{*ad}(Y_d^\dagger Y_d Y_u^\dagger)^{cp} \\
& - \frac{1}{2}Y_d^{*cd}Y_u^{*ap}(Y_u^\dagger Y_u)^{br} - \frac{1}{2}\delta^{rb}Y_u^{*cp}(Y_d^\dagger Y_d Y_d^\dagger)^{ad} - \frac{3}{4}\delta^{rb}Y_u^{*ap}(Y_u^\dagger Y_u Y_d^\dagger)^{cd} - \frac{9}{8}\delta^{rb}g_L^2Y_d^{*cd}Y_u^{*ap} - \frac{3}{2}\delta^{rb}Y_d^{*cd}(Y_d^\dagger Y_d Y_u^\dagger)^{ap} - \frac{3}{2}\delta^{rb}Y_u^{*cp}(Y_u^\dagger Y_u Y_d^\dagger)^{ad} \\
& - \frac{16}{3}\delta^{rb}g_s^2Y_d^{*ad}Y_u^{*cp} \Big\} C_{quqd}^{(\parallel)abcd} + \left( C_{quqd}^{(\parallel)*} \right)^{abcd} \left\{ \frac{1}{6}Y_u^{ar}Y_u^{cb}(Y_u^\dagger Y_d)^{pd} + \frac{1}{2}\delta^{pb}Y_d^{ad}(Y_u Y_u^\dagger Y_u)^{cr} + g_Y^2 \left( \frac{19}{27}\delta^{pb}Y_d^{ad}Y_u^{cr} + \frac{181}{72}\delta^{pb}Y_d^{cd}Y_u^{ar} \right) + Y_u^{ab}Y_u^{cr}(Y_u^\dagger Y_d)^{pd} \right. \\
& + \frac{9}{4}\delta^{pb}Y_u^{ar}(Y_d Y_d^\dagger Y_d)^{cd} + 3\delta^{pb}Y_d^{cd}(Y_u Y_u^\dagger Y_u)^{ar} - \frac{1}{12}Y_d^{ad}Y_u^{cr}(Y_u^\dagger Y_u)^{pb} - \frac{1}{4}\delta^{pb}Y_d^{ad}(Y_d Y_d^\dagger Y_u)^{cr} - \frac{1}{2}Y_d^{cd}Y_u^{ar}(Y_u^\dagger Y_u)^{pb} - \frac{1}{2}\delta^{pb}Y_u^{cr}(Y_d Y_d^\dagger Y_d)^{ad} \\
& - \frac{3}{4}\delta^{pb}Y_u^{ar}(Y_u Y_u^\dagger Y_d)^{cd} - \frac{9}{8}\delta^{pb}g_L^2Y_d^{cd}Y_u^{ar} - \frac{3}{2}\delta^{pb}Y_d^{cd}(Y_d Y_d^\dagger Y_u)^{ar} - \frac{3}{2}\delta^{pb}Y_u^{cr}(Y_u Y_u^\dagger Y_d)^{ad} - \frac{16}{3}\delta^{pb}g_s^2Y_d^{ad}Y_u^{cr} \Big\} + \left\{ \frac{1}{3}Y_u^{*ab}Y_u^{*cp}(Y_d^\dagger Y_u)^{dr} \right. \\
& + \frac{1}{2}Y_u^{*ap}Y_u^{*cb}(Y_d^\dagger Y_u)^{dr} + \frac{3}{4}\delta^{rb}Y_u^{*ap}(Y_d^\dagger Y_d Y_d^\dagger)^{cd} + g_Y^2 \left( \frac{181}{216}\delta^{rb}Y_d^{*cd}Y_u^{*ap} + \frac{19}{9}\delta^{rb}Y_d^{*ad}Y_u^{*cp} \right) + \delta^{rb}Y_d^{*cd}(Y_u^\dagger Y_u Y_u^\dagger)^{ap} + \frac{3}{2}\delta^{rb}Y_d^{*ad}(Y_u^\dagger Y_u Y_u^\dagger)^{cp} \\
& - \frac{1}{6}Y_d^{*cd}Y_u^{*ap}(Y_u^\dagger Y_u)^{br} - \frac{1}{4}Y_d^{*ad}Y_u^{*cp}(Y_u^\dagger Y_u)^{br} - \frac{1}{4}\delta^{rb}Y_u^{*ap}(Y_u^\dagger Y_u Y_d^\dagger)^{cd} - \frac{3}{8}\delta^{rb}g_L^2Y_d^{*cd}Y_u^{*ap} - \frac{1}{2}\delta^{rb}Y_d^{*cd}(Y_d^\dagger Y_d Y_u^\dagger)^{ap} - \frac{3}{4}\delta^{rb}Y_d^{*ad}(Y_d^\dagger Y_d Y_u^\dagger)^{cp} \\
& - \frac{3}{2}\delta^{rb}Y_u^{*cp}(Y_d^\dagger Y_d Y_d^\dagger)^{ad} - \frac{9}{2}\delta^{rb}Y_u^{*cp}(Y_u^\dagger Y_u Y_d^\dagger)^{ad} \Big\} C_{quqd}^{(\times)abcd} + \left( C_{quqd}^{(\times)*} \right)^{abcd} \left\{ \frac{1}{3}Y_u^{ab}Y_u^{cr}(Y_u^\dagger Y_d)^{pd} + \frac{1}{2}Y_u^{ar}Y_u^{cb}(Y_u^\dagger Y_d)^{pd} + \frac{3}{4}\delta^{pb}Y_u^{ar}(Y_d Y_d^\dagger Y_d)^{cd} \right. \\
& + g_Y^2 \left( \frac{181}{216}\delta^{pb}Y_d^{cd}Y_u^{ar} + \frac{19}{9}\delta^{pb}Y_d^{ad}Y_u^{cr} \right) + \delta^{pb}Y_d^{cd}(Y_u Y_u^\dagger Y_u)^{ar} + \frac{3}{2}\delta^{pb}Y_d^{ad}(Y_u Y_u^\dagger Y_u)^{cr} - \frac{1}{6}Y_d^{cd}Y_u^{ar}(Y_u^\dagger Y_u)^{pb} - \frac{1}{4}Y_d^{ad}Y_u^{cr}(Y_u^\dagger Y_u)^{pb} - \frac{1}{4}\delta^{pb}Y_u^{ar}(Y_u Y_u^\dagger Y_d)^{cd}
\end{aligned}$$

$$\begin{aligned}
& -\frac{3}{8}\delta^{pb}g_L^2Y_d^{cd}Y_u^{ar}-\frac{1}{2}\delta^{pb}Y_d^{cd}(Y_dY_d^\dagger Y_u)^{ar}-\frac{3}{4}\delta^{pb}Y_d^{ad}(Y_dY_d^\dagger Y_u)^{cr}-\frac{3}{2}\delta^{pb}Y_u^{cr}(Y_dY_d^\dagger Y_d)^{ad}-\frac{9}{2}\delta^{pb}Y_u^{cr}(Y_uY_u^\dagger Y_d)^{ad}\Bigg\}+\Bigg\{\frac{1}{6}Y_e^{*ab}Y_u^{*cp}(Y_u^\dagger Y_u)^{dr} \\
& +\frac{3}{8}\delta^{rd}g_L^2Y_e^{*ab}Y_u^{*cp}+\frac{1}{2}\delta^{rd}Y_e^{*ab}(Y_d^\dagger Y_d Y_u^\dagger)^{cp}-\frac{3}{4}\delta^{rd}Y_u^{*cp}(Y_e^\dagger Y_e Y_e^\dagger)^{ab}-\frac{181}{216}\delta^{rd}g_Y^2Y_e^{*ab}Y_u^{*cp}-\delta^{rd}Y_e^{*ab}(Y_u^\dagger Y_u Y_u^\dagger)^{cp}\Bigg\}C_{lequ}^{abcd} \\
& +C_{lequ}^{*abcd}\Bigg\{\frac{1}{6}Y_e^{ab}Y_u^{cr}(Y_u^\dagger Y_u)^{pd}+\frac{3}{8}\delta^{pd}g_L^2Y_e^{ab}Y_u^{cr}+\frac{1}{2}\delta^{pd}Y_e^{ab}(Y_dY_d^\dagger Y_u)^{cr}-\frac{3}{4}\delta^{pd}Y_u^{cr}(Y_eY_e^\dagger Y_e)^{ab}-\frac{181}{216}\delta^{pd}g_Y^2Y_e^{ab}Y_u^{cr}-\delta^{pd}Y_e^{ab}(Y_uY_u^\dagger Y_u)^{cr}\Bigg\} \\
& +\Bigg\{\frac{1}{2}\delta^{rb}Y_e^{*ad}(Y_u^\dagger Y_u Y_u^\dagger)^{cp}+\frac{125}{54}\delta^{rb}g_Y^2Y_e^{*ad}Y_u^{*cp}-\frac{1}{12}Y_e^{*ad}Y_u^{*cp}(Y_u^\dagger Y_u)^{br}-\frac{1}{4}\delta^{rb}Y_e^{*ad}(Y_d^\dagger Y_d Y_u^\dagger)^{cp}-\frac{1}{2}\delta^{rb}Y_u^{*cp}(Y_e^\dagger Y_e Y_e^\dagger)^{ad}\Bigg\}C_{luqe}^{abcd} \\
& +C_{luqe}^{*abcd}\Bigg\{\frac{1}{2}\delta^{pb}Y_e^{ad}(Y_uY_u^\dagger Y_u)^{cr}+\frac{125}{54}\delta^{pb}g_Y^2Y_e^{ad}Y_u^{cr}-\frac{1}{12}Y_e^{ad}Y_u^{cr}(Y_u^\dagger Y_u)^{pb}-\frac{1}{4}\delta^{pb}Y_e^{ad}(Y_dY_d^\dagger Y_u)^{cr}-\frac{1}{2}\delta^{pb}Y_u^{cr}(Y_eY_e^\dagger Y_e)^{ad}\Bigg\}+\Bigg\{\frac{16}{27}\delta^{pr}\delta^{ad}\delta^{bc}g_Y^4 \\
& +\frac{16}{9}\delta^{pr}\delta^{bc}g_Y^2(Y_eY_e^\dagger)^{da}\Bigg\}C_{\ell\ell}^{abcd}+\Bigg\{\frac{16}{81}\delta^{pr}\delta^{ad}\delta^{bc}g_Y^4+g_Y^2\Big(\frac{16}{9}\delta^{pr}\delta^{bc}(Y_uY_u^\dagger)^{da}-\frac{49}{81}\delta^{bc}Y_u^{*ap}Y_u^{dr}-\frac{26}{27}\delta^{cd}Y_u^{*ap}Y_u^{br}-\frac{16}{9}\delta^{pr}\delta^{bc}(Y_dY_d^\dagger)^{da}\Big) \\
& +6Y_u^{*cp}Y_u^{br}(Y_dY_d^\dagger)^{da}+6Y_u^{*ap}Y_u^{br}(Y_uY_u^\dagger)^{dc}-\frac{1}{3}\delta^{bc}g_L^2Y_u^{*ap}Y_u^{dr}-\frac{64}{27}\delta^{bc}g_s^2Y_u^{*ap}Y_u^{dr}-6Y_u^{*cp}Y_u^{dr}(Y_dY_d^\dagger)^{ba}\Bigg\}C_{qq}^{(\parallel)abcd}+\Bigg\{\frac{32}{81}\delta^{pr}\delta^{ad}\delta^{bc}g_Y^4 \\
& +g_Y^2\Big(\frac{32}{9}\delta^{pr}\delta^{bc}(Y_uY_u^\dagger)^{da}-\frac{13}{27}\delta^{cd}Y_u^{*ap}Y_u^{br}-\frac{98}{81}\delta^{bc}Y_u^{*ap}Y_u^{dr}-\frac{32}{9}\delta^{pr}\delta^{bc}(Y_dY_d^\dagger)^{da}\Big)+6Y_u^{*cp}Y_u^{dr}(Y_dY_d^\dagger)^{ba}+6Y_u^{*cp}Y_u^{br}(Y_dY_d^\dagger)^{da}+12Y_u^{*ap}Y_u^{br}(Y_uY_u^\dagger)^{dc} \\
& -\delta^{cd}g_L^2Y_u^{*ap}Y_u^{br}-\frac{128}{27}\delta^{bc}g_s^2Y_u^{*ap}Y_u^{dr}-6Y_u^{*ap}Y_u^{dr}(Y_uY_u^\dagger)^{bc}\Bigg\}C_{qq}^{(\times)abcd}+\Bigg\{\frac{13}{27}\delta^{ab}g_Y^2Y_u^{*cp}Y_u^{dr}-Y_u^{*cp}Y_u^{dr}(Y_eY_e^\dagger)^{ba}\Bigg\}C_{\ell q}^{(\parallel)abcd}+\Bigg\{\frac{13}{54}\delta^{ab}g_Y^2Y_u^{*cp}Y_u^{dr} \\
& +Y_u^{*cp}Y_u^{dr}(Y_eY_e^\dagger)^{ba}-\frac{1}{6}\delta^{ab}g_L^2Y_u^{*cp}Y_u^{dr}\Bigg\}C_{\ell q}^{(\times)abcd}, \tag{9.12}
\end{aligned}$$

## 9.7 $C_{Hd}$

$$\begin{aligned}
\beta_{C_{Hd}}^{(1)} & =\Bigg\{\frac{1}{2}(Y_d^\dagger Y_d)^{pr}-\frac{1}{18}\delta^{pr}g_Y^2\Bigg\}C_{HD}^{(\parallel)}+\Bigg\{(Y_d^\dagger Y_d)^{pr}-\frac{1}{9}\delta^{pr}g_Y^2\Bigg\}C_{HD}^{(\times)}+\frac{4}{9}\delta^{pr}\delta^{ab}g_Y^2C_{H\ell}^{(\parallel)ab}+\frac{2}{9}\delta^{pr}\delta^{ab}g_Y^2C_{H\ell}^{(\times)ab}+\frac{4}{9}\delta^{pr}\delta^{ab}g_Y^2C_{He}^{ab}-\Bigg\{\frac{4}{9}\delta^{pr}\delta^{ab}g_Y^2 \\
& +2Y_d^{*ap}Y_d^{br}\Bigg\}C_{Hq}^{(\parallel)ab}-\Bigg\{\frac{2}{9}\delta^{pr}\delta^{ab}g_Y^2+Y_d^{*ap}Y_d^{br}\Bigg\}C_{Hq}^{(\times)ab}-\frac{8}{9}\delta^{pr}\delta^{ab}g_Y^2C_{Hu}^{ab}+\Bigg\{\frac{1}{9}g_Y^2\Big(3\delta^{pa}\delta^{rb}+4\delta^{pr}\delta^{ab}\Big)+2\Big(T_2\delta^{pa}\delta^{rb}+2\delta^{rb}(Y_d^\dagger Y_d)^{pa} \\
& +2\delta^{pa}(Y_d^\dagger Y_d)^{br}\Big)\Bigg\}C_{Hd}^{ab}-\delta^{rb}C_{Hud}^{ab}(Y_d^\dagger Y_u)^{pa}-\delta^{pb}C_{Hud}^{*ab}(Y_u^\dagger Y_d)^{ar}-\Bigg\{\frac{2}{3}\delta^{pc}\delta^{rd}\delta^{ab}g_Y^2+2\delta^{pc}\delta^{rd}(Y_eY_e^\dagger)^{ba}\Bigg\}C_{\ell d}^{abcd}+\Bigg\{\frac{2}{3}\delta^{pc}\delta^{rd}\delta^{ab}g_Y^2
\end{aligned}$$



$$\begin{aligned}
& -6\left(\delta^{pc}\delta^{rd}(Y_d Y_d^\dagger)^{ba} - \delta^{pc}\delta^{rd}(Y_u Y_u^\dagger)^{ba}\right)\left\{C_{qd}^{(\parallel)abcd} + \left\{\frac{2}{9}\delta^{pc}\delta^{rd}\delta^{ab}g_Y^2 - 2\left(\delta^{pc}\delta^{rd}(Y_d Y_d^\dagger)^{ba} - \delta^{pc}\delta^{rd}(Y_u Y_u^\dagger)^{ba}\right)\right\}C_{qd}^{(\times)abcd} + \left\{4\left(\delta^{pa}\delta^{rd}(Y_d^\dagger Y_d)^{bc}\right.\right.\right. \\
& + 3\delta^{pa}\delta^{rb}(Y_d^\dagger Y_d)^{dc}) - \frac{4}{9}g_Y^2(\delta^{pa}\delta^{rd}\delta^{bc} + 3\delta^{pa}\delta^{rb}\delta^{cd})\left.\left.\right\}C_{dd}^{abcd} + \left\{2\delta^{pc}\delta^{rd}(Y_e^\dagger Y_e)^{ba} - \frac{2}{3}\delta^{pc}\delta^{rd}\delta^{ab}g_Y^2\right\}C_{ed}^{abcd} + \left\{\frac{4}{3}\delta^{pc}\delta^{rd}\delta^{ab}g_Y^2\right. \\
& \left.\left.- 6\delta^{pc}\delta^{rd}(Y_u^\dagger Y_u)^{ba}\right\}C_{ud}^{(\parallel)abcd} + \left\{\frac{4}{9}\delta^{pc}\delta^{rd}\delta^{ab}g_Y^2 - 2\delta^{pc}\delta^{rd}(Y_u^\dagger Y_u)^{ba}\right\}C_{ud}^{(\times)abcd}, \tag{9.13}
\end{aligned}$$

$$\begin{aligned}
\beta_{C_{Hd}^{pr}}^{(2)} = & \frac{19}{9}\delta^{pr}g_Y^2\mathbf{T}_{\ell H} - 3(Y_d^\dagger Y_d)^{pr}\mathbf{T}_{\ell H} + \left\{g_Y^2\left(\frac{1}{18}\mathbf{T}_2\delta^{pr} + \frac{485}{144}(Y_d^\dagger Y_d)^{pr}\right) + 2(Y_d^\dagger Y_u Y_u^\dagger Y_d)^{pr} + \frac{137}{48}g_L^2(Y_d^\dagger Y_d)^{pr} - \frac{7}{108}\delta^{pr}g_Y^2g_L^2 - \frac{5}{18}\delta^{pr}\lambda g_Y^2\right. \\
& - \frac{40}{81}\delta^{pr}g_Y^4 - \frac{1}{2}\mathbf{T}_2(Y_d^\dagger Y_d)^{pr} - \frac{8}{3}g_s^2(Y_d^\dagger Y_d)^{pr} - 4(Y_d^\dagger Y_d Y_d^\dagger Y_d)^{pr}\left.\right\}C_{HD}^{(\parallel)} + \left\{g_Y^2\left(\frac{1}{9}\mathbf{T}_2\delta^{pr} + \frac{47}{18}(Y_d^\dagger Y_d)^{pr}\right) + 9g_L^2(Y_d^\dagger Y_d)^{pr} - \frac{5}{18}\delta^{pr}\lambda g_Y^2\right. \\
& - \frac{181}{648}\delta^{pr}g_Y^4 - \mathbf{T}_2(Y_d^\dagger Y_d)^{pr} - \frac{41}{24}\delta^{pr}g_Y^2g_L^2 - 2(Y_d^\dagger Y_u Y_u^\dagger Y_d)^{pr} - 5(Y_d^\dagger Y_d Y_d^\dagger Y_d)^{pr} - \frac{16}{3}g_s^2(Y_d^\dagger Y_d)^{pr}\left.\right\}C_{HD}^{(\times)} + \left\{\frac{13}{9}g_Y^4(Y_d^\dagger Y_d)^{pr} + 4\delta^{pr}\lambda g_Y^4\right. \\
& - \delta^{pr}g_Y^4g_L^2 - \frac{13}{9}\delta^{pr}g_Y^6\left.\right\}C_{HB} - \frac{2}{3}\delta^{pr}g_Y^2g_L^4C_{HW} - \left\{\frac{16}{3}\delta^{pr}g_Y^2g_s^4 + \frac{80}{3}g_s^4(Y_d^\dagger Y_d)^{pr}\right\}C_{HG} + \left\{\delta^{pr}\lambda g_Y^2g_L^2 + \frac{7}{4}g_Y^2g_L^2(Y_d^\dagger Y_d)^{pr} + \frac{9}{4}\delta^{pr}g_Y^2g_L^4\right. \\
& - \frac{11}{12}\delta^{pr}g_Y^4g_L^2\left.\right\}C_{HWB} + \left\{3g_L^6(Y_d^\dagger Y_d)^{pr} - \frac{4}{3}\delta^{pr}g_Y^2g_L^6\right\}C_W + \left\{8g_s^6(Y_d^\dagger Y_d)^{pr} - \frac{80}{9}\delta^{pr}g_Y^2g_s^6\right\}C_G + \left\{\frac{3}{4}\delta^{rb}g_Y^2Y_d^{*ap} + \frac{9}{4}\delta^{rb}g_L^2Y_d^{*ap} - \frac{3}{2}\delta^{rb}\lambda Y_d^{*ap}\right. \\
& - \frac{3}{2}\delta^{rb}(Y_d^\dagger Y_d Y_d^\dagger)^{ap}\left.\right\}C_{dH}^{ab} + C_{dH}^{*ab}\left\{\frac{3}{4}\delta^{pb}g_Y^2Y_d^{ar} + \frac{9}{4}\delta^{pb}g_L^2Y_d^{ar} - \frac{3}{2}\delta^{pb}\lambda Y_d^{ar} - \frac{3}{2}\delta^{pb}(Y_d Y_d^\dagger Y_d)^{ar}\right\} + \left\{\frac{1}{2}\delta^{pr}g_Y^4Y_e^{*ab} + \delta^{pr}g_Y^2g_L^2Y_e^{*ab}\right. \\
& - \frac{1}{3}\delta^{pr}g_Y^2(Y_e^\dagger Y_e Y_e^\dagger)^{ab}\left.\right\}C_{eB}^{ab} + C_{eB}^{*ab}\left\{\frac{1}{2}\delta^{pr}g_Y^4Y_e^{ab} + \delta^{pr}g_Y^2g_L^2Y_e^{ab} - \frac{1}{3}\delta^{pr}g_Y^2(Y_e Y_e^\dagger Y_e)^{ab}\right\} - \frac{5}{12}\delta^{pr}g_Y^2g_L^2Y_e^{*ab}C_{eW}^{ab} - \frac{5}{12}\delta^{pr}g_Y^2g_L^2C_{eW}^{*ab}Y_e^{ab} \\
& + \left\{g_Y^2\left(\delta^{pr}(Y_d^\dagger Y_d Y_u^\dagger)^{ab} + \delta^{pr}(Y_u^\dagger Y_u Y_u^\dagger)^{ab} + \frac{7}{3}Y_d^{*ap}(Y_u^\dagger Y_d)^{br}\right) + \frac{35}{6}\delta^{pr}g_Y^4Y_u^{*ab} - 3\delta^{pr}g_Y^2g_L^2Y_u^{*ab}\right\}C_{uB}^{ab} + C_{uB}^{*ab}\left\{g_Y^2\left(\delta^{pr}(Y_d Y_d^\dagger Y_u)^{ab}\right.\right. \\
& + \delta^{pr}(Y_u Y_u^\dagger Y_u)^{ab} + \frac{7}{3}Y_d^{ar}(Y_d^\dagger Y_u)^{pb}) + \frac{35}{6}\delta^{pr}g_Y^4Y_u^{ab} - 3\delta^{pr}g_Y^2g_L^2Y_u^{ab}\left.\right\} - \frac{1}{4}\delta^{pr}g_Y^2g_L^2Y_u^{*ab}C_{uW}^{ab} - \frac{1}{4}\delta^{pr}g_Y^2g_L^2C_{uW}^{*ab}Y_u^{ab} + \left\{\frac{32}{9}\delta^{pr}g_Y^2g_s^2Y_u^{*ab}\right. \\
& + 16\delta^{pr}g_s^4Y_u^{*ab} - \frac{40}{3}g_s^2Y_d^{*ap}(Y_u^\dagger Y_d)^{br}\left.\right\}C_{uG}^{ab} + C_{uG}^{*ab}\left\{\frac{32}{9}\delta^{pr}g_Y^2g_s^2Y_u^{ab} + 16\delta^{pr}g_s^4Y_u^{ab} - \frac{40}{3}g_s^2Y_d^{ar}(Y_d^\dagger Y_u)^{pb}\right\} + \left\{g_Y^2g_L^2\left(\frac{7}{8}\delta^{rb}Y_d^{*ap}\right.\right. \\
& + 3\delta^{pr}Y_d^{*ab}) + g_Y^4\left(\frac{1}{6}\delta^{pr}Y_d^{*ab} + \frac{2665}{216}\delta^{rb}Y_d^{*ap}\right) + g_Y^2\left(\frac{2}{3}\delta^{rb}(Y_d^\dagger Y_d Y_d^\dagger)^{ap} - \frac{5}{6}\delta^{rb}(Y_u^\dagger Y_u Y_d^\dagger)^{ap} - \delta^{pr}(Y_d^\dagger Y_d Y_d^\dagger)^{ab} - \delta^{pr}(Y_u^\dagger Y_u Y_d^\dagger)^{ab} - \frac{3}{2}\mathbf{T}_2\delta^{rb}Y_d^{*ap}\right.
\end{aligned}$$

$$\begin{aligned}
& -4Y_d^{*ap}(Y_d^\dagger Y_d)^{br}) - \frac{32}{9}\delta^{rb}g_Y^2g_s^2Y_d^{*ap} - 9\delta^{rb}\lambda g_Y^2Y_d^{*ap}\Big\}C_{dB}^{ab} + C_{dB}^{*ab}\Big\{g_Y^2g_L^2\Big(\frac{7}{8}\delta^{pb}Y_d^{ar} + 3\delta^{pr}Y_d^{ab}\Big) + g_Y^4\Big(\frac{1}{6}\delta^{pr}Y_d^{ab} + \frac{2665}{216}\delta^{pb}Y_d^{ar}\Big) \\
& + g_Y^2\Big(\frac{2}{3}\delta^{pb}(Y_dY_d^\dagger Y_d)^{ar} - \frac{5}{6}\delta^{pb}(Y_uY_u^\dagger Y_d)^{ar} - \delta^{pr}(Y_dY_d^\dagger Y_d)^{ab} - \delta^{pr}(Y_uY_u^\dagger Y_d)^{ab} - \frac{3}{2}T_2\delta^{pb}Y_d^{ar} - 4Y_d^{ar}(Y_d^\dagger Y_d)^{pb}\Big) - \frac{32}{9}\delta^{pb}g_Y^2g_s^2Y_d^{ar} \\
& - 9\delta^{pb}\lambda g_Y^2Y_d^{ar}\Big\} + \Big\{g_Y^2g_L^2\Big(\frac{3}{4}\delta^{pr}Y_d^{*ab} + \frac{149}{48}\delta^{rb}Y_d^{*ap}\Big) + g_L^2\Big(\frac{9}{2}\delta^{rb}(Y_d^\dagger Y_dY_d^\dagger)^{ap} - \frac{9}{4}T_2\delta^{rb}Y_d^{*ap} - \frac{21}{4}\delta^{rb}(Y_u^\dagger Y_uY_d^\dagger)^{ap}\Big) - \frac{69}{16}\delta^{rb}g_L^4Y_d^{*ap} \\
& - \frac{9}{2}\delta^{rb}\lambda g_L^2Y_d^{*ap} - 8\delta^{rb}g_s^2g_L^2Y_d^{*ap}\Big\}C_{dW}^{ab} + C_{dW}^{*ab}\Big\{g_Y^2g_L^2\Big(\frac{3}{4}\delta^{pr}Y_d^{ab} + \frac{149}{48}\delta^{pb}Y_d^{ar}\Big) + g_L^2\Big(\frac{9}{2}\delta^{pb}(Y_dY_d^\dagger Y_d)^{ar} - \frac{9}{4}T_2\delta^{pb}Y_d^{ar} - \frac{21}{4}\delta^{pb}(Y_uY_u^\dagger Y_d)^{ar}\Big) \\
& - \frac{69}{16}\delta^{pb}g_L^4Y_d^{ar} - \frac{9}{2}\delta^{pb}\lambda g_L^2Y_d^{ar} - 8\delta^{pb}g_s^2g_L^2Y_d^{ar}\Big\} + \Big\{g_Y^2g_s^2\Big(\frac{22}{27}\delta^{rb}Y_d^{*ap} + \frac{32}{9}\delta^{pr}Y_d^{*ab}\Big) + g_s^4\Big(\frac{320}{9}\delta^{rb}Y_d^{*ap} - 16\delta^{pr}Y_d^{*ab}\Big) \\
& + g_s^2\Big(\frac{4}{3}\delta^{rb}(Y_d^\dagger Y_dY_d^\dagger)^{ap} + 12Y_d^{*ap}(Y_d^\dagger Y_d)^{br} - \frac{8}{3}\delta^{rb}(Y_u^\dagger Y_uY_d^\dagger)^{ap}\Big) + 10\delta^{rb}g_s^2g_L^2Y_d^{*ap}\Big\}C_{dG}^{ab} + C_{dG}^{*ab}\Big\{g_Y^2g_s^2\Big(\frac{22}{27}\delta^{pb}Y_d^{ar} + \frac{32}{9}\delta^{pr}Y_d^{ab}\Big) \\
& + g_s^4\Big(\frac{320}{9}\delta^{pb}Y_d^{ar} - 16\delta^{pr}Y_d^{ab}\Big) + g_s^2\Big(\frac{4}{3}\delta^{pb}(Y_dY_d^\dagger Y_d)^{ar} + 12Y_d^{ar}(Y_d^\dagger Y_d)^{pb} - \frac{8}{3}\delta^{pb}(Y_uY_u^\dagger Y_d)^{ar}\Big) + 10\delta^{pb}g_s^2g_L^2Y_d^{ar}\Big\} + \Big\{\delta^{pr}\delta^{ab}g_Y^2g_L^2 \\
& - \frac{1}{2}(Y_d^\dagger Y_d)^{pr}(Y_eY_e^\dagger)^{ba} - \frac{83}{162}\delta^{pr}\delta^{ab}g_Y^4 - g_Y^2\Big(\frac{49}{54}\delta^{pr}(Y_eY_e^\dagger)^{ba} + \frac{19}{18}\delta^{ab}(Y_d^\dagger Y_d)^{pr}\Big)\Big\}C_{H\ell}^{(\parallel)ab} + \Big\{\frac{1}{2}(Y_d^\dagger Y_d)^{pr}(Y_eY_e^\dagger)^{ba} + \frac{83}{108}\delta^{pr}\delta^{ab}g_Y^2g_L^2 \\
& - \frac{1}{12}\delta^{ab}g_L^2(Y_d^\dagger Y_d)^{pr} - \frac{83}{324}\delta^{pr}\delta^{ab}g_Y^4 - g_Y^2\Big(\frac{13}{27}\delta^{pr}(Y_eY_e^\dagger)^{ba} + \frac{19}{36}\delta^{ab}(Y_d^\dagger Y_d)^{pr}\Big)\Big\}C_{H\ell}^{(\times)ab} + \Big\{\frac{1}{2}(Y_d^\dagger Y_d)^{pr}(Y_e^\dagger Y_e)^{ba} + \frac{403}{162}\delta^{pr}\delta^{ab}g_Y^4 \\
& - g_Y^2\Big(\frac{19}{18}\delta^{ab}(Y_d^\dagger Y_d)^{pr} + \frac{77}{54}\delta^{pr}(Y_e^\dagger Y_e)^{ba}\Big)\Big\}C_{He}^{ab} + \Big\{g_Y^2\Big(\frac{7}{18}\delta^{pr}(Y_dY_d^\dagger)^{ba} + \frac{19}{18}\delta^{ab}(Y_d^\dagger Y_d)^{pr} + \frac{7}{6}\delta^{pr}(Y_uY_u^\dagger)^{ba} - \frac{179}{54}Y_d^{*ap}Y_d^{br}\Big) + \frac{3}{2}(Y_d^\dagger Y_d)^{pr}(Y_uY_u^\dagger)^{ba} \\
& + 3T_2Y_d^{*ap}Y_d^{br} + \frac{43}{12}Y_d^{br}(Y_u^\dagger Y_uY_d^\dagger)^{ap} + \frac{43}{12}Y_d^{*ap}(Y_uY_u^\dagger Y_d)^{br} + \frac{47}{12}Y_d^{br}(Y_d^\dagger Y_dY_d^\dagger)^{ap} + \frac{47}{12}Y_d^{*ap}(Y_dY_d^\dagger Y_d)^{br} + \frac{16}{3}g_s^2Y_d^{*ap}Y_d^{br} - \frac{13}{162}\delta^{pr}\delta^{ab}g_Y^4 \\
& - \delta^{pr}\delta^{ab}g_Y^2g_L^2 - \frac{3}{2}(Y_d^\dagger Y_d)^{pr}(Y_dY_d^\dagger)^{ba} - \frac{16}{9}\delta^{pr}\delta^{ab}g_Y^2g_s^2 - 12g_L^2Y_d^{*ap}Y_d^{br} - 16\delta^{pr}\delta^{ab}g_s^4\Big\}C_{Hq}^{(\parallel)ab} + \Big\{\frac{11}{36}\delta^{pr}\delta^{ab}g_Y^2g_L^2 + g_Y^2\Big(\frac{19}{36}\delta^{ab}(Y_d^\dagger Y_d)^{pr} \\
& + \frac{7}{9}\delta^{pr}(Y_dY_d^\dagger)^{ba} + \frac{5}{6}\delta^{pr}(Y_uY_u^\dagger)^{ba} - \frac{205}{216}Y_d^{*ap}Y_d^{br}\Big) + \frac{3}{2}T_2Y_d^{*ap}Y_d^{br} + \frac{3}{2}(Y_d^\dagger Y_d)^{pr}(Y_dY_d^\dagger)^{ba} + 3(Y_d^\dagger Y_d)^{pr}(Y_uY_u^\dagger)^{ba} + \frac{29}{6}Y_d^{br}(Y_d^\dagger Y_dY_d^\dagger)^{ap} \\
& + \frac{29}{6}Y_d^{*ap}(Y_dY_d^\dagger Y_d)^{br} - \frac{13}{324}\delta^{pr}\delta^{ab}g_Y^4 - \frac{8}{9}\delta^{pr}\delta^{ab}g_Y^2g_s^2 - g_L^2\Big(\frac{1}{4}\delta^{ab}(Y_d^\dagger Y_d)^{pr} + \frac{151}{24}Y_d^{*ap}Y_d^{br}\Big) - \frac{17}{6}Y_d^{br}(Y_u^\dagger Y_uY_d^\dagger)^{ap} - \frac{17}{6}Y_d^{*ap}(Y_uY_u^\dagger Y_d)^{br} \\
& - \frac{16}{3}g_s^2Y_d^{*ap}Y_d^{br} - 8\delta^{pr}\delta^{ab}g_s^4\Big\}C_{Hq}^{(\times)ab} + \Big\{\frac{77}{81}\delta^{pr}\delta^{ab}g_Y^4 + g_Y^2\Big(\frac{19}{9}\delta^{ab}(Y_d^\dagger Y_d)^{pr} + \frac{49}{18}\delta^{pr}(Y_u^\dagger Y_u)^{ba}\Big) + 8\delta^{pr}\delta^{ab}g_s^4 - \frac{3}{2}(Y_d^\dagger Y_d)^{pr}(Y_u^\dagger Y_u)^{ba}
\end{aligned}$$

$$\begin{aligned}
& -2(Y_d^\dagger Y_u)^{pa}(Y_u^\dagger Y_d)^{br} - \frac{32}{9}\delta^{pr}\delta^{ab}g_Y^2g_s^2 \Big\} C_{Hu}^{ab} + \left\{ g_Y^4 \left( \frac{67}{162}\delta^{pr}\delta^{ab} - \frac{127}{243}\delta^{pa}\delta^{rb} \right) + g_L^2 \left( \frac{93}{8}\delta^{rb}(Y_d^\dagger Y_d)^{pa} + \frac{93}{8}\delta^{pa}(Y_d^\dagger Y_d)^{br} - \frac{3}{4}T_2\delta^{pa}\delta^{rb} \right) \right. \\
& + g_Y^2 \left( \frac{19}{12}\delta^{pa}\delta^{rb} \text{Tr}[Y_u^\dagger Y_u] + \frac{53}{12}\delta^{pa}\delta^{rb} \text{Tr}[Y_e^\dagger Y_e] + \frac{1219}{216}\delta^{rb}(Y_d^\dagger Y_d)^{pa} + \frac{1219}{216}\delta^{pa}(Y_d^\dagger Y_d)^{br} - \frac{19}{18}\delta^{ab}(Y_d^\dagger Y_d)^{pr} - \frac{7}{6}\delta^{pr}(Y_d^\dagger Y_d)^{ba} \right. \\
& - \frac{41}{12}\delta^{pa}\delta^{rb} \text{Tr}[Y_d^\dagger Y_d] \Big) + g_s^2 \left( \frac{4}{3}\delta^{rb}(Y_d^\dagger Y_d)^{pa} + \frac{4}{3}\delta^{pa}(Y_d^\dagger Y_d)^{br} + 40\delta^{pa}\delta^{rb} \text{Tr}[Y_d^\dagger Y_d] + 40\delta^{pa}\delta^{rb} \text{Tr}[Y_u^\dagger Y_u] \right) + \frac{3}{2}(Y_d^\dagger Y_d)^{pr}(Y_d^\dagger Y_d)^{ba} + \frac{16}{9}\delta^{pr}\delta^{ab}g_Y^2g_s^2 \\
& + 3\delta^{pa}\delta^{rb}g_Y^2g_L^2 + 3\delta^{rb}(Y_d^\dagger Y_u Y_u^\dagger Y_d)^{pa} + 3\delta^{pa}(Y_d^\dagger Y_u Y_u^\dagger Y_d)^{br} + 6\delta^{pa}\delta^{rb} \text{Tr}[Y_d^\dagger Y_d Y_u^\dagger Y_u] + 8\delta^{pr}\delta^{ab}g_s^4 - \lambda \left( 9\delta^{rb}(Y_d^\dagger Y_d)^{pa} + 9\delta^{pa}(Y_d^\dagger Y_d)^{br} \right) \\
& - \frac{9}{2}(Y_d^\dagger Y_d)^{pa}(Y_d^\dagger Y_d)^{br} - 5T_2\delta^{rb}(Y_d^\dagger Y_d)^{pa} - 5T_2\delta^{pa}(Y_d^\dagger Y_d)^{br} - 6T_4\delta^{pa}\delta^{rb} - \frac{31}{4}\delta^{rb}(Y_d^\dagger Y_d Y_d^\dagger Y_d)^{pa} - \frac{31}{4}\delta^{pa}(Y_d^\dagger Y_d Y_d^\dagger Y_d)^{br} \Big\} C_{Hd}^{ab} \\
& + \left\{ \frac{1}{2}T_2\delta^{rb}(Y_d^\dagger Y_u)^{pa} + \frac{3}{2}(Y_d^\dagger Y_d)^{pr}(Y_d^\dagger Y_u)^{ba} + \frac{21}{4}\delta^{rb}(Y_d^\dagger Y_u Y_u^\dagger Y_u)^{pa} - \frac{1}{4}(Y_d^\dagger Y_d)^{br}(Y_d^\dagger Y_u)^{pa} - \frac{1}{2}\delta^{rb}(Y_d^\dagger Y_d Y_d^\dagger Y_u)^{pa} - g_Y^2 \left( \frac{17}{18}\delta^{pr}(Y_d^\dagger Y_u)^{ba} \right. \right. \\
& + \frac{71}{27}\delta^{rb}(Y_d^\dagger Y_u)^{pa} \Big) - 4\delta^{rb}g_s^2(Y_d^\dagger Y_u)^{pa} \Big\} C_{Hud}^{ab} + C_{Hud}^{*ab} \left\{ \frac{1}{2}T_2\delta^{pb}(Y_u^\dagger Y_d)^{ar} + \frac{3}{2}(Y_d^\dagger Y_d)^{pr}(Y_u^\dagger Y_d)^{ab} + \frac{21}{4}\delta^{pb}(Y_u^\dagger Y_u Y_u^\dagger Y_d)^{ar} - \frac{1}{4}(Y_d^\dagger Y_d)^{pb}(Y_u^\dagger Y_d)^{ar} \right. \\
& - \frac{1}{2}\delta^{pb}(Y_u^\dagger Y_d Y_d^\dagger Y_d)^{ar} - g_Y^2 \left( \frac{17}{18}\delta^{pr}(Y_u^\dagger Y_d)^{ab} + \frac{71}{27}\delta^{pb}(Y_u^\dagger Y_d)^{ar} \right) - 4\delta^{pb}g_s^2(Y_u^\dagger Y_d)^{ar} \Big\} + \left\{ \frac{3}{4}\delta^{pc}\delta^{rd}g_L^2(Y_e Y_e^\dagger)^{ba} + \delta^{rd}(Y_d^\dagger Y_d)^{pc}(Y_e Y_e^\dagger)^{ba} \right. \\
& + \delta^{pc}(Y_d^\dagger Y_d)^{dr}(Y_e Y_e^\dagger)^{ba} + g_Y^2 \left( \frac{4}{27}\delta^{rd}\delta^{ab}(Y_d^\dagger Y_d)^{pc} + \frac{4}{27}\delta^{pc}\delta^{ab}(Y_d^\dagger Y_d)^{dr} - \frac{61}{12}\delta^{pc}\delta^{rd}(Y_e Y_e^\dagger)^{ba} \right) + \frac{487}{486}\delta^{pc}\delta^{rd}\delta^{ab}g_Y^4 + 6\delta^{pc}\delta^{rd}(Y_e Y_e^\dagger Y_e Y_e^\dagger)^{ba} \\
& - \frac{3}{2}\delta^{pc}\delta^{rd}\delta^{ab}g_Y^2g_L^2 \Big\} C_{ld}^{abcd} + \left\{ \frac{5}{27}\delta^{cd}g_Y^2Y_d^{*ap}Y_d^{br} + Y_d^{*ap}Y_d^{br}(Y_e^\dagger Y_e)^{dc} \right\} C_{qe}^{abcd} + \left\{ \frac{2}{3}Y_u^{*ad}Y_d^{br}(Y_d^\dagger Y_u)^{pc} + \frac{2}{3}Y_d^{*ap}Y_u^{bc}(Y_u^\dagger Y_d)^{dr} - \frac{10}{27}\delta^{cd}g_Y^2Y_d^{*ap}Y_d^{br} \right. \\
& - 3Y_d^{*ap}Y_d^{br}(Y_u^\dagger Y_u)^{dc} \Big\} C_{qu}^{(ll)abcd} + \left\{ \frac{32}{27}\delta^{cd}g_s^2Y_d^{*ap}Y_d^{br} + 2Y_u^{*ad}Y_d^{br}(Y_d^\dagger Y_u)^{pc} + 2Y_d^{*ap}Y_u^{bc}(Y_u^\dagger Y_d)^{dr} - \frac{10}{81}\delta^{cd}g_Y^2Y_d^{*ap}Y_d^{br} - Y_d^{*ap}Y_d^{br}(Y_u^\dagger Y_u)^{dc} \right\} C_{qu}^{(\times)abcd} \\
& + \left\{ \frac{89}{486}\delta^{pc}\delta^{rd}\delta^{ab}g_Y^4 + g_Y^2 \left( \frac{5}{27}\delta^{cd}Y_d^{*ap}Y_d^{br} + \frac{41}{108}\delta^{pc}Y_d^{*ad}Y_d^{br} + \frac{41}{108}\delta^{rd}Y_d^{*ap}Y_d^{bc} - \frac{4}{27}\delta^{rd}\delta^{ab}(Y_d^\dagger Y_d)^{pc} - \frac{4}{27}\delta^{pc}\delta^{ab}(Y_d^\dagger Y_d)^{dr} - \frac{47}{12}\delta^{pc}\delta^{rd}(Y_d Y_d^\dagger)^{ba} \right. \right. \\
& - \frac{61}{12}\delta^{pc}\delta^{rd}(Y_u Y_u^\dagger)^{ba} \Big) + g_L^2 \left( \frac{9}{4}\delta^{pc}\delta^{rd}(Y_d Y_d^\dagger)^{ba} - \frac{3}{4}\delta^{pc}Y_d^{*ad}Y_d^{br} - \frac{3}{4}\delta^{rd}Y_d^{*ap}Y_d^{bc} - \frac{9}{4}\delta^{pc}\delta^{rd}(Y_u Y_u^\dagger)^{ba} \right) + g_s^2 \left( 40\delta^{pc}\delta^{rd}(Y_u Y_u^\dagger)^{ba} - 40\delta^{pc}\delta^{rd}(Y_d Y_d^\dagger)^{ba} \right) \\
& + \delta^{rd}Y_d^{bc}(Y_d^\dagger Y_d Y_d^\dagger)^{ap} + \delta^{pc}Y_d^{*ad}(Y_d Y_d^\dagger Y_d)^{br} + \frac{3}{2}\delta^{pc}\delta^{rd}\delta^{ab}g_Y^2g_L^2 + \frac{5}{2}\delta^{pc}Y_d^{br}(Y_d^\dagger Y_d Y_d^\dagger)^{ad} + \frac{5}{2}\delta^{rd}Y_d^{*ap}(Y_d Y_d^\dagger Y_d)^{bc} + \frac{8}{3}\delta^{pc}\delta^{rd}\delta^{ab}g_Y^2g_s^2 \\
& + 3Y_d^{*ap}Y_d^{br}(Y_d^\dagger Y_d)^{dc} + 3\delta^{rd}(Y_d^\dagger Y_d)^{pc}(Y_d Y_d^\dagger)^{ba} + 3\delta^{pc}(Y_d^\dagger Y_d)^{dr}(Y_d Y_d^\dagger)^{ba} + 18\delta^{pc}\delta^{rd}(Y_d Y_d^\dagger Y_d Y_d^\dagger)^{ba} - \frac{1}{3}Y_d^{*ad}Y_d^{br}(Y_d^\dagger Y_d)^{pc} - \frac{1}{3}Y_d^{*ap}Y_d^{bc}(Y_d^\dagger Y_d)^{dr} \\
& - \frac{3}{2}\delta^{pc}Y_d^{br}(Y_u^\dagger Y_u Y_d^\dagger)^{ad} - \frac{3}{2}\delta^{rd}Y_d^{*ap}(Y_u Y_u^\dagger Y_d)^{bc} - 3\delta^{rd}(Y_d^\dagger Y_d)^{pc}(Y_u Y_u^\dagger)^{ba} - 3\delta^{pc}(Y_d^\dagger Y_d)^{dr}(Y_u Y_u^\dagger)^{ba} - 18\delta^{pc}\delta^{rd}(Y_u Y_u^\dagger Y_u Y_u^\dagger)^{ba} \Big\} C_{qd}^{(ll)abcd}
\end{aligned}$$

$$\begin{aligned}
& + \left\{ \frac{89}{1458} \delta^{pc} \delta^{rd} \delta^{ab} g_Y^4 + \frac{1}{2} \delta^{pc} \delta^{rd} \delta^{ab} g_Y^2 g_L^2 + g_Y^2 g_s^2 \left( \frac{4}{27} \delta^{pr} \delta^{ab} \delta^{cd} - \frac{140}{243} \delta^{pc} \delta^{rd} \delta^{ab} \right) + \delta^{rd} (Y_d^\dagger Y_d)^{pc} (Y_d Y_d^\dagger)^{ba} + \delta^{pc} (Y_d^\dagger Y_d)^{dr} (Y_d Y_d^\dagger)^{ba} \right. \\
& + g_Y^2 \left( \frac{65}{36} \delta^{pc} Y_d^{*ad} Y_d^{br} + \frac{65}{36} \delta^{rd} Y_d^{*ap} Y_d^{bc} - \frac{4}{81} \delta^{rd} \delta^{ab} (Y_d^\dagger Y_d)^{pc} - \frac{4}{81} \delta^{pc} \delta^{ab} (Y_d^\dagger Y_d)^{dr} - \frac{13}{81} \delta^{cd} Y_d^{*ap} Y_d^{br} - \frac{55}{36} \delta^{pc} \delta^{rd} (Y_d Y_d^\dagger)^{ba} - \frac{61}{36} \delta^{pc} \delta^{rd} (Y_u Y_u^\dagger)^{ba} \right) \\
& + g_L^2 \left( \frac{3}{4} \delta^{pc} \delta^{rd} (Y_d Y_d^\dagger)^{ba} - \frac{3}{4} \delta^{pc} \delta^{rd} (Y_u Y_u^\dagger)^{ba} - \frac{9}{4} \delta^{pc} Y_d^{*ad} Y_d^{br} - \frac{9}{4} \delta^{rd} Y_d^{*ap} Y_d^{bc} \right) + g_s^2 \left( \frac{32}{27} \delta^{cd} Y_d^{*ap} Y_d^{br} + \frac{32}{3} \delta^{pc} \delta^{rd} (Y_u Y_u^\dagger)^{ba} - \frac{4}{27} \delta^{rd} \delta^{ab} (Y_d^\dagger Y_d)^{pc} \right. \\
& - \frac{4}{27} \delta^{pc} \delta^{ab} (Y_d^\dagger Y_d)^{dr} - \frac{4}{3} \delta^{pr} \delta^{ab} (Y_d^\dagger Y_d)^{dc} - \frac{4}{3} \delta^{pc} \delta^{rd} \delta^{ab} \text{Tr} [Y_d^\dagger Y_d] - \frac{32}{3} \delta^{pc} \delta^{rd} (Y_d Y_d^\dagger)^{ba} \Big) + \frac{3}{2} \delta^{pc} Y_d^{br} (Y_d^\dagger Y_d Y_d^\dagger)^{ad} + \frac{3}{2} \delta^{rd} Y_d^{*ap} (Y_d Y_d^\dagger Y_d)^{bc} \\
& + 3 Y_d^{*ap} Y_d^{br} (Y_d^\dagger Y_d)^{dc} + 3 \delta^{rd} Y_d^{bc} (Y_d^\dagger Y_d Y_d^\dagger)^{ap} + 3 \delta^{pc} Y_d^{*ad} (Y_d Y_d^\dagger Y_d)^{br} + 8 \delta^{pc} \delta^{rd} (Y_d Y_d^\dagger Y_d Y_d^\dagger)^{ba} - Y_d^{*ad} Y_d^{br} (Y_d^\dagger Y_d)^{pc} - Y_d^{*ap} Y_d^{bc} (Y_d^\dagger Y_d)^{dr} \\
& - \delta^{rd} (Y_d^\dagger Y_d)^{pc} (Y_u Y_u^\dagger)^{ba} - \delta^{pc} (Y_d^\dagger Y_d)^{dr} (Y_u Y_u^\dagger)^{ba} - \frac{9}{2} \delta^{pc} Y_d^{br} (Y_u^\dagger Y_u Y_d^\dagger)^{ad} - \frac{9}{2} \delta^{rd} Y_d^{*ap} (Y_u Y_u^\dagger Y_d)^{bc} - 6 \delta^{pc} \delta^{rd} (Y_u Y_u^\dagger Y_u Y_u^\dagger)^{ba} \Big\} C_{qd}^{(\times)abcd} \\
& + \left\{ \frac{16}{9} \delta^{pr} \delta^{ad} g_Y^2 (Y_e^\dagger Y_e)^{bc} - \frac{16}{27} \delta^{pr} \delta^{ab} \delta^{cd} g_Y^4 \right\} C_{ee}^{abcd} + \left\{ \frac{32}{9} \delta^{pr} \delta^{ad} g_Y^2 (Y_u^\dagger Y_u)^{bc} - \frac{64}{81} \delta^{pr} \delta^{ad} \delta^{bc} g_Y^4 \right\} C_{uu}^{abcd} + \left\{ g_Y^2 g_s^2 \left( \frac{4}{27} \delta^{pr} \delta^{ad} \delta^{bc} - \frac{152}{243} \delta^{pa} \delta^{rd} \delta^{bc} \right. \right. \\
& - 4 \delta^{pa} \delta^{rb} \delta^{cd} \Big) + g_Y^4 \left( \frac{64}{243} \delta^{pa} \delta^{rb} \delta^{cd} + \frac{232}{729} \delta^{pa} \delta^{rd} \delta^{bc} - \frac{16}{81} \delta^{pr} \delta^{ad} \delta^{bc} \right) + g_Y^2 \left( \frac{8}{27} \delta^{rb} \delta^{cd} (Y_d^\dagger Y_d)^{pa} + \frac{8}{27} \delta^{pa} \delta^{cd} (Y_d^\dagger Y_d)^{br} + \frac{16}{9} \delta^{pr} \delta^{ad} (Y_d^\dagger Y_d)^{bc} \right. \\
& - \frac{22}{81} \delta^{rb} \delta^{ad} (Y_d^\dagger Y_d)^{pc} - \frac{22}{81} \delta^{pa} \delta^{bc} (Y_d^\dagger Y_d)^{dr} - \frac{35}{18} \delta^{pa} \delta^{rd} (Y_d^\dagger Y_d)^{bc} - \frac{11}{2} \delta^{pa} \delta^{rb} (Y_d^\dagger Y_d)^{dc} \Big) + g_L^2 \left( \frac{15}{2} \delta^{pa} \delta^{rd} (Y_d^\dagger Y_d)^{bc} - \frac{9}{2} \delta^{pa} \delta^{rb} (Y_d^\dagger Y_d)^{dc} \right) \\
& + g_s^2 \left( \frac{92}{27} \delta^{rb} \delta^{ad} (Y_d^\dagger Y_d)^{pc} + \frac{92}{27} \delta^{pa} \delta^{bc} (Y_d^\dagger Y_d)^{dr} + 4 \delta^{pa} \delta^{rd} (Y_d^\dagger Y_d)^{bc} + 68 \delta^{pa} \delta^{rb} (Y_d^\dagger Y_d)^{dc} - \frac{4}{3} \delta^{pr} \delta^{ad} (Y_d^\dagger Y_d)^{bc} - \frac{4}{3} \delta^{pa} \delta^{rd} \delta^{bc} \text{Tr} [Y_d^\dagger Y_d] \right) \\
& + 4 \delta^{pa} (Y_d^\dagger Y_d)^{bc} (Y_d^\dagger Y_d)^{dr} + 4 \delta^{rb} (Y_d^\dagger Y_d)^{pc} (Y_d^\dagger Y_d)^{da} + 6 \delta^{pa} \delta^{rd} (Y_d^\dagger Y_u Y_u^\dagger Y_d)^{bc} + 6 \delta^{pa} \delta^{rb} (Y_d^\dagger Y_u Y_u^\dagger Y_d)^{dc} - 6 \delta^{rb} (Y_d^\dagger Y_d)^{pa} (Y_d^\dagger Y_d)^{dc} \\
& - 6 \delta^{pa} (Y_d^\dagger Y_d)^{br} (Y_d^\dagger Y_d)^{dc} - 20 \delta^{pa} \delta^{rd} (Y_d^\dagger Y_d Y_d^\dagger Y_d)^{bc} - 36 \delta^{pa} \delta^{rb} (Y_d^\dagger Y_d Y_d^\dagger Y_d)^{dc} \Big\} C_{dd}^{abcd} + \left\{ g_Y^2 \left( \frac{4}{27} \delta^{rd} \delta^{ab} (Y_d^\dagger Y_d)^{pc} + \frac{4}{27} \delta^{pc} \delta^{ab} (Y_d^\dagger Y_d)^{dr} \right. \right. \\
& + \frac{13}{12} \delta^{pc} \delta^{rd} (Y_e^\dagger Y_e)^{ba} \Big) - \frac{3}{4} \delta^{pc} \delta^{rd} g_L^2 (Y_e^\dagger Y_e)^{ba} - \delta^{rd} (Y_d^\dagger Y_d)^{pc} (Y_e^\dagger Y_e)^{ba} - \delta^{pc} (Y_d^\dagger Y_d)^{dr} (Y_e^\dagger Y_e)^{ba} - \frac{364}{243} \delta^{pc} \delta^{rd} \delta^{ab} g_Y^4 - 6 \delta^{pc} \delta^{rd} (Y_e^\dagger Y_e Y_e^\dagger Y_e)^{ba} \Big\} C_{ed}^{abcd} \\
& + \left\{ \frac{368}{243} \delta^{pc} \delta^{rd} \delta^{ab} g_Y^4 + \frac{9}{4} \delta^{pc} \delta^{rd} g_L^2 (Y_u^\dagger Y_u)^{ba} + 3 \delta^{rd} (Y_d^\dagger Y_d)^{pc} (Y_u^\dagger Y_u)^{ba} + 3 \delta^{pc} (Y_d^\dagger Y_d)^{dr} (Y_u^\dagger Y_u)^{ba} + \frac{16}{3} \delta^{pc} \delta^{rd} \delta^{ab} g_Y^2 g_s^2 + 18 \delta^{pc} \delta^{rd} (Y_u^\dagger Y_u Y_u^\dagger Y_u)^{ba} \right. \\
& - g_Y^2 \left( \frac{8}{27} \delta^{rd} \delta^{ab} (Y_d^\dagger Y_d)^{pc} + \frac{8}{27} \delta^{pc} \delta^{ab} (Y_d^\dagger Y_d)^{dr} + \frac{57}{4} \delta^{pc} \delta^{rd} (Y_u^\dagger Y_u)^{ba} \right) - 2 \delta^{pc} (Y_d^\dagger Y_u)^{da} (Y_u^\dagger Y_d)^{br} - 2 \delta^{rd} (Y_d^\dagger Y_u)^{pa} (Y_u^\dagger Y_d)^{bc} - 3 \delta^{pc} \delta^{rd} (Y_u^\dagger Y_d Y_d^\dagger Y_u)^{ba} \\
& - 40 \delta^{pc} \delta^{rd} g_s^2 (Y_u^\dagger Y_u)^{ba} \Big\} C_{ud}^{(\parallel)abcd} + \left\{ \frac{368}{729} \delta^{pc} \delta^{rd} \delta^{ab} g_Y^4 + \frac{3}{4} \delta^{pc} \delta^{rd} g_L^2 (Y_u^\dagger Y_u)^{ba} + g_Y^2 g_s^2 \left( \frac{2}{27} \delta^{pr} \delta^{ab} \delta^{cd} + \frac{506}{243} \delta^{pc} \delta^{rd} \delta^{ab} \right) + \delta^{rd} (Y_d^\dagger Y_d)^{pc} (Y_u^\dagger Y_u)^{ba} \right. \\
& + \delta^{pc} (Y_d^\dagger Y_d)^{dr} (Y_u^\dagger Y_u)^{ba} + g_s^2 \left( 16 \delta^{pc} \delta^{rd} (Y_u^\dagger Y_u)^{ba} - \frac{2}{27} \delta^{rd} \delta^{ab} (Y_d^\dagger Y_d)^{pc} - \frac{2}{27} \delta^{pc} \delta^{ab} (Y_d^\dagger Y_d)^{dr} - \frac{2}{3} \delta^{pr} \delta^{ab} (Y_d^\dagger Y_d)^{dc} - \frac{2}{3} \delta^{pc} \delta^{rd} \delta^{ab} \text{Tr} [Y_d^\dagger Y_d] \right) \Big\}
\end{aligned}$$

$$\begin{aligned}
& + 6\delta^{pc}\delta^{rd}(Y_u^\dagger Y_u Y_u^\dagger Y_u)^{ba} - g_Y^2 \left( \frac{8}{81}\delta^{rd}\delta^{ab}(Y_d^\dagger Y_d)^{pc} + \frac{8}{81}\delta^{pc}\delta^{ab}(Y_d^\dagger Y_d)^{dr} + \frac{19}{4}\delta^{pc}\delta^{rd}(Y_u^\dagger Y_u)^{ba} \right) - \delta^{pc}\delta^{rd}(Y_u^\dagger Y_d Y_d^\dagger Y_u)^{ba} - 6\delta^{pc}(Y_d^\dagger Y_u)^{da}(Y_u^\dagger Y_d)^{br} \\
& - 6\delta^{rd}(Y_d^\dagger Y_u)^{pa}(Y_u^\dagger Y_d)^{bc} \Big\} C_{ud}^{(\times)abcd} + \left\{ \frac{1}{6}Y_e^{*ab}Y_d^{dr}(Y_d^\dagger Y_d)^{pc} + \frac{3}{8}\delta^{pc}g_L^2 Y_e^{*ab}Y_d^{dr} + \frac{1}{2}\delta^{pc}Y_e^{*ab}(Y_u Y_u^\dagger Y_d)^{dr} - \frac{41}{216}\delta^{pc}g_Y^2 Y_e^{*ab}Y_d^{dr} - \frac{3}{4}\delta^{pc}Y_d^{dr}(Y_e^\dagger Y_e Y_e^\dagger)^{ab} \right. \\
& - \delta^{pc}Y_e^{*ab}(Y_d Y_d^\dagger Y_d)^{dr} \Big\} C_{ledq}^{abcd} + C_{ledq}^{*abcd} \left\{ \frac{1}{6}Y_d^{*dp}Y_e^{ab}(Y_d^\dagger Y_d)^{cr} + \frac{3}{8}\delta^{rc}g_L^2 Y_d^{*dp}Y_e^{ab} + \frac{1}{2}\delta^{rc}Y_e^{ab}(Y_u^\dagger Y_u Y_d^\dagger)^{dp} - \frac{41}{216}\delta^{rc}g_Y^2 Y_d^{*dp}Y_e^{ab} \right. \\
& - \frac{3}{4}\delta^{rc}Y_d^{*dp}(Y_e Y_e^\dagger Y_e)^{ab} - \delta^{rc}Y_e^{ab}(Y_d^\dagger Y_d Y_d^\dagger)^{dp} \Big\} + \left\{ \frac{1}{12}Y_d^{*ap}Y_u^{*cb}(Y_d^\dagger Y_d)^{dr} + \frac{1}{4}\delta^{rd}Y_u^{*cb}(Y_u^\dagger Y_u Y_d^\dagger)^{ap} + \frac{1}{2}Y_d^{*cp}Y_u^{*ab}(Y_d^\dagger Y_d)^{dr} + \frac{1}{2}\delta^{rd}Y_d^{*ap}(Y_u^\dagger Y_u Y_u^\dagger)^{cb} \right. \\
& + \frac{3}{4}\delta^{rd}Y_d^{*cp}(Y_d^\dagger Y_d Y_u^\dagger)^{ab} + \frac{9}{8}\delta^{rd}g_L^2 Y_d^{*cp}Y_u^{*ab} + \frac{3}{2}\delta^{rd}Y_d^{*ap}(Y_d^\dagger Y_d Y_u^\dagger)^{cb} + \frac{3}{2}\delta^{rd}Y_u^{*ab}(Y_u^\dagger Y_u Y_d^\dagger)^{cp} + \frac{16}{3}\delta^{rd}g_s^2 Y_d^{*ap}Y_u^{*cb} - \frac{1}{6}Y_d^{*ad}Y_d^{*cp}(Y_u^\dagger Y_d)^{br} \\
& - \frac{1}{2}\delta^{rd}Y_u^{*cb}(Y_d^\dagger Y_d Y_d^\dagger)^{ap} - g_Y^2 \left( \frac{41}{72}\delta^{rd}Y_d^{*cp}Y_u^{*ab} + \frac{17}{27}\delta^{rd}Y_d^{*ap}Y_u^{*cb} \right) - Y_d^{*ap}Y_d^{*cd}(Y_u^\dagger Y_d)^{br} - \frac{9}{4}\delta^{rd}Y_d^{*cp}(Y_u^\dagger Y_u Y_u^\dagger)^{ab} - 3\delta^{rd}Y_u^{*ab}(Y_d^\dagger Y_d Y_d^\dagger)^{cp} \Big\} C_{quqd}^{(II)abcd} \\
& + \left( C_{quqd}^{(II)*} \right)^{abcd} \left\{ \frac{1}{12}Y_d^{ar}Y_u^{cb}(Y_d^\dagger Y_d)^{pd} + \frac{1}{4}\delta^{pd}Y_u^{cb}(Y_u Y_u^\dagger Y_d)^{ar} + \frac{1}{2}Y_d^{cr}Y_u^{ab}(Y_d^\dagger Y_d)^{pd} + \frac{1}{2}\delta^{pd}Y_d^{ar}(Y_u Y_u^\dagger Y_u)^{cb} + \frac{3}{4}\delta^{pd}Y_d^{cr}(Y_d Y_d^\dagger Y_u)^{ab} + \frac{9}{8}\delta^{pd}g_L^2 Y_d^{cr}Y_u^{ab} \right. \\
& + \frac{3}{2}\delta^{pd}Y_d^{ar}(Y_d Y_d^\dagger Y_u)^{cb} + \frac{3}{2}\delta^{pd}Y_u^{ab}(Y_u Y_u^\dagger Y_d)^{cr} + \frac{16}{3}\delta^{pd}g_s^2 Y_d^{ar}Y_u^{cb} - \frac{1}{6}Y_d^{ad}Y_d^{cr}(Y_d^\dagger Y_u)^{pb} - \frac{1}{2}\delta^{pd}Y_u^{cb}(Y_d Y_d^\dagger Y_d)^{ar} - g_Y^2 \left( \frac{41}{72}\delta^{pd}Y_d^{cr}Y_u^{ab} + \frac{17}{27}\delta^{pd}Y_d^{ar}Y_u^{cb} \right) \\
& - Y_d^{ar}Y_d^{cd}(Y_d^\dagger Y_u)^{pb} - \frac{9}{4}\delta^{pd}Y_d^{cr}(Y_u Y_u^\dagger Y_u)^{ab} - 3\delta^{pd}Y_u^{ab}(Y_d Y_d^\dagger Y_d)^{cr} \Big\} + \left\{ \frac{1}{6}Y_d^{*cp}Y_u^{*ab}(Y_d^\dagger Y_d)^{dr} + \frac{1}{4}Y_d^{*ap}Y_u^{*cb}(Y_d^\dagger Y_d)^{dr} + \frac{1}{4}\delta^{rd}Y_d^{*cp}(Y_d^\dagger Y_d Y_u^\dagger)^{ab} \right. \\
& + \frac{3}{8}\delta^{rd}g_L^2 Y_d^{*cp}Y_u^{*ab} + \frac{1}{2}\delta^{rd}Y_u^{*ab}(Y_u^\dagger Y_u Y_d^\dagger)^{cp} + \frac{3}{4}\delta^{rd}Y_u^{*cb}(Y_u^\dagger Y_u Y_d^\dagger)^{ap} + \frac{3}{2}\delta^{rd}Y_d^{*ap}(Y_u^\dagger Y_u Y_u^\dagger)^{cb} + \frac{9}{2}\delta^{rd}Y_d^{*ap}(Y_d^\dagger Y_d Y_u^\dagger)^{cb} - \frac{1}{3}Y_d^{*ap}Y_d^{*cd}(Y_u^\dagger Y_d)^{br} \\
& - \frac{1}{2}Y_d^{*ad}Y_d^{*cp}(Y_u^\dagger Y_d)^{br} - \frac{3}{4}\delta^{rd}Y_d^{*cp}(Y_u^\dagger Y_u Y_u^\dagger)^{ab} - g_Y^2 \left( \frac{41}{216}\delta^{rd}Y_d^{*cp}Y_u^{*ab} + \frac{17}{9}\delta^{rd}Y_d^{*ap}Y_u^{*cb} \right) - \delta^{rd}Y_u^{*ab}(Y_d^\dagger Y_d Y_d^\dagger)^{cp} \\
& - \frac{3}{2}\delta^{rd}Y_u^{*cb}(Y_d^\dagger Y_d Y_d^\dagger)^{ap} \Big\} C_{quqd}^{(\times)abcd} + \left( C_{quqd}^{(\times)*} \right)^{abcd} \left\{ \frac{1}{6}Y_d^{cr}Y_u^{ab}(Y_d^\dagger Y_d)^{pd} + \frac{1}{4}Y_d^{ar}Y_u^{cb}(Y_d^\dagger Y_d)^{pd} + \frac{1}{4}\delta^{pd}Y_d^{cr}(Y_d Y_d^\dagger Y_u)^{ab} + \frac{3}{8}\delta^{pd}g_L^2 Y_d^{cr}Y_u^{ab} + \frac{1}{2}\delta^{pd}Y_u^{ab}(Y_u Y_u^\dagger Y_d)^{cr} \right. \\
& + \frac{3}{4}\delta^{pd}Y_u^{cb}(Y_u Y_u^\dagger Y_d)^{ar} + \frac{3}{2}\delta^{pd}Y_d^{ar}(Y_u Y_u^\dagger Y_u)^{cb} + \frac{9}{2}\delta^{pd}Y_d^{ar}(Y_d Y_d^\dagger Y_u)^{cb} - \frac{1}{3}Y_d^{ar}Y_d^{cd}(Y_d^\dagger Y_u)^{pb} - \frac{1}{2}Y_d^{ad}Y_d^{cr}(Y_d^\dagger Y_u)^{pb} - \frac{3}{4}\delta^{pd}Y_d^{cr}(Y_u Y_u^\dagger Y_u)^{ab} \\
& - g_Y^2 \left( \frac{41}{216}\delta^{pd}Y_d^{cr}Y_u^{ab} + \frac{17}{9}\delta^{pd}Y_d^{ar}Y_u^{cb} \right) - \delta^{pd}Y_u^{ab}(Y_d Y_d^\dagger Y_d)^{cr} - \frac{3}{2}\delta^{pd}Y_u^{cb}(Y_d Y_d^\dagger Y_d)^{ar} \Big\} + \frac{1}{3}Y_d^{*cp}Y_e^{*ab} C_{lequ}^{abcd}(Y_u^\dagger Y_d)^{dr} + \frac{1}{3} C_{lequ}^{*abcd} Y_d^{cr}Y_e^{ab}(Y_d^\dagger Y_u)^{pd} \\
& - \frac{1}{6}Y_d^{*cp}Y_e^{*ad} C_{luqe}^{abcd}(Y_u^\dagger Y_d)^{br} - \frac{1}{6} C_{luqe}^{*abcd} Y_d^{cr}Y_e^{ad}(Y_d^\dagger Y_u)^{pb} - \left\{ \frac{8}{27}\delta^{pr}\delta^{ad}\delta^{bc}g_Y^4 + \frac{8}{9}\delta^{pr}\delta^{bc}g_Y^2(Y_e Y_e^\dagger)^{da} \right\} C_{\ell\ell}^{abcd} + \left\{ \frac{1}{3}\delta^{bc}g_L^2 Y_d^{*ap}Y_d^{dr} \right. \\
& + g_Y^2 \left( \frac{8}{9}\delta^{pr}\delta^{bc}(Y_d Y_d^\dagger)^{da} - \frac{10}{27}\delta^{cd}Y_d^{*ap}Y_d^{br} - \frac{41}{81}\delta^{bc}Y_d^{*ap}Y_d^{dr} - \frac{8}{9}\delta^{pr}\delta^{bc}(Y_u Y_u^\dagger)^{da} \right) + \frac{64}{27}\delta^{bc}g_s^2 Y_d^{*ap}Y_d^{dr} + 6Y_d^{*ap}Y_d^{br}(Y_u Y_u^\dagger)^{dc} - \frac{8}{81}\delta^{pr}\delta^{ad}\delta^{bc}g_Y^4
\end{aligned}$$

$$\begin{aligned}
& -6Y_d^{*ap}Y_d^{br}(Y_dY_d^\dagger)^{dc} - 6Y_d^{*ap}Y_d^{dr}(Y_uY_u^\dagger)^{bc} \Big\} C_{qq}^{(\parallel)abcd} + \left\{ \delta^{cd}g_L^2Y_d^{*ap}Y_d^{br} + g_Y^2\left(\frac{16}{9}\delta^{pr}\delta^{bc}(Y_dY_d^\dagger)^{da} - \frac{5}{27}\delta^{cd}Y_d^{*ap}Y_d^{br} - \frac{82}{81}\delta^{bc}Y_d^{*ap}Y_d^{dr} \right. \right. \\
& - \frac{16}{9}\delta^{pr}\delta^{bc}(Y_uY_u^\dagger)^{da}) + \frac{128}{27}\delta^{bc}g_s^2Y_d^{*ap}Y_d^{dr} + 6Y_d^{*ap}Y_d^{dr}(Y_dY_d^\dagger)^{bc} - \frac{16}{81}\delta^{pr}\delta^{ad}\delta^{bc}g_Y^4 - 6Y_d^{*ap}Y_d^{dr}(Y_uY_u^\dagger)^{bc} - 6Y_d^{*ap}Y_d^{br}(Y_uY_u^\dagger)^{dc} \\
& - 12Y_d^{*ap}Y_d^{br}(Y_dY_d^\dagger)^{dc} \Big\} C_{qq}^{(\times)abcd} + \left\{ \frac{5}{27}\delta^{ab}g_Y^2Y_d^{*cp}Y_d^{dr} - Y_d^{*cp}Y_d^{dr}(Y_eY_e^\dagger)^{ba} \right\} C_{\ell q}^{(\parallel)abcd} + \left\{ \frac{5}{54}\delta^{ab}g_Y^2Y_d^{*cp}Y_d^{dr} + \frac{1}{6}\delta^{ab}g_L^2Y_d^{*cp}Y_d^{dr} \right. \\
& \left. - 2Y_d^{*cp}Y_d^{dr}(Y_eY_e^\dagger)^{ba} \right\} C_{\ell q}^{(\times)abcd}, \tag{9.14}
\end{aligned}$$

## 9.8 $C_{Hud}$

$$\begin{aligned}
\beta_{C_{Hud}^{pr}}^{(1)} &= C_{HD}^{(\parallel)}(Y_u^\dagger Y_d)^{pr} - C_{HD}^{(\times)}(Y_u^\dagger Y_d)^{pr} + 2\delta^{pa}C_{Hu}^{ab}(Y_u^\dagger Y_d)^{br} - 2\delta^{rb}C_{Hd}^{ab}(Y_u^\dagger Y_d)^{pa} + \left\{ 2T_2\delta^{pa}\delta^{rb} + 3\delta^{pa}(Y_d^\dagger Y_d)^{br} + 3\delta^{rb}(Y_u^\dagger Y_u)^{pa} \right. \\
& \left. - 3\delta^{pa}\delta^{rb}g_Y^2 \right\} C_{Hud}^{ab} + 4\delta^{pa}\delta^{rd}C_{ud}^{(\parallel)abcd}(Y_u^\dagger Y_d)^{bc} + 12\delta^{pa}\delta^{rd}C_{ud}^{(\times)abcd}(Y_u^\dagger Y_d)^{bc}, \tag{9.15}
\end{aligned}$$

$$\begin{aligned}
\beta_{C_{Hud}^{pr}}^{(2)} &= \left\{ \frac{137}{24}g_L^2(Y_u^\dagger Y_d)^{pr} - \frac{11}{24}g_Y^2(Y_u^\dagger Y_d)^{pr} - T_2(Y_u^\dagger Y_d)^{pr} - 2(Y_u^\dagger Y_d Y_d^\dagger Y_d)^{pr} - 2(Y_u^\dagger Y_u Y_u^\dagger Y_d)^{pr} - \frac{16}{3}g_s^2(Y_u^\dagger Y_d)^{pr} \right\} C_{HD}^{(\parallel)} + \left\{ \frac{1}{6}g_Y^2(Y_u^\dagger Y_d)^{pr} \right. \\
& + T_2(Y_u^\dagger Y_d)^{pr} + \frac{11}{4}(Y_u^\dagger Y_d Y_d^\dagger Y_d)^{pr} + \frac{11}{4}(Y_u^\dagger Y_u Y_u^\dagger Y_d)^{pr} + \frac{16}{3}g_s^2(Y_u^\dagger Y_d)^{pr} - \frac{3}{2}\lambda(Y_u^\dagger Y_d)^{pr} - \frac{27}{4}g_L^2(Y_u^\dagger Y_d)^{pr} \Big\} C_{HD}^{(\times)} - \frac{10}{9}g_Y^4 C_{HB}(Y_u^\dagger Y_d)^{pr} \\
& - \frac{4i}{3}g_Y^4 C_{H\tilde{B}}(Y_u^\dagger Y_d)^{pr} - \frac{160}{3}g_s^4 C_{HG}(Y_u^\dagger Y_d)^{pr} - \frac{3}{2}g_Y^2 g_L^2 C_{HWB}(Y_u^\dagger Y_d)^{pr} + ig_Y^2 g_L^2 C_{H\tilde{W}B}(Y_u^\dagger Y_d)^{pr} + 6g_L^6 C_W(Y_u^\dagger Y_d)^{pr} + 16g_s^6 C_G(Y_u^\dagger Y_d)^{pr} \\
& + C_{uH}^{*ab} \left\{ \frac{9}{2}\delta^{pb}g_L^2 Y_d^{ar} - 3\delta^{pb}\lambda Y_d^{ar} - 3\delta^{pb}(Y_d Y_d^\dagger Y_d)^{ar} \right\} + \left\{ \frac{9}{2}\delta^{rb}g_L^2 Y_u^{*ap} - 3\delta^{rb}\lambda Y_u^{*ap} - 3\delta^{rb}(Y_u^\dagger Y_u Y_u^\dagger)^{ap} \right\} C_{dH}^{ab} + \frac{7}{3}g_Y^2 Y_u^{*ap} C_{uB}^{ab}(Y_u^\dagger Y_d)^{br} \\
& + C_{uB}^{*ab} \left\{ \frac{2927}{108}\delta^{pb}g_Y^4 Y_d^{ar} - g_Y^2 \left( \frac{2}{3}\delta^{pb}(Y_u Y_u^\dagger Y_d)^{ar} + 3T_2\delta^{pb}Y_d^{ar} + \frac{11}{3}Y_d^{ar}(Y_u^\dagger Y_u)^{pb} + \frac{17}{3}\delta^{pb}(Y_d Y_d^\dagger Y_d)^{ar} \right) - \frac{5}{4}\delta^{pb}g_Y^2 g_L^2 Y_d^{ar} - \frac{160}{9}\delta^{pb}g_Y^2 g_s^2 Y_d^{ar} \right\} \\
& + \frac{3}{2}g_L^2 Y_u^{*ap} C_{uW}^{ab}(Y_u^\dagger Y_d)^{br} + C_{uW}^{*ab} \left\{ -g_L^2 \left( \frac{3}{2}Y_d^{ar}(Y_u^\dagger Y_u)^{pb} + \frac{3}{2}\delta^{pb}(Y_d Y_d^\dagger Y_d)^{ar} + \frac{9}{2}T_2\delta^{pb}Y_d^{ar} \right) - \frac{29}{24}\delta^{pb}g_Y^2 g_L^2 Y_d^{ar} - \frac{69}{8}\delta^{pb}g_L^4 Y_d^{ar} - 9\delta^{pb}\lambda g_L^2 Y_d^{ar} \right. \\
& \left. - 16\delta^{pb}g_s^2 g_L^2 Y_d^{ar} \right\} - \frac{16}{3}g_s^2 Y_u^{*ap} C_{uG}^{ab}(Y_u^\dagger Y_d)^{br} + C_{uG}^{*ab} \left\{ g_s^2 \left( \frac{8}{3}Y_d^{ar}(Y_u^\dagger Y_u)^{pb} + \frac{8}{3}\delta^{pb}(Y_u Y_u^\dagger Y_d)^{ar} - \frac{16}{3}\delta^{pb}(Y_d Y_d^\dagger Y_d)^{ar} \right) + \frac{124}{27}\delta^{pb}g_Y^2 g_s^2 Y_d^{ar} \right.
\end{aligned}$$

$$\begin{aligned}
& + 20\delta^{pb}g_s^2g_L^2Y_d^{ar} + \frac{640}{9}\delta^{pb}g_s^4Y_d^{ar} \Big\} + \left\{ g_Y^2 \left( \frac{4}{3}\delta^{rb}(Y_d^\dagger Y_d Y_u^\dagger)^{ap} + 3T_2\delta^{rb}Y_u^{*ap} + \frac{13}{3}Y_u^{*ap}(Y_d^\dagger Y_d)^{br} + \frac{13}{3}\delta^{rb}(Y_u^\dagger Y_u Y_u^\dagger)^{ap} \right) + \frac{32}{9}\delta^{rb}g_Y^2g_s^2Y_u^{*ap} \right. \\
& + \frac{25}{4}\delta^{rb}g_Y^2g_L^2Y_u^{*ap} - \frac{2563}{108}\delta^{rb}g_Y^4Y_u^{*ap} \Big\} C_{dB}^{ab} - \frac{11}{3}g_Y^2C_{dB}^{*ab}Y_d^{ar}(Y_u^\dagger Y_d)^{pb} + \left\{ -g_L^2 \left( \frac{3}{2}Y_u^{*ap}(Y_d^\dagger Y_d)^{br} + \frac{3}{2}\delta^{rb}(Y_u^\dagger Y_u Y_u^\dagger)^{ap} + \frac{9}{2}T_2\delta^{rb}Y_u^{*ap} \right) \right. \\
& - \frac{77}{24}\delta^{rb}g_Y^2g_L^2Y_u^{*ap} - \frac{69}{8}\delta^{rb}g_L^4Y_u^{*ap} - 9\delta^{rb}\lambda g_L^2Y_u^{*ap} - 16\delta^{rb}g_s^2g_L^2Y_u^{*ap} \Big\} C_{dW}^{ab} + \frac{3}{2}g_L^2C_{dW}^{*ab}Y_d^{ar}(Y_u^\dagger Y_d)^{pb} + \left\{ g_s^2 \left( \frac{8}{3}Y_u^{*ap}(Y_d^\dagger Y_d)^{br} \right. \right. \\
& + \frac{8}{3}\delta^{rb}(Y_d^\dagger Y_d Y_u^\dagger)^{ap} - \frac{16}{3}\delta^{rb}(Y_u^\dagger Y_u Y_u^\dagger)^{ap} \Big) + \frac{172}{27}\delta^{rb}g_Y^2g_s^2Y_u^{*ap} + 20\delta^{rb}g_s^2g_L^2Y_u^{*ap} + \frac{640}{9}\delta^{rb}g_s^4Y_u^{*ap} \Big\} C_{dG}^{ab} - \frac{16}{3}g_s^2C_{dG}^{*ab}Y_d^{ar}(Y_u^\dagger Y_d)^{pb} \\
& + \left\{ \frac{1}{9}\delta^{ab}g_Y^2(Y_u^\dagger Y_d)^{pr} - (Y_u^\dagger Y_d)^{pr}(Y_e Y_e^\dagger)^{ba} \right\} C_{H\ell}^{(\parallel)ab} + \left\{ \frac{1}{18}\delta^{ab}g_Y^2(Y_u^\dagger Y_d)^{pr} + (Y_u^\dagger Y_d)^{pr}(Y_e Y_e^\dagger)^{ba} - \frac{1}{6}\delta^{ab}g_L^2(Y_u^\dagger Y_d)^{pr} \right\} C_{H\ell}^{(\times)ab} + \left\{ \frac{1}{9}\delta^{ab}g_Y^2(Y_u^\dagger Y_d)^{pr} \right. \\
& + (Y_e^\dagger Y_e)^{ba}(Y_u^\dagger Y_d)^{pr} \Big\} C_{He}^{ab} + \left\{ \frac{4}{3}Y_d^{br}(Y_d^\dagger Y_d Y_u^\dagger)^{ap} + 3(Y_u^\dagger Y_d)^{pr}(Y_u Y_u^\dagger)^{ba} + \frac{16}{3}Y_u^{*ap}(Y_d Y_d^\dagger Y_d)^{br} - g_Y^2 \left( \frac{1}{9}\delta^{ab}(Y_u^\dagger Y_d)^{pr} + \frac{5}{27}Y_u^{*ap}Y_d^{br} \right) - \frac{4}{3}Y_u^{*ap}(Y_u Y_u^\dagger Y_d)^{br} \right. \\
& - 3(Y_u^\dagger Y_d)^{pr}(Y_d Y_d^\dagger)^{ba} - \frac{16}{3}Y_d^{br}(Y_u^\dagger Y_u Y_u^\dagger)^{ap} \Big\} C_{Hq}^{(\parallel)ab} + \left\{ g_Y^2 \left( \frac{35}{108}Y_u^{*ap}Y_d^{br} - \frac{1}{18}\delta^{ab}(Y_u^\dagger Y_d)^{pr} \right) + \frac{7}{6}Y_d^{br}(Y_d^\dagger Y_d Y_u^\dagger)^{ap} + 3(Y_u^\dagger Y_d)^{pr}(Y_d Y_d^\dagger)^{ba} \right. \\
& + 6(Y_u^\dagger Y_d)^{pr}(Y_u Y_u^\dagger)^{ba} - \frac{1}{6}Y_u^{*ap}(Y_u Y_u^\dagger Y_d)^{br} - g_L^2 \left( \frac{1}{2}\delta^{ab}(Y_u^\dagger Y_d)^{pr} + \frac{7}{12}Y_u^{*ap}Y_d^{br} \right) - \frac{4}{3}Y_u^{*ap}(Y_d Y_d^\dagger Y_d)^{br} - \frac{20}{3}Y_d^{br}(Y_u^\dagger Y_u Y_u^\dagger)^{ap} - 16g_s^2Y_u^{*ap}Y_d^{br} \Big\} C_{Hq}^{(\times)ab} \\
& + \left\{ \frac{1}{2}(Y_u^\dagger Y_d)^{br}(Y_u^\dagger Y_u)^{pa} + 8\delta^{pa}g_s^2(Y_u^\dagger Y_d)^{br} - T_2\delta^{pa}(Y_u^\dagger Y_d)^{br} - g_Y^2 \left( \frac{2}{9}\delta^{ab}(Y_u^\dagger Y_d)^{pr} + \frac{131}{54}\delta^{pa}(Y_u^\dagger Y_d)^{br} \right) - 3(Y_u^\dagger Y_d)^{pr}(Y_u^\dagger Y_u)^{ba} - 6\delta^{pa}(Y_u^\dagger Y_u Y_u^\dagger Y_d)^{br} \right. \\
& - \frac{15}{2}\delta^{pa}(Y_u^\dagger Y_d Y_d^\dagger Y_d)^{br} \Big\} C_{Hu}^{ab} + \left\{ T_2\delta^{rb}(Y_u^\dagger Y_d)^{pa} + g_Y^2 \left( \frac{1}{9}\delta^{ab}(Y_u^\dagger Y_d)^{pr} - \frac{11}{54}\delta^{rb}(Y_u^\dagger Y_d)^{pa} \right) + 3(Y_d^\dagger Y_d)^{ba}(Y_u^\dagger Y_d)^{pr} + 6\delta^{rb}(Y_u^\dagger Y_d Y_d^\dagger Y_d)^{pa} \right. \\
& + \frac{15}{2}\delta^{rb}(Y_u^\dagger Y_u Y_u^\dagger Y_d)^{pa} - \frac{1}{2}(Y_d^\dagger Y_d)^{br}(Y_u^\dagger Y_d)^{pa} - 8\delta^{rb}g_s^2(Y_u^\dagger Y_d)^{pa} \Big\} C_{Hd}^{ab} + \left\{ g_L^2 \left( \frac{93}{8}\delta^{pa}(Y_d^\dagger Y_d)^{br} + \frac{93}{8}\delta^{rb}(Y_u^\dagger Y_u)^{pa} - \frac{3}{4}T_2\delta^{pa}\delta^{rb} \right) \right. \\
& + g_Y^2 \left( \frac{455}{72}\delta^{pa}(Y_d^\dagger Y_d)^{br} + \frac{79}{12}\delta^{pa}\delta^{rb}\text{Tr}[Y_d^\dagger Y_d] + \frac{31}{4}\delta^{pa}\delta^{rb}\text{Tr}[Y_e^\dagger Y_e] + \frac{707}{72}\delta^{rb}(Y_u^\dagger Y_u)^{pa} + \frac{139}{12}\delta^{pa}\delta^{rb}\text{Tr}[Y_u^\dagger Y_u] \right) + g_s^2 \left( 40\delta^{pa}\delta^{rb}\text{Tr}[Y_d^\dagger Y_d] \right. \\
& + 40\delta^{pa}\delta^{rb}\text{Tr}[Y_u^\dagger Y_u] - \frac{8}{3}\delta^{pa}(Y_d^\dagger Y_d)^{br} - \frac{8}{3}\delta^{rb}(Y_u^\dagger Y_u)^{pa} \Big) + \frac{9}{4}\delta^{pa}(Y_d^\dagger Y_d Y_d^\dagger Y_d)^{br} + \frac{9}{4}\delta^{rb}(Y_u^\dagger Y_u Y_u^\dagger Y_u)^{pa} + 6(Y_d^\dagger Y_u)^{ba}(Y_u^\dagger Y_d)^{pr} + \frac{95}{12}\delta^{pa}\delta^{rb}g_Y^4 \\
& - \frac{1}{4}\delta^{pa}(Y_d^\dagger Y_u Y_u^\dagger Y_d)^{br} - \frac{1}{4}\delta^{rb}(Y_u^\dagger Y_d Y_d^\dagger Y_u)^{pa} - \lambda \left( 9\delta^{pa}(Y_d^\dagger Y_d)^{br} + 9\delta^{rb}(Y_u^\dagger Y_u)^{pa} \right) - 3(Y_d^\dagger Y_d)^{br}(Y_u^\dagger Y_u)^{pa} - 4\delta^{pa}\delta^{rb}g_Y^2g_s^2 - \frac{9}{2}T_4\delta^{pa}\delta^{rb} \\
& - \frac{9}{2}T_2\delta^{pa}(Y_d^\dagger Y_d)^{br} - \frac{9}{2}T_2\delta^{rb}(Y_u^\dagger Y_u)^{pa} - 15\delta^{pa}\delta^{rb}\text{Tr}[Y_d^\dagger Y_d Y_u^\dagger Y_u] \Big\} C_{Hud}^{ab} - 12C_{Hud}^{*ab}(Y_u^\dagger Y_d)^{pr}(Y_u^\dagger Y_d)^{ab} - \frac{34}{27}\delta^{pc}\delta^{ab}g_Y^2C_{\ell u}^{abcd}(Y_u^\dagger Y_d)^{dr}
\end{aligned}$$

$$\begin{aligned}
& + \frac{62}{27} \delta^{rd} \delta^{ab} g_Y^2 \mathcal{C}_{td}^{abcd} (Y_u^\dagger Y_d)^{pc} - \frac{8}{27} \delta^{cd} g_Y^2 Y_u^{*ap} \mathcal{C}_{qe}^{abcd} Y_d^{br} + \left\{ g_Y^2 \left( \frac{1}{2} \delta^{pc} Y_u^{*ad} Y_d^{br} + \frac{16}{27} \delta^{cd} Y_u^{*ap} Y_d^{br} + \frac{34}{27} \delta^{pc} \delta^{ab} (Y_u^\dagger Y_d)^{dr} \right) + \frac{4}{3} Y_u^{*ap} Y_u^{bc} (Y_u^\dagger Y_d)^{dr} \right. \\
& + 2\delta^{pc} Y_d^{br} (Y_d^\dagger Y_d Y_u^\dagger)^{ad} + 2\delta^{pc} Y_u^{*ad} (Y_d Y_d^\dagger Y_d)^{br} - \frac{2}{3} Y_u^{*ad} Y_d^{br} (Y_u^\dagger Y_u)^{pc} - \frac{3}{2} \delta^{pc} g_L^2 Y_u^{*ad} Y_d^{br} \left. \right\} \mathcal{C}_{qu}^{(II)abcd} + \left\{ g_s^2 \left( \frac{64}{27} \delta^{cd} Y_u^{*ap} Y_d^{br} - \frac{224}{27} \delta^{pc} \delta^{ab} (Y_u^\dagger Y_d)^{dr} \right) \right. \\
& + g_Y^2 \left( \frac{16}{81} \delta^{cd} Y_u^{*ap} Y_d^{br} + \frac{34}{81} \delta^{pc} \delta^{ab} (Y_u^\dagger Y_d)^{dr} + \frac{3}{2} \delta^{pc} Y_u^{*ad} Y_d^{br} \right) + 4Y_u^{*ap} Y_u^{bc} (Y_u^\dagger Y_d)^{dr} + 6\delta^{pc} Y_d^{br} (Y_d^\dagger Y_d Y_u^\dagger)^{ad} + 6\delta^{pc} Y_u^{*ad} (Y_d Y_d^\dagger Y_d)^{br} \\
& - 2Y_u^{*ad} Y_d^{br} (Y_u^\dagger Y_u)^{pc} - \frac{9}{2} \delta^{pc} g_L^2 Y_u^{*ad} Y_d^{br} \left. \right\} \mathcal{C}_{qu}^{(\times)abcd} + \left\{ \frac{4}{3} Y_d^{*ad} Y_d^{br} (Y_u^\dagger Y_d)^{pc} + 2\delta^{rd} Y_d^{bc} (Y_u^\dagger Y_u Y_u^\dagger)^{ap} + 2\delta^{rd} Y_u^{*ap} (Y_u Y_u^\dagger Y_d)^{bc} - \frac{2}{3} Y_u^{*ap} Y_d^{bc} (Y_d^\dagger Y_d)^{dr} \right. \\
& - g_Y^2 \left( \frac{8}{27} \delta^{cd} Y_u^{*ap} Y_d^{br} + \frac{3}{2} \delta^{rd} Y_u^{*ap} Y_d^{bc} + \frac{62}{27} \delta^{rd} \delta^{ab} (Y_u^\dagger Y_d)^{pc} \right) - \frac{3}{2} \delta^{rd} g_L^2 Y_u^{*ap} Y_d^{bc} \left. \right\} \mathcal{C}_{qd}^{(II)abcd} + \left\{ g_s^2 \left( \frac{64}{27} \delta^{cd} Y_u^{*ap} Y_d^{br} - \frac{224}{27} \delta^{rd} \delta^{ab} (Y_u^\dagger Y_d)^{pc} \right) \right. \\
& + 4Y_d^{*ad} Y_d^{br} (Y_u^\dagger Y_d)^{pc} + 6\delta^{rd} Y_d^{bc} (Y_u^\dagger Y_u Y_u^\dagger)^{ap} + 6\delta^{rd} Y_u^{*ap} (Y_u Y_u^\dagger Y_d)^{bc} - g_Y^2 \left( \frac{8}{81} \delta^{cd} Y_u^{*ap} Y_d^{br} + \frac{62}{81} \delta^{rd} \delta^{ab} (Y_u^\dagger Y_d)^{pc} + \frac{9}{2} \delta^{rd} Y_u^{*ap} Y_d^{bc} \right) \\
& - 2Y_u^{*ap} Y_d^{bc} (Y_d^\dagger Y_d)^{dr} - \frac{9}{2} \delta^{rd} g_L^2 Y_u^{*ap} Y_d^{bc} \left. \right\} \mathcal{C}_{qd}^{(\times)abcd} + \left\{ g_Y^2 \left( \frac{112}{81} \delta^{pa} \delta^{bc} (Y_u^\dagger Y_d)^{dr} + \frac{136}{27} \delta^{pa} \delta^{cd} (Y_u^\dagger Y_d)^{br} \right) - \frac{32}{27} \delta^{pa} \delta^{bc} g_s^2 (Y_u^\dagger Y_d)^{dr} \right. \\
& - 4\delta^{pa} (Y_u^\dagger Y_d)^{dr} (Y_u^\dagger Y_u)^{bc} \left. \right\} \mathcal{C}_{uu}^{abcd} + \left\{ g_Y^2 \left( \frac{64}{81} \delta^{rb} \delta^{ad} (Y_u^\dagger Y_d)^{pc} + \frac{124}{27} \delta^{rb} \delta^{cd} (Y_u^\dagger Y_d)^{pa} \right) - \frac{32}{27} \delta^{rb} \delta^{ad} g_s^2 (Y_u^\dagger Y_d)^{pc} - 4\delta^{rb} (Y_d^\dagger Y_d)^{da} (Y_u^\dagger Y_d)^{pc} \right. \\
& - \frac{34}{27} \delta^{pc} \delta^{ab} g_Y^2 \mathcal{C}_{eu}^{abcd} (Y_u^\dagger Y_d)^{dr} + \frac{62}{27} \delta^{rd} \delta^{ab} g_Y^2 \mathcal{C}_{ed}^{abcd} (Y_u^\dagger Y_d)^{pc} + \left\{ g_Y^2 \left( \frac{47}{6} \delta^{pa} \delta^{rd} (Y_u^\dagger Y_d)^{bc} - \frac{34}{27} \delta^{pa} \delta^{cd} (Y_u^\dagger Y_d)^{br} - \frac{124}{27} \delta^{rd} \delta^{ab} (Y_u^\dagger Y_d)^{pc} \right) \right. \\
& + 2\delta^{pa} (Y_d^\dagger Y_d)^{dr} (Y_u^\dagger Y_d)^{bc} + 2\delta^{rd} (Y_u^\dagger Y_d)^{bc} (Y_u^\dagger Y_u)^{pa} + \frac{15}{2} \delta^{pa} \delta^{rd} g_L^2 (Y_u^\dagger Y_d)^{bc} - 7\delta^{pa} \delta^{rd} (Y_u^\dagger Y_d Y_d^\dagger Y_d)^{bc} - 7\delta^{pa} \delta^{rd} (Y_u^\dagger Y_u Y_u^\dagger Y_d)^{bc} \\
& - 32\delta^{pa} \delta^{rd} g_s^2 (Y_u^\dagger Y_d)^{bc} \left. \right\} \mathcal{C}_{ud}^{(II)abcd} + \left\{ g_Y^2 \left( \frac{47}{2} \delta^{pa} \delta^{rd} (Y_u^\dagger Y_d)^{bc} - \frac{34}{81} \delta^{pa} \delta^{cd} (Y_u^\dagger Y_d)^{br} - \frac{124}{81} \delta^{rd} \delta^{ab} (Y_u^\dagger Y_d)^{pc} \right) + g_s^2 \left( 176\delta^{pa} \delta^{rd} (Y_u^\dagger Y_d)^{bc} \right. \right. \\
& - \frac{112}{27} \delta^{rd} \delta^{ab} (Y_u^\dagger Y_d)^{pc} - \frac{112}{27} \delta^{pa} \delta^{cd} (Y_u^\dagger Y_d)^{br} \left. \right) + 6\delta^{pa} (Y_d^\dagger Y_d)^{dr} (Y_u^\dagger Y_d)^{bc} + 6\delta^{rd} (Y_u^\dagger Y_d)^{bc} (Y_u^\dagger Y_u)^{pa} + \frac{45}{2} \delta^{pa} \delta^{rd} g_L^2 (Y_u^\dagger Y_d)^{bc} - 21\delta^{pa} \delta^{rd} (Y_u^\dagger Y_d Y_d^\dagger Y_d)^{bc} \\
& - 21\delta^{pa} \delta^{rd} (Y_u^\dagger Y_u Y_u^\dagger Y_d)^{bc} \left. \right\} \mathcal{C}_{ud}^{(\times)abcd} - \frac{2}{3} Y_e^{*ab} \mathcal{C}_{ledq}^{abcd} Y_d^{dr} (Y_u^\dagger Y_d)^{pc} + \mathcal{C}_{ledq}^{*abcd} \left\{ \frac{1}{3} Y_u^{*dp} Y_e^{ab} (Y_d^\dagger Y_d)^{cr} + \frac{3}{4} \delta^{rc} g_L^2 Y_u^{*dp} Y_e^{ab} + \frac{3}{4} \delta^{rc} g_Y^2 Y_u^{*dp} Y_e^{ab} \right. \\
& - \delta^{rc} Y_e^{ab} (Y_u^\dagger Y_u Y_u^\dagger)^{dp} \left. \right\} + \left\{ \frac{1}{6} Y_u^{*ap} Y_u^{*cb} (Y_d^\dagger Y_d)^{dr} + g_Y^2 \left( \frac{13}{18} \delta^{rd} Y_u^{*ap} Y_u^{*cb} + \frac{9}{4} \delta^{rd} Y_u^{*ab} Y_u^{*cp} \right) + Y_u^{*ab} Y_u^{*cp} (Y_d^\dagger Y_d)^{dr} + \frac{9}{4} \delta^{rd} g_L^2 Y_u^{*ab} Y_u^{*cp} \right. \\
& + 3\delta^{rd} Y_u^{*ap} (Y_d^\dagger Y_d Y_u^\dagger)^{cb} + 3\delta^{rd} Y_u^{*ap} (Y_u^\dagger Y_u Y_u^\dagger)^{cb} + \frac{32}{3} \delta^{rd} g_s^2 Y_u^{*ap} Y_u^{*cb} - \frac{1}{3} Y_d^{*ad} Y_u^{*cp} (Y_u^\dagger Y_d)^{br} - \frac{1}{2} \delta^{rd} Y_u^{*cb} (Y_u^\dagger Y_u Y_u^\dagger)^{ap} - 2Y_d^{*cd} Y_u^{*ap} (Y_u^\dagger Y_d)^{br}
\end{aligned}$$



$$\begin{aligned}
& -3\delta^{rd}Y_u^{*ab}(Y_u^\dagger Y_u Y_u^\dagger)^{cp} - 9\delta^{rd}Y_u^{*cp}(Y_d^\dagger Y_d Y_u^\dagger)^{ab} \Big\} C_{quqd}^{(\parallel)abcd} + \left(C_{quqd}^{(\parallel)*}\right)^{abcd} \Big\{ \frac{1}{6}Y_d^{ad}Y_d^{cr}(Y_u^\dagger Y_u)^{pb} + Y_d^{ar}Y_d^{cd}(Y_u^\dagger Y_u)^{pb} + \frac{9}{4}\delta^{pb}g_L^2Y_d^{ar}Y_d^{cd} + 3\delta^{pb}Y_d^{cr}(Y_d Y_d^\dagger Y_d)^{ad} \\
& + 3\delta^{pb}Y_d^{cr}(Y_u Y_u^\dagger Y_d)^{ad} + \frac{32}{3}\delta^{pb}g_s^2Y_d^{ad}Y_d^{cr} - \frac{1}{3}Y_d^{ar}Y_u^{cb}(Y_u^\dagger Y_d)^{pd} - \frac{1}{2}\delta^{pb}Y_d^{ad}(Y_d Y_d^\dagger Y_d)^{cr} - g_Y^2\left(\frac{5}{18}\delta^{pb}Y_d^{ad}Y_d^{cr} + \frac{3}{4}\delta^{pb}Y_d^{ar}Y_d^{cd}\right) - 2Y_d^{cr}Y_u^{ab}(Y_u^\dagger Y_d)^{pd} \\
& - 3\delta^{pb}Y_d^{cd}(Y_d Y_d^\dagger Y_d)^{ar} - 9\delta^{pb}Y_d^{ar}(Y_u Y_u^\dagger Y_d)^{cd} \Big\} + \left\{ \frac{1}{3}Y_u^{*ab}Y_u^{*cp}(Y_d^\dagger Y_d)^{dr} + \frac{1}{2}Y_u^{*ap}Y_u^{*cb}(Y_d^\dagger Y_d)^{dr} + \frac{3}{4}\delta^{rd}g_L^2Y_u^{*ab}Y_u^{*cp} + g_Y^2\left(\frac{3}{4}\delta^{rd}Y_u^{*ab}Y_u^{*cp} \right. \right. \\
& + \left. \frac{13}{6}\delta^{rd}Y_u^{*ap}Y_u^{*cb}\right) + 9\delta^{rd}Y_u^{*ap}(Y_d^\dagger Y_d Y_u^\dagger)^{cb} + 9\delta^{rd}Y_u^{*ap}(Y_u^\dagger Y_u Y_u^\dagger)^{cb} - \frac{2}{3}Y_d^{*cd}Y_u^{*ap}(Y_u^\dagger Y_d)^{br} - Y_d^{*ad}Y_u^{*cp}(Y_u^\dagger Y_d)^{br} - \delta^{rd}Y_u^{*ab}(Y_u^\dagger Y_u Y_u^\dagger)^{cp} \\
& - \frac{3}{2}\delta^{rd}Y_u^{*cb}(Y_u^\dagger Y_u Y_u^\dagger)^{ap} - 3\delta^{rd}Y_u^{*cp}(Y_d^\dagger Y_d Y_u^\dagger)^{ab} \Big\} C_{quqd}^{(\times)abcd} + \left(C_{quqd}^{(\times)*}\right)^{abcd} \Big\{ \frac{1}{3}Y_d^{ar}Y_d^{cd}(Y_u^\dagger Y_u)^{pb} + \frac{1}{2}Y_d^{ad}Y_d^{cr}(Y_u^\dagger Y_u)^{pb} + \frac{3}{4}\delta^{pb}g_L^2Y_d^{ar}Y_d^{cd} \\
& + 9\delta^{pb}Y_d^{cr}(Y_d Y_d^\dagger Y_d)^{ad} + 9\delta^{pb}Y_d^{cr}(Y_u Y_u^\dagger Y_d)^{ad} - \frac{2}{3}Y_d^{cr}Y_u^{ab}(Y_u^\dagger Y_d)^{pd} - g_Y^2\left(\frac{1}{4}\delta^{pb}Y_d^{ar}Y_d^{cd} + \frac{5}{6}\delta^{pb}Y_d^{ad}Y_d^{cr}\right) - Y_d^{ar}Y_u^{cb}(Y_u^\dagger Y_d)^{pd} - \delta^{pb}Y_d^{cd}(Y_d Y_d^\dagger Y_d)^{ar} \\
& - \frac{3}{2}\delta^{pb}Y_d^{ad}(Y_d Y_d^\dagger Y_d)^{cr} - 3\delta^{pb}Y_d^{ar}(Y_u Y_u^\dagger Y_d)^{cd} \Big\} + \frac{2}{3}Y_e^{*ab}Y_u^{*cp}C_{lequ}^{abcd}(Y_u^\dagger Y_d)^{dr} + C_{lequ}^{*abcd} \Big\{ \frac{1}{4}\delta^{pd}g_Y^2Y_d^{cr}Y_e^{ab} + \delta^{pd}Y_e^{ab}(Y_d Y_d^\dagger Y_d)^{cr} - \frac{1}{3}Y_d^{cr}Y_e^{ab}(Y_u^\dagger Y_u)^{pd} \\
& - \frac{3}{4}\delta^{pd}g_L^2Y_d^{cr}Y_e^{ab} \Big\} - \frac{1}{3}Y_e^{*ad}Y_u^{*cp}C_{luqe}^{abcd}(Y_u^\dagger Y_d)^{br} + C_{luqe}^{*abcd} \Big\{ \frac{1}{6}Y_d^{cr}Y_e^{ad}(Y_u^\dagger Y_u)^{pb} + 3\delta^{pb}Y_d^{cr}(Y_e Y_e^\dagger Y_e)^{ad} - \frac{1}{2}\delta^{pb}Y_e^{ad}(Y_d Y_d^\dagger Y_d)^{cr} - \frac{3}{2}\delta^{pb}g_Y^2Y_d^{cr}Y_e^{ad} \Big\} \\
& + \left\{ \frac{2}{3}\delta^{bc}g_L^2Y_u^{*ap}Y_d^{dr} + g_Y^2\left(\frac{8}{81}\delta^{bc}Y_u^{*ap}Y_d^{dr} + \frac{16}{27}\delta^{cd}Y_u^{*ap}Y_d^{br}\right) + \frac{128}{27}\delta^{bc}g_s^2Y_u^{*ap}Y_d^{dr} - 6Y_u^{*cp}Y_d^{br}(Y_d Y_d^\dagger)^{da} - 6Y_u^{*ap}Y_d^{dr}(Y_u Y_u^\dagger)^{bc} \right\} C_{qq}^{(\parallel)abcd} \\
& + \left\{ g_Y^2\left(\frac{16}{81}\delta^{bc}Y_u^{*ap}Y_d^{dr} + \frac{8}{27}\delta^{cd}Y_u^{*ap}Y_d^{br}\right) + 2\delta^{cd}g_L^2Y_u^{*ap}Y_d^{br} + \frac{256}{27}\delta^{bc}g_s^2Y_u^{*ap}Y_d^{dr} - 18Y_u^{*cp}Y_d^{dr}(Y_d Y_d^\dagger)^{ba} - 18Y_u^{*ap}Y_d^{br}(Y_u Y_u^\dagger)^{dc} \right\} C_{qq}^{(\times)abcd} \\
& - \frac{8}{27}\delta^{ab}g_Y^2Y_u^{*cp}C_{\ell q}^{(\parallel)abcd}Y_d^{dr} + \left\{ \frac{1}{3}\delta^{ab}g_L^2Y_u^{*cp}Y_d^{dr} - \frac{4}{27}\delta^{ab}g_Y^2Y_u^{*cp}Y_d^{dr} - 3Y_u^{*cp}Y_d^{dr}(Y_e Y_e^\dagger)^{ba} \right\} C_{\ell q}^{(\times)abcd}, \tag{9.16}
\end{aligned}$$

## 10 $(\bar{L}L)(\bar{R}R)$

### 10.1 $C_{\ell e}$

$$\begin{aligned}
\beta_{C_{\ell e}^{prst}}^{(1)} &= \left\{ 2\delta^{pa}\delta^{rb}(Y_e^\dagger Y_e)^{st} - \frac{2}{3}\delta^{pa}\delta^{rb}\delta^{st}g_Y^2 \right\} C_{H\ell}^{(\parallel)ab} + \left\{ \delta^{pa}\delta^{rb}(Y_e^\dagger Y_e)^{st} - \frac{1}{3}\delta^{pa}\delta^{rb}\delta^{st}g_Y^2 \right\} C_{H\ell}^{(\times)ab} - \left\{ \frac{1}{3}\delta^{pr}\delta^{sa}\delta^{tb}g_Y^2 + \delta^{sa}\delta^{tb}(Y_e Y_e^\dagger)^{pr} \right\} C_{He}^{ab} \\
&+ \left\{ \frac{1}{2}\left(\delta^{rb}\delta^{sc}\delta^{td}(Y_e Y_e^\dagger)^{pa} + \delta^{pa}\delta^{sc}\delta^{td}(Y_e Y_e^\dagger)^{br} + 2\delta^{pa}\delta^{sc}Y_e^{*rd}Y_e^{bt} + 2\delta^{rb}\delta^{td}Y_e^{*as}Y_e^{pc} + 2\delta^{pa}\delta^{rb}\delta^{td}(Y_e^\dagger Y_e)^{sc} + 2\delta^{pa}\delta^{rb}\delta^{sc}(Y_e^\dagger Y_e)^{dt} \right. \right.
\end{aligned}$$

$$\begin{aligned}
& + 4\delta^{rb}\delta^{sc}Y_e^{*ad}Y_e^{pt} + 4\delta^{pa}\delta^{td}Y_e^{*rs}Y_e^{bc} \Big) - \frac{2}{3}g_Y^2 \Big( 9\delta^{pa}\delta^{rb}\delta^{sc}\delta^{td} - \delta^{pr}\delta^{sc}\delta^{td}\delta^{ab} - 2\delta^{pa}\delta^{rb}\delta^{st}\delta^{cd} \Big) \Big\} C_{\ell e}^{abcd} - \frac{8}{3}\delta^{pa}\delta^{rb}\delta^{st}\delta^{cd}g_Y^2 C_{\ell u}^{abcd} \\
& + \frac{4}{3}\delta^{pa}\delta^{rb}\delta^{st}\delta^{cd}g_Y^2 C_{\ell d}^{abcd} - \frac{2}{3}\delta^{pr}\delta^{sc}\delta^{td}\delta^{ab}g_Y^2 C_{qe}^{abcd} + \left\{ \frac{8}{3}\delta^{pr}\delta^{sa}\delta^{tb}\delta^{cd}g_Y^2 - 4\delta^{sa}\delta^{tb}Y_e^{*rd}Y_e^{pc} \right\} C_{ee}^{abcd} - \frac{4}{3}\delta^{pr}\delta^{sa}\delta^{tb}\delta^{cd}g_Y^2 C_{eu}^{abcd} \\
& + \frac{2}{3}\delta^{pr}\delta^{sa}\delta^{tb}\delta^{cd}g_Y^2 C_{ed}^{abcd} - 3\delta^{pa}\delta^{tb}Y_e^{*rs}C_{\ell edq}^{abcd}Y_d^{dc} - 3\delta^{ra}\delta^{sb}C_{\ell edq}^{*abcd}Y_d^{dc}Y_e^{pt} + 3\delta^{pa}\delta^{tb}Y_e^{*rs}Y_u^{*cd}C_{\ell equ}^{abcd} + 3\delta^{ra}\delta^{sb}C_{\ell equ}^{*abcd}Y_e^{pt}Y_u^{cd} \\
& - \frac{3}{2}\delta^{pa}\delta^{td}Y_e^{*rs}Y_u^{*cb}C_{\ell uqe}^{abcd} - \frac{3}{2}\delta^{ra}\delta^{sd}C_{\ell uqe}^{*abcd}Y_e^{pt}Y_u^{cb} + \left\{ \frac{4}{3}g_Y^2 \Big( \delta^{pa}\delta^{rd}\delta^{st}\delta^{bc} + 2\delta^{pa}\delta^{rb}\delta^{st}\delta^{cd} \Big) - 2 \Big( \delta^{pa}\delta^{rd}Y_e^{*cs}Y_e^{bt} + 2\delta^{pa}\delta^{rb}Y_e^{*cs}Y_e^{dt} \Big) \right\} C_{\ell\ell}^{abcd} \\
& - \frac{4}{3}\delta^{pa}\delta^{rb}\delta^{st}\delta^{cd}g_Y^2 C_{\ell q}^{(\parallel)abcd} - \frac{2}{3}\delta^{pa}\delta^{rb}\delta^{st}\delta^{cd}g_Y^2 C_{\ell q}^{(\times)abcd}, \tag{10.1}
\end{aligned}$$

$$\begin{aligned}
\beta_{C_{\ell e}^{prst}}^{(2)} &= 2Y_e^{*rs}Y_e^{pt}\mathbf{T}_{\ell H} + 3(Y_e^\dagger Y_e)^{st}(C_{\ell HH}C_{\ell HH}^\dagger)^{rp} + \frac{11}{3}\delta^{st}g_Y^2(C_{\ell HH}C_{\ell HH}^\dagger)^{rp} - 3Y_e^{*rs}(C_{\ell HH}^\dagger C_{\ell HH}Y_e)^{pt} - 3Y_e^{pt}(C_{\ell HH}C_{\ell HH}^\dagger Y_e^\dagger)^{rs} \\
& - 17(C_{\ell HH}^\dagger Y_e^\dagger)^{ps}(C_{\ell HH}Y_e)^{rt} + \left\{ \frac{3}{4}Y_e^{pt}(Y_e^\dagger Y_e Y_e^\dagger)^{rs} + \frac{3}{4}Y_e^{*rs}(Y_e Y_e^\dagger Y_e)^{pt} - \frac{1}{36}g_Y^2 Y_e^{*rs}Y_e^{pt} - \frac{1}{12}g_L^2 Y_e^{*rs}Y_e^{pt} - \frac{1}{2}\lambda Y_e^{*rs}Y_e^{pt} \right\} C_{HD}^{(\parallel)} \\
& + \left\{ \frac{3}{4}Y_e^{pt}(Y_e^\dagger Y_e Y_e^\dagger)^{rs} + \frac{3}{4}Y_e^{*rs}(Y_e Y_e^\dagger Y_e)^{pt} - \frac{1}{18}g_Y^2 Y_e^{*rs}Y_e^{pt} - \frac{1}{2}\lambda Y_e^{*rs}Y_e^{pt} \right\} C_{HD}^{(\times)} + \left\{ g_Y^4 \Big( 9Y_e^{*rs}Y_e^{pt} - \delta^{st}(Y_e Y_e^\dagger)^{pr} - 5\delta^{pr}(Y_e^\dagger Y_e)^{st} \Big) \right. \\
& + \frac{4}{3}\delta^{pr}\delta^{st}g_Y^6 \Big\} C_{HB} + 3g_L^4 C_{HW}Y_e^{*rs}Y_e^{pt} + \left\{ \delta^{pr}\delta^{st}g_Y^4 g_L^2 + g_Y^2 g_L^2 \Big( \frac{9}{4}\delta^{st}(Y_e Y_e^\dagger)^{pr} - \frac{3}{4}\delta^{pr}(Y_e^\dagger Y_e)^{st} - \frac{9}{2}Y_e^{*rs}Y_e^{pt} \Big) \right\} C_{HWB} + \left\{ 10\delta^{pr}\delta^{st}g_Y^2 g_L^6 \right. \\
& - \frac{21}{2}g_L^6 Y_e^{*rs}Y_e^{pt} \Big\} C_W + \left\{ 3\delta^{pa}\delta^{tb}(Y_e^\dagger Y_e Y_e^\dagger)^{rs} - \frac{3}{2}\delta^{pa}\delta^{tb}\lambda Y_e^{*rs} \right\} C_{eH}^{ab} + C_{eH}^{*ab} \left\{ 3\delta^{ra}\delta^{sb}(Y_e Y_e^\dagger)^{pt} - \frac{3}{2}\delta^{ra}\delta^{sb}\lambda Y_e^{pt} \right\} + \left\{ g_Y^4 \Big( \delta^{pr}\delta^{tb}Y_e^{*as} \right. \right. \\
& - 2\delta^{pr}\delta^{st}Y_e^{*ab} - \frac{9}{2}\delta^{pa}\delta^{st}Y_e^{*rb} - \frac{441}{8}\delta^{pa}\delta^{tb}Y_e^{*rs} \Big) + g_Y^2 \Big( \delta^{pr}Y_e^{*as}(Y_e^\dagger Y_e)^{bt} + \frac{3}{2}\delta^{pa}Y_e^{*rb}(Y_e^\dagger Y_e)^{st} + 2\delta^{st}Y_e^{*rb}(Y_e Y_e^\dagger)^{pa} + 3Y_e^{*rs}Y_e^{*ab}Y_e^{pt} \\
& + 3\delta^{tb}Y_e^{*as}(Y_e Y_e^\dagger)^{pr} - \frac{3}{2}\delta^{pa}Y_e^{*rs}(Y_e^\dagger Y_e)^{bt} - 3\delta^{tb}Y_e^{*rs}(Y_e Y_e^\dagger)^{pa} - 12\delta^{pa}\delta^{tb}Y_e^{*rs}\text{Tr}[Y_d^\dagger Y_d] - \frac{27}{2}\delta^{pa}\delta^{tb}Y_e^{*rs}\text{Tr}[Y_u^\dagger Y_u] \Big) \\
& + \frac{39}{8}\delta^{pa}\delta^{tb}g_Y^2 g_L^2 Y_e^{*rs} \Big\} C_{eB}^{ab} + C_{eB}^{*ab} \left\{ g_Y^4 \Big( \delta^{pr}\delta^{sb}Y_e^{at} - 2\delta^{pr}\delta^{st}Y_e^{ab} - \frac{9}{2}\delta^{ra}\delta^{st}Y_e^{pb} - \frac{441}{8}\delta^{ra}\delta^{sb}Y_e^{pt} \Big) + g_Y^2 \Big( \delta^{pr}Y_e^{at}(Y_e^\dagger Y_e)^{sb} + \frac{3}{2}\delta^{ra}Y_e^{pb}(Y_e^\dagger Y_e)^{st} \right. \right. \\
& + 2\delta^{st}Y_e^{pb}(Y_e Y_e^\dagger)^{ar} + 3Y_e^{*rs}Y_e^{pt}Y_e^{ab} + 3\delta^{sb}Y_e^{at}(Y_e Y_e^\dagger)^{pr} - \frac{3}{2}\delta^{ra}Y_e^{pt}(Y_e^\dagger Y_e)^{sb} - 3\delta^{sb}Y_e^{pt}(Y_e Y_e^\dagger)^{ar} - 12\delta^{ra}\delta^{sb}Y_e^{pt}\text{Tr}[Y_d^\dagger Y_d] - \frac{27}{2}\delta^{ra}\delta^{sb}Y_e^{pt}\text{Tr}[Y_u^\dagger Y_u] \Big) \\
& + \frac{39}{8}\delta^{ra}\delta^{sb}g_Y^2 g_L^2 Y_e^{pt} \Big\} + \left\{ g_L^4 \Big( \frac{9}{2}\delta^{pr}\delta^{tb}Y_e^{*as} - \frac{69}{16}\delta^{pa}\delta^{tb}Y_e^{*rs} \Big) + g_Y^2 g_L^2 \Big( \frac{75}{16}\delta^{pa}\delta^{tb}Y_e^{*rs} - \frac{5}{4}\delta^{pa}\delta^{st}Y_e^{*rb} - \frac{5}{2}\delta^{pr}\delta^{tb}Y_e^{*as} \Big) + g_L^2 \Big( \frac{3}{4}\delta^{pa}Y_e^{*rs}(Y_e^\dagger Y_e)^{bt} \right. \right.
\end{aligned}$$

$$\begin{aligned}
& + \frac{27}{4} \delta^{pa} \delta^{tb} Y_e^{*rs} \text{Tr}[Y_u^\dagger Y_u] - \frac{3}{2} Y_e^{*rs} Y_e^{*ab} Y_e^{pt} - \frac{9}{4} \delta^{pa} Y_e^{*rb} (Y_e^\dagger Y_e)^{st} \Big\} C_{eW}^{ab} + C_{eW}^{*ab} \Big\{ g_L^4 \left( \frac{9}{2} \delta^{pr} \delta^{sb} Y_e^{at} - \frac{69}{16} \delta^{ra} \delta^{sb} Y_e^{pt} \right) + g_Y^2 g_L^2 \left( \frac{75}{16} \delta^{ra} \delta^{sb} Y_e^{pt} \right. \\
& - \frac{5}{4} \delta^{ra} \delta^{st} Y_e^{pb} - \frac{5}{2} \delta^{pr} \delta^{sb} Y_e^{at} \Big) + g_L^2 \left( \frac{3}{4} \delta^{ra} Y_e^{pt} (Y_e^\dagger Y_e)^{sb} + \frac{27}{4} \delta^{ra} \delta^{sb} Y_e^{pt} \text{Tr}[Y_u^\dagger Y_u] - \frac{3}{2} Y_e^{*rs} Y_e^{pt} Y_e^{ab} - \frac{9}{4} \delta^{ra} Y_e^{pb} (Y_e^\dagger Y_e)^{st} \right) \Big\} + \Big\{ \frac{5}{2} g_Y^2 Y_e^{*rs} Y_u^{*ab} Y_e^{pt} \\
& + \frac{10}{3} \delta^{pr} \delta^{st} g_Y^4 Y_u^{*ab} \Big\} C_{uB}^{ab} + C_{uB}^{*ab} \Big\{ \frac{5}{2} g_Y^2 Y_e^{*rs} Y_e^{pt} Y_u^{ab} + \frac{10}{3} \delta^{pr} \delta^{st} g_Y^4 Y_u^{ab} \Big\} + \frac{9}{4} g_L^2 Y_e^{*rs} Y_u^{*ab} C_{uW}^{ab} Y_e^{pt} + \frac{9}{4} g_L^2 C_{uW}^{*ab} Y_e^{*rs} Y_e^{pt} Y_u^{ab} \\
& + 8 g_s^2 Y_e^{*rs} Y_u^{*ab} C_{uG}^{ab} Y_e^{pt} + 8 g_s^2 C_{uG}^{*ab} Y_e^{*rs} Y_e^{pt} Y_u^{ab} + \Big\{ 13 g_Y^2 Y_d^{*ab} Y_e^{*rs} Y_e^{pt} - \frac{2}{3} \delta^{pr} \delta^{st} g_Y^4 Y_d^{*ab} \Big\} C_{dB}^{ab} + C_{dB}^{*ab} \Big\{ 13 g_Y^2 Y_e^{*rs} Y_d^{*ab} Y_e^{pt} \\
& - \frac{2}{3} \delta^{pr} \delta^{st} g_Y^4 Y_d^{*ab} \Big\} - \frac{9}{2} g_L^2 Y_d^{*ab} Y_e^{*rs} C_{dW}^{ab} Y_e^{pt} - \frac{9}{2} g_L^2 C_{dW}^{*ab} Y_e^{*rs} Y_d^{*ab} Y_e^{pt} + 8 g_s^2 Y_d^{*ab} Y_e^{*rs} C_{dG}^{ab} Y_e^{pt} + 8 g_s^2 C_{dG}^{*ab} Y_e^{*rs} Y_d^{*ab} Y_e^{pt} \\
& + \Big\{ \frac{1}{4} \delta^{rb} (Y_e^\dagger Y_e)^{st} (Y_e Y_e^\dagger)^{pa} + \frac{1}{4} \delta^{pa} (Y_e^\dagger Y_e)^{st} (Y_e Y_e^\dagger)^{br} + \frac{2}{3} Y_e^{*rs} Y_e^{pt} (Y_e Y_e^\dagger)^{ba} + g_L^2 \left( \frac{51}{4} \delta^{pa} \delta^{rb} (Y_e^\dagger Y_e)^{st} - \frac{15}{8} \delta^{pa} Y_e^{*rs} Y_e^{bt} - \frac{15}{8} \delta^{rb} Y_e^{*as} Y_e^{pt} \right) \\
& + g_Y^2 \left( \frac{2}{9} \delta^{ab} Y_e^{*rs} Y_e^{pt} + \frac{2}{3} T_2 \delta^{pa} \delta^{rb} \delta^{st} + \frac{67}{72} \delta^{pa} Y_e^{*rs} Y_e^{bt} + \frac{67}{72} \delta^{rb} Y_e^{*as} Y_e^{pt} + \frac{53}{4} \delta^{pa} \delta^{rb} (Y_e^\dagger Y_e)^{st} - \frac{1}{36} \delta^{rb} \delta^{st} (Y_e Y_e^\dagger)^{pa} - \frac{1}{36} \delta^{pa} \delta^{st} (Y_e Y_e^\dagger)^{br} \right) \\
& - \frac{3}{4} \delta^{pa} Y_e^{bt} (Y_e^\dagger Y_e Y_e^\dagger)^{rs} - \frac{3}{4} \delta^{rb} Y_e^{*as} (Y_e Y_e^\dagger Y_e)^{pt} - Y_e^{*rs} Y_e^{bt} (Y_e Y_e^\dagger)^{pa} - Y_e^{*as} Y_e^{pt} (Y_e Y_e^\dagger)^{br} - 2 T_2 \delta^{pa} \delta^{rb} (Y_e^\dagger Y_e)^{st} - 3 \delta^{rb} Y_e^{pt} (Y_e^\dagger Y_e Y_e^\dagger)^{as} \\
& - 3 \delta^{pa} Y_e^{*rs} (Y_e Y_e^\dagger Y_e)^{bt} - 3 \delta^{pa} \delta^{rb} (Y_e^\dagger Y_e Y_e^\dagger Y_e)^{st} - 6 \delta^{pa} \delta^{rb} \delta^{st} g_Y^2 g_L^2 - \frac{184}{27} \delta^{pa} \delta^{rb} \delta^{st} g_Y^4 \Big\} C_{H\ell}^{(\parallel)ab} + \Big\{ \frac{1}{2} \delta^{rb} (Y_e^\dagger Y_e)^{st} (Y_e Y_e^\dagger)^{pa} \\
& + \frac{1}{2} \delta^{pa} (Y_e^\dagger Y_e)^{st} (Y_e Y_e^\dagger)^{br} + g_L^2 \left( \frac{1}{6} \delta^{pr} Y_e^{*as} Y_e^{bt} + \frac{7}{12} \delta^{pa} Y_e^{*rs} Y_e^{bt} + \frac{7}{12} \delta^{rb} Y_e^{*as} Y_e^{pt} + \frac{265}{24} \delta^{pa} \delta^{rb} (Y_e^\dagger Y_e)^{st} - \frac{1}{3} \delta^{ab} Y_e^{*rs} Y_e^{pt} \right) + g_Y^2 \left( \frac{1}{9} \delta^{ab} Y_e^{*rs} Y_e^{pt} \right. \\
& + \frac{5}{18} \delta^{pa} Y_e^{*rs} Y_e^{bt} + \frac{5}{18} \delta^{rb} Y_e^{*as} Y_e^{pt} + \frac{1}{3} \delta^{st} \delta^{ab} (Y_e Y_e^\dagger)^{pr} + \frac{2}{3} \delta^{pa} \delta^{rb} \delta^{st} \text{Tr}[Y_e^\dagger Y_e] + \delta^{pa} \delta^{rb} \delta^{st} \text{Tr}[Y_d^\dagger Y_d] + \delta^{pa} \delta^{rb} \delta^{st} \text{Tr}[Y_u^\dagger Y_u] + \frac{53}{8} \delta^{pa} \delta^{rb} (Y_e^\dagger Y_e)^{st} \\
& - \frac{13}{18} \delta^{rb} \delta^{st} (Y_e Y_e^\dagger)^{pa} - \frac{13}{18} \delta^{pa} \delta^{st} (Y_e Y_e^\dagger)^{br} \Big) + \frac{4}{3} Y_e^{*rs} Y_e^{pt} (Y_e Y_e^\dagger)^{ba} - \frac{1}{2} Y_e^{*as} Y_e^{bt} (Y_e Y_e^\dagger)^{pr} - \frac{1}{2} Y_e^{*rs} Y_e^{bt} (Y_e Y_e^\dagger)^{pa} - \frac{1}{2} Y_e^{*as} Y_e^{pt} (Y_e Y_e^\dagger)^{br} \\
& - g_Y^2 g_L^2 \left( \frac{1}{9} \delta^{pr} \delta^{st} \delta^{ab} + \frac{25}{6} \delta^{pa} \delta^{rb} \delta^{st} \right) - T_2 \delta^{pa} \delta^{rb} (Y_e^\dagger Y_e)^{st} - \frac{5}{4} \delta^{pa} Y_e^{bt} (Y_e^\dagger Y_e Y_e^\dagger)^{rs} - \frac{5}{4} \delta^{rb} Y_e^{*as} (Y_e Y_e^\dagger Y_e)^{pt} - \frac{3}{2} \delta^{rb} Y_e^{pt} (Y_e^\dagger Y_e Y_e^\dagger)^{as} \\
& - \frac{3}{2} \delta^{pa} Y_e^{*rs} (Y_e Y_e^\dagger Y_e)^{bt} - 2 \delta^{pa} \delta^{rb} (Y_e^\dagger Y_e Y_e^\dagger Y_e)^{st} - \frac{92}{27} \delta^{pa} \delta^{rb} \delta^{st} g_Y^4 \Big\} C_{H\ell}^{(\times)ab} + \Big\{ \frac{1}{2} Y_e^{*rb} Y_e^{pa} (Y_e^\dagger Y_e)^{st} + \frac{1}{2} Y_e^{*rb} Y_e^{pt} (Y_e^\dagger Y_e)^{sa} + \frac{1}{2} Y_e^{*rs} Y_e^{pa} (Y_e^\dagger Y_e)^{bt} \\
& + g_Y^4 \left( \frac{1}{9} \delta^{pr} \delta^{st} \delta^{ab} - \frac{109}{54} \delta^{pr} \delta^{sa} \delta^{tb} \right) + T_2 \delta^{sa} \delta^{tb} (Y_e Y_e^\dagger)^{pr} + g_Y^2 \left( \frac{2}{9} \delta^{ab} Y_e^{*rs} Y_e^{pt} + \delta^{pr} \delta^{sa} \delta^{tb} \text{Tr}[Y_d^\dagger Y_d] + \delta^{pr} \delta^{sa} \delta^{tb} \text{Tr}[Y_u^\dagger Y_u] + \frac{155}{72} \delta^{sa} Y_e^{*rb} Y_e^{pt} \right. \\
& + \frac{155}{72} \delta^{tb} Y_e^{*rs} Y_e^{pa} - \frac{1}{6} \delta^{st} Y_e^{*rb} Y_e^{pa} - \frac{1}{3} \delta^{pr} \delta^{ab} (Y_e^\dagger Y_e)^{st} - \frac{31}{36} \delta^{pr} \delta^{tb} (Y_e^\dagger Y_e)^{sa} - \frac{31}{36} \delta^{pr} \delta^{sa} (Y_e^\dagger Y_e)^{bt} - \frac{325}{24} \delta^{sa} \delta^{tb} (Y_e Y_e^\dagger)^{pr} \Big) + \frac{3}{2} \delta^{sa} Y_e^{pt} (Y_e^\dagger Y_e Y_e^\dagger)^{rb}
\end{aligned}$$

$$\begin{aligned}
& + \frac{3}{2} \delta^{tb} Y_e^{*rs} (Y_e Y_e^\dagger Y_e)^{pa} + \frac{7}{4} \delta^{tb} Y_e^{pa} (Y_e^\dagger Y_e Y_e^\dagger)^{rs} + \frac{7}{4} \delta^{sa} Y_e^{*rb} (Y_e Y_e^\dagger Y_e)^{pt} + \frac{7}{2} \delta^{sa} \delta^{tb} (Y_e Y_e^\dagger Y_e Y_e^\dagger)^{pr} - \frac{1}{4} \delta^{tb} (Y_e^\dagger Y_e)^{sa} (Y_e Y_e^\dagger)^{pr} - \frac{1}{4} \delta^{sa} (Y_e^\dagger Y_e)^{bt} (Y_e Y_e^\dagger)^{pr} \\
& - \frac{2}{3} Y_e^{*rs} Y_e^{pt} (Y_e^\dagger Y_e)^{ba} - g_L^2 \left( \frac{3}{8} \delta^{sa} Y_e^{*rb} Y_e^{pt} + \frac{3}{8} \delta^{tb} Y_e^{*rs} Y_e^{pa} + \frac{33}{8} \delta^{sa} \delta^{tb} (Y_e Y_e^\dagger)^{pr} \right) - 3 \delta^{pr} \delta^{sa} \delta^{tb} g_Y^2 g_L^2 \left\} C_{He}^{ab} + \left\{ 2 Y_e^{*rs} Y_e^{pt} (Y_d Y_d^\dagger)^{ba} \right. \right. \\
& - \frac{2}{9} \delta^{ab} g_Y^2 Y_e^{*rs} Y_e^{pt} - 2 Y_e^{*rs} Y_e^{pt} (Y_u Y_u^\dagger)^{ba} \left. \right\} C_{Hq}^{(\parallel)ab} + \left\{ 2 Y_e^{*rs} Y_e^{pt} (Y_u Y_u^\dagger)^{ba} + 4 Y_e^{*rs} Y_e^{pt} (Y_d Y_d^\dagger)^{ba} - \frac{1}{9} \delta^{ab} g_Y^2 Y_e^{*rs} Y_e^{pt} - \delta^{ab} g_L^2 Y_e^{*rs} Y_e^{pt} \right\} C_{Hq}^{(\times)ab} \\
& + \left\{ 2 Y_e^{*rs} Y_e^{pt} (Y_u^\dagger Y_u)^{ba} - \frac{4}{9} \delta^{ab} g_Y^2 Y_e^{*rs} Y_e^{pt} \right\} C_{Hu}^{ab} + \left\{ \frac{2}{9} \delta^{ab} g_Y^2 Y_e^{*rs} Y_e^{pt} - 2 Y_e^{*rs} Y_e^{pt} (Y_d^\dagger Y_d)^{ba} \right\} C_{Hd}^{ab} - 2 Y_e^{*rs} C_{Hud}^{ab} Y_e^{pt} (Y_d^\dagger Y_u)^{ba} \\
& - 2 C_{Hud}^{*ab} Y_e^{*rs} Y_e^{pt} (Y_u^\dagger Y_d)^{ab} + \left\{ \frac{1}{4} \delta^{rb} \delta^{td} Y_e^{pc} (Y_e^\dagger Y_e Y_e^\dagger)^{as} + \frac{1}{4} \delta^{pa} \delta^{sc} Y_e^{*rd} (Y_e Y_e^\dagger Y_e)^{bt} + \frac{1}{2} T_2 \delta^{pa} \delta^{sc} Y_e^{*rd} Y_e^{bt} + \frac{1}{2} T_2 \delta^{rb} \delta^{td} Y_e^{*as} Y_e^{pc} \right. \\
& + \frac{1}{2} \delta^{sc} \delta^{td} (Y_e Y_e^\dagger)^{pr} (Y_e Y_e^\dagger)^{ba} + \frac{1}{2} \delta^{pa} \delta^{sc} Y_e^{bt} (Y_e^\dagger Y_e Y_e^\dagger)^{rd} + \frac{1}{2} \delta^{rb} \delta^{td} Y_e^{*as} (Y_e Y_e^\dagger Y_e)^{pc} + g_Y^2 g_L^2 \left( \frac{3}{2} \delta^{pr} \delta^{sc} \delta^{td} \delta^{ab} + \frac{27}{2} \delta^{pa} \delta^{rb} \delta^{sc} \delta^{td} \right) \\
& + g_Y^4 \left( \frac{398}{27} \delta^{pa} \delta^{rb} \delta^{st} \delta^{cd} + \frac{529}{6} \delta^{pa} \delta^{rb} \delta^{sc} \delta^{td} - \frac{2}{9} \delta^{pr} \delta^{st} \delta^{ab} \delta^{cd} - \frac{20}{27} \delta^{pr} \delta^{sc} \delta^{td} \delta^{ab} \right) + \delta^{pa} Y_e^{*rd} Y_e^{bc} (Y_e^\dagger Y_e)^{st} + \delta^{rb} Y_e^{*ad} Y_e^{pc} (Y_e^\dagger Y_e)^{st} \\
& + \delta^{pa} \delta^{rb} (Y_e^\dagger Y_e)^{st} (Y_e^\dagger Y_e)^{dc} + \delta^{sc} Y_e^{*ad} Y_e^{bt} (Y_e Y_e^\dagger)^{pr} + \delta^{td} Y_e^{*as} Y_e^{bc} (Y_e Y_e^\dagger)^{pr} + g_L^2 \left( \frac{15}{8} \delta^{pa} \delta^{sc} Y_e^{*rd} Y_e^{bt} + \frac{15}{8} \delta^{rb} \delta^{td} Y_e^{*as} Y_e^{pc} + \frac{33}{16} \delta^{rb} \delta^{sc} \delta^{td} (Y_e Y_e^\dagger)^{pa} \right. \\
& + \frac{33}{16} \delta^{pa} \delta^{sc} \delta^{td} (Y_e Y_e^\dagger)^{br} + 3 \delta^{rb} \delta^{sc} Y_e^{*ad} Y_e^{pt} + 3 \delta^{pa} \delta^{td} Y_e^{*rs} Y_e^{bc} + \frac{51}{8} \delta^{pa} \delta^{rb} \delta^{td} (Y_e^\dagger Y_e)^{sc} + \frac{51}{8} \delta^{pa} \delta^{rb} \delta^{sc} (Y_e^\dagger Y_e)^{dt} \Big) + g_Y^2 \left( \frac{1}{3} \delta^{st} \delta^{ab} Y_e^{*rd} Y_e^{pc} \right. \\
& + \frac{1}{3} \delta^{pr} \delta^{cd} Y_e^{*as} Y_e^{bt} + \frac{1}{3} \delta^{sc} \delta^{td} \delta^{ab} (Y_e Y_e^\dagger)^{pr} + \frac{7}{9} \delta^{sc} \delta^{ab} Y_e^{*rd} Y_e^{pt} + \frac{7}{9} \delta^{td} \delta^{ab} Y_e^{*rs} Y_e^{pc} + \frac{13}{8} \delta^{pa} \delta^{rb} \delta^{td} (Y_e^\dagger Y_e)^{sc} + \frac{13}{8} \delta^{pa} \delta^{rb} \delta^{sc} (Y_e^\dagger Y_e)^{dt} \\
& + \frac{103}{16} \delta^{rb} \delta^{sc} \delta^{td} (Y_e Y_e^\dagger)^{pa} + \frac{103}{16} \delta^{pa} \delta^{sc} \delta^{td} (Y_e Y_e^\dagger)^{br} + 9 \delta^{rb} \delta^{sc} Y_e^{*ad} Y_e^{pt} + 9 \delta^{pa} \delta^{td} Y_e^{*rs} Y_e^{bc} - \frac{4}{9} \delta^{pa} \delta^{cd} Y_e^{*rs} Y_e^{bt} - \frac{4}{9} \delta^{rb} \delta^{cd} Y_e^{*as} Y_e^{pt} \\
& - \frac{5}{9} \delta^{pr} \delta^{sc} Y_e^{*ad} Y_e^{bt} - \frac{5}{9} \delta^{pr} \delta^{td} Y_e^{*as} Y_e^{bc} - \delta^{pr} \delta^{sc} \delta^{td} (Y_e Y_e^\dagger)^{ba} - \frac{10}{9} \delta^{pa} \delta^{st} Y_e^{*rd} Y_e^{bc} - \frac{10}{9} \delta^{rb} \delta^{st} Y_e^{*ad} Y_e^{pc} - \frac{11}{8} \delta^{pa} \delta^{sc} Y_e^{*rd} Y_e^{bt} - \frac{11}{8} \delta^{rb} \delta^{td} Y_e^{*as} Y_e^{pc} \\
& - \frac{10}{3} \delta^{pa} \delta^{rb} \delta^{st} (Y_e^\dagger Y_e)^{dc} \Big) + 2 \delta^{rb} \delta^{sc} (Y_e^\dagger Y_e)^{dt} (Y_e Y_e^\dagger)^{pa} + 2 \delta^{pa} \delta^{td} (Y_e^\dagger Y_e)^{sc} (Y_e Y_e^\dagger)^{br} + \frac{9}{2} \delta^{pr} \delta^{sc} \delta^{td} \delta^{ab} g_L^4 - \frac{1}{4} \delta^{pa} \delta^{rb} \delta^{td} (Y_e^\dagger Y_e Y_e^\dagger Y_e)^{sc} \\
& - \frac{1}{4} \delta^{pa} \delta^{rb} \delta^{sc} (Y_e^\dagger Y_e Y_e^\dagger Y_e)^{dt} - \frac{1}{4} \delta^{rb} \delta^{sc} \delta^{td} (Y_e Y_e^\dagger Y_e Y_e^\dagger)^{pa} - \frac{1}{4} \delta^{pa} \delta^{sc} \delta^{td} (Y_e Y_e^\dagger Y_e Y_e^\dagger)^{br} - \frac{1}{2} Y_e^{*rd} Y_e^{*as} Y_e^{pc} Y_e^{bt} - \frac{3}{4} T_2 \delta^{rb} \delta^{sc} \delta^{td} (Y_e Y_e^\dagger)^{pa} \\
& - \frac{3}{4} T_2 \delta^{pa} \delta^{sc} \delta^{td} (Y_e Y_e^\dagger)^{br} - \left( \delta^{rb} \delta^{sc} Y_e^{*ad} Y_e^{pt} + \delta^{pa} \delta^{td} Y_e^{*rs} Y_e^{bc} \right) \text{Tr} [Y_e^\dagger Y_e] - \frac{5}{4} \delta^{pa} Y_e^{*rd} Y_e^{bt} (Y_e^\dagger Y_e)^{sc} - \frac{5}{4} \delta^{rb} Y_e^{*as} Y_e^{pc} (Y_e^\dagger Y_e)^{dt} \\
& - \frac{5}{4} \delta^{rb} \delta^{td} (Y_e^\dagger Y_e)^{sc} (Y_e Y_e^\dagger)^{pa} - \frac{5}{4} \delta^{pa} \delta^{sc} (Y_e^\dagger Y_e)^{dt} (Y_e Y_e^\dagger)^{br} - \frac{3}{2} T_2 \delta^{pa} \delta^{rb} \delta^{td} (Y_e^\dagger Y_e)^{sc} - \frac{3}{2} T_2 \delta^{pa} \delta^{rb} \delta^{sc} (Y_e^\dagger Y_e)^{dt} - 2 \delta^{pa} Y_e^{*rs} Y_e^{bt} (Y_e^\dagger Y_e)^{dc} \\
& - 2 \delta^{rb} Y_e^{*as} Y_e^{pt} (Y_e^\dagger Y_e)^{dc} - 2 \delta^{sc} Y_e^{*rd} Y_e^{bt} (Y_e Y_e^\dagger)^{pa} - 2 \delta^{td} Y_e^{*as} Y_e^{pc} (Y_e Y_e^\dagger)^{br} - 2 \delta^{sc} Y_e^{*rd} Y_e^{pt} (Y_e Y_e^\dagger)^{ba} - 2 \delta^{td} Y_e^{*rs} Y_e^{pc} (Y_e Y_e^\dagger)^{ba} \\
& - \frac{5}{2} \delta^{pa} \delta^{rb} (Y_e^\dagger Y_e)^{sc} (Y_e^\dagger Y_e)^{dt} - 3 \delta^{sc} \delta^{td} (Y_e Y_e^\dagger)^{pa} (Y_e Y_e^\dagger)^{br} - 6 \delta^{rb} \delta^{sc} Y_e^{pt} (Y_e^\dagger Y_e Y_e^\dagger)^{ad} - 6 \delta^{pa} \delta^{td} Y_e^{*rs} (Y_e Y_e^\dagger Y_e)^{bc} \left. \right\} C_{\ell e}^{abcd} + \left\{ g_Y^2 \left( \frac{8}{9} \delta^{pa} \delta^{cd} Y_e^{*rs} Y_e^{bt} \right. \right.
\end{aligned}$$

$$\begin{aligned}
& + \frac{8}{9} \delta^{rb} \delta^{cd} Y_e^{*as} Y_e^{pt} + 6 \delta^{pa} \delta^{rb} \delta^{st} (Y_u^\dagger Y_u)^{dc} - 3 \delta^{pa} \delta^{rb} (Y_e^\dagger Y_e)^{st} (Y_u^\dagger Y_u)^{dc} - \frac{256}{27} \delta^{pa} \delta^{rb} \delta^{st} \delta^{cd} g_Y^4 - \frac{32}{3} \delta^{pa} \delta^{rb} \delta^{st} \delta^{cd} g_Y^2 g_s^2 \Big\} C_{\ell u}^{abcd} \\
& + \left\{ 3 \delta^{pa} \delta^{rb} (Y_d^\dagger Y_d)^{dc} (Y_e^\dagger Y_e)^{st} + \frac{16}{3} \delta^{pa} \delta^{rb} \delta^{st} \delta^{cd} g_Y^2 g_s^2 + \frac{218}{27} \delta^{pa} \delta^{rb} \delta^{st} \delta^{cd} g_Y^4 - g_Y^2 \left( \frac{4}{9} \delta^{pa} \delta^{cd} Y_e^{*rs} Y_e^{bt} + \frac{4}{9} \delta^{rb} \delta^{cd} Y_e^{*as} Y_e^{pt} + 2 \delta^{pa} \delta^{rb} \delta^{st} (Y_d^\dagger Y_d)^{dc} \right) \right. \\
& - \frac{9}{2} \delta^{pa} Y_e^{*rs} Y_e^{bt} (Y_d^\dagger Y_d)^{dc} - \frac{9}{2} \delta^{rb} Y_e^{*as} Y_e^{pt} (Y_d^\dagger Y_d)^{dc} \Big\} C_{\ell d}^{abcd} + \left\{ g_Y^4 \left( \frac{2}{9} \delta^{pr} \delta^{st} \delta^{ab} \delta^{cd} - \frac{46}{27} \delta^{pr} \delta^{sc} \delta^{td} \delta^{ab} \right) + g_Y^2 \left( 2 \delta^{pr} \delta^{sc} \delta^{td} (Y_u Y_u^\dagger)^{ba} - \frac{1}{3} \delta^{st} \delta^{ab} Y_e^{*rd} Y_e^{pc} \right. \right. \\
& - \frac{1}{3} \delta^{sc} \delta^{td} \delta^{ab} (Y_e Y_e^\dagger)^{pr} - \frac{7}{9} \delta^{sc} \delta^{ab} Y_e^{*rd} Y_e^{pt} - \frac{7}{9} \delta^{td} \delta^{ab} Y_e^{*rs} Y_e^{pc} \Big) + \frac{3}{2} \delta^{sc} \delta^{td} (Y_d Y_d^\dagger)^{ba} (Y_e Y_e^\dagger)^{pr} + \frac{27}{2} \delta^{pr} \delta^{sc} \delta^{td} \delta^{ab} g_L^4 - \frac{3}{2} \delta^{pr} \delta^{sc} \delta^{td} \delta^{ab} g_Y^2 g_L^2 \\
& - \frac{3}{2} \delta^{sc} \delta^{td} (Y_e Y_e^\dagger)^{pr} (Y_u Y_u^\dagger)^{ba} - \frac{8}{3} \delta^{pr} \delta^{sc} \delta^{td} \delta^{ab} g_Y^2 g_s^2 - \frac{9}{2} \delta^{sc} Y_e^{*rd} Y_e^{pt} (Y_d Y_d^\dagger)^{ba} - \frac{9}{2} \delta^{td} Y_e^{*rs} Y_e^{pc} (Y_d Y_d^\dagger)^{ba} \Big\} C_{qe}^{abcd} + 6 Y_e^{*rs} Y_u^{*ad} C_{qu}^{abcd} Y_e^{pt} Y_u^{bc} \\
& + 18 Y_e^{*rs} Y_u^{*ad} C_{qu}^{abcd} Y_e^{pt} Y_u^{bc} + 6 Y_d^{*ad} Y_e^{*rs} C_{qd}^{abcd} Y_d^{bc} Y_e^{pt} + 18 Y_d^{*ad} Y_e^{*rs} C_{qd}^{abcd} Y_d^{bc} Y_e^{pt} + \left\{ g_Y^4 \left( \frac{8}{9} \delta^{pr} \delta^{st} \delta^{ab} \delta^{cd} - \frac{356}{27} \delta^{pr} \delta^{sa} \delta^{tb} \delta^{cd} \right) \right. \\
& + g_Y^2 \left( \frac{4}{3} \delta^{sa} \delta^{tb} \delta^{cd} (Y_e Y_e^\dagger)^{pr} + \frac{34}{9} \delta^{tb} \delta^{ad} Y_e^{*rs} Y_e^{pc} + \frac{34}{9} \delta^{sa} \delta^{cd} Y_e^{*rb} Y_e^{pt} + 37 \delta^{sa} \delta^{tb} Y_e^{*rd} Y_e^{pc} - \frac{4}{3} \delta^{st} \delta^{ad} Y_e^{*rb} Y_e^{pc} - \frac{28}{3} \delta^{pr} \delta^{sa} \delta^{tb} (Y_e^\dagger Y_e)^{dc} \right) \\
& + 8 T_2 \delta^{sa} \delta^{tb} Y_e^{*rd} Y_e^{pc} + 8 \delta^{sa} \delta^{tb} Y_e^{pc} (Y_e^\dagger Y_e Y_e^\dagger)^{rd} + 8 \delta^{sa} \delta^{tb} Y_e^{*rd} (Y_e Y_e^\dagger Y_e)^{pc} - 2 \delta^{tb} Y_e^{*rd} Y_e^{pa} (Y_e^\dagger Y_e)^{sc} - 2 \delta^{sa} Y_e^{*rb} Y_e^{pc} (Y_e^\dagger Y_e)^{dt} \\
& - 2 \delta^{sa} Y_e^{*rb} Y_e^{pt} (Y_e^\dagger Y_e)^{dc} - 2 \delta^{tb} Y_e^{*rs} Y_e^{pa} (Y_e^\dagger Y_e)^{dc} - 4 \delta^{sa} \delta^{tb} (Y_e^\dagger Y_e)^{dc} (Y_e Y_e^\dagger)^{pr} - 21 \delta^{sa} \delta^{tb} g_L^2 Y_e^{*rd} Y_e^{pc} \Big\} C_{ee}^{abcd} + \frac{64}{27} \delta^{pr} \delta^{st} \delta^{ad} \delta^{bc} g_Y^4 C_{uu}^{abcd} \\
& + \frac{16}{27} \delta^{pr} \delta^{st} \delta^{ad} \delta^{bc} g_Y^4 C_{dd}^{abcd} + \left\{ g_Y^4 \left( \frac{4}{9} \delta^{pr} \delta^{st} \delta^{ab} \delta^{cd} - \frac{230}{27} \delta^{pr} \delta^{sa} \delta^{tb} \delta^{cd} \right) + g_Y^2 \left( 3 \delta^{pr} \delta^{sa} \delta^{tb} (Y_u^\dagger Y_u)^{dc} - \frac{2}{3} \delta^{st} \delta^{cd} Y_e^{*rb} Y_e^{pa} - \frac{2}{3} \delta^{sa} \delta^{tb} \delta^{cd} (Y_e Y_e^\dagger)^{pr} \right. \right. \\
& - \frac{14}{9} \delta^{sa} \delta^{cd} Y_e^{*rb} Y_e^{pt} - \frac{14}{9} \delta^{tb} \delta^{cd} Y_e^{*rs} Y_e^{pa} \Big) + \frac{3}{2} \delta^{sa} \delta^{tb} (Y_u^\dagger Y_u)^{dc} (Y_e Y_e^\dagger)^{pr} - \frac{16}{3} \delta^{pr} \delta^{sa} \delta^{tb} \delta^{cd} g_Y^2 g_s^2 \Big\} C_{eu}^{abcd} + \left\{ g_Y^2 \left( \frac{1}{3} \delta^{st} \delta^{cd} Y_e^{*rb} Y_e^{pa} \right. \right. \\
& + \frac{1}{3} \delta^{sa} \delta^{tb} \delta^{cd} (Y_e Y_e^\dagger)^{pr} + \frac{7}{9} \delta^{sa} \delta^{cd} Y_e^{*rb} Y_e^{pt} + \frac{7}{9} \delta^{tb} \delta^{cd} Y_e^{*rs} Y_e^{pa} - \delta^{pr} \delta^{sa} \delta^{tb} (Y_d^\dagger Y_d)^{dc} \Big) + \frac{8}{3} \delta^{pr} \delta^{sa} \delta^{tb} \delta^{cd} g_Y^2 g_s^2 - g_Y^4 \left( \frac{2}{27} \delta^{pr} \delta^{sa} \delta^{tb} \delta^{cd} \right. \\
& + \frac{2}{9} \delta^{pr} \delta^{st} \delta^{ab} \delta^{cd} \Big) - \frac{3}{2} \delta^{sa} \delta^{tb} (Y_d^\dagger Y_d)^{dc} (Y_e Y_e^\dagger)^{pr} - \frac{9}{2} \delta^{sa} Y_e^{*rb} Y_e^{pt} (Y_d^\dagger Y_d)^{dc} - \frac{9}{2} \delta^{tb} Y_e^{*rs} Y_e^{pa} (Y_d^\dagger Y_d)^{dc} \Big\} C_{ed}^{abcd} + \left\{ g_Y^2 \left( \frac{1}{3} \delta^{pr} \delta^{tb} Y_e^{*as} Y_d^{dc} + \frac{5}{3} \delta^{pa} \delta^{st} Y_e^{*rb} Y_d^{dc} \right. \right. \\
& - \frac{205}{24} \delta^{pa} \delta^{tb} Y_e^{*rs} Y_d^{dc} \Big) + \frac{3}{2} Y_e^{*rs} Y_e^{*ab} Y_d^{dc} Y_e^{pt} + \frac{3}{2} \delta^{pa} \delta^{tb} Y_e^{*rs} Y_d^{dc} \text{Tr}[Y_e^\dagger Y_e] + \frac{27}{4} \delta^{pa} \delta^{tb} Y_e^{*rs} (Y_d Y_d^\dagger Y_d)^{dc} - \frac{3}{4} \delta^{pa} Y_e^{*rb} Y_d^{dc} (Y_e^\dagger Y_e)^{st} \\
& - \frac{3}{4} \delta^{tb} Y_e^{*as} Y_d^{dc} (Y_e Y_e^\dagger)^{pr} - \frac{3}{4} \delta^{pa} \delta^{tb} Y_e^{*rs} (Y_u Y_u^\dagger Y_d)^{dc} - \frac{9}{8} \delta^{pa} \delta^{tb} g_L^2 Y_e^{*rs} Y_d^{dc} - 20 \delta^{pa} \delta^{tb} g_s^2 Y_e^{*rs} Y_d^{dc} \Big\} C_{ledq}^{abcd} + C_{ledq}^{*abcd} \left\{ g_Y^2 \left( \frac{1}{3} \delta^{pr} \delta^{sb} Y_d^{*dc} Y_e^{at} \right. \right. \\
& + \frac{5}{3} \delta^{ra} \delta^{st} Y_d^{*dc} Y_e^{pb} - \frac{205}{24} \delta^{ra} \delta^{sb} Y_d^{*dc} Y_e^{pt} \Big) + \frac{3}{2} Y_d^{*dc} Y_e^{*rs} Y_e^{pt} Y_e^{ab} + \frac{3}{2} \delta^{ra} \delta^{sb} Y_d^{*dc} Y_e^{pt} \text{Tr}[Y_e^\dagger Y_e] + \frac{27}{4} \delta^{ra} \delta^{sb} Y_e^{pt} (Y_d^\dagger Y_d Y_d^\dagger)^{dc} - \frac{3}{4} \delta^{ra} Y_d^{*dc} Y_e^{pb} (Y_e^\dagger Y_e)^{st}
\end{aligned}$$

$$\begin{aligned}
& -\frac{3}{4}\delta^{sb}Y_d^{*dc}Y_e^{at}(Y_eY_e^\dagger)^{pr} - \frac{3}{4}\delta^{ra}\delta^{sb}Y_e^{pt}(Y_u^\dagger Y_u Y_d^\dagger)^{dc} - \frac{9}{8}\delta^{ra}\delta^{sb}g_L^2Y_d^{*dc}Y_e^{pt} - 20\delta^{ra}\delta^{sb}g_s^2Y_d^{*dc}Y_e^{pt} \Bigg\} + \left\{ \frac{3}{4}\delta^{pa}Y_e^{*rb}Y_u^{*cd}(Y_e^\dagger Y_e)^{st} \right. \\
& + \frac{3}{4}\delta^{tb}Y_e^{*as}Y_u^{*cd}(Y_eY_e^\dagger)^{pr} + \frac{3}{4}\delta^{pa}\delta^{tb}Y_e^{*rs}(Y_d^\dagger Y_d Y_u^\dagger)^{cd} + g_Y^2\left(\frac{73}{6}\delta^{pa}\delta^{tb}Y_e^{*rs}Y_u^{*cd} - \frac{1}{3}\delta^{pr}\delta^{tb}Y_e^{*as}Y_u^{*cd} - \frac{5}{3}\delta^{pa}\delta^{st}Y_e^{*rb}Y_u^{*cd}\right) + \frac{9}{2}\delta^{pa}\delta^{tb}g_L^2Y_e^{*rs}Y_u^{*cd} \\
& + 20\delta^{pa}\delta^{tb}g_s^2Y_e^{*rs}Y_u^{*cd} - \frac{3}{2}Y_e^{*rs}Y_e^{*ab}Y_u^{*cd}Y_e^{pt} - \frac{3}{2}\delta^{pa}\delta^{tb}Y_e^{*rs}Y_u^{*cd}\text{Tr}[Y_e^\dagger Y_e] - \frac{27}{4}\delta^{pa}\delta^{tb}Y_e^{*rs}(Y_u^\dagger Y_u Y_u^\dagger)^{cd} \Bigg\} C_{lequ}^{abcd} \\
& + C_{lequ}^{*abcd} \left\{ \frac{3}{4}\delta^{ra}Y_e^{pb}Y_u^{cd}(Y_e^\dagger Y_e)^{st} + \frac{3}{4}\delta^{sb}Y_e^{at}Y_u^{cd}(Y_eY_e^\dagger)^{pr} + \frac{3}{4}\delta^{ra}\delta^{sb}Y_e^{pt}(Y_dY_d^\dagger Y_u)^{cd} + g_Y^2\left(\frac{73}{6}\delta^{ra}\delta^{sb}Y_e^{pt}Y_u^{cd} - \frac{1}{3}\delta^{pr}\delta^{sb}Y_e^{at}Y_u^{cd} - \frac{5}{3}\delta^{ra}\delta^{st}Y_e^{pb}Y_u^{cd}\right) \right. \\
& + \frac{9}{2}\delta^{ra}\delta^{sb}g_L^2Y_e^{pt}Y_u^{cd} + 20\delta^{ra}\delta^{sb}g_s^2Y_e^{pt}Y_u^{cd} - \frac{3}{2}Y_e^{*rs}Y_e^{pt}Y_e^{ab}Y_u^{cd} - \frac{3}{2}\delta^{ra}\delta^{sb}Y_e^{pt}Y_u^{cd}\text{Tr}[Y_e^\dagger Y_e] - \frac{27}{4}\delta^{ra}\delta^{sb}Y_e^{pt}(Y_uY_u^\dagger Y_u)^{cd} \Bigg\} + \left\{ \frac{3}{4}Y_e^{*rs}Y_e^{*ad}Y_u^{*cb}Y_e^{pt} \right. \\
& + \frac{3}{4}\delta^{pa}\delta^{td}Y_e^{*rs}Y_u^{*cb}\text{Tr}[Y_e^\dagger Y_e] + g_Y^2\left(\frac{5}{12}\delta^{pr}\delta^{td}Y_e^{*as}Y_u^{*cb} + \frac{7}{12}\delta^{pa}\delta^{st}Y_e^{*rd}Y_u^{*cb} - \frac{617}{48}\delta^{pa}\delta^{td}Y_e^{*rs}Y_u^{*cb}\right) + \frac{27}{8}\delta^{pa}\delta^{td}Y_e^{*rs}(Y_u^\dagger Y_u Y_u^\dagger)^{cb} \\
& - \frac{3}{8}\delta^{pa}Y_e^{*rd}Y_u^{*cb}(Y_e^\dagger Y_e)^{st} - \frac{3}{8}\delta^{td}Y_e^{*as}Y_u^{*cb}(Y_eY_e^\dagger)^{pr} - \frac{9}{8}\delta^{pa}\delta^{td}Y_e^{*rs}(Y_d^\dagger Y_d Y_u^\dagger)^{cb} - \frac{45}{16}\delta^{pa}\delta^{td}g_L^2Y_e^{*rs}Y_u^{*cb} - 17\delta^{pa}\delta^{td}g_s^2Y_e^{*rs}Y_u^{*cb} \Bigg\} C_{luqe}^{abcd} \\
& + C_{luqe}^{*abcd} \left\{ \frac{3}{4}Y_e^{*rs}Y_e^{pt}Y_e^{ad}Y_u^{cb} + \frac{3}{4}\delta^{ra}\delta^{sd}Y_e^{pt}Y_u^{cb}\text{Tr}[Y_e^\dagger Y_e] + g_Y^2\left(\frac{5}{12}\delta^{pr}\delta^{sd}Y_e^{at}Y_u^{cb} + \frac{7}{12}\delta^{ra}\delta^{st}Y_e^{pd}Y_u^{cb} - \frac{617}{48}\delta^{ra}\delta^{sd}Y_e^{pt}Y_u^{cb}\right) \right. \\
& + \frac{27}{8}\delta^{ra}\delta^{sd}Y_e^{pt}(Y_uY_u^\dagger Y_u)^{cb} - \frac{3}{8}\delta^{ra}Y_e^{pd}Y_u^{cb}(Y_e^\dagger Y_e)^{st} - \frac{3}{8}\delta^{sd}Y_e^{at}Y_u^{cb}(Y_eY_e^\dagger)^{pr} - \frac{9}{8}\delta^{ra}\delta^{sd}Y_e^{pt}(Y_dY_d^\dagger Y_u)^{cb} - \frac{45}{16}\delta^{ra}\delta^{sd}g_L^2Y_e^{pt}Y_u^{cb} - 17\delta^{ra}\delta^{sd}g_s^2Y_e^{pt}Y_u^{cb} \Bigg\} \\
& + \left\{ g_Y^4\left(\frac{8}{9}\delta^{pr}\delta^{st}\delta^{ad}\delta^{bc} + \frac{40}{27}\delta^{pa}\delta^{rb}\delta^{st}\delta^{cd} - \frac{130}{27}\delta^{pa}\delta^{rd}\delta^{st}\delta^{bc}\right) + g_Y^2g_L^2\left(2\delta^{pa}\delta^{rd}\delta^{st}\delta^{bc} + 2\delta^{pa}\delta^{rb}\delta^{st}\delta^{cd} - \frac{4}{9}\delta^{pr}\delta^{st}\delta^{ad}\delta^{bc}\right) + g_L^2\left(\frac{1}{3}\delta^{pa}\delta^{bc}Y_e^{*rs}Y_e^{dt} \right. \right. \\
& + \frac{1}{3}\delta^{rd}\delta^{bc}Y_e^{*as}Y_e^{pt} + \frac{2}{3}\delta^{pr}\delta^{bc}Y_e^{*as}Y_e^{dt} + \frac{2}{3}\delta^{pa}\delta^{rd}\delta^{bc}(Y_e^\dagger Y_e)^{st} - \frac{15}{4}\delta^{pa}\delta^{rd}Y_e^{*cs}Y_e^{bt} - \frac{39}{2}\delta^{pa}\delta^{rb}Y_e^{*cs}Y_e^{dt} \Bigg) + g_Y^2\left(\frac{11}{9}\delta^{pa}\delta^{bc}Y_e^{*rs}Y_e^{dt} \right. \\
& + \frac{11}{9}\delta^{rd}\delta^{bc}Y_e^{*as}Y_e^{pt} + \frac{5}{2}\delta^{pa}\delta^{rb}Y_e^{*cs}Y_e^{dt} + \frac{11}{4}\delta^{pa}\delta^{rd}Y_e^{*cs}Y_e^{bt} - \frac{8}{9}\delta^{pa}\delta^{cd}Y_e^{*rs}Y_e^{bt} - \frac{8}{9}\delta^{rb}\delta^{cd}Y_e^{*as}Y_e^{pt} - \frac{4}{3}\delta^{pr}\delta^{bc}Y_e^{*as}Y_e^{dt} - 4\delta^{pa}\delta^{rd}\delta^{st}(Y_eY_e^\dagger)^{bc} \\
& - \frac{16}{3}\delta^{pa}\delta^{rb}\delta^{st}(Y_eY_e^\dagger)^{dc} \Bigg) + \frac{5}{2}\delta^{pa}\delta^{rd}Y_e^{bt}(Y_e^\dagger Y_e Y_e^\dagger)^{cs} + \frac{5}{2}\delta^{pa}\delta^{rd}Y_e^{*cs}(Y_eY_e^\dagger Y_e)^{bt} + 3\delta^{pa}\delta^{rb}Y_e^{dt}(Y_e^\dagger Y_e Y_e^\dagger)^{cs} + 3\delta^{pa}\delta^{rb}Y_e^{*cs}(Y_eY_e^\dagger Y_e)^{dt} \\
& + 5T_2\delta^{pa}\delta^{rd}Y_e^{*cs}Y_e^{bt} + 6T_2\delta^{pa}\delta^{rb}Y_e^{*cs}Y_e^{dt} - \delta^{rb}Y_e^{*as}Y_e^{dt}(Y_eY_e^\dagger)^{pc} - \delta^{pa}Y_e^{*cs}Y_e^{bt}(Y_eY_e^\dagger)^{dr} - \frac{3}{2}\delta^{rd}Y_e^{*as}Y_e^{bt}(Y_eY_e^\dagger)^{pc} - \frac{3}{2}\delta^{pa}Y_e^{*cs}Y_e^{dt}(Y_eY_e^\dagger)^{br} \\
& \left. - 2\delta^{pa}Y_e^{*rs}Y_e^{bt}(Y_eY_e^\dagger)^{dc} - 2\delta^{rb}Y_e^{*as}Y_e^{pt}(Y_eY_e^\dagger)^{dc} - 2\delta^{pa}\delta^{rb}(Y_e^\dagger Y_e)^{st}(Y_eY_e^\dagger)^{dc} - 3\delta^{pa}\delta^{rd}(Y_e^\dagger Y_e)^{st}(Y_eY_e^\dagger)^{bc} \right\} C_{\ell\ell}^{abcd} + \frac{8}{27}\delta^{pr}\delta^{st}\delta^{ad}\delta^{bc}g_Y^4C_{qq}^{(ll)abcd}
\end{aligned}$$

$$\begin{aligned}
& + \frac{16}{27} \delta^{pr} \delta^{st} \delta^{ad} \delta^{bc} g_Y^4 C_{qq}^{(\times)abcd} + \left\{ g_Y^2 \left( \frac{4}{9} \delta^{pa} \delta^{cd} Y_e^{*rs} Y_e^{bt} + \frac{4}{9} \delta^{rb} \delta^{cd} Y_e^{*as} Y_e^{pt} + 4 \delta^{pa} \delta^{rb} \delta^{st} (Y_u Y_u^\dagger)^{dc} \right) + 3 \delta^{pa} \delta^{rb} (Y_e^\dagger Y_e)^{st} (Y_u Y_u^\dagger)^{dc} \right. \\
& - 3 \delta^{pa} \delta^{rb} \delta^{st} \delta^{cd} g_Y^2 g_L^2 - 3 \delta^{pa} \delta^{rb} (Y_e^\dagger Y_e)^{st} (Y_d Y_d^\dagger)^{dc} - \frac{9}{2} \delta^{pa} Y_e^{*rs} Y_e^{bt} (Y_d Y_d^\dagger)^{dc} - \frac{9}{2} \delta^{rb} Y_e^{*as} Y_e^{pt} (Y_d Y_d^\dagger)^{dc} - \frac{16}{3} \delta^{pa} \delta^{rb} \delta^{st} \delta^{cd} g_Y^2 g_s^2 \\
& - \frac{224}{27} \delta^{pa} \delta^{rb} \delta^{st} \delta^{cd} g_Y^4 \left. \right\} C_{\ell q}^{(\parallel)abcd} + \left\{ g_L^2 \left( \delta^{pr} \delta^{cd} Y_e^{*as} Y_e^{bt} + \delta^{pa} \delta^{rb} \delta^{cd} (Y_e^\dagger Y_e)^{st} + 2 \delta^{pa} \delta^{cd} Y_e^{*rs} Y_e^{bt} + 2 \delta^{rb} \delta^{cd} Y_e^{*as} Y_e^{pt} \right) + g_Y^2 \left( \frac{2}{9} \delta^{pa} \delta^{cd} Y_e^{*rs} Y_e^{bt} \right. \right. \\
& + \frac{2}{9} \delta^{rb} \delta^{cd} Y_e^{*as} Y_e^{pt} + 2 \delta^{pa} \delta^{rb} \delta^{st} (Y_u Y_u^\dagger)^{dc} \left. \right) + \frac{3}{2} \delta^{pa} \delta^{rb} (Y_e^\dagger Y_e)^{st} (Y_u Y_u^\dagger)^{dc} - g_Y^2 g_L^2 \left( \frac{2}{3} \delta^{pr} \delta^{st} \delta^{ab} \delta^{cd} + 6 \delta^{pa} \delta^{rb} \delta^{st} \delta^{cd} \right) - \frac{3}{2} \delta^{pa} \delta^{rb} (Y_e^\dagger Y_e)^{st} (Y_d Y_d^\dagger)^{dc} \\
& - \frac{8}{3} \delta^{pa} \delta^{rb} \delta^{st} \delta^{cd} g_Y^2 g_s^2 - \frac{112}{27} \delta^{pa} \delta^{rb} \delta^{st} \delta^{cd} g_Y^4 - 9 \delta^{pa} Y_e^{*rs} Y_e^{bt} (Y_d Y_d^\dagger)^{dc} - 9 \delta^{rb} Y_e^{*as} Y_e^{pt} (Y_d Y_d^\dagger)^{dc} \left. \right\} C_{\ell q}^{(\times)abcd}, \tag{10.2}
\end{aligned}$$

## 10.2 $C_{\ell u}$

$$\begin{aligned}
\beta_{C_{\ell u}^{prst}}^{(1)} & = \left\{ \frac{4}{9} \delta^{pa} \delta^{rb} \delta^{st} g_Y^2 - 2 \delta^{pa} \delta^{rb} (Y_u^\dagger Y_u)^{st} \right\} C_{H\ell}^{(\parallel)ab} + \left\{ \frac{2}{9} \delta^{pa} \delta^{rb} \delta^{st} g_Y^2 - \delta^{pa} \delta^{rb} (Y_u^\dagger Y_u)^{st} \right\} C_{H\ell}^{(\times)ab} - \left\{ \frac{1}{3} \delta^{pr} \delta^{sa} \delta^{tb} g_Y^2 + \delta^{sa} \delta^{tb} (Y_e Y_e^\dagger)^{pr} \right\} C_{Hu}^{ab} \\
& - \frac{8}{9} \delta^{pa} \delta^{rb} \delta^{st} \delta^{cd} g_Y^2 C_{\ell e}^{abcd} + \left\{ \frac{2}{9} g_Y^2 \left( 3 \delta^{pr} \delta^{sc} \delta^{td} \delta^{ab} + 8 \delta^{pa} \delta^{rb} \delta^{st} \delta^{cd} + 18 \delta^{pa} \delta^{rb} \delta^{sc} \delta^{td} \right) + \frac{1}{2} \left( \delta^{rb} \delta^{sc} \delta^{td} (Y_e Y_e^\dagger)^{pa} + \delta^{pa} \delta^{sc} \delta^{td} (Y_e Y_e^\dagger)^{br} \right. \right. \\
& + 2 \delta^{pa} \delta^{rb} \delta^{td} (Y_u^\dagger Y_u)^{sc} + 2 \delta^{pa} \delta^{rb} \delta^{sc} (Y_u^\dagger Y_u)^{dt} \left. \right) \left. \right\} C_{\ell u}^{abcd} - \frac{8}{9} \delta^{pa} \delta^{rb} \delta^{st} \delta^{cd} g_Y^2 C_{\ell d}^{abcd} - \frac{2}{3} \delta^{pr} \delta^{sc} \delta^{td} \delta^{ab} g_Y^2 C_{qu}^{(\parallel)abcd} - \frac{2}{9} \delta^{pr} \delta^{sc} \delta^{td} \delta^{ab} g_Y^2 C_{qu}^{(\times)abcd} \\
& - \frac{8}{9} g_Y^2 \left\{ \delta^{pr} \delta^{sa} \delta^{td} \delta^{bc} + 3 \delta^{pr} \delta^{sa} \delta^{tb} \delta^{cd} \right\} C_{uu}^{abcd} + \left\{ \frac{2}{3} \delta^{pr} \delta^{sc} \delta^{td} \delta^{ab} g_Y^2 - \delta^{sc} \delta^{td} Y_e^{*rb} Y_e^{pa} \right\} C_{eu}^{abcd} + \frac{2}{3} \delta^{pr} \delta^{sa} \delta^{tb} \delta^{cd} g_Y^2 C_{ud}^{(\parallel)abcd} \\
& + \frac{2}{9} \delta^{pr} \delta^{sa} \delta^{tb} \delta^{cd} g_Y^2 C_{ud}^{(\times)abcd} - \frac{1}{2} \delta^{pa} \delta^{td} Y_e^{*rb} Y_u^{*cs} C_{\ell e qu}^{abcd} - \frac{1}{2} \delta^{ra} \delta^{sd} C_{\ell e qu}^{*abcd} Y_e^{pb} Y_u^{ct} + \delta^{pa} \delta^{tb} Y_e^{*rd} Y_u^{*cs} C_{\ell u qe}^{abcd} + \delta^{ra} \delta^{sb} C_{\ell u qe}^{*abcd} Y_e^{pd} Y_u^{ct} \\
& - \frac{8}{9} g_Y^2 \left\{ \delta^{pa} \delta^{rd} \delta^{st} \delta^{bc} + 2 \delta^{pa} \delta^{rb} \delta^{st} \delta^{cd} \right\} C_{\ell \ell}^{abcd} + \left\{ \frac{8}{9} \delta^{pa} \delta^{rb} \delta^{st} \delta^{cd} g_Y^2 - 2 \delta^{pa} \delta^{rb} Y_u^{*cs} Y_u^{dt} \right\} C_{\ell q}^{(\parallel)abcd} + \left\{ \frac{4}{9} \delta^{pa} \delta^{rb} \delta^{st} \delta^{cd} g_Y^2 - \delta^{pa} \delta^{rb} Y_u^{*cs} Y_u^{dt} \right\} C_{\ell q}^{(\times)abcd}, \tag{10.3}
\end{aligned}$$

$$\begin{aligned}
\beta_{C_{\ell u}^{prst}}^{(2)} & = -\frac{22}{9} \delta^{st} g_Y^2 (C_{\ell HH} C_{\ell HH}^\dagger)^{rp} - 3 (Y_u^\dagger Y_u)^{st} (C_{\ell HH} C_{\ell HH}^\dagger)^{rp} + \left\{ g_Y^4 \left( \frac{2}{3} \delta^{st} (Y_e Y_e^\dagger)^{pr} + \frac{11}{3} \delta^{pr} (Y_u^\dagger Y_u)^{st} \right) - \frac{8}{9} \delta^{pr} \delta^{st} g_Y^6 \right\} C_{HB} + \left\{ g_Y^2 g_L^2 \left( \frac{3}{4} \delta^{pr} (Y_u^\dagger Y_u)^{st} \right. \right. \\
& - \frac{3}{2} \delta^{st} (Y_e Y_e^\dagger)^{pr} \left. \right) - \frac{2}{3} \delta^{pr} \delta^{st} g_Y^4 g_L^2 \left. \right\} C_{HWB} - \frac{20}{3} \delta^{pr} \delta^{st} g_Y^2 g_L^6 C_W - \frac{160}{9} \delta^{pr} \delta^{st} g_Y^2 g_s^6 C_G + \left\{ g_Y^4 \left( \frac{4}{3} \delta^{pr} \delta^{st} Y_e^{*ab} - \frac{31}{3} \delta^{pa} \delta^{st} Y_e^{*rb} \right) - g_Y^2 \left( \frac{4}{3} \delta^{st} Y_e^{*rb} (Y_e Y_e^\dagger)^{pa} \right. \right.
\end{aligned}$$

$$\begin{aligned}
& + \frac{43}{6} \delta^{pa} Y_e^{*rb} (Y_u^\dagger Y_u)^{st} \Big\} C_{eB}^{ab} + C_{eB}^{*ab} \Big\{ g_Y^4 \Big( \frac{4}{3} \delta^{pr} \delta^{st} Y_e^{ab} - \frac{31}{3} \delta^{ra} \delta^{st} Y_e^{pb} \Big) - g_Y^2 \Big( \frac{4}{3} \delta^{st} Y_e^{pb} (Y_e Y_e^\dagger)^{ar} + \frac{43}{6} \delta^{ra} Y_e^{pb} (Y_u^\dagger Y_u)^{st} \Big) \Big\} + \Big\{ \frac{5}{6} \delta^{pa} \delta^{st} g_Y^2 g_L^2 Y_e^{*rb} \\
& + \frac{15}{4} \delta^{pa} g_L^2 Y_e^{*rb} (Y_u^\dagger Y_u)^{st} \Big\} C_{eW}^{ab} + C_{eW}^{*ab} \Big\{ \frac{5}{6} \delta^{ra} \delta^{st} g_Y^2 g_L^2 Y_e^{pb} + \frac{15}{4} \delta^{ra} g_L^2 Y_e^{pb} (Y_u^\dagger Y_u)^{st} \Big\} + \Big\{ g_Y^4 \Big( \frac{44}{27} \delta^{pr} \delta^{tb} Y_u^{*as} - \frac{20}{9} \delta^{pr} \delta^{st} Y_u^{*ab} \Big) \\
& + g_Y^2 \Big( \delta^{pr} Y_u^{*as} (Y_u^\dagger Y_u)^{bt} + 8 \delta^{tb} Y_u^{*as} (Y_e Y_e^\dagger)^{pr} \Big) + \frac{16}{3} \delta^{pr} \delta^{tb} g_Y^2 g_s^2 Y_u^{*as} \Big\} C_{uB}^{ab} + C_{uB}^{*ab} \Big\{ g_Y^4 \Big( \frac{44}{27} \delta^{pr} \delta^{sb} Y_u^{at} - \frac{20}{9} \delta^{pr} \delta^{st} Y_u^{ab} \Big) + g_Y^2 \Big( \delta^{pr} Y_u^{at} (Y_u^\dagger Y_u)^{sb} \\
& + 8 \delta^{sb} Y_u^{at} (Y_e Y_e^\dagger)^{pr} \Big) + \frac{16}{3} \delta^{pr} \delta^{sb} g_Y^2 g_s^2 Y_u^{at} \Big\} + \Big\{ \frac{7}{6} \delta^{pr} \delta^{tb} g_Y^2 g_L^2 Y_u^{*as} + \frac{9}{2} \delta^{pr} \delta^{tb} g_L^4 Y_u^{*as} + 6 \delta^{tb} g_L^2 Y_u^{*as} (Y_e Y_e^\dagger)^{pr} \Big\} C_{uW}^{ab} \\
& + C_{uW}^{*ab} \Big\{ \frac{7}{6} \delta^{pr} \delta^{sb} g_Y^2 g_L^2 Y_u^{at} + \frac{9}{2} \delta^{pr} \delta^{sb} g_L^4 Y_u^{at} + 6 \delta^{sb} g_L^2 Y_u^{at} (Y_e Y_e^\dagger)^{pr} \Big\} + \Big\{ \frac{52}{27} \delta^{pr} \delta^{tb} g_Y^2 g_s^2 Y_u^{*as} + 4 \delta^{tb} g_s^2 Y_u^{*as} (Y_e Y_e^\dagger)^{pr} \Big\} C_{uG}^{ab} \\
& + C_{uG}^{*ab} \Big\{ \frac{52}{27} \delta^{pr} \delta^{sb} g_Y^2 g_s^2 Y_u^{at} + 4 \delta^{sb} g_s^2 Y_u^{at} (Y_e Y_e^\dagger)^{pr} \Big\} + \frac{4}{9} \delta^{pr} \delta^{st} g_Y^4 Y_d^{*ab} C_{dB}^{ab} + \frac{4}{9} \delta^{pr} \delta^{st} g_Y^4 C_{dB}^{*ab} Y_d^{ab} + \Big\{ g_Y^2 \Big( \frac{1}{54} \delta^{rb} \delta^{st} (Y_e Y_e^\dagger)^{pa} \\
& + \frac{1}{54} \delta^{pa} \delta^{st} (Y_e Y_e^\dagger)^{br} + \frac{299}{36} \delta^{pa} \delta^{rb} (Y_u^\dagger Y_u)^{st} - \frac{4}{9} T_2 \delta^{pa} \delta^{rb} \delta^{st} \Big) + 2 T_2 \delta^{pa} \delta^{rb} (Y_u^\dagger Y_u)^{st} + 3 \delta^{pa} \delta^{rb} (Y_u^\dagger Y_u Y_u^\dagger Y_u)^{st} + 4 \delta^{pa} \delta^{rb} \delta^{st} g_Y^2 g_L^2 \\
& + \frac{32}{3} \delta^{pa} \delta^{rb} g_s^2 (Y_u^\dagger Y_u)^{st} - \frac{1}{4} \delta^{rb} (Y_u^\dagger Y_u)^{st} (Y_e Y_e^\dagger)^{pa} - \frac{1}{4} \delta^{pa} (Y_u^\dagger Y_u)^{st} (Y_e Y_e^\dagger)^{br} - \frac{142}{81} \delta^{pa} \delta^{rb} \delta^{st} g_Y^4 - \frac{51}{4} \delta^{pa} \delta^{rb} g_L^2 (Y_u^\dagger Y_u)^{st} \Big\} C_{H\ell}^{(\parallel)ab} \\
& + \Big\{ g_Y^2 g_L^2 \Big( \frac{2}{27} \delta^{pr} \delta^{st} \delta^{ab} + \frac{25}{9} \delta^{pa} \delta^{rb} \delta^{st} \Big) + T_2 \delta^{pa} \delta^{rb} (Y_u^\dagger Y_u)^{st} + g_Y^2 \Big( \frac{13}{27} \delta^{rb} \delta^{st} (Y_e Y_e^\dagger)^{pa} + \frac{13}{27} \delta^{pa} \delta^{st} (Y_e Y_e^\dagger)^{br} + \frac{299}{72} \delta^{pa} \delta^{rb} (Y_u^\dagger Y_u)^{st} \\
& - \frac{2}{9} \delta^{st} \delta^{ab} (Y_e Y_e^\dagger)^{pr} - \frac{4}{9} \delta^{pa} \delta^{rb} \delta^{st} \text{Tr} [Y_e^\dagger Y_e] - \frac{2}{3} \delta^{pa} \delta^{rb} \delta^{st} \text{Tr} [Y_d^\dagger Y_d] - \frac{2}{3} \delta^{pa} \delta^{rb} \delta^{st} \text{Tr} [Y_u^\dagger Y_u] \Big) + \frac{3}{2} \delta^{pa} \delta^{rb} (Y_u^\dagger Y_u Y_u^\dagger Y_u)^{st} + \frac{16}{3} \delta^{pa} \delta^{rb} g_s^2 (Y_u^\dagger Y_u)^{st} \\
& - \frac{1}{2} \delta^{rb} (Y_u^\dagger Y_u)^{st} (Y_e Y_e^\dagger)^{pa} - \frac{1}{2} \delta^{pa} (Y_u^\dagger Y_u)^{st} (Y_e Y_e^\dagger)^{br} - \frac{71}{81} \delta^{pa} \delta^{rb} \delta^{st} g_Y^4 - \frac{15}{8} \delta^{pa} \delta^{rb} g_L^2 (Y_u^\dagger Y_u)^{st} \Big\} C_{H\ell}^{(\times)ab} + \Big\{ T_2 \delta^{sa} \delta^{tb} (Y_e Y_e^\dagger)^{pr} \\
& + g_Y^2 \Big( \frac{1}{3} T_2 \delta^{pr} \delta^{sa} \delta^{tb} + \frac{179}{24} \delta^{sa} \delta^{tb} (Y_e Y_e^\dagger)^{pr} - \frac{101}{108} \delta^{pr} \delta^{tb} (Y_u^\dagger Y_u)^{sa} - \frac{101}{108} \delta^{pr} \delta^{sa} (Y_u^\dagger Y_u)^{bt} \Big) + \frac{400}{243} \delta^{pr} \delta^{sa} \delta^{tb} g_Y^4 + 3 \delta^{sa} \delta^{tb} (Y_e Y_e^\dagger Y_e Y_e^\dagger)^{pr} \\
& - \frac{1}{4} \delta^{tb} (Y_u^\dagger Y_u)^{sa} (Y_e Y_e^\dagger)^{pr} - \frac{1}{4} \delta^{sa} (Y_u^\dagger Y_u)^{bt} (Y_e Y_e^\dagger)^{pr} - 3 \delta^{pr} \delta^{sa} \delta^{tb} g_Y^2 g_L^2 - \frac{33}{8} \delta^{sa} \delta^{tb} g_L^2 (Y_e Y_e^\dagger)^{pr} \Big\} C_{Hu}^{ab} - \Big\{ \frac{55}{108} \delta^{pr} \delta^{sa} g_Y^2 (Y_d^\dagger Y_u)^{bt} \\
& + \frac{3}{4} \delta^{sa} (Y_d^\dagger Y_u)^{bt} (Y_e Y_e^\dagger)^{pr} \Big\} C_{Hud}^{ab} - C_{Hud}^{*ab} \Big\{ \frac{55}{108} \delta^{pr} \delta^{ta} g_Y^2 (Y_u^\dagger Y_d)^{sb} + \frac{3}{4} \delta^{ta} (Y_u^\dagger Y_d)^{sb} (Y_e Y_e^\dagger)^{pr} \Big\} + \Big\{ g_Y^2 \Big( \frac{20}{27} \delta^{pa} \delta^{st} Y_e^{*rd} Y_e^{bc} + \frac{20}{27} \delta^{rb} \delta^{st} Y_e^{*ad} Y_e^{pc} \\
& + \frac{20}{9} \delta^{pa} \delta^{rb} \delta^{st} (Y_e^\dagger Y_e)^{dc} \Big) + \frac{944}{81} \delta^{pa} \delta^{rb} \delta^{st} \delta^{cd} g_Y^4 - \delta^{pa} \delta^{rb} (Y_e^\dagger Y_e)^{dc} (Y_u^\dagger Y_u)^{st} \Big\} C_{\ell e}^{abcd} + \Big\{ \frac{1}{2} \delta^{sc} \delta^{td} (Y_e Y_e^\dagger)^{pr} (Y_e Y_e^\dagger)^{ba} + g_Y^2 g_L^2 \Big( \frac{3}{2} \delta^{pr} \delta^{sc} \delta^{td} \delta^{ab}
\end{aligned}$$



$$\begin{aligned}
& -9\delta^{pa}\delta^{rb}\delta^{sc}\delta^{td}) + g_Y^2 g_s^2 \left( \frac{64}{9}\delta^{pa}\delta^{rb}\delta^{st}\delta^{cd} - 16\delta^{pa}\delta^{rb}\delta^{sc}\delta^{td} \right) + g_Y^4 \left( \frac{214}{243}\delta^{pr}\delta^{sc}\delta^{td}\delta^{ab} + \frac{632}{81}\delta^{pa}\delta^{rb}\delta^{st}\delta^{cd} - \frac{574}{9}\delta^{pa}\delta^{rb}\delta^{sc}\delta^{td} \right) \\
& + g_L^2 \left( \frac{33}{16}\delta^{rb}\delta^{sc}\delta^{td}(Y_e Y_e^\dagger)^{pa} + \frac{33}{16}\delta^{pa}\delta^{sc}\delta^{td}(Y_e Y_e^\dagger)^{br} + \frac{51}{8}\delta^{pa}\delta^{rb}\delta^{td}(Y_u^\dagger Y_u)^{sc} + \frac{51}{8}\delta^{pa}\delta^{rb}\delta^{sc}(Y_u^\dagger Y_u)^{dt} \right) + 3\delta^{pa}\delta^{rb}(Y_u^\dagger Y_u)^{st}(Y_u^\dagger Y_u)^{dc} \\
& + \frac{9}{2}\delta^{pr}\delta^{sc}\delta^{td}\delta^{ab}g_L^4 + 8\delta^{pa}\delta^{rb}\delta^{st}\delta^{cd}g_s^4 - \frac{1}{4}\delta^{pa}\delta^{rb}\delta^{td}(Y_u^\dagger Y_d Y_d^\dagger Y_u)^{sc} - \frac{1}{4}\delta^{pa}\delta^{rb}\delta^{sc}(Y_u^\dagger Y_d Y_d^\dagger Y_u)^{dt} - \frac{1}{4}\delta^{pa}\delta^{rb}\delta^{td}(Y_u^\dagger Y_u Y_u^\dagger Y_u)^{sc} \\
& - \frac{1}{4}\delta^{pa}\delta^{rb}\delta^{sc}(Y_u^\dagger Y_u Y_u^\dagger Y_u)^{dt} - \frac{1}{4}\delta^{rb}\delta^{sc}\delta^{td}(Y_e Y_e^\dagger Y_e Y_e^\dagger)^{pa} - \frac{1}{4}\delta^{pa}\delta^{sc}\delta^{td}(Y_e Y_e^\dagger Y_e Y_e^\dagger)^{br} - \frac{3}{4}\text{T}_2\delta^{rb}\delta^{sc}\delta^{td}(Y_e Y_e^\dagger)^{pa} - \frac{3}{4}\text{T}_2\delta^{pa}\delta^{sc}\delta^{td}(Y_e Y_e^\dagger)^{br} \\
& - g_s^2 \left( \frac{16}{3}\delta^{pa}\delta^{rb}\delta^{td}(Y_u^\dagger Y_u)^{sc} + \frac{16}{3}\delta^{pa}\delta^{rb}\delta^{sc}(Y_u^\dagger Y_u)^{dt} \right) - \delta^{rb}\delta^{td}(Y_u^\dagger Y_u)^{sc}(Y_e Y_e^\dagger)^{pa} - \delta^{pa}\delta^{sc}(Y_u^\dagger Y_u)^{dt}(Y_e Y_e^\dagger)^{br} - g_Y^2 \left( \frac{23}{72}\delta^{pa}\delta^{rb}\delta^{td}(Y_u^\dagger Y_u)^{sc} \right. \\
& + \frac{23}{72}\delta^{pa}\delta^{rb}\delta^{sc}(Y_u^\dagger Y_u)^{dt} + \frac{4}{3}\delta^{pr}\delta^{sc}\delta^{td}(Y_e Y_e^\dagger)^{ba} + \frac{57}{16}\delta^{rb}\delta^{sc}\delta^{td}(Y_e Y_e^\dagger)^{pa} + \frac{57}{16}\delta^{pa}\delta^{sc}\delta^{td}(Y_e Y_e^\dagger)^{br} + 4\delta^{pa}\delta^{rb}\delta^{st}(Y_u^\dagger Y_u)^{dc} \Big) - \frac{3}{2}\text{T}_2\delta^{pa}\delta^{rb}\delta^{td}(Y_u^\dagger Y_u)^{sc} \\
& - \frac{3}{2}\text{T}_2\delta^{pa}\delta^{rb}\delta^{sc}(Y_u^\dagger Y_u)^{dt} - \frac{5}{2}\delta^{pa}\delta^{rb}(Y_u^\dagger Y_u)^{sc}(Y_u^\dagger Y_u)^{dt} - \frac{5}{2}\delta^{sc}\delta^{td}(Y_e Y_e^\dagger)^{pa}(Y_e Y_e^\dagger)^{br} - \frac{11}{4}\delta^{rb}\delta^{sc}(Y_u^\dagger Y_u)^{dt}(Y_e Y_e^\dagger)^{pa} \\
& - \frac{11}{4}\delta^{pa}\delta^{td}(Y_u^\dagger Y_u)^{sc}(Y_e Y_e^\dagger)^{br} \Big\} C_{\ell u}^{abcd} + \left\{ \frac{4}{3}\delta^{pa}\delta^{rb}\delta^{st}g_Y^2(Y_d^\dagger Y_d)^{dc} + \frac{584}{81}\delta^{pa}\delta^{rb}\delta^{st}\delta^{cd}g_Y^4 + 8\delta^{pa}\delta^{rb}\delta^{st}\delta^{cd}g_s^4 - \frac{1}{2}\delta^{pa}\delta^{rb}(Y_d^\dagger Y_u)^{dt}(Y_u^\dagger Y_d)^{sc} \right. \\
& - 3\delta^{pa}\delta^{rb}(Y_d^\dagger Y_d)^{dc}(Y_u^\dagger Y_u)^{st} - \frac{32}{9}\delta^{pa}\delta^{rb}\delta^{st}\delta^{cd}g_Y^2g_s^2 \Big\} C_{\ell d}^{abcd} - \frac{3}{2}Y_e^{*rd}Y_u^{*as}C_{qe}^{abcd}Y_e^{pc}Y_u^{bt} + \left\{ g_Y^2 \left( 2\delta^{pr}\delta^{sc}\delta^{td}(Y_u Y_u^\dagger)^{ba} - \frac{2}{27}\delta^{pr}\delta^{sc}Y_u^{*ad}Y_u^{bt} \right. \right. \\
& - \frac{2}{27}\delta^{pr}\delta^{td}Y_u^{*as}Y_u^{bc} \Big) + \frac{3}{2}\delta^{sc}\delta^{td}(Y_d Y_d^\dagger)^{ba}(Y_e Y_e^\dagger)^{pr} + \frac{1172}{243}\delta^{pr}\delta^{sc}\delta^{td}\delta^{ab}g_Y^4 + \frac{27}{2}\delta^{pr}\delta^{sc}\delta^{td}\delta^{ab}g_L^4 - \frac{3}{2}\delta^{pr}\delta^{sc}\delta^{td}\delta^{ab}g_Y^2g_L^2 \\
& - \frac{3}{2}\delta^{sc}\delta^{td}(Y_e Y_e^\dagger)^{pr}(Y_u Y_u^\dagger)^{ba} - \frac{8}{3}\delta^{pr}\delta^{sc}\delta^{td}\delta^{ab}g_Y^2g_s^2 \Big\} C_{qu}^{abcd} + \left\{ \frac{1}{2}\delta^{sc}\delta^{td}(Y_d Y_d^\dagger)^{ba}(Y_e Y_e^\dagger)^{pr} + g_Y^2g_s^2 \left( \frac{8}{27}\delta^{pr}\delta^{st}\delta^{ab}\delta^{cd} + \frac{1448}{243}\delta^{pr}\delta^{sc}\delta^{td}\delta^{ab} \right) \right. \\
& + g_Y^2 \left( \frac{2}{9}\delta^{pr}\delta^{sc}\delta^{td}(Y_u Y_u^\dagger)^{ba} + \frac{10}{9}\delta^{pr}\delta^{sc}Y_u^{*ad}Y_u^{bt} + \frac{10}{9}\delta^{pr}\delta^{td}Y_u^{*as}Y_u^{bc} - \frac{4}{9}\delta^{pr}\delta^{cd}Y_u^{*as}Y_u^{bt} \right) + \frac{1172}{729}\delta^{pr}\delta^{sc}\delta^{td}\delta^{ab}g_Y^4 + \frac{9}{2}\delta^{pr}\delta^{sc}\delta^{td}\delta^{ab}g_L^4 \\
& - \frac{1}{2}\delta^{pr}\delta^{sc}\delta^{td}\delta^{ab}g_Y^2g_L^2 - \frac{1}{2}\delta^{sc}\delta^{td}(Y_e Y_e^\dagger)^{pr}(Y_u Y_u^\dagger)^{ba} \Big\} C_{qu}^{(\times)abcd} + \left\{ \frac{16}{9}\delta^{st}\delta^{ad}g_Y^2Y_e^{*rb}Y_e^{pc} - \frac{32}{27}\delta^{pr}\delta^{st}\delta^{ab}\delta^{cd}g_Y^4 \right\} C_{ee}^{abcd} + \left\{ g_Y^2g_s^2 \left( \frac{8}{27}\delta^{pr}\delta^{st}\delta^{ad}\delta^{bc} \right. \right. \\
& - \frac{304}{243}\delta^{pr}\delta^{sa}\delta^{td}\delta^{bc} - 8\delta^{pr}\delta^{sa}\delta^{tb}\delta^{cd} \Big) + g_Y^4 \left( \frac{992}{729}\delta^{pr}\delta^{sa}\delta^{td}\delta^{bc} + \frac{944}{243}\delta^{pr}\delta^{sa}\delta^{tb}\delta^{cd} - \frac{128}{81}\delta^{pr}\delta^{st}\delta^{ad}\delta^{bc} \right) + g_Y^2 \left( \frac{34}{9}\delta^{pr}\delta^{sa}\delta^{td}(Y_u^\dagger Y_u)^{bc} \right. \\
& + 6\delta^{pr}\delta^{sa}\delta^{tb}(Y_u^\dagger Y_u)^{dc} \Big) + 3\delta^{sa}\delta^{td}(Y_u^\dagger Y_u)^{bc}(Y_e Y_e^\dagger)^{pr} + 3\delta^{sa}\delta^{tb}(Y_u^\dagger Y_u)^{dc}(Y_e Y_e^\dagger)^{pr} \Big\} C_{uu}^{abcd} - \frac{32}{81}\delta^{pr}\delta^{st}\delta^{ad}\delta^{bc}g_Y^4 C_{dd}^{abcd} + \left\{ \frac{3}{2}\text{T}_2\delta^{sc}\delta^{td}Y_e^{*rb}Y_e^{pa} \right. \\
& + \frac{3}{2}\delta^{sc}\delta^{td}Y_e^{pa}(Y_e^\dagger Y_e Y_e^\dagger)^{rb} + \frac{3}{2}\delta^{sc}\delta^{td}Y_e^{*rb}(Y_e Y_e^\dagger Y_e)^{pa} - \frac{1}{2}\delta^{sc}\delta^{td}(Y_e^\dagger Y_e)^{ba}(Y_e Y_e^\dagger)^{pr} - g_Y^2 \left( \frac{5}{3}\delta^{pr}\delta^{sc}\delta^{td}(Y_e^\dagger Y_e)^{ba} + \frac{47}{8}\delta^{sc}\delta^{td}Y_e^{*rb}Y_e^{pa} \right) \\
& - \frac{5}{4}\delta^{td}Y_e^{*rb}Y_e^{pa}(Y_u^\dagger Y_u)^{sc} - \frac{5}{4}\delta^{sc}Y_e^{*rb}Y_e^{pa}(Y_u^\dagger Y_u)^{dt} - \frac{1001}{243}\delta^{pr}\delta^{sc}\delta^{td}\delta^{ab}g_Y^4 - \frac{33}{8}\delta^{sc}\delta^{td}g_L^2Y_e^{*rb}Y_e^{pa} \Big\} C_{eu}^{abcd} + \left\{ \frac{8}{3}\delta^{pr}\delta^{sa}\delta^{tb}\delta^{cd}g_Y^2g_s^2 \right.
\end{aligned}$$

$$\begin{aligned}
& -\delta^{pr}\delta^{sa}\delta^{tb}g_Y^2(Y_d^\dagger Y_d)^{dc} - \frac{3}{2}\delta^{sa}\delta^{tb}(Y_d^\dagger Y_d)^{dc}(Y_e Y_e^\dagger)^{pr} - \frac{1019}{243}\delta^{pr}\delta^{sa}\delta^{tb}\delta^{cd}g_Y^4 \Big\} C_{ud}^{(\parallel)abcd} + \left\{ g_Y^2 g_s^2 \left( \frac{4}{27}\delta^{pr}\delta^{st}\delta^{ab}\delta^{cd} + \frac{580}{243}\delta^{pr}\delta^{sa}\delta^{tb}\delta^{cd} \right) \right. \\
& - \frac{1}{3}\delta^{pr}\delta^{sa}\delta^{tb}g_Y^2(Y_d^\dagger Y_d)^{dc} - \frac{1}{2}\delta^{sa}\delta^{tb}(Y_d^\dagger Y_d)^{dc}(Y_e Y_e^\dagger)^{pr} - \frac{1019}{729}\delta^{pr}\delta^{sa}\delta^{tb}\delta^{cd}g_Y^4 \Big\} C_{ud}^{(\times)abcd} + \left\{ \frac{3}{8}\delta^{pa}Y_e^{*rb}Y_u^{dt}(Y_u^\dagger Y_d)^{sc} - \frac{3}{4}\delta^{pa}Y_e^{*rb}Y_d^{dc}(Y_u^\dagger Y_u)^{st} \right. \\
& - \frac{10}{9}\delta^{pa}\delta^{st}g_Y^2Y_e^{*rb}Y_d^{dc} \Big\} C_{ledq}^{abcd} + C_{ledq}^{*abcd} \left\{ \frac{3}{8}\delta^{ra}Y_u^{*ds}Y_e^{pb}(Y_d^\dagger Y_u)^{ct} - \frac{3}{4}\delta^{ra}Y_d^{*dc}Y_e^{pb}(Y_u^\dagger Y_u)^{st} - \frac{10}{9}\delta^{ra}\delta^{st}g_Y^2Y_d^{*dc}Y_e^{pb} \right\} + \left\{ g_Y^2 \left( \frac{1}{9}\delta^{pr}\delta^{tb}Y_d^{*cd}Y_u^{*as} \right. \right. \\
& - \frac{7}{108}\delta^{pr}\delta^{tb}Y_d^{*ad}Y_u^{*cs} \Big) - \frac{1}{8}\delta^{tb}Y_d^{*ad}Y_u^{*cs}(Y_e Y_e^\dagger)^{pr} - \frac{3}{4}\delta^{tb}Y_d^{*cd}Y_u^{*as}(Y_e Y_e^\dagger)^{pr} \Big\} C_{quqd}^{(\parallel)abcd} + \left( C_{quqd}^{(\parallel)*} \right)^{abcd} \left\{ g_Y^2 \left( \frac{1}{9}\delta^{pr}\delta^{sb}Y_d^{cd}Y_u^{at} - \frac{7}{108}\delta^{pr}\delta^{sb}Y_d^{ad}Y_u^{ct} \right) \right. \\
& - \frac{1}{8}\delta^{sb}Y_d^{ad}Y_u^{ct}(Y_e Y_e^\dagger)^{pr} - \frac{3}{4}\delta^{sb}Y_d^{cd}Y_u^{at}(Y_e Y_e^\dagger)^{pr} \Big\} + \left\{ g_Y^2 \left( \frac{1}{27}\delta^{pr}\delta^{tb}Y_d^{*cd}Y_u^{*as} - \frac{7}{36}\delta^{pr}\delta^{tb}Y_d^{*ad}Y_u^{*cs} \right) - \frac{1}{4}\delta^{tb}Y_d^{*cd}Y_u^{*as}(Y_e Y_e^\dagger)^{pr} \right. \\
& - \frac{3}{8}\delta^{tb}Y_d^{*ad}Y_u^{*cs}(Y_e Y_e^\dagger)^{pr} \Big\} C_{quqd}^{(\times)abcd} + \left( C_{quqd}^{(\times)*} \right)^{abcd} \left\{ g_Y^2 \left( \frac{1}{27}\delta^{pr}\delta^{sb}Y_d^{cd}Y_u^{at} - \frac{7}{36}\delta^{pr}\delta^{sb}Y_d^{ad}Y_u^{ct} \right) - \frac{1}{4}\delta^{sb}Y_d^{cd}Y_u^{at}(Y_e Y_e^\dagger)^{pr} - \frac{3}{8}\delta^{sb}Y_d^{ad}Y_u^{ct}(Y_e Y_e^\dagger)^{pr} \right\} \\
& + \left\{ \frac{1}{8}\delta^{pa}\delta^{td}Y_e^{*rb}(Y_u^\dagger Y_u Y_u^\dagger)^{cs} + \frac{1}{4}T_2\delta^{pa}\delta^{td}Y_e^{*rb}Y_u^{*cs} + \frac{1}{4}\delta^{td}Y_e^{*ab}Y_u^{*cs}(Y_e Y_e^\dagger)^{pr} + \frac{1}{4}\delta^{pa}\delta^{td}Y_u^{*cs}(Y_e^\dagger Y_e Y_e^\dagger)^{rb} + \frac{3}{8}\delta^{pa}\delta^{td}Y_e^{*rb}(Y_d^\dagger Y_d Y_u^\dagger)^{cs} \right. \\
& + \frac{5}{8}\delta^{pa}Y_e^{*rb}Y_u^{*cs}(Y_u^\dagger Y_u)^{dt} + \frac{3}{4}\delta^{pa}Y_e^{*rb}Y_u^{*cd}(Y_u^\dagger Y_u)^{st} + \frac{15}{16}\delta^{pa}\delta^{td}g_L^2Y_e^{*rb}Y_u^{*cs} + g_Y^2 \left( \frac{10}{9}\delta^{pa}\delta^{st}Y_e^{*rb}Y_u^{*cd} + \frac{857}{144}\delta^{pa}\delta^{td}Y_e^{*rb}Y_u^{*cs} \right. \\
& - \frac{1}{27}\delta^{pr}\delta^{td}Y_e^{*ab}Y_u^{*cs} \Big) + \frac{5}{4}\delta^{td}Y_e^{*rb}Y_u^{*cs}(Y_e Y_e^\dagger)^{pa} + \frac{8}{3}\delta^{pa}\delta^{td}g_s^2Y_e^{*rb}Y_u^{*cs} \Big\} C_{lequ}^{abcd} + C_{lequ}^{*abcd} \left\{ \frac{1}{8}\delta^{ra}\delta^{sd}Y_e^{pb}(Y_u Y_u^\dagger Y_u)^{ct} + \frac{1}{4}T_2\delta^{ra}\delta^{sd}Y_e^{pb}Y_u^{ct} \right. \\
& + \frac{1}{4}\delta^{sd}Y_e^{ab}Y_u^{ct}(Y_e Y_e^\dagger)^{pr} + \frac{1}{4}\delta^{ra}\delta^{sd}Y_u^{ct}(Y_e Y_e^\dagger Y_e)^{pb} + \frac{3}{8}\delta^{ra}\delta^{sd}Y_e^{pb}(Y_d Y_d^\dagger Y_u)^{ct} + \frac{5}{8}\delta^{ra}Y_e^{pb}Y_u^{ct}(Y_u^\dagger Y_u)^{sd} + \frac{3}{4}\delta^{ra}Y_e^{pb}Y_u^{cd}(Y_u^\dagger Y_u)^{st} + \frac{15}{16}\delta^{ra}\delta^{sd}g_L^2Y_e^{pb}Y_u^{ct} \\
& + g_Y^2 \left( \frac{10}{9}\delta^{ra}\delta^{st}Y_e^{pb}Y_u^{cd} + \frac{857}{144}\delta^{ra}\delta^{sd}Y_e^{pb}Y_u^{ct} - \frac{1}{27}\delta^{pr}\delta^{sd}Y_e^{ab}Y_u^{ct} \right) + \frac{5}{4}\delta^{sd}Y_e^{pb}Y_u^{ct}(Y_e Y_e^\dagger)^{ar} + \frac{8}{3}\delta^{ra}\delta^{sd}g_s^2Y_e^{pb}Y_u^{ct} \Big\} + \left\{ \frac{9}{4}\delta^{pa}\delta^{tb}g_L^2Y_e^{*rd}Y_u^{*cs} \right. \\
& - \frac{1}{8}\delta^{pa}Y_e^{*rd}Y_u^{*cs}(Y_u^\dagger Y_u)^{bt} - \frac{1}{8}\delta^{tb}Y_e^{*ad}Y_u^{*cs}(Y_e Y_e^\dagger)^{pr} - \frac{1}{4}\delta^{tb}Y_e^{*rd}Y_u^{*cs}(Y_e Y_e^\dagger)^{pa} - \frac{3}{8}\delta^{pa}Y_e^{*rd}Y_u^{*cb}(Y_u^\dagger Y_u)^{st} - \frac{1}{2}\delta^{pa}\delta^{tb}Y_e^{*rd}(Y_d^\dagger Y_d Y_u^\dagger)^{cs} \\
& - \frac{1}{2}\delta^{pa}\delta^{tb}Y_e^{*rd}(Y_u^\dagger Y_u Y_u^\dagger)^{cs} - T_2\delta^{pa}\delta^{tb}Y_e^{*rd}Y_u^{*cs} - g_Y^2 \left( \frac{7}{108}\delta^{pr}\delta^{tb}Y_e^{*ad}Y_u^{*cs} + \frac{7}{18}\delta^{pa}\delta^{st}Y_e^{*rd}Y_u^{*cb} + \frac{133}{36}\delta^{pa}\delta^{tb}Y_e^{*rd}Y_u^{*cs} \right) \\
& - \delta^{pa}\delta^{tb}Y_u^{*cs}(Y_e^\dagger Y_e Y_e^\dagger)^{rd} - \frac{4}{3}\delta^{pa}\delta^{tb}g_s^2Y_e^{*rd}Y_u^{*cs} \Big\} C_{luqe}^{abcd} + C_{luqe}^{*abcd} \left\{ \frac{9}{4}\delta^{ra}\delta^{sb}g_L^2Y_e^{pd}Y_u^{ct} - \frac{1}{8}\delta^{ra}Y_e^{pd}Y_u^{ct}(Y_u^\dagger Y_u)^{sb} - \frac{1}{8}\delta^{sb}Y_e^{ad}Y_u^{ct}(Y_e Y_e^\dagger)^{pr} \right. \\
& - \frac{1}{4}\delta^{sb}Y_e^{pd}Y_u^{ct}(Y_e Y_e^\dagger)^{ar} - \frac{3}{8}\delta^{ra}Y_e^{pd}Y_u^{cb}(Y_u^\dagger Y_u)^{st} - \frac{1}{2}\delta^{ra}\delta^{sb}Y_e^{pd}(Y_d Y_d^\dagger Y_u)^{ct} - \frac{1}{2}\delta^{ra}\delta^{sb}Y_e^{pd}(Y_u Y_u^\dagger Y_u)^{ct} - T_2\delta^{ra}\delta^{sb}Y_e^{pd}Y_u^{ct} - g_Y^2 \left( \frac{7}{108}\delta^{pr}\delta^{sb}Y_e^{ad}Y_u^{ct} \right.
\end{aligned}$$

$$\begin{aligned}
& + \frac{7}{18} \delta^{ra} \delta^{st} Y_e^{pd} Y_u^{cb} + \frac{133}{36} \delta^{ra} \delta^{sb} Y_e^{pd} Y_u^{ct} - \delta^{ra} \delta^{sb} Y_u^{ct} (Y_e Y_e^\dagger Y_e)^{pd} - \frac{4}{3} \delta^{ra} \delta^{sb} g_s^2 Y_e^{pd} Y_u^{ct} \Bigg\} + \left\{ g_Y^2 g_L^2 \left( \frac{8}{27} \delta^{pr} \delta^{st} \delta^{ad} \delta^{bc} - \frac{4}{3} \delta^{pa} \delta^{rd} \delta^{st} \delta^{bc} \right. \right. \\
& - \frac{4}{3} \delta^{pa} \delta^{rb} \delta^{st} \delta^{cd} \Bigg) + g_Y^4 \left( \frac{20}{81} \delta^{pa} \delta^{rd} \delta^{st} \delta^{bc} + \frac{160}{81} \delta^{pa} \delta^{rb} \delta^{st} \delta^{cd} - \frac{16}{27} \delta^{pr} \delta^{st} \delta^{ad} \delta^{bc} \right) + g_Y^2 \left( \frac{8}{3} \delta^{pa} \delta^{rd} \delta^{st} (Y_e Y_e^\dagger)^{bc} + \frac{32}{9} \delta^{pa} \delta^{rb} \delta^{st} (Y_e Y_e^\dagger)^{dc} \right) \\
& + 2 \delta^{pa} \delta^{rb} (Y_u^\dagger Y_u)^{st} (Y_e Y_e^\dagger)^{dc} + 3 \delta^{pa} \delta^{rd} (Y_u^\dagger Y_u)^{st} (Y_e Y_e^\dagger)^{bc} \Bigg\} C_{\ell\ell}^{abcd} + \left\{ \frac{4}{9} \delta^{pr} \delta^{bc} g_Y^2 Y_u^{*as} Y_u^{dt} - \frac{16}{81} \delta^{pr} \delta^{st} \delta^{ad} \delta^{bc} g_Y^4 \right\} C_{qq}^{(\parallel)abcd} + \left\{ \frac{8}{9} \delta^{pr} \delta^{bc} g_Y^2 Y_u^{*as} Y_u^{dt} \right. \\
& - \frac{32}{81} \delta^{pr} \delta^{st} \delta^{ad} \delta^{bc} g_Y^4 \Bigg\} C_{qq}^{(\times)abcd} + \left\{ \frac{1}{2} \delta^{pa} \delta^{rb} Y_u^{dt} (Y_d^\dagger Y_d Y_u^\dagger)^{cs} + \frac{1}{2} \delta^{pa} \delta^{rb} Y_u^{*cs} (Y_d Y_d^\dagger Y_u)^{dt} + g_Y^2 \left( \frac{53}{36} \delta^{pa} \delta^{rb} Y_u^{*cs} Y_u^{dt} - \frac{8}{3} \delta^{pa} \delta^{rb} \delta^{st} (Y_u Y_u^\dagger)^{dc} \right) \right. \\
& + \frac{3}{2} \delta^{pa} \delta^{rb} Y_u^{dt} (Y_u^\dagger Y_u Y_u^\dagger)^{cs} + \frac{3}{2} \delta^{pa} \delta^{rb} Y_u^{*cs} (Y_u Y_u^\dagger Y_u)^{dt} + 2 \delta^{pa} \delta^{rb} \delta^{st} \delta^{cd} g_Y^2 g_L^2 + 3 T_2 \delta^{pa} \delta^{rb} Y_u^{*cs} Y_u^{dt} + 3 \delta^{pa} \delta^{rb} (Y_u^\dagger Y_u)^{st} (Y_d Y_d^\dagger)^{dc} \\
& + \frac{32}{9} \delta^{pa} \delta^{rb} \delta^{st} \delta^{cd} g_Y^2 g_s^2 + \frac{32}{3} \delta^{pa} \delta^{rb} g_s^2 Y_u^{*cs} Y_u^{dt} - \frac{5}{4} \delta^{rb} Y_u^{*cs} Y_u^{dt} (Y_e Y_e^\dagger)^{pa} - \frac{5}{4} \delta^{pa} Y_u^{*cs} Y_u^{dt} (Y_e Y_e^\dagger)^{br} - 3 \delta^{pa} \delta^{rb} (Y_u^\dagger Y_u)^{st} (Y_u Y_u^\dagger)^{dc} \\
& - \frac{392}{81} \delta^{pa} \delta^{rb} \delta^{st} \delta^{cd} g_Y^4 - \frac{51}{4} \delta^{pa} \delta^{rb} g_L^2 Y_u^{*cs} Y_u^{dt} - 16 \delta^{pa} \delta^{rb} \delta^{st} \delta^{cd} g_s^4 \Bigg\} C_{\ell q}^{(\parallel)abcd} + \left\{ \frac{1}{4} \delta^{pa} \delta^{rb} Y_u^{dt} (Y_d^\dagger Y_d Y_u^\dagger)^{cs} + \frac{1}{4} \delta^{pa} \delta^{rb} Y_u^{*cs} (Y_d Y_d^\dagger Y_u)^{dt} \right. \\
& + \frac{3}{4} \delta^{pa} \delta^{rb} Y_u^{dt} (Y_u^\dagger Y_u Y_u^\dagger)^{cs} + \frac{3}{4} \delta^{pa} \delta^{rb} Y_u^{*cs} (Y_u Y_u^\dagger Y_u)^{dt} + g_Y^2 g_L^2 \left( \frac{4}{9} \delta^{pr} \delta^{st} \delta^{ab} \delta^{cd} + 4 \delta^{pa} \delta^{rb} \delta^{st} \delta^{cd} \right) + g_Y^2 \left( \frac{53}{72} \delta^{pa} \delta^{rb} Y_u^{*cs} Y_u^{dt} - \frac{4}{3} \delta^{pa} \delta^{rb} \delta^{st} (Y_u Y_u^\dagger)^{dc} \right) \\
& + \frac{5}{4} \delta^{rb} Y_u^{*cs} Y_u^{dt} (Y_e Y_e^\dagger)^{pa} + \frac{5}{4} \delta^{pa} Y_u^{*cs} Y_u^{dt} (Y_e Y_e^\dagger)^{br} + \frac{3}{2} T_2 \delta^{pa} \delta^{rb} Y_u^{*cs} Y_u^{dt} + \frac{3}{2} \delta^{pa} \delta^{rb} (Y_u^\dagger Y_u)^{st} (Y_d Y_d^\dagger)^{dc} + \frac{16}{9} \delta^{pa} \delta^{rb} \delta^{st} \delta^{cd} g_Y^2 g_s^2 \\
& + \frac{15}{8} \delta^{pa} \delta^{rb} g_L^2 Y_u^{*cs} Y_u^{dt} + \frac{16}{3} \delta^{pa} \delta^{rb} g_s^2 Y_u^{*cs} Y_u^{dt} - \frac{3}{2} \delta^{pa} \delta^{rb} (Y_u^\dagger Y_u)^{st} (Y_u Y_u^\dagger)^{dc} - \frac{196}{81} \delta^{pa} \delta^{rb} \delta^{st} \delta^{cd} g_Y^4 - 8 \delta^{pa} \delta^{rb} \delta^{st} \delta^{cd} g_s^4 \Bigg\} C_{\ell q}^{(\times)abcd}, \tag{10.4}
\end{aligned}$$

### 10.3 $C_{\ell d}$

$$\begin{aligned}
\beta_{C_{\ell d}^{prst}}^{(1)} & = \left\{ 2 \delta^{pa} \delta^{rb} (Y_d^\dagger Y_d)^{st} - \frac{2}{9} \delta^{pa} \delta^{rb} \delta^{st} g_Y^2 \right\} C_{H\ell}^{(\parallel)ab} + \left\{ \delta^{pa} \delta^{rb} (Y_d^\dagger Y_d)^{st} - \frac{1}{9} \delta^{pa} \delta^{rb} \delta^{st} g_Y^2 \right\} C_{H\ell}^{(\times)ab} - \left\{ \frac{1}{3} \delta^{pr} \delta^{sa} \delta^{tb} g_Y^2 + \delta^{sa} \delta^{tb} (Y_e Y_e^\dagger)^{pr} \right\} C_{Hd}^{ab} \\
& + \frac{4}{9} \delta^{pa} \delta^{rb} \delta^{st} \delta^{cd} g_Y^2 C_{\ell e}^{abcd} - \frac{8}{9} \delta^{pa} \delta^{rb} \delta^{st} \delta^{cd} g_Y^2 C_{\ell u}^{abcd} + \left\{ \frac{1}{2} \left( \delta^{rb} \delta^{sc} \delta^{td} (Y_e Y_e^\dagger)^{pa} + \delta^{pa} \delta^{sc} \delta^{td} (Y_e Y_e^\dagger)^{br} + 2 \delta^{pa} \delta^{rb} \delta^{td} (Y_d^\dagger Y_d)^{sc} + 2 \delta^{pa} \delta^{rb} \delta^{sc} (Y_d^\dagger Y_d)^{dt} \right) \right. \\
& - \frac{2}{9} g_Y^2 \left( 9 \delta^{pa} \delta^{rb} \delta^{sc} \delta^{td} - 2 \delta^{pa} \delta^{rb} \delta^{st} \delta^{cd} - 3 \delta^{pr} \delta^{sc} \delta^{td} \delta^{ab} \right) \Bigg\} C_{\ell d}^{abcd} - \frac{2}{3} \delta^{pr} \delta^{sc} \delta^{td} \delta^{ab} g_Y^2 C_{qd}^{(\parallel)abcd} - \frac{2}{9} \delta^{pr} \delta^{sc} \delta^{td} \delta^{ab} g_Y^2 C_{qd}^{(\times)abcd} + \frac{4}{9} g_Y^2 \left\{ \delta^{pr} \delta^{sa} \delta^{td} \delta^{bc} \right. \\
& + 3 \delta^{pr} \delta^{sa} \delta^{tb} \delta^{cd} \Bigg\} C_{dd}^{abcd} + \left\{ \frac{2}{3} \delta^{pr} \delta^{sc} \delta^{td} \delta^{ab} g_Y^2 - \delta^{sc} \delta^{td} Y_e^{*rb} Y_e^{pa} \right\} C_{ed}^{abcd} - \frac{4}{3} \delta^{pr} \delta^{sc} \delta^{td} \delta^{ab} g_Y^2 C_{ud}^{(\parallel)abcd} - \frac{4}{9} \delta^{pr} \delta^{sc} \delta^{td} \delta^{ab} g_Y^2 C_{ud}^{(\times)abcd}
\end{aligned}$$

$$\begin{aligned}
& -\frac{1}{2}\delta^{pa}\delta^{sc}Y_e^{*rb}C_{\ell edq}^{abcd}Y_d^{dt}-\frac{1}{2}\delta^{ra}\delta^{tc}C_{\ell edq}^{*abcd}Y_d^{*ds}Y_e^{pb}+\frac{4}{9}g_Y^2\left\{\delta^{pa}\delta^{rd}\delta^{st}\delta^{bc}+2\delta^{pa}\delta^{rb}\delta^{st}\delta^{cd}\right\}C_{\ell\ell}^{abcd}-\left\{\frac{4}{9}\delta^{pa}\delta^{rb}\delta^{st}\delta^{cd}g_Y^2\right. \\
& \left.+2\delta^{pa}\delta^{rb}Y_d^{*cs}Y_d^{dt}\right\}C_{\ell q}^{(\parallel)abcd}-\left\{\frac{2}{9}\delta^{pa}\delta^{rb}\delta^{st}\delta^{cd}g_Y^2+\delta^{pa}\delta^{rb}Y_d^{*cs}Y_d^{dt}\right\}C_{\ell q}^{(\times)abcd}, \tag{10.5}
\end{aligned}$$

$$\begin{aligned}
\beta_{C_{\ell d}^{prst}}^{(2)} &= \frac{11}{9}\delta^{st}g_Y^2(C_{\ell HH}C_{\ell HH}^\dagger)^{rp}+3(Y_d^\dagger Y_d)^{st}(C_{\ell HH}C_{\ell HH}^\dagger)^{rp}+\left\{\frac{4}{9}\delta^{pr}\delta^{st}g_Y^6-g_Y^4\left(\frac{1}{3}\delta^{st}(Y_eY_e^\dagger)^{pr}+\frac{7}{3}\delta^{pr}(Y_d^\dagger Y_d)^{st}\right)\right\}C_{HB}+\left\{\frac{1}{3}\delta^{pr}\delta^{st}g_Y^4g_L^2\right. \\
& +g_Y^2g_L^2\left(\frac{3}{4}\delta^{st}(Y_eY_e^\dagger)^{pr}-\frac{3}{4}\delta^{pr}(Y_d^\dagger Y_d)^{st}\right)\left\}C_{HWB}+\frac{10}{3}\delta^{pr}\delta^{st}g_Y^2g_L^6C_W+\frac{80}{9}\delta^{pr}\delta^{st}g_Y^2g_s^6C_G+\left\{g_Y^4\left(\frac{7}{6}\delta^{pa}\delta^{st}Y_e^{*rb}-\frac{2}{3}\delta^{pr}\delta^{st}Y_e^{*ab}\right)\right. \\
& \left.+g_Y^2\left(\frac{2}{3}\delta^{st}Y_e^{*rb}(Y_eY_e^\dagger)^{pa}+\frac{3}{2}\delta^{pa}Y_e^{*rb}(Y_d^\dagger Y_d)^{st}\right)\right\}C_{eB}^{ab}+C_{eB}^{*ab}\left\{g_Y^4\left(\frac{7}{6}\delta^{ra}\delta^{st}Y_e^{pb}-\frac{2}{3}\delta^{pr}\delta^{st}Y_e^{ab}\right)+g_Y^2\left(\frac{2}{3}\delta^{st}Y_e^{pb}(Y_eY_e^\dagger)^{ar}+\frac{3}{2}\delta^{ra}Y_e^{pb}(Y_d^\dagger Y_d)^{st}\right)\right\} \\
& -\left\{\frac{5}{12}\delta^{pa}\delta^{st}g_Y^2g_L^2Y_e^{*rb}+\frac{9}{4}\delta^{pa}g_L^2Y_e^{*rb}(Y_d^\dagger Y_d)^{st}\right\}C_{eW}^{ab}-C_{eW}^{*ab}\left\{\frac{5}{12}\delta^{ra}\delta^{st}g_Y^2g_L^2Y_e^{pb}+\frac{9}{4}\delta^{ra}g_L^2Y_e^{pb}(Y_d^\dagger Y_d)^{st}\right\}+\frac{10}{9}\delta^{pr}\delta^{st}g_Y^4Y_u^{*ab}C_{uB}^{ab} \\
& +\frac{10}{9}\delta^{pr}\delta^{st}g_Y^4C_{uB}^{*ab}Y_u^{ab}+\left\{g_Y^4\left(\frac{17}{27}\delta^{pr}\delta^{tb}Y_d^{*as}-\frac{2}{9}\delta^{pr}\delta^{st}Y_d^{*ab}\right)+g_Y^2\left(\delta^{pr}Y_d^{*as}(Y_d^\dagger Y_d)^{bt}+\delta^{tb}Y_d^{*as}(Y_eY_e^\dagger)^{pr}\right)+\frac{16}{3}\delta^{pr}\delta^{tb}g_Y^2g_s^2Y_d^{*as}\right\}C_{dB}^{ab} \\
& +C_{dB}^{*ab}\left\{g_Y^4\left(\frac{17}{27}\delta^{pr}\delta^{sb}Y_d^{at}-\frac{2}{9}\delta^{pr}\delta^{st}Y_d^{ab}\right)+g_Y^2\left(\delta^{pr}Y_d^{at}(Y_d^\dagger Y_d)^{sb}+\delta^{sb}Y_d^{at}(Y_eY_e^\dagger)^{pr}\right)+\frac{16}{3}\delta^{pr}\delta^{sb}g_Y^2g_s^2Y_d^{at}\right\}+\left\{\frac{1}{6}\delta^{pr}\delta^{tb}g_Y^2g_L^2Y_d^{*as}\right. \\
& \left.+\frac{9}{2}\delta^{pr}\delta^{tb}g_L^4Y_d^{*as}\right\}C_{dW}^{ab}+C_{dW}^{*ab}\left\{\frac{1}{6}\delta^{pr}\delta^{sb}g_Y^2g_L^2Y_d^{at}+\frac{9}{2}\delta^{pr}\delta^{sb}g_L^4Y_d^{at}\right\}+\left\{\frac{28}{27}\delta^{pr}\delta^{tb}g_Y^2g_s^2Y_d^{*as}-4\delta^{tb}g_s^2Y_d^{*as}(Y_eY_e^\dagger)^{pr}\right\}C_{dG}^{ab} \\
& +C_{dG}^{*ab}\left\{\frac{28}{27}\delta^{pr}\delta^{sb}g_Y^2g_s^2Y_d^{at}-4\delta^{sb}g_s^2Y_d^{at}(Y_eY_e^\dagger)^{pr}\right\}+\left\{\frac{1}{4}\delta^{rb}(Y_d^\dagger Y_d)^{st}(Y_eY_e^\dagger)^{pa}+\frac{1}{4}\delta^{pa}(Y_d^\dagger Y_d)^{st}(Y_eY_e^\dagger)^{br}+g_Y^2\left(\frac{2}{9}T_2\delta^{pa}\delta^{rb}\delta^{st}\right.\right. \\
& \left.+\frac{253}{36}\delta^{pa}\delta^{rb}(Y_d^\dagger Y_d)^{st}-\frac{1}{108}\delta^{rb}\delta^{st}(Y_eY_e^\dagger)^{pa}-\frac{1}{108}\delta^{pa}\delta^{st}(Y_eY_e^\dagger)^{br}\right)+\frac{51}{4}\delta^{pa}\delta^{rb}g_L^2(Y_d^\dagger Y_d)^{st}-\frac{82}{81}\delta^{pa}\delta^{rb}\delta^{st}g_Y^4-2\delta^{pa}\delta^{rb}\delta^{st}g_Y^2g_L^2 \\
& -2T_2\delta^{pa}\delta^{rb}(Y_d^\dagger Y_d)^{st}-3\delta^{pa}\delta^{rb}(Y_d^\dagger Y_dY_d^\dagger Y_d)^{st}-\frac{32}{3}\delta^{pa}\delta^{rb}g_s^2(Y_d^\dagger Y_d)^{st}\left\}C_{H\ell}^{(\parallel)ab}+\left\{\frac{1}{2}\delta^{rb}(Y_d^\dagger Y_d)^{st}(Y_eY_e^\dagger)^{pa}+\frac{1}{2}\delta^{pa}(Y_d^\dagger Y_d)^{st}(Y_eY_e^\dagger)^{br}\right. \\
& \left.+g_Y^2\left(\frac{1}{9}\delta^{st}\delta^{ab}(Y_eY_e^\dagger)^{pr}+\frac{2}{9}\delta^{pa}\delta^{rb}\delta^{st}\text{Tr}[Y_e^\dagger Y_e]+\frac{1}{3}\delta^{pa}\delta^{rb}\delta^{st}\text{Tr}[Y_d^\dagger Y_d]+\frac{1}{3}\delta^{pa}\delta^{rb}\delta^{st}\text{Tr}[Y_u^\dagger Y_u]+\frac{253}{72}\delta^{pa}\delta^{rb}(Y_d^\dagger Y_d)^{st}-\frac{13}{54}\delta^{rb}\delta^{st}(Y_eY_e^\dagger)^{pa}\right.\right. \\
& \left.-\frac{13}{54}\delta^{pa}\delta^{st}(Y_eY_e^\dagger)^{br}\right)+\frac{87}{8}\delta^{pa}\delta^{rb}g_L^2(Y_d^\dagger Y_d)^{st}-\frac{41}{81}\delta^{pa}\delta^{rb}\delta^{st}g_Y^4-g_Y^2g_L^2\left(\frac{1}{27}\delta^{pr}\delta^{st}\delta^{ab}+\frac{25}{18}\delta^{pa}\delta^{rb}\delta^{st}\right)-T_2\delta^{pa}\delta^{rb}(Y_d^\dagger Y_d)^{st}
\end{aligned}$$

$$\begin{aligned}
& -\frac{3}{2}\delta^{pa}\delta^{rb}(Y_d^\dagger Y_d Y_d^\dagger Y_d)^{st} - \frac{16}{3}\delta^{pa}\delta^{rb}g_s^2(Y_d^\dagger Y_d)^{st} \Big\} C_{H\ell}^{(\times)ab} + \left\{ T_2\delta^{sa}\delta^{tb}(Y_e Y_e^\dagger)^{pr} + g_Y^2 \left( \frac{1}{3}T_2\delta^{pr}\delta^{sa}\delta^{tb} - \frac{73}{108}\delta^{pr}\delta^{tb}(Y_d^\dagger Y_d)^{sa} \right. \right. \\
& - \frac{73}{108}\delta^{pr}\delta^{sa}(Y_d^\dagger Y_d)^{bt} - \frac{121}{24}\delta^{sa}\delta^{tb}(Y_e Y_e^\dagger)^{pr} \Big) + 3\delta^{sa}\delta^{tb}(Y_e Y_e^\dagger Y_e Y_e^\dagger)^{pr} - \frac{1}{4}\delta^{tb}(Y_d^\dagger Y_d)^{sa}(Y_e Y_e^\dagger)^{pr} - \frac{1}{4}\delta^{sa}(Y_d^\dagger Y_d)^{bt}(Y_e Y_e^\dagger)^{pr} - \frac{853}{486}\delta^{pr}\delta^{sa}\delta^{tb}g_Y^4 \\
& - 3\delta^{pr}\delta^{sa}\delta^{tb}g_Y^2g_L^2 - \frac{33}{8}\delta^{sa}\delta^{tb}g_L^2(Y_e Y_e^\dagger)^{pr} \Big\} C_{Hd}^{ab} + \left\{ \frac{59}{108}\delta^{pr}\delta^{tb}g_Y^2(Y_d^\dagger Y_u)^{sa} + \frac{3}{4}\delta^{tb}(Y_d^\dagger Y_u)^{sa}(Y_e Y_e^\dagger)^{pr} \right\} C_{Hud}^{ab} \\
& + C_{Hud}^{*ab} \left\{ \frac{59}{108}\delta^{pr}\delta^{sb}g_Y^2(Y_u^\dagger Y_d)^{at} + \frac{3}{4}\delta^{sb}(Y_u^\dagger Y_d)^{at}(Y_e Y_e^\dagger)^{pr} \right\} + \left\{ \frac{50}{81}\delta^{pa}\delta^{rb}\delta^{st}\delta^{cd}g_Y^4 + \delta^{pa}\delta^{rb}(Y_d^\dagger Y_d)^{st}(Y_e^\dagger Y_e)^{dc} - g_Y^2 \left( \frac{10}{27}\delta^{pa}\delta^{st}Y_e^{*rd}Y_e^{bc} \right. \right. \\
& + \frac{10}{27}\delta^{rb}\delta^{st}Y_e^{*ad}Y_e^{pc} + \frac{10}{9}\delta^{pa}\delta^{rb}\delta^{st}(Y_e^\dagger Y_e)^{dc} \Big) \Big\} C_{\ell e}^{abcd} + \left\{ 2\delta^{pa}\delta^{rb}\delta^{st}g_Y^2(Y_u^\dagger Y_u)^{dc} + 8\delta^{pa}\delta^{rb}\delta^{st}\delta^{cd}g_s^4 - \frac{1}{2}\delta^{pa}\delta^{rb}(Y_d^\dagger Y_u)^{sc}(Y_u^\dagger Y_d)^{dt} \right. \\
& - 3\delta^{pa}\delta^{rb}(Y_d^\dagger Y_d)^{st}(Y_u^\dagger Y_u)^{dc} - \frac{280}{81}\delta^{pa}\delta^{rb}\delta^{st}\delta^{cd}g_Y^4 - \frac{32}{9}\delta^{pa}\delta^{rb}\delta^{st}\delta^{cd}g_Y^2g_s^2 \Big\} C_{\ell u}^{abcd} + \left\{ \frac{1}{2}\delta^{sc}\delta^{td}(Y_e Y_e^\dagger)^{pr}(Y_e Y_e^\dagger)^{ba} + g_Y^2g_L^2 \left( \frac{3}{2}\delta^{pr}\delta^{sc}\delta^{td}\delta^{ab} \right. \right. \\
& + \frac{9}{2}\delta^{pa}\delta^{rb}\delta^{sc}\delta^{td} \Big) + g_Y^4 \left( \frac{14}{81}\delta^{pa}\delta^{rb}\delta^{st}\delta^{cd} + \frac{418}{243}\delta^{pr}\delta^{sc}\delta^{td}\delta^{ab} + \frac{475}{18}\delta^{pa}\delta^{rb}\delta^{sc}\delta^{td} \right) + g_Y^2g_s^2 \left( \frac{16}{9}\delta^{pa}\delta^{rb}\delta^{st}\delta^{cd} + 8\delta^{pa}\delta^{rb}\delta^{sc}\delta^{td} \right) \\
& + g_L^2 \left( \frac{33}{16}\delta^{rb}\delta^{sc}\delta^{td}(Y_e Y_e^\dagger)^{pa} + \frac{33}{16}\delta^{pa}\delta^{sc}\delta^{td}(Y_e Y_e^\dagger)^{br} + \frac{51}{8}\delta^{pa}\delta^{rb}\delta^{td}(Y_d^\dagger Y_d)^{sc} + \frac{51}{8}\delta^{pa}\delta^{rb}\delta^{sc}(Y_d^\dagger Y_d)^{dt} \right) + g_Y^2 \left( \frac{61}{72}\delta^{pa}\delta^{rb}\delta^{td}(Y_d^\dagger Y_d)^{sc} \right. \\
& + \frac{61}{72}\delta^{pa}\delta^{rb}\delta^{sc}(Y_d^\dagger Y_d)^{dt} + \frac{39}{16}\delta^{rb}\delta^{sc}\delta^{td}(Y_e Y_e^\dagger)^{pa} + \frac{39}{16}\delta^{pa}\delta^{sc}\delta^{td}(Y_e Y_e^\dagger)^{br} - \frac{2}{3}\delta^{pa}\delta^{rb}\delta^{st}(Y_d^\dagger Y_d)^{dc} - \frac{4}{3}\delta^{pr}\delta^{sc}\delta^{td}(Y_e Y_e^\dagger)^{ba} \Big) + 2\delta^{rb}\delta^{sc}(Y_d^\dagger Y_d)^{dt}(Y_e Y_e^\dagger)^{pa} \\
& + 2\delta^{pa}\delta^{td}(Y_d^\dagger Y_d)^{sc}(Y_e Y_e^\dagger)^{br} + 3\delta^{pa}\delta^{rb}(Y_d^\dagger Y_d)^{st}(Y_d^\dagger Y_d)^{dc} + \frac{9}{2}\delta^{pr}\delta^{sc}\delta^{td}\delta^{ab}g_L^4 + 8\delta^{pa}\delta^{rb}\delta^{st}\delta^{cd}g_s^4 - \frac{1}{4}\delta^{pa}\delta^{rb}\delta^{td}(Y_d^\dagger Y_d Y_d^\dagger Y_d)^{sc} \\
& - \frac{1}{4}\delta^{pa}\delta^{rb}\delta^{sc}(Y_d^\dagger Y_d Y_d^\dagger Y_d)^{dt} - \frac{1}{4}\delta^{pa}\delta^{rb}\delta^{td}(Y_d^\dagger Y_u Y_u^\dagger Y_d)^{sc} - \frac{1}{4}\delta^{pa}\delta^{rb}\delta^{sc}(Y_d^\dagger Y_u Y_u^\dagger Y_d)^{dt} - \frac{1}{4}\delta^{rb}\delta^{sc}\delta^{td}(Y_e Y_e^\dagger Y_e Y_e^\dagger)^{pa} - \frac{1}{4}\delta^{pa}\delta^{sc}\delta^{td}(Y_e Y_e^\dagger Y_e Y_e^\dagger)^{br} \\
& - \frac{3}{4}T_2\delta^{rb}\delta^{sc}\delta^{td}(Y_e Y_e^\dagger)^{pa} - \frac{3}{4}T_2\delta^{pa}\delta^{sc}\delta^{td}(Y_e Y_e^\dagger)^{br} - g_s^2 \left( \frac{16}{3}\delta^{pa}\delta^{rb}\delta^{td}(Y_d^\dagger Y_d)^{sc} + \frac{16}{3}\delta^{pa}\delta^{rb}\delta^{sc}(Y_d^\dagger Y_d)^{dt} \right) - \frac{3}{2}T_2\delta^{pa}\delta^{rb}\delta^{td}(Y_d^\dagger Y_d)^{sc} \\
& - \frac{3}{2}T_2\delta^{pa}\delta^{rb}\delta^{sc}(Y_d^\dagger Y_d)^{dt} - \frac{7}{4}\delta^{rb}\delta^{td}(Y_d^\dagger Y_d)^{sc}(Y_e Y_e^\dagger)^{pa} - \frac{7}{4}\delta^{pa}\delta^{sc}(Y_d^\dagger Y_d)^{dt}(Y_e Y_e^\dagger)^{br} - \frac{5}{2}\delta^{pa}\delta^{rb}(Y_d^\dagger Y_d)^{sc}(Y_d^\dagger Y_d)^{dt} - \frac{5}{2}\delta^{sc}\delta^{td}(Y_e Y_e^\dagger)^{pa}(Y_e Y_e^\dagger)^{br} \Big\} C_{\ell d}^{abcd} \\
& - Y_d^{*as}Y_e^{*rd}C_{qe}^{abcd}Y_d^{bt}Y_e^{pc} + \left\{ g_Y^2 \left( \frac{10}{27}\delta^{pr}\delta^{sc}Y_d^{*ad}Y_d^{bt} + \frac{10}{27}\delta^{pr}\delta^{td}Y_d^{*as}Y_d^{bc} + 2\delta^{pr}\delta^{sc}\delta^{td}(Y_u Y_u^\dagger)^{ba} \right) + \frac{3}{2}\delta^{sc}\delta^{td}(Y_d Y_d^\dagger)^{ba}(Y_e Y_e^\dagger)^{pr} + \frac{27}{2}\delta^{pr}\delta^{sc}\delta^{td}\delta^{ab}g_L^4 \right. \\
& - \frac{220}{243}\delta^{pr}\delta^{sc}\delta^{td}\delta^{ab}g_Y^4 - \frac{3}{2}\delta^{pr}\delta^{sc}\delta^{td}\delta^{ab}g_Y^2g_L^2 - \frac{3}{2}\delta^{sc}\delta^{td}(Y_e Y_e^\dagger)^{pr}(Y_u Y_u^\dagger)^{ba} - \frac{8}{3}\delta^{pr}\delta^{sc}\delta^{td}\delta^{ab}g_Y^2g_s^2 \Big\} C_{qd}^{(\parallel)abcd} + \left\{ \frac{1}{2}\delta^{sc}\delta^{td}(Y_d Y_d^\dagger)^{ba}(Y_e Y_e^\dagger)^{pr} \right. \\
& + g_Y^2g_s^2 \left( \frac{140}{243}\delta^{pr}\delta^{sc}\delta^{td}\delta^{ab} - \frac{4}{27}\delta^{pr}\delta^{st}\delta^{ab}\delta^{cd} \right) + g_Y^2 \left( \frac{2}{9}\delta^{pr}\delta^{cd}Y_d^{*as}Y_d^{bt} + \frac{2}{9}\delta^{pr}\delta^{sc}\delta^{td}(Y_d Y_d^\dagger)^{ba} + \frac{4}{9}\delta^{pr}\delta^{sc}Y_d^{*ad}Y_d^{bt} + \frac{4}{9}\delta^{pr}\delta^{td}Y_d^{*as}Y_d^{bc} \right.
\end{aligned}$$

$$\begin{aligned}
& + \frac{2}{3} \delta^{pr} \delta^{sc} \delta^{td} (Y_u Y_u^\dagger)^{ba} \Big) + \frac{9}{2} \delta^{pr} \delta^{sc} \delta^{td} \delta^{ab} g_L^4 - \frac{220}{729} \delta^{pr} \delta^{sc} \delta^{td} \delta^{ab} g_Y^4 - \frac{1}{2} \delta^{pr} \delta^{sc} \delta^{td} \delta^{ab} g_Y^2 g_L^2 - \frac{1}{2} \delta^{sc} \delta^{td} (Y_e Y_e^\dagger)^{pr} (Y_u Y_u^\dagger)^{ba} \Big\} C_{qd}^{(\times)abcd} \\
& + \left\{ \frac{16}{27} \delta^{pr} \delta^{st} \delta^{ab} \delta^{cd} g_Y^4 - \frac{8}{9} \delta^{st} \delta^{ad} g_Y^2 Y_e^{*rb} Y_e^{pc} \right\} C_{ee}^{abcd} + \frac{64}{81} \delta^{pr} \delta^{st} \delta^{ad} \delta^{bc} g_Y^4 C_{uu}^{abcd} + \left\{ g_Y^4 \left( \frac{44}{243} \delta^{pr} \delta^{sa} \delta^{tb} \delta^{cd} + \frac{16}{81} \delta^{pr} \delta^{st} \delta^{ad} \delta^{bc} \right. \right. \\
& - \frac{448}{729} \delta^{pr} \delta^{sa} \delta^{td} \delta^{bc} \Big) + g_Y^2 g_s^2 \left( \frac{152}{243} \delta^{pr} \delta^{sa} \delta^{td} \delta^{bc} + 4 \delta^{pr} \delta^{sa} \delta^{tb} \delta^{cd} - \frac{4}{27} \delta^{pr} \delta^{st} \delta^{ad} \delta^{bc} \right) - g_Y^2 \left( \frac{14}{9} \delta^{pr} \delta^{sa} \delta^{td} (Y_d^\dagger Y_d)^{bc} + 2 \delta^{pr} \delta^{sa} \delta^{tb} (Y_d^\dagger Y_d)^{dc} \right) \\
& - 3 \delta^{sa} \delta^{td} (Y_d^\dagger Y_d)^{bc} (Y_e Y_e^\dagger)^{pr} - 3 \delta^{sa} \delta^{tb} (Y_d^\dagger Y_d)^{dc} (Y_e Y_e^\dagger)^{pr} \Big\} C_{dd}^{abcd} + \left\{ g_Y^2 \left( \frac{13}{8} \delta^{sc} \delta^{td} Y_e^{*rb} Y_e^{pa} - \frac{5}{3} \delta^{pr} \delta^{sc} \delta^{td} (Y_e^\dagger Y_e)^{ba} \right) + \frac{3}{2} T_2 \delta^{sc} \delta^{td} Y_e^{*rb} Y_e^{pa} \right. \\
& + \frac{3}{2} \delta^{sc} \delta^{td} Y_e^{pa} (Y_e^\dagger Y_e Y_e^\dagger)^{rb} + \frac{3}{2} \delta^{sc} \delta^{td} Y_e^{*rb} (Y_e Y_e^\dagger Y_e)^{pa} - \frac{1}{4} \delta^{td} Y_e^{*rb} Y_e^{pa} (Y_d^\dagger Y_d)^{sc} - \frac{1}{4} \delta^{sc} Y_e^{*rb} Y_e^{pa} (Y_d^\dagger Y_d)^{dt} - \frac{68}{243} \delta^{pr} \delta^{sc} \delta^{td} \delta^{ab} g_Y^4 \\
& - \frac{1}{2} \delta^{sc} \delta^{td} (Y_e^\dagger Y_e)^{ba} (Y_e Y_e^\dagger)^{pr} - \frac{33}{8} \delta^{sc} \delta^{td} g_L^2 Y_e^{*rb} Y_e^{pa} \Big\} C_{ed}^{abcd} + \left\{ \frac{3}{2} \delta^{sc} \delta^{td} (Y_u^\dagger Y_u)^{ba} (Y_e Y_e^\dagger)^{pr} + 3 \delta^{pr} \delta^{sc} \delta^{td} g_Y^2 (Y_u^\dagger Y_u)^{ba} - \frac{16}{3} \delta^{pr} \delta^{sc} \delta^{td} \delta^{ab} g_Y^2 g_s^2 \right. \\
& - \frac{1934}{243} \delta^{pr} \delta^{sc} \delta^{td} \delta^{ab} g_Y^4 \Big\} C_{ud}^{(\parallel)abcd} + \left\{ \frac{1}{2} \delta^{sc} \delta^{td} (Y_u^\dagger Y_u)^{ba} (Y_e Y_e^\dagger)^{pr} + \delta^{pr} \delta^{sc} \delta^{td} g_Y^2 (Y_u^\dagger Y_u)^{ba} - g_Y^2 g_s^2 \left( \frac{2}{27} \delta^{pr} \delta^{st} \delta^{ab} \delta^{cd} + \frac{506}{243} \delta^{pr} \delta^{sc} \delta^{td} \delta^{ab} \right) \right. \\
& - \frac{1934}{729} \delta^{pr} \delta^{sc} \delta^{td} \delta^{ab} g_Y^4 \Big\} C_{ud}^{(\times)abcd} + \left\{ \frac{1}{8} \delta^{pa} \delta^{sc} Y_e^{*rb} (Y_d Y_d^\dagger Y_d)^{dt} + \frac{1}{4} T_2 \delta^{pa} \delta^{sc} Y_e^{*rb} Y_d^{dt} + \frac{1}{4} \delta^{sc} Y_e^{*ab} Y_d^{dt} (Y_e Y_e^\dagger)^{pr} + \frac{1}{4} \delta^{pa} \delta^{sc} Y_d^{dt} (Y_e^\dagger Y_e Y_e^\dagger)^{rb} \right. \\
& + \frac{3}{8} \delta^{pa} \delta^{sc} Y_e^{*rb} (Y_u Y_u^\dagger Y_d)^{dt} + \frac{5}{8} \delta^{pa} Y_e^{*rb} Y_d^{dt} (Y_d^\dagger Y_d)^{sc} + \frac{3}{4} \delta^{pa} Y_e^{*rb} Y_d^{dc} (Y_d^\dagger Y_d)^{st} + g_Y^2 \left( \frac{5}{9} \delta^{pa} \delta^{st} Y_e^{*rb} Y_d^{dc} - \frac{5}{27} \delta^{pr} \delta^{sc} Y_e^{*ab} Y_d^{dt} - \frac{163}{144} \delta^{pa} \delta^{sc} Y_e^{*rb} Y_d^{dt} \right) \\
& + \frac{5}{4} \delta^{sc} Y_e^{*rb} Y_d^{dt} (Y_e Y_e^\dagger)^{pa} + \frac{8}{3} \delta^{pa} \delta^{sc} g_s^2 Y_e^{*rb} Y_d^{dt} - \frac{33}{16} \delta^{pa} \delta^{sc} g_L^2 Y_e^{*rb} Y_d^{dt} \Big\} C_{ledq}^{abcd} + C_{ledq}^{*abcd} \left\{ \frac{1}{8} \delta^{ra} \delta^{tc} Y_e^{pb} (Y_d^\dagger Y_d Y_d^\dagger)^{ds} + \frac{1}{4} T_2 \delta^{ra} \delta^{tc} Y_d^{*ds} Y_e^{pb} \right. \\
& + \frac{1}{4} \delta^{tc} Y_d^{*ds} Y_e^{ab} (Y_e Y_e^\dagger)^{pr} + \frac{1}{4} \delta^{ra} \delta^{tc} Y_d^{*ds} (Y_e Y_e^\dagger Y_e)^{pb} + \frac{3}{8} \delta^{ra} \delta^{tc} Y_e^{pb} (Y_u^\dagger Y_u Y_d^\dagger)^{ds} + \frac{5}{8} \delta^{ra} Y_d^{*ds} Y_e^{pb} (Y_d^\dagger Y_d)^{ct} + \frac{3}{4} \delta^{ra} Y_d^{*dc} Y_e^{pb} (Y_d^\dagger Y_d)^{st} \\
& + g_Y^2 \left( \frac{5}{9} \delta^{ra} \delta^{st} Y_d^{*dc} Y_e^{pb} - \frac{5}{27} \delta^{pr} \delta^{tc} Y_d^{*ds} Y_e^{ab} - \frac{163}{144} \delta^{ra} \delta^{tc} Y_d^{*ds} Y_e^{pb} \right) + \frac{5}{4} \delta^{tc} Y_d^{*ds} Y_e^{pb} (Y_e Y_e^\dagger)^{ar} + \frac{8}{3} \delta^{ra} \delta^{tc} g_s^2 Y_d^{*ds} Y_e^{pb} - \frac{33}{16} \delta^{ra} \delta^{tc} g_L^2 Y_d^{*ds} Y_e^{pb} \Big\} \\
& + \left\{ \frac{1}{8} \delta^{td} Y_d^{*as} Y_u^{*cb} (Y_e Y_e^\dagger)^{pr} + \frac{3}{4} \delta^{td} Y_d^{*cs} Y_u^{*ab} (Y_e Y_e^\dagger)^{pr} - g_Y^2 \left( \frac{1}{108} \delta^{pr} \delta^{td} Y_d^{*as} Y_u^{*cb} + \frac{5}{9} \delta^{pr} \delta^{td} Y_d^{*cs} Y_u^{*ab} \right) \right\} C_{quqd}^{(\parallel)abcd} + \left( C_{quqd}^{(\parallel)*} \right)^{abcd} \left\{ \frac{1}{8} \delta^{sd} Y_d^{at} Y_u^{cb} (Y_e Y_e^\dagger)^{pr} \right. \\
& + \frac{3}{4} \delta^{sd} Y_d^{ct} Y_u^{ab} (Y_e Y_e^\dagger)^{pr} - g_Y^2 \left( \frac{1}{108} \delta^{pr} \delta^{sd} Y_d^{at} Y_u^{cb} + \frac{5}{9} \delta^{pr} \delta^{sd} Y_d^{ct} Y_u^{ab} \right) \Big\} + \left\{ \frac{1}{4} \delta^{td} Y_d^{*cs} Y_u^{*ab} (Y_e Y_e^\dagger)^{pr} + \frac{3}{8} \delta^{td} Y_d^{*as} Y_u^{*cb} (Y_e Y_e^\dagger)^{pr} - g_Y^2 \left( \frac{1}{36} \delta^{pr} \delta^{td} Y_d^{*as} Y_u^{*cb} \right. \right. \\
& + \frac{5}{27} \delta^{pr} \delta^{td} Y_d^{*cs} Y_u^{*ab} \Big) \Big\} C_{quqd}^{(\times)abcd} + \left( C_{quqd}^{(\times)*} \right)^{abcd} \left\{ \frac{1}{4} \delta^{sd} Y_d^{ct} Y_u^{ab} (Y_e Y_e^\dagger)^{pr} + \frac{3}{8} \delta^{sd} Y_d^{at} Y_u^{cb} (Y_e Y_e^\dagger)^{pr} - g_Y^2 \left( \frac{1}{36} \delta^{pr} \delta^{sd} Y_d^{at} Y_u^{cb} + \frac{5}{27} \delta^{pr} \delta^{sd} Y_d^{ct} Y_u^{ab} \right) \right\}
\end{aligned}$$

$$\begin{aligned}
& + \left\{ \frac{3}{8} \delta^{pa} Y_d^{*cs} Y_e^{*rb} (Y_u^\dagger Y_d)^{dt} - \frac{5}{9} \delta^{pa} \delta^{st} g_Y^2 Y_e^{*rb} Y_u^{*cd} - \frac{3}{4} \delta^{pa} Y_e^{*rb} Y_u^{*cd} (Y_d^\dagger Y_d)^{st} \right\} C_{\ell equ}^{abcd} + C_{\ell equ}^{*abcd} \left\{ \frac{3}{8} \delta^{ra} Y_d^{ct} Y_e^{pb} (Y_d^\dagger Y_u)^{sd} - \frac{5}{9} \delta^{ra} \delta^{st} g_Y^2 Y_e^{pb} Y_u^{cd} \right. \\
& - \left. \frac{3}{4} \delta^{ra} Y_e^{pb} Y_u^{cd} (Y_d^\dagger Y_d)^{st} \right\} + \left\{ \frac{7}{36} \delta^{pa} \delta^{st} g_Y^2 Y_e^{*rd} Y_u^{*cb} + \frac{1}{4} \delta^{pa} Y_d^{*cs} Y_e^{*rd} (Y_u^\dagger Y_d)^{bt} + \frac{3}{8} \delta^{pa} Y_e^{*rd} Y_u^{*cb} (Y_d^\dagger Y_d)^{st} \right\} C_{\ell uqe}^{abcd} + C_{\ell uqe}^{*abcd} \left\{ \frac{7}{36} \delta^{ra} \delta^{st} g_Y^2 Y_e^{pd} Y_u^{cb} \right. \\
& + \left. \frac{1}{4} \delta^{ra} Y_d^{ct} Y_e^{pd} (Y_d^\dagger Y_u)^{sb} + \frac{3}{8} \delta^{ra} Y_e^{pd} Y_u^{cb} (Y_d^\dagger Y_d)^{st} \right\} + \left\{ g_Y^4 \left( \frac{8}{27} \delta^{pr} \delta^{st} \delta^{ad} \delta^{bc} - \frac{8}{81} \delta^{pa} \delta^{rb} \delta^{st} \delta^{cd} - \frac{82}{81} \delta^{pa} \delta^{rd} \delta^{st} \delta^{bc} \right) + g_Y^2 g_L^2 \left( \frac{2}{3} \delta^{pa} \delta^{rd} \delta^{st} \delta^{bc} \right. \right. \\
& + \left. \frac{2}{3} \delta^{pa} \delta^{rb} \delta^{st} \delta^{cd} - \frac{4}{27} \delta^{pr} \delta^{st} \delta^{ad} \delta^{bc} \right) - g_Y^2 \left( \frac{4}{3} \delta^{pa} \delta^{rd} \delta^{st} (Y_e Y_e^\dagger)^{bc} + \frac{16}{9} \delta^{pa} \delta^{rb} \delta^{st} (Y_e Y_e^\dagger)^{dc} \right) - 2 \delta^{pa} \delta^{rb} (Y_d^\dagger Y_d)^{st} (Y_e Y_e^\dagger)^{dc} \\
& - \left. 3 \delta^{pa} \delta^{rd} (Y_d^\dagger Y_d)^{st} (Y_e Y_e^\dagger)^{bc} \right\} C_{\ell \ell}^{abcd} + \left\{ \frac{8}{81} \delta^{pr} \delta^{st} \delta^{ad} \delta^{bc} g_Y^4 + \frac{4}{9} \delta^{pr} \delta^{bc} g_Y^2 Y_d^{*as} Y_d^{dt} \right\} C_{qq}^{(\parallel)abcd} + \left\{ \frac{16}{81} \delta^{pr} \delta^{st} \delta^{ad} \delta^{bc} g_Y^4 + \frac{8}{9} \delta^{pr} \delta^{bc} g_Y^2 Y_d^{*as} Y_d^{dt} \right\} C_{qq}^{(\times)abcd} \\
& + \left\{ \frac{1}{2} \delta^{pa} \delta^{rb} Y_d^{dt} (Y_u^\dagger Y_u Y_d^\dagger)^{cs} + \frac{1}{2} \delta^{pa} \delta^{rb} Y_d^{*cs} (Y_u Y_u^\dagger Y_d)^{dt} + g_Y^2 \left( \frac{4}{3} \delta^{pa} \delta^{rb} \delta^{st} (Y_u Y_u^\dagger)^{dc} - \frac{283}{36} \delta^{pa} \delta^{rb} Y_d^{*cs} Y_d^{dt} \right) + \frac{3}{2} \delta^{pa} \delta^{rb} Y_d^{dt} (Y_d^\dagger Y_d Y_d^\dagger)^{cs} \right. \\
& + \frac{3}{2} \delta^{pa} \delta^{rb} Y_d^{*cs} (Y_d Y_d^\dagger Y_d)^{dt} + 3 T_2 \delta^{pa} \delta^{rb} Y_d^{*cs} Y_d^{dt} + 3 \delta^{pa} \delta^{rb} (Y_d^\dagger Y_d)^{st} (Y_u Y_u^\dagger)^{dc} + \frac{32}{3} \delta^{pa} \delta^{rb} g_s^2 Y_d^{*cs} Y_d^{dt} - \frac{1}{4} \delta^{rb} Y_d^{*cs} Y_d^{dt} (Y_e Y_e^\dagger)^{pa} \\
& - \frac{1}{4} \delta^{pa} Y_d^{*cs} Y_d^{dt} (Y_e Y_e^\dagger)^{br} - \frac{56}{81} \delta^{pa} \delta^{rb} \delta^{st} \delta^{cd} g_Y^4 - \delta^{pa} \delta^{rb} \delta^{st} \delta^{cd} g_Y^2 g_L^2 - \frac{16}{9} \delta^{pa} \delta^{rb} \delta^{st} \delta^{cd} g_Y^2 g_s^2 - 3 \delta^{pa} \delta^{rb} (Y_d^\dagger Y_d)^{st} (Y_d Y_d^\dagger)^{dc} \\
& - \left. \frac{51}{4} \delta^{pa} \delta^{rb} g_L^2 Y_d^{*cs} Y_d^{dt} - 16 \delta^{pa} \delta^{rb} \delta^{st} \delta^{cd} g_s^4 \right\} C_{\ell q}^{(\parallel)abcd} + \left\{ \frac{1}{4} \delta^{pa} \delta^{rb} Y_d^{dt} (Y_u^\dagger Y_u Y_d^\dagger)^{cs} + \frac{1}{4} \delta^{pa} \delta^{rb} Y_d^{*cs} (Y_u Y_u^\dagger Y_d)^{dt} + \frac{3}{4} \delta^{pa} \delta^{rb} Y_d^{dt} (Y_d^\dagger Y_d Y_d^\dagger)^{cs} \right. \\
& + \frac{3}{4} \delta^{pa} \delta^{rb} Y_d^{*cs} (Y_d Y_d^\dagger Y_d)^{dt} + g_Y^2 \left( \frac{2}{3} \delta^{pa} \delta^{rb} \delta^{st} (Y_u Y_u^\dagger)^{dc} - \frac{283}{72} \delta^{pa} \delta^{rb} Y_d^{*cs} Y_d^{dt} \right) + \frac{3}{2} T_2 \delta^{pa} \delta^{rb} Y_d^{*cs} Y_d^{dt} + \frac{3}{2} \delta^{pa} \delta^{rb} (Y_d^\dagger Y_d)^{st} (Y_u Y_u^\dagger)^{dc} \\
& + \frac{15}{8} \delta^{pa} \delta^{rb} g_L^2 Y_d^{*cs} Y_d^{dt} + \frac{16}{3} \delta^{pa} \delta^{rb} g_s^2 Y_d^{*cs} Y_d^{dt} - \frac{28}{81} \delta^{pa} \delta^{rb} \delta^{st} \delta^{cd} g_Y^4 - \frac{1}{2} \delta^{rb} Y_d^{*cs} Y_d^{dt} (Y_e Y_e^\dagger)^{pa} - \frac{1}{2} \delta^{pa} Y_d^{*cs} Y_d^{dt} (Y_e Y_e^\dagger)^{br} - \frac{8}{9} \delta^{pa} \delta^{rb} \delta^{st} \delta^{cd} g_Y^2 g_s^2 \\
& - \left. g_Y^2 g_L^2 \left( \frac{2}{9} \delta^{pr} \delta^{st} \delta^{ab} \delta^{cd} + 2 \delta^{pa} \delta^{rb} \delta^{st} \delta^{cd} \right) - \frac{3}{2} \delta^{pa} \delta^{rb} (Y_d^\dagger Y_d)^{st} (Y_d Y_d^\dagger)^{dc} - 8 \delta^{pa} \delta^{rb} \delta^{st} \delta^{cd} g_s^4 \right\} C_{\ell q}^{(\times)abcd}, \tag{10.6}
\end{aligned}$$

#### 10.4 $C_{qe}$

$$\begin{aligned}
\beta_{C_{qe}^{prst}}^{(1)} & = \left\{ \frac{1}{9} \delta^{pr} \delta^{sa} \delta^{tb} g_Y^2 + \delta^{sa} \delta^{tb} (Y_u Y_u^\dagger)^{pr} - \delta^{sa} \delta^{tb} (Y_d Y_d^\dagger)^{pr} \right\} C_{He}^{ab} + \left\{ 2 \delta^{pa} \delta^{rb} (Y_e^\dagger Y_e)^{st} - \frac{2}{3} \delta^{pa} \delta^{rb} \delta^{st} g_Y^2 \right\} C_{Hq}^{(\parallel)ab} + \left\{ \delta^{pa} \delta^{rb} (Y_e^\dagger Y_e)^{st} \right. \\
& - \left. \frac{1}{3} \delta^{pa} \delta^{rb} \delta^{st} g_Y^2 \right\} C_{Hq}^{(\times)ab} - \frac{2}{9} \delta^{pr} \delta^{sc} \delta^{td} \delta^{ab} g_Y^2 C_{\ell e}^{abcd} + \left\{ \frac{2}{9} g_Y^2 \left( \delta^{pr} \delta^{sc} \delta^{td} \delta^{ab} + 6 \delta^{pa} \delta^{rb} \delta^{st} \delta^{cd} + 9 \delta^{pa} \delta^{rb} \delta^{sc} \delta^{td} \right) + \frac{1}{2} \left( \delta^{rb} \delta^{sc} \delta^{td} (Y_d Y_d^\dagger)^{pa} \right. \right.
\end{aligned}$$

$$\begin{aligned}
& + \delta^{pa} \delta^{sc} \delta^{td} (Y_d Y_d^\dagger)^{br} + \delta^{rb} \delta^{sc} \delta^{td} (Y_u Y_u^\dagger)^{pa} + \delta^{pa} \delta^{sc} \delta^{td} (Y_u Y_u^\dagger)^{br} + 2\delta^{pa} \delta^{rb} \delta^{td} (Y_e^\dagger Y_e)^{sc} + 2\delta^{pa} \delta^{rb} \delta^{sc} (Y_e^\dagger Y_e)^{dt} \Big\} C_{qe}^{abcd} - \frac{8}{3} \delta^{pa} \delta^{rb} \delta^{st} \delta^{cd} g_Y^2 C_{qu}^{(\parallel)abcd} \\
& - \frac{8}{9} \delta^{pa} \delta^{rb} \delta^{st} \delta^{cd} g_Y^2 C_{qu}^{(\times)abcd} + \frac{4}{3} \delta^{pa} \delta^{rb} \delta^{st} \delta^{cd} g_Y^2 C_{qd}^{(\parallel)abcd} + \frac{4}{9} \delta^{pa} \delta^{rb} \delta^{st} \delta^{cd} g_Y^2 C_{qd}^{(\times)abcd} - \frac{8}{9} \delta^{pr} \delta^{sa} \delta^{tb} \delta^{cd} g_Y^2 C_{ee}^{abcd} + \left\{ \frac{4}{9} \delta^{pr} \delta^{sa} \delta^{tb} \delta^{cd} g_Y^2 \right. \\
& - \delta^{sa} \delta^{tb} Y_u^{*rd} Y_u^{pc} \Big\} C_{eu}^{abcd} - \left\{ \frac{2}{9} \delta^{pr} \delta^{sa} \delta^{tb} \delta^{cd} g_Y^2 + \delta^{sa} \delta^{tb} Y_d^{*rd} Y_d^{pc} \right\} C_{ed}^{abcd} - \frac{1}{2} \delta^{rd} \delta^{tb} Y_e^{*as} C_{ledq}^{abcd} Y_d^{pc} - \frac{1}{2} \delta^{pd} \delta^{sb} C_{ledq}^{*abcd} Y_d^{*rc} Y_e^{at} \\
& - \frac{1}{2} \delta^{pc} \delta^{tb} Y_e^{*as} Y_u^{*rd} C_{lequ}^{abcd} - \frac{1}{2} \delta^{rc} \delta^{sb} C_{lequ}^{*abcd} Y_e^{at} Y_u^{pd} + \delta^{pc} \delta^{td} Y_e^{*as} Y_u^{*rb} C_{luqe}^{abcd} + \delta^{rc} \delta^{sd} C_{luqe}^{*abcd} Y_e^{at} Y_u^{pb} - \frac{4}{9} g_Y^2 \left\{ \delta^{pa} \delta^{rd} \delta^{st} \delta^{bc} \right. \\
& + 6\delta^{pa} \delta^{rb} \delta^{st} \delta^{cd} \Big\} C_{qq}^{(\parallel)abcd} - \frac{4}{9} g_Y^2 \left\{ 2\delta^{pa} \delta^{rd} \delta^{st} \delta^{bc} + 3\delta^{pa} \delta^{rb} \delta^{st} \delta^{cd} \right\} C_{qq}^{(\times)abcd} + \left\{ \frac{4}{3} \delta^{pc} \delta^{rd} \delta^{st} \delta^{ab} g_Y^2 - 2\delta^{pc} \delta^{rd} Y_e^{*as} Y_e^{bt} \right\} C_{\ell q}^{(\parallel)abcd} \\
& + \left\{ \frac{2}{3} \delta^{pc} \delta^{rd} \delta^{st} \delta^{ab} g_Y^2 - \delta^{pc} \delta^{rd} Y_e^{*as} Y_e^{bt} \right\} C_{\ell q}^{(\times)abcd}, \tag{10.7}
\end{aligned}$$

$$\begin{aligned}
\beta_{C_{qe}^{prst}}^{(2)} & = \left\{ g_Y^4 \left( \frac{5}{3} \delta^{pr} (Y_e^\dagger Y_e)^{st} + \frac{5}{3} \delta^{st} (Y_d Y_d^\dagger)^{pr} - \frac{1}{3} \delta^{st} (Y_u Y_u^\dagger)^{pr} \right) - \frac{4}{9} \delta^{pr} \delta^{st} g_Y^6 \right\} C_{HB} + \left\{ g_Y^2 g_L^2 \left( \frac{1}{4} \delta^{pr} (Y_e^\dagger Y_e)^{st} + \frac{9}{4} \delta^{st} (Y_d Y_d^\dagger)^{pr} - \frac{9}{4} \delta^{st} (Y_u Y_u^\dagger)^{pr} \right) \right. \\
& - \frac{1}{3} \delta^{pr} \delta^{st} g_Y^4 g_L^2 \Big\} C_{HWB} - \frac{10}{3} \delta^{pr} \delta^{st} g_Y^2 g_L^6 C_W - \frac{80}{9} \delta^{pr} \delta^{st} g_Y^2 g_s^6 C_G + \left\{ g_Y^4 \left( \frac{2}{3} \delta^{pr} \delta^{st} Y_e^{*ab} - \frac{5}{3} \delta^{pr} \delta^{tb} Y_e^{*as} \right) + g_Y^2 \left( 3\delta^{tb} Y_e^{*as} (Y_d Y_d^\dagger)^{pr} \right. \right. \\
& - \frac{1}{3} \delta^{pr} Y_e^{*as} (Y_e^\dagger Y_e)^{bt} - \frac{17}{3} \delta^{tb} Y_e^{*as} (Y_u Y_u^\dagger)^{pr} \Big\} C_{eB}^{ab} + C_{eB}^{*ab} \left\{ g_Y^4 \left( \frac{2}{3} \delta^{pr} \delta^{st} Y_e^{ab} - \frac{5}{3} \delta^{pr} \delta^{sb} Y_e^{at} \right) + g_Y^2 \left( 3\delta^{sb} Y_e^{at} (Y_d Y_d^\dagger)^{pr} - \frac{1}{3} \delta^{pr} Y_e^{at} (Y_e^\dagger Y_e)^{sb} \right. \right. \\
& - \frac{17}{3} \delta^{sb} Y_e^{at} (Y_u Y_u^\dagger)^{pr} \Big\} + \left\{ \frac{5}{6} \delta^{pr} \delta^{tb} g_Y^2 g_L^2 Y_e^{*as} + \frac{9}{2} \delta^{pr} \delta^{tb} g_L^4 Y_e^{*as} + 6\delta^{tb} g_L^2 Y_e^{*as} (Y_u Y_u^\dagger)^{pr} \right\} C_{eW}^{ab} + C_{eW}^{*ab} \left\{ \frac{5}{6} \delta^{pr} \delta^{sb} g_Y^2 g_L^2 Y_e^{at} + \frac{9}{2} \delta^{pr} \delta^{sb} g_L^4 Y_e^{at} \right. \\
& + 6\delta^{sb} g_L^2 Y_e^{at} (Y_u Y_u^\dagger)^{pr} \Big\} + \left\{ g_Y^4 \left( \frac{571}{54} \delta^{pa} \delta^{st} Y_u^{*rb} - \frac{10}{9} \delta^{pr} \delta^{st} Y_u^{*ab} \right) + g_Y^2 \left( 2\delta^{st} Y_u^{*rb} (Y_u Y_u^\dagger)^{pa} + \frac{19}{2} \delta^{pa} Y_u^{*rb} (Y_e^\dagger Y_e)^{st} - \delta^{st} Y_u^{*rb} (Y_d Y_d^\dagger)^{pa} \right) \right. \\
& + \frac{16}{3} \delta^{pa} \delta^{st} g_Y^2 g_s^2 Y_u^{*rb} \Big\} C_{uB}^{ab} + C_{uB}^{*ab} \left\{ g_Y^4 \left( \frac{571}{54} \delta^{ra} \delta^{st} Y_u^{pb} - \frac{10}{9} \delta^{pr} \delta^{st} Y_u^{ab} \right) + g_Y^2 \left( 2\delta^{st} Y_u^{pb} (Y_u Y_u^\dagger)^{ar} + \frac{19}{2} \delta^{ra} Y_u^{pb} (Y_e^\dagger Y_e)^{st} - \delta^{st} Y_u^{pb} (Y_d Y_d^\dagger)^{ar} \right) \right. \\
& + \frac{16}{3} \delta^{ra} \delta^{st} g_Y^2 g_s^2 Y_u^{pb} \Big\} + \left\{ \frac{11}{12} \delta^{pa} \delta^{st} g_Y^2 g_L^2 Y_u^{*rb} + \frac{15}{4} \delta^{pa} g_L^2 Y_u^{*rb} (Y_e^\dagger Y_e)^{st} \right\} C_{uW}^{ab} + C_{uW}^{*ab} \left\{ \frac{11}{12} \delta^{ra} \delta^{st} g_Y^2 g_L^2 Y_u^{pb} + \frac{15}{4} \delta^{ra} g_L^2 Y_u^{pb} (Y_e^\dagger Y_e)^{st} \right\}
\end{aligned}$$



$$\begin{aligned}
& + \left\{ 4\delta^{pa} g_s^2 Y_u^{*rb} (Y_e^\dagger Y_e)^{st} + \frac{148}{27} \delta^{pa} \delta^{st} g_Y^2 g_s^2 Y_u^{*rb} \right\} C_{uG}^{ab} + C_{uG}^{*ab} \left\{ 4\delta^{ra} g_s^2 Y_u^{pb} (Y_e^\dagger Y_e)^{st} + \frac{148}{27} \delta^{ra} \delta^{st} g_Y^2 g_s^2 Y_u^{pb} \right\} + \left\{ g_Y^4 \left( \frac{2}{9} \delta^{pr} \delta^{st} Y_d^{*ab} \right. \right. \\
& - \frac{215}{54} \delta^{pa} \delta^{st} Y_d^{*rb} \Big) + g_Y^2 \left( 2\delta^{st} Y_d^{*rb} (Y_d Y_d^\dagger)^{pa} - \frac{1}{2} \delta^{pa} Y_d^{*rb} (Y_e^\dagger Y_e)^{st} - \delta^{st} Y_d^{*rb} (Y_u Y_u^\dagger)^{pa} \right) + \frac{16}{3} \delta^{pa} \delta^{st} g_Y^2 g_s^2 Y_d^{*rb} \Big\} C_{dB}^{ab} + C_{dB}^{*ab} \left\{ g_Y^4 \left( \frac{2}{9} \delta^{pr} \delta^{st} Y_d^{ab} \right. \right. \\
& - \frac{215}{54} \delta^{ra} \delta^{st} Y_d^{pb} \Big) + g_Y^2 \left( 2\delta^{st} Y_d^{pb} (Y_d Y_d^\dagger)^{ar} - \frac{1}{2} \delta^{ra} Y_d^{pb} (Y_e^\dagger Y_e)^{st} - \delta^{st} Y_d^{pb} (Y_u Y_u^\dagger)^{ar} \right) + \frac{16}{3} \delta^{ra} \delta^{st} g_Y^2 g_s^2 Y_d^{pb} \Big\} - \left\{ \frac{7}{12} \delta^{pa} \delta^{st} g_Y^2 g_L^2 Y_d^{*rb} \right. \\
& + \frac{9}{4} \delta^{pa} g_L^2 Y_d^{*rb} (Y_e^\dagger Y_e)^{st} \Big\} C_{dW}^{ab} - C_{dW}^{*ab} \left\{ \frac{7}{12} \delta^{ra} \delta^{st} g_Y^2 g_L^2 Y_d^{pb} + \frac{9}{4} \delta^{ra} g_L^2 Y_d^{pb} (Y_e^\dagger Y_e)^{st} \right\} - \left\{ \frac{68}{27} \delta^{pa} \delta^{st} g_Y^2 g_s^2 Y_d^{*rb} + 4\delta^{pa} g_s^2 Y_d^{*rb} (Y_e^\dagger Y_e)^{st} \right\} C_{dG}^{ab} \\
& - C_{dG}^{*ab} \left\{ \frac{68}{27} \delta^{ra} \delta^{st} g_Y^2 g_s^2 Y_d^{pb} + 4\delta^{ra} g_s^2 Y_d^{pb} (Y_e^\dagger Y_e)^{st} \right\} + \left\{ \frac{1}{4} \delta^{tb} (Y_e^\dagger Y_e)^{sa} (Y_u Y_u^\dagger)^{pr} + \frac{1}{4} \delta^{sa} (Y_e^\dagger Y_e)^{bt} (Y_u Y_u^\dagger)^{pr} + \delta^{pr} \delta^{sa} \delta^{tb} g_Y^2 g_L^2 \right. \\
& + T_2 \delta^{sa} \delta^{tb} (Y_d Y_d^\dagger)^{pr} + g_s^2 \left( \frac{16}{3} \delta^{sa} \delta^{tb} (Y_d Y_d^\dagger)^{pr} - \frac{16}{3} \delta^{sa} \delta^{tb} (Y_u Y_u^\dagger)^{pr} \right) + g_L^2 \left( \frac{33}{8} \delta^{sa} \delta^{tb} (Y_u Y_u^\dagger)^{pr} - \frac{33}{8} \delta^{sa} \delta^{tb} (Y_d Y_d^\dagger)^{pr} \right) + g_Y^2 \left( \frac{1}{9} \delta^{pr} \delta^{ab} (Y_e^\dagger Y_e)^{st} \right. \\
& + \frac{31}{108} \delta^{pr} \delta^{tb} (Y_e^\dagger Y_e)^{sa} + \frac{31}{108} \delta^{pr} \delta^{sa} (Y_e^\dagger Y_e)^{bt} - \frac{1}{3} \delta^{pr} \delta^{sa} \delta^{tb} \text{Tr} [Y_d^\dagger Y_d] - \frac{1}{3} \delta^{pr} \delta^{sa} \delta^{tb} \text{Tr} [Y_u^\dagger Y_u] - \frac{139}{72} \delta^{sa} \delta^{tb} (Y_d Y_d^\dagger)^{pr} - \frac{305}{72} \delta^{sa} \delta^{tb} (Y_u Y_u^\dagger)^{pr} \\
& + 3\delta^{sa} \delta^{tb} (Y_d Y_d^\dagger Y_d Y_d^\dagger)^{pr} - \frac{1}{4} \delta^{tb} (Y_e^\dagger Y_e)^{sa} (Y_d Y_d^\dagger)^{pr} - \frac{1}{4} \delta^{sa} (Y_e^\dagger Y_e)^{bt} (Y_d Y_d^\dagger)^{pr} - g_Y^4 \left( \frac{1}{27} \delta^{pr} \delta^{st} \delta^{ab} + \frac{95}{162} \delta^{pr} \delta^{sa} \delta^{tb} \right) - T_2 \delta^{sa} \delta^{tb} (Y_u Y_u^\dagger)^{pr} \\
& - 3\delta^{sa} \delta^{tb} (Y_u Y_u^\dagger Y_u Y_u^\dagger)^{pr} \Big\} C_{He}^{ab} + \left\{ \frac{1}{4} \delta^{rb} (Y_e^\dagger Y_e)^{st} (Y_d Y_d^\dagger)^{pa} + \frac{1}{4} \delta^{pa} (Y_e^\dagger Y_e)^{st} (Y_d Y_d^\dagger)^{br} + \frac{1}{4} \delta^{rb} (Y_e^\dagger Y_e)^{st} (Y_u Y_u^\dagger)^{pa} + \frac{1}{4} \delta^{pa} (Y_e^\dagger Y_e)^{st} (Y_u Y_u^\dagger)^{br} \right. \\
& + g_Y^2 \left( \frac{2}{3} T_2 \delta^{pa} \delta^{rb} \delta^{st} - \frac{31}{108} \delta^{rb} \delta^{st} (Y_u Y_u^\dagger)^{pa} - \frac{31}{108} \delta^{pa} \delta^{st} (Y_u Y_u^\dagger)^{br} - \frac{59}{108} \delta^{rb} \delta^{st} (Y_d Y_d^\dagger)^{pa} - \frac{59}{108} \delta^{pa} \delta^{st} (Y_d Y_d^\dagger)^{br} - \frac{97}{12} \delta^{pa} \delta^{rb} (Y_e^\dagger Y_e)^{st} \right) \\
& + \frac{51}{4} \delta^{pa} \delta^{rb} g_L^2 (Y_e^\dagger Y_e)^{st} - \frac{4}{243} \delta^{pa} \delta^{rb} \delta^{st} g_Y^4 - 2T_2 \delta^{pa} \delta^{rb} (Y_e^\dagger Y_e)^{st} - 3\delta^{pa} \delta^{rb} (Y_e^\dagger Y_e Y_e^\dagger Y_e)^{st} - 6\delta^{pa} \delta^{rb} \delta^{st} g_Y^2 g_L^2 \Big\} C_{Hq}^{(\parallel)ab} \\
& + \left\{ \frac{1}{2} \delta^{rb} (Y_e^\dagger Y_e)^{st} (Y_d Y_d^\dagger)^{pa} + \frac{1}{2} \delta^{pa} (Y_e^\dagger Y_e)^{st} (Y_d Y_d^\dagger)^{br} + g_Y^2 \left( \frac{31}{108} \delta^{rb} \delta^{st} (Y_u Y_u^\dagger)^{pa} + \frac{31}{108} \delta^{pa} \delta^{st} (Y_u Y_u^\dagger)^{br} + \frac{1}{3} T_2 \delta^{pa} \delta^{rb} \delta^{st} - \frac{59}{54} \delta^{rb} \delta^{st} (Y_d Y_d^\dagger)^{pa} \right. \right. \\
& - \frac{59}{54} \delta^{pa} \delta^{st} (Y_d Y_d^\dagger)^{br} - \frac{97}{24} \delta^{pa} \delta^{rb} (Y_e^\dagger Y_e)^{st} \Big) + \frac{87}{8} \delta^{pa} \delta^{rb} g_L^2 (Y_e^\dagger Y_e)^{st} - \frac{2}{243} \delta^{pa} \delta^{rb} \delta^{st} g_Y^4 - \frac{1}{4} \delta^{rb} (Y_e^\dagger Y_e)^{st} (Y_u Y_u^\dagger)^{pa} - \frac{1}{4} \delta^{pa} (Y_e^\dagger Y_e)^{st} (Y_u Y_u^\dagger)^{br} \\
& - T_2 \delta^{pa} \delta^{rb} (Y_e^\dagger Y_e)^{st} - \frac{3}{2} \delta^{pa} \delta^{rb} (Y_e^\dagger Y_e Y_e^\dagger Y_e)^{st} - \frac{139}{54} \delta^{pa} \delta^{rb} \delta^{st} g_Y^2 g_L^2 \Big\} C_{Hq}^{(\times)ab} + \left\{ \frac{1}{2} \delta^{sc} \delta^{td} (Y_d Y_d^\dagger)^{pr} (Y_e Y_e^\dagger)^{ba} + g_Y^4 \left( \frac{2}{27} \delta^{pr} \delta^{st} \delta^{ab} \delta^{cd} \right. \right. \\
& + \frac{206}{81} \delta^{pr} \delta^{sc} \delta^{td} \delta^{ab} \Big) + g_Y^2 \left( \frac{5}{27} \delta^{pr} \delta^{sc} Y_e^{*ad} Y_e^{bt} + \frac{5}{27} \delta^{pr} \delta^{td} Y_e^{*as} Y_e^{bc} + \frac{1}{3} \delta^{pr} \delta^{sc} \delta^{td} (Y_e Y_e^\dagger)^{ba} - \frac{1}{9} \delta^{pr} \delta^{cd} Y_e^{*as} Y_e^{bt} \right) + \frac{9}{2} \delta^{pr} \delta^{sc} \delta^{td} \delta^{ab} g_L^4
\end{aligned}$$

$$\begin{aligned}
& -\frac{1}{2}\delta^{pr}\delta^{sc}\delta^{td}\delta^{ab}g_Y^2g_L^2 - \frac{1}{2}\delta^{sc}\delta^{td}(Y_eY_e^\dagger)^{ba}(Y_uY_u^\dagger)^{pr} \Big\} C_{\ell e}^{abcd} - \frac{3}{2}Y_e^{*as}Y_u^{*rd}C_{\ell u}^{abcd}Y_e^{bt}Y_u^{pc} - Y_d^{*rd}Y_e^{*as}C_{\ell d}^{abcd}Y_d^{pc}Y_e^{bt} + \left\{ g_Y^2g_L^2\left(\frac{1}{2}\delta^{pr}\delta^{sc}\delta^{td}\delta^{ab}\right. \right. \\
& - \frac{9}{2}\delta^{pa}\delta^{rb}\delta^{sc}\delta^{td}) + g_Y^2g_s^2\left(\frac{8}{9}\delta^{pr}\delta^{sc}\delta^{td}\delta^{ab} - 8\delta^{pa}\delta^{rb}\delta^{sc}\delta^{td}\right) + g_Y^4\left(\frac{3854}{243}\delta^{pa}\delta^{rb}\delta^{st}\delta^{cd} - \frac{2}{27}\delta^{pr}\delta^{st}\delta^{ab}\delta^{cd} - \frac{68}{81}\delta^{pr}\delta^{sc}\delta^{td}\delta^{ab} - \frac{589}{18}\delta^{pa}\delta^{rb}\delta^{sc}\delta^{td}\right) \\
& + \delta^{pa}\delta^{rb}(Y_e^\dagger Y_e)^{st}(Y_e^\dagger Y_e)^{dc} + \delta^{sc}\delta^{td}(Y_dY_d^\dagger)^{br}(Y_uY_u^\dagger)^{pa} + \delta^{sc}\delta^{td}(Y_dY_d^\dagger)^{pa}(Y_uY_u^\dagger)^{br} + g_L^2\left(\frac{33}{16}\delta^{rb}\delta^{sc}\delta^{td}(Y_dY_d^\dagger)^{pa} + \frac{33}{16}\delta^{pa}\delta^{sc}\delta^{td}(Y_dY_d^\dagger)^{br} \right. \\
& + \frac{33}{16}\delta^{rb}\delta^{sc}\delta^{td}(Y_uY_u^\dagger)^{pa} + \frac{33}{16}\delta^{pa}\delta^{sc}\delta^{td}(Y_uY_u^\dagger)^{br} + \frac{51}{8}\delta^{pa}\delta^{rb}\delta^{td}(Y_e^\dagger Y_e)^{sc} + \frac{51}{8}\delta^{pa}\delta^{rb}\delta^{sc}(Y_e^\dagger Y_e)^{dt}) + g_Y^2\left(\frac{439}{144}\delta^{rb}\delta^{sc}\delta^{td}(Y_dY_d^\dagger)^{pa} \right. \\
& + \frac{439}{144}\delta^{pa}\delta^{sc}\delta^{td}(Y_dY_d^\dagger)^{br} - \frac{2}{3}\delta^{pr}\delta^{sc}\delta^{td}(Y_uY_u^\dagger)^{ba} - \frac{19}{8}\delta^{pa}\delta^{rb}\delta^{td}(Y_e^\dagger Y_e)^{sc} - \frac{19}{8}\delta^{pa}\delta^{rb}\delta^{sc}(Y_e^\dagger Y_e)^{dt} - \frac{437}{144}\delta^{rb}\delta^{sc}\delta^{td}(Y_uY_u^\dagger)^{pa} \\
& - \frac{437}{144}\delta^{pa}\delta^{sc}\delta^{td}(Y_uY_u^\dagger)^{br} - \frac{10}{3}\delta^{pa}\delta^{rb}\delta^{st}(Y_e^\dagger Y_e)^{dc}) + \frac{3}{2}\delta^{sc}\delta^{td}(Y_dY_d^\dagger)^{pr}(Y_dY_d^\dagger)^{ba} + \frac{3}{2}\delta^{sc}\delta^{td}(Y_uY_u^\dagger)^{pr}(Y_uY_u^\dagger)^{ba} + 2\delta^{rb}\delta^{sc}(Y_e^\dagger Y_e)^{dt}(Y_dY_d^\dagger)^{pa} \\
& + 2\delta^{pa}\delta^{td}(Y_e^\dagger Y_e)^{sc}(Y_dY_d^\dagger)^{br} + \frac{27}{2}\delta^{pr}\delta^{sc}\delta^{td}\delta^{ab}g_L^4 + 16\delta^{pr}\delta^{sc}\delta^{td}\delta^{ab}g_s^4 - \frac{1}{4}\delta^{pa}\delta^{rb}\delta^{td}(Y_e^\dagger Y_eY_e^\dagger Y_e)^{sc} - \frac{1}{4}\delta^{pa}\delta^{rb}\delta^{sc}(Y_e^\dagger Y_eY_e^\dagger Y_e)^{dt} \\
& - \frac{1}{4}\delta^{rb}\delta^{sc}\delta^{td}(Y_dY_d^\dagger Y_dY_d^\dagger)^{pa} - \frac{1}{4}\delta^{pa}\delta^{sc}\delta^{td}(Y_dY_d^\dagger Y_dY_d^\dagger)^{br} - \frac{1}{4}\delta^{rb}\delta^{sc}\delta^{td}(Y_uY_u^\dagger Y_uY_u^\dagger)^{pa} - \frac{1}{4}\delta^{pa}\delta^{sc}\delta^{td}(Y_uY_u^\dagger Y_uY_u^\dagger)^{br} - \frac{3}{4}T_2\delta^{rb}\delta^{sc}\delta^{td}(Y_dY_d^\dagger)^{pa} \\
& - \frac{3}{4}T_2\delta^{pa}\delta^{sc}\delta^{td}(Y_dY_d^\dagger)^{br} - \frac{3}{4}T_2\delta^{rb}\delta^{sc}\delta^{td}(Y_uY_u^\dagger)^{pa} - \frac{3}{4}T_2\delta^{pa}\delta^{sc}\delta^{td}(Y_uY_u^\dagger)^{br} - \delta^{rb}\delta^{td}(Y_e^\dagger Y_e)^{sc}(Y_uY_u^\dagger)^{pa} - \delta^{pa}\delta^{sc}(Y_e^\dagger Y_e)^{dt}(Y_uY_u^\dagger)^{br} \\
& - g_s^2\left(\frac{8}{3}\delta^{rb}\delta^{sc}\delta^{td}(Y_dY_d^\dagger)^{pa} + \frac{8}{3}\delta^{pa}\delta^{sc}\delta^{td}(Y_dY_d^\dagger)^{br} + \frac{8}{3}\delta^{rb}\delta^{sc}\delta^{td}(Y_uY_u^\dagger)^{pa} + \frac{8}{3}\delta^{pa}\delta^{sc}\delta^{td}(Y_uY_u^\dagger)^{br}\right) - \frac{3}{2}T_2\delta^{pa}\delta^{rb}\delta^{td}(Y_e^\dagger Y_e)^{sc} \\
& - \frac{3}{2}T_2\delta^{pa}\delta^{rb}\delta^{sc}(Y_e^\dagger Y_e)^{dt} - \frac{3}{2}\delta^{sc}\delta^{td}(Y_dY_d^\dagger)^{ba}(Y_uY_u^\dagger)^{pr} - \frac{3}{2}\delta^{sc}\delta^{td}(Y_dY_d^\dagger)^{pr}(Y_uY_u^\dagger)^{ba} - \frac{7}{4}\delta^{rb}\delta^{td}(Y_e^\dagger Y_e)^{sc}(Y_dY_d^\dagger)^{pa} - \frac{7}{4}\delta^{pa}\delta^{sc}(Y_e^\dagger Y_e)^{dt}(Y_dY_d^\dagger)^{br} \\
& - \frac{5}{2}\delta^{pa}\delta^{rb}(Y_e^\dagger Y_e)^{sc}(Y_e^\dagger Y_e)^{dt} - \frac{5}{2}\delta^{sc}\delta^{td}(Y_dY_d^\dagger)^{pa}(Y_dY_d^\dagger)^{br} - \frac{5}{2}\delta^{sc}\delta^{td}(Y_uY_u^\dagger)^{pa}(Y_uY_u^\dagger)^{br} - \frac{11}{4}\delta^{rb}\delta^{sc}(Y_e^\dagger Y_e)^{dt}(Y_uY_u^\dagger)^{pa} \\
& - \frac{11}{4}\delta^{pa}\delta^{td}(Y_e^\dagger Y_e)^{sc}(Y_uY_u^\dagger)^{br} \Big\} C_{qe}^{abcd} + \left\{ g_Y^2\left(\frac{22}{27}\delta^{pa}\delta^{st}Y_u^{*rd}Y_u^{bc} + \frac{22}{27}\delta^{rb}\delta^{st}Y_u^{*ad}Y_u^{pc} + 6\delta^{pa}\delta^{rb}\delta^{st}(Y_u^\dagger Y_u)^{dc}\right) + \frac{5072}{243}\delta^{pa}\delta^{rb}\delta^{st}\delta^{cd}g_Y^4 \right. \\
& - 3\delta^{pa}\delta^{rb}(Y_e^\dagger Y_e)^{st}(Y_u^\dagger Y_u)^{dc} - \frac{32}{3}\delta^{pa}\delta^{rb}\delta^{st}\delta^{cd}g_Y^2g_s^2 \Big\} C_{qu}^{(\parallel)abcd} + \left\{ g_Y^2g_s^2\left(\frac{4}{27}\delta^{pr}\delta^{st}\delta^{ab}\delta^{cd} + \frac{2576}{243}\delta^{pa}\delta^{rb}\delta^{st}\delta^{cd}\right) + g_Y^2\left(\frac{16}{9}\delta^{pa}\delta^{rb}\delta^{st}(Y_u^\dagger Y_u)^{dc} \right. \right. \\
& + \frac{25}{9}\delta^{pa}\delta^{st}Y_u^{*rd}Y_u^{bc} + \frac{25}{9}\delta^{rb}\delta^{st}Y_u^{*ad}Y_u^{pc} - \frac{2}{9}\delta^{st}\delta^{ab}Y_u^{*rd}Y_u^{pc}) + \frac{5072}{729}\delta^{pa}\delta^{rb}\delta^{st}\delta^{cd}g_Y^4 - \delta^{pa}\delta^{rb}(Y_e^\dagger Y_e)^{st}(Y_u^\dagger Y_u)^{dc} \Big\} C_{qu}^{(\times)abcd} \\
& + \left\{ \frac{650}{243}\delta^{pa}\delta^{rb}\delta^{st}\delta^{cd}g_Y^4 + 3\delta^{pa}\delta^{rb}(Y_d^\dagger Y_d)^{dc}(Y_e^\dagger Y_e)^{st} + \frac{16}{3}\delta^{pa}\delta^{rb}\delta^{st}\delta^{cd}g_Y^2g_s^2 - g_Y^2\left(\frac{14}{27}\delta^{pa}\delta^{st}Y_d^{*rd}Y_d^{bc} + \frac{14}{27}\delta^{rb}\delta^{st}Y_d^{*ad}Y_d^{pc} \right. \right. \\
& + 2\delta^{pa}\delta^{rb}\delta^{st}(Y_d^\dagger Y_d)^{dc} \Big\} C_{qd}^{(\parallel)abcd} + \left\{ \frac{650}{729}\delta^{pa}\delta^{rb}\delta^{st}\delta^{cd}g_Y^4 + g_Y^2g_s^2\left(\frac{4}{27}\delta^{pr}\delta^{st}\delta^{ab}\delta^{cd} - \frac{880}{243}\delta^{pa}\delta^{rb}\delta^{st}\delta^{cd}\right) + \delta^{pa}\delta^{rb}(Y_d^\dagger Y_d)^{dc}(Y_e^\dagger Y_e)^{st} \right.
\end{aligned}$$

$$\begin{aligned}
& -g_Y^2 \left( \frac{2}{9} \delta^{st} \delta^{ab} Y_d^{*rd} Y_d^{pc} + \frac{8}{9} \delta^{pa} \delta^{rb} \delta^{st} (Y_d^\dagger Y_d)^{dc} + \frac{11}{9} \delta^{pa} \delta^{st} Y_d^{*rd} Y_d^{bc} + \frac{11}{9} \delta^{rb} \delta^{st} Y_d^{*ad} Y_d^{pc} \right) \left\{ C_{qd}^{(\times)abcd} + \left\{ g_Y^4 \left( \frac{308}{81} \delta^{pr} \delta^{sa} \delta^{tb} \delta^{cd} - \frac{8}{27} \delta^{pr} \delta^{st} \delta^{ab} \delta^{cd} \right) \right. \right. \\
& + \frac{28}{9} \delta^{pr} \delta^{sa} \delta^{tb} g_Y^2 (Y_e^\dagger Y_e)^{dc} + 4 \delta^{sa} \delta^{tb} (Y_e^\dagger Y_e)^{dc} (Y_u Y_u^\dagger)^{pr} - 4 \delta^{sa} \delta^{tb} (Y_e^\dagger Y_e)^{dc} (Y_d Y_d^\dagger)^{pr} \left. \right\} C_{ee}^{abcd} + \left\{ \frac{16}{9} \delta^{st} \delta^{ad} g_Y^2 Y_u^{*rb} Y_u^{pc} - \frac{64}{81} \delta^{pr} \delta^{st} \delta^{ad} \delta^{bc} g_Y^4 \right\} C_{uu}^{abcd} \\
& - \left\{ \frac{16}{81} \delta^{pr} \delta^{st} \delta^{ad} \delta^{bc} g_Y^4 + \frac{8}{9} \delta^{st} \delta^{ad} g_Y^2 Y_d^{*rb} Y_d^{pc} \right\} C_{dd}^{abcd} + \left\{ \frac{3}{2} T_2 \delta^{sa} \delta^{tb} Y_u^{*rd} Y_u^{pc} + \frac{3}{2} \delta^{sa} \delta^{tb} (Y_u^\dagger Y_u)^{dc} (Y_d Y_d^\dagger)^{pr} + \frac{3}{2} \delta^{sa} \delta^{tb} Y_u^{pc} (Y_u^\dagger Y_u Y_u^\dagger)^{rd} \right. \\
& + \frac{3}{2} \delta^{sa} \delta^{tb} Y_u^{*rd} (Y_u Y_u^\dagger Y_u)^{pc} + \frac{16}{9} \delta^{pr} \delta^{sa} \delta^{tb} \delta^{cd} g_Y^2 g_s^2 + \frac{16}{3} \delta^{sa} \delta^{tb} g_s^2 Y_u^{*rd} Y_u^{pc} - \frac{1}{2} \delta^{sa} \delta^{tb} Y_u^{pc} (Y_d^\dagger Y_d Y_u^\dagger)^{rd} - \frac{1}{2} \delta^{sa} \delta^{tb} Y_u^{*rd} (Y_d Y_d^\dagger Y_u)^{pc} \\
& - g_Y^4 \left( \frac{4}{27} \delta^{pr} \delta^{st} \delta^{ab} \delta^{cd} + \frac{178}{81} \delta^{pr} \delta^{sa} \delta^{tb} \delta^{cd} \right) - g_Y^2 \left( \delta^{pr} \delta^{sa} \delta^{tb} (Y_u^\dagger Y_u)^{dc} + \frac{583}{72} \delta^{sa} \delta^{tb} Y_u^{*rd} Y_u^{pc} \right) - \frac{5}{4} \delta^{tb} Y_u^{*rd} Y_u^{pc} (Y_e^\dagger Y_e)^{sa} - \frac{5}{4} \delta^{sa} Y_u^{*rd} Y_u^{pc} (Y_e^\dagger Y_e)^{bt} \\
& - \frac{3}{2} \delta^{sa} \delta^{tb} (Y_u^\dagger Y_u)^{dc} (Y_u Y_u^\dagger)^{pr} - \frac{33}{8} \delta^{sa} \delta^{tb} g_L^2 Y_u^{*rd} Y_u^{pc} - 8 \delta^{pr} \delta^{sa} \delta^{tb} \delta^{cd} g_s^4 \left. \right\} C_{eu}^{abcd} + \left\{ g_Y^4 \left( \frac{2}{27} \delta^{pr} \delta^{st} \delta^{ab} \delta^{cd} + \frac{98}{81} \delta^{pr} \delta^{sa} \delta^{tb} \delta^{cd} \right) \right. \\
& + g_Y^2 \left( \frac{1}{3} \delta^{pr} \delta^{sa} \delta^{tb} (Y_d^\dagger Y_d)^{dc} + \frac{197}{72} \delta^{sa} \delta^{tb} Y_d^{*rd} Y_d^{pc} \right) + \frac{3}{2} T_2 \delta^{sa} \delta^{tb} Y_d^{*rd} Y_d^{pc} + \frac{3}{2} \delta^{sa} \delta^{tb} (Y_d^\dagger Y_d)^{dc} (Y_u Y_u^\dagger)^{pr} + \frac{3}{2} \delta^{sa} \delta^{tb} Y_d^{pc} (Y_d^\dagger Y_d Y_d^\dagger)^{rd} \\
& + \frac{3}{2} \delta^{sa} \delta^{tb} Y_d^{*rd} (Y_d Y_d^\dagger Y_d)^{pc} + \frac{16}{3} \delta^{sa} \delta^{tb} g_s^2 Y_d^{*rd} Y_d^{pc} - \frac{1}{4} \delta^{tb} Y_d^{*rd} Y_d^{pc} (Y_e^\dagger Y_e)^{sa} - \frac{1}{4} \delta^{sa} Y_d^{*rd} Y_d^{pc} (Y_e^\dagger Y_e)^{bt} - \frac{1}{2} \delta^{sa} \delta^{tb} Y_d^{pc} (Y_u^\dagger Y_u Y_d^\dagger)^{rd} \\
& - \frac{1}{2} \delta^{sa} \delta^{tb} Y_d^{*rd} (Y_u Y_u^\dagger Y_d)^{pc} - \frac{8}{9} \delta^{pr} \delta^{sa} \delta^{tb} \delta^{cd} g_Y^2 g_s^2 - \frac{3}{2} \delta^{sa} \delta^{tb} (Y_d^\dagger Y_d)^{dc} (Y_d Y_d^\dagger)^{pr} - \frac{33}{8} \delta^{sa} \delta^{tb} g_L^2 Y_d^{*rd} Y_d^{pc} - 8 \delta^{pr} \delta^{sa} \delta^{tb} \delta^{cd} g_s^4 \left. \right\} C_{ed}^{abcd} \\
& + \left\{ \frac{1}{8} \delta^{rd} \delta^{tb} Y_d^{pc} (Y_e^\dagger Y_e Y_e^\dagger)^{as} + \frac{1}{4} T_2 \delta^{rd} \delta^{tb} Y_e^{*as} Y_d^{pc} + \frac{1}{4} \delta^{rd} Y_e^{*ab} Y_d^{pc} (Y_e^\dagger Y_e)^{st} + \frac{1}{4} \delta^{rd} \delta^{tb} Y_e^{*as} (Y_d Y_d^\dagger Y_d)^{pc} + \frac{1}{4} \delta^{rd} \delta^{tb} Y_e^{*as} (Y_u Y_u^\dagger Y_d)^{pc} \right. \\
& + \frac{5}{8} \delta^{rd} Y_e^{*as} Y_d^{pc} (Y_e^\dagger Y_e)^{bt} + \frac{3}{4} \delta^{tb} Y_e^{*as} Y_d^{dc} (Y_d Y_d^\dagger)^{pr} + g_Y^2 \left( \frac{7}{27} \delta^{rd} \delta^{st} Y_e^{*ab} Y_d^{pc} + \frac{221}{144} \delta^{rd} \delta^{tb} Y_e^{*as} Y_d^{pc} - \frac{1}{9} \delta^{pr} \delta^{tb} Y_e^{*as} Y_d^{dc} \right) + \frac{5}{4} \delta^{tb} Y_e^{*as} Y_d^{pc} (Y_d Y_d^\dagger)^{dr} \\
& + \frac{8}{3} \delta^{rd} \delta^{tb} g_s^2 Y_e^{*as} Y_d^{pc} - \frac{1}{4} \delta^{tb} Y_e^{*as} Y_d^{pc} (Y_u Y_u^\dagger)^{dr} - \frac{3}{4} \delta^{tb} Y_e^{*as} Y_d^{dc} (Y_u Y_u^\dagger)^{pr} - \frac{33}{16} \delta^{rd} \delta^{tb} g_L^2 Y_e^{*as} Y_d^{pc} \left. \right\} C_{ledq}^{abcd} + C_{ledq}^{*abcd} \left\{ \frac{1}{8} \delta^{pd} \delta^{sb} Y_d^{*rc} (Y_e Y_e^\dagger Y_e)^{at} \right. \\
& + \frac{1}{4} T_2 \delta^{pd} \delta^{sb} Y_d^{*rc} Y_e^{at} + \frac{1}{4} \delta^{pd} Y_d^{*rc} Y_e^{ab} (Y_e^\dagger Y_e)^{st} + \frac{1}{4} \delta^{pd} \delta^{sb} Y_e^{at} (Y_d^\dagger Y_d Y_d^\dagger)^{rc} + \frac{1}{4} \delta^{pd} \delta^{sb} Y_e^{at} (Y_u^\dagger Y_u Y_d^\dagger)^{rc} + \frac{5}{8} \delta^{pd} Y_d^{*rc} Y_e^{at} (Y_e^\dagger Y_e)^{sb} \\
& + \frac{3}{4} \delta^{sb} Y_d^{*dc} Y_e^{at} (Y_d Y_d^\dagger)^{pr} + g_Y^2 \left( \frac{7}{27} \delta^{pd} \delta^{st} Y_d^{*rc} Y_e^{ab} + \frac{221}{144} \delta^{pd} \delta^{sb} Y_d^{*rc} Y_e^{at} - \frac{1}{9} \delta^{pr} \delta^{sb} Y_d^{*dc} Y_e^{at} \right) + \frac{5}{4} \delta^{sb} Y_d^{*rc} Y_e^{at} (Y_d Y_d^\dagger)^{pd} + \frac{8}{3} \delta^{pd} \delta^{sb} g_s^2 Y_d^{*rc} Y_e^{at} \\
& - \frac{1}{4} \delta^{sb} Y_d^{*rc} Y_e^{at} (Y_u Y_u^\dagger)^{pd} - \frac{3}{4} \delta^{sb} Y_d^{*dc} Y_e^{at} (Y_u Y_u^\dagger)^{pr} - \frac{33}{16} \delta^{pd} \delta^{sb} g_L^2 Y_d^{*rc} Y_e^{at} \left. \right\} + \left\{ \frac{1}{8} \delta^{pa} Y_d^{*rd} Y_u^{*cb} (Y_e^\dagger Y_e)^{st} + \frac{3}{4} \delta^{pc} Y_d^{*rd} Y_u^{*ab} (Y_e^\dagger Y_e)^{st} \right. \\
& + g_Y^2 \left( \frac{11}{108} \delta^{pa} \delta^{st} Y_d^{*rd} Y_u^{*cb} + \frac{7}{9} \delta^{pc} \delta^{st} Y_d^{*rd} Y_u^{*ab} - \frac{7}{108} \delta^{pc} \delta^{st} Y_d^{*ad} Y_u^{*rb} - \frac{11}{9} \delta^{pa} \delta^{st} Y_d^{*cd} Y_u^{*rb} \right) - \frac{1}{8} \delta^{pc} Y_d^{*ad} Y_u^{*rb} (Y_e^\dagger Y_e)^{st}
\end{aligned}$$

$$\begin{aligned}
& -\frac{3}{4}\delta^{pa}Y_d^{*cd}Y_u^{*rb}(Y_e^\dagger Y_e)^{st}\left\{C_{quqd}^{(\parallel)abcd} + \left(C_{quqd}^{(\parallel)*}\right)^{abcd}\left\{\frac{1}{8}\delta^{ra}Y_d^{pd}Y_u^{cb}(Y_e^\dagger Y_e)^{st} + \frac{3}{4}\delta^{rc}Y_d^{pd}Y_u^{ab}(Y_e^\dagger Y_e)^{st} + g_Y^2\left(\frac{11}{108}\delta^{ra}\delta^{st}Y_d^{pd}Y_u^{cb} + \frac{7}{9}\delta^{rc}\delta^{st}Y_d^{pd}Y_u^{ab}\right.\right.\right. \\
& -\frac{7}{108}\delta^{rc}\delta^{st}Y_d^{ad}Y_u^{pb} - \frac{11}{9}\delta^{ra}\delta^{st}Y_d^{cd}Y_u^{pb}) - \frac{1}{8}\delta^{rc}Y_d^{ad}Y_u^{pb}(Y_e^\dagger Y_e)^{st} - \frac{3}{4}\delta^{ra}Y_d^{cd}Y_u^{pb}(Y_e^\dagger Y_e)^{st}\left.\left.\right\} + \left\{\frac{1}{4}\delta^{pc}Y_d^{*rd}Y_u^{*ab}(Y_e^\dagger Y_e)^{st} + \frac{3}{8}\delta^{pa}Y_d^{*rd}Y_u^{*cb}(Y_e^\dagger Y_e)^{st}\right.\right. \\
& + g_Y^2\left(\frac{5}{36}\delta^{pa}\delta^{st}Y_d^{*rd}Y_u^{*cb} + \frac{11}{54}\delta^{pc}\delta^{st}Y_d^{*rd}Y_u^{*ab} - \frac{13}{36}\delta^{pc}\delta^{st}Y_d^{*ad}Y_u^{*rb} - \frac{25}{54}\delta^{pa}\delta^{st}Y_d^{*cd}Y_u^{*rb}\right) - \frac{1}{4}\delta^{pa}Y_d^{*cd}Y_u^{*rb}(Y_e^\dagger Y_e)^{st} \\
& -\frac{3}{8}\delta^{pc}Y_d^{*ad}Y_u^{*rb}(Y_e^\dagger Y_e)^{st}\left\{C_{quqd}^{(\times)abcd} + \left(C_{quqd}^{(\times)*}\right)^{abcd}\left\{\frac{1}{4}\delta^{rc}Y_d^{pd}Y_u^{ab}(Y_e^\dagger Y_e)^{st} + \frac{3}{8}\delta^{ra}Y_d^{pd}Y_u^{cb}(Y_e^\dagger Y_e)^{st} + g_Y^2\left(\frac{5}{36}\delta^{ra}\delta^{st}Y_d^{pd}Y_u^{cb} + \frac{11}{54}\delta^{rc}\delta^{st}Y_d^{pd}Y_u^{ab}\right.\right.\right. \\
& -\frac{13}{36}\delta^{rc}\delta^{st}Y_d^{ad}Y_u^{pb} - \frac{25}{54}\delta^{ra}\delta^{st}Y_d^{cd}Y_u^{pb}) - \frac{1}{4}\delta^{ra}Y_d^{cd}Y_u^{pb}(Y_e^\dagger Y_e)^{st} - \frac{3}{8}\delta^{rc}Y_d^{ad}Y_u^{pb}(Y_e^\dagger Y_e)^{st}\left.\left.\right\} + \left\{\frac{1}{8}\delta^{pc}\delta^{tb}Y_u^{*rd}(Y_e^\dagger Y_e Y_e^\dagger)^{as} + \frac{1}{4}T_2\delta^{pc}\delta^{tb}Y_e^{*as}Y_u^{*rd}\right.\right. \\
& + \frac{1}{4}\delta^{pc}Y_e^{*ab}Y_u^{*rd}(Y_e^\dagger Y_e)^{st} + \frac{1}{4}\delta^{pc}\delta^{tb}Y_e^{*as}(Y_d^\dagger Y_d Y_u^\dagger)^{rd} + \frac{1}{4}\delta^{pc}\delta^{tb}Y_e^{*as}(Y_u^\dagger Y_u Y_u^\dagger)^{rd} + \frac{5}{8}\delta^{pc}Y_e^{*as}Y_u^{*rd}(Y_e^\dagger Y_e)^{bt} + \frac{3}{4}\delta^{tb}Y_e^{*as}Y_u^{*cd}(Y_u Y_u^\dagger)^{pr} \\
& + \frac{15}{16}\delta^{pc}\delta^{tb}g_L^2Y_e^{*as}Y_u^{*rd} + g_Y^2\left(\frac{1}{9}\delta^{pr}\delta^{tb}Y_e^{*as}Y_u^{*cd} + \frac{11}{27}\delta^{pc}\delta^{st}Y_e^{*ab}Y_u^{*rd} + \frac{773}{144}\delta^{pc}\delta^{tb}Y_e^{*as}Y_u^{*rd}\right) + \frac{5}{4}\delta^{tb}Y_e^{*as}Y_u^{*rd}(Y_u Y_u^\dagger)^{pc} \\
& + \frac{8}{3}\delta^{pc}\delta^{tb}g_s^2Y_e^{*as}Y_u^{*rd} - \frac{1}{4}\delta^{tb}Y_e^{*as}Y_u^{*rd}(Y_d Y_d^\dagger)^{pc} - \frac{3}{4}\delta^{tb}Y_e^{*as}Y_u^{*cd}(Y_d Y_d^\dagger)^{pr}\left\{C_{lequ}^{abcd} + C_{lequ}^{*abcd}\left\{\frac{1}{8}\delta^{rc}\delta^{sb}Y_u^{pd}(Y_e Y_e^\dagger Y_e)^{at} + \frac{1}{4}T_2\delta^{rc}\delta^{sb}Y_e^{at}Y_u^{pd}\right.\right. \\
& + \frac{1}{4}\delta^{rc}Y_e^{ab}Y_u^{pd}(Y_e^\dagger Y_e)^{st} + \frac{1}{4}\delta^{rc}\delta^{sb}Y_e^{at}(Y_d Y_d^\dagger Y_u)^{pd} + \frac{1}{4}\delta^{rc}\delta^{sb}Y_e^{at}(Y_u Y_u^\dagger Y_u)^{pd} + \frac{5}{8}\delta^{rc}Y_e^{at}Y_u^{pd}(Y_e^\dagger Y_e)^{sb} + \frac{3}{4}\delta^{sb}Y_e^{at}Y_u^{cd}(Y_u Y_u^\dagger)^{pr} + \frac{15}{16}\delta^{rc}\delta^{sb}g_L^2Y_e^{at}Y_u^{pd} \\
& + g_Y^2\left(\frac{1}{9}\delta^{pr}\delta^{sb}Y_e^{at}Y_u^{cd} + \frac{11}{27}\delta^{rc}\delta^{st}Y_e^{ab}Y_u^{pd} + \frac{773}{144}\delta^{rc}\delta^{sb}Y_e^{at}Y_u^{pd}\right) + \frac{5}{4}\delta^{sb}Y_e^{at}Y_u^{pd}(Y_u Y_u^\dagger)^{cr} + \frac{8}{3}\delta^{rc}\delta^{sb}g_s^2Y_e^{at}Y_u^{pd} - \frac{1}{4}\delta^{sb}Y_e^{at}Y_u^{pd}(Y_d Y_d^\dagger)^{cr} \\
& -\frac{3}{4}\delta^{sb}Y_e^{at}Y_u^{cd}(Y_d Y_d^\dagger)^{pr}\left.\left.\right\} + \left\{\frac{3}{8}\delta^{td}Y_e^{*as}Y_u^{*cb}(Y_d Y_d^\dagger)^{pr} + \frac{3}{8}\delta^{td}Y_e^{*as}Y_u^{*rb}(Y_d Y_d^\dagger)^{pc} + \frac{9}{4}\delta^{pc}\delta^{td}g_L^2Y_e^{*as}Y_u^{*rb} - \frac{1}{8}\delta^{pc}Y_e^{*ad}Y_u^{*rb}(Y_e^\dagger Y_e)^{st}\right.\right. \\
& -\frac{1}{8}\delta^{pc}Y_e^{*as}Y_u^{*rb}(Y_e^\dagger Y_e)^{dt} - \frac{1}{4}\delta^{td}Y_e^{*as}Y_u^{*rb}(Y_u Y_u^\dagger)^{pc} - \frac{3}{8}\delta^{td}Y_e^{*as}Y_u^{*cb}(Y_u Y_u^\dagger)^{pr} - \frac{1}{2}\delta^{pc}\delta^{td}Y_u^{*rb}(Y_e^\dagger Y_e Y_e^\dagger)^{as} - T_2\delta^{pc}\delta^{td}Y_e^{*as}Y_u^{*rb} \\
& - g_Y^2\left(\frac{13}{108}\delta^{pc}\delta^{st}Y_e^{*ad}Y_u^{*rb} + \frac{5}{36}\delta^{pr}\delta^{td}Y_e^{*as}Y_u^{*cb} + \frac{109}{36}\delta^{pc}\delta^{td}Y_e^{*as}Y_u^{*rb}\right) - \delta^{pc}\delta^{td}Y_e^{*as}(Y_u^\dagger Y_u Y_u^\dagger)^{rb} - \frac{4}{3}\delta^{pc}\delta^{td}g_s^2Y_e^{*as}Y_u^{*rb}\left.\left.\right\}C_{luqe}^{abcd} \right. \\
& + C_{luqe}^{*abcd}\left\{\frac{3}{8}\delta^{sd}Y_e^{at}Y_u^{cb}(Y_d Y_d^\dagger)^{pr} + \frac{3}{8}\delta^{sd}Y_e^{at}Y_u^{pb}(Y_d Y_d^\dagger)^{cr} + \frac{9}{4}\delta^{rc}\delta^{sd}g_L^2Y_e^{at}Y_u^{pb} - \frac{1}{8}\delta^{rc}Y_e^{ad}Y_u^{pb}(Y_e^\dagger Y_e)^{st} - \frac{1}{8}\delta^{rc}Y_e^{at}Y_u^{pb}(Y_e^\dagger Y_e)^{sd} - \frac{1}{4}\delta^{sd}Y_e^{at}Y_u^{pb}(Y_u Y_u^\dagger)^{cr}\right. \\
& -\frac{3}{8}\delta^{sd}Y_e^{at}Y_u^{cb}(Y_u Y_u^\dagger)^{pr} - \frac{1}{2}\delta^{rc}\delta^{sd}Y_u^{pb}(Y_e Y_e^\dagger Y_e)^{at} - T_2\delta^{rc}\delta^{sd}Y_e^{at}Y_u^{pb} - g_Y^2\left(\frac{13}{108}\delta^{rc}\delta^{st}Y_e^{ad}Y_u^{pb} + \frac{5}{36}\delta^{pr}\delta^{sd}Y_e^{at}Y_u^{cb} + \frac{109}{36}\delta^{rc}\delta^{sd}Y_e^{at}Y_u^{pb}\right) \\
& \left. -\delta^{rc}\delta^{sd}Y_e^{at}(Y_u Y_u^\dagger Y_u)^{pb} - \frac{4}{3}\delta^{rc}\delta^{sd}g_s^2Y_e^{at}Y_u^{pb}\right\} + \left\{\frac{4}{9}\delta^{pr}\delta^{bc}g_Y^2Y_e^{*as}Y_e^{dt} - \frac{8}{27}\delta^{pr}\delta^{st}\delta^{ad}\delta^{bc}g_Y^4\right\}C_{\ell\ell}^{abcd} + \left\{g_Y^2g_s^2\left(\frac{8}{27}\delta^{pr}\delta^{st}\delta^{ad}\delta^{bc}\right.\right.
\end{aligned}$$

$$\begin{aligned}
& -\frac{44}{243}\delta^{pa}\delta^{rd}\delta^{st}\delta^{bc} - 8\delta^{pa}\delta^{rb}\delta^{st}\delta^{cd}) + g_Y^2 g_L^2 \left( \frac{58}{27}\delta^{pa}\delta^{rd}\delta^{st}\delta^{bc} - 6\delta^{pa}\delta^{rb}\delta^{st}\delta^{cd} \right) + g_Y^4 \left( \frac{248}{243}\delta^{pa}\delta^{rb}\delta^{st}\delta^{cd} - \frac{8}{81}\delta^{pr}\delta^{st}\delta^{ad}\delta^{bc} \right. \\
& - \frac{158}{729}\delta^{pa}\delta^{rd}\delta^{st}\delta^{bc} \Big) + g_Y^2 \left( \frac{4}{9}\delta^{pa}\delta^{rd}\delta^{st}(Y_d Y_d^\dagger)^{bc} + \frac{16}{9}\delta^{pa}\delta^{rd}\delta^{st}(Y_u Y_u^\dagger)^{bc} + 8\delta^{pa}\delta^{rb}\delta^{st}(Y_u Y_u^\dagger)^{dc} \right) + 3\delta^{pa}\delta^{rd}(Y_e^\dagger Y_e)^{st}(Y_u Y_u^\dagger)^{bc} \\
& + 6\delta^{pa}\delta^{rb}(Y_e^\dagger Y_e)^{st}(Y_u Y_u^\dagger)^{dc} - 3\delta^{pa}\delta^{rd}(Y_e^\dagger Y_e)^{st}(Y_d Y_d^\dagger)^{bc} - 6\delta^{pa}\delta^{rb}(Y_e^\dagger Y_e)^{st}(Y_d Y_d^\dagger)^{dc} \Big\} C_{qq}^{(\parallel)abcd} + \left\{ g_Y^2 g_s^2 \left( \frac{16}{27}\delta^{pr}\delta^{st}\delta^{ad}\delta^{bc} - \frac{88}{243}\delta^{pa}\delta^{rd}\delta^{st}\delta^{bc} \right. \right. \\
& - 4\delta^{pa}\delta^{rb}\delta^{st}\delta^{cd} \Big) + g_Y^4 \left( \frac{124}{243}\delta^{pa}\delta^{rb}\delta^{st}\delta^{cd} - \frac{16}{81}\delta^{pr}\delta^{st}\delta^{ad}\delta^{bc} - \frac{316}{729}\delta^{pa}\delta^{rd}\delta^{st}\delta^{bc} \right) + g_Y^2 g_L^2 \left( \frac{16}{9}\delta^{pa}\delta^{rb}\delta^{st}\delta^{cd} - 2\delta^{pa}\delta^{rd}\delta^{st}\delta^{bc} \right) \\
& + g_Y^2 \left( \frac{8}{9}\delta^{pa}\delta^{rd}\delta^{st}(Y_d Y_d^\dagger)^{bc} + \frac{32}{9}\delta^{pa}\delta^{rd}\delta^{st}(Y_u Y_u^\dagger)^{bc} + 4\delta^{pa}\delta^{rb}\delta^{st}(Y_u Y_u^\dagger)^{dc} \right) + 3\delta^{pa}\delta^{rb}(Y_e^\dagger Y_e)^{st}(Y_u Y_u^\dagger)^{dc} + 6\delta^{pa}\delta^{rd}(Y_e^\dagger Y_e)^{st}(Y_u Y_u^\dagger)^{bc} \\
& - 3\delta^{pa}\delta^{rb}(Y_e^\dagger Y_e)^{st}(Y_d Y_d^\dagger)^{dc} - 6\delta^{pa}\delta^{rd}(Y_e^\dagger Y_e)^{st}(Y_d Y_d^\dagger)^{bc} \Big\} C_{qq}^{(\times)abcd} + \left\{ g_Y^2 \left( \frac{13}{4}\delta^{pc}\delta^{rd}Y_e^{*as}Y_e^{bt} - \frac{8}{3}\delta^{pc}\delta^{rd}\delta^{st}(Y_e Y_e^\dagger)^{ba} \right) + \frac{3}{2}\delta^{pc}\delta^{rd}Y_e^{bt}(Y_e^\dagger Y_e Y_e^\dagger)^{as} \right. \\
& + \frac{3}{2}\delta^{pc}\delta^{rd}Y_e^{*as}(Y_e Y_e^\dagger Y_e)^{bt} + 3T_2\delta^{pc}\delta^{rd}Y_e^{*as}Y_e^{bt} + 3\delta^{pc}\delta^{rd}\delta^{st}\delta^{ab}g_Y^2 g_L^2 - \frac{1}{4}\delta^{rd}Y_e^{*as}Y_e^{bt}(Y_d Y_d^\dagger)^{pc} - \frac{1}{4}\delta^{pc}Y_e^{*as}Y_e^{bt}(Y_d Y_d^\dagger)^{dr} \\
& - \delta^{pc}\delta^{rd}(Y_e^\dagger Y_e)^{st}(Y_e Y_e^\dagger)^{ba} - \frac{5}{4}\delta^{rd}Y_e^{*as}Y_e^{bt}(Y_u Y_u^\dagger)^{pc} - \frac{5}{4}\delta^{pc}Y_e^{*as}Y_e^{bt}(Y_u Y_u^\dagger)^{dr} - \frac{1816}{243}\delta^{pc}\delta^{rd}\delta^{st}\delta^{ab}g_Y^4 - \frac{51}{4}\delta^{pc}\delta^{rd}g_L^2 Y_e^{*as}Y_e^{bt} \Big\} C_{\ell q}^{(\parallel)abcd} \\
& + \left\{ \frac{3}{4}\delta^{pc}\delta^{rd}Y_e^{bt}(Y_e^\dagger Y_e Y_e^\dagger)^{as} + \frac{3}{4}\delta^{pc}\delta^{rd}Y_e^{*as}(Y_e Y_e^\dagger Y_e)^{bt} + g_Y^2 \left( \frac{13}{8}\delta^{pc}\delta^{rd}Y_e^{*as}Y_e^{bt} - \frac{4}{3}\delta^{pc}\delta^{rd}\delta^{st}(Y_e Y_e^\dagger)^{ba} \right) + \frac{5}{4}\delta^{rd}Y_e^{*as}Y_e^{bt}(Y_u Y_u^\dagger)^{pc} \right. \\
& + \frac{5}{4}\delta^{pc}Y_e^{*as}Y_e^{bt}(Y_u Y_u^\dagger)^{dr} + \frac{3}{2}T_2\delta^{pc}\delta^{rd}Y_e^{*as}Y_e^{bt} + \frac{44}{27}\delta^{pc}\delta^{rd}\delta^{st}\delta^{ab}g_Y^2 g_L^2 + \frac{15}{8}\delta^{pc}\delta^{rd}g_L^2 Y_e^{*as}Y_e^{bt} - \frac{1}{2}\delta^{rd}Y_e^{*as}Y_e^{bt}(Y_d Y_d^\dagger)^{pc} \\
& \left. - \frac{1}{2}\delta^{pc}Y_e^{*as}Y_e^{bt}(Y_d Y_d^\dagger)^{dr} - \frac{1}{2}\delta^{pc}\delta^{rd}(Y_e^\dagger Y_e)^{st}(Y_e Y_e^\dagger)^{ba} - \frac{908}{243}\delta^{pc}\delta^{rd}\delta^{st}\delta^{ab}g_Y^4 \right\} C_{\ell q}^{(\times)abcd}, \tag{10.8}
\end{aligned}$$

## 10.5 $C_{qu}^{(\parallel)}$

$$\begin{aligned}
\beta_{C_{qu}^{(\parallel)prst}}^{(1)} &= \left\{ \frac{4}{9}\delta^{pa}\delta^{rb}\delta^{st}g_Y^2 - 2\delta^{pa}\delta^{rb}(Y_u^\dagger Y_u)^{st} \right\} C_{Hq}^{(\parallel)ab} + \left\{ \frac{2}{9}\delta^{pa}\delta^{rb}\delta^{st}g_Y^2 - \delta^{pa}\delta^{rb}(Y_u^\dagger Y_u)^{st} \right\} C_{Hq}^{(\times)ab} + \left\{ \frac{1}{9}\delta^{pr}\delta^{sa}\delta^{tb}g_Y^2 + \delta^{sa}\delta^{tb}(Y_u Y_u^\dagger)^{pr} \right. \\
& - \delta^{sa}\delta^{tb}(Y_d Y_d^\dagger)^{pr} \Big\} C_{Hu}^{ab} - \frac{2}{9}\delta^{pr}\delta^{sc}\delta^{td}\delta^{ab}g_Y^2 C_{\ell u}^{abcd} - \frac{8}{9}\delta^{pa}\delta^{rb}\delta^{st}\delta^{cd}g_Y^2 C_{qe}^{abcd} + \left\{ \frac{1}{2} \left( \delta^{rb}\delta^{sc}\delta^{td}(Y_d Y_d^\dagger)^{pa} + \delta^{pa}\delta^{sc}\delta^{td}(Y_d Y_d^\dagger)^{br} + \delta^{rb}\delta^{sc}\delta^{td}(Y_u Y_u^\dagger)^{pa} \right. \right. \\
& + \delta^{pa}\delta^{sc}\delta^{td}(Y_u Y_u^\dagger)^{br} + 2\delta^{pa}\delta^{rb}\delta^{td}(Y_u^\dagger Y_u)^{sc} + 2\delta^{pa}\delta^{rb}\delta^{sc}(Y_u^\dagger Y_u)^{dt} \Big) + 2\delta^{pa}\delta^{rb}\delta^{sc}\delta^{td}g_s^2 - \frac{2}{9}g_Y^2 \left( 6\delta^{pa}\delta^{rb}\delta^{sc}\delta^{td} - \delta^{pr}\delta^{sc}\delta^{td}\delta^{ab} \right. \\
& \left. \left. - 8\delta^{pa}\delta^{rb}\delta^{st}\delta^{cd} \right) \right\} C_{qu}^{(\parallel)abcd} + \left\{ \frac{2}{27}g_Y^2 \left( \delta^{pr}\delta^{sc}\delta^{td}\delta^{ab} + 8\delta^{pa}\delta^{rb}\delta^{st}\delta^{cd} \right) + \delta^{pa}\delta^{sc}Y_u^{*rd}Y_u^{bt} + \delta^{rb}\delta^{td}Y_u^{*as}Y_u^{pc} - \frac{2}{9}g_s^2 \left( \delta^{pa}\delta^{rb}\delta^{st}\delta^{cd} \right. \right.
\end{aligned}$$

$$\begin{aligned}
& + 2\delta^{pr}\delta^{sc}\delta^{td}\delta^{ab}) \Big\} C_{qu}^{(\times)abcd} - \frac{8}{9}\delta^{pa}\delta^{rb}\delta^{st}\delta^{cd}g_Y^2 C_{qd}^{(\parallel)abcd} - \left\{ \frac{2}{9}\delta^{pa}\delta^{rb}\delta^{st}\delta^{cd}g_s^2 + \frac{8}{27}\delta^{pa}\delta^{rb}\delta^{st}\delta^{cd}g_Y^2 \right\} C_{qd}^{(\times)abcd} + \left\{ \frac{8}{27}g_Y^2 \left( \delta^{pr}\delta^{sa}\delta^{td}\delta^{bc} \right. \right. \\
& + 3\delta^{pr}\delta^{sa}\delta^{tb}\delta^{cd}) - \frac{4}{9}\delta^{pr}\delta^{sa}\delta^{td}\delta^{bc}g_s^2 - 2\delta^{sa}\delta^{tb}Y_u^{*rd}Y_u^{pc} \Big\} C_{uu}^{abcd} - \frac{2}{9}\delta^{pr}\delta^{sc}\delta^{td}\delta^{ab}g_Y^2 C_{eu}^{abcd} - \left\{ \frac{2}{9}\delta^{pr}\delta^{sa}\delta^{tb}\delta^{cd}g_Y^2 + \delta^{sa}\delta^{tb}Y_d^{*rd}Y_d^{pc} \right\} C_{ud}^{(\parallel)abcd} \\
& - \left\{ \frac{2}{27}\delta^{pr}\delta^{sa}\delta^{tb}\delta^{cd}g_Y^2 + \frac{2}{9}\delta^{pr}\delta^{sa}\delta^{tb}\delta^{cd}g_s^2 \right\} C_{ud}^{(\times)abcd} + \frac{1}{2}\delta^{pc}\delta^{tb}Y_d^{*rd}Y_u^{*as} C_{quqd}^{(\parallel)abcd} + \frac{1}{2}\delta^{rc}\delta^{sb} \left( C_{quqd}^{(\parallel)*} \right)^{abcd} Y_d^{pd}Y_u^{at} + \delta^{pa}\delta^{tb}Y_d^{*rd}Y_u^{*cs} C_{quqd}^{(\times)abcd} \\
& + \delta^{ra}\delta^{sb} \left( C_{quqd}^{(\times)*} \right)^{abcd} Y_d^{pd}Y_u^{ct} + \left\{ \frac{8}{27}g_Y^2 \left( \delta^{pa}\delta^{rd}\delta^{st}\delta^{bc} + 6\delta^{pa}\delta^{rb}\delta^{st}\delta^{cd} \right) - \frac{4}{9}\delta^{pa}\delta^{rd}\delta^{st}\delta^{bc}g_s^2 - 4\delta^{pa}\delta^{rb}Y_u^{*cs}Y_u^{dt} \right\} C_{qq}^{(\parallel)abcd} + \left\{ \frac{8}{27}g_Y^2 \left( 2\delta^{pa}\delta^{rd}\delta^{st}\delta^{bc} \right. \right. \\
& + 3\delta^{pa}\delta^{rb}\delta^{st}\delta^{cd}) - \frac{8}{9}\delta^{pa}\delta^{rd}\delta^{st}\delta^{bc}g_s^2 - 2\delta^{pa}\delta^{rb}Y_u^{*cs}Y_u^{dt} \Big\} C_{qq}^{(\times)abcd} - \frac{8}{9}\delta^{pc}\delta^{rd}\delta^{st}\delta^{ab}g_Y^2 C_{\ell q}^{(\parallel)abcd} - \frac{4}{9}\delta^{pc}\delta^{rd}\delta^{st}\delta^{ab}g_Y^2 C_{\ell q}^{(\times)abcd}, \tag{10.9}
\end{aligned}$$

$$\begin{aligned}
\beta_{C_{qu}^{(\parallel)prst}}^{(2)} &= \left\{ \frac{8}{27}\delta^{pr}\delta^{st}g_Y^6 + g_Y^4 \left( \frac{2}{9}\delta^{st}(Y_u Y_u^\dagger)^{pr} - \frac{10}{9}\delta^{st}(Y_d Y_d^\dagger)^{pr} - \frac{11}{9}\delta^{pr}(Y_u^\dagger Y_u)^{st} \right) \right\} C_{HB} + g_s^4 \left\{ \frac{2}{3}\delta^{st}(Y_d Y_d^\dagger)^{pr} + \frac{2}{3}\delta^{st}(Y_u Y_u^\dagger)^{pr} + \frac{4}{3}\delta^{pr}(Y_u^\dagger Y_u)^{st} \right. \\
& + 12Y_u^{*rs}Y_u^{pt} \Big\} C_{HG} + \left\{ \frac{2}{9}\delta^{pr}\delta^{st}g_Y^4 g_L^2 + g_Y^2 g_L^2 \left( \frac{3}{2}\delta^{st}(Y_u Y_u^\dagger)^{pr} - \frac{1}{4}\delta^{pr}(Y_u^\dagger Y_u)^{st} - \frac{3}{2}\delta^{st}(Y_d Y_d^\dagger)^{pr} \right) \right\} C_{HWB} + \left\{ \frac{20}{9}\delta^{pr}\delta^{st}g_Y^2 g_L^6 - \frac{10}{3}\delta^{pr}\delta^{st}g_s^2 g_L^6 \right\} C_W \\
& + \left\{ g_s^6 \left( \frac{3}{2}\delta^{st}(Y_d Y_d^\dagger)^{pr} + \frac{3}{2}\delta^{st}(Y_u Y_u^\dagger)^{pr} + 3\delta^{pr}(Y_u^\dagger Y_u)^{st} + 27Y_u^{*rs}Y_u^{pt} \right) + \frac{446}{27}\delta^{pr}\delta^{st}g_Y^2 g_s^6 + \frac{434}{9}\delta^{pr}\delta^{st}g_s^8 \right\} C_G - \frac{4}{9}\delta^{pr}\delta^{st}g_Y^4 Y_e^{*ab} C_{eB}^{ab} \\
& - \frac{4}{9}\delta^{pr}\delta^{st}g_Y^4 C_{eB}^{*ab} Y_e^{ab} + \left\{ g_Y^4 \left( \frac{20}{27}\delta^{pr}\delta^{st}Y_u^{*ab} + \frac{149}{81}\delta^{pa}\delta^{st}Y_u^{*rb} - \frac{8}{81}\delta^{pr}\delta^{tb}Y_u^{*as} \right) + g_Y^2 g_s^2 \left( 10\delta^{pa}\delta^{tb}Y_u^{*rs} - \frac{50}{27}\delta^{pr}\delta^{tb}Y_u^{*as} - \frac{115}{27}\delta^{pa}\delta^{st}Y_u^{*rb} \right) \right. \\
& + g_Y^2 \left( \frac{2}{3}\delta^{st}Y_u^{*rb}(Y_d Y_d^\dagger)^{pa} + \frac{4}{3}\delta^{tb}Y_u^{*as}(Y_d Y_d^\dagger)^{pr} - \frac{1}{3}\delta^{pr}Y_u^{*as}(Y_u^\dagger Y_u)^{bt} - \frac{1}{2}\delta^{pa}Y_u^{*rb}(Y_u^\dagger Y_u)^{st} - \frac{4}{3}\delta^{st}Y_u^{*rb}(Y_u Y_u^\dagger)^{pa} - 2\delta^{tb}Y_u^{*as}(Y_u Y_u^\dagger)^{pr} \Big\} C_{uB}^{ab} \\
& + C_{uB}^{*ab} \left\{ g_Y^4 \left( \frac{20}{27}\delta^{pr}\delta^{st}Y_u^{ab} + \frac{149}{81}\delta^{ra}\delta^{st}Y_u^{pb} - \frac{8}{81}\delta^{pr}\delta^{sb}Y_u^{at} \right) + g_Y^2 g_s^2 \left( 10\delta^{ra}\delta^{sb}Y_u^{pt} - \frac{50}{27}\delta^{pr}\delta^{sb}Y_u^{at} - \frac{115}{27}\delta^{ra}\delta^{st}Y_u^{pb} \right) + g_Y^2 \left( \frac{2}{3}\delta^{st}Y_u^{pb}(Y_d Y_d^\dagger)^{ar} \right. \right. \\
& + \frac{4}{3}\delta^{sb}Y_u^{at}(Y_d Y_d^\dagger)^{pr} - \frac{1}{3}\delta^{pr}Y_u^{at}(Y_u^\dagger Y_u)^{sb} - \frac{1}{2}\delta^{ra}Y_u^{pb}(Y_u^\dagger Y_u)^{st} - \frac{4}{3}\delta^{st}Y_u^{pb}(Y_u Y_u^\dagger)^{ar} - 2\delta^{sb}Y_u^{at}(Y_u Y_u^\dagger)^{pr} \Big\} + \left\{ g_s^2 g_L^2 \left( \frac{1}{6}\delta^{pa}\delta^{st}Y_u^{*rb} + \frac{4}{3}\delta^{pr}\delta^{tb}Y_u^{*as} \right. \right. \\
& + 9\delta^{pa}\delta^{tb}Y_u^{*rs} \Big\} + g_L^2 \left( 6\delta^{tb}Y_u^{*as}(Y_d Y_d^\dagger)^{pr} - \frac{9}{4}\delta^{pa}Y_u^{*rb}(Y_u^\dagger Y_u)^{st} \right) + \frac{9}{2}\delta^{pr}\delta^{tb}g_L^4 Y_u^{*as} - g_Y^2 g_L^2 \left( \frac{7}{18}\delta^{pr}\delta^{tb}Y_u^{*as} + \frac{11}{18}\delta^{pa}\delta^{st}Y_u^{*rb} \right) \Big\} C_{uW}^{ab}
\end{aligned}$$

$$\begin{aligned}
& + C_{uW}^{*ab} \left\{ g_s^2 g_L^2 \left( \frac{1}{6} \delta^{ra} \delta^{st} Y_u^{pb} + \frac{4}{3} \delta^{pr} \delta^{sb} Y_u^{at} + 9 \delta^{ra} \delta^{sb} Y_u^{pt} \right) + g_L^2 \left( 6 \delta^{sb} Y_u^{at} (Y_d Y_d^\dagger)^{pr} - \frac{9}{4} \delta^{ra} Y_u^{pb} (Y_u^\dagger Y_u)^{st} \right) + \frac{9}{2} \delta^{pr} \delta^{sb} g_L^4 Y_u^{at} - g_Y^2 g_L^2 \left( \frac{7}{18} \delta^{pr} \delta^{sb} Y_u^{at} \right. \right. \\
& + \left. \frac{11}{18} \delta^{ra} \delta^{st} Y_u^{pb} \right) \left. \right\} + \left\{ g_s^4 \left( \frac{19}{27} \delta^{pa} \delta^{st} Y_u^{*rb} + \frac{38}{27} \delta^{pr} \delta^{tb} Y_u^{*as} - \frac{4}{9} \delta^{pr} \delta^{st} Y_u^{*ab} - 29 \delta^{pa} \delta^{tb} Y_u^{*rs} \right) + g_Y^2 g_s^2 \left( \frac{7}{6} \delta^{pa} \delta^{tb} Y_u^{*rs} - \frac{49}{81} \delta^{pr} \delta^{tb} Y_u^{*as} \right. \right. \\
& - \frac{362}{81} \delta^{pa} \delta^{st} Y_u^{*rb} \left. \right) + g_s^2 \left( \frac{1}{3} \delta^{pr} Y_u^{*as} (Y_u^\dagger Y_u)^{bt} + \frac{1}{3} \delta^{st} Y_u^{*rb} (Y_u Y_u^\dagger)^{pa} + \frac{3}{2} \delta^{pa} Y_u^{*rs} (Y_u^\dagger Y_u)^{bt} + 3 T_2 \delta^{pa} \delta^{tb} Y_u^{*rs} + 3 \delta^{tb} Y_u^{*rs} (Y_u Y_u^\dagger)^{pa} \right. \\
& + \frac{17}{3} \delta^{tb} Y_u^{*as} (Y_d Y_d^\dagger)^{pr} - \frac{1}{6} \delta^{st} Y_u^{*rb} (Y_d Y_d^\dagger)^{pa} - 2 \delta^{pa} \delta^{tb} (Y_d^\dagger Y_d Y_u^\dagger)^{rs} - 3 \delta^{tb} Y_u^{*rs} (Y_d Y_d^\dagger)^{pa} - 4 \delta^{pa} Y_u^{*rb} (Y_u^\dagger Y_u)^{st} - 4 \delta^{tb} Y_u^{*as} (Y_u Y_u^\dagger)^{pr} \left. \right) \\
& - \frac{9}{2} \delta^{pa} \delta^{tb} g_s^2 g_L^2 Y_u^{*rs} \left. \right\} C_{uG}^{ab} + C_{uG}^{*ab} \left\{ g_s^4 \left( \frac{19}{27} \delta^{ra} \delta^{st} Y_u^{pb} + \frac{38}{27} \delta^{pr} \delta^{sb} Y_u^{at} - \frac{4}{9} \delta^{pr} \delta^{st} Y_u^{ab} - 29 \delta^{ra} \delta^{sb} Y_u^{pt} \right) + g_Y^2 g_s^2 \left( \frac{7}{6} \delta^{ra} \delta^{sb} Y_u^{pt} - \frac{49}{81} \delta^{pr} \delta^{sb} Y_u^{at} \right. \right. \\
& - \frac{362}{81} \delta^{ra} \delta^{st} Y_u^{pb} \left. \right) + g_s^2 \left( \frac{1}{3} \delta^{pr} Y_u^{at} (Y_u^\dagger Y_u)^{sb} + \frac{1}{3} \delta^{st} Y_u^{pb} (Y_u Y_u^\dagger)^{ar} + \frac{3}{2} \delta^{ra} Y_u^{pt} (Y_u^\dagger Y_u)^{sb} + 3 T_2 \delta^{ra} \delta^{sb} Y_u^{pt} + 3 \delta^{sb} Y_u^{pt} (Y_u Y_u^\dagger)^{ar} + \frac{17}{3} \delta^{sb} Y_u^{at} (Y_d Y_d^\dagger)^{pr} \right. \\
& - \frac{1}{6} \delta^{st} Y_u^{pb} (Y_d Y_d^\dagger)^{ar} - 2 \delta^{ra} \delta^{sb} (Y_d Y_d^\dagger Y_u)^{pt} - 3 \delta^{sb} Y_u^{pt} (Y_d Y_d^\dagger)^{ar} - 4 \delta^{ra} Y_u^{pb} (Y_u^\dagger Y_u)^{st} - 4 \delta^{sb} Y_u^{at} (Y_u Y_u^\dagger)^{pr} \left. \right) - \frac{9}{2} \delta^{ra} \delta^{sb} g_s^2 g_L^2 Y_u^{pt} \left. \right\} \\
& + \left\{ g_Y^2 \left( \frac{2}{3} \delta^{st} Y_d^{*rb} (Y_u Y_u^\dagger)^{pa} - \frac{4}{3} \delta^{st} Y_d^{*rb} (Y_d Y_d^\dagger)^{pa} - \frac{31}{6} \delta^{pa} Y_d^{*rb} (Y_u^\dagger Y_u)^{st} \right) - g_Y^4 \left( \frac{4}{27} \delta^{pr} \delta^{st} Y_d^{*ab} + \frac{145}{81} \delta^{pa} \delta^{st} Y_d^{*rb} \right) - \frac{139}{27} \delta^{pa} \delta^{st} g_Y^2 g_s^2 Y_d^{*rb} \right\} C_{dB}^{ab} \\
& + C_{dB}^{*ab} \left\{ g_Y^2 \left( \frac{2}{3} \delta^{st} Y_d^{pb} (Y_u Y_u^\dagger)^{ar} - \frac{4}{3} \delta^{st} Y_d^{pb} (Y_d Y_d^\dagger)^{ar} - \frac{31}{6} \delta^{ra} Y_d^{pb} (Y_u^\dagger Y_u)^{st} \right) - g_Y^4 \left( \frac{4}{27} \delta^{pr} \delta^{st} Y_d^{ab} + \frac{145}{81} \delta^{ra} \delta^{st} Y_d^{pb} \right) - \frac{139}{27} \delta^{ra} \delta^{st} g_Y^2 g_s^2 Y_d^{pb} \right\} \\
& + \left\{ \frac{1}{6} \delta^{pa} \delta^{st} g_s^2 g_L^2 Y_d^{*rb} + \frac{7}{18} \delta^{pa} \delta^{st} g_Y^2 g_L^2 Y_d^{*rb} + \frac{15}{4} \delta^{pa} g_L^2 Y_d^{*rb} (Y_u^\dagger Y_u)^{st} \right\} C_{dW}^{ab} + C_{dW}^{*ab} \left\{ \frac{1}{6} \delta^{ra} \delta^{st} g_s^2 g_L^2 Y_d^{pb} + \frac{7}{18} \delta^{ra} \delta^{st} g_Y^2 g_L^2 Y_d^{pb} \right. \\
& + \left. \frac{15}{4} \delta^{ra} g_L^2 Y_d^{pb} (Y_u^\dagger Y_u)^{st} \right\} + \left\{ g_s^4 \left( \frac{19}{27} \delta^{pa} \delta^{st} Y_d^{*rb} - \frac{4}{9} \delta^{pr} \delta^{st} Y_d^{*ab} \right) + g_s^2 \left( \frac{1}{3} \delta^{st} Y_d^{*rb} (Y_d Y_d^\dagger)^{pa} + Y_d^{*rb} Y_u^{*as} Y_u^{pt} + \frac{17}{3} \delta^{pa} Y_d^{*rb} (Y_u^\dagger Y_u)^{st} \right. \right. \\
& - \frac{1}{6} \delta^{st} Y_d^{*rb} (Y_u Y_u^\dagger)^{pa} - \frac{3}{2} \delta^{pa} Y_u^{*rs} (Y_d^\dagger Y_u)^{bt} \left. \right) + \frac{169}{81} \delta^{pa} \delta^{st} g_Y^2 g_s^2 Y_d^{*rb} \left. \right\} C_{dG}^{ab} + C_{dG}^{*ab} \left\{ g_s^4 \left( \frac{19}{27} \delta^{ra} \delta^{st} Y_d^{pb} - \frac{4}{9} \delta^{pr} \delta^{st} Y_d^{ab} \right) + g_s^2 \left( \frac{1}{3} \delta^{st} Y_d^{pb} (Y_d Y_d^\dagger)^{ar} \right. \right. \\
& + Y_u^{*rs} Y_d^{pb} Y_u^{at} + \frac{17}{3} \delta^{ra} Y_d^{pb} (Y_u^\dagger Y_u)^{st} - \frac{1}{6} \delta^{st} Y_d^{pb} (Y_u Y_u^\dagger)^{ar} - \frac{3}{2} \delta^{ra} Y_u^{pt} (Y_u^\dagger Y_d)^{sb} \left. \right) + \frac{169}{81} \delta^{ra} \delta^{st} g_Y^2 g_s^2 Y_d^{pb} \left. \right\} + \left\{ g_s^2 \left( \frac{7}{54} \delta^{rb} \delta^{st} (Y_u Y_u^\dagger)^{pa} \right. \right. \\
& + \frac{7}{54} \delta^{pa} \delta^{st} (Y_u Y_u^\dagger)^{br} + 17 \delta^{pa} \delta^{rb} (Y_u^\dagger Y_u)^{st} - \frac{7}{54} \delta^{rb} \delta^{st} (Y_d Y_d^\dagger)^{pa} - \frac{7}{54} \delta^{pa} \delta^{st} (Y_d Y_d^\dagger)^{br} \left. \right) + g_Y^2 \left( \frac{31}{162} \delta^{rb} \delta^{st} (Y_u Y_u^\dagger)^{pa} + \frac{31}{162} \delta^{pa} \delta^{st} (Y_u Y_u^\dagger)^{br} \right. \\
& + \frac{59}{162} \delta^{rb} \delta^{st} (Y_d Y_d^\dagger)^{pa} + \frac{59}{162} \delta^{pa} \delta^{st} (Y_d Y_d^\dagger)^{br} - \frac{4}{9} T_2 \delta^{pa} \delta^{rb} \delta^{st} - \frac{55}{12} \delta^{pa} \delta^{rb} (Y_u^\dagger Y_u)^{st} \left. \right) + 2 T_2 \delta^{pa} \delta^{rb} (Y_u^\dagger Y_u)^{st} + \frac{1538}{729} \delta^{pa} \delta^{rb} \delta^{st} g_Y^4
\end{aligned}$$

$$\begin{aligned}
& + 3\delta^{pa}\delta^{rb}(Y_u^\dagger Y_u Y_u^\dagger Y_u)^{st} + 4\delta^{pa}\delta^{rb}\delta^{st}g_Y^2g_L^2 - \frac{1}{4}\delta^{rb}(Y_u^\dagger Y_u)^{st}(Y_d Y_d^\dagger)^{pa} - \frac{1}{4}\delta^{pa}(Y_u^\dagger Y_u)^{st}(Y_d Y_d^\dagger)^{br} - \frac{1}{4}\delta^{rb}(Y_u^\dagger Y_u)^{st}(Y_u Y_u^\dagger)^{pa} - \frac{1}{4}\delta^{pa}(Y_u^\dagger Y_u)^{st}(Y_u Y_u^\dagger)^{br} \\
& - \frac{283}{243}\delta^{pa}\delta^{rb}\delta^{st}g_Y^2g_s^2 - \frac{51}{4}\delta^{pa}\delta^{rb}g_L^2(Y_u^\dagger Y_u)^{st} \Big\} C_{Hq}^{(\parallel)ab} + \left\{ \frac{1}{4}\delta^{rb}(Y_u^\dagger Y_u)^{st}(Y_u Y_u^\dagger)^{pa} + \frac{1}{4}\delta^{pa}(Y_u^\dagger Y_u)^{st}(Y_u Y_u^\dagger)^{br} + \frac{23}{54}\delta^{pa}\delta^{rb}\delta^{st}g_s^2g_L^2 \right. \\
& + T_2\delta^{pa}\delta^{rb}(Y_u^\dagger Y_u)^{st} + g_Y^2\left(\frac{59}{81}\delta^{rb}\delta^{st}(Y_d Y_d^\dagger)^{pa} + \frac{59}{81}\delta^{pa}\delta^{st}(Y_d Y_d^\dagger)^{br} - \frac{31}{162}\delta^{rb}\delta^{st}(Y_u Y_u^\dagger)^{pa} - \frac{31}{162}\delta^{pa}\delta^{st}(Y_u Y_u^\dagger)^{br} - \frac{2}{9}T_2\delta^{pa}\delta^{rb}\delta^{st} \right. \\
& - \frac{55}{24}\delta^{pa}\delta^{rb}(Y_u^\dagger Y_u)^{st} \Big) + g_s^2\left(\frac{17}{2}\delta^{pa}\delta^{rb}(Y_u^\dagger Y_u)^{st} - \frac{7}{54}\delta^{rb}\delta^{st}(Y_u Y_u^\dagger)^{pa} - \frac{7}{54}\delta^{pa}\delta^{st}(Y_u Y_u^\dagger)^{br} - \frac{7}{27}\delta^{rb}\delta^{st}(Y_d Y_d^\dagger)^{pa} - \frac{7}{27}\delta^{pa}\delta^{st}(Y_d Y_d^\dagger)^{br} \right) \\
& + \frac{769}{729}\delta^{pa}\delta^{rb}\delta^{st}g_Y^4 + \frac{3}{2}\delta^{pa}\delta^{rb}(Y_u^\dagger Y_u Y_u^\dagger Y_u)^{st} + \frac{139}{81}\delta^{pa}\delta^{rb}\delta^{st}g_Y^2g_L^2 - \frac{1}{2}\delta^{rb}(Y_u^\dagger Y_u)^{st}(Y_d Y_d^\dagger)^{pa} - \frac{1}{2}\delta^{pa}(Y_u^\dagger Y_u)^{st}(Y_d Y_d^\dagger)^{br} - \frac{283}{486}\delta^{pa}\delta^{rb}\delta^{st}g_Y^2g_s^2 \\
& - \frac{15}{8}\delta^{pa}\delta^{rb}g_L^2(Y_u^\dagger Y_u)^{st} \Big\} C_{Hq}^{(\times)ab} + \left\{ \frac{31}{486}\delta^{pr}\delta^{sa}\delta^{tb}g_Y^2g_s^2 + \frac{1}{4}\delta^{tb}(Y_u^\dagger Y_u)^{sa}(Y_u Y_u^\dagger)^{pr} + \frac{1}{4}\delta^{sa}(Y_u^\dagger Y_u)^{bt}(Y_u Y_u^\dagger)^{pr} + \frac{212}{729}\delta^{pr}\delta^{sa}\delta^{tb}g_Y^4 \right. \\
& + \delta^{pr}\delta^{sa}\delta^{tb}g_Y^2g_L^2 + T_2\delta^{sa}\delta^{tb}(Y_d Y_d^\dagger)^{pr} + g_s^2\left(\frac{17}{2}\delta^{sa}\delta^{tb}(Y_d Y_d^\dagger)^{pr} - \frac{7}{27}\delta^{pr}\delta^{tb}(Y_u^\dagger Y_u)^{sa} - \frac{7}{27}\delta^{pr}\delta^{sa}(Y_u^\dagger Y_u)^{bt} - \frac{17}{2}\delta^{sa}\delta^{tb}(Y_u Y_u^\dagger)^{pr} \right) \\
& + g_L^2\left(\frac{33}{8}\delta^{sa}\delta^{tb}(Y_u Y_u^\dagger)^{pr} - \frac{33}{8}\delta^{sa}\delta^{tb}(Y_d Y_d^\dagger)^{pr} \right) + g_Y^2\left(\frac{101}{324}\delta^{pr}\delta^{tb}(Y_u^\dagger Y_u)^{sa} + \frac{101}{324}\delta^{pr}\delta^{sa}(Y_u^\dagger Y_u)^{bt} + \frac{145}{24}\delta^{sa}\delta^{tb}(Y_u Y_u^\dagger)^{pr} - \frac{1}{9}T_2\delta^{pr}\delta^{sa}\delta^{tb} \right. \\
& - \frac{53}{24}\delta^{sa}\delta^{tb}(Y_d Y_d^\dagger)^{pr} \Big) + 3\delta^{sa}\delta^{tb}(Y_d Y_d^\dagger Y_d Y_d^\dagger)^{pr} - \frac{1}{4}\delta^{tb}(Y_u^\dagger Y_u)^{sa}(Y_d Y_d^\dagger)^{pr} - \frac{1}{4}\delta^{sa}(Y_u^\dagger Y_u)^{bt}(Y_d Y_d^\dagger)^{pr} - T_2\delta^{sa}\delta^{tb}(Y_u Y_u^\dagger)^{pr} \\
& - 3\delta^{sa}\delta^{tb}(Y_u Y_u^\dagger Y_u Y_u^\dagger)^{pr} \Big\} C_{Hu}^{ab} + \left\{ \frac{1}{27}\delta^{pr}\delta^{sa}g_s^2(Y_d^\dagger Y_u)^{bt} + \frac{55}{324}\delta^{pr}\delta^{sa}g_Y^2(Y_d^\dagger Y_u)^{bt} + \frac{3}{4}\delta^{sa}(Y_d^\dagger Y_u)^{bt}(Y_u Y_u^\dagger)^{pr} - \frac{3}{4}\delta^{sa}(Y_d^\dagger Y_u)^{bt}(Y_d Y_d^\dagger)^{pr} \right\} C_{Hud}^{ab} \\
& + C_{Hud}^{*ab} \left\{ \frac{1}{27}\delta^{pr}\delta^{ta}g_s^2(Y_u^\dagger Y_d)^{sb} + \frac{55}{324}\delta^{pr}\delta^{ta}g_Y^2(Y_u^\dagger Y_d)^{sb} + \frac{3}{4}\delta^{ta}(Y_u^\dagger Y_d)^{sb}(Y_u Y_u^\dagger)^{pr} - \frac{3}{4}\delta^{ta}(Y_u^\dagger Y_d)^{sb}(Y_d Y_d^\dagger)^{pr} \right\} + \left\{ \frac{4}{9}\delta^{pr}\delta^{sc}\delta^{td}g_Y^2(Y_e Y_e^\dagger)^{ba} \right. \\
& + \frac{1}{2}\delta^{sc}\delta^{td}(Y_d Y_d^\dagger)^{pr}(Y_e Y_e^\dagger)^{ba} + \frac{9}{2}\delta^{pr}\delta^{sc}\delta^{td}\delta^{ab}g_L^4 - \frac{37}{243}\delta^{pr}\delta^{sc}\delta^{td}\delta^{ab}g_Y^2g_s^2 - \frac{1}{2}\delta^{pr}\delta^{sc}\delta^{td}\delta^{ab}g_Y^2g_L^2 - \frac{1}{2}\delta^{sc}\delta^{td}(Y_e Y_e^\dagger)^{ba}(Y_u Y_u^\dagger)^{pr} \\
& - \frac{520}{729}\delta^{pr}\delta^{sc}\delta^{td}\delta^{ab}g_Y^4 \Big\} C_{\ell u}^{abcd} + \left\{ \frac{32}{729}\delta^{pa}\delta^{rb}\delta^{st}\delta^{cd}g_Y^4 + \frac{362}{243}\delta^{pa}\delta^{rb}\delta^{st}\delta^{cd}g_Y^2g_s^2 + \frac{20}{9}\delta^{pa}\delta^{rb}\delta^{st}g_Y^2(Y_e^\dagger Y_e)^{dc} - \delta^{pa}\delta^{rb}(Y_e^\dagger Y_e)^{dc}(Y_u^\dagger Y_u)^{st} \right\} C_{qe}^{abcd} \\
& + \left\{ g_Y^2g_L^2\left(\frac{1}{2}\delta^{pr}\delta^{sc}\delta^{td}\delta^{ab} + 3\delta^{pa}\delta^{rb}\delta^{sc}\delta^{td}\right) + g_Y^2g_s^2\left(\frac{253}{243}\delta^{pr}\delta^{sc}\delta^{td}\delta^{ab} + \frac{1004}{243}\delta^{pa}\delta^{rb}\delta^{st}\delta^{cd} + \frac{169}{18}\delta^{pa}\delta^{rb}\delta^{sc}\delta^{td}\right) + g_s^4\left(9\delta^{pa}\delta^{rb}\delta^{sc}\delta^{td} \right. \right. \\
& + \frac{83}{9}\delta^{pa}\delta^{rb}\delta^{st}\delta^{cd} + \frac{166}{9}\delta^{pr}\delta^{sc}\delta^{td}\delta^{ab} \Big) + g_Y^4\left(\frac{6776}{729}\delta^{pa}\delta^{rb}\delta^{st}\delta^{cd} + \frac{494}{27}\delta^{pa}\delta^{rb}\delta^{sc}\delta^{td} - \frac{218}{729}\delta^{pr}\delta^{sc}\delta^{td}\delta^{ab}\right) + \delta^{pa}Y_u^{*rd}Y_u^{bc}(Y_u^\dagger Y_u)^{st} \\
& + \delta^{rb}Y_u^{*ad}Y_u^{pc}(Y_u^\dagger Y_u)^{st} + \delta^{sc}Y_u^{*ad}Y_u^{bt}(Y_u Y_u^\dagger)^{pr} + \delta^{td}Y_u^{*as}Y_u^{bc}(Y_u Y_u^\dagger)^{pr} + \delta^{sc}\delta^{td}(Y_d Y_d^\dagger)^{br}(Y_u Y_u^\dagger)^{pa} + \delta^{sc}\delta^{td}(Y_d Y_d^\dagger)^{pa}(Y_u Y_u^\dagger)^{br} + g_s^2\left(\frac{4}{27}\delta^{pa}\delta^{st}Y_u^{*rd}Y_u^{bc} \right. \\
& + \frac{4}{27}\delta^{rb}\delta^{st}Y_u^{*ad}Y_u^{pc} + \frac{8}{27}\delta^{pr}\delta^{sc}Y_u^{*ad}Y_u^{bt} + \frac{8}{27}\delta^{pr}\delta^{td}Y_u^{*as}Y_u^{bc} + 6\delta^{rb}\delta^{sc}Y_u^{*ad}Y_u^{pt} + 6\delta^{pa}\delta^{td}Y_u^{*rs}Y_u^{bc} - 2\delta^{pa}\delta^{sc}Y_u^{*rd}Y_u^{bt} - 2\delta^{rb}\delta^{td}Y_u^{*as}Y_u^{pc}
\end{aligned}$$



$$\begin{aligned}
& -\frac{11}{3}\delta^{rb}\delta^{sc}\delta^{td}(Y_d Y_d^\dagger)^{pa} - \frac{11}{3}\delta^{pa}\delta^{sc}\delta^{td}(Y_d Y_d^\dagger)^{br} - \frac{11}{3}\delta^{rb}\delta^{sc}\delta^{td}(Y_u Y_u^\dagger)^{pa} - \frac{11}{3}\delta^{pa}\delta^{sc}\delta^{td}(Y_u Y_u^\dagger)^{br} - \frac{22}{3}\delta^{pa}\delta^{rb}\delta^{td}(Y_u^\dagger Y_u)^{sc} - \frac{22}{3}\delta^{pa}\delta^{rb}\delta^{sc}(Y_u^\dagger Y_u)^{dt} \\
& + g_L^2 \left( \frac{33}{16}\delta^{rb}\delta^{sc}\delta^{td}(Y_d Y_d^\dagger)^{pa} + \frac{33}{16}\delta^{pa}\delta^{sc}\delta^{td}(Y_d Y_d^\dagger)^{br} + \frac{33}{16}\delta^{rb}\delta^{sc}\delta^{td}(Y_u Y_u^\dagger)^{pa} + \frac{33}{16}\delta^{pa}\delta^{sc}\delta^{td}(Y_u Y_u^\dagger)^{br} + \frac{51}{8}\delta^{pa}\delta^{rb}\delta^{td}(Y_u^\dagger Y_u)^{sc} \right. \\
& + \frac{51}{8}\delta^{pa}\delta^{rb}\delta^{sc}(Y_u^\dagger Y_u)^{dt} \Big) + g_Y^2 \left( \frac{2}{81}\delta^{pr}\delta^{sc}Y_u^{*ad}Y_u^{bt} + \frac{2}{81}\delta^{pr}\delta^{td}Y_u^{*as}Y_u^{bc} + \frac{73}{72}\delta^{pa}\delta^{rb}\delta^{td}(Y_u^\dagger Y_u)^{sc} + \frac{73}{72}\delta^{pa}\delta^{rb}\delta^{sc}(Y_u^\dagger Y_u)^{dt} + \frac{523}{144}\delta^{rb}\delta^{sc}\delta^{td}(Y_u Y_u^\dagger)^{pa} \right. \\
& + \frac{523}{144}\delta^{pa}\delta^{sc}\delta^{td}(Y_u Y_u^\dagger)^{br} - \frac{41}{144}\delta^{rb}\delta^{sc}\delta^{td}(Y_d Y_d^\dagger)^{pa} - \frac{41}{144}\delta^{pa}\delta^{sc}\delta^{td}(Y_d Y_d^\dagger)^{br} - \frac{44}{81}\delta^{pa}\delta^{st}Y_u^{*rd}Y_u^{bc} - \frac{44}{81}\delta^{rb}\delta^{st}Y_u^{*ad}Y_u^{pc} - \frac{2}{3}\delta^{pr}\delta^{sc}\delta^{td}(Y_u Y_u^\dagger)^{ba} \\
& - 4\delta^{pa}\delta^{rb}\delta^{st}(Y_u^\dagger Y_u)^{dc} \Big) + \frac{3}{2}\delta^{sc}\delta^{td}(Y_d Y_d^\dagger)^{pr}(Y_d Y_d^\dagger)^{ba} + \frac{3}{2}\delta^{sc}\delta^{td}(Y_u Y_u^\dagger)^{pr}(Y_u Y_u^\dagger)^{ba} + 2\delta^{rb}\delta^{sc}(Y_u^\dagger Y_u)^{dt}(Y_u Y_u^\dagger)^{pa} + 2\delta^{pa}\delta^{td}(Y_u^\dagger Y_u)^{sc}(Y_u Y_u^\dagger)^{br} \\
& + 3\delta^{pa}\delta^{rb}(Y_u^\dagger Y_u)^{st}(Y_u^\dagger Y_u)^{dc} + \frac{27}{2}\delta^{pr}\delta^{sc}\delta^{td}\delta^{ab}g_L^4 - \frac{1}{4}\delta^{pa}\delta^{rb}\delta^{td}(Y_u^\dagger Y_d Y_d^\dagger Y_u)^{sc} - \frac{1}{4}\delta^{pa}\delta^{rb}\delta^{sc}(Y_u^\dagger Y_d Y_d^\dagger Y_u)^{dt} - \frac{1}{4}\delta^{pa}\delta^{rb}\delta^{td}(Y_u^\dagger Y_u Y_u^\dagger Y_u)^{sc} \\
& - \frac{1}{4}\delta^{pa}\delta^{rb}\delta^{sc}(Y_u^\dagger Y_u Y_u^\dagger Y_u)^{dt} - \frac{1}{4}\delta^{rb}\delta^{sc}\delta^{td}(Y_d Y_d^\dagger Y_d Y_d^\dagger)^{pa} - \frac{1}{4}\delta^{pa}\delta^{sc}\delta^{td}(Y_d Y_d^\dagger Y_d Y_d^\dagger)^{br} - \frac{1}{4}\delta^{rb}\delta^{sc}\delta^{td}(Y_u Y_u^\dagger Y_u Y_u^\dagger)^{pa} - \frac{1}{4}\delta^{pa}\delta^{sc}\delta^{td}(Y_u Y_u^\dagger Y_u Y_u^\dagger)^{br} \\
& - \frac{3}{4}T_2\delta^{rb}\delta^{sc}\delta^{td}(Y_d Y_d^\dagger)^{pa} - \frac{3}{4}T_2\delta^{pa}\delta^{sc}\delta^{td}(Y_d Y_d^\dagger)^{br} - \frac{3}{4}T_2\delta^{rb}\delta^{sc}\delta^{td}(Y_u Y_u^\dagger)^{pa} - \frac{3}{4}T_2\delta^{pa}\delta^{sc}\delta^{td}(Y_u Y_u^\dagger)^{br} - \delta^{rb}\delta^{td}(Y_u^\dagger Y_u)^{sc}(Y_d Y_d^\dagger)^{pa} \\
& - \delta^{pa}\delta^{sc}(Y_u^\dagger Y_u)^{dt}(Y_d Y_d^\dagger)^{br} - \frac{5}{4}\delta^{rb}\delta^{td}(Y_u^\dagger Y_u)^{sc}(Y_u Y_u^\dagger)^{pa} - \frac{5}{4}\delta^{pa}\delta^{sc}(Y_u^\dagger Y_u)^{dt}(Y_u Y_u^\dagger)^{br} - \frac{3}{2}T_2\delta^{pa}\delta^{rb}\delta^{td}(Y_u^\dagger Y_u)^{sc} - \frac{3}{2}T_2\delta^{pa}\delta^{rb}\delta^{sc}(Y_u^\dagger Y_u)^{dt} \\
& - \frac{3}{2}\delta^{sc}\delta^{td}(Y_d Y_d^\dagger)^{ba}(Y_u Y_u^\dagger)^{pr} - \frac{3}{2}\delta^{sc}\delta^{td}(Y_d Y_d^\dagger)^{pr}(Y_u Y_u^\dagger)^{ba} - \frac{5}{2}\delta^{pa}\delta^{rb}(Y_u^\dagger Y_u)^{sc}(Y_u^\dagger Y_u)^{dt} - \frac{5}{2}\delta^{sc}\delta^{td}(Y_d Y_d^\dagger)^{pa}(Y_d Y_d^\dagger)^{br} - \frac{5}{2}\delta^{sc}\delta^{td}(Y_u Y_u^\dagger)^{pa}(Y_u Y_u^\dagger)^{br} \\
& - \frac{11}{4}\delta^{rb}\delta^{sc}(Y_u^\dagger Y_u)^{dt}(Y_d Y_d^\dagger)^{pa} - \frac{11}{4}\delta^{pa}\delta^{td}(Y_u^\dagger Y_u)^{sc}(Y_d Y_d^\dagger)^{br} - \frac{9}{2}\delta^{pa}\delta^{rb}\delta^{sc}\delta^{td}g_s^2g_L^2 \Big\} C_{qu}^{(II)abcd} + \left\{ \frac{1}{6}\delta^{pr}\delta^{sc}\delta^{td}\delta^{ab}g_Y^2g_L^2 + \frac{1}{4}\delta^{rb}\delta^{td}Y_u^{pc}(Y_u^\dagger Y_u Y_u^\dagger)^{as} \right. \\
& + \frac{1}{4}\delta^{pa}\delta^{sc}Y_u^{*rd}(Y_u Y_u^\dagger Y_u)^{bt} + \frac{1}{2}T_2\delta^{pa}\delta^{sc}Y_u^{*rd}Y_u^{bt} + \frac{1}{2}T_2\delta^{rb}\delta^{td}Y_u^{*as}Y_u^{pc} + \frac{1}{2}\delta^{sc}Y_u^{*rd}Y_u^{bt}(Y_d Y_d^\dagger)^{pa} + \frac{1}{2}\delta^{td}Y_u^{*as}Y_u^{pc}(Y_d Y_d^\dagger)^{br} \\
& + \frac{1}{2}\delta^{sc}\delta^{td}(Y_d Y_d^\dagger)^{pr}(Y_d Y_d^\dagger)^{ba} + \frac{1}{2}\delta^{sc}\delta^{td}(Y_u Y_u^\dagger)^{pr}(Y_u Y_u^\dagger)^{ba} + \frac{1}{2}\delta^{pa}\delta^{sc}Y_u^{bt}(Y_u^\dagger Y_u Y_u^\dagger)^{rd} + \frac{1}{2}\delta^{rb}\delta^{td}Y_u^{*as}(Y_u Y_u^\dagger Y_u)^{pc} + g_L^2 \left( \frac{15}{8}\delta^{pa}\delta^{sc}Y_u^{*rd}Y_u^{bt} \right. \\
& + \frac{15}{8}\delta^{rb}\delta^{td}Y_u^{*as}Y_u^{pc} \Big) + g_s^2g_L^2 \left( \frac{27}{4}\delta^{pa}\delta^{rb}\delta^{sc}\delta^{td} - \delta^{pr}\delta^{sc}\delta^{td}\delta^{ab} \right) + g_Y^4 \left( \frac{6776}{2187}\delta^{pa}\delta^{rb}\delta^{st}\delta^{cd} - \frac{218}{2187}\delta^{pr}\delta^{sc}\delta^{td}\delta^{ab} \right) + g_Y^2g_s^2 \left( \frac{25}{4}\delta^{pa}\delta^{rb}\delta^{sc}\delta^{td} \right. \\
& - \frac{16}{81}\delta^{pr}\delta^{st}\delta^{ab}\delta^{cd} - \frac{1600}{729}\delta^{pr}\delta^{sc}\delta^{td}\delta^{ab} - \frac{7388}{729}\delta^{pa}\delta^{rb}\delta^{st}\delta^{cd} \Big) + g_s^4 \left( \frac{8}{27}\delta^{pr}\delta^{st}\delta^{ab}\delta^{cd} + \frac{812}{243}\delta^{pa}\delta^{rb}\delta^{st}\delta^{cd} + \frac{1516}{243}\delta^{pr}\delta^{sc}\delta^{td}\delta^{ab} \right. \\
& - \frac{177}{2}\delta^{pa}\delta^{rb}\delta^{sc}\delta^{td} \Big) + \delta^{pa}\delta^{rb}(Y_u^\dagger Y_u)^{st}(Y_u^\dagger Y_u)^{dc} + g_Y^2 \left( \frac{4}{27}\delta^{st}\delta^{ab}Y_u^{*rd}Y_u^{pc} + \frac{4}{27}\delta^{pr}\delta^{cd}Y_u^{*as}Y_u^{bt} + \frac{13}{72}\delta^{pa}\delta^{sc}Y_u^{*rd}Y_u^{bt} + \frac{13}{72}\delta^{rb}\delta^{td}Y_u^{*as}Y_u^{pc} \right. \\
& - \frac{2}{27}\delta^{pr}\delta^{sc}\delta^{td}(Y_u Y_u^\dagger)^{ba} - \frac{10}{27}\delta^{pr}\delta^{sc}Y_u^{*ad}Y_u^{bt} - \frac{10}{27}\delta^{pr}\delta^{td}Y_u^{*as}Y_u^{bc} - \frac{32}{27}\delta^{pa}\delta^{rb}\delta^{st}(Y_u^\dagger Y_u)^{dc} - \frac{50}{27}\delta^{pa}\delta^{st}Y_u^{*rd}Y_u^{bc} - \frac{50}{27}\delta^{rb}\delta^{st}Y_u^{*ad}Y_u^{pc} \Big) \\
& + g_s^2 \left( \frac{1}{9}\delta^{pa}\delta^{st}Y_u^{*rd}Y_u^{bc} + \frac{1}{9}\delta^{rb}\delta^{st}Y_u^{*ad}Y_u^{pc} + \frac{2}{9}\delta^{pr}\delta^{sc}Y_u^{*ad}Y_u^{bt} + \frac{2}{9}\delta^{pr}\delta^{td}Y_u^{*as}Y_u^{bc} + \frac{4}{9}\delta^{pa}\delta^{rb}\delta^{st}(Y_u^\dagger Y_u)^{dc} + \frac{4}{9}\delta^{pr}\delta^{sc}\delta^{td}(Y_u Y_u^\dagger)^{ba} + \frac{2}{3}\delta^{pa}\delta^{cd}Y_u^{*rs}Y_u^{bt} \right. \\
& + \frac{2}{3}\delta^{rb}\delta^{cd}Y_u^{*as}Y_u^{pt} + \frac{2}{3}\delta^{pr}\delta^{sc}\delta^{td}(Y_d Y_d^\dagger)^{ba} + \frac{4}{3}\delta^{sc}\delta^{ab}Y_u^{*rd}Y_u^{pt} + \frac{4}{3}\delta^{td}\delta^{ab}Y_u^{*rs}Y_u^{pc} + 18\delta^{rb}\delta^{sc}Y_u^{*ad}Y_u^{pt} + 18\delta^{pa}\delta^{td}Y_u^{*rs}Y_u^{bc} - \frac{2}{9}\delta^{st}\delta^{ab}Y_u^{*rd}Y_u^{pc}
\end{aligned}$$

$$\begin{aligned}
& -\frac{2}{9}\delta^{pr}\delta^{cd}Y_u^{*as}Y_u^{bt} - \frac{88}{3}\delta^{pa}\delta^{sc}Y_u^{*rd}Y_u^{bt} - \frac{88}{3}\delta^{rb}\delta^{td}Y_u^{*as}Y_u^{pc} \Big) + 3\delta^{pa}Y_u^{*rd}Y_u^{bc}(Y_u^\dagger Y_u)^{st} + 3\delta^{rb}Y_u^{*ad}Y_u^{pc}(Y_u^\dagger Y_u)^{st} + 3\delta^{sc}Y_u^{*ad}Y_u^{bt}(Y_u Y_u^\dagger)^{pr} \\
& + 3\delta^{td}Y_u^{*as}Y_u^{bc}(Y_u Y_u^\dagger)^{pr} + \frac{9}{2}\delta^{pr}\delta^{sc}\delta^{td}\delta^{ab}g_L^4 - \frac{1}{2}\delta^{sc}\delta^{td}(Y_d Y_d^\dagger)^{ba}(Y_u Y_u^\dagger)^{pr} - \frac{1}{2}\delta^{sc}\delta^{td}(Y_d Y_d^\dagger)^{pr}(Y_u Y_u^\dagger)^{ba} - \frac{3}{4}\delta^{pa}Y_u^{*rd}Y_u^{bt}(Y_u^\dagger Y_u)^{sc} \\
& - \frac{3}{4}\delta^{rb}Y_u^{*as}Y_u^{pc}(Y_u^\dagger Y_u)^{dt} - \frac{5}{4}\delta^{rb}\delta^{td}Y_u^{pc}(Y_d^\dagger Y_d Y_u^\dagger)^{as} - \frac{5}{4}\delta^{pa}\delta^{sc}Y_u^{*rd}(Y_d Y_d^\dagger Y_u)^{bt} - \frac{3}{2}\delta^{sc}Y_u^{*rd}Y_u^{bt}(Y_u Y_u^\dagger)^{pa} - \frac{3}{2}\delta^{td}Y_u^{*as}Y_u^{pc}(Y_u Y_u^\dagger)^{br} \\
& - \frac{3}{2}\delta^{pa}\delta^{sc}Y_u^{bt}(Y_d^\dagger Y_d Y_u^\dagger)^{rd} - \frac{3}{2}\delta^{rb}\delta^{td}Y_u^{*as}(Y_d Y_d^\dagger Y_u)^{pc} \Big\} C_{qu}^{(\times)abcd} + \left\{ g_s^2 \left( \frac{4}{27}\delta^{pa}\delta^{st}Y_d^{*rd}Y_d^{bc} + \frac{4}{27}\delta^{rb}\delta^{st}Y_d^{*ad}Y_d^{pc} \right) + g_Y^2 \left( \frac{28}{81}\delta^{pa}\delta^{st}Y_d^{*rd}Y_d^{bc} \right. \right. \\
& + \frac{28}{81}\delta^{rb}\delta^{st}Y_d^{*ad}Y_d^{pc} + \frac{4}{3}\delta^{pa}\delta^{rb}\delta^{st}(Y_d^\dagger Y_d)^{dc} \Big) + \frac{83}{9}\delta^{pa}\delta^{rb}\delta^{st}\delta^{cd}g_s^4 - \frac{40}{729}\delta^{pa}\delta^{rb}\delta^{st}\delta^{cd}g_Y^4 - \frac{1}{2}\delta^{pa}\delta^{rb}(Y_d^\dagger Y_u)^{dt}(Y_u^\dagger Y_d)^{sc} - \frac{3}{2}Y_d^{*rd}Y_u^{*as}Y_d^{pc}Y_u^{bt} \\
& - \frac{502}{243}\delta^{pa}\delta^{rb}\delta^{st}\delta^{cd}g_Y^2g_s^2 - 3\delta^{pa}\delta^{rb}(Y_d^\dagger Y_d)^{dc}(Y_u^\dagger Y_u)^{st} \Big\} C_{qd}^{(\parallel)abcd} + \left\{ g_Y^2g_s^2 \left( \frac{2419}{729}\delta^{pa}\delta^{rb}\delta^{st}\delta^{cd} - \frac{8}{81}\delta^{pr}\delta^{st}\delta^{ab}\delta^{cd} \right) + g_s^4 \left( \frac{4}{27}\delta^{pr}\delta^{st}\delta^{ab}\delta^{cd} \right. \right. \\
& + \frac{812}{243}\delta^{pa}\delta^{rb}\delta^{st}\delta^{cd} \Big) + g_s^2 \left( \frac{1}{9}\delta^{pa}\delta^{st}Y_d^{*rd}Y_d^{bc} + \frac{1}{9}\delta^{rb}\delta^{st}Y_d^{*ad}Y_d^{pc} + \frac{4}{9}\delta^{pa}\delta^{rb}\delta^{st}(Y_d^\dagger Y_d)^{dc} + \frac{2}{3}\delta^{pa}\delta^{cd}Y_u^{*rs}Y_u^{bt} + \frac{2}{3}\delta^{rb}\delta^{cd}Y_u^{*as}Y_u^{pt} - \frac{2}{9}\delta^{st}\delta^{ab}Y_d^{*rd}Y_d^{pc} \right) \\
& + g_Y^2 \left( \frac{4}{27}\delta^{st}\delta^{ab}Y_d^{*rd}Y_d^{pc} + \frac{16}{27}\delta^{pa}\delta^{rb}\delta^{st}(Y_d^\dagger Y_d)^{dc} + \frac{22}{27}\delta^{pa}\delta^{st}Y_d^{*rd}Y_d^{bc} + \frac{22}{27}\delta^{rb}\delta^{st}Y_d^{*ad}Y_d^{pc} \right) - \frac{40}{2187}\delta^{pa}\delta^{rb}\delta^{st}\delta^{cd}g_Y^4 - \frac{1}{4}\delta^{rb}Y_u^{*as}Y_d^{pc}(Y_d^\dagger Y_u)^{dt} \\
& - \frac{1}{4}\delta^{pa}Y_d^{*rd}Y_u^{bt}(Y_u^\dagger Y_d)^{sc} - \delta^{pa}\delta^{rb}(Y_d^\dagger Y_d)^{dc}(Y_u^\dagger Y_u)^{st} \Big\} C_{qd}^{(\times)abcd} + \frac{32}{81}\delta^{pr}\delta^{st}\delta^{ab}\delta^{cd}g_Y^4 C_{ee}^{abcd} + \left\{ g_Y^4 \left( \frac{128}{243}\delta^{pr}\delta^{st}\delta^{ad}\delta^{bc} - \frac{368}{729}\delta^{pr}\delta^{sa}\delta^{tb}\delta^{cd} \right. \right. \\
& - \frac{2144}{2187}\delta^{pr}\delta^{sa}\delta^{td}\delta^{bc} \Big) + g_Y^2g_s^2 \left( \frac{1520}{729}\delta^{pr}\delta^{sa}\delta^{td}\delta^{bc} + \frac{796}{243}\delta^{pr}\delta^{sa}\delta^{tb}\delta^{cd} - \frac{8}{81}\delta^{pr}\delta^{st}\delta^{ad}\delta^{bc} \right) + g_s^2 \left( \frac{4}{9}\delta^{st}\delta^{ad}Y_u^{*rb}Y_u^{pc} + \frac{4}{3}\delta^{tb}\delta^{ad}Y_u^{*rs}Y_u^{pc} \right. \\
& + \frac{4}{3}\delta^{sa}\delta^{bc}Y_u^{*rd}Y_u^{pt} + \frac{20}{9}\delta^{pr}\delta^{sa}\delta^{td}(Y_u^\dagger Y_u)^{bc} + 8\delta^{sa}\delta^{td}Y_u^{*rb}Y_u^{pc} + \frac{28}{3}\delta^{sa}\delta^{tb}Y_u^{*rd}Y_u^{pc} \Big) + g_Y^2 \left( \frac{157}{36}\delta^{sa}\delta^{tb}Y_u^{*rd}Y_u^{pc} - \frac{32}{27}\delta^{st}\delta^{ad}Y_u^{*rb}Y_u^{pc} \right. \\
& - \frac{34}{27}\delta^{pr}\delta^{sa}\delta^{td}(Y_u^\dagger Y_u)^{bc} - 2\delta^{pr}\delta^{sa}\delta^{tb}(Y_u^\dagger Y_u)^{dc} \Big) + 3T_2\delta^{sa}\delta^{tb}Y_u^{*rd}Y_u^{pc} + 3\delta^{sa}\delta^{td}(Y_u^\dagger Y_u)^{bc}(Y_d Y_d^\dagger)^{pr} + 3\delta^{sa}\delta^{tb}(Y_u^\dagger Y_u)^{dc}(Y_d Y_d^\dagger)^{pr} \\
& + 3\delta^{sa}\delta^{tb}Y_u^{pc}(Y_u^\dagger Y_u Y_u^\dagger)^{rd} + 3\delta^{sa}\delta^{tb}Y_u^{*rd}(Y_u Y_u^\dagger Y_u)^{pc} - g_s^4 \left( \frac{4}{27}\delta^{pr}\delta^{st}\delta^{ad}\delta^{bc} + \frac{2276}{243}\delta^{pr}\delta^{sa}\delta^{td}\delta^{bc} + \frac{130}{9}\delta^{pr}\delta^{sa}\delta^{tb}\delta^{cd} \right) - \delta^{sa}\delta^{tb}Y_u^{pc}(Y_d^\dagger Y_d Y_u^\dagger)^{rd} \\
& - \delta^{sa}\delta^{tb}Y_u^{*rd}(Y_d Y_d^\dagger Y_u)^{pc} - \frac{3}{2}\delta^{td}Y_u^{*rb}Y_u^{pa}(Y_u^\dagger Y_u)^{sc} - \frac{3}{2}\delta^{sc}Y_u^{*rb}Y_u^{pa}(Y_u^\dagger Y_u)^{dt} - 3\delta^{sa}\delta^{td}(Y_u^\dagger Y_u)^{bc}(Y_u Y_u^\dagger)^{pr} - 3\delta^{sa}\delta^{tb}(Y_u^\dagger Y_u)^{dc}(Y_u Y_u^\dagger)^{pr} \\
& - \frac{33}{4}\delta^{sa}\delta^{tb}g_L^2Y_u^{*rd}Y_u^{pc} \Big\} C_{uu}^{abcd} + \left\{ \frac{32}{243}\delta^{pr}\delta^{st}\delta^{ad}\delta^{bc}g_Y^4 + \frac{4}{9}\delta^{st}\delta^{ad}g_s^2Y_d^{*rb}Y_d^{pc} + \frac{16}{27}\delta^{st}\delta^{ad}g_Y^2Y_d^{*rb}Y_d^{pc} - \frac{8}{27}\delta^{pr}\delta^{st}\delta^{ad}\delta^{bc}g_s^4 \right\} C_{dd}^{abcd} \\
& + \left\{ \frac{1}{2}\delta^{sc}\delta^{td}(Y_e^\dagger Y_e)^{ba}(Y_u Y_u^\dagger)^{pr} + \frac{5}{9}\delta^{pr}\delta^{sc}\delta^{td}g_Y^2(Y_e^\dagger Y_e)^{ba} - \frac{37}{243}\delta^{pr}\delta^{sc}\delta^{td}\delta^{ab}g_Y^2g_s^2 - \frac{1}{2}\delta^{sc}\delta^{td}(Y_e^\dagger Y_e)^{ba}(Y_d Y_d^\dagger)^{pr} - \frac{763}{729}\delta^{pr}\delta^{sc}\delta^{td}\delta^{ab}g_Y^4 \right\} C_{eu}^{abcd} \\
& + \left\{ g_Y^2 \left( \frac{1}{3}\delta^{pr}\delta^{sa}\delta^{tb}(Y_d^\dagger Y_d)^{dc} - \frac{383}{72}\delta^{sa}\delta^{tb}Y_d^{*rd}Y_d^{pc} \right) + \frac{3}{2}T_2\delta^{sa}\delta^{tb}Y_d^{*rd}Y_d^{pc} + \frac{3}{2}\delta^{sa}\delta^{tb}(Y_d^\dagger Y_d)^{dc}(Y_u Y_u^\dagger)^{pr} + \frac{3}{2}\delta^{sa}\delta^{tb}Y_d^{pc}(Y_d^\dagger Y_d Y_d^\dagger)^{rd} \right.
\end{aligned}$$

$$\begin{aligned}
& + \frac{3}{2} \delta^{sa} \delta^{tb} Y_d^{*rd} (Y_d Y_d^\dagger Y_d)^{pc} + \frac{14}{3} \delta^{sa} \delta^{tb} g_s^2 Y_d^{*rd} Y_d^{pc} - \frac{97}{729} \delta^{pr} \delta^{sa} \delta^{tb} \delta^{cd} g_Y^4 - \frac{1}{2} \delta^{sa} \delta^{tb} Y_d^{pc} (Y_u^\dagger Y_u Y_d^\dagger)^{rd} - \frac{1}{2} \delta^{sa} \delta^{tb} Y_d^{*rd} (Y_u Y_u^\dagger Y_d)^{pc} \\
& - \frac{253}{243} \delta^{pr} \delta^{sa} \delta^{tb} \delta^{cd} g_Y^2 g_s^2 - \frac{5}{4} \delta^{tb} Y_d^{*rd} Y_d^{pc} (Y_u^\dagger Y_u)^{sa} - \frac{5}{4} \delta^{sa} Y_d^{*rd} Y_d^{pc} (Y_u^\dagger Y_u)^{bt} - \frac{3}{2} \delta^{sa} \delta^{tb} (Y_d^\dagger Y_d)^{dc} (Y_d Y_d^\dagger)^{pr} - \frac{33}{8} \delta^{sa} \delta^{tb} g_L^2 Y_d^{*rd} Y_d^{pc} \\
& - \frac{71}{9} \delta^{pr} \delta^{sa} \delta^{tb} \delta^{cd} g_s^4 \left\{ C_{ud}^{(\parallel)abcd} + \left\{ \frac{1}{9} \delta^{pr} \delta^{sa} \delta^{tb} g_Y^2 (Y_d^\dagger Y_d)^{dc} + \frac{1}{4} \delta^{sa} Y_u^{*rb} Y_d^{pc} (Y_d^\dagger Y_u)^{dt} + \frac{1}{4} \delta^{tb} Y_d^{*rd} Y_u^{pa} (Y_u^\dagger Y_d)^{sc} + \frac{1}{2} \delta^{sa} \delta^{tb} (Y_d^\dagger Y_d)^{dc} (Y_u Y_u^\dagger)^{pr} \right. \right. \\
& + g_s^4 \left( \frac{2}{27} \delta^{pr} \delta^{st} \delta^{ab} \delta^{cd} - \frac{448}{243} \delta^{pr} \delta^{sa} \delta^{tb} \delta^{cd} \right) + g_s^2 \left( \frac{2}{3} \delta^{sa} \delta^{cd} Y_u^{*rb} Y_u^{pt} + \frac{2}{3} \delta^{tb} \delta^{cd} Y_u^{*rs} Y_u^{pa} + \frac{2}{3} \delta^{pr} \delta^{sa} \delta^{tb} (Y_d^\dagger Y_d)^{dc} + 4 \delta^{sa} \delta^{tb} Y_d^{*rd} Y_d^{pc} \right) \\
& \left. - \frac{97}{2187} \delta^{pr} \delta^{sa} \delta^{tb} \delta^{cd} g_Y^4 - \frac{1}{2} \delta^{sa} \delta^{tb} (Y_d^\dagger Y_d)^{dc} (Y_d Y_d^\dagger)^{pr} - g_Y^2 g_s^2 \left( \frac{4}{81} \delta^{pr} \delta^{st} \delta^{ab} \delta^{cd} + \frac{1067}{729} \delta^{pr} \delta^{sa} \delta^{tb} \delta^{cd} \right) \right\} C_{ud}^{(\times)abcd} - \left\{ \frac{2}{27} \delta^{rd} \delta^{st} g_s^2 Y_e^{*ab} Y_d^{pc} \right. \\
& + \frac{14}{81} \delta^{rd} \delta^{st} g_Y^2 Y_e^{*ab} Y_d^{pc} + \frac{1}{4} \delta^{rd} Y_e^{*ab} Y_d^{pc} (Y_u^\dagger Y_u)^{st} \left\} C_{ledq}^{abcd} - C_{ledq}^{*abcd} \left\{ \frac{2}{27} \delta^{pd} \delta^{st} g_s^2 Y_d^{*rc} Y_e^{ab} + \frac{14}{81} \delta^{pd} \delta^{st} g_Y^2 Y_d^{*rc} Y_e^{ab} + \frac{1}{4} \delta^{pd} Y_d^{*rc} Y_e^{ab} (Y_u^\dagger Y_u)^{st} \right\} \\
& + \left\{ \frac{1}{8} \delta^{pa} Y_u^{*rb} Y_u^{*cs} (Y_d^\dagger Y_u)^{dt} + \frac{3}{4} \delta^{tb} Y_d^{*rd} Y_u^{*as} (Y_u Y_u^\dagger)^{pc} + g_s^2 \left( \frac{1}{54} \delta^{pa} \delta^{st} Y_d^{*rd} Y_u^{*cb} + \frac{1}{54} \delta^{pc} \delta^{st} Y_d^{*ad} Y_u^{*rb} + 2 \delta^{pa} \delta^{tb} Y_d^{*rd} Y_u^{*cs} - \frac{2}{27} \delta^{pr} \delta^{tb} Y_d^{*ad} Y_u^{*cs} \right. \right. \\
& - \frac{2}{9} \delta^{pa} \delta^{st} Y_d^{*cd} Y_u^{*rb} - \frac{2}{9} \delta^{pc} \delta^{st} Y_d^{*rd} Y_u^{*ab} - \frac{4}{9} \delta^{pr} \delta^{tb} Y_d^{*cd} Y_u^{*as} - \frac{97}{12} \delta^{pc} \delta^{tb} Y_d^{*rd} Y_u^{*as} - 9 \delta^{pa} \delta^{tb} Y_d^{*cd} Y_u^{*rs} \left. \right) + g_Y^2 \left( \frac{7}{324} \delta^{pr} \delta^{tb} Y_d^{*ad} Y_u^{*cs} \right. \\
& + \frac{7}{162} \delta^{pc} \delta^{st} Y_d^{*ad} Y_u^{*rb} + \frac{47}{144} \delta^{pc} \delta^{tb} Y_d^{*rd} Y_u^{*as} + \frac{22}{27} \delta^{pa} \delta^{st} Y_d^{*cd} Y_u^{*rb} - \frac{1}{27} \delta^{pr} \delta^{tb} Y_d^{*cd} Y_u^{*as} - \frac{11}{162} \delta^{pa} \delta^{st} Y_d^{*rd} Y_u^{*cb} - \frac{14}{27} \delta^{pc} \delta^{st} Y_d^{*rd} Y_u^{*ab} \left. \right) \\
& - \frac{1}{8} \delta^{pa} Y_d^{*rd} Y_u^{*cb} (Y_u^\dagger Y_u)^{st} - \frac{1}{8} \delta^{pc} Y_d^{*ad} Y_u^{*rb} (Y_u^\dagger Y_u)^{st} - \frac{1}{8} \delta^{tb} Y_d^{*ad} Y_u^{*cs} (Y_d Y_d^\dagger)^{pr} - \frac{1}{8} \delta^{tb} Y_d^{*ad} Y_u^{*cs} (Y_u Y_u^\dagger)^{pr} - \frac{1}{8} \delta^{pc} \delta^{tb} Y_d^{*rd} (Y_u^\dagger Y_u Y_u^\dagger)^{as} \\
& - \frac{1}{4} T_2 \delta^{pc} \delta^{tb} Y_d^{*rd} Y_u^{*as} - \frac{1}{4} \delta^{pc} \delta^{tb} Y_u^{*as} (Y_d^\dagger Y_d Y_d^\dagger)^{rd} - \frac{1}{4} \delta^{pc} \delta^{tb} Y_u^{*as} (Y_u^\dagger Y_u Y_d^\dagger)^{rd} - \frac{3}{8} \delta^{pc} \delta^{tb} Y_d^{*rd} (Y_d^\dagger Y_d Y_u^\dagger)^{as} - \frac{5}{8} \delta^{pc} Y_d^{*rd} Y_u^{*as} (Y_u^\dagger Y_u)^{bt} \\
& - \frac{3}{4} \delta^{pa} Y_d^{*cd} Y_u^{*rb} (Y_u^\dagger Y_u)^{st} - \frac{3}{4} \delta^{pc} Y_d^{*rd} Y_u^{*ab} (Y_u^\dagger Y_u)^{st} - \frac{3}{4} \delta^{tb} Y_d^{*cd} Y_u^{*as} (Y_d Y_d^\dagger)^{pr} - \frac{3}{4} \delta^{tb} Y_d^{*cd} Y_u^{*as} (Y_u Y_u^\dagger)^{pr} - \frac{15}{16} \delta^{pc} \delta^{tb} g_L^2 Y_d^{*rd} Y_u^{*as} \\
& - \frac{5}{4} \delta^{tb} Y_d^{*rd} Y_u^{*as} (Y_d Y_d^\dagger)^{pc} \left\} C_{quqd}^{(\parallel)abcd} + \left( C_{quqd}^{(\parallel)*} \right)^{abcd} \left\{ \frac{1}{8} \delta^{ra} Y_u^{pb} Y_u^{ct} (Y_u^\dagger Y_d)^{sd} + \frac{3}{4} \delta^{sb} Y_d^{pd} Y_u^{at} (Y_u Y_u^\dagger)^{cr} + g_s^2 \left( \frac{1}{54} \delta^{ra} \delta^{st} Y_d^{pd} Y_u^{cb} + \frac{1}{54} \delta^{rc} \delta^{st} Y_d^{ad} Y_u^{pb} \right. \right. \\
& + 2 \delta^{ra} \delta^{sb} Y_d^{pd} Y_u^{ct} - \frac{2}{27} \delta^{pr} \delta^{sb} Y_d^{ad} Y_u^{ct} - \frac{2}{9} \delta^{ra} \delta^{st} Y_d^{cd} Y_u^{pb} - \frac{2}{9} \delta^{rc} \delta^{st} Y_d^{pd} Y_u^{ab} - \frac{4}{9} \delta^{pr} \delta^{sb} Y_d^{cd} Y_u^{at} - \frac{97}{12} \delta^{rc} \delta^{sb} Y_d^{pd} Y_u^{at} - 9 \delta^{ra} \delta^{sb} Y_d^{cd} Y_u^{pt} \left. \right) \\
& + g_Y^2 \left( \frac{7}{324} \delta^{pr} \delta^{sb} Y_d^{ad} Y_u^{ct} + \frac{7}{162} \delta^{rc} \delta^{st} Y_d^{ad} Y_u^{pb} + \frac{47}{144} \delta^{rc} \delta^{sb} Y_d^{pd} Y_u^{at} + \frac{22}{27} \delta^{ra} \delta^{st} Y_d^{cd} Y_u^{pb} - \frac{1}{27} \delta^{pr} \delta^{sb} Y_d^{cd} Y_u^{at} - \frac{11}{162} \delta^{ra} \delta^{st} Y_d^{pd} Y_u^{cb} - \frac{14}{27} \delta^{rc} \delta^{st} Y_d^{pd} Y_u^{ab} \right) \\
& - \frac{1}{8} \delta^{ra} Y_d^{pd} Y_u^{cb} (Y_u^\dagger Y_u)^{st} - \frac{1}{8} \delta^{rc} Y_d^{ad} Y_u^{pb} (Y_u^\dagger Y_u)^{st} - \frac{1}{8} \delta^{sb} Y_d^{ad} Y_u^{ct} (Y_d Y_d^\dagger)^{pr} - \frac{1}{8} \delta^{sb} Y_d^{ad} Y_u^{ct} (Y_u Y_u^\dagger)^{pr} - \frac{1}{8} \delta^{rc} \delta^{sb} Y_d^{pd} (Y_u Y_u^\dagger Y_u)^{at} - \frac{1}{4} T_2 \delta^{rc} \delta^{sb} Y_d^{pd} Y_u^{at} \\
& - \frac{1}{4} \delta^{rc} \delta^{sb} Y_u^{at} (Y_d Y_d^\dagger Y_d)^{pd} - \frac{1}{4} \delta^{rc} \delta^{sb} Y_u^{at} (Y_u Y_u^\dagger Y_d)^{pd} - \frac{3}{8} \delta^{rc} \delta^{sb} Y_d^{pd} (Y_d Y_d^\dagger Y_u)^{at} - \frac{5}{8} \delta^{rc} Y_d^{pd} Y_u^{at} (Y_u^\dagger Y_u)^{sb} - \frac{3}{4} \delta^{ra} Y_d^{cd} Y_u^{pb} (Y_u^\dagger Y_u)^{st} - \frac{3}{4} \delta^{rc} Y_d^{pd} Y_u^{ab} (Y_u^\dagger Y_u)^{st}
\end{aligned}$$

$$\begin{aligned}
& -\frac{3}{4}\delta^{sb}Y_d^{cd}Y_u^{at}(Y_dY_d^\dagger)^{pr} - \frac{3}{4}\delta^{sb}Y_d^{cd}Y_u^{at}(Y_uY_u^\dagger)^{pr} - \frac{15}{16}\delta^{rc}\delta^{sb}g_L^2Y_d^{pd}Y_u^{at} - \frac{5}{4}\delta^{sb}Y_d^{pd}Y_u^{at}(Y_dY_d^\dagger)^{cr} \Bigg\} + \Bigg\{ \frac{1}{2}\delta^{pc}Y_u^{*rb}Y_u^{*as}(Y_d^\dagger Y_u)^{dt} + \frac{5}{8}\delta^{tb}Y_d^{*rd}Y_u^{*cs}(Y_uY_u^\dagger)^{pa} \\
& + g_Y^2 \Big( \frac{7}{108}\delta^{pr}\delta^{tb}Y_d^{*ad}Y_u^{*cs} + \frac{13}{54}\delta^{pc}\delta^{st}Y_d^{*ad}Y_u^{*rb} + \frac{25}{81}\delta^{pa}\delta^{st}Y_d^{*cd}Y_u^{*rb} + \frac{17}{12}\delta^{pa}\delta^{tb}Y_d^{*rd}Y_u^{*cs} - \frac{1}{81}\delta^{pr}\delta^{tb}Y_d^{*cd}Y_u^{*as} - \frac{5}{54}\delta^{pa}\delta^{st}Y_d^{*rd}Y_u^{*cb} \\
& - \frac{11}{81}\delta^{pc}\delta^{st}Y_d^{*rd}Y_u^{*ab} \Big) + g_s^2 \Big( \frac{9}{4}\delta^{pc}\delta^{tb}Y_d^{*rd}Y_u^{*as} - \frac{1}{9}\delta^{pa}\delta^{st}Y_d^{*rd}Y_u^{*cb} - \frac{1}{9}\delta^{pc}\delta^{st}Y_d^{*ad}Y_u^{*rb} - \frac{7}{54}\delta^{pa}\delta^{st}Y_d^{*cd}Y_u^{*rb} - \frac{7}{54}\delta^{pc}\delta^{st}Y_d^{*rd}Y_u^{*ab} \\
& - \frac{4}{27}\delta^{pr}\delta^{tb}Y_d^{*cd}Y_u^{*as} - \frac{2}{9}\delta^{pr}\delta^{tb}Y_d^{*ad}Y_u^{*cs} - 3\delta^{pa}\delta^{tb}Y_d^{*cd}Y_u^{*rs} - \frac{9}{2}\delta^{pc}\delta^{tb}Y_d^{*ad}Y_u^{*rs} - 5\delta^{pa}\delta^{tb}Y_d^{*rd}Y_u^{*cs} \Big) + \frac{9}{4}\delta^{pa}\delta^{tb}g_L^2Y_d^{*rd}Y_u^{*cs} \\
& - \frac{1}{8}\delta^{pa}Y_d^{*rd}Y_u^{*cs}(Y_u^\dagger Y_u)^{bt} - \frac{1}{4}\delta^{pa}Y_d^{*cd}Y_u^{*rb}(Y_u^\dagger Y_u)^{st} - \frac{1}{4}\delta^{pc}Y_d^{*rd}Y_u^{*ab}(Y_u^\dagger Y_u)^{st} - \frac{1}{4}\delta^{tb}Y_d^{*cd}Y_u^{*as}(Y_dY_d^\dagger)^{pr} - \frac{1}{4}\delta^{tb}Y_d^{*rd}Y_u^{*cs}(Y_dY_d^\dagger)^{pa} \\
& - \frac{1}{4}\delta^{tb}Y_d^{*cd}Y_u^{*as}(Y_uY_u^\dagger)^{pr} - \frac{3}{8}\delta^{pa}Y_d^{*rd}Y_u^{*cb}(Y_u^\dagger Y_u)^{st} - \frac{3}{8}\delta^{pc}Y_d^{*ad}Y_u^{*rb}(Y_u^\dagger Y_u)^{st} - \frac{3}{8}\delta^{tb}Y_d^{*ad}Y_u^{*cs}(Y_dY_d^\dagger)^{pr} - \frac{3}{8}\delta^{tb}Y_d^{*ad}Y_u^{*cs}(Y_uY_u^\dagger)^{pr} \\
& - \frac{1}{2}\delta^{pa}\delta^{tb}Y_d^{*rd}(Y_d^\dagger Y_d Y_u^\dagger)^{cs} - \frac{1}{2}\delta^{pa}\delta^{tb}Y_d^{*rd}(Y_u^\dagger Y_u Y_u^\dagger)^{cs} - T_2\delta^{pa}\delta^{tb}Y_d^{*rd}Y_u^{*cs} - \delta^{pa}\delta^{tb}Y_u^{*cs}(Y_d^\dagger Y_d Y_d^\dagger)^{rd} \Bigg\} C_{quqd}^{(\times)abcd} \\
& + \Big( C_{quqd}^{(\times)*} \Big)^{abcd} \Bigg\{ \frac{1}{2}\delta^{rc}Y_u^{pb}Y_u^{at}(Y_u^\dagger Y_d)^{sd} + \frac{5}{8}\delta^{sb}Y_d^{pd}Y_u^{ct}(Y_uY_u^\dagger)^{ar} + g_Y^2 \Big( \frac{7}{108}\delta^{pr}\delta^{sb}Y_d^{ad}Y_u^{ct} + \frac{13}{54}\delta^{rc}\delta^{st}Y_d^{ad}Y_u^{pb} + \frac{25}{81}\delta^{ra}\delta^{st}Y_d^{cd}Y_u^{pb} + \frac{17}{12}\delta^{ra}\delta^{sb}Y_d^{pd}Y_u^{ct} \\
& - \frac{1}{81}\delta^{pr}\delta^{sb}Y_d^{cd}Y_u^{at} - \frac{5}{54}\delta^{ra}\delta^{st}Y_d^{pd}Y_u^{cb} - \frac{11}{81}\delta^{rc}\delta^{st}Y_d^{pd}Y_u^{ab} \Big) + g_s^2 \Big( \frac{9}{4}\delta^{rc}\delta^{sb}Y_d^{pd}Y_u^{at} - \frac{1}{9}\delta^{ra}\delta^{st}Y_d^{pd}Y_u^{cb} - \frac{1}{9}\delta^{rc}\delta^{st}Y_d^{ad}Y_u^{pb} - \frac{7}{54}\delta^{ra}\delta^{st}Y_d^{cd}Y_u^{pb} \\
& - \frac{7}{54}\delta^{rc}\delta^{st}Y_d^{pd}Y_u^{ab} - \frac{4}{27}\delta^{pr}\delta^{sb}Y_d^{cd}Y_u^{at} - \frac{2}{9}\delta^{pr}\delta^{sb}Y_d^{ad}Y_u^{ct} - 3\delta^{ra}\delta^{sb}Y_d^{cd}Y_u^{pt} - \frac{9}{2}\delta^{rc}\delta^{sb}Y_d^{ad}Y_u^{pt} - 5\delta^{ra}\delta^{sb}Y_d^{pd}Y_u^{ct} \Big) + \frac{9}{4}\delta^{ra}\delta^{sb}g_L^2Y_d^{pd}Y_u^{ct} \\
& - \frac{1}{8}\delta^{ra}Y_d^{pd}Y_u^{ct}(Y_u^\dagger Y_u)^{sb} - \frac{1}{4}\delta^{ra}Y_d^{cd}Y_u^{pb}(Y_u^\dagger Y_u)^{st} - \frac{1}{4}\delta^{rc}Y_d^{pd}Y_u^{ab}(Y_u^\dagger Y_u)^{st} - \frac{1}{4}\delta^{sb}Y_d^{cd}Y_u^{at}(Y_dY_d^\dagger)^{pr} - \frac{1}{4}\delta^{sb}Y_d^{pd}Y_u^{ct}(Y_dY_d^\dagger)^{ar} - \frac{1}{4}\delta^{sb}Y_d^{cd}Y_u^{at}(Y_uY_u^\dagger)^{pr} \\
& - \frac{3}{8}\delta^{ra}Y_d^{pd}Y_u^{cb}(Y_u^\dagger Y_u)^{st} - \frac{3}{8}\delta^{rc}Y_d^{ad}Y_u^{pb}(Y_u^\dagger Y_u)^{st} - \frac{3}{8}\delta^{sb}Y_d^{ad}Y_u^{ct}(Y_dY_d^\dagger)^{pr} - \frac{3}{8}\delta^{sb}Y_d^{ad}Y_u^{ct}(Y_uY_u^\dagger)^{pr} - \frac{1}{2}\delta^{ra}\delta^{sb}Y_d^{pd}(Y_dY_d^\dagger Y_u)^{ct} - \frac{1}{2}\delta^{ra}\delta^{sb}Y_d^{pd}(Y_uY_u^\dagger Y_u)^{ct} \\
& - T_2\delta^{ra}\delta^{sb}Y_d^{pd}Y_u^{ct} - \delta^{ra}\delta^{sb}Y_u^{ct}(Y_dY_d^\dagger Y_d)^{pd} \Bigg\} + \Bigg\{ \frac{1}{4}\delta^{pc}Y_e^{*ab}Y_u^{*rd}(Y_u^\dagger Y_u)^{st} + \frac{1}{4}\delta^{td}Y_e^{*ab}Y_u^{*cs}(Y_dY_d^\dagger)^{pr} + \frac{1}{4}\delta^{td}Y_e^{*ab}Y_u^{*cs}(Y_uY_u^\dagger)^{pr} \\
& + g_Y^2 \Big( \frac{1}{81}\delta^{pr}\delta^{td}Y_e^{*ab}Y_u^{*cs} - \frac{22}{81}\delta^{pc}\delta^{st}Y_e^{*ab}Y_u^{*rd} \Big) + g_s^2 \Big( \frac{2}{27}\delta^{pc}\delta^{st}Y_e^{*ab}Y_u^{*rd} + \frac{4}{27}\delta^{pr}\delta^{td}Y_e^{*ab}Y_u^{*cs} + 3\delta^{pc}\delta^{td}Y_e^{*ab}Y_u^{*rs} \Big) \Bigg\} C_{lequ}^{abcd} \\
& + C_{lequ}^{*abcd} \Bigg\{ \frac{1}{4}\delta^{rc}Y_e^{ab}Y_u^{pd}(Y_u^\dagger Y_u)^{st} + \frac{1}{4}\delta^{sd}Y_e^{ab}Y_u^{ct}(Y_dY_d^\dagger)^{pr} + \frac{1}{4}\delta^{sd}Y_e^{ab}Y_u^{ct}(Y_uY_u^\dagger)^{pr} + g_Y^2 \Big( \frac{1}{81}\delta^{pr}\delta^{sd}Y_e^{ab}Y_u^{ct} - \frac{22}{81}\delta^{rc}\delta^{st}Y_e^{ab}Y_u^{pd} \Big) + g_s^2 \Big( \frac{2}{27}\delta^{rc}\delta^{st}Y_e^{ab}Y_u^{pd} \\
& + \frac{4}{27}\delta^{pr}\delta^{sd}Y_e^{ab}Y_u^{ct} + 3\delta^{rc}\delta^{sd}Y_e^{ab}Y_u^{pt} \Big) \Bigg\} + \Bigg\{ g_Y^2 \Big( \frac{7}{324}\delta^{pr}\delta^{tb}Y_e^{*ad}Y_u^{*cs} + \frac{13}{162}\delta^{pc}\delta^{st}Y_e^{*ad}Y_u^{*rb} \Big) - \frac{1}{8}\delta^{pc}Y_e^{*ad}Y_u^{*rb}(Y_u^\dagger Y_u)^{st} - \frac{1}{8}\delta^{tb}Y_e^{*ad}Y_u^{*cs}(Y_dY_d^\dagger)^{pr}
\end{aligned}$$

$$\begin{aligned}
& -\frac{1}{8}\delta^{tb}Y_e^{*ad}Y_u^{*cs}(Y_uY_u^\dagger)^{pr} - g_s^2\left(\frac{1}{27}\delta^{pc}\delta^{st}Y_e^{*ad}Y_u^{*rb} + \frac{2}{27}\delta^{pr}\delta^{tb}Y_e^{*ad}Y_u^{*cs} + \frac{3}{2}\delta^{pc}\delta^{tb}Y_e^{*ad}Y_u^{*rs}\right)\left\{C_{\ell uqe}^{abcd} + C_{\ell uqe}^{*abcd}\right\}g_Y^2\left(\frac{7}{324}\delta^{pr}\delta^{sb}Y_e^{ad}Y_u^{ct}\right. \\
& + \frac{13}{162}\delta^{rc}\delta^{st}Y_e^{ad}Y_u^{pb}) - \frac{1}{8}\delta^{rc}Y_e^{ad}Y_u^{pb}(Y_u^\dagger Y_u)^{st} - \frac{1}{8}\delta^{sb}Y_e^{ad}Y_u^{ct}(Y_dY_d^\dagger)^{pr} - \frac{1}{8}\delta^{sb}Y_e^{ad}Y_u^{ct}(Y_uY_u^\dagger)^{pr} - g_s^2\left(\frac{1}{27}\delta^{rc}\delta^{st}Y_e^{ad}Y_u^{pb} + \frac{2}{27}\delta^{pr}\delta^{sb}Y_e^{ad}Y_u^{ct}\right. \\
& + \left.\frac{3}{2}\delta^{rc}\delta^{sb}Y_e^{ad}Y_u^{pt}\right)\left\} + \frac{16}{81}\delta^{pr}\delta^{st}\delta^{ad}\delta^{bc}g_Y^4C_{\ell\ell}^{abcd} + \left\{g_Y^4\left(\frac{16}{243}\delta^{pr}\delta^{st}\delta^{ad}\delta^{bc} + \frac{224}{729}\delta^{pa}\delta^{rb}\delta^{st}\delta^{cd} - \frac{404}{2187}\delta^{pa}\delta^{rd}\delta^{st}\delta^{bc}\right) + g_Y^2g_s^2\left(\frac{434}{729}\delta^{pa}\delta^{rd}\delta^{st}\delta^{bc}\right.\right. \\
& + \frac{572}{243}\delta^{pa}\delta^{rb}\delta^{st}\delta^{cd} - \frac{16}{81}\delta^{pr}\delta^{st}\delta^{ad}\delta^{bc}) + g_Y^2g_L^2\left(4\delta^{pa}\delta^{rb}\delta^{st}\delta^{cd} - \frac{116}{81}\delta^{pa}\delta^{rd}\delta^{st}\delta^{bc}\right) + g_s^2\left(\frac{8}{9}\delta^{pr}\delta^{bc}Y_u^{*as}Y_u^{dt} + \frac{10}{9}\delta^{pa}\delta^{rd}\delta^{st}(Y_dY_d^\dagger)^{bc}\right. \\
& + \frac{10}{9}\delta^{pa}\delta^{rd}\delta^{st}(Y_uY_u^\dagger)^{bc} + \frac{4}{3}\delta^{pa}\delta^{bc}Y_u^{*rs}Y_u^{dt} + \frac{4}{3}\delta^{rd}\delta^{bc}Y_u^{*as}Y_u^{pt} + 8\delta^{pa}\delta^{rd}Y_u^{*cs}Y_u^{bt} + \frac{56}{3}\delta^{pa}\delta^{rb}Y_u^{*cs}Y_u^{dt}) + \delta^{pa}\delta^{rb}Y_u^{dt}(Y_d^\dagger Y_dY_u^\dagger)^{cs} \\
& + \delta^{pa}\delta^{rb}Y_u^{*cs}(Y_dY_d^\dagger Y_u)^{dt} + \frac{58}{27}\delta^{pa}\delta^{rd}\delta^{st}\delta^{bc}g_s^2g_L^2 + 3\delta^{pa}\delta^{rd}(Y_u^\dagger Y_u)^{st}(Y_dY_d^\dagger)^{bc} + 3\delta^{pa}\delta^{rb}Y_u^{dt}(Y_u^\dagger Y_uY_u^\dagger)^{cs} + 3\delta^{pa}\delta^{rb}Y_u^{*cs}(Y_uY_u^\dagger Y_u)^{dt} \\
& + 6T_2\delta^{pa}\delta^{rb}Y_u^{*cs}Y_u^{dt} + 6\delta^{pa}\delta^{rb}(Y_u^\dagger Y_u)^{st}(Y_dY_d^\dagger)^{dc} - g_s^4\left(\frac{8}{27}\delta^{pr}\delta^{st}\delta^{ad}\delta^{bc} + \frac{2168}{243}\delta^{pa}\delta^{rd}\delta^{st}\delta^{bc} + \frac{260}{9}\delta^{pa}\delta^{rb}\delta^{st}\delta^{cd}\right) - g_Y^2\left(\frac{4}{27}\delta^{pr}\delta^{bc}Y_u^{*as}Y_u^{dt}\right. \\
& + \frac{8}{27}\delta^{pa}\delta^{rd}\delta^{st}(Y_dY_d^\dagger)^{bc} + \frac{32}{27}\delta^{pa}\delta^{rd}\delta^{st}(Y_uY_u^\dagger)^{bc} + \frac{83}{18}\delta^{pa}\delta^{rb}Y_u^{*cs}Y_u^{dt} + \frac{16}{3}\delta^{pa}\delta^{rb}\delta^{st}(Y_uY_u^\dagger)^{dc}) - \frac{3}{2}\delta^{rd}Y_u^{*as}Y_u^{bt}(Y_uY_u^\dagger)^{pc} - \frac{3}{2}\delta^{pa}Y_u^{*cs}Y_u^{dt}(Y_uY_u^\dagger)^{br} \\
& - \frac{5}{2}\delta^{rb}Y_u^{*cs}Y_u^{dt}(Y_dY_d^\dagger)^{pa} - \frac{5}{2}\delta^{pa}Y_u^{*cs}Y_u^{dt}(Y_dY_d^\dagger)^{br} - 3\delta^{pa}\delta^{rd}(Y_u^\dagger Y_u)^{st}(Y_uY_u^\dagger)^{bc} - 6\delta^{pa}\delta^{rb}(Y_u^\dagger Y_u)^{st}(Y_uY_u^\dagger)^{dc} - \frac{51}{2}\delta^{pa}\delta^{rb}g_L^2Y_u^{*cs}Y_u^{dt}\left\}C_{qq}^{(\parallel)abcd} \right. \\
& + \left\{\frac{1}{2}\delta^{pa}\delta^{rb}Y_u^{dt}(Y_d^\dagger Y_dY_u^\dagger)^{cs} + \frac{1}{2}\delta^{pa}\delta^{rb}Y_u^{*cs}(Y_dY_d^\dagger Y_u)^{dt} + g_Y^2g_L^2\left(\frac{4}{3}\delta^{pa}\delta^{rd}\delta^{st}\delta^{bc} - \frac{32}{27}\delta^{pa}\delta^{rb}\delta^{st}\delta^{cd}\right) + g_Y^4\left(\frac{32}{243}\delta^{pr}\delta^{st}\delta^{ad}\delta^{bc} + \frac{112}{729}\delta^{pa}\delta^{rb}\delta^{st}\delta^{cd}\right.\right. \\
& - \frac{808}{2187}\delta^{pa}\delta^{rd}\delta^{st}\delta^{bc}) + g_Y^2g_s^2\left(\frac{286}{243}\delta^{pa}\delta^{rb}\delta^{st}\delta^{cd} + \frac{868}{729}\delta^{pa}\delta^{rd}\delta^{st}\delta^{bc} - \frac{32}{81}\delta^{pr}\delta^{st}\delta^{ad}\delta^{bc}\right) + g_s^2g_L^2\left(\frac{34}{9}\delta^{pa}\delta^{rb}\delta^{st}\delta^{cd} - 2\delta^{pa}\delta^{rd}\delta^{st}\delta^{bc}\right) \\
& + g_s^2\left(\frac{16}{9}\delta^{pr}\delta^{bc}Y_u^{*as}Y_u^{dt} + \frac{20}{9}\delta^{pa}\delta^{rd}\delta^{st}(Y_dY_d^\dagger)^{bc} + \frac{20}{9}\delta^{pa}\delta^{rd}\delta^{st}(Y_uY_u^\dagger)^{bc} + \frac{8}{3}\delta^{pa}\delta^{bc}Y_u^{*rs}Y_u^{dt} + \frac{8}{3}\delta^{rd}\delta^{bc}Y_u^{*as}Y_u^{pt} + \frac{28}{3}\delta^{pa}\delta^{rb}Y_u^{*cs}Y_u^{dt}\right. \\
& + 16\delta^{pa}\delta^{rd}Y_u^{*cs}Y_u^{bt}) + \frac{3}{2}\delta^{pa}\delta^{rb}Y_u^{dt}(Y_u^\dagger Y_uY_u^\dagger)^{cs} + \frac{3}{2}\delta^{pa}\delta^{rb}Y_u^{*cs}(Y_uY_u^\dagger Y_u)^{dt} + \frac{5}{2}\delta^{rb}Y_u^{*cs}Y_u^{dt}(Y_dY_d^\dagger)^{pa} + \frac{5}{2}\delta^{pa}Y_u^{*cs}Y_u^{dt}(Y_dY_d^\dagger)^{br} \\
& + 3T_2\delta^{pa}\delta^{rb}Y_u^{*cs}Y_u^{dt} + 3\delta^{pa}\delta^{rb}(Y_u^\dagger Y_u)^{st}(Y_dY_d^\dagger)^{dc} + \frac{15}{4}\delta^{pa}\delta^{rb}g_L^2Y_u^{*cs}Y_u^{dt} + 6\delta^{pa}\delta^{rd}(Y_u^\dagger Y_u)^{st}(Y_dY_d^\dagger)^{bc} - g_s^4\left(\frac{16}{27}\delta^{pr}\delta^{st}\delta^{ad}\delta^{bc}\right. \\
& + \frac{130}{9}\delta^{pa}\delta^{rb}\delta^{st}\delta^{cd} + \frac{4336}{243}\delta^{pa}\delta^{rd}\delta^{st}\delta^{bc}) - g_Y^2\left(\frac{8}{27}\delta^{pr}\delta^{bc}Y_u^{*as}Y_u^{dt} + \frac{16}{27}\delta^{pa}\delta^{rd}\delta^{st}(Y_dY_d^\dagger)^{bc} + \frac{83}{36}\delta^{pa}\delta^{rb}Y_u^{*cs}Y_u^{dt} + \frac{64}{27}\delta^{pa}\delta^{rd}\delta^{st}(Y_uY_u^\dagger)^{bc}\right. \\
& + \frac{8}{3}\delta^{pa}\delta^{rb}\delta^{st}(Y_uY_u^\dagger)^{dc}) - 3\delta^{rd}Y_u^{*as}Y_u^{bt}(Y_uY_u^\dagger)^{pc} - 3\delta^{pa}Y_u^{*cs}Y_u^{dt}(Y_uY_u^\dagger)^{br} - 3\delta^{pa}\delta^{rb}(Y_u^\dagger Y_u)^{st}(Y_uY_u^\dagger)^{dc} - 6\delta^{pa}\delta^{rd}(Y_u^\dagger Y_u)^{st}(Y_uY_u^\dagger)^{bc}\left\}C_{qq}^{(\times)abcd} \right. \\
& + \left\{\delta^{pc}\delta^{rd}(Y_u^\dagger Y_u)^{st}(Y_eY_e^\dagger)^{ba} + \frac{362}{243}\delta^{pc}\delta^{rd}\delta^{st}\delta^{ab}g_Y^2g_s^2 + \frac{16}{9}\delta^{pc}\delta^{rd}\delta^{st}g_Y^2(Y_eY_e^\dagger)^{ba} - 2\delta^{pc}\delta^{rd}\delta^{st}\delta^{ab}g_Y^2g_L^2 - \frac{3208}{729}\delta^{pc}\delta^{rd}\delta^{st}\delta^{ab}g_Y^4\right\}C_{\ell q}^{(\parallel)abcd}
\end{aligned}$$

$$\begin{aligned}
& + \left\{ \frac{1}{2} \delta^{pc} \delta^{rd} (Y_u^\dagger Y_u)^{st} (Y_e Y_e^\dagger)^{ba} + \frac{17}{27} \delta^{pc} \delta^{rd} \delta^{st} \delta^{ab} g_s^2 g_L^2 + \frac{181}{243} \delta^{pc} \delta^{rd} \delta^{st} \delta^{ab} g_Y^2 g_s^2 + \frac{8}{9} \delta^{pc} \delta^{rd} \delta^{st} g_Y^2 (Y_e Y_e^\dagger)^{ba} - \frac{88}{81} \delta^{pc} \delta^{rd} \delta^{st} \delta^{ab} g_Y^2 g_L^2 \right. \\
& \left. - \frac{1604}{729} \delta^{pc} \delta^{rd} \delta^{st} \delta^{ab} g_Y^4 \right\} C_{\ell q}^{(\times)abcd}, \tag{10.10}
\end{aligned}$$

## 10.6 $C_{qu}^{(\times)}$

$$\begin{aligned}
\beta_{C_{qu}^{(\times)prst}}^{(1)} = & \left\{ \delta^{pa} \delta^{sc} Y_u^{*rd} Y_u^{bt} + \delta^{rb} \delta^{td} Y_u^{*as} Y_u^{pc} + 2\delta^{rb} \delta^{sc} Y_u^{*ad} Y_u^{pt} + 2\delta^{pa} \delta^{td} Y_u^{*rs} Y_u^{bc} - 6\delta^{pa} \delta^{rb} \delta^{sc} \delta^{td} g_s^2 \right\} C_{qu}^{(\parallel)abcd} + \left\{ \frac{1}{2} \left( \delta^{rb} \delta^{sc} \delta^{td} (Y_d Y_d^\dagger)^{pa} \right. \right. \\
& + \delta^{pa} \delta^{sc} \delta^{td} (Y_d Y_d^\dagger)^{br} + \delta^{rb} \delta^{sc} \delta^{td} (Y_u Y_u^\dagger)^{pa} + \delta^{pa} \delta^{sc} \delta^{td} (Y_u Y_u^\dagger)^{br} + 2\delta^{pa} \delta^{rb} \delta^{td} (Y_u^\dagger Y_u)^{sc} + 2\delta^{pa} \delta^{rb} \delta^{sc} (Y_u^\dagger Y_u)^{dt} + 12\delta^{rb} \delta^{sc} Y_u^{*ad} Y_u^{pt} \\
& + 12\delta^{pa} \delta^{td} Y_u^{*rs} Y_u^{bc} \left. \right) - \frac{2}{3} g_s^2 \left( 24\delta^{pa} \delta^{rb} \delta^{sc} \delta^{td} - \delta^{pa} \delta^{rb} \delta^{st} \delta^{cd} - 2\delta^{pr} \delta^{sc} \delta^{td} \delta^{ab} \right) - \frac{4}{3} \delta^{pa} \delta^{rb} \delta^{sc} \delta^{td} g_Y^2 \left. \right\} C_{qu}^{(\times)abcd} + \frac{2}{3} \delta^{pa} \delta^{rb} \delta^{st} \delta^{cd} g_s^2 C_{qd}^{(\times)abcd} \\
& + \left\{ \frac{4}{3} \delta^{pr} \delta^{sa} \delta^{td} \delta^{bc} g_s^2 - 2\delta^{sa} \delta^{td} Y_u^{*rb} Y_u^{pc} \right\} C_{uu}^{abcd} + \left\{ \frac{2}{3} \delta^{pr} \delta^{sa} \delta^{tb} \delta^{cd} g_s^2 - \delta^{sa} \delta^{tb} Y_d^{*rd} Y_d^{pc} \right\} C_{ud}^{(\times)abcd} + \frac{1}{2} \left\{ 2\delta^{pa} \delta^{tb} Y_d^{*rd} Y_u^{*cs} - \delta^{pc} \delta^{tb} Y_d^{*ad} Y_u^{*rs} \right. \\
& - 6\delta^{pa} \delta^{tb} Y_d^{*cd} Y_u^{*rs} \left. \right\} C_{quqd}^{(\parallel)abcd} + \frac{1}{2} \left( C_{quqd}^{(\parallel)*} \right)^{abcd} \left\{ 2\delta^{ra} \delta^{sb} Y_d^{pd} Y_u^{ct} - \delta^{rc} \delta^{sb} Y_d^{ad} Y_u^{pt} - 6\delta^{ra} \delta^{sb} Y_d^{cd} Y_u^{pt} \right\} + \frac{1}{2} \left\{ \delta^{pc} \delta^{tb} Y_d^{*rd} Y_u^{*as} - 2\delta^{pa} \delta^{tb} Y_d^{*cd} Y_u^{*rs} \right. \\
& - 3\delta^{pc} \delta^{tb} Y_d^{*ad} Y_u^{*rs} \left. \right\} C_{quqd}^{(\times)abcd} + \frac{1}{2} \left( C_{quqd}^{(\times)*} \right)^{abcd} \left\{ \delta^{rc} \delta^{sb} Y_d^{pd} Y_u^{at} - 2\delta^{ra} \delta^{sb} Y_d^{cd} Y_u^{pt} - 3\delta^{rc} \delta^{sb} Y_d^{ad} Y_u^{pt} \right\} + \delta^{pc} \delta^{td} Y_e^{*ab} Y_u^{*rs} C_{\ell equ}^{abcd} + \delta^{rc} \delta^{sd} C_{\ell equ}^{*abcd} Y_e^{ab} Y_u^{pt} \\
& - \frac{1}{2} \delta^{pc} \delta^{tb} Y_e^{*ad} Y_u^{*rs} C_{\ell uqe}^{abcd} - \frac{1}{2} \delta^{rc} \delta^{sb} C_{\ell uqe}^{*abcd} Y_e^{ad} Y_u^{pt} + \left\{ \frac{4}{3} \delta^{pa} \delta^{rd} \delta^{st} \delta^{bc} g_s^2 - 2\delta^{pa} \delta^{rd} Y_u^{*cs} Y_u^{bt} \right\} C_{qq}^{(\parallel)abcd} + \left\{ \frac{8}{3} \delta^{pa} \delta^{rd} \delta^{st} \delta^{bc} g_s^2 \right. \\
& \left. - 4\delta^{pa} \delta^{rd} Y_u^{*cs} Y_u^{bt} \right\} C_{qq}^{(\times)abcd}, \tag{10.11}
\end{aligned}$$

$$\begin{aligned}
\beta_{C_{qu}^{(\times)prst}}^{(2)} = & 2Y_u^{*rs} Y_u^{pt} \mathbf{T}_{\ell H} + \left\{ \frac{1}{4} Y_u^{pt} (Y_d^\dagger Y_d Y_u^\dagger)^{rs} + \frac{1}{4} Y_u^{*rs} (Y_d Y_d^\dagger Y_u)^{pt} + \frac{3}{4} Y_u^{pt} (Y_u^\dagger Y_u Y_u^\dagger)^{rs} + \frac{3}{4} Y_u^{*rs} (Y_u Y_u^\dagger Y_u)^{pt} - \frac{1}{36} g_Y^2 Y_u^{*rs} Y_u^{pt} - \frac{1}{12} g_L^2 Y_u^{*rs} Y_u^{pt} \right. \\
& \left. - \frac{1}{2} \lambda Y_u^{*rs} Y_u^{pt} \right\} C_{HD}^{(\parallel)} + \left\{ \frac{3}{4} Y_u^{pt} (Y_u^\dagger Y_u Y_u^\dagger)^{rs} + \frac{3}{4} Y_u^{*rs} (Y_u Y_u^\dagger Y_u)^{pt} - \frac{1}{18} g_Y^2 Y_u^{*rs} Y_u^{pt} - \frac{1}{4} Y_u^{pt} (Y_d^\dagger Y_d Y_u^\dagger)^{rs} - \frac{1}{4} Y_u^{*rs} (Y_d Y_d^\dagger Y_u)^{pt} - \frac{1}{2} \lambda Y_u^{*rs} Y_u^{pt} \right\} C_{HD}^{(\times)} \\
& + \frac{25}{9} g_Y^4 C_{HB} Y_u^{*rs} Y_u^{pt} + 3g_L^4 C_{HW} Y_u^{*rs} Y_u^{pt} - g_s^4 \left\{ 2\delta^{st} (Y_d Y_d^\dagger)^{pr} + 2\delta^{st} (Y_u Y_u^\dagger)^{pr} + 4\delta^{pr} (Y_u^\dagger Y_u)^{st} + \frac{44}{3} Y_u^{*rs} Y_u^{pt} \right\} C_{HG} - \frac{5}{2} g_Y^2 g_L^2 C_{HWB} Y_u^{*rs} Y_u^{pt}
\end{aligned}$$

$$\begin{aligned}
& + \left\{ 10\delta^{pr}\delta^{st}g_s^2g_L^6 - \frac{21}{2}g_L^6Y_u^{*rs}Y_u^{pt} \right\} C_W + \left\{ g_s^6 \left( 79Y_u^{*rs}Y_u^{pt} - \frac{9}{2}\delta^{st}(Y_dY_d^\dagger)^{pr} - \frac{9}{2}\delta^{st}(Y_uY_u^\dagger)^{pr} - 9\delta^{pr}(Y_u^\dagger Y_u)^{st} \right) - 14\delta^{pr}\delta^{st}g_Y^2g_s^6 - \frac{74}{3}\delta^{pr}\delta^{st}g_s^8 \right\} C_G \\
& + \left\{ 3\delta^{pa}\delta^{tb}(Y_u^\dagger Y_u Y_u^\dagger)^{rs} - \frac{3}{2}\delta^{pa}\delta^{tb}\lambda Y_u^{*rs} \right\} C_{uH}^{ab} + C_{uH}^{*ab} \left\{ 3\delta^{ra}\delta^{sb}(Y_u Y_u^\dagger Y_u)^{pt} - \frac{3}{2}\delta^{ra}\delta^{sb}\lambda Y_u^{pt} \right\} - \frac{3}{2}g_Y^2Y_e^{*ab}Y_u^{*rs}C_{eB}^{ab}Y_u^{pt} \\
& - \frac{3}{2}g_Y^2C_{eB}^{*ab}Y_u^{*rs}Y_e^{ab}Y_u^{pt} + \frac{3}{4}g_L^2Y_e^{*ab}Y_u^{*rs}C_{eW}^{ab}Y_u^{pt} + \frac{3}{4}g_L^2C_{eW}^{*ab}Y_u^{*rs}Y_e^{ab}Y_u^{pt} + \left\{ g_Y^2g_s^2 \left( \frac{2}{9}\delta^{pr}\delta^{tb}Y_u^{*as} + \frac{10}{9}\delta^{pa}\delta^{tb}Y_u^{*rs} + \frac{19}{9}\delta^{pa}\delta^{st}Y_u^{*rb} \right) \right. \\
& + g_Y^2 \left( \frac{5}{6}\delta^{pa}Y_u^{*rs}(Y_u^\dagger Y_u)^{bt} + \frac{5}{3}\delta^{tb}Y_u^{*rs}(Y_u Y_u^\dagger)^{pa} + \frac{5}{2}\delta^{pa}\delta^{tb}Y_u^{*rs}\text{Tr}[Y_e^\dagger Y_e] + \frac{15}{2}\delta^{pa}\delta^{tb}Y_u^{*rs}\text{Tr}[Y_d^\dagger Y_d] - \frac{8}{3}\delta^{pa}\delta^{tb}(Y_d^\dagger Y_d Y_u^\dagger)^{rs} - \frac{17}{6}\delta^{tb}Y_u^{*rs}(Y_d Y_d^\dagger)^{pa} \right. \\
& \left. - 5Y_u^{*rs}Y_u^{*ab}Y_u^{pt} \right) + \frac{4655}{216}\delta^{pa}\delta^{tb}g_Y^4Y_u^{*rs} - \frac{35}{8}\delta^{pa}\delta^{tb}g_Y^2g_L^2Y_u^{*rs} \left\{ C_{uB}^{ab} + C_{uB}^{*ab} \right\} \left\{ g_Y^2g_s^2 \left( \frac{2}{9}\delta^{pr}\delta^{sb}Y_u^{at} + \frac{10}{9}\delta^{ra}\delta^{sb}Y_u^{pt} + \frac{19}{9}\delta^{ra}\delta^{st}Y_u^{pb} \right) \right. \\
& + g_Y^2 \left( \frac{5}{6}\delta^{ra}Y_u^{pt}(Y_u^\dagger Y_u)^{sb} + \frac{5}{3}\delta^{sb}Y_u^{pt}(Y_u Y_u^\dagger)^{ar} + \frac{5}{2}\delta^{ra}\delta^{sb}Y_u^{pt}\text{Tr}[Y_e^\dagger Y_e] + \frac{15}{2}\delta^{ra}\delta^{sb}Y_u^{pt}\text{Tr}[Y_d^\dagger Y_d] - \frac{8}{3}\delta^{ra}\delta^{sb}(Y_d Y_d^\dagger Y_u)^{pt} - \frac{17}{6}\delta^{sb}Y_u^{pt}(Y_d Y_d^\dagger)^{ar} \right. \\
& \left. - 5Y_u^{*rs}Y_u^{pt}Y_u^{ab} \right) + \frac{4655}{216}\delta^{ra}\delta^{sb}g_Y^4Y_u^{pt} - \frac{35}{8}\delta^{ra}\delta^{sb}g_Y^2g_L^2Y_u^{pt} \left\{ \right. \\
& + \left\{ g_s^2g_L^2 \left( \delta^{pa}\delta^{tb}Y_u^{*rs} - \frac{1}{2}\delta^{pa}\delta^{st}Y_u^{*rb} - 4\delta^{pr}\delta^{tb}Y_u^{*as} \right) + g_L^2 \left( \frac{3}{4}\delta^{pa}Y_u^{*rs}(Y_u^\dagger Y_u)^{bt} \right. \right. \\
& + \frac{9}{4}\delta^{pa}\delta^{tb}Y_u^{*rs}\text{Tr}[Y_e^\dagger Y_e] + \frac{27}{4}\delta^{pa}\delta^{tb}Y_u^{*rs}\text{Tr}[Y_d^\dagger Y_d] - \frac{3}{4}\delta^{tb}Y_u^{*rs}(Y_d Y_d^\dagger)^{pa} - 3\delta^{pa}\delta^{tb}(Y_d^\dagger Y_d Y_u^\dagger)^{rs} - \frac{9}{2}Y_u^{*rs}Y_u^{*ab}Y_u^{pt} \left. \right) - \frac{47}{48}\delta^{pa}\delta^{tb}g_Y^2g_L^2Y_u^{*rs} \\
& \left. - \frac{69}{16}\delta^{pa}\delta^{tb}g_L^4Y_u^{*rs} \right\} C_{uW}^{ab} + C_{uW}^{*ab} \left\{ g_s^2g_L^2 \left( \delta^{ra}\delta^{sb}Y_u^{pt} - \frac{1}{2}\delta^{ra}\delta^{st}Y_u^{pb} - 4\delta^{pr}\delta^{sb}Y_u^{at} \right) + g_L^2 \left( \frac{3}{4}\delta^{ra}Y_u^{pt}(Y_u^\dagger Y_u)^{sb} + \frac{9}{4}\delta^{ra}\delta^{sb}Y_u^{pt}\text{Tr}[Y_e^\dagger Y_e] \right. \right. \\
& + \frac{27}{4}\delta^{ra}\delta^{sb}Y_u^{pt}\text{Tr}[Y_d^\dagger Y_d] - \frac{3}{4}\delta^{sb}Y_u^{pt}(Y_d Y_d^\dagger)^{ar} - 3\delta^{ra}\delta^{sb}(Y_d Y_d^\dagger Y_u)^{pt} - \frac{9}{2}Y_u^{*rs}Y_u^{pt}Y_u^{ab} \left. \right) - \frac{47}{48}\delta^{ra}\delta^{sb}g_Y^2g_L^2Y_u^{pt} - \frac{69}{16}\delta^{ra}\delta^{sb}g_L^4Y_u^{pt} \left. \right\} \\
& + \left\{ g_s^4 \left( \frac{4}{3}\delta^{pr}\delta^{st}Y_u^{*ab} + \frac{23}{9}\delta^{pa}\delta^{tb}Y_u^{*rs} + \frac{53}{9}\delta^{pa}\delta^{st}Y_u^{*rb} + \frac{106}{9}\delta^{pr}\delta^{tb}Y_u^{*as} \right) + g_Y^2g_s^2 \left( \frac{22}{9}\delta^{pa}\delta^{st}Y_u^{*rb} + \frac{223}{54}\delta^{pa}\delta^{tb}Y_u^{*rs} - \frac{1}{9}\delta^{pr}\delta^{tb}Y_u^{*as} \right) \right. \\
& + g_s^2 \left( \frac{1}{2}\delta^{st}Y_u^{*rb}(Y_d Y_d^\dagger)^{pa} + \frac{2}{3}\delta^{pa}\delta^{tb}(Y_d^\dagger Y_d Y_u^\dagger)^{rs} + \frac{19}{3}\delta^{tb}Y_u^{*rs}(Y_d Y_d^\dagger)^{pa} + 8Y_u^{*rs}Y_u^{*ab}Y_u^{pt} - \text{T}_2\delta^{pa}\delta^{tb}Y_u^{*rs} - \delta^{pr}Y_u^{*as}(Y_u^\dagger Y_u)^{bt} - \delta^{st}Y_u^{*rb}(Y_u Y_u^\dagger)^{pa} \right. \\
& \left. - \frac{11}{6}\delta^{pa}Y_u^{*rs}(Y_u^\dagger Y_u)^{bt} - \frac{11}{3}\delta^{tb}Y_u^{*rs}(Y_u Y_u^\dagger)^{pa} - 5\delta^{tb}Y_u^{*as}(Y_d Y_d^\dagger)^{pr} \right) + \frac{23}{2}\delta^{pa}\delta^{tb}g_s^2g_L^2Y_u^{*rs} \left\{ C_{uG}^{ab} + C_{uG}^{*ab} \right\} \left\{ g_s^4 \left( \frac{4}{3}\delta^{pr}\delta^{st}Y_u^{ab} + \frac{23}{9}\delta^{ra}\delta^{sb}Y_u^{pt} \right. \right. \\
& + \frac{53}{9}\delta^{ra}\delta^{st}Y_u^{pb} + \frac{106}{9}\delta^{pr}\delta^{sb}Y_u^{at} \left. \right) + g_Y^2g_s^2 \left( \frac{22}{9}\delta^{ra}\delta^{st}Y_u^{pb} + \frac{223}{54}\delta^{ra}\delta^{sb}Y_u^{pt} - \frac{1}{9}\delta^{pr}\delta^{sb}Y_u^{at} \right) + g_s^2 \left( \frac{1}{2}\delta^{st}Y_u^{pb}(Y_d Y_d^\dagger)^{ar} + \frac{2}{3}\delta^{ra}\delta^{sb}(Y_d Y_d^\dagger Y_u)^{pt} \right. \\
& \left. + \frac{19}{3}\delta^{sb}Y_u^{pt}(Y_d Y_d^\dagger)^{ar} + 8Y_u^{*rs}Y_u^{pt}Y_u^{ab} - \text{T}_2\delta^{ra}\delta^{sb}Y_u^{pt} - \delta^{pr}Y_u^{at}(Y_u^\dagger Y_u)^{sb} - \delta^{st}Y_u^{pb}(Y_u Y_u^\dagger)^{ar} - \frac{11}{6}\delta^{ra}Y_u^{pt}(Y_u^\dagger Y_u)^{sb} - \frac{11}{3}\delta^{sb}Y_u^{pt}(Y_u Y_u^\dagger)^{ar} \right.
\end{aligned}$$

$$\begin{aligned}
& -5\delta^{sb}Y_u^{at}(Y_dY_d^\dagger)^{pr}) + \frac{23}{2}\delta^{ra}\delta^{sb}g_s^2g_L^2Y_u^{pt}\Bigg\} + \left\{g_Y^2\left(Y_d^{*rb}Y_u^{*as}Y_u^{pt} + \delta^{pa}Y_u^{*rs}(Y_d^\dagger Y_u)^{bt} - \frac{1}{2}Y_d^{*ab}Y_u^{*rs}Y_u^{pt}\right) + \frac{43}{9}\delta^{pa}\delta^{st}g_Y^2g_s^2Y_d^{*rb}\right\}C_{dB}^{ab} \\
& + C_{dB}^{*ab}\left\{g_Y^2\left(Y_u^{*rs}Y_d^{pb}Y_u^{at} + \delta^{ra}Y_u^{pt}(Y_u^\dagger Y_d)^{sb} - \frac{1}{2}Y_u^{*rs}Y_d^{ab}Y_u^{pt}\right) + \frac{43}{9}\delta^{ra}\delta^{st}g_Y^2g_s^2Y_d^{pb}\right\} + \left\{g_L^2\left(\frac{9}{4}Y_d^{*ab}Y_u^{*rs}Y_u^{pt} - \frac{3}{2}Y_d^{*rb}Y_u^{*as}Y_u^{pt} - 3\delta^{pa}Y_u^{*rs}(Y_d^\dagger Y_u)^{bt}\right)\right. \\
& - \frac{1}{2}\delta^{pa}\delta^{st}g_s^2g_L^2Y_d^{*rb}\Bigg\}C_{dW}^{ab} + C_{dW}^{*ab}\left\{g_L^2\left(\frac{9}{4}Y_u^{*rs}Y_d^{ab}Y_u^{pt} - \frac{3}{2}Y_u^{*rs}Y_d^{pb}Y_u^{at} - 3\delta^{ra}Y_u^{pt}(Y_u^\dagger Y_d)^{sb}\right) - \frac{1}{2}\delta^{ra}\delta^{st}g_s^2g_L^2Y_d^{pb}\right\} + \left\{g_s^4\left(\frac{4}{3}\delta^{pr}\delta^{st}Y_d^{*ab}\right.\right. \\
& + \frac{53}{9}\delta^{pa}\delta^{st}Y_d^{*rb}) + g_s^2\left(\frac{1}{2}\delta^{st}Y_d^{*rb}(Y_uY_u^\dagger)^{pa} + \frac{9}{2}\delta^{pa}Y_u^{*rs}(Y_d^\dagger Y_u)^{bt} + 8Y_d^{*ab}Y_u^{*rs}Y_u^{pt} - \delta^{st}Y_d^{*rb}(Y_dY_d^\dagger)^{pa} - 3Y_d^{*rb}Y_u^{*as}Y_u^{pt} - 5\delta^{pa}Y_d^{*rb}(Y_u^\dagger Y_u)^{st}\right) \\
& - \frac{11}{9}\delta^{pa}\delta^{st}g_Y^2g_s^2Y_d^{*rb}\Bigg\}C_{dG}^{ab} + C_{dG}^{*ab}\left\{g_s^4\left(\frac{4}{3}\delta^{pr}\delta^{st}Y_d^{ab} + \frac{53}{9}\delta^{ra}\delta^{st}Y_d^{pb}\right) + g_s^2\left(\frac{1}{2}\delta^{st}Y_d^{pb}(Y_uY_u^\dagger)^{ar} + \frac{9}{2}\delta^{ra}Y_u^{pt}(Y_u^\dagger Y_d)^{sb} + 8Y_u^{*rs}Y_d^{ab}Y_u^{pt}\right.\right. \\
& - \delta^{st}Y_d^{pb}(Y_dY_d^\dagger)^{ar} - 3Y_u^{*rs}Y_d^{pb}Y_u^{at} - 5\delta^{ra}Y_d^{pb}(Y_u^\dagger Y_u)^{st}) - \frac{11}{9}\delta^{ra}\delta^{st}g_Y^2g_s^2Y_d^{pb}\Bigg\} + \left\{\frac{2}{9}\delta^{ab}g_Y^2Y_u^{*rs}Y_u^{pt} + \frac{2}{3}Y_u^{*rs}Y_u^{pt}(Y_eY_e^\dagger)^{ba}\right\}C_{H\ell}^{(\parallel)ab} \\
& + \left\{\frac{1}{9}\delta^{ab}g_Y^2Y_u^{*rs}Y_u^{pt} + \frac{4}{3}Y_u^{*rs}Y_u^{pt}(Y_eY_e^\dagger)^{ba} - \frac{1}{3}\delta^{ab}g_L^2Y_u^{*rs}Y_u^{pt}\right\}C_{H\ell}^{(\times)ab} + \left\{\frac{2}{9}\delta^{ab}g_Y^2Y_u^{*rs}Y_u^{pt} - \frac{2}{3}Y_u^{*rs}Y_u^{pt}(Y_e^\dagger Y_e)^{ba}\right\}C_{He}^{ab} + \left\{\frac{3}{4}\delta^{pa}Y_u^{bt}(Y_u^\dagger Y_uY_u^\dagger)^{rs}\right. \\
& + \frac{3}{4}\delta^{rb}Y_u^{*as}(Y_uY_u^\dagger Y_u)^{pt} + g_L^2\left(\frac{15}{8}\delta^{pa}Y_u^{*rs}Y_u^{bt} + \frac{15}{8}\delta^{rb}Y_u^{*as}Y_u^{pt}\right) + Y_u^{*rs}Y_u^{bt}(Y_uY_u^\dagger)^{pa} + Y_u^{*as}Y_u^{pt}(Y_uY_u^\dagger)^{br} + g_s^2\left(\frac{7}{18}\delta^{rb}\delta^{st}(Y_dY_d^\dagger)^{pa}\right. \\
& + \frac{7}{18}\delta^{pa}\delta^{st}(Y_dY_d^\dagger)^{br} + \frac{8}{3}\delta^{pa}Y_u^{*rs}Y_u^{bt} + \frac{8}{3}\delta^{rb}Y_u^{*as}Y_u^{pt} - \frac{7}{18}\delta^{rb}\delta^{st}(Y_uY_u^\dagger)^{pa} - \frac{7}{18}\delta^{pa}\delta^{st}(Y_uY_u^\dagger)^{br} - 19\delta^{pa}\delta^{rb}(Y_u^\dagger Y_u)^{st}) + 2Y_u^{*rs}Y_u^{pt}(Y_dY_d^\dagger)^{ba} \\
& + 3\delta^{rb}Y_u^{pt}(Y_u^\dagger Y_uY_u^\dagger)^{as} + 3\delta^{pa}Y_u^{*rs}(Y_uY_u^\dagger Y_u)^{bt} + \frac{283}{81}\delta^{pa}\delta^{rb}\delta^{st}g_Y^2g_s^2 - \frac{1}{2}Y_u^{*rs}Y_u^{bt}(Y_dY_d^\dagger)^{pa} - \frac{1}{2}Y_u^{*as}Y_u^{pt}(Y_dY_d^\dagger)^{br} - \frac{1}{2}\delta^{rb}Y_u^{pt}(Y_d^\dagger Y_dY_u^\dagger)^{as} \\
& - \frac{1}{2}\delta^{pa}Y_u^{*rs}(Y_dY_d^\dagger Y_u)^{bt} - g_Y^2\left(\frac{2}{9}\delta^{ab}Y_u^{*rs}Y_u^{pt} + \frac{229}{216}\delta^{pa}Y_u^{*rs}Y_u^{bt} + \frac{229}{216}\delta^{rb}Y_u^{*as}Y_u^{pt}\right) - \frac{5}{4}\delta^{pa}Y_u^{bt}(Y_d^\dagger Y_dY_u^\dagger)^{rs} - \frac{5}{4}\delta^{rb}Y_u^{*as}(Y_dY_d^\dagger Y_u)^{pt} \\
& - 2Y_u^{*rs}Y_u^{pt}(Y_uY_u^\dagger)^{ba}\Bigg\}C_{Hq}^{(\parallel)ab} + \left\{\frac{1}{2}Y_u^{*rs}Y_u^{bt}(Y_uY_u^\dagger)^{pa} + \frac{1}{2}Y_u^{*as}Y_u^{pt}(Y_uY_u^\dagger)^{br} + g_L^2\left(\frac{67}{24}\delta^{pa}Y_u^{*rs}Y_u^{bt} + \frac{67}{24}\delta^{rb}Y_u^{*as}Y_u^{pt} - \delta^{ab}Y_u^{*rs}Y_u^{pt}\right)\right. \\
& + g_s^2\left(\frac{7}{18}\delta^{rb}\delta^{st}(Y_uY_u^\dagger)^{pa} + \frac{7}{18}\delta^{pa}\delta^{st}(Y_uY_u^\dagger)^{br} + \frac{7}{9}\delta^{rb}\delta^{st}(Y_dY_d^\dagger)^{pa} + \frac{7}{9}\delta^{pa}\delta^{st}(Y_dY_d^\dagger)^{br} - \frac{8}{3}\delta^{pa}Y_u^{*rs}Y_u^{bt} - \frac{8}{3}\delta^{rb}Y_u^{*as}Y_u^{pt} - \frac{19}{2}\delta^{pa}\delta^{rb}(Y_u^\dagger Y_u)^{st}\right) \\
& + \frac{3}{2}\delta^{rb}Y_u^{pt}(Y_u^\dagger Y_uY_u^\dagger)^{as} + \frac{3}{2}\delta^{pa}Y_u^{*rs}(Y_uY_u^\dagger Y_u)^{bt} + \frac{283}{162}\delta^{pa}\delta^{rb}\delta^{st}g_Y^2g_s^2 + 2Y_u^{*rs}Y_u^{pt}(Y_uY_u^\dagger)^{ba} + 4Y_u^{*rs}Y_u^{pt}(Y_dY_d^\dagger)^{ba} - g_Y^2\left(\frac{1}{9}\delta^{ab}Y_u^{*rs}Y_u^{pt}\right. \\
& + \frac{65}{216}\delta^{pa}Y_u^{*rs}Y_u^{bt} + \frac{65}{216}\delta^{rb}Y_u^{*as}Y_u^{pt}) - Y_u^{*rs}Y_u^{bt}(Y_dY_d^\dagger)^{pa} - Y_u^{*as}Y_u^{pt}(Y_dY_d^\dagger)^{br} - \delta^{rb}Y_u^{pt}(Y_d^\dagger Y_dY_u^\dagger)^{as} - \delta^{pa}Y_u^{*rs}(Y_dY_d^\dagger Y_u)^{bt} - \frac{23}{18}\delta^{pa}\delta^{rb}\delta^{st}g_s^2g_L^2 \\
& - \frac{3}{2}\delta^{pa}Y_u^{bt}(Y_u^\dagger Y_uY_u^\dagger)^{rs} - \frac{3}{2}\delta^{rb}Y_u^{*as}(Y_uY_u^\dagger Y_u)^{pt} - \frac{5}{2}\delta^{pa}Y_u^{bt}(Y_d^\dagger Y_dY_u^\dagger)^{rs} - \frac{5}{2}\delta^{rb}Y_u^{*as}(Y_dY_d^\dagger Y_u)^{pt}\Bigg\}C_{Hq}^{(\times)ab} + \left\{g_L^2\left(\frac{3}{8}\delta^{sa}Y_u^{*rb}Y_u^{pt} + \frac{3}{8}\delta^{tb}Y_u^{*rs}Y_u^{pa}\right)\right.
\end{aligned}$$



$$\begin{aligned}
& + g_s^2 \left( \frac{7}{9} \delta^{pr} \delta^{tb} (Y_u^\dagger Y_u)^{sa} + \frac{7}{9} \delta^{pr} \delta^{sa} (Y_u^\dagger Y_u)^{bt} + \frac{19}{2} \delta^{sa} \delta^{tb} (Y_u Y_u^\dagger)^{pr} - \frac{8}{3} \delta^{sa} Y_u^{*rb} Y_u^{pt} - \frac{8}{3} \delta^{tb} Y_u^{*rs} Y_u^{pa} - \frac{19}{2} \delta^{sa} \delta^{tb} (Y_d Y_d^\dagger)^{pr} \right) + \delta^{sa} Y_u^{pt} (Y_d^\dagger Y_d Y_u^\dagger)^{rb} \\
& + \delta^{tb} Y_u^{*rs} (Y_d Y_d^\dagger Y_u)^{pa} + 2 Y_u^{*rs} Y_u^{pt} (Y_u^\dagger Y_u)^{ba} - \frac{31}{162} \delta^{pr} \delta^{sa} \delta^{tb} g_Y^2 g_s^2 - \frac{1}{4} \delta^{tb} Y_u^{pa} (Y_d^\dagger Y_d Y_u^\dagger)^{rs} - \frac{1}{4} \delta^{sa} Y_u^{*rb} (Y_d Y_d^\dagger Y_u)^{pt} - \frac{1}{2} Y_u^{*rb} Y_u^{pt} (Y_u^\dagger Y_u)^{sa} \\
& - \frac{1}{2} Y_u^{*rs} Y_u^{pa} (Y_u^\dagger Y_u)^{bt} - g_Y^2 \left( \frac{4}{9} \delta^{ab} Y_u^{*rs} Y_u^{pt} + \frac{121}{216} \delta^{sa} Y_u^{*rb} Y_u^{pt} + \frac{121}{216} \delta^{tb} Y_u^{*rs} Y_u^{pa} \right) - \frac{3}{2} \delta^{sa} Y_u^{pt} (Y_u^\dagger Y_u Y_u^\dagger)^{rb} - \frac{3}{2} \delta^{tb} Y_u^{*rs} (Y_u Y_u^\dagger Y_u)^{pa} \\
& - \frac{9}{4} \delta^{tb} Y_u^{pa} (Y_u^\dagger Y_u Y_u^\dagger)^{rs} - \frac{9}{4} \delta^{sa} Y_u^{*rb} (Y_u Y_u^\dagger Y_u)^{pt} \Bigg\} C_{Hu}^{ab} + \left\{ \frac{2}{9} \delta^{ab} g_Y^2 Y_u^{*rs} Y_u^{pt} - 2 Y_u^{*rs} Y_u^{pt} (Y_d^\dagger Y_d)^{ba} \right\} C_{Hd}^{ab} + \left\{ \frac{1}{2} Y_d^{*rb} Y_u^{pt} (Y_u^\dagger Y_u)^{sa} \right. \\
& + \frac{1}{2} \delta^{sa} Y_u^{pt} (Y_d^\dagger Y_d Y_d^\dagger)^{rb} + g_s^2 \left( \frac{8}{3} \delta^{sa} Y_d^{*rb} Y_u^{pt} - \frac{1}{9} \delta^{pr} \delta^{sa} (Y_d^\dagger Y_u)^{bt} \right) + \frac{3}{2} \delta^{sa} Y_d^{*rb} (Y_d Y_d^\dagger Y_u)^{pt} - \frac{23}{72} \delta^{sa} g_Y^2 Y_d^{*rb} Y_u^{pt} - \frac{3}{8} \delta^{sa} g_L^2 Y_d^{*rb} Y_u^{pt} \\
& \left. - 2 Y_u^{*rs} Y_u^{pt} (Y_d^\dagger Y_u)^{ba} \right\} C_{Hud}^{ab} + C_{Hud}^{*ab} \left\{ \frac{1}{2} Y_u^{*rs} Y_d^{pb} (Y_u^\dagger Y_u)^{at} + \frac{1}{2} \delta^{ta} Y_u^{*rs} (Y_d Y_d^\dagger Y_d)^{pb} + g_s^2 \left( \frac{8}{3} \delta^{ta} Y_u^{*rs} Y_d^{pb} - \frac{1}{9} \delta^{pr} \delta^{ta} (Y_u^\dagger Y_d)^{sb} \right) + \frac{3}{2} \delta^{ta} Y_d^{pb} (Y_d^\dagger Y_d Y_u^\dagger)^{rs} \right. \\
& \left. - \frac{23}{72} \delta^{ta} g_Y^2 Y_u^{*rs} Y_d^{pb} - \frac{3}{8} \delta^{ta} g_L^2 Y_u^{*rs} Y_d^{pb} - 2 Y_u^{*rs} Y_u^{pt} (Y_u^\dagger Y_d)^{ab} \right\} + 2 Y_e^{*ad} Y_u^{*rs} C_{\ell e}^{abcd} Y_e^{bc} Y_u^{pt} + \left\{ \frac{37}{81} \delta^{pr} \delta^{sc} \delta^{td} \delta^{ab} g_Y^2 g_s^2 - g_Y^2 \left( \frac{26}{27} \delta^{sc} \delta^{ab} Y_u^{*rd} Y_u^{pt} \right. \right. \\
& \left. \left. + \frac{26}{27} \delta^{td} \delta^{ab} Y_u^{*rs} Y_u^{pc} \right) \right\} C_{\ell u}^{abcd} + \left\{ g_Y^2 \left( \frac{16}{27} \delta^{pa} \delta^{cd} Y_u^{*rs} Y_u^{bt} + \frac{16}{27} \delta^{rb} \delta^{cd} Y_u^{*as} Y_u^{pt} \right) - \frac{362}{81} \delta^{pa} \delta^{rb} \delta^{st} \delta^{cd} g_Y^2 g_s^2 \right\} C_{qe}^{abcd} + \left\{ \frac{1}{4} \delta^{rb} \delta^{td} Y_u^{pc} (Y_u^\dagger Y_u Y_u^\dagger)^{as} \right. \\
& + \frac{1}{4} \delta^{pa} \delta^{sc} Y_u^{*rd} (Y_u Y_u^\dagger Y_u)^{bt} + \frac{1}{2} T_2 \delta^{pa} \delta^{sc} Y_u^{*rd} Y_u^{bt} + \frac{1}{2} T_2 \delta^{rb} \delta^{td} Y_u^{*as} Y_u^{pc} + \frac{1}{2} \delta^{sc} Y_u^{*rd} Y_u^{bt} (Y_d Y_d^\dagger)^{pa} + \frac{1}{2} \delta^{td} Y_u^{*as} Y_u^{pc} (Y_d Y_d^\dagger)^{br} \\
& + \frac{1}{2} \delta^{pa} \delta^{sc} Y_u^{bt} (Y_u^\dagger Y_u Y_u^\dagger)^{rd} + \frac{1}{2} \delta^{rb} \delta^{td} Y_u^{*as} (Y_u Y_u^\dagger Y_u)^{pc} + g_L^2 \left( \frac{15}{8} \delta^{pa} \delta^{sc} Y_u^{*rd} Y_u^{bt} + \frac{15}{8} \delta^{rb} \delta^{td} Y_u^{*as} Y_u^{pc} + 3 \delta^{rb} \delta^{sc} Y_u^{*ad} Y_u^{pt} + 3 \delta^{pa} \delta^{td} Y_u^{*rs} Y_u^{bc} \right) \\
& + g_Y^2 \left( \frac{13}{72} \delta^{pa} \delta^{sc} Y_u^{*rd} Y_u^{bt} + \frac{13}{72} \delta^{rb} \delta^{td} Y_u^{*as} Y_u^{pc} + \frac{26}{27} \delta^{sc} \delta^{ab} Y_u^{*rd} Y_u^{pt} + \frac{26}{27} \delta^{td} \delta^{ab} Y_u^{*rs} Y_u^{pc} + \frac{25}{9} \delta^{rb} \delta^{sc} Y_u^{*ad} Y_u^{pt} + \frac{25}{9} \delta^{pa} \delta^{td} Y_u^{*rs} Y_u^{bc} \right. \\
& \left. - \frac{32}{27} \delta^{pa} \delta^{cd} Y_u^{*rs} Y_u^{bt} - \frac{32}{27} \delta^{rb} \delta^{cd} Y_u^{*as} Y_u^{pt} \right) + g_Y^2 g_s^2 \left( \frac{23}{6} \delta^{pa} \delta^{rb} \delta^{sc} \delta^{td} + \frac{724}{81} \delta^{pa} \delta^{rb} \delta^{st} \delta^{cd} - \frac{37}{81} \delta^{pr} \delta^{sc} \delta^{td} \delta^{ab} \right) + g_s^2 \left( \frac{2}{3} \delta^{pa} \delta^{sc} Y_u^{*rd} Y_u^{bt} \right. \\
& + \frac{2}{3} \delta^{rb} \delta^{td} Y_u^{*as} Y_u^{pc} + 3 \delta^{rb} \delta^{sc} \delta^{td} (Y_d Y_d^\dagger)^{pa} + 3 \delta^{pa} \delta^{sc} \delta^{td} (Y_d Y_d^\dagger)^{br} + 3 \delta^{rb} \delta^{sc} \delta^{td} (Y_u Y_u^\dagger)^{pa} + 3 \delta^{pa} \delta^{sc} \delta^{td} (Y_u Y_u^\dagger)^{br} + \frac{10}{3} \delta^{rb} \delta^{sc} Y_u^{*ad} Y_u^{pt} \\
& + \frac{10}{3} \delta^{pa} \delta^{td} Y_u^{*rs} Y_u^{bc} + 6 \delta^{pa} \delta^{rb} \delta^{td} (Y_u^\dagger Y_u)^{sc} + 6 \delta^{pa} \delta^{rb} \delta^{sc} (Y_u^\dagger Y_u)^{dt} - \frac{4}{9} \delta^{pa} \delta^{st} Y_u^{*rd} Y_u^{bc} - \frac{4}{9} \delta^{rb} \delta^{st} Y_u^{*ad} Y_u^{pc} - \frac{8}{9} \delta^{pr} \delta^{sc} Y_u^{*ad} Y_u^{bt} - \frac{8}{9} \delta^{pr} \delta^{td} Y_u^{*as} Y_u^{bc} \\
& + \frac{7}{4} \delta^{rb} \delta^{sc} Y_u^{pt} (Y_d^\dagger Y_d Y_u^\dagger)^{ad} + \frac{7}{4} \delta^{pa} \delta^{td} Y_u^{*rs} (Y_d Y_d^\dagger Y_u)^{bc} + \frac{27}{2} \delta^{pa} \delta^{rb} \delta^{sc} \delta^{td} g_s^2 g_L^2 - g_s^4 \left( \frac{11}{3} \delta^{pa} \delta^{rb} \delta^{st} \delta^{cd} + \frac{22}{3} \delta^{pr} \delta^{sc} \delta^{td} \delta^{ab} + 55 \delta^{pa} \delta^{rb} \delta^{sc} \delta^{td} \right) \\
& - \left( 3 \delta^{rb} \delta^{sc} Y_u^{*ad} Y_u^{pt} + 3 \delta^{pa} \delta^{td} Y_u^{*rs} Y_u^{bc} \right) \text{Tr}[Y_u^\dagger Y_u] - \frac{5}{4} \delta^{pa} Y_u^{*rd} Y_u^{bt} (Y_u^\dagger Y_u)^{sc} - \frac{5}{4} \delta^{rb} Y_u^{*as} Y_u^{pc} (Y_u^\dagger Y_u)^{dt} - \frac{5}{4} \delta^{rb} \delta^{td} Y_u^{pc} (Y_d^\dagger Y_d Y_u^\dagger)^{as} \\
& - \frac{5}{4} \delta^{pa} \delta^{sc} Y_u^{*rd} (Y_d Y_d^\dagger Y_u)^{bt} - \frac{3}{2} \delta^{pa} \delta^{sc} Y_u^{bt} (Y_d^\dagger Y_d Y_u^\dagger)^{rd} - \frac{3}{2} \delta^{rb} \delta^{td} Y_u^{*as} (Y_d Y_d^\dagger Y_u)^{pc} - \frac{5}{2} \delta^{sc} Y_u^{*rd} Y_u^{bt} (Y_u Y_u^\dagger)^{pa} - \frac{5}{2} \delta^{td} Y_u^{*as} Y_u^{pc} (Y_u Y_u^\dagger)^{br} \\
& - 6 \delta^{pa} Y_u^{*rs} Y_u^{bt} (Y_u^\dagger Y_u)^{dc} - 6 \delta^{rb} Y_u^{*as} Y_u^{pt} (Y_u^\dagger Y_u)^{dc} - 6 \delta^{sc} Y_u^{*rd} Y_u^{pt} (Y_u Y_u^\dagger)^{ba} - 6 \delta^{td} Y_u^{*rs} Y_u^{pc} (Y_u Y_u^\dagger)^{ba} - 6 \delta^{rb} \delta^{sc} Y_u^{pt} (Y_u^\dagger Y_u Y_u^\dagger)^{ad}
\end{aligned}$$

$$\begin{aligned}
& -6\delta^{pa}\delta^{td}Y_u^{*rs}(Y_uY_u^\dagger Y_u)^{bc} \Big\} C_{qu}^{(\parallel)abcd} + \left\{ g_s^2 g_L^2 \left( 3\delta^{pr}\delta^{sc}\delta^{td}\delta^{ab} + \frac{63}{4}\delta^{pa}\delta^{rb}\delta^{sc}\delta^{td} \right) + g_Y^2 g_s^2 \left( \frac{152}{243}\delta^{pr}\delta^{sc}\delta^{td}\delta^{ab} + \frac{77}{36}\delta^{pa}\delta^{rb}\delta^{sc}\delta^{td} \right. \right. \\
& + \frac{2236}{243}\delta^{pa}\delta^{rb}\delta^{st}\delta^{cd} \Big) + g_s^4 \left( \frac{628}{81}\delta^{pa}\delta^{rb}\delta^{st}\delta^{cd} + \frac{1364}{81}\delta^{pr}\delta^{sc}\delta^{td}\delta^{ab} - \frac{8}{9}\delta^{pr}\delta^{st}\delta^{ab}\delta^{cd} - \frac{357}{2}\delta^{pa}\delta^{rb}\delta^{sc}\delta^{td} \right) + \delta^{sc}\delta^{td}(Y_dY_d^\dagger)^{br}(Y_uY_u^\dagger)^{pa} \\
& + \delta^{sc}\delta^{td}(Y_dY_d^\dagger)^{pa}(Y_uY_u^\dagger)^{br} + g_L^2 \left( \frac{33}{16}\delta^{rb}\delta^{sc}\delta^{td}(Y_dY_d^\dagger)^{pa} + \frac{33}{16}\delta^{pa}\delta^{sc}\delta^{td}(Y_dY_d^\dagger)^{br} + \frac{33}{16}\delta^{rb}\delta^{sc}\delta^{td}(Y_uY_u^\dagger)^{pa} + \frac{33}{16}\delta^{pa}\delta^{sc}\delta^{td}(Y_uY_u^\dagger)^{br} \right. \\
& + \frac{51}{8}\delta^{pa}\delta^{rb}\delta^{td}(Y_u^\dagger Y_u)^{sc} + \frac{51}{8}\delta^{pa}\delta^{rb}\delta^{sc}(Y_u^\dagger Y_u)^{dt} + 9\delta^{rb}\delta^{sc}Y_u^{*ad}Y_u^{pt} + 9\delta^{pa}\delta^{td}Y_u^{*rs}Y_u^{bc} \Big) + g_Y^2 \left( \frac{26}{81}\delta^{sc}\delta^{ab}Y_u^{*rd}Y_u^{pt} + \frac{26}{81}\delta^{td}\delta^{ab}Y_u^{*rs}Y_u^{pc} \right. \\
& + \frac{73}{72}\delta^{pa}\delta^{rb}\delta^{td}(Y_u^\dagger Y_u)^{sc} + \frac{73}{72}\delta^{pa}\delta^{rb}\delta^{sc}(Y_u^\dagger Y_u)^{dt} + \frac{523}{144}\delta^{rb}\delta^{sc}\delta^{td}(Y_uY_u^\dagger)^{pa} + \frac{523}{144}\delta^{pa}\delta^{sc}\delta^{td}(Y_uY_u^\dagger)^{br} + \frac{25}{3}\delta^{rb}\delta^{sc}Y_u^{*ad}Y_u^{pt} + \frac{25}{3}\delta^{pa}\delta^{td}Y_u^{*rs}Y_u^{bc} \\
& - \frac{41}{144}\delta^{rb}\delta^{sc}\delta^{td}(Y_dY_d^\dagger)^{pa} - \frac{41}{144}\delta^{pa}\delta^{sc}\delta^{td}(Y_dY_d^\dagger)^{br} - \frac{32}{81}\delta^{pa}\delta^{cd}Y_u^{*rs}Y_u^{bt} - \frac{32}{81}\delta^{rb}\delta^{cd}Y_u^{*as}Y_u^{pt} \Big) + g_s^2 \left( \frac{2}{3}\delta^{pa}\delta^{rb}\delta^{cd}(Y_u^\dagger Y_u)^{st} + \frac{2}{3}\delta^{sc}\delta^{td}\delta^{ab}(Y_uY_u^\dagger)^{pr} \right. \\
& + \frac{4}{3}\delta^{st}\delta^{ab}Y_u^{*rd}Y_u^{pc} + \frac{4}{3}\delta^{pr}\delta^{cd}Y_u^{*as}Y_u^{bt} + \frac{16}{3}\delta^{rb}\delta^{sc}\delta^{td}(Y_dY_d^\dagger)^{pa} + \frac{16}{3}\delta^{pa}\delta^{sc}\delta^{td}(Y_dY_d^\dagger)^{br} + \frac{16}{3}\delta^{rb}\delta^{sc}\delta^{td}(Y_uY_u^\dagger)^{pa} + \frac{16}{3}\delta^{pa}\delta^{sc}\delta^{td}(Y_uY_u^\dagger)^{br} \\
& + 8\delta^{pa}\delta^{sc}Y_u^{*rd}Y_u^{bt} + 8\delta^{rb}\delta^{td}Y_u^{*as}Y_u^{pc} + \frac{32}{3}\delta^{pa}\delta^{rb}\delta^{td}(Y_u^\dagger Y_u)^{sc} + \frac{32}{3}\delta^{pa}\delta^{rb}\delta^{sc}(Y_u^\dagger Y_u)^{dt} + 58\delta^{rb}\delta^{sc}Y_u^{*ad}Y_u^{pt} + 58\delta^{pa}\delta^{td}Y_u^{*rs}Y_u^{bc} \\
& - \frac{1}{3}\delta^{pa}\delta^{st}Y_u^{*rd}Y_u^{bc} - \frac{1}{3}\delta^{rb}\delta^{st}Y_u^{*ad}Y_u^{pc} - \frac{2}{3}\delta^{pr}\delta^{sc}Y_u^{*ad}Y_u^{bt} - \frac{2}{3}\delta^{pr}\delta^{td}Y_u^{*as}Y_u^{bc} - \frac{4}{3}\delta^{pa}\delta^{rb}\delta^{st}(Y_u^\dagger Y_u)^{dc} - \frac{4}{3}\delta^{pr}\delta^{sc}\delta^{td}(Y_uY_u^\dagger)^{ba} - 2\delta^{pr}\delta^{sc}\delta^{td}(Y_dY_d^\dagger)^{ba} \\
& - \frac{65}{27}\delta^{pa}\delta^{cd}Y_u^{*rs}Y_u^{bt} - \frac{65}{27}\delta^{rb}\delta^{cd}Y_u^{*as}Y_u^{pt} - \frac{130}{27}\delta^{sc}\delta^{ab}Y_u^{*rd}Y_u^{pt} - \frac{130}{27}\delta^{td}\delta^{ab}Y_u^{*rs}Y_u^{pc} \Big) + 2\delta^{rb}\delta^{sc}(Y_u^\dagger Y_u)^{dt}(Y_uY_u^\dagger)^{pa} + 2\delta^{pa}\delta^{td}(Y_u^\dagger Y_u)^{sc}(Y_uY_u^\dagger)^{br} \\
& + 3\delta^{pa}\delta^{rb}\delta^{sc}\delta^{td}g_Y^2g_L^2 + \frac{21}{4}\delta^{rb}\delta^{sc}Y_u^{pt}(Y_d^\dagger Y_dY_u^\dagger)^{ad} + \frac{21}{4}\delta^{pa}\delta^{td}Y_u^{*rs}(Y_dY_d^\dagger Y_u)^{bc} + \frac{494}{27}\delta^{pa}\delta^{rb}\delta^{sc}\delta^{td}g_Y^4 - \frac{1}{4}\delta^{pa}\delta^{rb}\delta^{td}(Y_u^\dagger Y_dY_d^\dagger Y_u)^{sc} \\
& - \frac{1}{4}\delta^{pa}\delta^{rb}\delta^{sc}(Y_u^\dagger Y_dY_d^\dagger Y_u)^{dt} - \frac{1}{4}\delta^{pa}\delta^{rb}\delta^{td}(Y_u^\dagger Y_uY_u^\dagger Y_u)^{sc} - \frac{1}{4}\delta^{pa}\delta^{rb}\delta^{sc}(Y_u^\dagger Y_uY_u^\dagger Y_u)^{dt} - \frac{1}{4}\delta^{rb}\delta^{sc}\delta^{td}(Y_dY_d^\dagger Y_dY_d^\dagger)^{pa} - \frac{1}{4}\delta^{pa}\delta^{sc}\delta^{td}(Y_dY_d^\dagger Y_dY_d^\dagger)^{br} \\
& - \frac{1}{4}\delta^{rb}\delta^{sc}\delta^{td}(Y_uY_u^\dagger Y_uY_u^\dagger)^{pa} - \frac{1}{4}\delta^{pa}\delta^{sc}\delta^{td}(Y_uY_u^\dagger Y_uY_u^\dagger)^{br} - \frac{3}{4}T_2\delta^{rb}\delta^{sc}\delta^{td}(Y_dY_d^\dagger)^{pa} - \frac{3}{4}T_2\delta^{pa}\delta^{sc}\delta^{td}(Y_dY_d^\dagger)^{br} - \frac{3}{4}T_2\delta^{rb}\delta^{sc}\delta^{td}(Y_uY_u^\dagger)^{pa} \\
& - \frac{3}{4}T_2\delta^{pa}\delta^{sc}\delta^{td}(Y_uY_u^\dagger)^{br} - \delta^{rb}\delta^{td}(Y_u^\dagger Y_u)^{sc}(Y_dY_d^\dagger)^{pa} - \delta^{pa}\delta^{sc}(Y_u^\dagger Y_u)^{dt}(Y_dY_d^\dagger)^{br} - \left( 9\delta^{rb}\delta^{sc}Y_u^{*ad}Y_u^{pt} + 9\delta^{pa}\delta^{td}Y_u^{*rs}Y_u^{bc} \right) \text{Tr}[Y_u^\dagger Y_u] \\
& - \frac{5}{4}\delta^{rb}\delta^{td}(Y_u^\dagger Y_u)^{sc}(Y_uY_u^\dagger)^{pa} - \frac{5}{4}\delta^{pa}\delta^{sc}(Y_u^\dagger Y_u)^{dt}(Y_uY_u^\dagger)^{br} - \frac{3}{2}T_2\delta^{pa}\delta^{rb}\delta^{td}(Y_u^\dagger Y_u)^{sc} - \frac{3}{2}T_2\delta^{pa}\delta^{rb}\delta^{sc}(Y_u^\dagger Y_u)^{dt} - 2Y_u^{*rd}Y_u^{*as}Y_u^{pc}Y_u^{bt} \\
& - 2\delta^{pa}Y_u^{*rs}Y_u^{bt}(Y_u^\dagger Y_u)^{dc} - 2\delta^{rb}Y_u^{*as}Y_u^{pt}(Y_u^\dagger Y_u)^{dc} - 2\delta^{sc}Y_u^{*rd}Y_u^{pt}(Y_uY_u^\dagger)^{ba} - 2\delta^{td}Y_u^{*rs}Y_u^{pc}(Y_uY_u^\dagger)^{ba} - \frac{5}{2}\delta^{sc}\delta^{td}(Y_dY_d^\dagger)^{pa}(Y_dY_d^\dagger)^{br} \\
& - \frac{11}{4}\delta^{rb}\delta^{sc}(Y_u^\dagger Y_u)^{dt}(Y_dY_d^\dagger)^{pa} - \frac{11}{4}\delta^{pa}\delta^{td}(Y_u^\dagger Y_u)^{sc}(Y_dY_d^\dagger)^{br} - \frac{7}{2}\delta^{pa}\delta^{rb}(Y_u^\dagger Y_u)^{sc}(Y_u^\dagger Y_u)^{dt} - \frac{7}{2}\delta^{sc}\delta^{td}(Y_uY_u^\dagger)^{pa}(Y_uY_u^\dagger)^{br} - 18\delta^{rb}\delta^{sc}Y_u^{pt}(Y_u^\dagger Y_uY_u^\dagger)^{ad} \\
& - 18\delta^{pa}\delta^{td}Y_u^{*rs}(Y_uY_u^\dagger Y_u)^{bc} \Big\} C_{qu}^{(\times)abcd} + \left\{ g_Y^2 \left( \frac{16}{27}\delta^{pa}\delta^{cd}Y_u^{*rs}Y_u^{bt} + \frac{16}{27}\delta^{rb}\delta^{cd}Y_u^{*as}Y_u^{pt} \right) + 6Y_d^{*ad}Y_u^{*rs}Y_d^{bc}Y_u^{pt} - \frac{1}{4}Y_d^{*rd}Y_u^{*as}Y_d^{bc}Y_u^{pt} \right. \\
& - \frac{1}{4}Y_d^{*ad}Y_u^{*rs}Y_d^{pc}Y_u^{bt} - \frac{3}{4}\delta^{rb}Y_u^{*as}Y_d^{pc}(Y_d^\dagger Y_u)^{dt} - \frac{3}{4}\delta^{pa}Y_d^{*rd}Y_u^{bt}(Y_u^\dagger Y_d)^{sc} - g_s^2 \left( \frac{4}{9}\delta^{pa}\delta^{st}Y_d^{*rd}Y_d^{bc} + \frac{4}{9}\delta^{rb}\delta^{st}Y_d^{*ad}Y_d^{pc} \right) - \frac{11}{3}\delta^{pa}\delta^{rb}\delta^{st}\delta^{cd}g_s^4 \\
& \left. \right\}
\end{aligned}$$

$$\begin{aligned}
& -\frac{362}{81}\delta^{pa}\delta^{rb}\delta^{st}\delta^{cd}g_Y^2g_s^2\left\}C_{qd}^{(\parallel)abcd} + \left\{g_Y^2\left(\frac{16}{81}\delta^{pa}\delta^{cd}Y_u^{*rs}Y_u^{bt} + \frac{16}{81}\delta^{rb}\delta^{cd}Y_u^{*as}Y_u^{pt}\right) + g_s^4\left(\frac{628}{81}\delta^{pa}\delta^{rb}\delta^{st}\delta^{cd} - \frac{4}{9}\delta^{pr}\delta^{st}\delta^{ab}\delta^{cd}\right)\right. \\
& + g_s^2\left(\frac{2}{3}\delta^{st}\delta^{ab}Y_d^{*rd}Y_d^{pc} + \frac{2}{3}\delta^{pr}\delta^{cd}Y_u^{*as}Y_u^{bt} + \frac{2}{3}\delta^{pa}\delta^{rb}\delta^{cd}(Y_u^\dagger Y_u)^{st} - \frac{1}{3}\delta^{pa}\delta^{st}Y_d^{*rd}Y_d^{bc} - \frac{1}{3}\delta^{rb}\delta^{st}Y_d^{*ad}Y_d^{pc} - \frac{4}{3}\delta^{pa}\delta^{rb}\delta^{st}(Y_d^\dagger Y_d)^{dc}\right. \\
& - \frac{65}{27}\delta^{pa}\delta^{cd}Y_u^{*rs}Y_u^{bt} - \frac{65}{27}\delta^{rb}\delta^{cd}Y_u^{*as}Y_u^{pt}\left. + 18Y_d^{*ad}Y_u^{*rs}Y_d^{bc}Y_u^{pt} - \frac{3}{4}Y_d^{*rd}Y_u^{*as}Y_d^{bc}Y_u^{pt} - \frac{3}{4}Y_d^{*ad}Y_u^{*rs}Y_d^{pc}Y_u^{bt} - \frac{3}{2}\delta^{pa}\delta^{rb}(Y_d^\dagger Y_u)^{dt}(Y_u^\dagger Y_d)^{sc}\right. \\
& - \frac{5}{2}Y_d^{*rd}Y_u^{*as}Y_d^{pc}Y_u^{bt} - \frac{659}{243}\delta^{pa}\delta^{rb}\delta^{st}\delta^{cd}g_Y^2g_s^2\left\}C_{qd}^{(\times)abcd} + \left\{g_Y^2\left(\frac{92}{81}\delta^{tb}\delta^{ad}Y_u^{*rs}Y_u^{pc} + \frac{92}{81}\delta^{sa}\delta^{bc}Y_u^{*rd}Y_u^{pt} + \frac{104}{27}\delta^{sa}\delta^{cd}Y_u^{*rb}Y_u^{pt}\right.\right. \\
& + \frac{104}{27}\delta^{tb}\delta^{cd}Y_u^{*rs}Y_u^{pa} + \frac{295}{36}\delta^{sa}\delta^{td}Y_u^{*rb}Y_u^{pc}\left. + g_s^4\left(\frac{4}{9}\delta^{pr}\delta^{st}\delta^{ad}\delta^{bc} + \frac{1700}{81}\delta^{pr}\delta^{sa}\delta^{td}\delta^{bc} - \frac{14}{3}\delta^{pr}\delta^{sa}\delta^{tb}\delta^{cd}\right) + g_s^2\left(\frac{2}{3}\delta^{sa}\delta^{td}\delta^{bc}(Y_u Y_u^\dagger)^{pr}\right.\right. \\
& + 10\delta^{sa}\delta^{tb}Y_u^{*rd}Y_u^{pc} - \frac{2}{3}\delta^{st}\delta^{ad}Y_u^{*rb}Y_u^{pc} - \frac{34}{27}\delta^{tb}\delta^{ad}Y_u^{*rs}Y_u^{pc} - \frac{34}{27}\delta^{sa}\delta^{bc}Y_u^{*rd}Y_u^{pt} - \frac{14}{3}\delta^{sa}\delta^{td}Y_u^{*rb}Y_u^{pc} - \frac{20}{3}\delta^{pr}\delta^{sa}\delta^{td}(Y_u^\dagger Y_u)^{bc}\left. + 5T_2\delta^{sa}\delta^{td}Y_u^{*rb}Y_u^{pc} + 5\delta^{sa}\delta^{td}Y_u^{pc}(Y_u^\dagger Y_u Y_u^\dagger)^{rb} + 5\delta^{sa}\delta^{td}Y_u^{*rb}(Y_u Y_u^\dagger Y_u)^{pc} - \frac{1}{2}\delta^{tb}Y_u^{*rd}Y_u^{pa}(Y_u^\dagger Y_u)^{sc} - \frac{1}{2}\delta^{sa}Y_u^{*rb}Y_u^{pc}(Y_u^\dagger Y_u)^{dt}\right. \\
& - g_Y^2g_s^2\left(\frac{148}{81}\delta^{pr}\delta^{sa}\delta^{tb}\delta^{cd} + \frac{1216}{243}\delta^{pr}\delta^{sa}\delta^{td}\delta^{bc}\right) - 3\delta^{sa}\delta^{td}Y_u^{pc}(Y_d^\dagger Y_d Y_u^\dagger)^{rb} - 3\delta^{sa}\delta^{td}Y_u^{*rb}(Y_d Y_d^\dagger Y_u)^{pc} - 6\delta^{sa}Y_u^{*rb}Y_u^{pt}(Y_u^\dagger Y_u)^{dc} \\
& - 6\delta^{tb}Y_u^{*rs}Y_u^{pa}(Y_u^\dagger Y_u)^{dc} - \frac{51}{4}\delta^{sa}\delta^{td}g_L^2Y_u^{*rb}Y_u^{pc}\left\}C_{uu}^{abcd} + \left\{\frac{8}{9}\delta^{pr}\delta^{st}\delta^{ad}\delta^{bc}g_s^4 - \frac{4}{3}\delta^{st}\delta^{ad}g_s^2Y_d^{*rb}Y_d^{pc}\right\}C_{dd}^{abcd} + \left\{\frac{37}{81}\delta^{pr}\delta^{sc}\delta^{td}\delta^{ab}g_Y^2g_s^2\right. \\
& - g_Y^2\left(\frac{26}{27}\delta^{sc}\delta^{ab}Y_u^{*rd}Y_u^{pt} + \frac{26}{27}\delta^{td}\delta^{ab}Y_u^{*rs}Y_u^{pc}\right)\left\}C_{eu}^{abcd} + \left\{\frac{1}{4}\delta^{sa}Y_u^{*rb}Y_d^{pc}(Y_d^\dagger Y_u)^{dt} + \frac{1}{4}\delta^{tb}Y_d^{*rd}Y_u^{pa}(Y_u^\dagger Y_d)^{sc} + \frac{37}{81}\delta^{pr}\delta^{sa}\delta^{tb}\delta^{cd}g_Y^2g_s^2\right. \\
& + \frac{3}{4}\delta^{tb}Y_u^{*rs}Y_d^{pc}(Y_d^\dagger Y_u)^{da} + \frac{3}{4}\delta^{sa}Y_d^{*rd}Y_u^{pt}(Y_u^\dagger Y_d)^{bc} + 2\delta^{sa}\delta^{tb}g_s^2Y_d^{*rd}Y_d^{pc} - \frac{1}{3}\delta^{pr}\delta^{sa}\delta^{tb}\delta^{cd}g_s^4 - g_Y^2\left(\frac{26}{27}\delta^{sa}\delta^{cd}Y_u^{*rb}Y_u^{pt} + \frac{26}{27}\delta^{tb}\delta^{cd}Y_u^{*rs}Y_u^{pa}\right)\left\}C_{ud}^{(\parallel)abcd} \right. \\
& + \left\{g_s^4\left(\frac{592}{81}\delta^{pr}\delta^{sa}\delta^{tb}\delta^{cd} - \frac{2}{9}\delta^{pr}\delta^{st}\delta^{ab}\delta^{cd}\right) + g_s^2\left(\frac{1}{3}\delta^{st}\delta^{cd}Y_u^{*rb}Y_u^{pa} + \frac{1}{3}\delta^{sa}\delta^{tb}\delta^{cd}(Y_u Y_u^\dagger)^{pr} - \frac{4}{3}\delta^{sa}\delta^{tb}Y_d^{*rd}Y_d^{pc} - 2\delta^{pr}\delta^{sa}\delta^{tb}(Y_d^\dagger Y_d)^{dc}\right.\right. \\
& - \frac{65}{27}\delta^{sa}\delta^{cd}Y_u^{*rb}Y_u^{pt} - \frac{65}{27}\delta^{tb}\delta^{cd}Y_u^{*rs}Y_u^{pa}\left. + \frac{3}{2}T_2\delta^{sa}\delta^{tb}Y_d^{*rd}Y_d^{pc} + \frac{3}{2}\delta^{sa}\delta^{tb}Y_d^{pc}(Y_d^\dagger Y_d Y_d^\dagger)^{rd} + \frac{3}{2}\delta^{sa}\delta^{tb}Y_d^{*rd}(Y_d Y_d^\dagger Y_d)^{pc}\right. \\
& + \frac{487}{243}\delta^{pr}\delta^{sa}\delta^{tb}\delta^{cd}g_Y^2g_s^2 + \frac{9}{4}\delta^{tb}Y_u^{*rs}Y_d^{pc}(Y_d^\dagger Y_u)^{da} + \frac{9}{4}\delta^{sa}Y_d^{*rd}Y_u^{pt}(Y_u^\dagger Y_d)^{bc} - \frac{1}{2}\delta^{sa}\delta^{tb}Y_d^{pc}(Y_u^\dagger Y_u Y_d^\dagger)^{rd} - \frac{1}{2}\delta^{sa}\delta^{tb}Y_d^{*rd}(Y_u Y_u^\dagger Y_d)^{pc} \\
& - g_Y^2\left(\frac{26}{81}\delta^{sa}\delta^{cd}Y_u^{*rb}Y_u^{pt} + \frac{26}{81}\delta^{tb}\delta^{cd}Y_u^{*rs}Y_u^{pa} + \frac{383}{72}\delta^{sa}\delta^{tb}Y_d^{*rd}Y_d^{pc}\right) - \frac{5}{4}\delta^{tb}Y_d^{*rd}Y_d^{pc}(Y_u^\dagger Y_u)^{sa} - \frac{5}{4}\delta^{sa}Y_d^{*rd}Y_d^{pc}(Y_u^\dagger Y_u)^{bt} \\
& - \frac{33}{8}\delta^{sa}\delta^{tb}g_L^2Y_d^{*rd}Y_d^{pc}\left\}C_{ud}^{(\times)abcd} + \left\{\frac{2}{9}\delta^{rd}\delta^{st}g_s^2Y_e^{*ab}Y_d^{pc} + \frac{1}{4}\delta^{rd}Y_e^{*ab}Y_u^{pt}(Y_u^\dagger Y_d)^{sc}\right\}C_{ledq}^{abcd} + C_{ledq}^{*abcd}\left\{\frac{2}{9}\delta^{pd}\delta^{st}g_s^2Y_d^{*rc}Y_e^{ab}\right.
\end{aligned}$$

$$\begin{aligned}
& + \frac{1}{4} \delta^{pd} Y_u^{*rs} Y_e^{ab} (Y_d^\dagger Y_u)^{ct} \Bigg\} + \left\{ \frac{1}{8} \delta^{pa} Y_u^{*rs} Y_u^{*cb} (Y_d^\dagger Y_u)^{dt} + \frac{1}{8} \delta^{pa} Y_d^{*rd} Y_u^{*cs} (Y_u^\dagger Y_u)^{bt} + \frac{1}{8} \delta^{tb} Y_d^{*ad} Y_u^{*rs} (Y_d Y_d^\dagger)^{pc} + \frac{5}{8} \delta^{tb} Y_d^{*rd} Y_u^{*cs} (Y_u Y_u^\dagger)^{pa} \right. \\
& + \frac{3}{4} Y_d^{*ad} Y_u^{*rs} Y_u^{*cb} Y_u^{pt} + \frac{3}{4} \delta^{pc} Y_u^{*rb} Y_u^{*as} (Y_d^\dagger Y_u)^{dt} + \frac{3}{4} \delta^{pc} Y_u^{*rs} Y_u^{*ab} (Y_d^\dagger Y_u)^{dt} + \frac{3}{4} \delta^{tb} Y_d^{*cd} Y_u^{*rs} (Y_d Y_d^\dagger)^{pa} + g_L^2 \left( \frac{9}{4} \delta^{pa} \delta^{tb} Y_d^{*rd} Y_u^{*cs} \right. \\
& - \frac{15}{16} \delta^{pc} \delta^{tb} Y_d^{*ad} Y_u^{*rs} - \frac{9}{2} \delta^{pa} \delta^{tb} Y_d^{*cd} Y_u^{*rs} \Big) + g_Y^2 \left( \frac{17}{12} \delta^{pa} \delta^{tb} Y_d^{*rd} Y_u^{*cs} - \frac{23}{48} \delta^{pc} \delta^{tb} Y_d^{*ad} Y_u^{*rs} - \frac{8}{3} \delta^{pa} \delta^{tb} Y_d^{*cd} Y_u^{*rs} \right) + g_s^2 \left( \frac{2}{9} \delta^{pr} \delta^{tb} Y_d^{*ad} Y_u^{*cs} \right. \\
& + \frac{2}{3} \delta^{pa} \delta^{st} Y_d^{*cd} Y_u^{*rb} + \frac{2}{3} \delta^{pc} \delta^{st} Y_d^{*rd} Y_u^{*ab} + \frac{4}{3} \delta^{pr} \delta^{tb} Y_d^{*cd} Y_u^{*as} + \frac{33}{4} \delta^{pc} \delta^{tb} Y_d^{*rd} Y_u^{*as} + 10 \delta^{pa} \delta^{tb} Y_d^{*rd} Y_u^{*cs} - \frac{1}{18} \delta^{pa} \delta^{st} Y_d^{*rd} Y_u^{*cb} \\
& - \frac{1}{18} \delta^{pc} \delta^{st} Y_d^{*ad} Y_u^{*rb} - 6 \delta^{pc} \delta^{tb} Y_d^{*ad} Y_u^{*rs} - 17 \delta^{pa} \delta^{tb} Y_d^{*cd} Y_u^{*rs} \Big) + \left( \frac{3}{4} \delta^{pc} \delta^{tb} Y_d^{*ad} Y_u^{*rs} + \frac{9}{2} \delta^{pa} \delta^{tb} Y_d^{*cd} Y_u^{*rs} \right) \text{Tr} [Y_u^\dagger Y_u] + \frac{9}{8} \delta^{pc} \delta^{tb} Y_u^{*rs} (Y_d^\dagger Y_d Y_d^\dagger)^{ad} \\
& + \frac{9}{2} Y_d^{*cd} Y_u^{*rs} Y_u^{*ab} Y_u^{pt} + \frac{27}{4} \delta^{pa} \delta^{tb} Y_u^{*rs} (Y_d^\dagger Y_d Y_d^\dagger)^{cd} - \frac{1}{4} \delta^{tb} Y_d^{*rd} Y_u^{*cs} (Y_d Y_d^\dagger)^{pa} - \frac{1}{2} Y_d^{*rd} Y_u^{*as} Y_u^{*cb} Y_u^{pt} - \frac{1}{2} \delta^{pa} \delta^{tb} Y_d^{*rd} (Y_d^\dagger Y_d Y_u^\dagger)^{cs} \\
& - \frac{1}{2} \delta^{pa} \delta^{tb} Y_d^{*rd} (Y_u^\dagger Y_u Y_u^\dagger)^{cs} - \frac{5}{8} \delta^{pc} \delta^{tb} Y_u^{*rs} (Y_u^\dagger Y_u Y_d^\dagger)^{ad} - T_2 \delta^{pa} \delta^{tb} Y_d^{*rd} Y_u^{*cs} - \delta^{pa} \delta^{tb} Y_u^{*cs} (Y_d^\dagger Y_d Y_d^\dagger)^{rd} - \frac{3}{2} Y_d^{*rd} Y_u^{*ab} Y_u^{*cs} Y_u^{pt} \\
& - \frac{9}{4} \delta^{pa} \delta^{tb} Y_u^{*rs} (Y_u^\dagger Y_u Y_d^\dagger)^{cd} \Bigg\} C_{quqd}^{(\parallel)abcd} + \left( C_{quqd}^{(\parallel)*} \right)^{abcd} \left\{ \frac{1}{8} \delta^{ra} Y_u^{pt} Y_u^{cb} (Y_u^\dagger Y_d)^{sd} + \frac{1}{8} \delta^{ra} Y_d^{pd} Y_u^{ct} (Y_u^\dagger Y_u)^{sb} + \frac{1}{8} \delta^{sb} Y_d^{ad} Y_u^{pt} (Y_d Y_d^\dagger)^{cr} + \frac{5}{8} \delta^{sb} Y_d^{pd} Y_u^{ct} (Y_u Y_u^\dagger)^{ar} \right. \\
& + \frac{3}{4} Y_u^{*rs} Y_d^{ad} Y_u^{pt} Y_u^{cb} + \frac{3}{4} \delta^{rc} Y_u^{pb} Y_u^{at} (Y_u^\dagger Y_d)^{sd} + \frac{3}{4} \delta^{rc} Y_u^{pt} Y_u^{ab} (Y_u^\dagger Y_d)^{sd} + \frac{3}{4} \delta^{sb} Y_d^{cd} Y_u^{pt} (Y_d Y_d^\dagger)^{ar} + g_L^2 \left( \frac{9}{4} \delta^{ra} \delta^{sb} Y_d^{pd} Y_u^{ct} - \frac{15}{16} \delta^{rc} \delta^{sb} Y_d^{ad} Y_u^{pt} - \frac{9}{2} \delta^{ra} \delta^{sb} Y_d^{cd} Y_u^{pt} \right) \\
& + g_Y^2 \left( \frac{17}{12} \delta^{ra} \delta^{sb} Y_d^{pd} Y_u^{ct} - \frac{23}{48} \delta^{rc} \delta^{sb} Y_d^{ad} Y_u^{pt} - \frac{8}{3} \delta^{ra} \delta^{sb} Y_d^{cd} Y_u^{pt} \right) + g_s^2 \left( \frac{2}{9} \delta^{pr} \delta^{sb} Y_d^{ad} Y_u^{ct} + \frac{2}{3} \delta^{ra} \delta^{st} Y_d^{cd} Y_u^{pb} + \frac{2}{3} \delta^{rc} \delta^{st} Y_d^{pd} Y_u^{ab} + \frac{4}{3} \delta^{pr} \delta^{sb} Y_d^{cd} Y_u^{at} \right. \\
& + \frac{33}{4} \delta^{rc} \delta^{sb} Y_d^{pd} Y_u^{at} + 10 \delta^{ra} \delta^{sb} Y_d^{pd} Y_u^{ct} - \frac{1}{18} \delta^{ra} \delta^{st} Y_d^{pd} Y_u^{cb} - \frac{1}{18} \delta^{rc} \delta^{st} Y_d^{ad} Y_u^{pb} - 6 \delta^{rc} \delta^{sb} Y_d^{ad} Y_u^{pt} - 17 \delta^{ra} \delta^{sb} Y_d^{cd} Y_u^{pt} \Big) + \left( \frac{3}{4} \delta^{rc} \delta^{sb} Y_d^{ad} Y_u^{pt} \right. \\
& + \frac{9}{2} \delta^{ra} \delta^{sb} Y_d^{cd} Y_u^{pt} \Big) \text{Tr} [Y_u^\dagger Y_u] + \frac{9}{8} \delta^{rc} \delta^{sb} Y_u^{pt} (Y_d Y_d^\dagger Y_d)^{ad} + \frac{9}{2} Y_u^{*rs} Y_d^{cd} Y_u^{pt} Y_u^{ab} + \frac{27}{4} \delta^{ra} \delta^{sb} Y_u^{pt} (Y_d Y_d^\dagger Y_d)^{cd} - \frac{1}{4} \delta^{sb} Y_d^{pd} Y_u^{ct} (Y_d Y_d^\dagger)^{ar} - \frac{1}{2} Y_u^{*rs} Y_d^{pd} Y_u^{at} Y_u^{cb} \\
& - \frac{1}{2} \delta^{ra} \delta^{sb} Y_d^{pd} (Y_d Y_d^\dagger Y_u)^{ct} - \frac{1}{2} \delta^{ra} \delta^{sb} Y_d^{pd} (Y_u Y_u^\dagger Y_u)^{ct} - \frac{5}{8} \delta^{rc} \delta^{sb} Y_u^{pt} (Y_u Y_u^\dagger Y_d)^{ad} - T_2 \delta^{ra} \delta^{sb} Y_d^{pd} Y_u^{ct} - \delta^{ra} \delta^{sb} Y_u^{ct} (Y_d Y_d^\dagger Y_d)^{pd} - \frac{3}{2} Y_u^{*rs} Y_d^{pd} Y_u^{ab} Y_u^{ct} \\
& - \frac{9}{4} \delta^{ra} \delta^{sb} Y_u^{pt} (Y_u Y_u^\dagger Y_d)^{cd} \Bigg\} + \left\{ \frac{1}{4} \delta^{pc} Y_u^{*rs} Y_u^{*ab} (Y_d^\dagger Y_u)^{dt} + \frac{1}{4} \delta^{tb} Y_d^{*cd} Y_u^{*rs} (Y_d Y_d^\dagger)^{pa} + \frac{3}{8} \delta^{pa} Y_u^{*rs} Y_u^{*cb} (Y_d^\dagger Y_u)^{dt} + \frac{3}{8} \delta^{tb} Y_d^{*ad} Y_u^{*rs} (Y_d Y_d^\dagger)^{pc} \right. \\
& + \frac{3}{4} \delta^{tb} Y_d^{*rd} Y_u^{*as} (Y_u Y_u^\dagger)^{pc} + g_Y^2 \left( \frac{47}{144} \delta^{pc} \delta^{tb} Y_d^{*rd} Y_u^{*as} - \frac{8}{9} \delta^{pa} \delta^{tb} Y_d^{*cd} Y_u^{*rs} - \frac{23}{16} \delta^{pc} \delta^{tb} Y_d^{*ad} Y_u^{*rs} \right) + g_s^2 \left( \frac{1}{3} \delta^{pa} \delta^{st} Y_d^{*rd} Y_u^{*cb} + \frac{1}{3} \delta^{pc} \delta^{st} Y_d^{*ad} Y_u^{*rb} \right. \\
& + \frac{7}{18} \delta^{pa} \delta^{st} Y_d^{*cd} Y_u^{*rb} + \frac{7}{18} \delta^{pc} \delta^{st} Y_d^{*rd} Y_u^{*ab} + \frac{4}{9} \delta^{pr} \delta^{tb} Y_d^{*cd} Y_u^{*as} + \frac{2}{3} \delta^{pr} \delta^{tb} Y_d^{*ad} Y_u^{*cs} + 7 \delta^{pa} \delta^{tb} Y_d^{*rd} Y_u^{*cs} + \frac{119}{12} \delta^{pc} \delta^{tb} Y_d^{*rd} Y_u^{*as} \\
& - \frac{17}{3} \delta^{pa} \delta^{tb} Y_d^{*cd} Y_u^{*rs} - \frac{45}{2} \delta^{pc} \delta^{tb} Y_d^{*ad} Y_u^{*rs} \Big) + \left( \frac{3}{2} \delta^{pa} \delta^{tb} Y_d^{*cd} Y_u^{*rs} + \frac{9}{4} \delta^{pc} \delta^{tb} Y_d^{*ad} Y_u^{*rs} \right) \text{Tr} [Y_u^\dagger Y_u] + \frac{3}{2} Y_d^{*cd} Y_u^{*rs} Y_u^{*ab} Y_u^{pt} + \frac{9}{4} Y_d^{*ad} Y_u^{*rs} Y_u^{*cb} Y_u^{pt} \\
& + \frac{9}{4} \delta^{pa} \delta^{tb} Y_u^{*rs} (Y_d^\dagger Y_d Y_d^\dagger)^{cd} + \frac{27}{8} \delta^{pc} \delta^{tb} Y_u^{*rs} (Y_d^\dagger Y_d Y_d^\dagger)^{ad} - \frac{1}{8} \delta^{pa} Y_u^{*rb} Y_u^{*cs} (Y_d^\dagger Y_u)^{dt} - \frac{1}{8} \delta^{pc} \delta^{tb} Y_d^{*rd} (Y_u^\dagger Y_u Y_u^\dagger)^{as} - \frac{1}{4} T_2 \delta^{pc} \delta^{tb} Y_d^{*rd} Y_u^{*as}
\end{aligned}$$

$$\begin{aligned}
& -\frac{1}{4}\delta^{pc}\delta^{tb}Y_u^{*as}(Y_d^\dagger Y_d Y_d^\dagger)^{rd} - \frac{1}{4}\delta^{pc}\delta^{tb}Y_u^{*as}(Y_u^\dagger Y_u Y_d^\dagger)^{rd} - \frac{3}{8}\delta^{pc}\delta^{tb}Y_d^{*rd}(Y_d^\dagger Y_d Y_u^\dagger)^{as} - \frac{1}{2}Y_d^{*rd}Y_u^{*ab}Y_u^{*cs}Y_u^{pt} - \frac{3}{4}\delta^{pa}\delta^{tb}Y_u^{*rs}(Y_u^\dagger Y_u Y_d^\dagger)^{cd} \\
& - \frac{7}{8}\delta^{pc}Y_d^{*rd}Y_u^{*as}(Y_u^\dagger Y_u)^{bt} - g_L^2\left(\frac{15}{16}\delta^{pc}\delta^{tb}Y_d^{*rd}Y_u^{*as} + \frac{3}{2}\delta^{pa}\delta^{tb}Y_d^{*cd}Y_u^{*rs} + \frac{45}{16}\delta^{pc}\delta^{tb}Y_d^{*ad}Y_u^{*rs}\right) - \frac{5}{4}\delta^{tb}Y_d^{*rd}Y_u^{*as}(Y_d Y_d^\dagger)^{pc} - \frac{3}{2}Y_d^{*rd}Y_u^{*as}Y_u^{*cb}Y_u^{pt} \\
& - \frac{15}{8}\delta^{pc}\delta^{tb}Y_u^{*rs}(Y_u^\dagger Y_u Y_d^\dagger)^{ad} \Big\} C_{quqd}^{(\times)abcd} + \left(C_{quqd}^{(\times)*}\right)^{abcd} \Big\{ \frac{1}{4}\delta^{rc}Y_u^{pt}Y_u^{ab}(Y_u^\dagger Y_d)^{sd} + \frac{1}{4}\delta^{sb}Y_d^{cd}Y_u^{pt}(Y_d Y_d^\dagger)^{ar} + \frac{3}{8}\delta^{ra}Y_u^{pt}Y_u^{cb}(Y_u^\dagger Y_d)^{sd} + \frac{3}{8}\delta^{sb}Y_d^{ad}Y_u^{pt}(Y_d Y_d^\dagger)^{cr} \\
& + \frac{3}{4}\delta^{sb}Y_d^{pd}Y_u^{at}(Y_u Y_u^\dagger)^{cr} + g_Y^2\left(\frac{47}{144}\delta^{rc}\delta^{sb}Y_d^{pd}Y_u^{at} - \frac{8}{9}\delta^{ra}\delta^{sb}Y_d^{cd}Y_u^{pt} - \frac{23}{16}\delta^{rc}\delta^{sb}Y_d^{ad}Y_u^{pt}\right) + g_s^2\left(\frac{1}{3}\delta^{ra}\delta^{st}Y_d^{pd}Y_u^{cb} + \frac{1}{3}\delta^{rc}\delta^{st}Y_d^{ad}Y_u^{pb} + \frac{7}{18}\delta^{ra}\delta^{st}Y_d^{cd}Y_u^{pb} \right. \\
& + \frac{7}{18}\delta^{rc}\delta^{st}Y_d^{pd}Y_u^{ab} + \frac{4}{9}\delta^{pr}\delta^{sb}Y_d^{cd}Y_u^{at} + \frac{2}{3}\delta^{pr}\delta^{sb}Y_d^{ad}Y_u^{ct} + 7\delta^{ra}\delta^{sb}Y_d^{pd}Y_u^{ct} + \frac{119}{12}\delta^{rc}\delta^{sb}Y_d^{pd}Y_u^{at} - \frac{17}{3}\delta^{ra}\delta^{sb}Y_d^{cd}Y_u^{pt} - \frac{45}{2}\delta^{rc}\delta^{sb}Y_d^{ad}Y_u^{pt} \Big) \\
& + \left(\frac{3}{2}\delta^{ra}\delta^{sb}Y_d^{cd}Y_u^{pt} + \frac{9}{4}\delta^{rc}\delta^{sb}Y_d^{ad}Y_u^{pt}\right) \text{Tr}[Y_u^\dagger Y_u] + \frac{3}{2}Y_u^{*rs}Y_d^{cd}Y_u^{pt}Y_u^{ab} + \frac{9}{4}Y_u^{*rs}Y_d^{ad}Y_u^{pt}Y_u^{cb} + \frac{9}{4}\delta^{ra}\delta^{sb}Y_u^{pt}(Y_d Y_d^\dagger Y_d)^{cd} + \frac{27}{8}\delta^{rc}\delta^{sb}Y_u^{pt}(Y_d Y_d^\dagger Y_d)^{ad} \\
& - \frac{1}{8}\delta^{ra}Y_u^{pb}Y_u^{ct}(Y_u^\dagger Y_d)^{sd} - \frac{1}{8}\delta^{rc}\delta^{sb}Y_d^{pd}(Y_u Y_u^\dagger Y_u)^{at} - \frac{1}{4}T_2\delta^{rc}\delta^{sb}Y_d^{pd}Y_u^{at} - \frac{1}{4}\delta^{rc}\delta^{sb}Y_u^{at}(Y_d Y_d^\dagger Y_d)^{pd} - \frac{1}{4}\delta^{rc}\delta^{sb}Y_u^{at}(Y_u Y_u^\dagger Y_d)^{pd} \\
& - \frac{3}{8}\delta^{rc}\delta^{sb}Y_d^{pd}(Y_d Y_d^\dagger Y_u)^{at} - \frac{1}{2}Y_u^{*rs}Y_d^{pd}Y_u^{ab}Y_u^{ct} - \frac{3}{4}\delta^{ra}\delta^{sb}Y_u^{pt}(Y_u Y_u^\dagger Y_d)^{cd} - \frac{7}{8}\delta^{rc}Y_d^{pd}Y_u^{at}(Y_u^\dagger Y_u)^{sb} - g_L^2\left(\frac{15}{16}\delta^{rc}\delta^{sb}Y_d^{pd}Y_u^{at} + \frac{3}{2}\delta^{ra}\delta^{sb}Y_d^{cd}Y_u^{pt} \right. \\
& + \frac{45}{16}\delta^{rc}\delta^{sb}Y_d^{ad}Y_u^{pt} \Big) - \frac{5}{4}\delta^{sb}Y_d^{pd}Y_u^{at}(Y_d Y_d^\dagger)^{cr} - \frac{3}{2}Y_u^{*rs}Y_d^{pd}Y_u^{at}Y_u^{cb} - \frac{15}{8}\delta^{rc}\delta^{sb}Y_u^{pt}(Y_u Y_u^\dagger Y_d)^{ad} \Big\} + \left\{ \frac{3}{2}\delta^{pc}\delta^{td}g_L^2Y_e^{*ab}Y_u^{*rs} + \frac{11}{3}\delta^{pc}\delta^{td}g_Y^2Y_e^{*ab}Y_u^{*rs} \right. \\
& - \frac{1}{4}\delta^{td}Y_e^{*ab}Y_u^{*rs}(Y_d Y_d^\dagger)^{pc} - g_s^2\left(\frac{2}{9}\delta^{pc}\delta^{st}Y_e^{*ab}Y_u^{*rd} + \frac{4}{9}\delta^{pr}\delta^{td}Y_e^{*ab}Y_u^{*cs} + \delta^{pc}\delta^{td}Y_e^{*ab}Y_u^{*rs}\right) - \frac{3}{2}Y_e^{*ab}Y_u^{*rs}Y_u^{*cd}Y_u^{pt} - \frac{3}{2}\delta^{pc}\delta^{td}Y_e^{*ab}Y_u^{*rs} \text{Tr}[Y_u^\dagger Y_u] \\
& - \frac{9}{4}\delta^{pc}\delta^{td}Y_u^{*rs}(Y_e^\dagger Y_e Y_e^\dagger)^{ab} \Big\} C_{lequ}^{abcd} + C_{lequ}^{*abcd} \Big\{ \frac{3}{2}\delta^{rc}\delta^{sd}g_L^2Y_e^{ab}Y_u^{pt} + \frac{11}{3}\delta^{rc}\delta^{sd}g_Y^2Y_e^{ab}Y_u^{pt} - \frac{1}{4}\delta^{sd}Y_e^{ab}Y_u^{pt}(Y_d Y_d^\dagger)^{cr} - g_s^2\left(\frac{2}{9}\delta^{rc}\delta^{st}Y_e^{ab}Y_u^{pd} \right. \\
& + \frac{4}{9}\delta^{pr}\delta^{sd}Y_e^{ab}Y_u^{ct} + \delta^{rc}\delta^{sd}Y_e^{ab}Y_u^{pt} \Big) - \frac{3}{2}Y_u^{*rs}Y_e^{ab}Y_u^{pt}Y_u^{cd} - \frac{3}{2}\delta^{rc}\delta^{sd}Y_e^{ab}Y_u^{pt} \text{Tr}[Y_u^\dagger Y_u] - \frac{9}{4}\delta^{rc}\delta^{sd}Y_u^{pt}(Y_e Y_e^\dagger Y_e)^{ab} \Big\} + \left\{ \frac{1}{8}\delta^{tb}Y_e^{*ad}Y_u^{*rs}(Y_d Y_d^\dagger)^{pc} \right. \\
& + \frac{3}{4}Y_e^{*ad}Y_u^{*rs}Y_u^{*cb}Y_u^{pt} + \frac{3}{4}\delta^{pc}\delta^{tb}Y_e^{*ad}Y_u^{*rs} \text{Tr}[Y_u^\dagger Y_u] + g_s^2\left(\frac{1}{9}\delta^{pc}\delta^{st}Y_e^{*ad}Y_u^{*rb} + \frac{2}{9}\delta^{pr}\delta^{tb}Y_e^{*ad}Y_u^{*cs} - \frac{11}{6}\delta^{pc}\delta^{tb}Y_e^{*ad}Y_u^{*rs}\right) \\
& + \frac{9}{8}\delta^{pc}\delta^{tb}Y_u^{*rs}(Y_e^\dagger Y_e Y_e^\dagger)^{ad} - \frac{15}{16}\delta^{pc}\delta^{tb}g_L^2Y_e^{*ad}Y_u^{*rs} - \frac{589}{144}\delta^{pc}\delta^{tb}g_Y^2Y_e^{*ad}Y_u^{*rs} \Big\} C_{luqe}^{abcd} + C_{luqe}^{*abcd} \Big\{ \frac{1}{8}\delta^{sb}Y_e^{ad}Y_u^{pt}(Y_d Y_d^\dagger)^{cr} + \frac{3}{4}Y_u^{*rs}Y_e^{ad}Y_u^{pt}Y_u^{cb} \\
& + \frac{3}{4}\delta^{rc}\delta^{sb}Y_e^{ad}Y_u^{pt} \text{Tr}[Y_u^\dagger Y_u] + g_s^2\left(\frac{1}{9}\delta^{rc}\delta^{st}Y_e^{ad}Y_u^{pb} + \frac{2}{9}\delta^{pr}\delta^{sb}Y_e^{ad}Y_u^{ct} - \frac{11}{6}\delta^{rc}\delta^{sb}Y_e^{ad}Y_u^{pt}\right) + \frac{9}{8}\delta^{rc}\delta^{sb}Y_u^{pt}(Y_e Y_e^\dagger Y_e)^{ad} - \frac{15}{16}\delta^{rc}\delta^{sb}g_L^2Y_e^{ad}Y_u^{pt} \\
& - \frac{589}{144}\delta^{rc}\delta^{sb}g_Y^2Y_e^{ad}Y_u^{pt} \Big\} + \left\{ g_L^2\left(\frac{5}{3}\delta^{pa}\delta^{bc}Y_u^{*rs}Y_u^{dt} + \frac{5}{3}\delta^{rd}\delta^{bc}Y_u^{*as}Y_u^{pt} + \frac{33}{4}\delta^{pa}\delta^{rd}Y_u^{*cs}Y_u^{bt}\right) + g_Y^2\left(\frac{17}{81}\delta^{pa}\delta^{bc}Y_u^{*rs}Y_u^{dt} + \frac{17}{81}\delta^{rd}\delta^{bc}Y_u^{*as}Y_u^{pt} \right. \right. \\
& \left. \left. - \frac{32}{27}\delta^{pa}\delta^{cd}Y_u^{*rs}Y_u^{bt} - \frac{32}{27}\delta^{rb}\delta^{cd}Y_u^{*as}Y_u^{pt} - \frac{125}{36}\delta^{pa}\delta^{rd}Y_u^{*cs}Y_u^{bt}\right) + g_s^4\left(\frac{8}{9}\delta^{pr}\delta^{st}\delta^{ad}\delta^{bc} + \frac{1592}{81}\delta^{pa}\delta^{rd}\delta^{st}\delta^{bc} - \frac{28}{3}\delta^{pa}\delta^{rb}\delta^{st}\delta^{cd}\right) \right\}
\end{aligned}$$

$$\begin{aligned}
& + g_Y^2 g_s^2 \left( \frac{724}{81} \delta^{pa} \delta^{rb} \delta^{st} \delta^{cd} - \frac{346}{243} \delta^{pa} \delta^{rd} \delta^{st} \delta^{bc} \right) + \delta^{rd} Y_u^{*cs} Y_u^{bt} (Y_d Y_d^\dagger)^{pa} + \delta^{pa} Y_u^{*cs} Y_u^{bt} (Y_d Y_d^\dagger)^{dr} + g_s^2 \left( \frac{4}{3} \delta^{pa} \delta^{rd} \delta^{bc} (Y_u^\dagger Y_u)^{st} + 20 \delta^{pa} \delta^{rb} Y_u^{*cs} Y_u^{dt} \right. \\
& - \frac{34}{27} \delta^{pa} \delta^{bc} Y_u^{*rs} Y_u^{dt} - \frac{34}{27} \delta^{rd} \delta^{bc} Y_u^{*as} Y_u^{pt} - \frac{4}{3} \delta^{pr} \delta^{bc} Y_u^{*as} Y_u^{dt} - \frac{10}{3} \delta^{pa} \delta^{rd} \delta^{st} (Y_d Y_d^\dagger)^{bc} - \frac{10}{3} \delta^{pa} \delta^{rd} \delta^{st} (Y_u Y_u^\dagger)^{bc} - \frac{14}{3} \delta^{pa} \delta^{rd} Y_u^{*cs} Y_u^{bt} \Big) \\
& + \frac{3}{2} \delta^{pa} Y_u^{*rs} Y_u^{dt} (Y_d Y_d^\dagger)^{bc} + \frac{3}{2} \delta^{rb} Y_u^{*cs} Y_u^{pt} (Y_d Y_d^\dagger)^{da} + \frac{5}{2} \delta^{pa} \delta^{rd} Y_u^{bt} (Y_u^\dagger Y_u Y_u^\dagger)^{cs} + \frac{5}{2} \delta^{pa} \delta^{rd} Y_u^{*cs} (Y_u Y_u^\dagger Y_u)^{bt} + 5 T_2 \delta^{pa} \delta^{rd} Y_u^{*cs} Y_u^{bt} \\
& - \frac{1}{2} \delta^{pa} \delta^{rd} Y_u^{bt} (Y_d^\dagger Y_d Y_u^\dagger)^{cs} - \frac{1}{2} \delta^{pa} \delta^{rd} Y_u^{*cs} (Y_d Y_d^\dagger Y_u)^{bt} - \delta^{rb} Y_u^{*as} Y_u^{dt} (Y_u Y_u^\dagger)^{pc} - \delta^{pa} Y_u^{*cs} Y_u^{bt} (Y_u Y_u^\dagger)^{dr} - 6 \delta^{pa} Y_u^{*rs} Y_u^{bt} (Y_u Y_u^\dagger)^{dc} \\
& - 6 \delta^{rb} Y_u^{*as} Y_u^{pt} (Y_u Y_u^\dagger)^{dc} - \frac{58}{9} \delta^{pa} \delta^{rd} \delta^{st} \delta^{bc} g_s^2 g_L^2 \Big\} C_{qq}^{(\parallel)abcd} + \left\{ g_Y^2 \left( \frac{34}{81} \delta^{pa} \delta^{bc} Y_u^{*rs} Y_u^{dt} + \frac{34}{81} \delta^{rd} \delta^{bc} Y_u^{*as} Y_u^{pt} - \frac{16}{27} \delta^{pa} \delta^{cd} Y_u^{*rs} Y_u^{bt} \right. \right. \\
& - \frac{16}{27} \delta^{rb} \delta^{cd} Y_u^{*as} Y_u^{pt} - \frac{125}{18} \delta^{pa} \delta^{rd} Y_u^{*cs} Y_u^{bt} \Big) + g_L^2 \left( 8 \delta^{pa} \delta^{cd} Y_u^{*rs} Y_u^{bt} + 8 \delta^{rb} \delta^{cd} Y_u^{*as} Y_u^{pt} - \frac{69}{2} \delta^{pa} \delta^{rd} Y_u^{*cs} Y_u^{bt} \right) + g_s^2 g_L^2 \left( 6 \delta^{pa} \delta^{rd} \delta^{st} \delta^{bc} \right. \\
& - \frac{34}{3} \delta^{pa} \delta^{rb} \delta^{st} \delta^{cd} \Big) + g_s^4 \left( \frac{16}{9} \delta^{pr} \delta^{st} \delta^{ad} \delta^{bc} + \frac{3184}{81} \delta^{pa} \delta^{rd} \delta^{st} \delta^{bc} - \frac{14}{3} \delta^{pa} \delta^{rb} \delta^{st} \delta^{cd} \right) + g_Y^2 g_s^2 \left( \frac{362}{81} \delta^{pa} \delta^{rb} \delta^{st} \delta^{cd} - \frac{692}{243} \delta^{pa} \delta^{rd} \delta^{st} \delta^{bc} \right) \\
& + g_s^2 \left( \frac{8}{3} \delta^{pa} \delta^{rd} \delta^{bc} (Y_u^\dagger Y_u)^{st} + 10 \delta^{pa} \delta^{rb} Y_u^{*cs} Y_u^{dt} - \frac{68}{27} \delta^{pa} \delta^{bc} Y_u^{*rs} Y_u^{dt} - \frac{68}{27} \delta^{rd} \delta^{bc} Y_u^{*as} Y_u^{pt} - \frac{8}{3} \delta^{pr} \delta^{bc} Y_u^{*as} Y_u^{dt} - \frac{20}{3} \delta^{pa} \delta^{rd} \delta^{st} (Y_d Y_d^\dagger)^{bc} \right. \\
& - \frac{20}{3} \delta^{pa} \delta^{rd} \delta^{st} (Y_u Y_u^\dagger)^{bc} - \frac{28}{3} \delta^{pa} \delta^{rd} Y_u^{*cs} Y_u^{bt} \Big) + 5 \delta^{pa} \delta^{rd} Y_u^{bt} (Y_u^\dagger Y_u Y_u^\dagger)^{cs} + 5 \delta^{pa} \delta^{rd} Y_u^{*cs} (Y_u Y_u^\dagger Y_u)^{bt} + 10 T_2 \delta^{pa} \delta^{rd} Y_u^{*cs} Y_u^{bt} \\
& - \frac{1}{2} \delta^{rb} Y_u^{*as} Y_u^{dt} (Y_u Y_u^\dagger)^{pc} - \frac{1}{2} \delta^{pa} Y_u^{*cs} Y_u^{bt} (Y_u Y_u^\dagger)^{dr} - \delta^{rd} Y_u^{*cs} Y_u^{bt} (Y_d Y_d^\dagger)^{pa} - \delta^{pa} Y_u^{*cs} Y_u^{bt} (Y_d Y_d^\dagger)^{dr} - \delta^{pa} \delta^{rd} Y_u^{bt} (Y_d^\dagger Y_d Y_u^\dagger)^{cs} - \delta^{pa} \delta^{rd} Y_u^{*cs} (Y_d Y_d^\dagger Y_u)^{bt} \\
& - \frac{3}{2} \delta^{pa} Y_u^{*rs} Y_u^{dt} (Y_d Y_d^\dagger)^{bc} - \frac{3}{2} \delta^{rb} Y_u^{*cs} Y_u^{pt} (Y_d Y_d^\dagger)^{da} - 12 \delta^{pa} Y_u^{*rs} Y_u^{bt} (Y_u Y_u^\dagger)^{dc} - 12 \delta^{rb} Y_u^{*as} Y_u^{pt} (Y_u Y_u^\dagger)^{dc} \Big\} C_{qq}^{(\times)abcd} + \left\{ g_Y^2 \left( \frac{16}{27} \delta^{pc} \delta^{ab} Y_u^{*rs} Y_u^{dt} \right. \right. \\
& + \frac{16}{27} \delta^{rd} \delta^{ab} Y_u^{*cs} Y_u^{pt} \Big) - \frac{362}{81} \delta^{pc} \delta^{rd} \delta^{st} \delta^{ab} g_Y^2 g_s^2 \Big\} C_{\ell q}^{(\parallel)abcd} + \left\{ g_Y^2 \left( \frac{8}{27} \delta^{pc} \delta^{ab} Y_u^{*rs} Y_u^{dt} + \frac{8}{27} \delta^{rd} \delta^{ab} Y_u^{*cs} Y_u^{pt} \right) + g_L^2 \left( \frac{4}{3} \delta^{pc} \delta^{ab} Y_u^{*rs} Y_u^{dt} + \frac{4}{3} \delta^{rd} \delta^{ab} Y_u^{*cs} Y_u^{pt} \right) \right. \\
& \left. - \frac{17}{9} \delta^{pc} \delta^{rd} \delta^{st} \delta^{ab} g_s^2 g_L^2 - \frac{181}{81} \delta^{pc} \delta^{rd} \delta^{st} \delta^{ab} g_Y^2 g_s^2 \right\} C_{\ell q}^{(\times)abcd}, \tag{10.12}
\end{aligned}$$

## 10.7 $C_{qd}^{(\parallel)}$

$$\begin{aligned}
\beta_{C_{qd}^{(\parallel)prst}}^{(1)} & = \left\{ 2 \delta^{pa} \delta^{rb} (Y_d^\dagger Y_d)^{st} - \frac{2}{9} \delta^{pa} \delta^{rb} \delta^{st} g_Y^2 \right\} C_{Hq}^{(\parallel)ab} + \left\{ \delta^{pa} \delta^{rb} (Y_d^\dagger Y_d)^{st} - \frac{1}{9} \delta^{pa} \delta^{rb} \delta^{st} g_Y^2 \right\} C_{Hq}^{(\times)ab} + \left\{ \frac{1}{9} \delta^{pr} \delta^{sa} \delta^{tb} g_Y^2 + \delta^{sa} \delta^{tb} (Y_u Y_u^\dagger)^{pr} \right. \\
& \left. - \delta^{sa} \delta^{tb} (Y_d Y_d^\dagger)^{pr} \right\} C_{Hd}^{ab} - \frac{2}{9} \delta^{pr} \delta^{sc} \delta^{td} \delta^{ab} g_Y^2 C_{\ell d}^{abcd} + \frac{4}{9} \delta^{pa} \delta^{rb} \delta^{st} \delta^{cd} g_Y^2 C_{qe}^{abcd} - \frac{8}{9} \delta^{pa} \delta^{rb} \delta^{st} \delta^{cd} g_Y^2 C_{qu}^{abcd} - \left\{ \frac{2}{9} \delta^{pa} \delta^{rb} \delta^{st} \delta^{cd} g_s^2 \right. \\
& \left. + \frac{8}{27} \delta^{pa} \delta^{rb} \delta^{st} \delta^{cd} g_Y^2 \right\} C_{qu}^{(\times)abcd} + \left\{ \frac{2}{9} g_Y^2 \left( \delta^{pr} \delta^{sc} \delta^{td} \delta^{ab} + 2 \delta^{pa} \delta^{rb} \delta^{st} \delta^{cd} + 3 \delta^{pa} \delta^{rb} \delta^{sc} \delta^{td} \right) + \frac{1}{2} \left( \delta^{rb} \delta^{sc} \delta^{td} (Y_d Y_d^\dagger)^{pa} + \delta^{pa} \delta^{sc} \delta^{td} (Y_d Y_d^\dagger)^{br} \right. \right.
\end{aligned}$$

$$\begin{aligned}
& + \delta^{rb} \delta^{sc} \delta^{td} (Y_u Y_u^\dagger)^{pa} + \delta^{pa} \delta^{sc} \delta^{td} (Y_u Y_u^\dagger)^{br} + 2\delta^{pa} \delta^{rb} \delta^{td} (Y_d^\dagger Y_d)^{sc} + 2\delta^{pa} \delta^{rb} \delta^{sc} (Y_d^\dagger Y_d)^{dt} + 2\delta^{pa} \delta^{rb} \delta^{sc} \delta^{td} g_s^2 \Big\} C_{qd}^{(\parallel)abcd} + \left\{ \frac{2}{27} g_Y^2 \left( \delta^{pr} \delta^{sc} \delta^{td} \delta^{ab} \right. \right. \\
& + 2\delta^{pa} \delta^{rb} \delta^{st} \delta^{cd} \Big) + \delta^{pa} \delta^{sc} Y_d^{*rd} Y_d^{bt} + \delta^{rb} \delta^{td} Y_d^{*as} Y_d^{pc} - \frac{2}{9} g_s^2 \left( \delta^{pa} \delta^{rb} \delta^{st} \delta^{cd} + 2\delta^{pr} \delta^{sc} \delta^{td} \delta^{ab} \right) \Big\} C_{qd}^{(\times)abcd} - \left\{ \frac{4}{27} g_Y^2 \left( \delta^{pr} \delta^{sa} \delta^{td} \delta^{bc} + 3\delta^{pr} \delta^{sa} \delta^{tb} \delta^{cd} \right) \right. \\
& + \frac{4}{9} \delta^{pr} \delta^{sa} \delta^{td} \delta^{bc} g_s^2 + 2\delta^{sa} \delta^{tb} Y_d^{*rd} Y_d^{pc} \Big\} C_{dd}^{abcd} - \frac{2}{9} \delta^{pr} \delta^{sc} \delta^{td} \delta^{ab} g_Y^2 C_{ed}^{abcd} + \left\{ \frac{4}{9} \delta^{pr} \delta^{sc} \delta^{td} \delta^{ab} g_Y^2 - \delta^{sc} \delta^{td} Y_u^{*rb} Y_u^{pa} \right\} C_{ud}^{(\parallel)abcd} + \left\{ \frac{4}{27} \delta^{pr} \delta^{sc} \delta^{td} \delta^{ab} g_Y^2 \right. \\
& - \frac{2}{9} \delta^{pr} \delta^{sc} \delta^{td} \delta^{ab} g_s^2 \Big\} C_{ud}^{(\times)abcd} + \frac{1}{2} \delta^{pa} \delta^{td} Y_d^{*cs} Y_u^{*rb} C_{quqd}^{(\parallel)abcd} + \frac{1}{2} \delta^{ra} \delta^{sd} \left( C_{quqd}^{(\parallel)*} \right)^{abcd} Y_d^{ct} Y_u^{pb} + \delta^{pc} \delta^{td} Y_d^{*as} Y_u^{*rb} C_{quqd}^{(\times)abcd} + \delta^{rc} \delta^{sd} \left( C_{quqd}^{(\times)*} \right)^{abcd} Y_d^{at} Y_u^{pb} \\
& - \left\{ \frac{4}{27} g_Y^2 \left( \delta^{pa} \delta^{rd} \delta^{st} \delta^{bc} + 6\delta^{pa} \delta^{rb} \delta^{st} \delta^{cd} \right) + \frac{4}{9} \delta^{pa} \delta^{rd} \delta^{st} \delta^{bc} g_s^2 + 4\delta^{pa} \delta^{rb} Y_d^{*cs} Y_d^{dt} \right\} C_{qq}^{(\parallel)abcd} - \left\{ \frac{4}{27} g_Y^2 \left( 2\delta^{pa} \delta^{rd} \delta^{st} \delta^{bc} + 3\delta^{pa} \delta^{rb} \delta^{st} \delta^{cd} \right) \right. \\
& + \frac{8}{9} \delta^{pa} \delta^{rd} \delta^{st} \delta^{bc} g_s^2 + 2\delta^{pa} \delta^{rb} Y_d^{*cs} Y_d^{dt} \Big\} C_{qq}^{(\times)abcd} + \frac{4}{9} \delta^{pc} \delta^{rd} \delta^{st} \delta^{ab} g_Y^2 C_{\ell q}^{(\parallel)abcd} + \frac{2}{9} \delta^{pc} \delta^{rd} \delta^{st} \delta^{ab} g_Y^2 C_{\ell q}^{(\times)abcd}, \tag{10.13}
\end{aligned}$$

$$\begin{aligned}
\beta_{C_{qd}^{(\parallel)prst}}^{(2)} = & \left\{ g_Y^4 \left( \frac{5}{9} \delta^{st} (Y_d Y_d^\dagger)^{pr} + \frac{7}{9} \delta^{pr} (Y_d^\dagger Y_d)^{st} - \frac{1}{9} \delta^{st} (Y_u Y_u^\dagger)^{pr} \right) - \frac{4}{27} \delta^{pr} \delta^{st} g_Y^6 \right\} C_{HB} + g_s^4 \left\{ \frac{2}{3} \delta^{st} (Y_d Y_d^\dagger)^{pr} + \frac{2}{3} \delta^{st} (Y_u Y_u^\dagger)^{pr} + \frac{4}{3} \delta^{pr} (Y_d^\dagger Y_d)^{st} \right. \\
& + 12 Y_d^{*rs} Y_d^{pt} \Big\} C_{HG} + \left\{ g_Y^2 g_L^2 \left( \frac{1}{4} \delta^{pr} (Y_d^\dagger Y_d)^{st} + \frac{3}{4} \delta^{st} (Y_d Y_d^\dagger)^{pr} - \frac{3}{4} \delta^{st} (Y_u Y_u^\dagger)^{pr} \right) - \frac{1}{9} \delta^{pr} \delta^{st} g_Y^4 g_L^2 \right\} C_{HWB} - \left\{ \frac{10}{9} \delta^{pr} \delta^{st} g_Y^2 g_L^6 + \frac{10}{3} \delta^{pr} \delta^{st} g_s^2 g_L^6 \right\} C_W \\
& + \left\{ g_s^6 \left( \frac{3}{2} \delta^{st} (Y_d Y_d^\dagger)^{pr} + \frac{3}{2} \delta^{st} (Y_u Y_u^\dagger)^{pr} + 3\delta^{pr} (Y_d^\dagger Y_d)^{st} + 27 Y_d^{*rs} Y_d^{pt} \right) + \frac{434}{9} \delta^{pr} \delta^{st} g_s^8 - \frac{223}{27} \delta^{pr} \delta^{st} g_Y^2 g_s^6 \right\} C_G + \frac{2}{9} \delta^{pr} \delta^{st} g_Y^4 Y_e^{*ab} C_{eB}^{ab} \\
& + \frac{2}{9} \delta^{pr} \delta^{st} g_Y^4 C_{eB}^{*ab} Y_e^{ab} + \left\{ g_Y^4 \left( \frac{283}{162} \delta^{pa} \delta^{st} Y_u^{*rb} - \frac{10}{27} \delta^{pr} \delta^{st} Y_u^{*ab} \right) + g_Y^2 \left( \frac{2}{3} \delta^{st} Y_u^{*rb} (Y_u Y_u^\dagger)^{pa} + \frac{17}{6} \delta^{pa} Y_u^{*rb} (Y_d^\dagger Y_d)^{st} - \frac{1}{3} \delta^{st} Y_u^{*rb} (Y_d Y_d^\dagger)^{pa} \right) \right. \\
& + \frac{83}{27} \delta^{pa} \delta^{st} g_Y^2 g_s^2 Y_u^{*rb} \Big\} C_{uB}^{ab} + C_{uB}^{*ab} \left\{ g_Y^4 \left( \frac{283}{162} \delta^{ra} \delta^{st} Y_u^{pb} - \frac{10}{27} \delta^{pr} \delta^{st} Y_u^{ab} \right) + g_Y^2 \left( \frac{2}{3} \delta^{st} Y_u^{pb} (Y_u Y_u^\dagger)^{ar} + \frac{17}{6} \delta^{ra} Y_u^{pb} (Y_d^\dagger Y_d)^{st} - \frac{1}{3} \delta^{st} Y_u^{pb} (Y_d Y_d^\dagger)^{ar} \right) \right. \\
& + \frac{83}{27} \delta^{ra} \delta^{st} g_Y^2 g_s^2 Y_u^{pb} \Big\} + \left\{ \frac{1}{6} \delta^{pa} \delta^{st} g_s^2 g_L^2 Y_u^{*rb} + \frac{11}{36} \delta^{pa} \delta^{st} g_Y^2 g_L^2 Y_u^{*rb} + \frac{15}{4} \delta^{pa} g_L^2 Y_u^{*rb} (Y_d^\dagger Y_d)^{st} \right\} C_{uW}^{ab} + C_{uW}^{*ab} \left\{ \frac{1}{6} \delta^{ra} \delta^{st} g_s^2 g_L^2 Y_u^{pb} \right. \\
& + \frac{11}{36} \delta^{ra} \delta^{st} g_Y^2 g_L^2 Y_u^{pb} + \frac{15}{4} \delta^{ra} g_L^2 Y_u^{pb} (Y_d^\dagger Y_d)^{st} \Big\} + \left\{ g_s^4 \left( \frac{19}{27} \delta^{pa} \delta^{st} Y_u^{*rb} - \frac{4}{9} \delta^{pr} \delta^{st} Y_u^{*ab} \right) + g_s^2 \left( \frac{1}{3} \delta^{st} Y_u^{*rb} (Y_u Y_u^\dagger)^{pa} + Y_d^{*as} Y_u^{*rb} Y_d^{pt} \right) \right.
\end{aligned}$$

$$\begin{aligned}
& + \frac{17}{3} \delta^{pa} Y_u^{*rb} (Y_d^\dagger Y_d)^{st} - \frac{1}{6} \delta^{st} Y_u^{*rb} (Y_d Y_d^\dagger)^{pa} - \frac{3}{2} \delta^{pa} Y_d^{*rs} (Y_u^\dagger Y_d)^{bt} + \frac{190}{81} \delta^{pa} \delta^{st} g_Y^2 g_s^2 Y_u^{*rb} \Big\} C_{uG}^{ab} + C_{uG}^{*ab} \Big\{ g_s^4 \Big( \frac{19}{27} \delta^{ra} \delta^{st} Y_u^{pb} - \frac{4}{9} \delta^{pr} \delta^{st} Y_u^{ab} \Big) \\
& + g_s^2 \Big( \frac{1}{3} \delta^{st} Y_u^{pb} (Y_u Y_u^\dagger)^{ar} + Y_d^{*rs} Y_d^{at} Y_u^{pb} + \frac{17}{3} \delta^{ra} Y_u^{pb} (Y_d^\dagger Y_d)^{st} - \frac{1}{6} \delta^{st} Y_u^{pb} (Y_d Y_d^\dagger)^{ar} - \frac{3}{2} \delta^{ra} Y_d^{pt} (Y_d^\dagger Y_u)^{sb} \Big) + \frac{190}{81} \delta^{ra} \delta^{st} g_Y^2 g_s^2 Y_u^{pb} \Big\} + \Big\{ g_Y^4 \Big( \frac{2}{27} \delta^{pr} \delta^{st} Y_d^{*ab} \\
& + \frac{19}{81} \delta^{pr} \delta^{tb} Y_d^{*as} - \frac{71}{162} \delta^{pa} \delta^{st} Y_d^{*rb} \Big) + g_Y^2 g_s^2 \Big( \frac{59}{27} \delta^{pa} \delta^{st} Y_d^{*rb} - 2 \delta^{pa} \delta^{tb} Y_d^{*rs} - \frac{62}{27} \delta^{pr} \delta^{tb} Y_d^{*as} \Big) + g_Y^2 \Big( \frac{2}{3} \delta^{st} Y_d^{*rb} (Y_d Y_d^\dagger)^{pa} + \delta^{tb} Y_d^{*as} (Y_d Y_d^\dagger)^{pr} \\
& - \frac{1}{3} \delta^{pr} Y_d^{*as} (Y_d^\dagger Y_d)^{bt} - \frac{1}{3} \delta^{st} Y_d^{*rb} (Y_u Y_u^\dagger)^{pa} - \frac{1}{2} \delta^{pa} Y_d^{*rb} (Y_d^\dagger Y_d)^{st} - \frac{11}{3} \delta^{tb} Y_d^{*as} (Y_u Y_u^\dagger)^{pr} \Big) \Big\} C_{dB}^{ab} + C_{dB}^{*ab} \Big\{ g_Y^4 \Big( \frac{2}{27} \delta^{pr} \delta^{st} Y_d^{ab} + \frac{19}{81} \delta^{pr} \delta^{sb} Y_d^{at} \\
& - \frac{71}{162} \delta^{ra} \delta^{st} Y_d^{pb} \Big) + g_Y^2 g_s^2 \Big( \frac{59}{27} \delta^{ra} \delta^{st} Y_d^{pb} - 2 \delta^{ra} \delta^{sb} Y_d^{pt} - \frac{62}{27} \delta^{pr} \delta^{sb} Y_d^{at} \Big) + g_Y^2 \Big( \frac{2}{3} \delta^{st} Y_d^{pb} (Y_d Y_d^\dagger)^{ar} + \delta^{sb} Y_d^{at} (Y_d Y_d^\dagger)^{pr} - \frac{1}{3} \delta^{pr} Y_d^{at} (Y_d^\dagger Y_d)^{sb} \\
& - \frac{1}{3} \delta^{st} Y_d^{pb} (Y_u Y_u^\dagger)^{ar} - \frac{1}{2} \delta^{ra} Y_d^{pb} (Y_d^\dagger Y_d)^{st} - \frac{11}{3} \delta^{sb} Y_d^{at} (Y_u Y_u^\dagger)^{pr} \Big) \Big\} + \Big\{ g_s^2 g_L^2 \Big( \frac{1}{6} \delta^{pa} \delta^{st} Y_d^{*rb} + \frac{4}{3} \delta^{pr} \delta^{tb} Y_d^{*as} + 9 \delta^{pa} \delta^{tb} Y_d^{*rs} \Big) + g_L^2 \Big( 6 \delta^{tb} Y_d^{*as} (Y_u Y_u^\dagger)^{pr} \\
& - \frac{9}{4} \delta^{pa} Y_d^{*rb} (Y_d^\dagger Y_d)^{st} \Big) + \frac{9}{2} \delta^{pr} \delta^{tb} g_L^4 Y_d^{*as} - g_Y^2 g_L^2 \Big( \frac{1}{18} \delta^{pr} \delta^{tb} Y_d^{*as} + \frac{7}{36} \delta^{pa} \delta^{st} Y_d^{*rb} \Big) \Big\} C_{dW}^{ab} + C_{dW}^{*ab} \Big\{ g_s^2 g_L^2 \Big( \frac{1}{6} \delta^{ra} \delta^{st} Y_d^{pb} + \frac{4}{3} \delta^{pr} \delta^{sb} Y_d^{at} \\
& + 9 \delta^{ra} \delta^{sb} Y_d^{pt} \Big) + g_L^2 \Big( 6 \delta^{sb} Y_d^{at} (Y_u Y_u^\dagger)^{pr} - \frac{9}{4} \delta^{ra} Y_d^{pb} (Y_d^\dagger Y_d)^{st} \Big) + \frac{9}{2} \delta^{pr} \delta^{sb} g_L^4 Y_d^{at} - g_Y^2 g_L^2 \Big( \frac{1}{18} \delta^{pr} \delta^{sb} Y_d^{at} + \frac{7}{36} \delta^{ra} \delta^{st} Y_d^{pb} \Big) \Big\} + \Big\{ g_s^4 \Big( \frac{19}{27} \delta^{pa} \delta^{st} Y_d^{*rb} \\
& + \frac{38}{27} \delta^{pr} \delta^{tb} Y_d^{*as} - \frac{4}{9} \delta^{pr} \delta^{st} Y_d^{*ab} - 29 \delta^{pa} \delta^{tb} Y_d^{*rs} \Big) + g_s^2 \Big( \frac{1}{3} \delta^{pr} Y_d^{*as} (Y_d^\dagger Y_d)^{bt} + \frac{1}{3} \delta^{st} Y_d^{*rb} (Y_d Y_d^\dagger)^{pa} + \frac{3}{2} \delta^{pa} Y_d^{*rs} (Y_d^\dagger Y_d)^{bt} + 3 T_2 \delta^{pa} \delta^{tb} Y_d^{*rs} \\
& + 3 \delta^{tb} Y_d^{*rs} (Y_d Y_d^\dagger)^{pa} + \frac{17}{3} \delta^{tb} Y_d^{*as} (Y_u Y_u^\dagger)^{pr} - \frac{1}{6} \delta^{st} Y_d^{*rb} (Y_u Y_u^\dagger)^{pa} - 2 \delta^{pa} \delta^{tb} (Y_u^\dagger Y_u Y_d^\dagger)^{rs} - 3 \delta^{tb} Y_d^{*rs} (Y_u Y_u^\dagger)^{pa} - 4 \delta^{pa} Y_d^{*rb} (Y_d^\dagger Y_d)^{st} \\
& - 4 \delta^{tb} Y_d^{*as} (Y_d Y_d^\dagger)^{pr} \Big) - g_Y^2 g_s^2 \Big( \frac{43}{81} \delta^{pr} \delta^{tb} Y_d^{*as} + \frac{89}{81} \delta^{pa} \delta^{st} Y_d^{*rb} + \frac{17}{6} \delta^{pa} \delta^{tb} Y_d^{*rs} \Big) - \frac{9}{2} \delta^{pa} \delta^{tb} g_s^2 g_L^2 Y_d^{*rs} \Big\} C_{dG}^{ab} + C_{dG}^{*ab} \Big\{ g_s^4 \Big( \frac{19}{27} \delta^{ra} \delta^{st} Y_d^{pb} \\
& + \frac{38}{27} \delta^{pr} \delta^{sb} Y_d^{at} - \frac{4}{9} \delta^{pr} \delta^{st} Y_d^{ab} - 29 \delta^{ra} \delta^{sb} Y_d^{pt} \Big) + g_s^2 \Big( \frac{1}{3} \delta^{pr} Y_d^{at} (Y_d^\dagger Y_d)^{sb} + \frac{1}{3} \delta^{st} Y_d^{pb} (Y_d Y_d^\dagger)^{ar} + \frac{3}{2} \delta^{ra} Y_d^{pt} (Y_d^\dagger Y_d)^{sb} + 3 T_2 \delta^{ra} \delta^{sb} Y_d^{pt} \\
& + 3 \delta^{sb} Y_d^{pt} (Y_d Y_d^\dagger)^{ar} + \frac{17}{3} \delta^{sb} Y_d^{at} (Y_u Y_u^\dagger)^{pr} - \frac{1}{6} \delta^{st} Y_d^{pb} (Y_u Y_u^\dagger)^{ar} - 2 \delta^{ra} \delta^{sb} (Y_u Y_u^\dagger Y_d)^{pt} - 3 \delta^{sb} Y_d^{pt} (Y_u Y_u^\dagger)^{ar} - 4 \delta^{ra} Y_d^{pb} (Y_d^\dagger Y_d)^{st} - 4 \delta^{sb} Y_d^{at} (Y_d Y_d^\dagger)^{pr} \Big) \\
& - g_Y^2 g_s^2 \Big( \frac{43}{81} \delta^{pr} \delta^{sb} Y_d^{at} + \frac{89}{81} \delta^{ra} \delta^{st} Y_d^{pb} + \frac{17}{6} \delta^{ra} \delta^{sb} Y_d^{pt} \Big) - \frac{9}{2} \delta^{ra} \delta^{sb} g_s^2 g_L^2 Y_d^{pt} \Big\} + \Big\{ \frac{1}{4} \delta^{rb} (Y_d^\dagger Y_d)^{st} (Y_d Y_d^\dagger)^{pa} + \frac{1}{4} \delta^{pa} (Y_d^\dagger Y_d)^{st} (Y_d Y_d^\dagger)^{br} \\
& + \frac{1}{4} \delta^{rb} (Y_d^\dagger Y_d)^{st} (Y_u Y_u^\dagger)^{pa} + \frac{1}{4} \delta^{pa} (Y_d^\dagger Y_d)^{st} (Y_u Y_u^\dagger)^{br} + \frac{176}{243} \delta^{pa} \delta^{rb} \delta^{st} g_Y^2 g_s^2 + g_Y^2 \Big( \frac{2}{9} T_2 \delta^{pa} \delta^{rb} \delta^{st} + \frac{31}{12} \delta^{pa} \delta^{rb} (Y_d^\dagger Y_d)^{st} - \frac{31}{324} \delta^{rb} \delta^{st} (Y_u Y_u^\dagger)^{pa} \\
& - \frac{31}{324} \delta^{pa} \delta^{st} (Y_u Y_u^\dagger)^{br} - \frac{59}{324} \delta^{rb} \delta^{st} (Y_d Y_d^\dagger)^{pa} - \frac{59}{324} \delta^{pa} \delta^{st} (Y_d Y_d^\dagger)^{br} \Big) + g_s^2 \Big( \frac{7}{54} \delta^{rb} \delta^{st} (Y_u Y_u^\dagger)^{pa} + \frac{7}{54} \delta^{pa} \delta^{st} (Y_u Y_u^\dagger)^{br} - \frac{7}{54} \delta^{rb} \delta^{st} (Y_d Y_d^\dagger)^{pa}
\end{aligned}$$



$$\begin{aligned}
& -\frac{7}{54}\delta^{pa}\delta^{st}(Y_d Y_d^\dagger)^{br} - 17\delta^{pa}\delta^{rb}(Y_d^\dagger Y_d)^{st} + \frac{51}{4}\delta^{pa}\delta^{rb}g_L^2(Y_d^\dagger Y_d)^{st} - \frac{310}{729}\delta^{pa}\delta^{rb}\delta^{st}g_Y^4 - 2\delta^{pa}\delta^{rb}\delta^{st}g_Y^2g_L^2 - 2T_2\delta^{pa}\delta^{rb}(Y_d^\dagger Y_d)^{st} \\
& - 3\delta^{pa}\delta^{rb}(Y_d^\dagger Y_d Y_d^\dagger Y_d)^{st} \Big\} C_{Hq}^{(\parallel)ab} + \left\{ \frac{88}{243}\delta^{pa}\delta^{rb}\delta^{st}g_Y^2g_s^2 + \frac{23}{54}\delta^{pa}\delta^{rb}\delta^{st}g_s^2g_L^2 + \frac{1}{2}\delta^{rb}(Y_d^\dagger Y_d)^{st}(Y_d Y_d^\dagger)^{pa} + \frac{1}{2}\delta^{pa}(Y_d^\dagger Y_d)^{st}(Y_d Y_d^\dagger)^{br} \right. \\
& + g_Y^2 \left( \frac{31}{324}\delta^{rb}\delta^{st}(Y_u Y_u^\dagger)^{pa} + \frac{31}{324}\delta^{pa}\delta^{st}(Y_u Y_u^\dagger)^{br} + \frac{1}{9}T_2\delta^{pa}\delta^{rb}\delta^{st} + \frac{31}{24}\delta^{pa}\delta^{rb}(Y_d^\dagger Y_d)^{st} - \frac{59}{162}\delta^{rb}\delta^{st}(Y_d Y_d^\dagger)^{pa} - \frac{59}{162}\delta^{pa}\delta^{st}(Y_d Y_d^\dagger)^{br} \right) \\
& + \frac{87}{8}\delta^{pa}\delta^{rb}g_L^2(Y_d^\dagger Y_d)^{st} - \frac{155}{729}\delta^{pa}\delta^{rb}\delta^{st}g_Y^4 - \frac{1}{4}\delta^{rb}(Y_d^\dagger Y_d)^{st}(Y_u Y_u^\dagger)^{pa} - \frac{1}{4}\delta^{pa}(Y_d^\dagger Y_d)^{st}(Y_u Y_u^\dagger)^{br} - \frac{139}{162}\delta^{pa}\delta^{rb}\delta^{st}g_Y^2g_L^2 - T_2\delta^{pa}\delta^{rb}(Y_d^\dagger Y_d)^{st} \\
& \left. - g_s^2 \left( \frac{7}{54}\delta^{rb}\delta^{st}(Y_u Y_u^\dagger)^{pa} + \frac{7}{54}\delta^{pa}\delta^{st}(Y_u Y_u^\dagger)^{br} + \frac{7}{27}\delta^{rb}\delta^{st}(Y_d Y_d^\dagger)^{pa} + \frac{7}{27}\delta^{pa}\delta^{st}(Y_d Y_d^\dagger)^{br} + \frac{17}{2}\delta^{pa}\delta^{rb}(Y_d^\dagger Y_d)^{st} \right) - \frac{3}{2}\delta^{pa}\delta^{rb}(Y_d^\dagger Y_d Y_d^\dagger Y_d)^{st} \right\} C_{Hq}^{(\times)ab} \\
& + \left\{ \frac{241}{1458}\delta^{pr}\delta^{sa}\delta^{tb}g_Y^4 + \frac{1}{4}\delta^{tb}(Y_d^\dagger Y_d)^{sa}(Y_u Y_u^\dagger)^{pr} + \frac{1}{4}\delta^{sa}(Y_d^\dagger Y_d)^{bt}(Y_u Y_u^\dagger)^{pr} + \delta^{pr}\delta^{sa}\delta^{tb}g_Y^2g_L^2 + T_2\delta^{sa}\delta^{tb}(Y_d Y_d^\dagger)^{pr} + g_s^2 \left( \frac{7}{27}\delta^{pr}\delta^{tb}(Y_d^\dagger Y_d)^{sa} \right. \right. \\
& + \frac{7}{27}\delta^{pr}\delta^{sa}(Y_d^\dagger Y_d)^{bt} + \frac{17}{2}\delta^{sa}\delta^{tb}(Y_d Y_d^\dagger)^{pr} - \frac{17}{2}\delta^{sa}\delta^{tb}(Y_u Y_u^\dagger)^{pr} \Big) + g_Y^2 \left( \frac{73}{324}\delta^{pr}\delta^{tb}(Y_d^\dagger Y_d)^{sa} + \frac{73}{324}\delta^{pr}\delta^{sa}(Y_d^\dagger Y_d)^{bt} - \frac{1}{9}T_2\delta^{pr}\delta^{sa}\delta^{tb} \right. \\
& - \frac{1}{8}\delta^{sa}\delta^{tb}(Y_u Y_u^\dagger)^{pr} - \frac{49}{24}\delta^{sa}\delta^{tb}(Y_d Y_d^\dagger)^{pr} \Big) + g_L^2 \left( \frac{33}{8}\delta^{sa}\delta^{tb}(Y_u Y_u^\dagger)^{pr} - \frac{33}{8}\delta^{sa}\delta^{tb}(Y_d Y_d^\dagger)^{pr} \right) + 3\delta^{sa}\delta^{tb}(Y_d Y_d^\dagger Y_d Y_d^\dagger)^{pr} - \frac{1}{4}\delta^{tb}(Y_d^\dagger Y_d)^{sa}(Y_d Y_d^\dagger)^{pr} \\
& \left. - \frac{1}{4}\delta^{sa}(Y_d^\dagger Y_d)^{bt}(Y_d Y_d^\dagger)^{pr} - \frac{245}{486}\delta^{pr}\delta^{sa}\delta^{tb}g_Y^2g_s^2 - T_2\delta^{sa}\delta^{tb}(Y_u Y_u^\dagger)^{pr} - 3\delta^{sa}\delta^{tb}(Y_u Y_u^\dagger Y_u Y_u^\dagger)^{pr} \right\} C_{Hd}^{ab} + \left\{ \frac{1}{27}\delta^{pr}\delta^{tb}g_s^2(Y_d^\dagger Y_u)^{sa} \right. \\
& + \frac{3}{4}\delta^{tb}(Y_d^\dagger Y_u)^{sa}(Y_d Y_d^\dagger)^{pr} - \frac{59}{324}\delta^{pr}\delta^{tb}g_Y^2(Y_d^\dagger Y_u)^{sa} - \frac{3}{4}\delta^{tb}(Y_d^\dagger Y_u)^{sa}(Y_u Y_u^\dagger)^{pr} \Big\} C_{Hud}^{ab} + C_{Hud}^{*ab} \left\{ \frac{1}{27}\delta^{pr}\delta^{sb}g_s^2(Y_u^\dagger Y_d)^{at} + \frac{3}{4}\delta^{sb}(Y_u^\dagger Y_d)^{at}(Y_d Y_d^\dagger)^{pr} \right. \\
& \left. - \frac{59}{324}\delta^{pr}\delta^{sb}g_Y^2(Y_u^\dagger Y_d)^{at} - \frac{3}{4}\delta^{sb}(Y_u^\dagger Y_d)^{at}(Y_u Y_u^\dagger)^{pr} \right\} + \left\{ \frac{4}{9}\delta^{pr}\delta^{sc}\delta^{td}g_Y^2(Y_e Y_e^\dagger)^{ba} + \frac{1}{2}\delta^{sc}\delta^{td}(Y_d Y_d^\dagger)^{pr}(Y_e Y_e^\dagger)^{ba} + \frac{464}{729}\delta^{pr}\delta^{sc}\delta^{td}\delta^{ab}g_Y^4 \right. \\
& + \frac{167}{243}\delta^{pr}\delta^{sc}\delta^{td}\delta^{ab}g_Y^2g_s^2 + \frac{9}{2}\delta^{pr}\delta^{sc}\delta^{td}\delta^{ab}g_L^4 - \frac{1}{2}\delta^{pr}\delta^{sc}\delta^{td}\delta^{ab}g_Y^2g_L^2 - \frac{1}{2}\delta^{sc}\delta^{td}(Y_e Y_e^\dagger)^{ba}(Y_u Y_u^\dagger)^{pr} \Big\} C_{\ell d}^{abcd} + \left\{ \delta^{pa}\delta^{rb}(Y_d^\dagger Y_d)^{st}(Y_e^\dagger Y_e)^{dc} \right. \\
& + \frac{2306}{729}\delta^{pa}\delta^{rb}\delta^{st}\delta^{cd}g_Y^4 - \frac{232}{243}\delta^{pa}\delta^{rb}\delta^{st}\delta^{cd}g_Y^2g_s^2 - \frac{10}{9}\delta^{pa}\delta^{rb}\delta^{st}g_Y^2(Y_e^\dagger Y_e)^{dc} \Big\} C_{qe}^{abcd} + \left\{ g_s^2 \left( \frac{4}{27}\delta^{pa}\delta^{st}Y_u^{*rd}Y_u^{bc} + \frac{4}{27}\delta^{rb}\delta^{st}Y_u^{*ad}Y_u^{pc} \right) \right. \\
& + g_Y^2 \left( \frac{22}{81}\delta^{pa}\delta^{st}Y_u^{*rd}Y_u^{bc} + \frac{22}{81}\delta^{rb}\delta^{st}Y_u^{*ad}Y_u^{pc} + 2\delta^{pa}\delta^{rb}\delta^{st}(Y_u^\dagger Y_u)^{dc} \right) + \frac{1688}{729}\delta^{pa}\delta^{rb}\delta^{st}\delta^{cd}g_Y^4 + \frac{83}{9}\delta^{pa}\delta^{rb}\delta^{st}\delta^{cd}g_s^4 - \frac{1}{2}\delta^{pa}\delta^{rb}(Y_d^\dagger Y_u)^{sc}(Y_u^\dagger Y_d)^{dt} \\
& \left. - \frac{3}{2}Y_d^{*as}Y_u^{*rd}Y_d^{bt}Y_u^{pc} - \frac{400}{243}\delta^{pa}\delta^{rb}\delta^{st}\delta^{cd}g_Y^2g_s^2 - 3\delta^{pa}\delta^{rb}(Y_d^\dagger Y_d)^{st}(Y_u^\dagger Y_u)^{dc} \right\} C_{qu}^{(\parallel)abcd} + \left\{ \frac{1688}{2187}\delta^{pa}\delta^{rb}\delta^{st}\delta^{cd}g_Y^4 + g_Y^2g_s^2 \left( \frac{4}{81}\delta^{pr}\delta^{st}\delta^{ab}\delta^{cd} \right. \right. \\
& \left. \left. + \frac{3769}{729}\delta^{pa}\delta^{rb}\delta^{st}\delta^{cd} \right) + g_s^4 \left( \frac{4}{27}\delta^{pr}\delta^{st}\delta^{ab}\delta^{cd} + \frac{812}{243}\delta^{pa}\delta^{rb}\delta^{st}\delta^{cd} \right) + g_s^2 \left( \frac{1}{9}\delta^{pa}\delta^{st}Y_u^{*rd}Y_u^{bc} + \frac{1}{9}\delta^{rb}\delta^{st}Y_u^{*ad}Y_u^{pc} + \frac{4}{9}\delta^{pa}\delta^{rb}\delta^{st}(Y_u^\dagger Y_u)^{dc} \right. \right.
\end{aligned}$$

$$\begin{aligned}
& + \frac{2}{3} \delta^{pa} \delta^{cd} Y_d^{*rs} Y_d^{bt} + \frac{2}{3} \delta^{rb} \delta^{cd} Y_d^{*as} Y_d^{pt} - \frac{2}{9} \delta^{st} \delta^{ab} Y_u^{*rd} Y_u^{pc} \Big) + g_Y^2 \Big( \frac{16}{27} \delta^{pa} \delta^{rb} \delta^{st} (Y_u^\dagger Y_u)^{dc} + \frac{25}{27} \delta^{pa} \delta^{st} Y_u^{*rd} Y_u^{bc} + \frac{25}{27} \delta^{rb} \delta^{st} Y_u^{*ad} Y_u^{pc} \\
& - \frac{2}{27} \delta^{st} \delta^{ab} Y_u^{*rd} Y_u^{pc} \Big) - \frac{1}{4} \delta^{pa} Y_u^{*rd} Y_d^{bt} (Y_d^\dagger Y_u)^{sc} - \frac{1}{4} \delta^{rb} Y_d^{*as} Y_u^{pc} (Y_u^\dagger Y_d)^{dt} - \delta^{pa} \delta^{rb} (Y_d^\dagger Y_d)^{st} (Y_u^\dagger Y_u)^{dc} \Big\} C_{qu}^{(\times)abcd} + \left\{ g_Y^2 g_L^2 \Big( \frac{1}{2} \delta^{pr} \delta^{sc} \delta^{td} \delta^{ab} \right. \\
& - \frac{3}{2} \delta^{pa} \delta^{rb} \delta^{sc} \delta^{td} \Big) + g_Y^4 \Big( \frac{398}{729} \delta^{pa} \delta^{rb} \delta^{st} \delta^{cd} - \frac{14}{729} \delta^{pr} \delta^{sc} \delta^{td} \delta^{ab} - \frac{479}{54} \delta^{pa} \delta^{rb} \delta^{sc} \delta^{td} \Big) + g_Y^2 g_s^2 \Big( \frac{49}{243} \delta^{pr} \delta^{sc} \delta^{td} \delta^{ab} + \frac{200}{243} \delta^{pa} \delta^{rb} \delta^{st} \delta^{cd} \\
& - \frac{125}{18} \delta^{pa} \delta^{rb} \delta^{sc} \delta^{td} \Big) + g_s^4 \Big( 9 \delta^{pa} \delta^{rb} \delta^{sc} \delta^{td} + \frac{83}{9} \delta^{pa} \delta^{rb} \delta^{st} \delta^{cd} + \frac{166}{9} \delta^{pr} \delta^{sc} \delta^{td} \delta^{ab} \Big) + \delta^{pa} Y_d^{*rd} Y_d^{bc} (Y_d^\dagger Y_d)^{st} + \delta^{rb} Y_d^{*ad} Y_d^{pc} (Y_d^\dagger Y_d)^{st} \\
& + \delta^{sc} Y_d^{*ad} Y_d^{bt} (Y_d Y_d^\dagger)^{pr} + \delta^{td} Y_d^{*as} Y_d^{bc} (Y_d Y_d^\dagger)^{pr} + \delta^{sc} \delta^{td} (Y_d Y_d^\dagger)^{br} (Y_u Y_u^\dagger)^{pa} + \delta^{sc} \delta^{td} (Y_d Y_d^\dagger)^{pa} (Y_u Y_u^\dagger)^{br} + g_s^2 \Big( \frac{4}{27} \delta^{pa} \delta^{st} Y_d^{*rd} Y_d^{bc} + \frac{4}{27} \delta^{rb} \delta^{st} Y_d^{*ad} Y_d^{pc} \\
& + \frac{8}{27} \delta^{pr} \delta^{sc} Y_d^{*ad} Y_d^{bt} + \frac{8}{27} \delta^{pr} \delta^{td} Y_d^{*as} Y_d^{bc} + 6 \delta^{rb} \delta^{sc} Y_d^{*ad} Y_d^{pt} + 6 \delta^{pa} \delta^{td} Y_d^{*rs} Y_d^{bc} - 2 \delta^{pa} \delta^{sc} Y_d^{*rd} Y_d^{bt} - 2 \delta^{rb} \delta^{td} Y_d^{*as} Y_d^{pc} - \frac{11}{3} \delta^{rb} \delta^{sc} \delta^{td} (Y_d Y_d^\dagger)^{pa} \\
& - \frac{11}{3} \delta^{pa} \delta^{sc} \delta^{td} (Y_d Y_d^\dagger)^{br} - \frac{11}{3} \delta^{rb} \delta^{sc} \delta^{td} (Y_u Y_u^\dagger)^{pa} - \frac{11}{3} \delta^{pa} \delta^{sc} \delta^{td} (Y_u Y_u^\dagger)^{br} - \frac{22}{3} \delta^{pa} \delta^{rb} \delta^{td} (Y_d^\dagger Y_d)^{sc} - \frac{22}{3} \delta^{pa} \delta^{rb} \delta^{sc} (Y_d^\dagger Y_d)^{dt} \Big) \\
& + g_L^2 \Big( \frac{33}{16} \delta^{rb} \delta^{sc} \delta^{td} (Y_d Y_d^\dagger)^{pa} + \frac{33}{16} \delta^{pa} \delta^{sc} \delta^{td} (Y_d Y_d^\dagger)^{br} + \frac{33}{16} \delta^{rb} \delta^{sc} \delta^{td} (Y_u Y_u^\dagger)^{pa} + \frac{33}{16} \delta^{pa} \delta^{sc} \delta^{td} (Y_u Y_u^\dagger)^{br} + \frac{51}{8} \delta^{pa} \delta^{rb} \delta^{td} (Y_d^\dagger Y_d)^{sc} \\
& + \frac{51}{8} \delta^{pa} \delta^{rb} \delta^{sc} (Y_d^\dagger Y_d)^{dt} \Big) + g_Y^2 \Big( \frac{247}{144} \delta^{rb} \delta^{sc} \delta^{td} (Y_d Y_d^\dagger)^{pa} + \frac{247}{144} \delta^{pa} \delta^{sc} \delta^{td} (Y_d Y_d^\dagger)^{br} + \frac{157}{72} \delta^{pa} \delta^{rb} \delta^{td} (Y_d^\dagger Y_d)^{sc} + \frac{157}{72} \delta^{pa} \delta^{rb} \delta^{sc} (Y_d^\dagger Y_d)^{dt} \\
& - \frac{10}{81} \delta^{pr} \delta^{sc} Y_d^{*ad} Y_d^{bt} - \frac{10}{81} \delta^{pr} \delta^{td} Y_d^{*as} Y_d^{bc} - \frac{14}{81} \delta^{pa} \delta^{st} Y_d^{*rd} Y_d^{bc} - \frac{14}{81} \delta^{rb} \delta^{st} Y_d^{*ad} Y_d^{pc} - \frac{53}{144} \delta^{rb} \delta^{sc} \delta^{td} (Y_u Y_u^\dagger)^{pa} - \frac{53}{144} \delta^{pa} \delta^{sc} \delta^{td} (Y_u Y_u^\dagger)^{br} \\
& - \frac{2}{3} \delta^{pa} \delta^{rb} \delta^{st} (Y_d^\dagger Y_d)^{dc} - \frac{2}{3} \delta^{pr} \delta^{sc} \delta^{td} (Y_u Y_u^\dagger)^{ba} \Big) + \frac{3}{2} \delta^{sc} \delta^{td} (Y_d Y_d^\dagger)^{pr} (Y_d Y_d^\dagger)^{ba} + \frac{3}{2} \delta^{sc} \delta^{td} (Y_u Y_u^\dagger)^{pr} (Y_u Y_u^\dagger)^{ba} + 2 \delta^{rb} \delta^{sc} (Y_d^\dagger Y_d)^{dt} (Y_d Y_d^\dagger)^{pa} \\
& + 2 \delta^{pa} \delta^{td} (Y_d^\dagger Y_d)^{sc} (Y_d Y_d^\dagger)^{br} + 3 \delta^{pa} \delta^{rb} (Y_d^\dagger Y_d)^{st} (Y_d^\dagger Y_d)^{dc} + \frac{27}{2} \delta^{pr} \delta^{sc} \delta^{td} \delta^{ab} g_L^4 - \frac{1}{4} \delta^{pa} \delta^{rb} \delta^{td} (Y_d^\dagger Y_d Y_d^\dagger Y_d)^{sc} - \frac{1}{4} \delta^{pa} \delta^{rb} \delta^{sc} (Y_d^\dagger Y_d Y_d^\dagger Y_d)^{dt} \\
& - \frac{1}{4} \delta^{pa} \delta^{rb} \delta^{td} (Y_d^\dagger Y_u Y_u^\dagger Y_d)^{sc} - \frac{1}{4} \delta^{pa} \delta^{rb} \delta^{sc} (Y_d^\dagger Y_u Y_u^\dagger Y_d)^{dt} - \frac{1}{4} \delta^{rb} \delta^{sc} \delta^{td} (Y_d Y_d^\dagger Y_d Y_d^\dagger)^{pa} - \frac{1}{4} \delta^{pa} \delta^{sc} \delta^{td} (Y_d Y_d^\dagger Y_d Y_d^\dagger)^{br} - \frac{1}{4} \delta^{rb} \delta^{sc} \delta^{td} (Y_u Y_u^\dagger Y_u Y_u^\dagger)^{pa} \\
& - \frac{1}{4} \delta^{pa} \delta^{sc} \delta^{td} (Y_u Y_u^\dagger Y_u Y_u^\dagger)^{br} - \frac{3}{4} T_2 \delta^{rb} \delta^{sc} \delta^{td} (Y_d Y_d^\dagger)^{pa} - \frac{3}{4} T_2 \delta^{pa} \delta^{sc} \delta^{td} (Y_d Y_d^\dagger)^{br} - \frac{3}{4} T_2 \delta^{rb} \delta^{sc} \delta^{td} (Y_u Y_u^\dagger)^{pa} - \frac{3}{4} T_2 \delta^{pa} \delta^{sc} \delta^{td} (Y_u Y_u^\dagger)^{br} \\
& - \delta^{rb} \delta^{td} (Y_d^\dagger Y_d)^{sc} (Y_u Y_u^\dagger)^{pa} - \delta^{pa} \delta^{sc} (Y_d^\dagger Y_d)^{dt} (Y_u Y_u^\dagger)^{br} - \frac{5}{4} \delta^{rb} \delta^{td} (Y_d^\dagger Y_d)^{sc} (Y_d Y_d^\dagger)^{pa} - \frac{5}{4} \delta^{pa} \delta^{sc} (Y_d^\dagger Y_d)^{dt} (Y_d Y_d^\dagger)^{br} - \frac{3}{2} T_2 \delta^{pa} \delta^{rb} \delta^{td} (Y_d^\dagger Y_d)^{sc} \\
& - \frac{3}{2} T_2 \delta^{pa} \delta^{rb} \delta^{sc} (Y_d^\dagger Y_d)^{dt} - \frac{3}{2} \delta^{sc} \delta^{td} (Y_d Y_d^\dagger)^{ba} (Y_u Y_u^\dagger)^{pr} - \frac{3}{2} \delta^{sc} \delta^{td} (Y_d Y_d^\dagger)^{pr} (Y_u Y_u^\dagger)^{ba} - \frac{5}{2} \delta^{pa} \delta^{rb} (Y_d^\dagger Y_d)^{sc} (Y_d^\dagger Y_d)^{dt} - \frac{5}{2} \delta^{sc} \delta^{td} (Y_d Y_d^\dagger)^{pa} (Y_d Y_d^\dagger)^{br} \\
& - \frac{5}{2} \delta^{sc} \delta^{td} (Y_u Y_u^\dagger)^{pa} (Y_u Y_u^\dagger)^{br} - \frac{11}{4} \delta^{rb} \delta^{sc} (Y_d^\dagger Y_d)^{dt} (Y_u Y_u^\dagger)^{pa} - \frac{11}{4} \delta^{pa} \delta^{td} (Y_d^\dagger Y_d)^{sc} (Y_u Y_u^\dagger)^{br} - \frac{9}{2} \delta^{pa} \delta^{rb} \delta^{sc} \delta^{td} g_s^2 g_L^2 \Big\} C_{qd}^{(\parallel)abcd} + \left\{ \frac{1}{6} \delta^{pr} \delta^{sc} \delta^{td} \delta^{ab} g_Y^2 g_L^2 \right. \\
& + \frac{1}{4} \delta^{rb} \delta^{td} Y_d^{pc} (Y_d^\dagger Y_d Y_d^\dagger)^{as} + \frac{1}{4} \delta^{pa} \delta^{sc} Y_d^{*rd} (Y_d Y_d^\dagger Y_d)^{bt} + \frac{1}{2} T_2 \delta^{pa} \delta^{sc} Y_d^{*rd} Y_d^{bt} + \frac{1}{2} T_2 \delta^{rb} \delta^{td} Y_d^{*as} Y_d^{pc} + \frac{1}{2} \delta^{sc} \delta^{td} (Y_d Y_d^\dagger)^{pr} (Y_d Y_d^\dagger)^{ba} \\
& + \frac{1}{2} \delta^{sc} Y_d^{*rd} Y_d^{bt} (Y_u Y_u^\dagger)^{pa} + \frac{1}{2} \delta^{td} Y_d^{*as} Y_d^{pc} (Y_u Y_u^\dagger)^{br} + \frac{1}{2} \delta^{sc} \delta^{td} (Y_u Y_u^\dagger)^{pr} (Y_u Y_u^\dagger)^{ba} + \frac{1}{2} \delta^{pa} \delta^{sc} Y_d^{bt} (Y_d^\dagger Y_d Y_d^\dagger)^{rd} + \frac{1}{2} \delta^{rb} \delta^{td} Y_d^{*as} (Y_d Y_d^\dagger Y_d)^{pc}
\end{aligned}$$

$$\begin{aligned}
& + g_L^2 \left( \frac{15}{8} \delta^{pa} \delta^{sc} Y_d^{*rd} Y_d^{bt} + \frac{15}{8} \delta^{rb} \delta^{td} Y_d^{*as} Y_d^{pc} \right) + g_s^2 g_L^2 \left( \frac{27}{4} \delta^{pa} \delta^{rb} \delta^{sc} \delta^{td} - \delta^{pr} \delta^{sc} \delta^{td} \delta^{ab} \right) + g_Y^4 \left( \frac{398}{2187} \delta^{pa} \delta^{rb} \delta^{st} \delta^{cd} - \frac{14}{2187} \delta^{pr} \delta^{sc} \delta^{td} \delta^{ab} \right) \\
& + g_Y^2 g_s^2 \left( \frac{8}{81} \delta^{pr} \delta^{st} \delta^{ab} \delta^{cd} + \frac{1}{4} \delta^{pa} \delta^{rb} \delta^{sc} \delta^{td} - \frac{496}{729} \delta^{pr} \delta^{sc} \delta^{td} \delta^{ab} - \frac{1490}{729} \delta^{pa} \delta^{rb} \delta^{st} \delta^{cd} \right) + g_s^4 \left( \frac{8}{27} \delta^{pr} \delta^{st} \delta^{ab} \delta^{cd} + \frac{812}{243} \delta^{pa} \delta^{rb} \delta^{st} \delta^{cd} \right. \\
& + \frac{1516}{243} \delta^{pr} \delta^{sc} \delta^{td} \delta^{ab} - \frac{177}{2} \delta^{pa} \delta^{rb} \delta^{sc} \delta^{td} \left. \right) + \delta^{pa} \delta^{rb} (Y_d^\dagger Y_d)^{st} (Y_d^\dagger Y_d)^{dc} + g_Y^2 \left( \frac{61}{72} \delta^{pa} \delta^{sc} Y_d^{*rd} Y_d^{bt} + \frac{61}{72} \delta^{rb} \delta^{td} Y_d^{*as} Y_d^{pc} - \frac{2}{27} \delta^{st} \delta^{ab} Y_d^{*rd} Y_d^{pc} \right. \\
& - \frac{2}{27} \delta^{pr} \delta^{cd} Y_d^{*as} Y_d^{bt} - \frac{2}{27} \delta^{pr} \delta^{sc} \delta^{td} (Y_d Y_d^\dagger)^{ba} - \frac{4}{27} \delta^{pr} \delta^{sc} Y_d^{*ad} Y_d^{bt} - \frac{4}{27} \delta^{pr} \delta^{td} Y_d^{*as} Y_d^{bc} - \frac{2}{9} \delta^{pr} \delta^{sc} \delta^{td} (Y_u Y_u^\dagger)^{ba} - \frac{8}{27} \delta^{pa} \delta^{rb} \delta^{st} (Y_d^\dagger Y_d)^{dc} \\
& - \frac{11}{27} \delta^{pa} \delta^{st} Y_d^{*rd} Y_d^{bc} - \frac{11}{27} \delta^{rb} \delta^{st} Y_d^{*ad} Y_d^{pc} \left. \right) + g_s^2 \left( \frac{1}{9} \delta^{pa} \delta^{st} Y_d^{*rd} Y_d^{bc} + \frac{1}{9} \delta^{rb} \delta^{st} Y_d^{*ad} Y_d^{pc} + \frac{2}{9} \delta^{pr} \delta^{sc} Y_d^{*ad} Y_d^{bt} + \frac{2}{9} \delta^{pr} \delta^{td} Y_d^{*as} Y_d^{bc} + \frac{4}{9} \delta^{pa} \delta^{rb} \delta^{st} (Y_d^\dagger Y_d)^{dc} \right. \\
& + \frac{4}{9} \delta^{pr} \delta^{sc} \delta^{td} (Y_d Y_d^\dagger)^{ba} + \frac{2}{3} \delta^{pa} \delta^{cd} Y_d^{*rs} Y_d^{bt} + \frac{2}{3} \delta^{rb} \delta^{cd} Y_d^{*as} Y_d^{pt} + \frac{2}{3} \delta^{pr} \delta^{sc} \delta^{td} (Y_u Y_u^\dagger)^{ba} + \frac{4}{3} \delta^{sc} \delta^{ab} Y_d^{*rd} Y_d^{pt} + \frac{4}{3} \delta^{td} \delta^{ab} Y_d^{*rs} Y_d^{pc} + 18 \delta^{rb} \delta^{sc} Y_d^{*ad} Y_d^{pt} \\
& + 18 \delta^{pa} \delta^{td} Y_d^{*rs} Y_d^{bc} - \frac{2}{9} \delta^{st} \delta^{ab} Y_d^{*rd} Y_d^{pc} - \frac{2}{9} \delta^{pr} \delta^{cd} Y_d^{*as} Y_d^{bt} - \frac{88}{3} \delta^{pa} \delta^{sc} Y_d^{*rd} Y_d^{bt} - \frac{88}{3} \delta^{rb} \delta^{td} Y_d^{*as} Y_d^{pc} \left. \right) + 3 \delta^{pa} Y_d^{*rd} Y_d^{bc} (Y_d^\dagger Y_d)^{st} \\
& + 3 \delta^{rb} Y_d^{*ad} Y_d^{pc} (Y_d^\dagger Y_d)^{st} + 3 \delta^{sc} Y_d^{*ad} Y_d^{bt} (Y_d Y_d^\dagger)^{pr} + 3 \delta^{td} Y_d^{*as} Y_d^{bc} (Y_d Y_d^\dagger)^{pr} + \frac{9}{2} \delta^{pr} \delta^{sc} \delta^{td} \delta^{ab} g_L^4 - \frac{1}{2} \delta^{sc} \delta^{td} (Y_d Y_d^\dagger)^{ba} (Y_u Y_u^\dagger)^{pr} \\
& - \frac{1}{2} \delta^{sc} \delta^{td} (Y_d Y_d^\dagger)^{pr} (Y_u Y_u^\dagger)^{ba} - \frac{3}{4} \delta^{pa} Y_d^{*rd} Y_d^{bt} (Y_d^\dagger Y_d)^{sc} - \frac{3}{4} \delta^{rb} Y_d^{*as} Y_d^{pc} (Y_d^\dagger Y_d)^{dt} - \frac{5}{4} \delta^{rb} \delta^{td} Y_d^{pc} (Y_u^\dagger Y_u Y_d^\dagger)^{as} - \frac{5}{4} \delta^{pa} \delta^{sc} Y_d^{*rd} (Y_u Y_u^\dagger Y_d)^{bt} \\
& - \frac{3}{2} \delta^{sc} Y_d^{*rd} Y_d^{bt} (Y_d Y_d^\dagger)^{pa} - \frac{3}{2} \delta^{td} Y_d^{*as} Y_d^{pc} (Y_d Y_d^\dagger)^{br} - \frac{3}{2} \delta^{pa} \delta^{sc} Y_d^{bt} (Y_u^\dagger Y_u Y_d^\dagger)^{rd} - \frac{3}{2} \delta^{rb} \delta^{td} Y_d^{*as} (Y_u Y_u^\dagger Y_d)^{pc} \left. \right\} C_{qd}^{(\times)abcd} - \frac{16}{81} \delta^{pr} \delta^{st} \delta^{ab} \delta^{cd} g_Y^4 C_{ee}^{abcd} \\
& + \left\{ \frac{4}{9} \delta^{st} \delta^{ad} g_s^2 Y_u^{*rb} Y_u^{pc} + \frac{16}{27} \delta^{st} \delta^{ad} g_Y^2 Y_u^{*rb} Y_u^{pc} - \frac{64}{243} \delta^{pr} \delta^{st} \delta^{ad} \delta^{bc} g_Y^4 - \frac{8}{27} \delta^{pr} \delta^{st} \delta^{ad} \delta^{bc} g_s^4 \right\} C_{uu}^{abcd} + \left\{ g_Y^2 g_s^2 \left( \frac{10}{243} \delta^{pr} \delta^{sa} \delta^{tb} \delta^{cd} \right. \right. \\
& + \frac{4}{81} \delta^{pr} \delta^{st} \delta^{ad} \delta^{bc} - \frac{64}{729} \delta^{pr} \delta^{sa} \delta^{td} \delta^{bc} \left. \right) + g_Y^4 \left( \frac{160}{2187} \delta^{pr} \delta^{sa} \delta^{td} \delta^{bc} + \frac{100}{729} \delta^{pr} \delta^{sa} \delta^{tb} \delta^{cd} - \frac{16}{243} \delta^{pr} \delta^{st} \delta^{ad} \delta^{bc} \right) + g_s^2 \left( \frac{4}{9} \delta^{st} \delta^{ad} Y_d^{*rb} Y_d^{pc} \right. \\
& + \frac{4}{3} \delta^{tb} \delta^{ad} Y_d^{*rs} Y_d^{pc} + \frac{4}{3} \delta^{sa} \delta^{bc} Y_d^{*rd} Y_d^{pt} + \frac{20}{9} \delta^{pr} \delta^{sa} \delta^{td} (Y_d^\dagger Y_d)^{bc} + 8 \delta^{sa} \delta^{td} Y_d^{*rb} Y_d^{pc} + \frac{28}{3} \delta^{sa} \delta^{tb} Y_d^{*rd} Y_d^{pc} \left. \right) + g_Y^2 \left( \frac{14}{27} \delta^{pr} \delta^{sa} \delta^{td} (Y_d^\dagger Y_d)^{bc} \right. \\
& + \frac{2}{3} \delta^{pr} \delta^{sa} \delta^{tb} (Y_d^\dagger Y_d)^{dc} - \frac{8}{27} \delta^{st} \delta^{ad} Y_d^{*rb} Y_d^{pc} - \frac{35}{36} \delta^{sa} \delta^{tb} Y_d^{*rd} Y_d^{pc} \left. \right) + 3 T_2 \delta^{sa} \delta^{tb} Y_d^{*rd} Y_d^{pc} + 3 \delta^{sa} \delta^{td} (Y_d^\dagger Y_d)^{bc} (Y_u Y_u^\dagger)^{pr} + 3 \delta^{sa} \delta^{tb} (Y_d^\dagger Y_d)^{dc} (Y_u Y_u^\dagger)^{pr} \\
& + 3 \delta^{sa} \delta^{tb} Y_d^{pc} (Y_d^\dagger Y_d Y_d^\dagger)^{rd} + 3 \delta^{sa} \delta^{tb} Y_d^{*rd} (Y_d Y_d^\dagger Y_d)^{pc} - g_s^4 \left( \frac{4}{27} \delta^{pr} \delta^{st} \delta^{ad} \delta^{bc} + \frac{2276}{243} \delta^{pr} \delta^{sa} \delta^{td} \delta^{bc} + \frac{130}{9} \delta^{pr} \delta^{sa} \delta^{tb} \delta^{cd} \right) - \delta^{sa} \delta^{tb} Y_d^{pc} (Y_u^\dagger Y_u Y_d^\dagger)^{rd} \\
& - \delta^{sa} \delta^{tb} Y_d^{*rd} (Y_u Y_u^\dagger Y_d)^{pc} - \frac{3}{2} \delta^{td} Y_d^{*rb} Y_d^{pa} (Y_d^\dagger Y_d)^{sc} - \frac{3}{2} \delta^{sc} Y_d^{*rb} Y_d^{pa} (Y_d^\dagger Y_d)^{dt} - 3 \delta^{sa} \delta^{td} (Y_d^\dagger Y_d)^{bc} (Y_d Y_d^\dagger)^{pr} - 3 \delta^{sa} \delta^{tb} (Y_d^\dagger Y_d)^{dc} (Y_d Y_d^\dagger)^{pr} \\
& - \frac{33}{4} \delta^{sa} \delta^{tb} g_L^2 Y_d^{*rd} Y_d^{pc} \left. \right\} C_{dd}^{abcd} + \left\{ \frac{1}{2} \delta^{sc} \delta^{td} (Y_e^\dagger Y_e)^{ba} (Y_u Y_u^\dagger)^{pr} + \frac{5}{9} \delta^{pr} \delta^{sc} \delta^{td} g_Y^2 (Y_e^\dagger Y_e)^{ba} + \frac{167}{243} \delta^{pr} \delta^{sc} \delta^{td} \delta^{ab} g_Y^2 g_s^2 - \frac{1}{2} \delta^{sc} \delta^{td} (Y_e^\dagger Y_e)^{ba} (Y_d Y_d^\dagger)^{pr} \right. \\
& \left. - \frac{508}{729} \delta^{pr} \delta^{sc} \delta^{td} \delta^{ab} g_Y^4 \right\} C_{ed}^{abcd} + \left\{ \frac{98}{243} \delta^{pr} \delta^{sc} \delta^{td} \delta^{ab} g_Y^2 g_s^2 + \frac{3}{2} T_2 \delta^{sc} \delta^{td} Y_u^{*rb} Y_u^{pa} + \frac{3}{2} \delta^{sc} \delta^{td} (Y_u^\dagger Y_u)^{ba} (Y_d Y_d^\dagger)^{pr} + \frac{3}{2} \delta^{sc} \delta^{td} Y_u^{pa} (Y_u^\dagger Y_u Y_u^\dagger)^{rb} \right.
\end{aligned}$$

$$\begin{aligned}
& + \frac{3}{2} \delta^{sc} \delta^{td} Y_u^{*rb} (Y_u Y_u^\dagger Y_u)^{pa} + \frac{14}{3} \delta^{sc} \delta^{td} g_s^2 Y_u^{*rb} Y_u^{pa} - \frac{154}{729} \delta^{pr} \delta^{sc} \delta^{td} \delta^{ab} g_Y^4 - \frac{1}{2} \delta^{sc} \delta^{td} Y_u^{*pa} (Y_d^\dagger Y_d Y_u^\dagger)^{rb} - \frac{1}{2} \delta^{sc} \delta^{td} Y_u^{*rb} (Y_d Y_d^\dagger Y_u)^{pa} \\
& - g_Y^2 \left( \delta^{pr} \delta^{sc} \delta^{td} (Y_u^\dagger Y_u)^{ba} + \frac{287}{72} \delta^{sc} \delta^{td} Y_u^{*rb} Y_u^{pa} \right) - \frac{5}{4} \delta^{td} Y_u^{*rb} Y_u^{pa} (Y_d^\dagger Y_d)^{sc} - \frac{5}{4} \delta^{sc} Y_u^{*rb} Y_u^{pa} (Y_d^\dagger Y_d)^{dt} - \frac{3}{2} \delta^{sc} \delta^{td} (Y_u^\dagger Y_u)^{ba} (Y_u Y_u^\dagger)^{pr} \\
& - \frac{33}{8} \delta^{sc} \delta^{td} g_L^2 Y_u^{*rb} Y_u^{pa} - \frac{71}{9} \delta^{pr} \delta^{sc} \delta^{td} \delta^{ab} g_s^4 \left\} C_{ud}^{(\parallel)abcd} + \left\{ \frac{1}{4} \delta^{td} Y_u^{*rb} Y_d^{pc} (Y_d^\dagger Y_u)^{sa} + \frac{1}{4} \delta^{sc} Y_d^{*rd} Y_u^{pa} (Y_u^\dagger Y_d)^{bt} + \frac{1}{2} \delta^{sc} \delta^{td} (Y_u^\dagger Y_u)^{ba} (Y_d Y_d^\dagger)^{pr} \right. \\
& + g_Y^2 g_s^2 \left( \frac{2}{81} \delta^{pr} \delta^{st} \delta^{ab} \delta^{cd} + \frac{343}{729} \delta^{pr} \delta^{sc} \delta^{td} \delta^{ab} \right) + g_s^4 \left( \frac{2}{27} \delta^{pr} \delta^{st} \delta^{ab} \delta^{cd} - \frac{448}{243} \delta^{pr} \delta^{sc} \delta^{td} \delta^{ab} \right) + g_s^2 \left( \frac{2}{3} \delta^{sc} \delta^{ab} Y_d^{*rd} Y_d^{pt} + \frac{2}{3} \delta^{td} \delta^{ab} Y_d^{*rs} Y_d^{pc} \right. \\
& + \frac{2}{3} \delta^{pr} \delta^{sc} \delta^{td} (Y_u^\dagger Y_u)^{ba} + 4 \delta^{sc} \delta^{td} Y_u^{*rb} Y_u^{pa} \left. \right) - \frac{154}{2187} \delta^{pr} \delta^{sc} \delta^{td} \delta^{ab} g_Y^4 - \frac{1}{3} \delta^{pr} \delta^{sc} \delta^{td} g_Y^2 (Y_u^\dagger Y_u)^{ba} - \frac{1}{2} \delta^{sc} \delta^{td} (Y_u^\dagger Y_u)^{ba} (Y_u Y_u^\dagger)^{pr} \left\} C_{ud}^{(\times)abcd} \right. \\
& + \left\{ g_Y^2 \left( \frac{5}{81} \delta^{pr} \delta^{sc} Y_e^{*ab} Y_d^{dt} + \frac{7}{81} \delta^{rd} \delta^{st} Y_e^{*ab} Y_d^{pc} \right) - \frac{1}{4} \delta^{rd} Y_e^{*ab} Y_d^{pc} (Y_d^\dagger Y_d)^{st} - \frac{1}{4} \delta^{sc} Y_e^{*ab} Y_d^{dt} (Y_d Y_d^\dagger)^{pr} - \frac{1}{4} \delta^{sc} Y_e^{*ab} Y_d^{dt} (Y_u Y_u^\dagger)^{pr} - g_s^2 \left( \frac{2}{27} \delta^{rd} \delta^{st} Y_e^{*ab} Y_d^{pc} \right. \right. \\
& + \frac{4}{27} \delta^{pr} \delta^{sc} Y_e^{*ab} Y_d^{dt} + 3 \delta^{rd} \delta^{sc} Y_e^{*ab} Y_d^{pt} \left. \right) \left\} C_{ledq}^{abcd} + C_{ledq}^{*abcd} \left\{ g_Y^2 \left( \frac{5}{81} \delta^{pr} \delta^{tc} Y_d^{*ds} Y_e^{ab} + \frac{7}{81} \delta^{pd} \delta^{st} Y_d^{*rc} Y_e^{ab} \right) - \frac{1}{4} \delta^{pd} Y_d^{*rc} Y_e^{ab} (Y_d^\dagger Y_d)^{st} \right. \right. \\
& - \frac{1}{4} \delta^{tc} Y_d^{*ds} Y_e^{ab} (Y_d Y_d^\dagger)^{pr} - \frac{1}{4} \delta^{tc} Y_d^{*ds} Y_e^{ab} (Y_u Y_u^\dagger)^{pr} - g_s^2 \left( \frac{2}{27} \delta^{pd} \delta^{st} Y_d^{*rc} Y_e^{ab} + \frac{4}{27} \delta^{pr} \delta^{tc} Y_d^{*ds} Y_e^{ab} + 3 \delta^{pd} \delta^{tc} Y_d^{*rs} Y_e^{ab} \right) \left. \right\} + \left\{ \frac{1}{8} \delta^{pc} Y_d^{*rd} Y_d^{*as} (Y_u^\dagger Y_d)^{bt} \right. \\
& + \frac{3}{4} \delta^{td} Y_d^{*cs} Y_u^{*rb} (Y_d Y_d^\dagger)^{pa} + g_Y^2 \left( \frac{1}{324} \delta^{pr} \delta^{td} Y_d^{*as} Y_u^{*cb} + \frac{11}{324} \delta^{pa} \delta^{st} Y_d^{*rd} Y_u^{*cb} + \frac{5}{27} \delta^{pr} \delta^{td} Y_d^{*cs} Y_u^{*ab} + \frac{7}{27} \delta^{pc} \delta^{st} Y_d^{*rd} Y_u^{*ab} \right. \\
& - \frac{7}{324} \delta^{pc} \delta^{st} Y_d^{*ad} Y_u^{*rb} - \frac{37}{144} \delta^{pa} \delta^{td} Y_d^{*cs} Y_u^{*rb} - \frac{11}{27} \delta^{pa} \delta^{st} Y_d^{*cd} Y_u^{*rb} \left. \right) + g_s^2 \left( \frac{1}{54} \delta^{pa} \delta^{st} Y_d^{*rd} Y_u^{*cb} + \frac{1}{54} \delta^{pc} \delta^{st} Y_d^{*ad} Y_u^{*rb} + 2 \delta^{pc} \delta^{td} Y_d^{*as} Y_u^{*rb} \right. \\
& - \frac{2}{27} \delta^{pr} \delta^{td} Y_d^{*as} Y_u^{*cb} - \frac{2}{9} \delta^{pa} \delta^{st} Y_d^{*cd} Y_u^{*rb} - \frac{2}{9} \delta^{pc} \delta^{st} Y_d^{*rd} Y_u^{*ab} - \frac{4}{9} \delta^{pr} \delta^{td} Y_d^{*cs} Y_u^{*ab} - \frac{97}{12} \delta^{pa} \delta^{td} Y_d^{*cs} Y_u^{*rb} - 9 \delta^{pc} \delta^{td} Y_d^{*rs} Y_u^{*ab} \left. \right) \\
& - \frac{1}{8} \delta^{pa} Y_d^{*rd} Y_u^{*cb} (Y_d^\dagger Y_d)^{st} - \frac{1}{8} \delta^{pc} Y_d^{*ad} Y_u^{*rb} (Y_d^\dagger Y_d)^{st} - \frac{1}{8} \delta^{td} Y_d^{*as} Y_u^{*cb} (Y_d Y_d^\dagger)^{pr} - \frac{1}{8} \delta^{td} Y_d^{*as} Y_u^{*cb} (Y_u Y_u^\dagger)^{pr} - \frac{1}{8} \delta^{pa} \delta^{td} Y_u^{*rb} (Y_d^\dagger Y_d Y_d^\dagger)^{cs} \\
& - \frac{1}{4} T_2 \delta^{pa} \delta^{td} Y_d^{*cs} Y_u^{*rb} - \frac{1}{4} \delta^{pa} \delta^{td} Y_d^{*cs} (Y_d^\dagger Y_d Y_u^\dagger)^{rb} - \frac{1}{4} \delta^{pa} \delta^{td} Y_d^{*cs} (Y_u^\dagger Y_u Y_u^\dagger)^{rb} - \frac{3}{8} \delta^{pa} \delta^{td} Y_u^{*rb} (Y_u^\dagger Y_u Y_d^\dagger)^{cs} - \frac{5}{8} \delta^{pa} Y_d^{*cs} Y_u^{*rb} (Y_d^\dagger Y_d)^{dt} \\
& - \frac{3}{4} \delta^{pa} Y_d^{*cd} Y_u^{*rb} (Y_d^\dagger Y_d)^{st} - \frac{3}{4} \delta^{pc} Y_d^{*rd} Y_u^{*ab} (Y_d^\dagger Y_d)^{st} - \frac{3}{4} \delta^{td} Y_d^{*cs} Y_u^{*ab} (Y_d Y_d^\dagger)^{pr} - \frac{3}{4} \delta^{td} Y_d^{*cs} Y_u^{*ab} (Y_u Y_u^\dagger)^{pr} - \frac{15}{16} \delta^{pa} \delta^{td} g_L^2 Y_d^{*cs} Y_u^{*rb} \\
& - \frac{5}{4} \delta^{td} Y_d^{*cs} Y_u^{*rb} (Y_u Y_u^\dagger)^{pa} \left\} C_{quqd}^{(\parallel)abcd} + \left( C_{quqd}^{(\parallel)*} \right)^{abcd} \left\{ \frac{1}{8} \delta^{rc} Y_d^{pd} Y_d^{at} (Y_d^\dagger Y_u)^{sb} + \frac{3}{4} \delta^{sd} Y_d^{ct} Y_u^{pb} (Y_d Y_d^\dagger)^{ar} + g_Y^2 \left( \frac{1}{324} \delta^{pr} \delta^{sd} Y_d^{at} Y_u^{cb} + \frac{11}{324} \delta^{ra} \delta^{st} Y_d^{pd} Y_u^{cb} \right. \right. \\
& + \frac{5}{27} \delta^{pr} \delta^{sd} Y_d^{ct} Y_u^{ab} + \frac{7}{27} \delta^{rc} \delta^{st} Y_d^{pd} Y_u^{ab} - \frac{7}{324} \delta^{rc} \delta^{st} Y_d^{ad} Y_u^{pb} - \frac{37}{144} \delta^{ra} \delta^{sd} Y_d^{ct} Y_u^{pb} - \frac{11}{27} \delta^{ra} \delta^{st} Y_d^{cd} Y_u^{pb} \left. \right) + g_s^2 \left( \frac{1}{54} \delta^{ra} \delta^{st} Y_d^{pd} Y_u^{cb} + \frac{1}{54} \delta^{rc} \delta^{st} Y_d^{ad} Y_u^{pb} \right. \\
& + 2 \delta^{rc} \delta^{sd} Y_d^{at} Y_u^{pb} - \frac{2}{27} \delta^{pr} \delta^{sd} Y_d^{at} Y_u^{cb} - \frac{2}{9} \delta^{ra} \delta^{st} Y_d^{cd} Y_u^{pb} - \frac{2}{9} \delta^{rc} \delta^{st} Y_d^{pd} Y_u^{ab} - \frac{4}{9} \delta^{pr} \delta^{sd} Y_d^{ct} Y_u^{ab} - \frac{97}{12} \delta^{ra} \delta^{sd} Y_d^{ct} Y_u^{pb} - 9 \delta^{rc} \delta^{sd} Y_d^{pt} Y_u^{ab} \left. \right)
\end{aligned}$$

$$\begin{aligned}
& -\frac{1}{8}\delta^{ra}Y_d^{pd}Y_u^{cb}(Y_d^\dagger Y_d)^{st} - \frac{1}{8}\delta^{rc}Y_d^{ad}Y_u^{pb}(Y_d^\dagger Y_d)^{st} - \frac{1}{8}\delta^{sd}Y_d^{at}Y_u^{cb}(Y_d Y_d^\dagger)^{pr} - \frac{1}{8}\delta^{sd}Y_d^{at}Y_u^{cb}(Y_u Y_u^\dagger)^{pr} - \frac{1}{8}\delta^{ra}\delta^{sd}Y_u^{pb}(Y_d Y_d^\dagger Y_d)^{ct} - \frac{1}{4}T_2\delta^{ra}\delta^{sd}Y_d^{ct}Y_u^{pb} \\
& -\frac{1}{4}\delta^{ra}\delta^{sd}Y_d^{ct}(Y_d Y_d^\dagger Y_u)^{pb} - \frac{1}{4}\delta^{ra}\delta^{sd}Y_d^{ct}(Y_u Y_u^\dagger Y_u)^{pb} - \frac{3}{8}\delta^{ra}\delta^{sd}Y_u^{pb}(Y_u Y_u^\dagger Y_d)^{ct} - \frac{5}{8}\delta^{ra}Y_d^{ct}Y_u^{pb}(Y_d^\dagger Y_d)^{sd} - \frac{3}{4}\delta^{ra}Y_d^{cd}Y_u^{pb}(Y_d^\dagger Y_d)^{st} - \frac{3}{4}\delta^{rc}Y_d^{pd}Y_u^{ab}(Y_d^\dagger Y_d)^{st} \\
& -\frac{3}{4}\delta^{sd}Y_d^{ct}Y_u^{ab}(Y_d Y_d^\dagger)^{pr} - \frac{3}{4}\delta^{sd}Y_d^{ct}Y_u^{ab}(Y_u Y_u^\dagger)^{pr} - \frac{15}{16}\delta^{ra}\delta^{sd}g_L^2Y_d^{ct}Y_u^{pb} - \frac{5}{4}\delta^{sd}Y_d^{ct}Y_u^{pb}(Y_u Y_u^\dagger)^{ar} \Bigg\} + \left\{ \frac{1}{2}\delta^{pa}Y_d^{*rd}Y_d^{*cs}(Y_u^\dagger Y_d)^{bt} + \frac{5}{8}\delta^{td}Y_d^{*as}Y_u^{*rb}(Y_d Y_d^\dagger)^{pc} \right. \\
& + g_Y^2 \left( \frac{1}{108}\delta^{pr}\delta^{td}Y_d^{*as}Y_u^{*cb} + \frac{5}{108}\delta^{pa}\delta^{st}Y_d^{*rd}Y_u^{*cb} + \frac{5}{81}\delta^{pr}\delta^{td}Y_d^{*cs}Y_u^{*ab} + \frac{11}{162}\delta^{pc}\delta^{st}Y_d^{*rd}Y_u^{*ab} + \frac{3}{4}\delta^{pc}\delta^{td}Y_d^{*as}Y_u^{*rb} - \frac{13}{108}\delta^{pc}\delta^{st}Y_d^{*ad}Y_u^{*rb} \right. \\
& - \frac{25}{162}\delta^{pa}\delta^{st}Y_d^{*cd}Y_u^{*rb} \Bigg) + g_s^2 \left( \frac{9}{4}\delta^{pa}\delta^{td}Y_d^{*cs}Y_u^{*rb} - \frac{1}{9}\delta^{pa}\delta^{st}Y_d^{*rd}Y_u^{*cb} - \frac{1}{9}\delta^{pc}\delta^{st}Y_d^{*ad}Y_u^{*rb} - \frac{7}{54}\delta^{pa}\delta^{st}Y_d^{*cd}Y_u^{*rb} - \frac{7}{54}\delta^{pc}\delta^{st}Y_d^{*rd}Y_u^{*ab} \right. \\
& - \frac{4}{27}\delta^{pr}\delta^{td}Y_d^{*cs}Y_u^{*ab} - \frac{2}{9}\delta^{pr}\delta^{td}Y_d^{*as}Y_u^{*cb} - 3\delta^{pc}\delta^{td}Y_d^{*rs}Y_u^{*ab} - \frac{9}{2}\delta^{pa}\delta^{td}Y_d^{*rs}Y_u^{*cb} - 5\delta^{pc}\delta^{td}Y_d^{*as}Y_u^{*rb} \Bigg) + \frac{9}{4}\delta^{pc}\delta^{td}g_L^2Y_d^{*as}Y_u^{*rb} \\
& - \frac{1}{8}\delta^{pc}Y_d^{*as}Y_u^{*rb}(Y_d^\dagger Y_d)^{dt} - \frac{1}{4}\delta^{pa}Y_d^{*cd}Y_u^{*rb}(Y_d^\dagger Y_d)^{st} - \frac{1}{4}\delta^{pc}Y_d^{*rd}Y_u^{*ab}(Y_d^\dagger Y_d)^{st} - \frac{1}{4}\delta^{td}Y_d^{*cs}Y_u^{*ab}(Y_d Y_d^\dagger)^{pr} - \frac{1}{4}\delta^{td}Y_d^{*cs}Y_u^{*ab}(Y_u Y_u^\dagger)^{pr} \\
& - \frac{1}{4}\delta^{td}Y_d^{*as}Y_u^{*rb}(Y_u Y_u^\dagger)^{pc} - \frac{3}{8}\delta^{pa}Y_d^{*rd}Y_u^{*cb}(Y_d^\dagger Y_d)^{st} - \frac{3}{8}\delta^{pc}Y_d^{*ad}Y_u^{*rb}(Y_d^\dagger Y_d)^{st} - \frac{3}{8}\delta^{td}Y_d^{*as}Y_u^{*cb}(Y_d Y_d^\dagger)^{pr} - \frac{3}{8}\delta^{td}Y_d^{*as}Y_u^{*cb}(Y_u Y_u^\dagger)^{pr} \\
& - \frac{1}{2}\delta^{pc}\delta^{td}Y_u^{*rb}(Y_d^\dagger Y_d Y_d^\dagger)^{as} - \frac{1}{2}\delta^{pc}\delta^{td}Y_u^{*rb}(Y_u^\dagger Y_u Y_d^\dagger)^{as} - T_2\delta^{pc}\delta^{td}Y_d^{*as}Y_u^{*rb} - \delta^{pc}\delta^{td}Y_d^{*as}(Y_u^\dagger Y_u Y_u^\dagger)^{rb} \Bigg\} C_{quqd}^{(\times)abcd} \\
& + \left( C_{quqd}^{(\times)*} \right)^{abcd} \left\{ \frac{1}{2}\delta^{ra}Y_d^{pd}Y_d^{ct}(Y_d^\dagger Y_u)^{sb} + \frac{5}{8}\delta^{sd}Y_d^{at}Y_u^{pb}(Y_d Y_d^\dagger)^{cr} + g_Y^2 \left( \frac{1}{108}\delta^{pr}\delta^{sd}Y_d^{at}Y_u^{cb} + \frac{5}{108}\delta^{ra}\delta^{st}Y_d^{pd}Y_u^{cb} + \frac{5}{81}\delta^{pr}\delta^{sd}Y_d^{ct}Y_u^{ab} + \frac{11}{162}\delta^{rc}\delta^{st}Y_d^{pd}Y_u^{ab} \right. \right. \\
& + \frac{3}{4}\delta^{rc}\delta^{sd}Y_d^{at}Y_u^{pb} - \frac{13}{108}\delta^{rc}\delta^{st}Y_d^{ad}Y_u^{pb} - \frac{25}{162}\delta^{ra}\delta^{st}Y_d^{cd}Y_u^{pb} \Bigg) + g_s^2 \left( \frac{9}{4}\delta^{ra}\delta^{sd}Y_d^{ct}Y_u^{pb} - \frac{1}{9}\delta^{ra}\delta^{st}Y_d^{pd}Y_u^{cb} - \frac{1}{9}\delta^{rc}\delta^{st}Y_d^{ad}Y_u^{pb} - \frac{7}{54}\delta^{ra}\delta^{st}Y_d^{cd}Y_u^{pb} \right. \\
& - \frac{7}{54}\delta^{rc}\delta^{st}Y_d^{pd}Y_u^{ab} - \frac{4}{27}\delta^{pr}\delta^{sd}Y_d^{ct}Y_u^{ab} - \frac{2}{9}\delta^{pr}\delta^{sd}Y_d^{at}Y_u^{cb} - 3\delta^{rc}\delta^{sd}Y_d^{pt}Y_u^{ab} - \frac{9}{2}\delta^{ra}\delta^{sd}Y_d^{pt}Y_u^{cb} - 5\delta^{rc}\delta^{sd}Y_d^{at}Y_u^{pb} \Bigg) + \frac{9}{4}\delta^{rc}\delta^{sd}g_L^2Y_d^{at}Y_u^{pb} \\
& - \frac{1}{8}\delta^{rc}Y_d^{at}Y_u^{pb}(Y_d^\dagger Y_d)^{sd} - \frac{1}{4}\delta^{ra}Y_d^{cd}Y_u^{pb}(Y_d^\dagger Y_d)^{st} - \frac{1}{4}\delta^{rc}Y_d^{pd}Y_u^{ab}(Y_d^\dagger Y_d)^{st} - \frac{1}{4}\delta^{sd}Y_d^{ct}Y_u^{ab}(Y_d Y_d^\dagger)^{pr} - \frac{1}{4}\delta^{sd}Y_d^{ct}Y_u^{ab}(Y_u Y_u^\dagger)^{pr} - \frac{1}{4}\delta^{sd}Y_d^{at}Y_u^{pb}(Y_u Y_u^\dagger)^{cr} \\
& - \frac{3}{8}\delta^{ra}Y_d^{pd}Y_u^{cb}(Y_d^\dagger Y_d)^{st} - \frac{3}{8}\delta^{rc}Y_d^{ad}Y_u^{pb}(Y_d^\dagger Y_d)^{st} - \frac{3}{8}\delta^{sd}Y_d^{at}Y_u^{cb}(Y_d Y_d^\dagger)^{pr} - \frac{3}{8}\delta^{sd}Y_d^{at}Y_u^{cb}(Y_u Y_u^\dagger)^{pr} - \frac{1}{2}\delta^{rc}\delta^{sd}Y_u^{pb}(Y_d Y_d^\dagger Y_d)^{at} - \frac{1}{2}\delta^{rc}\delta^{sd}Y_u^{pb}(Y_u Y_u^\dagger Y_d)^{at} \\
& - T_2\delta^{rc}\delta^{sd}Y_d^{at}Y_u^{pb} - \delta^{rc}\delta^{sd}Y_d^{at}(Y_u Y_u^\dagger Y_u)^{pb} \Bigg\} + \left\{ \frac{2}{27}\delta^{pc}\delta^{st}g_s^2Y_e^{*ab}Y_u^{*rd} + \frac{11}{81}\delta^{pc}\delta^{st}g_Y^2Y_e^{*ab}Y_u^{*rd} + \frac{1}{4}\delta^{pc}Y_e^{*ab}Y_u^{*rd}(Y_d^\dagger Y_d)^{st} \right\} C_{lequ}^{abcd} \\
& + C_{lequ}^{*abcd} \left\{ \frac{2}{27}\delta^{rc}\delta^{st}g_s^2Y_e^{ab}Y_u^{pd} + \frac{11}{81}\delta^{rc}\delta^{st}g_Y^2Y_e^{ab}Y_u^{pd} + \frac{1}{4}\delta^{rc}Y_e^{ab}Y_u^{pd}(Y_d^\dagger Y_d)^{st} \right\} - \left\{ \frac{1}{27}\delta^{pc}\delta^{st}g_s^2Y_e^{*ad}Y_u^{*rb} + \frac{13}{324}\delta^{pc}\delta^{st}g_Y^2Y_e^{*ad}Y_u^{*rb} \right. \\
& + \frac{1}{8}\delta^{pc}Y_e^{*ad}Y_u^{*rb}(Y_d^\dagger Y_d)^{st} \Bigg\} C_{luqe}^{abcd} - C_{luqe}^{*abcd} \left\{ \frac{1}{27}\delta^{rc}\delta^{st}g_s^2Y_e^{ad}Y_u^{pb} + \frac{13}{324}\delta^{rc}\delta^{st}g_Y^2Y_e^{ad}Y_u^{pb} + \frac{1}{8}\delta^{rc}Y_e^{ad}Y_u^{pb}(Y_d^\dagger Y_d)^{st} \right\} - \frac{8}{81}\delta^{pr}\delta^{st}\delta^{ad}\delta^{bc}g_Y^4 C_{\ell\ell}^{abcd}
\end{aligned}$$

$$\begin{aligned}
& + \left\{ g_Y^2 g_L^2 \left( \frac{58}{81} \delta^{pa} \delta^{rd} \delta^{st} \delta^{bc} - 2 \delta^{pa} \delta^{rb} \delta^{st} \delta^{cd} \right) + g_Y^2 g_s^2 \left( \frac{8}{81} \delta^{pr} \delta^{st} \delta^{ad} \delta^{bc} - \frac{130}{729} \delta^{pa} \delta^{rd} \delta^{st} \delta^{bc} - \frac{184}{243} \delta^{pa} \delta^{rb} \delta^{st} \delta^{cd} \right) + g_Y^4 \left( \frac{104}{729} \delta^{pa} \delta^{rb} \delta^{st} \delta^{cd} \right. \right. \\
& - \frac{14}{2187} \delta^{pa} \delta^{rd} \delta^{st} \delta^{bc} - \frac{8}{243} \delta^{pr} \delta^{st} \delta^{ad} \delta^{bc} \left. \right) + g_s^2 \left( \frac{8}{9} \delta^{pr} \delta^{bc} Y_d^{*as} Y_d^{dt} + \frac{10}{9} \delta^{pa} \delta^{rd} \delta^{st} (Y_d Y_d^\dagger)^{bc} + \frac{10}{9} \delta^{pa} \delta^{rd} \delta^{st} (Y_u Y_u^\dagger)^{bc} + \frac{4}{3} \delta^{pa} \delta^{bc} Y_d^{*rs} Y_d^{dt} \right. \\
& + \frac{4}{3} \delta^{rd} \delta^{bc} Y_d^{*as} Y_d^{pt} + 8 \delta^{pa} \delta^{rd} Y_d^{*cs} Y_d^{bt} + \frac{56}{3} \delta^{pa} \delta^{rb} Y_d^{*cs} Y_d^{dt} \left. \right) + g_Y^2 \left( \frac{4}{27} \delta^{pa} \delta^{rd} \delta^{st} (Y_d Y_d^\dagger)^{bc} + \frac{16}{27} \delta^{pa} \delta^{rd} \delta^{st} (Y_u Y_u^\dagger)^{bc} + \frac{8}{3} \delta^{pa} \delta^{rb} \delta^{st} (Y_u Y_u^\dagger)^{dc} \right. \\
& - \frac{4}{27} \delta^{pr} \delta^{bc} Y_d^{*as} Y_d^{dt} - \frac{83}{18} \delta^{pa} \delta^{rb} Y_d^{*cs} Y_d^{dt} \left. \right) + \delta^{pa} \delta^{rb} Y_d^{dt} (Y_u^\dagger Y_u Y_d^\dagger)^{cs} + \delta^{pa} \delta^{rb} Y_d^{*cs} (Y_u Y_u^\dagger Y_d)^{dt} + \frac{58}{27} \delta^{pa} \delta^{rd} \delta^{st} \delta^{bc} g_s^2 g_L^2 + 3 \delta^{pa} \delta^{rd} (Y_d^\dagger Y_d)^{st} (Y_u Y_u^\dagger)^{bc} \\
& + 3 \delta^{pa} \delta^{rb} Y_d^{dt} (Y_d^\dagger Y_d Y_d^\dagger)^{cs} + 3 \delta^{pa} \delta^{rb} Y_d^{*cs} (Y_d Y_d^\dagger Y_d)^{dt} + 6 T_2 \delta^{pa} \delta^{rb} Y_d^{*cs} Y_d^{dt} + 6 \delta^{pa} \delta^{rb} (Y_d^\dagger Y_d)^{st} (Y_u Y_u^\dagger)^{dc} - g_s^4 \left( \frac{8}{27} \delta^{pr} \delta^{st} \delta^{ad} \delta^{bc} \right. \\
& + \frac{2168}{243} \delta^{pa} \delta^{rd} \delta^{st} \delta^{bc} + \frac{260}{9} \delta^{pa} \delta^{rb} \delta^{st} \delta^{cd} \left. \right) - \frac{3}{2} \delta^{rd} Y_d^{*as} Y_d^{bt} (Y_d Y_d^\dagger)^{pc} - \frac{3}{2} \delta^{pa} Y_d^{*cs} Y_d^{dt} (Y_d Y_d^\dagger)^{br} - \frac{5}{2} \delta^{rd} Y_d^{*as} Y_d^{bt} (Y_u Y_u^\dagger)^{pc} - \frac{5}{2} \delta^{pa} Y_d^{*cs} Y_d^{dt} (Y_u Y_u^\dagger)^{br} \\
& - 3 \delta^{pa} \delta^{rd} (Y_d^\dagger Y_d)^{st} (Y_d Y_d^\dagger)^{bc} - 6 \delta^{pa} \delta^{rb} (Y_d^\dagger Y_d)^{st} (Y_d Y_d^\dagger)^{dc} - \frac{51}{2} \delta^{pa} \delta^{rb} g_L^2 Y_d^{*cs} Y_d^{dt} \left. \right\} C_{qq}^{(\parallel)abcd} + \left\{ \frac{1}{2} \delta^{pa} \delta^{rb} Y_d^{dt} (Y_u^\dagger Y_u Y_d^\dagger)^{cs} + \frac{1}{2} \delta^{pa} \delta^{rb} Y_d^{*cs} (Y_u Y_u^\dagger Y_d)^{dt} \right. \\
& + g_Y^2 g_s^2 \left( \frac{16}{81} \delta^{pr} \delta^{st} \delta^{ad} \delta^{bc} - \frac{260}{729} \delta^{pa} \delta^{rd} \delta^{st} \delta^{bc} - \frac{92}{243} \delta^{pa} \delta^{rb} \delta^{st} \delta^{cd} \right) + g_Y^4 \left( \frac{52}{729} \delta^{pa} \delta^{rb} \delta^{st} \delta^{cd} - \frac{28}{2187} \delta^{pa} \delta^{rd} \delta^{st} \delta^{bc} - \frac{16}{243} \delta^{pr} \delta^{st} \delta^{ad} \delta^{bc} \right) \\
& + g_Y^2 g_L^2 \left( \frac{16}{27} \delta^{pa} \delta^{rb} \delta^{st} \delta^{cd} - \frac{2}{3} \delta^{pa} \delta^{rd} \delta^{st} \delta^{bc} \right) + g_s^2 g_L^2 \left( \frac{34}{9} \delta^{pa} \delta^{rb} \delta^{st} \delta^{cd} - 2 \delta^{pa} \delta^{rd} \delta^{st} \delta^{bc} \right) + g_s^2 \left( \frac{16}{9} \delta^{pr} \delta^{bc} Y_d^{*as} Y_d^{dt} + \frac{20}{9} \delta^{pa} \delta^{rd} \delta^{st} (Y_d Y_d^\dagger)^{bc} \right. \\
& + \frac{20}{9} \delta^{pa} \delta^{rd} \delta^{st} (Y_u Y_u^\dagger)^{bc} + \frac{8}{3} \delta^{pa} \delta^{bc} Y_d^{*rs} Y_d^{dt} + \frac{8}{3} \delta^{rd} \delta^{bc} Y_d^{*as} Y_d^{pt} + \frac{28}{3} \delta^{pa} \delta^{rb} Y_d^{*cs} Y_d^{dt} + 16 \delta^{pa} \delta^{rd} Y_d^{*cs} Y_d^{bt} \left. \right) + g_Y^2 \left( \frac{8}{27} \delta^{pa} \delta^{rd} \delta^{st} (Y_d Y_d^\dagger)^{bc} \right. \\
& + \frac{32}{27} \delta^{pa} \delta^{rd} \delta^{st} (Y_u Y_u^\dagger)^{bc} + \frac{4}{3} \delta^{pa} \delta^{rb} \delta^{st} (Y_u Y_u^\dagger)^{dc} - \frac{8}{27} \delta^{pr} \delta^{bc} Y_d^{*as} Y_d^{dt} - \frac{83}{36} \delta^{pa} \delta^{rb} Y_d^{*cs} Y_d^{dt} \left. \right) + \frac{3}{2} \delta^{pa} \delta^{rb} Y_d^{dt} (Y_d^\dagger Y_d Y_d^\dagger)^{cs} + \frac{3}{2} \delta^{pa} \delta^{rb} Y_d^{*cs} (Y_d Y_d^\dagger Y_d)^{dt} \\
& + \frac{5}{2} \delta^{rd} Y_d^{*as} Y_d^{bt} (Y_u Y_u^\dagger)^{pc} + \frac{5}{2} \delta^{pa} Y_d^{*cs} Y_d^{dt} (Y_u Y_u^\dagger)^{br} + 3 T_2 \delta^{pa} \delta^{rb} Y_d^{*cs} Y_d^{dt} + 3 \delta^{pa} \delta^{rb} (Y_d^\dagger Y_d)^{st} (Y_u Y_u^\dagger)^{dc} + \frac{15}{4} \delta^{pa} \delta^{rb} g_L^2 Y_d^{*cs} Y_d^{dt} \\
& + 6 \delta^{pa} \delta^{rd} (Y_d^\dagger Y_d)^{st} (Y_u Y_u^\dagger)^{bc} - g_s^4 \left( \frac{16}{27} \delta^{pr} \delta^{st} \delta^{ad} \delta^{bc} + \frac{130}{9} \delta^{pa} \delta^{rb} \delta^{st} \delta^{cd} + \frac{4336}{243} \delta^{pa} \delta^{rd} \delta^{st} \delta^{bc} \right) - 3 \delta^{rd} Y_d^{*as} Y_d^{bt} (Y_d Y_d^\dagger)^{pc} - 3 \delta^{pa} Y_d^{*cs} Y_d^{dt} (Y_d Y_d^\dagger)^{br} \\
& - 3 \delta^{pa} \delta^{rb} (Y_d^\dagger Y_d)^{st} (Y_d Y_d^\dagger)^{dc} - 6 \delta^{pa} \delta^{rd} (Y_d^\dagger Y_d)^{st} (Y_d Y_d^\dagger)^{bc} \left. \right\} C_{qq}^{(\times)abcd} + \left\{ \delta^{pc} \delta^{rd} \delta^{st} \delta^{ab} g_Y^2 g_L^2 - \frac{448}{729} \delta^{pc} \delta^{rd} \delta^{st} \delta^{ab} g_Y^4 - \frac{8}{9} \delta^{pc} \delta^{rd} \delta^{st} g_Y^2 (Y_e Y_e^\dagger)^{ba} \right. \\
& - \frac{232}{243} \delta^{pc} \delta^{rd} \delta^{st} \delta^{ab} g_Y^2 g_s^2 - \delta^{pc} \delta^{rd} (Y_d^\dagger Y_d)^{st} (Y_e Y_e^\dagger)^{ba} \left. \right\} C_{\ell q}^{(\parallel)abcd} + \left\{ \frac{44}{81} \delta^{pc} \delta^{rd} \delta^{st} \delta^{ab} g_Y^2 g_L^2 + \frac{17}{27} \delta^{pc} \delta^{rd} \delta^{st} \delta^{ab} g_s^2 g_L^2 - \frac{224}{729} \delta^{pc} \delta^{rd} \delta^{st} \delta^{ab} g_Y^4 \right. \\
& - \frac{4}{9} \delta^{pc} \delta^{rd} \delta^{st} g_Y^2 (Y_e Y_e^\dagger)^{ba} - \frac{116}{243} \delta^{pc} \delta^{rd} \delta^{st} \delta^{ab} g_Y^2 g_s^2 - \frac{1}{2} \delta^{pc} \delta^{rd} (Y_d^\dagger Y_d)^{st} (Y_e Y_e^\dagger)^{ba} \left. \right\} C_{\ell q}^{(\times)abcd}, \tag{10.14}
\end{aligned}$$

## 10.8 $C_{qd}^{(\times)}$

$$\begin{aligned}
\beta_{C_{qd}^{(\times)prst}}^{(1)} = & \frac{2}{3} \delta^{pa} \delta^{rb} \delta^{st} \delta^{cd} g_s^2 C_{qu}^{(\times)abcd} + \left\{ \delta^{pa} \delta^{sc} Y_d^{*rd} Y_d^{bt} + \delta^{rb} \delta^{td} Y_d^{*as} Y_d^{pc} + 2\delta^{rb} \delta^{sc} Y_d^{*ad} Y_d^{pt} + 2\delta^{pa} \delta^{td} Y_d^{*rs} Y_d^{bc} - 6\delta^{pa} \delta^{rb} \delta^{sc} \delta^{td} g_s^2 \right\} C_{qd}^{(\parallel)abcd} \\
& + \left\{ \frac{1}{2} \left( \delta^{rb} \delta^{sc} \delta^{td} (Y_d Y_d^\dagger)^{pa} + \delta^{pa} \delta^{sc} \delta^{td} (Y_d Y_d^\dagger)^{br} + \delta^{rb} \delta^{sc} \delta^{td} (Y_u Y_u^\dagger)^{pa} + \delta^{pa} \delta^{sc} \delta^{td} (Y_u Y_u^\dagger)^{br} + 2\delta^{pa} \delta^{rb} \delta^{td} (Y_d^\dagger Y_d)^{sc} + 2\delta^{pa} \delta^{rb} \delta^{sc} (Y_d^\dagger Y_d)^{dt} \right. \right. \\
& + 12\delta^{rb} \delta^{sc} Y_d^{*ad} Y_d^{pt} + 12\delta^{pa} \delta^{td} Y_d^{*rs} Y_d^{bc} \Big) + \frac{2}{3} \delta^{pa} \delta^{rb} \delta^{sc} \delta^{td} g_Y^2 - \frac{2}{3} g_s^2 \left( 24\delta^{pa} \delta^{rb} \delta^{sc} \delta^{td} - \delta^{pa} \delta^{rb} \delta^{st} \delta^{cd} - 2\delta^{pr} \delta^{sc} \delta^{td} \delta^{ab} \right) \Big\} C_{qd}^{(\times)abcd} \\
& + \left\{ \frac{4}{3} \delta^{pr} \delta^{sa} \delta^{td} \delta^{bc} g_s^2 - 2\delta^{sa} \delta^{td} Y_d^{*rb} Y_d^{pc} \right\} C_{dd}^{abcd} + \left\{ \frac{2}{3} \delta^{pr} \delta^{sc} \delta^{td} \delta^{ab} g_s^2 - \delta^{sc} \delta^{td} Y_u^{*rb} Y_u^{pa} \right\} C_{ud}^{(\times)abcd} - \delta^{rd} \delta^{sc} Y_e^{*ab} C_{ledq}^{abcd} Y_d^{pt} \\
& - \delta^{pd} \delta^{tc} C_{ledq}^{*abcd} Y_d^{*rs} Y_e^{ab} + \frac{1}{2} \left\{ 2\delta^{pc} \delta^{td} Y_d^{*as} Y_u^{*rb} - \delta^{pa} \delta^{td} Y_d^{*rs} Y_u^{*cb} - 6\delta^{pc} \delta^{td} Y_d^{*rs} Y_u^{*ab} \right\} C_{quqd}^{(\parallel)abcd} + \frac{1}{2} \left( C_{quqd}^{(\parallel)*} \right)^{abcd} \left\{ 2\delta^{rc} \delta^{sd} Y_d^{at} Y_u^{pb} - \delta^{ra} \delta^{sd} Y_d^{pt} Y_u^{cb} \right. \\
& - 6\delta^{rc} \delta^{sd} Y_d^{pt} Y_u^{ab} \Big\} + \frac{1}{2} \left\{ \delta^{pa} \delta^{td} Y_d^{*cs} Y_u^{*rb} - 2\delta^{pc} \delta^{td} Y_d^{*rs} Y_u^{*ab} - 3\delta^{pa} \delta^{td} Y_d^{*rs} Y_u^{*cb} \right\} C_{quqd}^{(\times)abcd} + \frac{1}{2} \left( C_{quqd}^{(\times)*} \right)^{abcd} \left\{ \delta^{ra} \delta^{sd} Y_d^{ct} Y_u^{pb} - 2\delta^{rc} \delta^{sd} Y_d^{pt} Y_u^{ab} \right. \\
& - 3\delta^{ra} \delta^{sd} Y_d^{pt} Y_u^{cb} \Big\} + \left\{ \frac{4}{3} \delta^{pa} \delta^{rd} \delta^{st} \delta^{bc} g_s^2 - 2\delta^{pa} \delta^{rd} Y_d^{*cs} Y_d^{bt} \right\} C_{qq}^{(\parallel)abcd} + \left\{ \frac{8}{3} \delta^{pa} \delta^{rd} \delta^{st} \delta^{bc} g_s^2 - 4\delta^{pa} \delta^{rd} Y_d^{*cs} Y_d^{bt} \right\} C_{qq}^{(\times)abcd}, \tag{10.15}
\end{aligned}$$

$$\begin{aligned}
\beta_{C_{qd}^{(\times)prst}}^{(2)} = & 2Y_d^{*rs} Y_d^{pt} \mathbf{T}_{\ell H} + \left\{ \frac{1}{4} Y_d^{pt} (Y_u^\dagger Y_u Y_d^\dagger)^{rs} + \frac{1}{4} Y_d^{*rs} (Y_u Y_u^\dagger Y_d)^{pt} + \frac{3}{4} Y_d^{pt} (Y_d^\dagger Y_d Y_d^\dagger)^{rs} + \frac{3}{4} Y_d^{*rs} (Y_d Y_d^\dagger Y_d)^{pt} - \frac{1}{36} g_Y^2 Y_d^{*rs} Y_d^{pt} - \frac{1}{12} g_L^2 Y_d^{*rs} Y_d^{pt} \right. \\
& - \frac{1}{2} \lambda Y_d^{*rs} Y_d^{pt} \Big\} C_{HD}^{(\parallel)} + \left\{ \frac{3}{4} Y_d^{pt} (Y_d^\dagger Y_d Y_d^\dagger)^{rs} + \frac{3}{4} Y_d^{*rs} (Y_d Y_d^\dagger Y_d)^{pt} - \frac{1}{18} g_Y^2 Y_d^{*rs} Y_d^{pt} - \frac{1}{4} Y_d^{pt} (Y_u^\dagger Y_u Y_d^\dagger)^{rs} - \frac{1}{4} Y_d^{*rs} (Y_u Y_u^\dagger Y_d)^{pt} - \frac{1}{2} \lambda Y_d^{*rs} Y_d^{pt} \right\} C_{HD}^{(\times)} \\
& + \frac{1}{9} g_Y^4 C_{HB} Y_d^{*rs} Y_d^{pt} + 3g_L^4 C_{HW} Y_d^{*rs} Y_d^{pt} - g_s^4 \left\{ 2\delta^{st} (Y_d Y_d^\dagger)^{pr} + 2\delta^{st} (Y_u Y_u^\dagger)^{pr} + 4\delta^{pr} (Y_d^\dagger Y_d)^{st} + \frac{44}{3} Y_d^{*rs} Y_d^{pt} \right\} C_{HG} - \frac{1}{2} g_Y^2 g_L^2 C_{HWB} Y_d^{*rs} Y_d^{pt} \\
& + \left\{ 10\delta^{pr} \delta^{st} g_s^2 g_L^6 - \frac{21}{2} g_L^6 Y_d^{*rs} Y_d^{pt} \right\} C_W + \left\{ g_s^6 \left( 79Y_d^{*rs} Y_d^{pt} - \frac{9}{2} \delta^{st} (Y_d Y_d^\dagger)^{pr} - \frac{9}{2} \delta^{st} (Y_u Y_u^\dagger)^{pr} - 9\delta^{pr} (Y_d^\dagger Y_d)^{st} \right) + 7\delta^{pr} \delta^{st} g_Y^2 g_s^6 - \frac{74}{3} \delta^{pr} \delta^{st} g_s^8 \right\} C_G \\
& + \left\{ 3\delta^{pa} \delta^{tb} (Y_d^\dagger Y_d Y_d^\dagger)^{rs} - \frac{3}{2} \delta^{pa} \delta^{tb} \lambda Y_d^{*rs} \right\} C_{dH}^{ab} + C_{dH}^{*ab} \left\{ 3\delta^{ra} \delta^{sb} (Y_d Y_d^\dagger Y_d)^{pt} - \frac{3}{2} \delta^{ra} \delta^{sb} \lambda Y_d^{pt} \right\} - g_Y^2 Y_d^{*rs} Y_e^{*ab} C_{eB}^{ab} Y_d^{pt} \\
& - g_Y^2 C_{eB}^{*ab} Y_d^{*rs} Y_d^{pt} Y_e^{ab} - \frac{3}{2} g_L^2 Y_d^{*rs} Y_e^{*ab} C_{eW}^{ab} Y_d^{pt} - \frac{3}{2} g_L^2 C_{eW}^{*ab} Y_d^{*rs} Y_d^{pt} Y_e^{ab} + \left\{ g_Y^2 \left( \frac{5}{2} Y_d^{*rs} Y_u^{*ab} Y_d^{pt} - Y_d^{*as} Y_u^{*rb} Y_d^{pt} - \delta^{pa} Y_d^{*rs} (Y_u^\dagger Y_d)^{bt} \right) \right.
\end{aligned}$$

$$\begin{aligned}
& -\frac{35}{9}\delta^{pa}\delta^{st}g_Y^2g_s^2Y_u^{*rb}\left\{C_{uB}^{ab}+C_{uB}^{*ab}\left\{g_Y^2\left(\frac{5}{2}Y_d^{*rs}Y_d^{pt}Y_u^{ab}-Y_d^{*rs}Y_d^{at}Y_u^{pb}-\delta^{ra}Y_d^{pt}(Y_d^\dagger Y_u)^{sb}\right)-\frac{35}{9}\delta^{ra}\delta^{st}g_Y^2g_s^2Y_u^{pb}\right\}+\left\{g_L^2\left(\frac{9}{4}Y_d^{*rs}Y_u^{*ab}Y_d^{pt}\right.\right.\right. \\
& -\frac{3}{2}Y_d^{*as}Y_u^{*rb}Y_d^{pt}-3\delta^{pa}Y_d^{*rs}(Y_u^\dagger Y_d)^{bt})-\frac{1}{2}\delta^{pa}\delta^{st}g_s^2g_L^2Y_u^{*rb}\left\{C_{uW}^{ab}+C_{uW}^{*ab}\left\{g_L^2\left(\frac{9}{4}Y_d^{*rs}Y_d^{pt}Y_u^{ab}-\frac{3}{2}Y_d^{*rs}Y_d^{at}Y_u^{pb}-3\delta^{ra}Y_d^{pt}(Y_d^\dagger Y_u)^{sb}\right)\right.\right. \\
& -\frac{1}{2}\delta^{ra}\delta^{st}g_s^2g_L^2Y_u^{pb}\left\}+\left\{g_s^4\left(\frac{4}{3}\delta^{pr}\delta^{st}Y_u^{*ab}+\frac{53}{9}\delta^{pa}\delta^{st}Y_u^{*rb}\right)+g_s^2\left(\frac{1}{2}\delta^{st}Y_u^{*rb}(Y_d Y_d^\dagger)^{pa}+\frac{9}{2}\delta^{pa}Y_d^{*rs}(Y_u^\dagger Y_d)^{bt}+8Y_d^{*rs}Y_u^{*ab}Y_d^{pt}-\delta^{st}Y_u^{*rb}(Y_u Y_u^\dagger)^{pa}\right.\right. \\
& -3Y_d^{*as}Y_u^{*rb}Y_d^{pt}-5\delta^{pa}Y_u^{*rb}(Y_d^\dagger Y_d)^{st})-\frac{14}{9}\delta^{pa}\delta^{st}g_Y^2g_s^2Y_u^{*rb}\left\{C_{uG}^{ab}+C_{uG}^{*ab}\left\{g_s^4\left(\frac{4}{3}\delta^{pr}\delta^{st}Y_u^{ab}+\frac{53}{9}\delta^{ra}\delta^{st}Y_u^{pb}\right)+g_s^2\left(\frac{1}{2}\delta^{st}Y_u^{pb}(Y_d Y_d^\dagger)^{ar}\right.\right. \\
& +\frac{9}{2}\delta^{ra}Y_d^{pt}(Y_d^\dagger Y_u)^{sb}+8Y_d^{*rs}Y_d^{pt}Y_u^{ab}-\delta^{st}Y_u^{pb}(Y_u Y_u^\dagger)^{ar}-3Y_d^{*rs}Y_d^{at}Y_u^{pb}-5\delta^{ra}Y_u^{pb}(Y_d^\dagger Y_d)^{st})-\frac{14}{9}\delta^{ra}\delta^{st}g_Y^2g_s^2Y_u^{pb}\left\}+\left\{g_Y^2g_s^2\left(\frac{14}{9}\delta^{pr}\delta^{tb}Y_d^{*as}\right.\right. \\
& -\frac{2}{9}\delta^{pa}\delta^{tb}Y_d^{*rs}-\frac{11}{9}\delta^{pa}\delta^{st}Y_d^{*rb})+g_Y^2\left(Y_d^{*rs}Y_d^{*ab}Y_d^{pt}+\frac{4}{3}\delta^{pa}\delta^{tb}(Y_u^\dagger Y_u Y_d^\dagger)^{rs}+\frac{13}{6}\delta^{tb}Y_d^{*rs}(Y_u Y_u^\dagger)^{pa}+4\delta^{pa}\delta^{tb}Y_d^{*rs}\text{Tr}[Y_e^\dagger Y_e]-\frac{1}{6}\delta^{pa}Y_d^{*rs}(Y_d^\dagger Y_d)^{bt}\right. \\
& -\frac{1}{3}\delta^{tb}Y_d^{*rs}(Y_d Y_d^\dagger)^{pa}-\frac{3}{2}\delta^{pa}\delta^{tb}Y_d^{*rs}\text{Tr}[Y_u^\dagger Y_u])+\frac{31}{8}\delta^{pa}\delta^{tb}g_Y^2g_L^2Y_d^{*rs}-\frac{763}{216}\delta^{pa}\delta^{tb}g_Y^4Y_d^{*rs}\left\{C_{dB}^{ab}+C_{dB}^{*ab}\left\{g_Y^2g_s^2\left(\frac{14}{9}\delta^{pr}\delta^{sb}Y_d^{at}-\frac{2}{9}\delta^{ra}\delta^{sb}Y_d^{pt}\right.\right. \\
& -\frac{11}{9}\delta^{ra}\delta^{st}Y_d^{pb})+g_Y^2\left(Y_d^{*rs}Y_d^{pt}Y_d^{ab}+\frac{4}{3}\delta^{ra}\delta^{sb}(Y_u Y_u^\dagger Y_d)^{pt}+\frac{13}{6}\delta^{sb}Y_d^{pt}(Y_u Y_u^\dagger)^{ar}+4\delta^{ra}\delta^{sb}Y_d^{pt}\text{Tr}[Y_e^\dagger Y_e]-\frac{1}{6}\delta^{ra}Y_d^{pt}(Y_d^\dagger Y_d)^{sb}-\frac{1}{3}\delta^{sb}Y_d^{pt}(Y_d Y_d^\dagger)^{ar}\right. \\
& -\frac{3}{2}\delta^{ra}\delta^{sb}Y_d^{pt}\text{Tr}[Y_u^\dagger Y_u])+\frac{31}{8}\delta^{ra}\delta^{sb}g_Y^2g_L^2Y_d^{pt}-\frac{763}{216}\delta^{ra}\delta^{sb}g_Y^4Y_d^{pt}\left\}+\left\{g_s^2g_L^2\left(\delta^{pa}\delta^{tb}Y_d^{*rs}-\frac{1}{2}\delta^{pa}\delta^{st}Y_d^{*rb}-4\delta^{pr}\delta^{tb}Y_d^{*as}\right)\right. \\
& +g_L^2\left(\frac{3}{4}\delta^{pa}Y_d^{*rs}(Y_d^\dagger Y_d)^{bt}+\frac{27}{4}\delta^{pa}\delta^{tb}Y_d^{*rs}\text{Tr}[Y_u^\dagger Y_u]-\frac{3}{4}\delta^{tb}Y_d^{*rs}(Y_u Y_u^\dagger)^{pa}-3\delta^{pa}\delta^{tb}(Y_u^\dagger Y_u Y_d^\dagger)^{rs}-\frac{9}{2}Y_d^{*rs}Y_d^{*ab}Y_d^{pt}\right)-\frac{95}{48}\delta^{pa}\delta^{tb}g_Y^2g_L^2Y_d^{*rs} \\
& -\frac{69}{16}\delta^{pa}\delta^{tb}g_L^4Y_d^{*rs}\left\{C_{dW}^{ab}+C_{dW}^{*ab}\left\{g_s^2g_L^2\left(\delta^{ra}\delta^{sb}Y_d^{pt}-\frac{1}{2}\delta^{ra}\delta^{st}Y_d^{pb}-4\delta^{pr}\delta^{sb}Y_d^{at}\right)+g_L^2\left(\frac{3}{4}\delta^{ra}Y_d^{pt}(Y_d^\dagger Y_d)^{sb}+\frac{27}{4}\delta^{ra}\delta^{sb}Y_d^{pt}\text{Tr}[Y_u^\dagger Y_u]\right.\right. \\
& -\frac{3}{4}\delta^{sb}Y_d^{pt}(Y_u Y_u^\dagger)^{ar}-3\delta^{ra}\delta^{sb}(Y_u Y_u^\dagger Y_d)^{pt}-\frac{9}{2}Y_d^{*rs}Y_d^{pt}Y_d^{ab})-\frac{95}{48}\delta^{ra}\delta^{sb}g_Y^2g_L^2Y_d^{pt}-\frac{69}{16}\delta^{ra}\delta^{sb}g_L^4Y_d^{pt}\left\}+\left\{g_s^4\left(\frac{4}{3}\delta^{pr}\delta^{st}Y_d^{*ab}+\frac{23}{9}\delta^{pa}\delta^{tb}Y_d^{*rs}\right.\right. \\
& +\frac{53}{9}\delta^{pa}\delta^{st}Y_d^{*rb}+\frac{106}{9}\delta^{pr}\delta^{tb}Y_d^{*as})+g_Y^2g_s^2\left(\frac{5}{9}\delta^{pr}\delta^{tb}Y_d^{*as}+\frac{7}{9}\delta^{pa}\delta^{st}Y_d^{*rb}+\frac{199}{54}\delta^{pa}\delta^{tb}Y_d^{*rs}\right)+g_s^2\left(\frac{1}{2}\delta^{st}Y_d^{*rb}(Y_u Y_u^\dagger)^{pa}+\frac{2}{3}\delta^{pa}\delta^{tb}(Y_u^\dagger Y_u Y_d^\dagger)^{rs}\right. \\
& +\frac{19}{3}\delta^{tb}Y_d^{*rs}(Y_u Y_u^\dagger)^{pa}+8Y_d^{*rs}Y_d^{*ab}Y_d^{pt}-\text{T}_2\delta^{pa}\delta^{tb}Y_d^{*rs}-\delta^{pr}Y_d^{*as}(Y_d^\dagger Y_d)^{bt}-\delta^{st}Y_d^{*rb}(Y_d Y_d^\dagger)^{pa}-\frac{11}{6}\delta^{pa}Y_d^{*rs}(Y_d^\dagger Y_d)^{bt}-\frac{11}{3}\delta^{tb}Y_d^{*rs}(Y_d Y_d^\dagger)^{pa} \\
& \left.-5\delta^{tb}Y_d^{*as}(Y_u Y_u^\dagger)^{pr}\right)+\frac{23}{2}\delta^{pa}\delta^{tb}g_s^2g_L^2Y_d^{*rs}\left\{C_{dG}^{ab}+C_{dG}^{*ab}\left\{g_s^4\left(\frac{4}{3}\delta^{pr}\delta^{st}Y_d^{ab}+\frac{23}{9}\delta^{ra}\delta^{sb}Y_d^{pt}+\frac{53}{9}\delta^{ra}\delta^{st}Y_d^{pb}+\frac{106}{9}\delta^{pr}\delta^{sb}Y_d^{at}\right)\right.\right.
\end{aligned}$$



$$\begin{aligned}
& + g_Y^2 g_s^2 \left( \frac{5}{9} \delta^{pr} \delta^{sb} Y_d^{at} + \frac{7}{9} \delta^{ra} \delta^{st} Y_d^{pb} + \frac{199}{54} \delta^{ra} \delta^{sb} Y_d^{pt} \right) + g_s^2 \left( \frac{1}{2} \delta^{st} Y_d^{pb} (Y_u Y_u^\dagger)^{ar} + \frac{2}{3} \delta^{ra} \delta^{sb} (Y_u Y_u^\dagger Y_d)^{pt} + \frac{19}{3} \delta^{sb} Y_d^{pt} (Y_u Y_u^\dagger)^{ar} + 8 Y_d^{*rs} Y_d^{pt} Y_d^{ab} \right. \\
& - T_2 \delta^{ra} \delta^{sb} Y_d^{pt} - \delta^{pr} Y_d^{at} (Y_d^\dagger Y_d)^{sb} - \delta^{st} Y_d^{pb} (Y_d Y_d^\dagger)^{ar} - \frac{11}{6} \delta^{ra} Y_d^{pt} (Y_d^\dagger Y_d)^{sb} - \frac{11}{3} \delta^{sb} Y_d^{pt} (Y_d Y_d^\dagger)^{ar} - 5 \delta^{sb} Y_d^{at} (Y_u Y_u^\dagger)^{pr} \left. \right) + \frac{23}{2} \delta^{ra} \delta^{sb} g_s^2 g_L^2 Y_d^{pt} \Bigg\} \\
& + \left\{ \frac{2}{9} \delta^{ab} g_Y^2 Y_d^{*rs} Y_d^{pt} + \frac{2}{3} Y_d^{*rs} Y_d^{pt} (Y_e Y_e^\dagger)^{ba} \right\} C_{H\ell}^{(\parallel)ab} + \left\{ \frac{1}{9} \delta^{ab} g_Y^2 Y_d^{*rs} Y_d^{pt} + \frac{4}{3} Y_d^{*rs} Y_d^{pt} (Y_e Y_e^\dagger)^{ba} - \frac{1}{3} \delta^{ab} g_L^2 Y_d^{*rs} Y_d^{pt} \right\} C_{H\ell}^{(\times)ab} + \left\{ \frac{2}{9} \delta^{ab} g_Y^2 Y_d^{*rs} Y_d^{pt} \right. \\
& - \frac{2}{3} Y_d^{*rs} Y_d^{pt} (Y_e^\dagger Y_e)^{ba} \Bigg\} C_{He}^{ab} + \left\{ \frac{1}{2} Y_d^{*rs} Y_d^{bt} (Y_u Y_u^\dagger)^{pa} + \frac{1}{2} Y_d^{*as} Y_d^{pt} (Y_u Y_u^\dagger)^{br} + \frac{1}{2} \delta^{rb} Y_d^{pt} (Y_u^\dagger Y_u Y_d^\dagger)^{as} + \frac{1}{2} \delta^{pa} Y_d^{*rs} (Y_u Y_u^\dagger Y_d)^{bt} + g_Y^2 \left( \frac{161}{216} \delta^{pa} Y_d^{*rs} Y_d^{bt} \right. \right. \\
& + \frac{161}{216} \delta^{rb} Y_d^{*as} Y_d^{pt} - \frac{2}{9} \delta^{ab} Y_d^{*rs} Y_d^{pt} \Bigg) + g_s^2 \left( \frac{7}{18} \delta^{rb} \delta^{st} (Y_d Y_d^\dagger)^{pa} + \frac{7}{18} \delta^{pa} \delta^{st} (Y_d Y_d^\dagger)^{br} + 19 \delta^{pa} \delta^{rb} (Y_d^\dagger Y_d)^{st} - \frac{7}{18} \delta^{rb} \delta^{st} (Y_u Y_u^\dagger)^{pa} - \frac{7}{18} \delta^{pa} \delta^{st} (Y_u Y_u^\dagger)^{br} \right. \\
& - \frac{8}{3} \delta^{pa} Y_d^{*rs} Y_d^{bt} - \frac{8}{3} \delta^{rb} Y_d^{*as} Y_d^{pt} \Bigg) + \frac{5}{4} \delta^{pa} Y_d^{bt} (Y_u^\dagger Y_u Y_d^\dagger)^{rs} + \frac{5}{4} \delta^{rb} Y_d^{*as} (Y_u Y_u^\dagger Y_d)^{pt} + 2 Y_d^{*rs} Y_d^{pt} (Y_d Y_d^\dagger)^{ba} - \frac{3}{4} \delta^{pa} Y_d^{bt} (Y_d^\dagger Y_d Y_d^\dagger)^{rs} \\
& - \frac{3}{4} \delta^{rb} Y_d^{*as} (Y_d Y_d^\dagger Y_d)^{pt} - g_L^2 \left( \frac{15}{8} \delta^{pa} Y_d^{*rs} Y_d^{bt} + \frac{15}{8} \delta^{rb} Y_d^{*as} Y_d^{pt} \right) - Y_d^{*rs} Y_d^{bt} (Y_d Y_d^\dagger)^{pa} - Y_d^{*as} Y_d^{pt} (Y_d Y_d^\dagger)^{br} - 2 Y_d^{*rs} Y_d^{pt} (Y_u Y_u^\dagger)^{ba} \\
& - \frac{176}{81} \delta^{pa} \delta^{rb} \delta^{st} g_Y^2 g_s^2 - 3 \delta^{rb} Y_d^{pt} (Y_d^\dagger Y_d Y_d^\dagger)^{as} - 3 \delta^{pa} Y_d^{*rs} (Y_d Y_d^\dagger Y_d)^{bt} \Bigg\} C_{Hq}^{(\parallel)ab} + \left\{ g_L^2 \left( \frac{11}{12} \delta^{pa} Y_d^{*rs} Y_d^{bt} + \frac{11}{12} \delta^{rb} Y_d^{*as} Y_d^{pt} - \delta^{ab} Y_d^{*rs} Y_d^{pt} \right) \right. \\
& + g_Y^2 \left( \frac{19}{54} \delta^{pa} Y_d^{*rs} Y_d^{bt} + \frac{19}{54} \delta^{rb} Y_d^{*as} Y_d^{pt} - \frac{1}{9} \delta^{ab} Y_d^{*rs} Y_d^{pt} \right) + g_s^2 \left( \frac{7}{18} \delta^{rb} \delta^{st} (Y_u Y_u^\dagger)^{pa} + \frac{7}{18} \delta^{pa} \delta^{st} (Y_u Y_u^\dagger)^{br} + \frac{7}{9} \delta^{rb} \delta^{st} (Y_d Y_d^\dagger)^{pa} + \frac{7}{9} \delta^{pa} \delta^{st} (Y_d Y_d^\dagger)^{br} \right. \\
& + \frac{19}{2} \delta^{pa} \delta^{rb} (Y_d^\dagger Y_d)^{st} - \frac{16}{3} \delta^{pa} Y_d^{*rs} Y_d^{bt} - \frac{16}{3} \delta^{rb} Y_d^{*as} Y_d^{pt} \Bigg) + 2 Y_d^{*rs} Y_d^{pt} (Y_u Y_u^\dagger)^{ba} + 4 Y_d^{*rs} Y_d^{pt} (Y_d Y_d^\dagger)^{ba} - \frac{1}{2} Y_d^{*rs} Y_d^{bt} (Y_d Y_d^\dagger)^{pa} - \frac{1}{2} Y_d^{*as} Y_d^{pt} (Y_d Y_d^\dagger)^{br} \\
& - \frac{1}{2} Y_d^{*rs} Y_d^{bt} (Y_u Y_u^\dagger)^{pa} - \frac{1}{2} Y_d^{*as} Y_d^{pt} (Y_u Y_u^\dagger)^{br} - \frac{1}{2} \delta^{rb} Y_d^{pt} (Y_u^\dagger Y_u Y_d^\dagger)^{as} - \frac{1}{2} \delta^{pa} Y_d^{*rs} (Y_u Y_u^\dagger Y_d)^{bt} - \frac{88}{81} \delta^{pa} \delta^{rb} \delta^{st} g_Y^2 g_s^2 - \frac{5}{4} \delta^{pa} Y_d^{bt} (Y_u^\dagger Y_u Y_d^\dagger)^{rs} \\
& - \frac{5}{4} \delta^{rb} Y_d^{*as} (Y_u Y_u^\dagger Y_d)^{pt} - \frac{23}{18} \delta^{pa} \delta^{rb} \delta^{st} g_s^2 g_L^2 - \frac{3}{2} \delta^{rb} Y_d^{pt} (Y_d^\dagger Y_d Y_d^\dagger)^{as} - \frac{3}{2} \delta^{pa} Y_d^{*rs} (Y_d Y_d^\dagger Y_d)^{bt} - \frac{9}{4} \delta^{pa} Y_d^{bt} (Y_d^\dagger Y_d Y_d^\dagger)^{rs} \\
& - \frac{9}{4} \delta^{rb} Y_d^{*as} (Y_d Y_d^\dagger Y_d)^{pt} \Bigg\} C_{Hq}^{(\times)ab} + \left\{ 2 Y_d^{*rs} Y_d^{pt} (Y_u^\dagger Y_u)^{ba} - \frac{4}{9} \delta^{ab} g_Y^2 Y_d^{*rs} Y_d^{pt} \right\} C_{Hu}^{ab} + \left\{ \frac{1}{4} \delta^{tb} Y_d^{pa} (Y_u^\dagger Y_u Y_d^\dagger)^{rs} + \frac{1}{4} \delta^{sa} Y_d^{*rb} (Y_u Y_u^\dagger Y_d)^{pt} \right. \\
& + \frac{1}{2} Y_d^{*rb} Y_d^{pt} (Y_d^\dagger Y_d)^{sa} + \frac{1}{2} Y_d^{*rs} Y_d^{pa} (Y_d^\dagger Y_d)^{bt} + g_Y^2 \left( \frac{2}{9} \delta^{ab} Y_d^{*rs} Y_d^{pt} - \frac{91}{216} \delta^{sa} Y_d^{*rb} Y_d^{pt} - \frac{91}{216} \delta^{tb} Y_d^{*rs} Y_d^{pa} \right) + g_s^2 \left( \frac{8}{3} \delta^{sa} Y_d^{*rb} Y_d^{pt} + \frac{8}{3} \delta^{tb} Y_d^{*rs} Y_d^{pa} \right. \\
& + \frac{19}{2} \delta^{sa} \delta^{tb} (Y_u Y_u^\dagger)^{pr} - \frac{7}{9} \delta^{pr} \delta^{tb} (Y_d^\dagger Y_d)^{sa} - \frac{7}{9} \delta^{pr} \delta^{sa} (Y_d^\dagger Y_d)^{bt} - \frac{19}{2} \delta^{sa} \delta^{tb} (Y_d Y_d^\dagger)^{pr} \Bigg) + \frac{3}{2} \delta^{sa} Y_d^{pt} (Y_d^\dagger Y_d Y_d^\dagger)^{rb} + \frac{3}{2} \delta^{tb} Y_d^{*rs} (Y_d Y_d^\dagger Y_d)^{pa} \\
& + \frac{245}{162} \delta^{pr} \delta^{sa} \delta^{tb} g_Y^2 g_s^2 + \frac{9}{4} \delta^{tb} Y_d^{pa} (Y_d^\dagger Y_d Y_d^\dagger)^{rs} + \frac{9}{4} \delta^{sa} Y_d^{*rb} (Y_d Y_d^\dagger Y_d)^{pt} - g_L^2 \left( \frac{3}{8} \delta^{sa} Y_d^{*rb} Y_d^{pt} + \frac{3}{8} \delta^{tb} Y_d^{*rs} Y_d^{pa} \right) - \delta^{sa} Y_d^{pt} (Y_u^\dagger Y_u Y_d^\dagger)^{rb} \\
& - \delta^{tb} Y_d^{*rs} (Y_u Y_u^\dagger Y_d)^{pa} - 2 Y_d^{*rs} Y_d^{pt} (Y_d^\dagger Y_d)^{ba} \Bigg\} C_{Hd}^{ab} + \left\{ \frac{1}{2} Y_d^{*rs} Y_u^{pa} (Y_d^\dagger Y_d)^{bt} + \frac{1}{2} \delta^{tb} Y_d^{*rs} (Y_u Y_u^\dagger Y_u)^{pa} + g_s^2 \left( \frac{8}{3} \delta^{tb} Y_d^{*rs} Y_u^{pa} - \frac{1}{9} \delta^{pr} \delta^{tb} (Y_d^\dagger Y_u)^{sa} \right) \right.
\end{aligned}$$

$$\begin{aligned}
& + \frac{3}{2} \delta^{tb} Y_u^{pa} (Y_u^\dagger Y_u Y_d^\dagger)^{rs} - \frac{3}{8} \delta^{tb} g_L^2 Y_d^{*rs} Y_u^{pa} - \frac{59}{72} \delta^{tb} g_Y^2 Y_d^{*rs} Y_u^{pa} - 2 Y_d^{*rs} Y_d^{pt} (Y_d^\dagger Y_u)^{ba} \left\{ C_{Hud}^{ab} + C_{Hud}^{*ab} \left\{ \frac{1}{2} Y_u^{*ra} Y_d^{pt} (Y_d^\dagger Y_d)^{sb} + \frac{1}{2} \delta^{sb} Y_d^{pt} (Y_u^\dagger Y_u Y_u^\dagger)^{ra} \right. \right. \\
& + g_s^2 \left( \frac{8}{3} \delta^{sb} Y_u^{*ra} Y_d^{pt} - \frac{1}{9} \delta^{pr} \delta^{sb} (Y_u^\dagger Y_d)^{at} \right) + \frac{3}{2} \delta^{sb} Y_u^{*ra} (Y_u Y_u^\dagger Y_d)^{pt} - \frac{3}{8} \delta^{sb} g_L^2 Y_u^{*ra} Y_d^{pt} - \frac{59}{72} \delta^{sb} g_Y^2 Y_u^{*ra} Y_d^{pt} - 2 Y_d^{*rs} Y_d^{pt} (Y_u^\dagger Y_d)^{ab} \left. \right\} \\
& + 2 Y_d^{*rs} Y_e^{*ad} C_{\ell e}^{abcd} Y_d^{pt} Y_e^{bc} + \left\{ g_Y^2 \left( \frac{22}{27} \delta^{sc} \delta^{ab} Y_d^{*rd} Y_d^{pt} + \frac{22}{27} \delta^{td} \delta^{ab} Y_d^{*rs} Y_d^{pc} \right) - \frac{3}{2} \delta^{sc} Y_d^{*rd} Y_d^{pt} (Y_e Y_e^\dagger)^{ba} - \frac{3}{2} \delta^{td} Y_d^{*rs} Y_d^{pc} (Y_e Y_e^\dagger)^{ba} \right. \\
& - \frac{167}{81} \delta^{pr} \delta^{sc} \delta^{td} \delta^{ab} g_Y^2 g_s^2 \left. \right\} C_{\ell d}^{abcd} + \left\{ \frac{232}{81} \delta^{pa} \delta^{rb} \delta^{st} \delta^{cd} g_Y^2 g_s^2 - g_Y^2 \left( \frac{20}{27} \delta^{pa} \delta^{cd} Y_d^{*rs} Y_d^{bt} + \frac{20}{27} \delta^{rb} \delta^{cd} Y_d^{*as} Y_d^{pt} \right) - \frac{3}{2} \delta^{pa} Y_d^{*rs} Y_d^{bt} (Y_e^\dagger Y_e)^{dc} \right. \\
& - \frac{3}{2} \delta^{rb} Y_d^{*as} Y_d^{pt} (Y_e^\dagger Y_e)^{dc} \left. \right\} C_{qe}^{abcd} + \left\{ g_Y^2 \left( \frac{40}{27} \delta^{pa} \delta^{cd} Y_d^{*rs} Y_d^{bt} + \frac{40}{27} \delta^{rb} \delta^{cd} Y_d^{*as} Y_d^{pt} \right) + 6 Y_d^{*rs} Y_u^{*ad} Y_d^{pt} Y_u^{bc} - \frac{1}{4} Y_d^{*rs} Y_u^{*ad} Y_d^{bt} Y_u^{pc} - \frac{1}{4} Y_d^{*as} Y_u^{rd} Y_d^{pt} Y_u^{bc} \right. \\
& - \frac{3}{4} \delta^{pa} Y_u^{*rd} Y_d^{bt} (Y_d^\dagger Y_u)^{sc} - \frac{3}{4} \delta^{rb} Y_d^{*as} Y_u^{pc} (Y_u^\dagger Y_d)^{dt} - g_s^2 \left( \frac{4}{9} \delta^{pa} \delta^{st} Y_u^{*rd} Y_u^{bc} + \frac{4}{9} \delta^{rb} \delta^{st} Y_u^{*ad} Y_u^{pc} \right) - \frac{11}{3} \delta^{pa} \delta^{rb} \delta^{st} \delta^{cd} g_s^4 \\
& - \frac{464}{81} \delta^{pa} \delta^{rb} \delta^{st} \delta^{cd} g_Y^2 g_s^2 \left. \right\} C_{qu}^{(\parallel)abcd} + \left\{ g_Y^2 \left( \frac{40}{81} \delta^{pa} \delta^{cd} Y_d^{*rs} Y_d^{bt} + \frac{40}{81} \delta^{rb} \delta^{cd} Y_d^{*as} Y_d^{pt} \right) + g_s^4 \left( \frac{628}{81} \delta^{pa} \delta^{rb} \delta^{st} \delta^{cd} - \frac{4}{9} \delta^{pr} \delta^{st} \delta^{ab} \delta^{cd} \right) \right. \\
& + g_s^2 \left( \frac{2}{3} \delta^{st} \delta^{ab} Y_u^{*rd} Y_u^{pc} + \frac{2}{3} \delta^{pr} \delta^{cd} Y_d^{*as} Y_d^{bt} + \frac{2}{3} \delta^{pa} \delta^{rb} \delta^{cd} (Y_d^\dagger Y_d)^{st} - \frac{1}{3} \delta^{pa} \delta^{st} Y_u^{*rd} Y_u^{bc} - \frac{1}{3} \delta^{rb} \delta^{st} Y_u^{*ad} Y_u^{pc} - \frac{4}{3} \delta^{pa} \delta^{rb} \delta^{st} (Y_u^\dagger Y_u)^{dc} \right. \\
& - \frac{65}{27} \delta^{pa} \delta^{cd} Y_d^{*rs} Y_d^{bt} - \frac{65}{27} \delta^{rb} \delta^{cd} Y_d^{*as} Y_d^{pt} \left. \right) + 18 Y_d^{*rs} Y_u^{*ad} Y_d^{pt} Y_u^{bc} - \frac{3}{4} Y_d^{*rs} Y_u^{*ad} Y_d^{bt} Y_u^{pc} - \frac{3}{4} Y_d^{*as} Y_u^{rd} Y_d^{pt} Y_u^{bc} - \frac{3}{2} \delta^{pa} \delta^{rb} (Y_d^\dagger Y_u)^{sc} (Y_u^\dagger Y_d)^{dt} \\
& - \frac{5}{2} Y_d^{*as} Y_u^{*rd} Y_d^{bt} Y_u^{pc} - \frac{1193}{243} \delta^{pa} \delta^{rb} \delta^{st} \delta^{cd} g_Y^2 g_s^2 \left. \right\} C_{qu}^{(\times)abcd} + \left\{ \frac{1}{4} \delta^{rb} \delta^{td} Y_d^{pc} (Y_d^\dagger Y_d Y_d^\dagger)^{as} + \frac{1}{4} \delta^{pa} \delta^{sc} Y_d^{*rd} (Y_d Y_d^\dagger Y_d)^{bt} + \frac{1}{2} T_2 \delta^{pa} \delta^{sc} Y_d^{*rd} Y_d^{bt} \right. \\
& + \frac{1}{2} T_2 \delta^{rb} \delta^{td} Y_d^{*as} Y_d^{pc} + \frac{1}{2} \delta^{sc} Y_d^{*rd} Y_d^{bt} (Y_u Y_u^\dagger)^{pa} + \frac{1}{2} \delta^{td} Y_d^{*as} Y_d^{pc} (Y_u Y_u^\dagger)^{br} + \frac{1}{2} \delta^{pa} \delta^{sc} Y_d^{bt} (Y_d^\dagger Y_d Y_d^\dagger)^{rd} + \frac{1}{2} \delta^{rb} \delta^{td} Y_d^{*as} (Y_d Y_d^\dagger Y_d)^{pc} \\
& + g_L^2 \left( \frac{15}{8} \delta^{pa} \delta^{sc} Y_d^{*rd} Y_d^{bt} + \frac{15}{8} \delta^{rb} \delta^{td} Y_d^{*as} Y_d^{pc} + 3 \delta^{rb} \delta^{sc} Y_d^{*ad} Y_d^{pt} + 3 \delta^{pa} \delta^{td} Y_d^{*rs} Y_d^{bc} \right) + g_Y^2 \left( \frac{1}{9} \delta^{rb} \delta^{sc} Y_d^{*ad} Y_d^{pt} + \frac{1}{9} \delta^{pa} \delta^{td} Y_d^{*rs} Y_d^{bc} \right. \\
& + \frac{61}{72} \delta^{pa} \delta^{sc} Y_d^{*rd} Y_d^{bt} + \frac{61}{72} \delta^{rb} \delta^{td} Y_d^{*as} Y_d^{pc} - \frac{20}{27} \delta^{pa} \delta^{cd} Y_d^{*rs} Y_d^{bt} - \frac{20}{27} \delta^{rb} \delta^{cd} Y_d^{*as} Y_d^{pt} - \frac{22}{27} \delta^{sc} \delta^{ab} Y_d^{*rd} Y_d^{pt} - \frac{22}{27} \delta^{td} \delta^{ab} Y_d^{*rs} Y_d^{pc} \left. \right) \\
& + g_Y^2 g_s^2 \left( \frac{167}{81} \delta^{pr} \delta^{sc} \delta^{td} \delta^{ab} + \frac{232}{81} \delta^{pa} \delta^{rb} \delta^{st} \delta^{cd} + \frac{29}{6} \delta^{pa} \delta^{rb} \delta^{sc} \delta^{td} \right) + g_s^2 \left( \frac{2}{3} \delta^{pa} \delta^{sc} Y_d^{*rd} Y_d^{bt} + \frac{2}{3} \delta^{rb} \delta^{td} Y_d^{*as} Y_d^{pc} + 3 \delta^{rb} \delta^{sc} \delta^{td} (Y_d Y_d^\dagger)^{pa} \right. \\
& + 3 \delta^{pa} \delta^{sc} \delta^{td} (Y_d Y_d^\dagger)^{br} + 3 \delta^{rb} \delta^{sc} \delta^{td} (Y_u Y_u^\dagger)^{pa} + 3 \delta^{pa} \delta^{sc} \delta^{td} (Y_u Y_u^\dagger)^{br} + \frac{10}{3} \delta^{rb} \delta^{sc} Y_d^{*ad} Y_d^{pt} + \frac{10}{3} \delta^{pa} \delta^{td} Y_d^{*rs} Y_d^{bc} + 6 \delta^{pa} \delta^{rb} \delta^{td} (Y_d^\dagger Y_d)^{sc} \\
& + 6 \delta^{pa} \delta^{rb} \delta^{sc} (Y_d^\dagger Y_d)^{dt} - \frac{4}{9} \delta^{pa} \delta^{st} Y_d^{*rd} Y_d^{bc} - \frac{4}{9} \delta^{rb} \delta^{st} Y_d^{*ad} Y_d^{pc} - \frac{8}{9} \delta^{pr} \delta^{sc} Y_d^{*ad} Y_d^{bt} - \frac{8}{9} \delta^{pr} \delta^{td} Y_d^{*as} Y_d^{bc} \left. \right) + \frac{7}{4} \delta^{rb} \delta^{sc} Y_d^{pt} (Y_u^\dagger Y_u Y_d^\dagger)^{ad} \\
& + \frac{7}{4} \delta^{pa} \delta^{td} Y_d^{*rs} (Y_u Y_u^\dagger Y_d)^{bc} + \frac{27}{2} \delta^{pa} \delta^{rb} \delta^{sc} \delta^{td} g_s^2 g_L^2 - g_s^4 \left( \frac{11}{3} \delta^{pa} \delta^{rb} \delta^{st} \delta^{cd} + \frac{22}{3} \delta^{pr} \delta^{sc} \delta^{td} \delta^{ab} + 55 \delta^{pa} \delta^{rb} \delta^{sc} \delta^{td} \right) - \left( 3 \delta^{rb} \delta^{sc} Y_d^{*ad} Y_d^{pt} \right.
\end{aligned}$$

$$\begin{aligned}
& + 3\delta^{pa}\delta^{td}Y_d^{*rs}Y_d^{bc} \Big) \text{Tr}[Y_d^\dagger Y_d] - \frac{5}{4}\delta^{pa}Y_d^{*rd}Y_d^{bt}(Y_d^\dagger Y_d)^{sc} - \frac{5}{4}\delta^{rb}Y_d^{*as}Y_d^{pc}(Y_d^\dagger Y_d)^{dt} - \frac{5}{4}\delta^{rb}\delta^{td}Y_d^{pc}(Y_u^\dagger Y_u Y_d^\dagger)^{as} - \frac{5}{4}\delta^{pa}\delta^{sc}Y_d^{*rd}(Y_u Y_u^\dagger Y_d)^{bt} \\
& - \frac{3}{2}\delta^{pa}\delta^{sc}Y_d^{bt}(Y_u^\dagger Y_u Y_d^\dagger)^{rd} - \frac{3}{2}\delta^{rb}\delta^{td}Y_d^{*as}(Y_u Y_u^\dagger Y_d)^{pc} - \frac{5}{2}\delta^{sc}Y_d^{*rd}Y_d^{bt}(Y_d Y_d^\dagger)^{pa} - \frac{5}{2}\delta^{td}Y_d^{*as}Y_d^{pc}(Y_d Y_d^\dagger)^{br} - 6\delta^{pa}Y_d^{*rs}Y_d^{bt}(Y_d^\dagger Y_d)^{dc} \\
& - 6\delta^{rb}Y_d^{*as}Y_d^{pt}(Y_d^\dagger Y_d)^{dc} - 6\delta^{sc}Y_d^{*rd}Y_d^{pt}(Y_d Y_d^\dagger)^{ba} - 6\delta^{td}Y_d^{*rs}Y_d^{pc}(Y_d Y_d^\dagger)^{ba} - 6\delta^{rb}\delta^{sc}Y_d^{pt}(Y_d^\dagger Y_d Y_d^\dagger)^{ad} - 6\delta^{pa}\delta^{td}Y_d^{*rs}(Y_d Y_d^\dagger Y_d)^{bc} \Big\} C_{qd}^{(\text{II})} abcd \\
& + \left\{ g_s^2 g_L^2 \left( 3\delta^{pr}\delta^{sc}\delta^{td}\delta^{ab} + \frac{63}{4}\delta^{pa}\delta^{rb}\delta^{sc}\delta^{td} \right) + g_Y^2 g_s^2 \left( \frac{356}{243}\delta^{pr}\delta^{sc}\delta^{td}\delta^{ab} + \frac{610}{243}\delta^{pa}\delta^{rb}\delta^{st}\delta^{cd} + \frac{245}{36}\delta^{pa}\delta^{rb}\delta^{sc}\delta^{td} \right) + g_s^4 \left( \frac{628}{81}\delta^{pa}\delta^{rb}\delta^{st}\delta^{cd} \right. \right. \\
& + \frac{1364}{81}\delta^{pr}\delta^{sc}\delta^{td}\delta^{ab} - \frac{8}{9}\delta^{pr}\delta^{st}\delta^{ab}\delta^{cd} - \frac{357}{2}\delta^{pa}\delta^{rb}\delta^{sc}\delta^{td} \Big) + \delta^{sc}\delta^{td}(Y_d Y_d^\dagger)^{br}(Y_u Y_u^\dagger)^{pa} + \delta^{sc}\delta^{td}(Y_d Y_d^\dagger)^{pa}(Y_u Y_u^\dagger)^{br} + g_Y^2 \left( \frac{1}{3}\delta^{rb}\delta^{sc}Y_d^{*ad}Y_d^{pt} \right. \\
& + \frac{1}{3}\delta^{pa}\delta^{td}Y_d^{*rs}Y_d^{bc} + \frac{247}{144}\delta^{rb}\delta^{sc}\delta^{td}(Y_d Y_d^\dagger)^{pa} + \frac{247}{144}\delta^{pa}\delta^{sc}\delta^{td}(Y_d Y_d^\dagger)^{br} + \frac{157}{72}\delta^{pa}\delta^{rb}\delta^{td}(Y_d^\dagger Y_d)^{sc} + \frac{157}{72}\delta^{pa}\delta^{rb}\delta^{sc}(Y_d^\dagger Y_d)^{dt} - \frac{20}{81}\delta^{pa}\delta^{cd}Y_d^{*rs}Y_d^{bt} \\
& - \frac{20}{81}\delta^{rb}\delta^{cd}Y_d^{*as}Y_d^{pt} - \frac{22}{81}\delta^{sc}\delta^{ab}Y_d^{*rd}Y_d^{pt} - \frac{22}{81}\delta^{td}\delta^{ab}Y_d^{*rs}Y_d^{pc} - \frac{53}{144}\delta^{rb}\delta^{sc}\delta^{td}(Y_u Y_u^\dagger)^{pa} - \frac{53}{144}\delta^{pa}\delta^{sc}\delta^{td}(Y_u Y_u^\dagger)^{br} \Big) + g_L^2 \left( \frac{33}{16}\delta^{rb}\delta^{sc}\delta^{td}(Y_d Y_d^\dagger)^{pa} \right. \\
& + \frac{33}{16}\delta^{pa}\delta^{sc}\delta^{td}(Y_d Y_d^\dagger)^{br} + \frac{33}{16}\delta^{rb}\delta^{sc}\delta^{td}(Y_u Y_u^\dagger)^{pa} + \frac{33}{16}\delta^{pa}\delta^{sc}\delta^{td}(Y_u Y_u^\dagger)^{br} + \frac{51}{8}\delta^{pa}\delta^{rb}\delta^{td}(Y_d^\dagger Y_d)^{sc} + \frac{51}{8}\delta^{pa}\delta^{rb}\delta^{sc}(Y_d^\dagger Y_d)^{dt} + 9\delta^{rb}\delta^{sc}Y_d^{*ad}Y_d^{pt} \\
& + 9\delta^{pa}\delta^{td}Y_d^{*rs}Y_d^{bc} \Big) + g_s^2 \left( \frac{2}{3}\delta^{pa}\delta^{rb}\delta^{cd}(Y_d^\dagger Y_d)^{st} + \frac{2}{3}\delta^{sc}\delta^{td}\delta^{ab}(Y_d Y_d^\dagger)^{pr} + \frac{4}{3}\delta^{st}\delta^{ab}Y_d^{*rd}Y_d^{pc} + \frac{4}{3}\delta^{pr}\delta^{cd}Y_d^{*as}Y_d^{bt} + \frac{16}{3}\delta^{rb}\delta^{sc}\delta^{td}(Y_d Y_d^\dagger)^{pa} \right. \\
& + \frac{16}{3}\delta^{pa}\delta^{sc}\delta^{td}(Y_d Y_d^\dagger)^{br} + \frac{16}{3}\delta^{rb}\delta^{sc}\delta^{td}(Y_u Y_u^\dagger)^{pa} + \frac{16}{3}\delta^{pa}\delta^{sc}\delta^{td}(Y_u Y_u^\dagger)^{br} + 8\delta^{pa}\delta^{sc}Y_d^{*rd}Y_d^{bt} + 8\delta^{rb}\delta^{td}Y_d^{*as}Y_d^{pc} + \frac{32}{3}\delta^{pa}\delta^{rb}\delta^{td}(Y_d^\dagger Y_d)^{sc} \\
& + \frac{32}{3}\delta^{pa}\delta^{rb}\delta^{sc}(Y_d^\dagger Y_d)^{dt} + 58\delta^{rb}\delta^{sc}Y_d^{*ad}Y_d^{pt} + 58\delta^{pa}\delta^{td}Y_d^{*rs}Y_d^{bc} - \frac{1}{3}\delta^{pa}\delta^{st}Y_d^{*rd}Y_d^{bc} - \frac{1}{3}\delta^{rb}\delta^{st}Y_d^{*ad}Y_d^{pc} - \frac{2}{3}\delta^{pr}\delta^{sc}Y_d^{*ad}Y_d^{bt} - \frac{2}{3}\delta^{pr}\delta^{td}Y_d^{*as}Y_d^{bc} \\
& - \frac{4}{3}\delta^{pa}\delta^{rb}\delta^{st}(Y_d^\dagger Y_d)^{dc} - \frac{4}{3}\delta^{pr}\delta^{sc}\delta^{td}(Y_d Y_d^\dagger)^{ba} - 2\delta^{pr}\delta^{sc}\delta^{td}(Y_u Y_u^\dagger)^{ba} - \frac{65}{27}\delta^{pa}\delta^{cd}Y_d^{*rs}Y_d^{bt} - \frac{65}{27}\delta^{rb}\delta^{cd}Y_d^{*as}Y_d^{pt} - \frac{130}{27}\delta^{sc}\delta^{ab}Y_d^{*rd}Y_d^{pt} \\
& - \frac{130}{27}\delta^{td}\delta^{ab}Y_d^{*rs}Y_d^{pc} \Big) + 2\delta^{rb}\delta^{sc}(Y_d^\dagger Y_d)^{dt}(Y_d Y_d^\dagger)^{pa} + 2\delta^{pa}\delta^{td}(Y_d^\dagger Y_d)^{sc}(Y_d Y_d^\dagger)^{br} + \frac{21}{4}\delta^{rb}\delta^{sc}Y_d^{pt}(Y_u^\dagger Y_u Y_d^\dagger)^{ad} + \frac{21}{4}\delta^{pa}\delta^{td}Y_d^{*rs}(Y_u Y_u^\dagger Y_d)^{bc} \\
& - \frac{1}{4}\delta^{pa}\delta^{rb}\delta^{td}(Y_d^\dagger Y_d Y_d^\dagger Y_d)^{sc} - \frac{1}{4}\delta^{pa}\delta^{rb}\delta^{sc}(Y_d^\dagger Y_d Y_d^\dagger Y_d)^{dt} - \frac{1}{4}\delta^{pa}\delta^{rb}\delta^{td}(Y_d^\dagger Y_u Y_u^\dagger Y_d)^{sc} - \frac{1}{4}\delta^{pa}\delta^{rb}\delta^{sc}(Y_d^\dagger Y_u Y_u^\dagger Y_d)^{dt} - \frac{1}{4}\delta^{rb}\delta^{sc}\delta^{td}(Y_d Y_d^\dagger Y_d Y_d^\dagger)^{pa} \\
& - \frac{1}{4}\delta^{pa}\delta^{sc}\delta^{td}(Y_d Y_d^\dagger Y_d Y_d^\dagger)^{br} - \frac{1}{4}\delta^{rb}\delta^{sc}\delta^{td}(Y_u Y_u^\dagger Y_u Y_u^\dagger)^{pa} - \frac{1}{4}\delta^{pa}\delta^{sc}\delta^{td}(Y_u Y_u^\dagger Y_u Y_u^\dagger)^{br} - \frac{3}{4}\text{T}_2\delta^{rb}\delta^{sc}\delta^{td}(Y_d Y_d^\dagger)^{pa} - \frac{3}{4}\text{T}_2\delta^{pa}\delta^{sc}\delta^{td}(Y_d Y_d^\dagger)^{br} \\
& - \frac{3}{4}\text{T}_2\delta^{rb}\delta^{sc}\delta^{td}(Y_u Y_u^\dagger)^{pa} - \frac{3}{4}\text{T}_2\delta^{pa}\delta^{sc}\delta^{td}(Y_u Y_u^\dagger)^{br} - \delta^{rb}\delta^{td}(Y_d^\dagger Y_d)^{sc}(Y_u Y_u^\dagger)^{pa} - \delta^{pa}\delta^{sc}(Y_d^\dagger Y_d)^{dt}(Y_u Y_u^\dagger)^{br} - \left( 9\delta^{rb}\delta^{sc}Y_d^{*ad}Y_d^{pt} \right. \\
& + 9\delta^{pa}\delta^{td}Y_d^{*rs}Y_d^{bc} \Big) \text{Tr}[Y_d^\dagger Y_d] - \frac{5}{4}\delta^{rb}\delta^{td}(Y_d^\dagger Y_d)^{sc}(Y_d Y_d^\dagger)^{pa} - \frac{5}{4}\delta^{pa}\delta^{sc}(Y_d^\dagger Y_d)^{dt}(Y_d Y_d^\dagger)^{br} - \frac{3}{2}\delta^{pa}\delta^{rb}\delta^{sc}\delta^{td}g_Y^2 g_L^2 - \frac{3}{2}\text{T}_2\delta^{pa}\delta^{rb}\delta^{td}(Y_d^\dagger Y_d)^{sc} \\
& - \frac{3}{2}\text{T}_2\delta^{pa}\delta^{rb}\delta^{sc}(Y_d^\dagger Y_d)^{dt} - 2Y_d^{*rd}Y_d^{*as}Y_d^{pc}Y_d^{bt} - 2\delta^{pa}Y_d^{*rs}Y_d^{bt}(Y_d^\dagger Y_d)^{dc} - 2\delta^{rb}Y_d^{*as}Y_d^{pt}(Y_d^\dagger Y_d)^{dc} - 2\delta^{sc}Y_d^{*rd}Y_d^{pt}(Y_d Y_d^\dagger)^{ba} - 2\delta^{td}Y_d^{*rs}Y_d^{pc}(Y_d Y_d^\dagger)^{ba} \\
& - \frac{5}{2}\delta^{sc}\delta^{td}(Y_u Y_u^\dagger)^{pa}(Y_u Y_u^\dagger)^{br} - \frac{11}{4}\delta^{rb}\delta^{sc}(Y_d^\dagger Y_d)^{dt}(Y_u Y_u^\dagger)^{pa} - \frac{11}{4}\delta^{pa}\delta^{td}(Y_d^\dagger Y_d)^{sc}(Y_u Y_u^\dagger)^{br} - \frac{7}{2}\delta^{pa}\delta^{rb}(Y_d^\dagger Y_d)^{sc}(Y_d^\dagger Y_d)^{dt} - \frac{7}{2}\delta^{sc}\delta^{td}(Y_d Y_d^\dagger)^{pa}(Y_d Y_d^\dagger)^{br}
\end{aligned}$$

$$\begin{aligned}
& -\frac{479}{54}\delta^{pa}\delta^{rb}\delta^{sc}\delta^{td}g_Y^4 - 18\delta^{rb}\delta^{sc}Y_d^{pt}(Y_d^\dagger Y_d Y_d^\dagger)^{ad} - 18\delta^{pa}\delta^{td}Y_d^{*rs}(Y_d Y_d^\dagger Y_d)^{bc} \Big\} C_{qd}^{(\times)abcd} + \Big\{ \frac{8}{9}\delta^{pr}\delta^{st}\delta^{ad}\delta^{bc}g_s^4 - \frac{4}{3}\delta^{st}\delta^{ad}g_s^2Y_u^{*rb}Y_u^{pc} \Big\} C_{uu}^{abcd} \\
& + \Big\{ g_Y^2 \Big( \frac{14}{81}\delta^{tb}\delta^{ad}Y_d^{*rs}Y_d^{pc} + \frac{14}{81}\delta^{sa}\delta^{bc}Y_d^{*rd}Y_d^{pt} + \frac{44}{27}\delta^{sa}\delta^{cd}Y_d^{*rb}Y_d^{pt} + \frac{44}{27}\delta^{tb}\delta^{cd}Y_d^{*rs}Y_d^{pa} - \frac{41}{36}\delta^{sa}\delta^{td}Y_d^{*rb}Y_d^{pc} \Big) + g_s^4 \Big( \frac{4}{9}\delta^{pr}\delta^{st}\delta^{ad}\delta^{bc} \\
& + \frac{1700}{81}\delta^{pr}\delta^{sa}\delta^{td}\delta^{bc} - \frac{14}{3}\delta^{pr}\delta^{sa}\delta^{tb}\delta^{cd} \Big) + g_s^2 \Big( \frac{2}{3}\delta^{sa}\delta^{td}\delta^{bc}(Y_d Y_d^\dagger)^{pr} + 10\delta^{sa}\delta^{tb}Y_d^{*rd}Y_d^{pc} - \frac{2}{3}\delta^{st}\delta^{ad}Y_d^{*rb}Y_d^{pc} - \frac{34}{27}\delta^{tb}\delta^{ad}Y_d^{*rs}Y_d^{pc} \\
& - \frac{34}{27}\delta^{sa}\delta^{bc}Y_d^{*rd}Y_d^{pt} - \frac{14}{3}\delta^{sa}\delta^{td}Y_d^{*rb}Y_d^{pc} - \frac{20}{3}\delta^{pr}\delta^{sa}\delta^{td}(Y_d^\dagger Y_d)^{bc} \Big) + 5T_2\delta^{sa}\delta^{td}Y_d^{*rb}Y_d^{pc} + 5\delta^{sa}\delta^{td}Y_d^{pc}(Y_d^\dagger Y_d Y_d^\dagger)^{rb} + 5\delta^{sa}\delta^{td}Y_d^{*rb}(Y_d Y_d^\dagger Y_d)^{pc} \\
& - \frac{1}{2}\delta^{tb}Y_d^{*rd}Y_d^{pa}(Y_d^\dagger Y_d)^{sc} - \frac{1}{2}\delta^{sa}Y_d^{*rb}Y_d^{pc}(Y_d^\dagger Y_d)^{dt} - g_Y^2 g_s^2 \Big( \frac{88}{243}\delta^{pr}\delta^{sa}\delta^{td}\delta^{bc} + \frac{334}{81}\delta^{pr}\delta^{sa}\delta^{tb}\delta^{cd} \Big) - 3\delta^{sa}\delta^{td}Y_d^{pc}(Y_u^\dagger Y_u Y_d^\dagger)^{rb} \\
& - 3\delta^{sa}\delta^{td}Y_d^{*rb}(Y_u Y_u^\dagger Y_d)^{pc} - 6\delta^{sa}Y_d^{*rb}Y_d^{pt}(Y_d^\dagger Y_d)^{dc} - 6\delta^{tb}Y_d^{*rs}Y_d^{pa}(Y_d^\dagger Y_d)^{dc} - \frac{51}{4}\delta^{sa}\delta^{td}g_L^2Y_d^{*rb}Y_d^{pc} \Big\} C_{dd}^{abcd} + \Big\{ g_Y^2 \Big( \frac{22}{27}\delta^{sc}\delta^{ab}Y_d^{*rd}Y_d^{pt} \\
& + \frac{22}{27}\delta^{td}\delta^{ab}Y_d^{*rs}Y_d^{pc} \Big) - \frac{3}{2}\delta^{sc}Y_d^{*rd}Y_d^{pt}(Y_e^\dagger Y_e)^{ba} - \frac{3}{2}\delta^{td}Y_d^{*rs}Y_d^{pc}(Y_e^\dagger Y_e)^{ba} - \frac{167}{81}\delta^{pr}\delta^{sc}\delta^{td}\delta^{ab}g_Y^2g_s^2 \Big\} C_{ed}^{abcd} + \Big\{ \frac{1}{4}\delta^{td}Y_u^{*rb}Y_d^{pc}(Y_d^\dagger Y_u)^{sa} \\
& + \frac{1}{4}\delta^{sc}Y_d^{*rd}Y_u^{pa}(Y_u^\dagger Y_d)^{bt} + \frac{3}{4}\delta^{sc}Y_u^{*rb}Y_d^{pt}(Y_d^\dagger Y_u)^{da} + \frac{3}{4}\delta^{td}Y_d^{*rs}Y_u^{pa}(Y_u^\dagger Y_d)^{bc} + 2\delta^{sc}\delta^{td}g_s^2Y_u^{*rb}Y_u^{pa} + \frac{334}{81}\delta^{pr}\delta^{sc}\delta^{td}\delta^{ab}g_Y^2g_s^2 - \frac{1}{3}\delta^{pr}\delta^{sc}\delta^{td}\delta^{ab}g_s^4 \\
& - g_Y^2 \Big( \frac{44}{27}\delta^{sc}\delta^{ab}Y_d^{*rd}Y_d^{pt} + \frac{44}{27}\delta^{td}\delta^{ab}Y_d^{*rs}Y_d^{pc} \Big) \Big\} C_{ud}^{(\parallel)abcd} + \Big\{ \frac{163}{243}\delta^{pr}\delta^{sc}\delta^{td}\delta^{ab}g_Y^2g_s^2 + g_s^4 \Big( \frac{592}{81}\delta^{pr}\delta^{sc}\delta^{td}\delta^{ab} - \frac{2}{9}\delta^{pr}\delta^{st}\delta^{ab}\delta^{cd} \Big) \\
& + g_s^2 \Big( \frac{1}{3}\delta^{st}\delta^{ab}Y_d^{*rd}Y_d^{pc} + \frac{1}{3}\delta^{sc}\delta^{td}\delta^{ab}(Y_d Y_d^\dagger)^{pr} - \frac{4}{3}\delta^{sc}\delta^{td}Y_u^{*rb}Y_u^{pa} - 2\delta^{pr}\delta^{sc}\delta^{td}(Y_u^\dagger Y_u)^{ba} - \frac{65}{27}\delta^{sc}\delta^{ab}Y_d^{*rd}Y_d^{pt} - \frac{65}{27}\delta^{td}\delta^{ab}Y_d^{*rs}Y_d^{pc} \Big) \\
& + \frac{3}{2}T_2\delta^{sc}\delta^{td}Y_u^{*rb}Y_u^{pa} + \frac{3}{2}\delta^{sc}\delta^{td}Y_u^{pa}(Y_u^\dagger Y_u Y_u^\dagger)^{rb} + \frac{3}{2}\delta^{sc}\delta^{td}Y_u^{*rb}(Y_u Y_u^\dagger Y_u)^{pa} + \frac{9}{4}\delta^{sc}Y_u^{*rb}Y_d^{pt}(Y_d^\dagger Y_u)^{da} + \frac{9}{4}\delta^{td}Y_d^{*rs}Y_u^{pa}(Y_u^\dagger Y_d)^{bc} \\
& - \frac{1}{2}\delta^{sc}\delta^{td}Y_u^{pa}(Y_d^\dagger Y_d Y_u^\dagger)^{rb} - \frac{1}{2}\delta^{sc}\delta^{td}Y_u^{*rb}(Y_d Y_d^\dagger Y_u)^{pa} - g_Y^2 \Big( \frac{44}{81}\delta^{sc}\delta^{ab}Y_d^{*rd}Y_d^{pt} + \frac{44}{81}\delta^{td}\delta^{ab}Y_d^{*rs}Y_d^{pc} + \frac{287}{72}\delta^{sc}\delta^{td}Y_u^{*rb}Y_u^{pa} \Big) - \frac{5}{4}\delta^{td}Y_u^{*rb}Y_u^{pa}(Y_d^\dagger Y_d)^{sc} \\
& - \frac{5}{4}\delta^{sc}Y_u^{*rb}Y_u^{pa}(Y_d^\dagger Y_d)^{dt} - \frac{33}{8}\delta^{sc}\delta^{td}g_L^2Y_u^{*rb}Y_u^{pa} \Big\} C_{ud}^{(\times)abcd} + \Big\{ \frac{1}{4}\delta^{sc}Y_e^{*ab}Y_d^{pt}(Y_u Y_u^\dagger)^{dr} + g_s^2 \Big( \frac{2}{9}\delta^{rd}\delta^{st}Y_e^{*ab}Y_d^{pc} + \frac{4}{9}\delta^{pr}\delta^{sc}Y_e^{*ab}Y_d^{dt} + \delta^{rd}\delta^{sc}Y_e^{*ab}Y_d^{pt} \Big) \\
& + \frac{3}{2}Y_d^{*rs}Y_e^{*ab}Y_d^{pt}Y_d^{dc} + \frac{3}{2}\delta^{rd}\delta^{sc}Y_e^{*ab}Y_d^{pt}\text{Tr}[Y_d^\dagger Y_d] + \frac{9}{4}\delta^{rd}\delta^{sc}Y_d^{pt}(Y_e^\dagger Y_e Y_e^\dagger)^{ab} - \frac{3}{8}\delta^{rd}\delta^{sc}g_L^2Y_e^{*ab}Y_d^{pt} - \frac{55}{24}\delta^{rd}\delta^{sc}g_Y^2Y_e^{*ab}Y_d^{pt} \Big\} C_{ledq}^{abcd} \\
& + C_{ledq}^{*abcd} \Big\{ \frac{1}{4}\delta^{tc}Y_d^{*rs}Y_e^{ab}(Y_u Y_u^\dagger)^{pd} + g_s^2 \Big( \frac{2}{9}\delta^{pd}\delta^{st}Y_d^{*rc}Y_e^{ab} + \frac{4}{9}\delta^{pr}\delta^{tc}Y_d^{*ds}Y_e^{ab} + \delta^{pd}\delta^{tc}Y_d^{*rs}Y_e^{ab} \Big) + \frac{3}{2}Y_d^{*rs}Y_d^{*dc}Y_d^{pt}Y_e^{ab} + \frac{3}{2}\delta^{pd}\delta^{tc}Y_d^{*rs}Y_e^{ab}\text{Tr}[Y_d^\dagger Y_d] \\
& + \frac{9}{4}\delta^{pd}\delta^{tc}Y_d^{*rs}(Y_e Y_e^\dagger Y_e)^{ab} - \frac{3}{8}\delta^{pd}\delta^{tc}g_L^2Y_d^{*rs}Y_e^{ab} - \frac{55}{24}\delta^{pd}\delta^{tc}g_Y^2Y_d^{*rs}Y_e^{ab} \Big\} + \Big\{ \frac{1}{8}\delta^{pc}Y_d^{*as}Y_u^{*rb}(Y_d^\dagger Y_d)^{dt} + \frac{1}{8}\delta^{pc}Y_d^{*rs}Y_d^{*ad}(Y_u^\dagger Y_d)^{bt}
\end{aligned}$$

$$\begin{aligned}
& + \frac{1}{8} \delta^{td} Y_d^{*rs} Y_u^{*cb} (Y_u Y_u^\dagger)^{pa} + \frac{5}{8} \delta^{td} Y_d^{*as} Y_u^{*rb} (Y_d Y_d^\dagger)^{pc} + \frac{3}{4} Y_d^{*rs} Y_d^{*ad} Y_u^{*cb} Y_d^{pt} + \frac{3}{4} \delta^{pa} Y_d^{*rd} Y_d^{*cs} (Y_u^\dagger Y_d)^{bt} + \frac{3}{4} \delta^{pa} Y_d^{*rs} Y_d^{*cd} (Y_u^\dagger Y_d)^{bt} \\
& + \frac{3}{4} \delta^{td} Y_d^{*rs} Y_u^{*ab} (Y_u Y_u^\dagger)^{pc} + g_s^2 \left( \frac{2}{9} \delta^{pr} \delta^{td} Y_d^{*as} Y_u^{*cb} + \frac{2}{3} \delta^{pa} \delta^{st} Y_d^{*cd} Y_u^{*rb} + \frac{2}{3} \delta^{pc} \delta^{st} Y_d^{*rd} Y_u^{*ab} + \frac{4}{3} \delta^{pr} \delta^{td} Y_d^{*cs} Y_u^{*ab} + \frac{33}{4} \delta^{pa} \delta^{td} Y_d^{*cs} Y_u^{*rb} \right. \\
& + 10 \delta^{pc} \delta^{td} Y_d^{*as} Y_u^{*rb} - \frac{1}{18} \delta^{pa} \delta^{st} Y_d^{*rd} Y_u^{*cb} - \frac{1}{18} \delta^{pc} \delta^{st} Y_d^{*ad} Y_u^{*rb} - 6 \delta^{pa} \delta^{td} Y_d^{*rs} Y_u^{*cb} - 17 \delta^{pc} \delta^{td} Y_d^{*rs} Y_u^{*ab} \Big) + g_L^2 \left( \frac{9}{4} \delta^{pc} \delta^{td} Y_d^{*as} Y_u^{*rb} \right. \\
& - \frac{15}{16} \delta^{pa} \delta^{td} Y_d^{*rs} Y_u^{*cb} - \frac{9}{2} \delta^{pc} \delta^{td} Y_d^{*rs} Y_u^{*ab} \Big) + g_Y^2 \left( \frac{3}{4} \delta^{pc} \delta^{td} Y_d^{*as} Y_u^{*rb} - \frac{19}{48} \delta^{pa} \delta^{td} Y_d^{*rs} Y_u^{*cb} - \frac{13}{6} \delta^{pc} \delta^{td} Y_d^{*rs} Y_u^{*ab} \right) + \left( \frac{3}{4} \delta^{pa} \delta^{td} Y_d^{*rs} Y_u^{*cb} \right. \\
& + \frac{9}{2} \delta^{pc} \delta^{td} Y_d^{*rs} Y_u^{*ab} \Big) \text{Tr} [Y_d^\dagger Y_d] + \frac{9}{8} \delta^{pa} \delta^{td} Y_d^{*rs} (Y_u^\dagger Y_u Y_u^\dagger)^{cb} + \frac{9}{2} Y_d^{*rs} Y_d^{*cd} Y_u^{*ab} Y_d^{pt} + \frac{27}{4} \delta^{pc} \delta^{td} Y_d^{*rs} (Y_u^\dagger Y_u Y_u^\dagger)^{ab} - \frac{1}{4} \delta^{td} Y_d^{*as} Y_u^{*rb} (Y_u Y_u^\dagger)^{pc} \\
& - \frac{1}{2} Y_d^{*ad} Y_d^{*cs} Y_u^{*rb} Y_d^{pt} - \frac{1}{2} \delta^{pc} \delta^{td} Y_u^{*rb} (Y_d^\dagger Y_d Y_d^\dagger)^{as} - \frac{1}{2} \delta^{pc} \delta^{td} Y_u^{*rb} (Y_u^\dagger Y_u Y_d^\dagger)^{as} - \frac{5}{8} \delta^{pa} \delta^{td} Y_d^{*rs} (Y_d^\dagger Y_d Y_u^\dagger)^{cb} - \text{T}_2 \delta^{pc} \delta^{td} Y_d^{*as} Y_u^{*rb} \\
& - \delta^{pc} \delta^{td} Y_d^{*as} (Y_u^\dagger Y_u Y_u^\dagger)^{rb} - \frac{3}{2} Y_d^{*as} Y_d^{*cd} Y_u^{*rb} Y_d^{pt} - \frac{9}{4} \delta^{pc} \delta^{td} Y_d^{*rs} (Y_d^\dagger Y_d Y_u^\dagger)^{ab} \Big\} C_{quqd}^{(\parallel)abcd} + \left( C_{quqd}^{(\parallel)*} \right)^{abcd} \Big\{ \frac{1}{8} \delta^{rc} Y_d^{at} Y_u^{pb} (Y_d^\dagger Y_d)^{sd} + \frac{1}{8} \delta^{rc} Y_d^{pt} Y_d^{ad} (Y_d^\dagger Y_u)^{sb} \\
& + \frac{1}{8} \delta^{sd} Y_d^{pt} Y_u^{cb} (Y_u Y_u^\dagger)^{ar} + \frac{5}{8} \delta^{sd} Y_d^{at} Y_u^{pb} (Y_d Y_d^\dagger)^{cr} + \frac{3}{4} Y_d^{*rs} Y_d^{pt} Y_d^{ad} Y_u^{cb} + \frac{3}{4} \delta^{ra} Y_d^{pd} Y_d^{ct} (Y_d^\dagger Y_u)^{sb} + \frac{3}{4} \delta^{ra} Y_d^{pt} Y_d^{cd} (Y_d^\dagger Y_u)^{sb} + \frac{3}{4} \delta^{sd} Y_d^{pt} Y_u^{ab} (Y_u Y_u^\dagger)^{cr} \\
& + g_s^2 \left( \frac{2}{9} \delta^{pr} \delta^{sd} Y_d^{at} Y_u^{cb} + \frac{2}{3} \delta^{ra} \delta^{st} Y_d^{cd} Y_u^{pb} + \frac{2}{3} \delta^{rc} \delta^{st} Y_d^{pd} Y_u^{ab} + \frac{4}{3} \delta^{pr} \delta^{sd} Y_d^{ct} Y_u^{ab} + \frac{33}{4} \delta^{ra} \delta^{sd} Y_d^{ct} Y_u^{pb} + 10 \delta^{rc} \delta^{sd} Y_d^{at} Y_u^{pb} - \frac{1}{18} \delta^{ra} \delta^{st} Y_d^{pd} Y_u^{cb} \right. \\
& - \frac{1}{18} \delta^{rc} \delta^{st} Y_d^{ad} Y_u^{pb} - 6 \delta^{ra} \delta^{sd} Y_d^{pt} Y_u^{cb} - 17 \delta^{rc} \delta^{sd} Y_d^{pt} Y_u^{ab} \Big) + g_L^2 \left( \frac{9}{4} \delta^{rc} \delta^{sd} Y_d^{at} Y_u^{pb} - \frac{15}{16} \delta^{ra} \delta^{sd} Y_d^{pt} Y_u^{cb} - \frac{9}{2} \delta^{rc} \delta^{sd} Y_d^{pt} Y_u^{ab} \right) + g_Y^2 \left( \frac{3}{4} \delta^{rc} \delta^{sd} Y_d^{at} Y_u^{pb} \right. \\
& - \frac{19}{48} \delta^{ra} \delta^{sd} Y_d^{pt} Y_u^{cb} - \frac{13}{6} \delta^{rc} \delta^{sd} Y_d^{pt} Y_u^{ab} \Big) + \left( \frac{3}{4} \delta^{ra} \delta^{sd} Y_d^{pt} Y_u^{cb} + \frac{9}{2} \delta^{rc} \delta^{sd} Y_d^{pt} Y_u^{ab} \right) \text{Tr} [Y_d^\dagger Y_d] + \frac{9}{8} \delta^{ra} \delta^{sd} Y_d^{pt} (Y_u Y_u^\dagger Y_u)^{cb} + \frac{9}{2} Y_d^{*rs} Y_d^{pt} Y_d^{cd} Y_u^{ab} \\
& + \frac{27}{4} \delta^{rc} \delta^{sd} Y_d^{pt} (Y_u Y_u^\dagger Y_u)^{ab} - \frac{1}{4} \delta^{sd} Y_d^{at} Y_u^{pb} (Y_u Y_u^\dagger)^{cr} - \frac{1}{2} Y_d^{*rs} Y_d^{ad} Y_d^{ct} Y_u^{pb} - \frac{1}{2} \delta^{rc} \delta^{sd} Y_u^{pb} (Y_d Y_d^\dagger Y_d)^{at} - \frac{1}{2} \delta^{rc} \delta^{sd} Y_u^{pb} (Y_u Y_u^\dagger Y_d)^{at} \\
& - \frac{5}{8} \delta^{ra} \delta^{sd} Y_d^{pt} (Y_d Y_d^\dagger Y_u)^{cb} - \text{T}_2 \delta^{rc} \delta^{sd} Y_d^{at} Y_u^{pb} - \delta^{rc} \delta^{sd} Y_d^{at} (Y_u Y_u^\dagger Y_u)^{pb} - \frac{3}{2} Y_d^{*rs} Y_d^{at} Y_d^{cd} Y_u^{pb} - \frac{9}{4} \delta^{rc} \delta^{sd} Y_d^{pt} (Y_d Y_d^\dagger Y_u)^{ab} \Big\} + \left\{ \frac{1}{4} \delta^{pa} Y_d^{*rs} Y_d^{*cd} (Y_u^\dagger Y_d)^{bt} \right. \\
& + \frac{1}{4} \delta^{td} Y_d^{*rs} Y_u^{*ab} (Y_u Y_u^\dagger)^{pc} + \frac{3}{8} \delta^{pc} Y_d^{*rs} Y_d^{*ad} (Y_u^\dagger Y_d)^{bt} + \frac{3}{8} \delta^{td} Y_d^{*rs} Y_u^{*cb} (Y_u Y_u^\dagger)^{pa} + \frac{3}{4} \delta^{td} Y_d^{*cs} Y_u^{*rb} (Y_d Y_d^\dagger)^{pa} + g_s^2 \left( \frac{1}{3} \delta^{pa} \delta^{st} Y_d^{*rd} Y_u^{*cb} \right. \\
& + \frac{1}{3} \delta^{pc} \delta^{st} Y_d^{*ad} Y_u^{*rb} + \frac{7}{18} \delta^{pa} \delta^{st} Y_d^{*cd} Y_u^{*rb} + \frac{7}{18} \delta^{pc} \delta^{st} Y_d^{*rd} Y_u^{*ab} + \frac{4}{9} \delta^{pr} \delta^{td} Y_d^{*cs} Y_u^{*ab} + \frac{2}{3} \delta^{pr} \delta^{td} Y_d^{*as} Y_u^{*cb} + 7 \delta^{pc} \delta^{td} Y_d^{*as} Y_u^{*rb} \\
& + \frac{119}{12} \delta^{pa} \delta^{td} Y_d^{*cs} Y_u^{*rb} - \frac{17}{3} \delta^{pc} \delta^{td} Y_d^{*rs} Y_u^{*ab} - \frac{45}{2} \delta^{pa} \delta^{td} Y_d^{*rs} Y_u^{*cb} \Big) + \left( \frac{3}{2} \delta^{pc} \delta^{td} Y_d^{*rs} Y_u^{*ab} + \frac{9}{4} \delta^{pa} \delta^{td} Y_d^{*rs} Y_u^{*cb} \right) \text{Tr} [Y_d^\dagger Y_d] + \frac{3}{2} Y_d^{*rs} Y_d^{*cd} Y_u^{*ab} Y_d^{pt} \\
& + \frac{9}{4} Y_d^{*rs} Y_d^{*ad} Y_u^{*cb} Y_d^{pt} + \frac{9}{4} \delta^{pc} \delta^{td} Y_d^{*rs} (Y_u^\dagger Y_u Y_u^\dagger)^{ab} + \frac{27}{8} \delta^{pa} \delta^{td} Y_d^{*rs} (Y_u^\dagger Y_u Y_u^\dagger)^{cb} - \frac{1}{8} \delta^{pc} Y_d^{*rd} Y_d^{*as} (Y_u^\dagger Y_d)^{bt} - \frac{1}{8} \delta^{pa} \delta^{td} Y_u^{*rb} (Y_d^\dagger Y_d Y_d^\dagger)^{cs} \\
& - \frac{1}{4} \text{T}_2 \delta^{pa} \delta^{td} Y_d^{*cs} Y_u^{*rb} - \frac{1}{4} \delta^{pa} \delta^{td} Y_d^{*cs} (Y_d^\dagger Y_d Y_u^\dagger)^{rb} - \frac{1}{4} \delta^{pa} \delta^{td} Y_d^{*cs} (Y_u^\dagger Y_u Y_u^\dagger)^{rb} - \frac{3}{8} \delta^{pa} \delta^{td} Y_u^{*rb} (Y_u^\dagger Y_u Y_d^\dagger)^{cs} - \frac{1}{2} Y_d^{*as} Y_d^{*cd} Y_u^{*rb} Y_d^{pt} \\
& - \frac{3}{4} \delta^{pc} \delta^{td} Y_d^{*rs} (Y_d^\dagger Y_d Y_u^\dagger)^{ab} - \frac{7}{8} \delta^{pa} Y_d^{*cs} Y_u^{*rb} (Y_d^\dagger Y_d)^{dt} - g_Y^2 \left( \frac{37}{144} \delta^{pa} \delta^{td} Y_d^{*cs} Y_u^{*rb} + \frac{13}{18} \delta^{pc} \delta^{td} Y_d^{*rs} Y_u^{*ab} + \frac{19}{16} \delta^{pa} \delta^{td} Y_d^{*rs} Y_u^{*cb} \right)
\end{aligned}$$

$$\begin{aligned}
& -g_L^2 \left( \frac{15}{16} \delta^{pa} \delta^{td} Y_d^{*cs} Y_u^{*rb} + \frac{3}{2} \delta^{pc} \delta^{td} Y_d^{*rs} Y_u^{*ab} + \frac{45}{16} \delta^{pa} \delta^{td} Y_d^{*rs} Y_u^{*cb} \right) - \frac{5}{4} \delta^{td} Y_d^{*cs} Y_u^{*rb} (Y_u Y_u^\dagger)^{pa} - \frac{3}{2} Y_d^{*ad} Y_d^{*cs} Y_u^{*rb} Y_d^{pt} \\
& - \frac{15}{8} \delta^{pa} \delta^{td} Y_d^{*rs} (Y_d^\dagger Y_d Y_u^\dagger)^{cb} \left\{ C_{quqd}^{(\times)abcd} + \left( C_{quqd}^{(\times)*} \right)^{abcd} \left\{ \frac{1}{4} \delta^{ra} Y_d^{pt} Y_d^{cd} (Y_d^\dagger Y_u)^{sb} + \frac{1}{4} \delta^{sd} Y_d^{pt} Y_u^{ab} (Y_u Y_u^\dagger)^{cr} + \frac{3}{8} \delta^{rc} Y_d^{pt} Y_d^{ad} (Y_d^\dagger Y_u)^{sb} + \frac{3}{8} \delta^{sd} Y_d^{pt} Y_u^{cb} (Y_u Y_u^\dagger)^{ar} \right. \right. \\
& + \frac{3}{4} \delta^{sd} Y_d^{ct} Y_u^{pb} (Y_d Y_d^\dagger)^{ar} + g_s^2 \left( \frac{1}{3} \delta^{ra} \delta^{st} Y_d^{pd} Y_u^{cb} + \frac{1}{3} \delta^{rc} \delta^{st} Y_d^{ad} Y_u^{pb} + \frac{7}{18} \delta^{ra} \delta^{st} Y_d^{cd} Y_u^{pb} + \frac{7}{18} \delta^{rc} \delta^{st} Y_d^{pd} Y_u^{ab} + \frac{4}{9} \delta^{pr} \delta^{sd} Y_d^{ct} Y_u^{ab} + \frac{2}{3} \delta^{pr} \delta^{sd} Y_d^{at} Y_u^{cb} \right. \\
& + 7 \delta^{rc} \delta^{sd} Y_d^{at} Y_u^{pb} + \frac{119}{12} \delta^{ra} \delta^{sd} Y_d^{ct} Y_u^{pb} - \frac{17}{3} \delta^{rc} \delta^{sd} Y_d^{pt} Y_u^{ab} - \frac{45}{2} \delta^{ra} \delta^{sd} Y_d^{pt} Y_u^{cb} \left. \right) + \left( \frac{3}{2} \delta^{rc} \delta^{sd} Y_d^{pt} Y_u^{ab} + \frac{9}{4} \delta^{ra} \delta^{sd} Y_d^{pt} Y_u^{cb} \right) \text{Tr} \left[ Y_d^\dagger Y_d \right] + \frac{3}{2} Y_d^{*rs} Y_d^{pt} Y_d^{cd} Y_u^{ab} \\
& + \frac{9}{4} Y_d^{*rs} Y_d^{pt} Y_d^{ad} Y_u^{cb} + \frac{9}{4} \delta^{rc} \delta^{sd} Y_d^{pt} (Y_u Y_u^\dagger Y_u)^{ab} + \frac{27}{8} \delta^{ra} \delta^{sd} Y_d^{pt} (Y_u Y_u^\dagger Y_u)^{cb} - \frac{1}{8} \delta^{rc} Y_d^{pd} Y_d^{at} (Y_d^\dagger Y_u)^{sb} - \frac{1}{8} \delta^{ra} \delta^{sd} Y_u^{pb} (Y_d Y_d^\dagger Y_d)^{ct} - \frac{1}{4} \text{T}_2 \delta^{ra} \delta^{sd} Y_d^{ct} Y_u^{pb} \\
& - \frac{1}{4} \delta^{ra} \delta^{sd} Y_d^{ct} (Y_d Y_d^\dagger Y_u)^{pb} - \frac{1}{4} \delta^{ra} \delta^{sd} Y_d^{ct} (Y_u Y_u^\dagger Y_u)^{pb} - \frac{3}{8} \delta^{ra} \delta^{sd} Y_u^{pb} (Y_u Y_u^\dagger Y_d)^{ct} - \frac{1}{2} Y_d^{*rs} Y_d^{at} Y_d^{cd} Y_u^{pb} - \frac{3}{4} \delta^{rc} \delta^{sd} Y_d^{pt} (Y_d Y_d^\dagger Y_u)^{ab} - \frac{7}{8} \delta^{ra} Y_d^{ct} Y_u^{pb} (Y_d^\dagger Y_d)^{sd} \\
& - g_Y^2 \left( \frac{37}{144} \delta^{ra} \delta^{sd} Y_d^{ct} Y_u^{pb} + \frac{13}{18} \delta^{rc} \delta^{sd} Y_d^{pt} Y_u^{ab} + \frac{19}{16} \delta^{ra} \delta^{sd} Y_d^{pt} Y_u^{cb} \right) - g_L^2 \left( \frac{15}{16} \delta^{ra} \delta^{sd} Y_d^{ct} Y_u^{pb} + \frac{3}{2} \delta^{rc} \delta^{sd} Y_d^{pt} Y_u^{ab} + \frac{45}{16} \delta^{ra} \delta^{sd} Y_d^{pt} Y_u^{cb} \right) - \frac{5}{4} \delta^{sd} Y_d^{ct} Y_u^{pb} (Y_u Y_u^\dagger)^{ar} \\
& - \frac{3}{2} Y_d^{*rs} Y_d^{ad} Y_d^{ct} Y_u^{pb} - \frac{15}{8} \delta^{ra} \delta^{sd} Y_d^{pt} (Y_d Y_d^\dagger Y_u)^{cb} \left. \right\} - \left\{ \frac{2}{9} \delta^{pc} \delta^{st} g_s^2 Y_e^{*ab} Y_u^{*rd} + \frac{1}{4} \delta^{pc} Y_d^{*rs} Y_e^{*ab} (Y_u^\dagger Y_d)^{dt} \right\} C_{lequ}^{abcd} - C_{lequ}^{*abcd} \left\{ \frac{2}{9} \delta^{rc} \delta^{st} g_s^2 Y_e^{ab} Y_u^{pd} \right. \\
& + \frac{1}{4} \delta^{rc} Y_d^{pt} Y_e^{ab} (Y_d^\dagger Y_u)^{sd} \left. \right\} + \left\{ \frac{1}{9} \delta^{pc} \delta^{st} g_s^2 Y_e^{*ad} Y_u^{*rb} + \frac{1}{8} \delta^{pc} Y_d^{*rs} Y_e^{*ad} (Y_u^\dagger Y_d)^{bt} - \frac{1}{4} Y_d^{*cs} Y_e^{*ad} Y_u^{*rb} Y_d^{pt} \right\} C_{luqe}^{abcd} + C_{luqe}^{*abcd} \left\{ \frac{1}{9} \delta^{rc} \delta^{st} g_s^2 Y_e^{ad} Y_u^{pb} \right. \\
& + \frac{1}{8} \delta^{rc} Y_d^{pt} Y_e^{ad} (Y_d^\dagger Y_u)^{sb} - \frac{1}{4} Y_d^{*rs} Y_d^{ct} Y_e^{ad} Y_u^{pb} \left. \right\} + \left\{ g_L^2 \left( \frac{5}{3} \delta^{pa} \delta^{bc} Y_d^{*rs} Y_d^{dt} + \frac{5}{3} \delta^{rd} \delta^{bc} Y_d^{*as} Y_d^{pt} + \frac{33}{4} \delta^{pa} \delta^{rd} Y_d^{*cs} Y_d^{bt} \right) + g_Y^2 \left( \frac{40}{27} \delta^{pa} \delta^{cd} Y_d^{*rs} Y_d^{bt} \right. \right. \\
& + \frac{40}{27} \delta^{rb} \delta^{cd} Y_d^{*as} Y_d^{pt} - \frac{1}{81} \delta^{pa} \delta^{bc} Y_d^{*rs} Y_d^{dt} - \frac{1}{81} \delta^{rd} \delta^{bc} Y_d^{*as} Y_d^{pt} - \frac{125}{36} \delta^{pa} \delta^{rd} Y_d^{*cs} Y_d^{bt} \left. \right) + g_s^4 \left( \frac{8}{9} \delta^{pr} \delta^{st} \delta^{ad} \delta^{bc} + \frac{1592}{81} \delta^{pa} \delta^{rd} \delta^{st} \delta^{bc} \right. \\
& - \frac{28}{3} \delta^{pa} \delta^{rb} \delta^{st} \delta^{cd} \left. \right) + g_Y^2 g_s^2 \left( \frac{86}{243} \delta^{pa} \delta^{rd} \delta^{st} \delta^{bc} - \frac{464}{81} \delta^{pa} \delta^{rb} \delta^{st} \delta^{cd} \right) + \delta^{rb} Y_d^{*as} Y_d^{dt} (Y_u Y_u^\dagger)^{pc} + g_s^2 \left( \frac{4}{3} \delta^{pa} \delta^{rd} \delta^{bc} (Y_d^\dagger Y_d)^{st} + 20 \delta^{pa} \delta^{rb} Y_d^{*cs} Y_d^{dt} \right. \\
& - \frac{34}{27} \delta^{pa} \delta^{bc} Y_d^{*rs} Y_d^{dt} - \frac{34}{27} \delta^{rd} \delta^{bc} Y_d^{*as} Y_d^{pt} - \frac{4}{3} \delta^{pr} \delta^{bc} Y_d^{*as} Y_d^{dt} - \frac{10}{3} \delta^{pa} \delta^{rd} \delta^{st} (Y_d Y_d^\dagger)^{bc} - \frac{10}{3} \delta^{pa} \delta^{rd} \delta^{st} (Y_u Y_u^\dagger)^{bc} - \frac{14}{3} \delta^{pa} \delta^{rd} Y_d^{*cs} Y_d^{bt} \left. \right) \\
& + \delta^{pa} Y_d^{*cs} Y_d^{bt} (Y_u Y_u^\dagger)^{dr} + \frac{3}{2} \delta^{pa} Y_d^{*rs} Y_d^{dt} (Y_u Y_u^\dagger)^{bc} + \frac{3}{2} \delta^{rd} Y_d^{*as} Y_d^{pt} (Y_u Y_u^\dagger)^{bc} + \frac{5}{2} \delta^{pa} \delta^{rd} Y_d^{bt} (Y_d^\dagger Y_d Y_d^\dagger)^{cs} + \frac{5}{2} \delta^{pa} \delta^{rd} Y_d^{*cs} (Y_d Y_d^\dagger Y_d)^{bt} \\
& + 5 \text{T}_2 \delta^{pa} \delta^{rd} Y_d^{*cs} Y_d^{bt} - \frac{1}{2} \delta^{pa} \delta^{rd} Y_d^{bt} (Y_u^\dagger Y_u Y_d^\dagger)^{cs} - \frac{1}{2} \delta^{pa} \delta^{rd} Y_d^{*cs} (Y_u Y_u^\dagger Y_d)^{bt} - \delta^{rb} Y_d^{*as} Y_d^{dt} (Y_d Y_d^\dagger)^{pc} - \delta^{pa} Y_d^{*cs} Y_d^{bt} (Y_d Y_d^\dagger)^{dr} \\
& - 6 \delta^{pa} Y_d^{*rs} Y_d^{bt} (Y_d Y_d^\dagger)^{dc} - 6 \delta^{rb} Y_d^{*as} Y_d^{pt} (Y_d Y_d^\dagger)^{dc} - \frac{58}{9} \delta^{pa} \delta^{rd} \delta^{st} \delta^{bc} g_s^2 g_L^2 \left. \right\} C_{qq}^{(\parallel)abcd} + \left\{ g_Y^2 \left( \frac{20}{27} \delta^{pa} \delta^{cd} Y_d^{*rs} Y_d^{bt} + \frac{20}{27} \delta^{rb} \delta^{cd} Y_d^{*as} Y_d^{pt} \right. \right. \\
& - \frac{2}{81} \delta^{pa} \delta^{bc} Y_d^{*rs} Y_d^{dt} - \frac{2}{81} \delta^{rd} \delta^{bc} Y_d^{*as} Y_d^{pt} - \frac{125}{18} \delta^{pa} \delta^{rd} Y_d^{*cs} Y_d^{bt} \left. \right) + g_L^2 \left( 8 \delta^{pa} \delta^{cd} Y_d^{*rs} Y_d^{bt} + 8 \delta^{rb} \delta^{cd} Y_d^{*as} Y_d^{pt} - \frac{69}{2} \delta^{pa} \delta^{rd} Y_d^{*cs} Y_d^{bt} \right)
\end{aligned}$$

$$\begin{aligned}
& + g_s^2 g_L^2 \left( 6 \delta^{pa} \delta^{rd} \delta^{st} \delta^{bc} - \frac{34}{3} \delta^{pa} \delta^{rb} \delta^{st} \delta^{cd} \right) + g_s^4 \left( \frac{16}{9} \delta^{pr} \delta^{st} \delta^{ad} \delta^{bc} + \frac{3184}{81} \delta^{pa} \delta^{rd} \delta^{st} \delta^{bc} - \frac{14}{3} \delta^{pa} \delta^{rb} \delta^{st} \delta^{cd} \right) + g_Y^2 g_s^2 \left( \frac{172}{243} \delta^{pa} \delta^{rd} \delta^{st} \delta^{bc} \right. \\
& - \frac{232}{81} \delta^{pa} \delta^{rb} \delta^{st} \delta^{cd} \left. \right) + g_s^2 \left( \frac{8}{3} \delta^{pa} \delta^{rd} \delta^{bc} (Y_d^\dagger Y_d)^{st} + 10 \delta^{pa} \delta^{rb} Y_d^{*cs} Y_d^{dt} - \frac{68}{27} \delta^{pa} \delta^{bc} Y_d^{*rs} Y_d^{dt} - \frac{68}{27} \delta^{rd} \delta^{bc} Y_d^{*as} Y_d^{pt} - \frac{8}{3} \delta^{pr} \delta^{bc} Y_d^{*as} Y_d^{dt} \right. \\
& - \frac{20}{3} \delta^{pa} \delta^{rd} \delta^{st} (Y_d Y_d^\dagger)^{bc} - \frac{20}{3} \delta^{pa} \delta^{rd} \delta^{st} (Y_u Y_u^\dagger)^{bc} - \frac{28}{3} \delta^{pa} \delta^{rd} Y_d^{*cs} Y_d^{bt} \left. \right) + 5 \delta^{pa} \delta^{rd} Y_d^{bt} (Y_d^\dagger Y_d Y_d^\dagger)^{cs} + 5 \delta^{pa} \delta^{rd} Y_d^{*cs} (Y_d Y_d^\dagger Y_d)^{bt} \\
& + 10 T_2 \delta^{pa} \delta^{rd} Y_d^{*cs} Y_d^{bt} - \frac{1}{2} \delta^{rb} Y_d^{*as} Y_d^{dt} (Y_d Y_d^\dagger)^{pc} - \frac{1}{2} \delta^{pa} Y_d^{*cs} Y_d^{bt} (Y_d Y_d^\dagger)^{dr} - \delta^{rb} Y_d^{*as} Y_d^{dt} (Y_u Y_u^\dagger)^{pc} - \delta^{pa} Y_d^{*cs} Y_d^{bt} (Y_u Y_u^\dagger)^{dr} - \delta^{pa} \delta^{rd} Y_d^{bt} (Y_u^\dagger Y_u Y_d^\dagger)^{cs} \\
& - \delta^{pa} \delta^{rd} Y_d^{*cs} (Y_u Y_u^\dagger Y_d)^{bt} - \frac{3}{2} \delta^{pa} Y_d^{*rs} Y_d^{dt} (Y_u Y_u^\dagger)^{bc} - \frac{3}{2} \delta^{rd} Y_d^{*as} Y_d^{pt} (Y_u Y_u^\dagger)^{bc} - 12 \delta^{pa} Y_d^{*rs} Y_d^{bt} (Y_d Y_d^\dagger)^{dc} - 12 \delta^{rb} Y_d^{*as} Y_d^{pt} (Y_d Y_d^\dagger)^{dc} \left. \right\} C_{qq}^{(\times)abcd} \\
& + \left\{ \frac{232}{81} \delta^{pc} \delta^{rd} \delta^{st} \delta^{ab} g_Y^2 g_s^2 - g_Y^2 \left( \frac{20}{27} \delta^{pc} \delta^{ab} Y_d^{*rs} Y_d^{dt} + \frac{20}{27} \delta^{rd} \delta^{ab} Y_d^{*cs} Y_d^{pt} \right) - \frac{3}{2} \delta^{pc} Y_d^{*rs} Y_d^{dt} (Y_e Y_e^\dagger)^{ba} - \frac{3}{2} \delta^{rd} Y_d^{*cs} Y_d^{pt} (Y_e Y_e^\dagger)^{ba} \right\} C_{\ell q}^{(\parallel)abcd} \\
& + \left\{ g_L^2 \left( \frac{4}{3} \delta^{pc} \delta^{ab} Y_d^{*rs} Y_d^{dt} + \frac{4}{3} \delta^{rd} \delta^{ab} Y_d^{*cs} Y_d^{pt} \right) + \frac{116}{81} \delta^{pc} \delta^{rd} \delta^{st} \delta^{ab} g_Y^2 g_s^2 - g_Y^2 \left( \frac{10}{27} \delta^{pc} \delta^{ab} Y_d^{*rs} Y_d^{dt} + \frac{10}{27} \delta^{rd} \delta^{ab} Y_d^{*cs} Y_d^{pt} \right) - \frac{17}{9} \delta^{pc} \delta^{rd} \delta^{st} \delta^{ab} g_s^2 g_L^2 \right. \\
& \left. - 3 \delta^{pc} Y_d^{*rs} Y_d^{dt} (Y_e Y_e^\dagger)^{ba} - 3 \delta^{rd} Y_d^{*cs} Y_d^{pt} (Y_e Y_e^\dagger)^{ba} \right\} C_{\ell q}^{(\times)abcd}, \tag{10.16}
\end{aligned}$$

## 11 $(\bar{R}R)(\bar{R}R)$

### 11.1 $C_{ee}$

$$\begin{aligned}
\beta_{C_{ee}^{prst}}^{(1)} & = \left\{ \frac{1}{2} \left( \delta^{sa} \delta^{tb} (Y_e^\dagger Y_e)^{pr} + \delta^{rb} \delta^{sa} (Y_e^\dagger Y_e)^{pt} + \delta^{pa} \delta^{tb} (Y_e^\dagger Y_e)^{sr} + \delta^{pa} \delta^{rb} (Y_e^\dagger Y_e)^{st} \right) - \frac{1}{6} g_Y^2 \left( \delta^{pa} \delta^{rb} \delta^{st} + \delta^{pt} \delta^{rb} \delta^{sa} + \delta^{pa} \delta^{rs} \delta^{tb} + \delta^{pr} \delta^{sa} \delta^{tb} \right) \right\} C_{He}^{ab} \\
& + \left\{ \frac{1}{3} g_Y^2 \left( \delta^{pc} \delta^{rd} \delta^{st} \delta^{ab} + \delta^{pt} \delta^{rd} \delta^{sc} \delta^{ab} + \delta^{pc} \delta^{rs} \delta^{td} \delta^{ab} + \delta^{pr} \delta^{sc} \delta^{td} \delta^{ab} \right) + \frac{1}{2} \left( -\delta^{pc} \delta^{rd} Y_e^{*as} Y_e^{bt} - \delta^{rd} \delta^{sc} Y_e^{*ap} Y_e^{bt} - \delta^{pc} \delta^{td} Y_e^{*as} Y_e^{br} \right. \right. \\
& \left. \left. - \delta^{sc} \delta^{td} Y_e^{*ap} Y_e^{br} \right) \right\} C_{\ell e}^{abcd} - \frac{1}{3} g_Y^2 \left\{ \delta^{pc} \delta^{rd} \delta^{st} \delta^{ab} + \delta^{pt} \delta^{rd} \delta^{sc} \delta^{ab} + \delta^{pc} \delta^{rs} \delta^{td} \delta^{ab} + \delta^{pr} \delta^{sc} \delta^{td} \delta^{ab} \right\} C_{qe}^{abcd} + \left\{ \delta^{rb} \delta^{sa} \delta^{td} (Y_e^\dagger Y_e)^{pc} + \delta^{pa} \delta^{rb} \delta^{td} (Y_e^\dagger Y_e)^{sc} \right. \\
& + \delta^{pa} \delta^{sc} \delta^{tb} (Y_e^\dagger Y_e)^{dr} + \delta^{pa} \delta^{rb} \delta^{sc} (Y_e^\dagger Y_e)^{dt} + \frac{4}{3} g_Y^2 \left( \delta^{pa} \delta^{rb} \delta^{st} \delta^{cd} + \delta^{pt} \delta^{rb} \delta^{sa} \delta^{cd} + \delta^{pa} \delta^{rs} \delta^{tb} \delta^{cd} + \delta^{pr} \delta^{sa} \delta^{tb} \delta^{cd} + 9 \delta^{pa} \delta^{rb} \delta^{sc} \delta^{td} \right) \left. \right\} C_{ee}^{abcd} \\
& - \frac{2}{3} g_Y^2 \left\{ \delta^{pa} \delta^{rb} \delta^{st} \delta^{cd} + \delta^{pt} \delta^{rb} \delta^{sa} \delta^{cd} + \delta^{pa} \delta^{rs} \delta^{tb} \delta^{cd} + \delta^{pr} \delta^{sa} \delta^{tb} \delta^{cd} \right\} C_{eu}^{abcd} + \frac{1}{3} g_Y^2 \left\{ \delta^{pa} \delta^{rb} \delta^{st} \delta^{cd} + \delta^{pt} \delta^{rb} \delta^{sa} \delta^{cd} + \delta^{pa} \delta^{rs} \delta^{tb} \delta^{cd} \right.
\end{aligned}$$

$$+ \delta^{pr} \delta^{sa} \delta^{tb} \delta^{cd} \left\} C_{ed}^{abcd}, \quad (11.1)$$

$$\begin{aligned} \beta_{C_{ee}^{prst}}^{(2)} = & \left\{ g_Y^6 \left( \frac{2}{3} \delta^{pt} \delta^{rs} + \frac{2}{3} \delta^{pr} \delta^{st} \right) - g_Y^4 \left( \frac{5}{2} \delta^{st} (Y_e^\dagger Y_e)^{pr} + \frac{5}{2} \delta^{rs} (Y_e^\dagger Y_e)^{pt} + \frac{5}{2} \delta^{pt} (Y_e^\dagger Y_e)^{sr} + \frac{5}{2} \delta^{pr} (Y_e^\dagger Y_e)^{st} \right) \right\} C_{HB} + \left\{ g_Y^4 g_L^2 \left( \frac{1}{2} \delta^{pt} \delta^{rs} + \frac{1}{2} \delta^{pr} \delta^{st} \right) \right. \\ & - g_Y^2 g_L^2 \left( \frac{3}{8} \delta^{st} (Y_e^\dagger Y_e)^{pr} + \frac{3}{8} \delta^{rs} (Y_e^\dagger Y_e)^{pt} + \frac{3}{8} \delta^{pt} (Y_e^\dagger Y_e)^{sr} + \frac{3}{8} \delta^{pr} (Y_e^\dagger Y_e)^{st} \right) \left. \right\} C_{HWB} + \left\{ g_Y^4 \left( 5 \delta^{pt} \delta^{rb} Y_e^{*as} + 5 \delta^{rb} \delta^{st} Y_e^{*ap} + 5 \delta^{pr} \delta^{tb} Y_e^{*as} \right. \right. \\ & + 5 \delta^{rs} \delta^{tb} Y_e^{*ap} - \delta^{pt} \delta^{rs} Y_e^{*ab} - \delta^{pr} \delta^{st} Y_e^{*ab} \left. \right) + g_Y^2 \left( \frac{1}{2} \delta^{pt} Y_e^{*as} (Y_e^\dagger Y_e)^{br} + \frac{1}{2} \delta^{st} Y_e^{*ap} (Y_e^\dagger Y_e)^{br} + \frac{1}{2} \delta^{pr} Y_e^{*as} (Y_e^\dagger Y_e)^{bt} + \frac{1}{2} \delta^{rs} Y_e^{*ap} (Y_e^\dagger Y_e)^{bt} \right. \\ & - \frac{15}{4} \delta^{tb} Y_e^{*as} (Y_e^\dagger Y_e)^{pr} - \frac{15}{4} \delta^{rb} Y_e^{*as} (Y_e^\dagger Y_e)^{pt} - \frac{15}{4} \delta^{tb} Y_e^{*ap} (Y_e^\dagger Y_e)^{sr} - \frac{15}{4} \delta^{rb} Y_e^{*ap} (Y_e^\dagger Y_e)^{st} \left. \right) \left\} C_{eB}^{ab} + C_{eB}^{*ab} \left\{ g_Y^4 \left( 5 \delta^{pb} \delta^{rs} Y_e^{at} + 5 \delta^{pb} \delta^{st} Y_e^{ar} \right. \right. \right. \\ & + 5 \delta^{pr} \delta^{sb} Y_e^{at} + 5 \delta^{pt} \delta^{sb} Y_e^{ar} - \delta^{pt} \delta^{rs} Y_e^{ab} - \delta^{pr} \delta^{st} Y_e^{ab} \left. \right) + g_Y^2 \left( \frac{1}{2} \delta^{rs} Y_e^{at} (Y_e^\dagger Y_e)^{pb} + \frac{1}{2} \delta^{st} Y_e^{ar} (Y_e^\dagger Y_e)^{pb} + \frac{1}{2} \delta^{pr} Y_e^{at} (Y_e^\dagger Y_e)^{sb} + \frac{1}{2} \delta^{pt} Y_e^{ar} (Y_e^\dagger Y_e)^{sb} \right. \\ & - \frac{15}{4} \delta^{sb} Y_e^{at} (Y_e^\dagger Y_e)^{pr} - \frac{15}{4} \delta^{sb} Y_e^{ar} (Y_e^\dagger Y_e)^{pt} - \frac{15}{4} \delta^{pb} Y_e^{at} (Y_e^\dagger Y_e)^{sr} - \frac{15}{4} \delta^{pb} Y_e^{ar} (Y_e^\dagger Y_e)^{st} \left. \right) \left\} + \left\{ g_L^2 \left( \frac{9}{8} \delta^{tb} Y_e^{*as} (Y_e^\dagger Y_e)^{pr} + \frac{9}{8} \delta^{rb} Y_e^{*as} (Y_e^\dagger Y_e)^{pt} \right. \right. \right. \\ & + \frac{9}{8} \delta^{tb} Y_e^{*ap} (Y_e^\dagger Y_e)^{sr} + \frac{9}{8} \delta^{rb} Y_e^{*ap} (Y_e^\dagger Y_e)^{st} \left. \right) - g_Y^2 g_L^2 \left( \frac{5}{4} \delta^{pt} \delta^{rb} Y_e^{*as} + \frac{5}{4} \delta^{rb} \delta^{st} Y_e^{*ap} + \frac{5}{4} \delta^{pr} \delta^{tb} Y_e^{*as} + \frac{5}{4} \delta^{rs} \delta^{tb} Y_e^{*ap} \right) \left\} C_{eW}^{ab} \right. \\ & + C_{eW}^{*ab} \left\{ g_L^2 \left( \frac{9}{8} \delta^{sb} Y_e^{at} (Y_e^\dagger Y_e)^{pr} + \frac{9}{8} \delta^{sb} Y_e^{ar} (Y_e^\dagger Y_e)^{pt} + \frac{9}{8} \delta^{pb} Y_e^{at} (Y_e^\dagger Y_e)^{sr} + \frac{9}{8} \delta^{pb} Y_e^{ar} (Y_e^\dagger Y_e)^{st} \right) - g_Y^2 g_L^2 \left( \frac{5}{4} \delta^{pb} \delta^{rs} Y_e^{at} + \frac{5}{4} \delta^{pb} \delta^{st} Y_e^{ar} + \frac{5}{4} \delta^{pr} \delta^{sb} Y_e^{at} \right. \right. \\ & + \frac{5}{4} \delta^{pt} \delta^{sb} Y_e^{ar} \left. \right) \left\} + g_Y^4 \left\{ \frac{5}{3} \delta^{pt} \delta^{rs} Y_u^{*ab} + \frac{5}{3} \delta^{pr} \delta^{st} Y_u^{*ab} \right\} C_{uB}^{ab} + g_Y^4 C_{uB}^{*ab} \left\{ \frac{5}{3} \delta^{pt} \delta^{rs} Y_u^{ab} + \frac{5}{3} \delta^{pr} \delta^{st} Y_u^{ab} \right\} - g_Y^4 \left\{ \frac{1}{3} \delta^{pt} \delta^{rs} Y_d^{*ab} + \frac{1}{3} \delta^{pr} \delta^{st} Y_d^{*ab} \right\} C_{dB}^{ab} \\ & - g_Y^4 C_{dB}^{*ab} \left\{ \frac{1}{3} \delta^{pt} \delta^{rs} Y_d^{ab} + \frac{1}{3} \delta^{pr} \delta^{st} Y_d^{ab} \right\} + \left\{ \frac{1}{8} \delta^{tb} (Y_e^\dagger Y_e)^{pa} (Y_e^\dagger Y_e)^{sr} + \frac{1}{8} \delta^{rb} (Y_e^\dagger Y_e)^{pa} (Y_e^\dagger Y_e)^{st} + \frac{1}{8} \delta^{tb} (Y_e^\dagger Y_e)^{pr} (Y_e^\dagger Y_e)^{sa} + \frac{1}{8} \delta^{rb} (Y_e^\dagger Y_e)^{pt} (Y_e^\dagger Y_e)^{sa} \right. \\ & + \frac{1}{8} \delta^{sa} (Y_e^\dagger Y_e)^{pt} (Y_e^\dagger Y_e)^{br} + \frac{1}{8} \delta^{pa} (Y_e^\dagger Y_e)^{st} (Y_e^\dagger Y_e)^{br} + \frac{1}{8} \delta^{sa} (Y_e^\dagger Y_e)^{pr} (Y_e^\dagger Y_e)^{bt} + \frac{1}{8} \delta^{pa} (Y_e^\dagger Y_e)^{sr} (Y_e^\dagger Y_e)^{bt} + g_Y^4 \left( \frac{1}{9} \delta^{pt} \delta^{rs} \delta^{ab} + \frac{1}{9} \delta^{pr} \delta^{st} \delta^{ab} + \frac{67}{54} \delta^{pa} \delta^{rb} \delta^{st} \right. \\ & + \frac{67}{54} \delta^{pt} \delta^{rb} \delta^{sa} + \frac{67}{54} \delta^{pa} \delta^{rs} \delta^{tb} + \frac{67}{54} \delta^{pr} \delta^{sa} \delta^{tb} \left. \right) + g_L^2 \left( \frac{51}{16} \delta^{sa} \delta^{tb} (Y_e^\dagger Y_e)^{pr} + \frac{51}{16} \delta^{rb} \delta^{sa} (Y_e^\dagger Y_e)^{pt} + \frac{51}{16} \delta^{pa} \delta^{tb} (Y_e^\dagger Y_e)^{sr} + \frac{51}{16} \delta^{pa} \delta^{rb} (Y_e^\dagger Y_e)^{st} \right) \\ & + g_Y^2 \left( \left( \frac{1}{2} \delta^{pa} \delta^{rb} \delta^{st} + \frac{1}{2} \delta^{pt} \delta^{rb} \delta^{sa} + \frac{1}{2} \delta^{pa} \delta^{rs} \delta^{tb} + \frac{1}{2} \delta^{pr} \delta^{sa} \delta^{tb} \right) \text{Tr} [Y_d^\dagger Y_d] + \left( \frac{1}{2} \delta^{pa} \delta^{rb} \delta^{st} + \frac{1}{2} \delta^{pt} \delta^{rb} \delta^{sa} + \frac{1}{2} \delta^{pa} \delta^{rs} \delta^{tb} + \frac{1}{2} \delta^{pr} \delta^{sa} \delta^{tb} \right) \text{Tr} [Y_u^\dagger Y_u] \right. \\ & - \frac{1}{6} \delta^{st} \delta^{ab} (Y_e^\dagger Y_e)^{pr} - \frac{1}{6} \delta^{rs} \delta^{ab} (Y_e^\dagger Y_e)^{pt} - \frac{1}{6} \delta^{pt} \delta^{ab} (Y_e^\dagger Y_e)^{sr} - \frac{1}{6} \delta^{pr} \delta^{ab} (Y_e^\dagger Y_e)^{st} - \frac{31}{72} \delta^{rb} \delta^{st} (Y_e^\dagger Y_e)^{pa} - \frac{31}{72} \delta^{rs} \delta^{tb} (Y_e^\dagger Y_e)^{pa} - \frac{31}{72} \delta^{pt} \delta^{rb} (Y_e^\dagger Y_e)^{sa} \end{aligned}$$



$$\begin{aligned}
& -\frac{31}{72}\delta^{pr}\delta^{tb}(Y_e^\dagger Y_e)^{sa} - \frac{31}{72}\delta^{pa}\delta^{st}(Y_e^\dagger Y_e)^{br} - \frac{31}{72}\delta^{pt}\delta^{sa}(Y_e^\dagger Y_e)^{br} - \frac{31}{72}\delta^{pa}\delta^{rs}(Y_e^\dagger Y_e)^{bt} - \frac{31}{72}\delta^{pr}\delta^{sa}(Y_e^\dagger Y_e)^{bt} - \frac{43}{16}\delta^{sa}\delta^{tb}(Y_e^\dagger Y_e)^{pr} \\
& - \frac{43}{16}\delta^{rb}\delta^{sa}(Y_e^\dagger Y_e)^{pt} - \frac{43}{16}\delta^{pa}\delta^{tb}(Y_e^\dagger Y_e)^{sr} - \frac{43}{16}\delta^{pa}\delta^{rb}(Y_e^\dagger Y_e)^{st} - \frac{1}{2}\text{T}_2\delta^{sa}\delta^{tb}(Y_e^\dagger Y_e)^{pr} - \frac{1}{2}\text{T}_2\delta^{rb}\delta^{sa}(Y_e^\dagger Y_e)^{pt} - \frac{1}{2}\text{T}_2\delta^{pa}\delta^{tb}(Y_e^\dagger Y_e)^{sr} \\
& - \frac{1}{2}\text{T}_2\delta^{pa}\delta^{rb}(Y_e^\dagger Y_e)^{st} - \frac{3}{4}\delta^{sa}\delta^{tb}(Y_e^\dagger Y_e Y_e^\dagger Y_e)^{pr} - \frac{3}{4}\delta^{rb}\delta^{sa}(Y_e^\dagger Y_e Y_e^\dagger Y_e)^{pt} - \frac{3}{4}\delta^{pa}\delta^{tb}(Y_e^\dagger Y_e Y_e^\dagger Y_e)^{sr} - \frac{3}{4}\delta^{pa}\delta^{rb}(Y_e^\dagger Y_e Y_e^\dagger Y_e)^{st} \\
& - g_Y^2 g_L^2 \left( \frac{3}{2}\delta^{pa}\delta^{rb}\delta^{st} + \frac{3}{2}\delta^{pt}\delta^{rb}\delta^{sa} + \frac{3}{2}\delta^{pa}\delta^{rs}\delta^{tb} + \frac{3}{2}\delta^{pr}\delta^{sa}\delta^{tb} \right) \Big\} C_{He}^{ab} + \left\{ \frac{3}{8}\delta^{rd}\delta^{sc}Y_e^{bt}(Y_e^\dagger Y_e Y_e^\dagger)^{ap} + \frac{3}{8}\delta^{sc}\delta^{td}Y_e^{br}(Y_e^\dagger Y_e Y_e^\dagger)^{ap} \right. \\
& + \frac{3}{8}\delta^{pc}\delta^{rd}Y_e^{bt}(Y_e^\dagger Y_e Y_e^\dagger)^{as} + \frac{3}{8}\delta^{pc}\delta^{td}Y_e^{br}(Y_e^\dagger Y_e Y_e^\dagger)^{as} + \frac{3}{8}\delta^{pc}\delta^{td}Y_e^{*as}(Y_e Y_e^\dagger Y_e)^{br} + \frac{3}{8}\delta^{sc}\delta^{td}Y_e^{*ap}(Y_e Y_e^\dagger Y_e)^{br} + \frac{3}{8}\delta^{pc}\delta^{rd}Y_e^{*as}(Y_e Y_e^\dagger Y_e)^{bt} \\
& + \frac{3}{8}\delta^{rd}\delta^{sc}Y_e^{*ap}(Y_e Y_e^\dagger Y_e)^{bt} + \frac{1}{2}\delta^{sc}Y_e^{*ad}Y_e^{bt}(Y_e^\dagger Y_e)^{pr} + \frac{1}{2}\delta^{td}Y_e^{*as}Y_e^{bc}(Y_e^\dagger Y_e)^{pr} + \frac{1}{2}\delta^{rd}Y_e^{*as}Y_e^{bc}(Y_e^\dagger Y_e)^{pt} + \frac{1}{2}\delta^{sc}Y_e^{*ad}Y_e^{br}(Y_e^\dagger Y_e)^{pt} \\
& + \frac{1}{2}\delta^{pc}Y_e^{*ad}Y_e^{bt}(Y_e^\dagger Y_e)^{sr} + \frac{1}{2}\delta^{td}Y_e^{*ap}Y_e^{bc}(Y_e^\dagger Y_e)^{sr} + \frac{1}{2}\delta^{pc}Y_e^{*ad}Y_e^{br}(Y_e^\dagger Y_e)^{st} + \frac{1}{2}\delta^{rd}Y_e^{*ap}Y_e^{bc}(Y_e^\dagger Y_e)^{st} + \frac{3}{4}\text{T}_2\delta^{pc}\delta^{rd}Y_e^{*as}Y_e^{bt} + \frac{3}{4}\text{T}_2\delta^{rd}\delta^{sc}Y_e^{*ap}Y_e^{bt} \\
& + \frac{3}{4}\text{T}_2\delta^{pc}\delta^{td}Y_e^{*as}Y_e^{br} + \frac{3}{4}\text{T}_2\delta^{sc}\delta^{td}Y_e^{*ap}Y_e^{br} + \frac{7}{8}\delta^{rd}Y_e^{*as}Y_e^{bt}(Y_e^\dagger Y_e)^{pc} + \frac{7}{8}\delta^{td}Y_e^{*as}Y_e^{br}(Y_e^\dagger Y_e)^{pc} + \frac{7}{8}\delta^{rd}Y_e^{*ap}Y_e^{bt}(Y_e^\dagger Y_e)^{sc} + \frac{7}{8}\delta^{td}Y_e^{*ap}Y_e^{br}(Y_e^\dagger Y_e)^{sc} \\
& + \frac{7}{8}\delta^{pc}Y_e^{*as}Y_e^{bt}(Y_e^\dagger Y_e)^{dr} + \frac{7}{8}\delta^{sc}Y_e^{*ap}Y_e^{bt}(Y_e^\dagger Y_e)^{dr} + \frac{7}{8}\delta^{pc}Y_e^{*as}Y_e^{br}(Y_e^\dagger Y_e)^{dt} + \frac{7}{8}\delta^{sc}Y_e^{*ap}Y_e^{br}(Y_e^\dagger Y_e)^{dt} + g_Y^2 g_L^2 \left( \frac{3}{4}\delta^{pc}\delta^{rd}\delta^{st}\delta^{ab} + \frac{3}{4}\delta^{pt}\delta^{rd}\delta^{sc}\delta^{ab} \right. \\
& + \frac{3}{4}\delta^{pc}\delta^{rs}\delta^{td}\delta^{ab} + \frac{3}{4}\delta^{pr}\delta^{sc}\delta^{td}\delta^{ab} \Big) + g_Y^2 \left( \frac{1}{6}\delta^{pr}\delta^{cd}Y_e^{*as}Y_e^{bt} + \frac{1}{6}\delta^{pt}\delta^{cd}Y_e^{*as}Y_e^{br} + \frac{1}{6}\delta^{rs}\delta^{cd}Y_e^{*ap}Y_e^{bt} + \frac{1}{6}\delta^{st}\delta^{cd}Y_e^{*ap}Y_e^{br} - \frac{5}{18}\delta^{pc}\delta^{rs}Y_e^{*ad}Y_e^{bt} \right. \\
& - \frac{5}{18}\delta^{pt}\delta^{rd}Y_e^{*as}Y_e^{bc} - \frac{5}{18}\delta^{pc}\delta^{st}Y_e^{*ad}Y_e^{br} - \frac{5}{18}\delta^{rd}\delta^{st}Y_e^{*ap}Y_e^{bc} - \frac{5}{18}\delta^{pr}\delta^{sc}Y_e^{*ad}Y_e^{bt} - \frac{5}{18}\delta^{pt}\delta^{sc}Y_e^{*ad}Y_e^{br} - \frac{5}{18}\delta^{pr}\delta^{td}Y_e^{*as}Y_e^{bc} \\
& - \frac{5}{18}\delta^{rs}\delta^{td}Y_e^{*ap}Y_e^{bc} - \frac{1}{2}\delta^{pc}\delta^{rd}\delta^{st}(Y_e Y_e^\dagger)^{ba} - \frac{1}{2}\delta^{pt}\delta^{rd}\delta^{sc}(Y_e Y_e^\dagger)^{ba} - \frac{1}{2}\delta^{pc}\delta^{rs}\delta^{td}(Y_e Y_e^\dagger)^{ba} - \frac{1}{2}\delta^{pr}\delta^{sc}\delta^{td}(Y_e Y_e^\dagger)^{ba} - \frac{25}{16}\delta^{pc}\delta^{rd}Y_e^{*as}Y_e^{bt} \\
& - \frac{25}{16}\delta^{rd}\delta^{sc}Y_e^{*ap}Y_e^{bt} - \frac{25}{16}\delta^{pc}\delta^{td}Y_e^{*as}Y_e^{br} - \frac{25}{16}\delta^{sc}\delta^{td}Y_e^{*ap}Y_e^{br} \Big) - \frac{1}{4}\delta^{sc}\delta^{td}(Y_e^\dagger Y_e)^{pr}(Y_e Y_e^\dagger)^{ba} - \frac{1}{4}\delta^{rd}\delta^{sc}(Y_e^\dagger Y_e)^{pt}(Y_e Y_e^\dagger)^{ba} - \frac{1}{4}\delta^{pc}\delta^{td}(Y_e^\dagger Y_e)^{sr}(Y_e Y_e^\dagger)^{ba} \\
& - \frac{1}{4}\delta^{pc}\delta^{rd}(Y_e^\dagger Y_e)^{st}(Y_e Y_e^\dagger)^{ba} - g_L^2 \left( \frac{51}{16}\delta^{pc}\delta^{rd}Y_e^{*as}Y_e^{bt} + \frac{51}{16}\delta^{rd}\delta^{sc}Y_e^{*ap}Y_e^{bt} + \frac{51}{16}\delta^{pc}\delta^{td}Y_e^{*as}Y_e^{br} + \frac{51}{16}\delta^{sc}\delta^{td}Y_e^{*ap}Y_e^{br} \right) - g_Y^4 \left( \frac{2}{9}\delta^{pt}\delta^{rs}\delta^{ab}\delta^{cd} \right. \\
& + \frac{2}{9}\delta^{pr}\delta^{st}\delta^{ab}\delta^{cd} + \frac{445}{108}\delta^{pc}\delta^{rd}\delta^{st}\delta^{ab} + \frac{445}{108}\delta^{pt}\delta^{rd}\delta^{sc}\delta^{ab} + \frac{445}{108}\delta^{pc}\delta^{rs}\delta^{td}\delta^{ab} + \frac{445}{108}\delta^{pr}\delta^{sc}\delta^{td}\delta^{ab} \Big) \Big\} C_{le}^{abcd} + \left\{ \frac{3}{4}\delta^{sc}\delta^{td}(Y_e^\dagger Y_e)^{pr}(Y_u Y_u^\dagger)^{ba} \right. \\
& + \frac{3}{4}\delta^{rd}\delta^{sc}(Y_e^\dagger Y_e)^{pt}(Y_u Y_u^\dagger)^{ba} + \frac{3}{4}\delta^{pc}\delta^{td}(Y_e^\dagger Y_e)^{sr}(Y_u Y_u^\dagger)^{ba} + \frac{3}{4}\delta^{pc}\delta^{rd}(Y_e^\dagger Y_e)^{st}(Y_u Y_u^\dagger)^{ba} + g_Y^4 \left( \frac{2}{9}\delta^{pt}\delta^{rs}\delta^{ab}\delta^{cd} + \frac{2}{9}\delta^{pr}\delta^{st}\delta^{ab}\delta^{cd} - \frac{11}{108}\delta^{pc}\delta^{rd}\delta^{st}\delta^{ab} \right. \\
& - \frac{11}{108}\delta^{pt}\delta^{rd}\delta^{sc}\delta^{ab} - \frac{11}{108}\delta^{pc}\delta^{rs}\delta^{td}\delta^{ab} - \frac{11}{108}\delta^{pr}\delta^{sc}\delta^{td}\delta^{ab} \Big) + g_Y^2 \left( \delta^{pc}\delta^{rd}\delta^{st}(Y_u Y_u^\dagger)^{ba} + \delta^{pt}\delta^{rd}\delta^{sc}(Y_u Y_u^\dagger)^{ba} + \delta^{pc}\delta^{rs}\delta^{td}(Y_u Y_u^\dagger)^{ba} \right. \\
& + \delta^{pr}\delta^{sc}\delta^{td}(Y_u Y_u^\dagger)^{ba} \Big) - \frac{3}{4}\delta^{sc}\delta^{td}(Y_e^\dagger Y_e)^{pr}(Y_d Y_d^\dagger)^{ba} - \frac{3}{4}\delta^{rd}\delta^{sc}(Y_e^\dagger Y_e)^{pt}(Y_d Y_d^\dagger)^{ba} - \frac{3}{4}\delta^{pc}\delta^{td}(Y_e^\dagger Y_e)^{sr}(Y_d Y_d^\dagger)^{ba} - \frac{3}{4}\delta^{pc}\delta^{rd}(Y_e^\dagger Y_e)^{st}(Y_d Y_d^\dagger)^{ba} \\
& - g_Y^2 g_L^2 \left( \frac{3}{4}\delta^{pc}\delta^{rd}\delta^{st}\delta^{ab} + \frac{3}{4}\delta^{pt}\delta^{rd}\delta^{sc}\delta^{ab} + \frac{3}{4}\delta^{pc}\delta^{rs}\delta^{td}\delta^{ab} + \frac{3}{4}\delta^{pr}\delta^{sc}\delta^{td}\delta^{ab} \right) - g_Y^2 g_s^2 \left( \frac{4}{3}\delta^{pc}\delta^{rd}\delta^{st}\delta^{ab} + \frac{4}{3}\delta^{pt}\delta^{rd}\delta^{sc}\delta^{ab} + \frac{4}{3}\delta^{pc}\delta^{rs}\delta^{td}\delta^{ab} \right.
\end{aligned}$$

$$\begin{aligned}
& + \frac{4}{3} \delta^{pr} \delta^{sc} \delta^{td} \delta^{ab} \Big) \Big\} C_{qe}^{abcd} + \left\{ g_Y^4 \left( \frac{308}{27} \delta^{pa} \delta^{rb} \delta^{st} \delta^{cd} + \frac{308}{27} \delta^{pt} \delta^{rb} \delta^{sa} \delta^{cd} + \frac{308}{27} \delta^{pa} \delta^{rs} \delta^{tb} \delta^{cd} + \frac{308}{27} \delta^{pr} \delta^{sa} \delta^{tb} \delta^{cd} - \frac{307}{3} \delta^{pa} \delta^{rb} \delta^{sc} \delta^{td} \right) \right. \\
& + g_L^2 \left( \frac{51}{8} \delta^{rb} \delta^{sa} \delta^{td} (Y_e^\dagger Y_e)^{pc} + \frac{51}{8} \delta^{pa} \delta^{rb} \delta^{td} (Y_e^\dagger Y_e)^{sc} + \frac{51}{8} \delta^{pa} \delta^{sc} \delta^{tb} (Y_e^\dagger Y_e)^{dr} + \frac{51}{8} \delta^{pa} \delta^{rb} \delta^{sc} (Y_e^\dagger Y_e)^{dt} \right) + 2 \delta^{sa} \delta^{tb} (Y_e^\dagger Y_e)^{pr} (Y_e^\dagger Y_e)^{dc} \\
& + 2 \delta^{rb} \delta^{sa} (Y_e^\dagger Y_e)^{pt} (Y_e^\dagger Y_e)^{dc} + 2 \delta^{pa} \delta^{tb} (Y_e^\dagger Y_e)^{sr} (Y_e^\dagger Y_e)^{dc} + 2 \delta^{pa} \delta^{rb} (Y_e^\dagger Y_e)^{st} (Y_e^\dagger Y_e)^{dc} + 4 \delta^{rb} \delta^{td} (Y_e^\dagger Y_e)^{pa} (Y_e^\dagger Y_e)^{sc} + 4 \delta^{pa} \delta^{sc} (Y_e^\dagger Y_e)^{br} (Y_e^\dagger Y_e)^{dt} \\
& - \frac{1}{4} \delta^{rb} \delta^{sa} \delta^{td} (Y_e^\dagger Y_e Y_e^\dagger Y_e)^{pc} - \frac{1}{4} \delta^{pa} \delta^{rb} \delta^{td} (Y_e^\dagger Y_e Y_e^\dagger Y_e)^{sc} - \frac{1}{4} \delta^{pa} \delta^{sc} \delta^{tb} (Y_e^\dagger Y_e Y_e^\dagger Y_e)^{dr} - \frac{1}{4} \delta^{pa} \delta^{rb} \delta^{sc} (Y_e^\dagger Y_e Y_e^\dagger Y_e)^{dt} - g_Y^2 \left( \frac{14}{3} \delta^{pa} \delta^{rb} \delta^{st} (Y_e^\dagger Y_e)^{dc} \right. \\
& + \frac{14}{3} \delta^{pt} \delta^{rb} \delta^{sa} (Y_e^\dagger Y_e)^{dc} + \frac{14}{3} \delta^{pa} \delta^{rs} \delta^{tb} (Y_e^\dagger Y_e)^{dc} + \frac{14}{3} \delta^{pr} \delta^{sa} \delta^{tb} (Y_e^\dagger Y_e)^{dc} + \frac{59}{8} \delta^{rb} \delta^{sa} \delta^{td} (Y_e^\dagger Y_e)^{pc} + \frac{59}{8} \delta^{pa} \delta^{rb} \delta^{td} (Y_e^\dagger Y_e)^{sc} + \frac{59}{8} \delta^{pa} \delta^{sc} \delta^{tb} (Y_e^\dagger Y_e)^{dr} \\
& + \frac{59}{8} \delta^{pa} \delta^{rb} \delta^{sc} (Y_e^\dagger Y_e)^{dt} \Big) - \frac{3}{2} T_2 \delta^{rb} \delta^{sa} \delta^{td} (Y_e^\dagger Y_e)^{pc} - \frac{3}{2} T_2 \delta^{pa} \delta^{rb} \delta^{td} (Y_e^\dagger Y_e)^{sc} - \frac{3}{2} T_2 \delta^{pa} \delta^{sc} \delta^{tb} (Y_e^\dagger Y_e)^{dr} - \frac{3}{2} T_2 \delta^{pa} \delta^{rb} \delta^{sc} (Y_e^\dagger Y_e)^{dt} \\
& - 2 \delta^{sa} \delta^{tb} (Y_e^\dagger Y_e)^{pc} (Y_e^\dagger Y_e)^{dr} - 2 \delta^{pa} \delta^{tb} (Y_e^\dagger Y_e)^{sc} (Y_e^\dagger Y_e)^{dr} - 2 \delta^{rb} \delta^{sa} (Y_e^\dagger Y_e)^{pc} (Y_e^\dagger Y_e)^{dt} - 2 \delta^{pa} \delta^{rb} (Y_e^\dagger Y_e)^{sc} (Y_e^\dagger Y_e)^{dt} \Big\} C_{ee}^{abcd} + g_Y^4 \left\{ \frac{32}{27} \delta^{pt} \delta^{rs} \delta^{ad} \delta^{bc} \right. \\
& + \frac{32}{27} \delta^{pr} \delta^{st} \delta^{ad} \delta^{bc} \Big\} C_{uu}^{abcd} + g_Y^4 \left\{ \frac{8}{27} \delta^{pt} \delta^{rs} \delta^{ad} \delta^{bc} + \frac{8}{27} \delta^{pr} \delta^{st} \delta^{ad} \delta^{bc} \right\} C_{dd}^{abcd} + \left\{ g_Y^4 \left( \frac{4}{9} \delta^{pt} \delta^{rs} \delta^{ab} \delta^{cd} + \frac{4}{9} \delta^{pr} \delta^{st} \delta^{ab} \delta^{cd} + \frac{128}{27} \delta^{pa} \delta^{rb} \delta^{st} \delta^{cd} \right. \right. \\
& + \frac{128}{27} \delta^{pt} \delta^{rb} \delta^{sa} \delta^{cd} + \frac{128}{27} \delta^{pa} \delta^{rs} \delta^{tb} \delta^{cd} + \frac{128}{27} \delta^{pr} \delta^{sa} \delta^{tb} \delta^{cd} \Big) + g_Y^2 \left( \frac{3}{2} \delta^{pa} \delta^{rb} \delta^{st} (Y_u^\dagger Y_u)^{dc} + \frac{3}{2} \delta^{pt} \delta^{rb} \delta^{sa} (Y_u^\dagger Y_u)^{dc} + \frac{3}{2} \delta^{pa} \delta^{rs} \delta^{tb} (Y_u^\dagger Y_u)^{dc} \right. \\
& + \frac{3}{2} \delta^{pr} \delta^{sa} \delta^{tb} (Y_u^\dagger Y_u)^{dc} \Big) - \frac{3}{4} \delta^{sa} \delta^{tb} (Y_e^\dagger Y_e)^{pr} (Y_u^\dagger Y_u)^{dc} - \frac{3}{4} \delta^{rb} \delta^{sa} (Y_e^\dagger Y_e)^{pt} (Y_u^\dagger Y_u)^{dc} - \frac{3}{4} \delta^{pa} \delta^{tb} (Y_e^\dagger Y_e)^{sr} (Y_u^\dagger Y_u)^{dc} - \frac{3}{4} \delta^{pa} \delta^{rb} (Y_e^\dagger Y_e)^{st} (Y_u^\dagger Y_u)^{dc} \\
& - g_Y^2 g_s^2 \left( \frac{8}{3} \delta^{pa} \delta^{rb} \delta^{st} \delta^{cd} + \frac{8}{3} \delta^{pt} \delta^{rb} \delta^{sa} \delta^{cd} + \frac{8}{3} \delta^{pa} \delta^{rs} \delta^{tb} \delta^{cd} + \frac{8}{3} \delta^{pr} \delta^{sa} \delta^{tb} \delta^{cd} \right) \Big\} C_{eu}^{abcd} + \left\{ \frac{3}{4} \delta^{sa} \delta^{tb} (Y_d^\dagger Y_d)^{dc} (Y_e^\dagger Y_e)^{pr} + \frac{3}{4} \delta^{rb} \delta^{sa} (Y_d^\dagger Y_d)^{dc} (Y_e^\dagger Y_e)^{pt} \right. \\
& + \frac{3}{4} \delta^{pa} \delta^{tb} (Y_d^\dagger Y_d)^{dc} (Y_e^\dagger Y_e)^{sr} + \frac{3}{4} \delta^{pa} \delta^{rb} (Y_d^\dagger Y_d)^{dc} (Y_e^\dagger Y_e)^{st} + g_Y^2 g_s^2 \left( \frac{4}{3} \delta^{pa} \delta^{rb} \delta^{st} \delta^{cd} + \frac{4}{3} \delta^{pt} \delta^{rb} \delta^{sa} \delta^{cd} + \frac{4}{3} \delta^{pa} \delta^{rs} \delta^{tb} \delta^{cd} + \frac{4}{3} \delta^{pr} \delta^{sa} \delta^{tb} \delta^{cd} \right) \\
& - g_Y^4 \left( \frac{1}{27} \delta^{pa} \delta^{rb} \delta^{st} \delta^{cd} + \frac{1}{27} \delta^{pt} \delta^{rb} \delta^{sa} \delta^{cd} + \frac{1}{27} \delta^{pa} \delta^{rs} \delta^{tb} \delta^{cd} + \frac{1}{27} \delta^{pr} \delta^{sa} \delta^{tb} \delta^{cd} + \frac{2}{9} \delta^{pt} \delta^{rs} \delta^{ab} \delta^{cd} + \frac{2}{9} \delta^{pr} \delta^{st} \delta^{ab} \delta^{cd} \right) - g_Y^2 \left( \frac{1}{2} \delta^{pa} \delta^{rb} \delta^{st} (Y_d^\dagger Y_d)^{dc} \right. \\
& + \frac{1}{2} \delta^{pt} \delta^{rb} \delta^{sa} (Y_d^\dagger Y_d)^{dc} + \frac{1}{2} \delta^{pa} \delta^{rs} \delta^{tb} (Y_d^\dagger Y_d)^{dc} + \frac{1}{2} \delta^{pr} \delta^{sa} \delta^{tb} (Y_d^\dagger Y_d)^{dc} \Big) \Big\} C_{ed}^{abcd} + \left\{ g_Y^2 \left( \frac{1}{6} \delta^{pt} \delta^{rb} Y_e^{*as} Y_d^{dc} + \frac{1}{6} \delta^{rb} \delta^{st} Y_e^{*ap} Y_d^{dc} + \frac{1}{6} \delta^{pr} \delta^{tb} Y_e^{*as} Y_d^{dc} \right. \right. \\
& + \frac{1}{6} \delta^{rs} \delta^{tb} Y_e^{*ap} Y_d^{dc} \Big) - \frac{9}{8} \delta^{tb} Y_e^{*as} Y_d^{dc} (Y_e^\dagger Y_e)^{pr} - \frac{9}{8} \delta^{rb} Y_e^{*as} Y_d^{dc} (Y_e^\dagger Y_e)^{pt} - \frac{9}{8} \delta^{tb} Y_e^{*ap} Y_d^{dc} (Y_e^\dagger Y_e)^{sr} - \frac{9}{8} \delta^{rb} Y_e^{*ap} Y_d^{dc} (Y_e^\dagger Y_e)^{st} \Big\} C_{ledq}^{abcd} \\
& + C_{ledq}^{*abcd} \left\{ g_Y^2 \left( \frac{1}{6} \delta^{pb} \delta^{rs} Y_d^{*dc} Y_e^{at} + \frac{1}{6} \delta^{pb} \delta^{st} Y_d^{*dc} Y_e^{ar} + \frac{1}{6} \delta^{pr} \delta^{sb} Y_d^{*dc} Y_e^{at} + \frac{1}{6} \delta^{pt} \delta^{sb} Y_d^{*dc} Y_e^{ar} \right) - \frac{9}{8} \delta^{sb} Y_d^{*dc} Y_e^{at} (Y_e^\dagger Y_e)^{pr} - \frac{9}{8} \delta^{sb} Y_d^{*dc} Y_e^{ar} (Y_e^\dagger Y_e)^{pt} \right.
\end{aligned}$$

$$\begin{aligned}
& -\frac{9}{8}\delta^{pb}Y_d^{*dc}Y_e^{at}(Y_e^\dagger Y_e)^{sr} - \frac{9}{8}\delta^{pb}Y_d^{*dc}Y_e^{ar}(Y_e^\dagger Y_e)^{st} \Bigg\} + \left\{ \frac{9}{8}\delta^{tb}Y_e^{*as}Y_u^{*cd}(Y_e^\dagger Y_e)^{pr} + \frac{9}{8}\delta^{rb}Y_e^{*as}Y_u^{*cd}(Y_e^\dagger Y_e)^{pt} + \frac{9}{8}\delta^{tb}Y_e^{*ap}Y_u^{*cd}(Y_e^\dagger Y_e)^{sr} \right. \\
& + \frac{9}{8}\delta^{rb}Y_e^{*ap}Y_u^{*cd}(Y_e^\dagger Y_e)^{st} - g_Y^2 \left( \frac{1}{6}\delta^{pt}\delta^{rb}Y_e^{*as}Y_u^{*cd} + \frac{1}{6}\delta^{rb}\delta^{st}Y_e^{*ap}Y_u^{*cd} + \frac{1}{6}\delta^{pr}\delta^{tb}Y_e^{*as}Y_u^{*cd} + \frac{1}{6}\delta^{rs}\delta^{tb}Y_e^{*ap}Y_u^{*cd} \right) \Bigg\} C_{\ell equ}^{abcd} \\
& + C_{\ell equ}^{*abcd} \left\{ \frac{9}{8}\delta^{sb}Y_e^{at}Y_u^{cd}(Y_e^\dagger Y_e)^{pr} + \frac{9}{8}\delta^{sb}Y_e^{ar}Y_u^{cd}(Y_e^\dagger Y_e)^{pt} + \frac{9}{8}\delta^{pb}Y_e^{at}Y_u^{cd}(Y_e^\dagger Y_e)^{sr} + \frac{9}{8}\delta^{pb}Y_e^{ar}Y_u^{cd}(Y_e^\dagger Y_e)^{st} - g_Y^2 \left( \frac{1}{6}\delta^{pb}\delta^{rs}Y_e^{at}Y_u^{cd} + \frac{1}{6}\delta^{pb}\delta^{st}Y_e^{ar}Y_u^{cd} \right. \right. \\
& + \frac{1}{6}\delta^{pr}\delta^{sb}Y_e^{at}Y_u^{cd} + \frac{1}{6}\delta^{pt}\delta^{sb}Y_e^{ar}Y_u^{cd} \Bigg) \Bigg\} + \left\{ g_Y^2 \left( \frac{5}{24}\delta^{pt}\delta^{rd}Y_e^{*as}Y_u^{*cb} + \frac{5}{24}\delta^{rd}\delta^{st}Y_e^{*ap}Y_u^{*cb} + \frac{5}{24}\delta^{pr}\delta^{td}Y_e^{*as}Y_u^{*cb} + \frac{5}{24}\delta^{rs}\delta^{td}Y_e^{*ap}Y_u^{*cb} \right) \right. \\
& - \frac{9}{16}\delta^{td}Y_e^{*as}Y_u^{*cb}(Y_e^\dagger Y_e)^{pr} - \frac{9}{16}\delta^{rd}Y_e^{*as}Y_u^{*cb}(Y_e^\dagger Y_e)^{pt} - \frac{9}{16}\delta^{td}Y_e^{*ap}Y_u^{*cb}(Y_e^\dagger Y_e)^{sr} - \frac{9}{16}\delta^{rd}Y_e^{*ap}Y_u^{*cb}(Y_e^\dagger Y_e)^{st} \Bigg\} C_{\ell uqe}^{abcd} \\
& + C_{\ell uqe}^{*abcd} \left\{ g_Y^2 \left( \frac{5}{24}\delta^{pd}\delta^{rs}Y_e^{at}Y_u^{cb} + \frac{5}{24}\delta^{pd}\delta^{st}Y_e^{ar}Y_u^{cb} + \frac{5}{24}\delta^{pr}\delta^{sd}Y_e^{at}Y_u^{cb} + \frac{5}{24}\delta^{pt}\delta^{sd}Y_e^{ar}Y_u^{cb} \right) - \frac{9}{16}\delta^{sd}Y_e^{at}Y_u^{cb}(Y_e^\dagger Y_e)^{pr} - \frac{9}{16}\delta^{sd}Y_e^{ar}Y_u^{cb}(Y_e^\dagger Y_e)^{pt} \right. \\
& - \frac{9}{16}\delta^{pd}Y_e^{at}Y_u^{cb}(Y_e^\dagger Y_e)^{sr} - \frac{9}{16}\delta^{pd}Y_e^{ar}Y_u^{cb}(Y_e^\dagger Y_e)^{st} \Bigg\} + \left\{ Y_e^{*ap}Y_e^{*cs}Y_e^{bt}Y_e^{dr} + Y_e^{*ap}Y_e^{*cs}Y_e^{br}Y_e^{dt} + g_Y^4 \left( \frac{4}{9}\delta^{pt}\delta^{rs}\delta^{ad}\delta^{bc} + \frac{4}{9}\delta^{pr}\delta^{st}\delta^{ad}\delta^{bc} \right) \right. \\
& - g_Y^2 \left( \frac{2}{3}\delta^{pr}\delta^{bc}Y_e^{*as}Y_e^{dt} + \frac{2}{3}\delta^{pt}\delta^{bc}Y_e^{*as}Y_e^{dr} + \frac{2}{3}\delta^{rs}\delta^{bc}Y_e^{*ap}Y_e^{dt} + \frac{2}{3}\delta^{st}\delta^{bc}Y_e^{*ap}Y_e^{dr} \right) \Bigg\} C_{\ell\ell}^{abcd} + g_Y^4 \left\{ \frac{4}{27}\delta^{pt}\delta^{rs}\delta^{ad}\delta^{bc} + \frac{4}{27}\delta^{pr}\delta^{st}\delta^{ad}\delta^{bc} \right\} C_{qq}^{(\parallel)abcd} \\
& + g_Y^4 \left\{ \frac{8}{27}\delta^{pt}\delta^{rs}\delta^{ad}\delta^{bc} + \frac{8}{27}\delta^{pr}\delta^{st}\delta^{ad}\delta^{bc} \right\} C_{qq}^{(\times)abcd}, \tag{11.2}
\end{aligned}$$

## 11.2 $C_{uu}$

$$\begin{aligned}
\beta_{C_{uu}^{prst}}^{(1)} &= \left\{ \frac{2}{9}g_Y^2 \left( \delta^{pa}\delta^{rb}\delta^{st} + \delta^{pr}\delta^{sa}\delta^{tb} \right) - \delta^{sa}\delta^{tb}(Y_u^\dagger Y_u)^{pr} - \delta^{pa}\delta^{rb}(Y_u^\dagger Y_u)^{st} \right\} C_{Hu}^{ab} - \frac{4}{9}g_Y^2 \left\{ \delta^{pc}\delta^{rd}\delta^{st}\delta^{ab} + \delta^{pr}\delta^{sc}\delta^{td}\delta^{ab} \right\} C_{\ell u}^{abcd} + \left\{ \frac{4}{9}g_Y^2 \left( \delta^{pc}\delta^{rd}\delta^{st}\delta^{ab} \right. \right. \\
& + \delta^{pr}\delta^{sc}\delta^{td}\delta^{ab} \Bigg) - \delta^{pc}\delta^{rd}Y_u^{*as}Y_u^{bt} - \delta^{sc}\delta^{td}Y_u^{*ap}Y_u^{br} \Bigg\} C_{qu}^{(\parallel)abcd} + \left\{ \frac{4}{27}g_Y^2 \left( \delta^{pc}\delta^{rd}\delta^{st}\delta^{ab} + \delta^{pr}\delta^{sc}\delta^{td}\delta^{ab} \right) - \frac{2}{9}g_s^2 \left( \delta^{pc}\delta^{rd}\delta^{st}\delta^{ab} + \delta^{pr}\delta^{sc}\delta^{td}\delta^{ab} \right. \right. \\
& - 3\delta^{pt}\delta^{rd}\delta^{sc}\delta^{ab} - 3\delta^{pc}\delta^{rs}\delta^{td}\delta^{ab} \Bigg) - \delta^{rd}\delta^{sc}Y_u^{*ap}Y_u^{bt} - \delta^{pc}\delta^{td}Y_u^{*as}Y_u^{br} \Bigg\} C_{qu}^{(\times)abcd} + \left\{ \frac{2}{9}g_s^2 \left( 3\delta^{pt}\delta^{rd}\delta^{sa}\delta^{bc} + 3\delta^{pa}\delta^{rs}\delta^{td}\delta^{bc} + 27\delta^{pa}\delta^{rd}\delta^{sc}\delta^{tb} \right. \right. \\
& - \delta^{pa}\delta^{rd}\delta^{st}\delta^{bc} - \delta^{pr}\delta^{sa}\delta^{td}\delta^{bc} - 9\delta^{pa}\delta^{rb}\delta^{sc}\delta^{td} \Bigg) + \frac{16}{27}g_Y^2 \left( \delta^{pa}\delta^{rd}\delta^{st}\delta^{bc} + \delta^{pr}\delta^{sa}\delta^{td}\delta^{bc} + 3\delta^{pa}\delta^{rb}\delta^{st}\delta^{cd} + 3\delta^{pr}\delta^{sa}\delta^{tb}\delta^{cd} + 9\delta^{pa}\delta^{rb}\delta^{sc}\delta^{td} \right)
\end{aligned}$$

$$\begin{aligned}
& + \delta^{rd} \delta^{sa} \delta^{tb} (Y_u^\dagger Y_u)^{pc} + \delta^{pa} \delta^{rb} \delta^{td} (Y_u^\dagger Y_u)^{sc} + \delta^{pa} \delta^{sc} \delta^{td} (Y_u^\dagger Y_u)^{br} + \delta^{pa} \delta^{rb} \delta^{sc} (Y_u^\dagger Y_u)^{dt} \Big\} C_{uu}^{abcd} - \frac{4}{9} g_Y^2 \Big\{ \delta^{pc} \delta^{rd} \delta^{st} \delta^{ab} + \delta^{pr} \delta^{sc} \delta^{td} \delta^{ab} \Big\} C_{eu}^{abcd} \\
& - \frac{4}{9} g_Y^2 \Big\{ \delta^{pa} \delta^{rb} \delta^{st} \delta^{cd} + \delta^{pr} \delta^{sa} \delta^{tb} \delta^{cd} \Big\} C_{ud}^{(\parallel)abcd} + \Big\{ \frac{1}{9} g_s^2 \Big( 3\delta^{pt} \delta^{rb} \delta^{sa} \delta^{cd} + 3\delta^{pa} \delta^{rs} \delta^{tb} \delta^{cd} - \delta^{pa} \delta^{rb} \delta^{st} \delta^{cd} - \delta^{pr} \delta^{sa} \delta^{tb} \delta^{cd} \Big) - \frac{4}{27} g_Y^2 \Big( \delta^{pa} \delta^{rb} \delta^{st} \delta^{cd} \\
& + \delta^{pr} \delta^{sa} \delta^{tb} \delta^{cd} \Big) \Big\} C_{ud}^{(\times)abcd}, \tag{11.3}
\end{aligned}$$

$$\begin{aligned}
\beta_{C_{uu}^{prst}}^{(2)} = & \Big\{ \frac{16}{27} \delta^{pr} \delta^{st} g_Y^6 - g_Y^4 \Big( \frac{22}{9} \delta^{st} (Y_u^\dagger Y_u)^{pr} + \frac{22}{9} \delta^{pr} (Y_u^\dagger Y_u)^{st} \Big) \Big\} C_{HB} + g_s^4 \Big\{ \frac{2}{3} \delta^{st} (Y_u^\dagger Y_u)^{pr} + \frac{2}{3} \delta^{pr} (Y_u^\dagger Y_u)^{st} - 2\delta^{rs} (Y_u^\dagger Y_u)^{pt} - 2\delta^{pt} (Y_u^\dagger Y_u)^{sr} \Big\} C_{HG} \\
& + \Big\{ \frac{4}{9} \delta^{pr} \delta^{st} g_Y^4 g_L^2 - g_Y^2 g_L^2 \Big( \frac{1}{2} \delta^{st} (Y_u^\dagger Y_u)^{pr} + \frac{1}{2} \delta^{pr} (Y_u^\dagger Y_u)^{st} \Big) \Big\} C_{HWB} + \Big\{ g_Y^2 g_s^6 \Big( \frac{388}{27} \delta^{pr} \delta^{st} + 28\delta^{pt} \delta^{rs} \Big) + g_s^6 \Big( \frac{3}{2} \delta^{st} (Y_u^\dagger Y_u)^{pr} + \frac{3}{2} \delta^{pr} (Y_u^\dagger Y_u)^{st} \\
& - \frac{9}{2} \delta^{rs} (Y_u^\dagger Y_u)^{pt} - \frac{9}{2} \delta^{pt} (Y_u^\dagger Y_u)^{sr} \Big) - g_s^8 \Big( \frac{29}{6} \delta^{pt} \delta^{rs} + \frac{331}{18} \delta^{pr} \delta^{st} \Big) \Big\} C_G - \frac{8}{9} \delta^{pr} \delta^{st} g_Y^4 Y_e^{*ab} C_{eB}^{ab} - \frac{8}{9} \delta^{pr} \delta^{st} g_Y^4 C_{eB}^{*ab} Y_e^{ab} + \Big\{ g_Y^4 \Big( \frac{40}{27} \delta^{pr} \delta^{st} Y_u^{*ab} \\
& - \frac{106}{81} \delta^{rb} \delta^{st} Y_u^{*ap} - \frac{106}{81} \delta^{pr} \delta^{tb} Y_u^{*as} \Big) + g_Y^2 \Big( \frac{9}{2} \delta^{tb} Y_u^{*as} (Y_u^\dagger Y_u)^{pr} + \frac{9}{2} \delta^{rb} Y_u^{*ap} (Y_u^\dagger Y_u)^{st} - \frac{2}{3} \delta^{st} Y_u^{*ap} (Y_u^\dagger Y_u)^{br} - \frac{2}{3} \delta^{pr} Y_u^{*as} (Y_u^\dagger Y_u)^{bt} \Big) \\
& - g_Y^2 g_s^2 \Big( \frac{52}{27} \delta^{rb} \delta^{st} Y_u^{*ap} + \frac{52}{27} \delta^{pr} \delta^{tb} Y_u^{*as} + \frac{44}{9} \delta^{pt} \delta^{rb} Y_u^{*as} + \frac{44}{9} \delta^{rs} \delta^{tb} Y_u^{*ap} \Big) \Big\} C_{uB}^{ab} + C_{uB}^{*ab} \Big\{ g_Y^4 \Big( \frac{40}{27} \delta^{pr} \delta^{st} Y_u^{ab} - \frac{106}{81} \delta^{pb} \delta^{st} Y_u^{ar} \\
& - \frac{106}{81} \delta^{pr} \delta^{sb} Y_u^{at} \Big) + g_Y^2 \Big( \frac{9}{2} \delta^{sb} Y_u^{at} (Y_u^\dagger Y_u)^{pr} + \frac{9}{2} \delta^{pb} Y_u^{ar} (Y_u^\dagger Y_u)^{st} - \frac{2}{3} \delta^{st} Y_u^{ar} (Y_u^\dagger Y_u)^{pb} - \frac{2}{3} \delta^{pr} Y_u^{at} (Y_u^\dagger Y_u)^{sb} \Big) - g_Y^2 g_s^2 \Big( \frac{52}{27} \delta^{pb} \delta^{st} Y_u^{ar} + \frac{52}{27} \delta^{pr} \delta^{sb} Y_u^{at} \\
& + \frac{44}{9} \delta^{pb} \delta^{rs} Y_u^{at} + \frac{44}{9} \delta^{pt} \delta^{sb} Y_u^{ar} \Big) \Big\} + \Big\{ g_s^2 g_L^2 \Big( \frac{2}{3} \delta^{rb} \delta^{st} Y_u^{*ap} + \frac{2}{3} \delta^{pr} \delta^{tb} Y_u^{*as} - 2\delta^{pt} \delta^{rb} Y_u^{*as} - 2\delta^{rs} \delta^{tb} Y_u^{*ap} \Big) + g_L^2 \Big( \frac{9}{4} \delta^{tb} Y_u^{*as} (Y_u^\dagger Y_u)^{pr} \\
& + \frac{9}{4} \delta^{rb} Y_u^{*ap} (Y_u^\dagger Y_u)^{st} \Big) - g_Y^2 g_L^2 \Big( \frac{7}{9} \delta^{rb} \delta^{st} Y_u^{*ap} + \frac{7}{9} \delta^{pr} \delta^{tb} Y_u^{*as} \Big) \Big\} C_{uW}^{ab} + C_{uW}^{*ab} \Big\{ g_s^2 g_L^2 \Big( \frac{2}{3} \delta^{pb} \delta^{st} Y_u^{ar} + \frac{2}{3} \delta^{pr} \delta^{sb} Y_u^{at} - 2\delta^{pb} \delta^{rs} Y_u^{at} - 2\delta^{pt} \delta^{sb} Y_u^{ar} \Big) \\
& + g_L^2 \Big( \frac{9}{4} \delta^{sb} Y_u^{at} (Y_u^\dagger Y_u)^{pr} + \frac{9}{4} \delta^{pb} Y_u^{ar} (Y_u^\dagger Y_u)^{st} \Big) - g_Y^2 g_L^2 \Big( \frac{7}{9} \delta^{pb} \delta^{st} Y_u^{ar} + \frac{7}{9} \delta^{pr} \delta^{sb} Y_u^{at} \Big) \Big\} + \Big\{ g_s^4 \Big( \frac{2}{3} \delta^{pt} \delta^{rs} Y_u^{*ab} + \frac{8}{9} \delta^{pt} \delta^{rb} Y_u^{*as} + \frac{8}{9} \delta^{rs} \delta^{tb} Y_u^{*ap} \\
& - \frac{2}{9} \delta^{pr} \delta^{st} Y_u^{*ab} - \frac{80}{27} \delta^{rb} \delta^{st} Y_u^{*ap} - \frac{80}{27} \delta^{pr} \delta^{tb} Y_u^{*as} \Big) + g_s^2 \Big( \frac{1}{6} \delta^{st} Y_u^{*ap} (Y_u^\dagger Y_u)^{br} + \frac{1}{6} \delta^{pr} Y_u^{*as} (Y_u^\dagger Y_u)^{bt} + 3\delta^{tb} Y_u^{*as} (Y_u^\dagger Y_u)^{pr} + 3\delta^{rb} Y_u^{*as} (Y_u^\dagger Y_u)^{pt} \\
& + 3\delta^{tb} Y_u^{*ap} (Y_u^\dagger Y_u)^{sr} + 3\delta^{rb} Y_u^{*ap} (Y_u^\dagger Y_u)^{st} - \frac{1}{2} \delta^{pt} Y_u^{*as} (Y_u^\dagger Y_u)^{br} - \frac{1}{2} \delta^{rs} Y_u^{*ap} (Y_u^\dagger Y_u)^{bt} \Big) - g_Y^2 g_s^2 \Big( \frac{8}{9} \delta^{pt} \delta^{rb} Y_u^{*as} + \frac{8}{9} \delta^{rs} \delta^{tb} Y_u^{*ap} + \frac{80}{81} \delta^{rb} \delta^{st} Y_u^{*ap} \\
& + \frac{80}{81} \delta^{pr} \delta^{tb} Y_u^{*as} \Big) \Big\} C_{uG}^{ab} + C_{uG}^{*ab} \Big\{ g_s^4 \Big( \frac{2}{3} \delta^{pt} \delta^{rs} Y_u^{ab} + \frac{8}{9} \delta^{pb} \delta^{rs} Y_u^{at} + \frac{8}{9} \delta^{pt} \delta^{sb} Y_u^{ar} - \frac{2}{9} \delta^{pr} \delta^{st} Y_u^{ab} - \frac{80}{27} \delta^{pb} \delta^{st} Y_u^{ar} - \frac{80}{27} \delta^{pr} \delta^{sb} Y_u^{at} \Big)
\end{aligned}$$

$$\begin{aligned}
& + g_s^2 \left( \frac{1}{6} \delta^{st} Y_u^{ar} (Y_u^\dagger Y_u)^{pb} + \frac{1}{6} \delta^{pr} Y_u^{at} (Y_u^\dagger Y_u)^{sb} + 3 \delta^{sb} Y_u^{at} (Y_u^\dagger Y_u)^{pr} + 3 \delta^{sb} Y_u^{ar} (Y_u^\dagger Y_u)^{pt} + 3 \delta^{pb} Y_u^{at} (Y_u^\dagger Y_u)^{sr} + 3 \delta^{pb} Y_u^{ar} (Y_u^\dagger Y_u)^{st} - \frac{1}{2} \delta^{rs} Y_u^{at} (Y_u^\dagger Y_u)^{pb} \right. \\
& - \frac{1}{2} \delta^{pt} Y_u^{ar} (Y_u^\dagger Y_u)^{sb} \left. \right) - g_Y^2 g_s^2 \left( \frac{8}{9} \delta^{pb} \delta^{rs} Y_u^{at} + \frac{8}{9} \delta^{pt} \delta^{sb} Y_u^{ar} + \frac{80}{81} \delta^{pb} \delta^{st} Y_u^{ar} + \frac{80}{81} \delta^{pr} \delta^{sb} Y_u^{at} \right) \left\{ - \frac{8}{27} \delta^{pr} \delta^{st} g_Y^4 Y_d^{*ab} C_{dB}^{ab} - \frac{8}{27} \delta^{pr} \delta^{st} g_Y^4 C_{dB}^{*ab} Y_d^{ab} \right. \\
& + g_s^4 \left\{ \frac{2}{3} \delta^{pt} \delta^{rs} Y_d^{*ab} - \frac{2}{9} \delta^{pr} \delta^{st} Y_d^{*ab} \right\} C_{dG}^{ab} + g_s^4 C_{dG}^{*ab} \left\{ \frac{2}{3} \delta^{pt} \delta^{rs} Y_d^{ab} - \frac{2}{9} \delta^{pr} \delta^{st} Y_d^{ab} \right\} + \left\{ g_Y^2 g_s^2 \left( \frac{91}{243} \delta^{pa} \delta^{rb} \delta^{st} + \frac{91}{243} \delta^{pr} \delta^{sa} \delta^{tb} - \frac{91}{81} \delta^{pt} \delta^{rb} \delta^{sa} \right. \right. \\
& - \frac{91}{81} \delta^{pa} \delta^{rs} \delta^{tb} \left. \right) + g_Y^2 g_L^2 \left( 2 \delta^{pa} \delta^{rb} \delta^{st} + 2 \delta^{pr} \delta^{sa} \delta^{tb} \right) + T_2 \delta^{sa} \delta^{tb} (Y_u^\dagger Y_u)^{pr} + T_2 \delta^{pa} \delta^{rb} (Y_u^\dagger Y_u)^{st} + g_s^2 \left( \frac{7}{18} \delta^{rs} \delta^{tb} (Y_u^\dagger Y_u)^{pa} + \frac{7}{18} \delta^{pt} \delta^{rb} (Y_u^\dagger Y_u)^{sa} \right. \\
& + \frac{7}{18} \delta^{pt} \delta^{sa} (Y_u^\dagger Y_u)^{br} + \frac{7}{18} \delta^{pa} \delta^{rs} (Y_u^\dagger Y_u)^{bt} + \frac{7}{2} \delta^{rb} \delta^{sa} (Y_u^\dagger Y_u)^{pt} + \frac{7}{2} \delta^{pa} \delta^{tb} (Y_u^\dagger Y_u)^{sr} + \frac{25}{6} \delta^{sa} \delta^{tb} (Y_u^\dagger Y_u)^{pr} + \frac{25}{6} \delta^{pa} \delta^{rb} (Y_u^\dagger Y_u)^{st} - \frac{7}{54} \delta^{rb} \delta^{st} (Y_u^\dagger Y_u)^{pa} \\
& - \frac{7}{54} \delta^{pr} \delta^{tb} (Y_u^\dagger Y_u)^{sa} - \frac{7}{54} \delta^{pa} \delta^{st} (Y_u^\dagger Y_u)^{br} - \frac{7}{54} \delta^{pr} \delta^{sa} (Y_u^\dagger Y_u)^{bt} \left. \right) + g_Y^2 \left( \frac{31}{72} \delta^{sa} \delta^{tb} (Y_u^\dagger Y_u)^{pr} + \frac{31}{72} \delta^{pa} \delta^{rb} (Y_u^\dagger Y_u)^{st} + \frac{101}{162} \delta^{rb} \delta^{st} (Y_u^\dagger Y_u)^{pa} \right. \\
& + \frac{101}{162} \delta^{pr} \delta^{tb} (Y_u^\dagger Y_u)^{sa} + \frac{101}{162} \delta^{pa} \delta^{st} (Y_u^\dagger Y_u)^{br} + \frac{101}{162} \delta^{pr} \delta^{sa} (Y_u^\dagger Y_u)^{bt} - \frac{2}{9} T_2 \delta^{pa} \delta^{rb} \delta^{st} - \frac{2}{9} T_2 \delta^{pr} \delta^{sa} \delta^{tb} \left. \right) + \frac{3}{2} \delta^{sa} \delta^{tb} (Y_u^\dagger Y_u Y_u^\dagger Y_u)^{pr} \\
& + \frac{3}{2} \delta^{pa} \delta^{rb} (Y_u^\dagger Y_u Y_u^\dagger Y_u)^{st} - \frac{1}{4} \delta^{rb} (Y_u^\dagger Y_u)^{pa} (Y_u^\dagger Y_u)^{st} - \frac{1}{4} \delta^{tb} (Y_u^\dagger Y_u)^{pr} (Y_u^\dagger Y_u)^{sa} - \frac{1}{4} \delta^{pa} (Y_u^\dagger Y_u)^{st} (Y_u^\dagger Y_u)^{br} - \frac{1}{4} \delta^{sa} (Y_u^\dagger Y_u)^{pr} (Y_u^\dagger Y_u)^{bt} - g_Y^4 \left( \frac{242}{729} \delta^{pa} \delta^{rb} \delta^{st} \right. \\
& + \frac{242}{729} \delta^{pr} \delta^{sa} \delta^{tb} \left. \right) - g_L^2 \left( \frac{51}{8} \delta^{sa} \delta^{tb} (Y_u^\dagger Y_u)^{pr} + \frac{51}{8} \delta^{pa} \delta^{rb} (Y_u^\dagger Y_u)^{st} \right) \left\{ C_{Hu}^{ab} + \left\{ g_s^2 \left( \frac{1}{54} \delta^{pa} \delta^{st} (Y_d^\dagger Y_u)^{br} + \frac{1}{54} \delta^{pr} \delta^{sa} (Y_d^\dagger Y_u)^{bt} - \frac{1}{18} \delta^{pt} \delta^{sa} (Y_d^\dagger Y_u)^{br} \right. \right. \right. \\
& - \frac{1}{18} \delta^{pa} \delta^{rs} (Y_d^\dagger Y_u)^{bt} \left. \right) + g_Y^2 \left( \frac{55}{162} \delta^{pa} \delta^{st} (Y_d^\dagger Y_u)^{br} + \frac{55}{162} \delta^{pr} \delta^{sa} (Y_d^\dagger Y_u)^{bt} \right) - \frac{3}{4} \delta^{sa} (Y_d^\dagger Y_u)^{bt} (Y_u^\dagger Y_u)^{pr} - \frac{3}{4} \delta^{pa} (Y_d^\dagger Y_u)^{br} (Y_u^\dagger Y_u)^{st} \left. \right\} C_{Hud}^{ab} \\
& + C_{Hud}^{*ab} \left\{ g_s^2 \left( \frac{1}{54} \delta^{ra} \delta^{st} (Y_u^\dagger Y_d)^{pb} + \frac{1}{54} \delta^{pr} \delta^{ta} (Y_u^\dagger Y_d)^{sb} - \frac{1}{18} \delta^{rs} \delta^{ta} (Y_u^\dagger Y_d)^{pb} - \frac{1}{18} \delta^{pt} \delta^{ra} (Y_u^\dagger Y_d)^{sb} \right) + g_Y^2 \left( \frac{55}{162} \delta^{ra} \delta^{st} (Y_u^\dagger Y_d)^{pb} + \frac{55}{162} \delta^{pr} \delta^{ta} (Y_u^\dagger Y_d)^{sb} \right) \right. \\
& - \frac{3}{4} \delta^{ta} (Y_u^\dagger Y_d)^{sb} (Y_u^\dagger Y_u)^{pr} - \frac{3}{4} \delta^{ra} (Y_u^\dagger Y_d)^{pb} (Y_u^\dagger Y_u)^{st} \left. \right\} + \left\{ \frac{1}{2} \delta^{sc} \delta^{td} (Y_u^\dagger Y_u)^{pr} (Y_e Y_e^\dagger)^{ba} + \frac{1}{2} \delta^{pc} \delta^{rd} (Y_u^\dagger Y_u)^{st} (Y_e Y_e^\dagger)^{ba} + g_Y^2 g_s^2 \left( \frac{50}{81} \delta^{pt} \delta^{rd} \delta^{sc} \delta^{ab} \right. \right. \\
& + \frac{50}{81} \delta^{pc} \delta^{rs} \delta^{td} \delta^{ab} - \frac{50}{243} \delta^{pc} \delta^{rd} \delta^{st} \delta^{ab} - \frac{50}{243} \delta^{pr} \delta^{sc} \delta^{td} \delta^{ab} \left. \right) + g_Y^2 \left( \frac{8}{9} \delta^{pc} \delta^{rd} \delta^{st} (Y_e Y_e^\dagger)^{ba} + \frac{8}{9} \delta^{pr} \delta^{sc} \delta^{td} (Y_e Y_e^\dagger)^{ba} \right) - g_Y^2 g_L^2 \left( \delta^{pc} \delta^{rd} \delta^{st} \delta^{ab} \right. \\
& + \delta^{pr} \delta^{sc} \delta^{td} \delta^{ab} \left. \right) - g_Y^4 \left( \frac{2003}{729} \delta^{pc} \delta^{rd} \delta^{st} \delta^{ab} + \frac{2003}{729} \delta^{pr} \delta^{sc} \delta^{td} \delta^{ab} \right) \left\{ C_{\ell u}^{abcd} + \left\{ \frac{1}{4} \delta^{sc} \delta^{td} Y_u^{br} (Y_d^\dagger Y_d Y_u^\dagger)^{ap} + \frac{1}{4} \delta^{pc} \delta^{rd} Y_u^{bt} (Y_d^\dagger Y_d Y_u^\dagger)^{as} \right. \right. \\
& + \frac{1}{4} \delta^{sc} \delta^{td} Y_u^{*ap} (Y_d Y_d^\dagger Y_u)^{br} + \frac{1}{4} \delta^{pc} \delta^{rd} Y_u^{*as} (Y_d Y_d^\dagger Y_u)^{bt} + \frac{3}{4} \delta^{sc} \delta^{td} Y_u^{br} (Y_u^\dagger Y_u Y_u^\dagger)^{ap} + \frac{3}{4} \delta^{pc} \delta^{rd} Y_u^{bt} (Y_u^\dagger Y_u Y_u^\dagger)^{as} + \frac{3}{4} \delta^{sc} \delta^{td} Y_u^{*ap} (Y_u Y_u^\dagger Y_u)^{br} \\
& + \frac{3}{4} \delta^{pc} \delta^{rd} Y_u^{*as} (Y_u Y_u^\dagger Y_u)^{bt} + g_s^2 \left( \frac{4}{27} \delta^{pc} \delta^{st} Y_u^{*ad} Y_u^{br} + \frac{4}{27} \delta^{rd} \delta^{st} Y_u^{*ap} Y_u^{bc} + \frac{4}{27} \delta^{pr} \delta^{sc} Y_u^{*ad} Y_u^{bt} + \frac{4}{27} \delta^{pr} \delta^{td} Y_u^{*as} Y_u^{bc} + 6 \delta^{pc} \delta^{rd} Y_u^{*as} Y_u^{bt} \right. \\
& + 6 \delta^{sc} \delta^{td} Y_u^{*ap} Y_u^{br} - \frac{4}{9} \delta^{pc} \delta^{rs} Y_u^{*ad} Y_u^{bt} - \frac{4}{9} \delta^{pt} \delta^{rd} Y_u^{*as} Y_u^{bc} - \frac{4}{9} \delta^{pt} \delta^{sc} Y_u^{*ad} Y_u^{br} - \frac{4}{9} \delta^{rs} \delta^{td} Y_u^{*ap} Y_u^{bc} - 2 \delta^{rd} \delta^{sc} Y_u^{*ap} Y_u^{bt} - 2 \delta^{pc} \delta^{td} Y_u^{*as} Y_u^{br} \left. \right)
\end{aligned}$$

$$\begin{aligned}
& + g_Y^2 g_L^2 \left( \delta^{pc} \delta^{rd} \delta^{st} \delta^{ab} + \delta^{pr} \delta^{sc} \delta^{td} \delta^{ab} \right) + g_Y^2 g_s^2 \left( \frac{482}{243} \delta^{pc} \delta^{rd} \delta^{st} \delta^{ab} + \frac{482}{243} \delta^{pr} \delta^{sc} \delta^{td} \delta^{ab} - \frac{50}{81} \delta^{pt} \delta^{rd} \delta^{sc} \delta^{ab} - \frac{50}{81} \delta^{pc} \delta^{rs} \delta^{td} \delta^{ab} \right) \\
& + \delta^{sc} Y_u^{*ad} Y_u^{bt} (Y_u^\dagger Y_u)^{pr} + \delta^{td} Y_u^{*as} Y_u^{bc} (Y_u^\dagger Y_u)^{pr} + \delta^{pc} Y_u^{*ad} Y_u^{br} (Y_u^\dagger Y_u)^{st} + \delta^{rd} Y_u^{*ap} Y_u^{bc} (Y_u^\dagger Y_u)^{st} + g_Y^2 \left( \frac{4}{81} \delta^{pc} \delta^{st} Y_u^{*ad} Y_u^{br} + \frac{4}{81} \delta^{rd} \delta^{st} Y_u^{*ap} Y_u^{bc} \right. \\
& + \frac{4}{81} \delta^{pr} \delta^{sc} Y_u^{*ad} Y_u^{bt} + \frac{4}{81} \delta^{pr} \delta^{td} Y_u^{*as} Y_u^{bc} - \frac{4}{3} \delta^{pc} \delta^{rd} \delta^{st} (Y_u Y_u^\dagger)^{ba} - \frac{4}{3} \delta^{pr} \delta^{sc} \delta^{td} (Y_u Y_u^\dagger)^{ba} - \frac{67}{24} \delta^{pc} \delta^{rd} Y_u^{*as} Y_u^{bt} - \frac{67}{24} \delta^{sc} \delta^{td} Y_u^{*ap} Y_u^{br} \Big) \\
& + \frac{3}{2} T_2 \delta^{pc} \delta^{rd} Y_u^{*as} Y_u^{bt} + \frac{3}{2} T_2 \delta^{sc} \delta^{td} Y_u^{*ap} Y_u^{br} + \frac{3}{2} \delta^{sc} \delta^{td} (Y_u^\dagger Y_u)^{pr} (Y_d Y_d^\dagger)^{ba} + \frac{3}{2} \delta^{pc} \delta^{rd} (Y_u^\dagger Y_u)^{st} (Y_d Y_d^\dagger)^{ba} + \frac{7}{4} \delta^{rd} Y_u^{*as} Y_u^{bt} (Y_u^\dagger Y_u)^{pc} \\
& + \frac{7}{4} \delta^{td} Y_u^{*ap} Y_u^{br} (Y_u^\dagger Y_u)^{sc} + \frac{7}{4} \delta^{pc} Y_u^{*as} Y_u^{bt} (Y_u^\dagger Y_u)^{dr} + \frac{7}{4} \delta^{sc} Y_u^{*ap} Y_u^{br} (Y_u^\dagger Y_u)^{dt} - g_L^2 \left( \frac{51}{8} \delta^{pc} \delta^{rd} Y_u^{*as} Y_u^{bt} + \frac{51}{8} \delta^{sc} \delta^{td} Y_u^{*ap} Y_u^{br} \right) - g_Y^4 \left( \frac{1093}{729} \delta^{pc} \delta^{rd} \delta^{st} \delta^{ab} \right. \\
& + \frac{1093}{729} \delta^{pr} \delta^{sc} \delta^{td} \delta^{ab} \Big) - g_s^4 \left( \frac{11}{3} \delta^{pt} \delta^{rd} \delta^{sc} \delta^{ab} + \frac{11}{3} \delta^{pc} \delta^{rs} \delta^{td} \delta^{ab} + \frac{61}{9} \delta^{pc} \delta^{rd} \delta^{st} \delta^{ab} + \frac{61}{9} \delta^{pr} \delta^{sc} \delta^{td} \delta^{ab} \right) - \frac{3}{2} \delta^{sc} \delta^{td} (Y_u^\dagger Y_u)^{pr} (Y_u Y_u^\dagger)^{ba} \\
& - \frac{3}{2} \delta^{pc} \delta^{rd} (Y_u^\dagger Y_u)^{st} (Y_u Y_u^\dagger)^{ba} \Big\} C_{qu}^{(\parallel)abcd} + \left\{ \frac{1}{4} \delta^{rd} \delta^{sc} Y_u^{bt} (Y_d^\dagger Y_d Y_u^\dagger)^{ap} + \frac{1}{4} \delta^{pc} \delta^{td} Y_u^{br} (Y_d^\dagger Y_d Y_u^\dagger)^{as} + \frac{1}{4} \delta^{pc} \delta^{td} Y_u^{*as} (Y_d Y_d^\dagger Y_u)^{br} + \frac{1}{4} \delta^{rd} \delta^{sc} Y_u^{*ap} (Y_d Y_d^\dagger Y_u)^{bt} \right. \\
& + \frac{1}{2} \delta^{sc} \delta^{td} (Y_u^\dagger Y_u)^{pr} (Y_d Y_d^\dagger)^{ba} + \frac{1}{2} \delta^{pc} \delta^{rd} (Y_u^\dagger Y_u)^{st} (Y_d Y_d^\dagger)^{ba} + \frac{3}{4} \delta^{rd} \delta^{sc} Y_u^{bt} (Y_u^\dagger Y_u Y_u^\dagger)^{ap} + \frac{3}{4} \delta^{pc} \delta^{td} Y_u^{br} (Y_u^\dagger Y_u Y_u^\dagger)^{as} + \frac{3}{4} \delta^{pc} \delta^{td} Y_u^{*as} (Y_u Y_u^\dagger Y_u)^{br} \\
& + \frac{3}{4} \delta^{rd} \delta^{sc} Y_u^{*ap} (Y_u Y_u^\dagger Y_u)^{bt} + g_s^2 g_L^2 \left( \frac{3}{2} \delta^{pt} \delta^{rd} \delta^{sc} \delta^{ab} + \frac{3}{2} \delta^{pc} \delta^{rs} \delta^{td} \delta^{ab} - \frac{1}{2} \delta^{pc} \delta^{rd} \delta^{st} \delta^{ab} - \frac{1}{2} \delta^{pr} \delta^{sc} \delta^{td} \delta^{ab} \right) + g_Y^2 g_L^2 \left( \frac{1}{3} \delta^{pc} \delta^{rd} \delta^{st} \delta^{ab} \right. \\
& + \frac{1}{3} \delta^{pr} \delta^{sc} \delta^{td} \delta^{ab} \Big) + g_s^4 \left( \frac{4}{27} \delta^{pr} \delta^{st} \delta^{ab} \delta^{cd} + \frac{52}{81} \delta^{pt} \delta^{rd} \delta^{sc} \delta^{ab} + \frac{52}{81} \delta^{pc} \delta^{rs} \delta^{td} \delta^{ab} - \frac{4}{9} \delta^{pt} \delta^{rs} \delta^{ab} \delta^{cd} - \frac{628}{243} \delta^{pc} \delta^{rd} \delta^{st} \delta^{ab} - \frac{628}{243} \delta^{pr} \delta^{sc} \delta^{td} \delta^{ab} \right) \\
& + g_Y^2 \left( \frac{8}{27} \delta^{pr} \delta^{cd} Y_u^{*as} Y_u^{bt} + \frac{8}{27} \delta^{st} \delta^{cd} Y_u^{*ap} Y_u^{br} - \frac{4}{27} \delta^{pc} \delta^{rd} \delta^{st} (Y_u Y_u^\dagger)^{ba} - \frac{4}{27} \delta^{pr} \delta^{sc} \delta^{td} (Y_u Y_u^\dagger)^{ba} - \frac{20}{27} \delta^{pc} \delta^{st} Y_u^{*ad} Y_u^{br} - \frac{20}{27} \delta^{rd} \delta^{st} Y_u^{*ap} Y_u^{bc} \right. \\
& - \frac{20}{27} \delta^{pr} \delta^{sc} Y_u^{*ad} Y_u^{bt} - \frac{20}{27} \delta^{pr} \delta^{td} Y_u^{*as} Y_u^{bc} - \frac{67}{24} \delta^{rd} \delta^{sc} Y_u^{*ap} Y_u^{bt} - \frac{67}{24} \delta^{pc} \delta^{td} Y_u^{*as} Y_u^{br} \Big) + g_s^2 \left( \frac{1}{9} \delta^{pc} \delta^{st} Y_u^{*ad} Y_u^{br} + \frac{1}{9} \delta^{rd} \delta^{st} Y_u^{*ap} Y_u^{bc} + \frac{1}{9} \delta^{pr} \delta^{sc} Y_u^{*ad} Y_u^{bt} \right. \\
& + \frac{1}{9} \delta^{pr} \delta^{td} Y_u^{*as} Y_u^{bc} + \frac{2}{9} \delta^{pc} \delta^{rd} \delta^{st} (Y_u Y_u^\dagger)^{ba} + \frac{2}{9} \delta^{pr} \delta^{sc} \delta^{td} (Y_u Y_u^\dagger)^{ba} + \frac{1}{3} \delta^{pt} \delta^{cd} Y_u^{*as} Y_u^{br} + \frac{1}{3} \delta^{rs} \delta^{cd} Y_u^{*ap} Y_u^{bt} + \frac{1}{3} \delta^{pc} \delta^{rd} \delta^{st} (Y_d Y_d^\dagger)^{ba} \\
& + \frac{1}{3} \delta^{pr} \delta^{sc} \delta^{td} (Y_d Y_d^\dagger)^{ba} + 2 \delta^{pc} \delta^{rd} Y_u^{*as} Y_u^{bt} + 2 \delta^{sc} \delta^{td} Y_u^{*ap} Y_u^{br} - \frac{1}{9} \delta^{pr} \delta^{cd} Y_u^{*as} Y_u^{bt} - \frac{1}{9} \delta^{st} \delta^{cd} Y_u^{*ap} Y_u^{br} - \frac{1}{3} \delta^{pc} \delta^{rs} Y_u^{*ad} Y_u^{bt} - \frac{1}{3} \delta^{pt} \delta^{rd} Y_u^{*as} Y_u^{bc} \\
& - \frac{1}{3} \delta^{pt} \delta^{sc} Y_u^{*ad} Y_u^{br} - \frac{1}{3} \delta^{rs} \delta^{td} Y_u^{*ap} Y_u^{bc} - \frac{2}{3} \delta^{pt} \delta^{rd} \delta^{sc} (Y_u Y_u^\dagger)^{ba} - \frac{2}{3} \delta^{pc} \delta^{rs} \delta^{td} (Y_u Y_u^\dagger)^{ba} - \delta^{pt} \delta^{rd} \delta^{sc} (Y_d Y_d^\dagger)^{ba} - \delta^{pc} \delta^{rs} \delta^{td} (Y_d Y_d^\dagger)^{ba} - 6 \delta^{rd} \delta^{sc} Y_u^{*ap} Y_u^{bt} \\
& - 6 \delta^{pc} \delta^{td} Y_u^{*as} Y_u^{br} \Big) + \frac{3}{2} T_2 \delta^{rd} \delta^{sc} Y_u^{*ap} Y_u^{bt} + \frac{3}{2} T_2 \delta^{pc} \delta^{td} Y_u^{*as} Y_u^{br} + \frac{7}{4} \delta^{td} Y_u^{*as} Y_u^{br} (Y_u^\dagger Y_u)^{pc} + \frac{7}{4} \delta^{rd} Y_u^{*ap} Y_u^{bt} (Y_u^\dagger Y_u)^{sc} + \frac{7}{4} \delta^{sc} Y_u^{*ap} Y_u^{bt} (Y_u^\dagger Y_u)^{dr} \\
& + \frac{7}{4} \delta^{pc} Y_u^{*as} Y_u^{br} (Y_u^\dagger Y_u)^{dt} + 3 \delta^{sc} Y_u^{*ad} Y_u^{bt} (Y_u^\dagger Y_u)^{pr} + 3 \delta^{td} Y_u^{*as} Y_u^{bc} (Y_u^\dagger Y_u)^{pr} + 3 \delta^{pc} Y_u^{*ad} Y_u^{br} (Y_u^\dagger Y_u)^{st} + 3 \delta^{rd} Y_u^{*ap} Y_u^{bc} (Y_u^\dagger Y_u)^{st} \\
& - \frac{1}{2} \delta^{sc} \delta^{td} (Y_u^\dagger Y_u)^{pr} (Y_u Y_u^\dagger)^{ba} - \frac{1}{2} \delta^{pc} \delta^{rd} (Y_u^\dagger Y_u)^{st} (Y_u Y_u^\dagger)^{ba} - g_L^2 \left( \frac{51}{8} \delta^{rd} \delta^{sc} Y_u^{*ap} Y_u^{bt} + \frac{51}{8} \delta^{pc} \delta^{td} Y_u^{*as} Y_u^{br} \right) - g_Y^4 \left( \frac{1093}{2187} \delta^{pc} \delta^{rd} \delta^{st} \delta^{ab} \right. \\
& + \frac{1093}{2187} \delta^{pr} \delta^{sc} \delta^{td} \delta^{ab} \Big) - g_Y^2 g_s^2 \left( \frac{32}{81} \delta^{pr} \delta^{st} \delta^{ab} \delta^{cd} + \frac{973}{486} \delta^{pt} \delta^{rd} \delta^{sc} \delta^{ab} + \frac{973}{486} \delta^{pc} \delta^{rs} \delta^{td} \delta^{ab} + \frac{4819}{1458} \delta^{pc} \delta^{rd} \delta^{st} \delta^{ab} + \frac{4819}{1458} \delta^{pr} \delta^{sc} \delta^{td} \delta^{ab} \right) \Big\} C_{qu}^{(\times)abcd}
\end{aligned}$$

$$\begin{aligned}
& + \frac{64}{81} \delta^{pr} \delta^{st} \delta^{ab} \delta^{cd} g_Y^4 C_{ee}^{abcd} + \left\{ g_Y^2 g_s^2 \left( \frac{1496}{243} \delta^{pa} \delta^{rb} \delta^{st} \delta^{cd} + \frac{1496}{243} \delta^{pr} \delta^{sa} \delta^{tb} \delta^{cd} + \frac{1840}{243} \delta^{pt} \delta^{rd} \delta^{sa} \delta^{bc} + \frac{1840}{243} \delta^{pa} \delta^{rs} \delta^{td} \delta^{bc} - \frac{32}{81} \delta^{pr} \delta^{st} \delta^{ad} \delta^{bc} \right. \right. \\
& - \frac{1232}{729} \delta^{pa} \delta^{rd} \delta^{st} \delta^{bc} - \frac{1232}{729} \delta^{pr} \delta^{sa} \delta^{td} \delta^{bc} - \frac{200}{81} \delta^{pt} \delta^{rb} \delta^{sa} \delta^{cd} - \frac{200}{81} \delta^{pa} \delta^{rs} \delta^{tb} \delta^{cd} - \frac{280}{9} \delta^{pa} \delta^{rb} \delta^{sc} \delta^{td} - \frac{104}{3} \delta^{pa} \delta^{rd} \delta^{sc} \delta^{tb} \Big) \\
& + g_Y^4 \left( \frac{256}{243} \delta^{pr} \delta^{st} \delta^{ad} \delta^{bc} + \frac{5504}{2187} \delta^{pa} \delta^{rd} \delta^{st} \delta^{bc} + \frac{5504}{2187} \delta^{pr} \delta^{sa} \delta^{td} \delta^{bc} + \frac{4736}{729} \delta^{pa} \delta^{rb} \delta^{st} \delta^{cd} + \frac{4736}{729} \delta^{pr} \delta^{sa} \delta^{tb} \delta^{cd} - \frac{52}{3} \delta^{pa} \delta^{rb} \delta^{sc} \delta^{td} \right) \\
& + g_s^4 \left( \frac{15}{2} \delta^{pa} \delta^{rd} \delta^{sc} \delta^{tb} + \frac{79}{9} \delta^{pa} \delta^{rb} \delta^{st} \delta^{cd} + \frac{79}{9} \delta^{pr} \delta^{sa} \delta^{tb} \delta^{cd} + \frac{1300}{81} \delta^{pt} \delta^{rd} \delta^{sa} \delta^{bc} + \frac{1300}{81} \delta^{pa} \delta^{rs} \delta^{td} \delta^{bc} - \frac{148}{243} \delta^{pa} \delta^{rd} \delta^{st} \delta^{bc} \right. \\
& - \frac{148}{243} \delta^{pr} \delta^{sa} \delta^{td} \delta^{bc} - \frac{7}{3} \delta^{pt} \delta^{rb} \delta^{sa} \delta^{cd} - \frac{7}{3} \delta^{pa} \delta^{rs} \delta^{tb} \delta^{cd} - \frac{71}{6} \delta^{pa} \delta^{rb} \delta^{sc} \delta^{td} \Big) + g_s^2 \left( \frac{10}{9} \delta^{pa} \delta^{rd} \delta^{st} (Y_u^\dagger Y_u)^{bc} + \frac{10}{9} \delta^{pr} \delta^{sa} \delta^{td} (Y_u^\dagger Y_u)^{bc} \right. \\
& - \frac{10}{3} \delta^{rd} \delta^{sa} \delta^{tb} (Y_u^\dagger Y_u)^{pc} - \frac{10}{3} \delta^{pa} \delta^{rb} \delta^{td} (Y_u^\dagger Y_u)^{sc} - \frac{10}{3} \delta^{pa} \delta^{sc} \delta^{td} (Y_u^\dagger Y_u)^{br} - \frac{10}{3} \delta^{pt} \delta^{rd} \delta^{sa} (Y_u^\dagger Y_u)^{bc} - \frac{10}{3} \delta^{pa} \delta^{rs} \delta^{td} (Y_u^\dagger Y_u)^{bc} - \frac{10}{3} \delta^{pa} \delta^{rb} \delta^{sc} (Y_u^\dagger Y_u)^{dt} \\
& - 6 \delta^{rb} \delta^{sa} \delta^{td} (Y_u^\dagger Y_u)^{pc} - 6 \delta^{pa} \delta^{rd} \delta^{tb} (Y_u^\dagger Y_u)^{sc} - 6 \delta^{pa} \delta^{rd} \delta^{sc} (Y_u^\dagger Y_u)^{bt} - 6 \delta^{pa} \delta^{sc} \delta^{tb} (Y_u^\dagger Y_u)^{dr} \Big) + g_L^2 \left( \frac{51}{8} \delta^{rd} \delta^{sa} \delta^{tb} (Y_u^\dagger Y_u)^{pc} + \frac{51}{8} \delta^{pa} \delta^{rb} \delta^{td} (Y_u^\dagger Y_u)^{sc} \right. \\
& + \frac{51}{8} \delta^{pa} \delta^{sc} \delta^{td} (Y_u^\dagger Y_u)^{br} + \frac{51}{8} \delta^{pa} \delta^{rb} \delta^{sc} (Y_u^\dagger Y_u)^{dt} \Big) + 3 \delta^{sa} \delta^{td} (Y_u^\dagger Y_u)^{pr} (Y_u^\dagger Y_u)^{bc} + 3 \delta^{pa} \delta^{rd} (Y_u^\dagger Y_u)^{st} (Y_u^\dagger Y_u)^{bc} + 3 \delta^{sa} \delta^{tb} (Y_u^\dagger Y_u)^{pr} (Y_u^\dagger Y_u)^{dc} \\
& + 3 \delta^{pa} \delta^{rb} (Y_u^\dagger Y_u)^{st} (Y_u^\dagger Y_u)^{dc} + 4 \delta^{rb} \delta^{td} (Y_u^\dagger Y_u)^{pa} (Y_u^\dagger Y_u)^{sc} + 4 \delta^{pa} \delta^{sc} (Y_u^\dagger Y_u)^{br} (Y_u^\dagger Y_u)^{dt} - \frac{1}{4} \delta^{rd} \delta^{sa} \delta^{tb} (Y_u^\dagger Y_d Y_d^\dagger Y_u)^{pc} - \frac{1}{4} \delta^{pa} \delta^{rb} \delta^{td} (Y_u^\dagger Y_d Y_d^\dagger Y_u)^{sc} \\
& - \frac{1}{4} \delta^{pa} \delta^{sc} \delta^{td} (Y_u^\dagger Y_d Y_d^\dagger Y_u)^{br} - \frac{1}{4} \delta^{pa} \delta^{rb} \delta^{sc} (Y_u^\dagger Y_d Y_d^\dagger Y_u)^{dt} - \frac{1}{4} \delta^{rd} \delta^{sa} \delta^{tb} (Y_u^\dagger Y_u Y_u^\dagger Y_u)^{pc} - \frac{1}{4} \delta^{pa} \delta^{rb} \delta^{td} (Y_u^\dagger Y_u Y_u^\dagger Y_u)^{sc} - \frac{1}{4} \delta^{pa} \delta^{sc} \delta^{td} (Y_u^\dagger Y_u Y_u^\dagger Y_u)^{br} \\
& - \frac{1}{4} \delta^{pa} \delta^{rb} \delta^{sc} (Y_u^\dagger Y_u Y_u^\dagger Y_u)^{dt} - g_Y^2 \left( \frac{47}{72} \delta^{rd} \delta^{sa} \delta^{tb} (Y_u^\dagger Y_u)^{pc} + \frac{47}{72} \delta^{pa} \delta^{rb} \delta^{td} (Y_u^\dagger Y_u)^{sc} + \frac{47}{72} \delta^{pa} \delta^{sc} \delta^{td} (Y_u^\dagger Y_u)^{br} + \frac{47}{72} \delta^{pa} \delta^{rb} \delta^{sc} (Y_u^\dagger Y_u)^{dt} \right. \\
& + \frac{68}{27} \delta^{pa} \delta^{rd} \delta^{st} (Y_u^\dagger Y_u)^{bc} + \frac{68}{27} \delta^{pr} \delta^{sa} \delta^{td} (Y_u^\dagger Y_u)^{bc} + 4 \delta^{pa} \delta^{rb} \delta^{st} (Y_u^\dagger Y_u)^{dc} + 4 \delta^{pr} \delta^{sa} \delta^{tb} (Y_u^\dagger Y_u)^{dc} \Big) - \frac{3}{2} T_2 \delta^{rd} \delta^{sa} \delta^{tb} (Y_u^\dagger Y_u)^{pc} \\
& - \frac{3}{2} T_2 \delta^{pa} \delta^{rb} \delta^{td} (Y_u^\dagger Y_u)^{sc} - \frac{3}{2} T_2 \delta^{pa} \delta^{sc} \delta^{td} (Y_u^\dagger Y_u)^{br} - \frac{3}{2} \delta^{pa} \delta^{td} (Y_u^\dagger Y_u)^{sc} (Y_u^\dagger Y_u)^{br} - \frac{3}{2} \delta^{rd} \delta^{sa} (Y_u^\dagger Y_u)^{pc} (Y_u^\dagger Y_u)^{bt} - \frac{3}{2} T_2 \delta^{pa} \delta^{rb} \delta^{sc} (Y_u^\dagger Y_u)^{dt} \\
& - \frac{5}{2} \delta^{sa} \delta^{tb} (Y_u^\dagger Y_u)^{pc} (Y_u^\dagger Y_u)^{dr} - \frac{5}{2} \delta^{pa} \delta^{rb} (Y_u^\dagger Y_u)^{sc} (Y_u^\dagger Y_u)^{dt} \Big\} C_{uu}^{abcd} + \left\{ \frac{64}{243} \delta^{pr} \delta^{st} \delta^{ad} \delta^{bc} g_Y^4 + g_s^4 \left( \frac{4}{9} \delta^{pt} \delta^{rs} \delta^{ad} \delta^{bc} - \frac{4}{27} \delta^{pr} \delta^{st} \delta^{ad} \delta^{bc} \right) \right\} C_{dd}^{abcd} \\
& + \left\{ g_Y^2 g_s^2 \left( \frac{50}{81} \delta^{pt} \delta^{rd} \delta^{sc} \delta^{ab} + \frac{50}{81} \delta^{pc} \delta^{rs} \delta^{td} \delta^{ab} - \frac{50}{243} \delta^{pc} \delta^{rd} \delta^{st} \delta^{ab} - \frac{50}{243} \delta^{pr} \delta^{sc} \delta^{td} \delta^{ab} \right) + g_Y^4 \left( \frac{1156}{729} \delta^{pc} \delta^{rd} \delta^{st} \delta^{ab} + \frac{1156}{729} \delta^{pr} \delta^{sc} \delta^{td} \delta^{ab} \right) \right. \\
& + g_Y^2 \left( \frac{10}{9} \delta^{pc} \delta^{rd} \delta^{st} (Y_e^\dagger Y_e)^{ba} + \frac{10}{9} \delta^{pr} \delta^{sc} \delta^{td} (Y_e^\dagger Y_e)^{ba} \right) - \frac{1}{2} \delta^{sc} \delta^{td} (Y_e^\dagger Y_e)^{ba} (Y_u^\dagger Y_u)^{pr} - \frac{1}{2} \delta^{pc} \delta^{rd} (Y_e^\dagger Y_e)^{ba} (Y_u^\dagger Y_u)^{st} \Big\} C_{eu}^{abcd} + \left\{ g_Y^2 g_s^2 \left( \frac{50}{81} \delta^{pt} \delta^{rb} \delta^{sa} \delta^{cd} \right. \right. \\
& + \frac{50}{81} \delta^{pa} \delta^{rs} \delta^{tb} \delta^{cd} - \frac{482}{243} \delta^{pa} \delta^{rb} \delta^{st} \delta^{cd} - \frac{482}{243} \delta^{pr} \delta^{sa} \delta^{tb} \delta^{cd} \Big) + g_Y^4 \left( \frac{868}{729} \delta^{pa} \delta^{rb} \delta^{st} \delta^{cd} + \frac{868}{729} \delta^{pr} \delta^{sa} \delta^{tb} \delta^{cd} \right) + g_s^4 \left( \frac{73}{18} \delta^{pa} \delta^{rb} \delta^{st} \delta^{cd} \right. \\
& + \frac{73}{18} \delta^{pr} \delta^{sa} \delta^{tb} \delta^{cd} - \frac{1}{6} \delta^{pt} \delta^{rb} \delta^{sa} \delta^{cd} - \frac{1}{6} \delta^{pa} \delta^{rs} \delta^{tb} \delta^{cd} \Big) + g_Y^2 \left( \frac{2}{3} \delta^{pa} \delta^{rb} \delta^{st} (Y_d^\dagger Y_d)^{dc} + \frac{2}{3} \delta^{pr} \delta^{sa} \delta^{tb} (Y_d^\dagger Y_d)^{dc} \right) - \frac{1}{4} \delta^{sa} \delta^{tb} (Y_d^\dagger Y_u)^{dr} (Y_u^\dagger Y_d)^{pc}
\end{aligned}$$

$$\begin{aligned}
& -\frac{1}{4}\delta^{pa}\delta^{rb}(Y_d^\dagger Y_u)^{dt}(Y_u^\dagger Y_d)^{sc} - \frac{3}{2}\delta^{sa}\delta^{tb}(Y_d^\dagger Y_d)^{dc}(Y_u^\dagger Y_u)^{pr} - \frac{3}{2}\delta^{pa}\delta^{rb}(Y_d^\dagger Y_d)^{dc}(Y_u^\dagger Y_u)^{st} \Big\} C_{ud}^{(\parallel)abcd} + \left\{ g_Y^4 \left( \frac{868}{2187}\delta^{pa}\delta^{rb}\delta^{st}\delta^{cd} + \frac{868}{2187}\delta^{pr}\delta^{sa}\delta^{tb}\delta^{cd} \right) \right. \\
& + g_s^4 \left( \frac{2}{27}\delta^{pr}\delta^{st}\delta^{ab}\delta^{cd} + \frac{386}{81}\delta^{pt}\delta^{rb}\delta^{sa}\delta^{cd} + \frac{386}{81}\delta^{pa}\delta^{rs}\delta^{tb}\delta^{cd} - \frac{26}{243}\delta^{pa}\delta^{rb}\delta^{st}\delta^{cd} - \frac{26}{243}\delta^{pr}\delta^{sa}\delta^{tb}\delta^{cd} - \frac{2}{9}\delta^{pt}\delta^{rs}\delta^{ab}\delta^{cd} \right) \\
& + g_Y^2 \left( \frac{2}{9}\delta^{pa}\delta^{rb}\delta^{st}(Y_d^\dagger Y_d)^{dc} + \frac{2}{9}\delta^{pr}\delta^{sa}\delta^{tb}(Y_d^\dagger Y_d)^{dc} \right) + g_s^2 \left( \frac{1}{3}\delta^{pa}\delta^{rb}\delta^{st}(Y_d^\dagger Y_d)^{dc} + \frac{1}{3}\delta^{pr}\delta^{sa}\delta^{tb}(Y_d^\dagger Y_d)^{dc} - \delta^{pt}\delta^{rb}\delta^{sa}(Y_d^\dagger Y_d)^{dc} - \delta^{pa}\delta^{rs}\delta^{tb}(Y_d^\dagger Y_d)^{dc} \right) \\
& - \frac{1}{4}\delta^{rb}\delta^{sa}(Y_d^\dagger Y_u)^{dt}(Y_u^\dagger Y_d)^{pc} - \frac{1}{4}\delta^{pa}\delta^{tb}(Y_d^\dagger Y_u)^{dr}(Y_u^\dagger Y_d)^{sc} - \frac{1}{2}\delta^{sa}\delta^{tb}(Y_d^\dagger Y_d)^{dc}(Y_u^\dagger Y_u)^{pr} - \frac{1}{2}\delta^{pa}\delta^{rb}(Y_d^\dagger Y_d)^{dc}(Y_u^\dagger Y_u)^{st} - g_Y^2 g_s^2 \left( \frac{16}{81}\delta^{pr}\delta^{st}\delta^{ab}\delta^{cd} \right. \\
& + \frac{193}{243}\delta^{pt}\delta^{rb}\delta^{sa}\delta^{cd} + \frac{193}{243}\delta^{pa}\delta^{rs}\delta^{tb}\delta^{cd} + \frac{967}{729}\delta^{pa}\delta^{rb}\delta^{st}\delta^{cd} + \frac{967}{729}\delta^{pr}\delta^{sa}\delta^{tb}\delta^{cd} \Big\} C_{ud}^{(\times)abcd} + \left\{ \frac{7}{8}\delta^{tb}Y_u^{*as}Y_u^{*cp}(Y_d^\dagger Y_u)^{dr} + \frac{7}{8}\delta^{rb}Y_u^{*ap}Y_u^{*cs}(Y_d^\dagger Y_u)^{dt} \right. \\
& + g_Y^2 \left( \frac{7}{162}\delta^{rb}\delta^{st}Y_d^{*ad}Y_u^{*cp} + \frac{7}{162}\delta^{pr}\delta^{tb}Y_d^{*ad}Y_u^{*cs} - \frac{2}{27}\delta^{rb}\delta^{st}Y_d^{*cd}Y_u^{*ap} - \frac{2}{27}\delta^{pr}\delta^{tb}Y_d^{*cd}Y_u^{*as} \right) + g_s^2 \left( \frac{1}{9}\delta^{pt}\delta^{rb}Y_d^{*ad}Y_u^{*cs} + \frac{1}{9}\delta^{rs}\delta^{tb}Y_d^{*ad}Y_u^{*cp} \right. \\
& + \frac{2}{3}\delta^{pt}\delta^{rb}Y_d^{*cd}Y_u^{*as} + \frac{2}{3}\delta^{rs}\delta^{tb}Y_d^{*cd}Y_u^{*ap} - \frac{1}{27}\delta^{rb}\delta^{st}Y_d^{*ad}Y_u^{*cp} - \frac{1}{27}\delta^{pr}\delta^{tb}Y_d^{*ad}Y_u^{*cs} - \frac{2}{9}\delta^{rb}\delta^{st}Y_d^{*cd}Y_u^{*ap} - \frac{2}{9}\delta^{pr}\delta^{tb}Y_d^{*cd}Y_u^{*as} \Big\} \\
& - \frac{3}{8}\delta^{tb}Y_d^{*ad}Y_u^{*cs}(Y_u^\dagger Y_u)^{pr} - \frac{3}{8}\delta^{rb}Y_d^{*ad}Y_u^{*cp}(Y_u^\dagger Y_u)^{st} - \frac{9}{4}\delta^{tb}Y_d^{*cd}Y_u^{*as}(Y_u^\dagger Y_u)^{pr} - \frac{9}{4}\delta^{rb}Y_d^{*cd}Y_u^{*ap}(Y_u^\dagger Y_u)^{st} \Big\} C_{quqd}^{(\parallel)abcd} + \left( C_{quqd}^{(\parallel)*} \right)^{abcd} \left\{ \frac{7}{8}\delta^{sb}Y_u^{at}Y_u^{cr}(Y_u^\dagger Y_d)^{pd} \right. \\
& + \frac{7}{8}\delta^{pb}Y_u^{ar}Y_u^{ct}(Y_u^\dagger Y_d)^{sd} + g_Y^2 \left( \frac{7}{162}\delta^{pb}\delta^{st}Y_d^{ad}Y_u^{cr} + \frac{7}{162}\delta^{pr}\delta^{sb}Y_d^{ad}Y_u^{ct} - \frac{2}{27}\delta^{pb}\delta^{st}Y_d^{cd}Y_u^{ar} - \frac{2}{27}\delta^{pr}\delta^{sb}Y_d^{cd}Y_u^{at} \right) + g_s^2 \left( \frac{1}{9}\delta^{pb}\delta^{rs}Y_d^{ad}Y_u^{ct} + \frac{1}{9}\delta^{pt}\delta^{sb}Y_d^{ad}Y_u^{cr} \right. \\
& + \frac{2}{3}\delta^{pb}\delta^{rs}Y_d^{cd}Y_u^{at} + \frac{2}{3}\delta^{pt}\delta^{sb}Y_d^{cd}Y_u^{ar} - \frac{1}{27}\delta^{pb}\delta^{st}Y_d^{ad}Y_u^{cr} - \frac{1}{27}\delta^{pr}\delta^{sb}Y_d^{ad}Y_u^{ct} - \frac{2}{9}\delta^{pb}\delta^{st}Y_d^{cd}Y_u^{ar} - \frac{2}{9}\delta^{pr}\delta^{sb}Y_d^{cd}Y_u^{at} \Big\} - \frac{3}{8}\delta^{sb}Y_d^{ad}Y_u^{ct}(Y_u^\dagger Y_u)^{pr} \\
& - \frac{3}{8}\delta^{pb}Y_d^{ad}Y_u^{cr}(Y_u^\dagger Y_u)^{st} - \frac{9}{4}\delta^{sb}Y_d^{cd}Y_u^{at}(Y_u^\dagger Y_u)^{pr} - \frac{9}{4}\delta^{pb}Y_d^{cd}Y_u^{ar}(Y_u^\dagger Y_u)^{st} \Big\} + \left\{ \frac{7}{8}\delta^{tb}Y_u^{*ap}Y_u^{*cs}(Y_d^\dagger Y_u)^{dr} + \frac{7}{8}\delta^{rb}Y_u^{*as}Y_u^{*cp}(Y_d^\dagger Y_u)^{dt} \right. \\
& + g_Y^2 \left( \frac{7}{54}\delta^{rb}\delta^{st}Y_d^{*ad}Y_u^{*cp} + \frac{7}{54}\delta^{pr}\delta^{tb}Y_d^{*ad}Y_u^{*cs} - \frac{2}{81}\delta^{rb}\delta^{st}Y_d^{*cd}Y_u^{*ap} - \frac{2}{81}\delta^{pr}\delta^{tb}Y_d^{*cd}Y_u^{*as} \right) + g_s^2 \left( \frac{2}{9}\delta^{pt}\delta^{rb}Y_d^{*cd}Y_u^{*as} + \frac{2}{9}\delta^{rs}\delta^{tb}Y_d^{*cd}Y_u^{*cp} \right. \\
& + \frac{1}{3}\delta^{pt}\delta^{rb}Y_d^{*ad}Y_u^{*cs} + \frac{1}{3}\delta^{rs}\delta^{tb}Y_d^{*ad}Y_u^{*cp} - \frac{2}{27}\delta^{rb}\delta^{st}Y_d^{*cd}Y_u^{*ap} - \frac{2}{27}\delta^{pr}\delta^{tb}Y_d^{*cd}Y_u^{*as} - \frac{1}{9}\delta^{rb}\delta^{st}Y_d^{*ad}Y_u^{*cp} - \frac{1}{9}\delta^{pr}\delta^{tb}Y_d^{*ad}Y_u^{*cs} \Big\} \\
& - \frac{3}{4}\delta^{tb}Y_d^{*cd}Y_u^{*as}(Y_u^\dagger Y_u)^{pr} - \frac{3}{4}\delta^{rb}Y_d^{*cd}Y_u^{*ap}(Y_u^\dagger Y_u)^{st} - \frac{9}{8}\delta^{tb}Y_d^{*ad}Y_u^{*cs}(Y_u^\dagger Y_u)^{pr} - \frac{9}{8}\delta^{rb}Y_d^{*ad}Y_u^{*cp}(Y_u^\dagger Y_u)^{st} \Big\} C_{quqd}^{(\times)abcd} + \left( C_{quqd}^{(\times)*} \right)^{abcd} \left\{ \frac{7}{8}\delta^{sb}Y_u^{ar}Y_u^{ct}(Y_u^\dagger Y_d)^{pd} \right. \\
& + \frac{7}{8}\delta^{pb}Y_u^{at}Y_u^{cr}(Y_u^\dagger Y_d)^{sd} + g_Y^2 \left( \frac{7}{54}\delta^{pb}\delta^{st}Y_d^{ad}Y_u^{cr} + \frac{7}{54}\delta^{pr}\delta^{sb}Y_d^{ad}Y_u^{ct} - \frac{2}{81}\delta^{pb}\delta^{st}Y_d^{cd}Y_u^{ar} - \frac{2}{81}\delta^{pr}\delta^{sb}Y_d^{cd}Y_u^{at} \right) + g_s^2 \left( \frac{2}{9}\delta^{pb}\delta^{rs}Y_d^{cd}Y_u^{at} + \frac{2}{9}\delta^{pt}\delta^{sb}Y_d^{cd}Y_u^{ar} \right. \\
& + \frac{1}{3}\delta^{pb}\delta^{rs}Y_d^{ad}Y_u^{ct} + \frac{1}{3}\delta^{pt}\delta^{sb}Y_d^{ad}Y_u^{cr} - \frac{2}{27}\delta^{pb}\delta^{st}Y_d^{cd}Y_u^{ar} - \frac{2}{27}\delta^{pr}\delta^{sb}Y_d^{cd}Y_u^{at} - \frac{1}{9}\delta^{pb}\delta^{st}Y_d^{ad}Y_u^{cr} - \frac{1}{9}\delta^{pr}\delta^{sb}Y_d^{ad}Y_u^{ct} \Big\} - \frac{3}{4}\delta^{sb}Y_d^{cd}Y_u^{at}(Y_u^\dagger Y_u)^{pr} \\
& - \frac{3}{4}\delta^{pb}Y_d^{cd}Y_u^{ar}(Y_u^\dagger Y_u)^{st} - \frac{9}{8}\delta^{sb}Y_d^{ad}Y_u^{ct}(Y_u^\dagger Y_u)^{pr} - \frac{9}{8}\delta^{pb}Y_d^{ad}Y_u^{cr}(Y_u^\dagger Y_u)^{st} \Big\} + \left\{ \frac{3}{4}\delta^{td}Y_e^{*ab}Y_u^{*cs}(Y_u^\dagger Y_u)^{pr} + \frac{3}{4}\delta^{rd}Y_e^{*ab}Y_u^{*cp}(Y_u^\dagger Y_u)^{st} \right.
\end{aligned}$$



$$\begin{aligned}
& + g_Y^2 \left( \frac{2}{81} \delta^{rd} \delta^{st} Y_e^{*ab} Y_u^{*cp} + \frac{2}{81} \delta^{pr} \delta^{td} Y_e^{*ab} Y_u^{*cs} \right) + g_s^2 \left( \frac{2}{27} \delta^{rd} \delta^{st} Y_e^{*ab} Y_u^{*cp} + \frac{2}{27} \delta^{pr} \delta^{td} Y_e^{*ab} Y_u^{*cs} - \frac{2}{9} \delta^{pt} \delta^{rd} Y_e^{*ab} Y_u^{*cs} \right. \\
& \left. - \frac{2}{9} \delta^{rs} \delta^{td} Y_e^{*ab} Y_u^{*cp} \right) \left\{ C_{lequ}^{abcd} + C_{lequ}^{*abcd} \left\{ \frac{3}{4} \delta^{sd} Y_e^{ab} Y_u^{ct} (Y_u^\dagger Y_u)^{pr} + \frac{3}{4} \delta^{pd} Y_e^{ab} Y_u^{cr} (Y_u^\dagger Y_u)^{st} + g_Y^2 \left( \frac{2}{81} \delta^{pd} \delta^{st} Y_e^{ab} Y_u^{cr} + \frac{2}{81} \delta^{pr} \delta^{sd} Y_e^{ab} Y_u^{ct} \right) \right. \right. \\
& + g_s^2 \left( \frac{2}{27} \delta^{pd} \delta^{st} Y_e^{ab} Y_u^{cr} + \frac{2}{27} \delta^{pr} \delta^{sd} Y_e^{ab} Y_u^{ct} - \frac{2}{9} \delta^{pd} \delta^{rs} Y_e^{ab} Y_u^{ct} - \frac{2}{9} \delta^{pt} \delta^{sd} Y_e^{ab} Y_u^{cr} \right) \left. \right\} + \left\{ g_Y^2 \left( \frac{7}{162} \delta^{rb} \delta^{st} Y_e^{*ad} Y_u^{*cp} + \frac{7}{162} \delta^{pr} \delta^{tb} Y_e^{*ad} Y_u^{*cs} \right) \right. \\
& + g_s^2 \left( \frac{1}{9} \delta^{pt} \delta^{rb} Y_e^{*ad} Y_u^{*cs} + \frac{1}{9} \delta^{rs} \delta^{tb} Y_e^{*ad} Y_u^{*cp} - \frac{1}{27} \delta^{rb} \delta^{st} Y_e^{*ad} Y_u^{*cp} - \frac{1}{27} \delta^{pr} \delta^{tb} Y_e^{*ad} Y_u^{*cs} \right) - \frac{3}{8} \delta^{tb} Y_e^{*ad} Y_u^{*cs} (Y_u^\dagger Y_u)^{pr} \\
& \left. - \frac{3}{8} \delta^{rb} Y_e^{*ad} Y_u^{*cp} (Y_u^\dagger Y_u)^{st} \right\} C_{luqe}^{abcd} + C_{luqe}^{*abcd} \left\{ g_Y^2 \left( \frac{7}{162} \delta^{pb} \delta^{st} Y_e^{ad} Y_u^{cr} + \frac{7}{162} \delta^{pr} \delta^{sb} Y_e^{ad} Y_u^{ct} \right) + g_s^2 \left( \frac{1}{9} \delta^{pb} \delta^{rs} Y_e^{ad} Y_u^{ct} + \frac{1}{9} \delta^{pt} \delta^{sb} Y_e^{ad} Y_u^{cr} \right. \right. \\
& \left. - \frac{1}{27} \delta^{pb} \delta^{st} Y_e^{ad} Y_u^{cr} - \frac{1}{27} \delta^{pr} \delta^{sb} Y_e^{ad} Y_u^{ct} \right) - \frac{3}{8} \delta^{sb} Y_e^{ad} Y_u^{ct} (Y_u^\dagger Y_u)^{pr} - \frac{3}{8} \delta^{pb} Y_e^{ad} Y_u^{cr} (Y_u^\dagger Y_u)^{st} \left. \right\} + \frac{32}{81} \delta^{pr} \delta^{st} \delta^{ad} \delta^{bc} g_Y^4 C_{\ell\ell}^{abcd} + \left\{ \frac{32}{243} \delta^{pr} \delta^{st} \delta^{ad} \delta^{bc} g_Y^4 \right. \\
& + g_s^2 \left( \frac{4}{9} \delta^{pr} \delta^{bc} Y_u^{*as} Y_u^{dt} + \frac{4}{9} \delta^{st} \delta^{bc} Y_u^{*ap} Y_u^{dr} - \frac{4}{3} \delta^{pt} \delta^{bc} Y_u^{*as} Y_u^{dr} - \frac{4}{3} \delta^{rs} \delta^{bc} Y_u^{*ap} Y_u^{dt} \right) + g_s^4 \left( \frac{8}{9} \delta^{pt} \delta^{rs} \delta^{ad} \delta^{bc} - \frac{8}{27} \delta^{pr} \delta^{st} \delta^{ad} \delta^{bc} \right) + 2 Y_u^{*ap} Y_u^{*cs} Y_u^{br} Y_u^{dt} \\
& \left. - g_Y^2 \left( \frac{8}{27} \delta^{pr} \delta^{bc} Y_u^{*as} Y_u^{dt} + \frac{8}{27} \delta^{st} \delta^{bc} Y_u^{*ap} Y_u^{dr} \right) \right\} C_{qq}^{(\parallel)abcd} + \left\{ \frac{64}{243} \delta^{pr} \delta^{st} \delta^{ad} \delta^{bc} g_Y^4 + g_s^2 \left( \frac{8}{9} \delta^{pr} \delta^{bc} Y_u^{*as} Y_u^{dt} + \frac{8}{9} \delta^{st} \delta^{bc} Y_u^{*ap} Y_u^{dr} - \frac{8}{3} \delta^{pt} \delta^{bc} Y_u^{*as} Y_u^{dr} \right. \right. \\
& \left. - \frac{8}{3} \delta^{rs} \delta^{bc} Y_u^{*ap} Y_u^{dt} \right) + g_s^4 \left( \frac{16}{9} \delta^{pt} \delta^{rs} \delta^{ad} \delta^{bc} - \frac{16}{27} \delta^{pr} \delta^{st} \delta^{ad} \delta^{bc} \right) + 4 Y_u^{*ap} Y_u^{*cs} Y_u^{br} Y_u^{dt} - g_Y^2 \left( \frac{16}{27} \delta^{pr} \delta^{bc} Y_u^{*as} Y_u^{dt} + \frac{16}{27} \delta^{st} \delta^{bc} Y_u^{*ap} Y_u^{dr} \right) \left. \right\} C_{qq}^{(\times)abcd}, \tag{11.4}
\end{aligned}$$

### 11.3 $C_{dd}$

$$\begin{aligned}
\beta_{C_{dd}^{prst}}^{(1)} & = \left\{ \delta^{sa} \delta^{tb} (Y_d^\dagger Y_d)^{pr} + \delta^{pa} \delta^{rb} (Y_d^\dagger Y_d)^{st} - \frac{1}{9} g_Y^2 \left( \delta^{pa} \delta^{rb} \delta^{st} + \delta^{pr} \delta^{sa} \delta^{tb} \right) \right\} C_{Hd}^{ab} + \frac{2}{9} g_Y^2 \left\{ \delta^{pc} \delta^{rd} \delta^{st} \delta^{ab} + \delta^{pr} \delta^{sc} \delta^{td} \delta^{ab} \right\} C_{\ell d}^{abcd} - \left\{ \frac{2}{9} g_Y^2 \left( \delta^{pc} \delta^{rd} \delta^{st} \delta^{ab} \right. \right. \\
& + \delta^{pr} \delta^{sc} \delta^{td} \delta^{ab} \left. \right) + \delta^{pc} \delta^{rd} Y_d^{*as} Y_d^{bt} + \delta^{sc} \delta^{td} Y_d^{*ap} Y_d^{br} \left. \right\} C_{qd}^{(\parallel)abcd} - \left\{ \frac{2}{27} g_Y^2 \left( \delta^{pc} \delta^{rd} \delta^{st} \delta^{ab} + \delta^{pr} \delta^{sc} \delta^{td} \delta^{ab} \right) + \frac{2}{9} g_s^2 \left( \delta^{pc} \delta^{rd} \delta^{st} \delta^{ab} + \delta^{pr} \delta^{sc} \delta^{td} \delta^{ab} \right. \right. \\
& \left. - 3 \delta^{pt} \delta^{rd} \delta^{sc} \delta^{ab} - 3 \delta^{pc} \delta^{rs} \delta^{td} \delta^{ab} \right) + \delta^{rd} \delta^{sc} Y_d^{*ap} Y_d^{bt} + \delta^{pc} \delta^{td} Y_d^{*as} Y_d^{br} \left. \right\} C_{qd}^{(\times)abcd} + \left\{ \frac{4}{27} g_Y^2 \left( \delta^{pa} \delta^{rd} \delta^{st} \delta^{bc} + \delta^{pr} \delta^{sa} \delta^{td} \delta^{bc} + 3 \delta^{pa} \delta^{rb} \delta^{st} \delta^{cd} \right. \right. \\
& + 3 \delta^{pr} \delta^{sa} \delta^{tb} \delta^{cd} + 9 \delta^{pa} \delta^{rb} \delta^{sc} \delta^{td} \left. \right) + \frac{2}{9} g_s^2 \left( 3 \delta^{pt} \delta^{rd} \delta^{sa} \delta^{bc} + 3 \delta^{pa} \delta^{rs} \delta^{td} \delta^{bc} + 27 \delta^{pa} \delta^{rd} \delta^{sc} \delta^{tb} - \delta^{pa} \delta^{rd} \delta^{st} \delta^{bc} - \delta^{pr} \delta^{sa} \delta^{td} \delta^{bc} - 9 \delta^{pa} \delta^{rb} \delta^{sc} \delta^{td} \right) \\
& \left. + \delta^{rd} \delta^{sa} \delta^{tb} (Y_d^\dagger Y_d)^{pc} + \delta^{pa} \delta^{rb} \delta^{td} (Y_d^\dagger Y_d)^{sc} + \delta^{pa} \delta^{sc} \delta^{td} (Y_d^\dagger Y_d)^{br} + \delta^{pa} \delta^{rb} \delta^{sc} (Y_d^\dagger Y_d)^{dt} \right\} C_{dd}^{abcd} + \frac{2}{9} g_Y^2 \left\{ \delta^{pc} \delta^{rd} \delta^{st} \delta^{ab} + \delta^{pr} \delta^{sc} \delta^{td} \delta^{ab} \right\} C_{ed}^{abcd}
\end{aligned}$$

$$\begin{aligned}
& -\frac{4}{9}g_Y^2 \left\{ \delta^{pc} \delta^{rd} \delta^{st} \delta^{ab} + \delta^{pr} \delta^{sc} \delta^{td} \delta^{ab} \right\} C_{ud}^{(\parallel)abcd} + \left\{ \frac{1}{9}g_s^2 \left( 3\delta^{pt} \delta^{rd} \delta^{sc} \delta^{ab} + 3\delta^{pc} \delta^{rs} \delta^{td} \delta^{ab} - \delta^{pc} \delta^{rd} \delta^{st} \delta^{ab} - \delta^{pr} \delta^{sc} \delta^{td} \delta^{ab} \right) - \frac{4}{27}g_Y^2 \left( \delta^{pc} \delta^{rd} \delta^{st} \delta^{ab} \right. \right. \\
& \left. \left. + \delta^{pr} \delta^{sc} \delta^{td} \delta^{ab} \right) \right\} C_{ud}^{(\times)abcd}, \tag{11.5}
\end{aligned}$$

$$\begin{aligned}
\beta_{C_{dd}^{prst}}^{(2)} = & \left\{ \frac{4}{27} \delta^{pr} \delta^{st} g_Y^6 - g_Y^4 \left( \frac{7}{9} \delta^{st} (Y_d^\dagger Y_d)^{pr} + \frac{7}{9} \delta^{pr} (Y_d^\dagger Y_d)^{st} \right) \right\} C_{HB} + g_s^4 \left\{ \frac{2}{3} \delta^{st} (Y_d^\dagger Y_d)^{pr} + \frac{2}{3} \delta^{pr} (Y_d^\dagger Y_d)^{st} - 2\delta^{rs} (Y_d^\dagger Y_d)^{pt} - 2\delta^{pt} (Y_d^\dagger Y_d)^{sr} \right\} C_{HG} \\
& + \left\{ \frac{1}{9} \delta^{pr} \delta^{st} g_Y^4 g_L^2 - g_Y^2 g_L^2 \left( \frac{1}{4} \delta^{st} (Y_d^\dagger Y_d)^{pr} + \frac{1}{4} \delta^{pr} (Y_d^\dagger Y_d)^{st} \right) \right\} C_{HWPB} + \left\{ g_Y^2 g_s^6 \left( \frac{97}{27} \delta^{pr} \delta^{st} + 7\delta^{pt} \delta^{rs} \right) + g_s^6 \left( \frac{3}{2} \delta^{st} (Y_d^\dagger Y_d)^{pr} + \frac{3}{2} \delta^{pr} (Y_d^\dagger Y_d)^{st} \right. \right. \\
& - \frac{9}{2} \delta^{rs} (Y_d^\dagger Y_d)^{pt} - \frac{9}{2} \delta^{pt} (Y_d^\dagger Y_d)^{sr} \left. \right) - g_s^8 \left( \frac{29}{6} \delta^{pt} \delta^{rs} + \frac{331}{18} \delta^{pr} \delta^{st} \right) \left\} C_G - \frac{2}{9} \delta^{pr} \delta^{st} g_Y^4 Y_e^{*ab} C_{eB}^{ab} - \frac{2}{9} \delta^{pr} \delta^{st} g_Y^4 C_{eB}^{*ab} Y_e^{ab} + \frac{10}{27} \delta^{pr} \delta^{st} g_Y^4 Y_u^{*ab} C_{uB}^{ab} \right. \\
& + \frac{10}{27} \delta^{pr} \delta^{st} g_Y^4 C_{uB}^{*ab} Y_u^{ab} + g_s^4 \left\{ \frac{2}{3} \delta^{pt} \delta^{rs} Y_u^{*ab} - \frac{2}{9} \delta^{pr} \delta^{st} Y_u^{*ab} \right\} C_{uG}^{ab} + g_s^4 C_{uG}^{*ab} \left\{ \frac{2}{3} \delta^{pt} \delta^{rs} Y_u^{ab} - \frac{2}{9} \delta^{pr} \delta^{st} Y_u^{ab} \right\} + \left\{ g_Y^2 g_s^2 \left( \frac{32}{27} \delta^{rb} \delta^{st} Y_d^{*ap} \right. \right. \\
& + \frac{32}{27} \delta^{pr} \delta^{tb} Y_d^{*as} + \frac{16}{9} \delta^{pt} \delta^{rb} Y_d^{*as} + \frac{16}{9} \delta^{rs} \delta^{tb} Y_d^{*ap} \left. \right) + g_Y^2 \left( \frac{1}{3} \delta^{st} Y_d^{*ap} (Y_d^\dagger Y_d)^{br} + \frac{1}{3} \delta^{pr} Y_d^{*as} (Y_d^\dagger Y_d)^{bt} - \frac{3}{2} \delta^{tb} Y_d^{*as} (Y_d^\dagger Y_d)^{pr} - \frac{3}{2} \delta^{rb} Y_d^{*ap} (Y_d^\dagger Y_d)^{st} \right) \\
& - g_Y^4 \left( \frac{2}{27} \delta^{pr} \delta^{st} Y_d^{*ab} + \frac{28}{81} \delta^{rb} \delta^{st} Y_d^{*ap} + \frac{28}{81} \delta^{pr} \delta^{tb} Y_d^{*as} \right) \left\} C_{dB}^{ab} + C_{dB}^{*ab} \left\{ g_Y^2 g_s^2 \left( \frac{32}{27} \delta^{pb} \delta^{st} Y_d^{ar} + \frac{32}{27} \delta^{pr} \delta^{sb} Y_d^{at} + \frac{16}{9} \delta^{pb} \delta^{rs} Y_d^{at} + \frac{16}{9} \delta^{pt} \delta^{sb} Y_d^{ar} \right) \right. \right. \\
& + g_Y^2 \left( \frac{1}{3} \delta^{st} Y_d^{ar} (Y_d^\dagger Y_d)^{pb} + \frac{1}{3} \delta^{pr} Y_d^{at} (Y_d^\dagger Y_d)^{sb} - \frac{3}{2} \delta^{sb} Y_d^{at} (Y_d^\dagger Y_d)^{pr} - \frac{3}{2} \delta^{pb} Y_d^{ar} (Y_d^\dagger Y_d)^{st} \right) - g_Y^4 \left( \frac{2}{27} \delta^{pr} \delta^{st} Y_d^{ab} + \frac{28}{81} \delta^{pb} \delta^{st} Y_d^{ar} + \frac{28}{81} \delta^{pr} \delta^{sb} Y_d^{at} \right) \left. \right\} \\
& + \left\{ g_Y^2 g_L^2 \left( \frac{1}{18} \delta^{rb} \delta^{st} Y_d^{*ap} + \frac{1}{18} \delta^{pr} \delta^{tb} Y_d^{*as} \right) + g_s^2 g_L^2 \left( \frac{2}{3} \delta^{rb} \delta^{st} Y_d^{*ap} + \frac{2}{3} \delta^{pr} \delta^{tb} Y_d^{*as} - 2\delta^{pt} \delta^{rb} Y_d^{*as} - 2\delta^{rs} \delta^{tb} Y_d^{*ap} \right) + g_L^2 \left( \frac{9}{4} \delta^{tb} Y_d^{*as} (Y_d^\dagger Y_d)^{pr} \right. \right. \\
& + \frac{9}{4} \delta^{rb} Y_d^{*ap} (Y_d^\dagger Y_d)^{st} \left. \right) \left\} C_{dW}^{ab} + C_{dW}^{*ab} \left\{ g_Y^2 g_L^2 \left( \frac{1}{18} \delta^{pb} \delta^{st} Y_d^{ar} + \frac{1}{18} \delta^{pr} \delta^{sb} Y_d^{at} \right) + g_s^2 g_L^2 \left( \frac{2}{3} \delta^{pb} \delta^{st} Y_d^{ar} + \frac{2}{3} \delta^{pr} \delta^{sb} Y_d^{at} - 2\delta^{pb} \delta^{rs} Y_d^{at} - 2\delta^{pt} \delta^{sb} Y_d^{ar} \right) \right. \right. \\
& + g_L^2 \left( \frac{9}{4} \delta^{sb} Y_d^{at} (Y_d^\dagger Y_d)^{pr} + \frac{9}{4} \delta^{pb} Y_d^{ar} (Y_d^\dagger Y_d)^{st} \right) \left. \right\} + \left\{ g_Y^2 g_s^2 \left( \frac{16}{81} \delta^{rb} \delta^{st} Y_d^{*ap} + \frac{16}{81} \delta^{pr} \delta^{tb} Y_d^{*as} + \frac{4}{9} \delta^{pt} \delta^{rb} Y_d^{*as} + \frac{4}{9} \delta^{rs} \delta^{tb} Y_d^{*ap} \right) + g_s^4 \left( \frac{2}{3} \delta^{pt} \delta^{rs} Y_d^{*ab} \right. \right. \\
& + \frac{8}{9} \delta^{pt} \delta^{rb} Y_d^{*as} + \frac{8}{9} \delta^{rs} \delta^{tb} Y_d^{*ap} - \frac{2}{9} \delta^{pr} \delta^{st} Y_d^{*ab} - \frac{80}{27} \delta^{rb} \delta^{st} Y_d^{*ap} - \frac{80}{27} \delta^{pr} \delta^{tb} Y_d^{*as} \left. \right) + g_s^2 \left( \frac{1}{6} \delta^{st} Y_d^{*ap} (Y_d^\dagger Y_d)^{br} + \frac{1}{6} \delta^{pr} Y_d^{*as} (Y_d^\dagger Y_d)^{bt} \right. \\
& \left. \left. + 3\delta^{tb} Y_d^{*as} (Y_d^\dagger Y_d)^{pr} + 3\delta^{rb} Y_d^{*as} (Y_d^\dagger Y_d)^{pt} + 3\delta^{tb} Y_d^{*ap} (Y_d^\dagger Y_d)^{sr} + 3\delta^{rb} Y_d^{*ap} (Y_d^\dagger Y_d)^{st} - \frac{1}{2} \delta^{pt} Y_d^{*as} (Y_d^\dagger Y_d)^{br} - \frac{1}{2} \delta^{rs} Y_d^{*ap} (Y_d^\dagger Y_d)^{bt} \right) \right\} C_{dG}^{ab}
\end{aligned}$$

$$\begin{aligned}
& + C_{dG}^{*ab} \left\{ g_Y^2 g_s^2 \left( \frac{16}{81} \delta^{pb} \delta^{st} Y_d^{ar} + \frac{16}{81} \delta^{pr} \delta^{sb} Y_d^{at} + \frac{4}{9} \delta^{pb} \delta^{rs} Y_d^{at} + \frac{4}{9} \delta^{pt} \delta^{sb} Y_d^{ar} \right) + g_s^4 \left( \frac{2}{3} \delta^{pt} \delta^{rs} Y_d^{ab} + \frac{8}{9} \delta^{pb} \delta^{rs} Y_d^{at} + \frac{8}{9} \delta^{pt} \delta^{sb} Y_d^{ar} - \frac{2}{9} \delta^{pr} \delta^{st} Y_d^{ab} \right. \right. \\
& - \frac{80}{27} \delta^{pb} \delta^{st} Y_d^{ar} - \frac{80}{27} \delta^{pr} \delta^{sb} Y_d^{at} \left. \right) + g_s^2 \left( \frac{1}{6} \delta^{st} Y_d^{ar} (Y_d^\dagger Y_d)^{pb} + \frac{1}{6} \delta^{pr} Y_d^{at} (Y_d^\dagger Y_d)^{sb} + 3 \delta^{sb} Y_d^{at} (Y_d^\dagger Y_d)^{pr} + 3 \delta^{sb} Y_d^{ar} (Y_d^\dagger Y_d)^{pt} + 3 \delta^{pb} Y_d^{at} (Y_d^\dagger Y_d)^{sr} \right. \\
& + 3 \delta^{pb} Y_d^{ar} (Y_d^\dagger Y_d)^{st} - \frac{1}{2} \delta^{rs} Y_d^{at} (Y_d^\dagger Y_d)^{pb} - \frac{1}{2} \delta^{pt} Y_d^{ar} (Y_d^\dagger Y_d)^{sb} \left. \right) \left. \right\} + \left\{ \frac{1}{4} \delta^{rb} (Y_d^\dagger Y_d)^{pa} (Y_d^\dagger Y_d)^{st} + \frac{1}{4} \delta^{tb} (Y_d^\dagger Y_d)^{pr} (Y_d^\dagger Y_d)^{sa} + \frac{1}{4} \delta^{pa} (Y_d^\dagger Y_d)^{st} (Y_d^\dagger Y_d)^{br} \right. \\
& + \frac{1}{4} \delta^{sa} (Y_d^\dagger Y_d)^{pr} (Y_d^\dagger Y_d)^{bt} + g_Y^2 g_s^2 \left( \frac{91}{162} \delta^{pt} \delta^{rb} \delta^{sa} + \frac{91}{162} \delta^{pa} \delta^{rs} \delta^{tb} - \frac{91}{486} \delta^{pa} \delta^{rb} \delta^{st} - \frac{91}{486} \delta^{pr} \delta^{sa} \delta^{tb} \right) + g_L^2 \left( \frac{51}{8} \delta^{sa} \delta^{tb} (Y_d^\dagger Y_d)^{pr} \right. \\
& + \frac{51}{8} \delta^{pa} \delta^{rb} (Y_d^\dagger Y_d)^{st} \left. \right) + g_Y^2 \left( \frac{1}{9} T_2 \delta^{pa} \delta^{rb} \delta^{st} + \frac{1}{9} T_2 \delta^{pr} \delta^{sa} \delta^{tb} + \frac{149}{72} \delta^{sa} \delta^{tb} (Y_d^\dagger Y_d)^{pr} + \frac{149}{72} \delta^{pa} \delta^{rb} (Y_d^\dagger Y_d)^{st} - \frac{73}{324} \delta^{rb} \delta^{st} (Y_d^\dagger Y_d)^{pa} \right. \\
& - \frac{73}{324} \delta^{pr} \delta^{tb} (Y_d^\dagger Y_d)^{sa} - \frac{73}{324} \delta^{pa} \delta^{st} (Y_d^\dagger Y_d)^{br} - \frac{73}{324} \delta^{pr} \delta^{sa} (Y_d^\dagger Y_d)^{bt} \left. \right) + g_s^2 \left( \frac{7}{54} \delta^{rb} \delta^{st} (Y_d^\dagger Y_d)^{pa} + \frac{7}{54} \delta^{pr} \delta^{tb} (Y_d^\dagger Y_d)^{sa} + \frac{7}{54} \delta^{pa} \delta^{st} (Y_d^\dagger Y_d)^{br} \right. \\
& + \frac{7}{54} \delta^{pr} \delta^{sa} (Y_d^\dagger Y_d)^{bt} - \frac{7}{18} \delta^{rs} \delta^{tb} (Y_d^\dagger Y_d)^{pa} - \frac{7}{18} \delta^{pt} \delta^{rb} (Y_d^\dagger Y_d)^{sa} - \frac{7}{18} \delta^{pt} \delta^{sa} (Y_d^\dagger Y_d)^{br} - \frac{7}{18} \delta^{pa} \delta^{rs} (Y_d^\dagger Y_d)^{bt} - \frac{7}{2} \delta^{rb} \delta^{sa} (Y_d^\dagger Y_d)^{pt} - \frac{7}{2} \delta^{pa} \delta^{tb} (Y_d^\dagger Y_d)^{sr} \\
& - \frac{25}{6} \delta^{sa} \delta^{tb} (Y_d^\dagger Y_d)^{pr} - \frac{25}{6} \delta^{pa} \delta^{rb} (Y_d^\dagger Y_d)^{st} \left. \right) - g_Y^4 \left( \frac{152}{729} \delta^{pa} \delta^{rb} \delta^{st} + \frac{152}{729} \delta^{pr} \delta^{sa} \delta^{tb} \right) - g_Y^2 g_L^2 \left( \delta^{pa} \delta^{rb} \delta^{st} + \delta^{pr} \delta^{sa} \delta^{tb} \right) - T_2 \delta^{sa} \delta^{tb} (Y_d^\dagger Y_d)^{pr} \\
& - T_2 \delta^{pa} \delta^{rb} (Y_d^\dagger Y_d)^{st} - \frac{3}{2} \delta^{sa} \delta^{tb} (Y_d^\dagger Y_d Y_d^\dagger Y_d)^{pr} - \frac{3}{2} \delta^{pa} \delta^{rb} (Y_d^\dagger Y_d Y_d^\dagger Y_d)^{st} \left. \right\} C_{Hd}^{ab} + \left\{ g_s^2 \left( \frac{1}{54} \delta^{rb} \delta^{st} (Y_d^\dagger Y_u)^{pa} + \frac{1}{54} \delta^{pr} \delta^{tb} (Y_d^\dagger Y_u)^{sa} \right. \right. \\
& - \frac{1}{18} \delta^{rs} \delta^{tb} (Y_d^\dagger Y_u)^{pa} - \frac{1}{18} \delta^{pt} \delta^{rb} (Y_d^\dagger Y_u)^{sa} \left. \right) + g_Y^2 \left( \frac{59}{324} \delta^{rb} \delta^{st} (Y_d^\dagger Y_u)^{pa} + \frac{59}{324} \delta^{pr} \delta^{tb} (Y_d^\dagger Y_u)^{sa} \right) - \frac{3}{4} \delta^{rb} (Y_d^\dagger Y_d)^{st} (Y_d^\dagger Y_u)^{pa} \\
& - \frac{3}{4} \delta^{tb} (Y_d^\dagger Y_d)^{pr} (Y_d^\dagger Y_u)^{sa} \left. \right\} C_{Hud}^{ab} + C_{Hud}^{*ab} \left\{ g_s^2 \left( \frac{1}{54} \delta^{pb} \delta^{st} (Y_u^\dagger Y_d)^{ar} + \frac{1}{54} \delta^{pr} \delta^{sb} (Y_u^\dagger Y_d)^{at} - \frac{1}{18} \delta^{pt} \delta^{sb} (Y_u^\dagger Y_d)^{ar} - \frac{1}{18} \delta^{pb} \delta^{rs} (Y_u^\dagger Y_d)^{at} \right) \right. \\
& + g_Y^2 \left( \frac{59}{324} \delta^{pb} \delta^{st} (Y_u^\dagger Y_d)^{ar} + \frac{59}{324} \delta^{pr} \delta^{sb} (Y_u^\dagger Y_d)^{at} \right) - \frac{3}{4} \delta^{pb} (Y_d^\dagger Y_d)^{st} (Y_u^\dagger Y_d)^{ar} - \frac{3}{4} \delta^{sb} (Y_d^\dagger Y_d)^{pr} (Y_u^\dagger Y_d)^{at} \left. \right\} + \left\{ g_Y^2 g_s^2 \left( \frac{25}{243} \delta^{pc} \delta^{rd} \delta^{st} \delta^{ab} \right. \right. \\
& + \frac{25}{243} \delta^{pr} \delta^{sc} \delta^{td} \delta^{ab} - \frac{25}{81} \delta^{pt} \delta^{rd} \delta^{sc} \delta^{ab} - \frac{25}{81} \delta^{pc} \delta^{rs} \delta^{td} \delta^{ab} \left. \right) + g_Y^2 g_L^2 \left( \frac{1}{2} \delta^{pc} \delta^{rd} \delta^{st} \delta^{ab} + \frac{1}{2} \delta^{pr} \delta^{sc} \delta^{td} \delta^{ab} \right) - \frac{1}{2} \delta^{sc} \delta^{td} (Y_d^\dagger Y_d)^{pr} (Y_e Y_e^\dagger)^{ba} \\
& - \frac{1}{2} \delta^{pc} \delta^{rd} (Y_d^\dagger Y_d)^{st} (Y_e Y_e^\dagger)^{ba} - g_Y^4 \left( \frac{937}{1458} \delta^{pc} \delta^{rd} \delta^{st} \delta^{ab} + \frac{937}{1458} \delta^{pr} \delta^{sc} \delta^{td} \delta^{ab} \right) - g_Y^2 \left( \frac{4}{9} \delta^{pc} \delta^{rd} \delta^{st} (Y_e Y_e^\dagger)^{ba} + \frac{4}{9} \delta^{pr} \delta^{sc} \delta^{td} (Y_e Y_e^\dagger)^{ba} \right) \left. \right\} C_{\ell d}^{abcd} \\
& + \left\{ \frac{1}{4} \delta^{sc} \delta^{td} Y_d^{br} (Y_u^\dagger Y_u Y_d^\dagger)^{ap} + \frac{1}{4} \delta^{pc} \delta^{rd} Y_d^{bt} (Y_u^\dagger Y_u Y_d^\dagger)^{as} + \frac{1}{4} \delta^{sc} \delta^{td} Y_d^{*ap} (Y_u Y_u^\dagger Y_d)^{br} + \frac{1}{4} \delta^{pc} \delta^{rd} Y_d^{*as} (Y_u Y_u^\dagger Y_d)^{bt} + \frac{3}{4} \delta^{sc} \delta^{td} Y_d^{br} (Y_d^\dagger Y_d Y_d^\dagger)^{ap} \right. \\
& + \frac{3}{4} \delta^{pc} \delta^{rd} Y_d^{bt} (Y_d^\dagger Y_d Y_d^\dagger)^{as} + \frac{3}{4} \delta^{sc} \delta^{td} Y_d^{*ap} (Y_d Y_d^\dagger Y_d)^{br} + \frac{3}{4} \delta^{pc} \delta^{rd} Y_d^{*as} (Y_d Y_d^\dagger Y_d)^{bt} + g_s^2 \left( \frac{4}{27} \delta^{pc} \delta^{st} Y_d^{*ad} Y_d^{br} + \frac{4}{27} \delta^{rd} \delta^{st} Y_d^{*ap} Y_d^{bc} \right. \\
& + \frac{4}{27} \delta^{pr} \delta^{sc} Y_d^{*ad} Y_d^{bt} + \frac{4}{27} \delta^{pr} \delta^{td} Y_d^{*as} Y_d^{bc} + 6 \delta^{pc} \delta^{rd} Y_d^{*as} Y_d^{bt} + 6 \delta^{sc} \delta^{td} Y_d^{*ap} Y_d^{br} - \frac{4}{9} \delta^{pc} \delta^{rs} Y_d^{*ad} Y_d^{bt} - \frac{4}{9} \delta^{pt} \delta^{rd} Y_d^{*as} Y_d^{bc} - \frac{4}{9} \delta^{pt} \delta^{sc} Y_d^{*ad} Y_d^{br} \left. \right\}
\end{aligned}$$

$$\begin{aligned}
& -\frac{4}{9}\delta^{rs}\delta^{td}Y_d^{*ap}Y_d^{bc} - 2\delta^{rd}\delta^{sc}Y_d^{*ap}Y_d^{bt} - 2\delta^{pc}\delta^{td}Y_d^{*as}Y_d^{br}) + g_Y^2 g_s^2 \left( \frac{25}{81}\delta^{pt}\delta^{rd}\delta^{sc}\delta^{ab} + \frac{25}{81}\delta^{pc}\delta^{rs}\delta^{td}\delta^{ab} - \frac{241}{243}\delta^{pc}\delta^{rd}\delta^{st}\delta^{ab} - \frac{241}{243}\delta^{pr}\delta^{sc}\delta^{td}\delta^{ab} \right) \\
& + \delta^{sc}Y_d^{*ad}Y_d^{bt}(Y_d^\dagger Y_d)^{pr} + \delta^{td}Y_d^{*as}Y_d^{bc}(Y_d^\dagger Y_d)^{pr} + \delta^{pc}Y_d^{*ad}Y_d^{br}(Y_d^\dagger Y_d)^{st} + \delta^{rd}Y_d^{*ap}Y_d^{bc}(Y_d^\dagger Y_d)^{st} + g_Y^2 \left( \frac{10}{81}\delta^{pc}\delta^{st}Y_d^{*ad}Y_d^{br} + \frac{10}{81}\delta^{rd}\delta^{st}Y_d^{*ap}Y_d^{bc} \right. \\
& + \frac{10}{81}\delta^{pr}\delta^{sc}Y_d^{*ad}Y_d^{bt} + \frac{10}{81}\delta^{pr}\delta^{td}Y_d^{*as}Y_d^{bc} + \frac{2}{3}\delta^{pc}\delta^{rd}\delta^{st}(Y_u Y_u^\dagger)^{ba} + \frac{2}{3}\delta^{pr}\delta^{sc}\delta^{td}(Y_u Y_u^\dagger)^{ba} - \frac{59}{24}\delta^{pc}\delta^{rd}Y_d^{*as}Y_d^{bt} - \frac{59}{24}\delta^{sc}\delta^{td}Y_d^{*ap}Y_d^{br} \Big) \\
& + \frac{3}{2}T_2\delta^{pc}\delta^{rd}Y_d^{*as}Y_d^{bt} + \frac{3}{2}T_2\delta^{sc}\delta^{td}Y_d^{*ap}Y_d^{br} + \frac{3}{2}\delta^{sc}\delta^{td}(Y_d^\dagger Y_d)^{pr}(Y_u Y_u^\dagger)^{ba} + \frac{3}{2}\delta^{pc}\delta^{rd}(Y_d^\dagger Y_d)^{st}(Y_u Y_u^\dagger)^{ba} + \frac{7}{4}\delta^{rd}Y_d^{*as}Y_d^{bt}(Y_d^\dagger Y_d)^{pc} \\
& + \frac{7}{4}\delta^{td}Y_d^{*ap}Y_d^{br}(Y_d^\dagger Y_d)^{sc} + \frac{7}{4}\delta^{pc}Y_d^{*as}Y_d^{bt}(Y_d^\dagger Y_d)^{dr} + \frac{7}{4}\delta^{sc}Y_d^{*ap}Y_d^{br}(Y_d^\dagger Y_d)^{dt} - g_L^2 \left( \frac{51}{8}\delta^{pc}\delta^{rd}Y_d^{*as}Y_d^{bt} + \frac{51}{8}\delta^{sc}\delta^{td}Y_d^{*ap}Y_d^{br} \right) - g_Y^4 \left( \frac{287}{1458}\delta^{pc}\delta^{rd}\delta^{st}\delta^{ab} \right. \\
& + \frac{287}{1458}\delta^{pr}\delta^{sc}\delta^{td}\delta^{ab} \Big) - g_Y^2 g_L^2 \left( \frac{1}{2}\delta^{pc}\delta^{rd}\delta^{st}\delta^{ab} + \frac{1}{2}\delta^{pr}\delta^{sc}\delta^{td}\delta^{ab} \right) - g_s^4 \left( \frac{11}{3}\delta^{pt}\delta^{rd}\delta^{sc}\delta^{ab} + \frac{11}{3}\delta^{pc}\delta^{rs}\delta^{td}\delta^{ab} + \frac{61}{9}\delta^{pc}\delta^{rd}\delta^{st}\delta^{ab} + \frac{61}{9}\delta^{pr}\delta^{sc}\delta^{td}\delta^{ab} \right) \\
& - \frac{3}{2}\delta^{sc}\delta^{td}(Y_d^\dagger Y_d)^{pr}(Y_d Y_d^\dagger)^{ba} - \frac{3}{2}\delta^{pc}\delta^{rd}(Y_d^\dagger Y_d)^{st}(Y_d Y_d^\dagger)^{ba} \Big\} C_{qd}^{(II)abcd} + \left\{ \frac{1}{4}\delta^{rd}\delta^{sc}Y_d^{bt}(Y_u^\dagger Y_u Y_d^\dagger)^{ap} + \frac{1}{4}\delta^{pc}\delta^{td}Y_d^{br}(Y_u^\dagger Y_u Y_d^\dagger)^{as} + \frac{1}{4}\delta^{pc}\delta^{td}Y_d^{*as}(Y_u Y_u^\dagger Y_d)^{br} \right. \\
& + \frac{1}{4}\delta^{rd}\delta^{sc}Y_d^{*ap}(Y_u Y_u^\dagger Y_d)^{bt} + \frac{1}{2}\delta^{sc}\delta^{td}(Y_d^\dagger Y_d)^{pr}(Y_u Y_u^\dagger)^{ba} + \frac{1}{2}\delta^{pc}\delta^{rd}(Y_d^\dagger Y_d)^{st}(Y_u Y_u^\dagger)^{ba} + \frac{3}{4}\delta^{rd}\delta^{sc}Y_d^{bt}(Y_d^\dagger Y_d Y_d^\dagger)^{ap} + \frac{3}{4}\delta^{pc}\delta^{td}Y_d^{br}(Y_d^\dagger Y_d Y_d^\dagger)^{as} \\
& + \frac{3}{4}\delta^{pc}\delta^{td}Y_d^{*as}(Y_d Y_d^\dagger Y_d)^{br} + \frac{3}{4}\delta^{rd}\delta^{sc}Y_d^{*ap}(Y_d Y_d^\dagger Y_d)^{bt} + g_s^2 g_L^2 \left( \frac{3}{2}\delta^{pt}\delta^{rd}\delta^{sc}\delta^{ab} + \frac{3}{2}\delta^{pc}\delta^{rs}\delta^{td}\delta^{ab} - \frac{1}{2}\delta^{pc}\delta^{rd}\delta^{st}\delta^{ab} - \frac{1}{2}\delta^{pr}\delta^{sc}\delta^{td}\delta^{ab} \right) \\
& + g_Y^2 g_s^2 \left( \frac{635}{486}\delta^{pt}\delta^{rd}\delta^{sc}\delta^{ab} + \frac{635}{486}\delta^{pc}\delta^{rs}\delta^{td}\delta^{ab} - \frac{8}{81}\delta^{pr}\delta^{st}\delta^{ab}\delta^{cd} - \frac{355}{1458}\delta^{pc}\delta^{rd}\delta^{st}\delta^{ab} - \frac{355}{1458}\delta^{pr}\delta^{sc}\delta^{td}\delta^{ab} \right) + g_s^4 \left( \frac{4}{27}\delta^{pr}\delta^{st}\delta^{ab}\delta^{cd} \right. \\
& + \frac{52}{81}\delta^{pt}\delta^{rd}\delta^{sc}\delta^{ab} + \frac{52}{81}\delta^{pc}\delta^{rs}\delta^{td}\delta^{ab} - \frac{4}{9}\delta^{pt}\delta^{rs}\delta^{ab}\delta^{cd} - \frac{628}{243}\delta^{pc}\delta^{rd}\delta^{st}\delta^{ab} - \frac{628}{243}\delta^{pr}\delta^{sc}\delta^{td}\delta^{ab} \Big) + g_Y^2 \left( \frac{2}{27}\delta^{pr}\delta^{cd}Y_d^{*as}Y_d^{bt} + \frac{2}{27}\delta^{st}\delta^{cd}Y_d^{*ap}Y_d^{br} \right. \\
& + \frac{2}{27}\delta^{pc}\delta^{rd}\delta^{st}(Y_d Y_d^\dagger)^{ba} + \frac{2}{27}\delta^{pr}\delta^{sc}\delta^{td}(Y_d Y_d^\dagger)^{ba} + \frac{4}{27}\delta^{pc}\delta^{st}Y_d^{*ad}Y_d^{br} + \frac{4}{27}\delta^{rd}\delta^{st}Y_d^{*ap}Y_d^{bc} + \frac{4}{27}\delta^{pr}\delta^{sc}Y_d^{*ad}Y_d^{bt} + \frac{4}{27}\delta^{pr}\delta^{td}Y_d^{*as}Y_d^{bc} \\
& + \frac{2}{9}\delta^{pc}\delta^{rd}\delta^{st}(Y_u Y_u^\dagger)^{ba} + \frac{2}{9}\delta^{pr}\delta^{sc}\delta^{td}(Y_u Y_u^\dagger)^{ba} - \frac{59}{24}\delta^{rd}\delta^{sc}Y_d^{*ap}Y_d^{bt} - \frac{59}{24}\delta^{pc}\delta^{td}Y_d^{*as}Y_d^{br} \Big) + g_s^2 \left( \frac{1}{9}\delta^{pc}\delta^{st}Y_d^{*ad}Y_d^{br} + \frac{1}{9}\delta^{rd}\delta^{st}Y_d^{*ap}Y_d^{bc} \right. \\
& + \frac{1}{9}\delta^{pr}\delta^{sc}Y_d^{*ad}Y_d^{bt} + \frac{1}{9}\delta^{pr}\delta^{td}Y_d^{*as}Y_d^{bc} + \frac{2}{9}\delta^{pc}\delta^{rd}\delta^{st}(Y_d Y_d^\dagger)^{ba} + \frac{2}{9}\delta^{pr}\delta^{sc}\delta^{td}(Y_d Y_d^\dagger)^{ba} + \frac{1}{3}\delta^{pt}\delta^{cd}Y_d^{*as}Y_d^{br} + \frac{1}{3}\delta^{rs}\delta^{cd}Y_d^{*ap}Y_d^{bt} + \frac{1}{3}\delta^{pc}\delta^{rd}\delta^{st}(Y_u Y_u^\dagger)^{ba} \\
& + \frac{1}{3}\delta^{pr}\delta^{sc}\delta^{td}(Y_u Y_u^\dagger)^{ba} + 2\delta^{pc}\delta^{rd}Y_d^{*as}Y_d^{bt} + 2\delta^{sc}\delta^{td}Y_d^{*ap}Y_d^{br} - \frac{1}{9}\delta^{pr}\delta^{cd}Y_d^{*as}Y_d^{bt} - \frac{1}{9}\delta^{st}\delta^{cd}Y_d^{*ap}Y_d^{br} - \frac{1}{3}\delta^{pc}\delta^{rs}Y_d^{*ad}Y_d^{bt} - \frac{1}{3}\delta^{pt}\delta^{rd}Y_d^{*as}Y_d^{bc} \\
& - \frac{1}{3}\delta^{pt}\delta^{sc}Y_d^{*ad}Y_d^{br} - \frac{1}{3}\delta^{rs}\delta^{td}Y_d^{*ap}Y_d^{bc} - \frac{2}{3}\delta^{pt}\delta^{rd}\delta^{sc}(Y_d Y_d^\dagger)^{ba} - \frac{2}{3}\delta^{pc}\delta^{rs}\delta^{td}(Y_d Y_d^\dagger)^{ba} - \delta^{pt}\delta^{rd}\delta^{sc}(Y_u Y_u^\dagger)^{ba} - \delta^{pc}\delta^{rs}\delta^{td}(Y_u Y_u^\dagger)^{ba} - 6\delta^{rd}\delta^{sc}Y_d^{*ap}Y_d^{bt} \\
& - 6\delta^{pc}\delta^{td}Y_d^{*as}Y_d^{br} \Big) + \frac{3}{2}T_2\delta^{rd}\delta^{sc}Y_d^{*ap}Y_d^{bt} + \frac{3}{2}T_2\delta^{pc}\delta^{td}Y_d^{*as}Y_d^{br} + \frac{7}{4}\delta^{td}Y_d^{*as}Y_d^{br}(Y_d^\dagger Y_d)^{pc} + \frac{7}{4}\delta^{rd}Y_d^{*ap}Y_d^{bt}(Y_d^\dagger Y_d)^{sc} + \frac{7}{4}\delta^{sc}Y_d^{*ap}Y_d^{bt}(Y_d^\dagger Y_d)^{dr} \\
& + \frac{7}{4}\delta^{pc}Y_d^{*as}Y_d^{br}(Y_d^\dagger Y_d)^{dt} + 3\delta^{sc}Y_d^{*ad}Y_d^{bt}(Y_d^\dagger Y_d)^{pr} + 3\delta^{td}Y_d^{*as}Y_d^{bc}(Y_d^\dagger Y_d)^{pr} + 3\delta^{pc}Y_d^{*ad}Y_d^{br}(Y_d^\dagger Y_d)^{st} + 3\delta^{rd}Y_d^{*ap}Y_d^{bc}(Y_d^\dagger Y_d)^{st} \\
& - \frac{1}{2}\delta^{sc}\delta^{td}(Y_d^\dagger Y_d)^{pr}(Y_d Y_d^\dagger)^{ba} - \frac{1}{2}\delta^{pc}\delta^{rd}(Y_d^\dagger Y_d)^{st}(Y_d Y_d^\dagger)^{ba} - g_L^2 \left( \frac{51}{8}\delta^{rd}\delta^{sc}Y_d^{*ap}Y_d^{bt} + \frac{51}{8}\delta^{pc}\delta^{td}Y_d^{*as}Y_d^{br} \right) - g_Y^4 \left( \frac{287}{4374}\delta^{pc}\delta^{rd}\delta^{st}\delta^{ab} \right.
\end{aligned}$$

$$\begin{aligned}
& + \frac{287}{4374} \delta^{pr} \delta^{sc} \delta^{td} \delta^{ab} \Big) - g_Y^2 g_L^2 \Big( \frac{1}{6} \delta^{pc} \delta^{rd} \delta^{st} \delta^{ab} + \frac{1}{6} \delta^{pr} \delta^{sc} \delta^{td} \delta^{ab} \Big) \Big\} C_{qd}^{(\times)abcd} + \frac{16}{81} \delta^{pr} \delta^{st} \delta^{ab} \delta^{cd} g_Y^4 C_{ee}^{abcd} + \left\{ \frac{64}{243} \delta^{pr} \delta^{st} \delta^{ad} \delta^{bc} g_Y^4 \right. \\
& + g_s^4 \left( \frac{4}{9} \delta^{pt} \delta^{rs} \delta^{ad} \delta^{bc} - \frac{4}{27} \delta^{pr} \delta^{st} \delta^{ad} \delta^{bc} \right) \Big\} C_{uu}^{abcd} + \left\{ g_Y^4 \left( \frac{16}{243} \delta^{pr} \delta^{st} \delta^{ad} \delta^{bc} + \frac{344}{2187} \delta^{pa} \delta^{rd} \delta^{st} \delta^{bc} + \frac{344}{2187} \delta^{pr} \delta^{sa} \delta^{td} \delta^{bc} + \frac{296}{729} \delta^{pa} \delta^{rb} \delta^{st} \delta^{cd} \right. \right. \\
& + \frac{296}{729} \delta^{pr} \delta^{sa} \delta^{tb} \delta^{cd} - \frac{1}{9} \delta^{pa} \delta^{rb} \delta^{sc} \delta^{td} \Big) + g_Y^2 g_s^2 \left( \frac{374}{243} \delta^{pa} \delta^{rb} \delta^{st} \delta^{cd} + \frac{374}{243} \delta^{pr} \delta^{sa} \delta^{tb} \delta^{cd} + \frac{460}{243} \delta^{pt} \delta^{rd} \delta^{sa} \delta^{bc} + \frac{460}{243} \delta^{pa} \delta^{rs} \delta^{td} \delta^{bc} \right. \\
& - \frac{8}{81} \delta^{pr} \delta^{st} \delta^{ad} \delta^{bc} - \frac{308}{729} \delta^{pa} \delta^{rd} \delta^{st} \delta^{bc} - \frac{308}{729} \delta^{pr} \delta^{sa} \delta^{td} \delta^{bc} - \frac{50}{81} \delta^{pt} \delta^{rb} \delta^{sa} \delta^{cd} - \frac{50}{81} \delta^{pa} \delta^{rs} \delta^{tb} \delta^{cd} - \frac{70}{9} \delta^{pa} \delta^{rb} \delta^{sc} \delta^{td} - \frac{26}{3} \delta^{pa} \delta^{rd} \delta^{sc} \delta^{tb} \Big) \\
& + g_s^4 \left( \frac{15}{2} \delta^{pa} \delta^{rd} \delta^{sc} \delta^{tb} + \frac{79}{9} \delta^{pa} \delta^{rb} \delta^{st} \delta^{cd} + \frac{79}{9} \delta^{pr} \delta^{sa} \delta^{tb} \delta^{cd} + \frac{1300}{81} \delta^{pt} \delta^{rd} \delta^{sa} \delta^{bc} + \frac{1300}{81} \delta^{pa} \delta^{rs} \delta^{td} \delta^{bc} - \frac{148}{243} \delta^{pa} \delta^{rd} \delta^{st} \delta^{bc} \right. \\
& - \frac{148}{243} \delta^{pr} \delta^{sa} \delta^{td} \delta^{bc} - \frac{7}{3} \delta^{pt} \delta^{rb} \delta^{sa} \delta^{cd} - \frac{7}{3} \delta^{pa} \delta^{rs} \delta^{tb} \delta^{cd} - \frac{71}{6} \delta^{pa} \delta^{rb} \delta^{sc} \delta^{td} \Big) + g_s^2 \left( \frac{10}{9} \delta^{pa} \delta^{rd} \delta^{st} (Y_d^\dagger Y_d)^{bc} + \frac{10}{9} \delta^{pr} \delta^{sa} \delta^{td} (Y_d^\dagger Y_d)^{bc} \right. \\
& - \frac{10}{3} \delta^{rd} \delta^{sa} \delta^{tb} (Y_d^\dagger Y_d)^{pc} - \frac{10}{3} \delta^{pa} \delta^{rb} \delta^{td} (Y_d^\dagger Y_d)^{sc} - \frac{10}{3} \delta^{pa} \delta^{sc} \delta^{td} (Y_d^\dagger Y_d)^{br} - \frac{10}{3} \delta^{pt} \delta^{rd} \delta^{sa} (Y_d^\dagger Y_d)^{bc} - \frac{10}{3} \delta^{pa} \delta^{rs} \delta^{td} (Y_d^\dagger Y_d)^{bc} - \frac{10}{3} \delta^{pa} \delta^{rb} \delta^{sc} (Y_d^\dagger Y_d)^{dt} \\
& - 6 \delta^{rb} \delta^{sa} \delta^{td} (Y_d^\dagger Y_d)^{pc} - 6 \delta^{pa} \delta^{rd} \delta^{tb} (Y_d^\dagger Y_d)^{sc} - 6 \delta^{pa} \delta^{rd} \delta^{sc} (Y_d^\dagger Y_d)^{bt} - 6 \delta^{pa} \delta^{sc} \delta^{tb} (Y_d^\dagger Y_d)^{dr} \Big) + g_L^2 \left( \frac{51}{8} \delta^{rd} \delta^{sa} \delta^{tb} (Y_d^\dagger Y_d)^{pc} + \frac{51}{8} \delta^{pa} \delta^{rb} \delta^{td} (Y_d^\dagger Y_d)^{sc} \right. \\
& + \frac{51}{8} \delta^{pa} \delta^{sc} \delta^{td} (Y_d^\dagger Y_d)^{br} + \frac{51}{8} \delta^{pa} \delta^{rb} \delta^{sc} (Y_d^\dagger Y_d)^{dt} \Big) + g_Y^2 \left( \frac{181}{72} \delta^{rd} \delta^{sa} \delta^{tb} (Y_d^\dagger Y_d)^{pc} + \frac{181}{72} \delta^{pa} \delta^{rb} \delta^{td} (Y_d^\dagger Y_d)^{sc} + \frac{181}{72} \delta^{pa} \delta^{sc} \delta^{td} (Y_d^\dagger Y_d)^{br} \right. \\
& + \frac{181}{72} \delta^{pa} \delta^{rb} \delta^{sc} (Y_d^\dagger Y_d)^{dt} - \frac{14}{27} \delta^{pa} \delta^{rd} \delta^{st} (Y_d^\dagger Y_d)^{bc} - \frac{14}{27} \delta^{pr} \delta^{sa} \delta^{td} (Y_d^\dagger Y_d)^{bc} - \frac{2}{3} \delta^{pa} \delta^{rb} \delta^{st} (Y_d^\dagger Y_d)^{dc} - \frac{2}{3} \delta^{pr} \delta^{sa} \delta^{tb} (Y_d^\dagger Y_d)^{dc} \Big) \\
& + 3 \delta^{sa} \delta^{td} (Y_d^\dagger Y_d)^{pr} (Y_d^\dagger Y_d)^{bc} + 3 \delta^{pa} \delta^{rd} (Y_d^\dagger Y_d)^{st} (Y_d^\dagger Y_d)^{bc} + 3 \delta^{sa} \delta^{tb} (Y_d^\dagger Y_d)^{pr} (Y_d^\dagger Y_d)^{dc} + 3 \delta^{pa} \delta^{rb} (Y_d^\dagger Y_d)^{st} (Y_d^\dagger Y_d)^{dc} + 4 \delta^{rb} \delta^{td} (Y_d^\dagger Y_d)^{pa} (Y_d^\dagger Y_d)^{sc} \\
& + 4 \delta^{pa} \delta^{sc} (Y_d^\dagger Y_d)^{br} (Y_d^\dagger Y_d)^{dt} - \frac{1}{4} \delta^{rd} \delta^{sa} \delta^{tb} (Y_d^\dagger Y_d Y_d^\dagger Y_d)^{pc} - \frac{1}{4} \delta^{pa} \delta^{rb} \delta^{td} (Y_d^\dagger Y_d Y_d^\dagger Y_d)^{sc} - \frac{1}{4} \delta^{pa} \delta^{sc} \delta^{td} (Y_d^\dagger Y_d Y_d^\dagger Y_d)^{br} - \frac{1}{4} \delta^{pa} \delta^{rb} \delta^{sc} (Y_d^\dagger Y_d Y_d^\dagger Y_d)^{dt} \\
& - \frac{1}{4} \delta^{rd} \delta^{sa} \delta^{tb} (Y_d^\dagger Y_u Y_u^\dagger Y_d)^{pc} - \frac{1}{4} \delta^{pa} \delta^{rb} \delta^{td} (Y_d^\dagger Y_u Y_u^\dagger Y_d)^{sc} - \frac{1}{4} \delta^{pa} \delta^{sc} \delta^{td} (Y_d^\dagger Y_u Y_u^\dagger Y_d)^{br} - \frac{1}{4} \delta^{pa} \delta^{rb} \delta^{sc} (Y_d^\dagger Y_u Y_u^\dagger Y_d)^{dt} - \frac{3}{2} T_2 \delta^{rd} \delta^{sa} \delta^{tb} (Y_d^\dagger Y_d)^{pc} \\
& - \frac{3}{2} T_2 \delta^{pa} \delta^{rb} \delta^{td} (Y_d^\dagger Y_d)^{sc} - \frac{3}{2} T_2 \delta^{pa} \delta^{sc} \delta^{td} (Y_d^\dagger Y_d)^{br} - \frac{3}{2} \delta^{pa} \delta^{td} (Y_d^\dagger Y_d)^{sc} (Y_d^\dagger Y_d)^{br} - \frac{3}{2} \delta^{rd} \delta^{sa} (Y_d^\dagger Y_d)^{pc} (Y_d^\dagger Y_d)^{bt} - \frac{3}{2} T_2 \delta^{pa} \delta^{rb} \delta^{sc} (Y_d^\dagger Y_d)^{dt} \\
& - \frac{5}{2} \delta^{sa} \delta^{tb} (Y_d^\dagger Y_d)^{pc} (Y_d^\dagger Y_d)^{dr} - \frac{5}{2} \delta^{pa} \delta^{rb} (Y_d^\dagger Y_d)^{sc} (Y_d^\dagger Y_d)^{dt} \Big\} C_{dd}^{abcd} + \left\{ \frac{1}{2} \delta^{sc} \delta^{td} (Y_d^\dagger Y_d)^{pr} (Y_e^\dagger Y_e)^{ba} + \frac{1}{2} \delta^{pc} \delta^{rd} (Y_d^\dagger Y_d)^{st} (Y_e^\dagger Y_e)^{ba} + g_Y^2 g_s^2 \left( \frac{25}{243} \delta^{pc} \delta^{rd} \delta^{st} \delta^{ab} \right. \right. \\
& + \frac{25}{243} \delta^{pr} \delta^{sc} \delta^{td} \delta^{ab} - \frac{25}{81} \delta^{pt} \delta^{rd} \delta^{sc} \delta^{ab} - \frac{25}{81} \delta^{pc} \delta^{rs} \delta^{td} \delta^{ab} \Big) + g_Y^4 \left( \frac{868}{729} \delta^{pc} \delta^{rd} \delta^{st} \delta^{ab} + \frac{868}{729} \delta^{pr} \delta^{sc} \delta^{td} \delta^{ab} \right) - g_Y^2 \left( \frac{5}{9} \delta^{pc} \delta^{rd} \delta^{st} (Y_e^\dagger Y_e)^{ba} \right. \\
& + \frac{5}{9} \delta^{pr} \delta^{sc} \delta^{td} (Y_e^\dagger Y_e)^{ba} \Big) \Big\} C_{ed}^{abcd} + \left\{ g_Y^2 g_s^2 \left( \frac{50}{81} \delta^{pt} \delta^{rd} \delta^{sc} \delta^{ab} + \frac{50}{81} \delta^{pc} \delta^{rs} \delta^{td} \delta^{ab} - \frac{482}{243} \delta^{pc} \delta^{rd} \delta^{st} \delta^{ab} - \frac{482}{243} \delta^{pr} \delta^{sc} \delta^{td} \delta^{ab} \right) + g_Y^4 \left( \frac{244}{729} \delta^{pc} \delta^{rd} \delta^{st} \delta^{ab} \right. \right. \\
& + \frac{244}{729} \delta^{pr} \delta^{sc} \delta^{td} \delta^{ab} \Big) + g_s^4 \left( \frac{73}{18} \delta^{pc} \delta^{rd} \delta^{st} \delta^{ab} + \frac{73}{18} \delta^{pr} \delta^{sc} \delta^{td} \delta^{ab} - \frac{1}{6} \delta^{pt} \delta^{rd} \delta^{sc} \delta^{ab} - \frac{1}{6} \delta^{pc} \delta^{rs} \delta^{td} \delta^{ab} \right) + g_Y^2 \left( \delta^{pc} \delta^{rd} \delta^{st} (Y_u^\dagger Y_u)^{ba} + \delta^{pr} \delta^{sc} \delta^{td} (Y_u^\dagger Y_u)^{ba} \right)
\end{aligned}$$

$$\begin{aligned}
& -\frac{1}{4}\delta^{sc}\delta^{td}(Y_d^\dagger Y_u)^{pa}(Y_u^\dagger Y_d)^{br} - \frac{1}{4}\delta^{pc}\delta^{rd}(Y_d^\dagger Y_u)^{sa}(Y_u^\dagger Y_d)^{bt} - \frac{3}{2}\delta^{sc}\delta^{td}(Y_d^\dagger Y_d)^{pr}(Y_u^\dagger Y_u)^{ba} - \frac{3}{2}\delta^{pc}\delta^{rd}(Y_d^\dagger Y_d)^{st}(Y_u^\dagger Y_u)^{ba} \Big\} C_{ud}^{(\parallel)abcd} + \left\{ g_Y^4 \left( \frac{244}{2187} \delta^{pc}\delta^{rd}\delta^{st}\delta^{ab} \right. \right. \\
& + \frac{244}{2187} \delta^{pr}\delta^{sc}\delta^{td}\delta^{ab} \Big) + g_s^4 \left( \frac{2}{27} \delta^{pr}\delta^{st}\delta^{ab}\delta^{cd} + \frac{386}{81} \delta^{pt}\delta^{rd}\delta^{sc}\delta^{ab} + \frac{386}{81} \delta^{pc}\delta^{rs}\delta^{td}\delta^{ab} - \frac{26}{243} \delta^{pc}\delta^{rd}\delta^{st}\delta^{ab} - \frac{26}{243} \delta^{pr}\delta^{sc}\delta^{td}\delta^{ab} \right. \\
& - \frac{2}{9} \delta^{pt}\delta^{rs}\delta^{ab}\delta^{cd} \Big) + g_Y^2 \left( \frac{1}{3} \delta^{pc}\delta^{rd}\delta^{st}(Y_u^\dagger Y_u)^{ba} + \frac{1}{3} \delta^{pr}\delta^{sc}\delta^{td}(Y_u^\dagger Y_u)^{ba} \right) + g_s^2 \left( \frac{1}{3} \delta^{pc}\delta^{rd}\delta^{st}(Y_u^\dagger Y_u)^{ba} + \frac{1}{3} \delta^{pr}\delta^{sc}\delta^{td}(Y_u^\dagger Y_u)^{ba} - \delta^{pt}\delta^{rd}\delta^{sc}(Y_u^\dagger Y_u)^{ba} \right. \\
& - \delta^{pc}\delta^{rs}\delta^{td}(Y_u^\dagger Y_u)^{ba} \Big) - \frac{1}{4} \delta^{pc}\delta^{td}(Y_d^\dagger Y_u)^{sa}(Y_u^\dagger Y_d)^{br} - \frac{1}{4} \delta^{rd}\delta^{sc}(Y_d^\dagger Y_u)^{pa}(Y_u^\dagger Y_d)^{bt} - \frac{1}{2} \delta^{sc}\delta^{td}(Y_d^\dagger Y_d)^{pr}(Y_u^\dagger Y_u)^{ba} - \frac{1}{2} \delta^{pc}\delta^{rd}(Y_d^\dagger Y_d)^{st}(Y_u^\dagger Y_u)^{ba} \\
& - g_Y^2 g_s^2 \left( \frac{4}{81} \delta^{pr}\delta^{st}\delta^{ab}\delta^{cd} + \frac{367}{729} \delta^{pc}\delta^{rd}\delta^{st}\delta^{ab} + \frac{367}{729} \delta^{pr}\delta^{sc}\delta^{td}\delta^{ab} + \frac{139}{243} \delta^{pt}\delta^{rd}\delta^{sc}\delta^{ab} + \frac{139}{243} \delta^{pc}\delta^{rs}\delta^{td}\delta^{ab} \right) \Big\} C_{ud}^{(\times)abcd} + \left\{ g_s^2 \left( \frac{2}{9} \delta^{pc}\delta^{rs}Y_e^{*ab}Y_d^{dt} \right. \right. \\
& + \frac{2}{9} \delta^{pt}\delta^{sc}Y_e^{*ab}Y_d^{dr} - \frac{2}{27} \delta^{pc}\delta^{st}Y_e^{*ab}Y_d^{dr} - \frac{2}{27} \delta^{pr}\delta^{sc}Y_e^{*ab}Y_d^{dt} \Big) - \frac{3}{4} \delta^{sc}Y_e^{*ab}Y_d^{dt}(Y_d^\dagger Y_d)^{pr} - \frac{3}{4} \delta^{pc}Y_e^{*ab}Y_d^{dr}(Y_d^\dagger Y_d)^{st} - g_Y^2 \left( \frac{5}{81} \delta^{pc}\delta^{st}Y_e^{*ab}Y_d^{dr} \right. \\
& + \frac{5}{81} \delta^{pr}\delta^{sc}Y_e^{*ab}Y_d^{dt} \Big) \Big\} C_{ledq}^{abcd} + C_{ledq}^{*abcd} \left\{ g_s^2 \left( \frac{2}{9} \delta^{pt}\delta^{rc}Y_d^{*ds}Y_e^{ab} + \frac{2}{9} \delta^{rs}\delta^{tc}Y_d^{*dp}Y_e^{ab} - \frac{2}{27} \delta^{rc}\delta^{st}Y_d^{*dp}Y_e^{ab} - \frac{2}{27} \delta^{pr}\delta^{tc}Y_d^{*ds}Y_e^{ab} \right) \right. \\
& - \frac{3}{4} \delta^{tc}Y_d^{*ds}Y_e^{ab}(Y_d^\dagger Y_d)^{pr} - \frac{3}{4} \delta^{rc}Y_d^{*dp}Y_e^{ab}(Y_d^\dagger Y_d)^{st} - g_Y^2 \left( \frac{5}{81} \delta^{rc}\delta^{st}Y_d^{*dp}Y_e^{ab} + \frac{5}{81} \delta^{pr}\delta^{tc}Y_d^{*ds}Y_e^{ab} \right) \Big\} + \left\{ \frac{7}{8} \delta^{td}Y_d^{*ap}Y_d^{*cs}(Y_u^\dagger Y_d)^{br} \right. \\
& + \frac{7}{8} \delta^{rd}Y_d^{*as}Y_d^{*cp}(Y_u^\dagger Y_d)^{bt} + g_s^2 \left( \frac{1}{9} \delta^{pt}\delta^{rd}Y_d^{*as}Y_u^{*cb} + \frac{1}{9} \delta^{rs}\delta^{td}Y_d^{*ap}Y_u^{*cb} + \frac{2}{3} \delta^{pt}\delta^{rd}Y_d^{*cs}Y_u^{*ab} + \frac{2}{3} \delta^{rs}\delta^{td}Y_d^{*cp}Y_u^{*ab} - \frac{1}{27} \delta^{rd}\delta^{st}Y_d^{*ap}Y_u^{*cb} \right. \\
& - \frac{1}{27} \delta^{pr}\delta^{td}Y_d^{*as}Y_u^{*cb} - \frac{2}{9} \delta^{rd}\delta^{st}Y_d^{*cp}Y_u^{*ab} - \frac{2}{9} \delta^{pr}\delta^{td}Y_d^{*cs}Y_u^{*ab} \Big) - \frac{3}{8} \delta^{td}Y_d^{*as}Y_u^{*cb}(Y_d^\dagger Y_d)^{pr} - \frac{3}{8} \delta^{rd}Y_d^{*ap}Y_u^{*cb}(Y_d^\dagger Y_d)^{st} - g_Y^2 \left( \frac{1}{324} \delta^{rd}\delta^{st}Y_d^{*ap}Y_u^{*cb} \right. \\
& + \frac{1}{324} \delta^{pr}\delta^{td}Y_d^{*as}Y_u^{*cb} + \frac{5}{27} \delta^{rd}\delta^{st}Y_d^{*cp}Y_u^{*ab} + \frac{5}{27} \delta^{pr}\delta^{td}Y_d^{*cs}Y_u^{*ab} \Big) - \frac{9}{4} \delta^{td}Y_d^{*cs}Y_u^{*ab}(Y_d^\dagger Y_d)^{pr} - \frac{9}{4} \delta^{rd}Y_d^{*cp}Y_u^{*ab}(Y_d^\dagger Y_d)^{st} \Big\} C_{quqd}^{(\parallel)abcd} \\
& + \left( C_{quqd}^{(\parallel)*} \right)^{abcd} \left\{ \frac{7}{8} \delta^{sd}Y_d^{ar}Y_d^{ct}(Y_d^\dagger Y_u)^{pb} + \frac{7}{8} \delta^{pd}Y_d^{at}Y_d^{cr}(Y_d^\dagger Y_u)^{sb} + g_s^2 \left( \frac{1}{9} \delta^{pd}\delta^{rs}Y_d^{at}Y_u^{cb} + \frac{1}{9} \delta^{pt}\delta^{sd}Y_d^{ar}Y_u^{cb} + \frac{2}{3} \delta^{pd}\delta^{rs}Y_d^{ct}Y_u^{ab} + \frac{2}{3} \delta^{pt}\delta^{sd}Y_d^{cr}Y_u^{ab} \right. \right. \\
& - \frac{1}{27} \delta^{pd}\delta^{st}Y_d^{ar}Y_u^{cb} - \frac{1}{27} \delta^{pr}\delta^{sd}Y_d^{at}Y_u^{cb} - \frac{2}{9} \delta^{pd}\delta^{st}Y_d^{cr}Y_u^{ab} - \frac{2}{9} \delta^{pr}\delta^{sd}Y_d^{ct}Y_u^{ab} \Big) - \frac{3}{8} \delta^{sd}Y_d^{at}Y_u^{cb}(Y_d^\dagger Y_d)^{pr} - \frac{3}{8} \delta^{pd}Y_d^{ar}Y_u^{cb}(Y_d^\dagger Y_d)^{st} - g_Y^2 \left( \frac{1}{324} \delta^{pd}\delta^{st}Y_d^{ar}Y_u^{cb} \right. \\
& + \frac{1}{324} \delta^{pr}\delta^{sd}Y_d^{at}Y_u^{cb} + \frac{5}{27} \delta^{pd}\delta^{st}Y_d^{cr}Y_u^{ab} + \frac{5}{27} \delta^{pr}\delta^{sd}Y_d^{ct}Y_u^{ab} \Big) - \frac{9}{4} \delta^{sd}Y_d^{ct}Y_u^{ab}(Y_d^\dagger Y_d)^{pr} - \frac{9}{4} \delta^{pd}Y_d^{cr}Y_u^{ab}(Y_d^\dagger Y_d)^{st} \Big\} + \left\{ \frac{7}{8} \delta^{td}Y_d^{*as}Y_d^{*cp}(Y_u^\dagger Y_d)^{br} \right. \\
& + \frac{7}{8} \delta^{rd}Y_d^{*ap}Y_d^{*cs}(Y_u^\dagger Y_d)^{bt} + g_s^2 \left( \frac{2}{9} \delta^{pt}\delta^{rd}Y_d^{*cs}Y_u^{*ab} + \frac{2}{9} \delta^{rs}\delta^{td}Y_d^{*cp}Y_u^{*ab} + \frac{1}{3} \delta^{pt}\delta^{rd}Y_d^{*as}Y_u^{*cb} + \frac{1}{3} \delta^{rs}\delta^{td}Y_d^{*ap}Y_u^{*cb} - \frac{2}{27} \delta^{rd}\delta^{st}Y_d^{*cp}Y_u^{*ab} \right. \\
& - \frac{2}{27} \delta^{pr}\delta^{td}Y_d^{*cs}Y_u^{*ab} - \frac{1}{9} \delta^{rd}\delta^{st}Y_d^{*ap}Y_u^{*cb} - \frac{1}{9} \delta^{pr}\delta^{td}Y_d^{*as}Y_u^{*cb} \Big) - \frac{3}{4} \delta^{td}Y_d^{*cs}Y_u^{*ab}(Y_d^\dagger Y_d)^{pr} - \frac{3}{4} \delta^{rd}Y_d^{*cp}Y_u^{*ab}(Y_d^\dagger Y_d)^{st} - g_Y^2 \left( \frac{1}{108} \delta^{rd}\delta^{st}Y_d^{*ap}Y_u^{*cb} \right.
\end{aligned}$$

$$\begin{aligned}
& + \frac{1}{108} \delta^{pr} \delta^{td} Y_d^{*as} Y_u^{*cb} + \frac{5}{81} \delta^{rd} \delta^{st} Y_d^{*cp} Y_u^{*ab} + \frac{5}{81} \delta^{pr} \delta^{td} Y_d^{*cs} Y_u^{*ab} \Big) - \frac{9}{8} \delta^{td} Y_d^{*as} Y_u^{*cb} (Y_d^\dagger Y_d)^{pr} - \frac{9}{8} \delta^{rd} Y_d^{*ap} Y_u^{*cb} (Y_d^\dagger Y_d)^{st} \Big\} C_{quqd}^{(\times)abcd} \\
& + \left( C_{quqd}^{(\times)*} \right)^{abcd} \left\{ \frac{7}{8} \delta^{sd} Y_d^{at} Y_d^{cr} (Y_d^\dagger Y_u)^{pb} + \frac{7}{8} \delta^{pd} Y_d^{ar} Y_d^{ct} (Y_d^\dagger Y_u)^{sb} + g_s^2 \left( \frac{2}{9} \delta^{pd} \delta^{rs} Y_d^{ct} Y_u^{ab} + \frac{2}{9} \delta^{pt} \delta^{sd} Y_d^{cr} Y_u^{ab} + \frac{1}{3} \delta^{pd} \delta^{rs} Y_d^{at} Y_u^{cb} + \frac{1}{3} \delta^{pt} \delta^{sd} Y_d^{ar} Y_u^{cb} \right. \right. \\
& - \frac{2}{27} \delta^{pd} \delta^{st} Y_d^{cr} Y_u^{ab} - \frac{2}{27} \delta^{pr} \delta^{sd} Y_d^{ct} Y_u^{ab} - \frac{1}{9} \delta^{pd} \delta^{st} Y_d^{ar} Y_u^{cb} - \frac{1}{9} \delta^{pr} \delta^{sd} Y_d^{at} Y_u^{cb} \Big) - \frac{3}{4} \delta^{sd} Y_d^{ct} Y_u^{ab} (Y_d^\dagger Y_d)^{pr} - \frac{3}{4} \delta^{pd} Y_d^{cr} Y_u^{ab} (Y_d^\dagger Y_d)^{st} - g_Y^2 \left( \frac{1}{108} \delta^{pd} \delta^{st} Y_d^{ar} Y_u^{cb} \right. \\
& + \frac{1}{108} \delta^{pr} \delta^{sd} Y_d^{at} Y_u^{cb} + \frac{5}{81} \delta^{pd} \delta^{st} Y_d^{cr} Y_u^{ab} + \frac{5}{81} \delta^{pr} \delta^{sd} Y_d^{ct} Y_u^{ab} \Big) - \frac{9}{8} \delta^{sd} Y_d^{at} Y_u^{cb} (Y_d^\dagger Y_d)^{pr} - \frac{9}{8} \delta^{pd} Y_d^{ar} Y_u^{cb} (Y_d^\dagger Y_d)^{st} \Big\} + \frac{8}{81} \delta^{pr} \delta^{st} \delta^{ad} \delta^{bc} g_Y^4 C_{\ell\ell}^{abcd} \\
& + \left\{ \frac{8}{243} \delta^{pr} \delta^{st} \delta^{ad} \delta^{bc} g_Y^4 + g_Y^2 \left( \frac{4}{27} \delta^{pr} \delta^{bc} Y_d^{*as} Y_d^{dt} + \frac{4}{27} \delta^{st} \delta^{bc} Y_d^{*ap} Y_d^{dr} \right) + g_s^2 \left( \frac{4}{9} \delta^{pr} \delta^{bc} Y_d^{*as} Y_d^{dt} + \frac{4}{9} \delta^{st} \delta^{bc} Y_d^{*ap} Y_d^{dr} - \frac{4}{3} \delta^{pt} \delta^{bc} Y_d^{*as} Y_d^{dr} \right. \right. \\
& - \frac{4}{3} \delta^{rs} \delta^{bc} Y_d^{*ap} Y_d^{dt} \Big) + g_s^4 \left( \frac{8}{9} \delta^{pt} \delta^{rs} \delta^{ad} \delta^{bc} - \frac{8}{27} \delta^{pr} \delta^{st} \delta^{ad} \delta^{bc} \right) + 2 Y_d^{*ap} Y_d^{*cs} Y_d^{br} Y_d^{dt} \Big\} C_{qq}^{(\parallel)abcd} + \left\{ \frac{16}{243} \delta^{pr} \delta^{st} \delta^{ad} \delta^{bc} g_Y^4 + g_Y^2 \left( \frac{8}{27} \delta^{pr} \delta^{bc} Y_d^{*as} Y_d^{dt} \right. \right. \\
& + \frac{8}{27} \delta^{st} \delta^{bc} Y_d^{*ap} Y_d^{dr} \Big) + g_s^2 \left( \frac{8}{9} \delta^{pr} \delta^{bc} Y_d^{*as} Y_d^{dt} + \frac{8}{9} \delta^{st} \delta^{bc} Y_d^{*ap} Y_d^{dr} - \frac{8}{3} \delta^{pt} \delta^{bc} Y_d^{*as} Y_d^{dr} - \frac{8}{3} \delta^{rs} \delta^{bc} Y_d^{*ap} Y_d^{dt} \right) + g_s^4 \left( \frac{16}{9} \delta^{pt} \delta^{rs} \delta^{ad} \delta^{bc} - \frac{16}{27} \delta^{pr} \delta^{st} \delta^{ad} \delta^{bc} \right) \\
& + 4 Y_d^{*ap} Y_d^{*cs} Y_d^{br} Y_d^{dt} \Big\} C_{qq}^{(\times)abcd}, \tag{11.6}
\end{aligned}$$

#### 11.4 $C_{eu}$

$$\begin{aligned}
\beta_{C_{eu}^{prst}}^{(1)} & = \left\{ \frac{4}{9} \delta^{pa} \delta^{rb} \delta^{st} g_Y^2 - 2 \delta^{pa} \delta^{rb} (Y_u^\dagger Y_u)^{st} \right\} C_{He}^{ab} + \left\{ 2 \delta^{sa} \delta^{tb} (Y_e^\dagger Y_e)^{pr} - \frac{2}{3} \delta^{pr} \delta^{sa} \delta^{tb} g_Y^2 \right\} C_{Hu}^{ab} - \frac{8}{9} \delta^{pc} \delta^{rd} \delta^{st} \delta^{ab} g_Y^2 C_{\ell e}^{abcd} + \left\{ \frac{4}{3} \delta^{pr} \delta^{sc} \delta^{td} \delta^{ab} g_Y^2 \right. \\
& - 2 \delta^{sc} \delta^{td} Y_e^{*ap} Y_e^{br} \Big\} C_{\ell u}^{abcd} + \left\{ \frac{8}{9} \delta^{pc} \delta^{rd} \delta^{st} \delta^{ab} g_Y^2 - 2 \delta^{pc} \delta^{rd} Y_u^{*as} Y_u^{bt} \right\} C_{qe}^{abcd} - \frac{4}{3} \delta^{pr} \delta^{sc} \delta^{td} \delta^{ab} g_Y^2 C_{qu}^{(\parallel)abcd} - \frac{4}{9} \delta^{pr} \delta^{sc} \delta^{td} \delta^{ab} g_Y^2 C_{qu}^{(\times)abcd} \\
& - \frac{32}{9} \delta^{pa} \delta^{rb} \delta^{st} \delta^{cd} g_Y^2 C_{ee}^{abcd} - \frac{16}{9} g_Y^2 \left\{ \delta^{pr} \delta^{sa} \delta^{td} \delta^{bc} + 3 \delta^{pr} \delta^{sa} \delta^{tb} \delta^{cd} \right\} C_{uu}^{abcd} + \left\{ \delta^{rb} \delta^{sc} \delta^{td} (Y_e^\dagger Y_e)^{pa} + \delta^{pa} \delta^{sc} \delta^{td} (Y_e^\dagger Y_e)^{br} + \delta^{pa} \delta^{rb} \delta^{td} (Y_u^\dagger Y_u)^{sc} \right. \\
& + \delta^{pa} \delta^{rb} \delta^{sc} (Y_u^\dagger Y_u)^{dt} - \frac{4}{9} g_Y^2 \left( 18 \delta^{pa} \delta^{rb} \delta^{sc} \delta^{td} - 3 \delta^{pr} \delta^{sc} \delta^{td} \delta^{ab} - 4 \delta^{pa} \delta^{rb} \delta^{st} \delta^{cd} \right) \Big\} C_{eu}^{abcd} - \frac{8}{9} \delta^{pa} \delta^{rb} \delta^{st} \delta^{cd} g_Y^2 C_{ed}^{abcd} + \frac{4}{3} \delta^{pr} \delta^{sa} \delta^{tb} \delta^{cd} g_Y^2 C_{ud}^{(\parallel)abcd} \\
& + \frac{4}{9} \delta^{pr} \delta^{sa} \delta^{tb} \delta^{cd} g_Y^2 C_{ud}^{(\times)abcd} + \delta^{rb} \delta^{td} Y_e^{*ap} Y_u^{*cs} C_{lequ}^{abcd} + \delta^{pb} \delta^{sd} C_{lequ}^{*abcd} Y_e^{ar} Y_u^{ct} + \delta^{rd} \delta^{tb} Y_e^{*ap} Y_u^{*cs} C_{luqe}^{abcd} + \delta^{pd} \delta^{sb} C_{luqe}^{*abcd} Y_e^{ar} Y_u^{ct}, \tag{11.7}
\end{aligned}$$

$$\begin{aligned}
\beta_{C_{eu}^{prst}}^{(2)} = & \left\{ g_Y^4 \left( \frac{20}{3} \delta^{st} (Y_e^\dagger Y_e)^{pr} + \frac{22}{3} \delta^{pr} (Y_u^\dagger Y_u)^{st} \right) - \frac{16}{9} \delta^{pr} \delta^{st} g_Y^6 \right\} C_{HB} + \left\{ g_Y^2 g_L^2 \left( \delta^{st} (Y_e^\dagger Y_e)^{pr} + \frac{3}{2} \delta^{pr} (Y_u^\dagger Y_u)^{st} \right) - \frac{4}{3} \delta^{pr} \delta^{st} g_Y^4 g_L^2 \right\} C_{HWB} \\
& - \frac{320}{9} \delta^{pr} \delta^{st} g_Y^2 g_s^6 C_G + \left\{ \frac{8}{3} \delta^{pr} \delta^{st} g_Y^4 Y_e^{*ab} - g_Y^2 \left( \frac{4}{3} \delta^{st} Y_e^{*ap} (Y_e^\dagger Y_e)^{br} + 2 \delta^{rb} Y_e^{*ap} (Y_u^\dagger Y_u)^{st} \right) \right\} C_{eB}^{ab} + C_{eB}^{*ab} \left\{ \frac{8}{3} \delta^{pr} \delta^{st} g_Y^4 Y_e^{ab} - g_Y^2 \left( \frac{4}{3} \delta^{st} Y_e^{ar} (Y_e^\dagger Y_e)^{pb} \right. \right. \\
& \left. \left. + 2 \delta^{pb} Y_e^{ar} (Y_u^\dagger Y_u)^{st} \right) \right\} + \frac{10}{3} \delta^{rb} \delta^{st} g_Y^2 g_L^2 Y_e^{*ap} C_{eW}^{ab} + \frac{10}{3} \delta^{pb} \delta^{st} g_Y^2 g_L^2 C_{eW}^{*ab} Y_e^{ar} + \left\{ g_Y^2 \left( 2 \delta^{pr} Y_u^{*as} (Y_u^\dagger Y_u)^{bt} + 8 \delta^{tb} Y_u^{*as} (Y_e^\dagger Y_e)^{pr} \right) \right. \\
& \left. + \frac{32}{3} \delta^{pr} \delta^{tb} g_Y^2 g_s^2 Y_u^{*as} - g_Y^4 \left( \frac{74}{27} \delta^{pr} \delta^{tb} Y_u^{*as} + \frac{40}{9} \delta^{pr} \delta^{st} Y_u^{*ab} \right) \right\} C_{uB}^{ab} + C_{uB}^{*ab} \left\{ g_Y^2 \left( 2 \delta^{pr} Y_u^{at} (Y_u^\dagger Y_u)^{sb} + 8 \delta^{sb} Y_u^{at} (Y_e^\dagger Y_e)^{pr} \right) + \frac{32}{3} \delta^{pr} \delta^{sb} g_Y^2 g_s^2 Y_u^{at} \right. \\
& \left. - g_Y^4 \left( \frac{74}{27} \delta^{pr} \delta^{sb} Y_u^{at} + \frac{40}{9} \delta^{pr} \delta^{st} Y_u^{ab} \right) \right\} + \frac{7}{3} \delta^{pr} \delta^{tb} g_Y^2 g_L^2 Y_u^{*as} C_{uW}^{ab} + \frac{7}{3} \delta^{pr} \delta^{sb} g_Y^2 g_L^2 C_{uW}^{*ab} Y_u^{at} + \left\{ \frac{104}{27} \delta^{pr} \delta^{tb} g_Y^2 g_s^2 Y_u^{*as} \right. \\
& \left. - 8 \delta^{tb} g_s^2 Y_u^{*as} (Y_e^\dagger Y_e)^{pr} \right\} C_{uG}^{ab} + C_{uG}^{*ab} \left\{ \frac{104}{27} \delta^{pr} \delta^{sb} g_Y^2 g_s^2 Y_u^{at} - 8 \delta^{sb} g_s^2 Y_u^{at} (Y_e^\dagger Y_e)^{pr} \right\} + \frac{8}{9} \delta^{pr} \delta^{st} g_Y^4 Y_d^{*ab} C_{dB}^{ab} + \frac{8}{9} \delta^{pr} \delta^{st} g_Y^4 C_{dB}^{*ab} Y_d^{ab} \\
& + \left\{ g_Y^4 \left( \frac{32}{81} \delta^{pa} \delta^{rb} \delta^{st} - \frac{4}{27} \delta^{pr} \delta^{st} \delta^{ab} \right) + g_Y^2 \left( \frac{4}{9} \delta^{st} \delta^{ab} (Y_e^\dagger Y_e)^{pr} + \frac{31}{27} \delta^{rb} \delta^{st} (Y_e^\dagger Y_e)^{pa} + \frac{31}{27} \delta^{pa} \delta^{st} (Y_e^\dagger Y_e)^{br} - \frac{4}{3} \delta^{pa} \delta^{rb} \delta^{st} \text{Tr} [Y_d^\dagger Y_d] \right. \right. \\
& \left. - \frac{4}{3} \delta^{pa} \delta^{rb} \delta^{st} \text{Tr} [Y_u^\dagger Y_u] - \frac{169}{36} \delta^{pa} \delta^{rb} (Y_u^\dagger Y_u)^{st} \right) + 2 T_2 \delta^{pa} \delta^{rb} (Y_u^\dagger Y_u)^{st} + 3 \delta^{pa} \delta^{rb} (Y_u^\dagger Y_u Y_u^\dagger Y_u)^{st} + 4 \delta^{pa} \delta^{rb} \delta^{st} g_Y^2 g_L^2 + \frac{32}{3} \delta^{pa} \delta^{rb} g_s^2 (Y_u^\dagger Y_u)^{st} \\
& \left. - \frac{1}{2} \delta^{rb} (Y_e^\dagger Y_e)^{pa} (Y_u^\dagger Y_u)^{st} - \frac{1}{2} \delta^{pa} (Y_e^\dagger Y_e)^{br} (Y_u^\dagger Y_u)^{st} - \frac{51}{4} \delta^{pa} \delta^{rb} g_L^2 (Y_u^\dagger Y_u)^{st} \right\} C_{He}^{ab} + \left\{ \frac{1}{2} \delta^{tb} (Y_e^\dagger Y_e)^{pr} (Y_u^\dagger Y_u)^{sa} + \frac{1}{2} \delta^{sa} (Y_e^\dagger Y_e)^{pr} (Y_u^\dagger Y_u)^{bt} \right. \\
& \left. + g_Y^2 \left( \frac{2}{3} T_2 \delta^{pr} \delta^{sa} \delta^{tb} + \frac{31}{12} \delta^{sa} \delta^{tb} (Y_e^\dagger Y_e)^{pr} - \frac{101}{54} \delta^{pr} \delta^{tb} (Y_u^\dagger Y_u)^{sa} - \frac{101}{54} \delta^{pr} \delta^{sa} (Y_u^\dagger Y_u)^{bt} \right) + \frac{51}{4} \delta^{sa} \delta^{tb} g_L^2 (Y_e^\dagger Y_e)^{pr} - 2 T_2 \delta^{sa} \delta^{tb} (Y_e^\dagger Y_e)^{pr} \right. \\
& \left. - \frac{658}{243} \delta^{pr} \delta^{sa} \delta^{tb} g_Y^4 - 3 \delta^{sa} \delta^{tb} (Y_e^\dagger Y_e Y_e^\dagger Y_e)^{pr} - 6 \delta^{pr} \delta^{sa} \delta^{tb} g_Y^2 g_L^2 \right\} C_{Hu}^{ab} + \left\{ \frac{3}{2} \delta^{sa} (Y_d^\dagger Y_u)^{bt} (Y_e^\dagger Y_e)^{pr} - \frac{55}{54} \delta^{pr} \delta^{sa} g_Y^2 (Y_d^\dagger Y_u)^{bt} \right\} C_{Hud}^{ab} \\
& + C_{Hud}^{*ab} \left\{ \frac{3}{2} \delta^{ta} (Y_e^\dagger Y_e)^{pr} (Y_u^\dagger Y_d)^{sb} - \frac{55}{54} \delta^{pr} \delta^{ta} g_Y^2 (Y_u^\dagger Y_d)^{sb} \right\} + \left\{ g_Y^4 \left( \frac{8}{27} \delta^{pr} \delta^{st} \delta^{ab} \delta^{cd} + \frac{470}{81} \delta^{pc} \delta^{rd} \delta^{st} \delta^{ab} \right) + \delta^{pc} \delta^{rd} (Y_u^\dagger Y_u)^{st} (Y_e Y_e^\dagger)^{ba} \right. \\
& \left. + g_Y^2 \left( \frac{20}{27} \delta^{pc} \delta^{st} Y_e^{*ad} Y_e^{br} + \frac{20}{27} \delta^{rd} \delta^{st} Y_e^{*ap} Y_e^{bc} + \frac{4}{3} \delta^{pc} \delta^{rd} \delta^{st} (Y_e Y_e^\dagger)^{ba} - \frac{4}{9} \delta^{st} \delta^{cd} Y_e^{*ap} Y_e^{br} \right) - 2 \delta^{pc} \delta^{rd} \delta^{st} \delta^{ab} g_Y^2 g_L^2 \right\} C_{\ell e}^{abcd} + \left\{ g_Y^2 \left( \frac{35}{4} \delta^{sc} \delta^{td} Y_e^{*ap} Y_e^{br} \right. \right. \\
& \left. - \frac{8}{3} \delta^{pr} \delta^{sc} \delta^{td} (Y_e Y_e^\dagger)^{ba} \right) + \frac{3}{2} \delta^{sc} \delta^{td} Y_e^{br} (Y_e^\dagger Y_e Y_e^\dagger)^{ap} + \frac{3}{2} \delta^{sc} \delta^{td} Y_e^{*ap} (Y_e Y_e^\dagger Y_e)^{br} + 3 T_2 \delta^{sc} \delta^{td} Y_e^{*ap} Y_e^{br} + 3 \delta^{pr} \delta^{sc} \delta^{td} \delta^{ab} g_Y^2 g_L^2 \\
& \left. - \frac{1}{2} \delta^{td} Y_e^{*ap} Y_e^{br} (Y_u^\dagger Y_u)^{sc} - \frac{1}{2} \delta^{sc} Y_e^{*ap} Y_e^{br} (Y_u^\dagger Y_u)^{dt} - \delta^{sc} \delta^{td} (Y_e^\dagger Y_e)^{pr} (Y_e Y_e^\dagger)^{ba} - \frac{787}{243} \delta^{pr} \delta^{sc} \delta^{td} \delta^{ab} g_Y^4 - \frac{51}{4} \delta^{sc} \delta^{td} g_L^2 Y_e^{*ap} Y_e^{br} \right\} C_{\ell u}^{abcd}
\end{aligned}$$



$$\begin{aligned}
& + \left\{ \frac{1}{2} \delta^{pc} \delta^{rd} Y_u^{bt} (Y_d^\dagger Y_d Y_u^\dagger)^{as} + \frac{1}{2} \delta^{pc} \delta^{rd} Y_u^{*as} (Y_d Y_d^\dagger Y_u)^{bt} + g_Y^2 \left( \frac{179}{36} \delta^{pc} \delta^{rd} Y_u^{*as} Y_u^{bt} - \frac{8}{3} \delta^{pc} \delta^{rd} \delta^{st} (Y_u Y_u^\dagger)^{ba} \right) + \frac{3}{2} \delta^{pc} \delta^{rd} Y_u^{bt} (Y_u^\dagger Y_u Y_u^\dagger)^{as} \right. \\
& + \frac{3}{2} \delta^{pc} \delta^{rd} Y_u^{*as} (Y_u Y_u^\dagger Y_u)^{bt} + 2 \delta^{pc} \delta^{rd} \delta^{st} \delta^{ab} g_Y^2 g_L^2 + 3 T_2 \delta^{pc} \delta^{rd} Y_u^{*as} Y_u^{bt} + 3 \delta^{pc} \delta^{rd} (Y_u^\dagger Y_u)^{st} (Y_d Y_d^\dagger)^{ba} + \frac{32}{9} \delta^{pc} \delta^{rd} \delta^{st} \delta^{ab} g_Y^2 g_s^2 \\
& + \frac{32}{3} \delta^{pc} \delta^{rd} g_s^2 Y_u^{*as} Y_u^{bt} - \frac{1}{2} \delta^{rd} Y_u^{*as} Y_u^{bt} (Y_e^\dagger Y_e)^{pc} - \frac{1}{2} \delta^{pc} Y_u^{*as} Y_u^{bt} (Y_e^\dagger Y_e)^{dr} - g_Y^4 \left( \frac{8}{27} \delta^{pr} \delta^{st} \delta^{ab} \delta^{cd} + \frac{278}{81} \delta^{pc} \delta^{rd} \delta^{st} \delta^{ab} \right) - 3 \delta^{pc} \delta^{rd} (Y_u^\dagger Y_u)^{st} (Y_u Y_u^\dagger)^{ba} \\
& \left. - \frac{51}{4} \delta^{pc} \delta^{rd} g_L^2 Y_u^{*as} Y_u^{bt} - 16 \delta^{pc} \delta^{rd} \delta^{st} \delta^{ab} g_s^4 \right\} C_{qe}^{abcd} + \left\{ g_Y^2 \left( 4 \delta^{pr} \delta^{sc} \delta^{td} (Y_u Y_u^\dagger)^{ba} - \frac{4}{27} \delta^{pr} \delta^{sc} Y_u^{*ad} Y_u^{bt} - \frac{4}{27} \delta^{pr} \delta^{td} Y_u^{*as} Y_u^{bc} \right) \right. \\
& + \frac{643}{243} \delta^{pr} \delta^{sc} \delta^{td} \delta^{ab} g_Y^4 + 3 \delta^{sc} \delta^{td} (Y_e^\dagger Y_e)^{pr} (Y_u Y_u^\dagger)^{ba} - 3 \delta^{pr} \delta^{sc} \delta^{td} \delta^{ab} g_Y^2 g_L^2 - 3 \delta^{sc} \delta^{td} (Y_e^\dagger Y_e)^{pr} (Y_d Y_d^\dagger)^{ba} - \frac{16}{3} \delta^{pr} \delta^{sc} \delta^{td} \delta^{ab} g_Y^2 g_s^2 \left. \right\} C_{qu}^{(||)abcd} \\
& + \left\{ \frac{643}{729} \delta^{pr} \delta^{sc} \delta^{td} \delta^{ab} g_Y^4 + g_Y^2 g_s^2 \left( \frac{16}{27} \delta^{pr} \delta^{st} \delta^{ab} \delta^{cd} + \frac{2896}{243} \delta^{pr} \delta^{sc} \delta^{td} \delta^{ab} \right) + \delta^{sc} \delta^{td} (Y_e^\dagger Y_e)^{pr} (Y_u Y_u^\dagger)^{ba} + g_Y^2 \left( \frac{4}{9} \delta^{pr} \delta^{sc} \delta^{td} (Y_u Y_u^\dagger)^{ba} \right. \right. \\
& + \frac{20}{9} \delta^{pr} \delta^{sc} Y_u^{*ad} Y_u^{bt} + \frac{20}{9} \delta^{pr} \delta^{td} Y_u^{*as} Y_u^{bc} - \frac{8}{9} \delta^{pr} \delta^{cd} Y_u^{*as} Y_u^{bt} \left. \right) - \delta^{pr} \delta^{sc} \delta^{td} \delta^{ab} g_Y^2 g_L^2 - \delta^{sc} \delta^{td} (Y_e^\dagger Y_e)^{pr} (Y_d Y_d^\dagger)^{ba} \left. \right\} C_{qu}^{(\times)abcd} + \left\{ g_Y^4 \left( \frac{3776}{81} \delta^{pa} \delta^{rb} \delta^{st} \delta^{cd} \right. \right. \\
& - \frac{32}{27} \delta^{pr} \delta^{st} \delta^{ab} \delta^{cd} \left. \right) + \frac{112}{9} \delta^{pa} \delta^{rb} \delta^{st} g_Y^2 (Y_e^\dagger Y_e)^{dc} - 8 \delta^{pa} \delta^{rb} (Y_e^\dagger Y_e)^{dc} (Y_u^\dagger Y_u)^{st} \left. \right\} C_{ee}^{abcd} + \left\{ g_Y^2 g_s^2 \left( \frac{16}{27} \delta^{pr} \delta^{st} \delta^{ad} \delta^{bc} - \frac{608}{243} \delta^{pr} \delta^{sa} \delta^{td} \delta^{bc} \right. \right. \\
& - 16 \delta^{pr} \delta^{sa} \delta^{tb} \delta^{cd} \left. \right) + g_Y^4 \left( \frac{17536}{729} \delta^{pr} \delta^{sa} \delta^{td} \delta^{bc} + \frac{9664}{243} \delta^{pr} \delta^{sa} \delta^{tb} \delta^{cd} - \frac{256}{81} \delta^{pr} \delta^{st} \delta^{ad} \delta^{bc} \right) + g_Y^2 \left( \frac{68}{9} \delta^{pr} \delta^{sa} \delta^{td} (Y_u^\dagger Y_u)^{bc} + 12 \delta^{pr} \delta^{sa} \delta^{tb} (Y_u^\dagger Y_u)^{dc} \right) \\
& - 6 \delta^{sa} \delta^{td} (Y_e^\dagger Y_e)^{pr} (Y_u^\dagger Y_u)^{bc} - 6 \delta^{sa} \delta^{tb} (Y_e^\dagger Y_e)^{pr} (Y_u^\dagger Y_u)^{dc} \left. \right\} C_{uu}^{abcd} - \frac{64}{81} \delta^{pr} \delta^{st} \delta^{ad} \delta^{bc} g_Y^4 C_{dd}^{abcd} + \left\{ g_Y^2 g_s^2 \left( \frac{64}{9} \delta^{pa} \delta^{rb} \delta^{st} \delta^{cd} + 32 \delta^{pa} \delta^{rb} \delta^{sc} \delta^{td} \right) \right. \\
& + g_Y^4 \left( \frac{176}{81} \delta^{pa} \delta^{rb} \delta^{st} \delta^{cd} + \frac{74}{9} \delta^{pa} \delta^{rb} \delta^{sc} \delta^{td} + \frac{3344}{243} \delta^{pr} \delta^{sc} \delta^{td} \delta^{ab} - \frac{16}{27} \delta^{pr} \delta^{st} \delta^{ab} \delta^{cd} \right) + \delta^{sc} \delta^{td} (Y_e^\dagger Y_e)^{pr} (Y_e^\dagger Y_e)^{ba} + g_L^2 \left( \frac{51}{8} \delta^{rb} \delta^{sc} \delta^{td} (Y_e^\dagger Y_e)^{pa} \right. \\
& + \frac{51}{8} \delta^{pa} \delta^{sc} \delta^{td} (Y_e^\dagger Y_e)^{br} + \frac{51}{8} \delta^{pa} \delta^{rb} \delta^{td} (Y_u^\dagger Y_u)^{sc} + \frac{51}{8} \delta^{pa} \delta^{rb} \delta^{sc} (Y_u^\dagger Y_u)^{dt} \left. \right) + g_Y^2 \left( \frac{21}{8} \delta^{rb} \delta^{sc} \delta^{td} (Y_e^\dagger Y_e)^{pa} + \frac{21}{8} \delta^{pa} \delta^{sc} \delta^{td} (Y_e^\dagger Y_e)^{br} \right. \\
& + \frac{193}{72} \delta^{pa} \delta^{rb} \delta^{td} (Y_u^\dagger Y_u)^{sc} + \frac{193}{72} \delta^{pa} \delta^{rb} \delta^{sc} (Y_u^\dagger Y_u)^{dt} - \frac{10}{3} \delta^{pr} \delta^{sc} \delta^{td} (Y_e^\dagger Y_e)^{ba} - 4 \delta^{pa} \delta^{rb} \delta^{st} (Y_u^\dagger Y_u)^{dc} \left. \right) + 3 \delta^{pa} \delta^{rb} (Y_u^\dagger Y_u)^{st} (Y_u^\dagger Y_u)^{dc} \\
& + 8 \delta^{pa} \delta^{rb} \delta^{st} \delta^{cd} g_s^4 - \frac{1}{4} \delta^{rb} \delta^{sc} \delta^{td} (Y_e^\dagger Y_e Y_e^\dagger Y_e)^{pa} - \frac{1}{4} \delta^{pa} \delta^{sc} \delta^{td} (Y_e^\dagger Y_e Y_e^\dagger Y_e)^{br} - \frac{1}{4} \delta^{pa} \delta^{rb} \delta^{td} (Y_u^\dagger Y_d Y_d^\dagger Y_u)^{sc} - \frac{1}{4} \delta^{pa} \delta^{rb} \delta^{sc} (Y_u^\dagger Y_d Y_d^\dagger Y_u)^{dt} \\
& - \frac{1}{4} \delta^{pa} \delta^{rb} \delta^{td} (Y_u^\dagger Y_u Y_u^\dagger Y_u)^{sc} - \frac{1}{4} \delta^{pa} \delta^{rb} \delta^{sc} (Y_u^\dagger Y_u Y_u^\dagger Y_u)^{dt} - g_s^2 \left( \frac{16}{3} \delta^{pa} \delta^{rb} \delta^{td} (Y_u^\dagger Y_u)^{sc} + \frac{16}{3} \delta^{pa} \delta^{rb} \delta^{sc} (Y_u^\dagger Y_u)^{dt} \right) - \frac{3}{2} T_2 \delta^{rb} \delta^{sc} \delta^{td} (Y_e^\dagger Y_e)^{pa} \\
& - \frac{3}{2} T_2 \delta^{pa} \delta^{sc} \delta^{td} (Y_e^\dagger Y_e)^{br} - \frac{3}{2} T_2 \delta^{pa} \delta^{rb} \delta^{td} (Y_u^\dagger Y_u)^{sc} - \frac{3}{2} T_2 \delta^{pa} \delta^{rb} \delta^{sc} (Y_u^\dagger Y_u)^{dt} - 2 \delta^{pa} \delta^{td} (Y_e^\dagger Y_e)^{br} (Y_u^\dagger Y_u)^{sc} - 2 \delta^{rb} \delta^{sc} (Y_e^\dagger Y_e)^{pa} (Y_u^\dagger Y_u)^{dt}
\end{aligned}$$

$$\begin{aligned}
& -\frac{5}{2}\delta^{sc}\delta^{td}(Y_e^\dagger Y_e)^{pa}(Y_e^\dagger Y_e)^{br}-\frac{5}{2}\delta^{pa}\delta^{rb}(Y_u^\dagger Y_u)^{sc}(Y_u^\dagger Y_u)^{dt}-\frac{7}{2}\delta^{rb}\delta^{td}(Y_e^\dagger Y_e)^{pa}(Y_u^\dagger Y_u)^{sc}-\frac{7}{2}\delta^{pa}\delta^{sc}(Y_e^\dagger Y_e)^{br}(Y_u^\dagger Y_u)^{dt}\Big\}C_{eu}^{abcd}+\Big\{g_Y^4\Big(\frac{8}{27}\delta^{pr}\delta^{st}\delta^{ab}\delta^{cd}\\
& +\frac{488}{81}\delta^{pa}\delta^{rb}\delta^{st}\delta^{cd}\Big)+\frac{4}{3}\delta^{pa}\delta^{rb}\delta^{st}g_Y^2(Y_d^\dagger Y_d)^{dc}+8\delta^{pa}\delta^{rb}\delta^{st}\delta^{cd}g_s^4-\frac{1}{2}\delta^{pa}\delta^{rb}(Y_d^\dagger Y_u)^{dt}(Y_u^\dagger Y_d)^{sc}-3\delta^{pa}\delta^{rb}(Y_d^\dagger Y_d)^{dc}(Y_u^\dagger Y_u)^{st}\\
& -\frac{32}{9}\delta^{pa}\delta^{rb}\delta^{st}\delta^{cd}g_Y^2g_s^2\Big\}C_{ed}^{abcd}+\Big\{\frac{392}{243}\delta^{pr}\delta^{sa}\delta^{tb}\delta^{cd}g_Y^4+3\delta^{sa}\delta^{tb}(Y_d^\dagger Y_d)^{dc}(Y_e^\dagger Y_e)^{pr}+\frac{16}{3}\delta^{pr}\delta^{sa}\delta^{tb}\delta^{cd}g_Y^2g_s^2-2\delta^{pr}\delta^{sa}\delta^{tb}g_Y^2(Y_d^\dagger Y_d)^{dc}\Big\}C_{ud}^{(\parallel)abcd}\\
& +\Big\{\frac{392}{729}\delta^{pr}\delta^{sa}\delta^{tb}\delta^{cd}g_Y^4+g_Y^2g_s^2\Big(\frac{8}{27}\delta^{pr}\delta^{st}\delta^{ab}\delta^{cd}+\frac{1160}{243}\delta^{pr}\delta^{sa}\delta^{tb}\delta^{cd}\Big)+\delta^{sa}\delta^{tb}(Y_d^\dagger Y_d)^{dc}(Y_e^\dagger Y_e)^{pr}-\frac{2}{3}\delta^{pr}\delta^{sa}\delta^{tb}g_Y^2(Y_d^\dagger Y_d)^{dc}\Big\}C_{ud}^{(\times)abcd}\\
& +\Big\{\frac{3}{2}\delta^{rb}Y_e^{*ap}Y_d^{dc}(Y_u^\dagger Y_u)^{st}-\frac{4}{9}\delta^{rb}\delta^{st}g_Y^2Y_e^{*ap}Y_d^{dc}-\frac{3}{4}\delta^{rb}Y_e^{*ap}Y_u^{dt}(Y_u^\dagger Y_d)^{sc}\Big\}C_{ledq}^{abcd}+C_{ledq}^{*abcd}\Big\{\frac{3}{2}\delta^{pb}Y_d^{*dc}Y_e^{ar}(Y_u^\dagger Y_u)^{st}-\frac{4}{9}\delta^{pb}\delta^{st}g_Y^2Y_d^{*dc}Y_e^{ar}\\
& -\frac{3}{4}\delta^{pb}Y_u^{*ds}Y_e^{ar}(Y_d^\dagger Y_u)^{ct}\Big\}+\Big\{\frac{1}{4}\delta^{tb}Y_d^{*ad}Y_u^{*cs}(Y_e^\dagger Y_e)^{pr}+g_Y^2\Big(\frac{2}{9}\delta^{pr}\delta^{tb}Y_d^{*cd}Y_u^{*as}-\frac{7}{54}\delta^{pr}\delta^{tb}Y_d^{*ad}Y_u^{*cs}\Big)+\frac{3}{2}\delta^{tb}Y_d^{*cd}Y_u^{*as}(Y_e^\dagger Y_e)^{pr}\Big\}C_{quqd}^{(\parallel)abcd}\\
& +\Big(C_{quqd}^{(\parallel)*}\Big)^{abcd}\Big\{\frac{1}{4}\delta^{sb}Y_d^{ad}Y_u^{ct}(Y_e^\dagger Y_e)^{pr}+g_Y^2\Big(\frac{2}{9}\delta^{pr}\delta^{sb}Y_d^{cd}Y_u^{at}-\frac{7}{54}\delta^{pr}\delta^{sb}Y_d^{ad}Y_u^{ct}\Big)+\frac{3}{2}\delta^{sb}Y_d^{cd}Y_u^{at}(Y_e^\dagger Y_e)^{pr}\Big\}+\Big\{\frac{1}{2}\delta^{tb}Y_d^{*cd}Y_u^{*as}(Y_e^\dagger Y_e)^{pr}\\
& +\frac{3}{4}\delta^{tb}Y_d^{*ad}Y_u^{*cs}(Y_e^\dagger Y_e)^{pr}+g_Y^2\Big(\frac{2}{27}\delta^{pr}\delta^{tb}Y_d^{*cd}Y_u^{*as}-\frac{7}{18}\delta^{pr}\delta^{tb}Y_d^{*ad}Y_u^{*cs}\Big)\Big\}C_{quqd}^{(\times)abcd}+\Big(C_{quqd}^{(\times)*}\Big)^{abcd}\Big\{\frac{1}{2}\delta^{sb}Y_d^{cd}Y_u^{at}(Y_e^\dagger Y_e)^{pr}+\frac{3}{4}\delta^{sb}Y_d^{ad}Y_u^{ct}(Y_e^\dagger Y_e)^{pr}\\
& +g_Y^2\Big(\frac{2}{27}\delta^{pr}\delta^{sb}Y_d^{cd}Y_u^{at}-\frac{7}{18}\delta^{pr}\delta^{sb}Y_d^{ad}Y_u^{ct}\Big)\Big\}+\Big\{g_Y^2\Big(\frac{4}{9}\delta^{rb}\delta^{st}Y_e^{*ap}Y_u^{*cd}+\frac{61}{72}\delta^{rb}\delta^{td}Y_e^{*ap}Y_u^{*cs}-\frac{2}{27}\delta^{pr}\delta^{td}Y_e^{*ab}Y_u^{*cs}\Big)+\frac{51}{8}\delta^{rb}\delta^{td}g_L^2Y_e^{*ap}Y_u^{*cs}\\
& -\frac{1}{4}\delta^{rb}\delta^{td}Y_u^{*cs}(Y_e^\dagger Y_e Y_e^\dagger)^{ap}-\frac{1}{4}\delta^{rb}\delta^{td}Y_e^{*ap}(Y_u^\dagger Y_u Y_u^\dagger)^{cs}-\frac{1}{2}T_2\delta^{rb}\delta^{td}Y_e^{*ap}Y_u^{*cs}-\frac{1}{2}\delta^{td}Y_e^{*ab}Y_u^{*cs}(Y_e^\dagger Y_e)^{pr}-\frac{3}{4}\delta^{rb}\delta^{td}Y_e^{*ap}(Y_d^\dagger Y_d Y_u^\dagger)^{cs}\\
& -\frac{5}{4}\delta^{td}Y_e^{*ap}Y_u^{*cs}(Y_e^\dagger Y_e)^{br}-\frac{5}{4}\delta^{rb}Y_e^{*ap}Y_u^{*cs}(Y_u^\dagger Y_u)^{dt}-\frac{3}{2}\delta^{rb}Y_e^{*ap}Y_u^{*cd}(Y_u^\dagger Y_u)^{st}-\frac{16}{3}\delta^{rb}\delta^{td}g_s^2Y_e^{*ap}Y_u^{*cs}\Big\}C_{lequ}^{abcd}+C_{lequ}^{*abcd}\Big\{g_Y^2\Big(\frac{4}{9}\delta^{pb}\delta^{st}Y_e^{ar}Y_u^{cd}\\
& +\frac{61}{72}\delta^{pb}\delta^{sd}Y_e^{ar}Y_u^{ct}-\frac{2}{27}\delta^{pr}\delta^{sd}Y_e^{ab}Y_u^{ct}\Big)+\frac{51}{8}\delta^{pb}\delta^{sd}g_L^2Y_e^{ar}Y_u^{ct}-\frac{1}{4}\delta^{pb}\delta^{sd}Y_u^{ct}(Y_e Y_e^\dagger Y_e)^{ar}-\frac{1}{4}\delta^{pb}\delta^{sd}Y_e^{ar}(Y_u Y_u^\dagger Y_u)^{ct}-\frac{1}{2}T_2\delta^{pb}\delta^{sd}Y_e^{ar}Y_u^{ct}\\
& -\frac{1}{2}\delta^{sd}Y_e^{ab}Y_u^{ct}(Y_e^\dagger Y_e)^{pr}-\frac{3}{4}\delta^{pb}\delta^{sd}Y_e^{ar}(Y_d Y_d^\dagger Y_u)^{ct}-\frac{5}{4}\delta^{sd}Y_e^{ar}Y_u^{ct}(Y_e^\dagger Y_e)^{pb}-\frac{5}{4}\delta^{pb}Y_e^{ar}Y_u^{ct}(Y_u^\dagger Y_u)^{sd}-\frac{3}{2}\delta^{pb}Y_e^{ar}Y_u^{cd}(Y_u^\dagger Y_u)^{st}-\frac{16}{3}\delta^{pb}\delta^{sd}g_s^2Y_e^{ar}Y_u^{ct}\Big\}\\
& +\Big\{\frac{1}{4}\delta^{tb}Y_e^{*ad}Y_u^{*cs}(Y_e^\dagger Y_e)^{pr}+\frac{1}{2}\delta^{tb}Y_e^{*ap}Y_u^{*cs}(Y_e^\dagger Y_e)^{dr}+\frac{1}{2}\delta^{rd}Y_e^{*ap}Y_u^{*cs}(Y_u^\dagger Y_u)^{bt}+\frac{3}{4}\delta^{rd}Y_e^{*ap}Y_u^{*cb}(Y_u^\dagger Y_u)^{st}+g_Y^2\Big(\frac{101}{72}\delta^{rd}\delta^{tb}Y_e^{*ap}Y_u^{*cs}\\
& -\frac{7}{54}\delta^{pr}\delta^{tb}Y_e^{*ad}Y_u^{*cs}-\frac{5}{9}\delta^{rd}\delta^{st}Y_e^{*ap}Y_u^{*cb}\Big)+\frac{51}{8}\delta^{rd}\delta^{tb}g_L^2Y_e^{*ap}Y_u^{*cs}-\frac{1}{4}\delta^{rd}\delta^{tb}Y_u^{*cs}(Y_e^\dagger Y_e Y_e^\dagger)^{ap}-\frac{1}{4}\delta^{rd}\delta^{tb}Y_e^{*ap}(Y_u^\dagger Y_u Y_u^\dagger)^{cs}
\end{aligned}$$

$$\begin{aligned}
& -\frac{1}{2}\text{T}_2\delta^{rd}\delta^{tb}Y_e^{*ap}Y_u^{*cs} - \frac{3}{4}\delta^{rd}\delta^{tb}Y_e^{*ap}(Y_d^\dagger Y_d Y_u^\dagger)^{cs} - \frac{14}{3}\delta^{rd}\delta^{tb}g_s^2Y_e^{*ap}Y_u^{*cs} \Big\} C_{\ell uqe}^{abcd} + C_{\ell uqe}^{*abcd} \Big\{ \frac{1}{4}\delta^{sb}Y_e^{ad}Y_u^{ct}(Y_e^\dagger Y_e)^{pr} + \frac{1}{2}\delta^{sb}Y_e^{ar}Y_u^{ct}(Y_e^\dagger Y_e)^{pd} \\
& + \frac{1}{2}\delta^{pd}Y_e^{ar}Y_u^{ct}(Y_u^\dagger Y_u)^{sb} + \frac{3}{4}\delta^{pd}Y_e^{ar}Y_u^{cb}(Y_u^\dagger Y_u)^{st} + g_Y^2 \Big( \frac{101}{72}\delta^{pd}\delta^{sb}Y_e^{ar}Y_u^{ct} - \frac{7}{54}\delta^{pr}\delta^{sb}Y_e^{ad}Y_u^{ct} - \frac{5}{9}\delta^{pd}\delta^{st}Y_e^{ar}Y_u^{cb} \Big) + \frac{51}{8}\delta^{pd}\delta^{sb}g_L^2Y_e^{ar}Y_u^{ct} \\
& - \frac{1}{4}\delta^{pd}\delta^{sb}Y_u^{ct}(Y_e Y_e^\dagger Y_e)^{ar} - \frac{1}{4}\delta^{pd}\delta^{sb}Y_e^{ar}(Y_u Y_u^\dagger Y_u)^{ct} - \frac{1}{2}\text{T}_2\delta^{pd}\delta^{sb}Y_e^{ar}Y_u^{ct} - \frac{3}{4}\delta^{pd}\delta^{sb}Y_e^{ar}(Y_d Y_d^\dagger Y_u)^{ct} - \frac{14}{3}\delta^{pd}\delta^{sb}g_s^2Y_e^{ar}Y_u^{ct} \Big\} \\
& + \Big\{ \frac{16}{9}\delta^{st}\delta^{bc}g_Y^2Y_e^{*ap}Y_e^{dr} - \frac{32}{27}\delta^{pr}\delta^{st}\delta^{ad}\delta^{bc}g_Y^4 \Big\} C_{\ell\ell}^{abcd} + \Big\{ \frac{8}{9}\delta^{pr}\delta^{bc}g_Y^2Y_u^{*as}Y_u^{dt} - \frac{32}{81}\delta^{pr}\delta^{st}\delta^{ad}\delta^{bc}g_Y^4 \Big\} C_{qq}^{(\parallel)abcd} + \Big\{ \frac{16}{9}\delta^{pr}\delta^{bc}g_Y^2Y_u^{*as}Y_u^{dt} \\
& - \frac{64}{81}\delta^{pr}\delta^{st}\delta^{ad}\delta^{bc}g_Y^4 \Big\} C_{qq}^{(\times)abcd} + Y_e^{*ap}Y_u^{*cs}C_{\ell q}^{(\parallel)abcd}Y_e^{br}Y_u^{dt} - Y_e^{*ap}Y_u^{*cs}C_{\ell q}^{(\times)abcd}Y_e^{br}Y_u^{dt}, \tag{11.8}
\end{aligned}$$

## 11.5 $C_{ed}$

$$\begin{aligned}
\beta_{C_{ed}^{prst}}^{(1)} & = \Big\{ 2\delta^{pa}\delta^{rb}(Y_d^\dagger Y_d)^{st} - \frac{2}{9}\delta^{pa}\delta^{rb}\delta^{st}g_Y^2 \Big\} C_{He}^{ab} + \Big\{ 2\delta^{sa}\delta^{tb}(Y_e^\dagger Y_e)^{pr} - \frac{2}{3}\delta^{pr}\delta^{sa}\delta^{tb}g_Y^2 \Big\} C_{Hd}^{ab} + \frac{4}{9}\delta^{pc}\delta^{rd}\delta^{st}\delta^{ab}g_Y^2C_{\ell e}^{abcd} + \Big\{ \frac{4}{3}\delta^{pr}\delta^{sc}\delta^{td}\delta^{ab}g_Y^2 \\
& - 2\delta^{sc}\delta^{td}Y_e^{*ap}Y_e^{br} \Big\} C_{\ell d}^{abcd} - \Big\{ \frac{4}{9}\delta^{pc}\delta^{rd}\delta^{st}\delta^{ab}g_Y^2 + 2\delta^{pc}\delta^{rd}Y_d^{*as}Y_d^{bt} \Big\} C_{qe}^{abcd} - \frac{4}{3}\delta^{pr}\delta^{sc}\delta^{td}\delta^{ab}g_Y^2C_{qd}^{(\parallel)abcd} - \frac{4}{9}\delta^{pr}\delta^{sc}\delta^{td}\delta^{ab}g_Y^2C_{qd}^{(\times)abcd} \\
& + \frac{16}{9}\delta^{pa}\delta^{rb}\delta^{st}\delta^{cd}g_Y^2C_{ee}^{abcd} + \frac{8}{9}g_Y^2 \Big\{ \delta^{pr}\delta^{sa}\delta^{td}\delta^{bc} + 3\delta^{pr}\delta^{sa}\delta^{tb}\delta^{cd} \Big\} C_{dd}^{abcd} - \frac{8}{9}\delta^{pa}\delta^{rb}\delta^{st}\delta^{cd}g_Y^2C_{eu}^{abcd} + \Big\{ \frac{4}{9}g_Y^2 \Big( \delta^{pa}\delta^{rb}\delta^{st}\delta^{cd} + 3\delta^{pr}\delta^{sc}\delta^{td}\delta^{ab} \\
& + 9\delta^{pa}\delta^{rb}\delta^{sc}\delta^{td} \Big) + \delta^{pa}\delta^{rb}\delta^{td}(Y_d^\dagger Y_d)^{sc} + \delta^{pa}\delta^{rb}\delta^{sc}(Y_d^\dagger Y_d)^{dt} + \delta^{rb}\delta^{sc}\delta^{td}(Y_e^\dagger Y_e)^{pa} + \delta^{pa}\delta^{sc}\delta^{td}(Y_e^\dagger Y_e)^{br} \Big\} C_{ed}^{abcd} - \frac{8}{3}\delta^{pr}\delta^{sc}\delta^{td}\delta^{ab}g_Y^2C_{ud}^{(\parallel)abcd} \\
& - \frac{8}{9}\delta^{pr}\delta^{sc}\delta^{td}\delta^{ab}g_Y^2C_{ud}^{(\times)abcd} + \delta^{rb}\delta^{sc}Y_e^{*ap}C_{\ell edq}^{abcd}Y_d^{dt} + \delta^{pb}\delta^{tc}C_{\ell edq}^{*abcd}Y_d^{ds}Y_e^{ar}, \tag{11.9}
\end{aligned}$$

$$\begin{aligned}
\beta_{C_{ed}^{prst}}^{(2)} & = \Big\{ \frac{8}{9}\delta^{pr}\delta^{st}g_Y^6 - g_Y^4 \Big( \frac{10}{3}\delta^{st}(Y_e^\dagger Y_e)^{pr} + \frac{14}{3}\delta^{pr}(Y_d^\dagger Y_d)^{st} \Big) \Big\} C_{HB} + \Big\{ \frac{2}{3}\delta^{pr}\delta^{st}g_Y^4g_L^2 - g_Y^2g_L^2 \Big( \frac{1}{2}\delta^{st}(Y_e^\dagger Y_e)^{pr} + \frac{3}{2}\delta^{pr}(Y_d^\dagger Y_d)^{st} \Big) \Big\} C_{HWB} \\
& + \frac{160}{9}\delta^{pr}\delta^{st}g_Y^2g_s^6C_G + \Big\{ g_Y^4 \Big( 4\delta^{rb}\delta^{st}Y_e^{*ap} - \frac{4}{3}\delta^{pr}\delta^{st}Y_e^{*ab} \Big) + g_Y^2 \Big( \frac{2}{3}\delta^{st}Y_e^{*ap}(Y_e^\dagger Y_e)^{br} - 7\delta^{rb}Y_e^{*ap}(Y_d^\dagger Y_d)^{st} \Big) \Big\} C_{eB}^{ab} + C_{eB}^{*ab} \Big\{ g_Y^4 \Big( 4\delta^{pb}\delta^{st}Y_e^{ar} \\
& - \frac{4}{3}\delta^{pr}\delta^{st}Y_e^{ab} \Big) + g_Y^2 \Big( \frac{2}{3}\delta^{st}Y_e^{ar}(Y_e^\dagger Y_e)^{pb} - 7\delta^{pb}Y_e^{ar}(Y_d^\dagger Y_d)^{st} \Big) \Big\} + \Big\{ \frac{9}{2}\delta^{rb}g_L^2Y_e^{*ap}(Y_d^\dagger Y_d)^{st} - \frac{5}{3}\delta^{rb}\delta^{st}g_Y^2g_L^2Y_e^{*ap} \Big\} C_{eW}^{ab} + C_{eW}^{*ab} \Big\{ \frac{9}{2}\delta^{pb}g_L^2Y_e^{ar}(Y_d^\dagger Y_d)^{st}
\end{aligned}$$

$$\begin{aligned}
& -\frac{5}{3}\delta^{pb}\delta^{st}g_Y^2g_L^2Y_e^{ar}\Big\} + \frac{20}{9}\delta^{pr}\delta^{st}g_Y^4Y_u^{*ab}C_{uB}^{ab} + \frac{20}{9}\delta^{pr}\delta^{st}g_Y^4C_{uB}^{*ab}Y_u^{ab} + \left\{g_Y^2\left(2\delta^{pr}Y_d^{*as}(Y_d^\dagger Y_d)^{bt} - 11\delta^{tb}Y_d^{*as}(Y_e^\dagger Y_e)^{pr}\right)\right. \\
& + \frac{32}{3}\delta^{pr}\delta^{tb}g_Y^2g_s^2Y_d^{*as} - g_Y^4\left(\frac{4}{9}\delta^{pr}\delta^{st}Y_d^{*ab} + \frac{128}{27}\delta^{pr}\delta^{tb}Y_d^{*as}\right)\Big\}C_{dB}^{ab} + C_{dB}^{*ab}\left\{g_Y^2\left(2\delta^{pr}Y_d^{at}(Y_d^\dagger Y_d)^{sb} - 11\delta^{sb}Y_d^{at}(Y_e^\dagger Y_e)^{pr}\right) + \frac{32}{3}\delta^{pr}\delta^{sb}g_Y^2g_s^2Y_d^{at}\right. \\
& - g_Y^4\left(\frac{4}{9}\delta^{pr}\delta^{st}Y_d^{ab} + \frac{128}{27}\delta^{pr}\delta^{sb}Y_d^{at}\right)\Big\} + \left\{\frac{1}{3}\delta^{pr}\delta^{tb}g_Y^2g_L^2Y_d^{*as} + \frac{9}{2}\delta^{tb}g_L^2Y_d^{*as}(Y_e^\dagger Y_e)^{pr}\right\}C_{dW}^{ab} + C_{dW}^{*ab}\left\{\frac{1}{3}\delta^{pr}\delta^{sb}g_Y^2g_L^2Y_d^{at} + \frac{9}{2}\delta^{sb}g_L^2Y_d^{at}(Y_e^\dagger Y_e)^{pr}\right\} \\
& + \left\{\frac{56}{27}\delta^{pr}\delta^{tb}g_Y^2g_s^2Y_d^{*as} + 8\delta^{tb}g_s^2Y_d^{*as}(Y_e^\dagger Y_e)^{pr}\right\}C_{dG}^{ab} + C_{dG}^{*ab}\left\{\frac{56}{27}\delta^{pr}\delta^{sb}g_Y^2g_s^2Y_d^{at} + 8\delta^{sb}g_s^2Y_d^{at}(Y_e^\dagger Y_e)^{pr}\right\} + \left\{\frac{1}{2}\delta^{rb}(Y_d^\dagger Y_d)^{st}(Y_e^\dagger Y_e)^{pa}\right. \\
& + \frac{1}{2}\delta^{pa}(Y_d^\dagger Y_d)^{st}(Y_e^\dagger Y_e)^{br} + g_Y^4\left(\frac{2}{27}\delta^{pr}\delta^{st}\delta^{ab} + \frac{74}{81}\delta^{pa}\delta^{rb}\delta^{st}\right) + g_Y^2\left(\frac{2}{3}\delta^{pa}\delta^{rb}\delta^{st}\text{Tr}[Y_d^\dagger Y_d] + \frac{2}{3}\delta^{pa}\delta^{rb}\delta^{st}\text{Tr}[Y_u^\dagger Y_u] + \frac{181}{36}\delta^{pa}\delta^{rb}(Y_d^\dagger Y_d)^{st}\right. \\
& - \frac{2}{9}\delta^{st}\delta^{ab}(Y_e^\dagger Y_e)^{pr} - \frac{31}{54}\delta^{rb}\delta^{st}(Y_e^\dagger Y_e)^{pa} - \frac{31}{54}\delta^{pa}\delta^{st}(Y_e^\dagger Y_e)^{br}\Big) + \frac{51}{4}\delta^{pa}\delta^{rb}g_L^2(Y_d^\dagger Y_d)^{st} - 2\delta^{pa}\delta^{rb}\delta^{st}g_Y^2g_L^2 - 2\text{T}_2\delta^{pa}\delta^{rb}(Y_d^\dagger Y_d)^{st} \\
& - 3\delta^{pa}\delta^{rb}(Y_d^\dagger Y_d Y_d^\dagger Y_d)^{st} - \frac{32}{3}\delta^{pa}\delta^{rb}g_s^2(Y_d^\dagger Y_d)^{st}\Big\}C_{He}^{ab} + \left\{\frac{1}{2}\delta^{tb}(Y_d^\dagger Y_d)^{sa}(Y_e^\dagger Y_e)^{pr} + \frac{1}{2}\delta^{sa}(Y_d^\dagger Y_d)^{bt}(Y_e^\dagger Y_e)^{pr} + g_Y^2\left(\frac{2}{3}\text{T}_2\delta^{pr}\delta^{sa}\delta^{tb}\right.\right. \\
& - \frac{73}{54}\delta^{pr}\delta^{tb}(Y_d^\dagger Y_d)^{sa} - \frac{73}{54}\delta^{pr}\delta^{sa}(Y_d^\dagger Y_d)^{bt} - \frac{65}{12}\delta^{sa}\delta^{tb}(Y_e^\dagger Y_e)^{pr}\Big) + \frac{51}{4}\delta^{sa}\delta^{tb}g_L^2(Y_e^\dagger Y_e)^{pr} - \frac{124}{243}\delta^{pr}\delta^{sa}\delta^{tb}g_Y^4 - 2\text{T}_2\delta^{sa}\delta^{tb}(Y_e^\dagger Y_e)^{pr} \\
& - 3\delta^{sa}\delta^{tb}(Y_e^\dagger Y_e Y_e^\dagger Y_e)^{pr} - 6\delta^{pr}\delta^{sa}\delta^{tb}g_Y^2g_L^2\Big\}C_{Hud}^{ab} + C_{Hud}^{*ab}\left\{\frac{59}{54}\delta^{pr}\delta^{tb}g_Y^2(Y_d^\dagger Y_u)^{sa} - \frac{3}{2}\delta^{tb}(Y_d^\dagger Y_u)^{sa}(Y_e^\dagger Y_e)^{pr}\right\} \\
& - \frac{3}{2}\delta^{sb}(Y_e^\dagger Y_e)^{pr}(Y_u^\dagger Y_d)^{at}\Big\} + \left\{\delta^{pc}\delta^{rd}\delta^{st}\delta^{ab}g_Y^2g_L^2 + g_Y^2\left(\frac{2}{9}\delta^{st}\delta^{cd}Y_e^{*ap}Y_e^{br} - \frac{10}{27}\delta^{pc}\delta^{st}Y_e^{*ad}Y_e^{br} - \frac{10}{27}\delta^{rd}\delta^{st}Y_e^{*ap}Y_e^{bc} - \frac{2}{3}\delta^{pc}\delta^{rd}\delta^{st}(Y_e Y_e^\dagger)^{ba}\right)\right. \\
& - g_Y^4\left(\frac{4}{27}\delta^{pr}\delta^{st}\delta^{ab}\delta^{cd} + \frac{361}{81}\delta^{pc}\delta^{rd}\delta^{st}\delta^{ab}\right) - \delta^{pc}\delta^{rd}(Y_d^\dagger Y_d)^{st}(Y_e Y_e^\dagger)^{ba}\Big\}C_{le}^{abcd} + \left\{\frac{3}{2}\delta^{sc}\delta^{td}Y_e^{br}(Y_e^\dagger Y_e Y_e^\dagger)^{ap} + \frac{3}{2}\delta^{sc}\delta^{td}Y_e^{*ap}(Y_e Y_e^\dagger Y_e)^{br}\right. \\
& + \frac{5}{2}\delta^{td}Y_e^{*ap}Y_e^{br}(Y_d^\dagger Y_d)^{sc} + \frac{5}{2}\delta^{sc}Y_e^{*ap}Y_e^{br}(Y_d^\dagger Y_d)^{dt} + 3\text{T}_2\delta^{sc}\delta^{td}Y_e^{*ap}Y_e^{br} + 3\delta^{pr}\delta^{sc}\delta^{td}\delta^{ab}g_Y^2g_L^2 - \delta^{sc}\delta^{td}(Y_e^\dagger Y_e)^{pr}(Y_e Y_e^\dagger)^{ba} - g_Y^2\left(\frac{1}{4}\delta^{sc}\delta^{td}Y_e^{*ap}Y_e^{br}\right. \\
& + \frac{8}{3}\delta^{pr}\delta^{sc}\delta^{td}(Y_e Y_e^\dagger)^{ba}\Big) - \frac{1837}{243}\delta^{pr}\delta^{sc}\delta^{td}\delta^{ab}g_Y^4 - \frac{51}{4}\delta^{sc}\delta^{td}g_L^2Y_e^{*ap}Y_e^{br}\Big\}C_{ld}^{abcd} + \left\{\frac{1}{2}\delta^{pc}\delta^{rd}Y_d^{bt}(Y_u^\dagger Y_u Y_d^\dagger)^{as} + \frac{1}{2}\delta^{pc}\delta^{rd}Y_d^{*as}(Y_u Y_u^\dagger Y_d)^{bt}\right. \\
& + g_Y^4\left(\frac{4}{27}\delta^{pr}\delta^{st}\delta^{ab}\delta^{cd} + \frac{49}{81}\delta^{pc}\delta^{rd}\delta^{st}\delta^{ab}\right) + g_Y^2\left(\frac{4}{3}\delta^{pc}\delta^{rd}\delta^{st}(Y_u Y_u^\dagger)^{ba} - \frac{265}{36}\delta^{pc}\delta^{rd}Y_d^{*as}Y_d^{bt}\right) + \frac{3}{2}\delta^{pc}\delta^{rd}Y_d^{bt}(Y_d^\dagger Y_d Y_d^\dagger)^{as} + \frac{3}{2}\delta^{pc}\delta^{rd}Y_d^{*as}(Y_d Y_d^\dagger Y_d)^{bt} \\
& + \frac{5}{2}\delta^{rd}Y_d^{*as}Y_d^{bt}(Y_e^\dagger Y_e)^{pc} + \frac{5}{2}\delta^{pc}Y_d^{*as}Y_d^{bt}(Y_e^\dagger Y_e)^{dr} + 3\text{T}_2\delta^{pc}\delta^{rd}Y_d^{*as}Y_d^{bt} + 3\delta^{pc}\delta^{rd}(Y_d^\dagger Y_d)^{st}(Y_u Y_u^\dagger)^{ba} + \frac{32}{3}\delta^{pc}\delta^{rd}g_s^2Y_d^{*as}Y_d^{bt}
\end{aligned}$$

$$\begin{aligned}
& -\delta^{pc}\delta^{rd}\delta^{st}\delta^{ab}g_Y^2g_L^2 - \frac{16}{9}\delta^{pc}\delta^{rd}\delta^{st}\delta^{ab}g_Y^2g_s^2 - 3\delta^{pc}\delta^{rd}(Y_d^\dagger Y_d)^{st}(Y_d Y_d^\dagger)^{ba} - \frac{51}{4}\delta^{pc}\delta^{rd}g_L^2Y_d^{*as}Y_d^{bt} - 16\delta^{pc}\delta^{rd}\delta^{st}\delta^{ab}g_s^4 \Big\} C_{qe}^{abcd} \\
& + \left\{ g_Y^2 \left( \frac{20}{27}\delta^{pr}\delta^{sc}Y_d^{*ad}Y_d^{bt} + \frac{20}{27}\delta^{pr}\delta^{td}Y_d^{*as}Y_d^{bc} + 4\delta^{pr}\delta^{sc}\delta^{td}(Y_u Y_u^\dagger)^{ba} \right) + 3\delta^{sc}\delta^{td}(Y_e^\dagger Y_e)^{pr}(Y_u Y_u^\dagger)^{ba} - \frac{683}{243}\delta^{pr}\delta^{sc}\delta^{td}\delta^{ab}g_Y^4 - 3\delta^{pr}\delta^{sc}\delta^{td}\delta^{ab}g_Y^2g_L^2 \right. \\
& - 3\delta^{sc}\delta^{td}(Y_e^\dagger Y_e)^{pr}(Y_d Y_d^\dagger)^{ba} - \frac{16}{3}\delta^{pr}\delta^{sc}\delta^{td}\delta^{ab}g_Y^2g_s^2 \Big\} C_{qd}^{(\parallel)abcd} + \left\{ g_Y^2g_s^2 \left( \frac{280}{243}\delta^{pr}\delta^{sc}\delta^{td}\delta^{ab} - \frac{8}{27}\delta^{pr}\delta^{st}\delta^{ab}\delta^{cd} \right) + \delta^{sc}\delta^{td}(Y_e^\dagger Y_e)^{pr}(Y_u Y_u^\dagger)^{ba} \right. \\
& + g_Y^2 \left( \frac{4}{9}\delta^{pr}\delta^{cd}Y_d^{*as}Y_d^{bt} + \frac{4}{9}\delta^{pr}\delta^{sc}\delta^{td}(Y_d Y_d^\dagger)^{ba} + \frac{8}{9}\delta^{pr}\delta^{sc}Y_d^{*ad}Y_d^{bt} + \frac{8}{9}\delta^{pr}\delta^{td}Y_d^{*as}Y_d^{bc} + \frac{4}{3}\delta^{pr}\delta^{sc}\delta^{td}(Y_u Y_u^\dagger)^{ba} \right) - \frac{683}{729}\delta^{pr}\delta^{sc}\delta^{td}\delta^{ab}g_Y^4 \\
& - \delta^{pr}\delta^{sc}\delta^{td}\delta^{ab}g_Y^2g_L^2 - \delta^{sc}\delta^{td}(Y_e^\dagger Y_e)^{pr}(Y_d Y_d^\dagger)^{ba} \Big\} C_{qd}^{(\times)abcd} + \left\{ g_Y^4 \left( \frac{16}{27}\delta^{pr}\delta^{st}\delta^{ab}\delta^{cd} - \frac{16}{81}\delta^{pa}\delta^{rb}\delta^{st}\delta^{cd} \right) + 8\delta^{pa}\delta^{rb}(Y_d^\dagger Y_d)^{st}(Y_e^\dagger Y_e)^{dc} \right. \\
& - \frac{56}{9}\delta^{pa}\delta^{rb}\delta^{st}g_Y^2(Y_e^\dagger Y_e)^{dc} \Big\} C_{ee}^{abcd} + \frac{128}{81}\delta^{pr}\delta^{st}\delta^{ad}\delta^{bc}g_Y^4C_{uu}^{abcd} + \left\{ g_Y^2g_s^2 \left( \frac{304}{243}\delta^{pr}\delta^{sa}\delta^{td}\delta^{bc} + 8\delta^{pr}\delta^{sa}\delta^{tb}\delta^{cd} - \frac{8}{27}\delta^{pr}\delta^{st}\delta^{ad}\delta^{bc} \right) \right. \\
& + g_Y^4 \left( \frac{32}{81}\delta^{pr}\delta^{st}\delta^{ad}\delta^{bc} + \frac{2992}{729}\delta^{pr}\delta^{sa}\delta^{td}\delta^{bc} + \frac{2032}{243}\delta^{pr}\delta^{sa}\delta^{tb}\delta^{cd} \right) + 6\delta^{sa}\delta^{td}(Y_d^\dagger Y_d)^{bc}(Y_e^\dagger Y_e)^{pr} + 6\delta^{sa}\delta^{tb}(Y_d^\dagger Y_d)^{dc}(Y_e^\dagger Y_e)^{pr} \\
& - g_Y^2 \left( \frac{28}{9}\delta^{pr}\delta^{sa}\delta^{td}(Y_d^\dagger Y_d)^{bc} + 4\delta^{pr}\delta^{sa}\delta^{tb}(Y_d^\dagger Y_d)^{dc} \right) \Big\} C_{dd}^{abcd} + \left\{ g_Y^4 \left( \frac{8}{27}\delta^{pr}\delta^{st}\delta^{ab}\delta^{cd} + \frac{272}{81}\delta^{pa}\delta^{rb}\delta^{st}\delta^{cd} \right) + 2\delta^{pa}\delta^{rb}\delta^{st}g_Y^2(Y_u^\dagger Y_u)^{dc} \right. \\
& + 8\delta^{pa}\delta^{rb}\delta^{st}\delta^{cd}g_s^4 - \frac{1}{2}\delta^{pa}\delta^{rb}(Y_d^\dagger Y_u)^{sc}(Y_u^\dagger Y_d)^{dt} - 3\delta^{pa}\delta^{rb}(Y_d^\dagger Y_d)^{st}(Y_u^\dagger Y_u)^{dc} - \frac{32}{9}\delta^{pa}\delta^{rb}\delta^{st}\delta^{cd}g_Y^2g_s^2 \Big\} C_{eu}^{abcd} + \left\{ g_Y^2g_s^2 \left( \frac{16}{9}\delta^{pa}\delta^{rb}\delta^{st}\delta^{cd} \right. \right. \\
& - 16\delta^{pa}\delta^{rb}\delta^{sc}\delta^{td} \Big) + g_Y^4 \left( \frac{3752}{243}\delta^{pr}\delta^{sc}\delta^{td}\delta^{ab} - \frac{4}{27}\delta^{pr}\delta^{st}\delta^{ab}\delta^{cd} - \frac{100}{81}\delta^{pa}\delta^{rb}\delta^{st}\delta^{cd} - \frac{127}{9}\delta^{pa}\delta^{rb}\delta^{sc}\delta^{td} \right) + g_L^2 \left( \frac{51}{8}\delta^{pa}\delta^{rb}\delta^{td}(Y_d^\dagger Y_d)^{sc} \right. \\
& + \frac{51}{8}\delta^{pa}\delta^{rb}\delta^{sc}(Y_d^\dagger Y_d)^{dt} + \frac{51}{8}\delta^{rb}\delta^{sc}\delta^{td}(Y_e^\dagger Y_e)^{pa} + \frac{51}{8}\delta^{pa}\delta^{sc}\delta^{td}(Y_e^\dagger Y_e)^{br} \Big) + \delta^{sc}\delta^{td}(Y_e^\dagger Y_e)^{pr}(Y_e^\dagger Y_e)^{ba} + g_Y^2 \left( \frac{277}{72}\delta^{pa}\delta^{rb}\delta^{td}(Y_d^\dagger Y_d)^{sc} \right. \\
& + \frac{277}{72}\delta^{pa}\delta^{rb}\delta^{sc}(Y_d^\dagger Y_d)^{dt} - \frac{2}{3}\delta^{pa}\delta^{rb}\delta^{st}(Y_d^\dagger Y_d)^{dc} - \frac{10}{3}\delta^{pr}\delta^{sc}\delta^{td}(Y_e^\dagger Y_e)^{ba} - \frac{27}{8}\delta^{rb}\delta^{sc}\delta^{td}(Y_e^\dagger Y_e)^{pa} - \frac{27}{8}\delta^{pa}\delta^{sc}\delta^{td}(Y_e^\dagger Y_e)^{br} \Big) \\
& + 3\delta^{pa}\delta^{rb}(Y_d^\dagger Y_d)^{st}(Y_d^\dagger Y_d)^{dc} + 4\delta^{rb}\delta^{td}(Y_d^\dagger Y_d)^{sc}(Y_e^\dagger Y_e)^{pa} + 4\delta^{pa}\delta^{sc}(Y_d^\dagger Y_d)^{dt}(Y_e^\dagger Y_e)^{br} + 8\delta^{pa}\delta^{rb}\delta^{st}\delta^{cd}g_s^4 - \frac{1}{4}\delta^{pa}\delta^{rb}\delta^{td}(Y_d^\dagger Y_d Y_d^\dagger Y_d)^{sc} \\
& - \frac{1}{4}\delta^{pa}\delta^{rb}\delta^{sc}(Y_d^\dagger Y_d Y_d^\dagger Y_d)^{dt} - \frac{1}{4}\delta^{pa}\delta^{rb}\delta^{td}(Y_d^\dagger Y_u Y_u^\dagger Y_d)^{sc} - \frac{1}{4}\delta^{pa}\delta^{rb}\delta^{sc}(Y_d^\dagger Y_u Y_u^\dagger Y_d)^{dt} - \frac{1}{4}\delta^{rb}\delta^{sc}\delta^{td}(Y_e^\dagger Y_e Y_e^\dagger Y_e)^{pa} - \frac{1}{4}\delta^{pa}\delta^{sc}\delta^{td}(Y_e^\dagger Y_e Y_e^\dagger Y_e)^{br} \\
& - \frac{1}{2}\delta^{rb}\delta^{sc}(Y_d^\dagger Y_d)^{dt}(Y_e^\dagger Y_e)^{pa} - \frac{1}{2}\delta^{pa}\delta^{td}(Y_d^\dagger Y_d)^{sc}(Y_e^\dagger Y_e)^{br} - g_s^2 \left( \frac{16}{3}\delta^{pa}\delta^{rb}\delta^{td}(Y_d^\dagger Y_d)^{sc} + \frac{16}{3}\delta^{pa}\delta^{rb}\delta^{sc}(Y_d^\dagger Y_d)^{dt} \right) - \frac{3}{2}T_2\delta^{pa}\delta^{rb}\delta^{td}(Y_d^\dagger Y_d)^{sc} \\
& - \frac{3}{2}T_2\delta^{pa}\delta^{rb}\delta^{sc}(Y_d^\dagger Y_d)^{dt} - \frac{3}{2}T_2\delta^{rb}\delta^{sc}\delta^{td}(Y_e^\dagger Y_e)^{pa} - \frac{3}{2}T_2\delta^{pa}\delta^{sc}\delta^{td}(Y_e^\dagger Y_e)^{br} - \frac{5}{2}\delta^{pa}\delta^{rb}(Y_d^\dagger Y_d)^{sc}(Y_d^\dagger Y_d)^{dt} - \frac{5}{2}\delta^{sc}\delta^{td}(Y_e^\dagger Y_e)^{pa}(Y_e^\dagger Y_e)^{br} \Big\} C_{ed}^{abcd}
\end{aligned}$$

$$\begin{aligned}
& + \left\{ 6\delta^{pr}\delta^{sc}\delta^{td}g_Y^2(Y_u^\dagger Y_u)^{ba} + \frac{2936}{243}\delta^{pr}\delta^{sc}\delta^{td}\delta^{ab}g_Y^4 - 3\delta^{sc}\delta^{td}(Y_e^\dagger Y_e)^{pr}(Y_u^\dagger Y_u)^{ba} - \frac{32}{3}\delta^{pr}\delta^{sc}\delta^{td}\delta^{ab}g_Y^2g_s^2 \right\} C_{ud}^{(\parallel)abcd} + \left\{ 2\delta^{pr}\delta^{sc}\delta^{td}g_Y^2(Y_u^\dagger Y_u)^{ba} \right. \\
& + \frac{2936}{729}\delta^{pr}\delta^{sc}\delta^{td}\delta^{ab}g_Y^4 - g_Y^2g_s^2\left(\frac{4}{27}\delta^{pr}\delta^{st}\delta^{ab}\delta^{cd} + \frac{1012}{243}\delta^{pr}\delta^{sc}\delta^{td}\delta^{ab}\right) - \delta^{sc}\delta^{td}(Y_e^\dagger Y_e)^{pr}(Y_u^\dagger Y_u)^{ba} \left. \right\} C_{ud}^{(\times)abcd} + \left\{ g_Y^2\left(\frac{2}{9}\delta^{rb}\delta^{st}Y_e^{*ap}Y_d^{dc} \right. \right. \\
& - \frac{10}{27}\delta^{pr}\delta^{sc}Y_e^{*ab}Y_d^{dt} - \frac{125}{72}\delta^{rb}\delta^{sc}Y_e^{*ap}Y_d^{dt} \left. \right) + \frac{33}{8}\delta^{rb}\delta^{sc}g_L^2Y_e^{*ap}Y_d^{dt} - \frac{1}{4}\delta^{rb}\delta^{sc}Y_d^{dt}(Y_e^\dagger Y_e Y_e^\dagger)^{ap} - \frac{1}{4}\delta^{rb}\delta^{sc}Y_e^{*ap}(Y_d Y_d^\dagger Y_d)^{dt} - \frac{1}{2}T_2\delta^{rb}\delta^{sc}Y_e^{*ap}Y_d^{dt} \\
& - \frac{1}{2}\delta^{sc}Y_e^{*ab}Y_d^{dt}(Y_e^\dagger Y_e)^{pr} - \frac{3}{4}\delta^{rb}\delta^{sc}Y_e^{*ap}(Y_u Y_u^\dagger Y_d)^{dt} - \frac{5}{4}\delta^{rb}Y_e^{*ap}Y_d^{dt}(Y_d^\dagger Y_d)^{sc} - \frac{5}{4}\delta^{sc}Y_e^{*ap}Y_d^{dt}(Y_e^\dagger Y_e)^{br} - \frac{3}{2}\delta^{rb}Y_e^{*ap}Y_d^{dc}(Y_d^\dagger Y_d)^{st} \\
& - \frac{16}{3}\delta^{rb}\delta^{sc}g_s^2Y_e^{*ap}Y_d^{dt} \left. \right\} C_{ledq}^{abcd} + C_{ledq}^{*abcd} \left\{ g_Y^2\left(\frac{2}{9}\delta^{pb}\delta^{st}Y_d^{*dc}Y_e^{ar} - \frac{10}{27}\delta^{pr}\delta^{tc}Y_d^{*ds}Y_e^{ab} - \frac{125}{72}\delta^{pb}\delta^{tc}Y_d^{*ds}Y_e^{ar} \right) + \frac{33}{8}\delta^{pb}\delta^{tc}g_L^2Y_d^{*ds}Y_e^{ar} \right. \\
& - \frac{1}{4}\delta^{pb}\delta^{tc}Y_e^{ar}(Y_d^\dagger Y_d Y_d^\dagger)^{ds} - \frac{1}{4}\delta^{pb}\delta^{tc}Y_d^{*ds}(Y_e Y_e^\dagger Y_e)^{ar} - \frac{1}{2}T_2\delta^{pb}\delta^{tc}Y_d^{*ds}Y_e^{ar} - \frac{1}{2}\delta^{tc}Y_d^{*ds}Y_e^{ab}(Y_e^\dagger Y_e)^{pr} - \frac{3}{4}\delta^{pb}\delta^{tc}Y_e^{ar}(Y_u^\dagger Y_u Y_d^\dagger)^{ds} \\
& - \frac{5}{4}\delta^{pb}Y_d^{*ds}Y_e^{ar}(Y_d^\dagger Y_d)^{ct} - \frac{5}{4}\delta^{tc}Y_d^{*ds}Y_e^{ar}(Y_e^\dagger Y_e)^{pb} - \frac{3}{2}\delta^{pb}Y_d^{*dc}Y_e^{ar}(Y_d^\dagger Y_d)^{st} - \frac{16}{3}\delta^{pb}\delta^{tc}g_s^2Y_d^{*ds}Y_e^{ar} \left. \right\} + \left\{ -\frac{1}{4}\delta^{td}Y_d^{*as}Y_u^{*cb}(Y_e^\dagger Y_e)^{pr} \right. \\
& - g_Y^2\left(\frac{1}{54}\delta^{pr}\delta^{td}Y_d^{*as}Y_u^{*cb} + \frac{10}{9}\delta^{pr}\delta^{td}Y_d^{*cs}Y_u^{*ab}\right) - \frac{3}{2}\delta^{td}Y_d^{*cs}Y_u^{*ab}(Y_e^\dagger Y_e)^{pr} \left. \right\} C_{quqd}^{(\parallel)abcd} + \left( C_{quqd}^{(\parallel)*} \right)^{abcd} \left\{ -\frac{1}{4}\delta^{sd}Y_d^{at}Y_u^{cb}(Y_e^\dagger Y_e)^{pr} - g_Y^2\left(\frac{1}{54}\delta^{pr}\delta^{sd}Y_d^{at}Y_u^{cb} \right. \right. \\
& + \frac{10}{9}\delta^{pr}\delta^{sd}Y_d^{ct}Y_u^{ab} \left. \right) - \frac{3}{2}\delta^{sd}Y_d^{ct}Y_u^{ab}(Y_e^\dagger Y_e)^{pr} \left. \right\} + \left\{ -\frac{1}{2}\delta^{td}Y_d^{*cs}Y_u^{*ab}(Y_e^\dagger Y_e)^{pr} - \frac{3}{4}\delta^{td}Y_d^{*as}Y_u^{*cb}(Y_e^\dagger Y_e)^{pr} - g_Y^2\left(\frac{1}{18}\delta^{pr}\delta^{td}Y_d^{*as}Y_u^{*cb} \right. \right. \\
& + \frac{10}{27}\delta^{pr}\delta^{td}Y_d^{*cs}Y_u^{*ab} \left. \right) \left. \right\} C_{quqd}^{(\times)abcd} + \left( C_{quqd}^{(\times)*} \right)^{abcd} \left\{ -\frac{1}{2}\delta^{sd}Y_d^{ct}Y_u^{ab}(Y_e^\dagger Y_e)^{pr} - \frac{3}{4}\delta^{sd}Y_d^{at}Y_u^{cb}(Y_e^\dagger Y_e)^{pr} - g_Y^2\left(\frac{1}{18}\delta^{pr}\delta^{sd}Y_d^{at}Y_u^{cb} + \frac{10}{27}\delta^{pr}\delta^{sd}Y_d^{ct}Y_u^{ab} \right) \right\} \\
& + \left\{ \frac{3}{2}\delta^{rb}Y_e^{*ap}Y_u^{*cd}(Y_d^\dagger Y_d)^{st} - \frac{2}{9}\delta^{rb}\delta^{st}g_Y^2Y_e^{*ap}Y_u^{*cd} - \frac{3}{4}\delta^{rb}Y_d^{*cs}Y_e^{*ap}(Y_u^\dagger Y_d)^{dt} \right\} C_{lequ}^{abcd} + C_{lequ}^{*abcd} \left\{ \frac{3}{2}\delta^{pb}Y_e^{ar}Y_u^{cd}(Y_d^\dagger Y_d)^{st} - \frac{2}{9}\delta^{pb}\delta^{st}g_Y^2Y_e^{ar}Y_u^{cd} \right. \\
& - \frac{3}{4}\delta^{pb}Y_d^{ct}Y_e^{ar}(Y_d^\dagger Y_u)^{sd} \left. \right\} + \left\{ \frac{5}{18}\delta^{rd}\delta^{st}g_Y^2Y_e^{*ap}Y_u^{*cb} + \frac{5}{4}\delta^{rd}Y_d^{*cs}Y_e^{*ap}(Y_u^\dagger Y_d)^{bt} - \frac{3}{4}\delta^{rd}Y_e^{*ap}Y_u^{*cb}(Y_d^\dagger Y_d)^{st} \right\} C_{luqe}^{abcd} + C_{luqe}^{*abcd} \left\{ \frac{5}{18}\delta^{pd}\delta^{st}g_Y^2Y_e^{ar}Y_u^{cb} \right. \\
& + \frac{5}{4}\delta^{pd}Y_d^{ct}Y_e^{ar}(Y_d^\dagger Y_u)^{sb} - \frac{3}{4}\delta^{pd}Y_e^{ar}Y_u^{cb}(Y_d^\dagger Y_d)^{st} \left. \right\} + \left\{ \frac{16}{27}\delta^{pr}\delta^{st}\delta^{ad}\delta^{bc}g_Y^4 - \frac{8}{9}\delta^{st}\delta^{bc}g_Y^2Y_e^{*ap}Y_e^{dr} \right\} C_{\ell\ell}^{abcd} + \left\{ \frac{16}{81}\delta^{pr}\delta^{st}\delta^{ad}\delta^{bc}g_Y^4 \right. \\
& + \frac{8}{9}\delta^{pr}\delta^{bc}g_Y^2Y_d^{*as}Y_d^{dt} \left. \right\} C_{qq}^{(\parallel)abcd} + \left\{ \frac{32}{81}\delta^{pr}\delta^{st}\delta^{ad}\delta^{bc}g_Y^4 + \frac{16}{9}\delta^{pr}\delta^{bc}g_Y^2Y_d^{*as}Y_d^{dt} \right\} C_{qq}^{(\times)abcd} + 4Y_d^{*cs}Y_e^{*ap}C_{\ell q}^{(\parallel)abcd}Y_d^{dt}Y_e^{br} + 8Y_d^{*cs}Y_e^{*ap}C_{\ell q}^{(\times)abcd}Y_d^{dt}Y_e^{br}, \quad (11.10)
\end{aligned}$$

## 11.6 $C_{ud}^{(\parallel)}$

$$\begin{aligned}
\beta_{C_{ud}^{(\parallel)prst}}^{(1)} = & \left\{ 2\delta^{pa}\delta^{rb}(Y_d^\dagger Y_d)^{st} - \frac{2}{9}\delta^{pa}\delta^{rb}\delta^{st}g_Y^2 \right\} C_{Hu}^{ab} + \left\{ \frac{4}{9}\delta^{pr}\delta^{sa}\delta^{tb}g_Y^2 - 2\delta^{sa}\delta^{tb}(Y_u^\dagger Y_u)^{pr} \right\} C_{Hd}^{ab} + \frac{4}{9}\delta^{pc}\delta^{rd}\delta^{st}\delta^{ab}g_Y^2 C_{\ell u}^{abcd} - \frac{8}{9}\delta^{pr}\delta^{sc}\delta^{td}\delta^{ab}g_Y^2 C_{\ell d}^{abcd} \\
& - \left\{ \frac{4}{9}\delta^{pc}\delta^{rd}\delta^{st}\delta^{ab}g_Y^2 + 2\delta^{pc}\delta^{rd}Y_d^{*as}Y_d^{bt} \right\} C_{qu}^{(\parallel)abcd} - \left\{ \frac{4}{27}\delta^{pc}\delta^{rd}\delta^{st}\delta^{ab}g_Y^2 + \frac{4}{9}\delta^{pc}\delta^{rd}\delta^{st}\delta^{ab}g_s^2 \right\} C_{qu}^{(\times)abcd} + \left\{ \frac{8}{9}\delta^{pr}\delta^{sc}\delta^{td}\delta^{ab}g_Y^2 \right. \\
& - 2\delta^{sc}\delta^{td}Y_u^{*ap}Y_u^{br} \left. \right\} C_{qd}^{(\parallel)abcd} + \left\{ \frac{8}{27}\delta^{pr}\delta^{sc}\delta^{td}\delta^{ab}g_Y^2 - \frac{4}{9}\delta^{pr}\delta^{sc}\delta^{td}\delta^{ab}g_s^2 \right\} C_{qd}^{(\times)abcd} - \left\{ \frac{4}{9}\delta^{pa}\delta^{rd}\delta^{st}\delta^{bc}g_s^2 + \frac{16}{27}g_Y^2 \left( \delta^{pa}\delta^{rd}\delta^{st}\delta^{bc} \right. \right. \\
& + 3\delta^{pa}\delta^{rb}\delta^{st}\delta^{cd} \left. \left. \right) \right\} C_{uu}^{abcd} - \left\{ \frac{4}{9}\delta^{pr}\delta^{sa}\delta^{td}\delta^{bc}g_s^2 + \frac{16}{27}g_Y^2 \left( \delta^{pr}\delta^{sa}\delta^{td}\delta^{bc} + 3\delta^{pr}\delta^{sa}\delta^{tb}\delta^{cd} \right) \right\} C_{dd}^{abcd} + \frac{4}{9}\delta^{pc}\delta^{rd}\delta^{st}\delta^{ab}g_Y^2 C_{eu}^{abcd} - \frac{8}{9}\delta^{pr}\delta^{sc}\delta^{td}\delta^{ab}g_Y^2 C_{ed}^{abcd} \\
& + \left\{ \delta^{pa}\delta^{rb}\delta^{td}(Y_d^\dagger Y_d)^{sc} + \delta^{pa}\delta^{rb}\delta^{sc}(Y_d^\dagger Y_d)^{dt} + \delta^{rb}\delta^{sc}\delta^{td}(Y_u^\dagger Y_u)^{pa} + \delta^{pa}\delta^{sc}\delta^{td}(Y_u^\dagger Y_u)^{br} - \frac{4}{9}g_Y^2 \left( 6\delta^{pa}\delta^{rb}\delta^{sc}\delta^{td} - \delta^{pa}\delta^{rb}\delta^{st}\delta^{cd} - 4\delta^{pr}\delta^{sc}\delta^{td}\delta^{ab} \right) \right. \\
& - 2\delta^{pa}\delta^{rb}\delta^{sc}\delta^{td}g_s^2 \left. \right\} C_{ud}^{(\parallel)abcd} + \left\{ \frac{4}{27}g_Y^2 \left( \delta^{pa}\delta^{rb}\delta^{st}\delta^{cd} + 4\delta^{pr}\delta^{sc}\delta^{td}\delta^{ab} \right) + \frac{2}{9}g_s^2 \left( 27\delta^{pa}\delta^{rb}\delta^{sc}\delta^{td} - \delta^{pr}\delta^{sc}\delta^{td}\delta^{ab} - \delta^{pa}\delta^{rb}\delta^{st}\delta^{cd} \right) \right\} C_{ud}^{(\times)abcd} \\
& - \delta^{rb}\delta^{td}Y_d^{*cs}Y_u^{ap} C_{quqd}^{(\parallel)abcd} - \delta^{pb}\delta^{sd} \left( C_{quqd}^{(\parallel)*} \right)^{abcd} Y_d^{ct}Y_u^{ar} + \delta^{rb}\delta^{td}Y_d^{*as}Y_u^{cp} C_{quqd}^{(\times)abcd} + \delta^{pb}\delta^{sd} \left( C_{quqd}^{(\times)*} \right)^{abcd} Y_d^{at}Y_u^{cr}, \tag{11.11}
\end{aligned}$$

$$\begin{aligned}
\beta_{C_{ud}^{(\parallel)prst}}^{(2)} = & \left\{ g_Y^4 \left( \frac{22}{9}\delta^{st}(Y_u^\dagger Y_u)^{pr} + \frac{28}{9}\delta^{pr}(Y_d^\dagger Y_d)^{st} \right) - \frac{16}{27}\delta^{pr}\delta^{st}g_Y^6 \right\} C_{HB} + g_s^4 \left\{ \frac{4}{3}\delta^{pr}(Y_d^\dagger Y_d)^{st} + \frac{4}{3}\delta^{st}(Y_u^\dagger Y_u)^{pr} \right\} C_{HG} + \left\{ g_Y^2 g_L^2 \left( \frac{1}{2}\delta^{st}(Y_u^\dagger Y_u)^{pr} + \delta^{pr}(Y_d^\dagger Y_d)^{st} \right) \right. \\
& - \frac{4}{9}\delta^{pr}\delta^{st}g_Y^4 g_L^2 \left. \right\} C_{HWB} + \left\{ g_s^6 \left( 3\delta^{pr}(Y_d^\dagger Y_d)^{st} + 3\delta^{st}(Y_u^\dagger Y_u)^{pr} \right) - \frac{388}{27}\delta^{pr}\delta^{st}g_Y^2 g_s^6 - \frac{331}{9}\delta^{pr}\delta^{st}g_s^8 \right\} C_G + \frac{8}{9}\delta^{pr}\delta^{st}g_Y^4 Y_e^{*ab} C_{eB}^{ab} \\
& + \frac{8}{9}\delta^{pr}\delta^{st}g_Y^4 C_{eB}^{*ab} Y_e^{ab} + \left\{ \frac{2}{3}\delta^{st}g_Y^2 Y_u^{*ap}(Y_u^\dagger Y_u)^{br} + \frac{76}{27}\delta^{rb}\delta^{st}g_Y^2 g_s^2 Y_u^{*ap} - g_Y^4 \left( \frac{2}{81}\delta^{rb}\delta^{st}Y_u^{*ap} + \frac{40}{27}\delta^{pr}\delta^{st}Y_u^{*ab} \right) \right\} C_{uB}^{ab} \\
& + C_{uB}^{*ab} \left\{ \frac{2}{3}\delta^{st}g_Y^2 Y_u^{ar}(Y_u^\dagger Y_u)^{pb} + \frac{76}{27}\delta^{pb}\delta^{st}g_Y^2 g_s^2 Y_u^{ar} - g_Y^4 \left( \frac{2}{81}\delta^{pb}\delta^{st}Y_u^{ar} + \frac{40}{27}\delta^{pr}\delta^{st}Y_u^{ab} \right) \right\} + \left\{ \frac{7}{9}\delta^{rb}\delta^{st}g_Y^2 g_L^2 Y_u^{*ap} + \frac{4}{3}\delta^{rb}\delta^{st}g_s^2 g_L^2 Y_u^{*ap} \right\} C_{uW}^{ab} \\
& + C_{uW}^{*ab} \left\{ \frac{7}{9}\delta^{pb}\delta^{st}g_Y^2 g_L^2 Y_u^{ar} + \frac{4}{3}\delta^{pb}\delta^{st}g_s^2 g_L^2 Y_u^{ar} \right\} + \left\{ g_s^2 \left( \frac{1}{3}\delta^{st}Y_u^{*ap}(Y_u^\dagger Y_u)^{br} + 12\delta^{rb}Y_d^{*as}(Y_u^\dagger Y_d)^{pt} - 6\delta^{rb}Y_u^{*ap}(Y_d^\dagger Y_d)^{st} \right) + \frac{98}{81}\delta^{rb}\delta^{st}g_Y^2 g_s^2 Y_u^{*ap} \right. \\
& - g_s^4 \left( \frac{4}{9}\delta^{pr}\delta^{st}Y_u^{*ab} + \frac{160}{27}\delta^{rb}\delta^{st}Y_u^{*ap} \right) \left. \right\} C_{uG}^{ab} + C_{uG}^{*ab} \left\{ g_s^2 \left( \frac{1}{3}\delta^{st}Y_u^{ar}(Y_u^\dagger Y_u)^{pb} + 12\delta^{pb}Y_d^{at}(Y_d^\dagger Y_u)^{sr} - 6\delta^{pb}Y_u^{ar}(Y_d^\dagger Y_d)^{st} \right) + \frac{98}{81}\delta^{pb}\delta^{st}g_Y^2 g_s^2 Y_u^{ar} \right.
\end{aligned}$$

$$\begin{aligned}
& -g_s^4 \left( \frac{4}{9} \delta^{pr} \delta^{st} Y_u^{ab} + \frac{160}{27} \delta^{pb} \delta^{st} Y_u^{ar} \right) \Bigg\} + \left\{ g_Y^4 \left( \frac{8}{27} \delta^{pr} \delta^{st} Y_d^{*ab} - \frac{104}{81} \delta^{pr} \delta^{tb} Y_d^{*as} \right) - g_Y^2 \left( \frac{4}{3} \delta^{pr} Y_d^{*as} (Y_d^\dagger Y_d)^{bt} + 6 \delta^{tb} Y_d^{*as} (Y_u^\dagger Y_u)^{pr} \right) \right. \\
& - \frac{116}{27} \delta^{pr} \delta^{tb} g_Y^2 g_s^2 Y_d^{*as} \Bigg\} C_{dB}^{ab} + C_{dB}^{*ab} \left\{ g_Y^4 \left( \frac{8}{27} \delta^{pr} \delta^{st} Y_d^{ab} - \frac{104}{81} \delta^{pr} \delta^{sb} Y_d^{at} \right) - g_Y^2 \left( \frac{4}{3} \delta^{pr} Y_d^{at} (Y_d^\dagger Y_d)^{sb} + 6 \delta^{sb} Y_d^{at} (Y_u^\dagger Y_u)^{pr} \right) - \frac{116}{27} \delta^{pr} \delta^{sb} g_Y^2 g_s^2 Y_d^{at} \right\} \\
& + \left\{ \frac{4}{3} \delta^{pr} \delta^{tb} g_s^2 g_L^2 Y_d^{*as} - \frac{2}{9} \delta^{pr} \delta^{tb} g_Y^2 g_L^2 Y_d^{*as} \right\} C_{dW}^{ab} + C_{dW}^{*ab} \left\{ \frac{4}{3} \delta^{pr} \delta^{sb} g_s^2 g_L^2 Y_d^{at} - \frac{2}{9} \delta^{pr} \delta^{sb} g_Y^2 g_L^2 Y_d^{at} \right\} + \left\{ g_s^2 \left( \frac{1}{3} \delta^{pr} Y_d^{*as} (Y_d^\dagger Y_d)^{bt} \right. \right. \\
& + 12 \delta^{tb} Y_u^{*ap} (Y_d^\dagger Y_u)^{sr} - 6 \delta^{tb} Y_d^{*as} (Y_u^\dagger Y_u)^{pr} \Bigg) - g_s^4 \left( \frac{4}{9} \delta^{pr} \delta^{st} Y_d^{*ab} + \frac{160}{27} \delta^{pr} \delta^{tb} Y_d^{*as} \right) - \frac{82}{81} \delta^{pr} \delta^{tb} g_Y^2 g_s^2 Y_d^{*as} \Bigg\} C_{dG}^{ab} + C_{dG}^{*ab} \left\{ g_s^2 \left( \frac{1}{3} \delta^{pr} Y_d^{at} (Y_d^\dagger Y_d)^{sb} \right. \right. \\
& + 12 \delta^{sb} Y_u^{ar} (Y_u^\dagger Y_d)^{pt} - 6 \delta^{sb} Y_d^{at} (Y_u^\dagger Y_u)^{pr} \Bigg) - g_s^4 \left( \frac{4}{9} \delta^{pr} \delta^{st} Y_d^{ab} + \frac{160}{27} \delta^{pr} \delta^{sb} Y_d^{at} \right) - \frac{82}{81} \delta^{pr} \delta^{sb} g_Y^2 g_s^2 Y_d^{at} \Bigg\} + \left\{ \frac{47}{243} \delta^{pa} \delta^{rb} \delta^{st} g_Y^2 g_s^2 \right. \\
& + \frac{1}{2} \delta^{rb} (Y_d^\dagger Y_d)^{st} (Y_u^\dagger Y_u)^{pa} + \frac{1}{2} \delta^{pa} (Y_d^\dagger Y_d)^{st} (Y_u^\dagger Y_u)^{br} + g_Y^2 \left( \frac{2}{9} T_2 \delta^{pa} \delta^{rb} \delta^{st} + \frac{101}{36} \delta^{pa} \delta^{rb} (Y_d^\dagger Y_d)^{st} - \frac{101}{162} \delta^{rb} \delta^{st} (Y_u^\dagger Y_u)^{pa} - \frac{101}{162} \delta^{pa} \delta^{st} (Y_u^\dagger Y_u)^{br} \right) \\
& + \frac{51}{4} \delta^{pa} \delta^{rb} g_L^2 (Y_d^\dagger Y_d)^{st} - \frac{298}{729} \delta^{pa} \delta^{rb} \delta^{st} g_Y^4 - g_s^2 \left( \frac{7}{27} \delta^{rb} \delta^{st} (Y_u^\dagger Y_u)^{pa} + \frac{7}{27} \delta^{pa} \delta^{st} (Y_u^\dagger Y_u)^{br} + \frac{25}{3} \delta^{pa} \delta^{rb} (Y_d^\dagger Y_d)^{st} \right) - 2 \delta^{pa} \delta^{rb} \delta^{st} g_Y^2 g_L^2 \\
& - 2 T_2 \delta^{pa} \delta^{rb} (Y_d^\dagger Y_d)^{st} - 3 \delta^{pa} \delta^{rb} (Y_d^\dagger Y_d Y_d^\dagger Y_d)^{st} \Bigg\} C_{Hu}^{ab} + \left\{ \frac{44}{243} \delta^{pr} \delta^{sa} \delta^{tb} g_Y^2 g_s^2 + g_Y^2 \left( \frac{73}{81} \delta^{pr} \delta^{tb} (Y_d^\dagger Y_d)^{sa} + \frac{73}{81} \delta^{pr} \delta^{sa} (Y_d^\dagger Y_d)^{bt} \right. \right. \\
& - \frac{4}{9} T_2 \delta^{pr} \delta^{sa} \delta^{tb} - \frac{89}{36} \delta^{sa} \delta^{tb} (Y_u^\dagger Y_u)^{pr} \Bigg) + g_s^2 \left( \frac{7}{27} \delta^{pr} \delta^{tb} (Y_d^\dagger Y_d)^{sa} + \frac{7}{27} \delta^{pr} \delta^{sa} (Y_d^\dagger Y_d)^{bt} + \frac{25}{3} \delta^{sa} \delta^{tb} (Y_u^\dagger Y_u)^{pr} \right) + \frac{1148}{729} \delta^{pr} \delta^{sa} \delta^{tb} g_Y^4 \\
& + 2 T_2 \delta^{sa} \delta^{tb} (Y_u^\dagger Y_u)^{pr} + 3 \delta^{sa} \delta^{tb} (Y_u^\dagger Y_u Y_u^\dagger Y_u)^{pr} + 4 \delta^{pr} \delta^{sa} \delta^{tb} g_Y^2 g_L^2 - \frac{1}{2} \delta^{tb} (Y_d^\dagger Y_d)^{sa} (Y_u^\dagger Y_u)^{pr} - \frac{1}{2} \delta^{sa} (Y_d^\dagger Y_d)^{bt} (Y_u^\dagger Y_u)^{pr} \\
& - \frac{51}{4} \delta^{sa} \delta^{tb} g_L^2 (Y_u^\dagger Y_u)^{pr} \Bigg\} C_{Hd}^{ab} + \left\{ g_s^2 \left( \frac{1}{27} \delta^{pr} \delta^{tb} (Y_d^\dagger Y_u)^{sa} + \frac{1}{27} \delta^{pa} \delta^{st} (Y_d^\dagger Y_u)^{br} - 7 \delta^{pa} \delta^{tb} (Y_d^\dagger Y_u)^{sr} \right) + \frac{3}{2} \delta^{pa} (Y_d^\dagger Y_d)^{st} (Y_d^\dagger Y_u)^{br} + \frac{3}{2} \delta^{tb} (Y_d^\dagger Y_u)^{sa} (Y_u^\dagger Y_u)^{pr} \right. \\
& - g_Y^2 \left( \frac{55}{162} \delta^{pa} \delta^{st} (Y_d^\dagger Y_u)^{br} + \frac{59}{81} \delta^{pr} \delta^{tb} (Y_d^\dagger Y_u)^{sa} \right) \Bigg\} C_{Hud}^{ab} + C_{Hud}^{*ab} \left\{ g_s^2 \left( \frac{1}{27} \delta^{ra} \delta^{st} (Y_u^\dagger Y_d)^{pb} + \frac{1}{27} \delta^{pr} \delta^{sb} (Y_u^\dagger Y_d)^{at} - 7 \delta^{ra} \delta^{sb} (Y_u^\dagger Y_d)^{pt} \right) \right. \\
& + \frac{3}{2} \delta^{ra} (Y_d^\dagger Y_d)^{st} (Y_u^\dagger Y_d)^{pb} + \frac{3}{2} \delta^{sb} (Y_u^\dagger Y_d)^{at} (Y_u^\dagger Y_u)^{pr} - g_Y^2 \left( \frac{55}{162} \delta^{ra} \delta^{st} (Y_u^\dagger Y_d)^{pb} + \frac{59}{81} \delta^{pr} \delta^{sb} (Y_u^\dagger Y_d)^{at} \right) \Bigg\} + \left\{ \frac{329}{729} \delta^{pc} \delta^{rd} \delta^{st} \delta^{ab} g_Y^4 + \delta^{pc} \delta^{rd} \delta^{st} \delta^{ab} g_Y^2 g_L^2 \right. \\
& - \frac{154}{243} \delta^{pc} \delta^{rd} \delta^{st} \delta^{ab} g_Y^2 g_s^2 - \frac{8}{9} \delta^{pc} \delta^{rd} \delta^{st} g_Y^2 (Y_e Y_e^\dagger)^{ba} - \delta^{pc} \delta^{rd} (Y_d^\dagger Y_d)^{st} (Y_e Y_e^\dagger)^{ba} \Bigg\} C_{\ell u}^{abcd} + \left\{ \frac{104}{243} \delta^{pr} \delta^{sc} \delta^{td} \delta^{ab} g_Y^2 g_s^2 + \delta^{sc} \delta^{td} (Y_u^\dagger Y_u)^{pr} (Y_e Y_e^\dagger)^{ba} \right. \\
& + \frac{16}{9} \delta^{pr} \delta^{sc} \delta^{td} g_Y^2 (Y_e Y_e^\dagger)^{ba} - \frac{826}{729} \delta^{pr} \delta^{sc} \delta^{td} \delta^{ab} g_Y^4 - 2 \delta^{pr} \delta^{sc} \delta^{td} \delta^{ab} g_Y^2 g_L^2 \Bigg\} C_{\ell d}^{abcd} + \left\{ \frac{1}{2} \delta^{pc} \delta^{rd} Y_d^{bt} (Y_u^\dagger Y_u Y_d^\dagger)^{as} + \frac{1}{2} \delta^{pc} \delta^{rd} Y_d^{*as} (Y_u Y_u^\dagger Y_d)^{bt} \right.
\end{aligned}$$



$$\begin{aligned}
& + g_s^2 \left( \frac{8}{27} \delta^{pc} \delta^{st} Y_u^{*ad} Y_u^{br} + \frac{8}{27} \delta^{rd} \delta^{st} Y_u^{*ap} Y_u^{bc} + 12 \delta^{pc} \delta^{rd} Y_d^{*as} Y_d^{bt} \right) + g_Y^2 \left( \frac{4}{3} \delta^{pc} \delta^{rd} \delta^{st} (Y_u Y_u^\dagger)^{ba} - \frac{4}{81} \delta^{pc} \delta^{st} Y_u^{*ad} Y_u^{br} - \frac{4}{81} \delta^{rd} \delta^{st} Y_u^{*ap} Y_u^{bc} \right. \\
& - \frac{5}{4} \delta^{pc} \delta^{rd} Y_d^{*as} Y_d^{bt} \left. \right) + \frac{823}{729} \delta^{pc} \delta^{rd} \delta^{st} \delta^{ab} g_Y^4 + \frac{3}{2} \delta^{pc} \delta^{rd} Y_d^{*as} (Y_d^\dagger Y_d^\dagger)^{bt} + \frac{3}{2} \delta^{pc} \delta^{rd} Y_d^{*as} (Y_d Y_d^\dagger)^{bt} + 3 T_2 \delta^{pc} \delta^{rd} Y_d^{*as} Y_d^{bt} \\
& + 3 \delta^{pc} \delta^{rd} (Y_d^\dagger Y_d)^{st} (Y_u Y_u^\dagger)^{ba} - \frac{1}{2} \delta^{rd} Y_d^{*as} Y_d^{bt} (Y_u^\dagger Y_u)^{pc} - \frac{1}{2} \delta^{pc} Y_d^{*as} Y_d^{bt} (Y_u^\dagger Y_u)^{dr} - \delta^{pc} \delta^{rd} \delta^{st} \delta^{ab} g_Y^2 g_L^2 - \frac{278}{243} \delta^{pc} \delta^{rd} \delta^{st} \delta^{ab} g_Y^2 g_s^2 \\
& - 3 \delta^{pc} \delta^{rd} (Y_d^\dagger Y_d)^{st} (Y_d Y_d^\dagger)^{ba} - \frac{51}{4} \delta^{pc} \delta^{rd} g_L^2 Y_d^{*as} Y_d^{bt} - \frac{122}{9} \delta^{pc} \delta^{rd} \delta^{st} \delta^{ab} g_s^4 \left. \right\} C_{qu}^{(\parallel)abcd} + \left\{ \frac{823}{2187} \delta^{pc} \delta^{rd} \delta^{st} \delta^{ab} g_Y^4 + g_s^4 \left( \frac{4}{27} \delta^{pr} \delta^{st} \delta^{ab} \delta^{cd} \right. \right. \\
& - \frac{1256}{243} \delta^{pc} \delta^{rd} \delta^{st} \delta^{ab} \left. \right) + g_Y^2 g_s^2 \left( \frac{16}{81} \delta^{pr} \delta^{st} \delta^{ab} \delta^{cd} + \frac{3167}{729} \delta^{pc} \delta^{rd} \delta^{st} \delta^{ab} \right) + \delta^{pc} \delta^{rd} (Y_d^\dagger Y_d)^{st} (Y_u Y_u^\dagger)^{ba} + g_Y^2 \left( \frac{4}{27} \delta^{pc} \delta^{rd} \delta^{st} (Y_u Y_u^\dagger)^{ba} + \frac{20}{27} \delta^{pc} \delta^{st} Y_u^{*ad} Y_u^{br} \right. \\
& + \frac{20}{27} \delta^{rd} \delta^{st} Y_u^{*ap} Y_u^{bc} - \frac{8}{27} \delta^{st} \delta^{cd} Y_u^{*ap} Y_u^{br} \left. \right) + g_s^2 \left( \frac{2}{9} \delta^{pc} \delta^{st} Y_u^{*ad} Y_u^{br} + \frac{2}{9} \delta^{rd} \delta^{st} Y_u^{*ap} Y_u^{bc} + \frac{4}{9} \delta^{pc} \delta^{rd} \delta^{st} (Y_u Y_u^\dagger)^{ba} + \frac{2}{3} \delta^{pc} \delta^{rd} \delta^{st} (Y_d Y_d^\dagger)^{ba} \right. \\
& + 4 \delta^{pc} \delta^{rd} Y_d^{*as} Y_d^{bt} - \frac{2}{9} \delta^{st} \delta^{cd} Y_u^{*ap} Y_u^{br} \left. \right) + 4 \delta^{rd} Y_u^{*ap} Y_d^{bt} (Y_d^\dagger Y_u)^{sc} + 4 \delta^{pc} Y_d^{*as} Y_u^{br} (Y_u^\dagger Y_d)^{dt} - \frac{1}{3} \delta^{pc} \delta^{rd} \delta^{st} \delta^{ab} g_Y^2 g_L^2 - \delta^{pc} \delta^{rd} \delta^{st} \delta^{ab} g_s^2 g_L^2 \\
& - \delta^{pc} \delta^{rd} (Y_d^\dagger Y_d)^{st} (Y_d Y_d^\dagger)^{ba} \left. \right\} C_{qu}^{(\times)abcd} + \left\{ \frac{1}{2} \delta^{sc} \delta^{td} Y_u^{br} (Y_d^\dagger Y_d Y_u^\dagger)^{ap} + \frac{1}{2} \delta^{sc} \delta^{td} Y_u^{*ap} (Y_d Y_d^\dagger Y_u)^{br} + g_s^2 \left( \frac{8}{27} \delta^{pr} \delta^{sc} Y_d^{*ad} Y_d^{bt} + \frac{8}{27} \delta^{pr} \delta^{td} Y_d^{*as} Y_d^{bc} \right. \right. \\
& + 12 \delta^{sc} \delta^{td} Y_u^{*ap} Y_u^{br} \left. \right) + g_Y^2 \left( \frac{3}{4} \delta^{sc} \delta^{td} Y_u^{*ap} Y_u^{br} - \frac{40}{81} \delta^{pr} \delta^{sc} Y_d^{*ad} Y_d^{bt} - \frac{40}{81} \delta^{pr} \delta^{td} Y_d^{*as} Y_d^{bc} - \frac{8}{3} \delta^{pr} \delta^{sc} \delta^{td} (Y_u Y_u^\dagger)^{ba} \right) + \frac{3}{2} \delta^{sc} \delta^{td} Y_u^{br} (Y_u^\dagger Y_u Y_u^\dagger)^{ap} \\
& + \frac{3}{2} \delta^{sc} \delta^{td} Y_u^{*ap} (Y_u Y_u^\dagger Y_u)^{br} + 2 \delta^{pr} \delta^{sc} \delta^{td} \delta^{ab} g_Y^2 g_L^2 + 3 T_2 \delta^{sc} \delta^{td} Y_u^{*ap} Y_u^{br} + 3 \delta^{sc} \delta^{td} (Y_u^\dagger Y_u)^{pr} (Y_d Y_d^\dagger)^{ba} + \frac{760}{243} \delta^{pr} \delta^{sc} \delta^{td} \delta^{ab} g_Y^2 g_s^2 \\
& - \frac{1}{2} \delta^{td} Y_u^{*ap} Y_u^{br} (Y_d^\dagger Y_d)^{sc} - \frac{1}{2} \delta^{sc} Y_u^{*ap} Y_u^{br} (Y_d^\dagger Y_d)^{dt} - \frac{614}{729} \delta^{pr} \delta^{sc} \delta^{td} \delta^{ab} g_Y^4 - 3 \delta^{sc} \delta^{td} (Y_u^\dagger Y_u)^{pr} (Y_u Y_u^\dagger)^{ba} - \frac{51}{4} \delta^{sc} \delta^{td} g_L^2 Y_u^{*ap} Y_u^{br} \\
& - \frac{122}{9} \delta^{pr} \delta^{sc} \delta^{td} \delta^{ab} g_s^4 \left. \right\} C_{qd}^{(\parallel)abcd} + \left\{ \frac{2}{3} \delta^{pr} \delta^{sc} \delta^{td} \delta^{ab} g_Y^2 g_L^2 + g_s^4 \left( \frac{4}{27} \delta^{pr} \delta^{st} \delta^{ab} \delta^{cd} - \frac{1256}{243} \delta^{pr} \delta^{sc} \delta^{td} \delta^{ab} \right) + g_Y^2 g_s^2 \left( \frac{16}{81} \delta^{pr} \delta^{st} \delta^{ab} \delta^{cd} \right. \right. \\
& - \frac{169}{729} \delta^{pr} \delta^{sc} \delta^{td} \delta^{ab} \left. \right) + \delta^{sc} \delta^{td} (Y_u^\dagger Y_u)^{pr} (Y_d Y_d^\dagger)^{ba} + g_s^2 \left( \frac{2}{9} \delta^{pr} \delta^{sc} Y_d^{*ad} Y_d^{bt} + \frac{2}{9} \delta^{pr} \delta^{td} Y_d^{*as} Y_d^{bc} + \frac{4}{9} \delta^{pr} \delta^{sc} \delta^{td} (Y_d Y_d^\dagger)^{ba} + \frac{2}{3} \delta^{pr} \delta^{sc} \delta^{td} (Y_u Y_u^\dagger)^{ba} \right. \\
& + 4 \delta^{sc} \delta^{td} Y_u^{*ap} Y_u^{br} - \frac{2}{9} \delta^{pr} \delta^{cd} Y_d^{*as} Y_d^{bt} \left. \right) + 4 \delta^{sc} Y_u^{*ap} Y_d^{bt} (Y_d^\dagger Y_u)^{dr} + 4 \delta^{td} Y_d^{*as} Y_u^{br} (Y_u^\dagger Y_d)^{pc} - \frac{614}{2187} \delta^{pr} \delta^{sc} \delta^{td} \delta^{ab} g_Y^4 - \delta^{pr} \delta^{sc} \delta^{td} \delta^{ab} g_s^2 g_L^2 \\
& - \delta^{sc} \delta^{td} (Y_u^\dagger Y_u)^{pr} (Y_u Y_u^\dagger)^{ba} - g_Y^2 \left( \frac{8}{27} \delta^{pr} \delta^{cd} Y_d^{*as} Y_d^{bt} + \frac{8}{27} \delta^{pr} \delta^{sc} \delta^{td} (Y_d Y_d^\dagger)^{ba} + \frac{16}{27} \delta^{pr} \delta^{sc} Y_d^{*ad} Y_d^{bt} + \frac{16}{27} \delta^{pr} \delta^{td} Y_d^{*as} Y_d^{bc} \right. \\
& + \frac{8}{9} \delta^{pr} \delta^{sc} \delta^{td} (Y_u Y_u^\dagger)^{ba} \left. \right) \left. \right\} C_{qd}^{(\times)abcd} - \frac{64}{81} \delta^{pr} \delta^{st} \delta^{ab} \delta^{cd} g_Y^4 C_{ee}^{abcd} + \left\{ g_Y^2 g_s^2 \left( \frac{16}{81} \delta^{pr} \delta^{st} \delta^{ad} \delta^{bc} + \frac{2624}{729} \delta^{pa} \delta^{rd} \delta^{st} \delta^{bc} - \frac{680}{243} \delta^{pa} \delta^{rb} \delta^{st} \delta^{cd} \right) \right. \\
& + g_Y^4 \left( \frac{8320}{2187} \delta^{pa} \delta^{rd} \delta^{st} \delta^{bc} + \frac{3904}{729} \delta^{pa} \delta^{rb} \delta^{st} \delta^{cd} - \frac{256}{243} \delta^{pr} \delta^{st} \delta^{ad} \delta^{bc} \right) + g_s^4 \left( \frac{158}{9} \delta^{pa} \delta^{rb} \delta^{st} \delta^{cd} - \frac{4}{27} \delta^{pr} \delta^{st} \delta^{ad} \delta^{bc} - \frac{296}{243} \delta^{pa} \delta^{rd} \delta^{st} \delta^{bc} \right) \\
& + g_Y^2 \left( \frac{68}{27} \delta^{pa} \delta^{rd} \delta^{st} (Y_u^\dagger Y_u)^{bc} + 4 \delta^{pa} \delta^{rb} \delta^{st} (Y_u^\dagger Y_u)^{dc} \right) + \frac{20}{9} \delta^{pa} \delta^{rd} \delta^{st} g_s^2 (Y_u^\dagger Y_u)^{bc} - \delta^{pa} \delta^{rb} (Y_d^\dagger Y_u)^{sc} (Y_u^\dagger Y_d)^{dt} - 6 \delta^{pa} \delta^{rd} (Y_d^\dagger Y_d)^{st} (Y_u^\dagger Y_u)^{bc}
\end{aligned}$$

$$\begin{aligned}
& -6\delta^{pa}\delta^{rb}(Y_d^\dagger Y_d)^{st}(Y_u^\dagger Y_u)^{dc} \Big\} C_{uu}^{abcd} + \left\{ g_Y^2 g_s^2 \left( \frac{16}{81} \delta^{pr} \delta^{st} \delta^{ad} \delta^{bc} + \frac{1928}{729} \delta^{pr} \delta^{sa} \delta^{td} \delta^{bc} - \frac{1088}{243} \delta^{pr} \delta^{sa} \delta^{tb} \delta^{cd} \right) + g_Y^4 \left( \frac{5536}{2187} \delta^{pr} \delta^{sa} \delta^{td} \delta^{bc} \right. \right. \\
& + \frac{3136}{729} \delta^{pr} \delta^{sa} \delta^{tb} \delta^{cd} - \frac{64}{243} \delta^{pr} \delta^{st} \delta^{ad} \delta^{bc} \Big) + g_s^4 \left( \frac{158}{9} \delta^{pr} \delta^{sa} \delta^{tb} \delta^{cd} - \frac{4}{27} \delta^{pr} \delta^{st} \delta^{ad} \delta^{bc} - \frac{296}{243} \delta^{pr} \delta^{sa} \delta^{td} \delta^{bc} \right) + g_Y^2 \left( \frac{56}{27} \delta^{pr} \delta^{sa} \delta^{td} (Y_d^\dagger Y_d)^{bc} \right. \\
& + \frac{8}{3} \delta^{pr} \delta^{sa} \delta^{tb} (Y_d^\dagger Y_d)^{dc} \Big) + \frac{20}{9} \delta^{pr} \delta^{sa} \delta^{td} g_s^2 (Y_d^\dagger Y_d)^{bc} - \delta^{sa} \delta^{tb} (Y_d^\dagger Y_u)^{dr} (Y_u^\dagger Y_d)^{pc} - 6\delta^{sa} \delta^{td} (Y_d^\dagger Y_d)^{bc} (Y_u^\dagger Y_u)^{pr} - 6\delta^{sa} \delta^{tb} (Y_d^\dagger Y_d)^{dc} (Y_u^\dagger Y_u)^{pr} \Big\} C_{dd}^{abcd} \\
& + \left\{ \delta^{pc} \delta^{rd} (Y_d^\dagger Y_d)^{st} (Y_e^\dagger Y_e)^{ba} + \frac{1544}{729} \delta^{pc} \delta^{rd} \delta^{st} \delta^{ab} g_Y^4 - \frac{154}{243} \delta^{pc} \delta^{rd} \delta^{st} \delta^{ab} g_Y^2 g_s^2 - \frac{10}{9} \delta^{pc} \delta^{rd} \delta^{st} g_Y^2 (Y_e^\dagger Y_e)^{ba} \right\} C_{eu}^{abcd} + \left\{ \frac{104}{243} \delta^{pr} \delta^{sc} \delta^{td} \delta^{ab} g_Y^2 g_s^2 \right. \\
& + \frac{20}{9} \delta^{pr} \delta^{sc} \delta^{td} g_Y^2 (Y_e^\dagger Y_e)^{ba} + \frac{2576}{729} \delta^{pr} \delta^{sc} \delta^{td} \delta^{ab} g_Y^4 - \delta^{sc} \delta^{td} (Y_e^\dagger Y_e)^{ba} (Y_u^\dagger Y_u)^{pr} \Big\} C_{ed}^{abcd} + \left\{ g_Y^4 \left( \frac{6368}{729} \delta^{pr} \delta^{sc} \delta^{td} \delta^{ab} - \frac{112}{729} \delta^{pa} \delta^{rb} \delta^{st} \delta^{cd} \right. \right. \\
& - \frac{2}{9} \delta^{pa} \delta^{rb} \delta^{sc} \delta^{td} \Big) + g_Y^2 g_s^2 \left( \frac{278}{243} \delta^{pa} \delta^{rb} \delta^{st} \delta^{cd} + \frac{1520}{243} \delta^{pr} \delta^{sc} \delta^{td} \delta^{ab} + \frac{194}{9} \delta^{pa} \delta^{rb} \delta^{sc} \delta^{td} \right) + g_s^4 \left( \frac{73}{9} \delta^{pr} \delta^{sc} \delta^{td} \delta^{ab} + \frac{73}{9} \delta^{pa} \delta^{rb} \delta^{st} \delta^{cd} \right. \\
& - \frac{71}{6} \delta^{pa} \delta^{rb} \delta^{sc} \delta^{td} \Big) + g_L^2 \left( \frac{51}{8} \delta^{pa} \delta^{rb} \delta^{td} (Y_d^\dagger Y_d)^{sc} + \frac{51}{8} \delta^{pa} \delta^{rb} \delta^{sc} (Y_d^\dagger Y_d)^{dt} + \frac{51}{8} \delta^{rb} \delta^{sc} \delta^{td} (Y_u^\dagger Y_u)^{pa} + \frac{51}{8} \delta^{pa} \delta^{sc} \delta^{td} (Y_u^\dagger Y_u)^{br} \right) \\
& + g_Y^2 \left( \frac{37}{72} \delta^{pa} \delta^{rb} \delta^{td} (Y_d^\dagger Y_d)^{sc} + \frac{37}{72} \delta^{pa} \delta^{rb} \delta^{sc} (Y_d^\dagger Y_d)^{dt} + \frac{97}{72} \delta^{rb} \delta^{sc} \delta^{td} (Y_u^\dagger Y_u)^{pa} + \frac{97}{72} \delta^{pa} \delta^{sc} \delta^{td} (Y_u^\dagger Y_u)^{br} - \frac{2}{3} \delta^{pa} \delta^{rb} \delta^{st} (Y_d^\dagger Y_d)^{dc} - 4\delta^{pr} \delta^{sc} \delta^{td} (Y_u^\dagger Y_u)^{ba} \right) \\
& + 3\delta^{pa} \delta^{rb} (Y_d^\dagger Y_d)^{st} (Y_d^\dagger Y_d)^{dc} + 3\delta^{sc} \delta^{td} (Y_u^\dagger Y_u)^{pr} (Y_u^\dagger Y_u)^{ba} - \frac{1}{4} \delta^{pa} \delta^{rb} \delta^{td} (Y_d^\dagger Y_d Y_d^\dagger Y_d)^{sc} - \frac{1}{4} \delta^{pa} \delta^{rb} \delta^{sc} (Y_d^\dagger Y_d Y_d^\dagger Y_d)^{dt} - \frac{1}{4} \delta^{pa} \delta^{rb} \delta^{td} (Y_d^\dagger Y_u Y_u^\dagger Y_d)^{sc} \\
& - \frac{1}{4} \delta^{pa} \delta^{rb} \delta^{sc} (Y_d^\dagger Y_u Y_u^\dagger Y_d)^{dt} - \frac{1}{4} \delta^{rb} \delta^{sc} \delta^{td} (Y_u^\dagger Y_d Y_d^\dagger Y_u)^{pa} - \frac{1}{4} \delta^{pa} \delta^{sc} \delta^{td} (Y_u^\dagger Y_d Y_d^\dagger Y_u)^{br} - \frac{1}{4} \delta^{rb} \delta^{sc} \delta^{td} (Y_u^\dagger Y_u Y_u^\dagger Y_u)^{pa} - \frac{1}{4} \delta^{pa} \delta^{sc} \delta^{td} (Y_u^\dagger Y_u Y_u^\dagger Y_u)^{br} \\
& - g_s^2 \left( \frac{10}{3} \delta^{pa} \delta^{rb} \delta^{td} (Y_d^\dagger Y_d)^{sc} + \frac{10}{3} \delta^{pa} \delta^{rb} \delta^{sc} (Y_d^\dagger Y_d)^{dt} + \frac{10}{3} \delta^{rb} \delta^{sc} \delta^{td} (Y_u^\dagger Y_u)^{pa} + \frac{10}{3} \delta^{pa} \delta^{sc} \delta^{td} (Y_u^\dagger Y_u)^{br} \right) - \frac{3}{2} T_2 \delta^{pa} \delta^{rb} \delta^{td} (Y_d^\dagger Y_d)^{sc} \\
& - \frac{3}{2} T_2 \delta^{pa} \delta^{rb} \delta^{sc} (Y_d^\dagger Y_d)^{dt} - \frac{3}{2} T_2 \delta^{rb} \delta^{sc} \delta^{td} (Y_u^\dagger Y_u)^{pa} - \frac{3}{2} T_2 \delta^{pa} \delta^{sc} \delta^{td} (Y_u^\dagger Y_u)^{br} - 2\delta^{rb} \delta^{sc} (Y_d^\dagger Y_d)^{dt} (Y_u^\dagger Y_u)^{pa} - 2\delta^{pa} \delta^{td} (Y_d^\dagger Y_d)^{sc} (Y_u^\dagger Y_u)^{br} \\
& - \frac{5}{2} \delta^{pa} \delta^{rb} (Y_d^\dagger Y_d)^{sc} (Y_d^\dagger Y_d)^{dt} - \frac{5}{2} \delta^{sc} \delta^{td} (Y_u^\dagger Y_u)^{pa} (Y_u^\dagger Y_u)^{br} - \frac{7}{2} \delta^{rb} \delta^{td} (Y_d^\dagger Y_d)^{sc} (Y_u^\dagger Y_u)^{pa} - \frac{7}{2} \delta^{pa} \delta^{sc} (Y_d^\dagger Y_d)^{dt} (Y_u^\dagger Y_u)^{br} \Big\} C_{ud}^{(\parallel)abcd} + \left\{ g_Y^4 \left( \frac{6368}{2187} \delta^{pr} \delta^{sc} \delta^{td} \delta^{ab} \right. \right. \\
& - \frac{112}{2187} \delta^{pa} \delta^{rb} \delta^{st} \delta^{cd} \Big) + g_s^4 \left( \frac{4}{27} \delta^{pr} \delta^{st} \delta^{ab} \delta^{cd} + \frac{15}{2} \delta^{pa} \delta^{rb} \delta^{sc} \delta^{td} - \frac{52}{243} \delta^{pr} \delta^{sc} \delta^{td} \delta^{ab} - \frac{52}{243} \delta^{pa} \delta^{rb} \delta^{st} \delta^{cd} \right) + g_Y^2 g_s^2 \left( \frac{16}{81} \delta^{pr} \delta^{st} \delta^{ab} \delta^{cd} \right. \\
& + \frac{304}{729} \delta^{pr} \delta^{sc} \delta^{td} \delta^{ab} + \frac{628}{729} \delta^{pa} \delta^{rb} \delta^{st} \delta^{cd} + \frac{25}{3} \delta^{pa} \delta^{rb} \delta^{sc} \delta^{td} \Big) + \delta^{pa} \delta^{rb} (Y_d^\dagger Y_d)^{st} (Y_d^\dagger Y_d)^{dc} + \delta^{sc} \delta^{td} (Y_u^\dagger Y_u)^{pr} (Y_u^\dagger Y_u)^{ba} + g_s^2 \left( \frac{2}{3} \delta^{pa} \delta^{rb} \delta^{st} (Y_d^\dagger Y_d)^{dc} \right. \\
& + \frac{2}{3} \delta^{pr} \delta^{sc} \delta^{td} (Y_u^\dagger Y_u)^{ba} - 6\delta^{pa} \delta^{rb} \delta^{td} (Y_d^\dagger Y_d)^{sc} - 6\delta^{pa} \delta^{rb} \delta^{sc} (Y_d^\dagger Y_d)^{dt} - 6\delta^{rb} \delta^{sc} \delta^{td} (Y_u^\dagger Y_u)^{pa} - 6\delta^{pa} \delta^{sc} \delta^{td} (Y_u^\dagger Y_u)^{br} \Big) + \frac{15}{2} \delta^{rb} \delta^{td} (Y_d^\dagger Y_u)^{sa} (Y_u^\dagger Y_d)^{pc} \\
& + \frac{15}{2} \delta^{pa} \delta^{sc} (Y_d^\dagger Y_u)^{dr} (Y_u^\dagger Y_d)^{bt} - g_Y^2 \left( \frac{2}{9} \delta^{pa} \delta^{rb} \delta^{st} (Y_d^\dagger Y_d)^{dc} + \frac{4}{3} \delta^{pr} \delta^{sc} \delta^{td} (Y_u^\dagger Y_u)^{ba} \right) \Big\} C_{ud}^{(\times)abcd} + \left\{ \frac{20}{81} \delta^{pr} \delta^{sc} g_Y^2 Y_e^{*ab} Y_d^{dt} + \frac{1}{2} \delta^{sc} Y_e^{*ab} Y_d^{dt} (Y_u^\dagger Y_u)^{pr} \right.
\end{aligned}$$

$$\begin{aligned}
& -\frac{4}{27}\delta^{pr}\delta^{sc}g_s^2Y_e^{*ab}Y_d^{dt}\Big\}C_{\ell edq}^{abcd}+C_{\ell edq}^{*abcd}\Big\{\frac{20}{81}\delta^{pr}\delta^{tc}g_Y^2Y_d^{*ds}Y_e^{ab}+\frac{1}{2}\delta^{tc}Y_d^{*ds}Y_e^{ab}(Y_u^\dagger Y_u)^{pr}-\frac{4}{27}\delta^{pr}\delta^{tc}g_s^2Y_d^{*ds}Y_e^{ab}\Big\}+\Big\{\frac{1}{4}\delta^{rb}Y_d^{*ad}Y_u^{*cp}(Y_d^\dagger Y_d)^{st} \\
& +\frac{1}{4}\delta^{td}Y_d^{*as}Y_u^{*cb}(Y_u^\dagger Y_u)^{pr}+\frac{1}{4}\delta^{rb}\delta^{td}Y_u^{*ap}(Y_d^\dagger Y_d Y_d^\dagger)^{cs}+\frac{1}{4}\delta^{rb}\delta^{td}Y_d^{*cs}(Y_u^\dagger Y_u Y_u^\dagger)^{ap}+\frac{1}{2}T_2\delta^{rb}\delta^{td}Y_d^{*cs}Y_u^{*ap}+\frac{3}{4}\delta^{rb}\delta^{td}Y_d^{*cs}(Y_d^\dagger Y_d Y_u^\dagger)^{ap} \\
& +\frac{3}{4}\delta^{rb}\delta^{td}Y_u^{*ap}(Y_u^\dagger Y_u Y_d^\dagger)^{cs}+g_Y^2\Big(\frac{1}{81}\delta^{pr}\delta^{td}Y_d^{*as}Y_u^{*cb}+\frac{2}{27}\delta^{rb}\delta^{st}Y_d^{*cd}Y_u^{*ap}+\frac{20}{27}\delta^{pr}\delta^{td}Y_d^{*cs}Y_u^{*ab}-\frac{7}{162}\delta^{rb}\delta^{st}Y_d^{*ad}Y_u^{*cp}-\frac{7}{24}\delta^{rb}\delta^{td}Y_d^{*cs}Y_u^{*ap}\Big) \\
& +g_s^2\Big(\frac{17}{2}\delta^{rb}\delta^{td}Y_d^{*cs}Y_u^{*ap}-\frac{2}{27}\delta^{rb}\delta^{st}Y_d^{*ad}Y_u^{*cp}-\frac{2}{27}\delta^{pr}\delta^{td}Y_d^{*as}Y_u^{*cb}-\frac{4}{9}\delta^{rb}\delta^{st}Y_d^{*cd}Y_u^{*ap}-\frac{4}{9}\delta^{pr}\delta^{td}Y_d^{*cs}Y_u^{*ab}-\frac{13}{2}\delta^{rb}\delta^{td}Y_d^{*as}Y_u^{*cp}\Big) \\
& +\frac{5}{4}\delta^{rb}Y_d^{*cs}Y_u^{*ap}(Y_d^\dagger Y_d)^{dt}+\frac{5}{4}\delta^{td}Y_d^{*cs}Y_u^{*ap}(Y_u^\dagger Y_u)^{br}+\frac{3}{2}\delta^{rb}Y_d^{*cd}Y_u^{*ap}(Y_d^\dagger Y_d)^{st}+\frac{3}{2}\delta^{td}Y_d^{*cs}Y_u^{*ab}(Y_u^\dagger Y_u)^{pr}-\frac{51}{8}\delta^{rb}\delta^{td}g_L^2Y_d^{*cs}Y_u^{*ap}\Big\}C_{quqd}^{(\parallel)abcd} \\
& +\Big(C_{quqd}^{(\parallel)*}\Big)^{abcd}\Big\{\frac{1}{4}\delta^{pb}Y_d^{ad}Y_u^{cr}(Y_d^\dagger Y_d)^{st}+\frac{1}{4}\delta^{sd}Y_d^{at}Y_u^{cb}(Y_u^\dagger Y_u)^{pr}+\frac{1}{4}\delta^{pb}\delta^{sd}Y_u^{ar}(Y_d Y_d^\dagger Y_d)^{ct}+\frac{1}{4}\delta^{pb}\delta^{sd}Y_d^{ct}(Y_u Y_u^\dagger Y_u)^{ar}+\frac{1}{2}T_2\delta^{pb}\delta^{sd}Y_d^{ct}Y_u^{ar} \\
& +\frac{3}{4}\delta^{pb}\delta^{sd}Y_d^{ct}(Y_d Y_d^\dagger Y_u)^{ar}+\frac{3}{4}\delta^{pb}\delta^{sd}Y_u^{ar}(Y_u Y_u^\dagger Y_d)^{ct}+g_Y^2\Big(\frac{1}{81}\delta^{pr}\delta^{sd}Y_d^{at}Y_u^{cb}+\frac{2}{27}\delta^{pb}\delta^{st}Y_d^{cd}Y_u^{ar}+\frac{20}{27}\delta^{pr}\delta^{sd}Y_d^{ct}Y_u^{ab}-\frac{7}{162}\delta^{pb}\delta^{st}Y_d^{ad}Y_u^{cr} \\
& -\frac{7}{24}\delta^{pb}\delta^{sd}Y_d^{ct}Y_u^{ar}\Big)+g_s^2\Big(\frac{17}{2}\delta^{pb}\delta^{sd}Y_d^{ct}Y_u^{ar}-\frac{2}{27}\delta^{pb}\delta^{st}Y_d^{ad}Y_u^{cr}-\frac{2}{27}\delta^{pr}\delta^{sd}Y_d^{at}Y_u^{cb}-\frac{4}{9}\delta^{pb}\delta^{st}Y_d^{cd}Y_u^{ar}-\frac{4}{9}\delta^{pr}\delta^{sd}Y_d^{ct}Y_u^{ab}-\frac{13}{2}\delta^{pb}\delta^{sd}Y_d^{at}Y_u^{cr}\Big) \\
& +\frac{5}{4}\delta^{pb}Y_d^{ct}Y_u^{ar}(Y_d^\dagger Y_d)^{sd}+\frac{5}{4}\delta^{sd}Y_d^{ct}Y_u^{ar}(Y_u^\dagger Y_u)^{pb}+\frac{3}{2}\delta^{pb}Y_d^{cd}Y_u^{ar}(Y_d^\dagger Y_d)^{st}+\frac{3}{2}\delta^{sd}Y_d^{ct}Y_u^{ab}(Y_u^\dagger Y_u)^{pr}-\frac{51}{8}\delta^{pb}\delta^{sd}g_L^2Y_d^{ct}Y_u^{ar}\Big\}+\Big\{\frac{1}{2}\delta^{rb}Y_d^{*cd}Y_u^{*ap}(Y_d^\dagger Y_d)^{st} \\
& +\frac{1}{2}\delta^{rb}Y_d^{*as}Y_u^{*cp}(Y_d^\dagger Y_d)^{dt}+\frac{1}{2}\delta^{td}Y_d^{*cs}Y_u^{*ab}(Y_u^\dagger Y_u)^{pr}+\frac{1}{2}\delta^{td}Y_d^{*as}Y_u^{*cp}(Y_u^\dagger Y_u)^{br}+\frac{3}{4}\delta^{rb}Y_d^{*ad}Y_u^{*cp}(Y_d^\dagger Y_d)^{st}+\frac{3}{4}\delta^{td}Y_d^{*as}Y_u^{*cb}(Y_u^\dagger Y_u)^{pr} \\
& +g_s^2\Big(7\delta^{rb}\delta^{td}Y_d^{*cs}Y_u^{*ap}-\frac{4}{27}\delta^{rb}\delta^{st}Y_d^{*cd}Y_u^{*ap}-\frac{4}{27}\delta^{pr}\delta^{td}Y_d^{*cs}Y_u^{*ab}-\frac{2}{9}\delta^{rb}\delta^{st}Y_d^{*ad}Y_u^{*cp}-\frac{2}{9}\delta^{pr}\delta^{td}Y_d^{*as}Y_u^{*cb}-7\delta^{rb}\delta^{td}Y_d^{*as}Y_u^{*cp}\Big) \\
& +g_Y^2\Big(\frac{2}{81}\delta^{rb}\delta^{st}Y_d^{*cd}Y_u^{*ap}+\frac{1}{27}\delta^{pr}\delta^{td}Y_d^{*as}Y_u^{*cb}+\frac{20}{81}\delta^{pr}\delta^{td}Y_d^{*cs}Y_u^{*ab}+\frac{7}{24}\delta^{rb}\delta^{td}Y_d^{*as}Y_u^{*cp}-\frac{7}{54}\delta^{rb}\delta^{st}Y_d^{*ad}Y_u^{*cp}\Big)+\frac{51}{8}\delta^{rb}\delta^{td}g_L^2Y_d^{*as}Y_u^{*cp} \\
& -\frac{1}{4}\delta^{rb}\delta^{td}Y_u^{*cp}(Y_d^\dagger Y_d Y_d^\dagger)^{as}-\frac{1}{4}\delta^{rb}\delta^{td}Y_d^{*as}(Y_u^\dagger Y_u Y_u^\dagger)^{cp}-\frac{1}{2}T_2\delta^{rb}\delta^{td}Y_d^{*as}Y_u^{*cp}-\frac{3}{4}\delta^{rb}\delta^{td}Y_d^{*as}(Y_d^\dagger Y_d Y_u^\dagger)^{cp}-\frac{3}{4}\delta^{rb}\delta^{td}Y_u^{*cp}(Y_u^\dagger Y_u Y_d^\dagger)^{as}\Big\}C_{quqd}^{(\times)abcd} \\
& +\Big(C_{quqd}^{(\times)*}\Big)^{abcd}\Big\{\frac{1}{2}\delta^{pb}Y_d^{cd}Y_u^{ar}(Y_d^\dagger Y_d)^{st}+\frac{1}{2}\delta^{pb}Y_d^{at}Y_u^{cr}(Y_d^\dagger Y_d)^{sd}+\frac{1}{2}\delta^{sd}Y_d^{ct}Y_u^{ab}(Y_u^\dagger Y_u)^{pr}+\frac{1}{2}\delta^{sd}Y_d^{at}Y_u^{cr}(Y_u^\dagger Y_u)^{pb}+\frac{3}{4}\delta^{pb}Y_d^{ad}Y_u^{cr}(Y_d^\dagger Y_d)^{st}+\frac{3}{4}\delta^{sd}Y_d^{at}Y_u^{cb}(Y_u^\dagger Y_u)^{pr} \\
& +g_s^2\Big(7\delta^{pb}\delta^{sd}Y_d^{ct}Y_u^{ar}-\frac{4}{27}\delta^{pb}\delta^{st}Y_d^{cd}Y_u^{ar}-\frac{4}{27}\delta^{pr}\delta^{sd}Y_d^{ct}Y_u^{ab}-\frac{2}{9}\delta^{pb}\delta^{st}Y_d^{ad}Y_u^{cr}-\frac{2}{9}\delta^{pr}\delta^{sd}Y_d^{at}Y_u^{cb}-7\delta^{pb}\delta^{sd}Y_d^{at}Y_u^{cr}\Big)+g_Y^2\Big(\frac{2}{81}\delta^{pb}\delta^{st}Y_d^{cd}Y_u^{ar} \\
& +\frac{1}{27}\delta^{pr}\delta^{sd}Y_d^{at}Y_u^{cb}+\frac{20}{81}\delta^{pr}\delta^{sd}Y_d^{ct}Y_u^{ab}+\frac{7}{24}\delta^{pb}\delta^{sd}Y_d^{at}Y_u^{cr}-\frac{7}{54}\delta^{pb}\delta^{st}Y_d^{ad}Y_u^{cr}\Big)+\frac{51}{8}\delta^{pb}\delta^{sd}g_L^2Y_d^{at}Y_u^{cr}-\frac{1}{4}\delta^{pb}\delta^{sd}Y_u^{cr}(Y_d Y_d^\dagger Y_d)^{at} \\
& -\frac{1}{4}\delta^{pb}\delta^{sd}Y_d^{at}(Y_u Y_u^\dagger Y_u)^{cr}-\frac{1}{2}T_2\delta^{pb}\delta^{sd}Y_d^{at}Y_u^{cr}-\frac{3}{4}\delta^{pb}\delta^{sd}Y_d^{at}(Y_d Y_d^\dagger Y_u)^{cr}-\frac{3}{4}\delta^{pb}\delta^{sd}Y_u^{cr}(Y_u Y_u^\dagger Y_d)^{at}\Big\}+\Big\{\frac{4}{27}\delta^{rd}\delta^{st}g_s^2Y_e^{*ab}Y_u^{*cp}
\end{aligned}$$

$$\begin{aligned}
& -\frac{2}{81}\delta^{rd}\delta^{st}g_Y^2Y_e^{*ab}Y_u^{*cp}-\frac{1}{2}\delta^{rd}Y_e^{*ab}Y_u^{*cp}(Y_d^\dagger Y_d)^{st}\Big\}C_{\ell equ}^{abcd}+C_{\ell equ}^{*abcd}\Big\{\frac{4}{27}\delta^{pd}\delta^{st}g_s^2Y_e^{ab}Y_u^{cr}-\frac{2}{81}\delta^{pd}\delta^{st}g_Y^2Y_e^{ab}Y_u^{cr}-\frac{1}{2}\delta^{pd}Y_e^{ab}Y_u^{cr}(Y_d^\dagger Y_d)^{st}\Big\} \\
& +\Big\{\frac{1}{4}\delta^{rb}Y_e^{*ad}Y_u^{*cp}(Y_d^\dagger Y_d)^{st}-\frac{7}{162}\delta^{rb}\delta^{st}g_Y^2Y_e^{*ad}Y_u^{*cp}-\frac{2}{27}\delta^{rb}\delta^{st}g_s^2Y_e^{*ad}Y_u^{*cp}\Big\}C_{\ell uqe}^{abcd}+C_{\ell uqe}^{*abcd}\Big\{\frac{1}{4}\delta^{pb}Y_e^{ad}Y_u^{cr}(Y_d^\dagger Y_d)^{st}-\frac{7}{162}\delta^{pb}\delta^{st}g_Y^2Y_e^{ad}Y_u^{cr} \\
& -\frac{2}{27}\delta^{pb}\delta^{st}g_s^2Y_e^{ad}Y_u^{cr}\Big\}-\frac{32}{81}\delta^{pr}\delta^{st}\delta^{ad}\delta^{bc}g_Y^4C_{\ell\ell}^{abcd}+\Big\{g_Y^2\Big(\frac{8}{27}\delta^{st}\delta^{bc}Y_u^{*ap}Y_u^{dr}-\frac{16}{27}\delta^{pr}\delta^{bc}Y_d^{*as}Y_d^{dt}\Big)+g_s^2\Big(\frac{8}{9}\delta^{pr}\delta^{bc}Y_d^{*as}Y_d^{dt}+\frac{8}{9}\delta^{st}\delta^{bc}Y_u^{*ap}Y_u^{dr}\Big) \\
& +2Y_d^{*as}Y_u^{*cp}Y_d^{bt}Y_u^{dr}-\frac{32}{243}\delta^{pr}\delta^{st}\delta^{ad}\delta^{bc}g_Y^4-\frac{16}{27}\delta^{pr}\delta^{st}\delta^{ad}\delta^{bc}g_s^4\Big\}C_{qq}^{(\parallel)abcd}+\Big\{g_Y^2\Big(\frac{16}{27}\delta^{st}\delta^{bc}Y_u^{*ap}Y_u^{dr}-\frac{32}{27}\delta^{pr}\delta^{bc}Y_d^{*as}Y_d^{dt}\Big) \\
& +g_s^2\Big(\frac{16}{9}\delta^{pr}\delta^{bc}Y_d^{*as}Y_d^{dt}+\frac{16}{9}\delta^{st}\delta^{bc}Y_u^{*ap}Y_u^{dr}\Big)-\frac{64}{243}\delta^{pr}\delta^{st}\delta^{ad}\delta^{bc}g_Y^4-\frac{32}{27}\delta^{pr}\delta^{st}\delta^{ad}\delta^{bc}g_s^4-2Y_d^{*as}Y_u^{*cp}Y_d^{bt}Y_u^{dr}\Big\}C_{qq}^{(\times)abcd}, \tag{11.12}
\end{aligned}$$

## 11.7 $C_{ud}^{(\times)}$

$$\begin{aligned}
\beta_{C_{ud}^{(\times)prst}}^{(1)} &= 2\delta^{pa}\delta^{tb}C_{Hud}^{ab}(Y_d^\dagger Y_u)^{sr}+2\delta^{ra}\delta^{sb}C_{Hud}^{*ab}(Y_u^\dagger Y_d)^{pt}+\Big\{\frac{4}{3}\delta^{pc}\delta^{rd}\delta^{st}\delta^{ab}g_s^2-2\delta^{pc}\delta^{rd}Y_d^{*as}Y_d^{bt}\Big\}C_{qu}^{(\times)abcd}+\Big\{\frac{4}{3}\delta^{pr}\delta^{sc}\delta^{td}\delta^{ab}g_s^2 \\
& -2\delta^{sc}\delta^{td}Y_u^{*ap}Y_u^{br}\Big\}C_{qd}^{(\times)abcd}+\frac{4}{3}\delta^{pa}\delta^{rd}\delta^{st}\delta^{bc}g_s^2C_{uu}^{abcd}+\frac{4}{3}\delta^{pr}\delta^{sa}\delta^{td}\delta^{bc}g_s^2C_{dd}^{abcd}+6\delta^{pa}\delta^{rb}\delta^{sc}\delta^{td}g_s^2C_{ud}^{(\parallel)abcd}+\Big\{\delta^{pa}\delta^{rb}\delta^{td}(Y_d^\dagger Y_d)^{sc} \\
& +\delta^{pa}\delta^{rb}\delta^{sc}(Y_d^\dagger Y_d)^{dt}+\delta^{rb}\delta^{sc}\delta^{td}(Y_u^\dagger Y_u)^{pa}+\delta^{pa}\delta^{sc}\delta^{td}(Y_u^\dagger Y_u)^{br}-\frac{2}{3}g_s^2\Big(3\delta^{pa}\delta^{rb}\delta^{sc}\delta^{td}-\delta^{pr}\delta^{sc}\delta^{td}\delta^{ab}-\delta^{pa}\delta^{rb}\delta^{st}\delta^{cd}\Big) \\
& -\frac{8}{3}\delta^{pa}\delta^{rb}\delta^{sc}\delta^{td}g_Y^2\Big\}C_{ud}^{(\times)abcd}+\delta^{rb}\delta^{td}Y_d^{*as}Y_u^{*cp}C_{quqd}^{(\parallel)abcd}+\delta^{pb}\delta^{sd}\Big(C_{quqd}^{(\parallel)*}\Big)^{abcd}Y_d^{at}Y_u^{cr}-\delta^{rb}\delta^{td}Y_d^{*cs}Y_u^{*ap}C_{quqd}^{(\times)abcd}-\delta^{pb}\delta^{sd}\Big(C_{quqd}^{(\times)*}\Big)^{abcd}Y_d^{ct}Y_u^{ar}, \tag{11.13}
\end{aligned}$$

$$\begin{aligned}
\beta_{C_{ud}^{(\times)prst}}^{(2)} &= -g_s^4\Big\{4\delta^{pr}(Y_d^\dagger Y_d)^{st}+4\delta^{st}(Y_u^\dagger Y_u)^{pr}\Big\}C_{HG}+\Big\{-g_s^6\Big(9\delta^{pr}(Y_d^\dagger Y_d)^{st}+9\delta^{st}(Y_u^\dagger Y_u)^{pr}\Big)-\frac{29}{3}\delta^{pr}\delta^{st}g_s^8-28\delta^{pr}\delta^{st}g_Y^2g_s^6\Big\}C_G \\
& +\Big\{\frac{20}{9}\delta^{rb}\delta^{st}g_Y^2g_s^2Y_u^{*ap}-3\delta^{rb}g_Y^2Y_d^{*as}(Y_u^\dagger Y_d)^{pt}\Big\}C_{uB}^{ab}+C_{uB}^{*ab}\Big\{\frac{20}{9}\delta^{pb}\delta^{st}g_Y^2g_s^2Y_u^{ar}-3\delta^{pb}g_Y^2Y_d^{at}(Y_d^\dagger Y_u)^{sr}\Big\}+\Big\{\frac{9}{2}\delta^{rb}g_L^2Y_d^{*as}(Y_u^\dagger Y_d)^{pt} \\
& -4\delta^{rb}\delta^{st}g_s^2g_L^2Y_u^{*ap}\Big\}C_{uW}^{ab}+C_{uW}^{*ab}\Big\{\frac{9}{2}\delta^{pb}g_L^2Y_d^{at}(Y_d^\dagger Y_u)^{sr}-4\delta^{pb}\delta^{st}g_s^2g_L^2Y_u^{ar}\Big\}+\Big\{\frac{2}{9}\delta^{rb}\delta^{st}g_Y^2g_s^2Y_u^{*ap}+g_s^4\Big(\frac{4}{3}\delta^{pr}\delta^{st}Y_u^{*ab}+\frac{16}{9}\delta^{rb}\delta^{st}Y_u^{*ap}\Big) \\
& +g_s^2\Big(12\delta^{rb}Y_d^{*as}(Y_u^\dagger Y_d)^{pt}-\delta^{st}Y_u^{*ap}(Y_u^\dagger Y_u)^{br}-6\delta^{rb}Y_u^{*ap}(Y_d^\dagger Y_d)^{st}\Big)\Big\}C_{uG}^{ab}+C_{uG}^{*ab}\Big\{\frac{2}{9}\delta^{pb}\delta^{st}g_Y^2g_s^2Y_u^{ar}+g_s^4\Big(\frac{4}{3}\delta^{pr}\delta^{st}Y_u^{ab}+\frac{16}{9}\delta^{pb}\delta^{st}Y_u^{ar}\Big)
\end{aligned}$$

$$\begin{aligned}
& + g_s^2 \left( 12 \delta^{pb} Y_d^{at} (Y_d^\dagger Y_u)^{sr} - \delta^{st} Y_u^{ar} (Y_u^\dagger Y_u)^{pb} - 6 \delta^{pb} Y_u^{ar} (Y_d^\dagger Y_d)^{st} \right) \Bigg\} + \left\{ 15 \delta^{tb} g_Y^2 Y_u^{*ap} (Y_d^\dagger Y_u)^{sr} - \frac{76}{9} \delta^{pr} \delta^{tb} g_Y^2 g_s^2 Y_d^{*as} \right\} C_{dB}^{ab} \\
& + C_{dB}^{*ab} \left\{ 15 \delta^{sb} g_Y^2 Y_u^{ar} (Y_u^\dagger Y_d)^{pt} - \frac{76}{9} \delta^{pr} \delta^{sb} g_Y^2 g_s^2 Y_d^{at} \right\} + \left\{ \frac{9}{2} \delta^{tb} g_L^2 Y_u^{*ap} (Y_d^\dagger Y_u)^{sr} - 4 \delta^{pr} \delta^{tb} g_s^2 g_L^2 Y_d^{*as} \right\} C_{dW}^{ab} + C_{dW}^{*ab} \left\{ \frac{9}{2} \delta^{sb} g_L^2 Y_u^{ar} (Y_u^\dagger Y_d)^{pt} \right. \\
& - 4 \delta^{pr} \delta^{sb} g_s^2 g_L^2 Y_d^{at} \Bigg\} + \left\{ g_s^4 \left( \frac{4}{3} \delta^{pr} \delta^{st} Y_d^{*ab} + \frac{16}{9} \delta^{pr} \delta^{tb} Y_d^{*as} \right) + g_s^2 \left( 12 \delta^{tb} Y_u^{*ap} (Y_d^\dagger Y_u)^{sr} - \delta^{pr} Y_d^{*as} (Y_d^\dagger Y_d)^{bt} - 6 \delta^{tb} Y_d^{*as} (Y_u^\dagger Y_u)^{pr} \right) \right. \\
& - \frac{10}{9} \delta^{pr} \delta^{tb} g_Y^2 g_s^2 Y_d^{*as} \Bigg\} C_{dG}^{ab} + C_{dG}^{*ab} \left\{ g_s^4 \left( \frac{4}{3} \delta^{pr} \delta^{st} Y_d^{ab} + \frac{16}{9} \delta^{pr} \delta^{sb} Y_d^{at} \right) + g_s^2 \left( 12 \delta^{sb} Y_u^{ar} (Y_u^\dagger Y_d)^{pt} - \delta^{pr} Y_d^{at} (Y_d^\dagger Y_d)^{sb} - 6 \delta^{sb} Y_d^{at} (Y_u^\dagger Y_u)^{pr} \right) \right. \\
& - \frac{10}{9} \delta^{pr} \delta^{sb} g_Y^2 g_s^2 Y_d^{at} \Bigg\} + \left\{ g_s^2 \left( \frac{7}{9} \delta^{rb} \delta^{st} (Y_u^\dagger Y_u)^{pa} + \frac{7}{9} \delta^{pa} \delta^{st} (Y_u^\dagger Y_u)^{br} - 7 \delta^{pa} \delta^{rb} (Y_d^\dagger Y_d)^{st} \right) + 3 \delta^{rb} (Y_d^\dagger Y_u)^{sa} (Y_u^\dagger Y_d)^{pt} + 3 \delta^{pa} (Y_d^\dagger Y_u)^{sr} (Y_u^\dagger Y_d)^{bt} \right. \\
& - \frac{47}{81} \delta^{pa} \delta^{rb} \delta^{st} g_Y^2 g_s^2 \Bigg\} C_{Hu}^{ab} + \left\{ g_s^2 \left( 7 \delta^{sa} \delta^{tb} (Y_u^\dagger Y_u)^{pr} - \frac{7}{9} \delta^{pr} \delta^{tb} (Y_d^\dagger Y_d)^{sa} - \frac{7}{9} \delta^{pr} \delta^{sa} (Y_d^\dagger Y_d)^{bt} \right) - \frac{44}{81} \delta^{pr} \delta^{sa} \delta^{tb} g_Y^2 g_s^2 - 3 \delta^{sa} (Y_d^\dagger Y_u)^{br} (Y_u^\dagger Y_d)^{pt} \right. \\
& - 3 \delta^{tb} (Y_d^\dagger Y_u)^{sr} (Y_u^\dagger Y_d)^{pa} \Bigg\} C_{Hd}^{ab} + \left\{ \frac{77}{36} \delta^{pa} \delta^{tb} g_Y^2 (Y_d^\dagger Y_u)^{sr} + \frac{51}{4} \delta^{pa} \delta^{tb} g_L^2 (Y_d^\dagger Y_u)^{sr} - \delta^{pa} (Y_d^\dagger Y_d)^{bt} (Y_d^\dagger Y_u)^{sr} - g_s^2 \left( \frac{1}{9} \delta^{pr} \delta^{tb} (Y_d^\dagger Y_u)^{sa} + \frac{1}{9} \delta^{pa} \delta^{st} (Y_d^\dagger Y_u)^{br} \right) \right. \\
& + \frac{25}{3} \delta^{pa} \delta^{tb} (Y_d^\dagger Y_u)^{sr} - \delta^{tb} (Y_d^\dagger Y_u)^{sr} (Y_u^\dagger Y_u)^{pa} - \frac{3}{2} \delta^{pa} \delta^{tb} (Y_d^\dagger Y_d Y_d^\dagger Y_u)^{sr} - \frac{3}{2} \delta^{pa} \delta^{tb} (Y_d^\dagger Y_u Y_u^\dagger Y_u)^{sr} - 2 T_2 \delta^{pa} \delta^{tb} (Y_d^\dagger Y_u)^{sr} \Bigg\} C_{Hud}^{ab} \\
& + C_{Hud}^{*ab} \left\{ \frac{77}{36} \delta^{ra} \delta^{sb} g_Y^2 (Y_u^\dagger Y_d)^{pt} + \frac{51}{4} \delta^{ra} \delta^{sb} g_L^2 (Y_u^\dagger Y_d)^{pt} - \delta^{ra} (Y_d^\dagger Y_d)^{sb} (Y_u^\dagger Y_d)^{pt} - g_s^2 \left( \frac{1}{9} \delta^{ra} \delta^{st} (Y_u^\dagger Y_d)^{pb} + \frac{1}{9} \delta^{pr} \delta^{sb} (Y_u^\dagger Y_d)^{at} + \frac{25}{3} \delta^{ra} \delta^{sb} (Y_u^\dagger Y_d)^{pt} \right) \right. \\
& - \delta^{sb} (Y_u^\dagger Y_d)^{pt} (Y_u^\dagger Y_u)^{ar} - \frac{3}{2} \delta^{ra} \delta^{sb} (Y_u^\dagger Y_d Y_d^\dagger Y_d)^{pt} - \frac{3}{2} \delta^{ra} \delta^{sb} (Y_u^\dagger Y_u Y_u^\dagger Y_d)^{pt} - 2 T_2 \delta^{ra} \delta^{sb} (Y_u^\dagger Y_d)^{pt} \Bigg\} + \frac{154}{81} \delta^{pc} \delta^{rd} \delta^{st} \delta^{ab} g_Y^2 g_s^2 C_{\ell u}^{abcd} \\
& - \frac{104}{81} \delta^{pr} \delta^{sc} \delta^{td} \delta^{ab} g_Y^2 g_s^2 C_{\ell d}^{abcd} + \left\{ 2 \delta^{pc} Y_u^{*ad} Y_d^{bt} (Y_d^\dagger Y_u)^{sr} + 2 \delta^{rd} Y_d^{*as} Y_u^{bc} (Y_u^\dagger Y_d)^{pt} + 4 \delta^{rd} Y_u^{*ap} Y_d^{bt} (Y_d^\dagger Y_u)^{sc} + 4 \delta^{pc} Y_d^{*as} Y_u^{br} (Y_u^\dagger Y_d)^{dt} \right. \\
& - g_s^2 \left( \frac{8}{9} \delta^{pc} \delta^{st} Y_u^{*ad} Y_u^{br} + \frac{8}{9} \delta^{rd} \delta^{st} Y_u^{*ap} Y_u^{bc} + 4 \delta^{pc} \delta^{rd} Y_d^{*as} Y_d^{bt} \right) - \frac{154}{81} \delta^{pc} \delta^{rd} \delta^{st} \delta^{ab} g_Y^2 g_s^2 - \frac{22}{3} \delta^{pc} \delta^{rd} \delta^{st} \delta^{ab} g_s^4 \Bigg\} C_{qu}^{(II)abcd} \\
& + \left\{ \frac{1}{2} \delta^{pc} \delta^{rd} Y_d^{bt} (Y_u^\dagger Y_u Y_d^\dagger)^{as} + \frac{1}{2} \delta^{pc} \delta^{rd} Y_d^{*as} (Y_u Y_u^\dagger Y_d)^{bt} + g_s^4 \left( \frac{104}{81} \delta^{pc} \delta^{rd} \delta^{st} \delta^{ab} - \frac{4}{9} \delta^{pr} \delta^{st} \delta^{ab} \delta^{cd} \right) + g_s^2 \left( \frac{2}{3} \delta^{st} \delta^{cd} Y_u^{*ap} Y_u^{br} - \frac{2}{3} \delta^{pc} \delta^{st} Y_u^{*ad} Y_u^{br} \right. \right. \\
& - \frac{2}{3} \delta^{rd} \delta^{st} Y_u^{*ap} Y_u^{bc} - \frac{4}{3} \delta^{pc} \delta^{rd} \delta^{st} (Y_u Y_u^\dagger)^{ba} - 2 \delta^{pc} \delta^{rd} \delta^{st} (Y_d Y_d^\dagger)^{ba} - 12 \delta^{pc} \delta^{rd} Y_d^{*as} Y_d^{bt} \Bigg\} + \frac{3}{2} \delta^{pc} \delta^{rd} Y_d^{bt} (Y_d^\dagger Y_d Y_d^\dagger)^{as} + \frac{3}{2} \delta^{pc} \delta^{rd} Y_d^{*as} (Y_d Y_d^\dagger Y_d)^{bt}
\end{aligned}$$

$$\begin{aligned}
& + 3T_2\delta^{pc}\delta^{rd}Y_d^{*as}Y_d^{bt} + 3\delta^{pc}\delta^{rd}\delta^{st}\delta^{ab}g_s^2g_L^2 + 6\delta^{pc}Y_u^{*ad}Y_d^{bt}(Y_d^\dagger Y_u)^{sr} + 6\delta^{rd}Y_d^{*as}Y_u^{bc}(Y_u^\dagger Y_d)^{pt} - \frac{1}{2}\delta^{rd}Y_d^{*as}Y_d^{bt}(Y_u^\dagger Y_u)^{pc} - \frac{1}{2}\delta^{pc}Y_d^{*as}Y_d^{bt}(Y_u^\dagger Y_u)^{dr} \\
& - \frac{271}{243}\delta^{pc}\delta^{rd}\delta^{st}\delta^{ab}g_Y^2g_s^2 - \frac{5}{4}\delta^{pc}\delta^{rd}g_Y^2Y_d^{*as}Y_d^{bt} - \frac{51}{4}\delta^{pc}\delta^{rd}g_L^2Y_d^{*as}Y_d^{bt} \Big\} C_{qu}^{(\times)abcd} + \Big\{ \frac{104}{81}\delta^{pr}\delta^{sc}\delta^{td}\delta^{ab}g_Y^2g_s^2 + 2\delta^{td}Y_u^{*ap}Y_d^{bc}(Y_d^\dagger Y_u)^{sr} \\
& + 2\delta^{sc}Y_d^{*ad}Y_u^{br}(Y_u^\dagger Y_d)^{pt} + 4\delta^{sc}Y_u^{*ap}Y_d^{bt}(Y_d^\dagger Y_u)^{dr} + 4\delta^{td}Y_d^{*as}Y_u^{br}(Y_u^\dagger Y_d)^{pc} - g_s^2\Big(\frac{8}{9}\delta^{pr}\delta^{sc}Y_d^{*ad}Y_d^{bt} + \frac{8}{9}\delta^{pr}\delta^{td}Y_d^{*as}Y_d^{bc} + 4\delta^{sc}\delta^{td}Y_u^{*ap}Y_u^{br}\Big) \\
& - \frac{22}{3}\delta^{pr}\delta^{sc}\delta^{td}\delta^{ab}g_s^4 \Big\} C_{qd}^{(\parallel)abcd} + \Big\{ \frac{1}{2}\delta^{sc}\delta^{td}Y_u^{br}(Y_d^\dagger Y_d Y_u^\dagger)^{ap} + \frac{1}{2}\delta^{sc}\delta^{td}Y_u^{*ap}(Y_d Y_d^\dagger Y_u)^{br} + \frac{3}{4}\delta^{sc}\delta^{td}g_Y^2Y_u^{*ap}Y_u^{br} + g_s^4\Big(\frac{104}{81}\delta^{pr}\delta^{sc}\delta^{td}\delta^{ab} \\
& - \frac{4}{9}\delta^{pr}\delta^{st}\delta^{ab}\delta^{cd}\Big) + g_s^2\Big(\frac{2}{3}\delta^{pr}\delta^{cd}Y_d^{*as}Y_d^{bt} - \frac{2}{3}\delta^{pr}\delta^{sc}Y_d^{*ad}Y_d^{bt} - \frac{2}{3}\delta^{pr}\delta^{td}Y_d^{*as}Y_d^{bc} - \frac{4}{3}\delta^{pr}\delta^{sc}\delta^{td}(Y_d Y_d^\dagger)^{ba} - 2\delta^{pr}\delta^{sc}\delta^{td}(Y_u Y_u^\dagger)^{ba} - 12\delta^{sc}\delta^{td}Y_u^{*ap}Y_u^{br}\Big) \\
& + \frac{3}{2}\delta^{sc}\delta^{td}Y_u^{br}(Y_u^\dagger Y_u Y_u^\dagger)^{ap} + \frac{3}{2}\delta^{sc}\delta^{td}Y_u^{*ap}(Y_u Y_u^\dagger Y_u)^{br} + 3T_2\delta^{sc}\delta^{td}Y_u^{*ap}Y_u^{br} + 3\delta^{pr}\delta^{sc}\delta^{td}\delta^{ab}g_s^2g_L^2 + 6\delta^{td}Y_u^{*ap}Y_d^{bc}(Y_d^\dagger Y_u)^{sr} \\
& + 6\delta^{sc}Y_d^{*ad}Y_u^{br}(Y_u^\dagger Y_d)^{pt} - \frac{1}{2}\delta^{td}Y_u^{*ap}Y_u^{br}(Y_d^\dagger Y_d)^{sc} - \frac{1}{2}\delta^{sc}Y_u^{*ap}Y_u^{br}(Y_d^\dagger Y_d)^{dt} - \frac{391}{243}\delta^{pr}\delta^{sc}\delta^{td}\delta^{ab}g_Y^2g_s^2 - \frac{51}{4}\delta^{sc}\delta^{td}g_L^2Y_u^{*ap}Y_u^{br} \Big\} C_{qd}^{(\times)abcd} \\
& + \Big\{ g_s^4\Big(\frac{4}{9}\delta^{pr}\delta^{st}\delta^{ad}\delta^{bc} + \frac{2600}{81}\delta^{pa}\delta^{rd}\delta^{st}\delta^{bc} - \frac{14}{3}\delta^{pa}\delta^{rb}\delta^{st}\delta^{cd}\Big) + \delta^{pa}\delta^{rd}(Y_d^\dagger Y_u)^{sc}(Y_u^\dagger Y_d)^{bt} - g_Y^2g_s^2\Big(\frac{616}{81}\delta^{pa}\delta^{rb}\delta^{st}\delta^{cd} + \frac{3232}{243}\delta^{pa}\delta^{rd}\delta^{st}\delta^{bc}\Big) \\
& - \frac{20}{3}\delta^{pa}\delta^{rd}\delta^{st}g_s^2(Y_u^\dagger Y_u)^{bc} \Big\} C_{uu}^{abcd} + \Big\{ g_s^4\Big(\frac{4}{9}\delta^{pr}\delta^{st}\delta^{ad}\delta^{bc} + \frac{2600}{81}\delta^{pr}\delta^{sa}\delta^{td}\delta^{bc} - \frac{14}{3}\delta^{pr}\delta^{sa}\delta^{tb}\delta^{cd}\Big) + \delta^{sa}\delta^{td}(Y_d^\dagger Y_u)^{br}(Y_u^\dagger Y_d)^{pc} \\
& - g_Y^2g_s^2\Big(\frac{208}{81}\delta^{pr}\delta^{sa}\delta^{tb}\delta^{cd} + \frac{2536}{243}\delta^{pr}\delta^{sa}\delta^{td}\delta^{bc}\Big) - \frac{20}{3}\delta^{pr}\delta^{sa}\delta^{td}g_s^2(Y_d^\dagger Y_d)^{bc} \Big\} C_{dd}^{abcd} + \frac{154}{81}\delta^{pc}\delta^{rd}\delta^{st}\delta^{ab}g_Y^2g_s^2 C_{eu}^{abcd} \\
& - \frac{104}{81}\delta^{pr}\delta^{sc}\delta^{td}\delta^{ab}g_Y^2g_s^2 C_{ed}^{abcd} + \Big\{ g_s^4\Big(\frac{15}{2}\delta^{pa}\delta^{rb}\delta^{sc}\delta^{td} - \frac{1}{3}\delta^{pr}\delta^{sc}\delta^{td}\delta^{ab} - \frac{1}{3}\delta^{pa}\delta^{rb}\delta^{st}\delta^{cd}\Big) + g_Y^2g_s^2\Big(\frac{154}{81}\delta^{pa}\delta^{rb}\delta^{st}\delta^{cd} + \frac{208}{81}\delta^{pr}\delta^{sc}\delta^{td}\delta^{ab} \\
& - \frac{2}{3}\delta^{pa}\delta^{rb}\delta^{sc}\delta^{td}\Big) + 6\delta^{rb}\delta^{sc}(Y_d^\dagger Y_u)^{da}(Y_u^\dagger Y_d)^{pt} + 6\delta^{pa}\delta^{td}(Y_d^\dagger Y_u)^{sr}(Y_u^\dagger Y_d)^{bc} + \frac{15}{2}\delta^{rb}\delta^{td}(Y_d^\dagger Y_u)^{sa}(Y_u^\dagger Y_d)^{pc} + \frac{15}{2}\delta^{pa}\delta^{sc}(Y_d^\dagger Y_u)^{dr}(Y_u^\dagger Y_d)^{bt} \\
& - g_s^2\Big(6\delta^{pa}\delta^{rb}\delta^{td}(Y_d^\dagger Y_d)^{sc} + 6\delta^{pa}\delta^{rb}\delta^{sc}(Y_d^\dagger Y_d)^{dt} + 6\delta^{rb}\delta^{sc}\delta^{td}(Y_u^\dagger Y_u)^{pa} + 6\delta^{pa}\delta^{sc}\delta^{td}(Y_u^\dagger Y_u)^{br}\Big) \Big\} C_{ud}^{(\parallel)abcd} + \Big\{ g_Y^2g_s^2\Big(\frac{532}{243}\delta^{pa}\delta^{rb}\delta^{st}\delta^{cd} \\
& + \frac{1720}{243}\delta^{pr}\delta^{sc}\delta^{td}\delta^{ab} - \frac{49}{9}\delta^{pa}\delta^{rb}\delta^{sc}\delta^{td}\Big) + g_s^4\Big(\frac{772}{81}\delta^{pr}\delta^{sc}\delta^{td}\delta^{ab} + \frac{772}{81}\delta^{pa}\delta^{rb}\delta^{st}\delta^{cd} - \frac{4}{9}\delta^{pr}\delta^{st}\delta^{ab}\delta^{cd} - \frac{71}{6}\delta^{pa}\delta^{rb}\delta^{sc}\delta^{td}\Big) \\
& + g_Y^2\Big(\frac{37}{72}\delta^{pa}\delta^{rb}\delta^{td}(Y_d^\dagger Y_d)^{sc} + \frac{37}{72}\delta^{pa}\delta^{rb}\delta^{sc}(Y_d^\dagger Y_d)^{dt} + \frac{97}{72}\delta^{rb}\delta^{sc}\delta^{td}(Y_u^\dagger Y_u)^{pa} + \frac{97}{72}\delta^{pa}\delta^{sc}\delta^{td}(Y_u^\dagger Y_u)^{br}\Big) + g_L^2\Big(\frac{51}{8}\delta^{pa}\delta^{rb}\delta^{td}(Y_d^\dagger Y_d)^{sc} \\
& + \frac{51}{8}\delta^{pa}\delta^{rb}\delta^{sc}(Y_d^\dagger Y_d)^{dt} + \frac{51}{8}\delta^{rb}\delta^{sc}\delta^{td}(Y_u^\dagger Y_u)^{pa} + \frac{51}{8}\delta^{pa}\delta^{sc}\delta^{td}(Y_u^\dagger Y_u)^{br}\Big) + 18\delta^{rb}\delta^{sc}(Y_d^\dagger Y_u)^{da}(Y_u^\dagger Y_d)^{pt} + 18\delta^{pa}\delta^{td}(Y_d^\dagger Y_u)^{sr}(Y_u^\dagger Y_d)^{bc}
\end{aligned}$$

$$\begin{aligned}
& -\frac{2}{9}\delta^{pa}\delta^{rb}\delta^{sc}\delta^{td}g_Y^4 - \frac{1}{4}\delta^{pa}\delta^{rb}\delta^{td}(Y_d^\dagger Y_d Y_d^\dagger Y_d)^{sc} - \frac{1}{4}\delta^{pa}\delta^{rb}\delta^{sc}(Y_d^\dagger Y_d Y_d^\dagger Y_d)^{dt} - \frac{1}{4}\delta^{pa}\delta^{rb}\delta^{td}(Y_d^\dagger Y_u Y_u^\dagger Y_d)^{sc} - \frac{1}{4}\delta^{pa}\delta^{rb}\delta^{sc}(Y_d^\dagger Y_u Y_u^\dagger Y_d)^{dt} \\
& - \frac{1}{4}\delta^{rb}\delta^{sc}\delta^{td}(Y_u^\dagger Y_d Y_d^\dagger Y_u)^{pa} - \frac{1}{4}\delta^{pa}\delta^{sc}\delta^{td}(Y_u^\dagger Y_d Y_d^\dagger Y_u)^{br} - \frac{1}{4}\delta^{rb}\delta^{sc}\delta^{td}(Y_u^\dagger Y_u Y_u^\dagger Y_u)^{pa} - \frac{1}{4}\delta^{pa}\delta^{sc}\delta^{td}(Y_u^\dagger Y_u Y_u^\dagger Y_u)^{br} - g_s^2\left(2\delta^{pa}\delta^{rb}\delta^{sc}(Y_d^\dagger Y_d)^{dc}\right. \\
& + 2\delta^{pr}\delta^{sc}\delta^{td}(Y_u^\dagger Y_u)^{ba} + \frac{10}{3}\delta^{pa}\delta^{rb}\delta^{td}(Y_d^\dagger Y_d)^{sc} + \frac{10}{3}\delta^{pa}\delta^{rb}\delta^{sc}(Y_d^\dagger Y_d)^{dt} + \frac{10}{3}\delta^{rb}\delta^{sc}\delta^{td}(Y_u^\dagger Y_u)^{pa} + \frac{10}{3}\delta^{pa}\delta^{sc}\delta^{td}(Y_u^\dagger Y_u)^{br}) \\
& - \frac{3}{2}\text{T}_2\delta^{pa}\delta^{rb}\delta^{td}(Y_d^\dagger Y_d)^{sc} - \frac{3}{2}\text{T}_2\delta^{pa}\delta^{rb}\delta^{sc}(Y_d^\dagger Y_d)^{dt} - \frac{3}{2}\text{T}_2\delta^{rb}\delta^{sc}\delta^{td}(Y_u^\dagger Y_u)^{pa} - \frac{3}{2}\text{T}_2\delta^{pa}\delta^{sc}\delta^{td}(Y_u^\dagger Y_u)^{br} - 2\delta^{rb}\delta^{sc}(Y_d^\dagger Y_d)^{dt}(Y_u^\dagger Y_u)^{pa} \\
& - 2\delta^{pa}\delta^{td}(Y_d^\dagger Y_d)^{sc}(Y_u^\dagger Y_u)^{br} - \frac{5}{2}\delta^{pa}\delta^{rb}(Y_d^\dagger Y_d)^{sc}(Y_d^\dagger Y_d)^{dt} - \frac{5}{2}\delta^{sc}\delta^{td}(Y_u^\dagger Y_u)^{pa}(Y_u^\dagger Y_u)^{br} - \frac{7}{2}\delta^{rb}\delta^{td}(Y_d^\dagger Y_d)^{sc}(Y_u^\dagger Y_u)^{pa} - \frac{7}{2}\delta^{pa}\delta^{sc}(Y_d^\dagger Y_d)^{dt}(Y_u^\dagger Y_u)^{br} \Big\} C_{ud}^{(\times)abcd} \\
& + \left\{ \frac{4}{9}\delta^{pr}\delta^{sc}g_s^2Y_e^{*ab}Y_d^{dt} - 2\delta^{sc}Y_e^{*ab}Y_u^{dr}(Y_u^\dagger Y_d)^{pt} \right\} C_{ledq}^{abcd} + C_{ledq}^{*abcd} \left\{ \frac{4}{9}\delta^{pr}\delta^{tc}g_s^2Y_d^{*ds}Y_e^{ab} - 2\delta^{tc}Y_u^{*dp}Y_e^{ab}(Y_d^\dagger Y_u)^{sr} \right\} + \left\{ \frac{7}{24}\delta^{rb}\delta^{td}g_Y^2Y_d^{*as}Y_u^{*cp} \right. \\
& + \frac{1}{2}\delta^{rb}Y_d^{*as}Y_u^{*cp}(Y_d^\dagger Y_d)^{dt} + \frac{1}{2}\delta^{td}Y_d^{*as}Y_u^{*cp}(Y_u^\dagger Y_u)^{br} + g_s^2\left(\frac{2}{9}\delta^{rb}\delta^{st}Y_d^{*ad}Y_u^{*cp} + \frac{2}{9}\delta^{pr}\delta^{td}Y_d^{*as}Y_u^{*cb} + \frac{4}{3}\delta^{rb}\delta^{st}Y_d^{*cd}Y_u^{*ap} + \frac{4}{3}\delta^{pr}\delta^{td}Y_d^{*cs}Y_u^{*ab} \right. \\
& + \frac{13}{2}\delta^{rb}\delta^{td}Y_d^{*cs}Y_u^{*ap} - \frac{17}{2}\delta^{rb}\delta^{td}Y_d^{*as}Y_u^{*cp}) + \frac{51}{8}\delta^{rb}\delta^{td}g_L^2Y_d^{*as}Y_u^{*cp} - \frac{1}{4}\delta^{rb}\delta^{td}Y_u^{*cp}(Y_d^\dagger Y_d Y_d^\dagger)^{as} - \frac{1}{4}\delta^{rb}\delta^{td}Y_d^{*as}(Y_u^\dagger Y_u Y_u^\dagger)^{cp} \\
& - \frac{1}{2}\text{T}_2\delta^{rb}\delta^{td}Y_d^{*as}Y_u^{*cp} - \frac{3}{4}\delta^{rb}\delta^{td}Y_d^{*as}(Y_d^\dagger Y_d Y_u^\dagger)^{cp} - \frac{3}{4}\delta^{rb}\delta^{td}Y_u^{*cp}(Y_u^\dagger Y_u Y_d^\dagger)^{as} - \delta^{td}Y_u^{*ap}Y_u^{*cb}(Y_d^\dagger Y_u)^{sr} - \delta^{rb}Y_d^{*ad}Y_d^{*cs}(Y_u^\dagger Y_d)^{pt} \\
& - 6\delta^{td}Y_u^{*ab}Y_u^{*cp}(Y_d^\dagger Y_u)^{sr} - 6\delta^{rb}Y_d^{*as}Y_d^{*cd}(Y_u^\dagger Y_d)^{pt} \Big\} C_{quqd}^{(\parallel)abcd} + \left( C_{quqd}^{(\parallel)*} \right)^{abcd} \left\{ \frac{7}{24}\delta^{pb}\delta^{sd}g_Y^2Y_d^{at}Y_u^{cr} + \frac{1}{2}\delta^{pb}Y_d^{at}Y_u^{cr}(Y_d^\dagger Y_d)^{sd} + \frac{1}{2}\delta^{sd}Y_d^{at}Y_u^{cr}(Y_u^\dagger Y_u)^{pb} \right. \\
& + g_s^2\left(\frac{2}{9}\delta^{pb}\delta^{st}Y_d^{ad}Y_u^{cr} + \frac{2}{9}\delta^{pr}\delta^{sd}Y_d^{at}Y_u^{cb} + \frac{4}{3}\delta^{pb}\delta^{st}Y_d^{cd}Y_u^{ar} + \frac{4}{3}\delta^{pr}\delta^{sd}Y_d^{ct}Y_u^{ab} + \frac{13}{2}\delta^{pb}\delta^{sd}Y_d^{ct}Y_u^{ar} - \frac{17}{2}\delta^{pb}\delta^{sd}Y_d^{at}Y_u^{cr} \right) + \frac{51}{8}\delta^{pb}\delta^{sd}g_L^2Y_d^{at}Y_u^{cr} \\
& - \frac{1}{4}\delta^{pb}\delta^{sd}Y_u^{cr}(Y_d Y_d^\dagger Y_d)^{at} - \frac{1}{4}\delta^{pb}\delta^{sd}Y_d^{at}(Y_u Y_u^\dagger Y_u)^{cr} - \frac{1}{2}\text{T}_2\delta^{pb}\delta^{sd}Y_d^{at}Y_u^{cr} - \frac{3}{4}\delta^{pb}\delta^{sd}Y_d^{at}(Y_d Y_d^\dagger Y_u)^{cr} - \frac{3}{4}\delta^{pb}\delta^{sd}Y_u^{cr}(Y_u Y_u^\dagger Y_d)^{at} \\
& - \delta^{pb}Y_d^{ad}Y_d^{ct}(Y_d^\dagger Y_u)^{sr} - \delta^{sd}Y_u^{ar}Y_u^{cb}(Y_u^\dagger Y_d)^{pt} - 6\delta^{pb}Y_d^{at}Y_d^{cd}(Y_d^\dagger Y_u)^{sr} - 6\delta^{sd}Y_u^{ab}Y_u^{cr}(Y_u^\dagger Y_d)^{pt} \Big\} + \left\{ \frac{1}{4}\delta^{rb}\delta^{td}Y_u^{*ap}(Y_d^\dagger Y_d Y_d^\dagger)^{cs} + \frac{1}{4}\delta^{rb}\delta^{td}Y_d^{*cs}(Y_u^\dagger Y_u Y_u^\dagger)^{ap} \right. \\
& + \frac{1}{2}\text{T}_2\delta^{rb}\delta^{td}Y_d^{*cs}Y_u^{*ap} + \frac{3}{4}\delta^{rb}\delta^{td}Y_d^{*cs}(Y_d^\dagger Y_d Y_u^\dagger)^{ap} + \frac{3}{4}\delta^{rb}\delta^{td}Y_u^{*ap}(Y_u^\dagger Y_u Y_d^\dagger)^{cs} + g_s^2\left(\frac{4}{9}\delta^{rb}\delta^{st}Y_d^{*cd}Y_u^{*ap} + \frac{4}{9}\delta^{pr}\delta^{td}Y_d^{*cs}Y_u^{*ab} \right. \\
& + \frac{2}{3}\delta^{rb}\delta^{st}Y_d^{*ad}Y_u^{*cp} + \frac{2}{3}\delta^{pr}\delta^{td}Y_d^{*as}Y_u^{*cb} + 7\delta^{rb}\delta^{td}Y_d^{*cs}Y_u^{*ap} - 7\delta^{rb}\delta^{td}Y_d^{*as}Y_u^{*cp}) + \frac{5}{4}\delta^{rb}Y_d^{*cs}Y_u^{*ap}(Y_d^\dagger Y_d)^{dt} + \frac{5}{4}\delta^{td}Y_d^{*cs}Y_u^{*ap}(Y_u^\dagger Y_u)^{br} \\
& - \frac{7}{24}\delta^{rb}\delta^{td}g_Y^2Y_d^{*cs}Y_u^{*ap} - 2\delta^{td}Y_u^{*ab}Y_u^{*cp}(Y_d^\dagger Y_u)^{sr} - 2\delta^{rb}Y_d^{*as}Y_d^{*cd}(Y_u^\dagger Y_d)^{pt} - 3\delta^{td}Y_u^{*ap}Y_u^{*cb}(Y_d^\dagger Y_u)^{sr} - 3\delta^{rb}Y_d^{*ad}Y_d^{*cs}(Y_u^\dagger Y_d)^{pt} \\
& - \frac{51}{8}\delta^{rb}\delta^{td}g_L^2Y_d^{*cs}Y_u^{*ap} \Big\} C_{quqd}^{(\times)abcd} + \left( C_{quqd}^{(\times)*} \right)^{abcd} \left\{ \frac{1}{4}\delta^{pb}\delta^{sd}Y_u^{ar}(Y_d Y_d^\dagger Y_d)^{ct} + \frac{1}{4}\delta^{pb}\delta^{sd}Y_d^{ct}(Y_u Y_u^\dagger Y_u)^{ar} + \frac{1}{2}\text{T}_2\delta^{pb}\delta^{sd}Y_d^{ct}Y_u^{ar} + \frac{3}{4}\delta^{pb}\delta^{sd}Y_d^{ct}(Y_d Y_d^\dagger Y_u)^{ar} \right.
\end{aligned}$$

$$\begin{aligned}
& + \frac{3}{4} \delta^{pb} \delta^{sd} Y_u^{ar} (Y_u Y_u^\dagger Y_d)^{ct} + g_s^2 \left( \frac{4}{9} \delta^{pb} \delta^{st} Y_d^{cd} Y_u^{ar} + \frac{4}{9} \delta^{pr} \delta^{sd} Y_d^{ct} Y_u^{ab} + \frac{2}{3} \delta^{pb} \delta^{st} Y_d^{ad} Y_u^{cr} + \frac{2}{3} \delta^{pr} \delta^{sd} Y_d^{at} Y_u^{cb} + 7 \delta^{pb} \delta^{sd} Y_d^{ct} Y_u^{ar} - 7 \delta^{pb} \delta^{sd} Y_d^{at} Y_u^{cr} \right) \\
& + \frac{5}{4} \delta^{pb} Y_d^{ct} Y_u^{ar} (Y_d^\dagger Y_d)^{sd} + \frac{5}{4} \delta^{sd} Y_d^{ct} Y_u^{ar} (Y_u^\dagger Y_u)^{pb} - \frac{7}{24} \delta^{pb} \delta^{sd} g_Y^2 Y_d^{ct} Y_u^{ar} - 2 \delta^{pb} Y_d^{at} Y_d^{cd} (Y_d^\dagger Y_u)^{sr} - 2 \delta^{sd} Y_u^{ab} Y_u^{cr} (Y_u^\dagger Y_d)^{pt} - 3 \delta^{pb} Y_d^{ad} Y_d^{ct} (Y_d^\dagger Y_u)^{sr} \\
& - 3 \delta^{sd} Y_u^{ar} Y_u^{cb} (Y_u^\dagger Y_d)^{pt} - \frac{51}{8} \delta^{pb} \delta^{sd} g_L^2 Y_d^{ct} Y_u^{ar} \Bigg\} + \left\{ 2 \delta^{rd} Y_d^{*cs} Y_e^{*ab} (Y_u^\dagger Y_d)^{pt} - \frac{4}{9} \delta^{rd} \delta^{st} g_s^2 Y_e^{*ab} Y_u^{*cp} \right\} C_{\ell equ}^{abcd} + C_{\ell equ}^{*abcd} \left\{ 2 \delta^{pd} Y_d^{ct} Y_e^{ab} (Y_d^\dagger Y_u)^{sr} \right. \\
& - \frac{4}{9} \delta^{pd} \delta^{st} g_s^2 Y_e^{ab} Y_u^{cr} \Bigg\} + \left\{ \frac{2}{9} \delta^{rb} \delta^{st} g_s^2 Y_e^{*ad} Y_u^{*cp} - \delta^{rb} Y_d^{*cs} Y_e^{*ad} (Y_u^\dagger Y_d)^{pt} \right\} C_{\ell uqe}^{abcd} + C_{\ell uqe}^{*abcd} \left\{ \frac{2}{9} \delta^{pb} \delta^{st} g_s^2 Y_e^{ad} Y_u^{cr} - \delta^{pb} Y_d^{ct} Y_e^{ad} (Y_d^\dagger Y_u)^{sr} \right\} \\
& + \left\{ \frac{16}{9} \delta^{pr} \delta^{st} \delta^{ad} \delta^{bc} g_s^4 + 2 Y_d^{*as} Y_u^{*cp} Y_d^{dt} Y_u^{br} - g_s^2 \left( \frac{8}{3} \delta^{pr} \delta^{bc} Y_d^{*as} Y_d^{dt} + \frac{8}{3} \delta^{st} \delta^{bc} Y_u^{*ap} Y_u^{dr} \right) \right\} C_{qq}^{(\parallel)abcd} + \left\{ \frac{32}{9} \delta^{pr} \delta^{st} \delta^{ad} \delta^{bc} g_s^4 + 10 Y_d^{*as} Y_u^{*cp} Y_d^{dt} Y_u^{br} \right. \\
& \left. - g_s^2 \left( \frac{16}{3} \delta^{pr} \delta^{bc} Y_d^{*as} Y_d^{dt} + \frac{16}{3} \delta^{st} \delta^{bc} Y_u^{*ap} Y_u^{dr} \right) \right\} C_{qq}^{(\times)abcd}, \tag{11.14}
\end{aligned}$$



## 12 $(\bar{L}R)(\bar{R}L)$ and $(\bar{L}R)(\bar{L}R)$

### 12.1 $C_{\ell edq}$

$$\begin{aligned}
\beta_{C_{\ell edq}^{prst}}^{(1)} = & -4\delta^{pa}\delta^{rd}Y_d^{*ts}C_{\ell e}^{abcd}Y_e^{bc} - 2\delta^{pa}\delta^{sc}Y_d^{*td}C_{\ell d}^{abcd}Y_e^{br} - 2\delta^{rd}\delta^{tb}Y_d^{*as}C_{qe}^{abcd}Y_e^{pc} - 4\delta^{sc}\delta^{tb}Y_d^{*ad}C_{qd}^{(\parallel)abcd}Y_e^{pr} - 12\delta^{sc}\delta^{tb}Y_d^{*ad}C_{qd}^{(\times)abcd}Y_e^{pr} \\
& + 2\delta^{rb}\delta^{sc}Y_d^{*td}C_{ed}^{abcd}Y_e^{pa} + \left\{ \frac{1}{2} \left( \delta^{pa}\delta^{rb}\delta^{sc}(Y_d Y_d^\dagger)^{dt} + \delta^{rb}\delta^{sc}\delta^{td}(Y_e Y_e^\dagger)^{pa} + \delta^{pa}\delta^{rb}\delta^{sc}(Y_u Y_u^\dagger)^{dt} + 2\delta^{pa}\delta^{rb}\delta^{td}(Y_d^\dagger Y_d)^{sc} + 2\delta^{pa}\delta^{sc}\delta^{td}(Y_e^\dagger Y_e)^{br} \right. \right. \\
& + 4\delta^{sc}\delta^{td}Y_e^{*ab}Y_e^{pr} + 12\delta^{pa}\delta^{rb}Y_d^{*ts}Y_d^{dc} \Big) - \frac{8}{3}\delta^{pa}\delta^{rb}\delta^{sc}\delta^{td}g_Y^2 - 8\delta^{pa}\delta^{rb}\delta^{sc}\delta^{td}g_s^2 \Big\} C_{\ell edq}^{abcd} + \left( C_{quqd}^{(\parallel)*} \right)^{abcd} \left\{ \delta^{sd}\delta^{ta}Y_e^{pr}Y_u^{cb} + 6\delta^{sd}\delta^{tc}Y_e^{pr}Y_u^{ab} \right\} \\
& + \left( C_{quqd}^{(\times)*} \right)^{abcd} \left\{ 2\delta^{sd}\delta^{tc}Y_e^{pr}Y_u^{ab} + 3\delta^{sd}\delta^{ta}Y_e^{pr}Y_u^{cb} \right\} + 2 \left\{ \delta^{pa}\delta^{rb}Y_d^{*cs}Y_u^{*td} - 3\delta^{pa}\delta^{rb}Y_d^{*ts}Y_u^{*cd} \right\} C_{\ell equ}^{abcd} + \left\{ 3\delta^{pa}\delta^{rd}Y_d^{*ts}Y_u^{*cb} \right. \\
& \left. - \delta^{pa}\delta^{rd}Y_d^{*cs}Y_u^{*tb} \right\} C_{\ell uqe}^{abcd} + 2\delta^{pa}\delta^{td}Y_d^{*cs}C_{\ell q}^{(\parallel)abcd}Y_e^{br} + 4\delta^{pa}\delta^{td}Y_d^{*cs}C_{\ell q}^{(\times)abcd}Y_e^{br}, \tag{12.1}
\end{aligned}$$

$$\begin{aligned}
\beta_{C_{\ell edq}^{prst}}^{(2)} = & -2 \left( 2Y_d^{*ts}Y_e^{pr} \mathbf{T}_{\ell H} - 3Y_d^{*ts} (C_{\ell HH}^\dagger C_{\ell HH} Y_e)^{pr} \right) + \left\{ \frac{1}{18}g_Y^2 Y_d^{*ts}Y_e^{pr} + \frac{1}{6}g_L^2 Y_d^{*ts}Y_e^{pr} + \lambda Y_d^{*ts}Y_e^{pr} - \frac{1}{2}Y_e^{pr}(Y_u^\dagger Y_u Y_d^\dagger)^{ts} - \frac{3}{2}Y_e^{pr}(Y_d^\dagger Y_d Y_d^\dagger)^{ts} \right. \\
& \left. - \frac{3}{2}Y_d^{*ts}(Y_e Y_e^\dagger Y_e)^{pr} \right\} C_{HD}^{(\parallel)} + \left\{ \frac{1}{9}g_Y^2 Y_d^{*ts}Y_e^{pr} + \frac{1}{2}Y_e^{pr}(Y_u^\dagger Y_u Y_d^\dagger)^{ts} + \lambda Y_d^{*ts}Y_e^{pr} - \frac{3}{2}Y_e^{pr}(Y_d^\dagger Y_d Y_d^\dagger)^{ts} - \frac{3}{2}Y_d^{*ts}(Y_e Y_e^\dagger Y_e)^{pr} \right\} C_{HD}^{(\times)} \\
& + \frac{14}{9}g_Y^4 C_{HB} Y_d^{*ts}Y_e^{pr} - \frac{40i}{9}g_Y^4 C_{H\bar{B}} Y_d^{*ts}Y_e^{pr} - 6g_L^4 C_{HW} Y_d^{*ts}Y_e^{pr} + \frac{32}{3}g_s^4 C_{HG} Y_d^{*ts}Y_e^{pr} + \frac{32i}{3}g_s^4 C_{H\bar{G}} Y_d^{*ts}Y_e^{pr} + 5g_Y^2 g_L^2 C_{HWB} Y_d^{*ts}Y_e^{pr} \\
& + 2ig_Y^2 g_L^2 C_{H\widetilde{WB}} Y_d^{*ts}Y_e^{pr} + 21g_L^6 C_W Y_d^{*ts}Y_e^{pr} - 88g_s^6 C_G Y_d^{*ts}Y_e^{pr} + 24ig_s^6 C_{\bar{G}} Y_d^{*ts}Y_e^{pr} + \left\{ 3\delta^{pa}\delta^{rb}\lambda Y_d^{*ts} - 6\delta^{pa}\delta^{rb}(Y_d^\dagger Y_d Y_d^\dagger)^{ts} \right\} C_{eH}^{ab} \\
& + C_{dH}^{*ab} \left\{ 3\delta^{sb}\delta^{ta}\lambda Y_e^{pr} - 6\delta^{sb}\delta^{ta}(Y_e Y_e^\dagger Y_e)^{pr} \right\} + \left\{ g_Y^2 \left( 2Y_d^{*ts}Y_e^{*ab}Y_e^{pr} + 3\delta^{pa}\delta^{rb}Y_d^{*ts} \text{Tr}[Y_u^\dagger Y_u] - \delta^{pa}Y_d^{*ts}(Y_e^\dagger Y_e)^{br} - 2\delta^{rb}Y_d^{*ts}(Y_e Y_e^\dagger)^{pa} \right. \right. \\
& \left. \left. - \frac{8}{3}\delta^{pa}\delta^{rb}(Y_u^\dagger Y_u Y_d^\dagger)^{ts} - 8\delta^{pa}\delta^{rb}Y_d^{*ts} \text{Tr}[Y_e^\dagger Y_e] \right) + \frac{9}{4}\delta^{pa}\delta^{rb}g_Y^2 g_L^2 Y_d^{*ts} + \frac{43}{12}\delta^{pa}\delta^{rb}g_Y^4 Y_d^{*ts} \right\} C_{eB}^{ab} - 6g_Y^2 C_{eB}^{*ab} Y_d^{*ts}Y_e^{pr}Y_e^{ab} \\
& + \left\{ g_L^2 \left( 3Y_d^{*ts}Y_e^{*ab}Y_e^{pr} + 6\delta^{pa}\delta^{rb}(Y_u^\dagger Y_u Y_d^\dagger)^{ts} - \frac{3}{2}\delta^{pa}Y_d^{*ts}(Y_e^\dagger Y_e)^{br} - \frac{27}{2}\delta^{pa}\delta^{rb}Y_d^{*ts} \text{Tr}[Y_u^\dagger Y_u] \right) + \frac{21}{8}\delta^{pa}\delta^{rb}g_Y^2 g_L^2 Y_d^{*ts} + \frac{69}{8}\delta^{pa}\delta^{rb}g_L^4 Y_d^{*ts} \right\} C_{eW}^{ab}
\end{aligned}$$

$$\begin{aligned}
& + 3g_L^2 \mathbf{C}_{eW}^{*ab} Y_d^{*ts} Y_e^{pr} Y_e^{ab} + g_Y^2 \left\{ \frac{14}{3} Y_d^{*as} Y_u^{*tb} Y_e^{pr} - 5 Y_d^{*ts} Y_u^{*ab} Y_e^{pr} \right\} \mathbf{C}_{uB}^{ab} - g_Y^2 \mathbf{C}_{uB}^{*ab} \left\{ 2\delta^{ta} Y_e^{pr} (Y_d^\dagger Y_u)^{sb} + 5 Y_d^{*ts} Y_e^{pr} Y_u^{ab} \right\} + g_L^2 \left\{ 3 Y_d^{*as} Y_u^{*tb} Y_e^{pr} \right. \\
& - \frac{9}{2} Y_d^{*ts} Y_u^{*ab} Y_e^{pr} \left. \right\} \mathbf{C}_{uW}^{ab} + g_L^2 \mathbf{C}_{uW}^{*ab} \left\{ 6\delta^{ta} Y_e^{pr} (Y_d^\dagger Y_u)^{sb} - \frac{9}{2} Y_d^{*ts} Y_e^{pr} Y_u^{ab} \right\} + g_s^2 \left\{ \frac{16}{3} Y_d^{*as} Y_u^{*tb} Y_e^{pr} - 16 Y_d^{*ts} Y_u^{*ab} Y_e^{pr} \right\} \mathbf{C}_{uG}^{ab} \\
& - g_s^2 \mathbf{C}_{uG}^{*ab} \left\{ 8\delta^{ta} Y_e^{pr} (Y_d^\dagger Y_u)^{sb} + 16 Y_d^{*ts} Y_e^{pr} Y_u^{ab} \right\} - 2g_Y^2 Y_d^{*ts} Y_d^{*ab} \mathbf{C}_{dB}^{ab} Y_e^{pr} + \mathbf{C}_{dB}^{*ab} \left\{ g_Y^2 \left( \frac{13}{3} \delta^{ta} Y_e^{pr} (Y_d^\dagger Y_d)^{sb} + \frac{26}{3} \delta^{sb} Y_e^{pr} (Y_d Y_d^\dagger)^{at} \right. \right. \\
& + 24\delta^{sb} \delta^{ta} Y_e^{pr} \text{Tr}[Y_d^\dagger Y_d] + 27\delta^{sb} \delta^{ta} Y_e^{pr} \text{Tr}[Y_u^\dagger Y_u] - \frac{37}{3} \delta^{sb} Y_e^{pr} (Y_u Y_u^\dagger)^{at} - 26 Y_d^{*ts} Y_d^{ab} Y_e^{pr} \left. \right) + \frac{400}{9} \delta^{sb} \delta^{ta} g_Y^2 g_s^2 Y_e^{pr} + \frac{6523}{108} \delta^{sb} \delta^{ta} g_Y^4 Y_e^{pr} \\
& - \frac{79}{4} \delta^{sb} \delta^{ta} g_Y^2 g_L^2 Y_e^{pr} \left. \right\} + 9g_L^2 Y_d^{*ts} Y_d^{*ab} \mathbf{C}_{dW}^{ab} Y_e^{pr} + \mathbf{C}_{dW}^{*ab} \left\{ g_L^2 \left( \frac{3}{2} \delta^{sb} Y_e^{pr} (Y_u Y_u^\dagger)^{at} + 9 Y_d^{*ts} Y_d^{ab} Y_e^{pr} - \frac{3}{2} \delta^{ta} Y_e^{pr} (Y_d^\dagger Y_d)^{sb} - \frac{27}{2} \delta^{sb} \delta^{ta} Y_e^{pr} \text{Tr}[Y_u^\dagger Y_u] \right) \right. \\
& + \frac{191}{24} \delta^{sb} \delta^{ta} g_Y^2 g_L^2 Y_e^{pr} + \frac{69}{8} \delta^{sb} \delta^{ta} g_L^4 Y_e^{pr} - 8\delta^{sb} \delta^{ta} g_s^2 g_L^2 Y_e^{pr} \left. \right\} - 16g_s^2 Y_d^{*ts} Y_d^{*ab} \mathbf{C}_{dG}^{ab} Y_e^{pr} + \mathbf{C}_{dG}^{*ab} \left\{ g_s^2 \left( \frac{8}{3} \delta^{ta} Y_e^{pr} (Y_d^\dagger Y_d)^{sb} + \frac{16}{3} \delta^{sb} Y_e^{pr} (Y_d Y_d^\dagger)^{at} \right. \right. \\
& - \frac{32}{3} \delta^{sb} Y_e^{pr} (Y_u Y_u^\dagger)^{at} - 16 Y_d^{*ts} Y_d^{ab} Y_e^{pr} \left. \right) + \frac{224}{9} \delta^{sb} \delta^{ta} g_s^4 Y_e^{pr} - \frac{244}{27} \delta^{sb} \delta^{ta} g_Y^2 g_s^2 Y_e^{pr} - 20\delta^{sb} \delta^{ta} g_s^2 g_L^2 Y_e^{pr} \left. \right\} + \left\{ \frac{3}{2} \delta^{pa} Y_e^{br} (Y_d^\dagger Y_d Y_d^\dagger)^{ts} \right. \\
& + 2 Y_d^{*ts} Y_e^{br} (Y_e Y_e^\dagger)^{pa} + \frac{15}{4} \delta^{pa} g_L^2 Y_d^{*ts} Y_e^{br} + 6\delta^{pa} Y_d^{*ts} (Y_e Y_e^\dagger Y_e)^{br} - g_Y^2 \left( \frac{4}{9} \delta^{ab} Y_d^{*ts} Y_e^{pr} + \frac{115}{36} \delta^{pa} Y_d^{*ts} Y_e^{br} \right) - \frac{4}{3} Y_d^{*ts} Y_e^{pr} (Y_e Y_e^\dagger)^{ba} \\
& - \frac{5}{2} \delta^{pa} Y_e^{br} (Y_u^\dagger Y_u Y_d^\dagger)^{ts} \left. \right\} \mathbf{C}_{H\ell}^{(\parallel)ab} + \left\{ g_L^2 \left( \frac{2}{3} \delta^{ab} Y_d^{*ts} Y_e^{pr} - \frac{11}{6} \delta^{pa} Y_d^{*ts} Y_e^{br} \right) + Y_d^{*ts} Y_e^{br} (Y_e Y_e^\dagger)^{pa} + \frac{5}{2} \delta^{pa} Y_e^{br} (Y_u^\dagger Y_u Y_d^\dagger)^{ts} + 3\delta^{pa} Y_d^{*ts} (Y_e Y_e^\dagger Y_e)^{br} \right. \\
& + \frac{9}{2} \delta^{pa} Y_e^{br} (Y_d^\dagger Y_d Y_d^\dagger)^{ts} - g_Y^2 \left( \frac{2}{9} \delta^{ab} Y_d^{*ts} Y_e^{pr} + \frac{11}{9} \delta^{pa} Y_d^{*ts} Y_e^{br} \right) - \frac{8}{3} Y_d^{*ts} Y_e^{pr} (Y_e Y_e^\dagger)^{ba} \left. \right\} \mathbf{C}_{H\ell}^{(\times)ab} + \left\{ \frac{3}{4} \delta^{rb} g_L^2 Y_d^{*ts} Y_e^{pa} + \frac{4}{3} Y_d^{*ts} Y_e^{pr} (Y_e^\dagger Y_e)^{ba} \right. \\
& - \frac{1}{2} \delta^{rb} Y_e^{pa} (Y_u^\dagger Y_u Y_d^\dagger)^{ts} - g_Y^2 \left( \frac{4}{9} \delta^{ab} Y_d^{*ts} Y_e^{pr} + \frac{191}{36} \delta^{rb} Y_d^{*ts} Y_e^{pa} \right) - Y_d^{*ts} Y_e^{pa} (Y_e^\dagger Y_e)^{br} - 3\delta^{rb} Y_d^{*ts} (Y_e Y_e^\dagger Y_e)^{pa} - \frac{9}{2} \delta^{rb} Y_e^{pa} (Y_d^\dagger Y_d Y_d^\dagger)^{ts} \left. \right\} \mathbf{C}_{He}^{ab} \\
& + \left\{ g_Y^2 \left( \frac{4}{9} \delta^{ab} Y_d^{*ts} Y_e^{pr} - \frac{17}{108} \delta^{tb} Y_d^{*as} Y_e^{pr} \right) + \frac{3}{2} \delta^{tb} Y_d^{*as} (Y_e Y_e^\dagger Y_e)^{pr} + 2 Y_d^{*as} Y_e^{pr} (Y_d Y_d^\dagger)^{bt} + \frac{15}{4} \delta^{tb} g_L^2 Y_d^{*as} Y_e^{pr} + 4 Y_d^{*ts} Y_e^{pr} (Y_u Y_u^\dagger)^{ba} \right. \\
& + \frac{16}{3} \delta^{tb} g_s^2 Y_d^{*as} Y_e^{pr} + 6\delta^{tb} Y_e^{pr} (Y_d^\dagger Y_d Y_d^\dagger)^{as} - Y_d^{*as} Y_e^{pr} (Y_u Y_u^\dagger)^{bt} - \delta^{tb} Y_e^{pr} (Y_u^\dagger Y_u Y_d^\dagger)^{as} - 4 Y_d^{*ts} Y_e^{pr} (Y_d Y_d^\dagger)^{ba} \left. \right\} \mathbf{C}_{Hq}^{(\parallel)ab} + \left\{ g_Y^2 \left( \frac{2}{9} \delta^{ab} Y_d^{*ts} Y_e^{pr} \right. \right. \\
& - \frac{1}{27} \delta^{tb} Y_d^{*as} Y_e^{pr} \left. \right) + g_L^2 \left( 2\delta^{ab} Y_d^{*ts} Y_e^{pr} - \frac{11}{6} \delta^{tb} Y_d^{*as} Y_e^{pr} \right) + Y_d^{*as} Y_e^{pr} (Y_d Y_d^\dagger)^{bt} + Y_d^{*as} Y_e^{pr} (Y_u Y_u^\dagger)^{bt} + \delta^{tb} Y_e^{pr} (Y_u^\dagger Y_u Y_d^\dagger)^{as} + 3\delta^{tb} Y_e^{pr} (Y_d^\dagger Y_d Y_d^\dagger)^{as} \\
& + \frac{9}{2} \delta^{tb} Y_d^{*as} (Y_e Y_e^\dagger Y_e)^{pr} + \frac{32}{3} \delta^{tb} g_s^2 Y_d^{*as} Y_e^{pr} - 4 Y_d^{*ts} Y_e^{pr} (Y_u Y_u^\dagger)^{ba} - 8 Y_d^{*ts} Y_e^{pr} (Y_d Y_d^\dagger)^{ba} \left. \right\} \mathbf{C}_{Hq}^{(\times)ab} + \left\{ \frac{8}{9} \delta^{ab} g_Y^2 Y_d^{*ts} Y_e^{pr} - 4 Y_d^{*ts} Y_e^{pr} (Y_u^\dagger Y_u)^{ba} \right\} \mathbf{C}_{Hu}^{ab}
\end{aligned}$$

$$\begin{aligned}
& + \left\{ \frac{3}{4} \delta^{sa} g_L^2 Y_d^{*tb} Y_e^{pr} + g_Y^2 \left( \frac{235}{108} \delta^{sa} Y_d^{*tb} Y_e^{pr} - \frac{4}{9} \delta^{ab} Y_d^{*ts} Y_e^{pr} \right) + 2\delta^{sa} Y_e^{pr} (Y_u^\dagger Y_u Y_d^\dagger)^{tb} + 4Y_d^{*ts} Y_e^{pr} (Y_d^\dagger Y_d)^{ba} - Y_d^{*tb} Y_e^{pr} (Y_d^\dagger Y_d)^{sa} - 3\delta^{sa} Y_e^{pr} (Y_d^\dagger Y_d Y_d^\dagger)^{tb} \right. \\
& - \frac{9}{2} \delta^{sa} Y_d^{*tb} (Y_e Y_e^\dagger Y_e)^{pr} - \frac{16}{3} \delta^{sa} g_s^2 Y_d^{*tb} Y_e^{pr} \left. \right\} C_{Hd}^{ab} + 4Y_d^{*ts} C_{Hud}^{ab} Y_e^{pr} (Y_d^\dagger Y_u)^{ba} + C_{Hud}^{*ab} \left\{ \frac{3}{4} \delta^{sb} g_L^2 Y_u^{*ta} Y_e^{pr} + \frac{59}{36} \delta^{sb} g_Y^2 Y_u^{*ta} Y_e^{pr} \right. \\
& + 4Y_d^{*ts} Y_e^{pr} (Y_u^\dagger Y_d)^{ab} - Y_u^{*ta} Y_e^{pr} (Y_d^\dagger Y_d)^{sb} - \delta^{sb} Y_e^{pr} (Y_u^\dagger Y_u Y_u^\dagger)^{ta} - \frac{16}{3} \delta^{sb} g_s^2 Y_u^{*ta} Y_e^{pr} \left. \right\} + \left\{ g_Y^2 \left( \frac{4}{9} \delta^{rd} \delta^{ab} Y_d^{*ts} Y_e^{pc} + \frac{32}{9} \delta^{pa} \delta^{cd} Y_d^{*ts} Y_e^{br} \right. \right. \\
& - 6\delta^{pa} \delta^{rd} Y_d^{*ts} Y_e^{bc} \left. \right) + 2\delta^{pa} \delta^{rd} Y_d^{*ts} Y_e^{bc} \text{Tr}[Y_e^\dagger Y_e] + 4\delta^{pa} Y_d^{*ts} Y_e^{br} (Y_e^\dagger Y_e)^{dc} + 4\delta^{rd} Y_d^{*ts} Y_e^{pc} (Y_e Y_e^\dagger)^{ba} + 12\delta^{pa} \delta^{rd} Y_d^{*ts} (Y_e Y_e^\dagger Y_e)^{bc} \\
& - 2Y_d^{*ts} Y_e^{*ad} Y_e^{pr} Y_e^{bc} - 6\delta^{pa} \delta^{rd} g_L^2 Y_d^{*ts} Y_e^{bc} \left. \right\} C_{\ell e}^{abcd} + \left\{ \frac{3}{2} \delta^{pa} Y_u^{*td} Y_e^{br} (Y_d^\dagger Y_u)^{sc} - \frac{64}{9} \delta^{pa} \delta^{cd} g_Y^2 Y_d^{*ts} Y_e^{br} \right\} C_{\ell u}^{abcd} + \left\{ g_Y^2 \left( \frac{32}{9} \delta^{pa} \delta^{cd} Y_d^{*ts} Y_e^{br} \right. \right. \\
& + \frac{49}{12} \delta^{pa} \delta^{sc} Y_d^{*td} Y_e^{br} - \frac{116}{27} \delta^{sc} \delta^{ab} Y_d^{*td} Y_e^{pr} \left. \right) + \frac{5}{2} \delta^{pa} Y_d^{*td} Y_e^{br} (Y_d^\dagger Y_d)^{sc} + 3\delta^{sc} Y_d^{*td} Y_e^{pr} (Y_e Y_e^\dagger)^{ba} + 3\delta^{pa} \delta^{sc} Y_e^{br} (Y_u^\dagger Y_u Y_d^\dagger)^{td} + 5\delta^{sc} Y_d^{*td} Y_e^{br} (Y_e Y_e^\dagger)^{pa} \\
& + 9\delta^{pa} Y_d^{*ts} Y_e^{br} (Y_d^\dagger Y_d)^{dc} - \frac{1}{2} \delta^{pa} \delta^{sc} Y_d^{*td} (Y_e Y_e^\dagger Y_e)^{br} - \text{T}_2 \delta^{pa} \delta^{sc} Y_d^{*td} Y_e^{br} - \delta^{pa} \delta^{sc} Y_e^{br} (Y_d^\dagger Y_d Y_d^\dagger)^{td} - \frac{15}{4} \delta^{pa} \delta^{sc} g_L^2 Y_d^{*td} Y_e^{br} \left. \right\} C_{\ell d}^{abcd} \\
& + \left\{ \frac{5}{2} \delta^{tb} Y_d^{*as} Y_e^{pc} (Y_e^\dagger Y_e)^{dr} + \frac{5}{2} \delta^{rd} \delta^{tb} Y_e^{pc} (Y_u^\dagger Y_u Y_d^\dagger)^{as} + 3\delta^{tb} Y_d^{*as} Y_e^{pr} (Y_e^\dagger Y_e)^{dc} + 5\delta^{rd} Y_d^{*as} Y_e^{pc} (Y_d Y_d^\dagger)^{bt} + 9\delta^{rd} Y_d^{*ts} Y_e^{pc} (Y_d Y_d^\dagger)^{ba} \right. \\
& - \frac{1}{2} \delta^{rd} \delta^{tb} Y_e^{pc} (Y_d^\dagger Y_d Y_d^\dagger)^{as} - \text{T}_2 \delta^{rd} \delta^{tb} Y_d^{*as} Y_e^{pc} - g_Y^2 \left( \frac{4}{9} \delta^{rd} \delta^{ab} Y_d^{*ts} Y_e^{pc} + \frac{32}{27} \delta^{tb} \delta^{cd} Y_d^{*as} Y_e^{pr} + \frac{79}{12} \delta^{rd} \delta^{tb} Y_d^{*as} Y_e^{pc} \right) - \delta^{rd} Y_d^{*as} Y_e^{pc} (Y_u Y_u^\dagger)^{bt} \\
& - \delta^{rd} \delta^{tb} Y_d^{*as} (Y_e Y_e^\dagger Y_e)^{pc} - \frac{15}{4} \delta^{rd} \delta^{tb} g_L^2 Y_d^{*as} Y_e^{pc} \left. \right\} C_{qe}^{abcd} + \left\{ \frac{1}{2} Y_d^{*as} Y_u^{*td} Y_e^{pr} Y_u^{bc} + \frac{64}{27} \delta^{tb} \delta^{cd} g_Y^2 Y_d^{*as} Y_e^{pr} - 12Y_d^{*ts} Y_u^{*ad} Y_e^{pr} Y_u^{bc} \right\} C_{qu}^{(\parallel)abcd} \\
& + \left\{ \frac{64}{81} \delta^{tb} \delta^{cd} g_Y^2 Y_d^{*as} Y_e^{pr} + \frac{3}{2} Y_d^{*as} Y_u^{*td} Y_e^{pr} Y_u^{bc} + \frac{112}{27} \delta^{tb} \delta^{cd} g_s^2 Y_d^{*as} Y_e^{pr} - 36Y_d^{*ts} Y_u^{*ad} Y_e^{pr} Y_u^{bc} \right\} C_{qu}^{(\times)abcd} + \left\{ g_Y^2 \left( \frac{116}{27} \delta^{sc} \delta^{ab} Y_d^{*td} Y_e^{pr} \right. \right. \\
& - \frac{32}{27} \delta^{tb} \delta^{cd} Y_d^{*as} Y_e^{pr} - \frac{14}{9} \delta^{sc} \delta^{tb} Y_d^{*ad} Y_e^{pr} \left. \right) + 6\delta^{sc} \delta^{tb} Y_d^{*ad} Y_e^{pr} \text{Tr}[Y_d^\dagger Y_d] + 12\delta^{tb} Y_d^{*as} Y_e^{pr} (Y_d^\dagger Y_d)^{dc} + 12\delta^{sc} Y_d^{*td} Y_e^{pr} (Y_d Y_d^\dagger)^{ba} \\
& + 12\delta^{sc} \delta^{tb} Y_e^{pr} (Y_d^\dagger Y_d Y_d^\dagger)^{ad} - \frac{7}{2} \delta^{sc} \delta^{tb} Y_e^{pr} (Y_u^\dagger Y_u Y_d^\dagger)^{ad} - 6Y_d^{*ts} Y_d^{*ad} Y_d^{bc} Y_e^{pr} - 6\delta^{sc} \delta^{tb} g_L^2 Y_d^{*ad} Y_e^{pr} - \frac{32}{3} \delta^{sc} \delta^{tb} g_s^2 Y_d^{*ad} Y_e^{pr} \left. \right\} C_{qd}^{(\parallel)abcd} \\
& + \left\{ g_Y^2 \left( \frac{116}{81} \delta^{sc} \delta^{ab} Y_d^{*td} Y_e^{pr} - \frac{32}{81} \delta^{tb} \delta^{cd} Y_d^{*as} Y_e^{pr} - \frac{14}{3} \delta^{sc} \delta^{tb} Y_d^{*ad} Y_e^{pr} \right) + g_s^2 \left( \frac{112}{27} \delta^{tb} \delta^{cd} Y_d^{*as} Y_e^{pr} + \frac{224}{27} \delta^{sc} \delta^{ab} Y_d^{*td} Y_e^{pr} - 128\delta^{sc} \delta^{tb} Y_d^{*ad} Y_e^{pr} \right) \right. \\
& + 4\delta^{tb} Y_d^{*as} Y_e^{pr} (Y_d^\dagger Y_d)^{dc} + 4\delta^{sc} Y_d^{*td} Y_e^{pr} (Y_d Y_d^\dagger)^{ba} + 18\delta^{sc} \delta^{tb} Y_d^{*ad} Y_e^{pr} \text{Tr}[Y_d^\dagger Y_d] + 36\delta^{sc} \delta^{tb} Y_e^{pr} (Y_d^\dagger Y_d Y_d^\dagger)^{ad} - \frac{21}{2} \delta^{sc} \delta^{tb} Y_e^{pr} (Y_u^\dagger Y_u Y_d^\dagger)^{ad} \\
\end{aligned}$$

$$\begin{aligned}
& -18Y_d^{*ts}Y_d^{*ad}Y_d^{bc}Y_e^{pr} - 18\delta^{sc}\delta^{tb}g_L^2Y_d^{*ad}Y_e^{pr} \Big\} C_{qd}^{(\times)abcd} + \left\{ \frac{4}{9}\delta^{rb}\delta^{ad}g_Y^2Y_d^{*ts}Y_e^{pc} + 4\delta^{rb}Y_d^{*ts}Y_e^{pa}(Y_e^\dagger Y_e)^{dc} \right\} C_{ee}^{abcd} + \left\{ \frac{32}{27}\delta^{sa}\delta^{bc}g_s^2Y_d^{*td}Y_e^{pr} \right. \\
& + 12\delta^{sa}Y_d^{*tb}Y_e^{pr}(Y_d^\dagger Y_d)^{dc} - g_Y^2 \left( \frac{172}{81}\delta^{sa}\delta^{bc}Y_d^{*td}Y_e^{pr} + \frac{232}{27}\delta^{sa}\delta^{cd}Y_d^{*tb}Y_e^{pr} \right) \Big\} C_{dd}^{abcd} - \left\{ \frac{1}{2}\delta^{rb}Y_u^{*td}Y_e^{pa}(Y_d^\dagger Y_u)^{sc} + \frac{8}{9}\delta^{rb}\delta^{cd}g_Y^2Y_d^{*ts}Y_e^{pa} \right\} C_{eu}^{abcd} \\
& + \left\{ \frac{1}{2}\delta^{rb}Y_d^{*td}Y_e^{pa}(Y_d^\dagger Y_d)^{sc} + \frac{1}{2}\delta^{sc}Y_d^{*td}Y_e^{pa}(Y_e^\dagger Y_e)^{br} + g_Y^2 \left( \frac{4}{9}\delta^{rb}\delta^{cd}Y_d^{*ts}Y_e^{pa} - \frac{116}{27}\delta^{sc}\delta^{ab}Y_d^{*td}Y_e^{pr} - \frac{61}{12}\delta^{rb}\delta^{sc}Y_d^{*td}Y_e^{pa} \right) + 3\delta^{sc}Y_d^{*td}Y_e^{pr}(Y_e^\dagger Y_e)^{ba} \right. \\
& + 3\delta^{rb}\delta^{sc}Y_e^{pa}(Y_u^\dagger Y_u Y_d^\dagger)^{td} + 9\delta^{rb}Y_d^{*ts}Y_e^{pa}(Y_d^\dagger Y_d)^{dc} + \frac{51}{4}\delta^{rb}\delta^{sc}g_L^2Y_d^{*td}Y_e^{pa} - 5T_2\delta^{rb}\delta^{sc}Y_d^{*td}Y_e^{pa} - 5\delta^{rb}\delta^{sc}Y_e^{pa}(Y_d^\dagger Y_d Y_d^\dagger)^{td} \\
& \left. - 5\delta^{rb}\delta^{sc}Y_d^{*td}(Y_e Y_e^\dagger Y_e)^{pa} \right\} C_{ed}^{abcd} + \left\{ \frac{232}{27}\delta^{sc}\delta^{ab}g_Y^2Y_d^{*td}Y_e^{pr} - \frac{3}{2}\delta^{sc}Y_u^{*tb}Y_e^{pr}(Y_d^\dagger Y_u)^{da} \right\} C_{ud}^{(\parallel)abcd} + \left\{ \frac{232}{81}\delta^{sc}\delta^{ab}g_Y^2Y_d^{*td}Y_e^{pr} \right. \\
& + \frac{112}{27}\delta^{sc}\delta^{ab}g_s^2Y_d^{*td}Y_e^{pr} - \frac{9}{2}\delta^{sc}Y_u^{*tb}Y_e^{pr}(Y_d^\dagger Y_u)^{da} \Big\} C_{ud}^{(\times)abcd} + \left\{ \delta^{rb}\delta^{sc}(Y_e Y_e^\dagger)^{pa}(Y_u Y_u^\dagger)^{dt} + g_Y^2 \left( \frac{13}{8}\delta^{pa}\delta^{sc}\delta^{td}(Y_e^\dagger Y_e)^{br} + \frac{247}{144}\delta^{pa}\delta^{rb}\delta^{sc}(Y_d Y_d^\dagger)^{dt} \right. \right. \\
& + \frac{157}{72}\delta^{pa}\delta^{rb}\delta^{td}(Y_d^\dagger Y_d)^{sc} + \frac{21}{4}\delta^{sc}\delta^{td}Y_e^{*ab}Y_e^{pr} + \frac{103}{16}\delta^{rb}\delta^{sc}\delta^{td}(Y_e Y_e^\dagger)^{pa} - \frac{53}{144}\delta^{pa}\delta^{rb}\delta^{sc}(Y_u Y_u^\dagger)^{dt} - \frac{11}{12}\delta^{pa}\delta^{rb}Y_d^{*ts}Y_d^{dc} \Big) + g_L^2 \left( \frac{3}{4}\delta^{sc}\delta^{td}Y_e^{*ab}Y_e^{pr} \right. \\
& + \frac{33}{16}\delta^{pa}\delta^{rb}\delta^{sc}(Y_d Y_d^\dagger)^{dt} + \frac{33}{16}\delta^{rb}\delta^{sc}\delta^{td}(Y_e Y_e^\dagger)^{pa} + \frac{33}{16}\delta^{pa}\delta^{rb}\delta^{sc}(Y_u Y_u^\dagger)^{dt} + \frac{9}{4}\delta^{pa}\delta^{rb}Y_d^{*ts}Y_d^{dc} + \frac{51}{8}\delta^{pa}\delta^{rb}\delta^{td}(Y_d^\dagger Y_d)^{sc} + \frac{51}{8}\delta^{pa}\delta^{sc}\delta^{td}(Y_e^\dagger Y_e)^{br} \Big) \\
& + g_s^2 \left( \frac{16}{3}\delta^{pa}\delta^{rb}\delta^{sc}(Y_d Y_d^\dagger)^{dt} + \frac{16}{3}\delta^{pa}\delta^{rb}\delta^{sc}(Y_u Y_u^\dagger)^{dt} + \frac{32}{3}\delta^{pa}\delta^{rb}\delta^{td}(Y_d^\dagger Y_d)^{sc} + 40\delta^{pa}\delta^{rb}Y_d^{*ts}Y_d^{dc} \right) + \frac{3}{2}\delta^{pa}\delta^{rb}Y_d^{*ts}(Y_u Y_u^\dagger Y_d)^{dc} \\
& + 2\delta^{pa}\delta^{rb}(Y_d^\dagger Y_d)^{sc}(Y_d Y_d^\dagger)^{dt} + 2\delta^{sc}\delta^{td}(Y_e^\dagger Y_e)^{br}(Y_e Y_e^\dagger)^{pa} + 3\delta^{pa}\delta^{rb}\delta^{sc}\delta^{td}g_Y^2g_L^2 + \frac{31}{9}\delta^{pa}\delta^{rb}\delta^{sc}\delta^{td}g_Y^2g_s^2 + 9\delta^{pa}\delta^{rb}\delta^{sc}\delta^{td}g_s^2g_L^2 \\
& + \frac{857}{54}\delta^{pa}\delta^{rb}\delta^{sc}\delta^{td}g_Y^4 - \frac{1}{4}\delta^{pa}\delta^{rb}\delta^{td}(Y_d^\dagger Y_d Y_d^\dagger Y_d)^{sc} - \frac{1}{4}\delta^{pa}\delta^{rb}\delta^{td}(Y_d^\dagger Y_u Y_u^\dagger Y_d)^{sc} - \frac{1}{4}\delta^{pa}\delta^{sc}\delta^{td}(Y_e^\dagger Y_e Y_e^\dagger Y_e)^{br} - \frac{1}{4}\delta^{pa}\delta^{rb}\delta^{sc}(Y_d Y_d^\dagger Y_d Y_d^\dagger)^{dt} \\
& - \frac{1}{4}\delta^{rb}\delta^{sc}\delta^{td}(Y_e Y_e^\dagger Y_e Y_e^\dagger)^{pa} - \frac{1}{4}\delta^{pa}\delta^{rb}\delta^{sc}(Y_u Y_u^\dagger Y_u Y_u^\dagger)^{dt} - \frac{1}{2}\delta^{sc}Y_e^{*ab}Y_e^{pr}(Y_u Y_u^\dagger)^{dt} - \frac{3}{4}T_2\delta^{pa}\delta^{rb}\delta^{sc}(Y_d Y_d^\dagger)^{dt} - \frac{3}{4}\delta^{pa}\delta^{sc}(Y_e^\dagger Y_e)^{br}(Y_d Y_d^\dagger)^{dt} \\
& - \frac{3}{4}T_2\delta^{rb}\delta^{sc}\delta^{td}(Y_e Y_e^\dagger)^{pa} - \frac{3}{4}\delta^{rb}\delta^{td}(Y_d^\dagger Y_d)^{sc}(Y_e Y_e^\dagger)^{pa} - \frac{3}{4}T_2\delta^{pa}\delta^{rb}\delta^{sc}(Y_u Y_u^\dagger)^{dt} - \delta^{pa}\delta^{sc}(Y_e^\dagger Y_e)^{br}(Y_u Y_u^\dagger)^{dt} - \frac{3}{2}T_2\delta^{pa}\delta^{rb}\delta^{td}(Y_d^\dagger Y_d)^{sc} \\
& - \frac{3}{2}T_2\delta^{pa}\delta^{sc}\delta^{td}(Y_e^\dagger Y_e)^{br} - 2\delta^{pa}\delta^{rb}(Y_d^\dagger Y_d)^{sc}(Y_u Y_u^\dagger)^{dt} - 3\delta^{sc}\delta^{td}Y_e^{*ab}Y_e^{pr}\text{Tr}[Y_d^\dagger Y_d] - 3\delta^{pa}\delta^{rb}Y_d^{*ts}Y_d^{dc}\text{Tr}[Y_e^\dagger Y_e] - \frac{9}{2}\delta^{pa}\delta^{td}(Y_d^\dagger Y_d)^{sc}(Y_e^\dagger Y_e)^{br} \\
& - \frac{9}{2}\delta^{rb}\delta^{sc}(Y_d Y_d^\dagger)^{dt}(Y_e Y_e^\dagger)^{pa} - \frac{9}{2}\delta^{sc}\delta^{td}Y_e^{pr}(Y_e^\dagger Y_e Y_e^\dagger)^{ab} - \frac{27}{2}\delta^{pa}\delta^{rb}Y_d^{*ts}(Y_d Y_d^\dagger Y_d)^{dc} - 108\delta^{pa}\delta^{rb}\delta^{sc}\delta^{td}g_s^4 \Big\} C_{ledq}^{abcd} - C_{ledq}^{*abcd} \Big\} 3Y_d^{*tc}Y_d^{*ds}Y_e^{pb}Y_e^{ar} \\
& + 6Y_d^{*ts}Y_d^{*dc}Y_e^{pr}Y_e^{ab} \Big\} + \left\{ Y_d^{*ad}Y_d^{*cs}Y_u^{*tb}Y_e^{pr} + 3Y_d^{*as}Y_d^{*cd}Y_u^{*tb}Y_e^{pr} - \frac{3}{2}Y_d^{*ts}Y_d^{*ad}Y_u^{*cb}Y_e^{pr} - 9Y_d^{*ts}Y_d^{*cd}Y_u^{*ab}Y_e^{pr} \right\} C_{quqd}^{(\parallel)abcd}
\end{aligned}$$

$$\begin{aligned}
& + \left( C_{quqd}^{(\parallel)*} \right)^{abcd} \left\{ g_Y^2 \left( \frac{67}{24} \delta^{sd} \delta^{ta} Y_e^{pr} Y_u^{cb} + \frac{19}{3} \delta^{sd} \delta^{tc} Y_e^{pr} Y_u^{ab} \right) + g_L^2 \left( \frac{15}{8} \delta^{sd} \delta^{ta} Y_e^{pr} Y_u^{cb} + 9 \delta^{sd} \delta^{tc} Y_e^{pr} Y_u^{ab} \right) + g_s^2 \left( 12 \delta^{sd} \delta^{ta} Y_e^{pr} Y_u^{cb} + 40 \delta^{sd} \delta^{tc} Y_e^{pr} Y_u^{ab} \right) \right. \\
& + \frac{5}{4} \delta^{sd} \delta^{ta} Y_e^{pr} (Y_d Y_d^\dagger Y_u)^{cb} + \frac{9}{2} \delta^{sd} \delta^{tc} Y_e^{pr} (Y_d Y_d^\dagger Y_u)^{ab} - \frac{1}{4} \delta^{tc} Y_d^{ad} Y_e^{pr} (Y_d^\dagger Y_u)^{sb} - \frac{1}{4} \delta^{sd} Y_e^{pr} Y_u^{cb} (Y_u Y_u^\dagger)^{at} - \left( \frac{3}{2} \delta^{sd} \delta^{ta} Y_e^{pr} Y_u^{cb} + 9 \delta^{sd} \delta^{tc} Y_e^{pr} Y_u^{ab} \right) \text{Tr} \left[ Y_d^\dagger Y_d \right] \\
& - \frac{3}{2} \delta^{ta} Y_d^{cd} Y_e^{pr} (Y_d^\dagger Y_u)^{sb} - \frac{3}{2} \delta^{sd} Y_e^{pr} Y_u^{ab} (Y_u Y_u^\dagger)^{ct} - \frac{9}{4} \delta^{sd} \delta^{ta} Y_e^{pr} (Y_u Y_u^\dagger Y_u)^{cb} - \frac{27}{2} \delta^{sd} \delta^{tc} Y_e^{pr} (Y_u Y_u^\dagger Y_u)^{ab} \left. \right\} + \left\{ Y_d^{*as} Y_d^{*cd} Y_u^{*tb} Y_e^{pr} + 3 Y_d^{*ad} Y_d^{*cs} Y_u^{*tb} Y_e^{pr} \right. \\
& - 3 Y_d^{*ts} Y_d^{*cd} Y_u^{*ab} Y_e^{pr} - \frac{9}{2} Y_d^{*ts} Y_d^{*ad} Y_u^{*cb} Y_e^{pr} \left. \right\} C_{quqd}^{(\times)abcd} + \left( C_{quqd}^{(\times)*} \right)^{abcd} \left\{ g_Y^2 \left( \frac{19}{9} \delta^{sd} \delta^{tc} Y_e^{pr} Y_u^{ab} + \frac{67}{8} \delta^{sd} \delta^{ta} Y_e^{pr} Y_u^{cb} \right) + g_L^2 \left( 3 \delta^{sd} \delta^{tc} Y_e^{pr} Y_u^{ab} \right. \right. \\
& + \frac{45}{8} \delta^{sd} \delta^{ta} Y_e^{pr} Y_u^{cb} \left. \right) + g_s^2 \left( \frac{40}{3} \delta^{sd} \delta^{tc} Y_e^{pr} Y_u^{ab} + 48 \delta^{sd} \delta^{ta} Y_e^{pr} Y_u^{cb} \right) + \frac{3}{2} \delta^{sd} \delta^{tc} Y_e^{pr} (Y_d Y_d^\dagger Y_u)^{ab} + \frac{15}{4} \delta^{sd} \delta^{ta} Y_e^{pr} (Y_d Y_d^\dagger Y_u)^{cb} - \frac{1}{2} \delta^{ta} Y_d^{cd} Y_e^{pr} (Y_d^\dagger Y_u)^{sb} \\
& - \frac{1}{2} \delta^{sd} Y_e^{pr} Y_u^{ab} (Y_u Y_u^\dagger)^{ct} - \frac{3}{4} \delta^{tc} Y_d^{ad} Y_e^{pr} (Y_d^\dagger Y_u)^{sb} - \frac{3}{4} \delta^{sd} Y_e^{pr} Y_u^{cb} (Y_u Y_u^\dagger)^{at} - \left( 3 \delta^{sd} \delta^{tc} Y_e^{pr} Y_u^{ab} + \frac{9}{2} \delta^{sd} \delta^{ta} Y_e^{pr} Y_u^{cb} \right) \text{Tr} \left[ Y_d^\dagger Y_d \right] - \frac{9}{2} \delta^{sd} \delta^{tc} Y_e^{pr} (Y_u Y_u^\dagger Y_u)^{ab} \\
& - \frac{27}{4} \delta^{sd} \delta^{ta} Y_e^{pr} (Y_u Y_u^\dagger Y_u)^{cb} \left. \right\} + \left\{ \frac{1}{4} \delta^{pa} Y_d^{*cs} Y_u^{*td} (Y_e^\dagger Y_e)^{br} + g_s^2 \left( \frac{64}{3} \delta^{pa} \delta^{rb} Y_d^{*cs} Y_u^{*td} - 40 \delta^{pa} \delta^{rb} Y_d^{*ts} Y_u^{*cd} \right) + g_L^2 \left( \frac{9}{2} \delta^{pa} \delta^{rb} Y_d^{*cs} Y_u^{*td} \right. \right. \\
& - 9 \delta^{pa} \delta^{rb} Y_d^{*ts} Y_u^{*cd} \left. \right) + g_Y^2 \left( \frac{59}{18} \delta^{pa} \delta^{rb} Y_d^{*cs} Y_u^{*td} - \frac{19}{3} \delta^{pa} \delta^{rb} Y_d^{*ts} Y_u^{*cd} \right) + \frac{5}{4} \delta^{rb} Y_d^{*cs} Y_u^{*td} (Y_e Y_e^\dagger)^{pa} + 3 \delta^{pa} \delta^{rb} Y_d^{*ts} Y_u^{*cd} \text{Tr} \left[ Y_e^\dagger Y_e \right] \\
& + \frac{27}{2} \delta^{pa} \delta^{rb} Y_d^{*ts} (Y_u^\dagger Y_u Y_u^\dagger)^{cd} - \delta^{pa} \delta^{rb} Y_u^{*td} (Y_d^\dagger Y_d Y_d^\dagger)^{cs} - \delta^{pa} \delta^{rb} Y_u^{*td} (Y_u^\dagger Y_u Y_d^\dagger)^{cs} - \frac{3}{2} \delta^{pa} \delta^{rb} Y_d^{*ts} (Y_d^\dagger Y_d Y_u^\dagger)^{cd} - 2 T_2 \delta^{pa} \delta^{rb} Y_d^{*cs} Y_u^{*td} \\
& - 2 \delta^{pa} \delta^{rb} Y_d^{*cs} (Y_u^\dagger Y_u Y_u^\dagger)^{td} \left. \right\} C_{lequ}^{abcd} + C_{lequ}^{*abcd} \left\{ \frac{1}{2} \delta^{tc} Y_e^{pr} Y_e^{ab} (Y_d^\dagger Y_u)^{sd} + \frac{3}{2} \delta^{tc} Y_e^{pb} Y_e^{ar} (Y_d^\dagger Y_u)^{sd} + 3 Y_d^{*ts} Y_e^{pr} Y_e^{ab} Y_u^{cd} \right\} + \left\{ \frac{1}{4} \delta^{pa} \delta^{rd} Y_u^{*tb} (Y_d^\dagger Y_d Y_d^\dagger)^{cs} \right. \\
& + \frac{1}{2} Y_d^{*cs} Y_e^{*ad} Y_u^{*tb} Y_e^{pr} + \frac{1}{2} T_2 \delta^{pa} \delta^{rd} Y_d^{*cs} Y_u^{*tb} + \frac{1}{2} \delta^{pa} \delta^{rd} Y_d^{*cs} (Y_d^\dagger Y_d Y_u^\dagger)^{tb} + \frac{1}{2} \delta^{pa} \delta^{rd} Y_d^{*cs} (Y_u^\dagger Y_u Y_u^\dagger)^{tb} + \frac{3}{4} \delta^{pa} \delta^{rd} Y_u^{*tb} (Y_u^\dagger Y_u Y_d^\dagger)^{cs} \\
& + g_L^2 \left( \frac{15}{8} \delta^{pa} \delta^{rd} Y_d^{*cs} Y_u^{*tb} + \frac{45}{8} \delta^{pa} \delta^{rd} Y_d^{*ts} Y_u^{*cb} \right) + g_Y^2 \left( \frac{281}{24} \delta^{pa} \delta^{rd} Y_d^{*ts} Y_u^{*cb} - \frac{49}{24} \delta^{pa} \delta^{rd} Y_d^{*cs} Y_u^{*tb} \right) + g_s^2 \left( 34 \delta^{pa} \delta^{rd} Y_d^{*ts} Y_u^{*cb} \right. \\
& - 14 \delta^{pa} \delta^{rd} Y_d^{*cs} Y_u^{*tb} \left. \right) + \frac{7}{4} \delta^{pa} Y_d^{*cs} Y_u^{*tb} (Y_e^\dagger Y_e)^{dr} + \frac{9}{4} \delta^{pa} \delta^{rd} Y_d^{*ts} (Y_d^\dagger Y_d Y_u^\dagger)^{cb} - \frac{3}{2} \delta^{rd} Y_d^{*cs} Y_u^{*tb} (Y_e Y_e^\dagger)^{pa} - \frac{3}{2} \delta^{pa} \delta^{rd} Y_d^{*ts} Y_u^{*cb} \text{Tr} \left[ Y_e^\dagger Y_e \right] \\
& - \frac{27}{4} \delta^{pa} \delta^{rd} Y_d^{*ts} (Y_u^\dagger Y_u Y_u^\dagger)^{cb} \left. \right\} C_{luqe}^{abcd} + C_{luqe}^{*abcd} \left\{ \frac{1}{4} \delta^{tc} Y_e^{pd} Y_e^{ar} (Y_d^\dagger Y_u)^{sb} - \frac{1}{4} \delta^{tc} Y_e^{pr} Y_e^{ad} (Y_d^\dagger Y_u)^{sb} - \frac{3}{2} Y_d^{*ts} Y_e^{pr} Y_e^{ad} Y_u^{cb} \right\} + \left\{ g_Y^2 \left( \frac{2}{9} \delta^{pa} \delta^{bc} Y_d^{*ts} Y_e^{dr} \right. \right. \\
& + \frac{64}{9} \delta^{pa} \delta^{cd} Y_d^{*ts} Y_e^{br} \left. \right) + 4 \delta^{pa} Y_d^{*ts} Y_e^{br} (Y_e Y_e^\dagger)^{dc} - \frac{10}{3} \delta^{pa} \delta^{bc} g_L^2 Y_d^{*ts} Y_e^{dr} \left. \right\} C_{\ell\ell}^{abcd} + \left\{ g_Y^2 \left( \frac{74}{81} \delta^{td} \delta^{bc} Y_d^{*as} Y_e^{pr} + \frac{64}{27} \delta^{tb} \delta^{cd} Y_d^{*as} Y_e^{pr} \right) \right. \\
& + \frac{32}{27} \delta^{td} \delta^{bc} g_s^2 Y_d^{*as} Y_e^{pr} + 12 \delta^{tb} Y_d^{*as} Y_e^{pr} (Y_d Y_d^\dagger)^{dc} - 3 \delta^{td} Y_d^{*as} Y_e^{pr} (Y_u Y_u^\dagger)^{bc} - \frac{10}{3} \delta^{td} \delta^{bc} g_L^2 Y_d^{*as} Y_e^{pr} \left. \right\} C_{qq}^{(\parallel)abcd} + \left\{ g_Y^2 \left( \frac{32}{27} \delta^{tb} \delta^{cd} Y_d^{*as} Y_e^{pr} \right. \right.
\end{aligned}$$

$$\begin{aligned}
& + \frac{148}{81} \delta^{td} \delta^{bc} Y_d^{*as} Y_e^{pr} \Big) + \frac{64}{27} \delta^{td} \delta^{bc} g_s^2 Y_d^{*as} Y_e^{pr} + 3 \delta^{td} Y_d^{*as} Y_e^{pr} (Y_u Y_u^\dagger)^{bc} + 24 \delta^{tb} Y_d^{*as} Y_e^{pr} (Y_d Y_d^\dagger)^{dc} - 16 \delta^{tb} \delta^{cd} g_L^2 Y_d^{*as} Y_e^{pr} \Big\} C_{qq}^{(\times)abcd} \\
& + \left\{ \frac{1}{2} \delta^{pa} \delta^{td} Y_e^{br} (Y_u^\dagger Y_u Y_d^\dagger)^{cs} + g_Y^2 \left( \frac{79}{12} \delta^{pa} \delta^{td} Y_d^{*cs} Y_e^{br} - \frac{32}{27} \delta^{td} \delta^{ab} Y_d^{*cs} Y_e^{pr} - \frac{32}{9} \delta^{pa} \delta^{cd} Y_d^{*ts} Y_e^{br} \right) + \delta^{pa} Y_d^{*cs} Y_e^{br} (Y_d Y_d^\dagger)^{dt} + \delta^{td} Y_d^{*cs} Y_e^{br} (Y_e Y_e^\dagger)^{pa} \right. \\
& + 3 \delta^{td} Y_d^{*cs} Y_e^{pr} (Y_e Y_e^\dagger)^{ba} + 9 \delta^{pa} Y_d^{*ts} Y_e^{br} (Y_d Y_d^\dagger)^{dc} - \delta^{pa} Y_d^{*cs} Y_e^{br} (Y_u Y_u^\dagger)^{dt} - \frac{5}{2} \delta^{pa} \delta^{td} Y_e^{br} (Y_d^\dagger Y_d Y_d^\dagger)^{cs} - \frac{5}{2} \delta^{pa} \delta^{td} Y_d^{*cs} (Y_e Y_e^\dagger Y_e)^{br} \\
& - 5 T_2 \delta^{pa} \delta^{td} Y_d^{*cs} Y_e^{br} - \frac{33}{4} \delta^{pa} \delta^{td} g_L^2 Y_d^{*cs} Y_e^{br} \Big\} C_{\ell q}^{(\parallel)abcd} + \left\{ \frac{1}{2} \delta^{pa} Y_d^{*cs} Y_e^{br} (Y_d Y_d^\dagger)^{dt} + \frac{1}{2} \delta^{td} Y_d^{*cs} Y_e^{br} (Y_e Y_e^\dagger)^{pa} + g_L^2 \left( \frac{69}{2} \delta^{pa} \delta^{td} Y_d^{*cs} Y_e^{br} \right. \right. \\
& - \frac{8}{3} \delta^{td} \delta^{ab} Y_d^{*cs} Y_e^{pr} - 8 \delta^{pa} \delta^{cd} Y_d^{*ts} Y_e^{br} \Big) + g_Y^2 \left( \frac{79}{6} \delta^{pa} \delta^{td} Y_d^{*cs} Y_e^{br} - \frac{16}{27} \delta^{td} \delta^{ab} Y_d^{*cs} Y_e^{pr} - \frac{16}{9} \delta^{pa} \delta^{cd} Y_d^{*ts} Y_e^{br} \right) + \delta^{pa} Y_d^{*cs} Y_e^{br} (Y_u Y_u^\dagger)^{dt} \\
& + \delta^{pa} \delta^{td} Y_e^{br} (Y_u^\dagger Y_u Y_d^\dagger)^{cs} + 6 \delta^{td} Y_d^{*cs} Y_e^{pr} (Y_e Y_e^\dagger)^{ba} + 18 \delta^{pa} Y_d^{*ts} Y_e^{br} (Y_d Y_d^\dagger)^{dc} - 5 \delta^{pa} \delta^{td} Y_e^{br} (Y_d^\dagger Y_d Y_d^\dagger)^{cs} - 5 \delta^{pa} \delta^{td} Y_d^{*cs} (Y_e Y_e^\dagger Y_e)^{br} \\
& \left. - 10 T_2 \delta^{pa} \delta^{td} Y_d^{*cs} Y_e^{br} \right\} C_{\ell q}^{(\times)abcd}, \tag{12.2}
\end{aligned}$$

## 12.2 $C_{quqd}^{(\parallel)}$

$$\begin{aligned}
\beta_{C_{quqd}^{(\parallel)prst}}^{(1)} &= \frac{2}{3} \delta^{pa} \delta^{rb} g_Y^2 C_{uB}^{ab} Y_d^{st} + 3 \delta^{pa} \delta^{rb} g_L^2 C_{uW}^{ab} Y_d^{st} + \frac{4}{3} g_s^2 \left\{ \delta^{pa} \delta^{rb} Y_d^{st} + 6 \delta^{rb} \delta^{sa} Y_d^{pt} \right\} C_{uG}^{ab} - \frac{10}{3} \delta^{sa} \delta^{tb} g_Y^2 C_{dB}^{ab} Y_u^{pr} + 3 \delta^{sa} \delta^{tb} g_L^2 C_{dW}^{ab} Y_u^{pr} \\
& + \frac{4}{3} g_s^2 \left\{ \delta^{sa} \delta^{tb} Y_u^{pr} + 6 \delta^{pa} \delta^{tb} Y_u^{sr} \right\} C_{dG}^{ab} - 4 \delta^{pa} \delta^{rd} C_{qu}^{(\parallel)abcd} Y_d^{st} Y_u^{bc} + 4 \left\{ \delta^{pa} \delta^{rd} Y_d^{bt} Y_u^{sc} - 3 \delta^{pa} \delta^{rd} Y_d^{st} Y_u^{bc} \right\} C_{qu}^{(\times)abcd} - 4 \delta^{sa} \delta^{td} C_{qd}^{(\parallel)abcd} Y_d^{bc} Y_u^{pr} \\
& - 4 \left\{ 3 \delta^{sa} \delta^{td} Y_d^{bc} Y_u^{pr} - \delta^{sa} \delta^{td} Y_d^{pc} Y_u^{br} \right\} C_{qd}^{(\times)abcd} - 4 \delta^{rb} \delta^{td} C_{ud}^{(\parallel)abcd} Y_d^{sc} Y_u^{pa} + 4 \delta^{rb} \delta^{td} C_{ud}^{(\times)abcd} Y_d^{pc} Y_u^{sa} + 2 \delta^{sd} \delta^{tc} C_{ledq}^{*abcd} Y_e^{ab} Y_u^{pr} + \left\{ \frac{1}{2} \left( \delta^{rb} \delta^{sc} \delta^{td} (Y_d Y_d^\dagger)^{pa} \right. \right. \\
& + \delta^{pa} \delta^{rb} \delta^{td} (Y_d Y_d^\dagger)^{sc} + \delta^{rb} \delta^{sc} \delta^{td} (Y_u Y_u^\dagger)^{pa} + \delta^{pa} \delta^{rb} \delta^{td} (Y_u Y_u^\dagger)^{sc} + 2 \delta^{pc} \delta^{rb} Y_d^{*ad} Y_d^{st} + 2 \delta^{sa} \delta^{td} Y_u^{*cb} Y_u^{pr} + 2 \delta^{pa} \delta^{rb} \delta^{sc} (Y_d^\dagger Y_d)^{dt} \\
& + 2 \delta^{pa} \delta^{sc} \delta^{td} (Y_u^\dagger Y_u)^{br} + 12 \delta^{pa} \delta^{rb} Y_d^{*cd} Y_d^{st} + 12 \delta^{sc} \delta^{td} Y_u^{*ab} Y_u^{pr} \Big) - \frac{11}{18} \delta^{pa} \delta^{rb} \delta^{sc} \delta^{td} g_Y^2 - \frac{4}{3} g_s^2 \left( 6 \delta^{pc} \delta^{rb} \delta^{sa} \delta^{td} + 13 \delta^{pa} \delta^{rb} \delta^{sc} \delta^{td} \right) \\
& \left. - \frac{3}{2} \delta^{pa} \delta^{rb} \delta^{sc} \delta^{td} g_L^2 \right\} C_{quqd}^{(\parallel)abcd} + \left\{ \frac{5}{9} \delta^{pc} \delta^{rb} \delta^{sa} \delta^{td} g_Y^2 + 2 \delta^{pa} \delta^{rb} Y_d^{*cd} Y_d^{st} + 2 \delta^{sc} \delta^{td} Y_u^{*ab} Y_u^{pr} + 3 \delta^{pc} \delta^{rb} Y_d^{*ad} Y_d^{st} + 3 \delta^{sa} \delta^{td} Y_u^{*cb} Y_u^{pr} \right. \\
& + 3 \delta^{pc} \delta^{rb} \delta^{sa} \delta^{td} g_L^2 - \frac{4}{3} g_s^2 \left( 3 \delta^{pa} \delta^{rb} \delta^{sc} \delta^{td} + 7 \delta^{pc} \delta^{rb} \delta^{sa} \delta^{td} \right) \Big\} C_{quqd}^{(\times)abcd} - 2 \delta^{pc} \delta^{rd} Y_e^{*ab} C_{\ell equ}^{abcd} Y_d^{st} + \delta^{pc} \delta^{rb} Y_e^{*ad} C_{\ell uqe}^{abcd} Y_d^{st} - 8 \delta^{pa} \delta^{sc} C_{qq}^{(\parallel)abcd} Y_d^{dt} Y_u^{br} \\
& + 8 \delta^{pa} \delta^{sc} C_{qq}^{(\times)abcd} Y_d^{dt} Y_u^{br}, \tag{12.3}
\end{aligned}$$

$$\begin{aligned}
\beta_{C_{quqd}^{(II)prst}}^{(2)} = & -4Y_d^{st}Y_u^{pr}\mathbf{T}_{\ell H} + \left\{ \frac{1}{18}g_Y^2Y_d^{st}Y_u^{pr} + \frac{1}{6}g_L^2Y_d^{st}Y_u^{pr} + \lambda Y_d^{st}Y_u^{pr} - \frac{1}{2}Y_d^{st}(Y_dY_d^\dagger Y_u)^{pr} - \frac{1}{2}Y_u^{pr}(Y_uY_u^\dagger Y_d)^{st} - \frac{3}{2}Y_u^{pr}(Y_dY_d^\dagger Y_d)^{st} - \frac{3}{2}Y_d^{st}(Y_uY_u^\dagger Y_u)^{pr} \right\} C_{HD}^{(II)} \\
& + \left\{ \frac{1}{9}g_Y^2Y_d^{st}Y_u^{pr} + \frac{1}{2}Y_d^{st}(Y_dY_d^\dagger Y_u)^{pr} + \frac{1}{2}Y_u^{pr}(Y_uY_u^\dagger Y_d)^{st} + \lambda Y_d^{st}Y_u^{pr} - \frac{3}{2}Y_u^{pr}(Y_dY_d^\dagger Y_d)^{st} - \frac{3}{2}Y_d^{st}(Y_uY_u^\dagger Y_u)^{pr} \right\} C_{HD}^{(\times)} + \frac{13}{9}g_Y^4C_{HB}Y_d^{st}Y_u^{pr} \\
& - \frac{13i}{9}g_Y^4C_{H\tilde{B}}Y_d^{st}Y_u^{pr} + 3g_L^4C_{HW}Y_d^{st}Y_u^{pr} - 3ig_L^4C_{H\tilde{W}}Y_d^{st}Y_u^{pr} + \frac{64}{3}g_s^4C_{HG}Y_d^{st}Y_u^{pr} - \frac{64i}{3}g_s^4C_{H\tilde{G}}Y_d^{st}Y_u^{pr} - \frac{3}{2}g_Y^2g_L^2C_{HWB}Y_d^{st}Y_u^{pr} \\
& + \frac{3i}{2}g_Y^2g_L^2C_{H\tilde{W}B}Y_d^{st}Y_u^{pr} + \frac{57}{2}g_L^6C_WY_d^{st}Y_u^{pr} + \frac{19i}{2}g_L^6C_{\tilde{W}}Y_d^{st}Y_u^{pr} + g_s^6 \left\{ 60Y_d^{pt}Y_u^{sr} - 166Y_d^{st}Y_u^{pr} \right\} C_G + g_s^6 \left\{ 124iY_d^{pt}Y_u^{sr} - \frac{82i}{3}Y_d^{st}Y_u^{pr} \right\} C_{\tilde{G}} \\
& + \left\{ 3\delta^{pa}\delta^{rb}\lambda Y_d^{st} - 6\delta^{pa}\delta^{rb}(Y_dY_d^\dagger Y_d)^{st} \right\} C_{uH}^{ab} + \left\{ 3\delta^{sa}\delta^{tb}\lambda Y_u^{pr} - 6\delta^{sa}\delta^{tb}(Y_uY_u^\dagger Y_u)^{pr} \right\} C_{dH}^{ab} + 3g_Y^2Y_e^{*ab}C_{eB}^{ab}Y_d^{st}Y_u^{pr} + 2g_Y^2C_{eB}^{*ab}Y_d^{st}Y_e^{ab}Y_u^{pr} \\
& - \frac{3}{2}g_L^2Y_e^{*ab}C_{eW}^{ab}Y_d^{st}Y_u^{pr} + 3g_L^2C_{eW}^{*ab}Y_d^{st}Y_e^{ab}Y_u^{pr} + \left\{ \frac{7}{9}\delta^{pa}\delta^{rb}g_Y^4Y_d^{st} + g_Y^2g_s^2\left(\frac{178}{9}\delta^{pa}\delta^{rb}Y_d^{st} - \frac{34}{3}\delta^{rb}\delta^{sa}Y_d^{pt}\right) + g_Y^2\left(\frac{1}{3}\delta^{rb}Y_d^{st}(Y_dY_d^\dagger)^{pa} \right. \right. \\
& + \frac{2}{3}\delta^{pa}Y_d^{st}(Y_u^\dagger Y_u)^{br} + \frac{4}{3}\delta^{rb}Y_d^{st}(Y_uY_u^\dagger)^{pa} + 5\delta^{sa}Y_u^{pr}(Y_u^\dagger Y_d)^{bt} + 14\delta^{pa}\delta^{rb}Y_d^{st}\text{Tr}[Y_u^\dagger Y_u] - \frac{1}{3}\delta^{pa}\delta^{rb}Y_d^{st}\text{Tr}[Y_e^\dagger Y_e] - \delta^{pa}\delta^{rb}Y_d^{st}\text{Tr}[Y_d^\dagger Y_d] \\
& \left. \left. - \frac{7}{3}\delta^{pa}\delta^{rb}(Y_uY_u^\dagger Y_d)^{st} - 5Y_u^{*ab}Y_d^{st}Y_u^{pr} \right) - \frac{1}{2}\delta^{pa}\delta^{rb}g_Y^2g_L^2Y_d^{st} \right\} C_{uB}^{ab} + g_Y^2C_{uB}^{*ab} \left\{ 10Y_d^{st}Y_u^{pr}Y_u^{ab} - \frac{5}{3}Y_d^{at}Y_u^{pr}Y_u^{sb} \right\} + \left\{ g_s^2g_L^2\left(29\delta^{pa}\delta^{rb}Y_d^{st} \right. \right. \\
& - 27\delta^{rb}\delta^{sa}Y_d^{pt} \left. \left. + g_L^2\left(\frac{3}{2}\delta^{sa}Y_u^{pr}(Y_u^\dagger Y_d)^{bt} + \frac{15}{2}\delta^{rb}Y_d^{st}(Y_dY_d^\dagger)^{pa} + 9\delta^{pa}\delta^{rb}Y_d^{st}\text{Tr}[Y_u^\dagger Y_u] - \frac{3}{2}\delta^{pa}\delta^{rb}Y_d^{st}\text{Tr}[Y_e^\dagger Y_e] - \frac{9}{2}Y_u^{*ab}Y_d^{st}Y_u^{pr} \right. \right. \right. \\
& \left. \left. - \frac{9}{2}\delta^{pa}\delta^{rb}(Y_uY_u^\dagger Y_d)^{st} - \frac{9}{2}\delta^{pa}\delta^{rb}Y_d^{st}\text{Tr}[Y_d^\dagger Y_d] \right) + \frac{35}{12}\delta^{pa}\delta^{rb}g_Y^2g_L^2Y_d^{st} + \frac{59}{6}\delta^{pa}\delta^{rb}g_L^4Y_d^{st} \right\} C_{uW}^{ab} + g_L^2C_{uW}^{*ab} \left\{ 9Y_d^{st}Y_u^{pr}Y_u^{ab} - \frac{3}{2}Y_d^{at}Y_u^{pr}Y_u^{sb} \right\} \\
& + \left\{ g_s^2g_L^2\left(3\delta^{rb}\delta^{sa}Y_d^{pt} - \frac{17}{2}\delta^{pa}\delta^{rb}Y_d^{st}\right) + g_Y^2g_s^2\left(\frac{151}{54}\delta^{pa}\delta^{rb}Y_d^{st} + \frac{49}{9}\delta^{rb}\delta^{sa}Y_d^{pt}\right) + g_s^4\left(\frac{364}{9}\delta^{pa}\delta^{rb}Y_d^{st} + 80\delta^{rb}\delta^{sa}Y_d^{pt}\right) + g_s^2\left(\frac{4}{3}\delta^{pa}\delta^{rb}(Y_uY_u^\dagger Y_d)^{st} \right. \right. \\
& + \frac{7}{3}\delta^{pa}Y_d^{st}(Y_u^\dagger Y_u)^{br} + \frac{14}{3}\delta^{rb}Y_d^{st}(Y_uY_u^\dagger)^{pa} - \frac{2}{3}\text{T}_2\delta^{pa}\delta^{rb}Y_d^{st} - 2\delta^{sa}Y_d^{pt}(Y_u^\dagger Y_u)^{br} - 2\delta^{pa}\delta^{rb}(Y_dY_d^\dagger Y_d)^{st} - 4\text{T}_2\delta^{rb}\delta^{sa}Y_d^{pt} - 4\delta^{rb}Y_d^{pt}(Y_dY_d^\dagger)^{sa} \\
& - 4\delta^{rb}Y_d^{pt}(Y_uY_u^\dagger)^{sa} - 4\delta^{rb}\delta^{sa}(Y_uY_u^\dagger Y_d)^{pt} - 6\delta^{pa}Y_u^{sr}(Y_u^\dagger Y_d)^{bt} - 9\delta^{sa}Y_u^{pr}(Y_u^\dagger Y_d)^{bt} - \frac{34}{3}\delta^{rb}Y_d^{st}(Y_dY_d^\dagger)^{pa} - 12\delta^{rb}\delta^{sa}(Y_dY_d^\dagger Y_d)^{pt} \\
& \left. \left. - 16Y_u^{*ab}Y_d^{st}Y_u^{pr} \right) \right\} C_{uG}^{ab} + g_s^2C_{uG}^{*ab} \left\{ \frac{20}{3}Y_d^{at}Y_u^{pr}Y_u^{sb} - 4Y_d^{at}Y_u^{pb}Y_u^{sr} - 16Y_d^{st}Y_u^{pr}Y_u^{ab} \right\} + \left\{ g_Y^2g_s^2\left(\frac{74}{3}\delta^{pa}\delta^{tb}Y_u^{sr} - \frac{170}{9}\delta^{sa}\delta^{tb}Y_u^{pr} \right) \right. \\
& \left. + g_Y^2\left(\frac{2}{3}\delta^{sa}Y_u^{pr}(Y_d^\dagger Y_d)^{bt} + Y_d^{*ab}Y_d^{st}Y_u^{pr} + \frac{4}{3}\delta^{tb}Y_u^{pr}(Y_dY_d^\dagger)^{sa} + 2\delta^{sa}\delta^{tb}Y_u^{pr}\text{Tr}[Y_d^\dagger Y_d] + 4\delta^{sa}\delta^{tb}(Y_uY_u^\dagger Y_u)^{pr} + 5\delta^{sa}\delta^{tb}Y_u^{pr}\text{Tr}[Y_u^\dagger Y_u] \right. \right.
\end{aligned}$$

$$\begin{aligned}
& -\frac{1}{3}\delta^{sa}\delta^{tb}(Y_d Y_d^\dagger Y_u)^{pr} - \frac{5}{3}\delta^{tb}Y_u^{pr}(Y_u Y_u^\dagger)^{sa} - 5\delta^{pa}Y_d^{st}(Y_d^\dagger Y_u)^{br} - \frac{22}{3}\delta^{sa}\delta^{tb}Y_u^{pr}\text{Tr}[Y_e^\dagger Y_e] \Big) + \frac{53}{9}\delta^{sa}\delta^{tb}g_Y^4 Y_u^{pr} - \frac{19}{2}\delta^{sa}\delta^{tb}g_Y^2 g_L^2 Y_u^{pr} \Big\} C_{dB}^{ab} \\
& + g_Y^2 C_{dB}^{*ab} \Big\{ \frac{1}{3}Y_d^{pb}Y_d^{st}Y_u^{ar} - 2Y_d^{st}Y_d^{ab}Y_u^{pr} \Big\} + \Big\{ \frac{11}{12}\delta^{sa}\delta^{tb}g_Y^2 g_L^2 Y_u^{pr} + g_s^2 g_L^2 \Big( 29\delta^{sa}\delta^{tb}Y_u^{pr} - 27\delta^{pa}\delta^{tb}Y_u^{sr} \Big) + g_L^2 \Big( \frac{3}{2}\delta^{pa}Y_d^{st}(Y_d^\dagger Y_u)^{br} \\
& + 3\delta^{sa}\delta^{tb}Y_u^{pr}\text{Tr}[Y_e^\dagger Y_e] + \frac{15}{2}\delta^{tb}Y_u^{pr}(Y_u Y_u^\dagger)^{sa} + 9\delta^{sa}\delta^{tb}Y_u^{pr}\text{Tr}[Y_d^\dagger Y_d] - \frac{9}{2}Y_d^{*ab}Y_d^{st}Y_u^{pr} - \frac{9}{2}\delta^{sa}\delta^{tb}(Y_d Y_d^\dagger Y_u)^{pr} - \frac{9}{2}\delta^{sa}\delta^{tb}Y_u^{pr}\text{Tr}[Y_u^\dagger Y_u] \Big) \\
& + \frac{59}{6}\delta^{sa}\delta^{tb}g_L^4 Y_u^{pr} \Big\} C_{dW}^{ab} + g_L^2 C_{dW}^{*ab} \Big\{ 9Y_d^{st}Y_d^{ab}Y_u^{pr} - \frac{3}{2}Y_d^{pb}Y_d^{st}Y_u^{ar} \Big\} + \Big\{ g_s^2 g_L^2 \Big( 3\delta^{pa}\delta^{tb}Y_u^{sr} - \frac{17}{2}\delta^{sa}\delta^{tb}Y_u^{pr} \Big) + g_s^4 \Big( \frac{364}{9}\delta^{sa}\delta^{tb}Y_u^{pr} + 80\delta^{pa}\delta^{tb}Y_u^{sr} \Big) \\
& + g_s^2 \Big( \frac{4}{3}\delta^{sa}\delta^{tb}(Y_d Y_d^\dagger Y_u)^{pr} + \frac{7}{3}\delta^{sa}Y_u^{pr}(Y_d^\dagger Y_d)^{bt} + \frac{14}{3}\delta^{tb}Y_u^{pr}(Y_d Y_d^\dagger)^{sa} - \frac{2}{3}\text{T}_2\delta^{sa}\delta^{tb}Y_u^{pr} - 2\delta^{pa}Y_u^{sr}(Y_d^\dagger Y_d)^{bt} - 2\delta^{sa}\delta^{tb}(Y_u Y_u^\dagger Y_u)^{pr} \\
& - 4\text{T}_2\delta^{pa}\delta^{tb}Y_u^{sr} - 4\delta^{tb}Y_u^{sr}(Y_d Y_d^\dagger)^{pa} - 4\delta^{tb}Y_u^{sr}(Y_u Y_u^\dagger)^{pa} - 4\delta^{pa}\delta^{tb}(Y_d Y_d^\dagger Y_u)^{sr} - 6\delta^{sa}Y_d^{pt}(Y_d^\dagger Y_u)^{br} - 9\delta^{pa}Y_d^{st}(Y_d^\dagger Y_u)^{br} - \frac{34}{3}\delta^{tb}Y_u^{pr}(Y_u Y_u^\dagger)^{sa} \\
& - 12\delta^{pa}\delta^{tb}(Y_u Y_u^\dagger Y_u)^{sr} - 16Y_d^{*ab}Y_d^{st}Y_u^{pr} \Big) - g_Y^2 g_s^2 \Big( \frac{23}{9}\delta^{pa}\delta^{tb}Y_u^{sr} + \frac{305}{54}\delta^{sa}\delta^{tb}Y_u^{pr} \Big) \Big\} C_{dG}^{ab} + g_s^2 C_{dG}^{*ab} \Big\{ \frac{20}{3}Y_d^{pb}Y_d^{st}Y_u^{ar} - 4Y_d^{pt}Y_d^{sb}Y_u^{ar} \\
& - 16Y_d^{st}Y_d^{ab}Y_u^{pr} \Big\} - \Big\{ \frac{4}{9}\delta^{ab}g_Y^2 Y_d^{st}Y_u^{pr} + \frac{4}{3}Y_d^{st}Y_u^{pr}(Y_e Y_e^\dagger)^{ba} \Big\} C_{H\ell}^{(\parallel)ab} + \Big\{ \frac{2}{3}\delta^{ab}g_L^2 Y_d^{st}Y_u^{pr} - \frac{2}{9}\delta^{ab}g_Y^2 Y_d^{st}Y_u^{pr} - \frac{8}{3}Y_d^{st}Y_u^{pr}(Y_e Y_e^\dagger)^{ba} \Big\} C_{H\ell}^{(\times)ab} \\
& + \Big\{ \frac{4}{3}Y_d^{st}Y_u^{pr}(Y_e^\dagger Y_e)^{ba} - \frac{4}{9}\delta^{ab}g_Y^2 Y_d^{st}Y_u^{pr} \Big\} C_{He}^{ab} + \Big\{ g_L^2 \Big( \frac{3}{4}\delta^{sa}Y_d^{bt}Y_u^{pr} - \frac{3}{4}\delta^{pa}Y_d^{st}Y_u^{br} \Big) + g_s^2 \Big( 4\delta^{sa}Y_d^{bt}Y_u^{pr} + 8\delta^{sa}Y_d^{pt}Y_u^{br} - 4\delta^{pa}Y_d^{st}Y_u^{br} - 8\delta^{pa}Y_d^{bt}Y_u^{sr} \Big) \\
& + g_Y^2 \Big( \frac{4}{9}\delta^{ab}Y_d^{st}Y_u^{pr} + \frac{317}{108}\delta^{pa}Y_d^{st}Y_u^{br} - \frac{49}{108}\delta^{sa}Y_d^{bt}Y_u^{pr} \Big) + Y_d^{st}Y_u^{br}(Y_d Y_d^\dagger)^{pa} + \delta^{pa}Y_d^{st}(Y_d Y_d^\dagger Y_u)^{br} + 2Y_d^{bt}Y_u^{pr}(Y_d Y_d^\dagger)^{sa} + \frac{5}{2}\delta^{sa}Y_d^{bt}(Y_u Y_u^\dagger Y_u)^{pr} \\
& + \frac{7}{2}\delta^{pa}Y_u^{br}(Y_u Y_u^\dagger Y_d)^{st} + 4Y_d^{st}Y_u^{pr}(Y_u Y_u^\dagger)^{ba} + 6\delta^{sa}Y_u^{pr}(Y_d Y_d^\dagger Y_d)^{bt} - Y_d^{bt}Y_u^{pr}(Y_u Y_u^\dagger)^{sa} - \delta^{sa}Y_u^{pr}(Y_u Y_u^\dagger Y_d)^{bt} - 2Y_d^{st}Y_u^{br}(Y_u Y_u^\dagger)^{pa} - \frac{5}{2}\delta^{pa}Y_u^{br}(Y_d Y_d^\dagger Y_d)^{st} \\
& - \frac{7}{2}\delta^{sa}Y_d^{bt}(Y_d Y_d^\dagger Y_u)^{pr} - 4Y_d^{st}Y_u^{pr}(Y_d Y_d^\dagger)^{ba} - 6\delta^{pa}Y_d^{st}(Y_u Y_u^\dagger Y_u)^{br} \Big\} C_{Hq}^{(\parallel)ab} + \Big\{ g_s^2 \Big( 4\delta^{pa}Y_d^{st}Y_u^{br} + 8\delta^{sa}Y_d^{bt}Y_u^{pr} - 8\delta^{sa}Y_d^{pt}Y_u^{br} - 16\delta^{pa}Y_d^{bt}Y_u^{sr} \Big) \\
& + g_Y^2 \Big( \frac{2}{9}\delta^{ab}Y_d^{st}Y_u^{pr} + \frac{35}{54}\delta^{sa}Y_d^{bt}Y_u^{pr} + \frac{91}{108}\delta^{pa}Y_d^{st}Y_u^{br} \Big) + g_L^2 \Big( 2\delta^{ab}Y_d^{st}Y_u^{pr} - \frac{5}{3}\delta^{sa}Y_d^{bt}Y_u^{pr} - \frac{29}{12}\delta^{pa}Y_d^{st}Y_u^{br} \Big) + Y_d^{bt}Y_u^{pr}(Y_d Y_d^\dagger)^{sa} + Y_d^{bt}Y_u^{pr}(Y_u Y_u^\dagger)^{sa} \\
& + \delta^{pa}Y_u^{br}(Y_d Y_d^\dagger Y_d)^{st} + \delta^{sa}Y_u^{pr}(Y_u Y_u^\dagger Y_d)^{bt} + 2Y_d^{st}Y_u^{br}(Y_d Y_d^\dagger)^{pa} + 2\delta^{pa}Y_d^{st}(Y_d Y_d^\dagger Y_u)^{br} + 3\delta^{sa}Y_u^{pr}(Y_d Y_d^\dagger Y_d)^{bt} + \frac{7}{2}\delta^{sa}Y_d^{bt}(Y_d Y_d^\dagger Y_u)^{pr} \\
& + \frac{7}{2}\delta^{sa}Y_d^{bt}(Y_u Y_u^\dagger Y_u)^{pr} + 7\delta^{pa}Y_u^{br}(Y_u Y_u^\dagger Y_d)^{st} - Y_d^{st}Y_u^{br}(Y_u Y_u^\dagger)^{pa} - 3\delta^{pa}Y_d^{st}(Y_u Y_u^\dagger Y_u)^{br} - 4Y_d^{st}Y_u^{pr}(Y_u Y_u^\dagger)^{ba} - 8Y_d^{st}Y_u^{pr}(Y_d Y_d^\dagger)^{ba} \Big\} C_{Hq}^{(\times)ab} \\
& + \Big\{ g_s^2 \Big( 4\delta^{rb}Y_d^{st}Y_u^{pa} - 8\delta^{rb}Y_d^{pt}Y_u^{sa} \Big) + g_Y^2 \Big( \frac{8}{9}\delta^{ab}Y_d^{st}Y_u^{pr} + \frac{149}{108}\delta^{rb}Y_d^{st}Y_u^{pa} \Big) + Y_d^{st}Y_u^{pa}(Y_u^\dagger Y_u)^{br} + \frac{3}{2}\delta^{rb}Y_u^{pa}(Y_u Y_u^\dagger Y_d)^{st} + 3\delta^{rb}Y_d^{st}(Y_u Y_u^\dagger Y_u)^{pa}
\end{aligned}$$



$$\begin{aligned}
& + \frac{7}{2} \delta^{rb} Y_u^{pa} (Y_d Y_d^\dagger Y_d)^{st} - \frac{3}{4} \delta^{rb} g_L^2 Y_d^{st} Y_u^{pa} - 2 \delta^{rb} Y_d^{st} (Y_d Y_d^\dagger Y_u)^{pa} - 4 Y_d^{st} Y_u^{pr} (Y_u^\dagger Y_u)^{ba} \Big\} C_{Hu}^{ab} + \Big\{ \frac{3}{4} \delta^{tb} g_L^2 Y_d^{sa} Y_u^{pr} + g_s^2 (8 \delta^{tb} Y_d^{pa} Y_u^{sr} - 4 \delta^{tb} Y_d^{sa} Y_u^{pr}) \\
& + g_Y^2 \left( \frac{263}{108} \delta^{tb} Y_d^{sa} Y_u^{pr} - \frac{4}{9} \delta^{ab} Y_d^{st} Y_u^{pr} \right) + 2 \delta^{tb} Y_u^{pr} (Y_u Y_u^\dagger Y_d)^{sa} + 4 Y_d^{st} Y_u^{pr} (Y_d^\dagger Y_d)^{ba} - Y_d^{sa} Y_u^{pr} (Y_d^\dagger Y_d)^{bt} - \frac{3}{2} \delta^{tb} Y_d^{sa} (Y_d Y_d^\dagger Y_u)^{pr} - 3 \delta^{tb} Y_u^{pr} (Y_d Y_d^\dagger Y_d)^{sa} \\
& - \frac{7}{2} \delta^{tb} Y_d^{sa} (Y_u Y_u^\dagger Y_u)^{pr} \Big\} C_{Hd}^{ab} + \Big\{ \frac{3}{4} \delta^{tb} g_L^2 Y_u^{pr} Y_u^{sa} + g_s^2 (8 \delta^{tb} Y_u^{pa} Y_u^{sr} - 4 \delta^{tb} Y_u^{pr} Y_u^{sa}) + 4 Y_d^{st} Y_u^{pr} (Y_d^\dagger Y_u)^{ba} - \frac{7}{12} \delta^{tb} g_Y^2 Y_u^{pr} Y_u^{sa} - Y_u^{pr} Y_u^{sa} (Y_d^\dagger Y_d)^{bt} \\
& - \delta^{tb} Y_u^{pr} (Y_u Y_u^\dagger Y_u)^{sa} - 2 \delta^{tb} Y_u^{sa} (Y_d Y_d^\dagger Y_u)^{pr} - 2 \delta^{tb} Y_u^{sa} (Y_u Y_u^\dagger Y_u)^{pr} \Big\} C_{Hud}^{ab} + C_{Hud}^{*ab} \Big\{ \frac{5}{12} \delta^{ra} g_Y^2 Y_d^{pb} Y_d^{st} + \frac{3}{4} \delta^{ra} g_L^2 Y_d^{pb} Y_d^{st} + g_s^2 (8 \delta^{ra} Y_d^{pt} Y_d^{sb} \\
& - 4 \delta^{ra} Y_d^{pb} Y_d^{st}) + 4 Y_d^{st} Y_u^{pr} (Y_u^\dagger Y_d)^{ab} - Y_d^{pb} Y_d^{st} (Y_u^\dagger Y_u)^{ar} - \delta^{ra} Y_d^{st} (Y_d Y_d^\dagger Y_d)^{pb} - 2 \delta^{ra} Y_d^{pb} (Y_d Y_d^\dagger Y_d)^{st} - 2 \delta^{ra} Y_d^{pb} (Y_u Y_u^\dagger Y_d)^{st} \Big\} - 4 Y_e^{*ad} C_{\ell e}^{abcd} Y_d^{st} Y_e^{bc} Y_u^{pr} \\
& + \frac{8}{27} \delta^{rd} \delta^{ab} g_Y^2 C_{\ell u}^{abcd} Y_d^{st} Y_u^{pc} + \Big\{ 3 \delta^{td} Y_d^{sc} Y_u^{pr} (Y_e Y_e^\dagger)^{ba} - \frac{40}{27} \delta^{td} \delta^{ab} g_Y^2 Y_d^{sc} Y_u^{pr} \Big\} C_{\ell d}^{abcd} + \Big\{ g_Y^2 \left( \frac{44}{27} \delta^{sa} \delta^{cd} Y_d^{bt} Y_u^{pr} - \frac{76}{27} \delta^{pa} \delta^{cd} Y_d^{st} Y_u^{br} \right) \\
& + 3 \delta^{sa} Y_d^{bt} Y_u^{pr} (Y_e^\dagger Y_e)^{dc} \Big\} C_{qe}^{abcd} + \Big\{ \frac{1}{2} \delta^{sa} Y_d^{bt} Y_u^{pc} (Y_u^\dagger Y_u)^{dr} + \frac{1}{2} \delta^{rd} \delta^{sa} Y_u^{pc} (Y_u Y_u^\dagger Y_d)^{bt} + g_s^2 \left( \frac{23}{3} \delta^{rd} \delta^{sa} Y_d^{bt} Y_u^{pc} + 12 \delta^{pa} \delta^{rd} Y_d^{bt} Y_u^{sc} - 8 \delta^{rd} \delta^{sa} Y_d^{pt} Y_u^{bc} \right. \\
& - 12 \delta^{pa} \delta^{rd} Y_d^{st} Y_u^{bc} \Big) + g_Y^2 \left( \frac{13}{18} \delta^{rd} \delta^{sa} Y_d^{bt} Y_u^{pc} + \frac{152}{27} \delta^{pa} \delta^{cd} Y_d^{st} Y_u^{br} - \frac{8}{27} \delta^{rd} \delta^{ab} Y_d^{st} Y_u^{pc} - \frac{5}{3} \delta^{pa} \delta^{rd} Y_d^{st} Y_u^{bc} - \frac{88}{27} \delta^{sa} \delta^{cd} Y_d^{bt} Y_u^{pr} \right) + \delta^{rd} Y_d^{bt} Y_u^{pc} (Y_d Y_d^\dagger)^{sa} \\
& + \delta^{rd} \delta^{sa} Y_d^{bt} (Y_d Y_d^\dagger Y_u)^{pc} + 2 \delta^{pa} \delta^{rd} Y_u^{bc} (Y_u Y_u^\dagger Y_d)^{st} + \frac{5}{2} Y_u^{*ad} Y_d^{bt} Y_u^{pr} Y_u^{sc} + 6 \delta^{pa} \delta^{rd} Y_d^{st} Y_u^{bc} \text{Tr}[Y_u^\dagger Y_u] + 12 \delta^{pa} Y_d^{st} Y_u^{br} (Y_u^\dagger Y_u)^{dc} + 12 \delta^{rd} Y_d^{st} Y_u^{pc} (Y_u Y_u^\dagger)^{ba} \\
& + 12 \delta^{pa} \delta^{rd} Y_d^{st} (Y_u Y_u^\dagger Y_u)^{bc} - \frac{1}{2} \delta^{rd} \delta^{sa} Y_u^{pc} (Y_d Y_d^\dagger Y_d)^{bt} - T_2 \delta^{rd} \delta^{sa} Y_d^{bt} Y_u^{pc} - g_L^2 \left( \frac{3}{2} \delta^{rd} \delta^{sa} Y_d^{bt} Y_u^{pc} + 3 \delta^{pa} \delta^{rd} Y_d^{st} Y_u^{bc} \right) - \delta^{rd} \delta^{sa} Y_d^{bt} (Y_u Y_u^\dagger Y_u)^{pc} \\
& - \frac{5}{2} \delta^{pa} Y_u^{sc} Y_u^{br} (Y_u^\dagger Y_d)^{dt} - 3 \delta^{rd} Y_d^{bt} Y_u^{pc} (Y_u Y_u^\dagger)^{sa} - \frac{7}{2} \delta^{pa} \delta^{rd} Y_d^{st} (Y_d Y_d^\dagger Y_u)^{bc} - 6 Y_u^{*ad} Y_d^{st} Y_u^{pr} Y_u^{bc} \Big\} C_{qu}^{(\parallel)abcd} + \Big\{ g_Y^2 \left( \frac{152}{81} \delta^{pa} \delta^{cd} Y_d^{st} Y_u^{br} - \frac{8}{81} \delta^{rd} \delta^{ab} Y_d^{st} Y_u^{pc} \right. \\
& - \frac{88}{81} \delta^{sa} \delta^{cd} Y_d^{bt} Y_u^{pr} - \frac{35}{9} \delta^{pa} \delta^{rd} Y_d^{bt} Y_u^{sc} - 5 \delta^{pa} \delta^{rd} Y_d^{st} Y_u^{bc} \Big) + g_s^2 \left( \frac{110}{27} \delta^{pa} \delta^{cd} Y_d^{st} Y_u^{br} + \frac{110}{27} \delta^{sa} \delta^{cd} Y_d^{bt} Y_u^{pr} + 6 \delta^{rd} \delta^{sa} Y_d^{bt} Y_u^{pc} + \frac{220}{27} \delta^{rd} \delta^{ab} Y_d^{st} Y_u^{pc} \right. \\
& + \frac{82}{3} \delta^{pa} \delta^{rd} Y_d^{bt} Y_u^{sc} - \frac{7}{9} \delta^{pa} \delta^{cd} Y_d^{bt} Y_u^{sr} - \frac{7}{9} \delta^{sa} \delta^{cd} Y_d^{pt} Y_u^{br} - \frac{8}{9} \delta^{rd} \delta^{ab} Y_d^{pt} Y_u^{sc} - 128 \delta^{pa} \delta^{rd} Y_d^{st} Y_u^{bc} \Big) + \frac{3}{2} \delta^{rd} Y_d^{bt} Y_u^{sc} (Y_u Y_u^\dagger)^{pa} + 4 \delta^{pa} Y_d^{st} Y_u^{br} (Y_u^\dagger Y_u)^{dc} \\
& + 4 \delta^{rd} Y_d^{st} Y_u^{pc} (Y_u Y_u^\dagger)^{ba} + 6 \delta^{pa} \delta^{rd} Y_u^{bc} (Y_u Y_u^\dagger Y_d)^{st} + \frac{15}{2} Y_u^{*ad} Y_d^{bt} Y_u^{pr} Y_u^{sc} + 18 \delta^{pa} \delta^{rd} Y_d^{st} Y_u^{bc} \text{Tr}[Y_u^\dagger Y_u] + 36 \delta^{pa} \delta^{rd} Y_d^{st} (Y_u Y_u^\dagger Y_u)^{bc} \\
& - g_L^2 \left( 3 \delta^{pa} \delta^{rd} Y_d^{bt} Y_u^{sc} + 9 \delta^{pa} \delta^{rd} Y_d^{st} Y_u^{bc} \right) - \delta^{sa} Y_u^{pc} Y_u^{br} (Y_u^\dagger Y_d)^{dt} - \delta^{pa} \delta^{rd} Y_u^{sc} (Y_d Y_d^\dagger Y_d)^{bt} - 2 T_2 \delta^{pa} \delta^{rd} Y_d^{bt} Y_u^{sc} - 2 \delta^{pa} \delta^{rd} Y_d^{bt} (Y_d Y_d^\dagger Y_u)^{sc} \\
& - 2 \delta^{pa} \delta^{rd} Y_d^{bt} (Y_u Y_u^\dagger Y_u)^{sc} - \frac{5}{2} \delta^{pa} Y_d^{bt} Y_u^{sc} (Y_u^\dagger Y_u)^{dr} - 3 \delta^{pa} \delta^{rd} Y_u^{sc} (Y_u Y_u^\dagger Y_d)^{bt} - 6 \delta^{rd} Y_d^{bt} Y_u^{sc} (Y_d Y_d^\dagger)^{pa} - \frac{21}{2} \delta^{pa} \delta^{rd} Y_d^{st} (Y_d Y_d^\dagger Y_u)^{bc}
\end{aligned}$$

$$\begin{aligned}
& -18Y_u^* ad Y_d^{st} Y_u^{pr} Y_u^{bc} \Big\} C_{qu}^{(\times)abcd} + \left\{ \frac{1}{2} \delta^{pa} Y_d^{sc} Y_u^{br} (Y_d^\dagger Y_d)^{dt} + \frac{1}{2} \delta^{pa} \delta^{td} Y_d^{sc} (Y_d Y_d^\dagger Y_u)^{br} + g_s^2 \left( \frac{23}{3} \delta^{pa} \delta^{td} Y_d^{sc} Y_u^{br} + 12 \delta^{sa} \delta^{td} Y_d^{pc} Y_u^{br} - 8 \delta^{pa} \delta^{td} Y_d^{bc} Y_u^{sr} \right. \right. \\
& - 12 \delta^{sa} \delta^{td} Y_d^{bc} Y_u^{pr} \Big) + g_Y^2 \left( \frac{40}{27} \delta^{td} \delta^{ab} Y_d^{sc} Y_u^{pr} + \frac{44}{27} \delta^{sa} \delta^{cd} Y_d^{bt} Y_u^{pr} - \frac{5}{18} \delta^{pa} \delta^{td} Y_d^{sc} Y_u^{br} - \frac{1}{3} \delta^{sa} \delta^{td} Y_d^{bc} Y_u^{pr} - \frac{76}{27} \delta^{pa} \delta^{cd} Y_d^{st} Y_u^{br} \right) + \delta^{td} Y_d^{sc} Y_u^{br} (Y_u Y_u^\dagger)^{pa} \\
& + \delta^{pa} \delta^{td} Y_u^{br} (Y_u Y_u^\dagger Y_d)^{sc} + 2 \delta^{sa} \delta^{td} Y_d^{bc} (Y_d Y_d^\dagger Y_u)^{pr} + \frac{5}{2} Y_d^* ad Y_d^{pc} Y_d^{st} Y_u^{br} + 6 \delta^{sa} \delta^{td} Y_d^{bc} Y_u^{pr} \text{Tr}[Y_d^\dagger Y_d] + 12 \delta^{sa} Y_d^{bt} Y_u^{pr} (Y_d^\dagger Y_d)^{dc} + 12 \delta^{td} Y_d^{sc} Y_u^{pr} (Y_d Y_d^\dagger)^{ba} \\
& + 12 \delta^{sa} \delta^{td} Y_u^{pr} (Y_d Y_d^\dagger Y_d)^{bc} - \frac{1}{2} \delta^{pa} \delta^{td} Y_d^{sc} (Y_u Y_u^\dagger Y_u)^{br} - T_2 \delta^{pa} \delta^{td} Y_d^{sc} Y_u^{br} - g_L^2 \left( \frac{3}{2} \delta^{pa} \delta^{td} Y_d^{sc} Y_u^{br} + 3 \delta^{sa} \delta^{td} Y_d^{bc} Y_u^{pr} \right) - \delta^{pa} \delta^{td} Y_u^{br} (Y_d Y_d^\dagger Y_d)^{sc} \\
& - \frac{5}{2} \delta^{sa} Y_d^{pc} Y_d^{bt} (Y_d^\dagger Y_u)^{dr} - 3 \delta^{td} Y_d^{sc} Y_u^{br} (Y_d Y_d^\dagger)^{pa} - \frac{7}{2} \delta^{sa} \delta^{td} Y_u^{pr} (Y_u Y_u^\dagger Y_d)^{bc} - 6 Y_d^* ad Y_d^{st} Y_d^{bc} Y_u^{pr} \Big\} C_{qd}^{(\parallel)abcd} + \left\{ g_Y^2 \left( \frac{40}{81} \delta^{td} \delta^{ab} Y_d^{sc} Y_u^{pr} + \frac{44}{81} \delta^{sa} \delta^{cd} Y_d^{bt} Y_u^{pr} \right. \right. \\
& + \frac{7}{9} \delta^{sa} \delta^{td} Y_d^{pc} Y_u^{br} - \frac{76}{81} \delta^{pa} \delta^{cd} Y_d^{st} Y_u^{br} - \delta^{sa} \delta^{td} Y_d^{bc} Y_u^{pr} \Big) + g_s^2 \left( \frac{110}{27} \delta^{pa} \delta^{cd} Y_d^{st} Y_u^{br} + \frac{110}{27} \delta^{sa} \delta^{cd} Y_d^{bt} Y_u^{pr} + 6 \delta^{pa} \delta^{td} Y_d^{sc} Y_u^{br} + \frac{220}{27} \delta^{td} \delta^{ab} Y_d^{sc} Y_u^{pr} \right. \\
& + \frac{82}{3} \delta^{sa} \delta^{td} Y_d^{pc} Y_u^{br} - \frac{7}{9} \delta^{pa} \delta^{cd} Y_d^{bt} Y_u^{sr} - \frac{7}{9} \delta^{sa} \delta^{cd} Y_d^{pt} Y_u^{br} - \frac{8}{9} \delta^{td} \delta^{ab} Y_d^{pc} Y_u^{sr} - 128 \delta^{sa} \delta^{td} Y_d^{bc} Y_u^{pr} \Big) + \frac{3}{2} \delta^{td} Y_d^{pc} Y_u^{br} (Y_d Y_d^\dagger)^{sa} + 4 \delta^{sa} Y_d^{bt} Y_u^{pr} (Y_d^\dagger Y_d)^{dc} \\
& + 4 \delta^{td} Y_d^{sc} Y_u^{pr} (Y_d Y_d^\dagger)^{ba} + 6 \delta^{sa} \delta^{td} Y_d^{bc} (Y_d Y_d^\dagger Y_u)^{pr} + \frac{15}{2} Y_d^* ad Y_d^{pc} Y_d^{st} Y_u^{br} + 18 \delta^{sa} \delta^{td} Y_d^{bc} Y_u^{pr} \text{Tr}[Y_d^\dagger Y_d] + 36 \delta^{sa} \delta^{td} Y_u^{pr} (Y_d Y_d^\dagger Y_d)^{bc} \\
& - g_L^2 \left( 3 \delta^{sa} \delta^{td} Y_d^{pc} Y_u^{br} + 9 \delta^{sa} \delta^{td} Y_d^{bc} Y_u^{pr} \right) - \delta^{pa} Y_d^{sc} Y_d^{bt} (Y_d^\dagger Y_u)^{dr} - \delta^{sa} \delta^{td} Y_d^{pc} (Y_u Y_u^\dagger Y_u)^{br} - 2 T_2 \delta^{sa} \delta^{td} Y_d^{pc} Y_u^{br} - 2 \delta^{sa} \delta^{td} Y_u^{br} (Y_d Y_d^\dagger Y_d)^{pc} \\
& - 2 \delta^{sa} \delta^{td} Y_u^{br} (Y_u Y_u^\dagger Y_d)^{pc} - \frac{5}{2} \delta^{sa} Y_d^{pc} Y_u^{br} (Y_d^\dagger Y_d)^{dt} - 3 \delta^{sa} \delta^{td} Y_d^{pc} (Y_d Y_d^\dagger Y_u)^{br} - 6 \delta^{td} Y_d^{pc} Y_u^{br} (Y_u Y_u^\dagger)^{sa} - \frac{21}{2} \delta^{sa} \delta^{td} Y_u^{pr} (Y_u Y_u^\dagger Y_d)^{bc} \\
& - 18 Y_d^* ad Y_d^{st} Y_d^{bc} Y_u^{pr} \Big\} C_{qd}^{(\times)abcd} + \left\{ g_s^2 \left( \frac{52}{27} \delta^{rb} \delta^{ad} Y_d^{st} Y_u^{pc} + \frac{40}{9} \delta^{rb} \delta^{ad} Y_d^{pt} Y_u^{sc} \right) + g_Y^2 \left( \frac{16}{81} \delta^{rb} \delta^{ad} Y_d^{st} Y_u^{pc} - \frac{32}{27} \delta^{rb} \delta^{cd} Y_d^{st} Y_u^{pa} \right) + 12 \delta^{rb} Y_d^{st} Y_u^{pa} (Y_u^\dagger Y_u)^{dc} \right. \\
& - 5 \delta^{rb} Y_u^{pa} Y_u^{sc} (Y_u^\dagger Y_d)^{dt} \Big\} C_{uu}^{abcd} + \left\{ g_s^2 \left( \frac{52}{27} \delta^{tb} \delta^{ad} Y_d^{sc} Y_u^{pr} + \frac{40}{9} \delta^{tb} \delta^{ad} Y_d^{pc} Y_u^{sr} \right) + g_Y^2 \left( \frac{40}{81} \delta^{tb} \delta^{ad} Y_d^{sc} Y_u^{pr} - \frac{80}{27} \delta^{tb} \delta^{cd} Y_d^{sa} Y_u^{pr} \right) + 12 \delta^{tb} Y_d^{sa} Y_u^{pr} (Y_d^\dagger Y_d)^{dc} \right. \\
& - 5 \delta^{tb} Y_d^{pc} Y_d^{sa} (Y_d^\dagger Y_u)^{dr} \Big\} C_{dd}^{abcd} + \frac{8}{27} \delta^{rd} \delta^{ab} g_Y^2 C_{eu}^{abcd} Y_d^{st} Y_u^{pc} + \left\{ 3 \delta^{td} Y_d^{sc} Y_u^{pr} (Y_e^\dagger Y_e)^{ba} - \frac{40}{27} \delta^{td} \delta^{ab} g_Y^2 Y_d^{sc} Y_u^{pr} \right\} C_{ed}^{abcd} + \left\{ g_s^2 \left( \frac{1}{3} \delta^{rb} \delta^{td} Y_d^{sc} Y_u^{pa} \right. \right. \\
& - 8 \delta^{rb} \delta^{td} Y_d^{pc} Y_u^{sa} \Big) + g_Y^2 \left( \frac{8}{27} \delta^{rb} \delta^{cd} Y_d^{st} Y_u^{pa} + \frac{80}{27} \delta^{td} \delta^{ab} Y_d^{sc} Y_u^{pr} - \frac{68}{9} \delta^{rb} \delta^{td} Y_d^{sc} Y_u^{pa} \right) + \delta^{rb} \delta^{td} Y_d^{sc} (Y_d Y_d^\dagger Y_u)^{pa} + \delta^{rb} \delta^{td} Y_u^{pa} (Y_u Y_u^\dagger Y_d)^{sc} \\
& + \frac{5}{2} \delta^{rb} Y_d^{sc} Y_u^{pa} (Y_d^\dagger Y_d)^{dt} + \frac{5}{2} \delta^{td} Y_d^{sc} Y_u^{pa} (Y_u^\dagger Y_u)^{br} + 3 T_2 \delta^{rb} \delta^{td} Y_d^{sc} Y_u^{pa} + 3 \delta^{rb} \delta^{td} Y_u^{pa} (Y_d Y_d^\dagger Y_d)^{sc} + 3 \delta^{rb} \delta^{td} Y_d^{sc} (Y_u Y_u^\dagger Y_u)^{pa} - \frac{3}{2} \delta^{rb} Y_d^{pc} Y_d^{st} (Y_d^\dagger Y_u)^{da} \\
& - \frac{3}{2} \delta^{td} Y_u^{pr} Y_u^{sa} (Y_u^\dagger Y_d)^{bc} - 9 \delta^{rb} \delta^{td} g_L^2 Y_d^{sc} Y_u^{pa} \Big\} C_{ud}^{(\parallel)abcd} + \left\{ g_Y^2 \left( \frac{8}{81} \delta^{rb} \delta^{cd} Y_d^{st} Y_u^{pa} + \frac{80}{81} \delta^{td} \delta^{ab} Y_d^{sc} Y_u^{pr} + \frac{16}{3} \delta^{rb} \delta^{td} Y_d^{pc} Y_u^{sa} \right) + g_s^2 \left( 4 \delta^{rb} \delta^{td} Y_d^{pc} Y_u^{sa} \right. \right. \\
& + \frac{110}{27} \delta^{td} \delta^{ab} Y_d^{sc} Y_u^{pr} + \frac{110}{27} \delta^{rb} \delta^{cd} Y_d^{st} Y_u^{pa} + 17 \delta^{rb} \delta^{td} Y_d^{sc} Y_u^{pa} - \frac{4}{9} \delta^{td} \delta^{ab} Y_d^{pc} Y_u^{sr} - \frac{4}{9} \delta^{rb} \delta^{cd} Y_d^{pt} Y_u^{sa} \Big) + 6 \delta^{rb} \delta^{td} g_L^2 Y_d^{pc} Y_u^{sa} - 2 T_2 \delta^{rb} \delta^{td} Y_d^{pc} Y_u^{sa}
\end{aligned}$$

$$\begin{aligned}
& -2\delta^{rb}\delta^{td}Y_u^{sa}(Y_dY_d^\dagger Y_d)^{pc} - 2\delta^{rb}\delta^{td}Y_d^{pc}(Y_dY_d^\dagger Y_u)^{sa} - 2\delta^{rb}\delta^{td}Y_u^{sa}(Y_uY_u^\dagger Y_d)^{pc} - 2\delta^{rb}\delta^{td}Y_d^{pc}(Y_uY_u^\dagger Y_u)^{sa} - 3\delta^{rb}Y_d^{pc}Y_u^{sa}(Y_d^\dagger Y_d)^{dt} \\
& - 3\delta^{td}Y_d^{pc}Y_u^{sa}(Y_u^\dagger Y_u)^{br} - \frac{9}{2}\delta^{rb}Y_d^{pc}Y_d^{st}(Y_d^\dagger Y_u)^{da} - \frac{9}{2}\delta^{td}Y_u^{pr}Y_u^{sa}(Y_u^\dagger Y_d)^{bc} \Big\} C_{ud}^{(\times)abcd} - \left\{ Y_e^{*ab}Y_d^{pc}Y_d^{st}Y_u^{dr} + 3Y_e^{*ab}Y_d^{st}Y_d^{dc}Y_u^{pr} \right\} C_{ledq}^{abcd} \\
& + C_{ledq}^{*abcd} \left\{ g_s^2 \left( \frac{2}{3}\delta^{sd}\delta^{tc}Y_e^{ab}Y_u^{pr} + 4\delta^{pd}\delta^{tc}Y_e^{ab}Y_u^{sr} \right) + \frac{167}{36}\delta^{sd}\delta^{tc}g_Y^2Y_e^{ab}Y_u^{pr} - \frac{1}{2}\delta^{pd}Y_d^{st}Y_e^{ab}(Y_d^\dagger Y_u)^{cr} - \frac{1}{2}\delta^{tc}Y_e^{ab}Y_u^{pr}(Y_uY_u^\dagger)^{sd} - \frac{3}{4}\delta^{sd}\delta^{tc}g_L^2Y_e^{ab}Y_u^{pr} \right. \\
& - \delta^{sd}\delta^{tc}Y_e^{ab}(Y_dY_d^\dagger Y_u)^{pr} - 3\delta^{sd}\delta^{tc}Y_e^{ab}Y_u^{pr} \text{Tr}[Y_d^\dagger Y_d] - \frac{9}{2}\delta^{sd}\delta^{tc}Y_u^{pr}(Y_eY_e^\dagger Y_e)^{ab} \Big\} + \left\{ \frac{7}{8}\delta^{pa}\delta^{rb}\delta^{sc}\delta^{td}g_Y^2g_L^2 + g_Y^2g_s^2 \left( \frac{29}{6}\delta^{pc}\delta^{rb}\delta^{sa}\delta^{td} \right. \right. \\
& + \frac{188}{27}\delta^{pa}\delta^{rb}\delta^{sc}\delta^{td} \Big) + g_s^2g_L^2 \left( \frac{33}{2}\delta^{pc}\delta^{rb}\delta^{sa}\delta^{td} + 24\delta^{pa}\delta^{rb}\delta^{sc}\delta^{td} \right) + g_Y^2 \left( \frac{9}{8}\delta^{pa}\delta^{sc}\delta^{td}(Y_u^\dagger Y_u)^{br} + \frac{13}{8}\delta^{pa}\delta^{rb}\delta^{sc}(Y_d^\dagger Y_d)^{dt} + \frac{109}{48}\delta^{pa}\delta^{rb}\delta^{td}(Y_dY_d^\dagger)^{sc} \right. \\
& + \frac{185}{48}\delta^{rb}\delta^{sc}\delta^{td}(Y_uY_u^\dagger)^{pa} + \frac{9}{2}\delta^{sc}\delta^{td}Y_u^{*ab}Y_u^{pr} - \frac{19}{72}\delta^{pc}\delta^{rb}Y_d^{*ad}Y_d^{st} - \frac{19}{48}\delta^{rb}\delta^{sc}\delta^{td}(Y_dY_d^\dagger)^{pa} - \frac{31}{72}\delta^{sa}\delta^{td}Y_u^{*cb}Y_u^{pr} - \frac{1}{2}\delta^{pa}\delta^{rb}Y_d^{*cd}Y_d^{st} \\
& - \frac{71}{48}\delta^{pa}\delta^{rb}\delta^{td}(Y_uY_u^\dagger)^{sc} \Big) + g_L^2 \left( \frac{33}{16}\delta^{rb}\delta^{sc}\delta^{td}(Y_dY_d^\dagger)^{pa} + \frac{33}{16}\delta^{pa}\delta^{rb}\delta^{td}(Y_dY_d^\dagger)^{sc} + \frac{33}{16}\delta^{rb}\delta^{sc}\delta^{td}(Y_uY_u^\dagger)^{pa} + \frac{33}{16}\delta^{pa}\delta^{rb}\delta^{td}(Y_uY_u^\dagger)^{sc} + \frac{9}{2}\delta^{pa}\delta^{rb}Y_d^{*cd}Y_d^{st} \right. \\
& + \frac{9}{2}\delta^{sc}\delta^{td}Y_u^{*ab}Y_u^{pr} + \frac{51}{8}\delta^{pa}\delta^{rb}\delta^{sc}(Y_d^\dagger Y_d)^{dt} + \frac{51}{8}\delta^{pa}\delta^{sc}\delta^{td}(Y_u^\dagger Y_u)^{br} - \frac{9}{8}\delta^{pc}\delta^{rb}Y_d^{*ad}Y_d^{st} - \frac{9}{8}\delta^{sa}\delta^{td}Y_u^{*cb}Y_u^{pr} \Big) + g_s^2 \left( 4\delta^{rb}\delta^{sa}\delta^{td}(Y_dY_d^\dagger)^{pc} \right. \\
& + 4\delta^{pc}\delta^{rb}\delta^{td}(Y_dY_d^\dagger)^{sa} + 4\delta^{rb}\delta^{sa}\delta^{td}(Y_uY_u^\dagger)^{pc} + 4\delta^{pc}\delta^{rb}\delta^{td}(Y_uY_u^\dagger)^{sa} + 6\delta^{rb}\delta^{sc}\delta^{td}(Y_dY_d^\dagger)^{pa} + 6\delta^{pa}\delta^{rb}\delta^{td}(Y_dY_d^\dagger)^{sc} + 6\delta^{rb}\delta^{sc}\delta^{td}(Y_uY_u^\dagger)^{pa} \\
& + 6\delta^{pa}\delta^{rb}\delta^{td}(Y_uY_u^\dagger)^{sc} + 8\delta^{rb}\delta^{sc}Y_d^{*ad}Y_d^{pt} + 8\delta^{pa}\delta^{td}Y_u^{*cb}Y_u^{sr} + 8\delta^{pc}\delta^{rb}\delta^{sa}(Y_d^\dagger Y_d)^{dt} + 8\delta^{pc}\delta^{sa}\delta^{td}(Y_u^\dagger Y_u)^{br} + 12\delta^{rb}\delta^{sa}Y_d^{*cd}Y_d^{pt} \\
& + 12\delta^{pc}\delta^{td}Y_u^{*ab}Y_u^{sr} + 12\delta^{pa}\delta^{rb}\delta^{sc}(Y_d^\dagger Y_d)^{dt} + 12\delta^{pa}\delta^{sc}\delta^{td}(Y_u^\dagger Y_u)^{br} + \frac{40}{3}\delta^{pc}\delta^{rb}Y_d^{*ad}Y_d^{st} + \frac{40}{3}\delta^{sa}\delta^{td}Y_u^{*cb}Y_u^{pr} + 42\delta^{pa}\delta^{rb}Y_d^{*cd}Y_d^{st} \\
& + 42\delta^{sc}\delta^{td}Y_u^{*ab}Y_u^{pr} \Big) + \frac{5}{4}\delta^{sa}\delta^{td}Y_u^{pr}(Y_d^\dagger Y_dY_u^\dagger)^{cb} + \frac{5}{4}\delta^{pc}\delta^{rb}Y_d^{st}(Y_u^\dagger Y_uY_d^\dagger)^{ad} + 2\delta^{pa}\delta^{rb}(Y_d^\dagger Y_d)^{dt}(Y_dY_d^\dagger)^{sc} + 2\delta^{sc}\delta^{td}(Y_u^\dagger Y_u)^{br}(Y_uY_u^\dagger)^{pa} \\
& + \frac{9}{2}\delta^{sc}\delta^{td}Y_u^{pr}(Y_d^\dagger Y_dY_u^\dagger)^{ab} + \frac{9}{2}\delta^{pa}\delta^{rb}Y_d^{st}(Y_u^\dagger Y_uY_d^\dagger)^{cd} - \frac{1}{4}\delta^{pa}Y_u^{*cb}Y_d^{st}(Y_d^\dagger Y_u)^{dr} - \frac{1}{4}\delta^{sc}Y_d^{*ad}Y_u^{pr}(Y_u^\dagger Y_d)^{bt} - \frac{1}{4}\delta^{rb}Y_d^{*ad}Y_d^{st}(Y_dY_d^\dagger)^{pc} \\
& - \frac{1}{4}\delta^{td}Y_u^{*cb}Y_u^{pr}(Y_uY_u^\dagger)^{sa} - \frac{1}{4}\delta^{pa}\delta^{rb}\delta^{sc}(Y_d^\dagger Y_dY_d^\dagger Y_d)^{dt} - \frac{1}{4}\delta^{pa}\delta^{rb}\delta^{sc}(Y_d^\dagger Y_uY_u^\dagger Y_d)^{dt} - \frac{1}{4}\delta^{pa}\delta^{sc}\delta^{td}(Y_u^\dagger Y_dY_d^\dagger Y_u)^{br} - \frac{1}{4}\delta^{pa}\delta^{sc}\delta^{td}(Y_u^\dagger Y_uY_u^\dagger Y_u)^{br} \\
& - \frac{1}{4}\delta^{rb}\delta^{sc}\delta^{td}(Y_dY_d^\dagger Y_dY_d^\dagger)^{pa} - \frac{1}{4}\delta^{pa}\delta^{rb}\delta^{td}(Y_dY_d^\dagger Y_dY_d^\dagger)^{sc} - \frac{1}{4}\delta^{rb}\delta^{sc}\delta^{td}(Y_uY_u^\dagger Y_uY_u^\dagger)^{pa} - \frac{1}{4}\delta^{pa}\delta^{rb}\delta^{td}(Y_uY_u^\dagger Y_uY_u^\dagger)^{sc} - \frac{1}{2}\delta^{sa}\delta^{td}Y_u^{*cb}(Y_dY_d^\dagger Y_u)^{pr} \\
& - \frac{1}{2}\delta^{pc}\delta^{rb}Y_d^{*ad}(Y_uY_u^\dagger Y_d)^{st} - \frac{29}{48}\delta^{pa}\delta^{rb}\delta^{sc}\delta^{td}g_L^4 - \frac{3}{4}\text{T}_2\delta^{rb}\delta^{sc}\delta^{td}(Y_dY_d^\dagger)^{pa} - \frac{3}{4}\text{T}_2\delta^{pa}\delta^{rb}\delta^{td}(Y_dY_d^\dagger)^{sc} - \frac{3}{4}\text{T}_2\delta^{rb}\delta^{sc}\delta^{td}(Y_uY_u^\dagger)^{pa} \\
& - \frac{3}{4}\text{T}_2\delta^{pa}\delta^{rb}\delta^{td}(Y_uY_u^\dagger)^{sc} - g_s^4 \left( \frac{364}{3}\delta^{pc}\delta^{rb}\delta^{sa}\delta^{td} + \frac{2080}{9}\delta^{pa}\delta^{rb}\delta^{sc}\delta^{td} \right) - \delta^{sc}\delta^{td}(Y_u^\dagger Y_u)^{br}(Y_dY_d^\dagger)^{pa} - \delta^{pa}\delta^{rb}(Y_d^\dagger Y_d)^{dt}(Y_uY_u^\dagger)^{sc} - \left( \frac{3}{2}\delta^{sa}\delta^{td}Y_u^{*cb}Y_u^{pr} \right. \\
& + 9\delta^{sc}\delta^{td}Y_u^{*ab}Y_u^{pr} \Big) \text{Tr}[Y_d^\dagger Y_d] - \left( \frac{3}{2}\delta^{pc}\delta^{rb}Y_d^{*ad}Y_d^{st} + 9\delta^{pa}\delta^{rb}Y_d^{*cd}Y_d^{st} \right) \text{Tr}[Y_u^\dagger Y_u] - \frac{5}{4}\delta^{pa}\delta^{td}(Y_u^\dagger Y_u)^{br}(Y_dY_d^\dagger)^{sc} - \frac{5}{4}\delta^{rb}\delta^{sc}(Y_d^\dagger Y_d)^{dt}(Y_uY_u^\dagger)^{pa} \\
& - \frac{3}{2}\text{T}_2\delta^{pa}\delta^{rb}\delta^{sc}(Y_d^\dagger Y_d)^{dt} - \frac{3}{2}\delta^{pc}Y_u^{*ab}Y_d^{st}(Y_d^\dagger Y_u)^{dr} - \frac{3}{2}\delta^{sa}Y_d^{*cd}Y_u^{pr}(Y_u^\dagger Y_d)^{bt} - \frac{3}{2}\text{T}_2\delta^{pa}\delta^{sc}\delta^{td}(Y_u^\dagger Y_u)^{br} - \frac{3}{2}\delta^{rb}Y_d^{*cd}Y_d^{st}(Y_dY_d^\dagger)^{pa}
\end{aligned}$$

$$\begin{aligned}
& -\frac{3}{2}\delta^{td}Y_u^{*ab}Y_u^{pr}(Y_uY_u^\dagger)^{sc} - 2\delta^{rb}\delta^{sc}(Y_d^\dagger Y_d)^{dt}(Y_dY_d^\dagger)^{pa} - 2\delta^{pa}\delta^{td}(Y_u^\dagger Y_u)^{br}(Y_uY_u^\dagger)^{sc} - \frac{9}{4}\delta^{pc}\delta^{rb}Y_d^{st}(Y_d^\dagger Y_dY_d^\dagger)^{ad} - \frac{9}{4}\delta^{sa}\delta^{td}Y_u^{pr}(Y_u^\dagger Y_uY_u^\dagger)^{cb} \\
& - 3\delta^{rb}\delta^{td}(Y_dY_d^\dagger)^{pa}(Y_uY_u^\dagger)^{sc} - 3\delta^{sc}\delta^{td}Y_u^{*ab}(Y_dY_d^\dagger Y_u)^{pr} - 3\delta^{pa}\delta^{rb}Y_d^{*cd}(Y_uY_u^\dagger Y_d)^{st} - \frac{7}{2}\delta^{pc}\delta^{sa}(Y_d^\dagger Y_u)^{dr}(Y_u^\dagger Y_d)^{bt} - \frac{7}{2}\delta^{pa}\delta^{sc}(Y_d^\dagger Y_d)^{dt}(Y_u^\dagger Y_u)^{br} \\
& - \frac{7}{2}\delta^{rb}\delta^{td}(Y_dY_d^\dagger)^{sc}(Y_uY_u^\dagger)^{pa} - \frac{515}{144}\delta^{pa}\delta^{rb}\delta^{sc}\delta^{td}g_Y^4 - \frac{27}{2}\delta^{pa}\delta^{rb}Y_d^{st}(Y_d^\dagger Y_dY_d^\dagger)^{cd} - \frac{27}{2}\delta^{sc}\delta^{td}Y_u^{pr}(Y_u^\dagger Y_uY_u^\dagger)^{ab} \Big\} C_{quqd}^{(\parallel)abcd} + \left(C_{quqd}^{(\parallel)*}\right)^{abcd} \Big\{ \frac{1}{2}Y_d^{ad}Y_d^{ct}Y_u^{pr}Y_u^{sb} \\
& + \frac{1}{2}Y_d^{pd}Y_d^{st}Y_u^{ar}Y_u^{cb} + \frac{3}{2}Y_d^{pd}Y_d^{at}Y_u^{sb}Y_u^{cr} - \frac{3}{2}Y_d^{sd}Y_d^{ct}Y_u^{pb}Y_u^{ar} - 3Y_d^{st}Y_d^{ad}Y_u^{pr}Y_u^{cb} - 18Y_d^{st}Y_d^{cd}Y_u^{pr}Y_u^{ab} \Big\} + \left\{ g_L^2 \left( \frac{3}{2}\delta^{pa}\delta^{rb}Y_d^{*cd}Y_d^{st} + \frac{3}{2}\delta^{sc}\delta^{td}Y_u^{*ab}Y_u^{pr} \right. \right. \\
& - \frac{27}{8}\delta^{pc}\delta^{rb}Y_d^{*ad}Y_d^{st} - \frac{27}{8}\delta^{sa}\delta^{td}Y_u^{*cb}Y_u^{pr} \Big) + g_Y^2g_s^2 \left( \frac{38}{9}\delta^{pa}\delta^{rb}\delta^{sc}\delta^{td} + \frac{427}{54}\delta^{pc}\delta^{rb}\delta^{sa}\delta^{td} \right) + g_s^2g_L^2 \left( 18\delta^{pa}\delta^{rb}\delta^{sc}\delta^{td} + \frac{63}{2}\delta^{pc}\delta^{rb}\delta^{sa}\delta^{td} \right) \\
& + \delta^{rb}\delta^{td}(Y_dY_d^\dagger)^{pc}(Y_uY_u^\dagger)^{sa} + g_Y^2 \left( \frac{2}{9}\delta^{pc}\delta^{rb}\delta^{td}(Y_dY_d^\dagger)^{sa} + \frac{10}{9}\delta^{pc}\delta^{rb}\delta^{sa}(Y_d^\dagger Y_d)^{dt} + \frac{3}{2}\delta^{sc}\delta^{td}Y_u^{*ab}Y_u^{pr} + \frac{20}{9}\delta^{rb}\delta^{sa}\delta^{td}(Y_uY_u^\dagger)^{pc} - \frac{1}{6}\delta^{pa}\delta^{rb}Y_d^{*cd}Y_d^{st} \right. \\
& - \frac{2}{9}\delta^{pc}\delta^{sa}\delta^{td}(Y_u^\dagger Y_u)^{br} - \frac{4}{9}\delta^{pc}\delta^{rb}\delta^{td}(Y_uY_u^\dagger)^{sa} - \frac{19}{24}\delta^{pc}\delta^{rb}Y_d^{*ad}Y_d^{st} - \frac{10}{9}\delta^{rb}\delta^{sa}\delta^{td}(Y_dY_d^\dagger)^{pc} - \frac{31}{24}\delta^{sa}\delta^{td}Y_u^{*cb}Y_u^{pr} \Big) + g_s^2 \left( 2\delta^{rb}\delta^{sc}\delta^{td}(Y_dY_d^\dagger)^{pa} \right. \\
& + 2\delta^{pa}\delta^{rb}\delta^{td}(Y_dY_d^\dagger)^{sc} + 2\delta^{rb}\delta^{sc}\delta^{td}(Y_uY_u^\dagger)^{pa} + 2\delta^{pa}\delta^{rb}\delta^{td}(Y_uY_u^\dagger)^{sc} + 4\delta^{rb}\delta^{sa}Y_d^{*cd}Y_d^{pt} + 4\delta^{pc}\delta^{td}Y_u^{*ab}Y_u^{sr} + 4\delta^{pa}\delta^{rb}\delta^{sc}(Y_d^\dagger Y_d)^{dt} \\
& + 4\delta^{pa}\delta^{sc}\delta^{td}(Y_u^\dagger Y_u)^{br} + \frac{14}{3}\delta^{rb}\delta^{sa}\delta^{td}(Y_dY_d^\dagger)^{pc} + \frac{14}{3}\delta^{pc}\delta^{rb}\delta^{td}(Y_dY_d^\dagger)^{sa} + \frac{14}{3}\delta^{rb}\delta^{sa}\delta^{td}(Y_uY_u^\dagger)^{pc} + \frac{14}{3}\delta^{pc}\delta^{rb}\delta^{td}(Y_uY_u^\dagger)^{sa} + 6\delta^{rb}\delta^{sc}Y_d^{*ad}Y_d^{pt} \\
& + 6\delta^{pa}\delta^{td}Y_u^{*cb}Y_u^{sr} + \frac{28}{3}\delta^{pc}\delta^{rb}\delta^{sa}(Y_d^\dagger Y_d)^{dt} + \frac{28}{3}\delta^{pc}\delta^{sa}\delta^{td}(Y_u^\dagger Y_u)^{br} + 14\delta^{pa}\delta^{rb}Y_d^{*cd}Y_d^{st} + 14\delta^{sc}\delta^{td}Y_u^{*ab}Y_u^{pr} + 49\delta^{pc}\delta^{rb}Y_d^{*ad}Y_d^{st} \\
& + 49\delta^{sa}\delta^{td}Y_u^{*cb}Y_u^{pr} \Big) + \frac{3}{2}\delta^{pc}\delta^{sa}(Y_d^\dagger Y_d)^{dt}(Y_u^\dagger Y_u)^{br} + \frac{3}{2}\delta^{rb}\delta^{td}(Y_dY_d^\dagger)^{sa}(Y_uY_u^\dagger)^{pc} + \frac{3}{2}\delta^{sc}\delta^{td}Y_u^{pr}(Y_d^\dagger Y_dY_u^\dagger)^{ab} + \frac{3}{2}\delta^{pa}\delta^{rb}Y_d^{st}(Y_u^\dagger Y_uY_d^\dagger)^{cd} \\
& + 2\delta^{pc}\delta^{rb}(Y_d^\dagger Y_d)^{dt}(Y_dY_d^\dagger)^{sa} + 2\delta^{rb}\delta^{td}(Y_dY_d^\dagger)^{pc}(Y_dY_d^\dagger)^{sa} + 2\delta^{sa}\delta^{td}(Y_u^\dagger Y_u)^{br}(Y_uY_u^\dagger)^{pc} + 2\delta^{rb}\delta^{td}(Y_uY_u^\dagger)^{pc}(Y_uY_u^\dagger)^{sa} + \frac{15}{4}\delta^{sa}\delta^{td}Y_u^{pr}(Y_d^\dagger Y_dY_u^\dagger)^{cb} \\
& + \frac{15}{4}\delta^{pc}\delta^{rb}Y_d^{st}(Y_u^\dagger Y_uY_d^\dagger)^{ad} + \frac{11}{2}\delta^{pa}\delta^{sc}(Y_d^\dagger Y_u)^{dr}(Y_u^\dagger Y_d)^{bt} + \frac{199}{12}\delta^{pc}\delta^{rb}\delta^{sa}\delta^{td}g_L^4 - \frac{1}{2}\delta^{pc}Y_u^{*ab}Y_d^{st}(Y_d^\dagger Y_u)^{dr} - \frac{1}{2}\delta^{sa}Y_d^{*cd}Y_u^{pr}(Y_u^\dagger Y_d)^{bt} \\
& - \frac{1}{2}\delta^{rb}Y_d^{*cd}Y_d^{st}(Y_dY_d^\dagger)^{pa} - \frac{1}{2}\delta^{sa}\delta^{td}(Y_u^\dagger Y_u)^{br}(Y_dY_d^\dagger)^{pc} - \frac{1}{2}\delta^{pc}\delta^{td}(Y_u^\dagger Y_u)^{br}(Y_dY_d^\dagger)^{sa} - \frac{1}{2}\delta^{rb}\delta^{sa}(Y_d^\dagger Y_d)^{dt}(Y_uY_u^\dagger)^{pc} - \frac{1}{2}\delta^{pc}\delta^{rb}(Y_d^\dagger Y_d)^{dt}(Y_uY_u^\dagger)^{sa} \\
& - \frac{1}{2}\delta^{td}Y_u^{*ab}Y_u^{pr}(Y_uY_u^\dagger)^{sc} - \frac{3}{4}\delta^{pa}Y_u^{*cb}Y_d^{st}(Y_d^\dagger Y_u)^{dr} - \frac{3}{4}\delta^{sc}Y_d^{*ad}Y_u^{pr}(Y_u^\dagger Y_d)^{bt} - \frac{3}{4}\delta^{rb}Y_d^{*ad}Y_d^{st}(Y_dY_d^\dagger)^{pc} - \frac{3}{4}\delta^{td}Y_u^{*cb}Y_u^{pr}(Y_uY_u^\dagger)^{sa} - g_s^4 \left( 89\delta^{pa}\delta^{rb}\delta^{sc}\delta^{td} \right. \\
& + \frac{1678}{9}\delta^{pc}\delta^{rb}\delta^{sa}\delta^{td} \Big) - \delta^{sc}\delta^{td}Y_u^{*ab}(Y_dY_d^\dagger Y_u)^{pr} - \delta^{pa}\delta^{rb}Y_d^{*cd}(Y_uY_u^\dagger Y_d)^{st} - \left( 3\delta^{sc}\delta^{td}Y_u^{*ab}Y_u^{pr} + \frac{9}{2}\delta^{sa}\delta^{td}Y_u^{*cb}Y_u^{pr} \right) \text{Tr}[Y_d^\dagger Y_d] - \left( 3\delta^{pa}\delta^{rb}Y_d^{*cd}Y_d^{st} \right. \\
& + \frac{9}{2}\delta^{pc}\delta^{rb}Y_d^{*ad}Y_d^{st} \Big) \text{Tr}[Y_u^\dagger Y_u] - \frac{115}{108}\delta^{pc}\delta^{rb}\delta^{sa}\delta^{td}g_Y^4 - \frac{3}{2}\delta^{sa}\delta^{td}Y_u^{*cb}(Y_dY_d^\dagger Y_u)^{pr} - \frac{3}{2}\delta^{pc}\delta^{rb}Y_d^{*ad}(Y_uY_u^\dagger Y_d)^{st} - \frac{9}{2}\delta^{pa}\delta^{rb}Y_d^{st}(Y_d^\dagger Y_dY_d^\dagger)^{cd} \\
& - \frac{9}{2}\delta^{sc}\delta^{td}Y_u^{pr}(Y_u^\dagger Y_uY_u^\dagger)^{ab} - \frac{27}{4}\delta^{pc}\delta^{rb}Y_d^{st}(Y_d^\dagger Y_dY_d^\dagger)^{ad} - \frac{27}{4}\delta^{sa}\delta^{td}Y_u^{pr}(Y_u^\dagger Y_uY_u^\dagger)^{cb} \Big\} C_{quqd}^{(\times)abcd} + \left(C_{quqd}^{(\times)*}\right)^{abcd} \Big\{ \frac{1}{2}Y_d^{pd}Y_d^{ct}Y_u^{sb}Y_u^{ar} + \frac{3}{2}Y_d^{ad}Y_d^{ct}Y_u^{pr}Y_u^{sb}
\end{aligned}$$

$$\begin{aligned}
& + \frac{3}{2} Y_d^{pd} Y_d^{st} Y_u^{ar} Y_u^{cb} - 6 Y_d^{st} Y_d^{cd} Y_u^{pr} Y_u^{ab} - 9 Y_d^{st} Y_d^{ad} Y_u^{pr} Y_u^{cb} \Big\} + \left\{ \frac{1}{2} \delta^{sc} Y_e^{*ab} Y_u^{pr} (Y_u^\dagger Y_d)^{dt} + \frac{1}{2} \delta^{rd} Y_e^{*ab} Y_d^{st} (Y_d Y_d^\dagger)^{pc} + \delta^{pc} \delta^{rd} Y_e^{*ab} (Y_u Y_u^\dagger Y_d)^{st} \right. \\
& + 3 \delta^{pc} \delta^{rd} Y_e^{*ab} Y_d^{st} \text{Tr}[Y_u^\dagger Y_u] + \frac{9}{2} \delta^{pc} \delta^{rd} Y_d^{st} (Y_e^\dagger Y_e Y_e^\dagger)^{ab} - g_s^2 \left( \frac{2}{3} \delta^{pc} \delta^{rd} Y_e^{*ab} Y_d^{st} + 4 \delta^{rd} \delta^{sc} Y_e^{*ab} Y_d^{pt} \right) - \frac{3}{2} \delta^{pc} \delta^{rd} g_L^2 Y_e^{*ab} Y_d^{st} \\
& - \frac{97}{18} \delta^{pc} \delta^{rd} g_Y^2 Y_e^{*ab} Y_d^{st} \Big\} C_{lequ}^{abcd} + C_{lequ}^{*abcd} \left\{ Y_d^{ct} Y_e^{ab} Y_u^{pr} Y_u^{sd} + 3 Y_d^{st} Y_e^{ab} Y_u^{pr} Y_u^{cd} \right\} + \left\{ g_s^2 \left( 2 \delta^{rb} \delta^{sc} Y_e^{*ad} Y_d^{pt} + 5 \delta^{pc} \delta^{rb} Y_e^{*ad} Y_d^{st} \right) \right. \\
& + \frac{119}{24} \delta^{pc} \delta^{rb} g_Y^2 Y_e^{*ad} Y_d^{st} - \frac{1}{4} \delta^{sc} Y_e^{*ad} Y_u^{pr} (Y_u^\dagger Y_d)^{bt} - \frac{1}{4} \delta^{rb} Y_e^{*ad} Y_d^{st} (Y_d Y_d^\dagger)^{pc} - \frac{1}{2} \delta^{pc} \delta^{rb} Y_e^{*ad} (Y_u Y_u^\dagger Y_d)^{st} - \frac{9}{8} \delta^{pc} \delta^{rb} g_L^2 Y_e^{*ad} Y_d^{st} \\
& - \frac{3}{2} \delta^{pc} \delta^{rb} Y_e^{*ad} Y_d^{st} \text{Tr}[Y_u^\dagger Y_u] - \frac{9}{4} \delta^{pc} \delta^{rb} Y_d^{st} (Y_e^\dagger Y_e Y_e^\dagger)^{ad} \Big\} C_{luqe}^{abcd} - \frac{3}{2} C_{luqe}^{*abcd} Y_d^{st} Y_e^{ad} Y_u^{pr} Y_u^{cb} + \left\{ g_L^2 \left( \frac{4}{3} \delta^{pa} \delta^{bc} Y_d^{st} Y_u^{dr} + \frac{4}{3} \delta^{sa} \delta^{bc} Y_d^{dt} Y_u^{pr} \right. \right. \\
& - 57 \delta^{pa} \delta^{sc} Y_d^{dt} Y_u^{br} \Big) + g_s^2 \left( \frac{2}{3} \delta^{pa} \delta^{sc} Y_d^{dt} Y_u^{br} + \frac{52}{27} \delta^{pa} \delta^{bc} Y_d^{st} Y_u^{dr} + \frac{52}{27} \delta^{sa} \delta^{bc} Y_d^{dt} Y_u^{pr} + \frac{34}{9} \delta^{pa} \delta^{bc} Y_d^{dt} Y_u^{sr} + \frac{34}{9} \delta^{sa} \delta^{bc} Y_d^{pt} Y_u^{dr} - 22 \delta^{pa} \delta^{sc} Y_d^{bt} Y_u^{dr} \right) \\
& + g_Y^2 \left( \frac{16}{81} \delta^{pa} \delta^{bc} Y_d^{st} Y_u^{dr} + \frac{152}{27} \delta^{pa} \delta^{cd} Y_d^{st} Y_u^{br} - \frac{32}{81} \delta^{sa} \delta^{bc} Y_d^{dt} Y_u^{pr} - \frac{19}{9} \delta^{pa} \delta^{sc} Y_d^{dt} Y_u^{br} - \frac{88}{27} \delta^{sa} \delta^{cd} Y_d^{bt} Y_u^{pr} \right) + 3 \delta^{pa} \delta^{sc} Y_u^{br} (Y_d Y_d^\dagger Y_d)^{dt} \\
& + 3 \delta^{pa} \delta^{sc} Y_d^{dt} (Y_u Y_u^\dagger Y_u)^{br} + 5 \delta^{pa} \delta^{sc} Y_d^{dt} (Y_d Y_d^\dagger Y_u)^{br} + 5 \delta^{pa} \delta^{sc} Y_u^{br} (Y_u Y_u^\dagger Y_d)^{dt} + 6 T_2 \delta^{pa} \delta^{sc} Y_d^{dt} Y_u^{br} + 10 \delta^{pa} Y_d^{dt} Y_u^{br} (Y_d Y_d^\dagger)^{sc} \\
& + 10 \delta^{sa} Y_d^{bt} Y_u^{dr} (Y_u Y_u^\dagger)^{pc} + 12 \delta^{sa} Y_d^{bt} Y_u^{pr} (Y_d Y_d^\dagger)^{dc} + 12 \delta^{pa} Y_d^{st} Y_u^{br} (Y_u Y_u^\dagger)^{dc} - 3 \delta^{pa} Y_d^{st} Y_u^{dr} (Y_d Y_d^\dagger)^{bc} - 3 \delta^{sa} Y_d^{dt} Y_u^{pr} (Y_u Y_u^\dagger)^{bc} - 10 \delta^{sa} Y_d^{bt} Y_u^{dr} (Y_d Y_d^\dagger)^{pc} \\
& - 10 \delta^{pa} Y_d^{dt} Y_u^{br} (Y_u Y_u^\dagger)^{sc} \Big\} C_{qq}^{(\parallel)abcd} + \left\{ g_s^2 \left( \frac{104}{27} \delta^{pa} \delta^{bc} Y_d^{st} Y_u^{dr} + \frac{104}{27} \delta^{sa} \delta^{bc} Y_d^{dt} Y_u^{pr} + \frac{68}{9} \delta^{pa} \delta^{bc} Y_d^{dt} Y_u^{sr} + \frac{68}{9} \delta^{sa} \delta^{bc} Y_d^{pt} Y_u^{dr} + 22 \delta^{pa} \delta^{sc} Y_d^{bt} Y_u^{dr} \right. \right. \\
& - \frac{2}{3} \delta^{pa} \delta^{sc} Y_d^{dt} Y_u^{br} \Big) + g_L^2 \left( 57 \delta^{pa} \delta^{sc} Y_d^{dt} Y_u^{br} - 8 \delta^{pa} \delta^{cd} Y_d^{st} Y_u^{br} - 8 \delta^{sa} \delta^{cd} Y_d^{bt} Y_u^{pr} \right) + g_Y^2 \left( \frac{32}{81} \delta^{pa} \delta^{bc} Y_d^{st} Y_u^{dr} + \frac{19}{9} \delta^{pa} \delta^{sc} Y_d^{dt} Y_u^{br} + \frac{76}{27} \delta^{pa} \delta^{cd} Y_d^{st} Y_u^{br} \right. \\
& - \frac{64}{81} \delta^{sa} \delta^{bc} Y_d^{dt} Y_u^{pr} - \frac{44}{27} \delta^{sa} \delta^{cd} Y_d^{bt} Y_u^{pr} \Big) + 3 \delta^{pa} Y_d^{st} Y_u^{dr} (Y_d Y_d^\dagger)^{bc} + 3 \delta^{sa} Y_d^{dt} Y_u^{pr} (Y_u Y_u^\dagger)^{bc} + 5 \delta^{pa} Y_d^{dt} Y_u^{br} (Y_d Y_d^\dagger)^{sc} + 5 \delta^{sa} Y_d^{bt} Y_u^{dr} (Y_u Y_u^\dagger)^{pc} \\
& + 24 \delta^{sa} Y_d^{bt} Y_u^{pr} (Y_d Y_d^\dagger)^{dc} + 24 \delta^{pa} Y_d^{st} Y_u^{br} (Y_u Y_u^\dagger)^{dc} - 3 \delta^{pa} \delta^{sc} Y_u^{br} (Y_d Y_d^\dagger Y_d)^{dt} - 3 \delta^{pa} \delta^{sc} Y_d^{dt} (Y_u Y_u^\dagger Y_u)^{br} - 5 \delta^{pa} \delta^{sc} Y_d^{dt} (Y_d Y_d^\dagger Y_u)^{br} \\
& - 5 \delta^{pa} \delta^{sc} Y_u^{br} (Y_u Y_u^\dagger Y_d)^{dt} - 6 T_2 \delta^{pa} \delta^{sc} Y_d^{dt} Y_u^{br} - 20 \delta^{sa} Y_d^{bt} Y_u^{dr} (Y_d Y_d^\dagger)^{pc} - 20 \delta^{pa} Y_d^{dt} Y_u^{br} (Y_u Y_u^\dagger)^{sc} \Big\} C_{qq}^{(\times)abcd} + \left\{ g_Y^2 \left( \frac{44}{27} \delta^{sc} \delta^{ab} Y_d^{dt} Y_u^{pr} \right. \right. \\
& - \frac{76}{27} \delta^{pc} \delta^{ab} Y_d^{st} Y_u^{dr} \Big) + 3 \delta^{sc} Y_d^{dt} Y_u^{pr} (Y_e Y_e^\dagger)^{ba} \Big\} C_{\ell q}^{(\parallel)abcd} + \left\{ g_Y^2 \left( \frac{22}{27} \delta^{sc} \delta^{ab} Y_d^{dt} Y_u^{pr} - \frac{38}{27} \delta^{pc} \delta^{ab} Y_d^{st} Y_u^{dr} \right) + 6 \delta^{sc} Y_d^{dt} Y_u^{pr} (Y_e Y_e^\dagger)^{ba} - g_L^2 \left( \frac{4}{3} \delta^{pc} \delta^{ab} Y_d^{st} Y_u^{dr} \right. \right. \\
& + \frac{4}{3} \delta^{sc} \delta^{ab} Y_d^{dt} Y_u^{pr} \Big) \Big\} C_{\ell q}^{(\times)abcd}, \tag{12.4}
\end{aligned}$$

### 12.3 $C_{quqd}^{(\times)}$

$$\begin{aligned}
\beta_{C_{quqd}^{(\times)prst}}^{(1)} = & -\frac{4}{3}\delta^{rb}\delta^{sa}g_Y^2C_{uB}^{ab}Y_d^{pt} - 6\delta^{rb}\delta^{sa}g_L^2C_{uW}^{ab}Y_d^{pt} - \frac{4}{3}g_s^2\left\{2\delta^{rb}\delta^{sa}Y_d^{pt} + 3\delta^{pa}\delta^{rb}Y_d^{st}\right\}C_{uG}^{ab} + \frac{20}{3}\delta^{pa}\delta^{tb}g_Y^2C_{dB}^{ab}Y_u^{sr} - 6\delta^{pa}\delta^{tb}g_L^2C_{dW}^{ab}Y_u^{sr} \\
& - \frac{4}{3}g_s^2\left\{2\delta^{pa}\delta^{tb}Y_u^{sr} + 3\delta^{sa}\delta^{tb}Y_u^{pr}\right\}C_{dG}^{ab} + 4\delta^{pa}\delta^{rd}C_{qu}^{(\parallel)abcd}Y_d^{bt}Y_u^{sc} + 4\delta^{sa}\delta^{td}C_{qd}^{(\parallel)abcd}Y_d^{pc}Y_u^{br} + 4\delta^{rb}\delta^{td}C_{ud}^{(\parallel)abcd}Y_d^{pc}Y_u^{sa} - 4\delta^{rb}\delta^{td}C_{ud}^{(\times)abcd}Y_d^{sc}Y_u^{pa} \\
& + \left\{\frac{5}{9}\delta^{pc}\delta^{rb}\delta^{sa}\delta^{td}g_Y^2 + \frac{4}{3}g_s^2\left(2\delta^{pc}\delta^{rb}\delta^{sa}\delta^{td} + 3\delta^{pa}\delta^{rb}\delta^{sc}\delta^{td}\right) + 3\delta^{pc}\delta^{rb}\delta^{sa}\delta^{td}g_L^2\right\}C_{quqd}^{(\parallel)abcd} + \left\{\frac{1}{2}\left(\delta^{rb}\delta^{sc}\delta^{td}(Y_dY_d^\dagger)^{pa} + \delta^{pa}\delta^{rb}\delta^{td}(Y_dY_d^\dagger)^{sc}\right.\right. \\
& + \delta^{rb}\delta^{sc}\delta^{td}(Y_uY_u^\dagger)^{pa} + \delta^{pa}\delta^{rb}\delta^{td}(Y_uY_u^\dagger)^{sc} + 2\delta^{pa}\delta^{rb}\delta^{sc}(Y_d^\dagger Y_d)^{dt} + 2\delta^{pa}\delta^{sc}\delta^{td}(Y_u^\dagger Y_u)^{br}) - \frac{11}{18}\delta^{pa}\delta^{rb}\delta^{sc}\delta^{td}g_Y^2 - \frac{4}{3}g_s^2\left(3\delta^{pc}\delta^{rb}\delta^{sa}\delta^{td}\right. \\
& \left.\left.- 5\delta^{pa}\delta^{rb}\delta^{sc}\delta^{td}\right) - \frac{3}{2}\delta^{pa}\delta^{rb}\delta^{sc}\delta^{td}g_L^2\right\}C_{quqd}^{(\times)abcd} + 8\delta^{pa}\delta^{sc}C_{qq}^{(\parallel)abcd}Y_d^{bt}Y_u^{dr} - 8\delta^{pa}\delta^{sc}C_{qq}^{(\times)abcd}Y_d^{bt}Y_u^{dr}, \tag{12.5}
\end{aligned}$$

$$\begin{aligned}
\beta_{C_{quqd}^{(\times)prst}}^{(2)} = & -15g_L^6C_WY_d^{pt}Y_u^{sr} - 19ig_L^6C_{\widetilde{W}}Y_d^{pt}Y_u^{sr} - g_s^6\left\{20Y_d^{pt}Y_u^{sr} + 30Y_d^{st}Y_u^{pr}\right\}C_G + g_s^6\left\{-\frac{124i}{3}Y_d^{pt}Y_u^{sr} - 62iY_d^{st}Y_u^{pr}\right\}C_{\widetilde{G}} + \left\{g_Y^2g_s^2\left(\frac{38}{3}\delta^{rb}\delta^{sa}Y_d^{pt} - \frac{2}{3}\delta^{pa}\delta^{rb}Y_d^{st}\right)\right. \\
& + g_Y^2\left(\frac{1}{3}\delta^{sa}Y_d^{pt}(Y_u^\dagger Y_u)^{br} + \frac{2}{3}T_2\delta^{rb}\delta^{sa}Y_d^{pt} + \frac{2}{3}\delta^{rb}Y_d^{pt}(Y_dY_d^\dagger)^{sa} + \frac{2}{3}\delta^{rb}Y_d^{pt}(Y_uY_u^\dagger)^{sa} - 5\delta^{pa}Y_u^{sr}(Y_u^\dagger Y_d)^{bt} - \frac{16}{3}\delta^{rb}\delta^{sa}(Y_uY_u^\dagger Y_d)^{pt}\right) + \frac{53}{27}\delta^{rb}\delta^{sa}g_Y^4Y_d^{pt} \\
& \left.- 4\delta^{rb}\delta^{sa}g_Y^2g_L^2Y_d^{pt}\right\}C_{uB}^{ab} - \frac{10}{3}g_Y^2C_{uB}^{*ab}Y_d^{at}Y_u^{pb}Y_u^{sr} + \left\{g_s^2g_L^2\left(49\delta^{rb}\delta^{sa}Y_d^{pt} - 15\delta^{pa}\delta^{rb}Y_d^{st}\right) + g_L^2\left(\frac{3}{2}\delta^{sa}Y_d^{pt}(Y_u^\dagger Y_u)^{br} + 3T_2\delta^{rb}\delta^{sa}Y_d^{pt}\right.\right. \\
& + \frac{9}{2}\delta^{pa}Y_u^{sr}(Y_u^\dagger Y_d)^{bt} - 3\delta^{rb}Y_d^{pt}(Y_dY_d^\dagger)^{sa}) - \frac{14}{3}\delta^{rb}\delta^{sa}g_Y^2g_L^2Y_d^{pt} - \frac{199}{6}\delta^{rb}\delta^{sa}g_L^4Y_d^{pt}\left.\right\}C_{uW}^{ab} - 3g_L^2C_{uW}^{*ab}Y_d^{at}Y_u^{pb}Y_u^{sr} + \left\{g_s^4\left(\frac{52}{3}\delta^{pa}\delta^{rb}Y_d^{st}\right.\right. \\
& - \frac{16}{9}\delta^{rb}\delta^{sa}Y_d^{pt}) + g_s^2g_L^2\left(7\delta^{rb}\delta^{sa}Y_d^{pt} - \frac{21}{2}\delta^{pa}\delta^{rb}Y_d^{st}\right) + g_s^2\left(\frac{2}{3}\delta^{sa}Y_d^{pt}(Y_u^\dagger Y_u)^{br} + \delta^{pa}Y_d^{st}(Y_u^\dagger Y_u)^{br} + \frac{4}{3}T_2\delta^{rb}\delta^{sa}Y_d^{pt} + \frac{4}{3}\delta^{rb}Y_d^{pt}(Y_dY_d^\dagger)^{sa}\right. \\
& + \frac{4}{3}\delta^{rb}Y_d^{pt}(Y_uY_u^\dagger)^{sa} + \frac{4}{3}\delta^{rb}\delta^{sa}(Y_uY_u^\dagger Y_d)^{pt} + 2T_2\delta^{pa}\delta^{rb}Y_d^{st} + 2\delta^{pa}Y_u^{sr}(Y_u^\dagger Y_d)^{bt} + 2\delta^{rb}Y_d^{st}(Y_dY_d^\dagger)^{pa} + 2\delta^{rb}Y_d^{st}(Y_uY_u^\dagger)^{pa} + 3\delta^{sa}Y_u^{pr}(Y_u^\dagger Y_d)^{bt} \\
& + 4\delta^{rb}\delta^{sa}(Y_dY_d^\dagger Y_d)^{pt} + 6\delta^{pa}\delta^{rb}(Y_dY_d^\dagger Y_d)^{st} - 4\delta^{pa}\delta^{rb}(Y_uY_u^\dagger Y_d)^{st}) - g_Y^2g_s^2\left(\frac{1}{3}\delta^{rb}\delta^{sa}Y_d^{pt} + \frac{79}{18}\delta^{pa}\delta^{rb}Y_d^{st}\right)\left.\right\}C_{uG}^{ab} + g_s^2C_{uG}^{*ab}\left\{\frac{4}{3}Y_d^{at}Y_u^{pb}Y_u^{sr}\right. \\
& \left.- 4Y_d^{at}Y_u^{pr}Y_u^{sb}\right\} + \left\{g_Y^2g_s^2\left(\frac{58}{3}\delta^{sa}\delta^{tb}Y_u^{pr} - \frac{158}{3}\delta^{pa}\delta^{tb}Y_u^{sr}\right) + g_Y^2\left(\delta^{sa}Y_d^{pt}(Y_d^\dagger Y_u)^{br} + \frac{8}{3}\delta^{pa}\delta^{tb}(Y_dY_d^\dagger Y_u)^{sr} - \frac{5}{3}\delta^{pa}Y_u^{sr}(Y_d^\dagger Y_d)^{bt} - \frac{10}{3}T_2\delta^{pa}\delta^{tb}Y_u^{sr}\right.\right. \\
& \left.- \frac{10}{3}\delta^{tb}Y_u^{sr}(Y_dY_d^\dagger)^{pa} - \frac{10}{3}\delta^{tb}Y_u^{sr}(Y_uY_u^\dagger)^{pa} - 8\delta^{pa}\delta^{tb}(Y_uY_u^\dagger Y_u)^{sr}\right) + 8\delta^{pa}\delta^{tb}g_Y^2g_L^2Y_u^{sr} - \frac{385}{27}\delta^{pa}\delta^{tb}g_Y^4Y_u^{sr}\left.\right\}C_{dB}^{ab} + \frac{2}{3}g_Y^2C_{dB}^{*ab}Y_d^{pt}Y_d^{sb}Y_u^{ar}
\end{aligned}$$

$$\begin{aligned}
& + \left\{ g_s^2 g_L^2 \left( 49 \delta^{pa} \delta^{tb} Y_u^{sr} - 15 \delta^{sa} \delta^{tb} Y_u^{pr} \right) + g_L^2 \left( \frac{3}{2} \delta^{pa} Y_u^{sr} (Y_d^\dagger Y_d)^{bt} + 3 T_2 \delta^{pa} \delta^{tb} Y_u^{sr} + \frac{9}{2} \delta^{sa} Y_d^{pt} (Y_d^\dagger Y_u)^{br} - 3 \delta^{tb} Y_u^{sr} (Y_u Y_u^\dagger)^{pa} \right) - \frac{8}{3} \delta^{pa} \delta^{tb} g_Y^2 g_L^2 Y_u^{sr} \right. \\
& - \left. \frac{199}{6} \delta^{pa} \delta^{tb} g_L^4 Y_u^{sr} \right\} C_{dW}^{ab} - 3 g_L^2 C_{dW}^{*ab} Y_d^{pt} Y_d^{sb} Y_u^{ar} + \left\{ g_s^2 g_L^2 \left( 7 \delta^{pa} \delta^{tb} Y_u^{sr} - \frac{21}{2} \delta^{sa} \delta^{tb} Y_u^{pr} \right) + g_Y^2 g_s^2 \left( \frac{7}{3} \delta^{pa} \delta^{tb} Y_u^{sr} - \frac{7}{18} \delta^{sa} \delta^{tb} Y_u^{pr} \right) \right. \\
& + g_s^4 \left( \frac{52}{3} \delta^{sa} \delta^{tb} Y_u^{pr} - \frac{16}{9} \delta^{pa} \delta^{tb} Y_u^{sr} \right) + g_s^2 \left( \frac{2}{3} \delta^{pa} Y_u^{sr} (Y_d^\dagger Y_d)^{bt} + \delta^{sa} Y_u^{pr} (Y_d^\dagger Y_d)^{bt} + \frac{4}{3} T_2 \delta^{pa} \delta^{tb} Y_u^{sr} + \frac{4}{3} \delta^{tb} Y_u^{sr} (Y_d Y_d^\dagger)^{pa} + \frac{4}{3} \delta^{tb} Y_u^{sr} (Y_u Y_u^\dagger)^{pa} \right. \\
& + \frac{4}{3} \delta^{pa} \delta^{tb} (Y_d Y_d^\dagger Y_u)^{sr} + 2 T_2 \delta^{sa} \delta^{tb} Y_u^{pr} + 2 \delta^{sa} Y_d^{pt} (Y_d^\dagger Y_u)^{br} + 2 \delta^{tb} Y_u^{pr} (Y_d Y_d^\dagger)^{sa} + 2 \delta^{tb} Y_u^{pr} (Y_u Y_u^\dagger)^{sa} + 3 \delta^{pa} Y_d^{st} (Y_d^\dagger Y_u)^{br} + 4 \delta^{pa} \delta^{tb} (Y_u Y_u^\dagger Y_u)^{sr} \\
& + 6 \delta^{sa} \delta^{tb} (Y_u Y_u^\dagger Y_u)^{pr} - 4 \delta^{sa} \delta^{tb} (Y_d Y_d^\dagger Y_u)^{pr} \left. \right\} C_{dG}^{ab} + g_s^2 C_{dG}^{*ab} \left\{ \frac{4}{3} Y_d^{pt} Y_d^{sb} Y_u^{ar} - 4 Y_d^{pb} Y_d^{st} Y_u^{ar} \right\} + \left\{ g_L^2 \left( 6 \delta^{pa} Y_d^{bt} Y_u^{sr} - 6 \delta^{sa} Y_d^{pt} Y_u^{br} \right) + g_s^2 \left( \frac{8}{3} \delta^{pa} Y_d^{bt} Y_u^{sr} \right. \right. \\
& + 4 \delta^{sa} Y_d^{bt} Y_u^{pr} - \frac{8}{3} \delta^{sa} Y_d^{pt} Y_u^{br} - 4 \delta^{pa} Y_d^{st} Y_u^{br} \left. \right) + g_Y^2 \left( \frac{1}{27} \delta^{sa} Y_d^{pt} Y_u^{br} - \frac{65}{27} \delta^{pa} Y_d^{bt} Y_u^{sr} \right) + \delta^{pa} Y_d^{bt} (Y_u Y_u^\dagger Y_u)^{sr} + 5 \delta^{pa} Y_d^{bt} (Y_d Y_d^\dagger Y_u)^{sr} - \delta^{sa} Y_u^{br} (Y_d Y_d^\dagger Y_d)^{pt} \\
& - 5 \delta^{sa} Y_u^{br} (Y_u Y_u^\dagger Y_d)^{pt} \left. \right\} C_{Hq}^{(II)ab} + \left\{ g_L^2 \left( \frac{7}{6} \delta^{pa} Y_d^{bt} Y_u^{sr} - \frac{29}{6} \delta^{sa} Y_d^{pt} Y_u^{br} \right) + g_Y^2 \left( \frac{19}{54} \delta^{sa} Y_d^{pt} Y_u^{br} - \frac{155}{54} \delta^{pa} Y_d^{bt} Y_u^{sr} \right) + g_s^2 \left( \frac{8}{3} \delta^{sa} Y_d^{pt} Y_u^{br} + 4 \delta^{pa} Y_d^{st} Y_u^{br} \right. \right. \\
& + \frac{16}{3} \delta^{pa} Y_d^{bt} Y_u^{sr} + 8 \delta^{sa} Y_d^{bt} Y_u^{pr} \left. \right) - \delta^{pa} Y_d^{bt} (Y_u Y_u^\dagger Y_u)^{sr} - 2 \delta^{sa} Y_u^{br} (Y_d Y_d^\dagger Y_d)^{pt} - 5 \delta^{pa} Y_d^{bt} (Y_d Y_d^\dagger Y_u)^{sr} - 10 \delta^{sa} Y_u^{br} (Y_u Y_u^\dagger Y_d)^{pt} \left. \right\} C_{Hq}^{(\times)ab} \\
& + \left\{ g_s^2 \left( \frac{8}{3} \delta^{rb} Y_d^{pt} Y_u^{sa} + 4 \delta^{rb} Y_d^{st} Y_u^{pa} \right) + \frac{31}{27} \delta^{rb} g_Y^2 Y_d^{pt} Y_u^{sa} - \delta^{rb} Y_u^{sa} (Y_d Y_d^\dagger Y_d)^{pt} - 5 \delta^{rb} Y_u^{sa} (Y_u Y_u^\dagger Y_d)^{pt} \right\} C_{Hu}^{ab} + \left\{ \delta^{tb} Y_d^{pa} (Y_u Y_u^\dagger Y_u)^{sr} \right. \\
& + 5 \delta^{tb} Y_d^{pa} (Y_d Y_d^\dagger Y_u)^{sr} - g_s^2 \left( \frac{8}{3} \delta^{tb} Y_d^{pa} Y_u^{sr} + 4 \delta^{tb} Y_d^{sa} Y_u^{pr} \right) - \frac{95}{27} \delta^{tb} g_Y^2 Y_d^{pa} Y_u^{sr} \left. \right\} C_{Hd}^{ab} + \left\{ 3 \delta^{tb} Y_u^{pa} (Y_d Y_d^\dagger Y_u)^{sr} + 4 \delta^{tb} Y_u^{pa} (Y_u Y_u^\dagger Y_u)^{sr} \right. \\
& + \frac{40}{9} \delta^{tb} g_Y^2 Y_u^{pa} Y_u^{sr} - g_s^2 \left( \frac{8}{3} \delta^{tb} Y_u^{pa} Y_u^{sr} + 4 \delta^{tb} Y_u^{pr} Y_u^{sa} \right) \left. \right\} C_{Hud}^{ab} + C_{Hud}^{*ab} \left\{ \frac{4}{9} \delta^{ra} g_Y^2 Y_d^{pt} Y_d^{sb} + 3 \delta^{ra} Y_d^{sb} (Y_u Y_u^\dagger Y_d)^{pt} + 4 \delta^{ra} Y_d^{sb} (Y_d Y_d^\dagger Y_d)^{pt} \right. \\
& - g_s^2 \left( \frac{8}{3} \delta^{ra} Y_d^{pt} Y_d^{sb} + 4 \delta^{ra} Y_d^{pb} Y_d^{st} \right) \left. \right\} - \frac{2}{27} \delta^{rd} \delta^{ab} g_Y^2 C_{\ell u}^{abcd} Y_d^{pt} Y_u^{sc} + \frac{10}{27} \delta^{td} \delta^{ab} g_Y^2 C_{\ell d}^{abcd} Y_d^{pc} Y_u^{sr} + g_Y^2 \left\{ \frac{10}{27} \delta^{pa} \delta^{cd} Y_d^{bt} Y_u^{sr} - \frac{2}{27} \delta^{sa} \delta^{cd} Y_d^{pt} Y_u^{br} \right\} C_{qe}^{abcd} \\
& + \left\{ g_s^2 \left( \frac{8}{3} \delta^{rd} \delta^{sa} Y_d^{pt} Y_u^{bc} + 4 \delta^{pa} \delta^{rd} Y_d^{st} Y_u^{bc} + 9 \delta^{rd} \delta^{sa} Y_d^{bt} Y_u^{pc} - \frac{188}{3} \delta^{pa} \delta^{rd} Y_d^{bt} Y_u^{sc} \right) + g_L^2 \left( 3 \delta^{rd} \delta^{sa} Y_d^{pt} Y_u^{bc} - 3 \delta^{pa} \delta^{rd} Y_d^{bt} Y_u^{sc} \right) + g_Y^2 \left( \frac{2}{27} \delta^{rd} \delta^{ab} Y_d^{pt} Y_u^{sc} \right. \right. \\
& + \frac{4}{27} \delta^{sa} \delta^{cd} Y_d^{pt} Y_u^{br} + \frac{5}{9} \delta^{rd} \delta^{sa} Y_d^{pt} Y_u^{bc} - \frac{20}{27} \delta^{pa} \delta^{cd} Y_d^{bt} Y_u^{sr} - \frac{35}{9} \delta^{pa} \delta^{rd} Y_d^{bt} Y_u^{sc} \left. \right) + \frac{3}{2} \delta^{rd} Y_d^{bt} Y_u^{sc} (Y_u Y_u^\dagger)^{pa} - Y_u^{*ad} Y_d^{bt} Y_u^{pc} Y_u^{sr} - \delta^{pa} \delta^{rd} Y_u^{sc} (Y_d Y_d^\dagger Y_d)^{bt} \\
& - \delta^{rd} \delta^{sa} Y_u^{bc} (Y_u Y_u^\dagger Y_d)^{pt} - \frac{3}{2} \delta^{sa} Y_u^{pc} Y_u^{br} (Y_u^\dagger Y_d)^{dt} - 2 T_2 \delta^{pa} \delta^{rd} Y_d^{bt} Y_u^{sc} - 2 \delta^{pa} \delta^{rd} Y_d^{bt} (Y_d Y_d^\dagger Y_u)^{sc} - 2 \delta^{pa} \delta^{rd} Y_d^{bt} (Y_u Y_u^\dagger Y_u)^{sc} - 3 \delta^{pa} Y_d^{bt} Y_u^{sc} (Y_u^\dagger Y_u)^{dr}
\end{aligned}$$

$$\begin{aligned}
& -3\delta^{pa}\delta^{rd}Y_u^{sc}(Y_uY_u^\dagger Y_d)^{bt} - 6\delta^{rd}Y_d^{bt}Y_u^{sc}(Y_dY_d^\dagger)^{pa} \Big\} C_{qu}^{(\parallel)abcd} + \left\{ \frac{1}{2}\delta^{rd}\delta^{sa}Y_u^{pc}(Y_uY_u^\dagger Y_d)^{bt} + g_L^2 \left( 9\delta^{rd}\delta^{sa}Y_d^{pt}Y_u^{bc} - \frac{3}{2}\delta^{rd}\delta^{sa}Y_d^{bt}Y_u^{pc} \right) + g_Y^2 \left( \frac{2}{81}\delta^{rd}\delta^{ab}Y_d^{pt}Y_u^{sc} \right. \right. \\
& + \frac{4}{81}\delta^{sa}\delta^{cd}Y_d^{pt}Y_u^{br} + \frac{13}{18}\delta^{rd}\delta^{sa}Y_d^{bt}Y_u^{pc} + \frac{5}{3}\delta^{rd}\delta^{sa}Y_d^{pt}Y_u^{bc} - \frac{20}{81}\delta^{pa}\delta^{cd}Y_d^{bt}Y_u^{sr} \Big) + g_s^2 \left( \frac{4}{27}\delta^{pa}\delta^{cd}Y_d^{bt}Y_u^{sr} + \frac{4}{27}\delta^{sa}\delta^{cd}Y_d^{pt}Y_u^{br} + \frac{8}{27}\delta^{rd}\delta^{ab}Y_d^{pt}Y_u^{sc} \right. \\
& + \frac{4}{9}\delta^{rd}\delta^{ab}Y_d^{st}Y_u^{pc} + \frac{50}{3}\delta^{rd}\delta^{sa}Y_d^{bt}Y_u^{pc} - \frac{1}{9}\delta^{pa}\delta^{cd}Y_d^{st}Y_u^{br} - \frac{1}{9}\delta^{sa}\delta^{cd}Y_d^{bt}Y_u^{pr} - 18\delta^{pa}\delta^{rd}Y_d^{bt}Y_u^{sc} \Big) + \delta^{sa}Y_d^{bt}Y_u^{pc}(Y_u^\dagger Y_u)^{dr} + \delta^{rd}Y_d^{bt}Y_u^{pc}(Y_dY_d^\dagger)^{sa} \\
& + \delta^{rd}\delta^{sa}Y_d^{bt}(Y_dY_d^\dagger Y_u)^{pc} - \frac{1}{2}\delta^{rd}\delta^{sa}Y_u^{pc}(Y_dY_d^\dagger Y_d)^{bt} - T_2\delta^{rd}\delta^{sa}Y_d^{bt}Y_u^{pc} - \delta^{rd}\delta^{sa}Y_d^{bt}(Y_uY_u^\dagger Y_u)^{pc} - 2\delta^{pa}Y_u^{sc}Y_u^{br}(Y_u^\dagger Y_d)^{dt} - 3Y_u^{*ad}Y_d^{bt}Y_u^{pc}Y_u^{sr} \\
& - 3\delta^{rd}Y_d^{bt}Y_u^{pc}(Y_uY_u^\dagger)^{sa} - 3\delta^{rd}\delta^{sa}Y_u^{bc}(Y_uY_u^\dagger Y_d)^{pt} \Big\} C_{qu}^{(\times)abcd} + \left\{ g_s^2 \left( \frac{8}{3}\delta^{pa}\delta^{td}Y_d^{bc}Y_u^{sr} + 4\delta^{sa}\delta^{td}Y_d^{bc}Y_u^{pr} + 9\delta^{pa}\delta^{td}Y_d^{sc}Y_u^{br} - \frac{188}{3}\delta^{sa}\delta^{td}Y_d^{pc}Y_u^{br} \right) \right. \\
& + g_L^2 \left( 3\delta^{pa}\delta^{td}Y_d^{bc}Y_u^{sr} - 3\delta^{sa}\delta^{td}Y_d^{pc}Y_u^{br} \right) + g_Y^2 \left( \frac{10}{27}\delta^{pa}\delta^{cd}Y_d^{bt}Y_u^{sr} + \frac{5}{9}\delta^{pa}\delta^{td}Y_d^{bc}Y_u^{sr} + \frac{7}{9}\delta^{sa}\delta^{td}Y_d^{pc}Y_u^{br} - \frac{2}{27}\delta^{sa}\delta^{cd}Y_d^{pt}Y_u^{br} - \frac{10}{27}\delta^{td}\delta^{ab}Y_d^{pc}Y_u^{sr} \right) \\
& + \frac{3}{2}\delta^{td}Y_d^{pc}Y_u^{br}(Y_dY_d^\dagger)^{sa} - Y_d^{*ad}Y_d^{pt}Y_d^{sc}Y_u^{br} - \delta^{pa}\delta^{td}Y_d^{bc}(Y_dY_d^\dagger Y_u)^{sr} - \delta^{sa}\delta^{td}Y_d^{pc}(Y_uY_u^\dagger Y_u)^{br} - \frac{3}{2}\delta^{pa}Y_d^{sc}Y_d^{bt}(Y_d^\dagger Y_u)^{dr} - 2T_2\delta^{sa}\delta^{td}Y_d^{pc}Y_u^{br} \\
& - 2\delta^{sa}\delta^{td}Y_u^{br}(Y_dY_d^\dagger Y_d)^{pc} - 2\delta^{sa}\delta^{td}Y_u^{br}(Y_uY_u^\dagger Y_d)^{pc} - 3\delta^{sa}Y_d^{pc}Y_u^{br}(Y_d^\dagger Y_d)^{dt} - 3\delta^{sa}\delta^{td}Y_d^{pc}(Y_dY_d^\dagger Y_u)^{br} - 6\delta^{td}Y_d^{pc}Y_u^{br}(Y_uY_u^\dagger)^{sa} \Big\} C_{qd}^{(\parallel)abcd} \\
& + \left\{ \frac{1}{2}\delta^{pa}\delta^{td}Y_d^{sc}(Y_dY_d^\dagger Y_u)^{br} + g_L^2 \left( 9\delta^{pa}\delta^{td}Y_d^{bc}Y_u^{sr} - \frac{3}{2}\delta^{pa}\delta^{td}Y_d^{sc}Y_u^{br} \right) + g_Y^2 \left( \frac{10}{81}\delta^{pa}\delta^{cd}Y_d^{bt}Y_u^{sr} + \frac{5}{3}\delta^{pa}\delta^{td}Y_d^{bc}Y_u^{sr} - \frac{2}{81}\delta^{sa}\delta^{cd}Y_d^{pt}Y_u^{br} - \frac{10}{81}\delta^{td}\delta^{ab}Y_d^{pc}Y_u^{sr} \right. \right. \\
& - \frac{5}{18}\delta^{pa}\delta^{td}Y_d^{sc}Y_u^{br} \Big) + g_s^2 \left( \frac{4}{27}\delta^{pa}\delta^{cd}Y_d^{bt}Y_u^{sr} + \frac{4}{27}\delta^{sa}\delta^{cd}Y_d^{pt}Y_u^{br} + \frac{8}{27}\delta^{td}\delta^{ab}Y_d^{pc}Y_u^{sr} + \frac{4}{9}\delta^{td}\delta^{ab}Y_d^{sc}Y_u^{pr} + \frac{50}{3}\delta^{pa}\delta^{td}Y_d^{sc}Y_u^{br} - \frac{1}{9}\delta^{pa}\delta^{cd}Y_d^{st}Y_u^{br} \right. \\
& - \frac{1}{9}\delta^{sa}\delta^{cd}Y_d^{bt}Y_u^{pr} - 18\delta^{sa}\delta^{td}Y_d^{pc}Y_u^{br} \Big) + \delta^{pa}Y_d^{sc}Y_u^{br}(Y_d^\dagger Y_d)^{dt} + \delta^{td}Y_d^{sc}Y_u^{br}(Y_uY_u^\dagger)^{pa} + \delta^{pa}\delta^{td}Y_u^{br}(Y_uY_u^\dagger Y_d)^{sc} - \frac{1}{2}\delta^{pa}\delta^{td}Y_d^{sc}(Y_uY_u^\dagger Y_u)^{br} \\
& - T_2\delta^{pa}\delta^{td}Y_d^{sc}Y_u^{br} - \delta^{pa}\delta^{td}Y_u^{br}(Y_dY_d^\dagger Y_d)^{sc} - 2\delta^{sa}Y_d^{pc}Y_d^{bt}(Y_d^\dagger Y_u)^{dr} - 3Y_d^{*ad}Y_d^{pt}Y_d^{sc}Y_u^{br} - 3\delta^{td}Y_d^{sc}Y_u^{br}(Y_dY_d^\dagger)^{pa} - 3\delta^{pa}\delta^{td}Y_d^{bc}(Y_dY_d^\dagger Y_u)^{sr} \Big\} C_{qd}^{(\times)abcd} \\
& + \left\{ g_Y^2 \left( \frac{8}{27}\delta^{rb}\delta^{cd}Y_d^{pt}Y_u^{sa} - \frac{40}{81}\delta^{rb}\delta^{ad}Y_d^{pt}Y_u^{sc} \right) - g_s^2 \left( \frac{40}{27}\delta^{rb}\delta^{ad}Y_d^{pt}Y_u^{sc} + \frac{20}{9}\delta^{rb}\delta^{ad}Y_d^{st}Y_u^{pc} \right) - \delta^{rb}Y_u^{pc}Y_u^{sa}(Y_u^\dagger Y_d)^{dt} \right\} C_{uu}^{abcd} + \left\{ g_Y^2 \left( \frac{20}{27}\delta^{tb}\delta^{cd}Y_d^{pa}Y_u^{sr} \right. \right. \\
& - \frac{100}{81}\delta^{tb}\delta^{ad}Y_d^{pc}Y_u^{sr} \Big) - g_s^2 \left( \frac{40}{27}\delta^{tb}\delta^{ad}Y_d^{pc}Y_u^{sr} + \frac{20}{9}\delta^{tb}\delta^{ad}Y_d^{sc}Y_u^{pr} \right) - \delta^{tb}Y_d^{pa}Y_d^{sc}(Y_d^\dagger Y_u)^{dr} \Big\} C_{dd}^{abcd} - \frac{2}{27}\delta^{rd}\delta^{ab}g_Y^2 C_{eu}^{abcd}Y_d^{pt}Y_u^{sc} + \frac{10}{27}\delta^{td}\delta^{ab}g_Y^2 C_{ed}^{abcd}Y_d^{pc}Y_u^{sr} \\
& + \left\{ g_s^2 \left( 31\delta^{rb}\delta^{td}Y_d^{sc}Y_u^{pa} - 56\delta^{rb}\delta^{td}Y_d^{pc}Y_u^{sa} \right) + g_Y^2 \left( \frac{16}{3}\delta^{rb}\delta^{td}Y_d^{pc}Y_u^{sa} - \frac{2}{27}\delta^{rb}\delta^{cd}Y_d^{pt}Y_u^{sa} - \frac{20}{27}\delta^{td}\delta^{ab}Y_d^{pc}Y_u^{sr} \right) + 6\delta^{rb}\delta^{td}g_L^2Y_d^{pc}Y_u^{sa} \right. \\
& - 2T_2\delta^{rb}\delta^{td}Y_d^{pc}Y_u^{sa} - 2\delta^{rb}\delta^{td}Y_u^{sa}(Y_dY_d^\dagger Y_d)^{pc} - 2\delta^{rb}\delta^{td}Y_d^{pc}(Y_dY_d^\dagger Y_u)^{sa} - 2\delta^{rb}\delta^{td}Y_u^{sa}(Y_uY_u^\dagger Y_d)^{pc} - 2\delta^{rb}\delta^{td}Y_d^{pc}(Y_uY_u^\dagger Y_u)^{sa}
\end{aligned}$$



$$\begin{aligned}
& -3\delta^{rb}Y_d^{pc}Y_u^{sa}(Y_d^\dagger Y_d)^{dt} - 3\delta^{td}Y_d^{pc}Y_u^{sa}(Y_u^\dagger Y_u)^{br} \Big\} C_{ud}^{(\parallel)abcd} + \left\{ g_s^2 \left( \frac{4}{27}\delta^{td}\delta^{ab}Y_d^{pc}Y_u^{sr} + \frac{4}{27}\delta^{rb}\delta^{cd}Y_d^{pt}Y_u^{sa} + \frac{2}{9}\delta^{td}\delta^{ab}Y_d^{sc}Y_u^{pr} + \frac{2}{9}\delta^{rb}\delta^{cd}Y_d^{st}Y_u^{pa} \right. \right. \\
& + \frac{127}{3}\delta^{rb}\delta^{td}Y_d^{sc}Y_u^{pa} - 28\delta^{rb}\delta^{td}Y_d^{pc}Y_u^{sa} \Big) + \delta^{rb}\delta^{td}Y_d^{sc}(Y_d Y_d^\dagger Y_u)^{pa} + \delta^{rb}\delta^{td}Y_u^{pa}(Y_u Y_u^\dagger Y_d)^{sc} + \frac{5}{2}\delta^{rb}Y_d^{sc}Y_u^{pa}(Y_d^\dagger Y_d)^{dt} + \frac{5}{2}\delta^{td}Y_d^{sc}Y_u^{pa}(Y_u^\dagger Y_u)^{br} \\
& + 3T_2\delta^{rb}\delta^{td}Y_d^{sc}Y_u^{pa} + 3\delta^{rb}\delta^{td}Y_u^{pa}(Y_d Y_d^\dagger Y_d)^{sc} + 3\delta^{rb}\delta^{td}Y_d^{sc}(Y_u Y_u^\dagger Y_u)^{pa} - g_Y^2 \left( \frac{2}{81}\delta^{rb}\delta^{cd}Y_d^{pt}Y_u^{sa} + \frac{20}{81}\delta^{td}\delta^{ab}Y_d^{pc}Y_u^{sr} + \frac{68}{9}\delta^{rb}\delta^{td}Y_d^{sc}Y_u^{pa} \right) \\
& - 9\delta^{rb}\delta^{td}g_L^2 Y_d^{sc}Y_u^{pa} \Big\} C_{ud}^{(\times)abcd} + \frac{1}{2}Y_e^{*ab}C_{ledq}^{abcd}Y_d^{pt}Y_d^{sc}Y_u^{dr} + C_{ledq}^{*abcd} \left\{ \frac{1}{2}\delta^{pd}\delta^{tc}Y_e^{ab}(Y_d Y_d^\dagger Y_u)^{sr} - \frac{5}{18}\delta^{pd}\delta^{tc}g_Y^2 Y_e^{ab}Y_u^{sr} - g_s^2 \left( \frac{4}{3}\delta^{pd}\delta^{tc}Y_e^{ab}Y_u^{sr} \right. \right. \\
& + 2\delta^{sd}\delta^{tc}Y_e^{ab}Y_u^{pr} \Big) - \frac{3}{2}\delta^{pd}\delta^{tc}g_L^2 Y_e^{ab}Y_u^{sr} \Big\} + \left\{ \frac{1}{4}\delta^{pa}\delta^{td}Y_u^{*cb}(Y_d Y_d^\dagger Y_u)^{sr} + \frac{1}{4}\delta^{rb}\delta^{sc}Y_d^{*ad}(Y_u Y_u^\dagger Y_d)^{pt} + g_L^2 \left( \frac{3}{2}\delta^{rb}\delta^{sc}Y_d^{*ad}Y_d^{pt} + \frac{3}{2}\delta^{pa}\delta^{td}Y_u^{*cb}Y_u^{sr} \right. \right. \\
& - \frac{9}{2}\delta^{rb}\delta^{sa}Y_d^{*cd}Y_d^{pt} - \frac{9}{2}\delta^{pc}\delta^{td}Y_u^{*ab}Y_u^{sr} \Big) + g_Y^2 g_s^2 \left( \frac{2}{9}\delta^{pa}\delta^{rb}\delta^{sc}\delta^{td} - \frac{527}{54}\delta^{pc}\delta^{rb}\delta^{sa}\delta^{td} \right) + g_s^2 g_L^2 \left( 6\delta^{pa}\delta^{rb}\delta^{sc}\delta^{td} - \frac{99}{2}\delta^{pc}\delta^{rb}\delta^{sa}\delta^{td} \right) \\
& + g_s^4 \left( \frac{40}{3}\delta^{pa}\delta^{rb}\delta^{sc}\delta^{td} + \frac{140}{9}\delta^{pc}\delta^{rb}\delta^{sa}\delta^{td} \right) + \delta^{pc}\delta^{sa}(Y_d^\dagger Y_d)^{dt}(Y_u^\dagger Y_u)^{br} + \delta^{rb}\delta^{td}(Y_d Y_d^\dagger)^{pc}(Y_u Y_u^\dagger)^{sa} + g_Y^2 \left( \frac{2}{9}\delta^{pc}\delta^{rb}\delta^{td}(Y_d Y_d^\dagger)^{sa} + \frac{10}{9}\delta^{pc}\delta^{rb}\delta^{sa}(Y_d^\dagger Y_d)^{dt} \right. \\
& + \frac{35}{18}\delta^{pa}\delta^{td}Y_u^{*cb}Y_u^{sr} + \frac{20}{9}\delta^{rb}\delta^{sa}\delta^{td}(Y_u Y_u^\dagger)^{pc} - \frac{1}{18}\delta^{rb}\delta^{sc}Y_d^{*ad}Y_d^{pt} - \frac{2}{9}\delta^{pc}\delta^{sa}\delta^{td}(Y_u^\dagger Y_u)^{br} - \frac{4}{9}\delta^{pc}\delta^{rb}\delta^{td}(Y_u Y_u^\dagger)^{sa} - \frac{5}{6}\delta^{rb}\delta^{sa}Y_d^{*cd}Y_d^{pt} \\
& - \frac{5}{6}\delta^{pc}\delta^{td}Y_u^{*ab}Y_u^{sr} - \frac{10}{9}\delta^{rb}\delta^{sa}\delta^{td}(Y_d Y_d^\dagger)^{pc} \Big) + \frac{3}{2}\delta^{rb}\delta^{td}(Y_d Y_d^\dagger)^{sa}(Y_u Y_u^\dagger)^{pc} + \frac{3}{2}\delta^{pc}\delta^{td}Y_u^{*ab}(Y_d Y_d^\dagger Y_u)^{sr} + \frac{3}{2}\delta^{rb}\delta^{sa}Y_d^{*cd}(Y_u Y_u^\dagger Y_d)^{pt} \\
& + 2\delta^{pc}\delta^{rb}(Y_d^\dagger Y_d)^{dt}(Y_d Y_d^\dagger)^{sa} + 2\delta^{rb}\delta^{td}(Y_d Y_d^\dagger)^{pc}(Y_d Y_d^\dagger)^{sa} + 2\delta^{sa}\delta^{td}(Y_u^\dagger Y_u)^{br}(Y_u Y_u^\dagger)^{pc} + 2\delta^{rb}\delta^{td}(Y_u Y_u^\dagger)^{pc}(Y_u Y_u^\dagger)^{sa} + 5\delta^{pa}\delta^{sc}(Y_d^\dagger Y_u)^{dr}(Y_u^\dagger Y_d)^{bt} \\
& + \frac{199}{12}\delta^{pc}\delta^{rb}\delta^{sa}\delta^{td}g_L^4 - \frac{1}{2}\delta^{sa}\delta^{td}(Y_u^\dagger Y_u)^{br}(Y_d Y_d^\dagger)^{pc} - \frac{1}{2}\delta^{pc}\delta^{td}(Y_u^\dagger Y_u)^{br}(Y_d Y_d^\dagger)^{sa} - \frac{1}{2}\delta^{rb}\delta^{sa}(Y_d^\dagger Y_d)^{dt}(Y_u Y_u^\dagger)^{pc} - \frac{1}{2}\delta^{pc}\delta^{rb}(Y_d^\dagger Y_d)^{dt}(Y_u Y_u^\dagger)^{sa} \\
& - g_s^2 \left( \frac{4}{3}\delta^{rb}\delta^{sa}\delta^{td}(Y_d Y_d^\dagger)^{pc} + \frac{4}{3}\delta^{pc}\delta^{rb}\delta^{td}(Y_d Y_d^\dagger)^{sa} + \frac{4}{3}\delta^{rb}\delta^{sa}\delta^{td}(Y_u Y_u^\dagger)^{pc} + \frac{4}{3}\delta^{pc}\delta^{rb}\delta^{td}(Y_u Y_u^\dagger)^{sa} + 2\delta^{rb}\delta^{sc}\delta^{td}(Y_d Y_d^\dagger)^{pa} + 2\delta^{pa}\delta^{rb}\delta^{td}(Y_d Y_d^\dagger)^{sc} \right. \\
& + 2\delta^{rb}\delta^{sc}\delta^{td}(Y_u Y_u^\dagger)^{pa} + 2\delta^{pa}\delta^{rb}\delta^{td}(Y_u Y_u^\dagger)^{sc} + \frac{8}{3}\delta^{rb}\delta^{sc}Y_d^{*ad}Y_d^{pt} + \frac{8}{3}\delta^{pa}\delta^{td}Y_u^{*cb}Y_u^{sr} + \frac{8}{3}\delta^{pc}\delta^{rb}\delta^{sa}(Y_d^\dagger Y_d)^{dt} + \frac{8}{3}\delta^{pc}\delta^{sa}\delta^{td}(Y_u^\dagger Y_u)^{br} \\
& + 4\delta^{pc}\delta^{rb}Y_d^{*ad}Y_d^{st} + 4\delta^{rb}\delta^{sa}Y_d^{*cd}Y_d^{pt} + 4\delta^{pc}\delta^{td}Y_u^{*ab}Y_u^{sr} + 4\delta^{sa}\delta^{td}Y_u^{*cb}Y_u^{pr} + 4\delta^{pa}\delta^{rb}\delta^{sc}(Y_d^\dagger Y_d)^{dt} + 4\delta^{pa}\delta^{sc}\delta^{td}(Y_u^\dagger Y_u)^{br} + 6\delta^{pa}\delta^{rb}Y_d^{*cd}Y_d^{st} \\
& + 6\delta^{sc}\delta^{td}Y_u^{*ab}Y_u^{pr} \Big) - \frac{115}{108}\delta^{pc}\delta^{rb}\delta^{sa}\delta^{td}g_Y^4 \Big\} C_{quqd}^{(\parallel)abcd} + \left( C_{quqd}^{(\parallel)*} \right)^{abcd} \left\{ \frac{1}{4}Y_d^{ad}Y_d^{ct}Y_u^{pb}Y_u^{sr} + \frac{1}{4}Y_d^{pt}Y_d^{sd}Y_u^{ar}Y_u^{cb} + \frac{3}{2}Y_d^{at}Y_d^{cd}Y_u^{pb}Y_u^{sr} + \frac{3}{2}Y_d^{pt}Y_d^{sd}Y_u^{ab}Y_u^{cr} \right. \\
& - \frac{1}{2}Y_d^{sd}Y_d^{at}Y_u^{pb}Y_u^{cr} \Big\} + \left\{ \frac{1}{2}\delta^{pc}\delta^{td}Y_u^{*ab}(Y_d Y_d^\dagger Y_u)^{sr} + \frac{1}{2}\delta^{rb}\delta^{sa}Y_d^{*cd}(Y_u Y_u^\dagger Y_d)^{pt} + \frac{3}{4}\delta^{pa}\delta^{td}Y_u^{*cb}(Y_d Y_d^\dagger Y_u)^{sr} + \frac{3}{4}\delta^{rb}\delta^{sc}Y_d^{*ad}(Y_u Y_u^\dagger Y_d)^{pt} \right. \\
& + \frac{7}{8}\delta^{pa}\delta^{rb}\delta^{sc}\delta^{td}g_Y^2 g_L^2 + g_s^4 \left( \frac{110}{3}\delta^{pc}\delta^{rb}\delta^{sa}\delta^{td} + \frac{971}{9}\delta^{pa}\delta^{rb}\delta^{sc}\delta^{td} \right) + g_s^2 \left( 2\delta^{rb}\delta^{sa}\delta^{td}(Y_d Y_d^\dagger)^{pc} + 2\delta^{pc}\delta^{rb}\delta^{td}(Y_d Y_d^\dagger)^{sa} + 2\delta^{rb}\delta^{sa}\delta^{td}(Y_u Y_u^\dagger)^{pc} \right. \\
& + 2\delta^{pc}\delta^{rb}\delta^{td}(Y_u Y_u^\dagger)^{sa} + 4\delta^{pc}\delta^{rb}\delta^{sa}(Y_d^\dagger Y_d)^{dt} + 4\delta^{pc}\delta^{sa}\delta^{td}(Y_u^\dagger Y_u)^{br} - \frac{4}{3}\delta^{rb}\delta^{sa}Y_d^{*cd}Y_d^{pt} - \frac{4}{3}\delta^{pc}\delta^{td}Y_u^{*ab}Y_u^{sr} - 2\delta^{pa}\delta^{rb}Y_d^{*cd}Y_d^{st} - 2\delta^{rb}\delta^{sc}Y_d^{*ad}Y_d^{pt}
\end{aligned}$$

$$\begin{aligned}
& -2\delta^{pa}\delta^{td}Y_u^{*cb}Y_u^{sr} - 2\delta^{sc}\delta^{td}Y_u^{*ab}Y_u^{pr} - 3\delta^{pc}\delta^{rb}Y_d^{*ad}Y_d^{st} - 3\delta^{sa}\delta^{td}Y_u^{*cb}Y_u^{pr} - 6\delta^{rb}\delta^{sc}\delta^{td}(Y_dY_d^\dagger)^{pa} - 6\delta^{pa}\delta^{rb}\delta^{td}(Y_dY_d^\dagger)^{sc} - 6\delta^{rb}\delta^{sc}\delta^{td}(Y_uY_u^\dagger)^{pa} \\
& - 6\delta^{pa}\delta^{rb}\delta^{td}(Y_uY_u^\dagger)^{sc} - 12\delta^{pa}\delta^{rb}\delta^{sc}(Y_d^\dagger Y_d)^{dt} - 12\delta^{pa}\delta^{sc}\delta^{td}(Y_u^\dagger Y_u)^{br} \Big) + g_Y^2 \Big( \frac{9}{8}\delta^{pa}\delta^{sc}\delta^{td}(Y_u^\dagger Y_u)^{br} + \frac{13}{8}\delta^{pa}\delta^{rb}\delta^{sc}(Y_d^\dagger Y_d)^{dt} \\
& + \frac{109}{48}\delta^{pa}\delta^{rb}\delta^{td}(Y_dY_d^\dagger)^{sc} + \frac{185}{48}\delta^{rb}\delta^{sc}\delta^{td}(Y_uY_u^\dagger)^{pa} + \frac{35}{6}\delta^{pa}\delta^{td}Y_u^{*cb}Y_u^{sr} - \frac{1}{6}\delta^{rb}\delta^{sc}Y_d^{*ad}Y_d^{pt} - \frac{5}{18}\delta^{rb}\delta^{sa}Y_d^{*cd}Y_d^{pt} - \frac{5}{18}\delta^{pc}\delta^{td}Y_u^{*ab}Y_u^{sr} \\
& - \frac{19}{48}\delta^{rb}\delta^{sc}\delta^{td}(Y_dY_d^\dagger)^{pa} - \frac{71}{48}\delta^{pa}\delta^{rb}\delta^{td}(Y_uY_u^\dagger)^{sc} \Big) + g_L^2 \Big( \frac{33}{16}\delta^{rb}\delta^{sc}\delta^{td}(Y_dY_d^\dagger)^{pa} + \frac{33}{16}\delta^{pa}\delta^{rb}\delta^{td}(Y_dY_d^\dagger)^{sc} + \frac{33}{16}\delta^{rb}\delta^{sc}\delta^{td}(Y_uY_u^\dagger)^{pa} \\
& + \frac{33}{16}\delta^{pa}\delta^{rb}\delta^{td}(Y_uY_u^\dagger)^{sc} + \frac{9}{2}\delta^{rb}\delta^{sc}Y_d^{*ad}Y_d^{pt} + \frac{9}{2}\delta^{pa}\delta^{td}Y_u^{*cb}Y_u^{sr} + \frac{51}{8}\delta^{pa}\delta^{rb}\delta^{sc}(Y_d^\dagger Y_d)^{dt} + \frac{51}{8}\delta^{pa}\delta^{sc}\delta^{td}(Y_u^\dagger Y_u)^{br} - \frac{3}{2}\delta^{rb}\delta^{sa}Y_d^{*cd}Y_d^{pt} \\
& - \frac{3}{2}\delta^{pc}\delta^{td}Y_u^{*ab}Y_u^{sr} \Big) + 2\delta^{pa}\delta^{rb}(Y_d^\dagger Y_d)^{dt}(Y_dY_d^\dagger)^{sc} + 2\delta^{sc}\delta^{td}(Y_u^\dagger Y_u)^{br}(Y_uY_u^\dagger)^{pa} - \frac{1}{4}\delta^{pa}\delta^{rb}\delta^{sc}(Y_d^\dagger Y_dY_d^\dagger Y_d)^{dt} - \frac{1}{4}\delta^{pa}\delta^{rb}\delta^{sc}(Y_d^\dagger Y_uY_u^\dagger Y_d)^{dt} \\
& - \frac{1}{4}\delta^{pa}\delta^{sc}\delta^{td}(Y_u^\dagger Y_dY_d^\dagger Y_u)^{br} - \frac{1}{4}\delta^{pa}\delta^{sc}\delta^{td}(Y_u^\dagger Y_uY_u^\dagger Y_u)^{br} - \frac{1}{4}\delta^{rb}\delta^{sc}\delta^{td}(Y_dY_d^\dagger Y_dY_d^\dagger)^{pa} - \frac{1}{4}\delta^{pa}\delta^{rb}\delta^{td}(Y_dY_d^\dagger Y_dY_d^\dagger)^{sc} - \frac{1}{4}\delta^{rb}\delta^{sc}\delta^{td}(Y_uY_u^\dagger Y_uY_u^\dagger)^{pa} \\
& - \frac{1}{4}\delta^{pa}\delta^{rb}\delta^{td}(Y_uY_u^\dagger Y_uY_u^\dagger)^{sc} - \frac{29}{48}\delta^{pa}\delta^{rb}\delta^{sc}\delta^{td}g_L^4 - \frac{3}{4}T_2\delta^{rb}\delta^{sc}\delta^{td}(Y_dY_d^\dagger)^{pa} - \frac{3}{4}T_2\delta^{pa}\delta^{rb}\delta^{td}(Y_dY_d^\dagger)^{sc} - \frac{3}{4}T_2\delta^{rb}\delta^{sc}\delta^{td}(Y_uY_u^\dagger)^{pa} \\
& - \frac{3}{4}T_2\delta^{pa}\delta^{rb}\delta^{td}(Y_uY_u^\dagger)^{sc} - g_Y^2g_s^2 \Big( \frac{19}{18}\delta^{pc}\delta^{rb}\delta^{sa}\delta^{td} + \frac{136}{27}\delta^{pa}\delta^{rb}\delta^{sc}\delta^{td} \Big) - g_s^2g_L^2 \Big( \frac{21}{2}\delta^{pc}\delta^{rb}\delta^{sa}\delta^{td} + 12\delta^{pa}\delta^{rb}\delta^{sc}\delta^{td} \Big) - \delta^{sc}\delta^{td}(Y_u^\dagger Y_u)^{br}(Y_dY_d^\dagger)^{pa} \\
& - \delta^{pa}\delta^{rb}(Y_d^\dagger Y_d)^{dt}(Y_uY_u^\dagger)^{sc} - \frac{5}{4}\delta^{pa}\delta^{td}(Y_u^\dagger Y_u)^{br}(Y_dY_d^\dagger)^{sc} - \frac{5}{4}\delta^{rb}\delta^{sc}(Y_d^\dagger Y_d)^{dt}(Y_uY_u^\dagger)^{pa} - \frac{3}{2}T_2\delta^{pa}\delta^{rb}\delta^{sc}(Y_d^\dagger Y_d)^{dt} - \frac{3}{2}T_2\delta^{pa}\delta^{sc}\delta^{td}(Y_u^\dagger Y_u)^{br} \\
& - 2\delta^{rb}\delta^{sc}(Y_d^\dagger Y_d)^{dt}(Y_dY_d^\dagger)^{pa} - 2\delta^{pa}\delta^{td}(Y_u^\dagger Y_u)^{br}(Y_uY_u^\dagger)^{sc} - 3\delta^{pc}\delta^{sa}(Y_d^\dagger Y_u)^{dr}(Y_u^\dagger Y_d)^{bt} - 3\delta^{pa}\delta^{sc}(Y_d^\dagger Y_d)^{dt}(Y_u^\dagger Y_u)^{br} - 3\delta^{rb}\delta^{td}(Y_dY_d^\dagger)^{pa}(Y_uY_u^\dagger)^{sc} \\
& - \frac{7}{2}\delta^{rb}\delta^{td}(Y_dY_d^\dagger)^{sc}(Y_uY_u^\dagger)^{pa} - \frac{515}{144}\delta^{pa}\delta^{rb}\delta^{sc}\delta^{td}g_Y^4 \Big\} C_{quqd}^{(\times)abcd} + \Big( C_{quqd}^{(\times)*} \Big)^{abcd} \Big\{ \frac{1}{2}Y_d^{at}Y_d^{cd}Y_u^{pb}Y_u^{sr} + \frac{1}{2}Y_d^{pt}Y_d^{sd}Y_u^{ab}Y_u^{cr} + \frac{3}{4}Y_d^{ad}Y_d^{ct}Y_u^{pb}Y_u^{sr} + \frac{3}{4}Y_d^{pt}Y_d^{sd}Y_u^{ar}Y_u^{cb} \\
& + 2Y_d^{pd}Y_d^{at}Y_u^{sb}Y_u^{cr} - Y_d^{sd}Y_d^{ct}Y_u^{pb}Y_u^{ar} \Big\} + \Big\{ \frac{5}{18}\delta^{rd}\delta^{sc}g_Y^2Y_e^{*ab}Y_d^{pt} + g_s^2 \Big( \frac{4}{3}\delta^{rd}\delta^{sc}Y_e^{*ab}Y_d^{pt} + 2\delta^{pc}\delta^{rd}Y_e^{*ab}Y_d^{st} \Big) + \frac{3}{2}\delta^{rd}\delta^{sc}g_L^2Y_e^{*ab}Y_d^{pt} \\
& - \frac{1}{2}\delta^{rd}\delta^{sc}Y_e^{*ab}(Y_uY_u^\dagger Y_d)^{pt} \Big\} C_{lequ}^{abcd} - \frac{1}{2}C_{lequ}^{*abcd}Y_d^{ct}Y_e^{ab}Y_u^{pd}Y_u^{sr} + \Big\{ \frac{1}{4}\delta^{rb}\delta^{sc}Y_e^{*ad}(Y_uY_u^\dagger Y_d)^{pt} + \frac{11}{18}\delta^{rb}\delta^{sc}g_Y^2Y_e^{*ad}Y_d^{pt} + \frac{3}{2}\delta^{rb}\delta^{sc}g_L^2Y_e^{*ad}Y_d^{pt} \\
& - g_s^2 \Big( \frac{2}{3}\delta^{rb}\delta^{sc}Y_e^{*ad}Y_d^{pt} + \delta^{pc}\delta^{rb}Y_e^{*ad}Y_d^{st} \Big) \Big\} C_{luqe}^{abcd} + \frac{1}{4}C_{luqe}^{*abcd}Y_d^{ct}Y_e^{ad}Y_u^{pb}Y_u^{sr} + \Big\{ g_L^2 \Big( 42\delta^{pa}\delta^{sc}Y_d^{bt}Y_u^{dr} - \frac{10}{3}\delta^{pa}\delta^{bc}Y_d^{dt}Y_u^{sr} - \frac{10}{3}\delta^{sa}\delta^{bc}Y_d^{pt}Y_u^{dr} \Big) \\
& + g_s^2 \Big( 56\delta^{pa}\delta^{sc}Y_d^{dt}Y_u^{br} - \frac{40}{27}\delta^{pa}\delta^{bc}Y_d^{dt}Y_u^{sr} - \frac{40}{27}\delta^{sa}\delta^{bc}Y_d^{pt}Y_u^{dr} - \frac{26}{9}\delta^{pa}\delta^{bc}Y_d^{st}Y_u^{dr} - \frac{26}{9}\delta^{sa}\delta^{bc}Y_d^{dt}Y_u^{pr} - 112\delta^{pa}\delta^{sc}Y_d^{bt}Y_u^{dr} \Big) + g_Y^2 \Big( \frac{4}{27}\delta^{sa}\delta^{cd}Y_d^{pt}Y_u^{br} \\
& + \frac{50}{81}\delta^{pa}\delta^{bc}Y_d^{dt}Y_u^{sr} + \frac{2}{3}\delta^{pa}\delta^{sc}Y_d^{bt}Y_u^{dr} - \frac{10}{81}\delta^{sa}\delta^{bc}Y_d^{pt}Y_u^{dr} - \frac{20}{27}\delta^{pa}\delta^{cd}Y_d^{bt}Y_u^{sr} \Big) + 5\delta^{pa}Y_d^{bt}Y_u^{dr}(Y_dY_d^\dagger)^{sc} + 5\delta^{sa}Y_d^{dt}Y_u^{br}(Y_uY_u^\dagger)^{pc} \\
& - 2\delta^{pa}\delta^{sc}Y_u^{dr}(Y_dY_d^\dagger Y_d)^{bt} - 2\delta^{pa}\delta^{sc}Y_d^{bt}(Y_uY_u^\dagger Y_u)^{dr} - 4T_2\delta^{pa}\delta^{sc}Y_d^{bt}Y_u^{dr} - 6\delta^{pa}\delta^{sc}Y_d^{bt}(Y_dY_d^\dagger Y_u)^{dr} - 6\delta^{pa}\delta^{sc}Y_u^{dr}(Y_uY_u^\dagger Y_d)^{bt}
\end{aligned}$$

$$\begin{aligned}
& -12\delta^{sa}Y_d^{dt}Y_u^{br}(Y_dY_d^\dagger)^{pc} - 12\delta^{pa}Y_d^{bt}Y_u^{dr}(Y_uY_u^\dagger)^{sc} \Big\} C_{qq}^{(\parallel)abcd} + \left\{ g_s^2 \left( 112\delta^{pa}\delta^{sc}Y_d^{bt}Y_u^{dr} - \frac{80}{27}\delta^{pa}\delta^{bc}Y_d^{dt}Y_u^{sr} - \frac{80}{27}\delta^{sa}\delta^{bc}Y_d^{pt}Y_u^{dr} - \frac{52}{9}\delta^{pa}\delta^{bc}Y_d^{st}Y_u^{dr} \right. \right. \\
& - \frac{52}{9}\delta^{sa}\delta^{bc}Y_d^{dt}Y_u^{pr} - 56\delta^{pa}\delta^{sc}Y_d^{dt}Y_u^{br} \Big) + g_Y^2 \left( \frac{2}{27}\delta^{sa}\delta^{cd}Y_d^{pt}Y_u^{br} + \frac{100}{81}\delta^{pa}\delta^{bc}Y_d^{dt}Y_u^{sr} - \frac{20}{81}\delta^{sa}\delta^{bc}Y_d^{pt}Y_u^{dr} - \frac{10}{27}\delta^{pa}\delta^{cd}Y_d^{bt}Y_u^{sr} - \frac{2}{3}\delta^{pa}\delta^{sc}Y_d^{bt}Y_u^{dr} \right) \\
& + g_L^2 \left( 2\delta^{pa}\delta^{cd}Y_d^{bt}Y_u^{sr} + 2\delta^{sa}\delta^{cd}Y_d^{pt}Y_u^{br} - 42\delta^{pa}\delta^{sc}Y_d^{bt}Y_u^{dr} \right) + 2\delta^{pa}\delta^{sc}Y_u^{dr}(Y_dY_d^\dagger)^{bt} + 2\delta^{pa}\delta^{sc}Y_d^{bt}(Y_uY_u^\dagger)^{dr} + 4T_2\delta^{pa}\delta^{sc}Y_d^{bt}Y_u^{dr} \\
& + 6\delta^{pa}\delta^{sc}Y_d^{bt}(Y_dY_d^\dagger Y_u)^{dr} + 6\delta^{pa}\delta^{sc}Y_u^{dr}(Y_uY_u^\dagger Y_d)^{bt} + 10\delta^{pa}Y_d^{bt}Y_u^{dr}(Y_dY_d^\dagger)^{sc} + 10\delta^{sa}Y_d^{dt}Y_u^{br}(Y_uY_u^\dagger)^{pc} - 6\delta^{sa}Y_d^{dt}Y_u^{br}(Y_dY_d^\dagger)^{pc} \\
& - 6\delta^{pa}Y_d^{bt}Y_u^{dr}(Y_uY_u^\dagger)^{sc} \Big\} C_{qq}^{(\times)abcd} + g_Y^2 \left\{ \frac{10}{27}\delta^{pc}\delta^{ab}Y_d^{dt}Y_u^{sr} - \frac{2}{27}\delta^{sc}\delta^{ab}Y_d^{pt}Y_u^{dr} \right\} C_{\ell q}^{(\parallel)abcd} + \left\{ g_Y^2 \left( \frac{5}{27}\delta^{pc}\delta^{ab}Y_d^{dt}Y_u^{sr} - \frac{1}{27}\delta^{sc}\delta^{ab}Y_d^{pt}Y_u^{dr} \right) \right. \\
& \left. + g_L^2 \left( \frac{1}{3}\delta^{pc}\delta^{ab}Y_d^{dt}Y_u^{sr} + \frac{1}{3}\delta^{sc}\delta^{ab}Y_d^{pt}Y_u^{dr} \right) \right\} C_{\ell q}^{(\times)abcd}, \tag{12.6}
\end{aligned}$$

## 12.4 $C_{\ell equ}$

$$\begin{aligned}
\beta_{C_{\ell equ}^{prst}}^{(1)} &= \frac{10}{3}\delta^{pa}\delta^{rb}g_Y^2C_{eB}^{ab}Y_u^{st} - 3\delta^{pa}\delta^{rb}g_L^2C_{eW}^{ab}Y_u^{st} - 6\delta^{sa}\delta^{tb}g_Y^2C_{uB}^{ab}Y_e^{pr} - 3\delta^{sa}\delta^{tb}g_L^2C_{uW}^{ab}Y_e^{pr} + 4\delta^{pa}\delta^{rd}C_{\ell e}^{abcd}Y_e^{bc}Y_u^{st} + 4\delta^{sa}\delta^{td}C_{qu}^{(\parallel)abcd}Y_e^{pr}Y_u^{bc} \\
& + 12\delta^{sa}\delta^{td}C_{qu}^{(\times)abcd}Y_e^{pr}Y_u^{bc} + 4\delta^{rb}\delta^{td}C_{eu}^{abcd}Y_e^{pa}Y_u^{sc} - 2 \left\{ 3\delta^{pa}\delta^{rb}Y_d^{dc}Y_u^{st} - \delta^{pa}\delta^{rb}Y_d^{sc}Y_u^{dt} \right\} C_{\ell edq}^{abcd} - \left\{ \delta^{sc}\delta^{tb}Y_d^{*ad}Y_e^{pr} + 6\delta^{sa}\delta^{tb}Y_d^{*cd}Y_e^{pr} \right\} C_{quqd}^{(\parallel)abcd} \\
& - \left\{ 2\delta^{sa}\delta^{tb}Y_d^{*cd}Y_e^{pr} + 3\delta^{sc}\delta^{tb}Y_d^{*ad}Y_e^{pr} \right\} C_{quqd}^{(\times)abcd} + \left\{ \frac{1}{2} \left( \delta^{pa}\delta^{rb}\delta^{td}(Y_dY_d^\dagger)^{sc} + \delta^{rb}\delta^{sc}\delta^{td}(Y_eY_e^\dagger)^{pa} + \delta^{pa}\delta^{rb}\delta^{td}(Y_uY_u^\dagger)^{sc} + 2\delta^{pa}\delta^{sc}\delta^{td}(Y_e^\dagger Y_e)^{br} \right. \right. \\
& \left. + 2\delta^{pa}\delta^{rb}\delta^{sc}(Y_u^\dagger Y_u)^{dt} + 4\delta^{sc}\delta^{td}Y_e^{*ab}Y_e^{pr} + 12\delta^{pa}\delta^{rb}Y_u^{*cd}Y_u^{st} \right) - \frac{3}{2}\delta^{pa}\delta^{rb}\delta^{sc}\delta^{td}g_L^2 - \frac{37}{6}\delta^{pa}\delta^{rb}\delta^{sc}\delta^{td}g_Y^2 - 8\delta^{pa}\delta^{rb}\delta^{sc}\delta^{td}g_s^2 \Big\} C_{\ell equ}^{abcd} \\
& + \left\{ \frac{16}{3}\delta^{pa}\delta^{rd}\delta^{sc}\delta^{tb}g_s^2 - \frac{5}{9}\delta^{pa}\delta^{rd}\delta^{sc}\delta^{tb}g_Y^2 - \delta^{sc}\delta^{tb}Y_e^{*ad}Y_e^{pr} - 3\delta^{pa}\delta^{rd}Y_u^{*cb}Y_u^{st} - 3\delta^{pa}\delta^{rd}\delta^{sc}\delta^{tb}g_L^2 \right\} C_{\ell uqe}^{abcd} + 4\delta^{pa}\delta^{sc}C_{\ell q}^{(\parallel)abcd}Y_e^{br}Y_u^{dt} \\
& - 4\delta^{pa}\delta^{sc}C_{\ell q}^{(\times)abcd}Y_e^{br}Y_u^{dt}, \tag{12.7}
\end{aligned}$$

$$\begin{aligned}
\beta_{C_{\ell equ}^{prst}}^{(2)} &= 2 \left( 2Y_e^{pr}Y_u^{st}T_{\ell H} - 3Y_u^{st}(C_{\ell HH}^\dagger C_{\ell HH}Y_e)^{pr} \right) + \left\{ \frac{1}{2}Y_e^{pr}(Y_dY_d^\dagger Y_u)^{st} + \frac{3}{2}Y_u^{st}(Y_eY_e^\dagger Y_e)^{pr} + \frac{3}{2}Y_e^{pr}(Y_uY_u^\dagger Y_u)^{st} - \frac{1}{18}g_Y^2Y_e^{pr}Y_u^{st} - \frac{1}{6}g_L^2Y_e^{pr}Y_u^{st} \right. \\
& - \lambda Y_e^{pr}Y_u^{st} \Big\} C_{HD}^{(\parallel)} + \left\{ \frac{3}{2}Y_u^{st}(Y_eY_e^\dagger Y_e)^{pr} + \frac{3}{2}Y_e^{pr}(Y_uY_u^\dagger Y_u)^{st} - \frac{1}{9}g_Y^2Y_e^{pr}Y_u^{st} - \frac{1}{2}Y_e^{pr}(Y_dY_d^\dagger Y_u)^{st} - \lambda Y_e^{pr}Y_u^{st} \right\} C_{HD}^{(\times)} - \frac{53}{9}g_Y^4C_{HB}Y_e^{pr}Y_u^{st} \\
& + \frac{53i}{9}g_Y^4C_{H\bar{B}}Y_e^{pr}Y_u^{st} - 3g_L^4C_{HW}Y_e^{pr}Y_u^{st} + 3ig_L^4C_{H\bar{W}}Y_e^{pr}Y_u^{st} - \frac{32}{3}g_s^4C_{HG}Y_e^{pr}Y_u^{st} + \frac{32i}{3}g_s^4C_{H\bar{G}}Y_e^{pr}Y_u^{st} + \frac{7}{2}g_Y^2g_L^2C_{HWB}Y_e^{pr}Y_u^{st}
\end{aligned}$$

$$\begin{aligned}
& -\frac{7i}{2}g_Y^2g_L^2C_{H\widetilde{W}B}Y_e^{pr}Y_u^{st}-\frac{57}{2}g_L^6C_WY_e^{pr}Y_u^{st}-\frac{19i}{2}g_L^6C_{\widetilde{W}}Y_e^{pr}Y_u^{st}+88g_s^6C_GY_e^{pr}Y_u^{st}+24ig_s^6C_{\widetilde{G}}Y_e^{pr}Y_u^{st}+\left\{6\delta^{pa}\delta^{rb}(Y_uY_u^\dagger Y_u)^{st}-3\delta^{pa}\delta^{rb}\lambda Y_u^{st}\right\}C_{eH}^{ab}\\
& +\left\{6\delta^{sa}\delta^{tb}(Y_eY_e^\dagger Y_e)^{pr}-3\delta^{sa}\delta^{tb}\lambda Y_e^{pr}\right\}C_{uH}^{ab}+\left\{g_Y^2\left(\frac{1}{3}\delta^{pa}\delta^{rb}(Y_dY_d^\dagger Y_u)^{st}+\frac{2}{3}\delta^{pa}Y_u^{st}(Y_e^\dagger Y_e)^{br}+\frac{4}{3}\delta^{rb}Y_u^{st}(Y_eY_e^\dagger)^{pa}+\frac{22}{3}\delta^{pa}\delta^{rb}Y_u^{st}\text{Tr}\left[Y_e^\dagger Y_e\right]\right.\right.\\
& -2\delta^{pa}\delta^{rb}Y_u^{st}\text{Tr}\left[Y_d^\dagger Y_d\right]-3Y_e^{*ab}Y_e^{pr}Y_u^{st}-4\delta^{pa}\delta^{rb}(Y_uY_u^\dagger Y_u)^{st}-5\delta^{pa}\delta^{rb}Y_u^{st}\text{Tr}\left[Y_u^\dagger Y_u\right]\left.\right)+\frac{7}{2}\delta^{pa}\delta^{rb}g_Y^2g_L^2Y_u^{st}+\frac{569}{27}\delta^{pa}\delta^{rb}g_Y^4Y_u^{st}\\
& -\frac{80}{9}\delta^{pa}\delta^{rb}g_Y^2g_s^2Y_u^{st}\left\}C_{eB}^{ab}+6g_Y^2C_{eB}^{*ab}Y_e^{pr}Y_e^{ab}Y_u^{st}+\left\{g_L^2\left(\frac{3}{2}Y_e^{*ab}Y_e^{pr}Y_u^{st}+\frac{9}{2}\delta^{pa}\delta^{rb}(Y_dY_d^\dagger Y_u)^{st}+\frac{9}{2}\delta^{pa}\delta^{rb}Y_u^{st}\text{Tr}\left[Y_u^\dagger Y_u\right]-3\delta^{pa}\delta^{rb}Y_u^{st}\text{Tr}\left[Y_e^\dagger Y_e\right]\right.\right.\\
& -9\delta^{pa}\delta^{rb}Y_u^{st}\text{Tr}\left[Y_d^\dagger Y_d\right]\left.\right)+8\delta^{pa}\delta^{rb}g_s^2g_L^2Y_u^{st}-\frac{59}{6}\delta^{pa}\delta^{rb}g_L^4Y_u^{st}-\frac{247}{12}\delta^{pa}\delta^{rb}g_Y^2g_L^2Y_u^{st}\left\}C_{eW}^{ab}-3g_L^2C_{eW}^{*ab}Y_e^{pr}Y_e^{ab}Y_u^{st}+\left\{g_Y^2\left(\frac{2}{3}\delta^{sa}Y_e^{pr}(Y_u^\dagger Y_u)^{bt}\right.\right.\\
& +\frac{4}{3}\delta^{tb}Y_e^{pr}(Y_uY_u^\dagger)^{sa}+\frac{7}{3}\delta^{tb}Y_e^{pr}(Y_dY_d^\dagger)^{sa}+3\delta^{sa}\delta^{tb}Y_e^{pr}\text{Tr}\left[Y_e^\dagger Y_e\right]+5Y_u^{*ab}Y_e^{pr}Y_u^{st}+8\delta^{sa}\delta^{tb}(Y_eY_e^\dagger Y_e)^{pr}+9\delta^{sa}\delta^{tb}Y_e^{pr}\text{Tr}\left[Y_d^\dagger Y_d\right]\\
& -6\delta^{sa}\delta^{tb}Y_e^{pr}\text{Tr}\left[Y_u^\dagger Y_u\right]\left.\right)-\frac{229}{27}\delta^{sa}\delta^{tb}g_Y^4Y_e^{pr}-\frac{27}{2}\delta^{sa}\delta^{tb}g_Y^2g_L^2Y_e^{pr}-\frac{448}{9}\delta^{sa}\delta^{tb}g_Y^2g_s^2Y_e^{pr}\left\}C_{uB}^{ab}-10g_Y^2C_{uB}^{*ab}Y_e^{pr}Y_u^{st}Y_u^{ab}\\
& +\left\{g_L^2\left(\frac{3}{2}\delta^{sa}\delta^{tb}Y_e^{pr}\text{Tr}\left[Y_e^\dagger Y_e\right]+\frac{9}{2}Y_u^{*ab}Y_e^{pr}Y_u^{st}+\frac{9}{2}\delta^{sa}\delta^{tb}Y_e^{pr}\text{Tr}\left[Y_d^\dagger Y_d\right]-\frac{15}{2}\delta^{tb}Y_e^{pr}(Y_dY_d^\dagger)^{sa}-9\delta^{sa}\delta^{tb}Y_e^{pr}\text{Tr}\left[Y_u^\dagger Y_u\right]\right)\right.\\
& -\frac{143}{12}\delta^{sa}\delta^{tb}g_Y^2g_L^2Y_e^{pr}-32\delta^{sa}\delta^{tb}g_s^2g_L^2Y_e^{pr}\left.\right\}C_{uW}^{ab}-9g_L^2C_{uW}^{*ab}Y_e^{pr}Y_u^{st}Y_u^{ab}+\left\{g_s^2\left(\frac{32}{3}\delta^{tb}Y_e^{pr}(Y_dY_d^\dagger)^{sa}+16Y_u^{*ab}Y_e^{pr}Y_u^{st}-\frac{8}{3}\delta^{sa}Y_e^{pr}(Y_u^\dagger Y_u)^{bt}\right.\right.\\
& -\frac{16}{3}\delta^{tb}Y_e^{pr}(Y_uY_u^\dagger)^{sa}\left.\right)+\frac{124}{27}\delta^{sa}\delta^{tb}g_Y^2g_s^2Y_e^{pr}+12\delta^{sa}\delta^{tb}g_s^2g_L^2Y_e^{pr}-\frac{224}{9}\delta^{sa}\delta^{tb}g_s^4Y_e^{pr}\left\}C_{uG}^{ab}+16g_s^2C_{uG}^{*ab}Y_e^{pr}Y_u^{st}Y_u^{ab}+g_Y^2\left\{9\delta^{sa}Y_e^{pr}(Y_d^\dagger Y_u)^{bt}\right.\right.\\
& -Y_d^{*ab}Y_e^{pr}Y_u^{st}\left.\right\}C_{dB}^{ab}+g_Y^2C_{dB}^{*ab}\left\{26Y_d^{ab}Y_e^{pr}Y_u^{st}-\frac{17}{3}Y_d^{sb}Y_e^{pr}Y_u^{at}\right\}+g_L^2\left\{\frac{9}{2}Y_d^{*ab}Y_e^{pr}Y_u^{st}-\frac{3}{2}\delta^{sa}Y_e^{pr}(Y_d^\dagger Y_u)^{bt}\right\}C_{dW}^{ab}+g_L^2C_{dW}^{*ab}\left\{\frac{3}{2}Y_d^{sb}Y_e^{pr}Y_u^{at}\right.\\
& -9Y_d^{ab}Y_e^{pr}Y_u^{st}\left.\right\}+g_s^2\left\{8\delta^{sa}Y_e^{pr}(Y_d^\dagger Y_u)^{bt}+16Y_d^{*ab}Y_e^{pr}Y_u^{st}\right\}C_{dG}^{ab}+g_s^2C_{dG}^{*ab}\left\{16Y_d^{ab}Y_e^{pr}Y_u^{st}-\frac{16}{3}Y_d^{sb}Y_e^{pr}Y_u^{at}\right\}+\left\{g_Y^2\left(\frac{4}{9}\delta^{ab}Y_e^{pr}Y_u^{st}\right.\right.\\
& +\frac{473}{108}\delta^{pa}Y_e^{br}Y_u^{st}\left.\right)+\frac{4}{3}Y_e^{pr}Y_u^{st}(Y_eY_e^\dagger)^{ba}+\frac{7}{2}\delta^{pa}Y_e^{br}(Y_dY_d^\dagger Y_u)^{st}-\frac{3}{4}\delta^{pa}g_L^2Y_e^{br}Y_u^{st}-2Y_e^{br}Y_u^{st}(Y_eY_e^\dagger)^{pa}-\frac{5}{2}\delta^{pa}Y_e^{br}(Y_uY_u^\dagger Y_u)^{st}\\
& -6\delta^{pa}Y_u^{st}(Y_eY_e^\dagger Y_e)^{br}\left.\right\}C_{H\ell}^{(\parallel)ab}+\left\{g_L^2\left(\frac{5}{3}\delta^{pa}Y_e^{br}Y_u^{st}-\frac{2}{3}\delta^{ab}Y_e^{pr}Y_u^{st}\right)+g_Y^2\left(\frac{2}{9}\delta^{ab}Y_e^{pr}Y_u^{st}+\frac{233}{54}\delta^{pa}Y_e^{br}Y_u^{st}\right)+\frac{8}{3}Y_e^{pr}Y_u^{st}(Y_eY_e^\dagger)^{ba}-Y_e^{br}Y_u^{st}(Y_eY_e^\dagger)^{pa}\right.\\
& \left.-3\delta^{pa}Y_u^{st}(Y_eY_e^\dagger Y_e)^{br}-\frac{7}{2}\delta^{pa}Y_e^{br}(Y_dY_d^\dagger Y_u)^{st}-\frac{7}{2}\delta^{pa}Y_e^{br}(Y_uY_u^\dagger Y_u)^{st}\right\}C_{H\ell}^{(\times)ab}+\left\{g_Y^2\left(\frac{4}{9}\delta^{ab}Y_e^{pr}Y_u^{st}+\frac{161}{108}\delta^{rb}Y_e^{pa}Y_u^{st}\right)+Y_e^{pa}Y_u^{st}(Y_e^\dagger Y_e)^{br}\right.
\end{aligned}$$

$$\begin{aligned}
& + \frac{3}{2} \delta^{rb} Y_e^{pa} (Y_d Y_d^\dagger Y_u)^{st} + 3 \delta^{rb} Y_u^{st} (Y_e Y_e^\dagger Y_e)^{pa} + \frac{7}{2} \delta^{rb} Y_e^{pa} (Y_u Y_u^\dagger Y_u)^{st} - \frac{3}{4} \delta^{rb} g_L^2 Y_e^{pa} Y_u^{st} - \frac{4}{3} Y_e^{pr} Y_u^{st} (Y_e^\dagger Y_e)^{ba} \Big\} C_{He}^{ab} + \left\{ \frac{3}{4} \delta^{sa} g_L^2 Y_e^{pr} Y_u^{bt} \right. \\
& + 2 Y_e^{pr} Y_u^{bt} (Y_u Y_u^\dagger)^{sa} + \frac{5}{2} \delta^{sa} Y_u^{bt} (Y_e Y_e^\dagger Y_e)^{pr} + 4 Y_e^{pr} Y_u^{st} (Y_d Y_d^\dagger)^{ba} + \frac{16}{3} \delta^{sa} g_s^2 Y_e^{pr} Y_u^{bt} + 6 \delta^{sa} Y_e^{pr} (Y_u Y_u^\dagger Y_u)^{bt} - g_Y^2 \left( \frac{4}{9} \delta^{ab} Y_e^{pr} Y_u^{st} + \frac{301}{108} \delta^{sa} Y_e^{pr} Y_u^{bt} \right) \\
& - Y_e^{pr} Y_u^{bt} (Y_d Y_d^\dagger)^{sa} - \delta^{sa} Y_e^{pr} (Y_d Y_d^\dagger Y_u)^{bt} - 4 Y_e^{pr} Y_u^{st} (Y_u Y_u^\dagger)^{ba} \Big\} C_{Hq}^{(II)ab} + \left\{ g_L^2 \left( \frac{29}{12} \delta^{sa} Y_e^{pr} Y_u^{bt} - 2 \delta^{ab} Y_e^{pr} Y_u^{st} \right) + g_Y^2 \left( \frac{61}{108} \delta^{sa} Y_e^{pr} Y_u^{bt} - \frac{2}{9} \delta^{ab} Y_e^{pr} Y_u^{st} \right) \right. \\
& + Y_e^{pr} Y_u^{bt} (Y_u Y_u^\dagger)^{sa} + 3 \delta^{sa} Y_e^{pr} (Y_u Y_u^\dagger Y_u)^{bt} + 4 Y_e^{pr} Y_u^{st} (Y_u Y_u^\dagger)^{ba} + 8 Y_e^{pr} Y_u^{st} (Y_d Y_d^\dagger)^{ba} - \delta^{sa} Y_u^{bt} (Y_e Y_e^\dagger Y_e)^{pr} - 2 Y_e^{pr} Y_u^{bt} (Y_d Y_d^\dagger)^{sa} - 2 \delta^{sa} Y_e^{pr} (Y_d Y_d^\dagger Y_u)^{bt} \\
& - \frac{16}{3} \delta^{sa} g_s^2 Y_e^{pr} Y_u^{bt} \Big\} C_{Hq}^{(\times)ab} + \left\{ \frac{3}{4} \delta^{tb} g_L^2 Y_e^{pr} Y_u^{sa} + g_Y^2 \left( \frac{347}{108} \delta^{tb} Y_e^{pr} Y_u^{sa} - \frac{8}{9} \delta^{ab} Y_e^{pr} Y_u^{st} \right) + 2 \delta^{tb} Y_e^{pr} (Y_d Y_d^\dagger Y_u)^{sa} + 4 Y_e^{pr} Y_u^{st} (Y_u^\dagger Y_u)^{ba} - Y_e^{pr} Y_u^{sa} (Y_u^\dagger Y_u)^{bt} \right. \\
& - 3 \delta^{tb} Y_e^{pr} (Y_u Y_u^\dagger Y_u)^{sa} - \frac{7}{2} \delta^{tb} Y_u^{sa} (Y_e Y_e^\dagger Y_e)^{pr} - \frac{16}{3} \delta^{tb} g_s^2 Y_e^{pr} Y_u^{sa} \Big\} C_{Hu}^{ab} + \left\{ \frac{4}{9} \delta^{ab} g_Y^2 Y_e^{pr} Y_u^{st} - 4 Y_e^{pr} Y_u^{st} (Y_d^\dagger Y_d)^{ba} \right\} C_{Hd}^{ab} - 4 C_{Hud}^{ab} Y_e^{pr} Y_u^{st} (Y_d^\dagger Y_u)^{ba} \\
& + C_{Hud}^{*ab} \left\{ Y_d^{sb} Y_e^{pr} (Y_u^\dagger Y_u)^{at} + \delta^{ta} Y_e^{pr} (Y_d Y_d^\dagger Y_d)^{sb} + \frac{49}{36} \delta^{ta} g_Y^2 Y_d^{sb} Y_e^{pr} + 2 \delta^{ta} Y_d^{sb} (Y_e Y_e^\dagger Y_e)^{pr} + \frac{16}{3} \delta^{ta} g_s^2 Y_d^{sb} Y_e^{pr} - \frac{3}{4} \delta^{ta} g_L^2 Y_d^{sb} Y_e^{pr} \right. \\
& - 4 Y_e^{pr} Y_u^{st} (Y_u^\dagger Y_d)^{ab} \Big\} + \left\{ g_Y^2 \left( 7 \delta^{pa} \delta^{rd} Y_e^{bc} Y_u^{st} - \frac{16}{27} \delta^{rd} \delta^{ab} Y_e^{pc} Y_u^{st} - \frac{100}{27} \delta^{pa} \delta^{cd} Y_e^{br} Y_u^{st} \right) + 2 Y_e^{*ad} Y_e^{pr} Y_e^{bc} Y_u^{st} + 3 \delta^{pa} \delta^{rd} g_L^2 Y_e^{bc} Y_u^{st} \right. \\
& - 2 \delta^{pa} \delta^{rd} Y_e^{bc} Y_u^{st} \text{Tr} \left[ Y_e^\dagger Y_e \right] - 4 \delta^{pa} Y_e^{br} Y_u^{st} (Y_e^\dagger Y_e)^{dc} - 4 \delta^{rd} Y_e^{pc} Y_u^{st} (Y_e Y_e^\dagger)^{ba} - 12 \delta^{pa} \delta^{rd} Y_u^{st} (Y_e Y_e^\dagger Y_e)^{bc} \Big\} C_{\ell e}^{abcd} + \left\{ \frac{1}{2} \delta^{pa} \delta^{td} Y_u^{sc} (Y_e Y_e^\dagger Y_e)^{br} \right. \\
& + \text{T}_2 \delta^{pa} \delta^{td} Y_e^{br} Y_u^{sc} + g_Y^2 \left( \frac{55}{18} \delta^{pa} \delta^{td} Y_e^{br} Y_u^{sc} + \frac{200}{27} \delta^{pa} \delta^{cd} Y_e^{br} Y_u^{st} - \frac{16}{27} \delta^{td} \delta^{ab} Y_e^{pr} Y_u^{sc} \right) + \delta^{pa} \delta^{td} Y_e^{br} (Y_u Y_u^\dagger Y_u)^{sc} + \frac{3}{2} \delta^{pa} \delta^{td} g_L^2 Y_e^{br} Y_u^{sc} \\
& - \frac{1}{2} \delta^{pa} Y_e^{br} Y_u^{sc} (Y_u^\dagger Y_u)^{dt} - \delta^{td} Y_e^{br} Y_u^{sc} (Y_e Y_e^\dagger)^{pa} - \delta^{pa} \delta^{td} Y_e^{br} (Y_d Y_d^\dagger Y_u)^{sc} - \frac{16}{3} \delta^{pa} \delta^{td} g_s^2 Y_e^{br} Y_u^{sc} \Big\} C_{\ell u}^{abcd} + \left\{ \frac{7}{2} \delta^{pa} Y_d^{sc} Y_e^{br} (Y_d^\dagger Y_u)^{dt} - \frac{100}{27} \delta^{pa} \delta^{cd} g_Y^2 Y_e^{br} Y_u^{st} \right. \\
& - 9 \delta^{pa} Y_e^{br} Y_u^{st} (Y_d^\dagger Y_d)^{dc} \Big\} C_{\ell d}^{abcd} + \left\{ \frac{1}{2} \delta^{rd} \delta^{sa} Y_e^{pc} (Y_u Y_u^\dagger Y_u)^{bt} + \text{T}_2 \delta^{rd} \delta^{sa} Y_e^{pc} Y_u^{bt} + g_Y^2 \left( \frac{16}{27} \delta^{rd} \delta^{ab} Y_e^{pc} Y_u^{st} + \frac{37}{18} \delta^{rd} \delta^{sa} Y_e^{pc} Y_u^{bt} + \frac{68}{27} \delta^{sa} \delta^{cd} Y_e^{pr} Y_u^{bt} \right) \right. \\
& + \delta^{rd} \delta^{sa} Y_u^{bt} (Y_e Y_e^\dagger Y_e)^{pc} + \frac{3}{2} \delta^{rd} \delta^{sa} g_L^2 Y_e^{pc} Y_u^{bt} + 4 \delta^{rd} Y_e^{pc} Y_u^{bt} (Y_d Y_d^\dagger)^{sa} - \frac{1}{2} \delta^{sa} Y_e^{pc} Y_u^{bt} (Y_e^\dagger Y_e)^{dr} - \frac{1}{2} \delta^{rd} \delta^{sa} Y_e^{pc} (Y_d Y_d^\dagger Y_u)^{bt} - \delta^{rd} Y_e^{pc} Y_u^{bt} (Y_u Y_u^\dagger)^{sa} \\
& - \frac{16}{3} \delta^{rd} \delta^{sa} g_s^2 Y_e^{pc} Y_u^{bt} - 9 \delta^{rd} Y_e^{pc} Y_u^{st} (Y_d Y_d^\dagger)^{ba} \Big\} C_{qe}^{abcd} + \left\{ g_Y^2 \left( \frac{16}{27} \delta^{td} \delta^{ab} Y_e^{pr} Y_u^{sc} + \frac{35}{9} \delta^{sa} \delta^{td} Y_e^{pr} Y_u^{bc} - \frac{136}{27} \delta^{sa} \delta^{cd} Y_e^{pr} Y_u^{bt} \right) + 3 \delta^{sa} \delta^{td} g_L^2 Y_e^{pr} Y_u^{bc} \right. \\
& + \frac{7}{2} \delta^{sa} \delta^{td} Y_e^{pr} (Y_d Y_d^\dagger Y_u)^{bc} + 6 Y_u^{*ad} Y_e^{pr} Y_u^{st} Y_u^{bc} + \frac{32}{3} \delta^{sa} \delta^{td} g_s^2 Y_e^{pr} Y_u^{bc} - 6 \delta^{sa} \delta^{td} Y_e^{pr} Y_u^{bc} \text{Tr} \left[ Y_u^\dagger Y_u \right] - 12 \delta^{sa} Y_e^{pr} Y_u^{bt} (Y_u^\dagger Y_u)^{dc} - 12 \delta^{td} Y_e^{pr} Y_u^{sc} (Y_u Y_u^\dagger)^{ba}
\end{aligned}$$

$$\begin{aligned}
& -12\delta^{sa}\delta^{td}Y_e^{pr}(Y_uY_u^\dagger Y_u)^{bc} \Big\} C_{qu}^{(\parallel)abcd} + \left\{ g_s^2 \left( 128\delta^{sa}\delta^{td}Y_e^{pr}Y_u^{bc} - \frac{112}{27}\delta^{sa}\delta^{cd}Y_e^{pr}Y_u^{bt} - \frac{224}{27}\delta^{td}\delta^{ab}Y_e^{pr}Y_u^{sc} \right) + g_Y^2 \left( \frac{16}{81}\delta^{td}\delta^{ab}Y_e^{pr}Y_u^{sc} + \frac{35}{3}\delta^{sa}\delta^{td}Y_e^{pr}Y_u^{bc} \right. \right. \\
& - \frac{136}{81}\delta^{sa}\delta^{cd}Y_e^{pr}Y_u^{bt} \Big) + 9\delta^{sa}\delta^{td}g_L^2Y_e^{pr}Y_u^{bc} + \frac{21}{2}\delta^{sa}\delta^{td}Y_e^{pr}(Y_dY_d^\dagger Y_u)^{bc} + 18Y_u^{*ad}Y_e^{pr}Y_u^{st}Y_u^{bc} - 4\delta^{sa}Y_e^{pr}Y_u^{bt}(Y_u^\dagger Y_u)^{dc} - 4\delta^{td}Y_e^{pr}Y_u^{sc}(Y_uY_u^\dagger)^{ba} \\
& - 18\delta^{sa}\delta^{td}Y_e^{pr}Y_u^{bc} \text{Tr}[Y_u^\dagger Y_u] - 36\delta^{sa}\delta^{td}Y_e^{pr}(Y_uY_u^\dagger Y_u)^{bc} \Big\} C_{qu}^{(\times)abcd} + \left\{ \frac{68}{27}\delta^{sa}\delta^{cd}g_Y^2Y_e^{pr}Y_u^{bt} + 12Y_d^{*ad}Y_d^{bc}Y_e^{pr}Y_u^{st} - \frac{1}{2}Y_d^{*ad}Y_d^{sc}Y_e^{pr}Y_u^{bt} - \frac{1}{2}Y_d^{*ad}Y_d^{sc}Y_e^{pr}Y_u^{bt} \right\} C_{qd}^{(\parallel)abcd} \\
& + \left\{ \frac{68}{81}\delta^{sa}\delta^{cd}g_Y^2Y_e^{pr}Y_u^{bt} + 36Y_d^{*ad}Y_d^{bc}Y_e^{pr}Y_u^{st} - \frac{3}{2}Y_d^{*ad}Y_d^{sc}Y_e^{pr}Y_u^{bt} - \frac{112}{27}\delta^{sa}\delta^{cd}g_s^2Y_e^{pr}Y_u^{bt} \right\} C_{qd}^{(\times)abcd} - \left\{ \frac{88}{27}\delta^{rb}\delta^{ad}g_Y^2Y_e^{pc}Y_u^{st} \right. \\
& + 4\delta^{rb}Y_e^{pa}Y_u^{st}(Y_e^\dagger Y_e)^{dc} \Big\} C_{ee}^{abcd} + \left\{ g_Y^2 \left( \frac{64}{27}\delta^{tb}\delta^{cd}Y_e^{pr}Y_u^{sa} - \frac{176}{81}\delta^{tb}\delta^{ad}Y_e^{pr}Y_u^{sc} \right) - \frac{32}{27}\delta^{tb}\delta^{ad}g_s^2Y_e^{pr}Y_u^{sc} - 12\delta^{tb}Y_e^{pr}Y_u^{sa}(Y_u^\dagger Y_u)^{dc} \right\} C_{uu}^{abcd} \\
& + \left\{ g_Y^2 \left( \frac{32}{27}\delta^{rb}\delta^{cd}Y_e^{pa}Y_u^{st} + \frac{242}{9}\delta^{rb}\delta^{td}Y_e^{pa}Y_u^{sc} - \frac{16}{27}\delta^{td}\delta^{ab}Y_e^{pr}Y_u^{sc} \right) + 9\delta^{rb}\delta^{td}g_L^2Y_e^{pa}Y_u^{sc} - \delta^{rb}\delta^{td}Y_e^{pa}(Y_dY_d^\dagger Y_u)^{sc} - \frac{5}{2}\delta^{td}Y_e^{pa}Y_u^{sc}(Y_e^\dagger Y_e)^{br} \right. \\
& - \frac{5}{2}\delta^{rb}Y_e^{pa}Y_u^{sc}(Y_u^\dagger Y_u)^{dt} - 3T_2\delta^{rb}\delta^{td}Y_e^{pa}Y_u^{sc} - 3\delta^{rb}\delta^{td}Y_u^{sc}(Y_eY_e^\dagger Y_e)^{pa} - 3\delta^{rb}\delta^{td}Y_e^{pa}(Y_uY_u^\dagger Y_u)^{sc} - \frac{16}{3}\delta^{rb}\delta^{td}g_s^2Y_e^{pa}Y_u^{sc} \Big\} C_{eu}^{abcd} \\
& + \left\{ \frac{3}{2}\delta^{rb}Y_d^{sc}Y_e^{pa}(Y_d^\dagger Y_u)^{dt} - \frac{16}{27}\delta^{rb}\delta^{cd}g_Y^2Y_e^{pa}Y_u^{st} - 9\delta^{rb}Y_e^{pa}Y_u^{st}(Y_d^\dagger Y_d)^{dc} \right\} C_{ed}^{abcd} + \left\{ \frac{3}{2}\delta^{tb}Y_d^{sc}Y_e^{pr}(Y_d^\dagger Y_u)^{da} - \frac{16}{27}\delta^{tb}\delta^{cd}g_Y^2Y_e^{pr}Y_u^{sa} \right\} C_{ud}^{(\parallel)abcd} \\
& + \left\{ \frac{9}{2}\delta^{tb}Y_d^{sc}Y_e^{pr}(Y_d^\dagger Y_u)^{da} - \frac{16}{81}\delta^{tb}\delta^{cd}g_Y^2Y_e^{pr}Y_u^{sa} - \frac{112}{27}\delta^{tb}\delta^{cd}g_s^2Y_e^{pr}Y_u^{sa} \right\} C_{ud}^{(\times)abcd} + \left\{ \frac{3}{4}\delta^{rb}Y_d^{sc}Y_u^{dt}(Y_eY_e^\dagger)^{pa} + g_L^2 \left( \frac{9}{4}\delta^{pa}\delta^{rb}Y_d^{dc}Y_u^{st} - \frac{3}{4}\delta^{pa}\delta^{rb}Y_d^{sc}Y_u^{dt} \right) \right. \\
& + g_s^2 \left( \frac{64}{3}\delta^{pa}\delta^{rb}Y_d^{sc}Y_u^{dt} - 40\delta^{pa}\delta^{rb}Y_d^{dc}Y_u^{st} \right) + 3\delta^{pa}\delta^{rb}Y_d^{dc}Y_u^{st} \text{Tr}[Y_e^\dagger Y_e] + \frac{27}{2}\delta^{pa}\delta^{rb}Y_u^{st}(Y_dY_d^\dagger Y_d)^{dc} - \frac{1}{4}\delta^{pa}Y_d^{sc}Y_u^{dt}(Y_e^\dagger Y_e)^{br} - g_Y^2 \left( \frac{5}{36}\delta^{pa}\delta^{rb}Y_d^{sc}Y_u^{dt} \right. \\
& + \frac{7}{12}\delta^{pa}\delta^{rb}Y_d^{dc}Y_u^{st} \Big) - \delta^{pa}\delta^{rb}Y_d^{sc}(Y_dY_d^\dagger Y_u)^{dt} - \delta^{pa}\delta^{rb}Y_d^{sc}(Y_uY_u^\dagger Y_u)^{dt} - \frac{3}{2}\delta^{pa}\delta^{rb}Y_u^{st}(Y_uY_u^\dagger Y_d)^{dc} - 2T_2\delta^{pa}\delta^{rb}Y_d^{sc}Y_u^{dt} \\
& - 2\delta^{pa}\delta^{rb}Y_u^{dt}(Y_dY_d^\dagger Y_d)^{sc} \Big\} C_{ledq}^{abcd} + C_{ledq}^{*abcd} \left\{ \frac{1}{2}\delta^{sd}Y_e^{pb}Y_e^{ar}(Y_d^\dagger Y_u)^{ct} + \frac{1}{2}\delta^{sd}Y_e^{pr}Y_e^{ab}(Y_d^\dagger Y_u)^{ct} + 3Y_d^{*dc}Y_e^{pr}Y_e^{ab}Y_u^{st} \right\} + \left\{ \frac{1}{4}\delta^{sa}Y_u^{*cb}Y_e^{pr}(Y_d^\dagger Y_u)^{dt} \right. \\
& + \frac{1}{4}\delta^{tb}Y_d^{*ad}Y_e^{pr}(Y_dY_d^\dagger)^{sc} + g_Y^2 \left( \frac{1}{24}\delta^{sc}\delta^{tb}Y_d^{*ad}Y_e^{pr} - \frac{17}{6}\delta^{sa}\delta^{tb}Y_d^{*cd}Y_e^{pr} \right) + g_L^2 \left( \frac{9}{8}\delta^{sc}\delta^{tb}Y_d^{*ad}Y_e^{pr} - \frac{9}{2}\delta^{sa}\delta^{tb}Y_d^{*cd}Y_e^{pr} \right) + \left( \frac{3}{2}\delta^{sc}\delta^{tb}Y_d^{*ad}Y_e^{pr} \right. \\
& + 9\delta^{sa}\delta^{tb}Y_d^{*cd}Y_e^{pr} \Big) \text{Tr}[Y_u^\dagger Y_u] + \frac{3}{2}\delta^{sc}Y_u^{*ab}Y_e^{pr}(Y_d^\dagger Y_u)^{dt} + \frac{3}{2}\delta^{tb}Y_d^{*cd}Y_e^{pr}(Y_dY_d^\dagger)^{sa} + \frac{9}{4}\delta^{sc}\delta^{tb}Y_e^{pr}(Y_d^\dagger Y_dY_d^\dagger)^{ad} + \frac{27}{2}\delta^{sa}\delta^{tb}Y_e^{pr}(Y_d^\dagger Y_dY_d^\dagger)^{cd} \\
& - g_s^2 \left( 12\delta^{sc}\delta^{tb}Y_d^{*ad}Y_e^{pr} + 40\delta^{sa}\delta^{tb}Y_d^{*cd}Y_e^{pr} \right) - \frac{5}{4}\delta^{sc}\delta^{tb}Y_e^{pr}(Y_u^\dagger Y_uY_d^\dagger)^{ad} - \frac{9}{2}\delta^{sa}\delta^{tb}Y_e^{pr}(Y_u^\dagger Y_uY_d^\dagger)^{cd} \Big\} C_{quqd}^{(\parallel)abcd} + \left( C_{quqd}^{(\parallel)*} \right)^{abcd} \left\{ \frac{3}{2}Y_d^{ad}Y_e^{pr}Y_u^{st}Y_u^{cb} \right.
\end{aligned}$$

$$\begin{aligned}
& + 9Y_d^{cd}Y_e^{pr}Y_u^{st}Y_u^{ab} - Y_d^{sd}Y_e^{pr}Y_u^{at}Y_u^{cb} - 3Y_d^{sd}Y_e^{pr}Y_u^{ab}Y_u^{ct} \Big\} + \left\{ \frac{1}{2}\delta^{sc}Y_u^{*ab}Y_e^{pr}(Y_d^\dagger Y_u)^{dt} + \frac{1}{2}\delta^{tb}Y_d^{*cd}Y_e^{pr}(Y_d Y_d^\dagger)^{sa} + \frac{3}{4}\delta^{sa}Y_u^{*cb}Y_e^{pr}(Y_d^\dagger Y_u)^{dt} \right. \\
& + \frac{3}{4}\delta^{tb}Y_d^{*ad}Y_e^{pr}(Y_d Y_d^\dagger)^{sc} + g_Y^2 \left( \frac{1}{8}\delta^{sc}\delta^{tb}Y_d^{*ad}Y_e^{pr} - \frac{17}{18}\delta^{sa}\delta^{tb}Y_d^{*cd}Y_e^{pr} \right) + g_L^2 \left( \frac{27}{8}\delta^{sc}\delta^{tb}Y_d^{*ad}Y_e^{pr} - \frac{3}{2}\delta^{sa}\delta^{tb}Y_d^{*cd}Y_e^{pr} \right) + \left( 3\delta^{sa}\delta^{tb}Y_d^{*cd}Y_e^{pr} \right. \\
& + \frac{9}{2}\delta^{sc}\delta^{tb}Y_d^{*ad}Y_e^{pr} \Big) \text{Tr}[Y_u^\dagger Y_u] + \frac{9}{2}\delta^{sa}\delta^{tb}Y_e^{pr}(Y_d^\dagger Y_d Y_d^\dagger)^{cd} + \frac{27}{4}\delta^{sc}\delta^{tb}Y_e^{pr}(Y_d^\dagger Y_d Y_d^\dagger)^{ad} - g_s^2 \left( \frac{40}{3}\delta^{sa}\delta^{tb}Y_d^{*cd}Y_e^{pr} + 48\delta^{sc}\delta^{tb}Y_d^{*ad}Y_e^{pr} \right) \\
& \left. - \frac{3}{2}\delta^{sa}\delta^{tb}Y_e^{pr}(Y_u^\dagger Y_u Y_d^\dagger)^{cd} - \frac{15}{4}\delta^{sc}\delta^{tb}Y_e^{pr}(Y_u^\dagger Y_u Y_d^\dagger)^{ad} \right\} C_{quqd}^{(\times)abcd} + \left( C_{quqd}^{(\times)*} \right)^{abcd} \left\{ 3Y_d^{cd}Y_e^{pr}Y_u^{st}Y_u^{ab} + \frac{9}{2}Y_d^{ad}Y_e^{pr}Y_u^{st}Y_u^{cb} - Y_d^{sd}Y_e^{pr}Y_u^{ab}Y_u^{ct} - 3Y_d^{sd}Y_e^{pr}Y_u^{at}Y_u^{cb} \right\} \\
& + \left\{ g_L^2 \left( \frac{3}{2}\delta^{sc}\delta^{td}Y_e^{*ab}Y_e^{pr} + \frac{33}{16}\delta^{pa}\delta^{rb}\delta^{td}(Y_d Y_d^\dagger)^{sc} + \frac{33}{16}\delta^{rb}\delta^{sc}\delta^{td}(Y_e Y_e^\dagger)^{pa} + \frac{33}{16}\delta^{pa}\delta^{rb}\delta^{td}(Y_u Y_u^\dagger)^{sc} + \frac{9}{2}\delta^{pa}\delta^{rb}Y_u^{*cd}Y_u^{st} + \frac{51}{8}\delta^{pa}\delta^{sc}\delta^{td}(Y_e^\dagger Y_e)^{br} \right. \right. \\
& + \frac{51}{8}\delta^{pa}\delta^{rb}\delta^{sc}(Y_u^\dagger Y_u)^{dt} \Big) + g_s^2 \left( \frac{16}{3}\delta^{pa}\delta^{rb}\delta^{td}(Y_d Y_d^\dagger)^{sc} + \frac{16}{3}\delta^{pa}\delta^{rb}\delta^{td}(Y_u Y_u^\dagger)^{sc} + \frac{32}{3}\delta^{pa}\delta^{rb}\delta^{sc}(Y_u^\dagger Y_u)^{dt} + 40\delta^{pa}\delta^{rb}Y_u^{*cd}Y_u^{st} \right) \\
& + g_Y^2 \left( \frac{145}{72}\delta^{pa}\delta^{rb}\delta^{sc}(Y_u^\dagger Y_u)^{dt} + \frac{79}{24}\delta^{pa}\delta^{sc}\delta^{td}(Y_e^\dagger Y_e)^{br} + \frac{811}{144}\delta^{pa}\delta^{rb}\delta^{td}(Y_u Y_u^\dagger)^{sc} + \frac{13}{2}\delta^{sc}\delta^{td}Y_e^{*ab}Y_e^{pr} + \frac{47}{6}\delta^{pa}\delta^{rb}Y_u^{*cd}Y_u^{st} \right. \\
& + \frac{389}{48}\delta^{rb}\delta^{sc}\delta^{td}(Y_e Y_e^\dagger)^{pa} - \frac{185}{144}\delta^{pa}\delta^{rb}\delta^{td}(Y_d Y_d^\dagger)^{sc} \Big) + \frac{3}{2}\delta^{pa}\delta^{rb}Y_u^{st}(Y_d^\dagger Y_d Y_u^\dagger)^{cd} + 2\delta^{sc}\delta^{td}(Y_e^\dagger Y_e)^{br}(Y_e Y_e^\dagger)^{pa} + 2\delta^{pa}\delta^{rb}(Y_u^\dagger Y_u)^{dt}(Y_u Y_u^\dagger)^{sc} \\
& + \frac{137}{24}\delta^{pa}\delta^{rb}\delta^{sc}\delta^{td}g_Y^2 g_L^2 + \frac{79}{9}\delta^{pa}\delta^{rb}\delta^{sc}\delta^{td}g_Y^2 g_s^2 + 13\delta^{pa}\delta^{rb}\delta^{sc}\delta^{td}g_s^2 g_L^2 + \frac{7255}{432}\delta^{pa}\delta^{rb}\delta^{sc}\delta^{td}g_Y^4 - \frac{1}{4}\delta^{pa}\delta^{sc}\delta^{td}(Y_e^\dagger Y_e Y_e^\dagger Y_e)^{br} \\
& - \frac{1}{4}\delta^{pa}\delta^{rb}\delta^{sc}(Y_u^\dagger Y_d Y_d^\dagger Y_u)^{dt} - \frac{1}{4}\delta^{pa}\delta^{rb}\delta^{sc}(Y_u^\dagger Y_u Y_u^\dagger Y_u)^{dt} - \frac{1}{4}\delta^{pa}\delta^{rb}\delta^{td}(Y_d Y_d^\dagger Y_d Y_d^\dagger)^{sc} - \frac{1}{4}\delta^{rb}\delta^{sc}\delta^{td}(Y_e Y_e^\dagger Y_e Y_e^\dagger)^{pa} - \frac{1}{4}\delta^{pa}\delta^{rb}\delta^{td}(Y_u Y_u^\dagger Y_u Y_u^\dagger)^{sc} \\
& - \frac{1}{2}\delta^{td}Y_e^{*ab}Y_e^{pr}(Y_d Y_d^\dagger)^{sc} - \frac{29}{48}\delta^{pa}\delta^{rb}\delta^{sc}\delta^{td}g_L^4 - \frac{3}{4}\text{T}_2\delta^{pa}\delta^{rb}\delta^{td}(Y_d Y_d^\dagger)^{sc} - \frac{3}{4}\text{T}_2\delta^{rb}\delta^{sc}\delta^{td}(Y_e Y_e^\dagger)^{pa} - \frac{3}{4}\text{T}_2\delta^{pa}\delta^{rb}\delta^{td}(Y_u Y_u^\dagger)^{sc} \\
& - \frac{5}{4}\delta^{rb}\delta^{sc}(Y_u^\dagger Y_u)^{dt}(Y_e Y_e^\dagger)^{pa} - \frac{5}{4}\delta^{pa}\delta^{td}(Y_e^\dagger Y_e)^{br}(Y_u Y_u^\dagger)^{sc} - \frac{3}{2}\text{T}_2\delta^{pa}\delta^{sc}\delta^{td}(Y_e^\dagger Y_e)^{br} - \frac{3}{2}\text{T}_2\delta^{pa}\delta^{rb}\delta^{sc}(Y_u^\dagger Y_u)^{dt} - 2\delta^{pa}\delta^{td}(Y_e^\dagger Y_e)^{br}(Y_d Y_d^\dagger)^{sc} \\
& - 2\delta^{pa}\delta^{rb}(Y_u^\dagger Y_u)^{dt}(Y_d Y_d^\dagger)^{sc} - 3\delta^{pa}\delta^{rb}Y_u^{*cd}Y_u^{st} \text{Tr}[Y_e^\dagger Y_e] - 3\delta^{sc}\delta^{td}Y_e^{*ab}Y_e^{pr} \text{Tr}[Y_u^\dagger Y_u] - \frac{7}{2}\delta^{pa}\delta^{sc}(Y_e^\dagger Y_e)^{br}(Y_u^\dagger Y_u)^{dt} - \frac{7}{2}\delta^{rb}\delta^{td}(Y_e Y_e^\dagger)^{pa}(Y_u Y_u^\dagger)^{sc} \\
& - \frac{9}{2}\delta^{sc}\delta^{td}Y_e^{pr}(Y_e^\dagger Y_e Y_e^\dagger)^{ab} - \frac{27}{2}\delta^{pa}\delta^{rb}Y_u^{st}(Y_u^\dagger Y_u Y_u^\dagger)^{cd} - 108\delta^{pa}\delta^{rb}\delta^{sc}\delta^{td}g_s^4 \Big\} C_{lequ}^{abcd} - C_{lequ}^{*abcd} \left\{ \frac{3}{2}Y_e^{pb}Y_e^{ar}Y_u^{sd}Y_u^{ct} + 6Y_e^{pr}Y_e^{ab}Y_u^{st}Y_u^{cd} \right\} \\
& + \left\{ \frac{1}{4}\delta^{tb}Y_e^{*ad}Y_e^{pr}(Y_d Y_d^\dagger)^{sc} + \frac{1}{2}\delta^{rd}\delta^{sc}(Y_u^\dagger Y_u)^{bt}(Y_e Y_e^\dagger)^{pa} + \frac{1}{2}\delta^{pa}\delta^{tb}(Y_e^\dagger Y_e)^{dr}(Y_u Y_u^\dagger)^{sc} + g_L^2 \left( \frac{9}{8}\delta^{sc}\delta^{tb}Y_e^{*ad}Y_e^{pr} + \frac{27}{8}\delta^{pa}\delta^{rd}Y_u^{*cb}Y_u^{st} \right) \right. \\
& + \delta^{pa}\delta^{rd}(Y_u^\dagger Y_u)^{bt}(Y_d Y_d^\dagger)^{sc} + g_Y^2 \left( \frac{2}{9}\delta^{pa}\delta^{rd}\delta^{tb}(Y_d Y_d^\dagger)^{sc} + \frac{2}{3}\delta^{pa}\delta^{sc}\delta^{tb}(Y_e^\dagger Y_e)^{dr} + \frac{10}{9}\delta^{pa}\delta^{rd}\delta^{sc}(Y_u^\dagger Y_u)^{bt} - \frac{4}{9}\delta^{pa}\delta^{rd}\delta^{tb}(Y_u Y_u^\dagger)^{sc} - \frac{181}{72}\delta^{sc}\delta^{tb}Y_e^{*ad}Y_e^{pr} \right. \\
& \left. - \frac{10}{3}\delta^{rd}\delta^{sc}\delta^{tb}(Y_e Y_e^\dagger)^{pa} - \frac{209}{24}\delta^{pa}\delta^{rd}Y_u^{*cb}Y_u^{st} \right) + \frac{3}{2}\delta^{pa}\delta^{rd}Y_u^{*cb}Y_u^{st} \text{Tr}[Y_e^\dagger Y_e] + \frac{3}{2}\delta^{sc}\delta^{tb}Y_e^{*ad}Y_e^{pr} \text{Tr}[Y_u^\dagger Y_u] + \frac{9}{4}\delta^{sc}\delta^{tb}Y_e^{pr}(Y_e^\dagger Y_e Y_e^\dagger)^{ad}
\end{aligned}$$

$$\begin{aligned}
& + \frac{27}{4} \delta^{pa} \delta^{rd} Y_u^{st} (Y_u^\dagger Y_u Y_u^\dagger)^{cb} + \frac{190}{9} \delta^{pa} \delta^{rd} \delta^{sc} \delta^{tb} g_Y^2 g_s^2 + \frac{632}{9} \delta^{pa} \delta^{rd} \delta^{sc} \delta^{tb} g_L^4 - \frac{155}{324} \delta^{pa} \delta^{rd} \delta^{sc} \delta^{tb} g_Y^4 - g_s^2 \left( \frac{14}{3} \delta^{sc} \delta^{tb} Y_e^{*ad} Y_e^{pr} \right. \\
& + \frac{16}{3} \delta^{pa} \delta^{rd} \delta^{tb} (Y_d Y_d^\dagger)^{sc} + \frac{16}{3} \delta^{pa} \delta^{rd} \delta^{tb} (Y_u Y_u^\dagger)^{sc} + \frac{32}{3} \delta^{pa} \delta^{rd} \delta^{sc} (Y_u^\dagger Y_u)^{bt} + 34 \delta^{pa} \delta^{rd} Y_u^{*cb} Y_u^{st} \Big) - \frac{3}{2} \delta^{pa} \delta^{sc} (Y_e^\dagger Y_e)^{dr} (Y_u^\dagger Y_u)^{bt} \\
& - \frac{3}{2} \delta^{rd} \delta^{tb} (Y_e Y_e^\dagger)^{pa} (Y_u Y_u^\dagger)^{sc} - 2 \delta^{sc} \delta^{tb} (Y_e^\dagger Y_e)^{dr} (Y_e Y_e^\dagger)^{pa} - 2 \delta^{rd} \delta^{tb} (Y_d Y_d^\dagger)^{sc} (Y_e Y_e^\dagger)^{pa} - 2 \delta^{pa} \delta^{rd} (Y_u^\dagger Y_u)^{bt} (Y_u Y_u^\dagger)^{sc} - \frac{9}{4} \delta^{pa} \delta^{rd} Y_u^{st} (Y_d^\dagger Y_d Y_u^\dagger)^{cb} \\
& - \frac{41}{3} \delta^{pa} \delta^{rd} \delta^{sc} \delta^{tb} g_Y^2 g_L^2 - 14 \delta^{pa} \delta^{rd} \delta^{sc} \delta^{tb} g_s^2 g_L^2 - \frac{199}{12} \delta^{pa} \delta^{rd} \delta^{sc} \delta^{tb} g_L^4 \Big\} C_{\ell u q e}^{abcd} + 3 C_{\ell u q e}^{*abcd} Y_e^{pr} Y_e^{ad} Y_u^{st} Y_u^{cb} + \left\{ -g_Y^2 \left( \frac{40}{27} \delta^{pa} \delta^{bc} Y_e^{dr} Y_u^{st} \right. \right. \\
& + \frac{200}{27} \delta^{pa} \delta^{cd} Y_e^{br} Y_u^{st} \Big) - \frac{4}{3} \delta^{pa} \delta^{bc} g_L^2 Y_e^{dr} Y_u^{st} - 4 \delta^{pa} Y_e^{br} Y_u^{st} (Y_e Y_e^\dagger)^{dc} \Big\} C_{\ell \ell}^{abcd} + \left\{ 3 \delta^{sa} Y_e^{pr} Y_u^{dt} (Y_d Y_d^\dagger)^{bc} - g_Y^2 \left( \frac{56}{81} \delta^{sa} \delta^{bc} Y_e^{pr} Y_u^{dt} + \frac{136}{27} \delta^{sa} \delta^{cd} Y_e^{pr} Y_u^{bt} \right) \right. \\
& - \frac{32}{27} \delta^{sa} \delta^{bc} g_s^2 Y_e^{pr} Y_u^{dt} - \frac{4}{3} \delta^{sa} \delta^{bc} g_L^2 Y_e^{pr} Y_u^{dt} - 12 \delta^{sa} Y_e^{pr} Y_u^{bt} (Y_u Y_u^\dagger)^{dc} \Big\} C_{qq}^{(\parallel)abcd} + \left\{ 8 \delta^{sa} \delta^{cd} g_L^2 Y_e^{pr} Y_u^{bt} - g_Y^2 \left( \frac{112}{81} \delta^{sa} \delta^{bc} Y_e^{pr} Y_u^{dt} + \frac{68}{27} \delta^{sa} \delta^{cd} Y_e^{pr} Y_u^{bt} \right) \right. \\
& - \frac{64}{27} \delta^{sa} \delta^{bc} g_s^2 Y_e^{pr} Y_u^{dt} - 3 \delta^{sa} Y_e^{pr} Y_u^{dt} (Y_d Y_d^\dagger)^{bc} - 24 \delta^{sa} Y_e^{pr} Y_u^{bt} (Y_u Y_u^\dagger)^{dc} \Big\} C_{qq}^{(\times)abcd} + \left\{ g_Y^2 \left( \frac{68}{27} \delta^{sc} \delta^{ab} Y_e^{pr} Y_u^{dt} + \frac{100}{27} \delta^{pa} \delta^{cd} Y_e^{br} Y_u^{st} + \frac{211}{18} \delta^{pa} \delta^{sc} Y_e^{br} Y_u^{dt} \right) \right. \\
& + 4 \delta^{pa} Y_e^{br} Y_u^{dt} (Y_d Y_d^\dagger)^{sc} + \frac{57}{2} \delta^{pa} \delta^{sc} g_L^2 Y_e^{br} Y_u^{dt} - \frac{3}{2} \delta^{pa} \delta^{sc} Y_u^{dt} (Y_e Y_e^\dagger Y_e)^{br} - \frac{3}{2} \delta^{pa} \delta^{sc} Y_e^{br} (Y_u Y_u^\dagger Y_u)^{dt} - \frac{5}{2} \delta^{pa} \delta^{sc} Y_e^{br} (Y_d Y_d^\dagger Y_u)^{dt} - 3 T_2 \delta^{pa} \delta^{sc} Y_e^{br} Y_u^{dt} \\
& - 5 \delta^{sc} Y_e^{br} Y_u^{dt} (Y_e Y_e^\dagger)^{pa} - 5 \delta^{pa} Y_e^{br} Y_u^{dt} (Y_u Y_u^\dagger)^{sc} - \frac{16}{3} \delta^{pa} \delta^{sc} g_s^2 Y_e^{br} Y_u^{dt} - 9 \delta^{pa} Y_e^{br} Y_u^{st} (Y_d Y_d^\dagger)^{dc} \Big\} C_{\ell q}^{(\parallel)abcd} + \left\{ g_Y^2 \left( \frac{34}{27} \delta^{sc} \delta^{ab} Y_e^{pr} Y_u^{dt} + \frac{50}{27} \delta^{pa} \delta^{cd} Y_e^{br} Y_u^{st} \right. \right. \\
& - \frac{211}{18} \delta^{pa} \delta^{sc} Y_e^{br} Y_u^{dt} \Big) + g_L^2 \left( \frac{4}{3} \delta^{sc} \delta^{ab} Y_e^{pr} Y_u^{dt} + 4 \delta^{pa} \delta^{cd} Y_e^{br} Y_u^{st} - \frac{57}{2} \delta^{pa} \delta^{sc} Y_e^{br} Y_u^{dt} \right) + \frac{3}{2} \delta^{pa} \delta^{sc} Y_u^{dt} (Y_e Y_e^\dagger Y_e)^{br} + \frac{3}{2} \delta^{pa} \delta^{sc} Y_e^{br} (Y_u Y_u^\dagger Y_u)^{dt} \\
& + \frac{5}{2} \delta^{pa} \delta^{sc} Y_e^{br} (Y_d Y_d^\dagger Y_u)^{dt} + 3 T_2 \delta^{pa} \delta^{sc} Y_e^{br} Y_u^{dt} + \frac{16}{3} \delta^{pa} \delta^{sc} g_s^2 Y_e^{br} Y_u^{dt} + 8 \delta^{pa} Y_e^{br} Y_u^{dt} (Y_d Y_d^\dagger)^{sc} - \frac{5}{2} \delta^{sc} Y_e^{br} Y_u^{dt} (Y_e Y_e^\dagger)^{pa} - \frac{5}{2} \delta^{pa} Y_e^{br} Y_u^{dt} (Y_u Y_u^\dagger)^{sc} \\
& - 18 \delta^{pa} Y_e^{br} Y_u^{st} (Y_d Y_d^\dagger)^{dc} \Big\} C_{\ell q}^{(\times)abcd}, \tag{12.8}
\end{aligned}$$

## 12.5 $C_{\ell u q e}$

$$\begin{aligned}
\beta_{C_{\ell u q e}^{prst}}^{(1)} &= \frac{20}{3} \delta^{pa} \delta^{tb} g_Y^2 C_{eB}^{ab} Y_u^{sr} - 6 \delta^{pa} \delta^{tb} g_L^2 C_{eW}^{ab} Y_u^{sr} - 12 \delta^{rb} \delta^{sa} g_Y^2 C_{uB}^{ab} Y_e^{pt} - 6 \delta^{rb} \delta^{sa} g_L^2 C_{uW}^{ab} Y_e^{pt} + 4 \delta^{pa} \delta^{rd} C_{\ell u}^{abcd} Y_e^{bt} Y_u^{sc} + 4 \delta^{sa} \delta^{td} C_{q e}^{abcd} Y_e^{pc} Y_u^{br} \\
& + 4 \delta^{rd} \delta^{tb} C_{e u}^{abcd} Y_e^{pa} Y_u^{sc} - \left\{ 3 \delta^{pa} \delta^{rd} \delta^{sc} \delta^{tb} g_L^2 + 5 \delta^{pa} \delta^{rd} \delta^{sc} \delta^{tb} g_Y^2 \right\} C_{\ell e q u}^{abcd} + \left\{ \frac{1}{2} \left( \delta^{pa} \delta^{rb} \delta^{td} (Y_d Y_d^\dagger)^{sc} + \delta^{rb} \delta^{sc} \delta^{td} (Y_e Y_e^\dagger)^{pa} + \delta^{pa} \delta^{rb} \delta^{td} (Y_u Y_u^\dagger)^{sc} \right. \right. \\
& + 2 \delta^{pa} \delta^{rb} \delta^{sc} (Y_e^\dagger Y_e)^{dt} + 2 \delta^{pa} \delta^{sc} \delta^{td} (Y_u^\dagger Y_u)^{br} \Big) + \frac{8}{3} \delta^{pa} \delta^{rb} \delta^{sc} \delta^{td} g_s^2 + \frac{49}{18} \delta^{pa} \delta^{rb} \delta^{sc} \delta^{td} g_Y^2 - \frac{3}{2} \delta^{pa} \delta^{rb} \delta^{sc} \delta^{td} g_L^2 \Big\} C_{\ell u q e}^{abcd} + 4 \delta^{pa} \delta^{sc} C_{\ell q}^{(\parallel)abcd} Y_e^{bt} Y_u^{dr}
\end{aligned}$$



$$-4\delta^{pa}\delta^{sc}\mathcal{C}_{\ell q}^{(\times)abcd}Y_e^{bt}Y_u^{dr}, \quad (12.9)$$

$$\begin{aligned} \beta_{\mathcal{C}_{\ell uge}^{prst}}^{(2)} = & -15g_L^6\mathcal{C}_W Y_e^{pt}Y_u^{sr} - 19ig_L^6\mathcal{C}_{\widetilde{W}} Y_e^{pt}Y_u^{sr} + \left\{ g_Y^2 \left( \frac{8}{3}\delta^{pa}\delta^{tb}(Y_d Y_d^\dagger Y_u)^{sr} - \frac{5}{3}\delta^{pa}Y_u^{sr}(Y_e^\dagger Y_e)^{bt} - \frac{10}{3}\text{T}_2\delta^{pa}\delta^{tb}Y_u^{sr} - \frac{10}{3}\delta^{tb}Y_u^{sr}(Y_e Y_e^\dagger)^{pa} - 8\delta^{pa}\delta^{tb}(Y_u Y_u^\dagger Y_u)^{sr} \right) \right. \\ & + 4\delta^{pa}\delta^{tb}g_Y^2g_L^2Y_u^{sr} - \frac{295}{9}\delta^{pa}\delta^{tb}g_Y^4Y_u^{sr} - \frac{440}{9}\delta^{pa}\delta^{tb}g_Y^2g_s^2Y_u^{sr} \Big\} \mathcal{C}_{eB}^{ab} + \left\{ g_L^2 \left( \frac{3}{2}\delta^{pa}Y_u^{sr}(Y_e^\dagger Y_e)^{bt} + 3\text{T}_2\delta^{pa}\delta^{tb}Y_u^{sr} \right) + \frac{32}{3}\delta^{pa}\delta^{tb}g_Y^2g_L^2Y_u^{sr} \right. \\ & + 44\delta^{pa}\delta^{tb}g_s^2g_L^2Y_u^{sr} - \frac{199}{6}\delta^{pa}\delta^{tb}g_L^4Y_u^{sr} \Big\} \mathcal{C}_{eW}^{ab} + \left\{ g_Y^2 \left( 3\delta^{sa}Y_e^{pt}(Y_u^\dagger Y_u)^{br} + 6\text{T}_2\delta^{rb}\delta^{sa}Y_e^{pt} + 6\delta^{rb}Y_e^{pt}(Y_d Y_d^\dagger)^{sa} + 6\delta^{rb}Y_e^{pt}(Y_u Y_u^\dagger)^{sa} \right. \right. \\ & + 16\delta^{rb}\delta^{sa}(Y_e Y_e^\dagger Y_e)^{pt} \Big) + \frac{233}{3}\delta^{rb}\delta^{sa}g_Y^4Y_e^{pt} - 8\delta^{rb}\delta^{sa}g_Y^2g_L^2Y_e^{pt} - 8\delta^{rb}\delta^{sa}g_Y^2g_s^2Y_e^{pt} \Big\} \mathcal{C}_{uB}^{ab} + \left\{ g_L^2 \left( \frac{3}{2}\delta^{sa}Y_e^{pt}(Y_u^\dagger Y_u)^{br} + 3\text{T}_2\delta^{rb}\delta^{sa}Y_e^{pt} \right. \right. \\ & - 3\delta^{rb}Y_e^{pt}(Y_d Y_d^\dagger)^{sa} \Big) + \frac{62}{3}\delta^{rb}\delta^{sa}g_Y^2g_L^2Y_e^{pt} - 4\delta^{rb}\delta^{sa}g_s^2g_L^2Y_e^{pt} - \frac{199}{6}\delta^{rb}\delta^{sa}g_L^4Y_e^{pt} \Big\} \mathcal{C}_{uW}^{ab} + \left\{ 8\delta^{rb}\delta^{sa}g_s^2g_L^2Y_e^{pt} + \frac{40}{3}\delta^{rb}\delta^{sa}g_Y^2g_s^2Y_e^{pt} \right\} \mathcal{C}_{uG}^{ab} \\ & + 9\delta^{sa}g_Y^2\mathcal{C}_{dB}^{ab}Y_e^{pt}(Y_d^\dagger Y_u)^{br} + 6g_Y^2\mathcal{C}_{dB}^{*ab}Y_d^{sb}Y_e^{pt}Y_u^{ar} + \frac{9}{2}\delta^{sa}g_L^2\mathcal{C}_{dW}^{ab}Y_e^{pt}(Y_d^\dagger Y_u)^{br} - 3g_L^2\mathcal{C}_{dW}^{*ab}Y_d^{sb}Y_e^{pt}Y_u^{ar} + \left\{ \delta^{pa}Y_e^{bt}(Y_u Y_u^\dagger Y_u)^{sr} + \frac{55}{27}\delta^{pa}g_Y^2Y_e^{bt}Y_u^{sr} \right. \\ & + 5\delta^{pa}Y_e^{bt}(Y_d Y_d^\dagger Y_u)^{sr} + 6\delta^{pa}g_L^2Y_e^{bt}Y_u^{sr} \Big\} \mathcal{C}_{H\ell}^{(\text{ll})ab} + \left\{ \frac{7}{6}\delta^{pa}g_L^2Y_e^{bt}Y_u^{sr} + \frac{325}{54}\delta^{pa}g_Y^2Y_e^{bt}Y_u^{sr} - \delta^{pa}Y_e^{bt}(Y_u Y_u^\dagger Y_u)^{sr} - 5\delta^{pa}Y_e^{bt}(Y_d Y_d^\dagger Y_u)^{sr} \right\} \mathcal{C}_{H\ell}^{(\times)ab} \\ & + \left\{ \delta^{tb}Y_e^{pa}(Y_u Y_u^\dagger Y_u)^{sr} + 5\delta^{tb}Y_e^{pa}(Y_d Y_d^\dagger Y_u)^{sr} - \frac{215}{27}\delta^{tb}g_Y^2Y_e^{pa}Y_u^{sr} \right\} \mathcal{C}_{He}^{ab} + \left\{ \frac{1}{3}\delta^{sa}g_Y^2Y_e^{pt}Y_u^{br} - \delta^{sa}Y_u^{br}(Y_e Y_e^\dagger Y_e)^{pt} - 6\delta^{sa}g_L^2Y_e^{pt}Y_u^{br} \right\} \mathcal{C}_{Hq}^{(\text{ll})ab} \\ & + \left\{ \frac{19}{6}\delta^{sa}g_Y^2Y_e^{pt}Y_u^{br} - 2\delta^{sa}Y_u^{br}(Y_e Y_e^\dagger Y_e)^{pt} - \frac{29}{6}\delta^{sa}g_L^2Y_e^{pt}Y_u^{br} \right\} \mathcal{C}_{Hq}^{(\times)ab} + \left\{ \frac{31}{3}\delta^{rb}g_Y^2Y_e^{pt}Y_u^{sa} - \delta^{rb}Y_u^{sa}(Y_e Y_e^\dagger Y_e)^{pt} \right\} \mathcal{C}_{Hu}^{ab} \\ & + \mathcal{C}_{Hud}^{*ab} \left\{ 4\delta^{ra}g_Y^2Y_d^{sb}Y_e^{pt} + 4\delta^{ra}Y_d^{sb}(Y_e Y_e^\dagger Y_e)^{pt} \right\} + \left\{ g_Y^2 \left( \frac{10}{27}\delta^{td}\delta^{ab}Y_e^{pc}Y_u^{sr} + \frac{10}{27}\delta^{pa}\delta^{cd}Y_e^{bt}Y_u^{sr} + 5\delta^{pa}\delta^{td}Y_e^{bc}Y_u^{sr} \right) + 3\delta^{pa}\delta^{td}g_L^2Y_e^{bc}Y_u^{sr} \right\} \mathcal{C}_{\ell e}^{abcd} + \left\{ \right. \\ & - g_Y^2 \left( \frac{2}{3}\delta^{rd}\delta^{ab}Y_e^{pt}Y_u^{sc} + \frac{20}{27}\delta^{pa}\delta^{cd}Y_e^{bt}Y_u^{sr} + \frac{163}{9}\delta^{pa}\delta^{rd}Y_e^{bt}Y_u^{sc} \right) - \delta^{pa}\delta^{rd}Y_u^{sc}(Y_e Y_e^\dagger Y_e)^{bt} - 2\text{T}_2\delta^{pa}\delta^{rd}Y_e^{bt}Y_u^{sc} - 2\delta^{pa}\delta^{rd}Y_e^{bt}(Y_d Y_d^\dagger Y_u)^{sc} \\ & - 2\delta^{pa}\delta^{rd}Y_e^{bt}(Y_u Y_u^\dagger Y_u)^{sc} - 3\delta^{pa}\delta^{rd}g_L^2Y_e^{bt}Y_u^{sc} - 3\delta^{pa}Y_e^{bt}Y_u^{sc}(Y_u^\dagger Y_u)^{dr} - 6\delta^{rd}Y_e^{bt}Y_u^{sc}(Y_e Y_e^\dagger)^{pa} - \frac{88}{3}\delta^{pa}\delta^{rd}g_s^2Y_e^{bt}Y_u^{sc} \Big\} \mathcal{C}_{\ell u}^{abcd} + \left\{ \frac{10}{27}\delta^{pa}\delta^{cd}g_Y^2Y_e^{bt}Y_u^{sr} \right. \\ & - \delta^{pa}Y_d^{sc}Y_e^{bt}(Y_d^\dagger Y_u)^{dr} \Big\} \mathcal{C}_{\ell d}^{abcd} + \left\{ 2\delta^{td}Y_e^{pc}Y_u^{br}(Y_d Y_d^\dagger)^{sa} - g_Y^2 \left( \frac{10}{27}\delta^{td}\delta^{ab}Y_e^{pc}Y_u^{sr} + \frac{2}{3}\delta^{sa}\delta^{cd}Y_e^{pt}Y_u^{br} + \frac{205}{9}\delta^{sa}\delta^{td}Y_e^{pc}Y_u^{br} \right) - \delta^{sa}\delta^{td}Y_e^{pc}(Y_u Y_u^\dagger Y_u)^{br} \right. \\ & - 2\text{T}_2\delta^{sa}\delta^{td}Y_e^{pc}Y_u^{br} - 2\delta^{sa}\delta^{td}Y_u^{br}(Y_e Y_e^\dagger Y_e)^{pc} - 3\delta^{sa}\delta^{td}g_L^2Y_e^{pc}Y_u^{br} - 3\delta^{sa}Y_e^{pc}Y_u^{br}(Y_e^\dagger Y_e)^{dt} - 3\delta^{sa}\delta^{td}Y_e^{pc}(Y_d Y_d^\dagger Y_u)^{br} - 6\delta^{td}Y_e^{pc}Y_u^{br}(Y_u Y_u^\dagger)^{sa} \Big\} \end{aligned}$$

$$\begin{aligned}
& -\frac{88}{3}\delta^{sa}\delta^{td}g_s^2Y_e^{pc}Y_u^{br}\left\}C_{qe}^{abcd} + \left\{g_Y^2\left(\frac{2}{3}\delta^{rd}\delta^{ab}Y_e^{pt}Y_u^{sc} + \frac{4}{3}\delta^{sa}\delta^{cd}Y_e^{pt}Y_u^{br} + 5\delta^{rd}\delta^{sa}Y_e^{pt}Y_u^{bc}\right) + 3\delta^{rd}\delta^{sa}g_L^2Y_e^{pt}Y_u^{bc}\right\}C_{qu}^{(\parallel)abcd} + \left\{g_Y^2\left(\frac{2}{9}\delta^{rd}\delta^{ab}Y_e^{pt}Y_u^{sc}\right.\right. \\
& + \frac{4}{9}\delta^{sa}\delta^{cd}Y_e^{pt}Y_u^{br} + 15\delta^{rd}\delta^{sa}Y_e^{pt}Y_u^{bc}\left.\right) + 9\delta^{rd}\delta^{sa}g_L^2Y_e^{pt}Y_u^{bc}\left\}C_{qu}^{(\times)abcd} - \frac{2}{3}\delta^{sa}\delta^{cd}g_Y^2C_{qd}^{(\parallel)abcd}Y_e^{pt}Y_u^{br} - \frac{2}{9}\delta^{sa}\delta^{cd}g_Y^2C_{qd}^{(\times)abcd}Y_e^{pt}Y_u^{br} \\
& - \frac{80}{27}\delta^{tb}\delta^{ad}g_Y^2C_{ee}^{abcd}Y_e^{pc}Y_u^{sr} + g_Y^2\left\{\frac{8}{3}\delta^{rb}\delta^{cd}Y_e^{pt}Y_u^{sa} - \frac{40}{9}\delta^{rb}\delta^{ad}Y_e^{pt}Y_u^{sc}\right\}C_{uu}^{abcd} + \left\{g_Y^2\left(\frac{8}{9}\delta^{rd}\delta^{tb}Y_e^{pa}Y_u^{sc} - \frac{2}{3}\delta^{rd}\delta^{ab}Y_e^{pt}Y_u^{sc} - \frac{20}{27}\delta^{tb}\delta^{cd}Y_e^{pa}Y_u^{sr}\right)\right. \\
& + 6\delta^{rd}\delta^{tb}g_L^2Y_e^{pa}Y_u^{sc} - 2T_2\delta^{rd}\delta^{tb}Y_e^{pa}Y_u^{sc} - 2\delta^{rd}\delta^{tb}Y_e^{pa}(Y_dY_d^\dagger Y_u)^{sc} - 2\delta^{rd}\delta^{tb}Y_u^{sc}(Y_eY_e^\dagger Y_e)^{pa} - 2\delta^{rd}\delta^{tb}Y_e^{pa}(Y_uY_u^\dagger Y_u)^{sc} - 3\delta^{rd}Y_e^{pa}Y_u^{sc}(Y_e^\dagger Y_e)^{bt} \\
& - 3\delta^{tb}Y_e^{pa}Y_u^{sc}(Y_u^\dagger Y_u)^{dr} - \frac{88}{3}\delta^{rd}\delta^{tb}g_s^2Y_e^{pa}Y_u^{sc}\left\}C_{eu}^{abcd} + \left\{\frac{10}{27}\delta^{tb}\delta^{cd}g_Y^2Y_e^{pa}Y_u^{sr} - \delta^{tb}Y_d^{sc}Y_e^{pa}(Y_d^\dagger Y_u)^{dr}\right\}C_{ed}^{abcd} - \frac{2}{3}\delta^{rb}\delta^{cd}g_Y^2C_{ud}^{(\parallel)abcd}Y_e^{pt}Y_u^{sa} \\
& - \frac{2}{9}\delta^{rb}\delta^{cd}g_Y^2C_{ud}^{(\times)abcd}Y_e^{pt}Y_u^{sa} + \left\{\frac{1}{2}\delta^{pa}Y_d^{sc}Y_u^{dr}(Y_e^\dagger Y_e)^{bt} + \frac{1}{2}\delta^{tb}Y_d^{sc}Y_u^{dr}(Y_eY_e^\dagger)^{pa} - \frac{9}{2}\delta^{pa}\delta^{tb}g_L^2Y_d^{dc}Y_u^{sr} - \frac{15}{2}\delta^{pa}\delta^{tb}g_Y^2Y_d^{dc}Y_u^{sr}\right\}C_{ledq}^{abcd} \\
& + \delta^{sd}C_{ledq}^{*abcd}Y_e^{pb}Y_e^{at}(Y_d^\dagger Y_u)^{cr} + \left\{g_L^2\left(\frac{3}{2}\delta^{rb}\delta^{sc}Y_d^{*ad}Y_e^{pt} - \frac{9}{2}\delta^{rb}\delta^{sa}Y_d^{*cd}Y_e^{pt}\right) - g_Y^2\left(\frac{1}{2}\delta^{rb}\delta^{sc}Y_d^{*ad}Y_e^{pt} + \frac{15}{2}\delta^{rb}\delta^{sa}Y_d^{*cd}Y_e^{pt}\right)\right\}C_{quqd}^{(\parallel)abcd} \\
& + \left\{g_L^2\left(\frac{9}{2}\delta^{rb}\delta^{sc}Y_d^{*ad}Y_e^{pt} - \frac{3}{2}\delta^{rb}\delta^{sa}Y_d^{*cd}Y_e^{pt}\right) - g_Y^2\left(\frac{3}{2}\delta^{rb}\delta^{sc}Y_d^{*ad}Y_e^{pt} + \frac{5}{2}\delta^{rb}\delta^{sa}Y_d^{*cd}Y_e^{pt}\right)\right\}C_{quqd}^{(\times)abcd} + \left\{\frac{1}{2}\delta^{sc}\delta^{tb}(Y_u^\dagger Y_u)^{dr}(Y_eY_e^\dagger)^{pa}\right. \\
& + \frac{1}{2}\delta^{pa}\delta^{rd}(Y_e^\dagger Y_e)^{bt}(Y_uY_u^\dagger)^{sc} + g_L^2\left(\frac{3}{2}\delta^{rd}\delta^{sc}Y_e^{*ab}Y_e^{pt} + \frac{9}{2}\delta^{pa}\delta^{tb}Y_u^{*cd}Y_u^{sr}\right) + g_Y^2\left(2\delta^{pa}\delta^{sc}\delta^{tb}(Y_u^\dagger Y_u)^{dr} + \frac{5}{2}\delta^{rd}\delta^{sc}Y_e^{*ab}Y_e^{pt} + \frac{10}{3}\delta^{pa}\delta^{rd}\delta^{sc}(Y_e^\dagger Y_e)^{bt}\right. \\
& + \frac{10}{3}\delta^{rd}\delta^{sc}\delta^{tb}(Y_eY_e^\dagger)^{pa} + 4\delta^{pa}\delta^{rd}\delta^{tb}(Y_uY_u^\dagger)^{sc} + \frac{15}{2}\delta^{pa}\delta^{tb}Y_u^{*cd}Y_u^{sr} - 2\delta^{pa}\delta^{rd}\delta^{tb}(Y_dY_d^\dagger)^{sc}\left.\right) + \frac{49}{3}\delta^{pa}\delta^{rd}\delta^{sc}\delta^{tb}g_Y^2g_L^2 + 22\delta^{pa}\delta^{rd}\delta^{sc}\delta^{tb}g_s^2g_L^2 \\
& + \frac{415}{12}\delta^{pa}\delta^{rd}\delta^{sc}\delta^{tb}g_Y^4 + \frac{110}{3}\delta^{pa}\delta^{rd}\delta^{sc}\delta^{tb}g_Y^2g_s^2 - \delta^{pa}\delta^{sc}(Y_e^\dagger Y_e)^{bt}(Y_u^\dagger Y_u)^{dr} - \delta^{rd}\delta^{tb}(Y_eY_e^\dagger)^{pa}(Y_uY_u^\dagger)^{sc} - 2\delta^{pa}\delta^{rd}(Y_e^\dagger Y_e)^{bt}(Y_dY_d^\dagger)^{sc} \\
& - 2\delta^{rd}\delta^{tb}(Y_dY_d^\dagger)^{sc}(Y_eY_e^\dagger)^{pa} - \frac{199}{12}\delta^{pa}\delta^{rd}\delta^{sc}\delta^{tb}g_L^4\left\}C_{lequ}^{abcd} + \left\{g_Y^2\left(\frac{17}{72}\delta^{pa}\delta^{sc}\delta^{td}(Y_u^\dagger Y_u)^{br} + \frac{5}{2}\delta^{pa}\delta^{td}Y_u^{*cb}Y_u^{sr} + \frac{455}{144}\delta^{pa}\delta^{rb}\delta^{td}(Y_dY_d^\dagger)^{sc}\right.\right. \\
& + \frac{11}{2}\delta^{rb}\delta^{sc}Y_e^{*ad}Y_e^{pt} - \frac{49}{24}\delta^{pa}\delta^{rb}\delta^{sc}(Y_e^\dagger Y_e)^{dt} - \frac{469}{144}\delta^{pa}\delta^{rb}\delta^{td}(Y_uY_u^\dagger)^{sc} - \frac{251}{48}\delta^{rb}\delta^{sc}\delta^{td}(Y_eY_e^\dagger)^{pa}\left.\right) + g_L^2\left(\frac{3}{2}\delta^{rb}\delta^{sc}Y_e^{*ad}Y_e^{pt} + \frac{33}{16}\delta^{pa}\delta^{rb}\delta^{td}(Y_dY_d^\dagger)^{sc}\right. \\
& + \frac{33}{16}\delta^{rb}\delta^{sc}\delta^{td}(Y_eY_e^\dagger)^{pa} + \frac{33}{16}\delta^{pa}\delta^{rb}\delta^{td}(Y_uY_u^\dagger)^{sc} + \frac{9}{2}\delta^{pa}\delta^{td}Y_u^{*cb}Y_u^{sr} + \frac{51}{8}\delta^{pa}\delta^{rb}\delta^{sc}(Y_e^\dagger Y_e)^{dt} + \frac{51}{8}\delta^{pa}\delta^{sc}\delta^{td}(Y_u^\dagger Y_u)^{br}\left.\right) + 2\delta^{pa}\delta^{rb}(Y_e^\dagger Y_e)^{dt}(Y_dY_d^\dagger)^{sc} \\
& + 48\delta^{pa}\delta^{rb}\delta^{sc}\delta^{td}g_s^4 - \frac{1}{4}\delta^{pa}\delta^{rb}\delta^{sc}(Y_e^\dagger Y_eY_e^\dagger Y_e)^{dt} - \frac{1}{4}\delta^{pa}\delta^{sc}\delta^{td}(Y_u^\dagger Y_dY_d^\dagger Y_u)^{br} - \frac{1}{4}\delta^{pa}\delta^{sc}\delta^{td}(Y_u^\dagger Y_uY_u^\dagger Y_u)^{br} - \frac{1}{4}\delta^{pa}\delta^{rb}\delta^{td}(Y_dY_d^\dagger Y_dY_d^\dagger)^{sc} \\
& - \frac{1}{4}\delta^{rb}\delta^{sc}\delta^{td}(Y_eY_e^\dagger Y_eY_e^\dagger)^{pa} - \frac{1}{4}\delta^{pa}\delta^{rb}\delta^{td}(Y_uY_u^\dagger Y_uY_u^\dagger)^{sc} - \frac{29}{48}\delta^{pa}\delta^{rb}\delta^{sc}\delta^{td}g_L^4 - \frac{3}{4}T_2\delta^{pa}\delta^{rb}\delta^{td}(Y_dY_d^\dagger)^{sc} - \frac{3}{4}T_2\delta^{rb}\delta^{sc}\delta^{td}(Y_eY_e^\dagger)^{pa}
\end{aligned}$$

$$\begin{aligned}
& -\frac{3}{4}\text{T}_2\delta^{pa}\delta^{rb}\delta^{td}(Y_uY_u^\dagger)^{sc}-\delta^{pa}\delta^{td}(Y_u^\dagger Y_u)^{br}(Y_dY_d^\dagger)^{sc}-\delta^{sc}\delta^{td}(Y_u^\dagger Y_u)^{br}(Y_eY_e^\dagger)^{pa}-\delta^{pa}\delta^{rb}(Y_e^\dagger Y_e)^{dt}(Y_uY_u^\dagger)^{sc}-g_s^2\left(\frac{16}{3}\delta^{pa}\delta^{rb}\delta^{td}(Y_dY_d^\dagger)^{sc}\right. \\
& +\frac{16}{3}\delta^{pa}\delta^{rb}\delta^{td}(Y_uY_u^\dagger)^{sc}+\frac{32}{3}\delta^{pa}\delta^{sc}\delta^{td}(Y_u^\dagger Y_u)^{br})-\frac{3}{2}\text{T}_2\delta^{pa}\delta^{rb}\delta^{sc}(Y_e^\dagger Y_e)^{dt}-\frac{3}{2}\text{T}_2\delta^{pa}\delta^{sc}\delta^{td}(Y_u^\dagger Y_u)^{br}-2\delta^{rb}\delta^{sc}(Y_e^\dagger Y_e)^{dt}(Y_eY_e^\dagger)^{pa} \\
& -2\delta^{pa}\delta^{td}(Y_u^\dagger Y_u)^{br}(Y_uY_u^\dagger)^{sc}-3\delta^{pa}\delta^{rb}\delta^{sc}\delta^{td}g_s^2g_L^2-3\delta^{pa}\delta^{sc}(Y_e^\dagger Y_e)^{dt}(Y_u^\dagger Y_u)^{br}-3\delta^{rb}\delta^{td}(Y_eY_e^\dagger)^{pa}(Y_uY_u^\dagger)^{sc}-\frac{61}{8}\delta^{pa}\delta^{rb}\delta^{sc}\delta^{td}g_Y^2g_L^2 \\
& -\frac{323}{27}\delta^{pa}\delta^{rb}\delta^{sc}\delta^{td}g_Y^2g_s^2-\frac{81995}{1296}\delta^{pa}\delta^{rb}\delta^{sc}\delta^{td}g_Y^4\Big\}C_{\ell u q e}^{abcd}+2C_{\ell u q e}^{*abcd}Y_e^{pd}Y_e^{at}Y_u^{sb}Y_u^{cr}+\left\{g_Y^2\left(\frac{20}{27}\delta^{pa}\delta^{cd}Y_e^{bt}Y_u^{sr}-\frac{50}{27}\delta^{pa}\delta^{bc}Y_e^{dt}Y_u^{sr}\right)\right. \\
& -\frac{10}{3}\delta^{pa}\delta^{bc}g_L^2Y_e^{dt}Y_u^{sr}\Big\}C_{\ell\ell}^{abcd}+\left\{g_Y^2\left(\frac{4}{3}\delta^{sa}\delta^{cd}Y_e^{pt}Y_u^{br}-\frac{10}{9}\delta^{sa}\delta^{bc}Y_e^{pt}Y_u^{dr}\right)-\frac{10}{3}\delta^{sa}\delta^{bc}g_L^2Y_e^{pt}Y_u^{dr}\right\}C_{qq}^{(\parallel)abcd}+\left\{g_Y^2\left(\frac{2}{3}\delta^{sa}\delta^{cd}Y_e^{pt}Y_u^{br}-\frac{20}{9}\delta^{sa}\delta^{bc}Y_e^{pt}Y_u^{dr}\right)\right. \\
& +2\delta^{sa}\delta^{cd}g_L^2Y_e^{pt}Y_u^{br}\Big\}C_{qq}^{(\times)abcd}+\left\{2\delta^{pa}Y_e^{bt}Y_u^{dr}(Y_dY_d^\dagger)^{sc}+21\delta^{pa}\delta^{sc}g_L^2Y_e^{bt}Y_u^{dr}-g_Y^2\left(\frac{10}{27}\delta^{pa}\delta^{cd}Y_e^{bt}Y_u^{sr}+\frac{2}{3}\delta^{sc}\delta^{ab}Y_e^{pt}Y_u^{dr}+\frac{97}{9}\delta^{pa}\delta^{sc}Y_e^{bt}Y_u^{dr}\right)\right. \\
& -\delta^{pa}\delta^{sc}Y_u^{dr}(Y_eY_e^\dagger Y_e)^{bt}-\delta^{pa}\delta^{sc}Y_e^{bt}(Y_uY_u^\dagger Y_u)^{dr}-2\text{T}_2\delta^{pa}\delta^{sc}Y_e^{bt}Y_u^{dr}-3\delta^{pa}\delta^{sc}Y_e^{bt}(Y_dY_d^\dagger Y_u)^{dr}-6\delta^{sc}Y_e^{bt}Y_u^{dr}(Y_eY_e^\dagger)^{pa}-6\delta^{pa}Y_e^{bt}Y_u^{dr}(Y_uY_u^\dagger)^{sc} \\
& -\frac{88}{3}\delta^{pa}\delta^{sc}g_s^2Y_e^{bt}Y_u^{dr}\Big\}C_{\ell q}^{(\parallel)abcd}+\left\{g_Y^2\left(\frac{97}{9}\delta^{pa}\delta^{sc}Y_e^{bt}Y_u^{dr}-\frac{5}{27}\delta^{pa}\delta^{cd}Y_e^{bt}Y_u^{sr}-\frac{1}{3}\delta^{sc}\delta^{ab}Y_e^{pt}Y_u^{dr}\right)+g_L^2\left(\frac{1}{3}\delta^{sc}\delta^{ab}Y_e^{pt}Y_u^{dr}+\delta^{pa}\delta^{cd}Y_e^{bt}Y_u^{sr}\right.\right. \\
& -21\delta^{pa}\delta^{sc}Y_e^{bt}Y_u^{dr})+\delta^{pa}\delta^{sc}Y_u^{dr}(Y_eY_e^\dagger Y_e)^{bt}+\delta^{pa}\delta^{sc}Y_e^{bt}(Y_uY_u^\dagger Y_u)^{dr}+2\text{T}_2\delta^{pa}\delta^{sc}Y_e^{bt}Y_u^{dr}+3\delta^{pa}\delta^{sc}Y_e^{bt}(Y_dY_d^\dagger Y_u)^{dr}+4\delta^{pa}Y_e^{bt}Y_u^{dr}(Y_dY_d^\dagger)^{sc} \\
& \left.+\frac{88}{3}\delta^{pa}\delta^{sc}g_s^2Y_e^{bt}Y_u^{dr}-3\delta^{sc}Y_e^{bt}Y_u^{dr}(Y_eY_e^\dagger)^{pa}-3\delta^{pa}Y_e^{bt}Y_u^{dr}(Y_uY_u^\dagger)^{sc}\right\}C_{\ell q}^{(\times)abcd}, \tag{12.10}
\end{aligned}$$

## 13 $(\bar{L}L)(\bar{L}L)$

### 13.1 $C_{\ell\ell}$

$$\begin{aligned}
\beta_{C_{\ell\ell}^{prst}}^{(1)} & = -2C_{\ell\ell HH}^{*ps}C_{\ell\ell HH}^{rt}+\left\{\frac{1}{2}\left(-\delta^{sa}\delta^{tb}(Y_eY_e^\dagger)^{pr}-\delta^{pa}\delta^{rb}(Y_eY_e^\dagger)^{st}\right)-\frac{1}{6}g_Y^2\left(\delta^{pa}\delta^{rb}\delta^{st}+\delta^{pr}\delta^{sa}\delta^{tb}\right)\right\}C_{H\ell}^{(\parallel)ab}+\left\{\frac{1}{12}g_L^2\left(2\delta^{pt}\delta^{rb}\delta^{sa}+2\delta^{pa}\delta^{rs}\delta^{tb}\right.\right. \\
& -\delta^{pa}\delta^{rb}\delta^{st}-\delta^{pr}\delta^{sa}\delta^{tb})+\frac{1}{2}\left(-\delta^{rb}\delta^{sa}(Y_eY_e^\dagger)^{pt}-\delta^{pa}\delta^{tb}(Y_eY_e^\dagger)^{sr}\right)-\frac{1}{12}g_Y^2\left(\delta^{pa}\delta^{rb}\delta^{st}+\delta^{pr}\delta^{sa}\delta^{tb}\right)\Big\}C_{H\ell}^{(\times)ab}+\left\{\frac{1}{3}g_Y^2\left(\delta^{pa}\delta^{rb}\delta^{st}\delta^{cd}+\delta^{pr}\delta^{sa}\delta^{tb}\delta^{cd}\right)\right. \\
& +\frac{1}{2}\left(-\delta^{pa}\delta^{rb}Y_e^{*td}Y_e^{sc}-\delta^{sa}\delta^{tb}Y_e^{*rd}Y_e^{pc}\right)\Big\}C_{\ell e}^{abcd}-\frac{2}{3}g_Y^2\left\{\delta^{pa}\delta^{rb}\delta^{st}\delta^{cd}+\delta^{pr}\delta^{sa}\delta^{tb}\delta^{cd}\right\}C_{\ell u}^{abcd}+\frac{1}{3}g_Y^2\left\{\delta^{pa}\delta^{rb}\delta^{st}\delta^{cd}+\delta^{pr}\delta^{sa}\delta^{tb}\delta^{cd}\right\}C_{\ell d}^{abcd} \\
& +\left\{\frac{1}{3}g_L^2\left(2\delta^{pt}\delta^{rd}\delta^{sa}\delta^{bc}+2\delta^{pa}\delta^{rs}\delta^{td}\delta^{bc}+18\delta^{pa}\delta^{rd}\delta^{sc}\delta^{tb}-\delta^{pa}\delta^{rd}\delta^{st}\delta^{bc}-\delta^{pr}\delta^{sa}\delta^{td}\delta^{bc}-9\delta^{pa}\delta^{rb}\delta^{sc}\delta^{td}\right)+\frac{1}{3}g_Y^2\left(\delta^{pa}\delta^{rd}\delta^{st}\delta^{bc}\right.\right.
\end{aligned}$$

$$\begin{aligned}
& + \delta^{pr} \delta^{sa} \delta^{td} \delta^{bc} + 2\delta^{pa} \delta^{rb} \delta^{st} \delta^{cd} + 2\delta^{pr} \delta^{sa} \delta^{tb} \delta^{cd} + 9\delta^{pa} \delta^{rb} \delta^{sc} \delta^{td} \Big) + \frac{1}{2} \Big( \delta^{rd} \delta^{sa} \delta^{tb} (Y_e Y_e^\dagger)^{pc} + \delta^{pa} \delta^{rb} \delta^{td} (Y_e Y_e^\dagger)^{sc} + \delta^{pa} \delta^{sc} \delta^{td} (Y_e Y_e^\dagger)^{br} \\
& + \delta^{pa} \delta^{rb} \delta^{sc} (Y_e Y_e^\dagger)^{dt} \Big) \Big\} C_{\ell\ell}^{abcd} - \frac{1}{3} g_Y^2 \Big\{ \delta^{pa} \delta^{rb} \delta^{st} \delta^{cd} + \delta^{pr} \delta^{sa} \delta^{tb} \delta^{cd} \Big\} C_{\ell q}^{(\parallel)abcd} + \Big\{ \frac{1}{2} g_L^2 \Big( 2\delta^{pt} \delta^{rb} \delta^{sa} \delta^{cd} + 2\delta^{pa} \delta^{rs} \delta^{tb} \delta^{cd} - \delta^{pa} \delta^{rb} \delta^{st} \delta^{cd} \\
& - \delta^{pr} \delta^{sa} \delta^{tb} \delta^{cd} \Big) - \frac{1}{6} g_Y^2 \Big( \delta^{pa} \delta^{rb} \delta^{st} \delta^{cd} + \delta^{pr} \delta^{sa} \delta^{tb} \delta^{cd} \Big) \Big\} C_{\ell q}^{(\times)abcd}, \tag{13.1}
\end{aligned}$$

$$\begin{aligned}
\beta_{C_{\ell\ell}^{prst}}^{(2)} &= \frac{1}{12} g_Y^2 \Big( 11\delta^{st} (C_{\ell HH} C_{\ell HH}^\dagger)^{rp} + 11\delta^{pr} (C_{\ell HH} C_{\ell HH}^\dagger)^{ts} - 48C_{\ell HH}^{*ps} C_{\ell HH}^{rt} \Big) + \frac{1}{4} \Big( 4(C_{\ell HH} C_{\ell HH}^\dagger)^{rs} (Y_e Y_e^\dagger)^{pt} \\
& + 4(C_{\ell HH} C_{\ell HH}^\dagger)^{tp} (Y_e Y_e^\dagger)^{sr} + 16T_2 C_{\ell HH}^{*ps} C_{\ell HH}^{rt} - 5(C_{\ell HH} C_{\ell HH}^\dagger)^{ts} (Y_e Y_e^\dagger)^{pr} - 5(C_{\ell HH} C_{\ell HH}^\dagger)^{rp} (Y_e Y_e^\dagger)^{st} \Big) \\
& + \frac{1}{2} g_L^2 \Big( 2\delta^{pt} (C_{\ell HH} C_{\ell HH}^\dagger)^{rs} + 2\delta^{rs} (C_{\ell HH} C_{\ell HH}^\dagger)^{tp} - \delta^{st} (C_{\ell HH} C_{\ell HH}^\dagger)^{rp} - \delta^{pr} (C_{\ell HH} C_{\ell HH}^\dagger)^{ts} - 18C_{\ell HH}^{*ps} C_{\ell HH}^{rt} \Big) + \Big\{ \frac{1}{3} \delta^{pr} \delta^{st} g_Y^6 \\
& - g_Y^4 \Big( \frac{1}{4} \delta^{st} (Y_e Y_e^\dagger)^{pr} + \frac{1}{4} \delta^{pr} (Y_e Y_e^\dagger)^{st} \Big) \Big\} C_{HB} + \Big\{ g_L^6 \Big( \frac{2}{3} \delta^{pt} \delta^{rs} - \frac{1}{3} \delta^{pr} \delta^{st} \Big) + g_L^4 \Big( \frac{3}{4} \delta^{st} (Y_e Y_e^\dagger)^{pr} + \frac{3}{4} \delta^{pr} (Y_e Y_e^\dagger)^{st} - \frac{3}{2} \delta^{rs} (Y_e Y_e^\dagger)^{pt} - \frac{3}{2} \delta^{pt} (Y_e Y_e^\dagger)^{sr} \Big) \Big\} C_{HW} \\
& + \Big\{ \frac{1}{4} \delta^{pr} \delta^{st} g_Y^4 g_L^2 + g_Y^2 g_L^4 \Big( \frac{1}{6} \delta^{pt} \delta^{rs} - \frac{1}{12} \delta^{pr} \delta^{st} \Big) + g_Y^2 g_L^2 \Big( \frac{1}{8} \delta^{rs} (Y_e Y_e^\dagger)^{pt} + \frac{1}{8} \delta^{pt} (Y_e Y_e^\dagger)^{sr} + \frac{1}{2} \delta^{st} (Y_e Y_e^\dagger)^{pr} + \frac{1}{2} \delta^{pr} (Y_e Y_e^\dagger)^{st} \Big) \Big\} C_{HWB} \\
& + \Big\{ g_Y^2 g_L^6 \Big( \frac{21}{2} \delta^{pt} \delta^{rs} - \frac{1}{4} \delta^{pr} \delta^{st} \Big) + g_L^6 \Big( \frac{3}{2} \delta^{rs} (Y_e Y_e^\dagger)^{pt} + \frac{3}{2} \delta^{pt} (Y_e Y_e^\dagger)^{sr} - \frac{3}{4} \delta^{st} (Y_e Y_e^\dagger)^{pr} - \frac{3}{4} \delta^{pr} (Y_e Y_e^\dagger)^{st} \Big) - g_L^8 \Big( \frac{20}{3} \delta^{pt} \delta^{rs} + \frac{95}{12} \delta^{pr} \delta^{st} \Big) \Big\} C_W \\
& + \Big\{ g_Y^4 \Big( \frac{27}{8} \delta^{pa} \delta^{st} Y_e^{*rb} + \frac{27}{8} \delta^{pr} \delta^{sa} Y_e^{*tb} - \frac{1}{2} \delta^{pr} \delta^{st} Y_e^{*ab} \Big) + g_Y^2 g_L^2 \Big( \frac{1}{4} \delta^{pa} \delta^{rs} Y_e^{*tb} + \frac{1}{4} \delta^{pt} \delta^{sa} Y_e^{*rb} - \frac{1}{8} \delta^{pa} \delta^{st} Y_e^{*rb} - \frac{1}{8} \delta^{pr} \delta^{sa} Y_e^{*tb} \Big) \\
& + g_Y^2 \Big( \frac{1}{2} \delta^{st} Y_e^{*rb} (Y_e Y_e^\dagger)^{pa} + \frac{1}{2} \delta^{pr} Y_e^{*tb} (Y_e Y_e^\dagger)^{sa} - 3\delta^{sa} Y_e^{*rb} (Y_e Y_e^\dagger)^{pt} - 3\delta^{pa} Y_e^{*tb} (Y_e Y_e^\dagger)^{sr} \Big) \Big\} C_{eB}^{ab} + C_{eB}^{*ab} \Big\{ g_Y^4 \Big( \frac{27}{8} \delta^{ra} \delta^{st} Y_e^{pb} + \frac{27}{8} \delta^{pr} \delta^{ta} Y_e^{sb} \\
& - \frac{1}{2} \delta^{pr} \delta^{st} Y_e^{ab} \Big) + g_Y^2 g_L^2 \Big( \frac{1}{4} \delta^{pt} \delta^{ra} Y_e^{sb} + \frac{1}{4} \delta^{rs} \delta^{ta} Y_e^{pb} - \frac{1}{8} \delta^{ra} \delta^{st} Y_e^{pb} - \frac{1}{8} \delta^{pr} \delta^{ta} Y_e^{sb} \Big) + g_Y^2 \Big( \frac{1}{2} \delta^{st} Y_e^{pb} (Y_e Y_e^\dagger)^{ar} + \frac{1}{2} \delta^{pr} Y_e^{sb} (Y_e Y_e^\dagger)^{at} - 3\delta^{ra} Y_e^{sb} (Y_e Y_e^\dagger)^{pt} \\
& - 3\delta^{ta} Y_e^{pb} (Y_e Y_e^\dagger)^{sr} \Big) \Big\} + \Big\{ g_Y^2 g_L^2 \Big( \frac{11}{16} \delta^{pa} \delta^{st} Y_e^{*rb} + \frac{11}{16} \delta^{pr} \delta^{sa} Y_e^{*tb} - 2\delta^{pa} \delta^{rs} Y_e^{*tb} - 2\delta^{pt} \delta^{sa} Y_e^{*rb} \Big) + g_L^4 \Big( \frac{1}{8} \delta^{pa} \delta^{rs} Y_e^{*tb} + \frac{1}{8} \delta^{pt} \delta^{sa} Y_e^{*rb} \\
& + \frac{1}{6} \delta^{pt} \delta^{rs} Y_e^{*ab} - \frac{1}{16} \delta^{pa} \delta^{st} Y_e^{*rb} - \frac{1}{16} \delta^{pr} \delta^{sa} Y_e^{*tb} - \frac{1}{12} \delta^{pr} \delta^{st} Y_e^{*ab} \Big) + g_L^2 \Big( \frac{3}{2} \delta^{sa} Y_e^{*tb} (Y_e Y_e^\dagger)^{pr} + \frac{3}{2} \delta^{pa} Y_e^{*rb} (Y_e Y_e^\dagger)^{st} - \frac{3}{4} \delta^{sa} Y_e^{*rb} (Y_e Y_e^\dagger)^{pt} \\
& - \frac{3}{4} \delta^{pa} Y_e^{*tb} (Y_e Y_e^\dagger)^{sr} \Big) \Big\} C_{eW}^{ab} + C_{eW}^{*ab} \Big\{ g_Y^2 g_L^2 \Big( \frac{11}{16} \delta^{ra} \delta^{st} Y_e^{pb} + \frac{11}{16} \delta^{pr} \delta^{ta} Y_e^{sb} - 2\delta^{pt} \delta^{ra} Y_e^{sb} - 2\delta^{rs} \delta^{ta} Y_e^{pb} \Big) + g_L^4 \Big( \frac{1}{8} \delta^{pt} \delta^{ra} Y_e^{sb} + \frac{1}{8} \delta^{rs} \delta^{ta} Y_e^{pb}
\end{aligned}$$

$$\begin{aligned}
& + \frac{1}{6} \delta^{pt} \delta^{rs} Y_e^{ab} - \frac{1}{16} \delta^{ra} \delta^{st} Y_e^{pb} - \frac{1}{16} \delta^{pr} \delta^{ta} Y_e^{sb} - \frac{1}{12} \delta^{pr} \delta^{st} Y_e^{ab} \Big) + g_L^2 \Big( \frac{3}{2} \delta^{ta} Y_e^{sb} (Y_e Y_e^\dagger)^{pr} + \frac{3}{2} \delta^{ra} Y_e^{pb} (Y_e Y_e^\dagger)^{st} - \frac{3}{4} \delta^{ra} Y_e^{sb} (Y_e Y_e^\dagger)^{pt} - \frac{3}{4} \delta^{ta} Y_e^{pb} (Y_e Y_e^\dagger)^{sr} \Big) \Big\} \\
& + \frac{5}{6} \delta^{pr} \delta^{st} g_Y^4 Y_u^{*ab} \mathbf{C}_{uB}^{ab} + \frac{5}{6} \delta^{pr} \delta^{st} g_Y^4 \mathbf{C}_{uB}^{*ab} Y_u^{ab} + g_L^4 \left\{ \frac{1}{2} \delta^{pt} \delta^{rs} Y_u^{*ab} - \frac{1}{4} \delta^{pr} \delta^{st} Y_u^{*ab} \right\} \mathbf{C}_{uW}^{ab} + g_L^4 \mathbf{C}_{uW}^{*ab} \left\{ \frac{1}{2} \delta^{pt} \delta^{rs} Y_u^{ab} - \frac{1}{4} \delta^{pr} \delta^{st} Y_u^{ab} \right\} \\
& - \frac{1}{6} \delta^{pr} \delta^{st} g_Y^4 Y_d^{*ab} \mathbf{C}_{dB}^{ab} - \frac{1}{6} \delta^{pr} \delta^{st} g_Y^4 \mathbf{C}_{dB}^{*ab} Y_d^{ab} + g_L^4 \left\{ \frac{1}{2} \delta^{pt} \delta^{rs} Y_d^{*ab} - \frac{1}{4} \delta^{pr} \delta^{st} Y_d^{*ab} \right\} \mathbf{C}_{dW}^{ab} + g_L^4 \mathbf{C}_{dW}^{*ab} \left\{ \frac{1}{2} \delta^{pt} \delta^{rs} Y_d^{ab} - \frac{1}{4} \delta^{pr} \delta^{st} Y_d^{ab} \right\} \\
& + \left\{ \frac{1}{2} T_2 \delta^{sa} \delta^{tb} (Y_e Y_e^\dagger)^{pr} + \frac{1}{2} T_2 \delta^{pa} \delta^{rb} (Y_e Y_e^\dagger)^{st} + g_Y^2 g_L^2 \left( \frac{91}{108} \delta^{pt} \delta^{rb} \delta^{sa} + \frac{91}{108} \delta^{pa} \delta^{rs} \delta^{tb} - \frac{415}{216} \delta^{pa} \delta^{rb} \delta^{st} - \frac{415}{216} \delta^{pr} \delta^{sa} \delta^{tb} \right) \right. \\
& + g_L^2 \left( \frac{1}{4} \delta^{rb} \delta^{sa} (Y_e Y_e^\dagger)^{pt} + \frac{1}{4} \delta^{pa} \delta^{tb} (Y_e Y_e^\dagger)^{sr} + \frac{29}{72} \delta^{rs} \delta^{tb} (Y_e Y_e^\dagger)^{pa} + \frac{29}{72} \delta^{pt} \delta^{rb} (Y_e Y_e^\dagger)^{sa} + \frac{29}{72} \delta^{pt} \delta^{sa} (Y_e Y_e^\dagger)^{br} + \frac{29}{72} \delta^{pa} \delta^{rs} (Y_e Y_e^\dagger)^{bt} \right. \\
& - \frac{29}{144} \delta^{rb} \delta^{st} (Y_e Y_e^\dagger)^{pa} - \frac{29}{144} \delta^{pr} \delta^{tb} (Y_e Y_e^\dagger)^{sa} - \frac{29}{144} \delta^{pa} \delta^{st} (Y_e Y_e^\dagger)^{br} - \frac{29}{144} \delta^{pr} \delta^{sa} (Y_e Y_e^\dagger)^{bt} - \frac{35}{16} \delta^{sa} \delta^{tb} (Y_e Y_e^\dagger)^{pr} - \frac{35}{16} \delta^{pa} \delta^{rb} (Y_e Y_e^\dagger)^{st} \Big) \\
& + g_Y^2 \left( \frac{1}{6} T_2 \delta^{pa} \delta^{rb} \delta^{st} + \frac{1}{6} T_2 \delta^{pr} \delta^{sa} \delta^{tb} + \frac{19}{16} \delta^{sa} \delta^{tb} (Y_e Y_e^\dagger)^{pr} + \frac{19}{16} \delta^{pa} \delta^{rb} (Y_e Y_e^\dagger)^{st} - \frac{1}{144} \delta^{rb} \delta^{st} (Y_e Y_e^\dagger)^{pa} - \frac{1}{144} \delta^{pr} \delta^{tb} (Y_e Y_e^\dagger)^{sa} \right. \\
& - \frac{1}{144} \delta^{pa} \delta^{st} (Y_e Y_e^\dagger)^{br} - \frac{1}{144} \delta^{pr} \delta^{sa} (Y_e Y_e^\dagger)^{bt} \Big) + \frac{3}{2} \delta^{sa} \delta^{tb} (Y_e Y_e^\dagger Y_e Y_e^\dagger)^{pr} + \frac{3}{2} \delta^{pa} \delta^{rb} (Y_e Y_e^\dagger Y_e Y_e^\dagger)^{st} - \frac{1}{8} \delta^{tb} (Y_e Y_e^\dagger)^{pa} (Y_e Y_e^\dagger)^{sr} - \frac{1}{8} \delta^{rb} (Y_e Y_e^\dagger)^{pt} (Y_e Y_e^\dagger)^{sa} \\
& - \frac{1}{8} \delta^{sa} (Y_e Y_e^\dagger)^{pt} (Y_e Y_e^\dagger)^{br} - \frac{1}{8} \delta^{pa} (Y_e Y_e^\dagger)^{sr} (Y_e Y_e^\dagger)^{bt} - g_Y^4 \left( \frac{17}{216} \delta^{pa} \delta^{rb} \delta^{st} + \frac{17}{216} \delta^{pr} \delta^{sa} \delta^{tb} \right) \Big\} \mathbf{C}_{He}^{(II)ab} + \left\{ \frac{1}{4} \delta^{tb} (Y_e Y_e^\dagger)^{pa} (Y_e Y_e^\dagger)^{sr} + \frac{1}{4} \delta^{rb} (Y_e Y_e^\dagger)^{pt} (Y_e Y_e^\dagger)^{sa} \right. \\
& + \frac{1}{4} \delta^{sa} (Y_e Y_e^\dagger)^{pt} (Y_e Y_e^\dagger)^{br} + \frac{1}{4} \delta^{pa} (Y_e Y_e^\dagger)^{sr} (Y_e Y_e^\dagger)^{bt} + \frac{1}{4} \delta^{rb} \delta^{sa} (Y_e Y_e^\dagger Y_e Y_e^\dagger)^{pt} + \frac{1}{4} \delta^{pa} \delta^{tb} (Y_e Y_e^\dagger Y_e Y_e^\dagger)^{sr} + \frac{1}{2} T_2 \delta^{rb} \delta^{sa} (Y_e Y_e^\dagger)^{pt} \\
& + \frac{1}{2} T_2 \delta^{pa} \delta^{tb} (Y_e Y_e^\dagger)^{sr} + \frac{5}{8} \delta^{sa} \delta^{tb} (Y_e Y_e^\dagger Y_e Y_e^\dagger)^{pr} + \frac{5}{8} \delta^{pa} \delta^{rb} (Y_e Y_e^\dagger Y_e Y_e^\dagger)^{st} + g_Y^2 g_L^2 \left( \frac{77}{108} \delta^{pt} \delta^{rb} \delta^{sa} + \frac{77}{108} \delta^{pa} \delta^{rs} \delta^{tb} - \frac{1}{18} \delta^{pr} \delta^{st} \delta^{ab} \right. \\
& - \frac{151}{108} \delta^{pa} \delta^{rb} \delta^{st} - \frac{151}{108} \delta^{pr} \delta^{sa} \delta^{tb} \Big) + g_L^4 \left( \frac{1}{18} \delta^{pr} \delta^{st} \delta^{ab} + \frac{13}{36} \delta^{pt} \delta^{rb} \delta^{sa} + \frac{13}{36} \delta^{pa} \delta^{rs} \delta^{tb} - \frac{1}{9} \delta^{pt} \delta^{rs} \delta^{ab} - \frac{71}{144} \delta^{pa} \delta^{rb} \delta^{st} - \frac{71}{144} \delta^{pr} \delta^{sa} \delta^{tb} \right) \\
& + g_Y^2 \left( \frac{1}{12} \delta^{st} \delta^{ab} (Y_e Y_e^\dagger)^{pr} + \frac{1}{12} \delta^{pr} \delta^{ab} (Y_e Y_e^\dagger)^{st} + \left( \frac{1}{4} \delta^{pa} \delta^{rb} \delta^{st} + \frac{1}{4} \delta^{pr} \delta^{sa} \delta^{tb} \right) \text{Tr}[Y_d^\dagger Y_d] + \left( \frac{1}{6} \delta^{pa} \delta^{rb} \delta^{st} + \frac{1}{6} \delta^{pr} \delta^{sa} \delta^{tb} \right) \text{Tr}[Y_e^\dagger Y_e] + \left( \frac{1}{4} \delta^{pa} \delta^{rb} \delta^{st} \right. \right. \\
& + \frac{1}{4} \delta^{pr} \delta^{sa} \delta^{tb} \Big) \text{Tr}[Y_u^\dagger Y_u] + \frac{19}{16} \delta^{rb} \delta^{sa} (Y_e Y_e^\dagger)^{pt} + \frac{19}{16} \delta^{pa} \delta^{tb} (Y_e Y_e^\dagger)^{sr} - \frac{13}{72} \delta^{rb} \delta^{st} (Y_e Y_e^\dagger)^{pa} - \frac{13}{72} \delta^{pr} \delta^{tb} (Y_e Y_e^\dagger)^{sa} - \frac{13}{72} \delta^{pa} \delta^{st} (Y_e Y_e^\dagger)^{br} \\
& - \frac{13}{72} \delta^{pr} \delta^{sa} (Y_e Y_e^\dagger)^{bt} \Big) + g_L^2 \left( \frac{1}{72} \delta^{rb} \delta^{st} (Y_e Y_e^\dagger)^{pa} + \frac{1}{72} \delta^{pr} \delta^{tb} (Y_e Y_e^\dagger)^{sa} + \frac{1}{72} \delta^{pa} \delta^{st} (Y_e Y_e^\dagger)^{br} + \frac{1}{72} \delta^{pr} \delta^{sa} (Y_e Y_e^\dagger)^{bt} + \frac{1}{8} \delta^{sa} \delta^{tb} (Y_e Y_e^\dagger)^{pr} \right. \\
& + \frac{1}{8} \delta^{pa} \delta^{rb} (Y_e Y_e^\dagger)^{st} + \frac{1}{6} \delta^{rs} \delta^{ab} (Y_e Y_e^\dagger)^{pt} + \frac{1}{6} \delta^{pt} \delta^{ab} (Y_e Y_e^\dagger)^{sr} + \left( \frac{1}{4} \delta^{pa} \delta^{rb} \delta^{st} + \frac{1}{4} \delta^{pr} \delta^{sa} \delta^{tb} - \frac{1}{2} \delta^{pt} \delta^{rb} \delta^{sa} - \frac{1}{2} \delta^{pa} \delta^{rs} \delta^{tb} \right) \text{Tr}[Y_d^\dagger Y_d] + \left( \frac{1}{4} \delta^{pa} \delta^{rb} \delta^{st} \right. \\
& + \frac{1}{4} \delta^{pr} \delta^{sa} \delta^{tb} - \frac{1}{2} \delta^{pt} \delta^{rb} \delta^{sa} - \frac{1}{2} \delta^{pa} \delta^{rs} \delta^{tb} \Big) \text{Tr}[Y_u^\dagger Y_u] - \frac{1}{36} \delta^{rs} \delta^{tb} (Y_e Y_e^\dagger)^{pa} - \frac{1}{36} \delta^{pt} \delta^{rb} (Y_e Y_e^\dagger)^{sa} - \frac{1}{36} \delta^{pt} \delta^{sa} (Y_e Y_e^\dagger)^{br} - \frac{1}{36} \delta^{pa} \delta^{rs} (Y_e Y_e^\dagger)^{bt}
\end{aligned}$$

$$\begin{aligned}
& -\frac{1}{12}\delta^{st}\delta^{ab}(Y_e Y_e^\dagger)^{pr} - \frac{1}{12}\delta^{pr}\delta^{ab}(Y_e Y_e^\dagger)^{st} - \frac{31}{16}\delta^{rb}\delta^{sa}(Y_e Y_e^\dagger)^{pt} - \frac{31}{16}\delta^{pa}\delta^{tb}(Y_e Y_e^\dagger)^{sr} - \frac{1}{4}\delta^{rb}(Y_e Y_e^\dagger)^{pa}(Y_e Y_e^\dagger)^{st} - \frac{1}{4}\delta^{tb}(Y_e Y_e^\dagger)^{pr}(Y_e Y_e^\dagger)^{sa} \\
& - \frac{1}{4}\delta^{pa}(Y_e Y_e^\dagger)^{st}(Y_e Y_e^\dagger)^{br} - \frac{1}{4}\delta^{sa}(Y_e Y_e^\dagger)^{pr}(Y_e Y_e^\dagger)^{bt} - g_Y^4 \left( \frac{17}{432}\delta^{pa}\delta^{rb}\delta^{st} + \frac{17}{432}\delta^{pr}\delta^{sa}\delta^{tb} \right) \left\{ C_{Hl}^{(\times)ab} + \left\{ \frac{1}{2}\delta^{rb}Y_e^{*ad}Y_e^{sc}(Y_e Y_e^\dagger)^{pt} + \frac{1}{2}\delta^{sa}Y_e^{*rd}Y_e^{bc}(Y_e Y_e^\dagger)^{pt} \right. \right. \\
& + \frac{1}{2}\delta^{pa}Y_e^{*td}Y_e^{bc}(Y_e Y_e^\dagger)^{sr} + \frac{1}{2}\delta^{tb}Y_e^{*ad}Y_e^{pc}(Y_e Y_e^\dagger)^{sr} + \frac{3}{4}T_2\delta^{pa}\delta^{rb}Y_e^{*td}Y_e^{sc} + \frac{3}{4}T_2\delta^{sa}\delta^{tb}Y_e^{*rd}Y_e^{pc} + \frac{3}{4}\delta^{sa}\delta^{tb}Y_e^{pc}(Y_e^\dagger Y_e Y_e^\dagger)^{rd} \\
& + \frac{3}{4}\delta^{pa}\delta^{rb}Y_e^{sc}(Y_e^\dagger Y_e Y_e^\dagger)^{td} + \frac{3}{4}\delta^{sa}\delta^{tb}Y_e^{*rd}(Y_e Y_e^\dagger Y_e)^{pc} + \frac{3}{4}\delta^{pa}\delta^{rb}Y_e^{*td}(Y_e Y_e^\dagger Y_e)^{sc} + \frac{7}{8}\delta^{tb}Y_e^{*rd}Y_e^{sc}(Y_e Y_e^\dagger)^{pa} + \frac{7}{8}\delta^{rb}Y_e^{*td}Y_e^{pc}(Y_e Y_e^\dagger)^{sa} \\
& + \frac{7}{8}\delta^{sa}Y_e^{*td}Y_e^{pc}(Y_e Y_e^\dagger)^{br} + \frac{7}{8}\delta^{pa}Y_e^{*rd}Y_e^{sc}(Y_e Y_e^\dagger)^{bt} + g_L^2 \left( \frac{1}{9}\delta^{pa}\delta^{rs}Y_e^{*td}Y_e^{bc} + \frac{1}{9}\delta^{pt}\delta^{rb}Y_e^{*ad}Y_e^{sc} + \frac{1}{9}\delta^{pt}\delta^{sa}Y_e^{*rd}Y_e^{bc} + \frac{1}{9}\delta^{rs}\delta^{tb}Y_e^{*ad}Y_e^{pc} \right. \\
& - \frac{1}{18}\delta^{pa}\delta^{st}Y_e^{*rd}Y_e^{bc} - \frac{1}{18}\delta^{rb}\delta^{st}Y_e^{*ad}Y_e^{pc} - \frac{1}{18}\delta^{pr}\delta^{sa}Y_e^{*td}Y_e^{bc} - \frac{1}{18}\delta^{pr}\delta^{tb}Y_e^{*ad}Y_e^{sc} - \frac{5}{4}\delta^{rb}\delta^{sa}Y_e^{*td}Y_e^{pc} - \frac{5}{4}\delta^{pa}\delta^{tb}Y_e^{*rd}Y_e^{sc} - \frac{23}{16}\delta^{pa}\delta^{rb}Y_e^{*td}Y_e^{sc} \\
& - \frac{23}{16}\delta^{sa}\delta^{tb}Y_e^{*rd}Y_e^{pc} \left. \right) + g_Y^2 g_L^2 \left( \frac{25}{108}\delta^{pa}\delta^{rb}\delta^{st}\delta^{cd} + \frac{25}{108}\delta^{pr}\delta^{sa}\delta^{tb}\delta^{cd} - \frac{25}{54}\delta^{pt}\delta^{rb}\delta^{sa}\delta^{cd} - \frac{25}{54}\delta^{pa}\delta^{rs}\delta^{tb}\delta^{cd} \right) - \frac{1}{4}\delta^{sa}\delta^{tb}(Y_e^\dagger Y_e)^{dc}(Y_e Y_e^\dagger)^{pr} \\
& - \frac{1}{4}\delta^{pa}\delta^{rb}(Y_e^\dagger Y_e)^{dc}(Y_e Y_e^\dagger)^{st} - g_Y^4 \left( \frac{277}{108}\delta^{pa}\delta^{rb}\delta^{st}\delta^{cd} + \frac{277}{108}\delta^{pr}\delta^{sa}\delta^{tb}\delta^{cd} \right) - g_Y^2 \left( \frac{5}{18}\delta^{pa}\delta^{st}Y_e^{*rd}Y_e^{bc} + \frac{5}{18}\delta^{rb}\delta^{st}Y_e^{*ad}Y_e^{pc} + \frac{5}{18}\delta^{pr}\delta^{sa}Y_e^{*td}Y_e^{bc} \right. \\
& + \frac{5}{18}\delta^{pr}\delta^{tb}Y_e^{*ad}Y_e^{sc} + \frac{13}{16}\delta^{pa}\delta^{rb}Y_e^{*td}Y_e^{sc} + \frac{13}{16}\delta^{sa}\delta^{tb}Y_e^{*rd}Y_e^{pc} + \frac{5}{6}\delta^{pa}\delta^{rb}\delta^{st}(Y_e^\dagger Y_e)^{dc} + \frac{5}{6}\delta^{pr}\delta^{sa}\delta^{tb}(Y_e^\dagger Y_e)^{dc} \left. \right) \left\{ C_{le}^{abcd} + \left\{ \frac{3}{4}\delta^{sa}\delta^{tb}(Y_u^\dagger Y_u)^{dc}(Y_e Y_e^\dagger)^{pr} \right. \right. \\
& + \frac{3}{4}\delta^{pa}\delta^{rb}(Y_u^\dagger Y_u)^{dc}(Y_e Y_e^\dagger)^{st} + g_Y^2 g_L^2 \left( \frac{25}{27}\delta^{pt}\delta^{rb}\delta^{sa}\delta^{cd} + \frac{25}{27}\delta^{pa}\delta^{rs}\delta^{tb}\delta^{cd} - \frac{25}{54}\delta^{pa}\delta^{rb}\delta^{st}\delta^{cd} - \frac{25}{54}\delta^{pr}\delta^{sa}\delta^{tb}\delta^{cd} \right) + g_Y^2 \left( \frac{3}{2}\delta^{pa}\delta^{rb}\delta^{st}(Y_u^\dagger Y_u)^{dc} \right. \\
& + \frac{3}{2}\delta^{pr}\delta^{sa}\delta^{tb}(Y_u^\dagger Y_u)^{dc} \left. \right) - g_Y^2 g_s^2 \left( \frac{8}{3}\delta^{pa}\delta^{rb}\delta^{st}\delta^{cd} + \frac{8}{3}\delta^{pr}\delta^{sa}\delta^{tb}\delta^{cd} \right) - g_Y^4 \left( \frac{263}{54}\delta^{pa}\delta^{rb}\delta^{st}\delta^{cd} + \frac{263}{54}\delta^{pr}\delta^{sa}\delta^{tb}\delta^{cd} \right) \left\{ C_{lu}^{abcd} + \left\{ g_Y^2 g_L^2 \left( \frac{25}{108}\delta^{pa}\delta^{rb}\delta^{st}\delta^{cd} \right. \right. \right. \\
& + \frac{25}{108}\delta^{pr}\delta^{sa}\delta^{tb}\delta^{cd} - \frac{25}{54}\delta^{pt}\delta^{rb}\delta^{sa}\delta^{cd} - \frac{25}{54}\delta^{pa}\delta^{rs}\delta^{tb}\delta^{cd} \left. \right) + g_Y^2 g_s^2 \left( \frac{4}{3}\delta^{pa}\delta^{rb}\delta^{st}\delta^{cd} + \frac{4}{3}\delta^{pr}\delta^{sa}\delta^{tb}\delta^{cd} \right) - \frac{3}{4}\delta^{sa}\delta^{tb}(Y_d^\dagger Y_d)^{dc}(Y_e Y_e^\dagger)^{pr} \\
& - \frac{3}{4}\delta^{pa}\delta^{rb}(Y_d^\dagger Y_d)^{dc}(Y_e Y_e^\dagger)^{st} - g_Y^4 \left( \frac{133}{108}\delta^{pa}\delta^{rb}\delta^{st}\delta^{cd} + \frac{133}{108}\delta^{pr}\delta^{sa}\delta^{tb}\delta^{cd} \right) - g_Y^2 \left( \frac{1}{2}\delta^{pa}\delta^{rb}\delta^{st}(Y_d^\dagger Y_d)^{dc} + \frac{1}{2}\delta^{pr}\delta^{sa}\delta^{tb}(Y_d^\dagger Y_d)^{dc} \right) \left. \right\} C_{ld}^{abcd} \\
& + \left\{ \frac{4}{9}\delta^{pr}\delta^{st}\delta^{ab}\delta^{cd}g_Y^4 + Y_e^{*rb}Y_e^{*td}Y_e^{pa}Y_e^{sc} - g_Y^2 \left( \frac{2}{3}\delta^{pr}\delta^{ad}Y_e^{*tb}Y_e^{sc} + \frac{2}{3}\delta^{st}\delta^{ad}Y_e^{*rb}Y_e^{pc} \right) \right\} C_{ee}^{abcd} + \frac{16}{27}\delta^{pr}\delta^{st}\delta^{ad}\delta^{bc}g_Y^4 C_{uu}^{abcd} + \frac{4}{27}\delta^{pr}\delta^{st}\delta^{ad}\delta^{bc}g_Y^4 C_{dd}^{abcd} \\
& + \left\{ g_Y^2 \left( \frac{5}{12}\delta^{pa}\delta^{st}Y_e^{*rb}Y_d^{dc} + \frac{5}{12}\delta^{pr}\delta^{sa}Y_e^{*tb}Y_d^{dc} \right) + g_L^2 \left( \frac{1}{12}\delta^{pa}\delta^{st}Y_e^{*rb}Y_d^{dc} + \frac{1}{12}\delta^{pr}\delta^{sa}Y_e^{*tb}Y_d^{dc} - \frac{1}{6}\delta^{pa}\delta^{rs}Y_e^{*tb}Y_d^{dc} - \frac{1}{6}\delta^{pt}\delta^{sa}Y_e^{*rb}Y_d^{dc} \right) \right. \\
& - \frac{9}{8}\delta^{sa}Y_e^{*rb}Y_d^{dc}(Y_e Y_e^\dagger)^{pt} - \frac{9}{8}\delta^{pa}Y_e^{*tb}Y_d^{dc}(Y_e Y_e^\dagger)^{sr} \left. \right\} C_{ledq}^{abcd} + C_{ledq}^{*abcd} \left\{ g_Y^2 \left( \frac{5}{12}\delta^{ra}\delta^{st}Y_d^{*dc}Y_e^{pb} + \frac{5}{12}\delta^{pr}\delta^{ta}Y_d^{*dc}Y_e^{sb} \right) + g_L^2 \left( \frac{1}{12}\delta^{ra}\delta^{st}Y_d^{*dc}Y_e^{pb} \right. \right.
\end{aligned}$$

$$\begin{aligned}
& + \frac{1}{12} \delta^{pr} \delta^{ta} Y_d^{*dc} Y_e^{sb} - \frac{1}{6} \delta^{pt} \delta^{ra} Y_d^{*dc} Y_e^{sb} - \frac{1}{6} \delta^{rs} \delta^{ta} Y_d^{*dc} Y_e^{pb} \Big) - \frac{9}{8} \delta^{ra} Y_d^{*dc} Y_e^{sb} (Y_e Y_e^\dagger)^{pt} - \frac{9}{8} \delta^{ta} Y_d^{*dc} Y_e^{pb} (Y_e Y_e^\dagger)^{sr} \Big\} + \left\{ g_L^2 \left( \frac{1}{6} \delta^{pa} \delta^{rs} Y_e^{*tb} Y_u^{*cd} \right. \right. \\
& + \frac{1}{6} \delta^{pt} \delta^{sa} Y_e^{*rb} Y_u^{*cd} - \frac{1}{12} \delta^{pa} \delta^{st} Y_e^{*rb} Y_u^{*cd} - \frac{1}{12} \delta^{pr} \delta^{sa} Y_e^{*tb} Y_u^{*cd} \Big) + \frac{9}{8} \delta^{sa} Y_e^{*rb} Y_u^{*cd} (Y_e Y_e^\dagger)^{pt} + \frac{9}{8} \delta^{pa} Y_e^{*tb} Y_u^{*cd} (Y_e Y_e^\dagger)^{sr} - g_Y^2 \left( \frac{5}{12} \delta^{pa} \delta^{st} Y_e^{*rb} Y_u^{*cd} \right. \\
& + \left. \left. \frac{5}{12} \delta^{pr} \delta^{sa} Y_e^{*tb} Y_u^{*cd} \right) \right\} C_{\ell equ}^{abcd} + C_{\ell equ}^{*abcd} \left\{ g_L^2 \left( \frac{1}{6} \delta^{pt} \delta^{ra} Y_e^{sb} Y_u^{cd} + \frac{1}{6} \delta^{rs} \delta^{ta} Y_e^{pb} Y_u^{cd} - \frac{1}{12} \delta^{ra} \delta^{st} Y_e^{pb} Y_u^{cd} - \frac{1}{12} \delta^{pr} \delta^{ta} Y_e^{sb} Y_u^{cd} \right) + \frac{9}{8} \delta^{ra} Y_e^{sb} Y_u^{cd} (Y_e Y_e^\dagger)^{pt} \right. \\
& + \frac{9}{8} \delta^{ta} Y_e^{pb} Y_u^{cd} (Y_e Y_e^\dagger)^{sr} - g_Y^2 \left( \frac{5}{12} \delta^{ra} \delta^{st} Y_e^{pb} Y_u^{cd} + \frac{5}{12} \delta^{pr} \delta^{ta} Y_e^{sb} Y_u^{cd} \right) \Big\} + \left\{ g_Y^2 \left( \frac{7}{48} \delta^{pa} \delta^{st} Y_e^{*rd} Y_u^{*cb} + \frac{7}{48} \delta^{pr} \delta^{sa} Y_e^{*td} Y_u^{*cb} \right) + g_L^2 \left( \frac{1}{24} \delta^{pa} \delta^{rs} Y_e^{*td} Y_u^{*cb} \right. \right. \\
& + \frac{1}{24} \delta^{pt} \delta^{sa} Y_e^{*rd} Y_u^{*cb} - \frac{1}{48} \delta^{pa} \delta^{st} Y_e^{*rd} Y_u^{*cb} - \frac{1}{48} \delta^{pr} \delta^{sa} Y_e^{*td} Y_u^{*cb} \Big) - \frac{9}{16} \delta^{sa} Y_e^{*rd} Y_u^{*cb} (Y_e Y_e^\dagger)^{pt} - \frac{9}{16} \delta^{pa} Y_e^{*td} Y_u^{*cb} (Y_e Y_e^\dagger)^{sr} \Big\} C_{\ell uqe}^{abcd} \\
& + C_{\ell uqe}^{*abcd} \left\{ g_Y^2 \left( \frac{7}{48} \delta^{ra} \delta^{st} Y_e^{pd} Y_u^{cb} + \frac{7}{48} \delta^{pr} \delta^{ta} Y_e^{sd} Y_u^{cb} \right) + g_L^2 \left( \frac{1}{24} \delta^{pt} \delta^{ra} Y_e^{sd} Y_u^{cb} + \frac{1}{24} \delta^{rs} \delta^{ta} Y_e^{pd} Y_u^{cb} - \frac{1}{48} \delta^{ra} \delta^{st} Y_e^{pd} Y_u^{cb} - \frac{1}{48} \delta^{pr} \delta^{ta} Y_e^{sd} Y_u^{cb} \right) \right. \\
& - \frac{9}{16} \delta^{ra} Y_e^{sd} Y_u^{cb} (Y_e Y_e^\dagger)^{pt} - \frac{9}{16} \delta^{ta} Y_e^{pd} Y_u^{cb} (Y_e Y_e^\dagger)^{sr} \Big\} + \left\{ \frac{1}{2} \delta^{sa} \delta^{tb} (Y_e Y_e^\dagger)^{pr} (Y_e Y_e^\dagger)^{dc} + \frac{1}{2} \delta^{pa} \delta^{rb} (Y_e Y_e^\dagger)^{st} (Y_e Y_e^\dagger)^{dc} + g_Y^2 g_L^2 \left( \frac{26}{27} \delta^{pa} \delta^{rb} \delta^{st} \delta^{cd} \right. \right. \\
& + \frac{26}{27} \delta^{pr} \delta^{sa} \delta^{tb} \delta^{cd} + \frac{115}{27} \delta^{pt} \delta^{rd} \delta^{sa} \delta^{bc} + \frac{115}{27} \delta^{pa} \delta^{rs} \delta^{td} \delta^{bc} - \frac{2}{9} \delta^{pr} \delta^{st} \delta^{ad} \delta^{bc} - \frac{25}{27} \delta^{pt} \delta^{rb} \delta^{sa} \delta^{cd} - \frac{25}{27} \delta^{pa} \delta^{rs} \delta^{tb} \delta^{cd} - \frac{44}{27} \delta^{pa} \delta^{rd} \delta^{st} \delta^{bc} \\
& - \frac{44}{27} \delta^{pr} \delta^{sa} \delta^{td} \delta^{bc} - \frac{15}{4} \delta^{pa} \delta^{rb} \delta^{sc} \delta^{td} - \frac{39}{2} \delta^{pa} \delta^{rd} \delta^{sc} \delta^{tb} \Big) + g_Y^4 \left( \frac{2}{9} \delta^{pr} \delta^{st} \delta^{ad} \delta^{bc} + \frac{43}{54} \delta^{pa} \delta^{rd} \delta^{st} \delta^{bc} + \frac{43}{54} \delta^{pr} \delta^{sa} \delta^{td} \delta^{bc} + \frac{37}{27} \delta^{pa} \delta^{rb} \delta^{st} \delta^{cd} \right. \\
& + \frac{37}{27} \delta^{pr} \delta^{sa} \delta^{tb} \delta^{cd} - \frac{101}{24} \delta^{pa} \delta^{rb} \delta^{sc} \delta^{td} \Big) + g_L^4 \left( \frac{17}{3} \delta^{pa} \delta^{rb} \delta^{st} \delta^{cd} + \frac{17}{3} \delta^{pr} \delta^{sa} \delta^{tb} \delta^{cd} + \frac{73}{9} \delta^{pt} \delta^{rd} \delta^{sa} \delta^{bc} + \frac{73}{9} \delta^{pa} \delta^{rs} \delta^{td} \delta^{bc} + \frac{49}{3} \delta^{pa} \delta^{rd} \delta^{sc} \delta^{tb} \right. \\
& - \frac{1}{18} \delta^{pa} \delta^{rd} \delta^{st} \delta^{bc} - \frac{1}{18} \delta^{pr} \delta^{sa} \delta^{td} \delta^{bc} - \frac{7}{3} \delta^{pt} \delta^{rb} \delta^{sa} \delta^{cd} - \frac{7}{3} \delta^{pa} \delta^{rs} \delta^{tb} \delta^{cd} - \frac{385}{24} \delta^{pa} \delta^{rb} \delta^{sc} \delta^{td} \Big) + g_L^2 \left( \frac{2}{3} \delta^{pa} \delta^{rd} \delta^{st} (Y_e Y_e^\dagger)^{bc} + \frac{2}{3} \delta^{pr} \delta^{sa} \delta^{td} (Y_e Y_e^\dagger)^{bc} \right. \\
& + \frac{33}{16} \delta^{rd} \delta^{sa} \delta^{tb} (Y_e Y_e^\dagger)^{pc} + \frac{33}{16} \delta^{pa} \delta^{rb} \delta^{td} (Y_e Y_e^\dagger)^{sc} + \frac{33}{16} \delta^{pa} \delta^{sc} \delta^{td} (Y_e Y_e^\dagger)^{br} + \frac{33}{16} \delta^{pa} \delta^{rb} \delta^{sc} (Y_e Y_e^\dagger)^{dt} - \frac{4}{3} \delta^{pt} \delta^{rd} \delta^{sa} (Y_e Y_e^\dagger)^{bc} - \frac{4}{3} \delta^{pa} \delta^{rs} \delta^{td} (Y_e Y_e^\dagger)^{bc} \Big) \\
& + \frac{3}{2} \delta^{rd} \delta^{sa} (Y_e Y_e^\dagger)^{pt} (Y_e Y_e^\dagger)^{bc} + \frac{3}{2} \delta^{pa} \delta^{td} (Y_e Y_e^\dagger)^{sr} (Y_e Y_e^\dagger)^{bc} + 2 \delta^{rd} \delta^{tb} (Y_e Y_e^\dagger)^{pa} (Y_e Y_e^\dagger)^{sc} + 2 \delta^{pa} \delta^{sc} (Y_e Y_e^\dagger)^{bt} (Y_e Y_e^\dagger)^{dr} - \frac{1}{4} \delta^{rd} \delta^{sa} \delta^{tb} (Y_e Y_e^\dagger Y_e Y_e^\dagger)^{pc} \\
& - \frac{1}{4} \delta^{pa} \delta^{rb} \delta^{td} (Y_e Y_e^\dagger Y_e Y_e^\dagger)^{sc} - \frac{1}{4} \delta^{pa} \delta^{sc} \delta^{td} (Y_e Y_e^\dagger Y_e Y_e^\dagger)^{br} - \frac{1}{4} \delta^{pa} \delta^{rb} \delta^{sc} (Y_e Y_e^\dagger Y_e Y_e^\dagger)^{dt} - \frac{3}{4} T_2 \delta^{rd} \delta^{sa} \delta^{tb} (Y_e Y_e^\dagger)^{pc} - \frac{3}{4} T_2 \delta^{pa} \delta^{rb} \delta^{td} (Y_e Y_e^\dagger)^{sc} \\
& - \frac{3}{4} T_2 \delta^{pa} \delta^{sc} \delta^{td} (Y_e Y_e^\dagger)^{br} - \frac{3}{4} \delta^{sa} \delta^{td} (Y_e Y_e^\dagger)^{pc} (Y_e Y_e^\dagger)^{br} - \frac{3}{4} \delta^{pa} \delta^{rd} (Y_e Y_e^\dagger)^{sc} (Y_e Y_e^\dagger)^{bt} - \frac{3}{4} T_2 \delta^{pa} \delta^{rb} \delta^{sc} (Y_e Y_e^\dagger)^{dt} - g_Y^2 \left( \delta^{pa} \delta^{rd} \delta^{st} (Y_e Y_e^\dagger)^{bc} \right. \\
& + \delta^{pr} \delta^{sa} \delta^{td} (Y_e Y_e^\dagger)^{bc} + \frac{4}{3} \delta^{pa} \delta^{rb} \delta^{st} (Y_e Y_e^\dagger)^{dc} + \frac{4}{3} \delta^{pr} \delta^{sa} \delta^{tb} (Y_e Y_e^\dagger)^{dc} + \frac{41}{16} \delta^{rd} \delta^{sa} \delta^{tb} (Y_e Y_e^\dagger)^{pc} + \frac{41}{16} \delta^{pa} \delta^{rb} \delta^{td} (Y_e Y_e^\dagger)^{sc} + \frac{41}{16} \delta^{pa} \delta^{sc} \delta^{td} (Y_e Y_e^\dagger)^{br} \\
& + \left. \left. \frac{41}{16} \delta^{pa} \delta^{rb} \delta^{sc} (Y_e Y_e^\dagger)^{dt} \right) - \frac{5}{2} \delta^{sa} \delta^{tb} (Y_e Y_e^\dagger)^{pc} (Y_e Y_e^\dagger)^{dr} - \frac{5}{2} \delta^{pa} \delta^{rb} (Y_e Y_e^\dagger)^{sc} (Y_e Y_e^\dagger)^{dt} \right\} C_{\ell \ell}^{abcd} + \left\{ \frac{2}{27} \delta^{pr} \delta^{st} \delta^{ad} \delta^{bc} g_Y^4 + g_L^4 \left( \frac{4}{3} \delta^{pt} \delta^{rs} \delta^{ad} \delta^{bc} \right. \right.
\end{aligned}$$

$$\begin{aligned}
& -\frac{2}{3}\delta^{pr}\delta^{st}\delta^{ad}\delta^{bc}\Big)\Big\}C_{qq}^{(\parallel)abcd} + \frac{4}{27}\delta^{pr}\delta^{st}\delta^{ad}\delta^{bc}g_Y^4C_{qq}^{(\times)abcd} + \left\{\frac{3}{4}\delta^{sa}\delta^{tb}(Y_dY_d^\dagger)^{dc}(Y_eY_e^\dagger)^{pr} + \frac{3}{4}\delta^{pa}\delta^{rb}(Y_dY_d^\dagger)^{dc}(Y_eY_e^\dagger)^{st} + g_Y^2g_L^2\left(\frac{25}{54}\delta^{pt}\delta^{rb}\delta^{sa}\delta^{cd}\right.\right. \\
& + \frac{25}{54}\delta^{pa}\delta^{rs}\delta^{tb}\delta^{cd} - \frac{53}{54}\delta^{pa}\delta^{rb}\delta^{st}\delta^{cd} - \frac{53}{54}\delta^{pr}\delta^{sa}\delta^{tb}\delta^{cd}\Big) + g_Y^4\left(\frac{23}{54}\delta^{pa}\delta^{rb}\delta^{st}\delta^{cd} + \frac{23}{54}\delta^{pr}\delta^{sa}\delta^{tb}\delta^{cd}\right) + g_L^4\left(7\delta^{pa}\delta^{rb}\delta^{st}\delta^{cd} + 7\delta^{pr}\delta^{sa}\delta^{tb}\delta^{cd}\right. \\
& - \frac{1}{2}\delta^{pt}\delta^{rb}\delta^{sa}\delta^{cd} - \frac{1}{2}\delta^{pa}\delta^{rs}\delta^{tb}\delta^{cd}\Big) + g_Y^2\left(\delta^{pa}\delta^{rb}\delta^{st}(Y_uY_u^\dagger)^{dc} + \delta^{pr}\delta^{sa}\delta^{tb}(Y_uY_u^\dagger)^{dc}\right) - \frac{3}{4}\delta^{sa}\delta^{tb}(Y_eY_e^\dagger)^{pr}(Y_uY_u^\dagger)^{dc} - \frac{3}{4}\delta^{pa}\delta^{rb}(Y_eY_e^\dagger)^{st}(Y_uY_u^\dagger)^{dc} \\
& - g_Y^2g_s^2\left(\frac{4}{3}\delta^{pa}\delta^{rb}\delta^{st}\delta^{cd} + \frac{4}{3}\delta^{pr}\delta^{sa}\delta^{tb}\delta^{cd}\right)\Big\}C_{\ell q}^{(\parallel)abcd} + \left\{\frac{3}{4}\delta^{rb}\delta^{sa}(Y_dY_d^\dagger)^{dc}(Y_eY_e^\dagger)^{pt} + \frac{3}{4}\delta^{pa}\delta^{tb}(Y_dY_d^\dagger)^{dc}(Y_eY_e^\dagger)^{sr} + \frac{3}{4}\delta^{rb}\delta^{sa}(Y_eY_e^\dagger)^{pt}(Y_uY_u^\dagger)^{dc}\right. \\
& + \frac{3}{4}\delta^{pa}\delta^{tb}(Y_eY_e^\dagger)^{sr}(Y_uY_u^\dagger)^{dc} + g_s^2g_L^2\left(4\delta^{pt}\delta^{rb}\delta^{sa}\delta^{cd} + 4\delta^{pa}\delta^{rs}\delta^{tb}\delta^{cd} - 2\delta^{pa}\delta^{rb}\delta^{st}\delta^{cd} - 2\delta^{pr}\delta^{sa}\delta^{tb}\delta^{cd}\right) + g_Y^4\left(\frac{23}{108}\delta^{pa}\delta^{rb}\delta^{st}\delta^{cd}\right. \\
& + \frac{23}{108}\delta^{pr}\delta^{sa}\delta^{tb}\delta^{cd}\Big) + g_L^4\left(\frac{1}{3}\delta^{pr}\delta^{st}\delta^{ab}\delta^{cd} + \frac{5}{12}\delta^{pa}\delta^{rb}\delta^{st}\delta^{cd} + \frac{5}{12}\delta^{pr}\delta^{sa}\delta^{tb}\delta^{cd} + \frac{20}{3}\delta^{pt}\delta^{rb}\delta^{sa}\delta^{cd} + \frac{20}{3}\delta^{pa}\delta^{rs}\delta^{tb}\delta^{cd} - \frac{2}{3}\delta^{pt}\delta^{rs}\delta^{ab}\delta^{cd}\right) \\
& + g_Y^2\left(\frac{1}{2}\delta^{pa}\delta^{rb}\delta^{st}(Y_uY_u^\dagger)^{dc} + \frac{1}{2}\delta^{pr}\delta^{sa}\delta^{tb}(Y_uY_u^\dagger)^{dc}\right) + g_L^2\left(\frac{1}{2}\delta^{pa}\delta^{rb}\delta^{st}(Y_dY_d^\dagger)^{dc} + \frac{1}{2}\delta^{pr}\delta^{sa}\delta^{tb}(Y_dY_d^\dagger)^{dc} + \frac{1}{2}\delta^{pa}\delta^{rb}\delta^{st}(Y_uY_u^\dagger)^{dc} + \frac{1}{2}\delta^{pr}\delta^{sa}\delta^{tb}(Y_uY_u^\dagger)^{dc}\right. \\
& - \delta^{pt}\delta^{rb}\delta^{sa}(Y_dY_d^\dagger)^{dc} - \delta^{pa}\delta^{rs}\delta^{tb}(Y_dY_d^\dagger)^{dc} - \delta^{pt}\delta^{rb}\delta^{sa}(Y_uY_u^\dagger)^{dc} - \delta^{pa}\delta^{rs}\delta^{tb}(Y_uY_u^\dagger)^{dc}\Big) - \frac{3}{4}\delta^{sa}\delta^{tb}(Y_eY_e^\dagger)^{pr}(Y_uY_u^\dagger)^{dc} - \frac{3}{4}\delta^{pa}\delta^{rb}(Y_eY_e^\dagger)^{st}(Y_uY_u^\dagger)^{dc} \\
& - g_Y^2g_s^2\left(\frac{2}{3}\delta^{pa}\delta^{rb}\delta^{st}\delta^{cd} + \frac{2}{3}\delta^{pr}\delta^{sa}\delta^{tb}\delta^{cd}\right) - g_Y^2g_L^2\left(\frac{1}{3}\delta^{pr}\delta^{st}\delta^{ab}\delta^{cd} + \frac{23}{27}\delta^{pt}\delta^{rb}\delta^{sa}\delta^{cd} + \frac{23}{27}\delta^{pa}\delta^{rs}\delta^{tb}\delta^{cd} + \frac{29}{27}\delta^{pa}\delta^{rb}\delta^{st}\delta^{cd}\right. \\
& \left. + \frac{29}{27}\delta^{pr}\delta^{sa}\delta^{tb}\delta^{cd}\right)\Big\}C_{\ell q}^{(\times)abcd}, \tag{13.2}
\end{aligned}$$

### 13.2 $C_{qq}^{(\parallel)}$

$$\begin{aligned}
\beta_{C_{qq}^{(\parallel)prst}}^{(1)} & = \left\{\frac{1}{18}g_Y^2\left(\delta^{pa}\delta^{rb}\delta^{st} + \delta^{pr}\delta^{sa}\delta^{tb}\right) + \frac{1}{2}\left(\delta^{sa}\delta^{tb}(Y_uY_u^\dagger)^{pr} + \delta^{pa}\delta^{rb}(Y_uY_u^\dagger)^{st} - \delta^{sa}\delta^{tb}(Y_dY_d^\dagger)^{pr} - \delta^{pa}\delta^{rb}(Y_dY_d^\dagger)^{st}\right)\right\}C_{Hq}^{(\parallel)ab} + \left\{\frac{1}{36}g_Y^2\left(\delta^{pa}\delta^{rb}\delta^{st}\right.\right. \\
& + \delta^{pr}\delta^{sa}\delta^{tb}\Big) + \frac{1}{2}\left(\delta^{sa}\delta^{tb}(Y_uY_u^\dagger)^{pr} + \delta^{pa}\delta^{rb}(Y_uY_u^\dagger)^{st}\right) - \frac{1}{12}g_L^2\left(\delta^{pa}\delta^{rb}\delta^{st} + \delta^{pr}\delta^{sa}\delta^{tb}\right)\Big\}C_{Hq}^{(\times)ab} - \frac{1}{9}g_Y^2\left\{\delta^{pa}\delta^{rb}\delta^{st}\delta^{cd} + \delta^{pr}\delta^{sa}\delta^{tb}\delta^{cd}\right\}C_{qe}^{abcd} \\
& + \left\{\frac{2}{9}g_Y^2\left(\delta^{pa}\delta^{rb}\delta^{st}\delta^{cd} + \delta^{pr}\delta^{sa}\delta^{tb}\delta^{cd}\right) + \frac{1}{2}\left(-\delta^{pa}\delta^{rb}Y_u^{*td}Y_u^{sc} - \delta^{sa}\delta^{tb}Y_u^{*rd}Y_u^{pc}\right)\right\}C_{qu}^{(\parallel)abcd} + \left\{\frac{2}{27}g_Y^2\left(\delta^{pa}\delta^{rb}\delta^{st}\delta^{cd} + \delta^{pr}\delta^{sa}\delta^{tb}\delta^{cd}\right) - \frac{1}{9}g_s^2\left(\delta^{pa}\delta^{rb}\delta^{st}\delta^{cd}\right.\right. \\
& + \delta^{pr}\delta^{sa}\delta^{tb}\delta^{cd}\Big)\Big\}C_{qu}^{(\times)abcd} + \left\{\frac{1}{2}\left(-\delta^{pa}\delta^{rb}Y_d^{*td}Y_d^{sc} - \delta^{sa}\delta^{tb}Y_d^{*rd}Y_d^{pc}\right) - \frac{1}{9}g_Y^2\left(\delta^{pa}\delta^{rb}\delta^{st}\delta^{cd} + \delta^{pr}\delta^{sa}\delta^{tb}\delta^{cd}\right)\right\}C_{qd}^{(\parallel)abcd} + \left\{-\frac{1}{27}g_Y^2\left(\delta^{pa}\delta^{rb}\delta^{st}\delta^{cd}\right.\right. \\
& + \delta^{pr}\delta^{sa}\delta^{tb}\delta^{cd}\Big) - \frac{1}{9}g_s^2\left(\delta^{pa}\delta^{rb}\delta^{st}\delta^{cd} + \delta^{pr}\delta^{sa}\delta^{tb}\delta^{cd}\right)\Big\}C_{qd}^{(\times)abcd} - \frac{1}{4}\left\{\delta^{pc}\delta^{sa}Y_d^{*rd}Y_u^{*tb} + \delta^{pa}\delta^{sc}Y_d^{*td}Y_u^{*rb}\right\}C_{quqd}^{(\parallel)abcd} - \frac{1}{4}\left(C_{quqd}^{(\parallel)*}\right)^{abcd}\left\{\delta^{rc}\delta^{ta}Y_d^{pd}Y_u^{sb}\right. \\
& \left. + \delta^{rc}\delta^{ta}Y_d^{pd}Y_u^{sb}\right\}
\end{aligned}$$



$$\begin{aligned}
& + \delta^{ra} \delta^{tc} Y_d^{sd} Y_u^{pb} \Bigg\} + \frac{1}{4} \left\{ \delta^{pc} \delta^{sa} Y_d^{*td} Y_u^{*rb} + \delta^{pa} \delta^{sc} Y_d^{*rd} Y_u^{*tb} \right\} C_{quqd}^{(\times)abcd} + \frac{1}{4} \left( C_{quqd}^{(\times)*} \right)^{abcd} \left\{ \delta^{rc} \delta^{ta} Y_d^{sd} Y_u^{pb} + \delta^{ra} \delta^{tc} Y_d^{pd} Y_u^{sb} \right\} + \left\{ \frac{1}{27} g_Y^2 \left( \delta^{pa} \delta^{rd} \delta^{st} \delta^{bc} \right. \right. \\
& + \delta^{pr} \delta^{sa} \delta^{td} \delta^{bc} + 6 \delta^{pa} \delta^{rb} \delta^{st} \delta^{cd} + 6 \delta^{pr} \delta^{sa} \delta^{tb} \delta^{cd} + 9 \delta^{pa} \delta^{rb} \delta^{sc} \delta^{td} \Big) + \frac{1}{2} \left( \delta^{rd} \delta^{sa} \delta^{tb} (Y_d Y_d^\dagger)^{pc} + \delta^{pa} \delta^{rb} \delta^{td} (Y_d Y_d^\dagger)^{sc} + \delta^{pa} \delta^{sc} \delta^{td} (Y_d Y_d^\dagger)^{br} \right. \\
& + \delta^{pa} \delta^{rb} \delta^{sc} (Y_d Y_d^\dagger)^{dt} + \delta^{rd} \delta^{sa} \delta^{tb} (Y_u Y_u^\dagger)^{pc} + \delta^{pa} \delta^{rb} \delta^{td} (Y_u Y_u^\dagger)^{sc} + \delta^{pa} \delta^{sc} \delta^{td} (Y_u Y_u^\dagger)^{br} + \delta^{pa} \delta^{rb} \delta^{sc} (Y_u Y_u^\dagger)^{dt} \Big) - \frac{2}{9} g_s^2 \left( \delta^{pa} \delta^{rd} \delta^{st} \delta^{bc} + \delta^{pr} \delta^{sa} \delta^{td} \delta^{bc} \right. \\
& + 9 \delta^{pa} \delta^{rb} \delta^{sc} \delta^{td} \Big) - \frac{1}{3} g_L^2 \left( \delta^{pa} \delta^{rd} \delta^{st} \delta^{bc} + \delta^{pr} \delta^{sa} \delta^{td} \delta^{bc} + 9 \delta^{pa} \delta^{rb} \delta^{sc} \delta^{td} \right) \Bigg\} C_{qq}^{(\parallel)abcd} + \left\{ \frac{1}{27} g_Y^2 \left( 2 \delta^{pa} \delta^{rd} \delta^{st} \delta^{bc} + 2 \delta^{pr} \delta^{sa} \delta^{td} \delta^{bc} + 3 \delta^{pa} \delta^{rb} \delta^{st} \delta^{cd} \right. \right. \\
& + 3 \delta^{pr} \delta^{sa} \delta^{tb} \delta^{cd} \Big) + \frac{2}{9} g_s^2 \left( 27 \delta^{pa} \delta^{rd} \delta^{sc} \delta^{tb} - 2 \delta^{pa} \delta^{rd} \delta^{st} \delta^{bc} - 2 \delta^{pr} \delta^{sa} \delta^{td} \delta^{bc} \right) + g_L^2 \left( 6 \delta^{pa} \delta^{rb} \delta^{sc} \delta^{td} - \delta^{pa} \delta^{rb} \delta^{st} \delta^{cd} - \delta^{pr} \delta^{sa} \delta^{tb} \delta^{cd} \right) \Bigg\} C_{qq}^{(\times)abcd} \\
& - \frac{1}{9} g_Y^2 \left\{ \delta^{pc} \delta^{rd} \delta^{st} \delta^{ab} + \delta^{pr} \delta^{sc} \delta^{td} \delta^{ab} \right\} C_{\ell q}^{(\parallel)abcd} + \left\{ -\frac{1}{18} g_Y^2 \left( \delta^{pc} \delta^{rd} \delta^{st} \delta^{ab} + \delta^{pr} \delta^{sc} \delta^{td} \delta^{ab} \right) - \frac{1}{6} g_L^2 \left( \delta^{pc} \delta^{rd} \delta^{st} \delta^{ab} + \delta^{pr} \delta^{sc} \delta^{td} \delta^{ab} \right) \right\} C_{\ell q}^{(\times)abcd}, \tag{13.3}
\end{aligned}$$

$$\begin{aligned}
\beta_{C_{qq}^{(\parallel)prst}}^{(2)} & = \left\{ \frac{1}{27} \delta^{pr} \delta^{st} g_Y^6 + g_Y^4 \left( \frac{1}{36} \delta^{st} (Y_u Y_u^\dagger)^{pr} + \frac{1}{36} \delta^{pr} (Y_u Y_u^\dagger)^{st} - \frac{5}{36} \delta^{st} (Y_d Y_d^\dagger)^{pr} - \frac{5}{36} \delta^{pr} (Y_d Y_d^\dagger)^{st} \right) \right\} C_{HB} + \left\{ g_L^4 \left( \frac{3}{4} \delta^{st} (Y_d Y_d^\dagger)^{pr} + \frac{3}{4} \delta^{pr} (Y_d Y_d^\dagger)^{st} \right. \right. \\
& + \frac{3}{4} \delta^{st} (Y_u Y_u^\dagger)^{pr} + \frac{3}{4} \delta^{pr} (Y_u Y_u^\dagger)^{st} \Big) - \frac{1}{3} \delta^{pr} \delta^{st} g_L^6 \Big\} C_{HW} + g_s^4 \left\{ \frac{1}{3} \delta^{st} (Y_d Y_d^\dagger)^{pr} + \frac{1}{3} \delta^{pr} (Y_d Y_d^\dagger)^{st} + \frac{1}{3} \delta^{st} (Y_u Y_u^\dagger)^{pr} + \frac{1}{3} \delta^{pr} (Y_u Y_u^\dagger)^{st} \right\} C_{HG} \\
& + \left\{ \frac{1}{36} \delta^{pr} \delta^{st} g_Y^4 g_L^2 + g_Y^2 g_L^2 \left( \frac{5}{24} \delta^{st} (Y_u Y_u^\dagger)^{pr} + \frac{5}{24} \delta^{pr} (Y_u Y_u^\dagger)^{st} - \frac{1}{12} \delta^{st} (Y_d Y_d^\dagger)^{pr} - \frac{1}{12} \delta^{pr} (Y_d Y_d^\dagger)^{st} \right) - \frac{1}{12} \delta^{pr} \delta^{st} g_Y^2 g_L^4 \right\} C_{HWB} + \left\{ g_s^2 g_L^6 \left( \frac{1}{6} \delta^{pr} \delta^{st} \right. \right. \\
& + 21 \delta^{pt} \delta^{rs} \Big) - \frac{1}{36} \delta^{pr} \delta^{st} g_Y^2 g_L^6 - g_L^6 \left( \frac{3}{4} \delta^{st} (Y_d Y_d^\dagger)^{pr} + \frac{3}{4} \delta^{pr} (Y_d Y_d^\dagger)^{st} + \frac{3}{4} \delta^{st} (Y_u Y_u^\dagger)^{pr} + \frac{3}{4} \delta^{pr} (Y_u Y_u^\dagger)^{st} \right) - \frac{95}{12} \delta^{pr} \delta^{st} g_L^8 \Big\} C_W + \left\{ \frac{97}{108} \delta^{pr} \delta^{st} g_Y^2 g_s^6 \right. \\
& + g_s^6 g_L^2 \left( \frac{63}{2} \delta^{pt} \delta^{rs} - \frac{97}{12} \delta^{pr} \delta^{st} \right) + g_s^6 \left( \frac{3}{4} \delta^{st} (Y_d Y_d^\dagger)^{pr} + \frac{3}{4} \delta^{pr} (Y_d Y_d^\dagger)^{st} + \frac{3}{4} \delta^{st} (Y_u Y_u^\dagger)^{pr} + \frac{3}{4} \delta^{pr} (Y_u Y_u^\dagger)^{st} \right) - \frac{331}{18} \delta^{pr} \delta^{st} g_s^8 \Big\} C_G - \frac{1}{18} \delta^{pr} \delta^{st} g_Y^4 Y_e^{*ab} C_{eB}^{ab} \\
& - \frac{1}{18} \delta^{pr} \delta^{st} g_Y^4 C_{eB}^{*ab} Y_e^{ab} - \frac{1}{12} \delta^{pr} \delta^{st} g_L^4 Y_e^{*ab} C_{eW}^{ab} - \frac{1}{12} \delta^{pr} \delta^{st} g_L^4 C_{eW}^{*ab} Y_e^{ab} + \left\{ g_Y^4 \left( \frac{5}{54} \delta^{pr} \delta^{st} Y_u^{*ab} - \frac{211}{648} \delta^{pa} \delta^{st} Y_u^{*rb} - \frac{211}{648} \delta^{pr} \delta^{sa} Y_u^{*tb} \right) \right. \\
& + g_Y^2 g_s^2 \left( \frac{1}{27} \delta^{pa} \delta^{st} Y_u^{*rb} + \frac{1}{27} \delta^{pr} \delta^{sa} Y_u^{*tb} \right) + g_Y^2 g_L^2 \left( \frac{7}{72} \delta^{pa} \delta^{st} Y_u^{*rb} + \frac{7}{72} \delta^{pr} \delta^{sa} Y_u^{*tb} \right) + g_Y^2 \left( \frac{1}{12} \delta^{st} Y_u^{*rb} (Y_d Y_d^\dagger)^{pa} + \frac{1}{12} \delta^{pr} Y_u^{*tb} (Y_d Y_d^\dagger)^{sa} \right. \\
& - \frac{1}{6} \delta^{st} Y_u^{*rb} (Y_u Y_u^\dagger)^{pa} - \frac{1}{6} \delta^{pr} Y_u^{*tb} (Y_u Y_u^\dagger)^{sa} - \frac{3}{4} \delta^{sa} Y_u^{*tb} (Y_d Y_d^\dagger)^{pr} - \frac{3}{4} \delta^{pa} Y_u^{*rb} (Y_d Y_d^\dagger)^{st} \Big) \Big\} C_{uB}^{ab} + C_{uB}^{*ab} \left\{ g_Y^4 \left( \frac{5}{54} \delta^{pr} \delta^{st} Y_u^{ab} - \frac{211}{648} \delta^{ra} \delta^{st} Y_u^{pb} \right. \right. \\
& - \frac{211}{648} \delta^{pr} \delta^{ta} Y_u^{sb} \Big) + g_Y^2 g_s^2 \left( \frac{1}{27} \delta^{ra} \delta^{st} Y_u^{pb} + \frac{1}{27} \delta^{pr} \delta^{ta} Y_u^{sb} \right) + g_Y^2 g_L^2 \left( \frac{7}{72} \delta^{ra} \delta^{st} Y_u^{pb} + \frac{7}{72} \delta^{pr} \delta^{ta} Y_u^{sb} \right) + g_Y^2 \left( \frac{1}{12} \delta^{st} Y_u^{pb} (Y_d Y_d^\dagger)^{ar} + \frac{1}{12} \delta^{pr} Y_u^{sb} (Y_d Y_d^\dagger)^{at} \right.
\end{aligned}$$

$$\begin{aligned}
& -\frac{1}{6}\delta^{st}Y_u^{pb}(Y_uY_u^\dagger)^{ar}-\frac{1}{6}\delta^{pr}Y_u^{sb}(Y_uY_u^\dagger)^{at}-\frac{3}{4}\delta^{ta}Y_u^{sb}(Y_dY_d^\dagger)^{pr}-\frac{3}{4}\delta^{ra}Y_u^{pb}(Y_dY_d^\dagger)^{st}\Bigg\}+\Bigg\{g_Y^2g_L^2\Big(\frac{7}{48}\delta^{pa}\delta^{st}Y_u^{*rb}+\frac{7}{48}\delta^{pr}\delta^{sa}Y_u^{*tb}\Big)+g_s^2g_L^2\Big(\frac{1}{2}\delta^{pa}\delta^{st}Y_u^{*rb}\\
& +\frac{1}{2}\delta^{pr}\delta^{sa}Y_u^{*tb}-\frac{3}{2}\delta^{pa}\delta^{rs}Y_u^{*tb}-\frac{3}{2}\delta^{pt}\delta^{sa}Y_u^{*rb}\Big)+g_L^2\Big(\frac{1}{8}\delta^{st}Y_u^{*rb}(Y_dY_d^\dagger)^{pa}+\frac{1}{8}\delta^{pr}Y_u^{*tb}(Y_dY_d^\dagger)^{sa}+\frac{9}{8}\delta^{sa}Y_u^{*tb}(Y_dY_d^\dagger)^{pr}+\frac{9}{8}\delta^{pa}Y_u^{*rb}(Y_dY_d^\dagger)^{st}\\
& +\frac{3}{2}\delta^{sa}Y_u^{*tb}(Y_uY_u^\dagger)^{pr}+\frac{3}{2}\delta^{pa}Y_u^{*rb}(Y_uY_u^\dagger)^{st}\Big)-g_L^4\Big(\frac{1}{16}\delta^{pa}\delta^{st}Y_u^{*rb}+\frac{1}{16}\delta^{pr}\delta^{sa}Y_u^{*tb}+\frac{1}{4}\delta^{pr}\delta^{st}Y_u^{*ab}\Big)\Bigg\}C_{uW}^{ab}+C_{uW}^{*ab}\Bigg\{g_Y^2g_L^2\Big(\frac{7}{48}\delta^{ra}\delta^{st}Y_u^{pb}\\
& +\frac{7}{48}\delta^{pr}\delta^{ta}Y_u^{sb}\Big)+g_s^2g_L^2\Big(\frac{1}{2}\delta^{ra}\delta^{st}Y_u^{pb}+\frac{1}{2}\delta^{pr}\delta^{ta}Y_u^{sb}-\frac{3}{2}\delta^{pt}\delta^{ra}Y_u^{sb}-\frac{3}{2}\delta^{rs}\delta^{ta}Y_u^{pb}\Big)+g_L^2\Big(\frac{1}{8}\delta^{st}Y_u^{pb}(Y_dY_d^\dagger)^{ar}+\frac{1}{8}\delta^{pr}Y_u^{sb}(Y_dY_d^\dagger)^{at}+\frac{9}{8}\delta^{ta}Y_u^{sb}(Y_dY_d^\dagger)^{pr}\\
& +\frac{9}{8}\delta^{ra}Y_u^{pb}(Y_dY_d^\dagger)^{st}+\frac{3}{2}\delta^{ta}Y_u^{sb}(Y_uY_u^\dagger)^{pr}+\frac{3}{2}\delta^{ra}Y_u^{pb}(Y_uY_u^\dagger)^{st}\Big)-g_L^4\Big(\frac{1}{16}\delta^{ra}\delta^{st}Y_u^{pb}+\frac{1}{16}\delta^{pr}\delta^{ta}Y_u^{sb}+\frac{1}{4}\delta^{pr}\delta^{st}Y_u^{ab}\Big)\Bigg\}+\Bigg\{g_s^2g_L^2\Big(\frac{1}{9}\delta^{pa}\delta^{st}Y_u^{*rb}\\
& +\frac{1}{9}\delta^{pr}\delta^{sa}Y_u^{*tb}\Big)+g_s^2\Big(\frac{1}{6}\delta^{st}Y_u^{*rb}(Y_uY_u^\dagger)^{pa}+\frac{1}{6}\delta^{pr}Y_u^{*tb}(Y_uY_u^\dagger)^{sa}+\frac{3}{2}\delta^{sa}Y_u^{*rb}(Y_dY_d^\dagger)^{pt}+\frac{3}{2}\delta^{pa}Y_u^{*tb}(Y_dY_d^\dagger)^{sr}+\frac{3}{2}\delta^{sa}Y_u^{*rb}(Y_uY_u^\dagger)^{pt}+\frac{3}{2}\delta^{pa}Y_u^{*tb}(Y_uY_u^\dagger)^{sr}\\
& -\frac{1}{12}\delta^{st}Y_u^{*rb}(Y_dY_d^\dagger)^{pa}-\frac{1}{12}\delta^{pr}Y_u^{*tb}(Y_dY_d^\dagger)^{sa}-\frac{3}{2}\delta^{sa}Y_u^{*tb}(Y_dY_d^\dagger)^{pr}-\frac{3}{2}\delta^{pa}Y_u^{*rb}(Y_dY_d^\dagger)^{st}\Big)-g_Y^2g_s^2\Big(\frac{25}{81}\delta^{pa}\delta^{st}Y_u^{*rb}+\frac{25}{81}\delta^{pr}\delta^{sa}Y_u^{*tb}\Big)\\
& -g_s^4\Big(\frac{2}{9}\delta^{pr}\delta^{st}Y_u^{*ab}+\frac{40}{27}\delta^{pa}\delta^{st}Y_u^{*rb}+\frac{40}{27}\delta^{pr}\delta^{sa}Y_u^{*tb}\Big)\Bigg\}C_{uG}^{ab}+C_{uG}^{*ab}\Bigg\{g_s^2g_L^2\Big(\frac{1}{9}\delta^{ra}\delta^{st}Y_u^{pb}+\frac{1}{9}\delta^{pr}\delta^{ta}Y_u^{sb}\Big)+g_s^2\Big(\frac{1}{6}\delta^{st}Y_u^{pb}(Y_uY_u^\dagger)^{ar}\\
& +\frac{1}{6}\delta^{pr}Y_u^{sb}(Y_uY_u^\dagger)^{at}+\frac{3}{2}\delta^{ra}Y_u^{sb}(Y_dY_d^\dagger)^{pt}+\frac{3}{2}\delta^{ta}Y_u^{pb}(Y_dY_d^\dagger)^{sr}+\frac{3}{2}\delta^{ra}Y_u^{sb}(Y_uY_u^\dagger)^{pt}+\frac{3}{2}\delta^{ta}Y_u^{pb}(Y_uY_u^\dagger)^{sr}-\frac{1}{12}\delta^{st}Y_u^{pb}(Y_dY_d^\dagger)^{ar}-\frac{1}{12}\delta^{pr}Y_u^{sb}(Y_dY_d^\dagger)^{at}\\
& -\frac{3}{2}\delta^{ta}Y_u^{sb}(Y_dY_d^\dagger)^{pr}-\frac{3}{2}\delta^{ra}Y_u^{pb}(Y_dY_d^\dagger)^{st}\Big)-g_Y^2g_s^2\Big(\frac{25}{81}\delta^{ra}\delta^{st}Y_u^{pb}+\frac{25}{81}\delta^{pr}\delta^{ta}Y_u^{sb}\Big)-g_s^4\Big(\frac{2}{9}\delta^{pr}\delta^{st}Y_u^{ab}+\frac{40}{27}\delta^{ra}\delta^{st}Y_u^{pb}+\frac{40}{27}\delta^{pr}\delta^{ta}Y_u^{sb}\Big)\Bigg\}\\
& +\Bigg\{g_Y^4\Big(\frac{35}{648}\delta^{pa}\delta^{st}Y_d^{*rb}+\frac{35}{648}\delta^{pr}\delta^{sa}Y_d^{*tb}-\frac{1}{54}\delta^{pr}\delta^{st}Y_d^{*ab}\Big)+g_Y^2\Big(\frac{1}{12}\delta^{st}Y_d^{*rb}(Y_uY_u^\dagger)^{pa}+\frac{1}{12}\delta^{pr}Y_d^{*tb}(Y_uY_u^\dagger)^{sa}-\frac{1}{6}\delta^{st}Y_d^{*rb}(Y_dY_d^\dagger)^{pa}\\
& -\frac{1}{6}\delta^{pr}Y_d^{*tb}(Y_dY_d^\dagger)^{sa}-\frac{3}{4}\delta^{sa}Y_d^{*tb}(Y_uY_u^\dagger)^{pr}-\frac{3}{4}\delta^{pa}Y_d^{*rb}(Y_uY_u^\dagger)^{st}\Big)-g_Y^2g_L^2\Big(\frac{5}{72}\delta^{pa}\delta^{st}Y_d^{*rb}+\frac{5}{72}\delta^{pr}\delta^{sa}Y_d^{*tb}\Big)-g_Y^2g_s^2\Big(\frac{11}{27}\delta^{pa}\delta^{st}Y_d^{*rb}\\
& +\frac{11}{27}\delta^{pr}\delta^{sa}Y_d^{*tb}\Big)\Bigg\}C_{dB}^{ab}+C_{dB}^{*ab}\Bigg\{g_Y^4\Big(\frac{35}{648}\delta^{ra}\delta^{st}Y_d^{pb}+\frac{35}{648}\delta^{pr}\delta^{ta}Y_d^{sb}-\frac{1}{54}\delta^{pr}\delta^{st}Y_d^{ab}\Big)+g_Y^2\Big(\frac{1}{12}\delta^{st}Y_d^{pb}(Y_uY_u^\dagger)^{ar}+\frac{1}{12}\delta^{pr}Y_d^{sb}(Y_uY_u^\dagger)^{at}\\
& -\frac{1}{6}\delta^{st}Y_d^{pb}(Y_dY_d^\dagger)^{ar}-\frac{1}{6}\delta^{pr}Y_d^{sb}(Y_dY_d^\dagger)^{at}-\frac{3}{4}\delta^{ta}Y_d^{sb}(Y_uY_u^\dagger)^{pr}-\frac{3}{4}\delta^{ra}Y_d^{pb}(Y_uY_u^\dagger)^{st}\Big)-g_Y^2g_L^2\Big(\frac{5}{72}\delta^{ra}\delta^{st}Y_d^{pb}+\frac{5}{72}\delta^{pr}\delta^{ta}Y_d^{sb}\Big)-g_Y^2g_s^2\Big(\frac{11}{27}\delta^{ra}\delta^{st}Y_d^{pb}\\
& +\frac{11}{27}\delta^{pr}\delta^{ta}Y_d^{sb}\Big)\Bigg\}+\Bigg\{g_s^2g_L^2\Big(\frac{1}{2}\delta^{pa}\delta^{st}Y_d^{*rb}+\frac{1}{2}\delta^{pr}\delta^{sa}Y_d^{*tb}-\frac{3}{2}\delta^{pa}\delta^{rs}Y_d^{*tb}-\frac{3}{2}\delta^{pt}\delta^{sa}Y_d^{*rb}\Big)+g_L^2\Big(\frac{1}{8}\delta^{st}Y_d^{*rb}(Y_uY_u^\dagger)^{pa}+\frac{1}{8}\delta^{pr}Y_d^{*tb}(Y_uY_u^\dagger)^{sa}\\
& +\frac{9}{8}\delta^{sa}Y_d^{*tb}(Y_uY_u^\dagger)^{pr}+\frac{9}{8}\delta^{pa}Y_d^{*rb}(Y_uY_u^\dagger)^{st}+\frac{3}{2}\delta^{sa}Y_d^{*tb}(Y_dY_d^\dagger)^{pr}+\frac{3}{2}\delta^{pa}Y_d^{*rb}(Y_dY_d^\dagger)^{st}\Big)-g_Y^2g_L^2\Big(\frac{1}{16}\delta^{pa}\delta^{st}Y_d^{*rb}+\frac{1}{16}\delta^{pr}\delta^{sa}Y_d^{*tb}\Big)\Bigg\}
\end{aligned}$$

$$\begin{aligned}
& -g_L^4 \left( \frac{1}{16} \delta^{pa} \delta^{st} Y_d^{*rb} + \frac{1}{16} \delta^{pr} \delta^{sa} Y_d^{*tb} + \frac{1}{4} \delta^{pr} \delta^{st} Y_d^{*ab} \right) \Big\} C_{dW}^{ab} + C_{dW}^{*ab} \Big\{ g_s^2 g_L^2 \left( \frac{1}{2} \delta^{ra} \delta^{st} Y_d^{pb} + \frac{1}{2} \delta^{pr} \delta^{ta} Y_d^{sb} - \frac{3}{2} \delta^{pt} \delta^{ra} Y_d^{sb} - \frac{3}{2} \delta^{rs} \delta^{ta} Y_d^{pb} \right) \right. \\
& + g_L^2 \left( \frac{1}{8} \delta^{st} Y_d^{pb} (Y_u Y_u^\dagger)^{ar} + \frac{1}{8} \delta^{pr} Y_d^{sb} (Y_u Y_u^\dagger)^{at} + \frac{9}{8} \delta^{ta} Y_d^{sb} (Y_u Y_u^\dagger)^{pr} + \frac{9}{8} \delta^{ra} Y_d^{pb} (Y_u Y_u^\dagger)^{st} + \frac{3}{2} \delta^{ta} Y_d^{sb} (Y_d Y_d^\dagger)^{pr} + \frac{3}{2} \delta^{ra} Y_d^{pb} (Y_d Y_d^\dagger)^{st} \right. \\
& + \frac{1}{16} \delta^{pr} \delta^{ta} Y_d^{sb} \Big) - g_L^4 \left( \frac{1}{16} \delta^{ra} \delta^{st} Y_d^{pb} + \frac{1}{16} \delta^{pr} \delta^{ta} Y_d^{sb} + \frac{1}{4} \delta^{pr} \delta^{st} Y_d^{ab} \right) \Big\} + \Big\{ g_s^2 g_L^2 \left( \frac{1}{9} \delta^{pa} \delta^{st} Y_d^{*rb} + \frac{1}{9} \delta^{pr} \delta^{sa} Y_d^{*tb} \right) + g_Y^2 g_s^2 \left( \frac{11}{81} \delta^{pa} \delta^{st} Y_d^{*rb} \right. \\
& + \frac{11}{81} \delta^{pr} \delta^{sa} Y_d^{*tb} \Big) + g_s^2 \left( \frac{1}{6} \delta^{st} Y_d^{*rb} (Y_d Y_d^\dagger)^{pa} + \frac{1}{6} \delta^{pr} Y_d^{*tb} (Y_d Y_d^\dagger)^{sa} + \frac{3}{2} \delta^{sa} Y_d^{*rb} (Y_d Y_d^\dagger)^{pt} + \frac{3}{2} \delta^{pa} Y_d^{*tb} (Y_d Y_d^\dagger)^{sr} + \frac{3}{2} \delta^{sa} Y_d^{*rb} (Y_u Y_u^\dagger)^{pt} \right. \\
& + \frac{3}{2} \delta^{pa} Y_d^{*tb} (Y_u Y_u^\dagger)^{sr} - \frac{1}{12} \delta^{st} Y_d^{*rb} (Y_u Y_u^\dagger)^{pa} - \frac{1}{12} \delta^{pr} Y_d^{*tb} (Y_u Y_u^\dagger)^{sa} - \frac{3}{2} \delta^{sa} Y_d^{*tb} (Y_u Y_u^\dagger)^{pr} - \frac{3}{2} \delta^{pa} Y_d^{*rb} (Y_u Y_u^\dagger)^{st} \Big) - g_s^4 \left( \frac{2}{9} \delta^{pr} \delta^{st} Y_d^{*ab} + \frac{40}{27} \delta^{pa} \delta^{st} Y_d^{*rb} \right. \\
& + \frac{40}{27} \delta^{pr} \delta^{sa} Y_d^{*tb} \Big) \Big\} C_{dG}^{ab} + C_{dG}^{*ab} \Big\{ g_s^2 g_L^2 \left( \frac{1}{9} \delta^{ra} \delta^{st} Y_d^{pb} + \frac{1}{9} \delta^{pr} \delta^{ta} Y_d^{sb} \right) + g_Y^2 g_s^2 \left( \frac{11}{81} \delta^{ra} \delta^{st} Y_d^{pb} + \frac{11}{81} \delta^{pr} \delta^{ta} Y_d^{sb} \right) + g_s^2 \left( \frac{1}{6} \delta^{st} Y_d^{pb} (Y_d Y_d^\dagger)^{ar} \right. \\
& + \frac{1}{6} \delta^{pr} Y_d^{sb} (Y_d Y_d^\dagger)^{at} + \frac{3}{2} \delta^{ra} Y_d^{sb} (Y_d Y_d^\dagger)^{pt} + \frac{3}{2} \delta^{ta} Y_d^{pb} (Y_d Y_d^\dagger)^{sr} + \frac{3}{2} \delta^{ra} Y_d^{sb} (Y_u Y_u^\dagger)^{pt} + \frac{3}{2} \delta^{ta} Y_d^{pb} (Y_u Y_u^\dagger)^{sr} - \frac{1}{12} \delta^{st} Y_d^{pb} (Y_u Y_u^\dagger)^{ar} - \frac{1}{12} \delta^{pr} Y_d^{sb} (Y_u Y_u^\dagger)^{at} \\
& - \frac{3}{2} \delta^{ta} Y_d^{sb} (Y_u Y_u^\dagger)^{pr} - \frac{3}{2} \delta^{ra} Y_d^{pb} (Y_u Y_u^\dagger)^{st} \Big) - g_s^4 \left( \frac{2}{9} \delta^{pr} \delta^{st} Y_d^{ab} + \frac{40}{27} \delta^{ra} \delta^{st} Y_d^{pb} + \frac{40}{27} \delta^{pr} \delta^{ta} Y_d^{sb} \right) \Big\} + \Big\{ \frac{1}{8} \delta^{tb} (Y_d Y_d^\dagger)^{sa} (Y_u Y_u^\dagger)^{pr} + \frac{1}{8} \delta^{sa} (Y_d Y_d^\dagger)^{bt} (Y_u Y_u^\dagger)^{pr} \\
& + \frac{1}{8} \delta^{rb} (Y_d Y_d^\dagger)^{pa} (Y_u Y_u^\dagger)^{st} + \frac{1}{8} \delta^{pa} (Y_d Y_d^\dagger)^{br} (Y_u Y_u^\dagger)^{st} + \frac{1}{2} T_2 \delta^{sa} \delta^{tb} (Y_d Y_d^\dagger)^{pr} + \frac{1}{2} T_2 \delta^{pa} \delta^{rb} (Y_d Y_d^\dagger)^{st} + g_Y^2 g_s^2 \left( \frac{91}{972} \delta^{pa} \delta^{rb} \delta^{st} + \frac{91}{972} \delta^{pr} \delta^{sa} \delta^{tb} \right) \\
& + g_Y^4 \left( \frac{881}{5832} \delta^{pa} \delta^{rb} \delta^{st} + \frac{881}{5832} \delta^{pr} \delta^{sa} \delta^{tb} \right) + g_Y^2 g_L^2 \left( \frac{415}{648} \delta^{pa} \delta^{rb} \delta^{st} + \frac{415}{648} \delta^{pr} \delta^{sa} \delta^{tb} \right) + g_Y^2 \left( \frac{31}{1296} \delta^{rb} \delta^{st} (Y_u Y_u^\dagger)^{pa} + \frac{31}{1296} \delta^{pr} \delta^{tb} (Y_u Y_u^\dagger)^{sa} \right. \\
& + \frac{31}{1296} \delta^{pa} \delta^{st} (Y_u Y_u^\dagger)^{br} + \frac{31}{1296} \delta^{pr} \delta^{sa} (Y_u Y_u^\dagger)^{bt} + \frac{59}{1296} \delta^{rb} \delta^{st} (Y_d Y_d^\dagger)^{pa} + \frac{59}{1296} \delta^{pr} \delta^{tb} (Y_d Y_d^\dagger)^{sa} + \frac{59}{1296} \delta^{pa} \delta^{st} (Y_d Y_d^\dagger)^{br} + \frac{59}{1296} \delta^{pr} \delta^{sa} (Y_d Y_d^\dagger)^{bt} \\
& + \frac{89}{144} \delta^{sa} \delta^{tb} (Y_u Y_u^\dagger)^{pr} + \frac{89}{144} \delta^{pa} \delta^{rb} (Y_u Y_u^\dagger)^{st} - \frac{1}{18} T_2 \delta^{pa} \delta^{rb} \delta^{st} - \frac{1}{18} T_2 \delta^{pr} \delta^{sa} \delta^{tb} - \frac{173}{144} \delta^{sa} \delta^{tb} (Y_d Y_d^\dagger)^{pr} - \frac{173}{144} \delta^{pa} \delta^{rb} (Y_d Y_d^\dagger)^{st} \Big) \\
& + g_s^2 \left( \frac{7}{108} \delta^{rb} \delta^{st} (Y_u Y_u^\dagger)^{pa} + \frac{7}{108} \delta^{pr} \delta^{tb} (Y_u Y_u^\dagger)^{sa} + \frac{7}{108} \delta^{pa} \delta^{st} (Y_u Y_u^\dagger)^{br} + \frac{7}{108} \delta^{pr} \delta^{sa} (Y_u Y_u^\dagger)^{bt} + \frac{25}{12} \delta^{sa} \delta^{tb} (Y_d Y_d^\dagger)^{pr} + \frac{25}{12} \delta^{pa} \delta^{rb} (Y_d Y_d^\dagger)^{st} \right. \\
& - \frac{7}{108} \delta^{rb} \delta^{st} (Y_d Y_d^\dagger)^{pa} - \frac{7}{108} \delta^{pr} \delta^{tb} (Y_d Y_d^\dagger)^{sa} - \frac{7}{108} \delta^{pa} \delta^{st} (Y_d Y_d^\dagger)^{br} - \frac{7}{108} \delta^{pr} \delta^{sa} (Y_d Y_d^\dagger)^{bt} - \frac{25}{12} \delta^{sa} \delta^{tb} (Y_u Y_u^\dagger)^{pr} - \frac{25}{12} \delta^{pa} \delta^{rb} (Y_u Y_u^\dagger)^{st} \Big) \\
& + g_L^2 \left( \frac{29}{144} \delta^{rb} \delta^{st} (Y_u Y_u^\dagger)^{pa} + \frac{29}{144} \delta^{pr} \delta^{tb} (Y_u Y_u^\dagger)^{sa} + \frac{29}{144} \delta^{pa} \delta^{st} (Y_u Y_u^\dagger)^{br} + \frac{29}{144} \delta^{pr} \delta^{sa} (Y_u Y_u^\dagger)^{bt} + \frac{35}{16} \delta^{sa} \delta^{tb} (Y_u Y_u^\dagger)^{pr} + \frac{35}{16} \delta^{pa} \delta^{rb} (Y_u Y_u^\dagger)^{st} \right. \\
& - \frac{29}{144} \delta^{rb} \delta^{st} (Y_d Y_d^\dagger)^{pa} - \frac{29}{144} \delta^{pr} \delta^{tb} (Y_d Y_d^\dagger)^{sa} - \frac{29}{144} \delta^{pa} \delta^{st} (Y_d Y_d^\dagger)^{br} - \frac{29}{144} \delta^{pr} \delta^{sa} (Y_d Y_d^\dagger)^{bt} - \frac{35}{16} \delta^{sa} \delta^{tb} (Y_d Y_d^\dagger)^{pr} - \frac{35}{16} \delta^{pa} \delta^{rb} (Y_d Y_d^\dagger)^{st} \Big) \\
& + \frac{3}{2} \delta^{sa} \delta^{tb} (Y_d Y_d^\dagger Y_d Y_d^\dagger)^{pr} + \frac{3}{2} \delta^{pa} \delta^{rb} (Y_d Y_d^\dagger Y_d Y_d^\dagger)^{st} - \frac{1}{8} \delta^{rb} (Y_d Y_d^\dagger)^{st} (Y_u Y_u^\dagger)^{pa} - \frac{1}{8} \delta^{tb} (Y_d Y_d^\dagger)^{pr} (Y_u Y_u^\dagger)^{sa} - \frac{1}{8} \delta^{pa} (Y_d Y_d^\dagger)^{st} (Y_u Y_u^\dagger)^{br}
\end{aligned}$$

$$\begin{aligned}
& -\frac{1}{8}\delta^{sa}(Y_d Y_d^\dagger)^{pr}(Y_u Y_u^\dagger)^{bt} - \frac{1}{2}\text{T}_2\delta^{sa}\delta^{tb}(Y_u Y_u^\dagger)^{pr} - \frac{1}{2}\text{T}_2\delta^{pa}\delta^{rb}(Y_u Y_u^\dagger)^{st} - \frac{3}{2}\delta^{sa}\delta^{tb}(Y_u Y_u^\dagger Y_u Y_u^\dagger)^{pr} - \frac{3}{2}\delta^{pa}\delta^{rb}(Y_u Y_u^\dagger Y_u Y_u^\dagger)^{st} \Big\} C_{Hq}^{(\parallel)ab} \\
& + \left\{ \frac{5}{8}\delta^{sa}\delta^{tb}(Y_d Y_d^\dagger Y_d Y_d^\dagger)^{pr} + \frac{5}{8}\delta^{pa}\delta^{rb}(Y_d Y_d^\dagger Y_d Y_d^\dagger)^{st} + g_Y^2 g_L^2 \left( \frac{5}{108}\delta^{pa}\delta^{rb}\delta^{st} + \frac{5}{108}\delta^{pr}\delta^{sa}\delta^{tb} \right) + g_Y^2 g_s^2 \left( \frac{91}{1944}\delta^{pa}\delta^{rb}\delta^{st} + \frac{91}{1944}\delta^{pr}\delta^{sa}\delta^{tb} \right) \right. \\
& + g_Y^4 \left( \frac{881}{11664}\delta^{pa}\delta^{rb}\delta^{st} + \frac{881}{11664}\delta^{pr}\delta^{sa}\delta^{tb} \right) + g_s^2 g_L^2 \left( \frac{31}{216}\delta^{pa}\delta^{rb}\delta^{st} + \frac{31}{216}\delta^{pr}\delta^{sa}\delta^{tb} - \frac{5}{12}\delta^{pt}\delta^{rb}\delta^{sa} - \frac{5}{12}\delta^{pa}\delta^{rs}\delta^{tb} \right) + g_s^2 \left( \frac{7}{4}\delta^{rb}\delta^{sa}(Y_d Y_d^\dagger)^{pt} \right. \\
& + \frac{7}{4}\delta^{pa}\delta^{tb}(Y_d Y_d^\dagger)^{sr} + \frac{7}{4}\delta^{rb}\delta^{sa}(Y_u Y_u^\dagger)^{pt} + \frac{7}{4}\delta^{pa}\delta^{tb}(Y_u Y_u^\dagger)^{sr} - \frac{7}{108}\delta^{rb}\delta^{st}(Y_u Y_u^\dagger)^{pa} - \frac{7}{108}\delta^{pr}\delta^{tb}(Y_u Y_u^\dagger)^{sa} - \frac{7}{108}\delta^{pa}\delta^{st}(Y_u Y_u^\dagger)^{br} \\
& - \frac{7}{108}\delta^{pr}\delta^{sa}(Y_u Y_u^\dagger)^{bt} - \frac{7}{54}\delta^{rb}\delta^{st}(Y_d Y_d^\dagger)^{pa} - \frac{7}{54}\delta^{pr}\delta^{tb}(Y_d Y_d^\dagger)^{sa} - \frac{7}{54}\delta^{pa}\delta^{st}(Y_d Y_d^\dagger)^{br} - \frac{7}{54}\delta^{pr}\delta^{sa}(Y_d Y_d^\dagger)^{bt} - \frac{25}{12}\delta^{sa}\delta^{tb}(Y_u Y_u^\dagger)^{pr} \\
& - \frac{25}{12}\delta^{pa}\delta^{rb}(Y_u Y_u^\dagger)^{st} \Big\} + g_Y^2 \left( \frac{59}{648}\delta^{rb}\delta^{st}(Y_d Y_d^\dagger)^{pa} + \frac{59}{648}\delta^{pr}\delta^{tb}(Y_d Y_d^\dagger)^{sa} + \frac{59}{648}\delta^{pa}\delta^{st}(Y_d Y_d^\dagger)^{br} + \frac{59}{648}\delta^{pr}\delta^{sa}(Y_d Y_d^\dagger)^{bt} + \frac{89}{144}\delta^{sa}\delta^{tb}(Y_u Y_u^\dagger)^{pr} \right. \\
& + \frac{89}{144}\delta^{pa}\delta^{rb}(Y_u Y_u^\dagger)^{st} - \frac{31}{1296}\delta^{rb}\delta^{st}(Y_u Y_u^\dagger)^{pa} - \frac{31}{1296}\delta^{pr}\delta^{tb}(Y_u Y_u^\dagger)^{sa} - \frac{31}{1296}\delta^{pa}\delta^{st}(Y_u Y_u^\dagger)^{br} - \frac{31}{1296}\delta^{pr}\delta^{sa}(Y_u Y_u^\dagger)^{bt} - \frac{1}{36}\text{T}_2\delta^{pa}\delta^{rb}\delta^{st} \\
& - \frac{1}{36}\text{T}_2\delta^{pr}\delta^{sa}\delta^{tb} \Big\} + g_L^2 \left( \frac{1}{72}\delta^{rb}\delta^{st}(Y_d Y_d^\dagger)^{pa} + \frac{1}{72}\delta^{pr}\delta^{tb}(Y_d Y_d^\dagger)^{sa} + \frac{1}{72}\delta^{pa}\delta^{st}(Y_d Y_d^\dagger)^{br} + \frac{1}{72}\delta^{pr}\delta^{sa}(Y_d Y_d^\dagger)^{bt} + \frac{1}{12}\text{T}_2\delta^{pa}\delta^{rb}\delta^{st} \right. \\
& + \frac{1}{12}\text{T}_2\delta^{pr}\delta^{sa}\delta^{tb} + \frac{1}{8}\delta^{sa}\delta^{tb}(Y_d Y_d^\dagger)^{pr} + \frac{1}{8}\delta^{pa}\delta^{rb}(Y_d Y_d^\dagger)^{st} + \frac{31}{144}\delta^{rb}\delta^{st}(Y_u Y_u^\dagger)^{pa} + \frac{31}{144}\delta^{pr}\delta^{tb}(Y_u Y_u^\dagger)^{sa} + \frac{31}{144}\delta^{pa}\delta^{st}(Y_u Y_u^\dagger)^{br} \\
& + \frac{31}{144}\delta^{pr}\delta^{sa}(Y_u Y_u^\dagger)^{bt} + \frac{37}{16}\delta^{sa}\delta^{tb}(Y_u Y_u^\dagger)^{pr} + \frac{37}{16}\delta^{pa}\delta^{rb}(Y_u Y_u^\dagger)^{st} \Big\} - \frac{1}{8}\delta^{rb}(Y_d Y_d^\dagger)^{st}(Y_u Y_u^\dagger)^{pa} - \frac{1}{8}\delta^{tb}(Y_d Y_d^\dagger)^{pr}(Y_u Y_u^\dagger)^{sa} - \frac{1}{8}\delta^{pa}(Y_d Y_d^\dagger)^{st}(Y_u Y_u^\dagger)^{br} \\
& - \frac{1}{8}\delta^{sa}(Y_d Y_d^\dagger)^{pr}(Y_u Y_u^\dagger)^{bt} - \frac{1}{4}\delta^{rb}(Y_d Y_d^\dagger)^{pa}(Y_d Y_d^\dagger)^{st} - \frac{1}{4}\delta^{tb}(Y_d Y_d^\dagger)^{pr}(Y_d Y_d^\dagger)^{sa} - \frac{1}{4}\delta^{pa}(Y_d Y_d^\dagger)^{st}(Y_d Y_d^\dagger)^{br} - \frac{1}{4}\delta^{sa}(Y_d Y_d^\dagger)^{pr}(Y_d Y_d^\dagger)^{bt} - \frac{1}{4}\delta^{rb}(Y_u Y_u^\dagger)^{pa}(Y_u Y_u^\dagger)^{st} \\
& - \frac{1}{4}\delta^{tb}(Y_u Y_u^\dagger)^{pr}(Y_u Y_u^\dagger)^{sa} - \frac{1}{4}\delta^{pa}(Y_u Y_u^\dagger)^{st}(Y_u Y_u^\dagger)^{br} - \frac{1}{4}\delta^{sa}(Y_u Y_u^\dagger)^{pr}(Y_u Y_u^\dagger)^{bt} - \frac{1}{4}\delta^{sa}\delta^{tb}(Y_d Y_d^\dagger Y_u Y_u^\dagger)^{pr} - \frac{1}{4}\delta^{pa}\delta^{rb}(Y_d Y_d^\dagger Y_u Y_u^\dagger)^{st} \\
& - \frac{1}{4}\delta^{sa}\delta^{tb}(Y_u Y_u^\dagger Y_d Y_d^\dagger)^{pr} - \frac{1}{4}\delta^{pa}\delta^{rb}(Y_u Y_u^\dagger Y_d Y_d^\dagger)^{st} - \frac{1}{2}\text{T}_2\delta^{sa}\delta^{tb}(Y_u Y_u^\dagger)^{pr} - \frac{1}{2}\text{T}_2\delta^{pa}\delta^{rb}(Y_u Y_u^\dagger)^{st} - \frac{7}{8}\delta^{sa}\delta^{tb}(Y_u Y_u^\dagger Y_u Y_u^\dagger)^{pr} \\
& - \frac{7}{8}\delta^{pa}\delta^{rb}(Y_u Y_u^\dagger Y_u Y_u^\dagger)^{st} - g_L^4 \left( \frac{83}{144}\delta^{pa}\delta^{rb}\delta^{st} + \frac{83}{144}\delta^{pr}\delta^{sa}\delta^{tb} \right) \Big\} C_{Hq}^{(\times)ab} + \left\{ \frac{1}{4}\delta^{sa}\delta^{tb}(Y_e^\dagger Y_e)^{dc}(Y_u Y_u^\dagger)^{pr} + \frac{1}{4}\delta^{pa}\delta^{rb}(Y_e^\dagger Y_e)^{dc}(Y_u Y_u^\dagger)^{st} \right. \\
& + g_Y^2 \left( \frac{5}{18}\delta^{pa}\delta^{rb}\delta^{st}(Y_e^\dagger Y_e)^{dc} + \frac{5}{18}\delta^{pr}\delta^{sa}\delta^{tb}(Y_e^\dagger Y_e)^{dc} \right) - \frac{1}{4}\delta^{sa}\delta^{tb}(Y_e^\dagger Y_e)^{dc}(Y_d Y_d^\dagger)^{pr} - \frac{1}{4}\delta^{pa}\delta^{rb}(Y_e^\dagger Y_e)^{dc}(Y_d Y_d^\dagger)^{st} - g_Y^2 g_s^2 \left( \frac{25}{486}\delta^{pa}\delta^{rb}\delta^{st}\delta^{cd} \right. \\
& + \frac{25}{486}\delta^{pr}\delta^{sa}\delta^{tb}\delta^{cd} \Big\} - g_Y^2 g_L^2 \left( \frac{25}{324}\delta^{pa}\delta^{rb}\delta^{st}\delta^{cd} + \frac{25}{324}\delta^{pr}\delta^{sa}\delta^{tb}\delta^{cd} \right) - g_Y^4 \left( \frac{2027}{2916}\delta^{pa}\delta^{rb}\delta^{st}\delta^{cd} + \frac{2027}{2916}\delta^{pr}\delta^{sa}\delta^{tb}\delta^{cd} \right) \Big\} C_{qe}^{abcd} \\
& + \left\{ \frac{3}{4}\text{T}_2\delta^{pa}\delta^{rb}Y_u^{*td}Y_u^{sc} + \frac{3}{4}\text{T}_2\delta^{sa}\delta^{tb}Y_u^{*rd}Y_u^{pc} + \frac{3}{4}\delta^{sa}\delta^{tb}(Y_u^\dagger Y_u)^{dc}(Y_d Y_d^\dagger)^{pr} + \frac{3}{4}\delta^{pa}\delta^{rb}(Y_u^\dagger Y_u)^{dc}(Y_d Y_d^\dagger)^{st} + \frac{3}{4}\delta^{sa}\delta^{tb}Y_u^{pc}(Y_u^\dagger Y_u Y_u^\dagger)^{rd} \right.
\end{aligned}$$

$$\begin{aligned}
& + \frac{3}{4} \delta^{pa} \delta^{rb} Y_u^{sc} (Y_u^\dagger Y_u Y_u^\dagger)^{td} + \frac{3}{4} \delta^{sa} \delta^{tb} Y_u^{*rd} (Y_u Y_u^\dagger Y_u)^{pc} + \frac{3}{4} \delta^{pa} \delta^{rb} Y_u^{*td} (Y_u Y_u^\dagger Y_u)^{sc} + g_s^2 \left( \frac{2}{27} \delta^{pa} \delta^{st} Y_u^{*rd} Y_u^{bc} + \frac{2}{27} \delta^{rb} \delta^{st} Y_u^{*ad} Y_u^{pc} \right. \\
& + \frac{2}{27} \delta^{pr} \delta^{sa} Y_u^{*td} Y_u^{bc} + \frac{2}{27} \delta^{pr} \delta^{tb} Y_u^{*ad} Y_u^{sc} + 3 \delta^{pa} \delta^{rb} Y_u^{*td} Y_u^{sc} + 3 \delta^{sa} \delta^{tb} Y_u^{*rd} Y_u^{pc} \left. \right) + g_Y^2 g_L^2 \left( \frac{25}{162} \delta^{pa} \delta^{rb} \delta^{st} \delta^{cd} + \frac{25}{162} \delta^{pr} \delta^{sa} \delta^{tb} \delta^{cd} \right) \\
& + g_Y^2 g_s^2 \left( \frac{241}{243} \delta^{pa} \delta^{rb} \delta^{st} \delta^{cd} + \frac{241}{243} \delta^{pr} \delta^{sa} \delta^{tb} \delta^{cd} \right) - \frac{1}{8} \delta^{rb} Y_u^{*td} Y_u^{sc} (Y_d Y_d^\dagger)^{pa} - \frac{1}{8} \delta^{tb} Y_u^{*rd} Y_u^{pc} (Y_d Y_d^\dagger)^{sa} - \frac{1}{8} \delta^{pa} Y_u^{*td} Y_u^{sc} (Y_d Y_d^\dagger)^{br} - \frac{1}{8} \delta^{sa} Y_u^{*rd} Y_u^{pc} (Y_d Y_d^\dagger)^{bt} \\
& - \frac{1}{4} \delta^{sa} \delta^{tb} Y_u^{pc} (Y_d^\dagger Y_d Y_u^\dagger)^{rd} - \frac{1}{4} \delta^{pa} \delta^{rb} Y_u^{sc} (Y_d^\dagger Y_d Y_u^\dagger)^{td} - \frac{1}{4} \delta^{sa} \delta^{tb} Y_u^{*rd} (Y_d Y_d^\dagger Y_u)^{pc} - \frac{1}{4} \delta^{pa} \delta^{rb} Y_u^{*td} (Y_d Y_d^\dagger Y_u)^{sc} - \frac{3}{4} \delta^{sa} \delta^{tb} (Y_u^\dagger Y_u)^{dc} (Y_u Y_u^\dagger)^{pr} \\
& - \frac{3}{4} \delta^{pa} \delta^{rb} (Y_u^\dagger Y_u)^{dc} (Y_u Y_u^\dagger)^{st} - g_L^2 \left( \frac{1}{18} \delta^{pa} \delta^{st} Y_u^{*rd} Y_u^{bc} + \frac{1}{18} \delta^{rb} \delta^{st} Y_u^{*ad} Y_u^{pc} + \frac{1}{18} \delta^{pr} \delta^{sa} Y_u^{*td} Y_u^{bc} + \frac{1}{18} \delta^{pr} \delta^{tb} Y_u^{*ad} Y_u^{sc} + \frac{23}{16} \delta^{pa} \delta^{rb} Y_u^{*td} Y_u^{sc} \right. \\
& + \frac{23}{16} \delta^{sa} \delta^{tb} Y_u^{*rd} Y_u^{pc} \left. \right) - g_Y^4 \left( \frac{313}{1458} \delta^{pa} \delta^{rb} \delta^{st} \delta^{cd} + \frac{313}{1458} \delta^{pr} \delta^{sa} \delta^{tb} \delta^{cd} \right) - g_s^4 \left( \frac{61}{18} \delta^{pa} \delta^{rb} \delta^{st} \delta^{cd} + \frac{61}{18} \delta^{pr} \delta^{sa} \delta^{tb} \delta^{cd} \right) - g_Y^2 \left( \frac{11}{162} \delta^{pa} \delta^{st} Y_u^{*rd} Y_u^{bc} \right. \\
& + \frac{11}{162} \delta^{rb} \delta^{st} Y_u^{*ad} Y_u^{pc} + \frac{11}{162} \delta^{pr} \delta^{sa} Y_u^{*td} Y_u^{bc} + \frac{11}{162} \delta^{pr} \delta^{tb} Y_u^{*ad} Y_u^{sc} + \frac{1}{2} \delta^{pa} \delta^{rb} \delta^{st} (Y_u^\dagger Y_u)^{dc} + \frac{1}{2} \delta^{pr} \delta^{sa} \delta^{tb} (Y_u^\dagger Y_u)^{dc} + \frac{47}{48} \delta^{pa} \delta^{rb} Y_u^{*td} Y_u^{sc} \\
& + \frac{47}{48} \delta^{sa} \delta^{tb} Y_u^{*rd} Y_u^{pc} \left. \right\} C_{qu}^{(\parallel)abcd} + \left\{ \frac{1}{8} \delta^{tb} Y_u^{*rd} Y_u^{sc} (Y_d Y_d^\dagger)^{pa} + \frac{1}{8} \delta^{rb} Y_u^{*td} Y_u^{pc} (Y_d Y_d^\dagger)^{sa} + \frac{1}{8} \delta^{sa} Y_u^{*td} Y_u^{pc} (Y_d Y_d^\dagger)^{br} + \frac{1}{8} \delta^{pa} Y_u^{*rd} Y_u^{sc} (Y_d Y_d^\dagger)^{bt} \right. \\
& + \frac{1}{4} \delta^{sa} \delta^{tb} (Y_u^\dagger Y_u)^{dc} (Y_d Y_d^\dagger)^{pr} + \frac{1}{4} \delta^{pa} \delta^{rb} (Y_u^\dagger Y_u)^{dc} (Y_d Y_d^\dagger)^{st} + \frac{7}{8} \delta^{tb} Y_u^{*rd} Y_u^{sc} (Y_u Y_u^\dagger)^{pa} + \frac{7}{8} \delta^{rb} Y_u^{*td} Y_u^{pc} (Y_u Y_u^\dagger)^{sa} + \frac{7}{8} \delta^{sa} Y_u^{*td} Y_u^{pc} (Y_u Y_u^\dagger)^{br} \\
& + \frac{7}{8} \delta^{pa} Y_u^{*rd} Y_u^{sc} (Y_u Y_u^\dagger)^{bt} + g_L^2 \left( \frac{1}{12} \delta^{pa} \delta^{st} Y_u^{*rd} Y_u^{bc} + \frac{1}{12} \delta^{rb} \delta^{st} Y_u^{*ad} Y_u^{pc} + \frac{1}{12} \delta^{pr} \delta^{sa} Y_u^{*td} Y_u^{bc} + \frac{1}{12} \delta^{pr} \delta^{tb} Y_u^{*ad} Y_u^{sc} - \frac{5}{4} \delta^{rb} \delta^{sa} Y_u^{*td} Y_u^{pc} \right. \\
& - \frac{5}{4} \delta^{pa} \delta^{tb} Y_u^{*rd} Y_u^{sc} \left. \right) + g_Y^2 g_L^2 \left( \frac{25}{486} \delta^{pa} \delta^{rb} \delta^{st} \delta^{cd} + \frac{25}{486} \delta^{pr} \delta^{sa} \delta^{tb} \delta^{cd} \right) + g_s^2 g_L^2 \left( \frac{1}{6} \delta^{pt} \delta^{rb} \delta^{sa} \delta^{cd} + \frac{1}{6} \delta^{pa} \delta^{rs} \delta^{tb} \delta^{cd} + \frac{173}{324} \delta^{pa} \delta^{rb} \delta^{st} \delta^{cd} \right. \\
& + \frac{173}{324} \delta^{pr} \delta^{sa} \delta^{tb} \delta^{cd} \left. \right) + g_s^4 \left( \frac{4}{27} \delta^{pr} \delta^{st} \delta^{ab} \delta^{cd} - \frac{287}{243} \delta^{pa} \delta^{rb} \delta^{st} \delta^{cd} - \frac{287}{243} \delta^{pr} \delta^{sa} \delta^{tb} \delta^{cd} \right) + g_Y^2 \left( \frac{1}{54} \delta^{pr} \delta^{ab} Y_u^{*td} Y_u^{sc} + \frac{1}{54} \delta^{st} \delta^{ab} Y_u^{*rd} Y_u^{pc} \right. \\
& - \frac{4}{27} \delta^{pa} \delta^{rb} \delta^{st} (Y_u^\dagger Y_u)^{dc} - \frac{4}{27} \delta^{pr} \delta^{sa} \delta^{tb} (Y_u^\dagger Y_u)^{dc} - \frac{25}{108} \delta^{pa} \delta^{st} Y_u^{*rd} Y_u^{bc} - \frac{25}{108} \delta^{rb} \delta^{st} Y_u^{*ad} Y_u^{pc} - \frac{25}{108} \delta^{pr} \delta^{sa} Y_u^{*td} Y_u^{bc} - \frac{25}{108} \delta^{pr} \delta^{tb} Y_u^{*ad} Y_u^{sc} \left. \right) \\
& + g_s^2 \left( \frac{1}{18} \delta^{pa} \delta^{st} Y_u^{*rd} Y_u^{bc} + \frac{1}{18} \delta^{rb} \delta^{st} Y_u^{*ad} Y_u^{pc} + \frac{1}{18} \delta^{pr} \delta^{sa} Y_u^{*td} Y_u^{bc} + \frac{1}{18} \delta^{pr} \delta^{tb} Y_u^{*ad} Y_u^{sc} + \frac{2}{9} \delta^{pa} \delta^{rb} \delta^{st} (Y_u^\dagger Y_u)^{dc} + \frac{2}{9} \delta^{pr} \delta^{sa} \delta^{tb} (Y_u^\dagger Y_u)^{dc} \right. \\
& + \delta^{pa} \delta^{rb} Y_u^{*td} Y_u^{sc} + \delta^{sa} \delta^{tb} Y_u^{*rd} Y_u^{pc} - \frac{1}{9} \delta^{pr} \delta^{ab} Y_u^{*td} Y_u^{sc} - \frac{1}{9} \delta^{st} \delta^{ab} Y_u^{*rd} Y_u^{pc} \left. \right) - \frac{1}{4} \delta^{sa} \delta^{tb} (Y_u^\dagger Y_u)^{dc} (Y_u Y_u^\dagger)^{pr} - \frac{1}{4} \delta^{pa} \delta^{rb} (Y_u^\dagger Y_u)^{dc} (Y_u Y_u^\dagger)^{st} \\
& - g_Y^4 \left( \frac{313}{4374} \delta^{pa} \delta^{rb} \delta^{st} \delta^{cd} + \frac{313}{4374} \delta^{pr} \delta^{sa} \delta^{tb} \delta^{cd} \right) - g_Y^2 g_s^2 \left( \frac{2}{81} \delta^{pr} \delta^{st} \delta^{ab} \delta^{cd} + \frac{1873}{2916} \delta^{pa} \delta^{rb} \delta^{st} \delta^{cd} + \frac{1873}{2916} \delta^{pr} \delta^{sa} \delta^{tb} \delta^{cd} \right) \left. \right\} C_{qu}^{(\times)abcd} \\
& + \left\{ \frac{3}{4} T_2 \delta^{pa} \delta^{rb} Y_d^{*td} Y_d^{sc} + \frac{3}{4} T_2 \delta^{sa} \delta^{tb} Y_d^{*rd} Y_d^{pc} + \frac{3}{4} \delta^{sa} \delta^{tb} (Y_d^\dagger Y_d)^{dc} (Y_u Y_u^\dagger)^{pr} + \frac{3}{4} \delta^{pa} \delta^{rb} (Y_d^\dagger Y_d)^{dc} (Y_u Y_u^\dagger)^{st} + \frac{3}{4} \delta^{sa} \delta^{tb} Y_d^{pc} (Y_d^\dagger Y_d Y_d^\dagger)^{rd} \right. \\
& + \frac{3}{4} \delta^{pa} \delta^{rb} Y_d^{sc} (Y_d^\dagger Y_d Y_d^\dagger)^{td} + \frac{3}{4} \delta^{sa} \delta^{tb} Y_d^{*rd} (Y_d Y_d^\dagger Y_d)^{pc} + \frac{3}{4} \delta^{pa} \delta^{rb} Y_d^{*td} (Y_d Y_d^\dagger Y_d)^{sc} + g_s^2 \left( \frac{2}{27} \delta^{pa} \delta^{st} Y_d^{*rd} Y_d^{bc} + \frac{2}{27} \delta^{rb} \delta^{st} Y_d^{*ad} Y_d^{pc} \right.
\end{aligned}$$

$$\begin{aligned}
& + \frac{2}{27} \delta^{pr} \delta^{sa} Y_d^{*td} Y_d^{bc} + \frac{2}{27} \delta^{pr} \delta^{tb} Y_d^{*ad} Y_d^{sc} + 3 \delta^{pa} \delta^{rb} Y_d^{*td} Y_d^{sc} + 3 \delta^{sa} \delta^{tb} Y_d^{*rd} Y_d^{pc} \Big) + g_Y^2 \Big( \frac{7}{162} \delta^{pa} \delta^{st} Y_d^{*rd} Y_d^{bc} + \frac{7}{162} \delta^{rb} \delta^{st} Y_d^{*ad} Y_d^{pc} \\
& + \frac{7}{162} \delta^{pr} \delta^{sa} Y_d^{*td} Y_d^{bc} + \frac{7}{162} \delta^{pr} \delta^{tb} Y_d^{*ad} Y_d^{sc} + \frac{1}{6} \delta^{pa} \delta^{rb} \delta^{st} (Y_d^\dagger Y_d)^{dc} + \frac{1}{6} \delta^{pr} \delta^{sa} \delta^{tb} (Y_d^\dagger Y_d)^{dc} - \frac{55}{48} \delta^{pa} \delta^{rb} Y_d^{*td} Y_d^{sc} - \frac{55}{48} \delta^{sa} \delta^{tb} Y_d^{*rd} Y_d^{pc} \Big) \\
& - \frac{1}{8} \delta^{rb} Y_d^{*td} Y_d^{sc} (Y_u Y_u^\dagger)^{pa} - \frac{1}{8} \delta^{tb} Y_d^{*rd} Y_d^{pc} (Y_u Y_u^\dagger)^{sa} - \frac{1}{8} \delta^{pa} Y_d^{*td} Y_d^{sc} (Y_u Y_u^\dagger)^{br} - \frac{1}{8} \delta^{sa} Y_d^{*rd} Y_d^{pc} (Y_u Y_u^\dagger)^{bt} - \frac{1}{4} \delta^{sa} \delta^{tb} Y_d^{pc} (Y_u^\dagger Y_u Y_d^\dagger)^{rd} \\
& - \frac{1}{4} \delta^{pa} \delta^{rb} Y_d^{sc} (Y_u^\dagger Y_u Y_d^\dagger)^{td} - \frac{1}{4} \delta^{sa} \delta^{tb} Y_d^{*rd} (Y_u Y_u^\dagger Y_d)^{pc} - \frac{1}{4} \delta^{pa} \delta^{rb} Y_d^{*td} (Y_u Y_u^\dagger Y_d)^{sc} - \frac{3}{4} \delta^{sa} \delta^{tb} (Y_d^\dagger Y_d)^{dc} (Y_d Y_d^\dagger)^{pr} - \frac{3}{4} \delta^{pa} \delta^{rb} (Y_d^\dagger Y_d)^{dc} (Y_d Y_d^\dagger)^{st} \\
& - g_L^2 \Big( \frac{1}{18} \delta^{pa} \delta^{st} Y_d^{*rd} Y_d^{bc} + \frac{1}{18} \delta^{rb} \delta^{st} Y_d^{*ad} Y_d^{pc} + \frac{1}{18} \delta^{pr} \delta^{sa} Y_d^{*td} Y_d^{bc} + \frac{1}{18} \delta^{pr} \delta^{tb} Y_d^{*ad} Y_d^{sc} + \frac{23}{16} \delta^{pa} \delta^{rb} Y_d^{*td} Y_d^{sc} + \frac{23}{16} \delta^{sa} \delta^{tb} Y_d^{*rd} Y_d^{pc} \Big) \\
& - g_Y^2 g_L^2 \Big( \frac{25}{324} \delta^{pa} \delta^{rb} \delta^{st} \delta^{cd} + \frac{25}{324} \delta^{pr} \delta^{sa} \delta^{tb} \delta^{cd} \Big) - g_Y^4 \Big( \frac{443}{2916} \delta^{pa} \delta^{rb} \delta^{st} \delta^{cd} + \frac{443}{2916} \delta^{pr} \delta^{sa} \delta^{tb} \delta^{cd} \Big) - g_Y^2 g_s^2 \Big( \frac{241}{486} \delta^{pa} \delta^{rb} \delta^{st} \delta^{cd} + \frac{241}{486} \delta^{pr} \delta^{sa} \delta^{tb} \delta^{cd} \Big) \\
& - g_s^4 \Big( \frac{61}{18} \delta^{pa} \delta^{rb} \delta^{st} \delta^{cd} + \frac{61}{18} \delta^{pr} \delta^{sa} \delta^{tb} \delta^{cd} \Big) \Big\} C_{qd}^{(\parallel)abcd} + \left\{ \frac{1}{8} \delta^{tb} Y_d^{*rd} Y_d^{sc} (Y_u Y_u^\dagger)^{pa} + \frac{1}{8} \delta^{rb} Y_d^{*td} Y_d^{pc} (Y_u Y_u^\dagger)^{sa} + \frac{1}{8} \delta^{sa} Y_d^{*td} Y_d^{pc} (Y_u Y_u^\dagger)^{br} \right. \\
& + \frac{1}{8} \delta^{pa} Y_d^{*rd} Y_d^{sc} (Y_u Y_u^\dagger)^{bt} + \frac{1}{4} \delta^{sa} \delta^{tb} (Y_d^\dagger Y_d)^{dc} (Y_u Y_u^\dagger)^{pr} + \frac{1}{4} \delta^{pa} \delta^{rb} (Y_d^\dagger Y_d)^{dc} (Y_u Y_u^\dagger)^{st} + \frac{7}{8} \delta^{tb} Y_d^{*rd} Y_d^{sc} (Y_d Y_d^\dagger)^{pa} + \frac{7}{8} \delta^{rb} Y_d^{*td} Y_d^{pc} (Y_d Y_d^\dagger)^{sa} \\
& + \frac{7}{8} \delta^{sa} Y_d^{*td} Y_d^{pc} (Y_d Y_d^\dagger)^{br} + \frac{7}{8} \delta^{pa} Y_d^{*rd} Y_d^{sc} (Y_d Y_d^\dagger)^{bt} + g_L^2 \Big( \frac{1}{12} \delta^{pa} \delta^{st} Y_d^{*rd} Y_d^{bc} + \frac{1}{12} \delta^{rb} \delta^{st} Y_d^{*ad} Y_d^{pc} + \frac{1}{12} \delta^{pr} \delta^{sa} Y_d^{*td} Y_d^{bc} + \frac{1}{12} \delta^{pr} \delta^{tb} Y_d^{*ad} Y_d^{sc} \\
& - \frac{5}{4} \delta^{rb} \delta^{sa} Y_d^{*td} Y_d^{pc} - \frac{5}{4} \delta^{pa} \delta^{tb} Y_d^{*rd} Y_d^{sc} \Big) + g_s^2 g_L^2 \Big( \frac{1}{6} \delta^{pt} \delta^{rb} \delta^{sa} \delta^{cd} + \frac{1}{6} \delta^{pa} \delta^{rs} \delta^{tb} \delta^{cd} + \frac{173}{324} \delta^{pa} \delta^{rb} \delta^{st} \delta^{cd} + \frac{173}{324} \delta^{pr} \delta^{sa} \delta^{tb} \delta^{cd} \Big) \\
& + g_Y^2 g_s^2 \Big( \frac{191}{2916} \delta^{pa} \delta^{rb} \delta^{st} \delta^{cd} + \frac{191}{2916} \delta^{pr} \delta^{sa} \delta^{tb} \delta^{cd} - \frac{2}{81} \delta^{pr} \delta^{st} \delta^{ab} \delta^{cd} \Big) + g_s^4 \Big( \frac{4}{27} \delta^{pr} \delta^{st} \delta^{ab} \delta^{cd} - \frac{287}{243} \delta^{pa} \delta^{rb} \delta^{st} \delta^{cd} - \frac{287}{243} \delta^{pr} \delta^{sa} \delta^{tb} \delta^{cd} \Big) \\
& + g_Y^2 \Big( \frac{1}{54} \delta^{pr} \delta^{ab} Y_d^{*td} Y_d^{sc} + \frac{1}{54} \delta^{st} \delta^{ab} Y_d^{*rd} Y_d^{pc} + \frac{2}{27} \delta^{pa} \delta^{rb} \delta^{st} (Y_d^\dagger Y_d)^{dc} + \frac{2}{27} \delta^{pr} \delta^{sa} \delta^{tb} (Y_d^\dagger Y_d)^{dc} + \frac{11}{108} \delta^{pa} \delta^{st} Y_d^{*rd} Y_d^{bc} + \frac{11}{108} \delta^{rb} \delta^{st} Y_d^{*ad} Y_d^{pc} \\
& + \frac{11}{108} \delta^{pr} \delta^{sa} Y_d^{*td} Y_d^{bc} + \frac{11}{108} \delta^{pr} \delta^{tb} Y_d^{*ad} Y_d^{sc} \Big) + g_s^2 \Big( \frac{1}{18} \delta^{pa} \delta^{st} Y_d^{*rd} Y_d^{bc} + \frac{1}{18} \delta^{rb} \delta^{st} Y_d^{*ad} Y_d^{pc} + \frac{1}{18} \delta^{pr} \delta^{sa} Y_d^{*td} Y_d^{bc} + \frac{1}{18} \delta^{pr} \delta^{tb} Y_d^{*ad} Y_d^{sc} \\
& + \frac{2}{9} \delta^{pa} \delta^{rb} \delta^{st} (Y_d^\dagger Y_d)^{dc} + \frac{2}{9} \delta^{pr} \delta^{sa} \delta^{tb} (Y_d^\dagger Y_d)^{dc} + \delta^{pa} \delta^{rb} Y_d^{*td} Y_d^{sc} + \delta^{sa} \delta^{tb} Y_d^{*rd} Y_d^{pc} - \frac{1}{9} \delta^{pr} \delta^{ab} Y_d^{*td} Y_d^{sc} - \frac{1}{9} \delta^{st} \delta^{ab} Y_d^{*rd} Y_d^{pc} \Big) \\
& - \frac{1}{4} \delta^{sa} \delta^{tb} (Y_d^\dagger Y_d)^{dc} (Y_d Y_d^\dagger)^{pr} - \frac{1}{4} \delta^{pa} \delta^{rb} (Y_d^\dagger Y_d)^{dc} (Y_d Y_d^\dagger)^{st} - g_Y^2 g_L^2 \Big( \frac{25}{972} \delta^{pa} \delta^{rb} \delta^{st} \delta^{cd} + \frac{25}{972} \delta^{pr} \delta^{sa} \delta^{tb} \delta^{cd} \Big) - g_Y^4 \Big( \frac{443}{8748} \delta^{pa} \delta^{rb} \delta^{st} \delta^{cd} \\
& + \frac{443}{8748} \delta^{pr} \delta^{sa} \delta^{tb} \delta^{cd} \Big) \Big\} C_{qd}^{(\times)abcd} + \frac{4}{81} \delta^{pr} \delta^{st} \delta^{ab} \delta^{cd} g_Y^4 C_{ee}^{abcd} + \left\{ \frac{16}{243} \delta^{pr} \delta^{st} \delta^{ad} \delta^{bc} g_Y^4 + g_s^2 \Big( \frac{2}{9} \delta^{pr} \delta^{ad} Y_u^{*tb} Y_u^{sc} + \frac{2}{9} \delta^{st} \delta^{ad} Y_u^{*rb} Y_u^{pc} \Big) \right. \\
& - \frac{4}{27} \delta^{pr} \delta^{st} \delta^{ad} \delta^{bc} g_s^4 - g_Y^2 \Big( \frac{4}{27} \delta^{pr} \delta^{ad} Y_u^{*tb} Y_u^{sc} + \frac{4}{27} \delta^{st} \delta^{ad} Y_u^{*rb} Y_u^{pc} \Big) \Big\} C_{uu}^{abcd} + \left\{ \frac{4}{243} \delta^{pr} \delta^{st} \delta^{ad} \delta^{bc} g_Y^4 + g_Y^2 \Big( \frac{2}{27} \delta^{pr} \delta^{ad} Y_d^{*tb} Y_d^{sc} + \frac{2}{27} \delta^{st} \delta^{ad} Y_d^{*rb} Y_d^{pc} \Big) \right. \\
& + g_s^2 \Big( \frac{2}{9} \delta^{pr} \delta^{ad} Y_d^{*tb} Y_d^{sc} + \frac{2}{9} \delta^{st} \delta^{ad} Y_d^{*rb} Y_d^{pc} \Big) - \frac{4}{27} \delta^{pr} \delta^{st} \delta^{ad} \delta^{bc} g_s^4 \Big\} C_{dd}^{abcd} + \left\{ \frac{1}{4} Y_d^{*td} Y_u^{*rb} Y_d^{sc} Y_u^{pa} + \frac{1}{4} Y_d^{*rd} Y_u^{*tb} Y_d^{pc} Y_u^{sa} \right\} C_{ud}^{(\parallel)abcd} - \left\{ \frac{1}{4} Y_d^{*rd} Y_u^{*tb} Y_d^{sc} Y_u^{pa} \right.
\end{aligned}$$

$$\begin{aligned}
& + \frac{1}{4} Y_d^{*td} Y_u^{*rb} Y_d^{pc} Y_u^{sa} \left\{ C_{ud}^{(\times)abcd} + \left\{ \frac{1}{8} \delta^{td} Y_e^{*ab} Y_d^{*sc} (Y_u Y_u^\dagger)^{pr} + \frac{1}{8} \delta^{rd} Y_e^{*ab} Y_d^{*pc} (Y_u Y_u^\dagger)^{st} + g_L^2 \left( \frac{1}{36} \delta^{rd} \delta^{st} Y_e^{*ab} Y_d^{*pc} + \frac{1}{36} \delta^{pr} \delta^{td} Y_e^{*ab} Y_d^{*sc} \right) \right. \right. \\
& - g_Y^2 \left( \frac{7}{324} \delta^{rd} \delta^{st} Y_e^{*ab} Y_d^{*pc} + \frac{7}{324} \delta^{pr} \delta^{td} Y_e^{*ab} Y_d^{*sc} \right) - g_s^2 \left( \frac{1}{27} \delta^{rd} \delta^{st} Y_e^{*ab} Y_d^{*pc} + \frac{1}{27} \delta^{pr} \delta^{td} Y_e^{*ab} Y_d^{*sc} \right) \left\{ C_{ledq}^{abcd} + C_{ledq}^{*abcd} \left\{ \frac{1}{8} \delta^{sd} Y_d^{*tc} Y_e^{*ab} (Y_u Y_u^\dagger)^{pr} \right. \right. \\
& + \frac{1}{8} \delta^{pd} Y_d^{*rc} Y_e^{*ab} (Y_u Y_u^\dagger)^{st} + g_L^2 \left( \frac{1}{36} \delta^{pd} \delta^{st} Y_d^{*rc} Y_e^{*ab} + \frac{1}{36} \delta^{pr} \delta^{sd} Y_d^{*tc} Y_e^{*ab} \right) - g_Y^2 \left( \frac{7}{324} \delta^{pd} \delta^{st} Y_d^{*rc} Y_e^{*ab} + \frac{7}{324} \delta^{pr} \delta^{sd} Y_d^{*tc} Y_e^{*ab} \right) - g_s^2 \left( \frac{1}{27} \delta^{pd} \delta^{st} Y_d^{*rc} Y_e^{*ab} \right. \\
& + \frac{1}{27} \delta^{pr} \delta^{sd} Y_d^{*tc} Y_e^{*ab} \left. \right\} + \left\{ \frac{1}{16} \delta^{sc} Y_d^{*ad} Y_u^{*tb} (Y_d Y_d^\dagger)^{pr} + \frac{1}{16} \delta^{pc} Y_d^{*ad} Y_u^{*rb} (Y_d Y_d^\dagger)^{st} + \frac{1}{16} \delta^{sa} Y_d^{*td} Y_u^{*cb} (Y_u Y_u^\dagger)^{pr} + \frac{1}{16} \delta^{pa} Y_d^{*rd} Y_u^{*cb} (Y_u Y_u^\dagger)^{st} \right. \\
& + \frac{1}{8} T_2 \delta^{pc} \delta^{sa} Y_d^{*rd} Y_u^{*tb} + \frac{1}{8} T_2 \delta^{pa} \delta^{sc} Y_d^{*td} Y_u^{*rb} + \frac{1}{8} \delta^{pc} \delta^{sa} Y_u^{*tb} (Y_d^\dagger Y_d Y_d^\dagger)^{rd} + \frac{1}{8} \delta^{pa} \delta^{sc} Y_u^{*rb} (Y_d^\dagger Y_d Y_d^\dagger)^{td} + \frac{1}{8} \delta^{pa} \delta^{sc} Y_d^{*td} (Y_d^\dagger Y_d Y_u^\dagger)^{rb} \\
& + \frac{1}{8} \delta^{pc} \delta^{sa} Y_d^{*rd} (Y_d^\dagger Y_d Y_u^\dagger)^{tb} + \frac{1}{8} \delta^{pc} \delta^{sa} Y_u^{*tb} (Y_u^\dagger Y_u Y_d^\dagger)^{rd} + \frac{1}{8} \delta^{pa} \delta^{sc} Y_u^{*rb} (Y_u^\dagger Y_u Y_d^\dagger)^{td} + \frac{1}{8} \delta^{pa} \delta^{sc} Y_d^{*td} (Y_u^\dagger Y_u Y_u^\dagger)^{rb} + \frac{1}{8} \delta^{pc} \delta^{sa} Y_d^{*rd} (Y_u^\dagger Y_u Y_u^\dagger)^{tb} \\
& + \frac{5}{16} \delta^{sa} Y_d^{*rd} Y_u^{*tb} (Y_d Y_d^\dagger)^{pc} + \frac{5}{16} \delta^{pa} Y_d^{*td} Y_u^{*rb} (Y_d Y_d^\dagger)^{sc} + \frac{5}{16} \delta^{sc} Y_d^{*td} Y_u^{*rb} (Y_u Y_u^\dagger)^{pa} + \frac{5}{16} \delta^{pc} Y_d^{*rd} Y_u^{*tb} (Y_u Y_u^\dagger)^{sa} + \frac{3}{8} \delta^{sa} Y_d^{*cd} Y_u^{*tb} (Y_d Y_d^\dagger)^{pr} \\
& + \frac{3}{8} \delta^{pa} Y_d^{*cd} Y_u^{*rb} (Y_d Y_d^\dagger)^{st} + \frac{3}{8} \delta^{sc} Y_d^{*td} Y_u^{*ab} (Y_u Y_u^\dagger)^{pr} + \frac{3}{8} \delta^{pc} Y_d^{*rd} Y_u^{*ab} (Y_u Y_u^\dagger)^{st} + g_L^2 \left( \frac{1}{12} \delta^{pa} \delta^{st} Y_d^{*cd} Y_u^{*rb} + \frac{1}{12} \delta^{pc} \delta^{st} Y_d^{*rd} Y_u^{*ab} \right. \\
& + \frac{1}{12} \delta^{pr} \delta^{sa} Y_d^{*cd} Y_u^{*tb} + \frac{1}{12} \delta^{pr} \delta^{sc} Y_d^{*td} Y_u^{*ab} - \frac{7}{144} \delta^{pa} \delta^{st} Y_d^{*rd} Y_u^{*cb} - \frac{7}{144} \delta^{pc} \delta^{st} Y_d^{*ad} Y_u^{*rb} - \frac{7}{144} \delta^{pr} \delta^{sa} Y_d^{*td} Y_u^{*cb} - \frac{7}{144} \delta^{pr} \delta^{sc} Y_d^{*ad} Y_u^{*tb} \\
& - \frac{21}{32} \delta^{pc} \delta^{sa} Y_d^{*rd} Y_u^{*tb} - \frac{21}{32} \delta^{pa} \delta^{sc} Y_d^{*td} Y_u^{*rb} \left. \right) + g_Y^2 \left( \frac{7}{1296} \delta^{pc} \delta^{st} Y_d^{*ad} Y_u^{*rb} + \frac{7}{1296} \delta^{pr} \delta^{sc} Y_d^{*ad} Y_u^{*tb} + \frac{11}{108} \delta^{pa} \delta^{st} Y_d^{*cd} Y_u^{*rb} \right. \\
& + \frac{11}{108} \delta^{pr} \delta^{sa} Y_d^{*cd} Y_u^{*tb} - \frac{11}{1296} \delta^{pa} \delta^{st} Y_d^{*rd} Y_u^{*cb} - \frac{11}{1296} \delta^{pr} \delta^{sa} Y_d^{*td} Y_u^{*cb} - \frac{7}{108} \delta^{pc} \delta^{st} Y_d^{*rd} Y_u^{*ab} - \frac{7}{108} \delta^{pr} \delta^{sc} Y_d^{*td} Y_u^{*ab} \\
& - \frac{37}{96} \delta^{pc} \delta^{sa} Y_d^{*rd} Y_u^{*tb} - \frac{37}{96} \delta^{pa} \delta^{sc} Y_d^{*td} Y_u^{*rb} \left. \right) + g_s^2 \left( \frac{1}{108} \delta^{pa} \delta^{st} Y_d^{*rd} Y_u^{*cb} + \frac{1}{108} \delta^{pc} \delta^{st} Y_d^{*ad} Y_u^{*rb} + \frac{1}{108} \delta^{pr} \delta^{sa} Y_d^{*td} Y_u^{*cb} + \frac{1}{108} \delta^{pr} \delta^{sc} Y_d^{*ad} Y_u^{*tb} \right. \\
& + \frac{17}{8} \delta^{pc} \delta^{sa} Y_d^{*rd} Y_u^{*tb} + \frac{17}{8} \delta^{pa} \delta^{sc} Y_d^{*td} Y_u^{*rb} - \frac{1}{9} \delta^{pa} \delta^{st} Y_d^{*cd} Y_u^{*rb} - \frac{1}{9} \delta^{pc} \delta^{st} Y_d^{*rd} Y_u^{*ab} - \frac{1}{9} \delta^{pr} \delta^{sa} Y_d^{*cd} Y_u^{*tb} - \frac{1}{9} \delta^{pr} \delta^{sc} Y_d^{*td} Y_u^{*ab} \\
& - \frac{13}{8} \delta^{pc} \delta^{sa} Y_d^{*td} Y_u^{*rb} - \frac{13}{8} \delta^{pa} \delta^{sc} Y_d^{*rd} Y_u^{*tb} \left. \right\} C_{quqd}^{(\parallel)abcd} + \left( C_{quqd}^{(\parallel)*} \right)^{abcd} \left\{ \frac{1}{16} \delta^{tc} Y_d^{*ad} Y_u^{*sb} (Y_d Y_d^\dagger)^{pr} + \frac{1}{16} \delta^{rc} Y_d^{*ad} Y_u^{*pb} (Y_d Y_d^\dagger)^{st} + \frac{1}{16} \delta^{ta} Y_d^{*sd} Y_u^{*cb} (Y_u Y_u^\dagger)^{pr} \right. \\
& + \frac{1}{16} \delta^{ra} Y_d^{*pd} Y_u^{*cb} (Y_u Y_u^\dagger)^{st} + \frac{1}{8} T_2 \delta^{rc} \delta^{ta} Y_d^{*pd} Y_u^{*sb} + \frac{1}{8} T_2 \delta^{ra} \delta^{tc} Y_d^{*sd} Y_u^{*pb} + \frac{1}{8} \delta^{rc} \delta^{ta} Y_u^{*sb} (Y_d Y_d^\dagger Y_d)^{pd} + \frac{1}{8} \delta^{ra} \delta^{tc} Y_u^{*pb} (Y_d Y_d^\dagger Y_d)^{sd} \\
& + \frac{1}{8} \delta^{ra} \delta^{tc} Y_d^{*sd} (Y_d Y_d^\dagger Y_u)^{pb} + \frac{1}{8} \delta^{rc} \delta^{ta} Y_d^{*pd} (Y_d Y_d^\dagger Y_u)^{sb} + \frac{1}{8} \delta^{rc} \delta^{ta} Y_u^{*sb} (Y_u Y_u^\dagger Y_d)^{pd} + \frac{1}{8} \delta^{ra} \delta^{tc} Y_u^{*pb} (Y_u Y_u^\dagger Y_d)^{sd} + \frac{1}{8} \delta^{ra} \delta^{tc} Y_d^{*sd} (Y_u Y_u^\dagger Y_u)^{pb} \\
& + \frac{1}{8} \delta^{rc} \delta^{ta} Y_d^{*pd} (Y_u Y_u^\dagger Y_u)^{sb} + \frac{5}{16} \delta^{ta} Y_d^{*pd} Y_u^{*sb} (Y_d Y_d^\dagger)^{cr} + \frac{5}{16} \delta^{ra} Y_d^{*sd} Y_u^{*pb} (Y_d Y_d^\dagger)^{ct} + \frac{5}{16} \delta^{tc} Y_d^{*sd} Y_u^{*pb} (Y_u Y_u^\dagger)^{ar} + \frac{5}{16} \delta^{rc} Y_d^{*pd} Y_u^{*sb} (Y_u Y_u^\dagger)^{at} + \frac{3}{8} \delta^{ta} Y_d^{*cd} Y_u^{*sb} (Y_d Y_d^\dagger)^{pr} \\
& + \frac{3}{8} \delta^{ra} Y_d^{*cd} Y_u^{*pb} (Y_d Y_d^\dagger)^{st} + \frac{3}{8} \delta^{tc} Y_d^{*sd} Y_u^{*ab} (Y_u Y_u^\dagger)^{pr} + \frac{3}{8} \delta^{rc} Y_d^{*pd} Y_u^{*ab} (Y_u Y_u^\dagger)^{st} + g_L^2 \left( \frac{1}{12} \delta^{ra} \delta^{st} Y_d^{*cd} Y_u^{*pb} + \frac{1}{12} \delta^{rc} \delta^{st} Y_d^{*pd} Y_u^{*ab} + \frac{1}{12} \delta^{pr} \delta^{ta} Y_d^{*cd} Y_u^{*sb} \right.
\end{aligned}$$

$$\begin{aligned}
& + \frac{1}{12} \delta^{pr} \delta^{tc} Y_d^{sd} Y_u^{ab} - \frac{7}{144} \delta^{ra} \delta^{st} Y_d^{pd} Y_u^{cb} - \frac{7}{144} \delta^{rc} \delta^{st} Y_d^{ad} Y_u^{pb} - \frac{7}{144} \delta^{pr} \delta^{ta} Y_d^{sd} Y_u^{cb} - \frac{7}{144} \delta^{pr} \delta^{tc} Y_d^{ad} Y_u^{sb} - \frac{21}{32} \delta^{rc} \delta^{ta} Y_d^{pd} Y_u^{sb} - \frac{21}{32} \delta^{ra} \delta^{tc} Y_d^{sd} Y_u^{pb} \\
& + g_Y^2 \left( \frac{7}{1296} \delta^{rc} \delta^{st} Y_d^{ad} Y_u^{pb} + \frac{7}{1296} \delta^{pr} \delta^{tc} Y_d^{ad} Y_u^{sb} + \frac{11}{108} \delta^{ra} \delta^{st} Y_d^{cd} Y_u^{pb} + \frac{11}{108} \delta^{pr} \delta^{ta} Y_d^{cd} Y_u^{sb} - \frac{11}{1296} \delta^{ra} \delta^{st} Y_d^{pd} Y_u^{cb} - \frac{11}{1296} \delta^{pr} \delta^{ta} Y_d^{sd} Y_u^{cb} \right. \\
& - \frac{7}{108} \delta^{rc} \delta^{st} Y_d^{pd} Y_u^{ab} - \frac{7}{108} \delta^{pr} \delta^{tc} Y_d^{sd} Y_u^{ab} - \frac{37}{96} \delta^{rc} \delta^{ta} Y_d^{pd} Y_u^{sb} - \frac{37}{96} \delta^{ra} \delta^{tc} Y_d^{sd} Y_u^{pb} \Big) + g_s^2 \left( \frac{1}{108} \delta^{ra} \delta^{st} Y_d^{pd} Y_u^{cb} + \frac{1}{108} \delta^{rc} \delta^{st} Y_d^{ad} Y_u^{pb} \right. \\
& + \frac{1}{108} \delta^{pr} \delta^{ta} Y_d^{sd} Y_u^{cb} + \frac{1}{108} \delta^{pr} \delta^{tc} Y_d^{ad} Y_u^{sb} + \frac{17}{8} \delta^{rc} \delta^{ta} Y_d^{pd} Y_u^{sb} + \frac{17}{8} \delta^{ra} \delta^{tc} Y_d^{sd} Y_u^{pb} - \frac{1}{9} \delta^{ra} \delta^{st} Y_d^{cd} Y_u^{pb} - \frac{1}{9} \delta^{rc} \delta^{st} Y_d^{pd} Y_u^{ab} - \frac{1}{9} \delta^{pr} \delta^{ta} Y_d^{cd} Y_u^{sb} \\
& \left. - \frac{1}{9} \delta^{pr} \delta^{tc} Y_d^{sd} Y_u^{ab} - \frac{13}{8} \delta^{rc} \delta^{ta} Y_d^{sd} Y_u^{pb} - \frac{13}{8} \delta^{ra} \delta^{tc} Y_d^{pd} Y_u^{sb} \right) \Bigg\} + \left\{ \frac{1}{8} \delta^{sa} Y_d^{*cd} Y_u^{*tb} (Y_d Y_d^\dagger)^{pr} + \frac{1}{8} \delta^{sc} Y_d^{*rd} Y_u^{*tb} (Y_d Y_d^\dagger)^{pa} + \frac{1}{8} \delta^{pa} Y_d^{*cd} Y_u^{*rb} (Y_d Y_d^\dagger)^{st} \right. \\
& + \frac{1}{8} \delta^{pc} Y_d^{*td} Y_u^{*rb} (Y_d Y_d^\dagger)^{sa} + \frac{1}{8} \delta^{sc} Y_d^{*td} Y_u^{*ab} (Y_u Y_u^\dagger)^{pr} + \frac{1}{8} \delta^{sa} Y_d^{*td} Y_u^{*rb} (Y_u Y_u^\dagger)^{pc} + \frac{1}{8} \delta^{pc} Y_d^{*rd} Y_u^{*ab} (Y_u Y_u^\dagger)^{st} + \frac{1}{8} \delta^{pa} Y_d^{*rd} Y_u^{*tb} (Y_u Y_u^\dagger)^{sc} \\
& + \frac{3}{16} \delta^{sc} Y_d^{*ad} Y_u^{*tb} (Y_d Y_d^\dagger)^{pr} + \frac{3}{16} \delta^{pc} Y_d^{*ad} Y_u^{*rb} (Y_d Y_d^\dagger)^{st} + \frac{3}{16} \delta^{sa} Y_d^{*td} Y_u^{*cb} (Y_u Y_u^\dagger)^{pr} + \frac{3}{16} \delta^{pa} Y_d^{*rd} Y_u^{*cb} (Y_u Y_u^\dagger)^{st} + g_s^2 \left( \frac{7}{4} \delta^{pc} \delta^{sa} Y_d^{*rd} Y_u^{*tb} \right. \\
& + \frac{7}{4} \delta^{pa} \delta^{sc} Y_d^{*td} Y_u^{*rb} - \frac{1}{18} \delta^{pa} \delta^{st} Y_d^{*rd} Y_u^{*cb} - \frac{1}{18} \delta^{pc} \delta^{st} Y_d^{*ad} Y_u^{*rb} - \frac{1}{18} \delta^{pr} \delta^{sa} Y_d^{*td} Y_u^{*cb} - \frac{1}{18} \delta^{pr} \delta^{sc} Y_d^{*ad} Y_u^{*tb} - \frac{7}{108} \delta^{pa} \delta^{st} Y_d^{*cd} Y_u^{*rb} \\
& - \frac{7}{108} \delta^{pc} \delta^{st} Y_d^{*rd} Y_u^{*ab} - \frac{7}{108} \delta^{pr} \delta^{sa} Y_d^{*cd} Y_u^{*tb} - \frac{7}{108} \delta^{pr} \delta^{sc} Y_d^{*td} Y_u^{*ab} - \frac{7}{4} \delta^{pc} \delta^{sa} Y_d^{*td} Y_u^{*rb} - \frac{7}{4} \delta^{pa} \delta^{sc} Y_d^{*rd} Y_u^{*tb} \Big) + g_Y^2 \left( \frac{13}{432} \delta^{pc} \delta^{st} Y_d^{*ad} Y_u^{*rb} \right. \\
& + \frac{13}{432} \delta^{pr} \delta^{sc} Y_d^{*ad} Y_u^{*tb} + \frac{25}{648} \delta^{pa} \delta^{st} Y_d^{*cd} Y_u^{*rb} + \frac{25}{648} \delta^{pr} \delta^{sa} Y_d^{*cd} Y_u^{*tb} + \frac{37}{96} \delta^{pc} \delta^{sa} Y_d^{*td} Y_u^{*rb} + \frac{37}{96} \delta^{pa} \delta^{sc} Y_d^{*rd} Y_u^{*tb} - \frac{5}{432} \delta^{pa} \delta^{st} Y_d^{*rd} Y_u^{*cb} \\
& - \frac{5}{432} \delta^{pr} \delta^{sa} Y_d^{*td} Y_u^{*cb} - \frac{11}{648} \delta^{pc} \delta^{st} Y_d^{*rd} Y_u^{*ab} - \frac{11}{648} \delta^{pr} \delta^{sc} Y_d^{*td} Y_u^{*ab} \Big) + g_L^2 \left( \frac{5}{72} \delta^{pa} \delta^{st} Y_d^{*cd} Y_u^{*rb} + \frac{5}{72} \delta^{pc} \delta^{st} Y_d^{*rd} Y_u^{*ab} + \frac{5}{72} \delta^{pr} \delta^{sa} Y_d^{*cd} Y_u^{*tb} \right. \\
& + \frac{5}{72} \delta^{pr} \delta^{sc} Y_d^{*td} Y_u^{*ab} + \frac{21}{32} \delta^{pc} \delta^{sa} Y_d^{*td} Y_u^{*rb} + \frac{21}{32} \delta^{pa} \delta^{sc} Y_d^{*rd} Y_u^{*tb} - \frac{1}{48} \delta^{pa} \delta^{st} Y_d^{*rd} Y_u^{*cb} - \frac{1}{48} \delta^{pc} \delta^{st} Y_d^{*ad} Y_u^{*rb} - \frac{1}{48} \delta^{pr} \delta^{sa} Y_d^{*td} Y_u^{*cb} \\
& - \frac{1}{48} \delta^{pr} \delta^{sc} Y_d^{*ad} Y_u^{*tb} \Big) - \frac{1}{8} T_2 \delta^{pc} \delta^{sa} Y_d^{*td} Y_u^{*rb} - \frac{1}{8} T_2 \delta^{pa} \delta^{sc} Y_d^{*rd} Y_u^{*tb} - \frac{1}{8} \delta^{pa} \delta^{sc} Y_u^{*tb} (Y_d^\dagger Y_d Y_d^\dagger)^{rd} - \frac{1}{8} \delta^{pc} \delta^{sa} Y_u^{*rb} (Y_d^\dagger Y_d Y_d^\dagger)^{td} \\
& - \frac{1}{8} \delta^{pc} \delta^{sa} Y_d^{*td} (Y_d^\dagger Y_d Y_u^\dagger)^{rb} - \frac{1}{8} \delta^{pa} \delta^{sc} Y_d^{*rd} (Y_d^\dagger Y_d Y_u^\dagger)^{tb} - \frac{1}{8} \delta^{pa} \delta^{sc} Y_u^{*tb} (Y_u^\dagger Y_u Y_d^\dagger)^{rd} - \frac{1}{8} \delta^{pc} \delta^{sa} Y_u^{*rb} (Y_u^\dagger Y_u Y_d^\dagger)^{td} - \frac{1}{8} \delta^{pc} \delta^{sa} Y_d^{*td} (Y_u^\dagger Y_u Y_u^\dagger)^{rb} \\
& \left. - \frac{1}{8} \delta^{pa} \delta^{sc} Y_d^{*rd} (Y_u^\dagger Y_u Y_u^\dagger)^{tb} \right\} C_{quqd}^{(\times)abcd} + \left( C_{quqd}^{(\times)*} \right)^{abcd} \left\{ \frac{1}{8} \delta^{ta} Y_d^{*cd} Y_u^{*sb} (Y_d Y_d^\dagger)^{pr} + \frac{1}{8} \delta^{ra} Y_d^{*cd} Y_u^{*pb} (Y_d Y_d^\dagger)^{st} + \frac{1}{8} \delta^{tc} Y_d^{*pd} Y_u^{*sb} (Y_d Y_d^\dagger)^{ar} + \frac{1}{8} \delta^{rc} Y_d^{*sd} Y_u^{*pb} (Y_d Y_d^\dagger)^{st} \right. \\
& + \frac{1}{8} \delta^{tc} Y_d^{*sd} Y_u^{*ab} (Y_u Y_u^\dagger)^{pr} + \frac{1}{8} \delta^{rc} Y_d^{*pd} Y_u^{*ab} (Y_u Y_u^\dagger)^{st} + \frac{1}{8} \delta^{ta} Y_d^{*sd} Y_u^{*pb} (Y_u Y_u^\dagger)^{cr} + \frac{1}{8} \delta^{ra} Y_d^{*pd} Y_u^{*sb} (Y_u Y_u^\dagger)^{ct} + \frac{3}{16} \delta^{tc} Y_d^{*ad} Y_u^{*sb} (Y_d Y_d^\dagger)^{pr} + \frac{3}{16} \delta^{rc} Y_d^{*ad} Y_u^{*pb} (Y_d Y_d^\dagger)^{st} \\
& + \frac{3}{16} \delta^{ta} Y_d^{*sd} Y_u^{*cb} (Y_u Y_u^\dagger)^{pr} + \frac{3}{16} \delta^{ra} Y_d^{*pd} Y_u^{*cb} (Y_u Y_u^\dagger)^{st} + g_s^2 \left( \frac{7}{4} \delta^{rc} \delta^{ta} Y_d^{*pd} Y_u^{*sb} + \frac{7}{4} \delta^{ra} \delta^{tc} Y_d^{*sd} Y_u^{*pb} - \frac{1}{18} \delta^{ra} \delta^{st} Y_d^{*pd} Y_u^{*cb} - \frac{1}{18} \delta^{rc} \delta^{st} Y_d^{*ad} Y_u^{*pb} - \frac{1}{18} \delta^{pr} \delta^{ta} Y_d^{*sd} Y_u^{*cb} \right. \\
& - \frac{1}{18} \delta^{pr} \delta^{tc} Y_d^{*ad} Y_u^{*sb} - \frac{7}{108} \delta^{ra} \delta^{st} Y_d^{*cd} Y_u^{*pb} - \frac{7}{108} \delta^{rc} \delta^{st} Y_d^{*pd} Y_u^{*ab} - \frac{7}{108} \delta^{pr} \delta^{ta} Y_d^{*cd} Y_u^{*sb} - \frac{7}{108} \delta^{pr} \delta^{tc} Y_d^{*sd} Y_u^{*ab} - \frac{7}{4} \delta^{rc} \delta^{ta} Y_d^{*sd} Y_u^{*pb} - \frac{7}{4} \delta^{ra} \delta^{tc} Y_d^{*pd} Y_u^{*sb} \Big) \\
& \left. + g_Y^2 \left( \frac{13}{432} \delta^{rc} \delta^{st} Y_d^{*ad} Y_u^{*pb} + \frac{13}{432} \delta^{pr} \delta^{tc} Y_d^{*ad} Y_u^{*sb} + \frac{25}{648} \delta^{ra} \delta^{st} Y_d^{*cd} Y_u^{*pb} + \frac{25}{648} \delta^{pr} \delta^{ta} Y_d^{*cd} Y_u^{*sb} + \frac{37}{96} \delta^{rc} \delta^{ta} Y_d^{*sd} Y_u^{*pb} + \frac{37}{96} \delta^{ra} \delta^{tc} Y_d^{*pd} Y_u^{*sb} \right) \right\}
\end{aligned}$$



$$\begin{aligned}
& -\frac{5}{432}\delta^{ra}\delta^{st}Y_d^{pd}Y_u^{cb}-\frac{5}{432}\delta^{pr}\delta^{ta}Y_d^{sd}Y_u^{cb}-\frac{11}{648}\delta^{rc}\delta^{st}Y_d^{pd}Y_u^{ab}-\frac{11}{648}\delta^{pr}\delta^{tc}Y_d^{sd}Y_u^{ab})+g_L^2\left(\frac{5}{72}\delta^{ra}\delta^{st}Y_d^{cd}Y_u^{pb}+\frac{5}{72}\delta^{rc}\delta^{st}Y_d^{pd}Y_u^{ab}+\frac{5}{72}\delta^{pr}\delta^{ta}Y_d^{cd}Y_u^{sb}\right. \\
& +\frac{5}{72}\delta^{pr}\delta^{tc}Y_d^{sd}Y_u^{ab}+\frac{21}{32}\delta^{rc}\delta^{ta}Y_d^{sd}Y_u^{pb}+\frac{21}{32}\delta^{ra}\delta^{tc}Y_d^{pd}Y_u^{sb}-\frac{1}{48}\delta^{ra}\delta^{st}Y_d^{pd}Y_u^{cb}-\frac{1}{48}\delta^{rc}\delta^{st}Y_d^{ad}Y_u^{pb}-\frac{1}{48}\delta^{pr}\delta^{ta}Y_d^{sd}Y_u^{cb}-\frac{1}{48}\delta^{pr}\delta^{tc}Y_d^{ad}Y_u^{sb}) \\
& -\frac{1}{8}T_2\delta^{rc}\delta^{ta}Y_d^{sd}Y_u^{pb}-\frac{1}{8}T_2\delta^{ra}\delta^{tc}Y_d^{pd}Y_u^{sb}-\frac{1}{8}\delta^{ra}\delta^{tc}Y_u^{sb}(Y_dY_d^\dagger Y_d)^{pd}-\frac{1}{8}\delta^{rc}\delta^{ta}Y_u^{pb}(Y_dY_d^\dagger Y_d)^{sd}-\frac{1}{8}\delta^{rc}\delta^{ta}Y_d^{sd}(Y_dY_d^\dagger Y_u)^{pb} \\
& \left.-\frac{1}{8}\delta^{ra}\delta^{tc}Y_d^{pd}(Y_dY_d^\dagger Y_u)^{sb}-\frac{1}{8}\delta^{ra}\delta^{tc}Y_u^{sb}(Y_uY_u^\dagger Y_d)^{pd}-\frac{1}{8}\delta^{rc}\delta^{ta}Y_u^{pb}(Y_uY_u^\dagger Y_d)^{sd}-\frac{1}{8}\delta^{rc}\delta^{ta}Y_d^{sd}(Y_uY_u^\dagger Y_u)^{pb}-\frac{1}{8}\delta^{ra}\delta^{tc}Y_d^{pd}(Y_uY_u^\dagger Y_u)^{sb}\right\} \\
& +\left\{g_s^2\left(\frac{1}{27}\delta^{pc}\delta^{st}Y_e^{*ab}Y_u^{*rd}+\frac{1}{27}\delta^{pr}\delta^{sc}Y_e^{*ab}Y_u^{*td}\right)-\frac{1}{8}\delta^{sc}Y_e^{*ab}Y_u^{*td}(Y_dY_d^\dagger)^{pr}-\frac{1}{8}\delta^{pc}Y_e^{*ab}Y_u^{*rd}(Y_dY_d^\dagger)^{st}-g_L^2\left(\frac{1}{36}\delta^{pc}\delta^{st}Y_e^{*ab}Y_u^{*rd}\right.\right. \\
& \left.+\frac{1}{36}\delta^{pr}\delta^{sc}Y_e^{*ab}Y_u^{*td}\right)-g_Y^2\left(\frac{11}{324}\delta^{pc}\delta^{st}Y_e^{*ab}Y_u^{*rd}+\frac{11}{324}\delta^{pr}\delta^{sc}Y_e^{*ab}Y_u^{*td}\right)\Big\}C_{lequ}^{abcd}+C_{lequ}^{*abcd}\left\{g_s^2\left(\frac{1}{27}\delta^{rc}\delta^{st}Y_e^{ab}Y_u^{pd}+\frac{1}{27}\delta^{pr}\delta^{tc}Y_e^{ab}Y_u^{sd}\right)\right. \\
& \left.-\frac{1}{8}\delta^{tc}Y_e^{ab}Y_u^{sd}(Y_dY_d^\dagger)^{pr}-\frac{1}{8}\delta^{rc}Y_e^{ab}Y_u^{pd}(Y_dY_d^\dagger)^{st}-g_L^2\left(\frac{1}{36}\delta^{rc}\delta^{st}Y_e^{ab}Y_u^{pd}+\frac{1}{36}\delta^{pr}\delta^{tc}Y_e^{ab}Y_u^{sd}\right)-g_Y^2\left(\frac{11}{324}\delta^{rc}\delta^{st}Y_e^{ab}Y_u^{pd}+\frac{11}{324}\delta^{pr}\delta^{tc}Y_e^{ab}Y_u^{sd}\right)\right\} \\
& +\left\{\frac{1}{16}\delta^{sc}Y_e^{*ad}Y_u^{*tb}(Y_dY_d^\dagger)^{pr}+\frac{1}{16}\delta^{pc}Y_e^{*ad}Y_u^{*rb}(Y_dY_d^\dagger)^{st}+g_Y^2\left(\frac{13}{1296}\delta^{pc}\delta^{st}Y_e^{*ad}Y_u^{*rb}+\frac{13}{1296}\delta^{pr}\delta^{sc}Y_e^{*ad}Y_u^{*tb}\right)-g_L^2\left(\frac{1}{144}\delta^{pc}\delta^{st}Y_e^{*ad}Y_u^{*rb}\right.\right. \\
& \left.+\frac{1}{144}\delta^{pr}\delta^{sc}Y_e^{*ad}Y_u^{*tb}\right)-g_s^2\left(\frac{1}{54}\delta^{pc}\delta^{st}Y_e^{*ad}Y_u^{*rb}+\frac{1}{54}\delta^{pr}\delta^{sc}Y_e^{*ad}Y_u^{*tb}\right)\Big\}C_{luqe}^{abcd}+C_{luqe}^{*abcd}\left\{\frac{1}{16}\delta^{tc}Y_e^{ad}Y_u^{sb}(Y_dY_d^\dagger)^{pr}+\frac{1}{16}\delta^{rc}Y_e^{ad}Y_u^{pb}(Y_dY_d^\dagger)^{st}\right. \\
& \left.+g_Y^2\left(\frac{13}{1296}\delta^{rc}\delta^{st}Y_e^{ad}Y_u^{pb}+\frac{13}{1296}\delta^{pr}\delta^{tc}Y_e^{ad}Y_u^{sb}\right)-g_L^2\left(\frac{1}{144}\delta^{rc}\delta^{st}Y_e^{ad}Y_u^{pb}+\frac{1}{144}\delta^{pr}\delta^{tc}Y_e^{ad}Y_u^{sb}\right)-g_s^2\left(\frac{1}{54}\delta^{rc}\delta^{st}Y_e^{ad}Y_u^{pb}+\frac{1}{54}\delta^{pr}\delta^{tc}Y_e^{ad}Y_u^{sb}\right)\right\} \\
& +\left\{\frac{2}{81}\delta^{pr}\delta^{st}\delta^{ad}\delta^{bc}g_Y^4-\frac{2}{9}\delta^{pr}\delta^{st}\delta^{ad}\delta^{bc}g_L^4\right\}C_{\ell\ell}^{abcd}+\left\{g_s^2g_L^2\left(\frac{166}{81}\delta^{pa}\delta^{rd}\delta^{st}\delta^{bc}+\frac{166}{81}\delta^{pr}\delta^{sa}\delta^{td}\delta^{bc}+\frac{32}{3}\delta^{pt}\delta^{rd}\delta^{sa}\delta^{bc}+\frac{32}{3}\delta^{pa}\delta^{rs}\delta^{td}\delta^{bc}\right.\right. \\
& +\frac{59}{2}\delta^{pa}\delta^{rb}\delta^{sc}\delta^{td}-21\delta^{pa}\delta^{rd}\delta^{sc}\delta^{tb})+g_Y^4\left(\frac{2}{243}\delta^{pr}\delta^{st}\delta^{ad}\delta^{bc}+\frac{43}{4374}\delta^{pa}\delta^{rd}\delta^{st}\delta^{bc}+\frac{43}{4374}\delta^{pr}\delta^{sa}\delta^{td}\delta^{bc}+\frac{37}{729}\delta^{pa}\delta^{rb}\delta^{st}\delta^{cd}\right. \\
& +\frac{37}{729}\delta^{pr}\delta^{sa}\delta^{tb}\delta^{cd}+\frac{17}{72}\delta^{pa}\delta^{rb}\delta^{sc}\delta^{td})+g_Y^2g_L^2\left(\frac{53}{81}\delta^{pa}\delta^{rb}\delta^{st}\delta^{cd}+\frac{53}{81}\delta^{pr}\delta^{sa}\delta^{tb}\delta^{cd}-\frac{101}{243}\delta^{pa}\delta^{rd}\delta^{st}\delta^{bc}-\frac{101}{243}\delta^{pr}\delta^{sa}\delta^{td}\delta^{bc}\right. \\
& -\frac{5}{12}\delta^{pa}\delta^{rb}\delta^{sc}\delta^{td})+g_Y^2g_s^2\left(\frac{187}{243}\delta^{pa}\delta^{rb}\delta^{st}\delta^{cd}+\frac{187}{243}\delta^{pr}\delta^{sa}\delta^{tb}\delta^{cd}-\frac{4}{81}\delta^{pr}\delta^{st}\delta^{ad}\delta^{bc}-\frac{104}{729}\delta^{pa}\delta^{rd}\delta^{st}\delta^{bc}-\frac{104}{729}\delta^{pr}\delta^{sa}\delta^{td}\delta^{bc}\right. \\
& \left.-\frac{35}{18}\delta^{pa}\delta^{rb}\delta^{sc}\delta^{td})+g_L^4\left(14\delta^{pa}\delta^{rb}\delta^{st}\delta^{cd}+14\delta^{pr}\delta^{sa}\delta^{tb}\delta^{cd}-\frac{7}{18}\delta^{pa}\delta^{rd}\delta^{st}\delta^{bc}-\frac{7}{18}\delta^{pr}\delta^{sa}\delta^{td}\delta^{bc}-\frac{2}{3}\delta^{pr}\delta^{st}\delta^{ad}\delta^{bc}-\frac{385}{24}\delta^{pa}\delta^{rb}\delta^{sc}\delta^{td}\right) \\
& \left.+g_s^4\left(\frac{158}{9}\delta^{pa}\delta^{rb}\delta^{st}\delta^{cd}+\frac{158}{9}\delta^{pr}\delta^{sa}\delta^{tb}\delta^{cd}-\frac{94}{243}\delta^{pa}\delta^{rd}\delta^{st}\delta^{bc}-\frac{94}{243}\delta^{pr}\delta^{sa}\delta^{td}\delta^{bc}-\frac{71}{6}\delta^{pa}\delta^{rb}\delta^{sc}\delta^{td}\right)+\delta^{sa}\delta^{tb}(Y_dY_d^\dagger)^{dr}(Y_uY_u^\dagger)^{pc}\right.
\end{aligned}$$

$$\begin{aligned}
& + \delta^{pa} \delta^{rb} (Y_d Y_d^\dagger)^{dt} (Y_u Y_u^\dagger)^{sc} + \delta^{sa} \delta^{tb} (Y_d Y_d^\dagger)^{pc} (Y_u Y_u^\dagger)^{dr} + \delta^{pa} \delta^{rb} (Y_d Y_d^\dagger)^{sc} (Y_u Y_u^\dagger)^{dt} + g_s^2 \left( \frac{5}{9} \delta^{pa} \delta^{rd} \delta^{st} (Y_d Y_d^\dagger)^{bc} + \frac{5}{9} \delta^{pr} \delta^{sa} \delta^{td} (Y_d Y_d^\dagger)^{bc} \right. \\
& + \frac{5}{9} \delta^{pa} \delta^{rd} \delta^{st} (Y_u Y_u^\dagger)^{bc} + \frac{5}{9} \delta^{pr} \delta^{sa} \delta^{td} (Y_u Y_u^\dagger)^{bc} - \frac{5}{3} \delta^{rd} \delta^{sa} \delta^{tb} (Y_d Y_d^\dagger)^{pc} - \frac{5}{3} \delta^{pa} \delta^{rb} \delta^{td} (Y_d Y_d^\dagger)^{sc} - \frac{5}{3} \delta^{pa} \delta^{sc} \delta^{td} (Y_d Y_d^\dagger)^{br} - \frac{5}{3} \delta^{pa} \delta^{rb} \delta^{sc} (Y_d Y_d^\dagger)^{dt} \\
& - \frac{5}{3} \delta^{rd} \delta^{sa} \delta^{tb} (Y_u Y_u^\dagger)^{pc} - \frac{5}{3} \delta^{pa} \delta^{rb} \delta^{td} (Y_u Y_u^\dagger)^{sc} - \frac{5}{3} \delta^{pa} \delta^{sc} \delta^{td} (Y_u Y_u^\dagger)^{br} - \frac{5}{3} \delta^{pa} \delta^{rb} \delta^{sc} (Y_u Y_u^\dagger)^{dt} \Big) + g_L^2 \left( \frac{2}{3} \delta^{pa} \delta^{rd} \delta^{st} (Y_d Y_d^\dagger)^{bc} + \frac{2}{3} \delta^{pr} \delta^{sa} \delta^{td} (Y_d Y_d^\dagger)^{bc} \right. \\
& + \frac{2}{3} \delta^{pa} \delta^{rd} \delta^{st} (Y_u Y_u^\dagger)^{bc} + \frac{2}{3} \delta^{pr} \delta^{sa} \delta^{td} (Y_u Y_u^\dagger)^{bc} + \frac{33}{16} \delta^{rd} \delta^{sa} \delta^{tb} (Y_d Y_d^\dagger)^{pc} + \frac{33}{16} \delta^{pa} \delta^{rb} \delta^{td} (Y_d Y_d^\dagger)^{sc} + \frac{33}{16} \delta^{pa} \delta^{sc} \delta^{td} (Y_d Y_d^\dagger)^{br} + \frac{33}{16} \delta^{pa} \delta^{rb} \delta^{sc} (Y_d Y_d^\dagger)^{dt} \\
& + \frac{33}{16} \delta^{rd} \delta^{sa} \delta^{tb} (Y_u Y_u^\dagger)^{pc} + \frac{33}{16} \delta^{pa} \delta^{rb} \delta^{td} (Y_u Y_u^\dagger)^{sc} + \frac{33}{16} \delta^{pa} \delta^{sc} \delta^{td} (Y_u Y_u^\dagger)^{br} + \frac{33}{16} \delta^{pa} \delta^{rb} \delta^{sc} (Y_u Y_u^\dagger)^{dt} \Big) + g_Y^2 \left( \frac{43}{144} \delta^{rd} \delta^{sa} \delta^{tb} (Y_u Y_u^\dagger)^{pc} \right. \\
& + \frac{43}{144} \delta^{pa} \delta^{rb} \delta^{td} (Y_u Y_u^\dagger)^{sc} + \frac{43}{144} \delta^{pa} \delta^{sc} \delta^{td} (Y_u Y_u^\dagger)^{br} + \frac{43}{144} \delta^{pa} \delta^{rb} \delta^{sc} (Y_u Y_u^\dagger)^{dt} + \frac{199}{144} \delta^{rd} \delta^{sa} \delta^{tb} (Y_d Y_d^\dagger)^{pc} + \frac{199}{144} \delta^{pa} \delta^{rb} \delta^{td} (Y_d Y_d^\dagger)^{sc} \\
& + \frac{199}{144} \delta^{pa} \delta^{sc} \delta^{td} (Y_d Y_d^\dagger)^{br} + \frac{199}{144} \delta^{pa} \delta^{rb} \delta^{sc} (Y_d Y_d^\dagger)^{dt} - \frac{1}{27} \delta^{pa} \delta^{rd} \delta^{st} (Y_d Y_d^\dagger)^{bc} - \frac{1}{27} \delta^{pr} \delta^{sa} \delta^{td} (Y_d Y_d^\dagger)^{bc} - \frac{4}{27} \delta^{pa} \delta^{rd} \delta^{st} (Y_u Y_u^\dagger)^{bc} \\
& - \frac{4}{27} \delta^{pr} \delta^{sa} \delta^{td} (Y_u Y_u^\dagger)^{bc} - \frac{2}{3} \delta^{pa} \delta^{rb} \delta^{st} (Y_u Y_u^\dagger)^{dc} - \frac{2}{3} \delta^{pr} \delta^{sa} \delta^{tb} (Y_u Y_u^\dagger)^{dc} \Big) + \frac{3}{2} \delta^{sa} \delta^{tb} (Y_d Y_d^\dagger)^{pr} (Y_d Y_d^\dagger)^{dc} + \frac{3}{2} \delta^{pa} \delta^{rb} (Y_d Y_d^\dagger)^{st} (Y_d Y_d^\dagger)^{dc} \\
& + \frac{3}{2} \delta^{sa} \delta^{tb} (Y_u Y_u^\dagger)^{pr} (Y_u Y_u^\dagger)^{dc} + \frac{3}{2} \delta^{pa} \delta^{rb} (Y_u Y_u^\dagger)^{st} (Y_u Y_u^\dagger)^{dc} - \frac{1}{4} \delta^{rd} \delta^{sa} \delta^{tb} (Y_d Y_d^\dagger Y_d Y_d^\dagger)^{pc} - \frac{1}{4} \delta^{pa} \delta^{rb} \delta^{td} (Y_d Y_d^\dagger Y_d Y_d^\dagger)^{sc} - \frac{1}{4} \delta^{pa} \delta^{sc} \delta^{td} (Y_d Y_d^\dagger Y_d Y_d^\dagger)^{br} \\
& - \frac{1}{4} \delta^{pa} \delta^{rb} \delta^{sc} (Y_d Y_d^\dagger Y_d Y_d^\dagger)^{dt} - \frac{1}{4} \delta^{rd} \delta^{sa} \delta^{tb} (Y_u Y_u^\dagger Y_u Y_u^\dagger)^{pc} - \frac{1}{4} \delta^{pa} \delta^{rb} \delta^{td} (Y_u Y_u^\dagger Y_u Y_u^\dagger)^{sc} - \frac{1}{4} \delta^{pa} \delta^{sc} \delta^{td} (Y_u Y_u^\dagger Y_u Y_u^\dagger)^{br} - \frac{1}{4} \delta^{pa} \delta^{rb} \delta^{sc} (Y_u Y_u^\dagger Y_u Y_u^\dagger)^{dt} \\
& - \frac{3}{4} T_2 \delta^{rd} \delta^{sa} \delta^{tb} (Y_d Y_d^\dagger)^{pc} - \frac{3}{4} T_2 \delta^{pa} \delta^{rb} \delta^{td} (Y_d Y_d^\dagger)^{sc} - \frac{3}{4} T_2 \delta^{pa} \delta^{sc} \delta^{td} (Y_d Y_d^\dagger)^{br} - \frac{3}{4} T_2 \delta^{pa} \delta^{rb} \delta^{sc} (Y_d Y_d^\dagger)^{dt} - \frac{3}{4} T_2 \delta^{rd} \delta^{sa} \delta^{tb} (Y_u Y_u^\dagger)^{pc} \\
& - \frac{3}{4} T_2 \delta^{pa} \delta^{rb} \delta^{td} (Y_u Y_u^\dagger)^{sc} - \frac{3}{4} T_2 \delta^{pa} \delta^{sc} \delta^{td} (Y_u Y_u^\dagger)^{br} - \frac{3}{4} T_2 \delta^{pa} \delta^{rb} \delta^{sc} (Y_u Y_u^\dagger)^{dt} - \delta^{rd} \delta^{sa} (Y_d Y_d^\dagger)^{bt} (Y_u Y_u^\dagger)^{pc} - \delta^{pa} \delta^{td} (Y_d Y_d^\dagger)^{br} (Y_u Y_u^\dagger)^{sc} \\
& - \delta^{pa} \delta^{td} (Y_d Y_d^\dagger)^{sc} (Y_u Y_u^\dagger)^{br} - \delta^{rd} \delta^{sa} (Y_d Y_d^\dagger)^{pc} (Y_u Y_u^\dagger)^{bt} - \frac{3}{2} \delta^{sa} \delta^{td} (Y_d Y_d^\dagger)^{bc} (Y_u Y_u^\dagger)^{pr} - \frac{3}{2} \delta^{sa} \delta^{tb} (Y_d Y_d^\dagger)^{dc} (Y_u Y_u^\dagger)^{pr} - \frac{3}{2} \delta^{pa} \delta^{rd} (Y_d Y_d^\dagger)^{bc} (Y_u Y_u^\dagger)^{st} \\
& - \frac{3}{2} \delta^{pa} \delta^{rb} (Y_d Y_d^\dagger)^{dc} (Y_u Y_u^\dagger)^{st} - \frac{3}{2} \delta^{sa} \delta^{td} (Y_d Y_d^\dagger)^{pr} (Y_u Y_u^\dagger)^{bc} - \frac{3}{2} \delta^{pa} \delta^{rd} (Y_d Y_d^\dagger)^{st} (Y_u Y_u^\dagger)^{bc} - \frac{3}{2} \delta^{sa} \delta^{tb} (Y_d Y_d^\dagger)^{pr} (Y_u Y_u^\dagger)^{dc} - \frac{3}{2} \delta^{pa} \delta^{rb} (Y_d Y_d^\dagger)^{st} (Y_u Y_u^\dagger)^{dc} \\
& - \frac{7}{4} \delta^{rd} \delta^{tb} (Y_d Y_d^\dagger)^{sa} (Y_u Y_u^\dagger)^{pc} - \frac{7}{4} \delta^{rb} \delta^{td} (Y_d Y_d^\dagger)^{pa} (Y_u Y_u^\dagger)^{sc} - \frac{7}{4} \delta^{pa} \delta^{sc} (Y_d Y_d^\dagger)^{dt} (Y_u Y_u^\dagger)^{br} - \frac{7}{4} \delta^{pa} \delta^{sc} (Y_d Y_d^\dagger)^{br} (Y_u Y_u^\dagger)^{dt} - \frac{5}{2} \delta^{sa} \delta^{tb} (Y_d Y_d^\dagger)^{pc} (Y_d Y_d^\dagger)^{dr} \\
& - \frac{5}{2} \delta^{pa} \delta^{rb} (Y_d Y_d^\dagger)^{sc} (Y_d Y_d^\dagger)^{dt} - \frac{5}{2} \delta^{sa} \delta^{tb} (Y_u Y_u^\dagger)^{pc} (Y_u Y_u^\dagger)^{dr} - \frac{5}{2} \delta^{pa} \delta^{rb} (Y_u Y_u^\dagger)^{sc} (Y_u Y_u^\dagger)^{dt} \Big\} C_{qq}^{(\parallel)abcd} + \left\{ g_s^2 g_L^2 \left( \frac{50}{81} \delta^{pa} \delta^{rd} \delta^{st} \delta^{bc} + \frac{50}{81} \delta^{pr} \delta^{sa} \delta^{td} \delta^{bc} \right. \right. \\
& + \delta^{pt} \delta^{rb} \delta^{sa} \delta^{cd} + \delta^{pa} \delta^{rs} \delta^{tb} \delta^{cd} + \frac{3}{2} \delta^{pa} \delta^{rd} \delta^{sc} \delta^{tb} + \frac{14}{3} \delta^{pt} \delta^{rd} \delta^{sa} \delta^{bc} + \frac{14}{3} \delta^{pa} \delta^{rs} \delta^{td} \delta^{bc} - \frac{17}{18} \delta^{pa} \delta^{rb} \delta^{st} \delta^{cd} - \frac{17}{18} \delta^{pr} \delta^{sa} \delta^{tb} \delta^{cd} \\
& - 14 \delta^{pa} \delta^{rb} \delta^{sc} \delta^{td} \Big) + g_Y^2 g_L^2 \left( \frac{20}{243} \delta^{pa} \delta^{rd} \delta^{st} \delta^{bc} + \frac{20}{243} \delta^{pr} \delta^{sa} \delta^{td} \delta^{bc} - \frac{53}{81} \delta^{pa} \delta^{rb} \delta^{st} \delta^{cd} - \frac{53}{81} \delta^{pr} \delta^{sa} \delta^{tb} \delta^{cd} - \frac{13}{6} \delta^{pa} \delta^{rb} \delta^{sc} \delta^{td} \right) \\
& + g_L^4 \left( \frac{17}{3} \delta^{pa} \delta^{rd} \delta^{st} \delta^{bc} + \frac{17}{3} \delta^{pr} \delta^{sa} \delta^{td} \delta^{bc} + \frac{49}{3} \delta^{pa} \delta^{rb} \delta^{sc} \delta^{td} - \frac{1}{6} \delta^{pa} \delta^{rb} \delta^{st} \delta^{cd} - \frac{1}{6} \delta^{pr} \delta^{sa} \delta^{tb} \delta^{cd} \right) + g_Y^4 \left( \frac{4}{243} \delta^{pr} \delta^{st} \delta^{ad} \delta^{bc} + \frac{43}{2187} \delta^{pa} \delta^{rd} \delta^{st} \delta^{bc} \right.
\end{aligned}$$

$$\begin{aligned}
& + \frac{43}{2187} \delta^{pr} \delta^{sa} \delta^{td} \delta^{bc} + \frac{37}{1458} \delta^{pa} \delta^{rb} \delta^{st} \delta^{cd} + \frac{37}{1458} \delta^{pr} \delta^{sa} \delta^{tb} \delta^{cd} \Big) + g_Y^2 g_s^2 \Big( \frac{187}{486} \delta^{pa} \delta^{rb} \delta^{st} \delta^{cd} + \frac{187}{486} \delta^{pr} \delta^{sa} \delta^{tb} \delta^{cd} - \frac{8}{81} \delta^{pr} \delta^{st} \delta^{ad} \delta^{bc} \\
& - \frac{208}{729} \delta^{pa} \delta^{rd} \delta^{st} \delta^{bc} - \frac{208}{729} \delta^{pr} \delta^{sa} \delta^{td} \delta^{bc} - \frac{13}{6} \delta^{pa} \delta^{rd} \delta^{sc} \delta^{tb} \Big) + g_s^4 \Big( \frac{15}{2} \delta^{pa} \delta^{rd} \delta^{sc} \delta^{tb} + \frac{79}{9} \delta^{pa} \delta^{rb} \delta^{st} \delta^{cd} + \frac{79}{9} \delta^{pr} \delta^{sa} \delta^{tb} \delta^{cd} - \frac{188}{243} \delta^{pa} \delta^{rd} \delta^{st} \delta^{bc} \\
& - \frac{188}{243} \delta^{pr} \delta^{sa} \delta^{td} \delta^{bc} \Big) + \delta^{sa} \delta^{tb} (Y_d Y_d^\dagger)^{dr} (Y_u Y_u^\dagger)^{pc} + \delta^{pa} \delta^{rb} (Y_d Y_d^\dagger)^{dt} (Y_u Y_u^\dagger)^{sc} + \delta^{sa} \delta^{tb} (Y_d Y_d^\dagger)^{pc} (Y_u Y_u^\dagger)^{dr} + g_s^2 \Big( \frac{10}{9} \delta^{pa} \delta^{rd} \delta^{st} (Y_d Y_d^\dagger)^{bc} \\
& + \frac{10}{9} \delta^{pr} \delta^{sa} \delta^{td} (Y_d Y_d^\dagger)^{bc} + \frac{10}{9} \delta^{pa} \delta^{rd} \delta^{st} (Y_u Y_u^\dagger)^{bc} + \frac{10}{9} \delta^{pr} \delta^{sa} \delta^{td} (Y_u Y_u^\dagger)^{bc} - 3 \delta^{rb} \delta^{sa} \delta^{td} (Y_d Y_d^\dagger)^{pc} - 3 \delta^{pa} \delta^{rd} \delta^{tb} (Y_d Y_d^\dagger)^{sc} - 3 \delta^{pa} \delta^{rd} \delta^{sc} (Y_d Y_d^\dagger)^{bt} \\
& - 3 \delta^{pa} \delta^{sc} \delta^{tb} (Y_d Y_d^\dagger)^{dr} - 3 \delta^{rb} \delta^{sa} \delta^{td} (Y_u Y_u^\dagger)^{pc} - 3 \delta^{pa} \delta^{rd} \delta^{tb} (Y_u Y_u^\dagger)^{sc} - 3 \delta^{pa} \delta^{rd} \delta^{sc} (Y_u Y_u^\dagger)^{bt} - 3 \delta^{pa} \delta^{sc} \delta^{tb} (Y_u Y_u^\dagger)^{dr} \Big) + \delta^{pa} \delta^{rb} (Y_d Y_d^\dagger)^{sc} (Y_u Y_u^\dagger)^{dt} \\
& + g_L^2 \Big( \delta^{pa} \delta^{rb} \delta^{st} (Y_d Y_d^\dagger)^{dc} + \delta^{pr} \delta^{sa} \delta^{tb} (Y_d Y_d^\dagger)^{dc} + \delta^{pa} \delta^{rb} \delta^{st} (Y_u Y_u^\dagger)^{dc} + \delta^{pr} \delta^{sa} \delta^{tb} (Y_u Y_u^\dagger)^{dc} \Big) + \frac{3}{2} \delta^{sa} \delta^{td} (Y_d Y_d^\dagger)^{pr} (Y_d Y_d^\dagger)^{bc} + \frac{3}{2} \delta^{pa} \delta^{rd} (Y_d Y_d^\dagger)^{st} (Y_d Y_d^\dagger)^{bc} \\
& + \frac{3}{2} \delta^{sa} \delta^{td} (Y_u Y_u^\dagger)^{pr} (Y_u Y_u^\dagger)^{bc} + \frac{3}{2} \delta^{pa} \delta^{rd} (Y_u Y_u^\dagger)^{st} (Y_u Y_u^\dagger)^{bc} + \frac{7}{4} \delta^{rd} \delta^{tb} (Y_d Y_d^\dagger)^{sa} (Y_u Y_u^\dagger)^{pc} + \frac{7}{4} \delta^{rb} \delta^{td} (Y_d Y_d^\dagger)^{pa} (Y_u Y_u^\dagger)^{sc} + \frac{7}{4} \delta^{pa} \delta^{sc} (Y_d Y_d^\dagger)^{dt} (Y_u Y_u^\dagger)^{br} \\
& + \frac{7}{4} \delta^{pa} \delta^{sc} (Y_d Y_d^\dagger)^{br} (Y_u Y_u^\dagger)^{dt} + 2 \delta^{rb} \delta^{td} (Y_d Y_d^\dagger)^{pa} (Y_d Y_d^\dagger)^{sc} + 2 \delta^{pa} \delta^{sc} (Y_d Y_d^\dagger)^{br} (Y_d Y_d^\dagger)^{dt} + 2 \delta^{rb} \delta^{td} (Y_u Y_u^\dagger)^{pa} (Y_u Y_u^\dagger)^{sc} + 2 \delta^{pa} \delta^{sc} (Y_u Y_u^\dagger)^{br} (Y_u Y_u^\dagger)^{dt} \\
& - g_Y^2 \Big( \frac{2}{27} \delta^{pa} \delta^{rd} \delta^{st} (Y_d Y_d^\dagger)^{bc} + \frac{2}{27} \delta^{pr} \delta^{sa} \delta^{td} (Y_d Y_d^\dagger)^{bc} + \frac{8}{27} \delta^{pa} \delta^{rd} \delta^{st} (Y_u Y_u^\dagger)^{bc} + \frac{8}{27} \delta^{pr} \delta^{sa} \delta^{td} (Y_u Y_u^\dagger)^{bc} + \frac{1}{3} \delta^{pa} \delta^{rb} \delta^{st} (Y_u Y_u^\dagger)^{dc} + \frac{1}{3} \delta^{pr} \delta^{sa} \delta^{tb} (Y_u Y_u^\dagger)^{dc} \Big) \\
& - \frac{5}{4} \delta^{sa} \delta^{tb} (Y_d Y_d^\dagger)^{pc} (Y_d Y_d^\dagger)^{dr} - \frac{5}{4} \delta^{pa} \delta^{rb} (Y_d Y_d^\dagger)^{sc} (Y_d Y_d^\dagger)^{dt} - \frac{5}{4} \delta^{sa} \delta^{tb} (Y_u Y_u^\dagger)^{pc} (Y_u Y_u^\dagger)^{dr} - \frac{5}{4} \delta^{pa} \delta^{rb} (Y_u Y_u^\dagger)^{sc} (Y_u Y_u^\dagger)^{dt} - \frac{3}{2} \delta^{sa} \delta^{td} (Y_d Y_d^\dagger)^{bc} (Y_u Y_u^\dagger)^{pr} \\
& - \frac{3}{2} \delta^{sa} \delta^{tb} (Y_d Y_d^\dagger)^{dc} (Y_u Y_u^\dagger)^{pr} - \frac{3}{2} \delta^{pa} \delta^{rd} (Y_d Y_d^\dagger)^{bc} (Y_u Y_u^\dagger)^{st} - \frac{3}{2} \delta^{pa} \delta^{rb} (Y_d Y_d^\dagger)^{dc} (Y_u Y_u^\dagger)^{st} - \frac{3}{2} \delta^{sa} \delta^{td} (Y_d Y_d^\dagger)^{pr} (Y_u Y_u^\dagger)^{bc} - \frac{3}{2} \delta^{pa} \delta^{rd} (Y_d Y_d^\dagger)^{st} (Y_u Y_u^\dagger)^{bc} \\
& - \frac{3}{2} \delta^{sa} \delta^{tb} (Y_d Y_d^\dagger)^{pr} (Y_u Y_u^\dagger)^{dc} - \frac{3}{2} \delta^{pa} \delta^{rb} (Y_d Y_d^\dagger)^{st} (Y_u Y_u^\dagger)^{dc} \Big\} C_{qq}^{(\times)abcd} + \left\{ \frac{1}{4} \delta^{sc} \delta^{td} (Y_d Y_d^\dagger)^{pr} (Y_e Y_e^\dagger)^{ba} + \frac{1}{4} \delta^{pc} \delta^{rd} (Y_d Y_d^\dagger)^{st} (Y_e Y_e^\dagger)^{ba} + g_L^4 \Big( \frac{7}{3} \delta^{pc} \delta^{rd} \delta^{st} \delta^{ab} \right. \\
& + \frac{7}{3} \delta^{pr} \delta^{sc} \delta^{td} \delta^{ab} \Big) + g_Y^2 \Big( \frac{2}{9} \delta^{pc} \delta^{rd} \delta^{st} (Y_e Y_e^\dagger)^{ba} + \frac{2}{9} \delta^{pr} \delta^{sc} \delta^{td} (Y_e Y_e^\dagger)^{ba} \Big) - \frac{1}{4} \delta^{sc} \delta^{td} (Y_e Y_e^\dagger)^{ba} (Y_u Y_u^\dagger)^{pr} - \frac{1}{4} \delta^{pc} \delta^{rd} (Y_e Y_e^\dagger)^{ba} (Y_u Y_u^\dagger)^{st} \\
& - g_Y^4 \Big( \frac{1}{1458} \delta^{pc} \delta^{rd} \delta^{st} \delta^{ab} + \frac{1}{1458} \delta^{pr} \delta^{sc} \delta^{td} \delta^{ab} \Big) - g_Y^2 g_s^2 \Big( \frac{25}{486} \delta^{pc} \delta^{rd} \delta^{st} \delta^{ab} + \frac{25}{486} \delta^{pr} \delta^{sc} \delta^{td} \delta^{ab} \Big) - g_Y^2 g_L^2 \Big( \frac{53}{162} \delta^{pc} \delta^{rd} \delta^{st} \delta^{ab} \\
& + \frac{53}{162} \delta^{pr} \delta^{sc} \delta^{td} \delta^{ab} \Big) \Big\} C_{\ell q}^{(\parallel)abcd} + \left\{ g_s^2 g_L^2 \Big( \frac{1}{6} \delta^{pt} \delta^{rd} \delta^{sc} \delta^{ab} + \frac{1}{6} \delta^{pc} \delta^{rs} \delta^{td} \delta^{ab} + \frac{37}{108} \delta^{pc} \delta^{rd} \delta^{st} \delta^{ab} + \frac{37}{108} \delta^{pr} \delta^{sc} \delta^{td} \delta^{ab} \Big) + g_Y^2 \Big( \frac{1}{9} \delta^{pc} \delta^{rd} \delta^{st} (Y_e Y_e^\dagger)^{ba} \right. \\
& + \frac{1}{9} \delta^{pr} \delta^{sc} \delta^{td} (Y_e Y_e^\dagger)^{ba} \Big) + g_L^2 \Big( \frac{1}{6} \delta^{pc} \delta^{rd} \delta^{st} (Y_e Y_e^\dagger)^{ba} + \frac{1}{6} \delta^{pr} \delta^{sc} \delta^{td} (Y_e Y_e^\dagger)^{ba} \Big) - \frac{1}{4} \delta^{sc} \delta^{td} (Y_e Y_e^\dagger)^{ba} (Y_u Y_u^\dagger)^{pr} - \frac{1}{4} \delta^{pc} \delta^{rd} (Y_e Y_e^\dagger)^{ba} (Y_u Y_u^\dagger)^{st} \\
& - g_Y^4 \Big( \frac{1}{2916} \delta^{pc} \delta^{rd} \delta^{st} \delta^{ab} + \frac{1}{2916} \delta^{pr} \delta^{sc} \delta^{td} \delta^{ab} \Big) - g_Y^2 g_s^2 \Big( \frac{25}{972} \delta^{pc} \delta^{rd} \delta^{st} \delta^{ab} + \frac{25}{972} \delta^{pr} \delta^{sc} \delta^{td} \delta^{ab} \Big) - g_L^4 \Big( \frac{1}{36} \delta^{pc} \delta^{rd} \delta^{st} \delta^{ab} + \frac{1}{36} \delta^{pr} \delta^{sc} \delta^{td} \delta^{ab} \Big) \\
& \left. - g_Y^2 g_L^2 \Big( \frac{11}{162} \delta^{pc} \delta^{rd} \delta^{st} \delta^{ab} + \frac{11}{162} \delta^{pr} \delta^{sc} \delta^{td} \delta^{ab} \Big) \right\} C_{\ell q}^{(\times)abcd}, \tag{13.4}
\end{aligned}$$

### 13.3 $C_{qq}^{(\times)}$

$$\begin{aligned}
\beta_{C_{qq}^{(\times)prst}}^{(1)} = & \left\{ \frac{1}{6} g_L^2 \left( \delta^{pa} \delta^{rb} \delta^{st} + \delta^{pr} \delta^{sa} \delta^{tb} \right) + \frac{1}{2} \left( -\delta^{sa} \delta^{tb} (Y_d Y_d^\dagger)^{pr} - \delta^{pa} \delta^{rb} (Y_d Y_d^\dagger)^{st} - \delta^{sa} \delta^{tb} (Y_u Y_u^\dagger)^{pr} - \delta^{pa} \delta^{rb} (Y_u Y_u^\dagger)^{st} \right) \right\} C_{Hq}^{(\times)ab} + \left\{ \frac{1}{3} g_s^2 \left( \delta^{pt} \delta^{rb} \delta^{sa} \delta^{cd} \right. \right. \\
& + \delta^{pa} \delta^{rs} \delta^{tb} \delta^{cd} \left. \right) + \frac{1}{2} \left( -\delta^{rb} \delta^{sa} Y_u^{*td} Y_u^{pc} - \delta^{pa} \delta^{tb} Y_u^{*rd} Y_u^{sc} \right) \left. \right\} C_{qu}^{(\times)abcd} + \left\{ \frac{1}{3} g_s^2 \left( \delta^{pt} \delta^{rb} \delta^{sa} \delta^{cd} + \delta^{pa} \delta^{rs} \delta^{tb} \delta^{cd} \right) + \frac{1}{2} \left( -\delta^{rb} \delta^{sa} Y_d^{*td} Y_d^{pc} - \delta^{pa} \delta^{tb} Y_d^{*rd} Y_d^{sc} \right) \right\} C_{qd}^{(\times)abcd} \\
& + \frac{1}{4} \left\{ \delta^{pc} \delta^{sa} Y_d^{*rd} Y_u^{*tb} + \delta^{pa} \delta^{sc} Y_d^{*td} Y_u^{*rb} \right\} C_{quqd}^{(\parallel)abcd} + \frac{1}{4} \left( C_{quqd}^{(\parallel)*} \right)^{abcd} \left\{ \delta^{rc} \delta^{ta} Y_d^{pd} Y_u^{sb} + \delta^{ra} \delta^{tc} Y_d^{sd} Y_u^{pb} \right\} - \frac{1}{4} \left\{ \delta^{pc} \delta^{sa} Y_d^{*td} Y_u^{*rb} \right. \\
& + \delta^{pa} \delta^{sc} Y_d^{*rd} Y_u^{*tb} \left. \right\} C_{quqd}^{(\times)abcd} - \frac{1}{4} \left( C_{quqd}^{(\times)*} \right)^{abcd} \left\{ \delta^{rc} \delta^{ta} Y_d^{sd} Y_u^{pb} + \delta^{ra} \delta^{tc} Y_d^{pd} Y_u^{sb} \right\} + \left\{ \frac{2}{3} g_s^2 \left( \delta^{pt} \delta^{rd} \delta^{sa} \delta^{bc} + \delta^{pa} \delta^{rs} \delta^{td} \delta^{bc} + 9 \delta^{pa} \delta^{rd} \delta^{sc} \delta^{tb} \right) \right. \\
& + \frac{2}{3} g_L^2 \left( \delta^{pa} \delta^{rd} \delta^{st} \delta^{bc} + \delta^{pr} \delta^{sa} \delta^{td} \delta^{bc} + 9 \delta^{pa} \delta^{rb} \delta^{sc} \delta^{td} \right) \left. \right\} C_{qq}^{(\parallel)abcd} + \left\{ \frac{1}{3} \delta^{pa} \delta^{rb} \delta^{sc} \delta^{td} g_Y^2 + \frac{1}{2} \left( \delta^{rd} \delta^{sa} \delta^{tb} (Y_d Y_d^\dagger)^{pc} + \delta^{pa} \delta^{rb} \delta^{td} (Y_d Y_d^\dagger)^{sc} \right. \right. \\
& + \delta^{pa} \delta^{sc} \delta^{td} (Y_d Y_d^\dagger)^{br} + \delta^{pa} \delta^{rb} \delta^{sc} (Y_d Y_d^\dagger)^{dt} + \delta^{rd} \delta^{sa} \delta^{tb} (Y_u Y_u^\dagger)^{pc} + \delta^{pa} \delta^{rb} \delta^{td} (Y_u Y_u^\dagger)^{sc} + \delta^{pa} \delta^{sc} \delta^{td} (Y_u Y_u^\dagger)^{br} + \delta^{pa} \delta^{rb} \delta^{sc} (Y_u Y_u^\dagger)^{dt} \left. \right) \\
& + g_L^2 \left( 2 \delta^{pa} \delta^{rb} \delta^{st} \delta^{cd} + 2 \delta^{pr} \delta^{sa} \delta^{tb} \delta^{cd} - 3 \delta^{pa} \delta^{rb} \delta^{sc} \delta^{td} \right) - \frac{2}{3} g_s^2 \left( 3 \delta^{pa} \delta^{rb} \delta^{sc} \delta^{td} - 2 \delta^{pt} \delta^{rd} \delta^{sa} \delta^{bc} - 2 \delta^{pa} \delta^{rs} \delta^{td} \delta^{bc} \right) \left. \right\} C_{qq}^{(\times)abcd} + \frac{1}{3} g_L^2 \left\{ \delta^{pc} \delta^{rd} \delta^{st} \delta^{ab} \right. \\
& + \delta^{pr} \delta^{sc} \delta^{td} \delta^{ab} \left. \right\} C_{\ell q}^{(\times)abcd}, \tag{13.5}
\end{aligned}$$

$$\begin{aligned}
\beta_{C_{qq}^{(\times)prst}}^{(2)} = & \left\{ \frac{2}{3} \delta^{pr} \delta^{st} g_L^6 - g_L^4 \left( \frac{3}{2} \delta^{st} (Y_d Y_d^\dagger)^{pr} + \frac{3}{2} \delta^{pr} (Y_d Y_d^\dagger)^{st} + \frac{3}{2} \delta^{st} (Y_u Y_u^\dagger)^{pr} + \frac{3}{2} \delta^{pr} (Y_u Y_u^\dagger)^{st} \right) \right\} C_{HW} - g_s^4 \left\{ \delta^{rs} (Y_d Y_d^\dagger)^{pt} + \delta^{pt} (Y_d Y_d^\dagger)^{sr} + \delta^{rs} (Y_u Y_u^\dagger)^{pt} \right. \\
& + \delta^{pt} (Y_u Y_u^\dagger)^{sr} \left. \right\} C_{HG} + \left\{ \frac{1}{6} \delta^{pr} \delta^{st} g_Y^2 g_L^4 - g_Y^2 g_L^2 \left( \frac{1}{24} \delta^{st} (Y_u Y_u^\dagger)^{pr} + \frac{1}{24} \delta^{pr} (Y_u Y_u^\dagger)^{st} + \frac{5}{24} \delta^{st} (Y_d Y_d^\dagger)^{pr} + \frac{5}{24} \delta^{pr} (Y_d Y_d^\dagger)^{st} \right) \right\} C_{HWB} \\
& + \left\{ g_L^6 \left( \frac{3}{2} \delta^{st} (Y_d Y_d^\dagger)^{pr} + \frac{3}{2} \delta^{pr} (Y_d Y_d^\dagger)^{st} + \frac{3}{2} \delta^{st} (Y_u Y_u^\dagger)^{pr} + \frac{3}{2} \delta^{pr} (Y_u Y_u^\dagger)^{st} \right) + \frac{7}{6} \delta^{pr} \delta^{st} g_Y^2 g_L^6 - g_s^2 g_L^6 \left( \frac{1}{2} \delta^{pt} \delta^{rs} + 7 \delta^{pr} \delta^{st} \right) - \frac{20}{3} \delta^{pr} \delta^{st} g_L^8 \right\} C_W \\
& + \left\{ g_s^6 g_L^2 \left( \frac{97}{6} \delta^{pr} \delta^{st} - \frac{63}{4} \delta^{pt} \delta^{rs} \right) + \frac{7}{4} \delta^{pt} \delta^{rs} g_Y^2 g_s^6 - g_s^6 \left( \frac{9}{4} \delta^{rs} (Y_d Y_d^\dagger)^{pt} + \frac{9}{4} \delta^{pt} (Y_d Y_d^\dagger)^{sr} + \frac{9}{4} \delta^{rs} (Y_u Y_u^\dagger)^{pt} + \frac{9}{4} \delta^{pt} (Y_u Y_u^\dagger)^{sr} \right) - \frac{29}{6} \delta^{pt} \delta^{rs} g_s^8 \right\} C_G \\
& + \frac{1}{6} \delta^{pr} \delta^{st} g_L^4 Y_e^{*ab} C_{eW}^{ab} + \frac{1}{6} \delta^{pr} \delta^{st} g_L^4 C_{eW}^{*ab} Y_e^{ab} + \left\{ g_Y^2 \left( \frac{3}{4} \delta^{sa} Y_u^{*tb} (Y_d Y_d^\dagger)^{pr} + \frac{3}{4} \delta^{pa} Y_u^{*rb} (Y_d Y_d^\dagger)^{st} + \frac{3}{2} \delta^{sa} Y_u^{*tb} (Y_u Y_u^\dagger)^{pr} + \frac{3}{2} \delta^{pa} Y_u^{*rb} (Y_u Y_u^\dagger)^{st} \right) \right.
\end{aligned}$$

$$\begin{aligned}
& -g_Y^2 g_L^2 \left( \frac{7}{36} \delta^{pa} \delta^{st} Y_u^{*rb} + \frac{7}{36} \delta^{pr} \delta^{sa} Y_u^{*tb} \right) - g_Y^2 g_s^2 \left( \frac{13}{9} \delta^{pa} \delta^{rs} Y_u^{*tb} + \frac{13}{9} \delta^{pt} \delta^{sa} Y_u^{*rb} \right) \Big\} C_{uB}^{ab} + C_{uB}^{*ab} \Big\{ g_Y^2 \left( \frac{3}{4} \delta^{ta} Y_u^{sb} (Y_d Y_d^\dagger)^{pr} + \frac{3}{4} \delta^{ra} Y_u^{pb} (Y_d Y_d^\dagger)^{st} \right. \\
& + \frac{3}{2} \delta^{ta} Y_u^{sb} (Y_u Y_u^\dagger)^{pr} + \frac{3}{2} \delta^{ra} Y_u^{pb} (Y_u Y_u^\dagger)^{st} \Big) - g_Y^2 g_L^2 \left( \frac{7}{36} \delta^{ra} \delta^{st} Y_u^{pb} + \frac{7}{36} \delta^{pr} \delta^{ta} Y_u^{sb} \right) - g_Y^2 g_s^2 \left( \frac{13}{9} \delta^{pt} \delta^{ra} Y_u^{sb} + \frac{13}{9} \delta^{rs} \delta^{ta} Y_u^{pb} \right) \Big\} + \Big\{ g_L^4 \left( \frac{1}{8} \delta^{pa} \delta^{st} Y_u^{*rb} \right. \\
& + \frac{1}{8} \delta^{pr} \delta^{sa} Y_u^{*tb} + \frac{1}{2} \delta^{pr} \delta^{st} Y_u^{*ab} \Big) + g_s^2 g_L^2 \left( \frac{1}{2} \delta^{pa} \delta^{rs} Y_u^{*tb} + \frac{1}{2} \delta^{pt} \delta^{sa} Y_u^{*rb} - \frac{5}{6} \delta^{pa} \delta^{st} Y_u^{*rb} - \frac{5}{6} \delta^{pr} \delta^{sa} Y_u^{*tb} \right) - g_Y^2 g_L^2 \left( \frac{4}{9} \delta^{pa} \delta^{st} Y_u^{*rb} + \frac{4}{9} \delta^{pr} \delta^{sa} Y_u^{*tb} \right) \\
& - g_L^2 \left( \frac{1}{4} \delta^{st} Y_u^{*rb} (Y_d Y_d^\dagger)^{pa} + \frac{1}{4} \delta^{pr} Y_u^{*tb} (Y_d Y_d^\dagger)^{sa} + \frac{3}{4} \delta^{sa} Y_u^{*tb} (Y_u Y_u^\dagger)^{pr} + \frac{3}{4} \delta^{pa} Y_u^{*rb} (Y_u Y_u^\dagger)^{st} + \frac{9}{8} \delta^{sa} Y_u^{*tb} (Y_d Y_d^\dagger)^{pr} + \frac{9}{8} \delta^{pa} Y_u^{*rb} (Y_d Y_d^\dagger)^{st} \right) \Big\} C_{uW}^{ab} \\
& + C_{uW}^{*ab} \Big\{ g_L^4 \left( \frac{1}{8} \delta^{ra} \delta^{st} Y_u^{pb} + \frac{1}{8} \delta^{pr} \delta^{ta} Y_u^{sb} + \frac{1}{2} \delta^{pr} \delta^{st} Y_u^{ab} \right) + g_s^2 g_L^2 \left( \frac{1}{2} \delta^{pt} \delta^{ra} Y_u^{sb} + \frac{1}{2} \delta^{rs} \delta^{ta} Y_u^{pb} - \frac{5}{6} \delta^{ra} \delta^{st} Y_u^{pb} - \frac{5}{6} \delta^{pr} \delta^{ta} Y_u^{sb} \right) - g_Y^2 g_L^2 \left( \frac{4}{9} \delta^{ra} \delta^{st} Y_u^{pb} \right. \\
& + \frac{4}{9} \delta^{pr} \delta^{ta} Y_u^{sb} \Big) - g_L^2 \left( \frac{1}{4} \delta^{st} Y_u^{pb} (Y_d Y_d^\dagger)^{ar} + \frac{1}{4} \delta^{pr} Y_u^{sb} (Y_d Y_d^\dagger)^{at} + \frac{3}{4} \delta^{ta} Y_u^{sb} (Y_u Y_u^\dagger)^{pr} + \frac{3}{4} \delta^{ra} Y_u^{pb} (Y_u Y_u^\dagger)^{st} + \frac{9}{8} \delta^{ta} Y_u^{sb} (Y_d Y_d^\dagger)^{pr} + \frac{9}{8} \delta^{ra} Y_u^{pb} (Y_d Y_d^\dagger)^{st} \right) \Big\} \\
& + \Big\{ g_s^4 \left( \frac{4}{9} \delta^{pa} \delta^{rs} Y_u^{*tb} + \frac{4}{9} \delta^{pt} \delta^{sa} Y_u^{*rb} + \frac{2}{3} \delta^{pt} \delta^{rs} Y_u^{*ab} \right) + g_s^2 \left( \frac{1}{4} \delta^{rs} Y_u^{*tb} (Y_d Y_d^\dagger)^{pa} + \frac{1}{4} \delta^{pt} Y_u^{*rb} (Y_d Y_d^\dagger)^{sa} + \frac{3}{2} \delta^{sa} Y_u^{*tb} (Y_d Y_d^\dagger)^{pr} + \frac{3}{2} \delta^{pa} Y_u^{*rb} (Y_d Y_d^\dagger)^{st} \right. \\
& + \frac{3}{2} \delta^{sa} Y_u^{*tb} (Y_u Y_u^\dagger)^{pr} + \frac{3}{2} \delta^{pa} Y_u^{*rb} (Y_u Y_u^\dagger)^{st} - \frac{1}{2} \delta^{rs} Y_u^{*tb} (Y_u Y_u^\dagger)^{pa} - \frac{1}{2} \delta^{pt} Y_u^{*rb} (Y_u Y_u^\dagger)^{sa} - \frac{3}{2} \delta^{sa} Y_u^{*rb} (Y_d Y_d^\dagger)^{pt} - \frac{3}{2} \delta^{pa} Y_u^{*tb} (Y_d Y_d^\dagger)^{sr} \Big) \\
& - g_s^2 g_L^2 \left( \frac{2}{9} \delta^{pa} \delta^{st} Y_u^{*rb} + \frac{2}{9} \delta^{pr} \delta^{sa} Y_u^{*tb} \right) - g_Y^2 g_s^2 \left( \frac{4}{9} \delta^{pa} \delta^{rs} Y_u^{*tb} + \frac{4}{9} \delta^{pt} \delta^{sa} Y_u^{*rb} \right) \Big\} C_{uG}^{ab} + C_{uG}^{*ab} \Big\{ g_s^4 \left( \frac{4}{9} \delta^{pt} \delta^{ra} Y_u^{sb} + \frac{4}{9} \delta^{rs} \delta^{ta} Y_u^{pb} + \frac{2}{3} \delta^{pt} \delta^{rs} Y_u^{ab} \right) \\
& + g_s^2 \left( \frac{1}{4} \delta^{pt} Y_u^{sb} (Y_d Y_d^\dagger)^{ar} + \frac{1}{4} \delta^{rs} Y_u^{pb} (Y_d Y_d^\dagger)^{at} + \frac{3}{2} \delta^{ta} Y_u^{sb} (Y_d Y_d^\dagger)^{pr} + \frac{3}{2} \delta^{ra} Y_u^{pb} (Y_d Y_d^\dagger)^{st} + \frac{3}{2} \delta^{ta} Y_u^{sb} (Y_u Y_u^\dagger)^{pr} + \frac{3}{2} \delta^{ra} Y_u^{pb} (Y_u Y_u^\dagger)^{st} - \frac{1}{2} \delta^{pt} Y_u^{sb} (Y_u Y_u^\dagger)^{ar} \right. \\
& - \frac{1}{2} \delta^{rs} Y_u^{pb} (Y_u Y_u^\dagger)^{at} - \frac{3}{2} \delta^{ra} Y_u^{sb} (Y_d Y_d^\dagger)^{pt} - \frac{3}{2} \delta^{ta} Y_u^{pb} (Y_d Y_d^\dagger)^{sr} \Big) - g_s^2 g_L^2 \left( \frac{2}{9} \delta^{ra} \delta^{st} Y_u^{pb} + \frac{2}{9} \delta^{pr} \delta^{ta} Y_u^{sb} \right) - g_Y^2 g_s^2 \left( \frac{4}{9} \delta^{pt} \delta^{ra} Y_u^{sb} + \frac{4}{9} \delta^{rs} \delta^{ta} Y_u^{pb} \right) \Big\} \\
& + \Big\{ g_Y^2 g_L^2 \left( \frac{5}{36} \delta^{pa} \delta^{st} Y_d^{*rb} + \frac{5}{36} \delta^{pr} \delta^{sa} Y_d^{*tb} \right) + g_Y^2 \left( \frac{3}{4} \delta^{sa} Y_d^{*tb} (Y_u Y_u^\dagger)^{pr} + \frac{3}{4} \delta^{pa} Y_d^{*rb} (Y_u Y_u^\dagger)^{st} \right) - g_Y^2 g_s^2 \left( \frac{1}{9} \delta^{pa} \delta^{rs} Y_d^{*tb} + \frac{1}{9} \delta^{pt} \delta^{sa} Y_d^{*rb} \right) \Big\} C_{dB}^{ab} \\
& + C_{dB}^{*ab} \Big\{ g_Y^2 g_L^2 \left( \frac{5}{36} \delta^{ra} \delta^{st} Y_d^{pb} + \frac{5}{36} \delta^{pr} \delta^{ta} Y_d^{sb} \right) + g_Y^2 \left( \frac{3}{4} \delta^{ta} Y_d^{sb} (Y_u Y_u^\dagger)^{pr} + \frac{3}{4} \delta^{ra} Y_d^{pb} (Y_u Y_u^\dagger)^{st} \right) - g_Y^2 g_s^2 \left( \frac{1}{9} \delta^{pt} \delta^{ra} Y_d^{sb} + \frac{1}{9} \delta^{rs} \delta^{ta} Y_d^{pb} \right) \Big\} \\
& + \Big\{ g_L^4 \left( \frac{1}{8} \delta^{pa} \delta^{st} Y_d^{*rb} + \frac{1}{8} \delta^{pr} \delta^{sa} Y_d^{*tb} + \frac{1}{2} \delta^{pr} \delta^{st} Y_d^{*ab} \right) + g_Y^2 g_L^2 \left( \frac{2}{9} \delta^{pa} \delta^{st} Y_d^{*rb} + \frac{2}{9} \delta^{pr} \delta^{sa} Y_d^{*tb} \right) + g_s^2 g_L^2 \left( \frac{1}{2} \delta^{pa} \delta^{rs} Y_d^{*tb} + \frac{1}{2} \delta^{pt} \delta^{sa} Y_d^{*rb} \right. \\
& - \frac{5}{6} \delta^{pa} \delta^{st} Y_d^{*rb} - \frac{5}{6} \delta^{pr} \delta^{sa} Y_d^{*tb} \Big) - g_L^2 \left( \frac{1}{4} \delta^{st} Y_d^{*rb} (Y_u Y_u^\dagger)^{pa} + \frac{1}{4} \delta^{pr} Y_d^{*tb} (Y_u Y_u^\dagger)^{sa} + \frac{3}{4} \delta^{sa} Y_d^{*tb} (Y_d Y_d^\dagger)^{pr} + \frac{3}{4} \delta^{pa} Y_d^{*rb} (Y_d Y_d^\dagger)^{st} + \frac{9}{8} \delta^{sa} Y_d^{*tb} (Y_u Y_u^\dagger)^{pr} \right.
\end{aligned}$$

$$\begin{aligned}
& + \frac{9}{8} \delta^{pa} Y_d^{*rb} (Y_u Y_u^\dagger)^{st} \Big) \Big\} C_{dW}^{ab} + C_{dW}^{*ab} \Big\{ g_L^4 \Big( \frac{1}{8} \delta^{ra} \delta^{st} Y_d^{pb} + \frac{1}{8} \delta^{pr} \delta^{ta} Y_d^{sb} + \frac{1}{2} \delta^{pr} \delta^{st} Y_d^{ab} \Big) + g_Y^2 g_L^2 \Big( \frac{2}{9} \delta^{ra} \delta^{st} Y_d^{pb} + \frac{2}{9} \delta^{pr} \delta^{ta} Y_d^{sb} \Big) + g_s^2 g_L^2 \Big( \frac{1}{2} \delta^{pt} \delta^{ra} Y_d^{sb} \\
& + \frac{1}{2} \delta^{rs} \delta^{ta} Y_d^{pb} - \frac{5}{6} \delta^{ra} \delta^{st} Y_d^{pb} - \frac{5}{6} \delta^{pr} \delta^{ta} Y_d^{sb} \Big) - g_L^2 \Big( \frac{1}{4} \delta^{st} Y_d^{pb} (Y_u Y_u^\dagger)^{ar} + \frac{1}{4} \delta^{pr} Y_d^{sb} (Y_u Y_u^\dagger)^{at} + \frac{3}{4} \delta^{ta} Y_d^{sb} (Y_d Y_d^\dagger)^{pr} + \frac{3}{4} \delta^{ra} Y_d^{pb} (Y_d Y_d^\dagger)^{st} + \frac{9}{8} \delta^{ta} Y_d^{sb} (Y_u Y_u^\dagger)^{pr} \\
& + \frac{9}{8} \delta^{ra} Y_d^{pb} (Y_u Y_u^\dagger)^{st} \Big) \Big\} + \Big\{ g_Y^2 g_s^2 \Big( \frac{2}{9} \delta^{pa} \delta^{rs} Y_d^{*tb} + \frac{2}{9} \delta^{pt} \delta^{sa} Y_d^{*rb} \Big) + g_s^4 \Big( \frac{4}{9} \delta^{pa} \delta^{rs} Y_d^{*tb} + \frac{4}{9} \delta^{pt} \delta^{sa} Y_d^{*rb} + \frac{2}{3} \delta^{pt} \delta^{rs} Y_d^{*ab} \Big) + g_s^2 \Big( \frac{1}{4} \delta^{rs} Y_d^{*tb} (Y_u Y_u^\dagger)^{pa} \\
& + \frac{1}{4} \delta^{pt} Y_d^{*rb} (Y_u Y_u^\dagger)^{sa} + \frac{3}{2} \delta^{sa} Y_d^{*tb} (Y_d Y_d^\dagger)^{pr} + \frac{3}{2} \delta^{pa} Y_d^{*rb} (Y_d Y_d^\dagger)^{st} + \frac{3}{2} \delta^{sa} Y_d^{*tb} (Y_u Y_u^\dagger)^{pr} + \frac{3}{2} \delta^{pa} Y_d^{*rb} (Y_u Y_u^\dagger)^{st} - \frac{1}{2} \delta^{rs} Y_d^{*tb} (Y_d Y_d^\dagger)^{pa} \\
& - \frac{1}{2} \delta^{pt} Y_d^{*rb} (Y_d Y_d^\dagger)^{sa} - \frac{3}{2} \delta^{sa} Y_d^{*rb} (Y_u Y_u^\dagger)^{pt} - \frac{3}{2} \delta^{pa} Y_d^{*tb} (Y_u Y_u^\dagger)^{sr} \Big) - g_s^2 g_L^2 \Big( \frac{2}{9} \delta^{pa} \delta^{st} Y_d^{*rb} + \frac{2}{9} \delta^{pr} \delta^{sa} Y_d^{*tb} \Big) \Big\} C_{dG}^{ab} + C_{dG}^{*ab} \Big\{ g_Y^2 g_s^2 \Big( \frac{2}{9} \delta^{pt} \delta^{ra} Y_d^{sb} \\
& + \frac{2}{9} \delta^{rs} \delta^{ta} Y_d^{pb} \Big) + g_s^4 \Big( \frac{4}{9} \delta^{pt} \delta^{ra} Y_d^{sb} + \frac{4}{9} \delta^{rs} \delta^{ta} Y_d^{pb} + \frac{2}{3} \delta^{pt} \delta^{rs} Y_d^{ab} \Big) + g_s^2 \Big( \frac{1}{4} \delta^{pt} Y_d^{sb} (Y_u Y_u^\dagger)^{ar} + \frac{1}{4} \delta^{rs} Y_d^{pb} (Y_u Y_u^\dagger)^{at} + \frac{3}{2} \delta^{ta} Y_d^{sb} (Y_d Y_d^\dagger)^{pr} + \frac{3}{2} \delta^{ra} Y_d^{pb} (Y_d Y_d^\dagger)^{st} \\
& + \frac{3}{2} \delta^{ta} Y_d^{sb} (Y_u Y_u^\dagger)^{pr} + \frac{3}{2} \delta^{ra} Y_d^{pb} (Y_u Y_u^\dagger)^{st} - \frac{1}{2} \delta^{pt} Y_d^{sb} (Y_d Y_d^\dagger)^{ar} - \frac{1}{2} \delta^{rs} Y_d^{pb} (Y_d Y_d^\dagger)^{at} - \frac{3}{2} \delta^{ra} Y_d^{sb} (Y_u Y_u^\dagger)^{pt} - \frac{3}{2} \delta^{ta} Y_d^{pb} (Y_u Y_u^\dagger)^{sr} \Big) - g_s^2 g_L^2 \Big( \frac{2}{9} \delta^{ra} \delta^{st} Y_d^{pb} \\
& + \frac{2}{9} \delta^{pr} \delta^{ta} Y_d^{sb} \Big) \Big\} + \Big\{ \frac{1}{8} \delta^{rb} (Y_d Y_d^\dagger)^{st} (Y_u Y_u^\dagger)^{pa} + \frac{1}{8} \delta^{rb} (Y_u Y_u^\dagger)^{pa} (Y_u Y_u^\dagger)^{st} + \frac{1}{8} \delta^{tb} (Y_d Y_d^\dagger)^{pr} (Y_u Y_u^\dagger)^{sa} + \frac{1}{8} \delta^{tb} (Y_u Y_u^\dagger)^{pr} (Y_u Y_u^\dagger)^{sa} + \frac{1}{8} \delta^{pa} (Y_d Y_d^\dagger)^{st} (Y_u Y_u^\dagger)^{br} \\
& + \frac{1}{8} \delta^{pa} (Y_u Y_u^\dagger)^{st} (Y_u Y_u^\dagger)^{br} + \frac{1}{8} \delta^{sa} (Y_d Y_d^\dagger)^{pr} (Y_u Y_u^\dagger)^{bt} + \frac{1}{8} \delta^{sa} (Y_u Y_u^\dagger)^{pr} (Y_u Y_u^\dagger)^{bt} + g_s^2 \Big( \frac{7}{36} \delta^{rs} \delta^{tb} (Y_d Y_d^\dagger)^{pa} + \frac{7}{36} \delta^{pt} \delta^{rb} (Y_d Y_d^\dagger)^{sa} + \frac{7}{36} \delta^{pt} \delta^{sa} (Y_d Y_d^\dagger)^{br} \\
& + \frac{7}{36} \delta^{pa} \delta^{rs} (Y_d Y_d^\dagger)^{bt} + \frac{7}{4} \delta^{rb} \delta^{sa} (Y_d Y_d^\dagger)^{pt} + \frac{7}{4} \delta^{pa} \delta^{tb} (Y_d Y_d^\dagger)^{sr} - \frac{7}{36} \delta^{rs} \delta^{tb} (Y_u Y_u^\dagger)^{pa} - \frac{7}{36} \delta^{pt} \delta^{rb} (Y_u Y_u^\dagger)^{sa} - \frac{7}{36} \delta^{pt} \delta^{sa} (Y_u Y_u^\dagger)^{br} - \frac{7}{36} \delta^{pa} \delta^{rs} (Y_u Y_u^\dagger)^{bt} \\
& - \frac{7}{4} \delta^{rb} \delta^{sa} (Y_u Y_u^\dagger)^{pt} - \frac{7}{4} \delta^{pa} \delta^{tb} (Y_u Y_u^\dagger)^{sr} \Big) + g_L^2 \Big( \frac{1}{4} \delta^{sa} \delta^{tb} (Y_d Y_d^\dagger)^{pr} + \frac{1}{4} \delta^{pa} \delta^{rb} (Y_d Y_d^\dagger)^{st} + \frac{29}{72} \delta^{rb} \delta^{st} (Y_d Y_d^\dagger)^{pa} + \frac{29}{72} \delta^{pr} \delta^{tb} (Y_d Y_d^\dagger)^{sa} + \frac{29}{72} \delta^{pa} \delta^{st} (Y_d Y_d^\dagger)^{br} \\
& + \frac{29}{72} \delta^{pr} \delta^{sa} (Y_d Y_d^\dagger)^{bt} - \frac{1}{4} \delta^{sa} \delta^{tb} (Y_u Y_u^\dagger)^{pr} - \frac{1}{4} \delta^{pa} \delta^{rb} (Y_u Y_u^\dagger)^{st} - \frac{29}{72} \delta^{rb} \delta^{st} (Y_u Y_u^\dagger)^{pa} - \frac{29}{72} \delta^{pr} \delta^{tb} (Y_u Y_u^\dagger)^{sa} - \frac{29}{72} \delta^{pa} \delta^{st} (Y_u Y_u^\dagger)^{br} - \frac{29}{72} \delta^{pr} \delta^{sa} (Y_u Y_u^\dagger)^{bt} \\
& - \frac{1}{8} \delta^{rb} (Y_d Y_d^\dagger)^{pa} (Y_d Y_d^\dagger)^{st} - \frac{1}{8} \delta^{tb} (Y_d Y_d^\dagger)^{pr} (Y_d Y_d^\dagger)^{sa} - \frac{1}{8} \delta^{pa} (Y_d Y_d^\dagger)^{st} (Y_d Y_d^\dagger)^{br} - \frac{1}{8} \delta^{sa} (Y_d Y_d^\dagger)^{pr} (Y_d Y_d^\dagger)^{bt} - \frac{1}{8} \delta^{tb} (Y_d Y_d^\dagger)^{sa} (Y_u Y_u^\dagger)^{pr} - \frac{1}{8} \delta^{sa} (Y_d Y_d^\dagger)^{bt} (Y_u Y_u^\dagger)^{pr} \\
& - \frac{1}{8} \delta^{rb} (Y_d Y_d^\dagger)^{pa} (Y_u Y_u^\dagger)^{st} - \frac{1}{8} \delta^{pa} (Y_d Y_d^\dagger)^{br} (Y_u Y_u^\dagger)^{st} - g_Y^2 g_s^2 \Big( \frac{91}{324} \delta^{pt} \delta^{rb} \delta^{sa} + \frac{91}{324} \delta^{pa} \delta^{rs} \delta^{tb} \Big) - g_Y^2 g_L^2 \Big( \frac{91}{324} \delta^{pa} \delta^{rb} \delta^{st} + \frac{91}{324} \delta^{pr} \delta^{sa} \delta^{tb} \Big) \Big\} C_{Hq}^{(II)ab} \\
& + \Big\{ \frac{1}{4} \delta^{rb} (Y_d Y_d^\dagger)^{pa} (Y_d Y_d^\dagger)^{st} + \frac{1}{4} \delta^{tb} (Y_d Y_d^\dagger)^{pr} (Y_d Y_d^\dagger)^{sa} + \frac{1}{4} \delta^{pa} (Y_d Y_d^\dagger)^{st} (Y_d Y_d^\dagger)^{br} + \frac{1}{4} \delta^{sa} (Y_d Y_d^\dagger)^{pr} (Y_d Y_d^\dagger)^{bt} + \frac{1}{4} \delta^{tb} (Y_d Y_d^\dagger)^{sa} (Y_u Y_u^\dagger)^{pr} \\
& + \frac{1}{4} \delta^{sa} (Y_d Y_d^\dagger)^{bt} (Y_u Y_u^\dagger)^{pr} + \frac{1}{4} \delta^{rb} (Y_d Y_d^\dagger)^{pa} (Y_u Y_u^\dagger)^{st} + \frac{1}{4} \delta^{pa} (Y_d Y_d^\dagger)^{br} (Y_u Y_u^\dagger)^{st} + \frac{1}{4} \delta^{sa} \delta^{tb} (Y_d Y_d^\dagger Y_d Y_d^\dagger)^{pr} + \frac{1}{4} \delta^{pa} \delta^{rb} (Y_d Y_d^\dagger Y_d Y_d^\dagger)^{st} \\
& + \frac{1}{4} \delta^{sa} \delta^{tb} (Y_u Y_u^\dagger Y_u Y_u^\dagger)^{pr} + \frac{1}{4} \delta^{pa} \delta^{rb} (Y_u Y_u^\dagger Y_u Y_u^\dagger)^{st} + \frac{3}{8} \delta^{rb} (Y_d Y_d^\dagger)^{st} (Y_u Y_u^\dagger)^{pa} + \frac{3}{8} \delta^{rb} (Y_u Y_u^\dagger)^{pa} (Y_u Y_u^\dagger)^{st} + \frac{3}{8} \delta^{tb} (Y_d Y_d^\dagger)^{pr} (Y_u Y_u^\dagger)^{sa}
\end{aligned}$$

$$\begin{aligned}
& + \frac{3}{8} \delta^{tb} (Y_u Y_u^\dagger)^{pr} (Y_u Y_u^\dagger)^{sa} + \frac{3}{8} \delta^{pa} (Y_d Y_d^\dagger)^{st} (Y_u Y_u^\dagger)^{br} + \frac{3}{8} \delta^{pa} (Y_u Y_u^\dagger)^{st} (Y_u Y_u^\dagger)^{br} + \frac{3}{8} \delta^{sa} (Y_d Y_d^\dagger)^{pr} (Y_u Y_u^\dagger)^{bt} + \frac{3}{8} \delta^{sa} (Y_u Y_u^\dagger)^{pr} (Y_u Y_u^\dagger)^{bt} + \frac{1}{2} T_2 \delta^{sa} \delta^{tb} (Y_d Y_d^\dagger)^{pr} \\
& + \frac{1}{2} T_2 \delta^{pa} \delta^{rb} (Y_d Y_d^\dagger)^{st} + \frac{1}{2} T_2 \delta^{sa} \delta^{tb} (Y_u Y_u^\dagger)^{pr} + \frac{1}{2} T_2 \delta^{pa} \delta^{rb} (Y_u Y_u^\dagger)^{st} + \frac{1}{2} \delta^{sa} \delta^{tb} (Y_d Y_d^\dagger Y_u Y_u^\dagger)^{pr} + \frac{1}{2} \delta^{pa} \delta^{rb} (Y_d Y_d^\dagger Y_u Y_u^\dagger)^{st} \\
& + \frac{1}{2} \delta^{sa} \delta^{tb} (Y_u Y_u^\dagger Y_d Y_d^\dagger)^{pr} + \frac{1}{2} \delta^{pa} \delta^{rb} (Y_u Y_u^\dagger Y_d Y_d^\dagger)^{st} + g_s^2 g_L^2 \left( \frac{5}{36} \delta^{pa} \delta^{rb} \delta^{st} + \frac{5}{36} \delta^{pr} \delta^{sa} \delta^{tb} - \frac{31}{72} \delta^{pt} \delta^{rb} \delta^{sa} - \frac{31}{72} \delta^{pa} \delta^{rs} \delta^{tb} \right) \\
& + g_Y^2 g_L^2 \left( \frac{109}{324} \delta^{pa} \delta^{rb} \delta^{st} + \frac{109}{324} \delta^{pr} \delta^{sa} \delta^{tb} \right) + g_L^4 \left( \frac{19}{36} \delta^{pa} \delta^{rb} \delta^{st} + \frac{19}{36} \delta^{pr} \delta^{sa} \delta^{tb} \right) + g_s^2 \left( \frac{7}{36} \delta^{rs} \delta^{tb} (Y_u Y_u^\dagger)^{pa} + \frac{7}{36} \delta^{pt} \delta^{rb} (Y_u Y_u^\dagger)^{sa} + \frac{7}{36} \delta^{pt} \delta^{sa} (Y_u Y_u^\dagger)^{br} \right. \\
& + \frac{7}{36} \delta^{pa} \delta^{rs} (Y_u Y_u^\dagger)^{bt} + \frac{7}{18} \delta^{rs} \delta^{tb} (Y_d Y_d^\dagger)^{pa} + \frac{7}{18} \delta^{pt} \delta^{rb} (Y_d Y_d^\dagger)^{sa} + \frac{7}{18} \delta^{pt} \delta^{sa} (Y_d Y_d^\dagger)^{br} + \frac{7}{18} \delta^{pa} \delta^{rs} (Y_d Y_d^\dagger)^{bt} + \frac{25}{12} \delta^{sa} \delta^{tb} (Y_d Y_d^\dagger)^{pr} \\
& + \frac{25}{12} \delta^{pa} \delta^{rb} (Y_d Y_d^\dagger)^{st} + \frac{25}{12} \delta^{sa} \delta^{tb} (Y_u Y_u^\dagger)^{pr} + \frac{25}{12} \delta^{pa} \delta^{rb} (Y_u Y_u^\dagger)^{st} - \frac{7}{4} \delta^{rb} \delta^{sa} (Y_u Y_u^\dagger)^{pt} - \frac{7}{4} \delta^{pa} \delta^{tb} (Y_u Y_u^\dagger)^{sr} \Big) - g_Y^2 g_s^2 \left( \frac{91}{648} \delta^{pt} \delta^{rb} \delta^{sa} + \frac{91}{648} \delta^{pa} \delta^{rs} \delta^{tb} \right) \\
& - g_Y^2 \left( \frac{89}{144} \delta^{sa} \delta^{tb} (Y_u Y_u^\dagger)^{pr} + \frac{89}{144} \delta^{pa} \delta^{rb} (Y_u Y_u^\dagger)^{st} + \frac{173}{144} \delta^{sa} \delta^{tb} (Y_d Y_d^\dagger)^{pr} + \frac{173}{144} \delta^{pa} \delta^{rb} (Y_d Y_d^\dagger)^{st} \right) - g_L^2 \left( \frac{1}{36} \delta^{rb} \delta^{st} (Y_d Y_d^\dagger)^{pa} + \frac{1}{36} \delta^{pr} \delta^{tb} (Y_d Y_d^\dagger)^{sa} \right. \\
& + \frac{1}{36} \delta^{pa} \delta^{st} (Y_d Y_d^\dagger)^{br} + \frac{1}{36} \delta^{pr} \delta^{sa} (Y_d Y_d^\dagger)^{bt} + \frac{1}{6} T_2 \delta^{pa} \delta^{rb} \delta^{st} + \frac{1}{6} T_2 \delta^{pr} \delta^{sa} \delta^{tb} + \frac{31}{72} \delta^{rb} \delta^{st} (Y_u Y_u^\dagger)^{pa} + \frac{31}{72} \delta^{pr} \delta^{tb} (Y_u Y_u^\dagger)^{sa} + \frac{31}{72} \delta^{pa} \delta^{st} (Y_u Y_u^\dagger)^{br} \\
& + \frac{31}{72} \delta^{pr} \delta^{sa} (Y_u Y_u^\dagger)^{bt} + \frac{31}{16} \delta^{sa} \delta^{tb} (Y_d Y_d^\dagger)^{pr} + \frac{31}{16} \delta^{pa} \delta^{rb} (Y_d Y_d^\dagger)^{st} + \frac{35}{16} \delta^{sa} \delta^{tb} (Y_u Y_u^\dagger)^{pr} + \frac{35}{16} \delta^{pa} \delta^{rb} (Y_u Y_u^\dagger)^{st} \Big) \Big\} C_{Hq}^{(\times)ab} + \left\{ g_Y^2 g_s^2 \left( \frac{25}{162} \delta^{pt} \delta^{rb} \delta^{sa} \delta^{cd} \right. \right. \\
& + \frac{25}{162} \delta^{pa} \delta^{rs} \delta^{tb} \delta^{cd} \Big) + g_Y^2 g_L^2 \left( \frac{25}{162} \delta^{pa} \delta^{rb} \delta^{st} \delta^{cd} + \frac{25}{162} \delta^{pr} \delta^{sa} \delta^{tb} \delta^{cd} \right) \Big\} C_{qe}^{abcd} + \left\{ \frac{1}{8} \delta^{rb} Y_u^{*td} Y_u^{sc} (Y_d Y_d^\dagger)^{pa} + \frac{1}{8} \delta^{tb} Y_u^{*rd} Y_u^{pc} (Y_d Y_d^\dagger)^{sa} \right. \\
& + \frac{1}{8} \delta^{pa} Y_u^{*td} Y_u^{sc} (Y_d Y_d^\dagger)^{br} + \frac{1}{8} \delta^{sa} Y_u^{*rd} Y_u^{pc} (Y_d Y_d^\dagger)^{bt} + \frac{1}{2} \delta^{sa} Y_u^{*td} Y_u^{bc} (Y_u Y_u^\dagger)^{pr} + \frac{1}{2} \delta^{tb} Y_u^{*ad} Y_u^{sc} (Y_u Y_u^\dagger)^{pr} + \frac{1}{2} \delta^{pa} Y_u^{*rd} Y_u^{bc} (Y_u Y_u^\dagger)^{st} + \frac{1}{2} \delta^{rb} Y_u^{*ad} Y_u^{pc} (Y_u Y_u^\dagger)^{st} \\
& + \frac{7}{8} \delta^{rb} Y_u^{*td} Y_u^{sc} (Y_u Y_u^\dagger)^{pa} + \frac{7}{8} \delta^{tb} Y_u^{*rd} Y_u^{pc} (Y_u Y_u^\dagger)^{sa} + \frac{7}{8} \delta^{pa} Y_u^{*td} Y_u^{sc} (Y_u Y_u^\dagger)^{br} + \frac{7}{8} \delta^{sa} Y_u^{*rd} Y_u^{pc} (Y_u Y_u^\dagger)^{bt} + g_L^2 \left( \frac{1}{9} \delta^{pa} \delta^{st} Y_u^{*rd} Y_u^{bc} + \frac{1}{9} \delta^{rb} \delta^{st} Y_u^{*ad} Y_u^{pc} \right. \\
& + \frac{1}{9} \delta^{pr} \delta^{sa} Y_u^{*td} Y_u^{bc} + \frac{1}{9} \delta^{pr} \delta^{tb} Y_u^{*ad} Y_u^{sc} - \frac{5}{4} \delta^{pa} \delta^{rb} Y_u^{*td} Y_u^{sc} - \frac{5}{4} \delta^{sa} \delta^{tb} Y_u^{*rd} Y_u^{pc} \Big) - g_s^2 \left( \frac{2}{9} \delta^{pa} \delta^{rs} Y_u^{*td} Y_u^{bc} + \frac{2}{9} \delta^{pt} \delta^{rb} Y_u^{*ad} Y_u^{sc} + \frac{2}{9} \delta^{pt} \delta^{sa} Y_u^{*rd} Y_u^{bc} \right. \\
& + \frac{2}{9} \delta^{rs} \delta^{tb} Y_u^{*ad} Y_u^{pc} + \delta^{rb} \delta^{sa} Y_u^{*td} Y_u^{pc} + \delta^{pa} \delta^{tb} Y_u^{*rd} Y_u^{sc} \Big) - g_Y^2 g_s^2 \left( \frac{25}{81} \delta^{pt} \delta^{rb} \delta^{sa} \delta^{cd} + \frac{25}{81} \delta^{pa} \delta^{rs} \delta^{tb} \delta^{cd} \right) - g_s^4 \left( \frac{11}{6} \delta^{pt} \delta^{rb} \delta^{sa} \delta^{cd} + \frac{11}{6} \delta^{pa} \delta^{rs} \delta^{tb} \delta^{cd} \right) \\
& - g_Y^2 g_L^2 \left( \frac{25}{81} \delta^{pa} \delta^{rb} \delta^{st} \delta^{cd} + \frac{25}{81} \delta^{pr} \delta^{sa} \delta^{tb} \delta^{cd} \right) \Big\} C_{qu}^{(\parallel)abcd} + \left\{ \frac{3}{4} T_2 \delta^{rb} \delta^{sa} Y_u^{*td} Y_u^{pc} + \frac{3}{4} T_2 \delta^{pa} \delta^{tb} Y_u^{*rd} Y_u^{sc} + \frac{3}{4} \delta^{pa} \delta^{tb} Y_u^{sc} (Y_u^\dagger Y_u Y_u^\dagger)^{rd} \right. \\
& + \frac{3}{4} \delta^{rb} \delta^{sa} Y_u^{pc} (Y_u^\dagger Y_u Y_u^\dagger)^{td} + \frac{3}{4} \delta^{rb} \delta^{sa} Y_u^{*td} (Y_u Y_u^\dagger Y_u)^{pc} + \frac{3}{4} \delta^{pa} \delta^{tb} Y_u^{*rd} (Y_u Y_u^\dagger Y_u)^{sc} + g_s^2 \left( \frac{1}{3} \delta^{pt} \delta^{ab} Y_u^{*rd} Y_u^{sc} + \frac{1}{3} \delta^{rs} \delta^{ab} Y_u^{*td} Y_u^{pc} - \frac{1}{6} \delta^{pa} \delta^{rs} Y_u^{*td} Y_u^{bc} \right. \\
& - \frac{1}{6} \delta^{pt} \delta^{rb} Y_u^{*ad} Y_u^{sc} - \frac{1}{6} \delta^{pt} \delta^{sa} Y_u^{*rd} Y_u^{bc} - \frac{1}{6} \delta^{rs} \delta^{tb} Y_u^{*ad} Y_u^{pc} - \frac{2}{3} \delta^{pt} \delta^{rb} \delta^{sa} (Y_u^\dagger Y_u)^{dc} - \frac{2}{3} \delta^{pa} \delta^{rs} \delta^{tb} (Y_u^\dagger Y_u)^{dc} - 3 \delta^{rb} \delta^{sa} Y_u^{*td} Y_u^{pc} - 3 \delta^{pa} \delta^{tb} Y_u^{*rd} Y_u^{sc} \Big) \\
& + \frac{3}{2} \delta^{sa} Y_u^{*td} Y_u^{bc} (Y_u Y_u^\dagger)^{pr} + \frac{3}{2} \delta^{tb} Y_u^{*ad} Y_u^{sc} (Y_u Y_u^\dagger)^{pr} + \frac{3}{2} \delta^{pa} Y_u^{*rd} Y_u^{bc} (Y_u Y_u^\dagger)^{st} + \frac{3}{2} \delta^{rb} Y_u^{*ad} Y_u^{pc} (Y_u Y_u^\dagger)^{st} - \frac{1}{8} \delta^{tb} Y_u^{*rd} Y_u^{sc} (Y_d Y_d^\dagger)^{pa} - \frac{1}{8} \delta^{rb} Y_u^{*td} Y_u^{pc} (Y_d Y_d^\dagger)^{sa}
\end{aligned}$$

$$\begin{aligned}
& -\frac{1}{8}\delta^{sa}Y_u^*tdY_u^{pc}(Y_dY_d^\dagger)^{br}-\frac{1}{8}\delta^{pa}Y_u^*rdY_u^{sc}(Y_dY_d^\dagger)^{bt}-\frac{1}{4}\delta^{pa}\delta^{tb}Y_u^{sc}(Y_d^\dagger Y_dY_u^\dagger)^{rd}-\frac{1}{4}\delta^{rb}\delta^{sa}Y_u^{pc}(Y_d^\dagger Y_dY_u^\dagger)^{td}-\frac{1}{4}\delta^{rb}\delta^{sa}Y_u^*td(Y_dY_d^\dagger Y_u)^{pc} \\
& -\frac{1}{4}\delta^{pa}\delta^{tb}Y_u^*rd(Y_dY_d^\dagger Y_u)^{sc}-g_Y^2\left(\frac{47}{48}\delta^{rb}\delta^{sa}Y_u^*tdY_u^{pc}+\frac{47}{48}\delta^{pa}\delta^{tb}Y_u^*rdY_u^{sc}\right)-g_L^2\left(\frac{1}{6}\delta^{pa}\delta^{st}Y_u^*rdY_u^{bc}+\frac{1}{6}\delta^{rb}\delta^{st}Y_u^*adY_u^{pc}+\frac{1}{6}\delta^{pr}\delta^{sa}Y_u^*tdY_u^{bc}\right. \\
& +\frac{1}{6}\delta^{pr}\delta^{tb}Y_u^*adY_u^{sc}+\frac{23}{16}\delta^{rb}\delta^{sa}Y_u^*tdY_u^{pc}+\frac{23}{16}\delta^{pa}\delta^{tb}Y_u^*rdY_u^{sc}\Big)-g_Y^2g_s^2\left(\frac{703}{972}\delta^{pt}\delta^{rb}\delta^{sa}\delta^{cd}+\frac{703}{972}\delta^{pa}\delta^{rs}\delta^{tb}\delta^{cd}\right)-g_Y^2g_L^2\left(\frac{25}{243}\delta^{pa}\delta^{rb}\delta^{st}\delta^{cd}\right. \\
& +\frac{25}{243}\delta^{pr}\delta^{sa}\delta^{tb}\delta^{cd}\Big)-g_s^2g_L^2\left(\frac{1}{12}\delta^{pt}\delta^{rb}\delta^{sa}\delta^{cd}+\frac{1}{12}\delta^{pa}\delta^{rs}\delta^{tb}\delta^{cd}+\frac{173}{162}\delta^{pa}\delta^{rb}\delta^{st}\delta^{cd}+\frac{173}{162}\delta^{pr}\delta^{sa}\delta^{tb}\delta^{cd}\right)-g_s^4\left(\frac{1}{81}\delta^{pt}\delta^{rb}\delta^{sa}\delta^{cd}\right. \\
& +\frac{1}{81}\delta^{pa}\delta^{rs}\delta^{tb}\delta^{cd}+\frac{4}{9}\delta^{pt}\delta^{rs}\delta^{ab}\delta^{cd}\Big)\Big\}C_{qu}^{(\times)abcd}+\left\{\frac{1}{8}\delta^{rb}Y_d^*tdY_d^{sc}(Y_uY_u^\dagger)^{pa}+\frac{1}{8}\delta^{tb}Y_d^*rdY_d^{pc}(Y_uY_u^\dagger)^{sa}+\frac{1}{8}\delta^{pa}Y_d^*tdY_d^{sc}(Y_uY_u^\dagger)^{br}+\frac{1}{8}\delta^{sa}Y_d^*rdY_d^{pc}(Y_uY_u^\dagger)^{bt}\right. \\
& +\frac{1}{2}\delta^{sa}Y_d^*tdY_d^{bc}(Y_dY_d^\dagger)^{pr}+\frac{1}{2}\delta^{tb}Y_d^*adY_d^{sc}(Y_dY_d^\dagger)^{pr}+\frac{1}{2}\delta^{pa}Y_d^*rdY_d^{bc}(Y_dY_d^\dagger)^{st}+\frac{1}{2}\delta^{rb}Y_d^*adY_d^{pc}(Y_dY_d^\dagger)^{st}+\frac{7}{8}\delta^{rb}Y_d^*tdY_d^{sc}(Y_dY_d^\dagger)^{pa}+\frac{7}{8}\delta^{tb}Y_d^*rdY_d^{pc}(Y_dY_d^\dagger)^{sa} \\
& +\frac{7}{8}\delta^{pa}Y_d^*tdY_d^{sc}(Y_dY_d^\dagger)^{br}+\frac{7}{8}\delta^{sa}Y_d^*rdY_d^{pc}(Y_dY_d^\dagger)^{bt}+g_L^2\left(\frac{1}{9}\delta^{pa}\delta^{st}Y_d^*rdY_d^{bc}+\frac{1}{9}\delta^{rb}\delta^{st}Y_d^*adY_d^{pc}+\frac{1}{9}\delta^{pr}\delta^{sa}Y_d^*tdY_d^{bc}+\frac{1}{9}\delta^{pr}\delta^{tb}Y_d^*adY_d^{sc}\right. \\
& -\frac{5}{4}\delta^{pa}\delta^{rb}Y_d^*tdY_d^{sc}-\frac{5}{4}\delta^{sa}\delta^{tb}Y_d^*rdY_d^{pc}\Big)+g_Y^2g_s^2\left(\frac{25}{162}\delta^{pt}\delta^{rb}\delta^{sa}\delta^{cd}+\frac{25}{162}\delta^{pa}\delta^{rs}\delta^{tb}\delta^{cd}\right)+g_Y^2g_L^2\left(\frac{25}{162}\delta^{pa}\delta^{rb}\delta^{st}\delta^{cd}+\frac{25}{162}\delta^{pr}\delta^{sa}\delta^{tb}\delta^{cd}\right) \\
& -g_s^2\left(\frac{2}{9}\delta^{pa}\delta^{rs}Y_d^*tdY_d^{bc}+\frac{2}{9}\delta^{pt}\delta^{rb}Y_d^*adY_d^{sc}+\frac{2}{9}\delta^{pt}\delta^{sa}Y_d^*rdY_d^{bc}+\frac{2}{9}\delta^{rs}\delta^{tb}Y_d^*adY_d^{pc}+\delta^{rb}\delta^{sa}Y_d^*tdY_d^{pc}+\delta^{pa}\delta^{tb}Y_d^*rdY_d^{sc}\right)-g_s^4\left(\frac{11}{6}\delta^{pt}\delta^{rb}\delta^{sa}\delta^{cd}\right. \\
& +\frac{11}{6}\delta^{pa}\delta^{rs}\delta^{tb}\delta^{cd}\Big)\Big\}C_{qd}^{(II)abcd}+\left\{\frac{3}{4}T_2\delta^{rb}\delta^{sa}Y_d^*tdY_d^{pc}+\frac{3}{4}T_2\delta^{pa}\delta^{tb}Y_d^*rdY_d^{sc}+\frac{3}{4}\delta^{pa}\delta^{tb}Y_d^{sc}(Y_d^\dagger Y_dY_d^\dagger)^{rd}+\frac{3}{4}\delta^{rb}\delta^{sa}Y_d^{pc}(Y_d^\dagger Y_dY_d^\dagger)^{td}\right. \\
& +\frac{3}{4}\delta^{rb}\delta^{sa}Y_d^*td(Y_dY_d^\dagger Y_d)^{pc}+\frac{3}{4}\delta^{pa}\delta^{tb}Y_d^*rd(Y_dY_d^\dagger Y_d)^{sc}+g_Y^2g_s^2\left(\frac{689}{972}\delta^{pt}\delta^{rb}\delta^{sa}\delta^{cd}+\frac{689}{972}\delta^{pa}\delta^{rs}\delta^{tb}\delta^{cd}\right)+g_Y^2g_L^2\left(\frac{25}{486}\delta^{pa}\delta^{rb}\delta^{st}\delta^{cd}\right. \\
& +\frac{25}{486}\delta^{pr}\delta^{sa}\delta^{tb}\delta^{cd}\Big)+g_s^2\left(\frac{1}{3}\delta^{pt}\delta^{ab}Y_d^*rdY_d^{sc}+\frac{1}{3}\delta^{rs}\delta^{ab}Y_d^*tdY_d^{pc}-\frac{1}{6}\delta^{pa}\delta^{rs}Y_d^*tdY_d^{bc}-\frac{1}{6}\delta^{pt}\delta^{rb}Y_d^*adY_d^{sc}-\frac{1}{6}\delta^{pt}\delta^{sa}Y_d^*rdY_d^{bc}-\frac{1}{6}\delta^{rs}\delta^{tb}Y_d^*adY_d^{pc}\right. \\
& -\frac{2}{3}\delta^{pt}\delta^{rb}\delta^{sa}(Y_d^\dagger Y_d)^{dc}-\frac{2}{3}\delta^{pa}\delta^{rs}\delta^{tb}(Y_d^\dagger Y_d)^{dc}-3\delta^{rb}\delta^{sa}Y_d^*tdY_d^{pc}-3\delta^{pa}\delta^{tb}Y_d^*rdY_d^{sc}\Big)+\frac{3}{2}\delta^{sa}Y_d^*tdY_d^{bc}(Y_dY_d^\dagger)^{pr}+\frac{3}{2}\delta^{tb}Y_d^*adY_d^{sc}(Y_dY_d^\dagger)^{pr} \\
& +\frac{3}{2}\delta^{pa}Y_d^*rdY_d^{bc}(Y_dY_d^\dagger)^{st}+\frac{3}{2}\delta^{rb}Y_d^*adY_d^{pc}(Y_dY_d^\dagger)^{st}-\frac{1}{8}\delta^{tb}Y_d^*rdY_d^{sc}(Y_uY_u^\dagger)^{pa}-\frac{1}{8}\delta^{rb}Y_d^*tdY_d^{pc}(Y_uY_u^\dagger)^{sa}-\frac{1}{8}\delta^{sa}Y_d^*tdY_d^{pc}(Y_uY_u^\dagger)^{br}-\frac{1}{8}\delta^{pa}Y_d^*rdY_d^{sc}(Y_uY_u^\dagger)^{bt} \\
& -\frac{1}{4}\delta^{pa}\delta^{tb}Y_d^{sc}(Y_u^\dagger Y_uY_d^\dagger)^{rd}-\frac{1}{4}\delta^{rb}\delta^{sa}Y_d^{pc}(Y_u^\dagger Y_uY_d^\dagger)^{td}-\frac{1}{4}\delta^{rb}\delta^{sa}Y_d^*td(Y_uY_u^\dagger Y_d)^{pc}-\frac{1}{4}\delta^{pa}\delta^{tb}Y_d^*rd(Y_uY_u^\dagger Y_d)^{sc}-g_Y^2\left(\frac{55}{48}\delta^{rb}\delta^{sa}Y_d^*tdY_d^{pc}\right. \\
& +\frac{55}{48}\delta^{pa}\delta^{tb}Y_d^*rdY_d^{sc}\Big)-g_L^2\left(\frac{1}{6}\delta^{pa}\delta^{st}Y_d^*rdY_d^{bc}+\frac{1}{6}\delta^{rb}\delta^{st}Y_d^*adY_d^{pc}+\frac{1}{6}\delta^{pr}\delta^{sa}Y_d^*tdY_d^{bc}+\frac{1}{6}\delta^{pr}\delta^{tb}Y_d^*adY_d^{sc}+\frac{23}{16}\delta^{rb}\delta^{sa}Y_d^*tdY_d^{pc}+\frac{23}{16}\delta^{pa}\delta^{tb}Y_d^*rdY_d^{sc}\right) \\
& -g_s^2g_L^2\left(\frac{1}{12}\delta^{pt}\delta^{rb}\delta^{sa}\delta^{cd}+\frac{1}{12}\delta^{pa}\delta^{rs}\delta^{tb}\delta^{cd}+\frac{173}{162}\delta^{pa}\delta^{rb}\delta^{st}\delta^{cd}+\frac{173}{162}\delta^{pr}\delta^{sa}\delta^{tb}\delta^{cd}\right)-g_s^4\left(\frac{1}{81}\delta^{pt}\delta^{rb}\delta^{sa}\delta^{cd}+\frac{1}{81}\delta^{pa}\delta^{rs}\delta^{tb}\delta^{cd}\right. \\
& +\frac{4}{9}\delta^{pt}\delta^{rs}\delta^{ab}\delta^{cd}\Big)\Big\}C_{qd}^{(\times)abcd}+\left\{\frac{4}{9}\delta^{pt}\delta^{rs}\delta^{ad}\delta^{bc}g_s^4+Y_u^*rY_u^*tdY_u^{pa}Y_u^{sc}-g_s^2\left(\frac{2}{3}\delta^{pt}\delta^{ad}Y_u^*rY_u^{sc}+\frac{2}{3}\delta^{rs}\delta^{ad}Y_u^*tY_u^{pc}\right)\right\}C_{uu}^{abcd}+\left\{\frac{4}{9}\delta^{pt}\delta^{rs}\delta^{ad}\delta^{bc}g_s^4\right.
\end{aligned}$$



$$\begin{aligned}
& + Y_d^{*rb} Y_d^{*td} Y_d^{pa} Y_d^{sc} - g_s^2 \left( \frac{2}{3} \delta^{pt} \delta^{ad} Y_d^{*rb} Y_d^{sc} + \frac{2}{3} \delta^{rs} \delta^{ad} Y_d^{*tb} Y_d^{pc} \right) \left\{ C_{dd}^{abcd} - \left\{ \frac{1}{4} Y_d^{*td} Y_u^{*rb} Y_d^{sc} Y_u^{pa} + \frac{1}{4} Y_d^{*rd} Y_u^{*tb} Y_d^{pc} Y_u^{sa} \right\} C_{ud}^{(||)abcd} + \left\{ \frac{1}{4} Y_d^{*rd} Y_u^{*tb} Y_d^{sc} Y_u^{pa} \right. \right. \\
& + \left. \frac{1}{4} Y_d^{*td} Y_u^{*rb} Y_d^{pc} Y_u^{sa} \right\} C_{ud}^{(\times)abcd} + \left\{ g_s^2 \left( \frac{1}{9} \delta^{pt} \delta^{rd} Y_e^{*ab} Y_d^{sc} + \frac{1}{9} \delta^{rs} \delta^{td} Y_e^{*ab} Y_d^{pc} \right) - \frac{1}{8} \delta^{td} Y_e^{*ab} Y_d^{sc} (Y_u Y_u^\dagger)^{pr} - \frac{1}{8} \delta^{rd} Y_e^{*ab} Y_d^{pc} (Y_u Y_u^\dagger)^{st} - \frac{3}{8} \delta^{td} Y_e^{*ab} Y_d^{sc} (Y_d Y_d^\dagger)^{pr} \right. \\
& - \left. \frac{3}{8} \delta^{rd} Y_e^{*ab} Y_d^{pc} (Y_d Y_d^\dagger)^{st} - g_L^2 \left( \frac{1}{18} \delta^{rd} \delta^{st} Y_e^{*ab} Y_d^{pc} + \frac{1}{18} \delta^{pr} \delta^{td} Y_e^{*ab} Y_d^{sc} \right) \right\} C_{ledq}^{abcd} + C_{ledq}^{*abcd} \left\{ g_s^2 \left( \frac{1}{9} \delta^{pd} \delta^{rs} Y_d^{*tc} Y_e^{ab} + \frac{1}{9} \delta^{pt} \delta^{sd} Y_d^{*rc} Y_e^{ab} \right) \right. \\
& - \left. \frac{1}{8} \delta^{sd} Y_d^{*tc} Y_e^{ab} (Y_u Y_u^\dagger)^{pr} - \frac{1}{8} \delta^{pd} Y_d^{*rc} Y_e^{ab} (Y_u Y_u^\dagger)^{st} - \frac{3}{8} \delta^{sd} Y_d^{*tc} Y_e^{ab} (Y_d Y_d^\dagger)^{pr} - \frac{3}{8} \delta^{pd} Y_d^{*rc} Y_e^{ab} (Y_d Y_d^\dagger)^{st} - g_L^2 \left( \frac{1}{18} \delta^{pd} \delta^{st} Y_d^{*rc} Y_e^{ab} + \frac{1}{18} \delta^{pr} \delta^{sd} Y_d^{*tc} Y_e^{ab} \right) \right\} \\
& + \left\{ \frac{1}{8} \delta^{sc} Y_d^{*td} Y_u^{*rb} (Y_d Y_d^\dagger)^{pa} + \frac{1}{8} \delta^{pc} Y_d^{*rd} Y_u^{*tb} (Y_d Y_d^\dagger)^{sa} + \frac{1}{8} \delta^{sa} Y_d^{*rd} Y_u^{*tb} (Y_u Y_u^\dagger)^{pc} + \frac{1}{8} \delta^{pa} Y_d^{*td} Y_u^{*rb} (Y_u Y_u^\dagger)^{sc} + g_Y^2 \left( \frac{37}{96} \delta^{pc} \delta^{sa} Y_d^{*rd} Y_u^{*tb} \right. \right. \\
& + \left. \frac{37}{96} \delta^{pa} \delta^{sc} Y_d^{*td} Y_u^{*rb} \right) + g_L^2 \left( \frac{7}{72} \delta^{pa} \delta^{st} Y_d^{*rd} Y_u^{*cb} + \frac{7}{72} \delta^{pc} \delta^{st} Y_d^{*ad} Y_u^{*rb} + \frac{7}{72} \delta^{pr} \delta^{sa} Y_d^{*td} Y_u^{*cb} + \frac{7}{72} \delta^{pr} \delta^{sc} Y_d^{*ad} Y_u^{*tb} + \frac{21}{32} \delta^{pc} \delta^{sa} Y_d^{*rd} Y_u^{*tb} \right. \\
& + \left. \frac{21}{32} \delta^{pa} \delta^{sc} Y_d^{*td} Y_u^{*rb} - \frac{1}{6} \delta^{pa} \delta^{st} Y_d^{*cd} Y_u^{*rb} - \frac{1}{6} \delta^{pc} \delta^{st} Y_d^{*rd} Y_u^{*ab} - \frac{1}{6} \delta^{pr} \delta^{sa} Y_d^{*cd} Y_u^{*tb} - \frac{1}{6} \delta^{pr} \delta^{sc} Y_d^{*td} Y_u^{*ab} \right) + g_s^2 \left( \frac{1}{3} \delta^{pa} \delta^{rs} Y_d^{*cd} Y_u^{*tb} \right. \\
& + \frac{1}{3} \delta^{pc} \delta^{rs} Y_d^{*td} Y_u^{*ab} + \frac{1}{3} \delta^{pt} \delta^{sa} Y_d^{*cd} Y_u^{*rb} + \frac{1}{3} \delta^{pt} \delta^{sc} Y_d^{*rd} Y_u^{*ab} + \frac{13}{8} \delta^{pc} \delta^{sa} Y_d^{*td} Y_u^{*rb} + \frac{13}{8} \delta^{pa} \delta^{sc} Y_d^{*rd} Y_u^{*tb} - \frac{1}{36} \delta^{pa} \delta^{rs} Y_d^{*td} Y_u^{*cb} \\
& - \frac{1}{36} \delta^{pc} \delta^{rs} Y_d^{*ad} Y_u^{*tb} - \frac{1}{36} \delta^{pt} \delta^{sa} Y_d^{*rd} Y_u^{*cb} - \frac{1}{36} \delta^{pt} \delta^{sc} Y_d^{*ad} Y_u^{*rb} - \frac{17}{8} \delta^{pc} \delta^{sa} Y_d^{*rd} Y_u^{*tb} - \frac{17}{8} \delta^{pa} \delta^{sc} Y_d^{*td} Y_u^{*rb} \Big) - \frac{1}{16} \delta^{sc} Y_d^{*ad} Y_u^{*tb} (Y_d Y_d^\dagger)^{pr} \\
& - \frac{1}{16} \delta^{pc} Y_d^{*ad} Y_u^{*rb} (Y_d Y_d^\dagger)^{st} - \frac{1}{16} \delta^{sa} Y_d^{*td} Y_u^{*cb} (Y_u Y_u^\dagger)^{pr} - \frac{1}{16} \delta^{pa} Y_d^{*rd} Y_u^{*cb} (Y_u Y_u^\dagger)^{st} - \frac{1}{8} T_2 \delta^{pc} \delta^{sa} Y_d^{*rd} Y_u^{*tb} - \frac{1}{8} T_2 \delta^{pa} \delta^{sc} Y_d^{*td} Y_u^{*rb} \\
& - \frac{1}{8} \delta^{pc} \delta^{sa} Y_u^{*tb} (Y_d^\dagger Y_d Y_d^\dagger)^{rd} - \frac{1}{8} \delta^{pa} \delta^{sc} Y_u^{*rb} (Y_d^\dagger Y_d Y_d^\dagger)^{td} - \frac{1}{8} \delta^{pa} \delta^{sc} Y_d^{*td} (Y_d^\dagger Y_d Y_u^\dagger)^{rb} - \frac{1}{8} \delta^{pc} \delta^{sa} Y_d^{*rd} (Y_d^\dagger Y_d Y_u^\dagger)^{tb} - \frac{1}{8} \delta^{pc} \delta^{sa} Y_u^{*tb} (Y_u^\dagger Y_u Y_d^\dagger)^{rd} \\
& - \frac{1}{8} \delta^{pa} \delta^{sc} Y_u^{*rb} (Y_u^\dagger Y_u Y_d^\dagger)^{td} - \frac{1}{8} \delta^{pa} \delta^{sc} Y_d^{*td} (Y_u^\dagger Y_u Y_u^\dagger)^{rb} - \frac{1}{8} \delta^{pc} \delta^{sa} Y_d^{*rd} (Y_u^\dagger Y_u Y_u^\dagger)^{tb} - \frac{3}{16} \delta^{sa} Y_d^{*td} Y_u^{*cb} (Y_d Y_d^\dagger)^{pr} - \frac{3}{16} \delta^{pa} Y_d^{*rd} Y_u^{*cb} (Y_d Y_d^\dagger)^{st} \\
& - \frac{3}{16} \delta^{sc} Y_d^{*ad} Y_u^{*tb} (Y_u Y_u^\dagger)^{pr} - \frac{3}{16} \delta^{pc} Y_d^{*ad} Y_u^{*rb} (Y_u Y_u^\dagger)^{st} - \frac{3}{8} \delta^{sa} Y_d^{*cd} Y_u^{*tb} (Y_d Y_d^\dagger)^{pr} - \frac{3}{8} \delta^{pa} Y_d^{*cd} Y_u^{*rb} (Y_d Y_d^\dagger)^{st} - \frac{3}{8} \delta^{sc} Y_d^{*td} Y_u^{*ab} (Y_u Y_u^\dagger)^{pr} \\
& - \frac{3}{8} \delta^{pc} Y_d^{*rd} Y_u^{*ab} (Y_u Y_u^\dagger)^{st} - \frac{9}{8} \delta^{sc} Y_d^{*td} Y_u^{*ab} (Y_d Y_d^\dagger)^{pr} - \frac{9}{8} \delta^{pc} Y_d^{*rd} Y_u^{*ab} (Y_d Y_d^\dagger)^{st} - \frac{9}{8} \delta^{sa} Y_d^{*cd} Y_u^{*tb} (Y_u Y_u^\dagger)^{pr} - \frac{9}{8} \delta^{pa} Y_d^{*cd} Y_u^{*rb} (Y_u Y_u^\dagger)^{st} \Big\} C_{quqd}^{(||)abcd} \\
& + \left( C_{quqd}^{(||)*} \right)^{abcd} \left\{ \frac{1}{8} \delta^{tc} Y_d^{sd} Y_u^{pb} (Y_d Y_d^\dagger)^{ar} + \frac{1}{8} \delta^{rc} Y_d^{pd} Y_u^{sb} (Y_d Y_d^\dagger)^{at} + \frac{1}{8} \delta^{ta} Y_d^{pd} Y_u^{sb} (Y_u Y_u^\dagger)^{cr} + \frac{1}{8} \delta^{ra} Y_d^{sd} Y_u^{pb} (Y_u Y_u^\dagger)^{ct} + g_Y^2 \left( \frac{37}{96} \delta^{rc} \delta^{ta} Y_d^{pd} Y_u^{sb} + \frac{37}{96} \delta^{ra} \delta^{tc} Y_d^{sd} Y_u^{pb} \right) \right. \\
& + g_L^2 \left( \frac{7}{72} \delta^{ra} \delta^{st} Y_d^{pd} Y_u^{cb} + \frac{7}{72} \delta^{rc} \delta^{st} Y_d^{ad} Y_u^{pb} + \frac{7}{72} \delta^{pr} \delta^{ta} Y_d^{sd} Y_u^{cb} + \frac{7}{72} \delta^{pr} \delta^{tc} Y_d^{ad} Y_u^{sb} + \frac{21}{32} \delta^{rc} \delta^{ta} Y_d^{pd} Y_u^{sb} + \frac{21}{32} \delta^{ra} \delta^{tc} Y_d^{sd} Y_u^{pb} - \frac{1}{6} \delta^{ra} \delta^{st} Y_d^{cd} Y_u^{pb} \right. \\
& - \left. \frac{1}{6} \delta^{rc} \delta^{st} Y_d^{pd} Y_u^{ab} - \frac{1}{6} \delta^{pr} \delta^{ta} Y_d^{cd} Y_u^{sb} - \frac{1}{6} \delta^{pr} \delta^{tc} Y_d^{sd} Y_u^{ab} \right) + g_s^2 \left( \frac{1}{3} \delta^{pt} \delta^{ra} Y_d^{cd} Y_u^{sb} + \frac{1}{3} \delta^{pt} \delta^{rc} Y_d^{sd} Y_u^{ab} + \frac{1}{3} \delta^{rs} \delta^{ta} Y_d^{cd} Y_u^{pb} + \frac{1}{3} \delta^{rs} \delta^{tc} Y_d^{pd} Y_u^{ab} \right.
\end{aligned}$$

$$\begin{aligned}
& + \frac{13}{8} \delta^{rc} \delta^{ta} Y_d^{sd} Y_u^{pb} + \frac{13}{8} \delta^{ra} \delta^{tc} Y_d^{pd} Y_u^{sb} - \frac{1}{36} \delta^{pt} \delta^{ra} Y_d^{sd} Y_u^{cb} - \frac{1}{36} \delta^{pt} \delta^{rc} Y_d^{ad} Y_u^{sb} - \frac{1}{36} \delta^{rs} \delta^{ta} Y_d^{pd} Y_u^{cb} - \frac{1}{36} \delta^{rs} \delta^{tc} Y_d^{ad} Y_u^{pb} - \frac{17}{8} \delta^{rc} \delta^{ta} Y_d^{pd} Y_u^{sb} \\
& - \frac{17}{8} \delta^{ra} \delta^{tc} Y_d^{sd} Y_u^{pb} \Big) - \frac{1}{16} \delta^{tc} Y_d^{ad} Y_u^{sb} (Y_d Y_d^\dagger)^{pr} - \frac{1}{16} \delta^{rc} Y_d^{ad} Y_u^{pb} (Y_d Y_d^\dagger)^{st} - \frac{1}{16} \delta^{ta} Y_d^{sd} Y_u^{cb} (Y_u Y_u^\dagger)^{pr} - \frac{1}{16} \delta^{ra} Y_d^{pd} Y_u^{cb} (Y_u Y_u^\dagger)^{st} - \frac{1}{8} T_2 \delta^{rc} \delta^{ta} Y_d^{pd} Y_u^{sb} \\
& - \frac{1}{8} T_2 \delta^{ra} \delta^{tc} Y_d^{sd} Y_u^{pb} - \frac{1}{8} \delta^{rc} \delta^{ta} Y_u^{sb} (Y_d Y_d^\dagger Y_d)^{pd} - \frac{1}{8} \delta^{ra} \delta^{tc} Y_u^{pb} (Y_d Y_d^\dagger Y_d)^{sd} - \frac{1}{8} \delta^{ra} \delta^{tc} Y_d^{sd} (Y_d Y_d^\dagger Y_u)^{pb} - \frac{1}{8} \delta^{rc} \delta^{ta} Y_d^{pd} (Y_d Y_d^\dagger Y_u)^{sb} \\
& - \frac{1}{8} \delta^{rc} \delta^{ta} Y_u^{sb} (Y_u Y_u^\dagger Y_d)^{pd} - \frac{1}{8} \delta^{ra} \delta^{tc} Y_u^{pb} (Y_u Y_u^\dagger Y_d)^{sd} - \frac{1}{8} \delta^{ra} \delta^{tc} Y_d^{sd} (Y_u Y_u^\dagger Y_u)^{pb} - \frac{1}{8} \delta^{rc} \delta^{ta} Y_d^{pd} (Y_u Y_u^\dagger Y_u)^{sb} - \frac{3}{16} \delta^{ta} Y_d^{sd} Y_u^{cb} (Y_d Y_d^\dagger)^{pr} \\
& - \frac{3}{16} \delta^{ra} Y_d^{pd} Y_u^{cb} (Y_d Y_d^\dagger)^{st} - \frac{3}{16} \delta^{tc} Y_d^{ad} Y_u^{sb} (Y_u Y_u^\dagger)^{pr} - \frac{3}{16} \delta^{rc} Y_d^{ad} Y_u^{pb} (Y_u Y_u^\dagger)^{st} - \frac{3}{8} \delta^{ta} Y_d^{cd} Y_u^{sb} (Y_d Y_d^\dagger)^{pr} - \frac{3}{8} \delta^{ra} Y_d^{cd} Y_u^{pb} (Y_d Y_d^\dagger)^{st} - \frac{3}{8} \delta^{tc} Y_d^{sd} Y_u^{ab} (Y_u Y_u^\dagger)^{pr} \\
& - \frac{3}{8} \delta^{rc} Y_d^{pd} Y_u^{ab} (Y_u Y_u^\dagger)^{st} - \frac{9}{8} \delta^{tc} Y_d^{sd} Y_u^{ab} (Y_d Y_d^\dagger)^{pr} - \frac{9}{8} \delta^{rc} Y_d^{pd} Y_u^{ab} (Y_d Y_d^\dagger)^{st} - \frac{9}{8} \delta^{ta} Y_d^{cd} Y_u^{sb} (Y_u Y_u^\dagger)^{pr} - \frac{9}{8} \delta^{ra} Y_d^{cd} Y_u^{pb} (Y_u Y_u^\dagger)^{st} \Big\} + \left\{ \frac{1}{8} T_2 \delta^{pc} \delta^{sa} Y_d^{*td} Y_u^{*rb} \right. \\
& + \frac{1}{8} T_2 \delta^{pa} \delta^{sc} Y_d^{*rd} Y_u^{*tb} + \frac{1}{8} \delta^{pa} \delta^{sc} Y_u^{*tb} (Y_d^\dagger Y_d Y_d^\dagger)^{rd} + \frac{1}{8} \delta^{pc} \delta^{sa} Y_u^{*rb} (Y_d^\dagger Y_d Y_d^\dagger)^{td} + \frac{1}{8} \delta^{pc} \delta^{sa} Y_d^{*td} (Y_d^\dagger Y_d Y_u^\dagger)^{rb} + \frac{1}{8} \delta^{pa} \delta^{sc} Y_d^{*rd} (Y_d^\dagger Y_d Y_u^\dagger)^{tb} \\
& + \frac{1}{8} \delta^{pa} \delta^{sc} Y_u^{*tb} (Y_u^\dagger Y_u Y_d^\dagger)^{rd} + \frac{1}{8} \delta^{pc} \delta^{sa} Y_u^{*rb} (Y_u^\dagger Y_u Y_d^\dagger)^{td} + \frac{1}{8} \delta^{pc} \delta^{sa} Y_d^{*td} (Y_u^\dagger Y_u Y_u^\dagger)^{rb} + \frac{1}{8} \delta^{pa} \delta^{sc} Y_d^{*rd} (Y_u^\dagger Y_u Y_u^\dagger)^{tb} + \frac{5}{16} \delta^{sa} Y_d^{*td} Y_u^{*rb} (Y_d Y_d^\dagger)^{pc} \\
& + \frac{5}{16} \delta^{pa} Y_d^{*rd} Y_u^{*tb} (Y_d Y_d^\dagger)^{sc} + \frac{5}{16} \delta^{sc} Y_d^{*rd} Y_u^{*tb} (Y_u Y_u^\dagger)^{pa} + \frac{5}{16} \delta^{pc} Y_d^{*td} Y_u^{*rb} (Y_u Y_u^\dagger)^{sa} + g_L^2 \left( \frac{1}{24} \delta^{pa} \delta^{st} Y_d^{*rd} Y_u^{*cb} + \frac{1}{24} \delta^{pc} \delta^{st} Y_d^{*ad} Y_u^{*rb} \right. \\
& + \frac{1}{24} \delta^{pr} \delta^{sa} Y_d^{*td} Y_u^{*cb} + \frac{1}{24} \delta^{pr} \delta^{sc} Y_d^{*ad} Y_u^{*tb} - \frac{5}{36} \delta^{pa} \delta^{st} Y_d^{*cd} Y_u^{*rb} - \frac{5}{36} \delta^{pc} \delta^{st} Y_d^{*rd} Y_u^{*ab} - \frac{5}{36} \delta^{pr} \delta^{sa} Y_d^{*cd} Y_u^{*tb} - \frac{5}{36} \delta^{pr} \delta^{sc} Y_d^{*td} Y_u^{*ab} \\
& - \frac{21}{32} \delta^{pc} \delta^{sa} Y_d^{*td} Y_u^{*rb} - \frac{21}{32} \delta^{pa} \delta^{sc} Y_d^{*rd} Y_u^{*tb} \Big) + g_s^2 \left( \frac{1}{6} \delta^{pa} \delta^{rs} Y_d^{*td} Y_u^{*cb} + \frac{1}{6} \delta^{pc} \delta^{rs} Y_d^{*ad} Y_u^{*tb} + \frac{1}{6} \delta^{pt} \delta^{sa} Y_d^{*rd} Y_u^{*cb} + \frac{1}{6} \delta^{pt} \delta^{sc} Y_d^{*ad} Y_u^{*rb} \right. \\
& + \frac{7}{36} \delta^{pa} \delta^{rs} Y_d^{*cd} Y_u^{*tb} + \frac{7}{36} \delta^{pc} \delta^{rs} Y_d^{*td} Y_u^{*ab} + \frac{7}{36} \delta^{pt} \delta^{sa} Y_d^{*cd} Y_u^{*rb} + \frac{7}{36} \delta^{pt} \delta^{sc} Y_d^{*rd} Y_u^{*ab} + \frac{7}{4} \delta^{pc} \delta^{sa} Y_d^{*td} Y_u^{*rb} + \frac{7}{4} \delta^{pa} \delta^{sc} Y_d^{*rd} Y_u^{*tb} \\
& - \frac{7}{4} \delta^{pc} \delta^{sa} Y_d^{*rd} Y_u^{*tb} - \frac{7}{4} \delta^{pa} \delta^{sc} Y_d^{*td} Y_u^{*rb} \Big) - \frac{1}{8} \delta^{sa} Y_d^{*cd} Y_u^{*tb} (Y_d Y_d^\dagger)^{pr} - \frac{1}{8} \delta^{pa} Y_d^{*cd} Y_u^{*rb} (Y_d Y_d^\dagger)^{st} - \frac{1}{8} \delta^{sc} Y_d^{*td} Y_u^{*ab} (Y_u Y_u^\dagger)^{pr} - \frac{1}{8} \delta^{pc} Y_d^{*rd} Y_u^{*ab} (Y_u Y_u^\dagger)^{st} \\
& - \frac{3}{16} \delta^{sc} Y_d^{*ad} Y_u^{*tb} (Y_d Y_d^\dagger)^{pr} - \frac{3}{16} \delta^{pc} Y_d^{*ad} Y_u^{*rb} (Y_d Y_d^\dagger)^{st} - \frac{3}{16} \delta^{sa} Y_d^{*td} Y_u^{*cb} (Y_u Y_u^\dagger)^{pr} - \frac{3}{16} \delta^{pa} Y_d^{*rd} Y_u^{*cb} (Y_u Y_u^\dagger)^{st} - \frac{3}{8} \delta^{sc} Y_d^{*td} Y_u^{*ab} (Y_d Y_d^\dagger)^{pr} \\
& - \frac{3}{8} \delta^{pc} Y_d^{*rd} Y_u^{*ab} (Y_d Y_d^\dagger)^{st} - \frac{3}{8} \delta^{sa} Y_d^{*cd} Y_u^{*tb} (Y_u Y_u^\dagger)^{pr} - \frac{3}{8} \delta^{pa} Y_d^{*cd} Y_u^{*rb} (Y_u Y_u^\dagger)^{st} - \frac{9}{16} \delta^{sa} Y_d^{*td} Y_u^{*cb} (Y_d Y_d^\dagger)^{pr} - \frac{9}{16} \delta^{pa} Y_d^{*rd} Y_u^{*cb} (Y_d Y_d^\dagger)^{st} \\
& - \frac{9}{16} \delta^{sc} Y_d^{*ad} Y_u^{*tb} (Y_u Y_u^\dagger)^{pr} - \frac{9}{16} \delta^{pc} Y_d^{*ad} Y_u^{*rb} (Y_u Y_u^\dagger)^{st} - g_Y^2 \left( \frac{37}{96} \delta^{pc} \delta^{sa} Y_d^{*td} Y_u^{*rb} + \frac{37}{96} \delta^{pa} \delta^{sc} Y_d^{*rd} Y_u^{*tb} \right) \Big\} C_{quqd}^{(\times)abcd} + \left( C_{quqd}^{(\times)*} \right)^{abcd} \left\{ \frac{1}{8} T_2 \delta^{rc} \delta^{ta} Y_d^{sd} Y_u^{pb} \right. \\
& + \frac{1}{8} T_2 \delta^{ra} \delta^{tc} Y_d^{pd} Y_u^{sb} + \frac{1}{8} \delta^{ra} \delta^{tc} Y_u^{sb} (Y_d Y_d^\dagger Y_d)^{pd} + \frac{1}{8} \delta^{rc} \delta^{ta} Y_u^{pb} (Y_d Y_d^\dagger Y_d)^{sd} + \frac{1}{8} \delta^{rc} \delta^{ta} Y_d^{sd} (Y_d Y_d^\dagger Y_u)^{pb} + \frac{1}{8} \delta^{ra} \delta^{tc} Y_d^{pd} (Y_d Y_d^\dagger Y_u)^{sb} \\
& + \frac{1}{8} \delta^{ra} \delta^{tc} Y_u^{sb} (Y_u Y_u^\dagger Y_d)^{pd} + \frac{1}{8} \delta^{rc} \delta^{ta} Y_u^{pb} (Y_u Y_u^\dagger Y_d)^{sd} + \frac{1}{8} \delta^{rc} \delta^{ta} Y_d^{sd} (Y_u Y_u^\dagger Y_u)^{pb} + \frac{1}{8} \delta^{ra} \delta^{tc} Y_d^{pd} (Y_u Y_u^\dagger Y_u)^{sb} + \frac{5}{16} \delta^{ta} Y_d^{sd} Y_u^{pb} (Y_d Y_d^\dagger)^{cr} \\
& + \frac{5}{16} \delta^{ra} Y_d^{pd} Y_u^{sb} (Y_d Y_d^\dagger)^{ct} + \frac{5}{16} \delta^{tc} Y_d^{pd} Y_u^{sb} (Y_u Y_u^\dagger)^{ar} + \frac{5}{16} \delta^{rc} Y_d^{sd} Y_u^{pb} (Y_u Y_u^\dagger)^{at} + g_L^2 \left( \frac{1}{24} \delta^{ra} \delta^{st} Y_d^{pd} Y_u^{cb} + \frac{1}{24} \delta^{rc} \delta^{st} Y_d^{ad} Y_u^{pb} + \frac{1}{24} \delta^{pr} \delta^{ta} Y_d^{sd} Y_u^{cb} \right.
\end{aligned}$$

$$\begin{aligned}
& + \frac{1}{24} \delta^{pr} \delta^{tc} Y_d^{ad} Y_u^{sb} - \frac{5}{36} \delta^{ra} \delta^{st} Y_d^{cd} Y_u^{pb} - \frac{5}{36} \delta^{rc} \delta^{st} Y_d^{pd} Y_u^{ab} - \frac{5}{36} \delta^{pr} \delta^{ta} Y_d^{cd} Y_u^{sb} - \frac{5}{36} \delta^{pr} \delta^{tc} Y_d^{sd} Y_u^{ab} - \frac{21}{32} \delta^{rc} \delta^{ta} Y_d^{sd} Y_u^{pb} - \frac{21}{32} \delta^{ra} \delta^{tc} Y_d^{pd} Y_u^{sb} \\
& + g_s^2 \left( \frac{1}{6} \delta^{pt} \delta^{ra} Y_d^{sd} Y_u^{cb} + \frac{1}{6} \delta^{pt} \delta^{rc} Y_d^{ad} Y_u^{sb} + \frac{1}{6} \delta^{rs} \delta^{ta} Y_d^{pd} Y_u^{cb} + \frac{1}{6} \delta^{rs} \delta^{tc} Y_d^{ad} Y_u^{pb} + \frac{7}{36} \delta^{pt} \delta^{ra} Y_d^{cd} Y_u^{sb} + \frac{7}{36} \delta^{pt} \delta^{rc} Y_d^{sd} Y_u^{ab} + \frac{7}{36} \delta^{rs} \delta^{ta} Y_d^{cd} Y_u^{pb} \right. \\
& + \frac{7}{36} \delta^{rs} \delta^{tc} Y_d^{pd} Y_u^{ab} + \frac{7}{4} \delta^{rc} \delta^{ta} Y_d^{sd} Y_u^{pb} + \frac{7}{4} \delta^{ra} \delta^{tc} Y_d^{pd} Y_u^{sb} - \frac{7}{4} \delta^{rc} \delta^{ta} Y_d^{pd} Y_u^{sb} - \frac{7}{4} \delta^{ra} \delta^{tc} Y_d^{sd} Y_u^{pb} \left. \right) - \frac{1}{8} \delta^{ta} Y_d^{cd} Y_u^{sb} (Y_d Y_d^\dagger)^{pr} - \frac{1}{8} \delta^{ra} Y_d^{cd} Y_u^{pb} (Y_d Y_d^\dagger)^{st} \\
& - \frac{1}{8} \delta^{tc} Y_d^{sd} Y_u^{ab} (Y_u Y_u^\dagger)^{pr} - \frac{1}{8} \delta^{rc} Y_d^{pd} Y_u^{ab} (Y_u Y_u^\dagger)^{st} - \frac{3}{16} \delta^{tc} Y_d^{ad} Y_u^{sb} (Y_d Y_d^\dagger)^{pr} - \frac{3}{16} \delta^{rc} Y_d^{ad} Y_u^{pb} (Y_d Y_d^\dagger)^{st} - \frac{3}{16} \delta^{ta} Y_d^{sd} Y_u^{cb} (Y_u Y_u^\dagger)^{pr} - \frac{3}{16} \delta^{ra} Y_d^{pd} Y_u^{cb} (Y_u Y_u^\dagger)^{st} \\
& - \frac{3}{8} \delta^{tc} Y_d^{sd} Y_u^{ab} (Y_d Y_d^\dagger)^{pr} - \frac{3}{8} \delta^{rc} Y_d^{pd} Y_u^{ab} (Y_d Y_d^\dagger)^{st} - \frac{3}{8} \delta^{ta} Y_d^{cd} Y_u^{sb} (Y_u Y_u^\dagger)^{pr} - \frac{3}{8} \delta^{ra} Y_d^{cd} Y_u^{pb} (Y_u Y_u^\dagger)^{st} - \frac{9}{16} \delta^{ta} Y_d^{sd} Y_u^{cb} (Y_d Y_d^\dagger)^{pr} - \frac{9}{16} \delta^{ra} Y_d^{pd} Y_u^{cb} (Y_d Y_d^\dagger)^{st} \\
& - \frac{9}{16} \delta^{tc} Y_d^{ad} Y_u^{sb} (Y_u Y_u^\dagger)^{pr} - \frac{9}{16} \delta^{rc} Y_d^{ad} Y_u^{pb} (Y_u Y_u^\dagger)^{st} - g_Y^2 \left( \frac{37}{96} \delta^{rc} \delta^{ta} Y_d^{sd} Y_u^{pb} + \frac{37}{96} \delta^{ra} \delta^{tc} Y_d^{pd} Y_u^{sb} \right) \left. \right\} + \left\{ \frac{1}{8} \delta^{sc} Y_e^{*ab} Y_u^{*td} (Y_d Y_d^\dagger)^{pr} + \frac{1}{8} \delta^{pc} Y_e^{*ab} Y_u^{*rd} (Y_d Y_d^\dagger)^{st} \right. \\
& + \frac{3}{8} \delta^{sc} Y_e^{*ab} Y_u^{*td} (Y_u Y_u^\dagger)^{pr} + \frac{3}{8} \delta^{pc} Y_e^{*ab} Y_u^{*rd} (Y_u Y_u^\dagger)^{st} + g_L^2 \left( \frac{1}{18} \delta^{pc} \delta^{st} Y_e^{*ab} Y_u^{*rd} + \frac{1}{18} \delta^{pr} \delta^{sc} Y_e^{*ab} Y_u^{*td} \right) - g_s^2 \left( \frac{1}{9} \delta^{pc} \delta^{rs} Y_e^{*ab} Y_u^{*td} \right. \\
& + \left. \frac{1}{9} \delta^{pt} \delta^{sc} Y_e^{*ab} Y_u^{*rd} \right) \left. \right\} C_{lequ}^{abcd} + C_{lequ}^{*abcd} \left\{ \frac{1}{8} \delta^{tc} Y_e^{ab} Y_u^{sd} (Y_d Y_d^\dagger)^{pr} + \frac{1}{8} \delta^{rc} Y_e^{ab} Y_u^{pd} (Y_d Y_d^\dagger)^{st} + \frac{3}{8} \delta^{tc} Y_e^{ab} Y_u^{sd} (Y_u Y_u^\dagger)^{pr} + \frac{3}{8} \delta^{rc} Y_e^{ab} Y_u^{pd} (Y_u Y_u^\dagger)^{st} \right. \\
& + g_L^2 \left( \frac{1}{18} \delta^{rc} \delta^{st} Y_e^{ab} Y_u^{pd} + \frac{1}{18} \delta^{pr} \delta^{tc} Y_e^{ab} Y_u^{sd} \right) - g_s^2 \left( \frac{1}{9} \delta^{pt} \delta^{rc} Y_e^{ab} Y_u^{sd} + \frac{1}{9} \delta^{rs} \delta^{tc} Y_e^{ab} Y_u^{pd} \right) \left. \right\} + \left\{ g_L^2 \left( \frac{1}{72} \delta^{pc} \delta^{st} Y_e^{*ad} Y_u^{*rb} + \frac{1}{72} \delta^{pr} \delta^{sc} Y_e^{*ad} Y_u^{*tb} \right) \right. \\
& + g_s^2 \left( \frac{1}{18} \delta^{pc} \delta^{rs} Y_e^{*ad} Y_u^{*tb} + \frac{1}{18} \delta^{pt} \delta^{sc} Y_e^{*ad} Y_u^{*rb} \right) - \frac{1}{16} \delta^{sc} Y_e^{*ad} Y_u^{*tb} (Y_d Y_d^\dagger)^{pr} - \frac{1}{16} \delta^{pc} Y_e^{*ad} Y_u^{*rb} (Y_d Y_d^\dagger)^{st} - \frac{3}{16} \delta^{sc} Y_e^{*ad} Y_u^{*tb} (Y_u Y_u^\dagger)^{pr} \\
& - \frac{3}{16} \delta^{pc} Y_e^{*ad} Y_u^{*rb} (Y_u Y_u^\dagger)^{st} \left. \right\} C_{luqe}^{abcd} + C_{luqe}^{*abcd} \left\{ g_L^2 \left( \frac{1}{72} \delta^{rc} \delta^{st} Y_e^{ad} Y_u^{pb} + \frac{1}{72} \delta^{pr} \delta^{tc} Y_e^{ad} Y_u^{sb} \right) + g_s^2 \left( \frac{1}{18} \delta^{pt} \delta^{rc} Y_e^{ad} Y_u^{sb} + \frac{1}{18} \delta^{rs} \delta^{tc} Y_e^{ad} Y_u^{pb} \right) \right. \\
& - \frac{1}{16} \delta^{tc} Y_e^{ad} Y_u^{sb} (Y_d Y_d^\dagger)^{pr} - \frac{1}{16} \delta^{rc} Y_e^{ad} Y_u^{pb} (Y_d Y_d^\dagger)^{st} - \frac{3}{16} \delta^{tc} Y_e^{ad} Y_u^{sb} (Y_u Y_u^\dagger)^{pr} - \frac{3}{16} \delta^{rc} Y_e^{ad} Y_u^{pb} (Y_u Y_u^\dagger)^{st} \left. \right\} + \frac{4}{9} \delta^{pr} \delta^{st} \delta^{ad} \delta^{bc} g_L^4 C_{\ell\ell}^{abcd} \\
& + \left\{ g_s^4 \left( \frac{15}{2} \delta^{pa} \delta^{rd} \delta^{sc} \delta^{tb} + \frac{1246}{81} \delta^{pt} \delta^{rd} \delta^{sa} \delta^{bc} + \frac{1246}{81} \delta^{pa} \delta^{rs} \delta^{td} \delta^{bc} - \frac{14}{3} \delta^{pt} \delta^{rb} \delta^{sa} \delta^{cd} - \frac{14}{3} \delta^{pa} \delta^{rs} \delta^{tb} \delta^{cd} \right) + g_Y^2 g_s^2 \left( \frac{115}{243} \delta^{pt} \delta^{rd} \delta^{sa} \delta^{bc} \right. \right. \\
& + \frac{115}{243} \delta^{pa} \delta^{rs} \delta^{td} \delta^{bc} - \frac{25}{81} \delta^{pt} \delta^{rb} \delta^{sa} \delta^{cd} - \frac{25}{81} \delta^{pa} \delta^{rs} \delta^{tb} \delta^{cd} - \frac{13}{6} \delta^{pa} \delta^{rd} \delta^{sc} \delta^{tb} \left. \right) + g_L^4 \left( \frac{4}{3} \delta^{pr} \delta^{st} \delta^{ad} \delta^{bc} + \frac{79}{9} \delta^{pa} \delta^{rd} \delta^{st} \delta^{bc} + \frac{79}{9} \delta^{pr} \delta^{sa} \delta^{td} \delta^{bc} \right. \\
& + \frac{49}{3} \delta^{pa} \delta^{rb} \delta^{sc} \delta^{td} - \delta^{pa} \delta^{rb} \delta^{st} \delta^{cd} - \delta^{pr} \delta^{sa} \delta^{tb} \delta^{cd} \left. \right) + g_Y^2 g_L^2 \left( \frac{115}{243} \delta^{pa} \delta^{rd} \delta^{st} \delta^{bc} + \frac{115}{243} \delta^{pr} \delta^{sa} \delta^{td} \delta^{bc} - \frac{25}{81} \delta^{pa} \delta^{rb} \delta^{st} \delta^{cd} - \frac{25}{81} \delta^{pr} \delta^{sa} \delta^{tb} \delta^{cd} \right. \\
& - \frac{13}{6} \delta^{pa} \delta^{rb} \delta^{sc} \delta^{td} \left. \right) + \delta^{rd} \delta^{sa} (Y_d Y_d^\dagger)^{bt} (Y_u Y_u^\dagger)^{pc} + \delta^{pa} \delta^{td} (Y_d Y_d^\dagger)^{br} (Y_u Y_u^\dagger)^{sc} + \delta^{pa} \delta^{td} (Y_d Y_d^\dagger)^{sc} (Y_u Y_u^\dagger)^{br} + \delta^{rd} \delta^{sa} (Y_d Y_d^\dagger)^{pc} (Y_u Y_u^\dagger)^{bt} \\
& + \frac{3}{2} \delta^{sa} \delta^{td} (Y_d Y_d^\dagger)^{pr} (Y_d Y_d^\dagger)^{bc} + \frac{3}{2} \delta^{pa} \delta^{rd} (Y_d Y_d^\dagger)^{st} (Y_d Y_d^\dagger)^{bc} + \frac{3}{2} \delta^{sa} \delta^{td} (Y_d Y_d^\dagger)^{bc} (Y_u Y_u^\dagger)^{pr} + \frac{3}{2} \delta^{pa} \delta^{rd} (Y_d Y_d^\dagger)^{bc} (Y_u Y_u^\dagger)^{st} + \frac{3}{2} \delta^{sa} \delta^{td} (Y_d Y_d^\dagger)^{pr} (Y_u Y_u^\dagger)^{bc}
\end{aligned}$$

$$\begin{aligned}
& + \frac{3}{2} \delta^{pa} \delta^{rd} (Y_d Y_d^\dagger)^{st} (Y_u Y_u^\dagger)^{bc} + \frac{3}{2} \delta^{sa} \delta^{td} (Y_u Y_u^\dagger)^{pr} (Y_u Y_u^\dagger)^{bc} + \frac{3}{2} \delta^{pa} \delta^{rd} (Y_u Y_u^\dagger)^{st} (Y_u Y_u^\dagger)^{bc} + \frac{7}{4} \delta^{rd} \delta^{tb} (Y_d Y_d^\dagger)^{sa} (Y_u Y_u^\dagger)^{pc} + \frac{7}{4} \delta^{rb} \delta^{td} (Y_d Y_d^\dagger)^{pa} (Y_u Y_u^\dagger)^{sc} \\
& + \frac{7}{4} \delta^{pa} \delta^{sc} (Y_d Y_d^\dagger)^{dt} (Y_u Y_u^\dagger)^{br} + \frac{7}{4} \delta^{pa} \delta^{sc} (Y_d Y_d^\dagger)^{br} (Y_u Y_u^\dagger)^{dt} + 2 \delta^{rb} \delta^{td} (Y_d Y_d^\dagger)^{pa} (Y_d Y_d^\dagger)^{sc} + 2 \delta^{pa} \delta^{sc} (Y_d Y_d^\dagger)^{br} (Y_d Y_d^\dagger)^{dt} + 2 \delta^{rb} \delta^{td} (Y_u Y_u^\dagger)^{pa} (Y_u Y_u^\dagger)^{sc} \\
& + 2 \delta^{pa} \delta^{sc} (Y_u Y_u^\dagger)^{br} (Y_u Y_u^\dagger)^{dt} - \frac{3}{4} \delta^{pa} \delta^{td} (Y_d Y_d^\dagger)^{sc} (Y_d Y_d^\dagger)^{br} - \frac{3}{4} \delta^{rd} \delta^{sa} (Y_d Y_d^\dagger)^{pc} (Y_d Y_d^\dagger)^{bt} - \frac{3}{4} \delta^{pa} \delta^{td} (Y_u Y_u^\dagger)^{sc} (Y_u Y_u^\dagger)^{br} - \frac{3}{4} \delta^{rd} \delta^{sa} (Y_u Y_u^\dagger)^{pc} (Y_u Y_u^\dagger)^{bt} \\
& - g_s^2 g_L^2 \left( \frac{158}{81} \delta^{pa} \delta^{rd} \delta^{st} \delta^{bc} + \frac{158}{81} \delta^{pr} \delta^{sa} \delta^{td} \delta^{bc} + \frac{77}{9} \delta^{pt} \delta^{rd} \delta^{sa} \delta^{bc} + \frac{77}{9} \delta^{pa} \delta^{rs} \delta^{td} \delta^{bc} + \frac{33}{2} \delta^{pa} \delta^{rd} \delta^{sc} \delta^{tb} + 41 \delta^{pa} \delta^{rb} \delta^{sc} \delta^{td} \right) \\
& - g_L^2 \left( \frac{4}{3} \delta^{pa} \delta^{rd} \delta^{st} (Y_d Y_d^\dagger)^{bc} + \frac{4}{3} \delta^{pr} \delta^{sa} \delta^{td} (Y_d Y_d^\dagger)^{bc} + \frac{4}{3} \delta^{pa} \delta^{rd} \delta^{st} (Y_u Y_u^\dagger)^{bc} + \frac{4}{3} \delta^{pr} \delta^{sa} \delta^{td} (Y_u Y_u^\dagger)^{bc} \right) - g_s^2 \left( \frac{5}{3} \delta^{pt} \delta^{rd} \delta^{sa} (Y_d Y_d^\dagger)^{bc} + \frac{5}{3} \delta^{pa} \delta^{rs} \delta^{td} (Y_d Y_d^\dagger)^{bc} \right. \\
& + \frac{5}{3} \delta^{pt} \delta^{rd} \delta^{sa} (Y_u Y_u^\dagger)^{bc} + \frac{5}{3} \delta^{pa} \delta^{rs} \delta^{td} (Y_u Y_u^\dagger)^{bc} + 3 \delta^{rb} \delta^{sa} \delta^{td} (Y_d Y_d^\dagger)^{pc} + 3 \delta^{pa} \delta^{rd} \delta^{tb} (Y_d Y_d^\dagger)^{sc} + 3 \delta^{pa} \delta^{rd} \delta^{sc} (Y_d Y_d^\dagger)^{bt} + 3 \delta^{pa} \delta^{sc} \delta^{tb} (Y_d Y_d^\dagger)^{dr} \\
& \left. + 3 \delta^{rb} \delta^{sa} \delta^{td} (Y_u Y_u^\dagger)^{pc} + 3 \delta^{pa} \delta^{rd} \delta^{tb} (Y_u Y_u^\dagger)^{sc} + 3 \delta^{pa} \delta^{rd} \delta^{sc} (Y_u Y_u^\dagger)^{bt} + 3 \delta^{pa} \delta^{sc} \delta^{tb} (Y_u Y_u^\dagger)^{dr} \right) \Bigg\} C_{qq}^{(\parallel)abcd} + \left\{ \frac{17}{72} \delta^{pa} \delta^{rb} \delta^{sc} \delta^{td} g_Y^4 \right. \\
& + g_s^4 \left( \frac{2492}{81} \delta^{pt} \delta^{rd} \delta^{sa} \delta^{bc} + \frac{2492}{81} \delta^{pa} \delta^{rs} \delta^{td} \delta^{bc} - \frac{7}{3} \delta^{pt} \delta^{rb} \delta^{sa} \delta^{cd} - \frac{7}{3} \delta^{pa} \delta^{rs} \delta^{tb} \delta^{cd} - \frac{71}{6} \delta^{pa} \delta^{rb} \delta^{sc} \delta^{td} \right) + g_Y^2 g_s^2 \left( \frac{230}{243} \delta^{pt} \delta^{rd} \delta^{sa} \delta^{bc} \right. \\
& + \frac{230}{243} \delta^{pa} \delta^{rs} \delta^{td} \delta^{bc} - \frac{25}{162} \delta^{pt} \delta^{rb} \delta^{sa} \delta^{cd} - \frac{25}{162} \delta^{pa} \delta^{rs} \delta^{tb} \delta^{cd} - \frac{35}{18} \delta^{pa} \delta^{rb} \delta^{sc} \delta^{td} \Bigg) + g_Y^2 g_L^2 \left( \frac{41}{243} \delta^{pa} \delta^{rd} \delta^{st} \delta^{bc} + \frac{41}{243} \delta^{pr} \delta^{sa} \delta^{td} \delta^{bc} \right. \\
& + \frac{82}{81} \delta^{pa} \delta^{rb} \delta^{st} \delta^{cd} + \frac{82}{81} \delta^{pr} \delta^{sa} \delta^{tb} \delta^{cd} - \frac{5}{12} \delta^{pa} \delta^{rb} \delta^{sc} \delta^{td} \Bigg) + g_s^2 g_L^2 \left( \frac{2}{3} \delta^{pt} \delta^{rd} \delta^{sa} \delta^{bc} + \frac{2}{3} \delta^{pa} \delta^{rs} \delta^{td} \delta^{bc} + \frac{17}{3} \delta^{pa} \delta^{rb} \delta^{st} \delta^{cd} + \frac{17}{3} \delta^{pr} \delta^{sa} \delta^{tb} \delta^{cd} \right. \\
& - \frac{262}{81} \delta^{pa} \delta^{rd} \delta^{st} \delta^{bc} - \frac{262}{81} \delta^{pr} \delta^{sa} \delta^{td} \delta^{bc} - \frac{37}{6} \delta^{pt} \delta^{rb} \delta^{sa} \delta^{cd} - \frac{37}{6} \delta^{pa} \delta^{rs} \delta^{tb} \delta^{cd} - \frac{49}{2} \delta^{pa} \delta^{rb} \delta^{sc} \delta^{td} - 30 \delta^{pa} \delta^{rd} \delta^{sc} \delta^{tb} \Bigg) + g_L^4 \left( \frac{46}{3} \delta^{pa} \delta^{rb} \delta^{st} \delta^{cd} \right. \\
& + \frac{46}{3} \delta^{pr} \delta^{sa} \delta^{tb} \delta^{cd} - \frac{7}{3} \delta^{pa} \delta^{rd} \delta^{st} \delta^{bc} - \frac{7}{3} \delta^{pr} \delta^{sa} \delta^{td} \delta^{bc} - \frac{385}{24} \delta^{pa} \delta^{rb} \delta^{sc} \delta^{td} \Bigg) + \delta^{rd} \delta^{sa} (Y_d Y_d^\dagger)^{bt} (Y_u Y_u^\dagger)^{pc} + \delta^{pa} \delta^{td} (Y_d Y_d^\dagger)^{br} (Y_u Y_u^\dagger)^{sc} \\
& + \delta^{pa} \delta^{td} (Y_d Y_d^\dagger)^{sc} (Y_u Y_u^\dagger)^{br} + \delta^{rd} \delta^{sa} (Y_d Y_d^\dagger)^{pc} (Y_u Y_u^\dagger)^{bt} + g_Y^2 \left( \frac{43}{144} \delta^{rd} \delta^{sa} \delta^{tb} (Y_u Y_u^\dagger)^{pc} + \frac{43}{144} \delta^{pa} \delta^{rb} \delta^{td} (Y_u Y_u^\dagger)^{sc} + \frac{43}{144} \delta^{pa} \delta^{sc} \delta^{td} (Y_u Y_u^\dagger)^{br} \right. \\
& + \frac{43}{144} \delta^{pa} \delta^{rb} \delta^{sc} (Y_u Y_u^\dagger)^{dt} + \frac{199}{144} \delta^{rd} \delta^{sa} \delta^{tb} (Y_d Y_d^\dagger)^{pc} + \frac{199}{144} \delta^{pa} \delta^{rb} \delta^{td} (Y_d Y_d^\dagger)^{sc} + \frac{199}{144} \delta^{pa} \delta^{sc} \delta^{td} (Y_d Y_d^\dagger)^{br} + \frac{199}{144} \delta^{pa} \delta^{rb} \delta^{sc} (Y_d Y_d^\dagger)^{dt} \Bigg) \\
& + g_L^2 \left( \frac{33}{16} \delta^{rd} \delta^{sa} \delta^{tb} (Y_d Y_d^\dagger)^{pc} + \frac{33}{16} \delta^{pa} \delta^{rb} \delta^{td} (Y_d Y_d^\dagger)^{sc} + \frac{33}{16} \delta^{pa} \delta^{sc} \delta^{td} (Y_d Y_d^\dagger)^{br} + \frac{33}{16} \delta^{pa} \delta^{rb} \delta^{sc} (Y_d Y_d^\dagger)^{dt} + \frac{33}{16} \delta^{rd} \delta^{sa} \delta^{tb} (Y_u Y_u^\dagger)^{pc} \right. \\
& + \frac{33}{16} \delta^{pa} \delta^{rb} \delta^{td} (Y_u Y_u^\dagger)^{sc} + \frac{33}{16} \delta^{pa} \delta^{sc} \delta^{td} (Y_u Y_u^\dagger)^{br} + \frac{33}{16} \delta^{pa} \delta^{rb} \delta^{sc} (Y_u Y_u^\dagger)^{dt} - 2 \delta^{pa} \delta^{rb} \delta^{st} (Y_d Y_d^\dagger)^{dc} - 2 \delta^{pr} \delta^{sa} \delta^{tb} (Y_d Y_d^\dagger)^{dc} - 2 \delta^{pa} \delta^{rb} \delta^{st} (Y_u Y_u^\dagger)^{dc} \\
& - 2 \delta^{pr} \delta^{sa} \delta^{tb} (Y_u Y_u^\dagger)^{dc} \Bigg) + \frac{3}{2} \delta^{sa} \delta^{tb} (Y_d Y_d^\dagger)^{pr} (Y_d Y_d^\dagger)^{dc} + \frac{3}{2} \delta^{pa} \delta^{rb} (Y_d Y_d^\dagger)^{st} (Y_d Y_d^\dagger)^{dc} + \frac{3}{2} \delta^{sa} \delta^{tb} (Y_d Y_d^\dagger)^{dc} (Y_u Y_u^\dagger)^{pr} + \frac{3}{2} \delta^{pa} \delta^{rb} (Y_d Y_d^\dagger)^{dc} (Y_u Y_u^\dagger)^{st} \\
& + \frac{3}{2} \delta^{sa} \delta^{tb} (Y_d Y_d^\dagger)^{pr} (Y_u Y_u^\dagger)^{dc} + \frac{3}{2} \delta^{pa} \delta^{rb} (Y_d Y_d^\dagger)^{st} (Y_u Y_u^\dagger)^{dc} + \frac{3}{2} \delta^{sa} \delta^{tb} (Y_u Y_u^\dagger)^{pr} (Y_u Y_u^\dagger)^{dc} + \frac{3}{2} \delta^{pa} \delta^{rb} (Y_u Y_u^\dagger)^{st} (Y_u Y_u^\dagger)^{dc} - \frac{1}{4} \delta^{rd} \delta^{sa} \delta^{tb} (Y_d Y_d^\dagger Y_d Y_d^\dagger)^{pc} \\
& - \frac{1}{4} \delta^{pa} \delta^{rb} \delta^{td} (Y_d Y_d^\dagger Y_d Y_d^\dagger)^{sc} - \frac{1}{4} \delta^{pa} \delta^{sc} \delta^{td} (Y_d Y_d^\dagger Y_d Y_d^\dagger)^{br} - \frac{1}{4} \delta^{pa} \delta^{rb} \delta^{sc} (Y_d Y_d^\dagger Y_d Y_d^\dagger)^{dt} - \frac{1}{4} \delta^{rd} \delta^{sa} \delta^{tb} (Y_u Y_u^\dagger Y_u Y_u^\dagger)^{pc} - \frac{1}{4} \delta^{pa} \delta^{rb} \delta^{td} (Y_u Y_u^\dagger Y_u Y_u^\dagger)^{sc}
\end{aligned}$$

$$\begin{aligned}
& -\frac{1}{4}\delta^{pa}\delta^{sc}\delta^{td}(Y_uY_u^\dagger Y_uY_u^\dagger)^{br} - \frac{1}{4}\delta^{pa}\delta^{rb}\delta^{sc}(Y_uY_u^\dagger Y_uY_u^\dagger)^{dt} - \frac{3}{4}T_2\delta^{rd}\delta^{sa}\delta^{tb}(Y_dY_d^\dagger)^{pc} - \frac{3}{4}T_2\delta^{pa}\delta^{rb}\delta^{td}(Y_dY_d^\dagger)^{sc} - \frac{3}{4}T_2\delta^{pa}\delta^{sc}\delta^{td}(Y_dY_d^\dagger)^{br} \\
& - \frac{3}{4}T_2\delta^{pa}\delta^{rb}\delta^{sc}(Y_dY_d^\dagger)^{dt} - \frac{3}{4}T_2\delta^{rd}\delta^{sa}\delta^{tb}(Y_uY_u^\dagger)^{pc} - \frac{3}{4}T_2\delta^{pa}\delta^{rb}\delta^{td}(Y_uY_u^\dagger)^{sc} - \frac{3}{4}T_2\delta^{pa}\delta^{sc}\delta^{td}(Y_uY_u^\dagger)^{br} - \frac{3}{4}T_2\delta^{pa}\delta^{rb}\delta^{sc}(Y_uY_u^\dagger)^{dt} \\
& - \delta^{sa}\delta^{tb}(Y_dY_d^\dagger)^{dr}(Y_uY_u^\dagger)^{pc} - \delta^{pa}\delta^{rb}(Y_dY_d^\dagger)^{dt}(Y_uY_u^\dagger)^{sc} - \delta^{sa}\delta^{tb}(Y_dY_d^\dagger)^{pc}(Y_uY_u^\dagger)^{dr} - \delta^{pa}\delta^{rb}(Y_dY_d^\dagger)^{sc}(Y_uY_u^\dagger)^{dt} - g_s^2\left(\frac{5}{3}\delta^{rd}\delta^{sa}\delta^{tb}(Y_dY_d^\dagger)^{pc}\right. \\
& + \frac{5}{3}\delta^{pa}\delta^{rb}\delta^{td}(Y_dY_d^\dagger)^{sc} + \frac{5}{3}\delta^{pa}\delta^{sc}\delta^{td}(Y_dY_d^\dagger)^{br} + \frac{5}{3}\delta^{pa}\delta^{rb}\delta^{sc}(Y_dY_d^\dagger)^{dt} + \frac{5}{3}\delta^{rd}\delta^{sa}\delta^{tb}(Y_uY_u^\dagger)^{pc} + \frac{5}{3}\delta^{pa}\delta^{rb}\delta^{td}(Y_uY_u^\dagger)^{sc} + \frac{5}{3}\delta^{pa}\delta^{sc}\delta^{td}(Y_uY_u^\dagger)^{br} \\
& + \frac{5}{3}\delta^{pa}\delta^{rb}\delta^{sc}(Y_uY_u^\dagger)^{dt} + \frac{10}{3}\delta^{pt}\delta^{rd}\delta^{sa}(Y_dY_d^\dagger)^{bc} + \frac{10}{3}\delta^{pa}\delta^{rs}\delta^{td}(Y_dY_d^\dagger)^{bc} + \frac{10}{3}\delta^{pt}\delta^{rd}\delta^{sa}(Y_uY_u^\dagger)^{bc} + \frac{10}{3}\delta^{pa}\delta^{rs}\delta^{td}(Y_uY_u^\dagger)^{bc}) \\
& - \frac{3}{2}\delta^{pa}\delta^{td}(Y_dY_d^\dagger)^{sc}(Y_dY_d^\dagger)^{br} - \frac{3}{2}\delta^{rd}\delta^{sa}(Y_dY_d^\dagger)^{pc}(Y_dY_d^\dagger)^{bt} - \frac{3}{2}\delta^{pa}\delta^{td}(Y_uY_u^\dagger)^{sc}(Y_uY_u^\dagger)^{br} - \frac{3}{2}\delta^{rd}\delta^{sa}(Y_uY_u^\dagger)^{pc}(Y_uY_u^\dagger)^{bt} - \frac{7}{4}\delta^{rd}\delta^{tb}(Y_dY_d^\dagger)^{sa}(Y_uY_u^\dagger)^{pc} \\
& - \frac{7}{4}\delta^{rb}\delta^{td}(Y_dY_d^\dagger)^{pa}(Y_uY_u^\dagger)^{sc} - \frac{7}{4}\delta^{pa}\delta^{sc}(Y_dY_d^\dagger)^{dt}(Y_uY_u^\dagger)^{br} - \frac{7}{4}\delta^{pa}\delta^{sc}(Y_dY_d^\dagger)^{br}(Y_uY_u^\dagger)^{dt} \Big\} C_{qq}^{(\times)abcd} + \left\{ g_Y^2 g_s^2 \left( \frac{25}{162} \delta^{pt} \delta^{rd} \delta^{sc} \delta^{ab} + \frac{25}{162} \delta^{pc} \delta^{rs} \delta^{td} \delta^{ab} \right) \right. \\
& + g_Y^2 g_L^2 \left( \frac{25}{162} \delta^{pc} \delta^{rd} \delta^{st} \delta^{ab} + \frac{25}{162} \delta^{pr} \delta^{sc} \delta^{td} \delta^{ab} \right) - g_L^4 \left( \frac{1}{6} \delta^{pc} \delta^{rd} \delta^{st} \delta^{ab} + \frac{1}{6} \delta^{pr} \delta^{sc} \delta^{td} \delta^{ab} \right) \Big\} C_{\ell q}^{(\parallel)abcd} + \left\{ \frac{1}{4} \delta^{sc} \delta^{td} (Y_d Y_d^\dagger)^{pr} (Y_e Y_e^\dagger)^{ba} \right. \\
& + \frac{1}{4} \delta^{pc} \delta^{rd} (Y_d Y_d^\dagger)^{st} (Y_e Y_e^\dagger)^{ba} + \frac{1}{4} \delta^{sc} \delta^{td} (Y_e Y_e^\dagger)^{ba} (Y_u Y_u^\dagger)^{pr} + \frac{1}{4} \delta^{pc} \delta^{rd} (Y_e Y_e^\dagger)^{ba} (Y_u Y_u^\dagger)^{st} + g_Y^2 g_s^2 \left( \frac{25}{324} \delta^{pt} \delta^{rd} \delta^{sc} \delta^{ab} + \frac{25}{324} \delta^{pc} \delta^{rs} \delta^{td} \delta^{ab} \right) \\
& + g_L^4 \left( \frac{23}{9} \delta^{pc} \delta^{rd} \delta^{st} \delta^{ab} + \frac{23}{9} \delta^{pr} \delta^{sc} \delta^{td} \delta^{ab} \right) - g_s^2 g_L^2 \left( \frac{1}{18} \delta^{pc} \delta^{rd} \delta^{st} \delta^{ab} + \frac{1}{18} \delta^{pr} \delta^{sc} \delta^{td} \delta^{ab} + \frac{37}{36} \delta^{pt} \delta^{rd} \delta^{sc} \delta^{ab} + \frac{37}{36} \delta^{pc} \delta^{rs} \delta^{td} \delta^{ab} \right) \\
& \left. - g_Y^2 g_L^2 \left( \frac{11}{81} \delta^{pc} \delta^{rd} \delta^{st} \delta^{ab} + \frac{11}{81} \delta^{pr} \delta^{sc} \delta^{td} \delta^{ab} \right) - g_L^2 \left( \frac{1}{3} \delta^{pc} \delta^{rd} \delta^{st} (Y_e Y_e^\dagger)^{ba} + \frac{1}{3} \delta^{pr} \delta^{sc} \delta^{td} (Y_e Y_e^\dagger)^{ba} \right) \right\} C_{\ell q}^{(\times)abcd}, \tag{13.6}
\end{aligned}$$

### 13.4 $C_{\ell q}^{(\parallel)}$

$$\begin{aligned}
\beta_{C_{\ell q}^{(\parallel)prst}}^{(1)} &= \left\{ \frac{1}{9} \delta^{pa} \delta^{rb} \delta^{st} g_Y^2 + \delta^{pa} \delta^{rb} (Y_u Y_u^\dagger)^{st} - \delta^{pa} \delta^{rb} (Y_d Y_d^\dagger)^{st} \right\} C_{H\ell}^{(\parallel)ab} + \left\{ \frac{1}{18} \delta^{pa} \delta^{rb} \delta^{st} g_Y^2 + \delta^{pa} \delta^{rb} (Y_u Y_u^\dagger)^{st} - \frac{1}{6} \delta^{pa} \delta^{rb} \delta^{st} g_L^2 \right\} C_{H\ell}^{(\times)ab} \\
& - \left\{ \frac{1}{3} \delta^{pr} \delta^{sa} \delta^{tb} g_Y^2 + \delta^{sa} \delta^{tb} (Y_e Y_e^\dagger)^{pr} \right\} C_{Hq}^{(\parallel)ab} - \left\{ \frac{1}{6} \delta^{pr} \delta^{sa} \delta^{tb} g_L^2 + \frac{1}{6} \delta^{pr} \delta^{sa} \delta^{tb} g_Y^2 \right\} C_{Hq}^{(\times)ab} - \frac{2}{9} \delta^{pa} \delta^{rb} \delta^{st} \delta^{cd} g_Y^2 C_{\ell e}^{abcd} + \left\{ \frac{4}{9} \delta^{pa} \delta^{rb} \delta^{st} \delta^{cd} g_Y^2 \right. \\
& - \delta^{pa} \delta^{rb} Y_u^{*td} Y_u^{sc} \Big\} C_{\ell u}^{abcd} - \left\{ \frac{2}{9} \delta^{pa} \delta^{rb} \delta^{st} \delta^{cd} g_Y^2 + \delta^{pa} \delta^{rb} Y_d^{*td} Y_d^{sc} \right\} C_{\ell d}^{abcd} + \left\{ \frac{2}{3} \delta^{pr} \delta^{sa} \delta^{tb} \delta^{cd} g_Y^2 - \delta^{sa} \delta^{tb} Y_e^{*rd} Y_e^{pc} \right\} C_{qe}^{abcd} - \frac{4}{3} \delta^{pr} \delta^{sa} \delta^{tb} \delta^{cd} g_Y^2 C_{qu}^{(\parallel)abcd} \\
& - \frac{4}{9} \delta^{pr} \delta^{sa} \delta^{tb} \delta^{cd} g_Y^2 C_{qu}^{(\times)abcd} + \frac{2}{3} \delta^{pr} \delta^{sa} \delta^{tb} \delta^{cd} g_Y^2 C_{qd}^{(\parallel)abcd} + \frac{2}{9} \delta^{pr} \delta^{sa} \delta^{tb} \delta^{cd} g_Y^2 C_{qd}^{(\times)abcd} + \frac{1}{2} \delta^{pa} \delta^{sc} Y_e^{*rb} Y_u^{*td} C_{\ell e q u}^{abcd} + \frac{1}{2} \delta^{ra} \delta^{tc} C_{\ell e q u}^{*abcd} Y_e^{pb} Y_u^{sd} \\
& + \frac{1}{2} \delta^{pa} \delta^{sc} Y_e^{*rd} Y_u^{*tb} C_{\ell u q e}^{abcd} + \frac{1}{2} \delta^{ra} \delta^{tc} C_{\ell u q e}^{*abcd} Y_e^{pd} Y_u^{sb} - \left\{ \frac{2}{9} g_Y^2 \left( \delta^{pa} \delta^{rd} \delta^{st} \delta^{bc} + 2 \delta^{pa} \delta^{rb} \delta^{st} \delta^{cd} \right) + \frac{2}{3} \delta^{pa} \delta^{rd} \delta^{st} \delta^{bc} g_L^2 \right\} C_{\ell \ell}^{abcd} - \left\{ \frac{2}{9} g_Y^2 \left( \delta^{pr} \delta^{sa} \delta^{td} \delta^{bc} \right. \right.
\end{aligned}$$

$$\begin{aligned}
& + 6\delta^{pr}\delta^{sa}\delta^{tb}\delta^{cd}) + \frac{2}{3}\delta^{pr}\delta^{sa}\delta^{td}\delta^{bc}g_L^2 \Big\} C_{qq}^{(\parallel)abcd} - \left\{ \frac{2}{9}g_Y^2 \left( 2\delta^{pr}\delta^{sa}\delta^{td}\delta^{bc} + 3\delta^{pr}\delta^{sa}\delta^{tb}\delta^{cd} \right) + 2\delta^{pr}\delta^{sa}\delta^{tb}\delta^{cd}g_L^2 \right\} C_{qq}^{(\times)abcd} + \left\{ \frac{1}{9}g_Y^2 \left( 2\delta^{pa}\delta^{rb}\delta^{st}\delta^{cd} \right. \right. \\
& + 6\delta^{pr}\delta^{sc}\delta^{td}\delta^{ab} - 9\delta^{pa}\delta^{rb}\delta^{sc}\delta^{td} \Big) + \frac{1}{2} \left( \delta^{pa}\delta^{rb}\delta^{td}(Y_d Y_d^\dagger)^{sc} + \delta^{pa}\delta^{rb}\delta^{sc}(Y_d Y_d^\dagger)^{dt} + \delta^{rb}\delta^{sc}\delta^{td}(Y_e Y_e^\dagger)^{pa} + \delta^{pa}\delta^{sc}\delta^{td}(Y_e Y_e^\dagger)^{br} + \delta^{pa}\delta^{rb}\delta^{td}(Y_u Y_u^\dagger)^{sc} \right. \\
& + \delta^{pa}\delta^{rb}\delta^{sc}(Y_u Y_u^\dagger)^{dt} \Big) - 3\delta^{pa}\delta^{rb}\delta^{sc}\delta^{td}g_L^2 \Big\} C_{\ell q}^{(\parallel)abcd} + \left\{ \frac{1}{9}g_Y^2 \left( \delta^{pa}\delta^{rb}\delta^{st}\delta^{cd} + 3\delta^{pr}\delta^{sc}\delta^{td}\delta^{ab} \right) + \frac{1}{3}g_L^2 \left( 18\delta^{pa}\delta^{rb}\delta^{sc}\delta^{td} - \delta^{pr}\delta^{sc}\delta^{td}\delta^{ab} \right. \right. \\
& \left. \left. - 3\delta^{pa}\delta^{rb}\delta^{st}\delta^{cd} \right) \right\} C_{\ell q}^{(\times)abcd}, \tag{13.7}
\end{aligned}$$

$$\begin{aligned}
\beta_{C_{\ell q}^{(\parallel)prst}}^{(2)} = & \frac{1}{2} \left( (C_{\ell HH} C_{\ell HH}^\dagger)^{rp} (Y_u Y_u^\dagger)^{st} - 5(C_{\ell HH} C_{\ell HH}^\dagger)^{rp} (Y_d Y_d^\dagger)^{st} \right) - \frac{11}{18} \delta^{st} g_Y^2 (C_{\ell HH} C_{\ell HH}^\dagger)^{rp} - \delta^{st} g_L^2 (C_{\ell HH} C_{\ell HH}^\dagger)^{rp} + \left\{ g_Y^4 \left( \frac{1}{6} \delta^{st} (Y_e Y_e^\dagger)^{pr} \right. \right. \\
& + \frac{5}{6} \delta^{pr} (Y_d Y_d^\dagger)^{st} - \frac{1}{6} \delta^{pr} (Y_u Y_u^\dagger)^{st} \Big) - \frac{2}{9} \delta^{pr} \delta^{st} g_Y^6 \Big\} C_{HB} + \left\{ g_L^4 \left( \frac{3}{2} \delta^{pr} (Y_d Y_d^\dagger)^{st} + \frac{3}{2} \delta^{st} (Y_e Y_e^\dagger)^{pr} + \frac{3}{2} \delta^{pr} (Y_u Y_u^\dagger)^{st} \right) - \frac{2}{3} \delta^{pr} \delta^{st} g_L^6 \right\} C_{HW} \\
& + \left\{ g_Y^2 g_L^2 \left( \frac{4}{3} \delta^{pr} (Y_d Y_d^\dagger)^{st} - \frac{1}{2} \delta^{st} (Y_e Y_e^\dagger)^{pr} - \frac{13}{12} \delta^{pr} (Y_u Y_u^\dagger)^{st} \right) - \frac{1}{6} \delta^{pr} \delta^{st} g_Y^2 g_L^4 - \frac{1}{6} \delta^{pr} \delta^{st} g_Y^4 g_L^2 \right\} C_{HWB} + \left\{ \frac{1}{6} \delta^{pr} \delta^{st} g_Y^2 g_L^6 - g_L^6 \left( \frac{3}{2} \delta^{pr} (Y_d Y_d^\dagger)^{st} \right. \right. \\
& + \frac{3}{2} \delta^{st} (Y_e Y_e^\dagger)^{pr} + \frac{3}{2} \delta^{pr} (Y_u Y_u^\dagger)^{st} \Big) - \frac{95}{6} \delta^{pr} \delta^{st} g_L^8 \Big\} C_W - \left\{ \frac{40}{9} \delta^{pr} \delta^{st} g_Y^2 g_s^6 + \frac{40}{3} \delta^{pr} \delta^{st} g_s^6 g_L^2 \right\} C_G + \left\{ g_Y^4 \left( \frac{1}{3} \delta^{pr} \delta^{st} Y_e^{*ab} - \frac{11}{12} \delta^{pa} \delta^{st} Y_e^{*rb} \right) \right. \\
& + g_Y^2 \left( \frac{1}{2} \delta^{pa} Y_e^{*rb} (Y_u Y_u^\dagger)^{st} - \frac{1}{3} \delta^{st} Y_e^{*rb} (Y_e Y_e^\dagger)^{pa} \right) - \frac{1}{4} \delta^{pa} \delta^{st} g_Y^2 g_L^2 Y_e^{*rb} \Big\} C_{eB}^{ab} + C_{eB}^{*ab} \left\{ g_Y^4 \left( \frac{1}{3} \delta^{pr} \delta^{st} Y_e^{ab} - \frac{11}{12} \delta^{ra} \delta^{st} Y_e^{pb} \right) + g_Y^2 \left( \frac{1}{2} \delta^{ra} Y_e^{pb} (Y_u Y_u^\dagger)^{st} \right. \right. \\
& - \frac{1}{3} \delta^{st} Y_e^{pb} (Y_e Y_e^\dagger)^{ar} \Big) - \frac{1}{4} \delta^{ra} \delta^{st} g_Y^2 g_L^2 Y_e^{pb} \Big\} + \left\{ \frac{5}{24} \delta^{pa} \delta^{st} g_Y^2 g_L^2 Y_e^{*rb} + g_L^2 \left( \frac{9}{4} \delta^{pa} Y_e^{*rb} (Y_u Y_u^\dagger)^{st} + 3\delta^{pa} Y_e^{*rb} (Y_d Y_d^\dagger)^{st} \right) - g_L^4 \left( \frac{1}{8} \delta^{pa} \delta^{st} Y_e^{*rb} \right. \right. \\
& + \frac{1}{6} \delta^{pr} \delta^{st} Y_e^{*ab} \Big) \Big\} C_{eW}^{ab} + C_{eW}^{*ab} \left\{ \frac{5}{24} \delta^{ra} \delta^{st} g_Y^2 g_L^2 Y_e^{pb} + g_L^2 \left( \frac{9}{4} \delta^{ra} Y_e^{pb} (Y_u Y_u^\dagger)^{st} + 3\delta^{ra} Y_e^{pb} (Y_d Y_d^\dagger)^{st} \right) - g_L^4 \left( \frac{1}{8} \delta^{ra} \delta^{st} Y_e^{pb} + \frac{1}{6} \delta^{pr} \delta^{st} Y_e^{ab} \right) \right\} \\
& + \left\{ \frac{7}{36} \delta^{pr} \delta^{sa} g_Y^2 g_L^2 Y_u^{*tb} + g_Y^2 \left( \delta^{pr} Y_u^{*tb} (Y_u Y_u^\dagger)^{sa} + \frac{5}{2} \delta^{sa} Y_u^{*tb} (Y_e Y_e^\dagger)^{pr} - \frac{1}{2} \delta^{pr} Y_u^{*tb} (Y_d Y_d^\dagger)^{sa} \right) + \frac{8}{3} \delta^{pr} \delta^{sa} g_Y^2 g_s^2 Y_u^{*tb} - g_Y^4 \left( \frac{5}{9} \delta^{pr} \delta^{st} Y_u^{*ab} \right. \right. \\
& + \frac{77}{108} \delta^{pr} \delta^{sa} Y_u^{*tb} \Big) \Big\} C_{uB}^{ab} + C_{uB}^{*ab} \left\{ \frac{7}{36} \delta^{pr} \delta^{ta} g_Y^2 g_L^2 Y_u^{sb} + g_Y^2 \left( \delta^{pr} Y_u^{sb} (Y_u Y_u^\dagger)^{at} + \frac{5}{2} \delta^{ta} Y_u^{sb} (Y_e Y_e^\dagger)^{pr} - \frac{1}{2} \delta^{pr} Y_u^{sb} (Y_d Y_d^\dagger)^{at} \right) + \frac{8}{3} \delta^{pr} \delta^{ta} g_Y^2 g_s^2 Y_u^{sb} \right. \\
& \left. \left. - g_Y^4 \left( \frac{5}{9} \delta^{pr} \delta^{st} Y_u^{ab} + \frac{77}{108} \delta^{pr} \delta^{ta} Y_u^{sb} \right) \right\} + \left\{ g_L^2 \left( \frac{1}{4} \delta^{pr} Y_u^{*tb} (Y_d Y_d^\dagger)^{sa} + \frac{9}{4} \delta^{sa} Y_u^{*tb} (Y_e Y_e^\dagger)^{pr} \right) + \frac{4}{3} \delta^{pr} \delta^{sa} g_s^2 g_L^2 Y_u^{*tb} - \frac{31}{72} \delta^{pr} \delta^{sa} g_Y^2 g_L^2 Y_u^{*tb} \right.
\end{aligned}$$

$$\begin{aligned}
& -g_L^4 \left( \frac{1}{8} \delta^{pr} \delta^{sa} Y_u^{*tb} + \frac{1}{2} \delta^{pr} \delta^{st} Y_u^{*ab} \right) \Big\} C_{uW}^{ab} + C_{uW}^{*ab} \Big\{ g_L^2 \left( \frac{1}{4} \delta^{pr} Y_u^{sb} (Y_d Y_d^\dagger)^{at} + \frac{9}{4} \delta^{ta} Y_u^{sb} (Y_e Y_e^\dagger)^{pr} \right) + \frac{4}{3} \delta^{pr} \delta^{ta} g_s^2 g_L^2 Y_u^{sb} - \frac{31}{72} \delta^{pr} \delta^{ta} g_Y^2 g_L^2 Y_u^{sb} \\
& - g_L^4 \left( \frac{1}{8} \delta^{pr} \delta^{ta} Y_u^{sb} + \frac{1}{2} \delta^{pr} \delta^{st} Y_u^{ab} \right) \Big\} + \Big\{ \frac{2}{9} \delta^{pr} \delta^{sa} g_s^2 g_L^2 Y_u^{*tb} + \frac{74}{27} \delta^{pr} \delta^{sa} g_Y^2 g_s^2 Y_u^{*tb} - 4 \delta^{sa} g_s^2 Y_u^{*tb} (Y_e Y_e^\dagger)^{pr} \Big\} C_{uG}^{ab} + C_{uG}^{*ab} \Big\{ \frac{2}{9} \delta^{pr} \delta^{ta} g_s^2 g_L^2 Y_u^{sb} \\
& + \frac{74}{27} \delta^{pr} \delta^{ta} g_Y^2 g_s^2 Y_u^{sb} - 4 \delta^{ta} g_s^2 Y_u^{sb} (Y_e Y_e^\dagger)^{pr} \Big\} + \Big\{ g_Y^4 \left( \frac{1}{9} \delta^{pr} \delta^{st} Y_d^{*ab} + \frac{109}{108} \delta^{pr} \delta^{sa} Y_d^{*tb} \right) + g_Y^2 \left( \delta^{pr} Y_d^{*tb} (Y_d Y_d^\dagger)^{sa} - \frac{1}{2} \delta^{pr} Y_d^{*tb} (Y_u Y_u^\dagger)^{sa} \right) \\
& + \frac{8}{3} \delta^{pr} \delta^{sa} g_Y^2 g_s^2 Y_d^{*tb} - \frac{5}{36} \delta^{pr} \delta^{sa} g_Y^2 g_L^2 Y_d^{*tb} \Big\} C_{dB}^{ab} + C_{dB}^{*ab} \Big\{ g_Y^4 \left( \frac{1}{9} \delta^{pr} \delta^{st} Y_d^{ab} + \frac{109}{108} \delta^{pr} \delta^{ta} Y_d^{sb} \right) + g_Y^2 \left( \delta^{pr} Y_d^{sb} (Y_d Y_d^\dagger)^{at} - \frac{1}{2} \delta^{pr} Y_d^{sb} (Y_u Y_u^\dagger)^{at} \right) \\
& + \frac{8}{3} \delta^{pr} \delta^{ta} g_Y^2 g_s^2 Y_d^{sb} - \frac{5}{36} \delta^{pr} \delta^{ta} g_Y^2 g_L^2 Y_d^{sb} \Big\} + \Big\{ \frac{11}{72} \delta^{pr} \delta^{sa} g_Y^2 g_L^2 Y_d^{*tb} + g_L^2 \left( \frac{1}{4} \delta^{pr} Y_d^{*tb} (Y_u Y_u^\dagger)^{sa} + 3 \delta^{sa} Y_d^{*tb} (Y_e Y_e^\dagger)^{pr} \right) + \frac{4}{3} \delta^{pr} \delta^{sa} g_s^2 g_L^2 Y_d^{*tb} \\
& - g_L^4 \left( \frac{1}{8} \delta^{pr} \delta^{sa} Y_d^{*tb} + \frac{1}{2} \delta^{pr} \delta^{st} Y_d^{*ab} \right) \Big\} C_{dW}^{ab} + C_{dW}^{*ab} \Big\{ \frac{11}{72} \delta^{pr} \delta^{ta} g_Y^2 g_L^2 Y_d^{sb} + g_L^2 \left( \frac{1}{4} \delta^{pr} Y_d^{sb} (Y_u Y_u^\dagger)^{at} + 3 \delta^{ta} Y_d^{sb} (Y_e Y_e^\dagger)^{pr} \right) + \frac{4}{3} \delta^{pr} \delta^{ta} g_s^2 g_L^2 Y_d^{sb} \\
& - g_L^4 \left( \frac{1}{8} \delta^{pr} \delta^{ta} Y_d^{sb} + \frac{1}{2} \delta^{pr} \delta^{st} Y_d^{ab} \right) \Big\} + \Big\{ \frac{2}{9} \delta^{pr} \delta^{sa} g_s^2 g_L^2 Y_d^{*tb} - \frac{34}{27} \delta^{pr} \delta^{sa} g_Y^2 g_s^2 Y_d^{*tb} \Big\} C_{dG}^{ab} + C_{dG}^{*ab} \Big\{ \frac{2}{9} \delta^{pr} \delta^{ta} g_s^2 g_L^2 Y_d^{sb} - \frac{34}{27} \delta^{pr} \delta^{ta} g_Y^2 g_s^2 Y_d^{sb} \Big\} \\
& + \Big\{ \frac{77}{324} \delta^{pa} \delta^{rb} \delta^{st} g_Y^4 + \frac{1}{4} \delta^{rb} (Y_e Y_e^\dagger)^{pa} (Y_u Y_u^\dagger)^{st} + \frac{1}{4} \delta^{pa} (Y_e Y_e^\dagger)^{br} (Y_u Y_u^\dagger)^{st} + \frac{77}{108} \delta^{pa} \delta^{rb} \delta^{st} g_Y^2 g_L^2 + T_2 \delta^{pa} \delta^{rb} (Y_d Y_d^\dagger)^{st} + g_s^2 \left( \frac{16}{3} \delta^{pa} \delta^{rb} (Y_d Y_d^\dagger)^{st} \right. \\
& - \frac{16}{3} \delta^{pa} \delta^{rb} (Y_u Y_u^\dagger)^{st} \Big) + g_Y^2 \left( \frac{1}{216} \delta^{rb} \delta^{st} (Y_e Y_e^\dagger)^{pa} + \frac{1}{216} \delta^{pa} \delta^{st} (Y_e Y_e^\dagger)^{br} + \frac{289}{72} \delta^{pa} \delta^{rb} (Y_u Y_u^\dagger)^{st} - \frac{1}{9} T_2 \delta^{pa} \delta^{rb} \delta^{st} - \frac{85}{72} \delta^{pa} \delta^{rb} (Y_d Y_d^\dagger)^{st} \right) \\
& + g_L^2 \left( \frac{35}{8} \delta^{pa} \delta^{rb} (Y_u Y_u^\dagger)^{st} - \frac{29}{72} \delta^{rb} \delta^{st} (Y_e Y_e^\dagger)^{pa} - \frac{29}{72} \delta^{pa} \delta^{st} (Y_e Y_e^\dagger)^{br} - \frac{35}{8} \delta^{pa} \delta^{rb} (Y_d Y_d^\dagger)^{st} \right) + 3 \delta^{pa} \delta^{rb} (Y_d Y_d^\dagger Y_d Y_d^\dagger)^{st} - T_2 \delta^{pa} \delta^{rb} (Y_u Y_u^\dagger)^{st} \\
& - 3 \delta^{pa} \delta^{rb} (Y_u Y_u^\dagger Y_u Y_u^\dagger)^{st} \Big\} C_{H\ell}^{(II)ab} + \Big\{ \frac{77}{648} \delta^{pa} \delta^{rb} \delta^{st} g_Y^4 + g_Y^2 g_L^2 \left( \frac{1}{54} \delta^{pr} \delta^{st} \delta^{ab} - \frac{1}{54} \delta^{pa} \delta^{rb} \delta^{st} \right) + g_L^4 \left( \frac{1}{18} \delta^{pr} \delta^{st} \delta^{ab} - \frac{71}{72} \delta^{pa} \delta^{rb} \delta^{st} \right) \\
& + g_Y^2 \left( \frac{13}{108} \delta^{rb} \delta^{st} (Y_e Y_e^\dagger)^{pa} + \frac{13}{108} \delta^{pa} \delta^{st} (Y_e Y_e^\dagger)^{br} + \frac{289}{72} \delta^{pa} \delta^{rb} (Y_u Y_u^\dagger)^{st} - \frac{1}{18} \delta^{st} \delta^{ab} (Y_e Y_e^\dagger)^{pr} - \frac{1}{9} \delta^{pa} \delta^{rb} \delta^{st} \text{Tr} [Y_e^\dagger Y_e] - \frac{1}{6} \delta^{pa} \delta^{rb} \delta^{st} \text{Tr} [Y_d^\dagger Y_d] \right. \\
& - \frac{1}{6} \delta^{pa} \delta^{rb} \delta^{st} \text{Tr} [Y_u^\dagger Y_u] \Big) + g_L^2 \left( \frac{1}{36} \delta^{rb} \delta^{st} (Y_e Y_e^\dagger)^{pa} + \frac{1}{36} \delta^{pa} \delta^{st} (Y_e Y_e^\dagger)^{br} + \frac{1}{4} \delta^{pa} \delta^{rb} (Y_d Y_d^\dagger)^{st} + \frac{1}{2} \delta^{pa} \delta^{rb} \delta^{st} \text{Tr} [Y_d^\dagger Y_d] + \frac{1}{2} \delta^{pa} \delta^{rb} \delta^{st} \text{Tr} [Y_u^\dagger Y_u] \right. \\
& + \frac{37}{8} \delta^{pa} \delta^{rb} (Y_u Y_u^\dagger)^{st} - \frac{1}{6} \delta^{st} \delta^{ab} (Y_e Y_e^\dagger)^{pr} \Big) + \frac{5}{4} \delta^{pa} \delta^{rb} (Y_d Y_d^\dagger Y_d Y_d^\dagger)^{st} - \frac{1}{2} \delta^{rb} (Y_d Y_d^\dagger)^{st} (Y_e Y_e^\dagger)^{pa} - \frac{1}{2} \delta^{pa} (Y_d Y_d^\dagger)^{st} (Y_e Y_e^\dagger)^{br} - \frac{1}{2} \delta^{pa} \delta^{rb} (Y_d Y_d^\dagger Y_u Y_u^\dagger)^{st} \\
& \left. - \frac{1}{2} \delta^{pa} \delta^{rb} (Y_u Y_u^\dagger Y_d Y_d^\dagger)^{st} - T_2 \delta^{pa} \delta^{rb} (Y_u Y_u^\dagger)^{st} - \frac{7}{4} \delta^{pa} \delta^{rb} (Y_u Y_u^\dagger Y_u Y_u^\dagger)^{st} - \frac{16}{3} \delta^{pa} \delta^{rb} g_s^2 (Y_u Y_u^\dagger)^{st} \right\} C_{H\ell}^{(\times)ab} + \Big\{ T_2 \delta^{sa} \delta^{tb} (Y_e Y_e^\dagger)^{pr}
\end{aligned}$$

$$\begin{aligned}
& + g_Y^2 \left( \frac{1}{3} T_2 \delta^{pr} \delta^{sa} \delta^{tb} - \frac{31}{216} \delta^{pr} \delta^{tb} (Y_u Y_u^\dagger)^{sa} - \frac{31}{216} \delta^{pr} \delta^{sa} (Y_u Y_u^\dagger)^{bt} - \frac{59}{216} \delta^{pr} \delta^{tb} (Y_d Y_d^\dagger)^{sa} - \frac{59}{216} \delta^{pr} \delta^{sa} (Y_d Y_d^\dagger)^{bt} - \frac{47}{24} \delta^{sa} \delta^{tb} (Y_e Y_e^\dagger)^{pr} \right) \\
& + g_L^2 \left( \frac{29}{72} \delta^{pr} \delta^{tb} (Y_u Y_u^\dagger)^{sa} + \frac{29}{72} \delta^{pr} \delta^{sa} (Y_u Y_u^\dagger)^{bt} - \frac{29}{72} \delta^{pr} \delta^{tb} (Y_d Y_d^\dagger)^{sa} - \frac{29}{72} \delta^{pr} \delta^{sa} (Y_d Y_d^\dagger)^{bt} - \frac{35}{8} \delta^{sa} \delta^{tb} (Y_e Y_e^\dagger)^{pr} \right) + 3 \delta^{sa} \delta^{tb} (Y_e Y_e^\dagger Y_e Y_e^\dagger)^{pr} \\
& - \frac{1}{4} \delta^{tb} (Y_e Y_e^\dagger)^{pr} (Y_u Y_u^\dagger)^{sa} - \frac{1}{4} \delta^{sa} (Y_e Y_e^\dagger)^{pr} (Y_u Y_u^\dagger)^{bt} - \frac{1061}{972} \delta^{pr} \delta^{sa} \delta^{tb} g_Y^4 - \frac{1061}{324} \delta^{pr} \delta^{sa} \delta^{tb} g_Y^2 g_L^2 \left\} C_{Hq}^{(\parallel)ab} + \left\{ g_Y^2 \left( \frac{31}{216} \delta^{pr} \delta^{tb} (Y_u Y_u^\dagger)^{sa} \right. \right. \\
& + \frac{31}{216} \delta^{pr} \delta^{sa} (Y_u Y_u^\dagger)^{bt} + \frac{1}{6} T_2 \delta^{pr} \delta^{sa} \delta^{tb} - \frac{59}{108} \delta^{pr} \delta^{tb} (Y_d Y_d^\dagger)^{sa} - \frac{59}{108} \delta^{pr} \delta^{sa} (Y_d Y_d^\dagger)^{bt} \right) + g_L^2 \left( \frac{1}{36} \delta^{pr} \delta^{tb} (Y_d Y_d^\dagger)^{sa} + \frac{1}{36} \delta^{pr} \delta^{sa} (Y_d Y_d^\dagger)^{bt} \right. \\
& + \frac{1}{6} T_2 \delta^{pr} \delta^{sa} \delta^{tb} + \frac{1}{4} \delta^{sa} \delta^{tb} (Y_e Y_e^\dagger)^{pr} + \frac{31}{72} \delta^{pr} \delta^{tb} (Y_u Y_u^\dagger)^{sa} + \frac{31}{72} \delta^{pr} \delta^{sa} (Y_u Y_u^\dagger)^{bt} \Big) + \frac{5}{4} \delta^{sa} \delta^{tb} (Y_e Y_e^\dagger Y_e Y_e^\dagger)^{pr} - \frac{1}{4} \delta^{tb} (Y_e Y_e^\dagger)^{pr} (Y_u Y_u^\dagger)^{sa} \\
& - \frac{1}{4} \delta^{sa} (Y_e Y_e^\dagger)^{pr} (Y_u Y_u^\dagger)^{bt} - \frac{1}{2} \delta^{tb} (Y_d Y_d^\dagger)^{sa} (Y_e Y_e^\dagger)^{pr} - \frac{1}{2} \delta^{sa} (Y_d Y_d^\dagger)^{bt} (Y_e Y_e^\dagger)^{pr} - \frac{1061}{1944} \delta^{pr} \delta^{sa} \delta^{tb} g_Y^4 - \frac{83}{72} \delta^{pr} \delta^{sa} \delta^{tb} g_L^4 \\
& - \frac{323}{162} \delta^{pr} \delta^{sa} \delta^{tb} g_Y^2 g_L^2 \left\} C_{Hq}^{(\times)ab} + \left\{ \frac{73}{162} \delta^{pa} \delta^{rb} \delta^{st} \delta^{cd} g_Y^4 + \frac{1}{2} \delta^{pa} \delta^{rb} (Y_e^\dagger Y_e)^{dc} (Y_u Y_u^\dagger)^{st} + \frac{37}{54} \delta^{pa} \delta^{rb} \delta^{st} \delta^{cd} g_Y^2 g_L^2 + g_Y^2 \left( \frac{5}{27} \delta^{pa} \delta^{st} Y_e^{*rd} Y_e^{bc} \right. \right. \\
& + \frac{5}{27} \delta^{rb} \delta^{st} Y_e^{*ad} Y_e^{pc} + \frac{5}{9} \delta^{pa} \delta^{rb} \delta^{st} (Y_e^\dagger Y_e)^{dc} \Big) - \frac{1}{2} \delta^{pa} \delta^{rb} (Y_e^\dagger Y_e)^{dc} (Y_d Y_d^\dagger)^{st} - g_L^2 \left( \frac{1}{9} \delta^{pa} \delta^{st} Y_e^{*rd} Y_e^{bc} + \frac{1}{9} \delta^{rb} \delta^{st} Y_e^{*ad} Y_e^{pc} \right) \left\} C_{\ell e}^{abcd} + \left\{ \frac{107}{81} \delta^{pa} \delta^{rb} \delta^{st} \delta^{cd} g_Y^4 \right. \right. \\
& + \frac{3}{2} T_2 \delta^{pa} \delta^{rb} Y_u^{*td} Y_u^{sc} + \frac{3}{2} \delta^{pa} \delta^{rb} (Y_u^\dagger Y_u)^{dc} (Y_d Y_d^\dagger)^{st} + \frac{3}{2} \delta^{pa} \delta^{rb} Y_u^{sc} (Y_u^\dagger Y_u Y_u^\dagger)^{td} + \frac{3}{2} \delta^{pa} \delta^{rb} Y_u^{*td} (Y_u Y_u^\dagger Y_u)^{sc} + \frac{16}{9} \delta^{pa} \delta^{rb} \delta^{st} \delta^{cd} g_Y^2 g_s^2 \\
& + \frac{16}{3} \delta^{pa} \delta^{rb} g_s^2 Y_u^{*td} Y_u^{sc} - \frac{1}{4} \delta^{rb} Y_u^{*td} Y_u^{sc} (Y_e Y_e^\dagger)^{pa} - \frac{1}{4} \delta^{pa} Y_u^{*td} Y_u^{sc} (Y_e Y_e^\dagger)^{br} - \frac{1}{2} \delta^{pa} \delta^{rb} Y_u^{sc} (Y_d^\dagger Y_d Y_u^\dagger)^{td} - \frac{1}{2} \delta^{pa} \delta^{rb} Y_u^{*td} (Y_d Y_d^\dagger Y_u)^{sc} \\
& - g_Y^2 \left( \delta^{pa} \delta^{rb} \delta^{st} (Y_u^\dagger Y_u)^{dc} + \frac{133}{72} \delta^{pa} \delta^{rb} Y_u^{*td} Y_u^{sc} \right) - \frac{37}{27} \delta^{pa} \delta^{rb} \delta^{st} \delta^{cd} g_Y^2 g_L^2 - \frac{3}{2} \delta^{pa} \delta^{rb} (Y_u^\dagger Y_u)^{dc} (Y_u Y_u^\dagger)^{st} - \frac{23}{8} \delta^{pa} \delta^{rb} g_L^2 Y_u^{*td} Y_u^{sc} \\
& - 8 \delta^{pa} \delta^{rb} \delta^{st} \delta^{cd} g_s^4 \left\} C_{\ell u}^{abcd} + \left\{ \frac{73}{162} \delta^{pa} \delta^{rb} \delta^{st} \delta^{cd} g_Y^4 + \frac{37}{54} \delta^{pa} \delta^{rb} \delta^{st} \delta^{cd} g_Y^2 g_L^2 + g_Y^2 \left( \frac{1}{3} \delta^{pa} \delta^{rb} \delta^{st} (Y_d^\dagger Y_d)^{dc} - \frac{109}{72} \delta^{pa} \delta^{rb} Y_d^{*td} Y_d^{sc} \right) \right. \right. \\
& + \frac{3}{2} T_2 \delta^{pa} \delta^{rb} Y_d^{*td} Y_d^{sc} + \frac{3}{2} \delta^{pa} \delta^{rb} (Y_d^\dagger Y_d)^{dc} (Y_u Y_u^\dagger)^{st} + \frac{3}{2} \delta^{pa} \delta^{rb} Y_d^{sc} (Y_d^\dagger Y_d Y_d^\dagger)^{td} + \frac{3}{2} \delta^{pa} \delta^{rb} Y_d^{*td} (Y_d Y_d^\dagger Y_d)^{sc} + \frac{16}{3} \delta^{pa} \delta^{rb} g_s^2 Y_d^{*td} Y_d^{sc} \\
& - \frac{1}{2} \delta^{pa} \delta^{rb} Y_d^{sc} (Y_u^\dagger Y_u Y_d^\dagger)^{td} - \frac{1}{2} \delta^{pa} \delta^{rb} Y_d^{*td} (Y_u Y_u^\dagger Y_d)^{sc} - \frac{8}{9} \delta^{pa} \delta^{rb} \delta^{st} \delta^{cd} g_Y^2 g_s^2 - \frac{3}{2} \delta^{pa} \delta^{rb} (Y_d^\dagger Y_d)^{dc} (Y_d Y_d^\dagger)^{st} - \frac{23}{8} \delta^{pa} \delta^{rb} g_L^2 Y_d^{*td} Y_d^{sc} \\
& - 8 \delta^{pa} \delta^{rb} \delta^{st} \delta^{cd} g_s^4 \left\} C_{\ell d}^{abcd} + \left\{ \frac{47}{486} \delta^{pr} \delta^{sa} \delta^{tb} \delta^{cd} g_Y^4 + \frac{3}{2} T_2 \delta^{sa} \delta^{tb} Y_e^{*rd} Y_e^{pc} + \frac{3}{2} \delta^{sa} \delta^{tb} Y_e^{pc} (Y_e^\dagger Y_e Y_e^\dagger)^{rd} + \frac{3}{2} \delta^{sa} \delta^{tb} Y_e^{*rd} (Y_e Y_e^\dagger Y_e)^{pc} \right. \right. \\
& - \frac{1}{4} \delta^{tb} Y_e^{*rd} Y_e^{pc} (Y_u Y_u^\dagger)^{sa} - \frac{1}{4} \delta^{sa} Y_e^{*rd} Y_e^{pc} (Y_u Y_u^\dagger)^{bt} - \frac{61}{162} \delta^{pr} \delta^{sa} \delta^{tb} \delta^{cd} g_Y^2 g_L^2 - \frac{1}{2} \delta^{sa} \delta^{tb} (Y_e^\dagger Y_e)^{dc} (Y_e Y_e^\dagger)^{pr} - g_Y^2 \left( \frac{5}{8} \delta^{sa} \delta^{tb} Y_e^{*rd} Y_e^{pc} \right. \\
& + \frac{5}{3} \delta^{pr} \delta^{sa} \delta^{tb} (Y_e^\dagger Y_e)^{dc} \Big) - \frac{23}{8} \delta^{sa} \delta^{tb} g_L^2 Y_e^{*rd} Y_e^{pc} \left\} C_{qe}^{abcd} + \left\{ \frac{61}{81} \delta^{pr} \delta^{sa} \delta^{tb} \delta^{cd} g_Y^2 g_L^2 + g_Y^2 \left( \frac{11}{27} \delta^{pr} \delta^{sa} Y_u^{*td} Y_u^{bc} + \frac{11}{27} \delta^{pr} \delta^{tb} Y_u^{*ad} Y_u^{sc} \right. \right.
\end{aligned}$$



$$\begin{aligned}
& + 3\delta^{pr}\delta^{sa}\delta^{tb}(Y_u^\dagger Y_u)^{dc} \Big) + \frac{3}{2}\delta^{sa}\delta^{tb}(Y_u^\dagger Y_u)^{dc}(Y_e Y_e^\dagger)^{pr} - g_L^2 \Big( \frac{1}{9}\delta^{pr}\delta^{sa}Y_u^{*td}Y_u^{bc} + \frac{1}{9}\delta^{pr}\delta^{tb}Y_u^{*ad}Y_u^{sc} \Big) - \frac{947}{243}\delta^{pr}\delta^{sa}\delta^{tb}\delta^{cd}g_Y^4 \\
& - \frac{16}{3}\delta^{pr}\delta^{sa}\delta^{tb}\delta^{cd}g_Y^2g_s^2 \Big\} C_{qu}^{(\parallel)abcd} + \left\{ \frac{61}{243}\delta^{pr}\delta^{sa}\delta^{tb}\delta^{cd}g_Y^2g_L^2 + \frac{1}{2}\delta^{sa}\delta^{tb}(Y_u^\dagger Y_u)^{dc}(Y_e Y_e^\dagger)^{pr} + g_L^2 \Big( \frac{1}{6}\delta^{pr}\delta^{sa}Y_u^{*td}Y_u^{bc} + \frac{1}{6}\delta^{pr}\delta^{tb}Y_u^{*ad}Y_u^{sc} \right) \right. \\
& + g_Y^2g_s^2 \Big( \frac{2}{27}\delta^{pr}\delta^{st}\delta^{ab}\delta^{cd} + \frac{1288}{243}\delta^{pr}\delta^{sa}\delta^{tb}\delta^{cd} \Big) + g_Y^2 \Big( \frac{8}{9}\delta^{pr}\delta^{sa}\delta^{tb}(Y_u^\dagger Y_u)^{dc} + \frac{25}{18}\delta^{pr}\delta^{sa}Y_u^{*td}Y_u^{bc} + \frac{25}{18}\delta^{pr}\delta^{tb}Y_u^{*ad}Y_u^{sc} - \frac{1}{9}\delta^{pr}\delta^{ab}Y_u^{*td}Y_u^{sc} \Big) \\
& + \frac{82}{81}\delta^{pr}\delta^{sa}\delta^{tb}\delta^{cd}g_s^2g_L^2 - \frac{947}{729}\delta^{pr}\delta^{sa}\delta^{tb}\delta^{cd}g_Y^4 \Big\} C_{qu}^{(\times)abcd} + \left\{ \frac{8}{3}\delta^{pr}\delta^{sa}\delta^{tb}\delta^{cd}g_Y^2g_s^2 - \frac{61}{162}\delta^{pr}\delta^{sa}\delta^{tb}\delta^{cd}g_Y^2g_L^2 - \frac{241}{486}\delta^{pr}\delta^{sa}\delta^{tb}\delta^{cd}g_Y^4 \right. \\
& - g_L^2 \Big( \frac{1}{9}\delta^{pr}\delta^{sa}Y_d^{*td}Y_d^{bc} + \frac{1}{9}\delta^{pr}\delta^{tb}Y_d^{*ad}Y_d^{sc} \Big) - g_Y^2 \Big( \frac{7}{27}\delta^{pr}\delta^{sa}Y_d^{*td}Y_d^{bc} + \frac{7}{27}\delta^{pr}\delta^{tb}Y_d^{*ad}Y_d^{sc} + \delta^{pr}\delta^{sa}\delta^{tb}(Y_d^\dagger Y_d)^{dc} \Big) - \frac{3}{2}\delta^{sa}\delta^{tb}(Y_d^\dagger Y_d)^{dc}(Y_e Y_e^\dagger)^{pr} \Big\} C_{qd}^{(\parallel)abcd} \\
& + \left\{ g_L^2 \Big( \frac{1}{6}\delta^{pr}\delta^{sa}Y_d^{*td}Y_d^{bc} + \frac{1}{6}\delta^{pr}\delta^{tb}Y_d^{*ad}Y_d^{sc} \Big) + g_Y^2g_s^2 \Big( \frac{2}{27}\delta^{pr}\delta^{st}\delta^{ab}\delta^{cd} - \frac{440}{243}\delta^{pr}\delta^{sa}\delta^{tb}\delta^{cd} \Big) + \frac{82}{81}\delta^{pr}\delta^{sa}\delta^{tb}\delta^{cd}g_s^2g_L^2 - \frac{61}{486}\delta^{pr}\delta^{sa}\delta^{tb}\delta^{cd}g_Y^2g_L^2 \right. \\
& - \frac{241}{1458}\delta^{pr}\delta^{sa}\delta^{tb}\delta^{cd}g_Y^4 - \frac{1}{2}\delta^{sa}\delta^{tb}(Y_d^\dagger Y_d)^{dc}(Y_e Y_e^\dagger)^{pr} - g_Y^2 \Big( \frac{1}{9}\delta^{pr}\delta^{ab}Y_d^{*td}Y_d^{sc} + \frac{4}{9}\delta^{pr}\delta^{sa}\delta^{tb}(Y_d^\dagger Y_d)^{dc} + \frac{11}{18}\delta^{pr}\delta^{sa}Y_d^{*td}Y_d^{bc} \\
& + \frac{11}{18}\delta^{pr}\delta^{tb}Y_d^{*ad}Y_d^{sc} \Big) \Big\} C_{qd}^{(\times)abcd} + \left\{ \frac{4}{9}\delta^{st}\delta^{ad}g_Y^2Y_e^{*rb}Y_e^{pc} - \frac{8}{27}\delta^{pr}\delta^{st}\delta^{ab}\delta^{cd}g_Y^4 \right\} C_{ee}^{abcd} + \left\{ \frac{8}{9}\delta^{pr}\delta^{ad}g_Y^2Y_u^{*tb}Y_u^{sc} - \frac{32}{81}\delta^{pr}\delta^{st}\delta^{ad}\delta^{bc}g_Y^4 \right\} C_{uu}^{abcd} \\
& - \left\{ \frac{8}{81}\delta^{pr}\delta^{st}\delta^{ad}\delta^{bc}g_Y^4 + \frac{4}{9}\delta^{pr}\delta^{ad}g_Y^2Y_d^{*tb}Y_d^{sc} \right\} C_{dd}^{abcd} + \frac{1}{2}Y_e^{*rb}Y_u^{*td}C_{eu}^{abcd}Y_e^{pa}Y_u^{sc} + \left\{ \frac{1}{4}\delta^{pa}Y_e^{*rb}Y_d^{sc}(Y_u Y_u^\dagger)^{dt} + \frac{3}{4}\delta^{pa}Y_e^{*rb}Y_d^{dc}(Y_u Y_u^\dagger)^{st} \right. \\
& + g_Y^2 \Big( \frac{7}{54}\delta^{pr}\delta^{td}Y_e^{*ab}Y_d^{sc} - \frac{5}{18}\delta^{pa}\delta^{st}Y_e^{*rb}Y_d^{dc} \Big) + g_L^2 \Big( \frac{1}{18}\delta^{pr}\delta^{td}Y_e^{*ab}Y_d^{sc} + \frac{1}{6}\delta^{pa}\delta^{st}Y_e^{*rb}Y_d^{dc} - \frac{1}{4}\delta^{pa}\delta^{td}Y_e^{*rb}Y_d^{sc} \Big) - \frac{5}{8}\delta^{pa}Y_e^{*rb}Y_d^{sc}(Y_d Y_d^\dagger)^{dt} \\
& - \frac{5}{8}\delta^{td}Y_e^{*rb}Y_d^{sc}(Y_e Y_e^\dagger)^{pa} \Big\} C_{ledq}^{abcd} + C_{ledq}^{*abcd} \left\{ \frac{1}{4}\delta^{ra}Y_d^{*tc}Y_e^{pb}(Y_u Y_u^\dagger)^{sd} + \frac{3}{4}\delta^{ra}Y_d^{*dc}Y_e^{pb}(Y_u Y_u^\dagger)^{st} + g_Y^2 \Big( \frac{7}{54}\delta^{pr}\delta^{sd}Y_d^{*tc}Y_e^{ab} - \frac{5}{18}\delta^{ra}\delta^{st}Y_d^{*dc}Y_e^{pb} \right) \right. \\
& + g_L^2 \Big( \frac{1}{18}\delta^{pr}\delta^{sd}Y_d^{*tc}Y_e^{ab} + \frac{1}{6}\delta^{ra}\delta^{st}Y_d^{*dc}Y_e^{pb} - \frac{1}{4}\delta^{ra}\delta^{sd}Y_d^{*tc}Y_e^{pb} \Big) - \frac{5}{8}\delta^{ra}Y_d^{*tc}Y_e^{pb}(Y_d Y_d^\dagger)^{sd} - \frac{5}{8}\delta^{sd}Y_d^{*tc}Y_e^{pb}(Y_e Y_e^\dagger)^{ar} \Big\} + \left\{ \frac{1}{8}\delta^{sc}Y_d^{*ad}Y_u^{*tb}(Y_e Y_e^\dagger)^{pr} \right. \\
& + \frac{3}{4}\delta^{sa}Y_d^{*cd}Y_u^{*tb}(Y_e Y_e^\dagger)^{pr} + g_L^2 \Big( \frac{1}{6}\delta^{pr}\delta^{sa}Y_d^{*cd}Y_u^{*tb} + \frac{1}{6}\delta^{pr}\delta^{sc}Y_d^{*td}Y_u^{*ab} - \frac{7}{72}\delta^{pr}\delta^{sa}Y_d^{*td}Y_u^{*cb} - \frac{7}{72}\delta^{pr}\delta^{sc}Y_d^{*ad}Y_u^{*tb} \Big) + g_Y^2 \Big( \frac{11}{216}\delta^{pr}\delta^{sa}Y_d^{*td}Y_u^{*cb} \\
& + \frac{7}{18}\delta^{pr}\delta^{sc}Y_d^{*td}Y_u^{*ab} - \frac{7}{216}\delta^{pr}\delta^{sc}Y_d^{*ad}Y_u^{*tb} - \frac{11}{18}\delta^{pr}\delta^{sa}Y_d^{*cd}Y_u^{*tb} \Big) \Big\} C_{quqd}^{(\parallel)abcd} + (C_{quqd}^{(\parallel)*})^{abcd} \left\{ \frac{1}{8}\delta^{tc}Y_d^{ad}Y_u^{sb}(Y_e Y_e^\dagger)^{pr} + \frac{3}{4}\delta^{ta}Y_d^{cd}Y_u^{sb}(Y_e Y_e^\dagger)^{pr} \right. \\
& + g_L^2 \Big( \frac{1}{6}\delta^{pr}\delta^{ta}Y_d^{cd}Y_u^{sb} + \frac{1}{6}\delta^{pr}\delta^{tc}Y_d^{sd}Y_u^{ab} - \frac{7}{72}\delta^{pr}\delta^{ta}Y_d^{sd}Y_u^{cb} - \frac{7}{72}\delta^{pr}\delta^{tc}Y_d^{ad}Y_u^{sb} \Big) + g_Y^2 \Big( \frac{11}{216}\delta^{pr}\delta^{ta}Y_d^{sd}Y_u^{cb} + \frac{7}{18}\delta^{pr}\delta^{tc}Y_d^{sd}Y_u^{ab} - \frac{7}{216}\delta^{pr}\delta^{tc}Y_d^{ad}Y_u^{sb}
\end{aligned}$$

$$\begin{aligned}
& -\frac{11}{18}\delta^{pr}\delta^{ta}Y_d^{cd}Y_u^{sb}\Big)\Big\} + \Big\{\frac{1}{4}\delta^{sa}Y_d^{*cd}Y_u^{*tb}(Y_eY_e^\dagger)^{pr} + \frac{3}{8}\delta^{sc}Y_d^{*ad}Y_u^{*tb}(Y_eY_e^\dagger)^{pr} + g_Y^2\Big(\frac{5}{72}\delta^{pr}\delta^{sa}Y_d^{*td}Y_u^{*cb} + \frac{11}{108}\delta^{pr}\delta^{sc}Y_d^{*td}Y_u^{*ab} \\
& -\frac{13}{72}\delta^{pr}\delta^{sc}Y_d^{*ad}Y_u^{*tb} - \frac{25}{108}\delta^{pr}\delta^{sa}Y_d^{*cd}Y_u^{*tb}\Big) + g_L^2\Big(\frac{5}{36}\delta^{pr}\delta^{sa}Y_d^{*cd}Y_u^{*tb} + \frac{5}{36}\delta^{pr}\delta^{sc}Y_d^{*td}Y_u^{*ab} - \frac{1}{24}\delta^{pr}\delta^{sa}Y_d^{*td}Y_u^{*cb} \\
& -\frac{1}{24}\delta^{pr}\delta^{sc}Y_d^{*ad}Y_u^{*tb}\Big)\Big\} C_{quqd}^{(\times)abcd} + \Big(C_{quqd}^{(\times)*}\Big)^{abcd}\Big\{\frac{1}{4}\delta^{ta}Y_d^{cd}Y_u^{sb}(Y_eY_e^\dagger)^{pr} + \frac{3}{8}\delta^{tc}Y_d^{ad}Y_u^{sb}(Y_eY_e^\dagger)^{pr} + g_Y^2\Big(\frac{5}{72}\delta^{pr}\delta^{ta}Y_d^{sd}Y_u^{cb} + \frac{11}{108}\delta^{pr}\delta^{tc}Y_d^{sd}Y_u^{ab} \\
& -\frac{13}{72}\delta^{pr}\delta^{tc}Y_d^{ad}Y_u^{sb} - \frac{25}{108}\delta^{pr}\delta^{ta}Y_d^{cd}Y_u^{sb}\Big) + g_L^2\Big(\frac{5}{36}\delta^{pr}\delta^{ta}Y_d^{cd}Y_u^{sb} + \frac{5}{36}\delta^{pr}\delta^{tc}Y_d^{sd}Y_u^{ab} - \frac{1}{24}\delta^{pr}\delta^{ta}Y_d^{sd}Y_u^{cb} - \frac{1}{24}\delta^{pr}\delta^{tc}Y_d^{ad}Y_u^{sb}\Big)\Big\} \\
& + \Big\{g_L^2\Big(\frac{21}{16}\delta^{pa}\delta^{sc}Y_e^{*rb}Y_u^{*td} - \frac{1}{18}\delta^{pr}\delta^{sc}Y_e^{*ab}Y_u^{*td} - \frac{1}{6}\delta^{pa}\delta^{st}Y_e^{*rb}Y_u^{*cd}\Big) + g_Y^2\Big(\frac{11}{54}\delta^{pr}\delta^{sc}Y_e^{*ab}Y_u^{*td} + \frac{5}{18}\delta^{pa}\delta^{st}Y_e^{*rb}Y_u^{*cd} + \frac{271}{144}\delta^{pa}\delta^{sc}Y_e^{*rb}Y_u^{*td}\Big) \\
& -\frac{1}{4}\text{T}_2\delta^{pa}\delta^{sc}Y_e^{*rb}Y_u^{*td} - \frac{1}{4}\delta^{sc}Y_e^{*ab}Y_u^{*td}(Y_eY_e^\dagger)^{pr} - \frac{1}{4}\delta^{pa}\delta^{sc}Y_e^{*rb}(Y_d^\dagger Y_d Y_u^\dagger)^{td} - \frac{1}{4}\delta^{pa}\delta^{sc}Y_u^{*td}(Y_e^\dagger Y_e Y_e^\dagger)^{rb} - \frac{1}{4}\delta^{pa}\delta^{sc}Y_e^{*rb}(Y_u^\dagger Y_u Y_u^\dagger)^{td} \\
& -\frac{5}{8}\delta^{sc}Y_e^{*rb}Y_u^{*td}(Y_eY_e^\dagger)^{pa} - \frac{5}{8}\delta^{pa}Y_e^{*rb}Y_u^{*td}(Y_uY_u^\dagger)^{sc} - \frac{3}{4}\delta^{pa}Y_e^{*rb}Y_u^{*cd}(Y_uY_u^\dagger)^{st} - \frac{8}{3}\delta^{pa}\delta^{sc}g_s^2Y_e^{*rb}Y_u^{*td}\Big\} C_{lequ}^{abcd} + C_{lequ}^{*abcd}\Big\{g_L^2\Big(\frac{21}{16}\delta^{ra}\delta^{tc}Y_e^{pb}Y_u^{sd} \\
& -\frac{1}{18}\delta^{pr}\delta^{tc}Y_e^{ab}Y_u^{sd} - \frac{1}{6}\delta^{ra}\delta^{st}Y_e^{pb}Y_u^{cd}\Big) + g_Y^2\Big(\frac{11}{54}\delta^{pr}\delta^{tc}Y_e^{ab}Y_u^{sd} + \frac{5}{18}\delta^{ra}\delta^{st}Y_e^{pb}Y_u^{cd} + \frac{271}{144}\delta^{ra}\delta^{tc}Y_e^{pb}Y_u^{sd}\Big) - \frac{1}{4}\text{T}_2\delta^{ra}\delta^{tc}Y_e^{pb}Y_u^{sd} - \frac{1}{4}\delta^{tc}Y_e^{ab}Y_u^{sd}(Y_eY_e^\dagger)^{pr} \\
& -\frac{1}{4}\delta^{ra}\delta^{tc}Y_e^{pb}(Y_dY_d^\dagger Y_u)^{sd} - \frac{1}{4}\delta^{ra}\delta^{tc}Y_u^{sd}(Y_eY_e^\dagger Y_e)^{pb} - \frac{1}{4}\delta^{ra}\delta^{tc}Y_e^{pb}(Y_uY_u^\dagger Y_u)^{sd} - \frac{5}{8}\delta^{tc}Y_e^{pb}Y_u^{sd}(Y_eY_e^\dagger)^{ar} - \frac{5}{8}\delta^{ra}Y_e^{pb}Y_u^{sd}(Y_uY_u^\dagger)^{ct} - \frac{3}{4}\delta^{ra}Y_e^{pb}Y_u^{cd}(Y_uY_u^\dagger)^{st} \\
& -\frac{8}{3}\delta^{ra}\delta^{tc}g_s^2Y_e^{pb}Y_u^{sd}\Big)\Big\} + \Big\{\frac{1}{8}\delta^{sc}Y_e^{*ad}Y_u^{*tb}(Y_eY_e^\dagger)^{pr} + \frac{1}{4}\delta^{sc}Y_e^{*rd}Y_u^{*tb}(Y_eY_e^\dagger)^{pa} + \frac{1}{4}\delta^{pa}Y_e^{*rd}Y_u^{*tb}(Y_uY_u^\dagger)^{sc} + \frac{3}{8}\delta^{pa}Y_e^{*rd}Y_u^{*cb}(Y_uY_u^\dagger)^{st} \\
& + g_L^2\Big(\frac{21}{16}\delta^{pa}\delta^{sc}Y_e^{*rd}Y_u^{*tb} - \frac{1}{72}\delta^{pr}\delta^{sc}Y_e^{*ad}Y_u^{*tb} - \frac{1}{24}\delta^{pa}\delta^{st}Y_e^{*rd}Y_u^{*cb}\Big) + g_Y^2\Big(\frac{311}{144}\delta^{pa}\delta^{sc}Y_e^{*rd}Y_u^{*tb} - \frac{13}{216}\delta^{pr}\delta^{sc}Y_e^{*ad}Y_u^{*tb} - \frac{7}{72}\delta^{pa}\delta^{st}Y_e^{*rd}Y_u^{*cb}\Big) \\
& -\frac{1}{4}\text{T}_2\delta^{pa}\delta^{sc}Y_e^{*rd}Y_u^{*tb} - \frac{1}{4}\delta^{pa}\delta^{sc}Y_e^{*rd}(Y_d^\dagger Y_d Y_u^\dagger)^{tb} - \frac{1}{4}\delta^{pa}\delta^{sc}Y_u^{*tb}(Y_e^\dagger Y_e Y_e^\dagger)^{rd} - \frac{1}{4}\delta^{pa}\delta^{sc}Y_e^{*rd}(Y_u^\dagger Y_u Y_u^\dagger)^{tb} - \frac{7}{3}\delta^{pa}\delta^{sc}g_s^2Y_e^{*rd}Y_u^{*tb}\Big\} C_{luqe}^{abcd} \\
& + C_{luqe}^{*abcd}\Big\{\frac{1}{8}\delta^{tc}Y_e^{ad}Y_u^{sb}(Y_eY_e^\dagger)^{pr} + \frac{1}{4}\delta^{tc}Y_e^{pd}Y_u^{sb}(Y_eY_e^\dagger)^{ar} + \frac{1}{4}\delta^{ra}Y_e^{pd}Y_u^{sb}(Y_uY_u^\dagger)^{ct} + \frac{3}{8}\delta^{ra}Y_e^{pd}Y_u^{cb}(Y_uY_u^\dagger)^{st} + g_L^2\Big(\frac{21}{16}\delta^{ra}\delta^{tc}Y_e^{pd}Y_u^{sb} - \frac{1}{72}\delta^{pr}\delta^{tc}Y_e^{ad}Y_u^{sb} \\
& -\frac{1}{24}\delta^{ra}\delta^{st}Y_e^{pd}Y_u^{cb}\Big) + g_Y^2\Big(\frac{311}{144}\delta^{ra}\delta^{tc}Y_e^{pd}Y_u^{sb} - \frac{13}{216}\delta^{pr}\delta^{tc}Y_e^{ad}Y_u^{sb} - \frac{7}{72}\delta^{ra}\delta^{st}Y_e^{pd}Y_u^{cb}\Big) - \frac{1}{4}\text{T}_2\delta^{ra}\delta^{tc}Y_e^{pd}Y_u^{sb} - \frac{1}{4}\delta^{ra}\delta^{tc}Y_e^{pd}(Y_dY_d^\dagger Y_u)^{sb} \\
& -\frac{1}{4}\delta^{ra}\delta^{tc}Y_u^{sb}(Y_eY_e^\dagger Y_e)^{pd} - \frac{1}{4}\delta^{ra}\delta^{tc}Y_e^{pd}(Y_uY_u^\dagger Y_u)^{sb} - \frac{7}{3}\delta^{ra}\delta^{tc}g_s^2Y_e^{pd}Y_u^{sb}\Big)\Big\} + \Big\{g_Y^4\Big(\frac{46}{81}\delta^{pa}\delta^{rb}\delta^{st}\delta^{cd} + \frac{53}{81}\delta^{pa}\delta^{rd}\delta^{st}\delta^{bc} - \frac{4}{27}\delta^{pr}\delta^{st}\delta^{ad}\delta^{bc}\Big) \\
& + g_Y^2g_L^2\Big(\frac{2}{27}\delta^{pr}\delta^{st}\delta^{ad}\delta^{bc} + \frac{28}{27}\delta^{pa}\delta^{rb}\delta^{st}\delta^{cd} + \frac{68}{27}\delta^{pa}\delta^{rd}\delta^{st}\delta^{bc}\Big) + g_L^4\Big(\frac{34}{3}\delta^{pa}\delta^{rb}\delta^{st}\delta^{cd} - \frac{1}{9}\delta^{pa}\delta^{rd}\delta^{st}\delta^{bc} - \frac{2}{9}\delta^{pr}\delta^{st}\delta^{ad}\delta^{bc}\Big)
\end{aligned}$$

$$\begin{aligned}
& + \delta^{pa} \delta^{rb} (Y_d Y_d^\dagger)^{st} (Y_e Y_e^\dagger)^{dc} + g_Y^2 \left( \frac{2}{3} \delta^{pa} \delta^{rd} \delta^{st} (Y_e Y_e^\dagger)^{bc} + \frac{8}{9} \delta^{pa} \delta^{rb} \delta^{st} (Y_e Y_e^\dagger)^{dc} \right) + \frac{4}{3} \delta^{pa} \delta^{rd} \delta^{st} g_L^2 (Y_e Y_e^\dagger)^{bc} - \delta^{pa} \delta^{rb} (Y_e Y_e^\dagger)^{dc} (Y_u Y_u^\dagger)^{st} \\
& - 3 \delta^{pa} \delta^{rd} (Y_e Y_e^\dagger)^{bc} (Y_u Y_u^\dagger)^{st} \left\{ C_{\ell\ell}^{abcd} + \left\{ g_Y^2 g_s^2 \left( \frac{4}{27} \delta^{pr} \delta^{st} \delta^{ad} \delta^{bc} - \frac{22}{243} \delta^{pr} \delta^{sa} \delta^{td} \delta^{bc} - 4 \delta^{pr} \delta^{sa} \delta^{tb} \delta^{cd} \right) + g_Y^2 g_L^2 \left( \frac{722}{243} \delta^{pr} \delta^{sa} \delta^{td} \delta^{bc} \right. \right. \right. \\
& - \frac{182}{81} \delta^{pr} \delta^{sa} \delta^{tb} \delta^{cd} \left. \left. \left. \right) + g_Y^4 \left( \frac{245}{729} \delta^{pr} \delta^{sa} \delta^{td} \delta^{bc} + \frac{286}{243} \delta^{pr} \delta^{sa} \delta^{tb} \delta^{cd} - \frac{4}{81} \delta^{pr} \delta^{st} \delta^{ad} \delta^{bc} \right) + g_L^4 \left( 28 \delta^{pr} \delta^{sa} \delta^{tb} \delta^{cd} - \frac{7}{9} \delta^{pr} \delta^{sa} \delta^{td} \delta^{bc} - \frac{4}{3} \delta^{pr} \delta^{st} \delta^{ad} \delta^{bc} \right) \right. \right. \\
& + g_L^2 \left( \frac{4}{3} \delta^{pr} \delta^{sa} \delta^{td} (Y_d Y_d^\dagger)^{bc} + \frac{4}{3} \delta^{pr} \delta^{sa} \delta^{td} (Y_u Y_u^\dagger)^{bc} \right) + g_Y^2 \left( \frac{2}{9} \delta^{pr} \delta^{sa} \delta^{td} (Y_d Y_d^\dagger)^{bc} + \frac{8}{9} \delta^{pr} \delta^{sa} \delta^{td} (Y_u Y_u^\dagger)^{bc} + 4 \delta^{pr} \delta^{sa} \delta^{tb} (Y_u Y_u^\dagger)^{dc} \right) \\
& + 3 \delta^{sa} \delta^{tb} (Y_d Y_d^\dagger)^{dc} (Y_e Y_e^\dagger)^{pr} - \frac{130}{81} \delta^{pr} \delta^{sa} \delta^{td} \delta^{bc} g_s^2 g_L^2 - 3 \delta^{sa} \delta^{td} (Y_e Y_e^\dagger)^{pr} (Y_u Y_u^\dagger)^{bc} - 3 \delta^{sa} \delta^{tb} (Y_e Y_e^\dagger)^{pr} (Y_u Y_u^\dagger)^{dc} \left\} C_{qq}^{(\parallel)abcd} \right. \\
& + \left\{ g_s^2 g_L^2 \left( \frac{136}{81} \delta^{pr} \delta^{sa} \delta^{td} \delta^{bc} - 6 \delta^{pr} \delta^{sa} \delta^{tb} \delta^{cd} \right) + g_Y^2 g_s^2 \left( \frac{8}{27} \delta^{pr} \delta^{st} \delta^{ad} \delta^{bc} - \frac{44}{243} \delta^{pr} \delta^{sa} \delta^{td} \delta^{bc} - 2 \delta^{pr} \delta^{sa} \delta^{tb} \delta^{cd} \right) + g_L^4 \left( \frac{34}{3} \delta^{pr} \delta^{sa} \delta^{td} \delta^{bc} \right. \right. \\
& - \frac{1}{3} \delta^{pr} \delta^{sa} \delta^{tb} \delta^{cd} \left. \left. \right) + g_Y^4 \left( \frac{143}{243} \delta^{pr} \delta^{sa} \delta^{tb} \delta^{cd} + \frac{490}{729} \delta^{pr} \delta^{sa} \delta^{td} \delta^{bc} - \frac{8}{81} \delta^{pr} \delta^{st} \delta^{ad} \delta^{bc} \right) + g_Y^2 g_L^2 \left( \frac{350}{81} \delta^{pr} \delta^{sa} \delta^{tb} \delta^{cd} - \frac{32}{243} \delta^{pr} \delta^{sa} \delta^{td} \delta^{bc} \right) \right. \\
& + g_L^2 \left( 2 \delta^{pr} \delta^{sa} \delta^{tb} (Y_d Y_d^\dagger)^{dc} + 2 \delta^{pr} \delta^{sa} \delta^{tb} (Y_u Y_u^\dagger)^{dc} \right) + g_Y^2 \left( \frac{4}{9} \delta^{pr} \delta^{sa} \delta^{td} (Y_d Y_d^\dagger)^{bc} + \frac{16}{9} \delta^{pr} \delta^{sa} \delta^{td} (Y_u Y_u^\dagger)^{bc} + 2 \delta^{pr} \delta^{sa} \delta^{tb} (Y_u Y_u^\dagger)^{dc} \right) \\
& + 3 \delta^{sa} \delta^{td} (Y_d Y_d^\dagger)^{bc} (Y_e Y_e^\dagger)^{pr} - 3 \delta^{sa} \delta^{td} (Y_e Y_e^\dagger)^{pr} (Y_u Y_u^\dagger)^{bc} - 3 \delta^{sa} \delta^{tb} (Y_e Y_e^\dagger)^{pr} (Y_u Y_u^\dagger)^{dc} \left\} C_{qq}^{(\times)abcd} + \left\{ \frac{1}{2} \delta^{sc} \delta^{td} (Y_e Y_e^\dagger)^{pr} (Y_e Y_e^\dagger)^{ba} + g_Y^2 g_L^2 \left( \frac{91}{81} \delta^{pr} \delta^{sc} \delta^{td} \delta^{ab} \right. \right. \right. \\
& + \frac{21}{4} \delta^{pa} \delta^{rb} \delta^{sc} \delta^{td} - \frac{5}{27} \delta^{pa} \delta^{rb} \delta^{st} \delta^{cd} \left. \left. \right) + g_Y^4 \left( \frac{469}{243} \delta^{pr} \delta^{sc} \delta^{td} \delta^{ab} - \frac{11}{81} \delta^{pa} \delta^{rb} \delta^{st} \delta^{cd} - \frac{31}{72} \delta^{pa} \delta^{rb} \delta^{sc} \delta^{td} \right) + g_Y^2 g_s^2 \left( \frac{8}{9} \delta^{pa} \delta^{rb} \delta^{st} \delta^{cd} + 4 \delta^{pa} \delta^{rb} \delta^{sc} \delta^{td} \right) \\
& + g_L^4 \left( \frac{14}{3} \delta^{pr} \delta^{sc} \delta^{td} \delta^{ab} + 14 \delta^{pa} \delta^{rb} \delta^{st} \delta^{cd} - \frac{385}{24} \delta^{pa} \delta^{rb} \delta^{sc} \delta^{td} \right) + \delta^{pa} \delta^{rb} (Y_d Y_d^\dagger)^{dt} (Y_u Y_u^\dagger)^{sc} + \delta^{pa} \delta^{rb} (Y_d Y_d^\dagger)^{sc} (Y_u Y_u^\dagger)^{dt} + g_L^2 \left( \frac{33}{16} \delta^{pa} \delta^{rb} \delta^{td} (Y_d Y_d^\dagger)^{sc} \right. \\
& + \frac{33}{16} \delta^{pa} \delta^{rb} \delta^{sc} (Y_d Y_d^\dagger)^{dt} + \frac{33}{16} \delta^{rb} \delta^{sc} \delta^{td} (Y_e Y_e^\dagger)^{pa} + \frac{33}{16} \delta^{pa} \delta^{sc} \delta^{td} (Y_e Y_e^\dagger)^{br} + \frac{33}{16} \delta^{pa} \delta^{rb} \delta^{td} (Y_u Y_u^\dagger)^{sc} + \frac{33}{16} \delta^{pa} \delta^{rb} \delta^{sc} (Y_u Y_u^\dagger)^{dt} \left. \right) \\
& + g_Y^2 \left( \frac{7}{144} \delta^{pa} \delta^{rb} \delta^{td} (Y_d Y_d^\dagger)^{sc} + \frac{7}{144} \delta^{pa} \delta^{rb} \delta^{sc} (Y_d Y_d^\dagger)^{dt} + \frac{23}{16} \delta^{rb} \delta^{sc} \delta^{td} (Y_e Y_e^\dagger)^{pa} + \frac{23}{16} \delta^{pa} \delta^{sc} \delta^{td} (Y_e Y_e^\dagger)^{br} + \frac{427}{144} \delta^{pa} \delta^{rb} \delta^{td} (Y_u Y_u^\dagger)^{sc} \right. \\
& + \frac{427}{144} \delta^{pa} \delta^{rb} \delta^{sc} (Y_u Y_u^\dagger)^{dt} - \frac{2}{3} \delta^{pa} \delta^{rb} \delta^{st} (Y_u Y_u^\dagger)^{dc} - \frac{4}{3} \delta^{pr} \delta^{sc} \delta^{td} (Y_e Y_e^\dagger)^{ba} \left. \right) + \frac{3}{2} \delta^{pa} \delta^{rb} (Y_d Y_d^\dagger)^{st} (Y_d Y_d^\dagger)^{dc} + \frac{3}{2} \delta^{pa} \delta^{rb} (Y_u Y_u^\dagger)^{st} (Y_u Y_u^\dagger)^{dc} \\
& + 12 \delta^{pa} \delta^{rb} \delta^{sc} \delta^{td} g_s^2 g_L^2 + 16 \delta^{pa} \delta^{rb} \delta^{st} \delta^{cd} g_s^4 - \frac{1}{4} \delta^{pa} \delta^{rb} \delta^{td} (Y_d Y_d^\dagger Y_d Y_d^\dagger)^{sc} - \frac{1}{4} \delta^{pa} \delta^{rb} \delta^{sc} (Y_d Y_d^\dagger Y_d Y_d^\dagger)^{dt} - \frac{1}{4} \delta^{rb} \delta^{sc} \delta^{td} (Y_e Y_e^\dagger Y_e Y_e^\dagger)^{pa} \\
& - \frac{1}{4} \delta^{pa} \delta^{sc} \delta^{td} (Y_e Y_e^\dagger Y_e Y_e^\dagger)^{br} - \frac{1}{4} \delta^{pa} \delta^{rb} \delta^{td} (Y_u Y_u^\dagger Y_u Y_u^\dagger)^{sc} - \frac{1}{4} \delta^{pa} \delta^{rb} \delta^{sc} (Y_u Y_u^\dagger Y_u Y_u^\dagger)^{dt} - \frac{3}{4} T_2 \delta^{pa} \delta^{rb} \delta^{td} (Y_d Y_d^\dagger)^{sc} - \frac{3}{4} T_2 \delta^{pa} \delta^{rb} \delta^{sc} (Y_d Y_d^\dagger)^{dt} \\
& - \frac{3}{4} T_2 \delta^{rb} \delta^{sc} \delta^{td} (Y_e Y_e^\dagger)^{pa} - \frac{3}{4} T_2 \delta^{pa} \delta^{sc} \delta^{td} (Y_e Y_e^\dagger)^{br} - \frac{3}{4} T_2 \delta^{pa} \delta^{rb} \delta^{td} (Y_u Y_u^\dagger)^{sc} - \frac{3}{4} T_2 \delta^{pa} \delta^{rb} \delta^{sc} (Y_u Y_u^\dagger)^{dt} - \delta^{pa} \delta^{td} (Y_e Y_e^\dagger)^{br} (Y_u Y_u^\dagger)^{sc} \\
& - \delta^{rb} \delta^{sc} (Y_e Y_e^\dagger)^{pa} (Y_u Y_u^\dagger)^{dt} - g_s^2 \left( \frac{8}{3} \delta^{pa} \delta^{rb} \delta^{td} (Y_d Y_d^\dagger)^{sc} + \frac{8}{3} \delta^{pa} \delta^{rb} \delta^{sc} (Y_d Y_d^\dagger)^{dt} + \frac{8}{3} \delta^{pa} \delta^{rb} \delta^{td} (Y_u Y_u^\dagger)^{sc} + \frac{8}{3} \delta^{pa} \delta^{rb} \delta^{sc} (Y_u Y_u^\dagger)^{dt} \right)
\end{aligned}$$

$$\begin{aligned}
& -\frac{3}{2}\delta^{pa}\delta^{rb}(Y_d Y_d^\dagger)^{dc}(Y_u Y_u^\dagger)^{st} - \frac{3}{2}\delta^{pa}\delta^{rb}(Y_d Y_d^\dagger)^{st}(Y_u Y_u^\dagger)^{dc} - \frac{7}{4}\delta^{rb}\delta^{td}(Y_e Y_e^\dagger)^{pa}(Y_u Y_u^\dagger)^{sc} - \frac{7}{4}\delta^{pa}\delta^{sc}(Y_e Y_e^\dagger)^{br}(Y_u Y_u^\dagger)^{dt} - \frac{5}{2}\delta^{pa}\delta^{rb}(Y_d Y_d^\dagger)^{sc}(Y_d Y_d^\dagger)^{dt} \\
& - \frac{5}{2}\delta^{sc}\delta^{td}(Y_e Y_e^\dagger)^{pa}(Y_e Y_e^\dagger)^{br} - \frac{5}{2}\delta^{pa}\delta^{rb}(Y_u Y_u^\dagger)^{sc}(Y_u Y_u^\dagger)^{dt} \Big\} C_{\ell q}^{(\parallel)abcd} + \left\{ \frac{4}{9}\delta^{pa}\delta^{rb}\delta^{st}\delta^{cd}g_Y^2g_s^2 + g_Y^4\left(\frac{469}{486}\delta^{pr}\delta^{sc}\delta^{td}\delta^{ab} - \frac{11}{162}\delta^{pa}\delta^{rb}\delta^{st}\delta^{cd}\right) \right. \\
& + g_Y^2g_L^2\left(\frac{2}{27}\delta^{pa}\delta^{rb}\delta^{st}\delta^{cd} + \frac{1}{9}\delta^{pr}\delta^{st}\delta^{ab}\delta^{cd} + \frac{5}{2}\delta^{pa}\delta^{rb}\delta^{sc}\delta^{td} - \frac{91}{81}\delta^{pr}\delta^{sc}\delta^{td}\delta^{ab}\right) + g_L^4\left(\frac{1}{3}\delta^{pr}\delta^{st}\delta^{ab}\delta^{cd} + \frac{5}{6}\delta^{pa}\delta^{rb}\delta^{st}\delta^{cd} + \frac{49}{3}\delta^{pa}\delta^{rb}\delta^{sc}\delta^{td} \right. \\
& - \frac{1}{18}\delta^{pr}\delta^{sc}\delta^{td}\delta^{ab}) + \delta^{pa}\delta^{rb}(Y_d Y_d^\dagger)^{dt}(Y_u Y_u^\dagger)^{sc} + \delta^{pa}\delta^{rb}(Y_d Y_d^\dagger)^{sc}(Y_u Y_u^\dagger)^{dt} + g_L^2\left(\frac{1}{3}\delta^{pr}\delta^{sc}\delta^{td}(Y_e Y_e^\dagger)^{ba} + \delta^{pa}\delta^{rb}\delta^{st}(Y_d Y_d^\dagger)^{dc} + \delta^{pa}\delta^{rb}\delta^{st}(Y_u Y_u^\dagger)^{dc}\right) \\
& + \frac{7}{4}\delta^{rb}\delta^{td}(Y_e Y_e^\dagger)^{pa}(Y_u Y_u^\dagger)^{sc} + \frac{7}{4}\delta^{pa}\delta^{sc}(Y_e Y_e^\dagger)^{br}(Y_u Y_u^\dagger)^{dt} + 2\delta^{rb}\delta^{td}(Y_d Y_d^\dagger)^{sc}(Y_e Y_e^\dagger)^{pa} + 2\delta^{pa}\delta^{sc}(Y_d Y_d^\dagger)^{dt}(Y_e Y_e^\dagger)^{br} + 8\delta^{pa}\delta^{rb}\delta^{st}\delta^{cd}g_s^4 \\
& - g_s^2g_L^2\left(4\delta^{pa}\delta^{rb}\delta^{st}\delta^{cd} + 12\delta^{pa}\delta^{rb}\delta^{sc}\delta^{td}\right) - g_Y^2\left(\frac{1}{3}\delta^{pa}\delta^{rb}\delta^{st}(Y_u Y_u^\dagger)^{dc} + \frac{2}{3}\delta^{pr}\delta^{sc}\delta^{td}(Y_e Y_e^\dagger)^{ba}\right) - \frac{5}{4}\delta^{pa}\delta^{rb}(Y_d Y_d^\dagger)^{sc}(Y_d Y_d^\dagger)^{dt} \\
& \left. - \frac{5}{4}\delta^{sc}\delta^{td}(Y_e Y_e^\dagger)^{pa}(Y_e Y_e^\dagger)^{br} - \frac{5}{4}\delta^{pa}\delta^{rb}(Y_u Y_u^\dagger)^{sc}(Y_u Y_u^\dagger)^{dt} - \frac{3}{2}\delta^{pa}\delta^{rb}(Y_d Y_d^\dagger)^{dc}(Y_u Y_u^\dagger)^{st} - \frac{3}{2}\delta^{pa}\delta^{rb}(Y_d Y_d^\dagger)^{st}(Y_u Y_u^\dagger)^{dc} \right\} C_{\ell q}^{(\times)abcd}, \tag{13.8}
\end{aligned}$$

### 13.5 $C_{\ell q}^{(\times)}$

$$\begin{aligned}
\beta_{C_{\ell q}^{(\times)prst}}^{(1)} &= \left\{ \frac{1}{3}\delta^{pa}\delta^{rb}\delta^{st}g_L^2 - \delta^{pa}\delta^{rb}(Y_d Y_d^\dagger)^{st} - \delta^{pa}\delta^{rb}(Y_u Y_u^\dagger)^{st} \right\} C_{H\ell}^{(\times)ab} + \left\{ \frac{1}{3}\delta^{pr}\delta^{sa}\delta^{tb}g_L^2 - \delta^{sa}\delta^{tb}(Y_e Y_e^\dagger)^{pr} \right\} C_{Hq}^{(\times)ab} + \frac{1}{2}\delta^{pa}\delta^{td}Y_e^{*rb}C_{\ell edq}^{abcd}Y_d^{sc} \\
& + \frac{1}{2}\delta^{ra}\delta^{sd}C_{\ell edq}^{*abcd}Y_d^{tc}Y_e^{pb} - \frac{1}{2}\delta^{pa}\delta^{sc}Y_e^{*rb}Y_u^{*td}C_{\ell equ}^{abcd} - \frac{1}{2}\delta^{ra}\delta^{tc}C_{\ell equ}^{*abcd}Y_e^{pb}Y_u^{sd} - \frac{1}{2}\delta^{pa}\delta^{sc}Y_e^{*rd}Y_u^{*tb}C_{\ell uqe}^{abcd} - \frac{1}{2}\delta^{ra}\delta^{tc}C_{\ell uqe}^{*abcd}Y_e^{pd}Y_u^{sb} \\
& + \frac{4}{3}\delta^{pa}\delta^{rd}\delta^{st}\delta^{bc}g_L^2C_{\ell\ell}^{abcd} + \frac{4}{3}\delta^{pr}\delta^{sa}\delta^{td}\delta^{bc}g_L^2C_{qq}^{(\parallel)abcd} + 4\delta^{pr}\delta^{sa}\delta^{tb}\delta^{cd}g_L^2C_{qq}^{(\times)abcd} + 6\delta^{pa}\delta^{rb}\delta^{sc}\delta^{td}g_L^2C_{\ell q}^{(\parallel)abcd} + \left\{ \frac{1}{3}g_L^2\left(2\delta^{pr}\delta^{sc}\delta^{td}\delta^{ab} \right. \right. \\
& + 6\delta^{pa}\delta^{rb}\delta^{st}\delta^{cd} - 9\delta^{pa}\delta^{rb}\delta^{sc}\delta^{td}) + \frac{1}{2}\left(\delta^{pa}\delta^{rb}\delta^{td}(Y_d Y_d^\dagger)^{sc} + \delta^{pa}\delta^{rb}\delta^{sc}(Y_d Y_d^\dagger)^{dt} + \delta^{rb}\delta^{sc}\delta^{td}(Y_e Y_e^\dagger)^{pa} + \delta^{pa}\delta^{sc}\delta^{td}(Y_e Y_e^\dagger)^{br} + \delta^{pa}\delta^{rb}\delta^{td}(Y_u Y_u^\dagger)^{sc} \right. \\
& \left. \left. + \delta^{pa}\delta^{rb}\delta^{sc}(Y_u Y_u^\dagger)^{dt}\right) - \delta^{pa}\delta^{rb}\delta^{sc}\delta^{td}g_Y^2 \right\} C_{\ell q}^{(\times)abcd}, \tag{13.9}
\end{aligned}$$

$$\begin{aligned}
\beta_{C_{\ell q}^{(\times)prst}}^{(2)} &= 2\delta^{st}g_L^2(C_{\ell HH}C_{\ell HH}^\dagger)^{rp} + 2\left((C_{\ell HH}C_{\ell HH}^\dagger)^{rp}(Y_d Y_d^\dagger)^{st} + (C_{\ell HH}C_{\ell HH}^\dagger)^{rp}(Y_u Y_u^\dagger)^{st}\right) + \left\{ \frac{4}{3}\delta^{pr}\delta^{st}g_L^6 - g_L^4\left(3\delta^{pr}(Y_d Y_d^\dagger)^{st} + 3\delta^{st}(Y_e Y_e^\dagger)^{pr} \right. \right. \\
& \left. \left. + 3\delta^{pr}(Y_u Y_u^\dagger)^{st}\right) \right\} C_{HW} + \left\{ \frac{1}{3}\delta^{pr}\delta^{st}g_Y^2g_L^4 + g_Y^2g_L^2\left(\frac{1}{4}\delta^{st}(Y_e Y_e^\dagger)^{pr} - \frac{1}{12}\delta^{pr}(Y_u Y_u^\dagger)^{st} - \frac{5}{12}\delta^{pr}(Y_d Y_d^\dagger)^{st}\right) \right\} C_{HWB} + \left\{ g_L^6\left(3\delta^{pr}(Y_d Y_d^\dagger)^{st} + 3\delta^{st}(Y_e Y_e^\dagger)^{pr} \right. \right. \\
& \left. \left. + 3\delta^{pr}(Y_u Y_u^\dagger)^{st}\right) - 7\delta^{pr}\delta^{st}g_Y^2g_L^6 - \frac{40}{3}\delta^{pr}\delta^{st}g_L^8 \right\} C_W + \frac{80}{3}\delta^{pr}\delta^{st}g_s^6g_L^2C_G + \left\{ \frac{1}{2}\delta^{pa}\delta^{st}g_Y^2g_L^2Y_e^{*rb} - g_Y^2\left(\frac{1}{2}\delta^{pa}Y_e^{*rb}(Y_u Y_u^\dagger)^{st} \right. \right.
\end{aligned}$$

$$\begin{aligned}
& + 2\delta^{pa} Y_e^{*rb} (Y_d Y_d^\dagger)^{st} \Big) \Big\} C_{eB}^{ab} + C_{eB}^{*ab} \Big\{ \frac{1}{2} \delta^{ra} \delta^{st} g_Y^2 g_L^2 Y_e^{pb} - g_Y^2 \Big( \frac{1}{2} \delta^{ra} Y_e^{pb} (Y_u Y_u^\dagger)^{st} + 2\delta^{ra} Y_e^{pb} (Y_d Y_d^\dagger)^{st} \Big) \Big\} + \Big\{ g_L^4 \Big( \frac{1}{4} \delta^{pa} \delta^{st} Y_e^{*rb} + \frac{1}{3} \delta^{pr} \delta^{st} Y_e^{*ab} \Big) \\
& - g_L^2 \Big( \frac{3}{2} \delta^{pa} Y_e^{*rb} (Y_d Y_d^\dagger)^{st} + \frac{9}{4} \delta^{pa} Y_e^{*rb} (Y_u Y_u^\dagger)^{st} \Big) \Big\} C_{eW}^{ab} + C_{eW}^{*ab} \Big\{ g_L^4 \Big( \frac{1}{4} \delta^{ra} \delta^{st} Y_e^{pb} + \frac{1}{3} \delta^{pr} \delta^{st} Y_e^{ab} \Big) - g_L^2 \Big( \frac{3}{2} \delta^{ra} Y_e^{pb} (Y_d Y_d^\dagger)^{st} + \frac{9}{4} \delta^{ra} Y_e^{pb} (Y_u Y_u^\dagger)^{st} \Big) \Big\} \\
& - \Big\{ \frac{7}{18} \delta^{pr} \delta^{sa} g_Y^2 g_L^2 Y_u^{*tb} + \frac{5}{2} \delta^{sa} g_Y^2 Y_u^{*tb} (Y_e Y_e^\dagger)^{pr} \Big\} C_{uB}^{ab} - C_{uB}^{*ab} \Big\{ \frac{7}{18} \delta^{pr} \delta^{ta} g_Y^2 g_L^2 Y_u^{sb} + \frac{5}{2} \delta^{ta} g_Y^2 Y_u^{sb} (Y_e Y_e^\dagger)^{pr} \Big\} + \Big\{ g_L^4 \Big( \frac{1}{4} \delta^{pr} \delta^{sa} Y_u^{*tb} \\
& + \delta^{pr} \delta^{st} Y_u^{*ab} \Big) + \frac{16}{9} \delta^{pr} \delta^{sa} g_Y^2 g_L^2 Y_u^{*tb} - g_L^2 \Big( \frac{1}{2} \delta^{pr} Y_u^{*tb} (Y_d Y_d^\dagger)^{sa} + \frac{9}{4} \delta^{sa} Y_u^{*tb} (Y_e Y_e^\dagger)^{pr} \Big) - \frac{8}{3} \delta^{pr} \delta^{sa} g_s^2 g_L^2 Y_u^{*tb} \Big\} C_{uW}^{ab} + C_{uW}^{*ab} \Big\{ g_L^4 \Big( \frac{1}{4} \delta^{pr} \delta^{ta} Y_u^{sb} \\
& + \delta^{pr} \delta^{st} Y_u^{ab} \Big) + \frac{16}{9} \delta^{pr} \delta^{ta} g_Y^2 g_L^2 Y_u^{sb} - g_L^2 \Big( \frac{1}{2} \delta^{pr} Y_u^{sb} (Y_d Y_d^\dagger)^{at} + \frac{9}{4} \delta^{ta} Y_u^{sb} (Y_e Y_e^\dagger)^{pr} \Big) - \frac{8}{3} \delta^{pr} \delta^{ta} g_s^2 g_L^2 Y_u^{sb} \Big\} + \Big\{ 4\delta^{sa} g_s^2 Y_u^{*tb} (Y_e Y_e^\dagger)^{pr} \\
& - \frac{4}{9} \delta^{pr} \delta^{sa} g_s^2 g_L^2 Y_u^{*tb} \Big\} C_{uG}^{ab} + C_{uG}^{*ab} \Big\{ 4\delta^{ta} g_s^2 Y_u^{sb} (Y_e Y_e^\dagger)^{pr} - \frac{4}{9} \delta^{pr} \delta^{ta} g_s^2 g_L^2 Y_u^{sb} \Big\} + \Big\{ \frac{5}{18} \delta^{pr} \delta^{sa} g_Y^2 g_L^2 Y_d^{*tb} - 4\delta^{sa} g_Y^2 Y_d^{*tb} (Y_e Y_e^\dagger)^{pr} \Big\} C_{dB}^{ab} \\
& + C_{dB}^{*ab} \Big\{ \frac{5}{18} \delta^{pr} \delta^{ta} g_Y^2 g_L^2 Y_d^{sb} - 4\delta^{ta} g_Y^2 Y_d^{sb} (Y_e Y_e^\dagger)^{pr} \Big\} + \Big\{ g_L^4 \Big( \frac{1}{4} \delta^{pr} \delta^{sa} Y_d^{*tb} + \delta^{pr} \delta^{st} Y_d^{*ab} \Big) - \frac{8}{9} \delta^{pr} \delta^{sa} g_Y^2 g_L^2 Y_d^{*tb} - g_L^2 \Big( \frac{1}{2} \delta^{pr} Y_d^{*tb} (Y_u Y_u^\dagger)^{sa} \\
& + \frac{3}{2} \delta^{sa} Y_d^{*tb} (Y_e Y_e^\dagger)^{pr} \Big) - \frac{8}{3} \delta^{pr} \delta^{sa} g_s^2 g_L^2 Y_d^{*tb} \Big\} C_{dW}^{ab} + C_{dW}^{*ab} \Big\{ g_L^4 \Big( \frac{1}{4} \delta^{pr} \delta^{ta} Y_d^{sb} + \delta^{pr} \delta^{st} Y_d^{ab} \Big) - \frac{8}{9} \delta^{pr} \delta^{ta} g_Y^2 g_L^2 Y_d^{sb} - g_L^2 \Big( \frac{1}{2} \delta^{pr} Y_d^{sb} (Y_u Y_u^\dagger)^{at} \\
& + \frac{3}{2} \delta^{ta} Y_d^{sb} (Y_e Y_e^\dagger)^{pr} \Big) - \frac{8}{3} \delta^{pr} \delta^{ta} g_s^2 g_L^2 Y_d^{sb} \Big\} + \Big\{ 4\delta^{sa} g_s^2 Y_d^{*tb} (Y_e Y_e^\dagger)^{pr} - \frac{4}{9} \delta^{pr} \delta^{sa} g_s^2 g_L^2 Y_d^{*tb} \Big\} C_{dG}^{ab} + C_{dG}^{*ab} \Big\{ 4\delta^{ta} g_s^2 Y_d^{sb} (Y_e Y_e^\dagger)^{pr} \\
& - \frac{4}{9} \delta^{pr} \delta^{ta} g_s^2 g_L^2 Y_d^{sb} \Big\} + \Big\{ \frac{31}{54} \delta^{pa} \delta^{rb} \delta^{st} g_Y^2 g_L^2 + g_L^2 \Big( \frac{1}{2} \delta^{pa} \delta^{rb} (Y_d Y_d^\dagger)^{st} + \frac{29}{36} \delta^{rb} \delta^{st} (Y_e Y_e^\dagger)^{pa} + \frac{29}{36} \delta^{pa} \delta^{st} (Y_e Y_e^\dagger)^{br} - \frac{1}{2} \delta^{pa} \delta^{rb} (Y_u Y_u^\dagger)^{st} \Big) \\
& - \frac{1}{4} \delta^{rb} (Y_d Y_d^\dagger)^{st} (Y_e Y_e^\dagger)^{pa} - \frac{1}{4} \delta^{pa} (Y_d Y_d^\dagger)^{st} (Y_e Y_e^\dagger)^{br} - \frac{1}{4} \delta^{rb} (Y_e Y_e^\dagger)^{pa} (Y_u Y_u^\dagger)^{st} - \frac{1}{4} \delta^{pa} (Y_e Y_e^\dagger)^{br} (Y_u Y_u^\dagger)^{st} \Big\} C_{H\ell}^{(\parallel)ab} + \Big\{ \frac{1}{2} \delta^{rb} (Y_d Y_d^\dagger)^{st} (Y_e Y_e^\dagger)^{pa} \\
& + \frac{1}{2} \delta^{pa} (Y_d Y_d^\dagger)^{st} (Y_e Y_e^\dagger)^{br} + \frac{1}{2} \delta^{rb} (Y_e Y_e^\dagger)^{pa} (Y_u Y_u^\dagger)^{st} + \frac{1}{2} \delta^{pa} (Y_e Y_e^\dagger)^{br} (Y_u Y_u^\dagger)^{st} + \frac{1}{2} \delta^{pa} \delta^{rb} (Y_d Y_d^\dagger Y_d Y_d^\dagger)^{st} + \frac{1}{2} \delta^{pa} \delta^{rb} (Y_u Y_u^\dagger Y_u Y_u^\dagger)^{st} + g_L^4 \Big( \frac{13}{18} \delta^{pa} \delta^{rb} \delta^{st} \\
& - \frac{1}{9} \delta^{pr} \delta^{st} \delta^{ab} \Big) + T_2 \delta^{pa} \delta^{rb} (Y_d Y_d^\dagger)^{st} + T_2 \delta^{pa} \delta^{rb} (Y_u Y_u^\dagger)^{st} + g_s^2 \Big( \frac{16}{3} \delta^{pa} \delta^{rb} (Y_d Y_d^\dagger)^{st} + \frac{16}{3} \delta^{pa} \delta^{rb} (Y_u Y_u^\dagger)^{st} \Big) + \delta^{pa} \delta^{rb} (Y_d Y_d^\dagger Y_u Y_u^\dagger)^{st} \\
& + \delta^{pa} \delta^{rb} (Y_u Y_u^\dagger Y_d Y_d^\dagger)^{st} + g_L^2 \Big( \frac{1}{3} \delta^{st} \delta^{ab} (Y_e Y_e^\dagger)^{pr} - \frac{1}{18} \delta^{rb} \delta^{st} (Y_e Y_e^\dagger)^{pa} - \frac{1}{18} \delta^{pa} \delta^{st} (Y_e Y_e^\dagger)^{br} - \delta^{pa} \delta^{rb} \delta^{st} \text{Tr} [Y_d^\dagger Y_d] - \delta^{pa} \delta^{rb} \delta^{st} \text{Tr} [Y_u^\dagger Y_u] \\
& - \frac{31}{8} \delta^{pa} \delta^{rb} (Y_d Y_d^\dagger)^{st} - \frac{35}{8} \delta^{pa} \delta^{rb} (Y_u Y_u^\dagger)^{st} \Big) + \frac{77}{54} \delta^{pa} \delta^{rb} \delta^{st} g_Y^2 g_L^2 - g_Y^2 \Big( \frac{85}{72} \delta^{pa} \delta^{rb} (Y_d Y_d^\dagger)^{st} + \frac{289}{72} \delta^{pa} \delta^{rb} (Y_u Y_u^\dagger)^{st} \Big) \Big\} C_{H\ell}^{(\times)ab} + \Big\{ \frac{1}{4} \delta^{tb} (Y_e Y_e^\dagger)^{pr} (Y_u Y_u^\dagger)^{sa}
\end{aligned}$$

$$\begin{aligned}
& + \frac{1}{4} \delta^{sa} (Y_e Y_e^\dagger)^{pr} (Y_u Y_u^\dagger)^{bt} + \frac{89}{162} \delta^{pr} \delta^{sa} \delta^{tb} g_Y^2 g_L^2 + g_L^2 \left( \frac{1}{2} \delta^{sa} \delta^{tb} (Y_e Y_e^\dagger)^{pr} + \frac{29}{36} \delta^{pr} \delta^{tb} (Y_d Y_d^\dagger)^{sa} + \frac{29}{36} \delta^{pr} \delta^{sa} (Y_d Y_d^\dagger)^{bt} - \frac{29}{36} \delta^{pr} \delta^{tb} (Y_u Y_u^\dagger)^{sa} \right. \\
& - \frac{29}{36} \delta^{pr} \delta^{sa} (Y_u Y_u^\dagger)^{bt} \left. - \frac{1}{4} \delta^{tb} (Y_d Y_d^\dagger)^{sa} (Y_e Y_e^\dagger)^{pr} - \frac{1}{4} \delta^{sa} (Y_d Y_d^\dagger)^{bt} (Y_e Y_e^\dagger)^{pr} \right\} C_{Hq}^{(\parallel)ab} + \left\{ \frac{1}{2} \delta^{tb} (Y_d Y_d^\dagger)^{sa} (Y_e Y_e^\dagger)^{pr} + \frac{1}{2} \delta^{sa} (Y_d Y_d^\dagger)^{bt} (Y_e Y_e^\dagger)^{pr} \right. \\
& + \frac{1}{2} \delta^{sa} \delta^{tb} (Y_e Y_e^\dagger Y_e Y_e^\dagger)^{pr} + \frac{3}{4} \delta^{tb} (Y_e Y_e^\dagger)^{pr} (Y_u Y_u^\dagger)^{sa} + \frac{3}{4} \delta^{sa} (Y_e Y_e^\dagger)^{pr} (Y_u Y_u^\dagger)^{bt} + T_2 \delta^{sa} \delta^{tb} (Y_e Y_e^\dagger)^{pr} + \frac{19}{18} \delta^{pr} \delta^{sa} \delta^{tb} g_L^4 + \frac{229}{162} \delta^{pr} \delta^{sa} \delta^{tb} g_Y^2 g_L^2 \\
& - g_L^2 \left( \frac{1}{18} \delta^{pr} \delta^{tb} (Y_d Y_d^\dagger)^{sa} + \frac{1}{18} \delta^{pr} \delta^{sa} (Y_d Y_d^\dagger)^{bt} + \frac{1}{3} T_2 \delta^{pr} \delta^{sa} \delta^{tb} + \frac{31}{36} \delta^{pr} \delta^{tb} (Y_u Y_u^\dagger)^{sa} + \frac{31}{36} \delta^{pr} \delta^{sa} (Y_u Y_u^\dagger)^{bt} + \frac{31}{8} \delta^{sa} \delta^{tb} (Y_e Y_e^\dagger)^{pr} \right) \\
& - \frac{47}{24} \delta^{sa} \delta^{tb} g_Y^2 (Y_e Y_e^\dagger)^{pr} \left. \right\} C_{Hq}^{(\times)ab} + \left\{ g_L^2 \left( \frac{2}{9} \delta^{pa} \delta^{st} Y_e^{*rd} Y_e^{bc} + \frac{2}{9} \delta^{rb} \delta^{st} Y_e^{*ad} Y_e^{pc} \right) - \frac{37}{27} \delta^{pa} \delta^{rb} \delta^{st} \delta^{cd} g_Y^2 g_L^2 \right\} C_{\ell e}^{abcd} + \left\{ \frac{1}{4} \delta^{rb} Y_u^{*td} Y_u^{sc} (Y_e Y_e^\dagger)^{pa} \right. \\
& + \frac{1}{4} \delta^{pa} Y_u^{*td} Y_u^{sc} (Y_e Y_e^\dagger)^{br} + \frac{74}{27} \delta^{pa} \delta^{rb} \delta^{st} \delta^{cd} g_Y^2 g_L^2 - \frac{5}{2} \delta^{pa} \delta^{rb} g_L^2 Y_u^{*td} Y_u^{sc} \left. \right\} C_{\ell u}^{abcd} + \left\{ \frac{5}{4} \delta^{rb} Y_d^{*td} Y_d^{sc} (Y_e Y_e^\dagger)^{pa} + \frac{5}{4} \delta^{pa} Y_d^{*td} Y_d^{sc} (Y_e Y_e^\dagger)^{br} \right. \\
& - \frac{37}{27} \delta^{pa} \delta^{rb} \delta^{st} \delta^{cd} g_Y^2 g_L^2 - \frac{5}{2} \delta^{pa} \delta^{rb} g_L^2 Y_d^{*td} Y_d^{sc} \left. \right\} C_{\ell d}^{abcd} + \left\{ \frac{1}{4} \delta^{tb} Y_e^{*rd} Y_e^{pc} (Y_u Y_u^\dagger)^{sa} + \frac{1}{4} \delta^{sa} Y_e^{*rd} Y_e^{pc} (Y_u Y_u^\dagger)^{bt} + \frac{61}{81} \delta^{pr} \delta^{sa} \delta^{tb} \delta^{cd} g_Y^2 g_L^2 \right. \\
& + \frac{5}{4} \delta^{tb} Y_e^{*rd} Y_e^{pc} (Y_d Y_d^\dagger)^{sa} + \frac{5}{4} \delta^{sa} Y_e^{*rd} Y_e^{pc} (Y_d Y_d^\dagger)^{bt} - \frac{5}{2} \delta^{sa} \delta^{tb} g_L^2 Y_e^{*rd} Y_e^{pc} \left. \right\} C_{qe}^{abcd} + \left\{ g_L^2 \left( \frac{2}{9} \delta^{pr} \delta^{sa} Y_u^{*td} Y_u^{bc} + \frac{2}{9} \delta^{pr} \delta^{tb} Y_u^{*ad} Y_u^{sc} \right) \right. \\
& - \frac{122}{81} \delta^{pr} \delta^{sa} \delta^{tb} \delta^{cd} g_Y^2 g_L^2 \left. \right\} C_{qu}^{(\parallel)abcd} + \left\{ -\frac{122}{243} \delta^{pr} \delta^{sa} \delta^{tb} \delta^{cd} g_Y^2 g_L^2 - g_L^2 \left( \frac{1}{3} \delta^{pr} \delta^{sa} Y_u^{*td} Y_u^{bc} + \frac{1}{3} \delta^{pr} \delta^{tb} Y_u^{*ad} Y_u^{sc} \right) - \frac{164}{81} \delta^{pr} \delta^{sa} \delta^{tb} \delta^{cd} g_s^2 g_L^2 \right\} C_{qu}^{(\times)abcd} \\
& + \left\{ \frac{61}{81} \delta^{pr} \delta^{sa} \delta^{tb} \delta^{cd} g_Y^2 g_L^2 + g_L^2 \left( \frac{2}{9} \delta^{pr} \delta^{sa} Y_d^{*td} Y_d^{bc} + \frac{2}{9} \delta^{pr} \delta^{tb} Y_d^{*ad} Y_d^{sc} \right) \right\} C_{qd}^{(\parallel)abcd} + \left\{ \frac{61}{243} \delta^{pr} \delta^{sa} \delta^{tb} \delta^{cd} g_Y^2 g_L^2 - g_L^2 \left( \frac{1}{3} \delta^{pr} \delta^{sa} Y_d^{*td} Y_d^{bc} \right. \right. \\
& + \frac{1}{3} \delta^{pr} \delta^{tb} Y_d^{*ad} Y_d^{sc} \left. \right) - \frac{164}{81} \delta^{pr} \delta^{sa} \delta^{tb} \delta^{cd} g_s^2 g_L^2 \left. \right\} C_{qd}^{(\times)abcd} - \frac{1}{2} Y_e^{*rb} Y_u^{*td} C_{eu}^{abcd} Y_e^{pa} Y_u^{sc} + 2 Y_d^{*td} Y_e^{*rb} C_{ed}^{abcd} Y_d^{sc} Y_e^{pa} + \left\{ g_L^2 \left( \frac{17}{16} \delta^{pa} \delta^{td} Y_e^{*rb} Y_d^{sc} \right. \right. \\
& - \frac{1}{9} \delta^{pr} \delta^{td} Y_e^{*ab} Y_d^{sc} - \frac{1}{3} \delta^{pa} \delta^{st} Y_e^{*rb} Y_d^{dc} \left. \right) - \frac{5}{144} \delta^{pa} \delta^{td} g_Y^2 Y_e^{*rb} Y_d^{sc} - \frac{1}{4} T_2 \delta^{pa} \delta^{td} Y_e^{*rb} Y_d^{sc} - \frac{1}{4} \delta^{td} Y_e^{*ab} Y_d^{sc} (Y_e Y_e^\dagger)^{pr} - \frac{1}{4} \delta^{pa} Y_e^{*rb} Y_d^{sc} (Y_u Y_u^\dagger)^{dt} \\
& - \frac{1}{4} \delta^{pa} \delta^{td} Y_d^{sc} (Y_e^\dagger Y_e Y_e^\dagger)^{rb} - \frac{1}{4} \delta^{pa} \delta^{td} Y_e^{*rb} (Y_d Y_d^\dagger Y_d)^{sc} - \frac{1}{4} \delta^{pa} \delta^{td} Y_e^{*rb} (Y_u Y_u^\dagger Y_d)^{sc} - \frac{3}{4} \delta^{pa} Y_e^{*rb} Y_d^{dc} (Y_d Y_d^\dagger)^{st} - \frac{3}{4} \delta^{pa} Y_e^{*rb} Y_d^{dc} (Y_u Y_u^\dagger)^{st} \\
& - \frac{8}{3} \delta^{pa} \delta^{td} g_s^2 Y_e^{*rb} Y_d^{sc} \left. \right\} C_{\ell edq}^{abcd} + C_{\ell edq}^{*abcd} \left\{ g_L^2 \left( \frac{17}{16} \delta^{ra} \delta^{sd} Y_d^{*tc} Y_e^{pb} - \frac{1}{9} \delta^{pr} \delta^{sd} Y_d^{*tc} Y_e^{ab} - \frac{1}{3} \delta^{ra} \delta^{st} Y_d^{*dc} Y_e^{pb} \right) - \frac{5}{144} \delta^{ra} \delta^{sd} g_Y^2 Y_d^{*tc} Y_e^{pb} \right. \\
& - \frac{1}{4} T_2 \delta^{ra} \delta^{sd} Y_d^{*tc} Y_e^{pb} - \frac{1}{4} \delta^{sd} Y_d^{*tc} Y_e^{ab} (Y_e Y_e^\dagger)^{pr} - \frac{1}{4} \delta^{ra} Y_d^{*tc} Y_e^{pb} (Y_u Y_u^\dagger)^{sd} - \frac{1}{4} \delta^{ra} \delta^{sd} Y_e^{pb} (Y_d^\dagger Y_d Y_d^\dagger)^{tc} - \frac{1}{4} \delta^{ra} \delta^{sd} Y_e^{pb} (Y_u^\dagger Y_u Y_d^\dagger)^{tc}
\end{aligned}$$

$$\begin{aligned}
& -\frac{1}{4}\delta^{ra}\delta^{sd}Y_d^{*tc}(Y_eY_e^\dagger Y_e)^{pb} - \frac{3}{4}\delta^{ra}Y_d^{*dc}Y_e^{pb}(Y_dY_d^\dagger)^{st} - \frac{3}{4}\delta^{ra}Y_d^{*dc}Y_e^{pb}(Y_uY_u^\dagger)^{st} - \frac{8}{3}\delta^{ra}\delta^{sd}g_s^2Y_d^{*tc}Y_e^{pb} \Bigg\} + \Bigg\{ g_L^2\Big(\frac{7}{36}\delta^{pr}\delta^{sa}Y_d^{*td}Y_u^{*cb} \\
& + \frac{7}{36}\delta^{pr}\delta^{sc}Y_d^{*ad}Y_u^{*tb} - \frac{1}{3}\delta^{pr}\delta^{sa}Y_d^{*cd}Y_u^{*tb} - \frac{1}{3}\delta^{pr}\delta^{sc}Y_d^{*td}Y_u^{*ab}\Big) - \frac{1}{8}\delta^{sa}Y_d^{*td}Y_u^{*cb}(Y_eY_e^\dagger)^{pr} - \frac{1}{8}\delta^{sc}Y_d^{*ad}Y_u^{*tb}(Y_eY_e^\dagger)^{pr} - \frac{3}{4}\delta^{sa}Y_d^{*cd}Y_u^{*tb}(Y_eY_e^\dagger)^{pr} \\
& - \frac{3}{4}\delta^{sc}Y_d^{*td}Y_u^{*ab}(Y_eY_e^\dagger)^{pr} \Bigg\} C_{quqd}^{(\parallel)abcd} + \Big(C_{quqd}^{(\parallel)*}\Big)^{abcd} \Bigg\{ g_L^2\Big(\frac{7}{36}\delta^{pr}\delta^{ta}Y_d^{*sd}Y_u^{cb} + \frac{7}{36}\delta^{pr}\delta^{tc}Y_d^{*ad}Y_u^{sb} - \frac{1}{3}\delta^{pr}\delta^{ta}Y_d^{*cd}Y_u^{sb} - \frac{1}{3}\delta^{pr}\delta^{tc}Y_d^{*sd}Y_u^{ab}\Big) - \frac{1}{8}\delta^{ta}Y_d^{*sd}Y_u^{cb}(Y_eY_e^\dagger)^{pr} \\
& - \frac{1}{8}\delta^{tc}Y_d^{*ad}Y_u^{sb}(Y_eY_e^\dagger)^{pr} - \frac{3}{4}\delta^{ta}Y_d^{*cd}Y_u^{sb}(Y_eY_e^\dagger)^{pr} - \frac{3}{4}\delta^{tc}Y_d^{*sd}Y_u^{ab}(Y_eY_e^\dagger)^{pr} \Bigg\} + \Bigg\{ g_L^2\Big(\frac{1}{12}\delta^{pr}\delta^{sa}Y_d^{*td}Y_u^{*cb} + \frac{1}{12}\delta^{pr}\delta^{sc}Y_d^{*ad}Y_u^{*tb} - \frac{5}{18}\delta^{pr}\delta^{sa}Y_d^{*cd}Y_u^{*tb} \\
& - \frac{5}{18}\delta^{pr}\delta^{sc}Y_d^{*td}Y_u^{*ab}\Big) - \frac{1}{4}\delta^{sa}Y_d^{*cd}Y_u^{*tb}(Y_eY_e^\dagger)^{pr} - \frac{1}{4}\delta^{sc}Y_d^{*td}Y_u^{*ab}(Y_eY_e^\dagger)^{pr} - \frac{3}{8}\delta^{sa}Y_d^{*td}Y_u^{*cb}(Y_eY_e^\dagger)^{pr} - \frac{3}{8}\delta^{sc}Y_d^{*ad}Y_u^{*tb}(Y_eY_e^\dagger)^{pr} \Bigg\} C_{quqd}^{(\times)abcd} \\
& + \Big(C_{quqd}^{(\times)*}\Big)^{abcd} \Bigg\{ g_L^2\Big(\frac{1}{12}\delta^{pr}\delta^{ta}Y_d^{*sd}Y_u^{cb} + \frac{1}{12}\delta^{pr}\delta^{tc}Y_d^{*ad}Y_u^{sb} - \frac{5}{18}\delta^{pr}\delta^{ta}Y_d^{*cd}Y_u^{sb} - \frac{5}{18}\delta^{pr}\delta^{tc}Y_d^{*sd}Y_u^{ab}\Big) - \frac{1}{4}\delta^{ta}Y_d^{*cd}Y_u^{sb}(Y_eY_e^\dagger)^{pr} - \frac{1}{4}\delta^{tc}Y_d^{*sd}Y_u^{ab}(Y_eY_e^\dagger)^{pr} \\
& - \frac{3}{8}\delta^{ta}Y_d^{*sd}Y_u^{cb}(Y_eY_e^\dagger)^{pr} - \frac{3}{8}\delta^{tc}Y_d^{*ad}Y_u^{sb}(Y_eY_e^\dagger)^{pr} \Bigg\} + \Bigg\{ \frac{1}{4}T_2\delta^{pa}\delta^{sc}Y_e^{*rb}Y_u^{*td} + \frac{1}{4}\delta^{pa}Y_e^{*rb}Y_u^{*td}(Y_dY_d^\dagger)^{sc} + \frac{1}{4}\delta^{sc}Y_e^{*ab}Y_u^{*td}(Y_eY_e^\dagger)^{pr} \\
& + \frac{1}{4}\delta^{pa}\delta^{sc}Y_e^{*rb}(Y_d^\dagger Y_d Y_u^\dagger)^{td} + \frac{1}{4}\delta^{pa}\delta^{sc}Y_u^{*td}(Y_e^\dagger Y_e Y_e^\dagger)^{rb} + \frac{1}{4}\delta^{pa}\delta^{sc}Y_e^{*rb}(Y_u^\dagger Y_u Y_u^\dagger)^{td} + \frac{3}{4}\delta^{pa}Y_e^{*rb}Y_u^{*cd}(Y_dY_d^\dagger)^{st} + \frac{3}{4}\delta^{pa}Y_e^{*rb}Y_u^{*cd}(Y_uY_u^\dagger)^{st} \\
& + g_L^2\Big(\frac{1}{9}\delta^{pr}\delta^{sc}Y_e^{*ab}Y_u^{*td} + \frac{1}{3}\delta^{pa}\delta^{st}Y_e^{*rb}Y_u^{*cd} - \frac{21}{16}\delta^{pa}\delta^{sc}Y_e^{*rb}Y_u^{*td}\Big) + \frac{8}{3}\delta^{pa}\delta^{sc}g_s^2Y_e^{*rb}Y_u^{*td} - \frac{271}{144}\delta^{pa}\delta^{sc}g_Y^2Y_e^{*rb}Y_u^{*td} \Bigg\} C_{lequ}^{abcd} \\
& + C_{lequ}^{*abcd} \Bigg\{ \frac{1}{4}T_2\delta^{ra}\delta^{tc}Y_e^{pb}Y_u^{sd} + \frac{1}{4}\delta^{ra}Y_e^{pb}Y_u^{sd}(Y_dY_d^\dagger)^{ct} + \frac{1}{4}\delta^{tc}Y_e^{ab}Y_u^{sd}(Y_eY_e^\dagger)^{pr} + \frac{1}{4}\delta^{ra}\delta^{tc}Y_e^{pb}(Y_dY_d^\dagger Y_u)^{sd} + \frac{1}{4}\delta^{ra}\delta^{tc}Y_u^{sd}(Y_eY_e^\dagger Y_e)^{pb} \\
& + \frac{1}{4}\delta^{ra}\delta^{tc}Y_e^{pb}(Y_uY_u^\dagger Y_u)^{sd} + \frac{3}{4}\delta^{ra}Y_e^{pb}Y_u^{cd}(Y_dY_d^\dagger)^{st} + \frac{3}{4}\delta^{ra}Y_e^{pb}Y_u^{cd}(Y_uY_u^\dagger)^{st} + g_L^2\Big(\frac{1}{9}\delta^{pr}\delta^{tc}Y_e^{ab}Y_u^{sd} + \frac{1}{3}\delta^{ra}\delta^{st}Y_e^{pb}Y_u^{cd} - \frac{21}{16}\delta^{ra}\delta^{tc}Y_e^{pb}Y_u^{sd}\Big) \\
& + \frac{8}{3}\delta^{ra}\delta^{tc}g_s^2Y_e^{pb}Y_u^{sd} - \frac{271}{144}\delta^{ra}\delta^{tc}g_Y^2Y_e^{pb}Y_u^{sd} \Bigg\} + \Bigg\{ \frac{1}{4}T_2\delta^{pa}\delta^{sc}Y_e^{*rd}Y_u^{*tb} + \frac{1}{4}\delta^{pa}\delta^{sc}Y_e^{*rd}(Y_d^\dagger Y_d Y_u^\dagger)^{tb} + \frac{1}{4}\delta^{pa}\delta^{sc}Y_u^{*tb}(Y_e^\dagger Y_e Y_e^\dagger)^{rd} \\
& + \frac{1}{4}\delta^{pa}\delta^{sc}Y_e^{*rd}(Y_u^\dagger Y_u Y_u^\dagger)^{tb} + \frac{3}{8}\delta^{pa}Y_e^{*rd}Y_u^{*tb}(Y_dY_d^\dagger)^{sc} + g_L^2\Big(\frac{1}{36}\delta^{pr}\delta^{sc}Y_e^{*ad}Y_u^{*tb} + \frac{1}{12}\delta^{pa}\delta^{st}Y_e^{*rd}Y_u^{*cb} - \frac{21}{16}\delta^{pa}\delta^{sc}Y_e^{*rd}Y_u^{*tb}\Big) \\
& + \frac{7}{3}\delta^{pa}\delta^{sc}g_s^2Y_e^{*rd}Y_u^{*tb} - \frac{1}{8}\delta^{sc}Y_e^{*ad}Y_u^{*tb}(Y_eY_e^\dagger)^{pr} - \frac{3}{8}\delta^{pa}Y_e^{*rd}Y_u^{*cb}(Y_dY_d^\dagger)^{st} - \frac{3}{8}\delta^{pa}Y_e^{*rd}Y_u^{*cb}(Y_uY_u^\dagger)^{st} - \frac{311}{144}\delta^{pa}\delta^{sc}g_Y^2Y_e^{*rd}Y_u^{*tb} \Bigg\} C_{luqe}^{abcd} \\
& + C_{luqe}^{*abcd} \Bigg\{ \frac{1}{4}T_2\delta^{ra}\delta^{tc}Y_e^{pd}Y_u^{sb} + \frac{1}{4}\delta^{ra}\delta^{tc}Y_e^{pd}(Y_dY_d^\dagger Y_u)^{sb} + \frac{1}{4}\delta^{ra}\delta^{tc}Y_u^{sb}(Y_eY_e^\dagger Y_e)^{pd} + \frac{1}{4}\delta^{ra}\delta^{tc}Y_e^{pd}(Y_uY_u^\dagger Y_u)^{sb} + \frac{3}{8}\delta^{ra}Y_e^{pd}Y_u^{sb}(Y_dY_d^\dagger)^{ct}
\end{aligned}$$

$$\begin{aligned}
& + g_L^2 \left( \frac{1}{36} \delta^{pr} \delta^{tc} Y_e^{ad} Y_u^{sb} + \frac{1}{12} \delta^{ra} \delta^{st} Y_e^{pd} Y_u^{cb} - \frac{21}{16} \delta^{ra} \delta^{tc} Y_e^{pd} Y_u^{sb} \right) + \frac{7}{3} \delta^{ra} \delta^{tc} g_s^2 Y_e^{pd} Y_u^{sb} - \frac{1}{8} \delta^{tc} Y_e^{ad} Y_u^{sb} (Y_e Y_e^\dagger)^{pr} - \frac{3}{8} \delta^{ra} Y_e^{pd} Y_u^{cb} (Y_d Y_d^\dagger)^{st} \\
& - \frac{3}{8} \delta^{ra} Y_e^{pd} Y_u^{cb} (Y_u Y_u^\dagger)^{st} - \frac{311}{144} \delta^{ra} \delta^{tc} g_Y^2 Y_e^{pd} Y_u^{sb} \Bigg\} + \left\{ g_L^4 \left( \frac{4}{9} \delta^{pr} \delta^{st} \delta^{ad} \delta^{bc} + \frac{146}{9} \delta^{pa} \delta^{rd} \delta^{st} \delta^{bc} - \frac{14}{3} \delta^{pa} \delta^{rb} \delta^{st} \delta^{cd} \right) + 3 \delta^{pa} \delta^{rd} (Y_d Y_d^\dagger)^{st} (Y_e Y_e^\dagger)^{bc} \right. \\
& + 3 \delta^{pa} \delta^{rd} (Y_e Y_e^\dagger)^{bc} (Y_u Y_u^\dagger)^{st} - g_Y^2 g_L^2 \left( \frac{74}{27} \delta^{pa} \delta^{rb} \delta^{st} \delta^{cd} + \frac{154}{27} \delta^{pa} \delta^{rd} \delta^{st} \delta^{bc} \right) - \frac{8}{3} \delta^{pa} \delta^{rd} \delta^{st} g_L^2 (Y_e Y_e^\dagger)^{bc} \Bigg\} C_{\ell\ell}^{abcd} + \left\{ g_L^4 \left( \frac{8}{3} \delta^{pr} \delta^{st} \delta^{ad} \delta^{bc} \right. \right. \\
& + \frac{158}{9} \delta^{pr} \delta^{sa} \delta^{td} \delta^{bc} - 2 \delta^{pr} \delta^{sa} \delta^{tb} \delta^{cd} \Bigg) + 3 \delta^{sa} \delta^{td} (Y_d Y_d^\dagger)^{bc} (Y_e Y_e^\dagger)^{pr} + 3 \delta^{sa} \delta^{td} (Y_e Y_e^\dagger)^{pr} (Y_u Y_u^\dagger)^{bc} + \frac{260}{81} \delta^{pr} \delta^{sa} \delta^{td} \delta^{bc} g_s^2 g_L^2 \\
& - g_Y^2 g_L^2 \left( \frac{122}{81} \delta^{pr} \delta^{sa} \delta^{tb} \delta^{cd} + \frac{922}{243} \delta^{pr} \delta^{sa} \delta^{td} \delta^{bc} \right) - g_L^2 \left( \frac{8}{3} \delta^{pr} \delta^{sa} \delta^{td} (Y_d Y_d^\dagger)^{bc} + \frac{8}{3} \delta^{pr} \delta^{sa} \delta^{td} (Y_u Y_u^\dagger)^{bc} \right) \Bigg\} C_{qq}^{abcd} + \left\{ g_s^2 g_L^2 \left( 12 \delta^{pr} \delta^{sa} \delta^{tb} \delta^{cd} \right. \right. \\
& - \frac{272}{81} \delta^{pr} \delta^{sa} \delta^{td} \delta^{bc} \Bigg) + g_L^4 \left( \frac{92}{3} \delta^{pr} \delta^{sa} \delta^{tb} \delta^{cd} - \frac{14}{3} \delta^{pr} \delta^{sa} \delta^{td} \delta^{bc} \right) + 3 \delta^{sa} \delta^{tb} (Y_d Y_d^\dagger)^{dc} (Y_e Y_e^\dagger)^{pr} + 3 \delta^{sa} \delta^{tb} (Y_e Y_e^\dagger)^{pr} (Y_u Y_u^\dagger)^{dc} - g_Y^2 g_L^2 \left( \frac{422}{243} \delta^{pr} \delta^{sa} \delta^{td} \delta^{bc} \right. \\
& + \frac{556}{81} \delta^{pr} \delta^{sa} \delta^{tb} \delta^{cd} \Bigg) - g_L^2 \left( 4 \delta^{pr} \delta^{sa} \delta^{tb} (Y_d Y_d^\dagger)^{dc} + 4 \delta^{pr} \delta^{sa} \delta^{tb} (Y_u Y_u^\dagger)^{dc} \right) \Bigg\} C_{qq}^{(\times)abcd} + \left\{ g_L^4 \left( \frac{49}{3} \delta^{pa} \delta^{rb} \delta^{sc} \delta^{td} - \frac{1}{3} \delta^{pr} \delta^{sc} \delta^{td} \delta^{ab} - \delta^{pa} \delta^{rb} \delta^{st} \delta^{cd} \right) \right. \\
& + g_Y^2 g_L^2 \left( \frac{61}{81} \delta^{pr} \delta^{sc} \delta^{td} \delta^{ab} + \frac{37}{27} \delta^{pa} \delta^{rb} \delta^{st} \delta^{cd} - \frac{3}{2} \delta^{pa} \delta^{rb} \delta^{sc} \delta^{td} \right) + \delta^{pa} \delta^{td} (Y_e Y_e^\dagger)^{br} (Y_u Y_u^\dagger)^{sc} + \delta^{rb} \delta^{sc} (Y_e Y_e^\dagger)^{pa} (Y_u Y_u^\dagger)^{dt} + \frac{7}{4} \delta^{rb} \delta^{td} (Y_e Y_e^\dagger)^{pa} (Y_u Y_u^\dagger)^{sc} \\
& + \frac{7}{4} \delta^{pa} \delta^{sc} (Y_e Y_e^\dagger)^{br} (Y_u Y_u^\dagger)^{dt} + 2 \delta^{rb} \delta^{td} (Y_d Y_d^\dagger)^{sc} (Y_e Y_e^\dagger)^{pa} + 2 \delta^{pa} \delta^{sc} (Y_d Y_d^\dagger)^{dt} (Y_e Y_e^\dagger)^{br} - \frac{1}{4} \delta^{rb} \delta^{sc} (Y_d Y_d^\dagger)^{dt} (Y_e Y_e^\dagger)^{pa} - \frac{1}{4} \delta^{pa} \delta^{td} (Y_d Y_d^\dagger)^{sc} (Y_e Y_e^\dagger)^{br} \\
& - 24 \delta^{pa} \delta^{rb} \delta^{sc} \delta^{td} g_s^2 g_L^2 \Bigg\} C_{\ell q}^{abcd} + \left\{ \frac{1}{2} \delta^{sc} \delta^{td} (Y_e Y_e^\dagger)^{pr} (Y_e Y_e^\dagger)^{ba} + g_Y^2 g_L^2 \left( \frac{50}{27} \delta^{pa} \delta^{rb} \delta^{st} \delta^{cd} + \frac{314}{81} \delta^{pr} \delta^{sc} \delta^{td} \delta^{ab} - \frac{11}{4} \delta^{pa} \delta^{rb} \delta^{sc} \delta^{td} \right) \right. \\
& + g_s^2 g_L^2 \left( 8 \delta^{pa} \delta^{rb} \delta^{st} \delta^{cd} - 12 \delta^{pa} \delta^{rb} \delta^{sc} \delta^{td} \right) + g_L^4 \left( \frac{46}{9} \delta^{pr} \delta^{sc} \delta^{td} \delta^{ab} + \frac{40}{3} \delta^{pa} \delta^{rb} \delta^{st} \delta^{cd} - \frac{2}{3} \delta^{pr} \delta^{st} \delta^{ab} \delta^{cd} - \frac{385}{24} \delta^{pa} \delta^{rb} \delta^{sc} \delta^{td} \right) \\
& + \delta^{pa} \delta^{td} (Y_e Y_e^\dagger)^{br} (Y_u Y_u^\dagger)^{sc} + \delta^{rb} \delta^{sc} (Y_e Y_e^\dagger)^{pa} (Y_u Y_u^\dagger)^{dt} + g_Y^2 \left( \frac{7}{144} \delta^{pa} \delta^{rb} \delta^{td} (Y_d Y_d^\dagger)^{sc} + \frac{7}{144} \delta^{pa} \delta^{rb} \delta^{sc} (Y_d Y_d^\dagger)^{dt} + \frac{23}{16} \delta^{rb} \delta^{sc} \delta^{td} (Y_e Y_e^\dagger)^{pa} \right. \\
& + \frac{23}{16} \delta^{pa} \delta^{sc} \delta^{td} (Y_e Y_e^\dagger)^{br} + \frac{427}{144} \delta^{pa} \delta^{rb} \delta^{td} (Y_u Y_u^\dagger)^{sc} + \frac{427}{144} \delta^{pa} \delta^{rb} \delta^{sc} (Y_u Y_u^\dagger)^{dt} \Bigg) + g_L^2 \left( \frac{33}{16} \delta^{pa} \delta^{rb} \delta^{td} (Y_d Y_d^\dagger)^{sc} + \frac{33}{16} \delta^{pa} \delta^{rb} \delta^{sc} (Y_d Y_d^\dagger)^{dt} \right. \\
& + \frac{33}{16} \delta^{rb} \delta^{sc} \delta^{td} (Y_e Y_e^\dagger)^{pa} + \frac{33}{16} \delta^{pa} \delta^{sc} \delta^{td} (Y_e Y_e^\dagger)^{br} + \frac{33}{16} \delta^{pa} \delta^{rb} \delta^{td} (Y_u Y_u^\dagger)^{sc} + \frac{33}{16} \delta^{pa} \delta^{rb} \delta^{sc} (Y_u Y_u^\dagger)^{dt} - \frac{2}{3} \delta^{pr} \delta^{sc} \delta^{td} (Y_e Y_e^\dagger)^{ba} - 2 \delta^{pa} \delta^{rb} \delta^{st} (Y_d Y_d^\dagger)^{dc} \\
& - 2 \delta^{pa} \delta^{rb} \delta^{st} (Y_u Y_u^\dagger)^{dc} \Bigg) + \frac{3}{2} \delta^{pa} \delta^{rb} (Y_d Y_d^\dagger)^{st} (Y_d Y_d^\dagger)^{dc} + \frac{3}{2} \delta^{pa} \delta^{rb} (Y_d Y_d^\dagger)^{dc} (Y_u Y_u^\dagger)^{st} + \frac{3}{2} \delta^{pa} \delta^{rb} (Y_d Y_d^\dagger)^{st} (Y_u Y_u^\dagger)^{dc} + \frac{3}{2} \delta^{pa} \delta^{rb} (Y_u Y_u^\dagger)^{st} (Y_u Y_u^\dagger)^{dc} \\
& + 4 \delta^{pa} \delta^{rb} \delta^{sc} \delta^{td} g_Y^2 g_s^2 - \frac{1}{4} \delta^{pa} \delta^{rb} \delta^{td} (Y_d Y_d^\dagger Y_d Y_d^\dagger)^{sc} - \frac{1}{4} \delta^{pa} \delta^{rb} \delta^{sc} (Y_d Y_d^\dagger Y_d Y_d^\dagger)^{dt} - \frac{1}{4} \delta^{rb} \delta^{sc} \delta^{td} (Y_e Y_e^\dagger Y_e Y_e^\dagger)^{pa} - \frac{1}{4} \delta^{pa} \delta^{sc} \delta^{td} (Y_e Y_e^\dagger Y_e Y_e^\dagger)^{br} \\
& - \frac{1}{4} \delta^{pa} \delta^{rb} \delta^{td} (Y_u Y_u^\dagger Y_u Y_u^\dagger)^{sc} - \frac{1}{4} \delta^{pa} \delta^{rb} \delta^{sc} (Y_u Y_u^\dagger Y_u Y_u^\dagger)^{dt} - \frac{31}{72} \delta^{pa} \delta^{rb} \delta^{sc} \delta^{td} g_Y^4 - \frac{1}{2} \delta^{rb} \delta^{sc} (Y_d Y_d^\dagger)^{dt} (Y_e Y_e^\dagger)^{pa} - \frac{1}{2} \delta^{pa} \delta^{td} (Y_d Y_d^\dagger)^{sc} (Y_e Y_e^\dagger)^{br}
\end{aligned}$$



$$\begin{aligned}
& -\frac{3}{4}\text{T}_2\delta^{pa}\delta^{rb}\delta^{td}(Y_dY_d^\dagger)^{sc} - \frac{3}{4}\text{T}_2\delta^{pa}\delta^{rb}\delta^{sc}(Y_dY_d^\dagger)^{dt} - \frac{3}{4}\text{T}_2\delta^{rb}\delta^{sc}\delta^{td}(Y_eY_e^\dagger)^{pa} - \frac{3}{4}\text{T}_2\delta^{pa}\delta^{sc}\delta^{td}(Y_eY_e^\dagger)^{br} - \frac{3}{4}\text{T}_2\delta^{pa}\delta^{rb}\delta^{td}(Y_uY_u^\dagger)^{sc} \\
& - \frac{3}{4}\text{T}_2\delta^{pa}\delta^{rb}\delta^{sc}(Y_uY_u^\dagger)^{dt} - \delta^{pa}\delta^{rb}(Y_dY_d^\dagger)^{dt}(Y_uY_u^\dagger)^{sc} - \delta^{pa}\delta^{rb}(Y_dY_d^\dagger)^{sc}(Y_uY_u^\dagger)^{dt} - g_s^2\left(\frac{8}{3}\delta^{pa}\delta^{rb}\delta^{td}(Y_dY_d^\dagger)^{sc} + \frac{8}{3}\delta^{pa}\delta^{rb}\delta^{sc}(Y_dY_d^\dagger)^{dt}\right. \\
& \left. + \frac{8}{3}\delta^{pa}\delta^{rb}\delta^{td}(Y_uY_u^\dagger)^{sc} + \frac{8}{3}\delta^{pa}\delta^{rb}\delta^{sc}(Y_uY_u^\dagger)^{dt}\right) - \frac{7}{4}\delta^{rb}\delta^{td}(Y_eY_e^\dagger)^{pa}(Y_uY_u^\dagger)^{sc} - \frac{7}{4}\delta^{pa}\delta^{sc}(Y_eY_e^\dagger)^{br}(Y_uY_u^\dagger)^{dt} \Big\} C_{\ell q}^{(\times)abcd}, \tag{13.10}
\end{aligned}$$
